# Supplementary material for: En-gauging Naturalness
Source: arXiv:1310.4500 source file (2014-05-02)
Supplement: Supplementary file 1 [file SupplementaryQSMxEW-Regime1.pdf]

# Electroweak Quiver Gauge Model

Superpotential, Rotations and Interactions for eigenstates  
‘Regime-1 of QEWmld2L3’  
including Renormalization Group Equations  
and one-loop Self-Energies

Authors: A.Bharucha, M.McGarrie & A.Goudelis (SARAH 3.3.0)

April 12, 2014

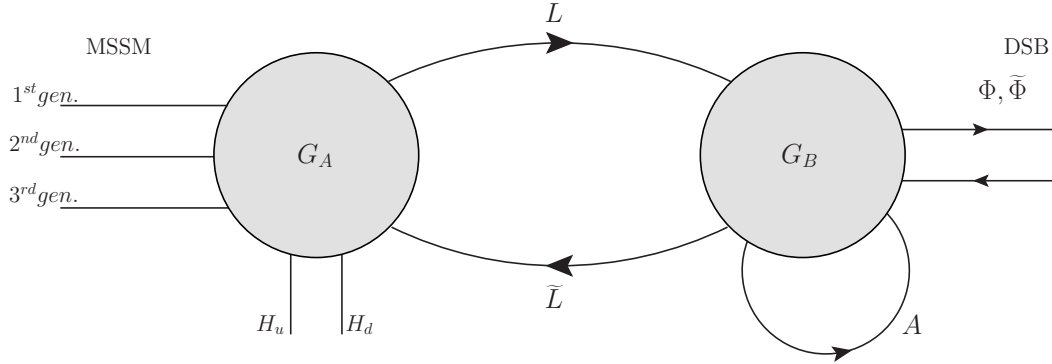

Figure 1: A picture to represent the quiver module of the electroweak sector. The electroweak part of the supersymmetric standard model are on one gauge site, with messenger fields ( $\Phi, \tilde{\Phi}$ ) coupled to another site. The linking fields ( $L, \tilde{L}$ ) connect the two sites. The adjoint field ( $A$ ) is charged on the second site. The singlet field ( $K$ ) is not shown.

This file was automatically generated by SARAH version 3.3.0.  
and then edited by M. McGarrie References: **“En-gauging Naturalness”, ArXiv: 1310.4500,**  
**published in THE EUROPEAN PHYSICAL JOURNAL C (Particles and Fields),**  
**Comput.Phys.Commun.182:808-833,2011 (1002.0840) ,**  
**Comput.Phys.Commun.181:1077-1086,2010 (0909.2863) , arXiv: 0806.0538**  
Package Homepage: [projects.hepforge.org/sarah/](http://projects.hepforge.org/sarah/)  
by **Florian Staub, fnstaub@th.physik.uni-bonn.de**

# Contents

|          |                                                                           |           |
|----------|---------------------------------------------------------------------------|-----------|
| <b>1</b> | <b>Superfields</b>                                                        | <b>4</b>  |
| 1.1      | Vector Superfields . . . . .                                              | 4         |
| 1.2      | Chiral Superfields . . . . .                                              | 4         |
| <b>2</b> | <b>Superpotential and Lagrangian</b>                                      | <b>4</b>  |
| 2.1      | Superpotential . . . . .                                                  | 4         |
| 2.2      | Softbreaking terms . . . . .                                              | 4         |
| 2.3      | Gauge fixing terms . . . . .                                              | 5         |
| 2.3.1    | Gauge fixing terms for eigenstates 'GaugeESAxB' . . . . .                 | 5         |
| 2.3.2    | Gauge fixing terms for eigenstates 'AxBSB' . . . . .                      | 5         |
| 2.4      | Fields integrated out . . . . .                                           | 5         |
| <b>3</b> | <b>Renormalization Group Equations</b>                                    | <b>6</b>  |
| 3.1      | Anomalous Dimensions . . . . .                                            | 6         |
| 3.2      | Gauge Couplings . . . . .                                                 | 7         |
| 3.3      | Gaugino Mass Parameters . . . . .                                         | 8         |
| 3.4      | Trilinear Superpotential Parameters . . . . .                             | 8         |
| 3.5      | Bilinear Superpotential Parameters . . . . .                              | 9         |
| 3.6      | Linear Superpotential Parameters . . . . .                                | 10        |
| 3.7      | Trilinear Soft-Breaking Parameters . . . . .                              | 10        |
| 3.8      | Bilinear Soft-Breaking Parameters . . . . .                               | 12        |
| 3.9      | Linear Soft-Breaking Parameters . . . . .                                 | 13        |
| 3.10     | Soft-Breaking Scalar Masses . . . . .                                     | 13        |
| <b>4</b> | <b>Field Rotations</b>                                                    | <b>21</b> |
| 4.1      | Rotations in gauge sector for eigenstates 'AxBSB' . . . . .               | 21        |
| 4.2      | Rotations in Mass sector for eigenstates 'AxBSB' . . . . .                | 22        |
| 4.2.1    | Mass Matrices for Scalars . . . . .                                       | 22        |
| 4.2.2    | Mass Matrices for Fermions . . . . .                                      | 30        |
| <b>5</b> | <b>Vacuum Expectation Values</b>                                          | <b>34</b> |
| <b>6</b> | <b>Tadpole Equations</b>                                                  | <b>34</b> |
| <b>7</b> | <b>Particle content for eigenstates 'AxBSB'</b>                           | <b>34</b> |
| <b>8</b> | <b>One Loop Self-Energy and One Loop Tadpoles for eigenstates 'AxBSB'</b> | <b>36</b> |
| 8.1      | One Loop Self-Energy . . . . .                                            | 36        |
| 8.2      | Tadpoles . . . . .                                                        | 98        |
| <b>9</b> | <b>Interactions for eigenstates 'AxBSB'</b>                               | <b>99</b> |
| 9.1      | Three Scalar-Interaction . . . . .                                        | 99        |
| 9.2      | Two Scalar-One Vector Boson-Interaction . . . . .                         | 122       |
| 9.3      | One Scalar-Two Vector Boson-Interaction . . . . .                         | 163       |
| 9.4      | Two Fermion-One Vector Boson-Interaction . . . . .                        | 178       |

|      |                                                    |     |
|------|----------------------------------------------------|-----|
| 9.5  | Two Fermion-One Scalar Boson-Interaction . . . . . | 213 |
| 9.6  | Three Vector Boson-Interaction . . . . .           | 271 |
| 9.7  | Four Scalar-Interaction . . . . .                  | 275 |
| 9.8  | Two Scalar-Two Vector Boson-Interaction . . . . .  | 343 |
| 9.9  | Four Vector Boson-Interaction . . . . .            | 494 |
| 9.10 | Two Ghosts-One Vector Boson-Interaction . . . . .  | 504 |
| 9.11 | Two Ghosts-One Scalar-Interaction . . . . .        | 520 |

# 1 Superfields

## 1.1 Vector Superfields

| SF          | Spin $\frac{1}{2}$ | Spin 1 | $SU(N)$ | Coupling | Name         |
|-------------|--------------------|--------|---------|----------|--------------|
| $\hat{B}_B$ | $\tilde{B}_B$      | $B_B$  | $U(1)$  | $g_{B1}$ | Bhypercharge |
| $\hat{W}_B$ | $\tilde{W}_B$      | $W_B$  | $SU(2)$ | $g_{B2}$ | Bleft        |
| $\hat{B}_A$ | $\tilde{B}_A$      | $B_A$  | $U(1)$  | $g_{A1}$ | Ahypercharge |
| $\hat{W}_A$ | $\tilde{W}_A$      | $W_A$  | $SU(2)$ | $g_{A2}$ | Aleft        |
| $\hat{G}_A$ | $\tilde{G}_A$      | $g$    | $SU(3)$ | $g_3$    | Acolor       |

## 1.2 Chiral Superfields

| SF                | Spin 0          | Spin $\frac{1}{2}$ | Generations | $(U(1) \otimes SU(2) \otimes U(1) \otimes SU(2) \otimes SU(3))$         |
|-------------------|-----------------|--------------------|-------------|-------------------------------------------------------------------------|
| $\hat{Q}$         | $\hat{q}$       | $q$                | 3           | $(0, \mathbf{1}, \frac{1}{6}, \mathbf{2}, \mathbf{3})$                  |
| $\hat{L}$         | $\tilde{l}$     | $l$                | 3           | $(0, \mathbf{1}, -\frac{1}{2}, \mathbf{2}, \mathbf{1})$                 |
| $\hat{H}_d$       | $\tilde{H}_d$   | $H_d$              | 1           | $(0, \mathbf{1}, -\frac{1}{2}, \mathbf{2}, \mathbf{1})$                 |
| $\hat{H}_u$       | $\tilde{H}_u$   | $H_u$              | 1           | $(0, \mathbf{1}, \frac{1}{2}, \mathbf{2}, \mathbf{1})$                  |
| $\hat{u}_R$       | $\tilde{u}_R^*$ | $u_R^*$            | 3           | $(0, \mathbf{1}, -\frac{2}{3}, \mathbf{1}, \mathbf{\bar{3}})$           |
| $\hat{d}_R$       | $\tilde{d}_R^*$ | $d_R^*$            | 3           | $(0, \mathbf{1}, \frac{1}{3}, \mathbf{1}, \mathbf{\bar{3}})$            |
| $\hat{e}_R$       | $\tilde{e}_R^*$ | $e_R^*$            | 3           | $(0, \mathbf{1}, 1, \mathbf{1}, \mathbf{1})$                            |
| $\hat{L}$         | $L_s$           | $L_f$              | 1           | $(\frac{1}{2}, \mathbf{\bar{2}}, -\frac{1}{2}, \mathbf{2}, \mathbf{1})$ |
| $\hat{\tilde{L}}$ | $\tilde{L}_s$   | $\tilde{L}_f$      | 1           | $(-\frac{1}{2}, \mathbf{2}, \frac{1}{2}, \mathbf{\bar{2}}, \mathbf{1})$ |
| $\hat{K}$         | $K_s$           | $K_f$              | 1           | $(0, \mathbf{1}, 0, \mathbf{1}, \mathbf{1})$                            |
| $\hat{Ad}$        | $Ad_s$          | $Ad_f$             | 1           | $(0, \mathbf{3}, 0, \mathbf{1}, \mathbf{1})$                            |

# 2 Superpotential and Lagrangian

## 2.1 Superpotential

$$W = Y_u \hat{u}_R \hat{Q} \hat{H}_u - Y_d \hat{d}_R \hat{Q} \hat{H}_d - Y_e \hat{e}_R \hat{L} \hat{H}_d + \mu \hat{H}_u \hat{H}_d + \frac{1}{2} Y_K \hat{K} \hat{L} \hat{\tilde{L}} - \frac{1}{2} \Omega \hat{K} + Y_A \hat{L} \hat{Ad} \hat{\tilde{L}} \quad (1)$$

## 2.2 Softbreaking terms

$$\begin{aligned}
-L_{SB,W} = & -H_d^0 H_u^0 B_\mu + H_d^- H_u^+ B_\mu - \frac{1}{2} K_s L_\Omega + \frac{1}{\sqrt{2}} Ad_s^1 \varphi_{l1} \tilde{\varphi}_{lt1} T_A + Ad_s^3 \varphi_{l2} \tilde{\varphi}_{lt1} T_A + Ad_s^2 \varphi_{l1} \tilde{\varphi}_{lt2} T_A \\
& - \frac{1}{\sqrt{2}} Ad_s^1 \varphi_{l2} \tilde{\varphi}_{lt2} T_A + \frac{1}{\sqrt{2}} Ad_s^1 \varphi_{l3} \tilde{\varphi}_{lt3} T_A + Ad_s^3 \varphi_{l4} \tilde{\varphi}_{lt3} T_A + Ad_s^2 \varphi_{l3} \tilde{\varphi}_{lt4} T_A - \frac{1}{\sqrt{2}} Ad_s^1 \varphi_{l4} \tilde{\varphi}_{lt4} T_A
\end{aligned}$$

$$\begin{aligned}
& + \frac{1}{2} \left( K_s \varphi_{l1} \tilde{\varphi}_{lt1} T_K + K_s \varphi_{l2} \tilde{\varphi}_{lt2} T_K + K_s \varphi_{l3} \tilde{\varphi}_{lt3} T_K + K_s \varphi_{l4} \tilde{\varphi}_{lt4} T_K \right) + H_d^0 \tilde{d}_{R,iAt1}^* \delta_{At1At2} \tilde{d}_{L,jAt2} T_{d,ij} \\
& - H_d^- \tilde{d}_{R,iAt1}^* \delta_{At1At2} \tilde{u}_{L,jAt2} T_{d,ij} + H_d^0 \tilde{e}_{R,i}^* \tilde{e}_{L,j} T_{e,ij} - H_d^- \tilde{e}_{R,i}^* \tilde{\nu}_{L,j} T_{e,ij} - H_u^+ \tilde{u}_{R,iAt1}^* \delta_{At1At2} \tilde{d}_{L,jAt2} T_{u,ij} \\
& + H_u^0 \tilde{u}_{R,iAt1}^* \delta_{At1At2} \tilde{u}_{L,jAt2} T_{u,ij} + \text{h.c.} \tag{2}
\end{aligned}$$

$$\begin{aligned}
-L_{SB,\phi} = & + m_{Ad}^2 |Ad_s^1|^2 + m_{Ad}^2 |Ad_s^2|^2 + m_{Ad}^2 |Ad_s^3|^2 + m_{H_d}^2 |H_d^0|^2 + m_{H_d}^2 |H_d^-|^2 + m_{H_u}^2 |H_u^0|^2 + m_{H_u}^2 |H_u^+|^2 \\
& + m_K^2 |K_s|^2 + m_L^2 |\varphi_{l1}|^2 + m_L^2 |\varphi_{l2}|^2 + m_L^2 |\varphi_{l3}|^2 + m_L^2 |\varphi_{l4}|^2 + m_L^2 |\tilde{\varphi}_{lt1}|^2 + m_L^2 |\tilde{\varphi}_{lt2}|^2 + m_L^2 |\tilde{\varphi}_{lt3}|^2 \\
& + m_L^2 |\tilde{\varphi}_{lt4}|^2 + \tilde{d}_{L,iAt1}^* \delta_{At1At2} m_{q,ij}^2 \tilde{d}_{L,jAt2} + \tilde{d}_{R,iAt1}^* \delta_{At1At2} m_{d,ij}^2 \tilde{d}_{R,jAt2} + \tilde{e}_{L,i}^* m_{l,ij}^2 \tilde{e}_{L,j} + \tilde{e}_{R,i}^* m_{e,ij}^2 \tilde{e}_{R,j} \\
& + \tilde{u}_{L,iAt1}^* \delta_{At1At2} m_{q,ij}^2 \tilde{u}_{L,jAt2} + \tilde{u}_{R,iAt1}^* \delta_{At1At2} m_{u,ij}^2 \tilde{u}_{R,jAt2} + \tilde{\nu}_{L,i}^* m_{l,ij}^2 \tilde{\nu}_{L,j} \tag{3}
\end{aligned}$$

$$-L_{SB,\lambda} = \frac{1}{2} \left( M_3 \tilde{G}_{A,aAt1} \tilde{G}_{A,aAt2} + m_{W_A} \tilde{W}_{A,i}^2 + m_{W_B} \tilde{W}_{B,i}^2 + \tilde{B}_A^2 m_{B_A} + \tilde{B}_B^2 m_{B_B} + \text{h.c.} \right) \tag{4}$$

## 2.3 Gauge fixing terms

### 2.3.1 Gauge fixing terms for eigenstates 'GaugeESAxB'

$$L_{GF} = -\frac{1}{2} |\partial_\mu B_A|^2 \xi_{B_A}^{-1} - \frac{1}{2} |\partial_\mu B_B|^2 \xi_{B_B}^{-1} - \frac{1}{2} |\partial_\mu g|^2 \xi_g^{-1} - \frac{1}{2} |\partial_\mu W_A|^2 \xi_{W_A}^{-1} - \frac{1}{2} |\partial_\mu W_B|^2 \xi_{W_B}^{-1} \tag{5}$$

### 2.3.2 Gauge fixing terms for eigenstates 'AxBSB'

$$\begin{aligned}
L_{GF} = & -\frac{1}{2} \left| -\left( -\sigma_{Lt1} - \sigma_{Lt4} + \sigma_{L1} + \sigma_{L4} \right) v_{Lv} \xi_{B_L} \left( g_{A1} \cos \theta_1 - g_{B1} \sin \theta_1 \right) + \partial_\mu B_L \right|^2 \xi_{B_L}^{-1} \\
& -\frac{1}{2} \left| -\left( -\sigma_{Lt1} - \sigma_{Lt4} + \sigma_{L1} + \sigma_{L4} \right) v_{Lv} \xi_{B_H} \left( g_{A1} \sin \theta_1 + g_{B1} \cos \theta_1 \right) + \partial_\mu B_H \right|^2 \xi_{B_H}^{-1} - \frac{1}{2} |\partial_\mu g|^2 \xi_g^{-1} \\
& -\frac{1}{2} \left| \frac{1}{2} \left( 2\partial_\mu W_L^1 - i v_{Lv} \left( -\tilde{\varphi}_{lt2} - \tilde{\varphi}_{lt3} - \varphi_{l2}^* - \varphi_{l3}^* + \varphi_{l2} + \varphi_{l3} + \tilde{\varphi}_{lt2}^* + \tilde{\varphi}_{lt3}^* \right) \xi_{W_L^1} \left( g_{A2} \cos \theta_2 - g_{B2} \sin \theta_2 \right) \right) \right|^2 \xi_{W_L^1}^{-1} \\
& -\frac{1}{2} \left| \frac{1}{2} \left( 2\partial_\mu W_H^1 + i v_{Lv} \left( -\tilde{\varphi}_{lt2} - \tilde{\varphi}_{lt3} - \varphi_{l2}^* - \varphi_{l3}^* + \varphi_{l2} + \varphi_{l3} + \tilde{\varphi}_{lt2}^* + \tilde{\varphi}_{lt3}^* \right) \xi_{W_H^1} \left( g_{A2} \sin \theta_2 + g_{B2} \cos \theta_2 \right) \right) \right|^2 \xi_{W_H^1}^{-1} \\
& -\frac{1}{2} \left| \frac{1}{2} \left( 2\partial_\mu W_L^2 + v_{Lv} \left( -\tilde{\varphi}_{lt3} - \tilde{\varphi}_{lt3}^* - \varphi_{l3} - \varphi_{l3}^* + \varphi_{l2} + \tilde{\varphi}_{lt2} + \varphi_{l2}^* + \tilde{\varphi}_{lt2}^* \right) \xi_{W_L^2} \left( g_{A2} \cos \theta_2 - g_{B2} \sin \theta_2 \right) \right) \right|^2 \xi_{W_L^2}^{-1} \\
& -\frac{1}{2} \left| \frac{1}{2} \left( 2\partial_\mu W_H^2 - v_{Lv} \left( -\tilde{\varphi}_{lt3} - \tilde{\varphi}_{lt3}^* - \varphi_{l3} - \varphi_{l3}^* + \varphi_{l2} + \tilde{\varphi}_{lt2} + \varphi_{l2}^* + \tilde{\varphi}_{lt2}^* \right) \xi_{W_H^2} \left( g_{A2} \sin \theta_2 + g_{B2} \cos \theta_2 \right) \right) \right|^2 \xi_{W_H^2}^{-1} \\
& -\frac{1}{2} \left| -\left( -\sigma_{L4} - \sigma_{Lt1} + \sigma_{L1} + \sigma_{Lt4} \right) v_{Lv} \xi_{W_L^3} \left( g_{A2} \cos \theta_2 - g_{B2} \sin \theta_2 \right) + \partial_\mu W_L^3 \right|^2 \xi_{W_L^3}^{-1} \\
& -\frac{1}{2} \left| -\left( -\sigma_{L4} - \sigma_{Lt1} + \sigma_{L1} + \sigma_{Lt4} \right) v_{Lv} \xi_{W_H^3} \left( g_{A2} \sin \theta_2 + g_{B2} \cos \theta_2 \right) + \partial_\mu W_H^3 \right|^2 \xi_{W_H^3}^{-1} \tag{6}
\end{aligned}$$

## 2.4 Fields integrated out

None

### 3 Renormalization Group Equations

#### 3.1 Anomalous Dimensions

$$\gamma_{\hat{Q}}^{(1)} = -\frac{1}{30} \left( 45g_{A2}^2 + 80g_3^2 + g_{A1}^2 \right) \mathbf{1} + Y_d^\dagger Y_d + Y_u^\dagger Y_u \quad (7)$$

$$\begin{aligned} \gamma_{\hat{Q}}^{(2)} = & +\frac{1}{180} \left( 1215g_{A2}^4 - 160g_3^4 + 18g_{A1}^2 g_{A2}^2 + 32g_3^2 (45g_{A2}^2 + g_{A1}^2) + 47g_{A1}^4 \right) \mathbf{1} \\ & + \frac{1}{5} \left( -5 \left( Y_d^\dagger Y_d Y_d^\dagger Y_d + Y_u^\dagger Y_u Y_u^\dagger Y_u \right) + Y_d^\dagger Y_d (2g_{A1}^2 - 5\text{Tr}(Y_d Y_d^\dagger)) - 5\text{Tr}(Y_e Y_e^\dagger) \right) \\ & + Y_u^\dagger Y_u (4g_{A1}^2 - 5\text{Tr}(Y_u Y_u^\dagger)) \end{aligned} \quad (8)$$

$$\gamma_{\hat{L}}^{(1)} = -\frac{3}{10} \left( 5g_{A2}^2 + g_{A1}^2 \right) \mathbf{1} + Y_e^\dagger Y_e \quad (9)$$

$$\gamma_{\hat{L}}^{(2)} = -2Y_e^\dagger Y_e Y_e^\dagger Y_e + \frac{9}{100} \left( 10g_{A1}^2 g_{A2}^2 + 27g_{A1}^4 + 75g_{A2}^4 \right) \mathbf{1} + Y_e^\dagger Y_e \left( \frac{6}{5} g_{A1}^2 - \text{Tr}(Y_d Y_d^\dagger) - \text{Tr}(Y_e Y_e^\dagger) \right) \quad (10)$$

$$\gamma_{\hat{H}_d}^{(1)} = -\frac{3}{10} \left( 5g_{A2}^2 + g_{A1}^2 \right) + \text{Tr}(Y_d Y_d^\dagger) + \text{Tr}(Y_e Y_e^\dagger) \quad (11)$$

$$\begin{aligned} \gamma_{\hat{H}_d}^{(2)} = & +\frac{243}{100} g_{A1}^4 + \frac{9}{10} g_{A1}^2 g_{A2}^2 + \frac{27}{4} g_{A2}^4 + \frac{2}{15} \left( 40g_3^2 - g_{A1}^2 \right) \text{Tr}(Y_d Y_d^\dagger) + \frac{6}{5} g_{A1}^2 \text{Tr}(Y_e Y_e^\dagger) - 2\text{Tr}(Y_d Y_d^\dagger Y_d Y_d^\dagger) \\ & - \text{Tr}(Y_d Y_u^\dagger Y_u Y_d^\dagger) - 3\text{Tr}(Y_e Y_e^\dagger Y_e Y_e^\dagger) \end{aligned} \quad (12)$$

$$\gamma_{\hat{H}_u}^{(1)} = -\frac{3}{10} \left( 5g_{A2}^2 + g_{A1}^2 \right) + \text{Tr}(Y_u Y_u^\dagger) \quad (13)$$

$$\gamma_{\hat{H}_u}^{(2)} = -2\text{Tr}(Y_u Y_u^\dagger Y_u Y_u^\dagger) + \frac{243}{100} g_{A1}^4 + \frac{27}{4} g_{A2}^4 + \frac{4}{15} \left( 20g_3^2 + g_{A1}^2 \right) \text{Tr}(Y_u Y_u^\dagger) + \frac{9}{10} g_{A1}^2 g_{A2}^2 - \text{Tr}(Y_d Y_u^\dagger Y_u Y_d^\dagger) \quad (14)$$

$$\gamma_{\hat{u}_R}^{(1)} = -\frac{8}{15} \left( 5g_3^2 + g_{A1}^2 \right) \mathbf{1} + Y_u^* Y_u^T \quad (15)$$

$$\begin{aligned} \gamma_{\hat{u}_R}^{(2)} = & -\frac{8}{45} \left( -16g_3^2 g_{A1}^2 - 25g_{A1}^4 + 5g_3^4 \right) \mathbf{1} - Y_u^* Y_d^T Y_d^* Y_u^T - Y_u^* Y_u^T Y_u^* Y_u^T \\ & - \frac{1}{5} Y_u^* Y_u^T \left( -15g_{A2}^2 + 5\text{Tr}(Y_u Y_u^\dagger) + g_{A1}^2 \right) \end{aligned} \quad (16)$$

$$\gamma_{\hat{d}_R}^{(1)} = -\frac{2}{15} \left( 20g_3^2 + g_{A1}^2 \right) \mathbf{1} + Y_d^* Y_d^T \quad (17)$$

$$\begin{aligned} \gamma_{\hat{d}_R}^{(2)} = & -\frac{2}{225} \left( 100g_3^4 - 119g_{A1}^4 - 80g_3^2 g_{A1}^2 \right) \mathbf{1} - Y_d^* Y_d^T Y_d^* Y_d^T - Y_d^* Y_u^T Y_u^* Y_d^T \\ & + \frac{1}{5} Y_d^* Y_d^T \left( 15g_{A2}^2 - 5\text{Tr}(Y_d Y_d^\dagger) - 5\text{Tr}(Y_e Y_e^\dagger) + g_{A1}^2 \right) \end{aligned} \quad (18)$$

$$\gamma_{\hat{e}_R}^{(1)} = 2Y_e^* Y_e^T - \frac{6}{5} g_{A1}^2 \mathbf{1} \quad (19)$$

$$\gamma_{\hat{e}_R}^{(2)} = -2Y_e^* Y_e^T Y_e^* Y_e^T + \frac{54}{5} g_{A1}^4 \mathbf{1} + Y_e^* Y_e^T \left( -2\text{Tr}(Y_d Y_d^\dagger) - 2\text{Tr}(Y_e Y_e^\dagger) + 6g_{A2}^2 - \frac{6}{5} g_{A1}^2 \right) \quad (20)$$

$$\gamma_{\hat{L}}^{(1)} = \frac{1}{20} \left( 30|Y_A|^2 + 5|Y_K|^2 - 6 \left( 5g_{A2}^2 + 5g_{B2}^2 + g_{A1}^2 + g_{B1}^2 \right) \right) \quad (21)$$

$$\gamma_{\hat{L}}^{(2)} = \frac{1}{400} \left( 12 \left( 30g_{A1}^2 (g_{A2}^2 + g_{B1}^2 + g_{B2}^2) + 5 \left( 3g_{B1}^4 + 45g_{A2}^4 - 5g_{B2}^4 + 6g_{A2}^2 (5g_{B2}^2 + g_{B1}^2) + 6g_{B1}^2 g_{B2}^2 \right) + 81g_{A1}^4 \right) \right)$$

$$-2100Y_A^2Y_A^{*,2} - 125Y_K^2Y_K^{*,2} + 300|Y_A|^2(8g_{B2}^2 - Y_KY_K^*) \quad (22)$$

$$\gamma_{\hat{L}}^{(1)} = \frac{1}{20} \left( 30|Y_A|^2 + 5|Y_K|^2 - 6(5g_{A2}^2 + 5g_{B2}^2 + g_{A1}^2 + g_{B1}^2) \right) \quad (23)$$

$$\gamma_{\hat{L}}^{(2)} = \frac{1}{400} \left( 12 \left( 30g_{A1}^2(g_{A2}^2 + g_{B1}^2 + g_{B2}^2) + 5(3g_{B1}^4 + 45g_{A2}^4 - 5g_{B2}^4 + 6g_{A2}^2(5g_{B2}^2 + g_{B1}^2) + 6g_{B1}^2g_{B2}^2) + 81g_{A1}^4 \right) \right. \\ \left. - 2100Y_A^2Y_A^{*,2} - 125Y_K^2Y_K^{*,2} + 300|Y_A|^2(8g_{B2}^2 - Y_KY_K^*) \right) \quad (24)$$

$$\gamma_{\hat{K}}^{(1)} = |Y_K|^2 \quad (25)$$

$$\gamma_{\hat{K}}^{(2)} = -\frac{1}{10} |Y_K|^2 \left( 30Y_A Y_A^* + 5Y_K Y_K^* - 6(5g_{A2}^2 + 5g_{B2}^2 + g_{A1}^2 + g_{B1}^2) \right) \quad (26)$$

$$\gamma_{\hat{Ad}}^{(1)} = 2|Y_A|^2 - 4g_{B2}^2 \quad (27)$$

$$\gamma_{\hat{Ad}}^{(2)} = -6Y_A^2Y_A^{*,2} + 8g_{B2}^4 + \frac{1}{5}|Y_A|^2 \left( -10g_{B2}^2 + 30g_{A2}^2 - 5Y_K Y_K^* + 6g_{A1}^2 + 6g_{B1}^2 \right) \quad (28)$$

### 3.2 Gauge Couplings

$$\beta_{g_{B1}}^{(1)} = \frac{6}{5}g_{B1}^3 \quad (29)$$

$$\beta_{g_{B1}}^{(2)} = \frac{3}{25}g_{B1}^3 \left( -30|Y_A|^2 - 5|Y_K|^2 + 6(5g_{A2}^2 + 5g_{B2}^2 + g_{A1}^2 + g_{B1}^2) \right) \quad (30)$$

$$\beta_{g_{B2}}^{(1)} = -2g_{B2}^3 \quad (31)$$

$$\beta_{g_{B2}}^{(2)} = \frac{1}{5}g_{B2}^3 \left( 30g_{A2}^2 - 5|Y_K|^2 + 6g_{A1}^2 + 6g_{B1}^2 + 70g_{B2}^2 - 70|Y_A|^2 \right) \quad (32)$$

$$\beta_{g_{A1}}^{(1)} = \frac{39}{5}g_{A1}^3 \quad (33)$$

$$\beta_{g_{A1}}^{(2)} = \frac{1}{75}g_{A1}^3 \left( 1320g_3^2 + 651g_{A1}^2 + 675g_{A2}^2 + 54g_{B1}^2 + 270g_{B2}^2 - 270|Y_A|^2 - 45|Y_K|^2 - 70\text{Tr}(Y_d Y_d^\dagger) - 270\text{Tr}(Y_e Y_e^\dagger) \right. \\ \left. - 130\text{Tr}(Y_u Y_u^\dagger) \right) \quad (34)$$

$$\beta_{g_{A2}}^{(1)} = 3g_{A2}^3 \quad (35)$$

$$\beta_{g_{A2}}^{(2)} = \frac{1}{5}g_{A2}^3 \left( 120g_3^2 + 15g_{A1}^2 + 195g_{A2}^2 + 6g_{B1}^2 + 30g_{B2}^2 - 30|Y_A|^2 - 5|Y_K|^2 - 10\text{Tr}(Y_d Y_d^\dagger) - 10\text{Tr}(Y_e Y_e^\dagger) \right. \\ \left. - 10\text{Tr}(Y_u Y_u^\dagger) \right) \quad (36)$$

$$\beta_{g_3}^{(1)} = -3g_3^3 \quad (37)$$

$$\beta_{g_3}^{(2)} = \frac{1}{15}g_3^3 \left( 135g_{A2}^2 - 20\text{Tr}(Y_d Y_d^\dagger) - 20\text{Tr}(Y_u Y_u^\dagger) + 210g_3^2 + 33g_{A1}^2 \right) \quad (38)$$

### 3.3 Gaugino Mass Parameters

$$\beta_{m_{B_B}}^{(1)} = \frac{12}{5} g_{B1}^2 m_{B_B} \quad (39)$$

$$\begin{aligned} \beta_{m_{B_B}}^{(2)} = & \frac{6}{25} g_{B1}^2 \left( 6 \left( 2g_{B1}^2 m_{B_B} + 5g_{A2}^2 (m_{W_A} + m_{B_B}) + 5g_{B2}^2 m_{B_B} + 5g_{B2}^2 m_{W_B} + g_{A1}^2 (m_{B_A} + m_{B_B}) \right) - 30Y_A^* (m_{B_B} Y_A - T_A) \right. \\ & \left. + Y_K^* (-5m_{B_B} Y_K + 5T_K) \right) \end{aligned} \quad (40)$$

$$\beta_{m_{W_B}}^{(1)} = -4g_{B2}^2 m_{W_B} \quad (41)$$

$$\begin{aligned} \beta_{m_{W_B}}^{(2)} = & \frac{2}{5} g_{B2}^2 \left( 6g_{A1}^2 m_{B_A} + 30g_{A2}^2 m_{W_A} + 6g_{B1}^2 m_{B_B} + 6g_{A1}^2 m_{W_B} + 30g_{A2}^2 m_{W_B} + 6g_{B1}^2 m_{W_B} + 140g_{B2}^2 m_{W_B} \right. \\ & \left. - 70Y_A^* (m_{W_B} Y_A - T_A) + Y_K^* (-5m_{W_B} Y_K + 5T_K) \right) \end{aligned} \quad (42)$$

$$\beta_{m_{B_A}}^{(1)} = \frac{78}{5} g_{A1}^2 m_{B_A} \quad (43)$$

$$\begin{aligned} \beta_{m_{B_A}}^{(2)} = & \frac{2}{75} g_{A1}^2 \left( -270Y_A^* (m_{B_A} Y_A - T_A) - 45Y_K^* (m_{B_A} Y_K - T_K) \right. \\ & + 2 \left( 620g_3^2 m_{B_A} + 650g_{A1}^2 m_{B_A} + 315g_{A2}^2 m_{B_A} + 27g_{B1}^2 m_{B_A} + 135g_{B2}^2 m_{B_A} + 315g_{A2}^2 m_{W_A} + 27g_{B1}^2 m_{B_B} + 135g_{B2}^2 m_{W_B} \right. \\ & + 620g_3^2 M_3 - 35m_{B_A} \text{Tr}(Y_d Y_d^\dagger) - 135m_{B_A} \text{Tr}(Y_e Y_e^\dagger) - 65m_{B_A} \text{Tr}(Y_u Y_u^\dagger) + 35\text{Tr}(Y_d^\dagger T_d) \\ & \left. \left. + 135\text{Tr}(Y_e^\dagger T_e) + 65\text{Tr}(Y_u^\dagger T_u) \right) \right) \end{aligned} \quad (44)$$

$$\beta_{m_{W_A}}^{(1)} = 6g_{A2}^2 m_{W_A} \quad (45)$$

$$\begin{aligned} \beta_{m_{W_A}}^{(2)} = & \frac{2}{5} g_{A2}^2 \left( 15g_{A1}^2 m_{B_A} + 120g_3^2 m_{W_A} + 15g_{A1}^2 m_{W_A} + 390g_{A2}^2 m_{W_A} + 6g_{B1}^2 m_{W_A} + 30g_{B2}^2 m_{W_A} + 6g_{B1}^2 m_{B_B} + 30g_{B2}^2 m_{W_B} \right. \\ & + 120g_3^2 M_3 - 30Y_A^* (m_{W_A} Y_A - T_A) + Y_K^* (-5m_{W_A} Y_K + 5T_K) - 10m_{W_A} \text{Tr}(Y_d Y_d^\dagger) - 10m_{W_A} \text{Tr}(Y_e Y_e^\dagger) \\ & \left. - 10m_{W_A} \text{Tr}(Y_u Y_u^\dagger) + 10\text{Tr}(Y_d^\dagger T_d) + 10\text{Tr}(Y_e^\dagger T_e) + 10\text{Tr}(Y_u^\dagger T_u) \right) \end{aligned} \quad (46)$$

$$\beta_{M_3}^{(1)} = -6g_3^2 M_3 \quad (47)$$

$$\begin{aligned} \beta_{M_3}^{(2)} = & \frac{2}{15} g_3^2 \left( 33g_{A1}^2 m_{B_A} + 135g_{A2}^2 m_{W_A} + 420g_3^2 M_3 + 33g_{A1}^2 M_3 + 135g_{A2}^2 M_3 - 20M_3 \text{Tr}(Y_d Y_d^\dagger) - 20M_3 \text{Tr}(Y_u Y_u^\dagger) \right. \\ & \left. + 20\text{Tr}(Y_d^\dagger T_d) + 20\text{Tr}(Y_u^\dagger T_u) \right) \end{aligned} \quad (48)$$

### 3.4 Trilinear Superpotential Parameters

$$\beta_{Y_u}^{(1)} = 2Y_u Y_u^\dagger Y_u + Y_u \left( -3g_{A2}^2 - \frac{13}{15} g_{A1}^2 - \frac{16}{3} g_3^2 + \text{Tr}(Y_u Y_u^\dagger) \right) + Y_u Y_d^\dagger Y_d \quad (49)$$

$$\begin{aligned} \beta_{Y_u}^{(2)} = & + \frac{3}{5} g_{A1}^2 Y_u Y_u^\dagger Y_u + 3g_{A2}^2 Y_u Y_u^\dagger Y_u - Y_u Y_d^\dagger Y_d Y_d^\dagger Y_d - Y_u Y_d^\dagger Y_d Y_u^\dagger Y_u \\ & - 2Y_u Y_u^\dagger Y_u Y_u^\dagger Y_u + Y_u Y_d^\dagger Y_d \left( \frac{2}{5} g_{A1}^2 - \text{Tr}(Y_d Y_d^\dagger) - \text{Tr}(Y_e Y_e^\dagger) \right) - 2Y_u Y_u^\dagger Y_u \text{Tr}(Y_u Y_u^\dagger) \end{aligned}$$



$$\begin{aligned}
& + Y_u \left( -\frac{16}{9}g_3^4 + \frac{136}{45}g_3^2g_{A1}^2 + \frac{3211}{450}g_{A1}^4 + 8g_3^2g_{A2}^2 + g_{A1}^2g_{A2}^2 + \frac{27}{2}g_{A2}^4 + \frac{4}{15}(20g_3^2 + g_{A1}^2) \text{Tr}(Y_u Y_u^\dagger) \right. \\
& \left. - \text{Tr}(Y_d Y_u^\dagger Y_u Y_d^\dagger) - 2\text{Tr}(Y_u Y_u^\dagger Y_u Y_u^\dagger) \right)
\end{aligned} \tag{50}$$

$$\beta_{Y_d}^{(1)} = 2Y_d Y_d^\dagger Y_d + Y_d \left( -3g_{A2}^2 - \frac{16}{3}g_3^2 - \frac{7}{15}g_{A1}^2 + \text{Tr}(Y_d Y_d^\dagger) + \text{Tr}(Y_e Y_e^\dagger) \right) + Y_d Y_u^\dagger Y_u \tag{51}$$

$$\begin{aligned}
\beta_{Y_d}^{(2)} = & + \frac{4}{5}g_{A1}^2 Y_d Y_u^\dagger Y_u - 2Y_d Y_d^\dagger Y_d Y_d^\dagger Y_d - Y_d Y_u^\dagger Y_u Y_d^\dagger Y_d - Y_d Y_u^\dagger Y_u Y_u^\dagger Y_u \\
& + Y_d Y_d^\dagger Y_d \left( -2\text{Tr}(Y_d Y_d^\dagger) - 2\text{Tr}(Y_e Y_e^\dagger) + 3g_{A2}^2 + \frac{3}{5}g_{A1}^2 \right) - Y_d Y_u^\dagger Y_u \text{Tr}(Y_u Y_u^\dagger) \\
& + Y_d \left( -\frac{16}{9}g_3^4 + \frac{8}{9}g_3^2g_{A1}^2 + \frac{1687}{450}g_{A1}^4 + 8g_3^2g_{A2}^2 + g_{A1}^2g_{A2}^2 + \frac{27}{2}g_{A2}^4 + \frac{2}{15}(40g_3^2 - g_{A1}^2) \text{Tr}(Y_d Y_d^\dagger) \right. \\
& \left. + \frac{6}{5}g_{A1}^2 \text{Tr}(Y_e Y_e^\dagger) - 2\text{Tr}(Y_d Y_d^\dagger Y_d Y_d^\dagger) - \text{Tr}(Y_d Y_u^\dagger Y_u Y_d^\dagger) - 3\text{Tr}(Y_e Y_e^\dagger Y_e Y_e^\dagger) \right)
\end{aligned} \tag{52}$$

$$\beta_{Y_e}^{(1)} = 3Y_e Y_e^\dagger Y_e + Y_e \left( -3g_{A2}^2 - \frac{9}{5}g_{A1}^2 + \text{Tr}(Y_d Y_d^\dagger) + \text{Tr}(Y_e Y_e^\dagger) \right) \tag{53}$$

$$\begin{aligned}
\beta_{Y_e}^{(2)} = & -4Y_e Y_e^\dagger Y_e Y_e^\dagger Y_e + Y_e Y_e^\dagger Y_e \left( -3\text{Tr}(Y_d Y_d^\dagger) - 3\text{Tr}(Y_e Y_e^\dagger) + 6g_{A2}^2 \right) \\
& + Y_e \left( \frac{783}{50}g_{A1}^4 + \frac{9}{5}g_{A1}^2g_{A2}^2 + \frac{27}{2}g_{A2}^4 + \frac{2}{15}(40g_3^2 - g_{A1}^2) \text{Tr}(Y_d Y_d^\dagger) + \frac{6}{5}g_{A1}^2 \text{Tr}(Y_e Y_e^\dagger) - 2\text{Tr}(Y_d Y_d^\dagger Y_d Y_d^\dagger) \right. \\
& \left. - \text{Tr}(Y_d Y_u^\dagger Y_u Y_d^\dagger) - 3\text{Tr}(Y_e Y_e^\dagger Y_e Y_e^\dagger) \right)
\end{aligned} \tag{54}$$

$$\beta_{Y_K}^{(1)} = \frac{3}{10}Y_K \left( 10|Y_A|^2 - 2(5g_{A2}^2 + 5g_{B2}^2 + g_{A1}^2 + g_{B1}^2) + 5|Y_K|^2 \right) \tag{55}$$

$$\begin{aligned}
\beta_{Y_K}^{(2)} = & -\frac{3}{200}Y_K \left( -4(30g_{A1}^2(g_{A2}^2 + g_{B1}^2 + g_{B2}^2) + 5(3g_{B1}^4 + 45g_{A2}^4 - 5g_{B2}^4 + 6g_{A2}^2(5g_{B2}^2 + g_{B1}^2) + 6g_{B1}^2g_{B2}^2) + 81g_{A1}^4) \right. \\
& \left. - 40(5g_{A2}^2 + 5g_{B2}^2 + g_{A1}^2 + g_{B1}^2)|Y_K|^2 + 700Y_A^2Y_A^{*,2} + 75Y_K^2Y_K^{*,2} - 100|Y_A|^2(-3Y_KY_K^* + 8g_{B2}^2) \right)
\end{aligned} \tag{56}$$

$$\beta_{Y_A}^{(1)} = \frac{1}{10}Y_A \left( -2(15g_{A2}^2 + 35g_{B2}^2 + 3g_{A1}^2 + 3g_{B1}^2) + 50|Y_A|^2 + 5|Y_K|^2 \right) \tag{57}$$

$$\begin{aligned}
\beta_{Y_A}^{(2)} = & -\frac{1}{200}Y_A \left( -4(243g_{A1}^4 + 5(135g_{A2}^4 + 18g_{A2}^2(5g_{B2}^2 + g_{B1}^2) + 18g_{B1}^2g_{B2}^2 + 65g_{B2}^4 + 9g_{B1}^4) + 90g_{A1}^2(g_{A2}^2 + g_{B1}^2 + g_{B2}^2) \right. \\
& \left. + 3300Y_A^2Y_A^{*,2} + 125Y_K^2Y_K^{*,2} - 20|Y_A|^2(-25Y_KY_K^* + 4(15g_{A2}^2 + 25g_{B2}^2 + 3g_{A1}^2 + 3g_{B1}^2)) \right)
\end{aligned} \tag{58}$$

### 3.5 Bilinear Superpotential Parameters

$$\beta_\mu^{(1)} = -3g_{A2}^2\mu - \frac{3}{5}g_{A1}^2\mu + \mu \text{Tr}(Y_d Y_d^\dagger) + \mu \text{Tr}(Y_e Y_e^\dagger) + \mu \text{Tr}(Y_u Y_u^\dagger) \tag{59}$$

$$\begin{aligned}
\beta_\mu^{(2)} = & \frac{1}{150}\mu \left( 729g_{A1}^4 + 270g_{A1}^2g_{A2}^2 + 2025g_{A2}^4 + 20(40g_3^2 - g_{A1}^2) \text{Tr}(Y_d Y_d^\dagger) + 180g_{A1}^2 \text{Tr}(Y_e Y_e^\dagger) \right. \\
& + 800g_3^2 \text{Tr}(Y_u Y_u^\dagger) + 40g_{A1}^2 \text{Tr}(Y_u Y_u^\dagger) - 300\text{Tr}(Y_d Y_d^\dagger Y_d Y_d^\dagger) - 300\text{Tr}(Y_d Y_u^\dagger Y_u Y_d^\dagger) \\
& \left. - 450\text{Tr}(Y_e Y_e^\dagger Y_e Y_e^\dagger) - 300\text{Tr}(Y_u Y_u^\dagger Y_u Y_u^\dagger) \right)
\end{aligned} \tag{60}$$

### 3.6 Linear Superpotential Parameters

$$\beta_{\Omega}^{(1)} = \Omega |Y_K|^2 \quad (61)$$

$$\beta_{\Omega}^{(2)} = -\frac{1}{10} \Omega |Y_K|^2 \left( 30 Y_A Y_A^* + 5 Y_K Y_K^* - 6 \left( 5 g_{A2}^2 + 5 g_{B2}^2 + g_{A1}^2 + g_{B1}^2 \right) \right) \quad (62)$$

### 3.7 Trilinear Soft-Breaking Parameters

$$\begin{aligned} \beta_{T_u}^{(1)} = & +2Y_u Y_d^\dagger T_d + 3Y_u Y_u^\dagger T_u + T_u Y_d^\dagger Y_d + 3T_u Y_u^\dagger Y_u - \frac{16}{3} g_3^2 T_u - \frac{13}{15} g_{A1}^2 T_u - 3g_{A2}^2 T_u \\ & + T_u \text{Tr} \left( Y_u Y_u^\dagger \right) + Y_u \left( 2\text{Tr} \left( Y_u^\dagger T_u \right) + 6g_{A2}^2 m_{W_A} + \frac{26}{15} g_{A1}^2 m_{B_A} + \frac{32}{3} g_3^2 M_3 \right) \end{aligned} \quad (63)$$

$$\begin{aligned} \beta_{T_u}^{(2)} = & +\frac{4}{5} g_{A1}^2 Y_u Y_d^\dagger T_d - \frac{6}{5} g_{A1}^2 m_{B_A} Y_u Y_u^\dagger Y_u - 6g_{A2}^2 m_{W_A} Y_u Y_u^\dagger Y_u + \frac{7}{5} g_{A1}^2 Y_u Y_u^\dagger T_u \\ & + 3g_{A2}^2 Y_u Y_u^\dagger T_u + \frac{2}{5} g_{A1}^2 T_u Y_d^\dagger Y_d + \frac{2}{5} g_{A1}^2 T_u Y_u^\dagger Y_u + 6g_{A2}^2 T_u Y_u^\dagger Y_u \\ & - 2Y_u Y_d^\dagger Y_d Y_d^\dagger T_d - Y_u Y_d^\dagger Y_d Y_u^\dagger T_u - 2Y_u Y_d^\dagger T_d Y_d^\dagger Y_d - 2Y_u Y_d^\dagger T_d Y_u^\dagger Y_u \\ & - 3Y_u Y_u^\dagger Y_u Y_u^\dagger T_u - 4Y_u Y_u^\dagger T_u Y_u^\dagger Y_u - T_u Y_d^\dagger Y_d Y_d^\dagger Y_d - 2T_u Y_d^\dagger Y_d Y_u^\dagger Y_u \\ & - 3T_u Y_u^\dagger Y_u Y_u^\dagger Y_u - \frac{16}{9} g_3^4 T_u + \frac{136}{45} g_3^2 g_{A1}^2 T_u + \frac{3211}{450} g_{A1}^4 T_u + 8g_3^2 g_{A2}^2 T_u + g_{A1}^2 g_{A2}^2 T_u + \frac{27}{2} g_{A2}^4 T_u \\ & - 2Y_u Y_d^\dagger T_d \text{Tr} \left( Y_d Y_d^\dagger \right) - T_u Y_d^\dagger Y_d \text{Tr} \left( Y_d Y_d^\dagger \right) - 2Y_u Y_d^\dagger T_d \text{Tr} \left( Y_e Y_e^\dagger \right) \\ & - T_u Y_d^\dagger Y_d \text{Tr} \left( Y_e Y_e^\dagger \right) - 3Y_u Y_u^\dagger T_u \text{Tr} \left( Y_u Y_u^\dagger \right) - 3T_u Y_u^\dagger Y_u \text{Tr} \left( Y_u Y_u^\dagger \right) \\ & + \frac{16}{3} g_3^2 T_u \text{Tr} \left( Y_u Y_u^\dagger \right) + \frac{4}{15} g_{A1}^2 T_u \text{Tr} \left( Y_u Y_u^\dagger \right) \\ & - \frac{2}{5} Y_u Y_d^\dagger Y_d \left( 2g_{A1}^2 m_{B_A} + 5\text{Tr} \left( Y_d^\dagger T_d \right) + 5\text{Tr} \left( Y_e^\dagger T_e \right) \right) - 4Y_u Y_u^\dagger Y_u \text{Tr} \left( Y_u^\dagger T_u \right) \\ & - T_u \text{Tr} \left( Y_d Y_u^\dagger Y_u Y_d^\dagger \right) - 2T_u \text{Tr} \left( Y_u Y_u^\dagger Y_u Y_u^\dagger \right) \\ & + Y_u \left( -\frac{272}{45} g_3^2 g_{A1}^2 m_{B_A} - \frac{6422}{225} g_{A1}^4 m_{B_A} - 2g_{A1}^2 g_{A2}^2 m_{B_A} - 16g_3^2 g_{A2}^2 m_{W_A} - 2g_{A1}^2 g_{A2}^2 m_{W_A} - 54g_{A2}^4 m_{W_A} \right. \\ & + \frac{64}{9} g_3^4 M_3 - \frac{272}{45} g_3^2 g_{A1}^2 M_3 - 16g_3^2 g_{A2}^2 M_3 - \frac{8}{15} \left( 20g_3^2 M_3 + g_{A1}^2 m_{B_A} \right) \text{Tr} \left( Y_u Y_u^\dagger \right) \\ & \left. + \frac{8}{15} \left( 20g_3^2 + g_{A1}^2 \right) \text{Tr} \left( Y_u^\dagger T_u \right) - 2\text{Tr} \left( Y_d Y_u^\dagger T_u Y_d^\dagger \right) - 2\text{Tr} \left( Y_u Y_d^\dagger T_d Y_u^\dagger \right) - 8\text{Tr} \left( Y_u Y_u^\dagger T_u Y_u^\dagger \right) \right) \end{aligned} \quad (64)$$

$$\begin{aligned} \beta_{T_d}^{(1)} = & +3Y_d Y_d^\dagger T_d + 2Y_d Y_u^\dagger T_u + 3T_d Y_d^\dagger Y_d + T_d Y_u^\dagger Y_u - \frac{16}{3} g_3^2 T_d - \frac{7}{15} g_{A1}^2 T_d - 3g_{A2}^2 T_d \\ & + T_d \text{Tr} \left( Y_d Y_d^\dagger \right) + T_d \text{Tr} \left( Y_e Y_e^\dagger \right) + Y_d \left( 2\text{Tr} \left( Y_d^\dagger T_d \right) + 2\text{Tr} \left( Y_e^\dagger T_e \right) + 6g_{A2}^2 m_{W_A} + \frac{14}{15} g_{A1}^2 m_{B_A} + \frac{32}{3} g_3^2 M_3 \right) \end{aligned} \quad (65)$$

$$\begin{aligned} \beta_{T_d}^{(2)} = & +g_{A1}^2 Y_d Y_d^\dagger T_d + 3g_{A2}^2 Y_d Y_d^\dagger T_d - \frac{8}{5} g_{A1}^2 m_{B_A} Y_d Y_u^\dagger Y_u + \frac{8}{5} g_{A1}^2 Y_d Y_u^\dagger T_u \\ & + \frac{4}{5} g_{A1}^2 T_d Y_d^\dagger Y_d + 6g_{A2}^2 T_d Y_d^\dagger Y_d + \frac{4}{5} g_{A1}^2 T_d Y_u^\dagger Y_u - 3Y_d Y_d^\dagger Y_d Y_d^\dagger T_d \end{aligned}$$

$$\begin{aligned}
& -4Y_d Y_d^\dagger T_d Y_d^\dagger Y_d - Y_d Y_u^\dagger Y_u Y_d^\dagger T_d - 2Y_d Y_u^\dagger Y_u Y_u^\dagger T_u - 2Y_d Y_u^\dagger T_u Y_d^\dagger Y_d \\
& -2Y_d Y_u^\dagger T_u Y_u^\dagger Y_u - 3T_d Y_d^\dagger Y_d Y_d^\dagger Y_d - 2T_d Y_u^\dagger Y_u Y_d^\dagger Y_d - T_d Y_u^\dagger Y_u Y_u^\dagger Y_u \\
& -\frac{16}{9}g_3^4 T_d + \frac{8}{9}g_3^2 g_{A1}^2 T_d + \frac{1687}{450}g_{A1}^4 T_d + 8g_3^2 g_{A2}^2 T_d + g_{A1}^2 g_{A2}^2 T_d + \frac{27}{2}g_{A2}^4 T_d \\
& -3Y_d Y_d^\dagger T_d \text{Tr}(Y_d Y_d^\dagger) - 3T_d Y_d^\dagger Y_d \text{Tr}(Y_d Y_d^\dagger) + \frac{16}{3}g_3^2 T_d \text{Tr}(Y_d Y_d^\dagger) \\
& -\frac{2}{15}g_{A1}^2 T_d \text{Tr}(Y_d Y_d^\dagger) - 3Y_d Y_d^\dagger T_d \text{Tr}(Y_e Y_e^\dagger) - 3T_d Y_d^\dagger Y_d \text{Tr}(Y_e Y_e^\dagger) \\
& +\frac{6}{5}g_{A1}^2 T_d \text{Tr}(Y_e Y_e^\dagger) - 2Y_d Y_u^\dagger T_u \text{Tr}(Y_u Y_u^\dagger) - T_d Y_u^\dagger Y_u \text{Tr}(Y_u Y_u^\dagger) \\
& +Y_d Y_d^\dagger Y_d \left( -4\text{Tr}(Y_d^\dagger T_d) - 4\text{Tr}(Y_e^\dagger T_e) - 6g_{A2}^2 m_{W_A} - \frac{6}{5}g_{A1}^2 m_{B_A} \right) - 2Y_d Y_u^\dagger Y_u \text{Tr}(Y_u^\dagger T_u) \\
& -2T_d \text{Tr}(Y_d Y_d^\dagger Y_d Y_d^\dagger) - T_d \text{Tr}(Y_d Y_u^\dagger Y_u Y_d^\dagger) - 3T_d \text{Tr}(Y_e Y_e^\dagger Y_e Y_e^\dagger) \\
& +Y_d \left( -\frac{16}{9}g_3^2 g_{A1}^2 m_{B_A} - \frac{3374}{225}g_{A1}^4 m_{B_A} - 2g_{A1}^2 g_{A2}^2 m_{B_A} - 16g_3^2 g_{A2}^2 m_{W_A} - 2g_{A1}^2 g_{A2}^2 m_{W_A} - 54g_{A2}^4 m_{W_A} \right. \\
& +\frac{64}{9}g_3^4 M_3 - \frac{16}{9}g_3^2 g_{A1}^2 M_3 - 16g_3^2 g_{A2}^2 M_3 + \frac{4}{15} \left( -40g_3^2 M_3 + g_{A1}^2 m_{B_A} \right) \text{Tr}(Y_d Y_d^\dagger) \\
& -\frac{12}{5}g_{A1}^2 m_{B_A} \text{Tr}(Y_e Y_e^\dagger) + \frac{32}{3}g_3^2 \text{Tr}(Y_d^\dagger T_d) - \frac{4}{15}g_{A1}^2 \text{Tr}(Y_d^\dagger T_d) + \frac{12}{5}g_{A1}^2 \text{Tr}(Y_e^\dagger T_e) \\
& \left. -8\text{Tr}(Y_d Y_d^\dagger T_d Y_d^\dagger) - 2\text{Tr}(Y_d Y_u^\dagger T_u Y_d^\dagger) - 12\text{Tr}(Y_e Y_e^\dagger T_e Y_e^\dagger) - 2\text{Tr}(Y_u Y_d^\dagger T_d Y_u^\dagger) \right) \tag{66}
\end{aligned}$$

$$\begin{aligned}
\beta_{T_e}^{(1)} &= +4Y_e Y_e^\dagger T_e + 5T_e Y_e^\dagger Y_e - \frac{9}{5}g_{A1}^2 T_e - 3g_{A2}^2 T_e + T_e \text{Tr}(Y_d Y_d^\dagger) + T_e \text{Tr}(Y_e Y_e^\dagger) \\
&+ Y_e \left( 2\text{Tr}(Y_d^\dagger T_d) + 2\text{Tr}(Y_e^\dagger T_e) + 6g_{A2}^2 m_{W_A} + \frac{18}{5}g_{A1}^2 m_{B_A} \right) \tag{67}
\end{aligned}$$

$$\begin{aligned}
\beta_{T_e}^{(2)} &= +\frac{6}{5}g_{A1}^2 Y_e Y_e^\dagger T_e + 6g_{A2}^2 Y_e Y_e^\dagger T_e - \frac{6}{5}g_{A1}^2 T_e Y_e^\dagger Y_e + 12g_{A2}^2 T_e Y_e^\dagger Y_e \\
&-6Y_e Y_e^\dagger Y_e Y_e^\dagger T_e - 8Y_e Y_e^\dagger T_e Y_e^\dagger Y_e - 6T_e Y_e^\dagger Y_e Y_e^\dagger Y_e + \frac{783}{50}g_{A1}^4 T_e + \frac{9}{5}g_{A1}^2 g_{A2}^2 T_e + \frac{27}{2}g_{A2}^4 T_e \\
&-4Y_e Y_e^\dagger T_e \text{Tr}(Y_d Y_d^\dagger) - 5T_e Y_e^\dagger Y_e \text{Tr}(Y_d Y_d^\dagger) + \frac{16}{3}g_3^2 T_e \text{Tr}(Y_d Y_d^\dagger) \\
&-\frac{2}{15}g_{A1}^2 T_e \text{Tr}(Y_d Y_d^\dagger) - 4Y_e Y_e^\dagger T_e \text{Tr}(Y_e Y_e^\dagger) - 5T_e Y_e^\dagger Y_e \text{Tr}(Y_e Y_e^\dagger) \\
&+\frac{6}{5}g_{A1}^2 T_e \text{Tr}(Y_e Y_e^\dagger) - 6Y_e Y_e^\dagger Y_e \left( 2g_{A2}^2 m_{W_A} + \text{Tr}(Y_d^\dagger T_d) + \text{Tr}(Y_e^\dagger T_e) \right) - 2T_e \text{Tr}(Y_d Y_d^\dagger Y_d Y_d^\dagger) \\
&-T_e \text{Tr}(Y_d Y_u^\dagger Y_u Y_d^\dagger) - 3T_e \text{Tr}(Y_e Y_e^\dagger Y_e Y_e^\dagger) \\
&-\frac{2}{75}Y_e \left( 2349g_{A1}^4 m_{B_A} + 135g_{A1}^2 g_{A2}^2 m_{B_A} + 135g_{A1}^2 g_{A2}^2 m_{W_A} + 2025g_{A2}^4 m_{W_A} - 10 \left( -40g_3^2 M_3 + g_{A1}^2 m_{B_A} \right) \text{Tr}(Y_d Y_d^\dagger) \right. \\
&+ 90g_{A1}^2 m_{B_A} \text{Tr}(Y_e Y_e^\dagger) - 400g_3^2 \text{Tr}(Y_d^\dagger T_d) + 10g_{A1}^2 \text{Tr}(Y_d^\dagger T_d) - 90g_{A1}^2 \text{Tr}(Y_e^\dagger T_e) \\
&\left. + 300\text{Tr}(Y_d Y_d^\dagger T_d Y_d^\dagger) + 75\text{Tr}(Y_d Y_u^\dagger T_u Y_d^\dagger) + 450\text{Tr}(Y_e Y_e^\dagger T_e Y_e^\dagger) + 75\text{Tr}(Y_u Y_d^\dagger T_d Y_u^\dagger) \right) \tag{68}
\end{aligned}$$

$$\beta_{T_K}^{(1)} = +3Y_A^* \left( 2Y_K T_A + Y_A T_K \right)$$

$$+ \frac{3}{10} \left( - \left( -15|Y_K|^2 + 2 \left( 5g_{A2}^2 + 5g_{B2}^2 + g_{A1}^2 + g_{B1}^2 \right) \right) T_K + 4 \left( 5g_{A2}^2 m_{W_A} + 5g_{B2}^2 m_{W_B} + g_{A1}^2 m_{B_A} + g_{B1}^2 m_{B_B} \right) Y_K \right) \quad (69)$$

$$\begin{aligned} \beta_{T_K}^{(2)} = & -\frac{3}{200} \left( 375 Y_K^2 Y_K^{*,2} T_K \right. \\ & + 40|Y_K|^2 \left( 2 \left( 5g_{A2}^2 m_{W_A} + 5g_{B2}^2 m_{W_B} + g_{A1}^2 m_{B_A} + g_{B1}^2 m_{B_B} \right) Y_K - 3 \left( 5g_{A2}^2 + 5g_{B2}^2 + g_{A1}^2 + g_{B1}^2 \right) T_K \right) \\ & + 4 \left( 4 \left( 81g_{A1}^4 m_{B_A} + 3g_{A1}^2 \left( 5g_{A2}^2 (m_{B_A} + m_{W_A}) + 5g_{B2}^2 (m_{B_A} + m_{W_B}) + g_{B1}^2 (m_{B_A} + m_{B_B}) \right) \right) \right. \\ & + 5 \left( 3g_{A2}^2 \left( 5g_{B2}^2 (m_{W_A} + m_{W_B}) + g_{B1}^2 (m_{W_A} + m_{B_B}) \right) \right) \\ & + 3g_{B1}^2 g_{B2}^2 (m_{B_B} + m_{W_B}) + 3g_{B1}^4 m_{B_B} + 45g_{A2}^4 m_{W_A} - 5g_{B2}^4 m_{W_B} \left. \right) Y_K \\ & - \left( 5 \left( 3g_{B1}^4 + 45g_{A2}^4 - 5g_{B2}^4 + 6g_{A2}^2 (5g_{B2}^2 + g_{B1}^2) + 6g_{B1}^2 g_{B2}^2 \right) + 6g_{A1}^2 (5g_{A2}^2 + 5g_{B2}^2 + g_{B1}^2) + 81g_{A1}^4 \right) T_K \left. \right) \\ & + 700 Y_A Y_A^{*,2} \left( 4 Y_K T_A + Y_A T_K \right) \\ & + 100 Y_A^* \left( 2 Y_K \left( 3|Y_K|^2 - 8g_{B2}^2 \right) T_A + Y_A \left( 16g_{B2}^2 m_{W_B} Y_K + \left( -8g_{B2}^2 + 9|Y_K|^2 \right) T_K \right) \right) \end{aligned} \quad (70)$$

$$\begin{aligned} \beta_{T_A}^{(1)} = & -\frac{1}{10} \left( -150|Y_A|^2 + 30g_{A2}^2 - 5|Y_K|^2 + 6g_{A1}^2 + 6g_{B1}^2 + 70g_{B2}^2 \right) T_A \\ & + \frac{1}{5} Y_A \left( 30g_{A2}^2 m_{W_A} + 5Y_K^* T_K + 6g_{A1}^2 m_{B_A} + 6g_{B1}^2 m_{B_B} + 70g_{B2}^2 m_{W_B} \right) \end{aligned} \quad (71)$$

$$\begin{aligned} \beta_{T_A}^{(2)} = & \frac{1}{200} \left( -16500 Y_A^2 Y_A^{*,2} T_A \right. \\ & + \left( 4 \left( 18g_{A1}^2 \left( 5g_{A2}^2 + 5g_{B2}^2 + g_{B1}^2 \right) + 243g_{A1}^4 + 5 \left( 135g_{A2}^4 + 18g_{A2}^2 \left( 5g_{B2}^2 + g_{B1}^2 \right) + 18g_{B1}^2 g_{B2}^2 + 65g_{B2}^4 + 9g_{B1}^4 \right) \right) \right. \\ & - 125 Y_K^2 Y_K^{*,2} \left. \right) T_A \\ & - 4 Y_A \left( 4 \left( 243g_{A1}^4 m_{B_A} + 9g_{A1}^2 \left( 5g_{A2}^2 (m_{B_A} + m_{W_A}) \right. \right. \right. \\ & + 5g_{B2}^2 (m_{B_A} + m_{W_B}) + g_{B1}^2 (m_{B_A} + m_{B_B}) \left. \left. \left. \right) \right) \right. \\ & + 5 \left( 135g_{A2}^4 m_{W_A} + 65g_{B2}^4 m_{W_B} \right. \\ & + 9g_{A2}^2 \left( 5g_{B2}^2 (m_{W_A} + m_{W_B}) + g_{B1}^2 (m_{W_A} + m_{B_B}) \right) + 9g_{B1}^2 g_{B2}^2 (m_{B_B} + m_{W_B}) + 9g_{B1}^4 m_{B_B} \left. \right) \left. \right) \\ & + 125 Y_K Y_K^{*,2} T_K \left. \right) \\ & - 20|Y_A|^2 \left( -3 \left( -25 Y_K Y_K^* + 4 \left( 15g_{A2}^2 + 25g_{B2}^2 + 3g_{A1}^2 + 3g_{B1}^2 \right) \right) T_A \right. \\ & + 2 Y_A \left( 25 Y_K^* T_K + 4 \left( 15g_{A2}^2 m_{W_A} + 25g_{B2}^2 m_{W_B} + 3g_{A1}^2 m_{B_A} + 3g_{B1}^2 m_{B_B} \right) \right) \left. \right) \end{aligned} \quad (72)$$

### 3.8 Bilinear Soft-Breaking Parameters

$$\beta_{B_\mu}^{(1)} = +B_\mu \left( -3g_{A2}^2 - \frac{3}{5}g_{A1}^2 + \text{Tr}(Y_d Y_d^\dagger) + \text{Tr}(Y_e Y_e^\dagger) + \text{Tr}(Y_u Y_u^\dagger) \right)$$

$$+ \frac{2}{5}\mu \left( 15g_{A2}^2 m_{W_A} + 3g_{A1}^2 m_{B_A} + 5\text{Tr}(Y_d^\dagger T_d) + 5\text{Tr}(Y_e^\dagger T_e) + 5\text{Tr}(Y_u^\dagger T_u) \right) \quad (73)$$

$$\begin{aligned} \beta_{B_\mu}^{(2)} = & + B_\mu \left( \frac{243}{50} g_{A1}^4 + \frac{9}{5} g_{A1}^2 g_{A2}^2 + \frac{27}{2} g_{A2}^4 + \frac{2}{15} (40g_3^2 - g_{A1}^2) \text{Tr}(Y_d Y_d^\dagger) + \frac{6}{5} g_{A1}^2 \text{Tr}(Y_e Y_e^\dagger) + \frac{16}{3} g_3^2 \text{Tr}(Y_u Y_u^\dagger) \right. \\ & + \frac{4}{15} g_{A1}^2 \text{Tr}(Y_u Y_u^\dagger) - 2\text{Tr}(Y_d Y_d^\dagger Y_d Y_d^\dagger) - 2\text{Tr}(Y_d Y_u^\dagger Y_u Y_d^\dagger) - 3\text{Tr}(Y_e Y_e^\dagger Y_e Y_e^\dagger) - 2\text{Tr}(Y_u Y_u^\dagger Y_u Y_u^\dagger) \Big) \\ & - \frac{2}{75} \mu \left( 729 g_{A1}^4 m_{B_A} + 135 g_{A1}^2 g_{A2}^2 m_{B_A} + 135 g_{A1}^2 g_{A2}^2 m_{W_A} + 2025 g_{A2}^4 m_{W_A} - 10 \left( -40g_3^2 M_3 + g_{A1}^2 m_{B_A} \right) \text{Tr}(Y_d Y_d^\dagger) \right. \\ & + 90 g_{A1}^2 m_{B_A} \text{Tr}(Y_e Y_e^\dagger) + 20 g_{A1}^2 m_{B_A} \text{Tr}(Y_u Y_u^\dagger) + 400 g_3^2 M_3 \text{Tr}(Y_u Y_u^\dagger) - 400 g_3^2 \text{Tr}(Y_d^\dagger T_d) \\ & + 10 g_{A1}^2 \text{Tr}(Y_d^\dagger T_d) - 90 g_{A1}^2 \text{Tr}(Y_e^\dagger T_e) - 400 g_3^2 \text{Tr}(Y_u^\dagger T_u) - 20 g_{A1}^2 \text{Tr}(Y_u^\dagger T_u) \\ & + 300 \text{Tr}(Y_d Y_d^\dagger T_d Y_d^\dagger) + 150 \text{Tr}(Y_d Y_u^\dagger T_u Y_d^\dagger) + 450 \text{Tr}(Y_e Y_e^\dagger T_e Y_e^\dagger) + 150 \text{Tr}(Y_u Y_d^\dagger T_d Y_u^\dagger) \\ & \left. + 300 \text{Tr}(Y_u Y_u^\dagger T_u Y_u^\dagger) \right) \end{aligned} \quad (74)$$

### 3.9 Linear Soft-Breaking Parameters

$$\beta_{L\Omega}^{(1)} = Y_K^* \left( 2\Omega T_K + Y_K L_\Omega \right) \quad (75)$$

$$\begin{aligned} \beta_{L\Omega}^{(2)} = & -\frac{1}{10} Y_K^* \left( Y_K \left( 30|Y_A|^2 + 5|Y_K|^2 - 6 \left( 5g_{A2}^2 + 5g_{B2}^2 + g_{A1}^2 + g_{B1}^2 \right) \right) L_\Omega \right. \\ & + 4\Omega \left( 3 \left( 5g_{A2}^2 m_{W_A} + 5g_{B2}^2 m_{W_B} + g_{A1}^2 m_{B_A} + g_{B1}^2 m_{B_B} \right) Y_K - \left( 3 \left( 5g_{A2}^2 + 5g_{B2}^2 + g_{A1}^2 + g_{B1}^2 \right) - 5|Y_K|^2 \right) T_K \right. \\ & \left. \left. + 15 Y_A^* \left( Y_A T_K + Y_K T_A \right) \right) \right) \end{aligned} \quad (76)$$

### 3.10 Soft-Breaking Scalar Masses

$$\sigma_{1,1} = 2\sqrt{\frac{3}{5}} g_{B1} \left( -m_L^2 + m_L^2 \right) \quad (77)$$

$$\begin{aligned} \sigma_{1,3} = & \frac{1}{\sqrt{15}} g_{A1} \left( 3 \left( -2\text{Tr}(m_u^2) - 2m_L^2 + 2m_L^2 - m_{H_d}^2 + m_{H_u}^2 \right. \right. \\ & \left. \left. + \text{Tr}(m_d^2) + \text{Tr}(m_e^2) \right) - 3\text{conj}(\text{trace}(\text{ml}2)) + \text{conj}(\text{trace}(\text{mq}2)) \right) \end{aligned} \quad (78)$$

$$\sigma_{1,5} = \frac{1}{\sqrt{3}} \text{conj}(\text{trace}(\text{mq}2)) \quad (79)$$

$$\text{Tr}2\text{U}1(1,1) = \frac{3}{5} g_{B1}^2 (m_L^2 + m_L^2) \quad (80)$$

$$\text{Tr}2\text{U}1(1,3) = -\frac{3}{5} g_{A1} g_{B1} (m_L^2 + m_L^2) \quad (81)$$

$$\sigma_{3,1} = \frac{1}{20} \sqrt{\frac{3}{5}} g_{B1} \left( -m_L^2 + m_L^2 \right) \left( -30|Y_A|^2 - 5|Y_K|^2 + 6 \left( 5g_{A2}^2 + 5g_{B2}^2 + g_{A1}^2 + g_{B1}^2 \right) \right) \quad (82)$$

$$\sigma_{2,2} = 3m_{Ad}^2 + m_L^2 + m_{\bar{L}}^2 \quad (83)$$

$$\text{Tr}2\text{U}1(3,1) = -\frac{3}{5}g_{A1}g_{B1}(m_L^2 + m_{\bar{L}}^2) \quad (84)$$

$$\begin{aligned} \text{Tr}2\text{U}1(3,3) = & \frac{1}{30}g_{A1}^2 \left( 3 \left( 2\text{Tr}(m_d^2) + 3m_{H_d}^2 + 3m_{H_u}^2 + 6\text{Tr}(m_e^2) + 6m_L^2 + 6m_{\bar{L}}^2 + 8\text{Tr}(m_u^2) \right) \right. \\ & \left. + 9\text{conj}(\text{trace}(\text{ml}2)) + \text{conj}(\text{trace}(\text{mq}2)) \right) \end{aligned} \quad (85)$$

$$\begin{aligned} \sigma_{3,3} = & \frac{1}{60} \frac{1}{\sqrt{15}} g_{A1} \left( -27g_{A1}^2 m_{H_d}^2 - 135g_{A2}^2 m_{H_d}^2 + 27g_{A1}^2 m_{H_u}^2 + 135g_{A2}^2 m_{H_u}^2 - 54g_{A1}^2 m_L^2 - 270g_{A2}^2 m_L^2 - 54g_{B1}^2 m_L^2 \right. \\ & - 270g_{B2}^2 m_L^2 + 54g_{A1}^2 m_{\bar{L}}^2 + 270g_{A2}^2 m_{\bar{L}}^2 + 54g_{B1}^2 m_{\bar{L}}^2 + 270g_{B2}^2 m_{\bar{L}}^2 + 270 \left( -m_{\bar{L}}^2 + m_L^2 \right) |Y_A|^2 \\ & + 45 \left( -m_{\bar{L}}^2 + m_L^2 \right) |Y_K|^2 - 27g_{A1}^2 \text{conj}(\text{trace}(\text{ml}2)) - 135g_{A2}^2 \text{conj}(\text{trace}(\text{ml}2)) + 80g_3^2 \text{conj}(\text{trace}(\text{mq}2)) \\ & + g_{A1}^2 \text{conj}(\text{trace}(\text{mq}2)) \\ & + 45g_{A2}^2 \text{conj}(\text{trace}(\text{mq}2)) + 240g_3^2 \text{Tr}(m_d^2) + 12g_{A1}^2 \text{Tr}(m_d^2) + 108g_{A1}^2 \text{Tr}(m_e^2) - 480g_3^2 \text{Tr}(m_u^2) - 96g_{A1}^2 \text{Tr}(m_u^2) \\ & + 90m_{H_d}^2 \text{Tr}(Y_d Y_d^\dagger) + 90m_{H_d}^2 \text{Tr}(Y_e Y_e^\dagger) - 90m_{H_u}^2 \text{Tr}(Y_u Y_u^\dagger) - 60\text{Tr}(Y_d Y_d^\dagger m_d^{2*}) \\ & - 30\text{Tr}(Y_d m_q^{2*} Y_d^\dagger) - 180\text{Tr}(Y_e Y_e^\dagger m_e^{2*}) + 90\text{Tr}(Y_e m_l^{2*} Y_e^\dagger) + 120\text{Tr}(Y_u Y_u^\dagger m_u^{2*}) \\ & \left. - 30\text{Tr}(Y_u m_q^{2*} Y_u^\dagger) \right) \end{aligned} \quad (86)$$

$$\sigma_{2,4} = \frac{1}{2} \left( 2m_L^2 + 2m_{\bar{L}}^2 + m_{H_d}^2 + m_{H_u}^2 + \text{conj}(\text{trace}(\text{ml}2)) + \text{conj}(\text{trace}(\text{mq}2)) \right) \quad (87)$$

$$\sigma_{2,5} = \frac{1}{6} \left( 2\text{conj}(\text{trace}(\text{mq}2)) + 3 \left( \text{Tr}(m_d^2) + \text{Tr}(m_u^2) \right) \right) \quad (88)$$

$$\begin{aligned} \sigma_{3,5} = & \frac{1}{60} \frac{1}{\sqrt{3}} \left( \left( 45g_{A2}^2 + 80g_3^2 + g_{A1}^2 \right) \text{conj}(\text{trace}(\text{mq}2)) \right. \\ & \left. - 30 \left( \text{Tr}(Y_d Y_d^\dagger m_d^{2*}) + \text{Tr}(Y_d m_q^{2*} Y_d^\dagger) + \text{Tr}(Y_u Y_u^\dagger m_u^{2*}) + \text{Tr}(Y_u m_q^{2*} Y_u^\dagger) \right) \right) \end{aligned} \quad (89)$$

$$\begin{aligned} \beta_{m_q^2}^{(1)} = & -\frac{2}{15}g_{A1}^2 \mathbf{1} |m_{B_A}|^2 - 6g_{A2}^2 \mathbf{1} |m_{W_A}|^2 - \frac{32}{3}g_3^2 \mathbf{1} |M_3|^2 + 2m_{H_d}^2 Y_d^\dagger Y_d + 2m_{H_u}^2 Y_u^\dagger Y_u + 2T_d^\dagger T_d \\ & + 2T_u^\dagger T_u + m_q^2 Y_d^\dagger Y_d + m_q^2 Y_u^\dagger Y_u + 2Y_d^\dagger m_d^2 Y_d + Y_d^\dagger Y_d m_q^2 + 2Y_u^\dagger m_u^2 Y_u \\ & + Y_u^\dagger Y_u m_q^2 + \frac{1}{\sqrt{15}} g_{A1} \mathbf{1} \sigma_{1,3} + \mathbf{1} \sigma_{1,5} + \frac{1}{\sqrt{3}} \mathbf{1} \sigma_{1,5} \end{aligned} \quad (90)$$

$$\begin{aligned} \beta_{m_q^2}^{(2)} = & -\frac{128}{3}g_3^4 \mathbf{1} |M_3|^2 + \frac{32}{45}g_3^2 g_{A1}^2 \mathbf{1} |M_3|^2 + 32g_3^2 g_{A2}^2 \mathbf{1} |M_3|^2 \\ & + \frac{1}{5}g_{A2}^2 \left( 5 \left( 16g_3^2 (2m_{W_A} + M_3) + 69g_{A2}^2 m_{W_A} \right) + g_{A1}^2 (2m_{W_A} + m_{B_A}) \right) \mathbf{1} m_{W,A^*} + \frac{16}{45}g_3^2 g_{A1}^2 m_{B_A} \mathbf{1} M_3^* \\ & + 16g_3^2 g_{A2}^2 m_{W_A} \mathbf{1} M_3^* + \frac{4}{5}g_{A1}^2 m_{H_d}^2 Y_d^\dagger Y_d + \frac{8}{5}g_{A1}^2 m_{H_u}^2 Y_u^\dagger Y_u \\ & + \frac{1}{45}g_{A1}^2 m_{B,A^*} \left( \left( 16g_3^2 (2m_{B_A} + M_3) + 3 \left( 3g_{A2}^2 (2m_{B_A} + m_{W_A}) + 47g_{A1}^2 m_{B_A} \right) \right) \mathbf{1} \right. \\ & \left. + 36 \left( 2m_{B_A} Y_d^\dagger Y_d - 2Y_u^\dagger T_u + 4m_{B_A} Y_u^\dagger Y_u - Y_d^\dagger T_d \right) \right) \end{aligned}$$

$$\begin{aligned}
& -\frac{4}{5}g_{A1}^2 m_{BA} T_d^\dagger Y_d + \frac{4}{5}g_{A1}^2 T_d^\dagger T_d - \frac{8}{5}g_{A1}^2 m_{BA} T_u^\dagger Y_u + \frac{8}{5}g_{A1}^2 T_u^\dagger T_u \\
& + \frac{2}{5}g_{A1}^2 m_q^2 Y_d^\dagger Y_d + \frac{4}{5}g_{A1}^2 m_q^2 Y_u^\dagger Y_u + \frac{4}{5}g_{A1}^2 Y_d^\dagger m_d^2 Y_d + \frac{2}{5}g_{A1}^2 Y_d^\dagger Y_d m_q^2 \\
& + \frac{8}{5}g_{A1}^2 Y_u^\dagger m_u^2 Y_u + \frac{4}{5}g_{A1}^2 Y_u^\dagger Y_u m_q^2 - 4m_{H_d}^2 Y_d^\dagger Y_d Y_d^\dagger Y_d - 2Y_d^\dagger Y_d T_d^\dagger T_d \\
& - 2Y_d^\dagger T_d T_d^\dagger Y_d - 4m_{H_u}^2 Y_u^\dagger Y_u Y_u^\dagger Y_u - 2Y_u^\dagger Y_u T_u^\dagger T_u - 2Y_u^\dagger T_u T_u^\dagger Y_u \\
& - 2T_d^\dagger Y_d Y_d^\dagger T_d - 2T_d^\dagger T_d Y_d^\dagger Y_d - 2T_u^\dagger Y_u Y_u^\dagger T_u - 2T_u^\dagger T_u Y_u^\dagger Y_u \\
& - m_q^2 Y_d^\dagger Y_d Y_d^\dagger Y_d - m_q^2 Y_u^\dagger Y_u Y_u^\dagger Y_u - 2Y_d^\dagger m_d^2 Y_d Y_d^\dagger Y_d - 2Y_d^\dagger Y_d m_q^2 Y_d^\dagger Y_d \\
& - 2Y_d^\dagger Y_d Y_d^\dagger m_d^2 Y_d - Y_d^\dagger Y_d Y_d^\dagger Y_d m_q^2 - 2Y_u^\dagger m_u^2 Y_u Y_u^\dagger Y_u - 2Y_u^\dagger Y_u m_q^2 Y_u^\dagger Y_u \\
& - 2Y_u^\dagger Y_u Y_u^\dagger m_u^2 Y_u - Y_u^\dagger Y_u Y_u^\dagger Y_u m_q^2 + 6g_{A2}^4 \mathbf{1}\sigma_{2,4} + \frac{32}{3}g_3^4 \mathbf{1}\sigma_{2,5} + \frac{2}{15}g_{A1}^2 \mathbf{1}\text{Tr}2\text{U}1(3,3) + 4\frac{1}{\sqrt{15}}g_{A1} \mathbf{1}\sigma_{3,3} + 4\mathbf{1}\sigma_{3,5} \\
& + 4\frac{1}{\sqrt{3}}\mathbf{1}\sigma_{3,5} - 4m_{H_d}^2 Y_d^\dagger Y_d \text{Tr}(Y_d Y_d^\dagger) - 2T_d^\dagger T_d \text{Tr}(Y_d Y_d^\dagger) - m_q^2 Y_d^\dagger Y_d \text{Tr}(Y_d Y_d^\dagger) \\
& - 2Y_d^\dagger m_d^2 Y_d \text{Tr}(Y_d Y_d^\dagger) - Y_d^\dagger Y_d m_q^2 \text{Tr}(Y_d Y_d^\dagger) - 4m_{H_d}^2 Y_d^\dagger Y_d \text{Tr}(Y_e Y_e^\dagger) \\
& - 2T_d^\dagger T_d \text{Tr}(Y_e Y_e^\dagger) - m_q^2 Y_d^\dagger Y_d \text{Tr}(Y_e Y_e^\dagger) - 2Y_d^\dagger m_d^2 Y_d \text{Tr}(Y_e Y_e^\dagger) \\
& - Y_d^\dagger Y_d m_q^2 \text{Tr}(Y_e Y_e^\dagger) - 4m_{H_u}^2 Y_u^\dagger Y_u \text{Tr}(Y_u Y_u^\dagger) - 2T_u^\dagger T_u \text{Tr}(Y_u Y_u^\dagger) \\
& - m_q^2 Y_u^\dagger Y_u \text{Tr}(Y_u Y_u^\dagger) - 2Y_u^\dagger m_u^2 Y_u \text{Tr}(Y_u Y_u^\dagger) - Y_u^\dagger Y_u m_q^2 \text{Tr}(Y_u Y_u^\dagger) \\
& - 2T_d^\dagger Y_d \text{Tr}(Y_d^\dagger T_d) - 2T_d^\dagger Y_d \text{Tr}(Y_e^\dagger T_e) - 2T_u^\dagger Y_u \text{Tr}(Y_u^\dagger T_u) \\
& - 2Y_d^\dagger T_d \text{Tr}(T_d^* Y_d^T) - 2Y_d^\dagger Y_d \text{Tr}(T_d^* T_d^T) - 2Y_d^\dagger T_d \text{Tr}(T_e^* Y_e^T) \\
& - 2Y_d^\dagger Y_d \text{Tr}(T_e^* T_e^T) - 2Y_u^\dagger T_u \text{Tr}(T_u^* Y_u^T) - 2Y_u^\dagger Y_u \text{Tr}(T_u^* T_u^T) \\
& - 2Y_d^\dagger Y_d \text{Tr}(m_d^2 Y_d Y_d^\dagger) - 2Y_d^\dagger Y_d \text{Tr}(m_e^2 Y_e Y_e^\dagger) - 2Y_d^\dagger Y_d \text{Tr}(m_l^2 Y_e^\dagger Y_e) \\
& - 2Y_d^\dagger Y_d \text{Tr}(m_q^2 Y_d^\dagger Y_d) - 2Y_u^\dagger Y_u \text{Tr}(m_q^2 Y_u^\dagger Y_u) - 2Y_u^\dagger Y_u \text{Tr}(m_u^2 Y_u Y_u^\dagger)
\end{aligned} \tag{91}$$

$$\begin{aligned}
\beta_{m_l^2}^{(1)} &= -\frac{6}{5}g_{A1}^2 \mathbf{1}|m_{BA}|^2 - 6g_{A2}^2 \mathbf{1}|m_{WA}|^2 + 2m_{H_d}^2 Y_e^\dagger Y_e + 2T_e^\dagger T_e + m_l^2 Y_e^\dagger Y_e + 2Y_e^\dagger m_e^2 Y_e \\
&+ Y_e^\dagger Y_e m_l^2 - \sqrt{\frac{3}{5}}g_{A1} \mathbf{1}\sigma_{1,3}
\end{aligned} \tag{92}$$

$$\begin{aligned}
\beta_{m_l^2}^{(2)} &= +\frac{3}{5}g_{A2}^2 \left( 115g_{A2}^2 m_{WA} + 3g_{A1}^2 (2m_{WA} + m_{BA}) \right) \mathbf{1}m_{W,A^*} + \frac{12}{5}g_{A1}^2 m_{H_d}^2 Y_e^\dagger Y_e \\
&+ \frac{3}{25}g_{A1}^2 m_{B,A^*} \left( -20Y_e^\dagger T_e + 3 \left( 5g_{A2}^2 (2m_{BA} + m_{WA}) + 81g_{A1}^2 m_{BA} \right) \mathbf{1} + 40m_{BA} Y_e^\dagger Y_e \right) - \frac{12}{5}g_{A1}^2 m_{BA} T_e^\dagger Y_e \\
&+ \frac{12}{5}g_{A1}^2 T_e^\dagger T_e + \frac{6}{5}g_{A1}^2 m_l^2 Y_e^\dagger Y_e + \frac{12}{5}g_{A1}^2 Y_e^\dagger m_e^2 Y_e + \frac{6}{5}g_{A1}^2 Y_e^\dagger Y_e m_l^2 \\
&- 8m_{H_d}^2 Y_e^\dagger Y_e Y_e^\dagger Y_e - 4Y_e^\dagger Y_e T_e^\dagger T_e - 4Y_e^\dagger T_e T_e^\dagger Y_e - 4T_e^\dagger Y_e Y_e^\dagger T_e \\
&- 4T_e^\dagger T_e Y_e^\dagger Y_e - 2m_l^2 Y_e^\dagger Y_e Y_e^\dagger Y_e - 4Y_e^\dagger m_e^2 Y_e Y_e^\dagger Y_e - 4Y_e^\dagger Y_e m_l^2 Y_e^\dagger Y_e
\end{aligned}$$

$$\begin{aligned}
& -4Y_e^\dagger Y_e Y_e^\dagger m_e^2 Y_e - 2Y_e^\dagger Y_e Y_e^\dagger Y_e m_l^2 + 6g_{A2}^4 \mathbf{1}\sigma_{2,4} + \frac{6}{5}g_{A1}^2 \mathbf{1}\text{Tr}2\text{U1}(3,3) - 4\sqrt{\frac{3}{5}}g_{A1} \mathbf{1}\sigma_{3,3} \\
& -4m_{H_d}^2 Y_e^\dagger Y_e \text{Tr}(Y_d Y_d^\dagger) - 2T_e^\dagger T_e \text{Tr}(Y_d Y_d^\dagger) - m_l^2 Y_e^\dagger Y_e \text{Tr}(Y_d Y_d^\dagger) \\
& -2Y_e^\dagger m_e^2 Y_e \text{Tr}(Y_d Y_d^\dagger) - Y_e^\dagger Y_e m_l^2 \text{Tr}(Y_d Y_d^\dagger) - 4m_{H_d}^2 Y_e^\dagger Y_e \text{Tr}(Y_e Y_e^\dagger) \\
& -2T_e^\dagger T_e \text{Tr}(Y_e Y_e^\dagger) - m_l^2 Y_e^\dagger Y_e \text{Tr}(Y_e Y_e^\dagger) - 2Y_e^\dagger m_e^2 Y_e \text{Tr}(Y_e Y_e^\dagger) \\
& -Y_e^\dagger Y_e m_l^2 \text{Tr}(Y_e Y_e^\dagger) - 2T_e^\dagger Y_e \text{Tr}(Y_d^\dagger T_d) - 2T_e^\dagger Y_e \text{Tr}(Y_e^\dagger T_e) \\
& -2Y_e^\dagger T_e \text{Tr}(T_d^* T_d^T) - 2Y_e^\dagger Y_e \text{Tr}(T_d^* T_d^T) - 2Y_e^\dagger T_e \text{Tr}(T_e^* T_e^T) \\
& -2Y_e^\dagger Y_e \text{Tr}(T_e^* T_e^T) - 2Y_e^\dagger Y_e \text{Tr}(m_d^2 Y_d Y_d^\dagger) - 2Y_e^\dagger Y_e \text{Tr}(m_e^2 Y_e Y_e^\dagger) \\
& -2Y_e^\dagger Y_e \text{Tr}(m_l^2 Y_e^\dagger Y_e) - 2Y_e^\dagger Y_e \text{Tr}(m_q^2 Y_d^\dagger Y_d)
\end{aligned} \tag{93}$$

$$\begin{aligned}
\beta_{m_{H_d}^2}^{(1)} &= -\frac{6}{5}g_{A1}^2 |m_{B_A}|^2 - 6g_{A2}^2 |m_{W_A}|^2 - \sqrt{\frac{3}{5}}g_{A1}\sigma_{1,3} + 2m_{H_d}^2 \text{Tr}(Y_d Y_d^\dagger) + 2m_{H_d}^2 \text{Tr}(Y_e Y_e^\dagger) + 2\text{Tr}(T_d^* T_d^T) \\
&+ 2\text{Tr}(T_e^* T_e^T) + 2\text{Tr}(m_d^2 Y_d Y_d^\dagger) + 2\text{Tr}(m_e^2 Y_e Y_e^\dagger) + 2\text{Tr}(m_l^2 Y_e^\dagger Y_e) + 2\text{Tr}(m_q^2 Y_d^\dagger Y_d)
\end{aligned} \tag{94}$$

$$\begin{aligned}
\beta_{m_{H_d}^2}^{(2)} &= \frac{1}{75} \left( g_{A1}^2 m_{B,A^*} \left( 2187g_{A1}^2 m_{B_A} + 270g_{A2}^2 m_{B_A} + 135g_{A2}^2 m_{W_A} - 40m_{B_A} \text{Tr}(Y_d Y_d^\dagger) + 360m_{B_A} \text{Tr}(Y_e Y_e^\dagger) + 20\text{Tr}(Y_d^\dagger T_d) \right. \right. \\
&\quad \left. \left. - 180\text{Tr}(Y_e^\dagger T_e) \right) \right. \\
&+ 5 \left( 9g_{A2}^2 \left( 115g_{A2}^2 m_{W_A} + 3g_{A1}^2 (2m_{W_A} + m_{B_A}) \right) m_{W,A^*} \right. \\
&+ 2 \left( 45g_{A2}^4 \sigma_{2,4} + 9g_{A1}^2 \text{Tr}2\text{U1}(3,3) - 6\sqrt{15}g_{A1}\sigma_{3,3} + 2 \left( 40g_3^2 m_{H_d}^2 + 80g_3^2 |M_3|^2 - g_{A1}^2 m_{H_d}^2 \right) \text{Tr}(Y_d Y_d^\dagger) \right. \\
&+ 18g_{A1}^2 m_{H_d}^2 \text{Tr}(Y_e Y_e^\dagger) - 80g_3^2 M_3^* \text{Tr}(Y_d^\dagger T_d) + 2g_{A1}^2 m_{B_A} \text{Tr}(T_d^* Y_d^T) - 80g_3^2 M_3 \text{Tr}(T_d^* Y_d^T) \\
&+ 80g_3^2 \text{Tr}(T_d^* T_d^T) - 2g_{A1}^2 \text{Tr}(T_d^* T_d^T) - 18g_{A1}^2 m_{B_A} \text{Tr}(T_e^* Y_e^T) + 18g_{A1}^2 \text{Tr}(T_e^* T_e^T) \\
&+ 80g_3^2 \text{Tr}(m_d^2 Y_d Y_d^\dagger) - 2g_{A1}^2 \text{Tr}(m_d^2 Y_d Y_d^\dagger) + 18g_{A1}^2 \text{Tr}(m_e^2 Y_e Y_e^\dagger) + 18g_{A1}^2 \text{Tr}(m_l^2 Y_e^\dagger Y_e) \\
&+ 80g_3^2 \text{Tr}(m_q^2 Y_d^\dagger Y_d) - 2g_{A1}^2 \text{Tr}(m_q^2 Y_d^\dagger Y_d) - 60m_{H_d}^2 \text{Tr}(Y_d Y_d^\dagger Y_d Y_d^\dagger) - 60\text{Tr}(Y_d Y_d^\dagger T_d T_d^\dagger) \\
&- 15m_{H_d}^2 \text{Tr}(Y_d Y_u^\dagger Y_u Y_d^\dagger) - 15m_{H_u}^2 \text{Tr}(Y_d Y_u^\dagger Y_u Y_d^\dagger) - 15\text{Tr}(Y_d Y_u^\dagger T_u T_d^\dagger) \\
&- 60\text{Tr}(Y_d T_d^\dagger T_d Y_d^\dagger) - 15\text{Tr}(Y_d T_u^\dagger T_u Y_d^\dagger) - 90m_{H_d}^2 \text{Tr}(Y_e Y_e^\dagger Y_e Y_e^\dagger) - 90\text{Tr}(Y_e Y_e^\dagger T_e T_e^\dagger) \\
&- 90\text{Tr}(Y_e T_e^\dagger T_e Y_e^\dagger) - 15\text{Tr}(Y_u Y_d^\dagger T_d T_u^\dagger) - 15\text{Tr}(Y_u T_d^\dagger T_d Y_u^\dagger) - 60\text{Tr}(m_d^2 Y_d Y_d^\dagger Y_d Y_d^\dagger) \\
&- 15\text{Tr}(m_d^2 Y_d Y_u^\dagger Y_u Y_d^\dagger) - 90\text{Tr}(m_e^2 Y_e Y_e^\dagger Y_e Y_e^\dagger) - 90\text{Tr}(m_l^2 Y_e^\dagger Y_e Y_e^\dagger Y_e) - 60\text{Tr}(m_q^2 Y_d^\dagger Y_d Y_d^\dagger Y_d) \\
&\left. \left. - 15\text{Tr}(m_q^2 Y_d^\dagger Y_d Y_u^\dagger Y_u) - 15\text{Tr}(m_q^2 Y_u^\dagger Y_u Y_d^\dagger Y_d) - 15\text{Tr}(m_u^2 Y_u Y_d^\dagger Y_d Y_u^\dagger) \right) \right)
\end{aligned} \tag{95}$$

$$\beta_{m_{H_u}^2}^{(1)} = -\frac{6}{5}g_{A1}^2 |m_{B_A}|^2 - 6g_{A2}^2 |m_{W_A}|^2 + \sqrt{\frac{3}{5}}g_{A1}\sigma_{1,3} + 2m_{H_u}^2 \text{Tr}(Y_u Y_u^\dagger) + 2\text{Tr}(T_u^* T_u^T) + 2\text{Tr}(m_q^2 Y_u^\dagger Y_u)$$



$$+ 2\text{Tr}\left(m_u^2 Y_u Y_u^\dagger\right) \quad (96)$$

$$\begin{aligned} \beta_{m_{H_u}^2}^{(2)} = & \frac{1}{75} \left( g_{A1}^2 m_{B,A^*} \left( 27 \left( 5g_{A2}^2 (2m_{B_A} + m_{W_A}) + 81g_{A1}^2 m_{B_A} \right) - 40\text{Tr}\left(Y_u^\dagger T_u\right) + 80m_{B_A} \text{Tr}\left(Y_u Y_u^\dagger\right) \right) \right. \\ & + 5 \left( 9g_{A2}^2 \left( 115g_{A2}^2 m_{W_A} + 3g_{A1}^2 (2m_{W_A} + m_{B_A}) \right) m_{W,A^*} \right. \\ & + 2 \left( 45g_{A2}^4 \sigma_{2,4} + 9g_{A1}^2 \text{Tr}2U1(3,3) + 6\sqrt{15}g_{A1}\sigma_{3,3} + 4 \left( 20g_3^2 m_{H_u}^2 + 40g_3^2 |M_3|^2 + g_{A1}^2 m_{H_u}^2 \right) \text{Tr}\left(Y_u Y_u^\dagger\right) \right. \\ & - 80g_3^2 M_3^* \text{Tr}\left(Y_u^\dagger T_u\right) - 4g_{A1}^2 m_{B_A} \text{Tr}\left(T_u^* Y_u^T\right) - 80g_3^2 M_3 \text{Tr}\left(T_u^* Y_u^T\right) + 80g_3^2 \text{Tr}\left(T_u^* T_u^T\right) \\ & + 4g_{A1}^2 \text{Tr}\left(T_u^* T_u^T\right) + 80g_3^2 \text{Tr}\left(m_q^2 Y_u^\dagger Y_u\right) + 4g_{A1}^2 \text{Tr}\left(m_q^2 Y_u^\dagger Y_u\right) + 80g_3^2 \text{Tr}\left(m_u^2 Y_u Y_u^\dagger\right) \\ & + 4g_{A1}^2 \text{Tr}\left(m_u^2 Y_u Y_u^\dagger\right) - 15m_{H_d}^2 \text{Tr}\left(Y_d Y_u^\dagger Y_u Y_d^\dagger\right) - 15m_{H_u}^2 \text{Tr}\left(Y_d Y_u^\dagger Y_u Y_d^\dagger\right) \\ & - 15\text{Tr}\left(Y_d Y_u^\dagger T_u T_d^\dagger\right) - 15\text{Tr}\left(Y_d T_u^\dagger T_u Y_d^\dagger\right) - 15\text{Tr}\left(Y_u Y_d^\dagger T_d T_u^\dagger\right) - 60m_{H_u}^2 \text{Tr}\left(Y_u Y_u^\dagger Y_u Y_u^\dagger\right) \\ & - 60\text{Tr}\left(Y_u Y_u^\dagger T_u T_u^\dagger\right) - 15\text{Tr}\left(Y_u T_d^\dagger T_d Y_u^\dagger\right) - 60\text{Tr}\left(Y_u T_u^\dagger T_u Y_u^\dagger\right) \\ & - 15\text{Tr}\left(m_d^2 Y_d Y_u^\dagger Y_u Y_d^\dagger\right) - 15\text{Tr}\left(m_q^2 Y_d^\dagger Y_d Y_u^\dagger Y_u\right) - 15\text{Tr}\left(m_q^2 Y_u^\dagger Y_u Y_d^\dagger Y_d\right) \\ & \left. \left. - 60\text{Tr}\left(m_q^2 Y_u^\dagger Y_u Y_u^\dagger Y_u\right) - 15\text{Tr}\left(m_u^2 Y_u Y_d^\dagger Y_d Y_u^\dagger\right) - 60\text{Tr}\left(m_u^2 Y_u Y_u^\dagger Y_u Y_u^\dagger\right) \right) \right) \quad (97) \end{aligned}$$

$$\begin{aligned} \beta_{m_u^2}^{(1)} = & -\frac{32}{15} g_{A1}^2 \mathbf{1} |m_{B_A}|^2 - \frac{32}{3} g_3^2 \mathbf{1} |M_3|^2 + 2m_{H_u}^2 Y_u Y_u^\dagger + 2T_u T_u^\dagger + m_u^2 Y_u Y_u^\dagger + 2Y_u m_q^2 Y_u^\dagger \\ & + Y_u Y_u^\dagger m_u^2 - 4\frac{1}{\sqrt{15}} g_{A1} \mathbf{1} \sigma_{1,3} + \mathbf{1} \sigma_{1,5} + \frac{1}{\sqrt{3}} \mathbf{1} \sigma_{1,5} \quad (98) \end{aligned}$$

$$\begin{aligned} \beta_{m_u^2}^{(2)} = & -\frac{128}{45} g_3^2 \left( 15g_3^2 M_3 - 2g_{A1}^2 (2M_3 + m_{B_A}) \right) \mathbf{1} M_3^* - \frac{2}{5} g_{A1}^2 m_{H_u}^2 Y_u Y_u^\dagger + 6g_{A2}^2 m_{H_u}^2 Y_u Y_u^\dagger \\ & + 12g_{A2}^2 |m_{W_A}|^2 Y_u Y_u^\dagger + \frac{2}{5} g_{A1}^2 m_{B_A} Y_u T_u^\dagger - 6g_{A2}^2 m_{W_A} Y_u T_u^\dagger - 6g_{A2}^2 m_{W,A^*} T_u Y_u^\dagger \\ & + \frac{2}{45} g_{A1}^2 m_{B,A^*} \left( 16 \left( 75g_{A1}^2 m_{B_A} + 8g_3^2 (2m_{B_A} + M_3) \right) \mathbf{1} + 9 \left( -2m_{B_A} Y_u Y_u^\dagger + T_u Y_u^\dagger \right) \right) - \frac{2}{5} g_{A1}^2 T_u T_u^\dagger \\ & + 6g_{A2}^2 T_u T_u^\dagger - \frac{1}{5} g_{A1}^2 m_u^2 Y_u Y_u^\dagger + 3g_{A2}^2 m_u^2 Y_u Y_u^\dagger - \frac{2}{5} g_{A1}^2 Y_u m_q^2 Y_u^\dagger \\ & + 6g_{A2}^2 Y_u m_q^2 Y_u^\dagger - \frac{1}{5} g_{A1}^2 Y_u Y_u^\dagger m_u^2 + 3g_{A2}^2 Y_u Y_u^\dagger m_u^2 - 2m_{H_d}^2 Y_u Y_d^\dagger Y_d Y_u^\dagger \\ & - 2m_{H_u}^2 Y_u Y_d^\dagger Y_d Y_u^\dagger - 2Y_u Y_d^\dagger T_d T_u^\dagger - 4m_{H_u}^2 Y_u Y_u^\dagger Y_u Y_u^\dagger - 2Y_u Y_u^\dagger T_u T_u^\dagger \\ & - 2Y_u T_d^\dagger T_d Y_u^\dagger - 2Y_u T_u^\dagger T_u Y_u^\dagger - 2T_u Y_d^\dagger Y_d T_u^\dagger - 2T_u Y_u^\dagger Y_u T_u^\dagger \\ & - 2T_u T_d^\dagger Y_d Y_u^\dagger - 2T_u T_u^\dagger Y_u Y_u^\dagger - m_u^2 Y_u Y_d^\dagger Y_d Y_u^\dagger - m_u^2 Y_u Y_u^\dagger Y_u Y_u^\dagger \\ & - 2Y_u m_q^2 Y_d^\dagger Y_d Y_u^\dagger - 2Y_u m_q^2 Y_u^\dagger Y_u Y_u^\dagger - 2Y_u Y_d^\dagger m_d^2 Y_d Y_u^\dagger \\ & - 2Y_u Y_d^\dagger Y_d m_q^2 Y_u^\dagger - Y_u Y_d^\dagger Y_d Y_u^\dagger m_u^2 - 2Y_u Y_u^\dagger m_u^2 Y_u Y_u^\dagger - 2Y_u Y_u^\dagger Y_u m_q^2 Y_u^\dagger \\ & - Y_u Y_u^\dagger Y_u Y_u^\dagger m_u^2 + \frac{32}{3} g_3^4 \mathbf{1} \sigma_{2,5} + \frac{32}{15} g_{A1}^2 \mathbf{1} \text{Tr}2U1(3,3) - 16\frac{1}{\sqrt{15}} g_{A1} \mathbf{1} \sigma_{3,3} + 4\mathbf{1} \sigma_{3,5} + 4\frac{1}{\sqrt{3}} \mathbf{1} \sigma_{3,5} \\ & - 4m_{H_u}^2 Y_u Y_u^\dagger \text{Tr}\left(Y_u Y_u^\dagger\right) - 2T_u T_u^\dagger \text{Tr}\left(Y_u Y_u^\dagger\right) - m_u^2 Y_u Y_u^\dagger \text{Tr}\left(Y_u Y_u^\dagger\right) \end{aligned}$$

$$\begin{aligned}
& -2Y_u m_q^2 Y_u^\dagger \text{Tr}(Y_u Y_u^\dagger) - Y_u Y_u^\dagger m_u^2 \text{Tr}(Y_u Y_u^\dagger) - 2Y_u T_u^\dagger \text{Tr}(Y_u^\dagger T_u) \\
& -2T_u Y_u^\dagger \text{Tr}(T_u^* Y_u^T) - 2Y_u Y_u^\dagger \text{Tr}(T_u^* T_u^T) - 2Y_u Y_u^\dagger \text{Tr}(m_q^2 Y_u^\dagger Y_u) \\
& -2Y_u Y_u^\dagger \text{Tr}(m_u^2 Y_u Y_u^\dagger)
\end{aligned} \tag{99}$$

$$\begin{aligned}
\beta_{m_d^2}^{(1)} = & -\frac{8}{15} g_{A1}^2 \mathbf{1} |m_{B_A}|^2 - \frac{32}{3} g_3^2 \mathbf{1} |M_3|^2 + 2m_{H_d}^2 Y_d Y_d^\dagger + 2T_d T_d^\dagger + m_d^2 Y_d Y_d^\dagger + 2Y_d m_q^2 Y_d^\dagger \\
& + Y_d Y_d^\dagger m_d^2 + 2\frac{1}{\sqrt{15}} g_{A1} \mathbf{1} \sigma_{1,3} + \mathbf{1} \sigma_{1,5} + \frac{1}{\sqrt{3}} \mathbf{1} \sigma_{1,5}
\end{aligned} \tag{100}$$

$$\begin{aligned}
\beta_{m_d^2}^{(2)} = & -\frac{64}{45} g_3^2 \left( 30g_3^2 M_3 - g_{A1}^2 (2M_3 + m_{B_A}) \right) \mathbf{1} M_3^* + \frac{2}{5} g_{A1}^2 m_{H_d}^2 Y_d Y_d^\dagger + 6g_{A2}^2 m_{H_d}^2 Y_d Y_d^\dagger \\
& + 12g_{A2}^2 |m_{W_A}|^2 Y_d Y_d^\dagger - \frac{2}{5} g_{A1}^2 m_{B_A} Y_d T_d^\dagger - 6g_{A2}^2 m_{W_A} Y_d T_d^\dagger \\
& + \frac{2}{225} g_{A1}^2 m_{B,A^*} \left( 4 \left( 357g_{A1}^2 m_{B_A} + 40g_3^2 (2m_{B_A} + M_3) \right) \right) \mathbf{1} - 45T_d Y_d^\dagger + 90m_{B_A} Y_d Y_d^\dagger \\
& - 6g_{A2}^2 m_{W,A^*} T_d Y_d^\dagger + \frac{2}{5} g_{A1}^2 T_d T_d^\dagger + 6g_{A2}^2 T_d T_d^\dagger + \frac{1}{5} g_{A1}^2 m_d^2 Y_d Y_d^\dagger \\
& + 3g_{A2}^2 m_d^2 Y_d Y_d^\dagger + \frac{2}{5} g_{A1}^2 Y_d m_q^2 Y_d^\dagger + 6g_{A2}^2 Y_d m_q^2 Y_d^\dagger + \frac{1}{5} g_{A1}^2 Y_d Y_d^\dagger m_d^2 \\
& + 3g_{A2}^2 Y_d Y_d^\dagger m_d^2 - 4m_{H_d}^2 Y_d Y_d^\dagger Y_d Y_d^\dagger - 2Y_d Y_d^\dagger T_d T_d^\dagger - 2m_{H_d}^2 Y_d Y_u^\dagger Y_u Y_d^\dagger \\
& - 2m_{H_u}^2 Y_d Y_u^\dagger Y_u Y_d^\dagger - 2Y_d Y_u^\dagger T_u T_d^\dagger - 2Y_d T_d^\dagger T_d Y_d^\dagger - 2Y_d T_u^\dagger T_u Y_d^\dagger \\
& - 2T_d Y_d^\dagger Y_d T_d^\dagger - 2T_d Y_u^\dagger Y_u T_d^\dagger - 2T_d T_d^\dagger Y_d Y_d^\dagger - 2T_d T_u^\dagger Y_u Y_d^\dagger \\
& - m_d^2 Y_d Y_d^\dagger Y_d Y_d^\dagger - m_d^2 Y_d Y_u^\dagger Y_u Y_d^\dagger - 2Y_d m_q^2 Y_d^\dagger Y_d Y_d^\dagger - 2Y_d m_q^2 Y_u^\dagger Y_u Y_d^\dagger \\
& - 2Y_d Y_d^\dagger m_d^2 Y_d Y_d^\dagger - 2Y_d Y_d^\dagger Y_d m_q^2 Y_d^\dagger - Y_d Y_d^\dagger Y_d Y_d^\dagger m_d^2 - 2Y_d Y_u^\dagger m_u^2 Y_u Y_d^\dagger \\
& - 2Y_d Y_u^\dagger Y_u m_q^2 Y_d^\dagger - Y_d Y_u^\dagger Y_u Y_d^\dagger m_d^2 + \frac{32}{3} g_3^4 \mathbf{1} \sigma_{2,5} + \frac{8}{15} g_{A1}^2 \mathbf{1} \text{Tr} 2U1(3,3) + 8\frac{1}{\sqrt{15}} g_{A1} \mathbf{1} \sigma_{3,3} \\
& + 41\sigma_{3,5} + 4\frac{1}{\sqrt{3}} \mathbf{1} \sigma_{3,5} - 4m_{H_d}^2 Y_d Y_d^\dagger \text{Tr}(Y_d Y_d^\dagger) - 2T_d T_d^\dagger \text{Tr}(Y_d Y_d^\dagger) \\
& - m_d^2 Y_d Y_d^\dagger \text{Tr}(Y_d Y_d^\dagger) - 2Y_d m_q^2 Y_d^\dagger \text{Tr}(Y_d Y_d^\dagger) - Y_d Y_d^\dagger m_d^2 \text{Tr}(Y_d Y_d^\dagger) \\
& - 4m_{H_d}^2 Y_d Y_d^\dagger \text{Tr}(Y_e Y_e^\dagger) - 2T_d T_d^\dagger \text{Tr}(Y_e Y_e^\dagger) - m_d^2 Y_d Y_d^\dagger \text{Tr}(Y_e Y_e^\dagger) \\
& - 2Y_d m_q^2 Y_d^\dagger \text{Tr}(Y_e Y_e^\dagger) - Y_d Y_d^\dagger m_d^2 \text{Tr}(Y_e Y_e^\dagger) - 2Y_d T_d^\dagger \text{Tr}(Y_d^\dagger T_d) \\
& - 2Y_d T_d^\dagger \text{Tr}(Y_e^\dagger T_e) - 2T_d Y_d^\dagger \text{Tr}(T_d^* Y_d^T) - 2Y_d Y_d^\dagger \text{Tr}(T_d^* T_d^T) \\
& - 2T_d Y_d^\dagger \text{Tr}(T_e^* Y_e^T) - 2Y_d Y_d^\dagger \text{Tr}(T_e^* T_e^T) - 2Y_d Y_d^\dagger \text{Tr}(m_d^2 Y_d Y_d^\dagger) \\
& - 2Y_d Y_d^\dagger \text{Tr}(m_e^2 Y_e Y_e^\dagger) - 2Y_d Y_d^\dagger \text{Tr}(m_l^2 Y_e^\dagger Y_e) - 2Y_d Y_d^\dagger \text{Tr}(m_q^2 Y_d^\dagger Y_d)
\end{aligned} \tag{101}$$

$$\beta_{m_e^2}^{(1)} = -\frac{24}{5} g_{A1}^2 \mathbf{1} |m_{B_A}|^2 + 2 \left( 2m_{H_d}^2 Y_e Y_e^\dagger + 2T_e T_e^\dagger + 2Y_e m_l^2 Y_e^\dagger + m_e^2 Y_e Y_e^\dagger + Y_e Y_e^\dagger m_e^2 \right)$$

$$+ 2\sqrt{\frac{3}{5}}g_{A1}\mathbf{1}\sigma_{1,3} \quad (102)$$

$$\begin{aligned} \beta_{m_e}^{(2)} = & + \frac{12}{5}g_{A1}^2m_{B,A^*} \left( -2m_{B_A}Y_eY_e^\dagger + 54g_{A1}^2m_{B_A}\mathbf{1} + T_eY_e^\dagger \right) + \frac{8}{5}g_{A1}\mathbf{1} \left( 3g_{A1}\text{Tr}2\text{U1}(3,3) + \sqrt{15}\sigma_{3,3} \right) \\ & - \frac{2}{5} \left( 30g_{A2}^2m_{W,A^*}T_eY_e^\dagger + 6g_{A1}^2T_eT_e^\dagger - 30g_{A2}^2T_eT_e^\dagger + 3g_{A1}^2m_e^2Y_eY_e^\dagger \right. \\ & - 15g_{A2}^2m_e^2Y_eY_e^\dagger + 6g_{A1}^2Y_eY_e^\dagger Y_eY_e^\dagger - 30g_{A2}^2Y_eY_e^\dagger Y_eY_e^\dagger + 3g_{A1}^2Y_eY_e^\dagger m_e^2 \\ & - 15g_{A2}^2Y_eY_e^\dagger m_e^2 + 20m_{H_d}^2Y_eY_e^\dagger Y_eY_e^\dagger + 10Y_eY_e^\dagger T_eT_e^\dagger + 10Y_eT_e^\dagger T_eY_e^\dagger \\ & + 10T_eY_e^\dagger Y_eT_e^\dagger + 10T_eT_e^\dagger Y_eY_e^\dagger + 5m_e^2Y_eY_e^\dagger Y_eY_e^\dagger + 10Y_eY_e^\dagger Y_eY_e^\dagger \\ & + 10Y_eY_e^\dagger m_e^2Y_eY_e^\dagger + 10Y_eY_e^\dagger Y_eY_e^\dagger m_e^2 + 5Y_eY_e^\dagger Y_eY_e^\dagger m_e^2 + 10T_eT_e^\dagger \text{Tr}(Y_dY_d^\dagger) \\ & + 5m_e^2Y_eY_e^\dagger \text{Tr}(Y_dY_d^\dagger) + 10Y_eY_e^\dagger Y_eY_e^\dagger \text{Tr}(Y_dY_d^\dagger) + 5Y_eY_e^\dagger m_e^2 \text{Tr}(Y_dY_d^\dagger) \\ & + 10T_eT_e^\dagger \text{Tr}(Y_eY_e^\dagger) + 5m_e^2Y_eY_e^\dagger \text{Tr}(Y_eY_e^\dagger) + 10Y_eY_e^\dagger Y_eY_e^\dagger \text{Tr}(Y_eY_e^\dagger) \\ & + 5Y_eY_e^\dagger m_e^2 \text{Tr}(Y_eY_e^\dagger) + Y_eT_e^\dagger (10\text{Tr}(Y_d^\dagger T_d) + 10\text{Tr}(Y_e^\dagger T_e) + 30g_{A2}^2m_{W_A} - 6g_{A1}^2m_{B_A}) \\ & + 10T_eY_e^\dagger \text{Tr}(T_d^*Y_d^T) + 10T_eY_e^\dagger \text{Tr}(T_e^*Y_e^T) \\ & + 2Y_eY_e^\dagger (3g_{A1}^2m_{H_d}^2 - 15g_{A2}^2m_{H_d}^2 - 30g_{A2}^2|m_{W_A}|^2 + 10m_{H_d}^2\text{Tr}(Y_dY_d^\dagger) + 10m_{H_d}^2\text{Tr}(Y_eY_e^\dagger) + 5\text{Tr}(T_d^*T_d^T) \\ & + 5\text{Tr}(T_e^*T_e^T) + 5\text{Tr}(m_d^2Y_dY_d^\dagger) + 5\text{Tr}(m_e^2Y_eY_e^\dagger) + 5\text{Tr}(m_l^2Y_e^\dagger Y_e) + 5\text{Tr}(m_q^2Y_d^\dagger Y_d) \Big) \end{aligned} \quad (103)$$

$$\begin{aligned} \beta_{m_L}^{(1)} = & \frac{1}{10} \left( -12g_{A1}^2|m_{B_A}|^2 - 60g_{A2}^2|m_{W_A}|^2 - 12g_{B1}^2|m_{B_B}|^2 - 60g_{B2}^2|m_{W_B}|^2 + 30m_{Ad}^2|Y_A|^2 + 30m_L^2|Y_A|^2 \right. \\ & + 30m_L^2|Y_A|^2 + 5m_K^2|Y_K|^2 + 5m_L^2|Y_K|^2 + 5m_L^2|Y_K|^2 + 30|T_A|^2 + 5|T_K|^2 + 2\sqrt{15}g_{B1}\sigma_{1,1} \\ & \left. - 2\sqrt{15}g_{A1}\sigma_{1,3} \right) \end{aligned} \quad (104)$$

$$\begin{aligned} \beta_{m_L}^{(2)} = & + \frac{9}{25}g_{A1}^2 \left( 5(g_{A2}^2(2m_{B_A} + m_{W_A}) + g_{B1}^2(2m_{B_A} + m_{B_B}) + g_{B2}^2(2m_{B_A} + m_{W_B})) + 81g_{A1}^2m_{B_A} \right) m_{B,A^*} \\ & + \frac{1}{20} \left( 72g_{A1}^2g_{B2}^2|m_{W_B}|^2 + 360g_{A2}^2g_{B2}^2|m_{W_B}|^2 + 72g_{B1}^2g_{B2}^2|m_{W_B}|^2 - 420g_{B2}^4|m_{W_B}|^2 \right. \\ & + 240g_{B2}^2m_{Ad}^2|Y_A|^2 + 240g_{B2}^2m_L^2|Y_A|^2 + 240g_{B2}^2m_L^2|Y_A|^2 + 240g_{B2}^2|T_A|^2 \\ & + 12g_{A2}^2(115g_{A2}^2m_{W_A} + 15g_{B2}^2m_{W_B} + 30g_{B2}^2m_{W_A} + 3g_{A1}^2(2m_{W_A} + m_{B_A}) + 3g_{B1}^2m_{B_B} + 6g_{B1}^2m_{W_A})m_{W,A^*} \\ & + 36g_{B1}^2(2g_{B2}^2m_{B_B} + 3g_{B1}^2m_{B_B} + g_{A1}^2(2m_{B_B} + m_{B_A}) + g_{A2}^2(2m_{B_B} + m_{W_A}) \\ & + g_{B2}^2m_{W_B})m_{B,B^*} + 36g_{A1}^2g_{B2}^2m_{B_A}m_{W,B^*} \\ & + 180g_{A2}^2g_{B2}^2m_{W_A}m_{W,B^*} \\ & + 36g_{B1}^2g_{B2}^2m_{B_B}m_{W,B^*} + 480g_{B2}^2Y_A|m_{W_B}|^2Y_A^* - 420m_{Ad}^2Y_A^2Y_A^{*,2} \\ & - 420m_L^2Y_A^2Y_A^{*,2} - 420m_L^2Y_A^2Y_A^{*,2} - 30m_{Ad}^2Y_K|Y_A|^2Y_K^* - 30m_K^2Y_K|Y_A|^2Y_K^* \\ & - 60m_L^2Y_K|Y_A|^2Y_K^* - 60m_L^2Y_K|Y_A|^2Y_K^* - 25m_K^2Y_K^2Y_K^{*,2} - 25m_L^2Y_K^2Y_K^{*,2} - 25m_L^2Y_K^2Y_K^{*,2} \end{aligned}$$

$$\begin{aligned}
& -240g_{B2}^2m_{W_B}Y_AT_A^* - 240g_{B2}^2m_{W,B^*}Y_A^*T_A - 840|Y_A|^2T_A^*T_A - 30|Y_K|^2T_A^*T_A - 30Y_KY_A^*T_K^*T_A \\
& - 30Y_AY_K^*T_A^*T_K - 30|Y_A|^2T_K^*T_K - 50|Y_K|^2T_K^*T_K + 120g_{B2}^4\sigma_{2,2} + 120g_{A2}^4\sigma_{2,4} \\
& + 24g_{B1}^2\text{Tr}2\text{U}1(1,1) - 24g_{A1}g_{B1}\text{Tr}2\text{U}1(1,3) \\
& - 24g_{A1}g_{B1}\text{Tr}2\text{U}1(3,1) + 24g_{A1}^2\text{Tr}2\text{U}1(3,3) + 16\sqrt{15}g_{B1}\sigma_{3,1} - 16\sqrt{15}g_{A1}\sigma_{3,3}
\end{aligned} \tag{105}$$

$$\begin{aligned}
\beta_{m_L^2}^{(1)} = & \frac{1}{10} \left( -12g_{A1}^2|m_{B_A}|^2 - 60g_{A2}^2|m_{W_A}|^2 - 12g_{B1}^2|m_{B_B}|^2 - 60g_{B2}^2|m_{W_B}|^2 + 30m_{Ad}^2|Y_A|^2 + 30m_L^2|Y_A|^2 \right. \\
& + 30m_L^2|Y_A|^2 + 5m_K^2|Y_K|^2 + 5m_L^2|Y_K|^2 + 5m_L^2|Y_K|^2 + 30|T_A|^2 + 5|T_K|^2 - 2\sqrt{15}g_{B1}\sigma_{1,1} \\
& \left. + 2\sqrt{15}g_{A1}\sigma_{1,3} \right)
\end{aligned} \tag{106}$$

$$\begin{aligned}
\beta_{m_L^2}^{(2)} = & + \frac{9}{25}g_{A1}^2 \left( 5 \left( g_{A2}^2(2m_{B_A} + m_{W_A}) + g_{B1}^2(2m_{B_A} + m_{B_B}) + g_{B2}^2(2m_{B_A} + m_{W_B}) \right) + 81g_{A1}^2m_{B_A} \right) m_{B,A^*} \\
& + \frac{1}{20} \left( 72g_{A1}^2g_{B2}^2|m_{W_B}|^2 + 360g_{A2}^2g_{B2}^2|m_{W_B}|^2 + 72g_{B1}^2g_{B2}^2|m_{W_B}|^2 - 420g_{B2}^4|m_{W_B}|^2 \right. \\
& + 240g_{B2}^2m_{Ad}^2|Y_A|^2 + 240g_{B2}^2m_L^2|Y_A|^2 + 240g_{B2}^2m_L^2|Y_A|^2 + 240g_{B2}^2|T_A|^2 \\
& + 12g_{A2}^2 \left( 115g_{A2}^2m_{W_A} + 15g_{B2}^2m_{W_B} + 30g_{B2}^2m_{W_A} + 3g_{A1}^2(2m_{W_A} + m_{B_A}) + 3g_{B1}^2m_{B_B} + 6g_{B1}^2m_{W_A} \right) m_{W,A^*} \\
& + 36g_{B1}^2 \left( 2g_{B2}^2m_{B_B} + 3g_{B1}^2m_{B_B} + g_{A1}^2(2m_{B_B} + m_{B_A}) + g_{A2}^2(2m_{B_B} + m_{W_A}) \right. \\
& \left. + g_{B2}^2m_{W_B} \right) m_{B,B^*} + 36g_{A1}^2g_{B2}^2m_{B_A}m_{W,B^*} \\
& + 180g_{A2}^2g_{B2}^2m_{W_A}m_{W,B^*} + 36g_{B1}^2g_{B2}^2m_{B_B}m_{W,B^*} + 480g_{B2}^2Y_A|m_{W_B}|^2Y_A^* - 420m_{Ad}^2Y_A^*Y_A^{*,2} \\
& - 420m_L^2Y_A^*Y_A^{*,2} - 420m_L^2Y_A^*Y_A^{*,2} - 30m_{Ad}^2Y_K|Y_A|^2Y_K^* - 30m_K^2Y_K|Y_A|^2Y_K^* \\
& - 60m_L^2Y_K|Y_A|^2Y_K^* - 60m_L^2Y_K|Y_A|^2Y_K^* - 25m_K^2Y_K^*Y_K^{*,2} - 25m_L^2Y_K^*Y_K^{*,2} - 25m_L^2Y_K^*Y_K^{*,2} \\
& - 240g_{B2}^2m_{W_B}Y_AT_A^* - 240g_{B2}^2m_{W,B^*}Y_A^*T_A - 840|Y_A|^2T_A^*T_A - 30|Y_K|^2T_A^*T_A - 30Y_KY_A^*T_K^*T_A \\
& - 30Y_AY_K^*T_A^*T_K - 30|Y_A|^2T_K^*T_K - 50|Y_K|^2T_K^*T_K + 120g_{B2}^4\sigma_{2,2} + 120g_{A2}^4\sigma_{2,4} + 24g_{B1}^2\text{Tr}2\text{U}1(1,1) \\
& - 24g_{A1}g_{B1}\text{Tr}2\text{U}1(1,3) \\
& - 24g_{A1}g_{B1}\text{Tr}2\text{U}1(3,1) + 24g_{A1}^2\text{Tr}2\text{U}1(3,3) - 16\sqrt{15}g_{B1}\sigma_{3,1} + 16\sqrt{15}g_{A1}\sigma_{3,3}
\end{aligned} \tag{107}$$

$$\beta_{m_K^2}^{(1)} = 2 \left( (m_K^2 + m_L^2 + m_L^2)|Y_K|^2 + |T_K|^2 \right) \tag{108}$$

$$\begin{aligned}
\beta_{m_K^2}^{(2)} = & \frac{2}{5} \left( -5(m_K^2 + m_L^2 + m_L^2)Y_K^2Y_K^{*,2} \right. \\
& + Y_K^* \left( 3g_{A1}^2m_K^2Y_K + 15g_{A2}^2m_K^2Y_K + 3g_{B1}^2m_K^2Y_K + 15g_{B2}^2m_K^2Y_K + 3g_{A1}^2m_L^2Y_K + 15g_{A2}^2m_L^2Y_K \right. \\
& + 3g_{B1}^2m_L^2Y_K + 15g_{B2}^2m_L^2Y_K + 3g_{A1}^2m_L^2Y_K + 15g_{A2}^2m_L^2Y_K + 3g_{B1}^2m_L^2Y_K + 15g_{B2}^2m_L^2Y_K \\
& + 6g_{B1}^2Y_K|m_{B_B}|^2 + 30g_{B2}^2Y_K|m_{W_B}|^2 - 15m_{Ad}^2Y_K|Y_A|^2 - 15m_K^2Y_K|Y_A|^2 - 30m_L^2Y_K|Y_A|^2 \\
& - 30m_L^2Y_K|Y_A|^2 - 15Y_K|T_A|^2 - 10Y_K|T_K|^2 + 3g_{A1}^2m_{B,A^*}(2m_{B_A}Y_K - T_K) \\
& \left. \left. + 15g_{A2}^2m_{W,A^*}(2m_{W_A}Y_K - T_K) - 3g_{B1}^2m_{B,B^*}T_K - 15g_{B2}^2m_{W,B^*}T_K - 15Y_AT_A^*T_K \right) \right)
\end{aligned}$$

$$\begin{aligned}
& -3T_K^* \left( - \left( 5g_{A2}^2 + 5g_{B2}^2 + g_{A1}^2 + g_{B1}^2 \right) T_K \right. \\
& \left. + \left( 5g_{A2}^2 m_{W_A} + 5g_{B2}^2 m_{W_B} + g_{A1}^2 m_{B_A} + g_{B1}^2 m_{B_B} \right) Y_K + 5Y_A^* \left( Y_A T_K + Y_K T_A \right) \right) \quad (109)
\end{aligned}$$

$$\beta_{m_{A_d}^2}^{(1)} = 4 \left( -4g_{B2}^2 |m_{W_B}|^2 + \left( m_{A_d}^2 + m_L^2 + m_{\tilde{L}}^2 \right) |Y_A|^2 + |T_A|^2 \right) \quad (110)$$

$$\begin{aligned}
\beta_{m_{A_d}^2}^{(2)} = & -\frac{2}{5} \left( -6g_{A1}^2 |T_A|^2 - 30g_{A2}^2 |T_A|^2 - 6g_{B1}^2 |T_A|^2 + 10g_{B2}^2 |T_A|^2 + 60 \left( m_{A_d}^2 + m_L^2 + m_{\tilde{L}}^2 \right) Y_A^2 Y_A^{*,2} \right. \\
& + 6g_{A1}^2 m_{B_A} Y_A T_A^* + 30g_{A2}^2 m_{W_A} Y_A T_A^* + 6g_{B1}^2 m_{B_B} Y_A T_A^* - 10g_{B2}^2 m_{W_B} Y_A T_A^* + 5|Y_K|^2 T_A^* T_A \\
& + Y_A^* \left( -6g_{A1}^2 m_{A_d}^2 Y_A - 30g_{A2}^2 m_{A_d}^2 Y_A - 6g_{B1}^2 m_{A_d}^2 Y_A + 10g_{B2}^2 m_{A_d}^2 Y_A - 6g_{A1}^2 m_L^2 Y_A - 30g_{A2}^2 m_L^2 Y_A \right. \\
& - 6g_{B1}^2 m_L^2 Y_A + 10g_{B2}^2 m_L^2 Y_A - 6g_{A1}^2 m_{\tilde{L}}^2 Y_A - 30g_{A2}^2 m_{\tilde{L}}^2 Y_A - 6g_{B1}^2 m_{\tilde{L}}^2 Y_A + 10g_{B2}^2 m_{\tilde{L}}^2 Y_A \\
& - 12g_{B1}^2 Y_A |m_{B_B}|^2 + 5m_{A_d}^2 Y_A |Y_K|^2 + 5m_K^2 Y_A |Y_K|^2 + 10m_L^2 Y_A |Y_K|^2 + 10m_{\tilde{L}}^2 Y_A |Y_K|^2 \\
& + 120Y_A |T_A|^2 + 5Y_A |T_K|^2 + 6g_{B1}^2 m_{B,B^*} T_A + 5Y_K T_K^* T_A + 6g_{A1}^2 m_{B,A^*} \left( -2m_{B_A} Y_A + T_A \right) \\
& \left. + 30g_{A2}^2 m_{W,A^*} \left( -2m_{W_A} Y_A + T_A \right) \right) \\
& - 10g_{B2}^2 m_{W,B^*} \left( 16g_{B2}^2 m_{W_B} + Y_A^* \left( -2m_{W_B} Y_A + T_A \right) \right) + 5Y_A Y_K^* T_A^* T_K - 40g_{B2}^4 \sigma_{2,2} \quad (111)
\end{aligned}$$

## 4 Field Rotations

### 4.1 Rotations in gauge sector for eigenstates 'AxBSB'

$$\begin{pmatrix} B_{A,\rho} \\ B_{B,\rho} \end{pmatrix} = Z_V^B \begin{pmatrix} B_{L,\rho} \\ B_{H,\rho} \end{pmatrix} \quad (112)$$

$$\begin{pmatrix} W_{A,1\rho} \\ W_{B,1\rho} \end{pmatrix} = Z_V^W \begin{pmatrix} W_{L,\rho}^1 \\ W_{H,\rho}^1 \end{pmatrix} \quad (113)$$

$$\begin{pmatrix} W_{A,2\rho} \\ W_{B,2\rho} \end{pmatrix} = Z_V^W \begin{pmatrix} W_{L,\rho}^2 \\ W_{H,\rho}^2 \end{pmatrix} \quad (114)$$

$$\begin{pmatrix} W_{A,3\rho} \\ W_{B,3\rho} \end{pmatrix} = Z_V^W \begin{pmatrix} W_{L,\rho}^3 \\ W_{H,\rho}^3 \end{pmatrix} \quad (115)$$

$$\begin{pmatrix} \tilde{B}_A \\ \tilde{B}_B \end{pmatrix} = Z_V^B \begin{pmatrix} \tilde{B}_L \\ \tilde{B}_H \end{pmatrix} \quad (116)$$

$$\begin{pmatrix} \tilde{W}_{A,1} \\ \tilde{W}_{B,1} \end{pmatrix} = Z_V^W \begin{pmatrix} \tilde{B}_L \\ \tilde{B}_L \end{pmatrix} \quad (117)$$

$$\begin{pmatrix} \tilde{W}_{A,2} \\ \tilde{W}_{B,2} \end{pmatrix} = Z_V^W \begin{pmatrix} \tilde{B}_L \\ \tilde{B}_L \end{pmatrix} \quad (118)$$

$$\begin{pmatrix} \tilde{W}_{A,3} \\ \tilde{W}_{B,3} \end{pmatrix} = Z_V^W \begin{pmatrix} \tilde{B}_L \\ \tilde{B}_L \end{pmatrix} \quad (119)$$

$$(120)$$

The mixing matrices are parametrized by

$$Z_V^B = \begin{pmatrix} \cos \theta_1 & -\sin \theta_1 \\ \sin \theta_1 & \cos \theta_1 \end{pmatrix} \quad (121)$$

$$Z_V^W = \begin{pmatrix} \cos \theta_2 & -\sin \theta_2 \\ \sin \theta_2 & \cos \theta_2 \end{pmatrix} \quad (122)$$

$$Z_V^W = \begin{pmatrix} \cos \theta_2 & -\sin \theta_2 \\ \sin \theta_2 & \cos \theta_2 \end{pmatrix} \quad (123)$$

$$Z_V^W = \begin{pmatrix} \cos \theta_2 & -\sin \theta_2 \\ \sin \theta_2 & \cos \theta_2 \end{pmatrix} \quad (124)$$

$$Z_V^B = \begin{pmatrix} \cos \theta_1 & -\sin \theta_1 \\ \sin \theta_1 & \cos \theta_1 \end{pmatrix} \quad (125)$$

$$Z_V^W = \begin{pmatrix} \cos \theta_2 & -\sin \theta_2 \\ \sin \theta_2 & \cos \theta_2 \end{pmatrix} \quad (126)$$

$$Z_V^W = \begin{pmatrix} \cos \theta_2 & -\sin \theta_2 \\ \sin \theta_2 & \cos \theta_2 \end{pmatrix} \quad (127)$$

$$Z_V^W = \begin{pmatrix} \cos \theta_2 & -\sin \theta_2 \\ \sin \theta_2 & \cos \theta_2 \end{pmatrix} \quad (128)$$

$$(129)$$

## 4.2 Rotations in Mass sector for eigenstates 'AxBSB'

### 4.2.1 Mass Matrices for Scalars

- **Mass matrix for Linking fields real scalars** , Basis:  $(\phi_{L1}, \phi_{Lt1}, \phi_{L4}, \phi_{Lt4}), (\phi_{L1}, \phi_{Lt1}, \phi_{L4}, \phi_{Lt4})$

$$m_{\phi_L^0}^2 = \begin{pmatrix} m_{11} & m_{21} & m_{31} & m_{41} \\ m_{21} & m_{22} & m_{32} & m_{42} \\ m_{31} & m_{32} & m_{33} & m_{43} \\ m_{41} & m_{42} & m_{43} & m_{44} \end{pmatrix} \quad (130)$$

$$m_{11} = 2m_L^2 + \frac{1}{2}v_{Lv}^2|Y_K|^2 + (g_{A1}^2 + g_{A2}^2 + g_{B1}^2 + g_{B2}^2)v_{Lv}^2 + v_{Lv}^2|Y_A|^2 \quad (131)$$

$$m_{21} = \frac{1}{2} \left( -\Omega \Re(Y_K) + v_{Lv}^2 \left( -2(g_{A1}^2 + g_{A2}^2 + g_{B1}^2 + g_{B2}^2) + 2|Y_A|^2 + 3|Y_K|^2 \right) \right) \quad (132)$$

$$m_{22} = 2m_L^2 + \frac{1}{2} v_{Lv}^2 |Y_K|^2 + \left( g_{A1}^2 + g_{A2}^2 + g_{B1}^2 + g_{B2}^2 \right) v_{Lv}^2 + v_{Lv}^2 |Y_A|^2 \quad (133)$$

$$m_{31} = \frac{1}{2} v_{Lv}^2 \left( 2 \left( -g_{A2}^2 - g_{B2}^2 + g_{A1}^2 + g_{B1}^2 \right) - 2|Y_A|^2 + |Y_K|^2 \right) \quad (134)$$

$$m_{32} = \frac{1}{2} v_{Lv}^2 \left( -2 \left( -g_{A2}^2 - g_{B2}^2 + g_{A1}^2 + g_{B1}^2 + |Y_A|^2 \right) + |Y_K|^2 \right) \quad (135)$$

$$m_{33} = 2m_L^2 + \frac{1}{2} v_{Lv}^2 |Y_K|^2 + \left( g_{A1}^2 + g_{A2}^2 + g_{B1}^2 + g_{B2}^2 \right) v_{Lv}^2 + v_{Lv}^2 |Y_A|^2 \quad (136)$$

$$m_{41} = \frac{1}{2} v_{Lv}^2 \left( -2 \left( -g_{A2}^2 - g_{B2}^2 + g_{A1}^2 + g_{B1}^2 + |Y_A|^2 \right) + |Y_K|^2 \right) \quad (137)$$

$$m_{42} = \frac{1}{2} v_{Lv}^2 \left( 2 \left( -g_{A2}^2 - g_{B2}^2 + g_{A1}^2 + g_{B1}^2 \right) - 2|Y_A|^2 + |Y_K|^2 \right) \quad (138)$$

$$m_{43} = \frac{1}{2} \left( -\Omega \Re(Y_K) + v_{Lv}^2 \left( -2(g_{A1}^2 + g_{A2}^2 + g_{B1}^2 + g_{B2}^2) + 2|Y_A|^2 + 3|Y_K|^2 \right) \right) \quad (139)$$

$$m_{44} = 2m_L^2 + \frac{1}{2} v_{Lv}^2 |Y_K|^2 + \left( g_{A1}^2 + g_{A2}^2 + g_{B1}^2 + g_{B2}^2 \right) v_{Lv}^2 + v_{Lv}^2 |Y_A|^2 \quad (140)$$

This matrix is diagonalized by  $Z_{Ls}^{DR}$ :

$$Z_{Ls}^{DR} m_{\phi_L^0}^2 Z_{Ls}^{DR,\dagger} = m_{2,\phi_L^0}^{dia} \quad (141)$$

with

$$\phi_{L1} = \sum_j Z_{Ls,j1}^{DR,*} \phi_{L,j}^0, \quad \phi_{Lt1} = \sum_j Z_{Ls,j2}^{DR,*} \phi_{L,j}^0, \quad \phi_{L4} = \sum_j Z_{Ls,j3}^{DR,*} \phi_{L,j}^0 \quad (142)$$

$$\phi_{Lt4} = \sum_j Z_{Ls,j4}^{DR,*} \phi_{L,j}^0 \quad (143)$$

- **Mass matrix for Heavy B gauge boson, Basis:**  $(\sigma_{L1}, \sigma_{Lt1}, \sigma_{L4}, \sigma_{Lt4}), (\sigma_{L1}, \sigma_{Lt1}, \sigma_{L4}, \sigma_{Lt4})$

$$m_{\sigma_L^0}^2 = \begin{pmatrix} m_{11} & m_{21} & m_{31} & m_{41} \\ m_{21} & m_{22} & m_{32} & m_{42} \\ m_{31} & m_{32} & m_{33} & m_{43} \\ m_{41} & m_{42} & m_{43} & m_{44} \end{pmatrix} + \xi_{B_L} m^2(B_L) + \xi_{B_H} m^2(B_H) + \xi_{W_L^3} m^2(W_L^3) + \xi_{W_H^3} m^2(W_H^3) \quad (144)$$

$$m_{11} = 2m_L^2 + \frac{1}{2} v_{Lv}^2 \left( 2|Y_A|^2 + |Y_K|^2 \right) \quad (145)$$

$$m_{21} = \frac{1}{2} \left( 2v_{Lv}^2 |Y_A|^2 + \Omega \Re(Y_K) - v_{Lv}^2 |Y_K|^2 \right) \quad (146)$$

$$m_{22} = 2m_L^2 + \frac{1}{2} v_{Lv}^2 \left( 2|Y_A|^2 + |Y_K|^2 \right) \quad (147)$$

$$m_{31} = \frac{1}{2} v_{Lv}^2 \left( -2|Y_A|^2 + |Y_K|^2 \right) \quad (148)$$

$$m_{32} = \frac{1}{2} v_{Lv}^2 \left( -2|Y_A|^2 + |Y_K|^2 \right) \quad (149)$$

$$m_{33} = 2m_L^2 + \frac{1}{2}v_{Lv}^2(2|Y_A|^2 + |Y_K|^2) \quad (150)$$

$$m_{41} = \frac{1}{2}v_{Lv}^2(-2|Y_A|^2 + |Y_K|^2) \quad (151)$$

$$m_{42} = \frac{1}{2}v_{Lv}^2(-2|Y_A|^2 + |Y_K|^2) \quad (152)$$

$$m_{43} = \frac{1}{2}(2v_{Lv}^2|Y_A|^2 + \Omega\Re(Y_K) - v_{Lv}^2|Y_K|^2) \quad (153)$$

$$m_{44} = 2m_L^2 + \frac{1}{2}v_{Lv}^2(2|Y_A|^2 + |Y_K|^2) \quad (154)$$

Gauge fixing contributions:

$$m^2(\xi_{B_L}) = \begin{pmatrix} m_{11} & m_{21} & m_{31} & m_{41} \\ m_{21} & m_{22} & m_{32} & m_{42} \\ m_{31} & m_{32} & m_{33} & m_{43} \\ m_{41} & m_{42} & m_{43} & m_{44} \end{pmatrix} \quad (155)$$

$$m_{11} = v_{Lv}^2(g_{A1} \cos \theta_1 - g_{B1} \sin \theta_1)^2 \quad (156)$$

$$m_{21} = -v_{Lv}^2(g_{A1} \cos \theta_1 - g_{B1} \sin \theta_1)^2 \quad (157)$$

$$m_{22} = v_{Lv}^2(g_{A1} \cos \theta_1 - g_{B1} \sin \theta_1)^2 \quad (158)$$

$$m_{31} = v_{Lv}^2(g_{A1} \cos \theta_1 - g_{B1} \sin \theta_1)^2 \quad (159)$$

$$m_{32} = -v_{Lv}^2(g_{A1} \cos \theta_1 - g_{B1} \sin \theta_1)^2 \quad (160)$$

$$m_{33} = v_{Lv}^2(g_{A1} \cos \theta_1 - g_{B1} \sin \theta_1)^2 \quad (161)$$

$$m_{41} = -v_{Lv}^2(g_{A1} \cos \theta_1 - g_{B1} \sin \theta_1)^2 \quad (162)$$

$$m_{42} = v_{Lv}^2(g_{A1} \cos \theta_1 - g_{B1} \sin \theta_1)^2 \quad (163)$$

$$m_{43} = -v_{Lv}^2(g_{A1} \cos \theta_1 - g_{B1} \sin \theta_1)^2 \quad (164)$$

$$m_{44} = v_{Lv}^2(g_{A1} \cos \theta_1 - g_{B1} \sin \theta_1)^2 \quad (165)$$

$$m^2(\xi_{B_H}) = \begin{pmatrix} m_{11} & m_{21} & m_{31} & m_{41} \\ m_{21} & m_{22} & m_{32} & m_{42} \\ m_{31} & m_{32} & m_{33} & m_{43} \\ m_{41} & m_{42} & m_{43} & m_{44} \end{pmatrix} \quad (166)$$

$$m_{11} = v_{Lv}^2(g_{A1} \sin \theta_1 + g_{B1} \cos \theta_1)^2 \quad (167)$$



$$m_{21} = -v_{Lv}^2 \left( g_{A1} \sin \theta_1 + g_{B1} \cos \theta_1 \right)^2 \quad (168)$$

$$m_{22} = v_{Lv}^2 \left( g_{A1} \sin \theta_1 + g_{B1} \cos \theta_1 \right)^2 \quad (169)$$

$$m_{31} = v_{Lv}^2 \left( g_{A1} \sin \theta_1 + g_{B1} \cos \theta_1 \right)^2 \quad (170)$$

$$m_{32} = -v_{Lv}^2 \left( g_{A1} \sin \theta_1 + g_{B1} \cos \theta_1 \right)^2 \quad (171)$$

$$m_{33} = v_{Lv}^2 \left( g_{A1} \sin \theta_1 + g_{B1} \cos \theta_1 \right)^2 \quad (172)$$

$$m_{41} = -v_{Lv}^2 \left( g_{A1} \sin \theta_1 + g_{B1} \cos \theta_1 \right)^2 \quad (173)$$

$$m_{42} = v_{Lv}^2 \left( g_{A1} \sin \theta_1 + g_{B1} \cos \theta_1 \right)^2 \quad (174)$$

$$m_{43} = -v_{Lv}^2 \left( g_{A1} \sin \theta_1 + g_{B1} \cos \theta_1 \right)^2 \quad (175)$$

$$m_{44} = v_{Lv}^2 \left( g_{A1} \sin \theta_1 + g_{B1} \cos \theta_1 \right)^2 \quad (176)$$

$$m^2(\xi_{W_L^3}) = \begin{pmatrix} m_{11} & m_{21} & m_{31} & m_{41} \\ m_{21} & m_{22} & m_{32} & m_{42} \\ m_{31} & m_{32} & m_{33} & m_{43} \\ m_{41} & m_{42} & m_{43} & m_{44} \end{pmatrix} \quad (177)$$

$$m_{11} = v_{Lv}^2 \left( g_{A2} \cos \theta_2 - g_{B2} \sin \theta_2 \right)^2 \quad (178)$$

$$m_{21} = -v_{Lv}^2 \left( g_{A2} \cos \theta_2 - g_{B2} \sin \theta_2 \right)^2 \quad (179)$$

$$m_{22} = v_{Lv}^2 \left( g_{A2} \cos \theta_2 - g_{B2} \sin \theta_2 \right)^2 \quad (180)$$

$$m_{31} = -v_{Lv}^2 \left( g_{A2} \cos \theta_2 - g_{B2} \sin \theta_2 \right)^2 \quad (181)$$

$$m_{32} = v_{Lv}^2 \left( g_{A2} \cos \theta_2 - g_{B2} \sin \theta_2 \right)^2 \quad (182)$$

$$m_{33} = v_{Lv}^2 \left( g_{A2} \cos \theta_2 - g_{B2} \sin \theta_2 \right)^2 \quad (183)$$

$$m_{41} = v_{Lv}^2 \left( g_{A2} \cos \theta_2 - g_{B2} \sin \theta_2 \right)^2 \quad (184)$$

$$m_{42} = -v_{Lv}^2 \left( g_{A2} \cos \theta_2 - g_{B2} \sin \theta_2 \right)^2 \quad (185)$$

$$m_{43} = -v_{Lv}^2 \left( g_{A2} \cos \theta_2 - g_{B2} \sin \theta_2 \right)^2 \quad (186)$$

$$m_{44} = v_{Lv}^2 \left( g_{A2} \cos \theta_2 - g_{B2} \sin \theta_2 \right)^2 \quad (187)$$

$$m^2(\xi_{W_H^3}) = \begin{pmatrix} m_{11} & m_{21} & m_{31} & m_{41} \\ m_{21} & m_{22} & m_{32} & m_{42} \\ m_{31} & m_{32} & m_{33} & m_{43} \\ m_{41} & m_{42} & m_{43} & m_{44} \end{pmatrix} \quad (188)$$

$$m_{11} = v_{Lv}^2 \left( g_{A2} \sin \theta_2 + g_{B2} \cos \theta_2 \right)^2 \quad (189)$$

$$m_{21} = -v_{Lv}^2 \left( g_{A2} \sin \theta_2 + g_{B2} \cos \theta_2 \right)^2 \quad (190)$$

$$m_{22} = v_{Lv}^2 \left( g_{A2} \sin \theta_2 + g_{B2} \cos \theta_2 \right)^2 \quad (191)$$

$$m_{31} = -v_{Lv}^2 \left( g_{A2} \sin \theta_2 + g_{B2} \cos \theta_2 \right)^2 \quad (192)$$

$$m_{32} = v_{Lv}^2 \left( g_{A2} \sin \theta_2 + g_{B2} \cos \theta_2 \right)^2 \quad (193)$$

$$m_{33} = v_{Lv}^2 \left( g_{A2} \sin \theta_2 + g_{B2} \cos \theta_2 \right)^2 \quad (194)$$

$$m_{41} = v_{Lv}^2 \left( g_{A2} \sin \theta_2 + g_{B2} \cos \theta_2 \right)^2 \quad (195)$$

$$m_{42} = -v_{Lv}^2 \left( g_{A2} \sin \theta_2 + g_{B2} \cos \theta_2 \right)^2 \quad (196)$$

$$m_{43} = -v_{Lv}^2 \left( g_{A2} \sin \theta_2 + g_{B2} \cos \theta_2 \right)^2 \quad (197)$$

$$m_{44} = v_{Lv}^2 \left( g_{A2} \sin \theta_2 + g_{B2} \cos \theta_2 \right)^2 \quad (198)$$

This matrix is diagonalized by  $Z_{Ls}^{Di}$ :

$$Z_{Ls}^{Di} m_{\sigma_L^0}^2 Z_{Ls}^{Di,\dagger} = m_{2,\sigma_L^0}^{dia} \quad (199)$$

with

$$\sigma_{L1} = \sum_j Z_{Ls,j1}^{Di,*} \sigma_{L,j}^0, \quad \sigma_{Lt1} = \sum_j Z_{Ls,j2}^{Di,*} \sigma_{L,j}^0, \quad \sigma_{L4} = \sum_j Z_{Ls,j3}^{Di,*} \sigma_{L,j}^0 \quad (200)$$

$$\sigma_{Lt4} = \sum_j Z_{Ls,j4}^{Di,*} \sigma_{L,j}^0 \quad (201)$$

- **Mass matrix for Linking fields charged scalars** , Basis:  $(\varphi_{l2}, \tilde{\varphi}_{lt3}, \tilde{\varphi}_{lt2}^*, \varphi_{l3}^*), (\varphi_{l2}^*, \tilde{\varphi}_{lt3}^*, \tilde{\varphi}_{lt2}, \varphi_{l3})$

$$m_{\sigma_L^\pm}^2 = \begin{pmatrix} m_{11} & m_{21}^* & m_{31}^* & \frac{1}{2}(g_{A2}^2 + g_{B2}^2)v_{Lv}^2 \\ m_{21} & m_{22} & \frac{1}{2}(g_{A2}^2 + g_{B2}^2)v_{Lv}^2 & m_{42}^* \\ m_{31} & \frac{1}{2}(g_{A2}^2 + g_{B2}^2)v_{Lv}^2 & m_{33} & m_{43}^* \\ \frac{1}{2}(g_{A2}^2 + g_{B2}^2)v_{Lv}^2 & m_{42} & m_{43} & m_{44} \end{pmatrix} \quad (202)$$

$$+ \xi_{W_L^1} m^2(W_L^1) + \xi_{W_H^1} m^2(W_H^1) + \xi_{W_L^2} m^2(W_L^2) + \xi_{W_H^2} m^2(W_H^2)$$

$$m_{11} = \frac{1}{8} \left( 4(g_{A2}^2 + g_{B2}^2) v_{Lv}^2 + 8m_L^2 + 8v_{Lv}^2 |Y_A|^2 \right) \quad (203)$$

$$m_{21} = \frac{1}{8} v_{Lv}^2 \left( -4(g_{A2}^2 + g_{B2}^2) + 8|Y_A|^2 \right) \quad (204)$$

$$m_{22} = \frac{1}{8} \left( 4(g_{A2}^2 + g_{B2}^2) v_{Lv}^2 + 8m_L^2 + 8v_{Lv}^2 |Y_A|^2 \right) \quad (205)$$

$$m_{31} = \frac{1}{8} \left( -2\Omega Y_K - 4(g_{A2}^2 + g_{B2}^2) v_{Lv}^2 + 4v_{Lv}^2 |Y_K|^2 \right) \quad (206)$$

$$m_{33} = \frac{1}{8} \left( 4(g_{A2}^2 + g_{B2}^2) v_{Lv}^2 + 8m_L^2 + 8v_{Lv}^2 |Y_A|^2 \right) \quad (207)$$

$$m_{42} = \frac{1}{8} \left( -2\Omega Y_K - 4(g_{A2}^2 + g_{B2}^2) v_{Lv}^2 + 4v_{Lv}^2 |Y_K|^2 \right) \quad (208)$$

$$m_{43} = \frac{1}{8} v_{Lv}^2 \left( -4(g_{A2}^2 + g_{B2}^2) + 8|Y_A|^2 \right) \quad (209)$$

$$m_{44} = \frac{1}{8} \left( 4(g_{A2}^2 + g_{B2}^2) v_{Lv}^2 + 8m_L^2 + 8v_{Lv}^2 |Y_A|^2 \right) \quad (210)$$

Gauge fixing contributions:

$$m^2(\xi_{W_L^1}) = \begin{pmatrix} m_{11} & m_{21}^* & m_{31}^* & m_{41}^* \\ m_{21} & m_{22} & m_{32}^* & m_{42}^* \\ m_{31} & m_{32} & m_{33} & m_{43}^* \\ m_{41} & m_{42} & m_{43} & m_{44} \end{pmatrix} \quad (211)$$

$$m_{11} = \frac{1}{4} v_{Lv}^2 \left( g_{A2} \cos \theta_2 - g_{B2} \sin \theta_2 \right)^2 \quad (212)$$

$$m_{21} = -\frac{1}{4} v_{Lv}^2 \left( g_{A2} \cos \theta_2 - g_{B2} \sin \theta_2 \right)^2 \quad (213)$$

$$m_{22} = \frac{1}{4} v_{Lv}^2 \left( g_{A2} \cos \theta_2 - g_{B2} \sin \theta_2 \right)^2 \quad (214)$$

$$m_{31} = \frac{1}{4} v_{Lv}^2 \left( g_{A2} \cos \theta_2 - g_{B2} \sin \theta_2 \right)^2 \quad (215)$$

$$m_{32} = -\frac{1}{4} v_{Lv}^2 \left( g_{A2} \cos \theta_2 - g_{B2} \sin \theta_2 \right)^2 \quad (216)$$

$$m_{33} = \frac{1}{4} v_{Lv}^2 \left( g_{A2} \cos \theta_2 - g_{B2} \sin \theta_2 \right)^2 \quad (217)$$

$$m_{41} = -\frac{1}{4} v_{Lv}^2 \left( g_{A2} \cos \theta_2 - g_{B2} \sin \theta_2 \right)^2 \quad (218)$$

$$m_{42} = \frac{1}{4} v_{Lv}^2 \left( g_{A2} \cos \theta_2 - g_{B2} \sin \theta_2 \right)^2 \quad (219)$$

$$m_{43} = -\frac{1}{4} v_{Lv}^2 \left( g_{A2} \cos \theta_2 - g_{B2} \sin \theta_2 \right)^2 \quad (220)$$

$$m_{44} = \frac{1}{4} v_{Lv}^2 \left( g_{A2} \cos \theta_2 - g_{B2} \sin \theta_2 \right)^2 \quad (221)$$

$$m^2(\xi_{W_H^1}) = \begin{pmatrix} m_{11} & m_{21}^* & m_{31}^* & m_{41}^* \\ m_{21} & m_{22} & m_{32}^* & m_{42}^* \\ m_{31} & m_{32} & m_{33} & m_{43}^* \\ m_{41} & m_{42} & m_{43} & m_{44} \end{pmatrix} \quad (222)$$

$$m_{11} = \frac{1}{4}v_{Lv}^2 \left( g_{A2} \sin \theta_2 + g_{B2} \cos \theta_2 \right)^2 \quad (223)$$

$$m_{21} = -\frac{1}{4}v_{Lv}^2 \left( g_{A2} \sin \theta_2 + g_{B2} \cos \theta_2 \right)^2 \quad (224)$$

$$m_{22} = \frac{1}{4}v_{Lv}^2 \left( g_{A2} \sin \theta_2 + g_{B2} \cos \theta_2 \right)^2 \quad (225)$$

$$m_{31} = \frac{1}{4}v_{Lv}^2 \left( g_{A2} \sin \theta_2 + g_{B2} \cos \theta_2 \right)^2 \quad (226)$$

$$m_{32} = -\frac{1}{4}v_{Lv}^2 \left( g_{A2} \sin \theta_2 + g_{B2} \cos \theta_2 \right)^2 \quad (227)$$

$$m_{33} = \frac{1}{4}v_{Lv}^2 \left( g_{A2} \sin \theta_2 + g_{B2} \cos \theta_2 \right)^2 \quad (228)$$

$$m_{41} = -\frac{1}{4}v_{Lv}^2 \left( g_{A2} \sin \theta_2 + g_{B2} \cos \theta_2 \right)^2 \quad (229)$$

$$m_{42} = \frac{1}{4}v_{Lv}^2 \left( g_{A2} \sin \theta_2 + g_{B2} \cos \theta_2 \right)^2 \quad (230)$$

$$m_{43} = -\frac{1}{4}v_{Lv}^2 \left( g_{A2} \sin \theta_2 + g_{B2} \cos \theta_2 \right)^2 \quad (231)$$

$$m_{44} = \frac{1}{4}v_{Lv}^2 \left( g_{A2} \sin \theta_2 + g_{B2} \cos \theta_2 \right)^2 \quad (232)$$

$$m^2(\xi_{W_L^2}) = \begin{pmatrix} m_{11} & m_{21}^* & m_{31}^* & m_{41}^* \\ m_{21} & m_{22} & m_{32}^* & m_{42}^* \\ m_{31} & m_{32} & m_{33} & m_{43}^* \\ m_{41} & m_{42} & m_{43} & m_{44} \end{pmatrix} \quad (233)$$

$$m_{11} = \frac{1}{4}v_{Lv}^2 \left( g_{A2} \cos \theta_2 - g_{B2} \sin \theta_2 \right)^2 \quad (234)$$

$$m_{21} = -\frac{1}{4}v_{Lv}^2 \left( g_{A2} \cos \theta_2 - g_{B2} \sin \theta_2 \right)^2 \quad (235)$$

$$m_{22} = \frac{1}{4}v_{Lv}^2 \left( g_{A2} \cos \theta_2 - g_{B2} \sin \theta_2 \right)^2 \quad (236)$$

$$m_{31} = \frac{1}{4}v_{Lv}^2 \left( g_{A2} \cos \theta_2 - g_{B2} \sin \theta_2 \right)^2 \quad (237)$$

$$m_{32} = -\frac{1}{4}v_{Lv}^2 \left( g_{A2} \cos \theta_2 - g_{B2} \sin \theta_2 \right)^2 \quad (238)$$

$$m_{33} = \frac{1}{4}v_{Lv}^2 \left( g_{A2} \cos \theta_2 - g_{B2} \sin \theta_2 \right)^2 \quad (239)$$

$$m_{41} = -\frac{1}{4}v_{Lv}^2 \left( g_{A2} \cos \theta_2 - g_{B2} \sin \theta_2 \right)^2 \quad (240)$$

$$m_{42} = \frac{1}{4}v_{Lv}^2 \left( g_{A2} \cos \theta_2 - g_{B2} \sin \theta_2 \right)^2 \quad (241)$$

$$m_{43} = -\frac{1}{4}v_{Lv}^2 \left( g_{A2} \cos \theta_2 - g_{B2} \sin \theta_2 \right)^2 \quad (242)$$

$$m_{44} = \frac{1}{4}v_{Lv}^2 \left( g_{A2} \cos \theta_2 - g_{B2} \sin \theta_2 \right)^2 \quad (243)$$

$$m^2(\xi_{W_H^2}) = \begin{pmatrix} m_{11} & m_{21}^* & m_{31}^* & m_{41}^* \\ m_{21} & m_{22} & m_{32}^* & m_{42}^* \\ m_{31} & m_{32} & m_{33} & m_{43}^* \\ m_{41} & m_{42} & m_{43} & m_{44} \end{pmatrix} \quad (244)$$

$$m_{11} = \frac{1}{4}v_{Lv}^2 \left( g_{A2} \sin \theta_2 + g_{B2} \cos \theta_2 \right)^2 \quad (245)$$

$$m_{21} = -\frac{1}{4}v_{Lv}^2 \left( g_{A2} \sin \theta_2 + g_{B2} \cos \theta_2 \right)^2 \quad (246)$$

$$m_{22} = \frac{1}{4}v_{Lv}^2 \left( g_{A2} \sin \theta_2 + g_{B2} \cos \theta_2 \right)^2 \quad (247)$$

$$m_{31} = \frac{1}{4}v_{Lv}^2 \left( g_{A2} \sin \theta_2 + g_{B2} \cos \theta_2 \right)^2 \quad (248)$$

$$m_{32} = -\frac{1}{4}v_{Lv}^2 \left( g_{A2} \sin \theta_2 + g_{B2} \cos \theta_2 \right)^2 \quad (249)$$

$$m_{33} = \frac{1}{4}v_{Lv}^2 \left( g_{A2} \sin \theta_2 + g_{B2} \cos \theta_2 \right)^2 \quad (250)$$

$$m_{41} = -\frac{1}{4}v_{Lv}^2 \left( g_{A2} \sin \theta_2 + g_{B2} \cos \theta_2 \right)^2 \quad (251)$$

$$m_{42} = \frac{1}{4}v_{Lv}^2 \left( g_{A2} \sin \theta_2 + g_{B2} \cos \theta_2 \right)^2 \quad (252)$$

$$m_{43} = -\frac{1}{4}v_{Lv}^2 \left( g_{A2} \sin \theta_2 + g_{B2} \cos \theta_2 \right)^2 \quad (253)$$

$$m_{44} = \frac{1}{4}v_{Lv}^2 \left( g_{A2} \sin \theta_2 + g_{B2} \cos \theta_2 \right)^2 \quad (254)$$

This matrix is diagonalized by  $Z_{Ls}^{od}$ :

$$Z_{Ls}^{od} m_{\sigma_L^\pm}^2 Z_{Ls}^{od,\dagger} = m_{2,\sigma_L^\pm}^{dia} \quad (255)$$

with

$$\varphi_{l2} = \sum_j Z_{Ls,j1}^{od,*} \sigma_{L,j}^\pm, \quad \tilde{\varphi}_{lt3} = \sum_j Z_{Ls,j2}^{od,*} \sigma_{L,j}^\pm, \quad \tilde{\varphi}_{lt2} = \sum_j Z_{Ls,j3}^{od} \sigma_{L,j}^{\pm,*} \quad (256)$$

$$\varphi_{l3} = \sum_j Z_{Ls,j4}^{od} \sigma_{L,j}^{\pm,*} \quad (257)$$

- **Mass matrix for Final heavy scalars 1** , Basis:  $(K_s, Ad_s^1), (K_s^*, Ad_s^{1,*})$

$$m_{\phi_{AK}^s}^2 = \begin{pmatrix} v_{Lv}^2 |Y_K|^2 + m_K^2 & 0 \\ 0 & 2v_{Lv}^2 |Y_A|^2 + m_{Ad}^2 \end{pmatrix} \quad (258)$$

This matrix is diagonalized by  $Z_{AK}^s$ :

$$Z_{AK}^s m_{\phi_{AK}^s}^2 Z_{AK}^{s,\dagger} = m_{2,\phi_{AK}^s}^{dia} \quad (259)$$

with

$$K_s = \sum_j Z_{AK,j1}^{s,*} \phi_{AK,j}^s, \quad Ad_s^1 = \sum_j Z_{AK,j2}^{s,*} \phi_{AK,j}^s \quad (260)$$

- **Mass matrix for Final heavy scalars 2** , Basis:  $(Ad_s^2, Ad_s^{3,*}), (Ad_s^{2,*}, Ad_s^3)$

$$m_{\phi_B^s}^2 = \begin{pmatrix} 2v_{Lv}^2 |Y_A|^2 + m_{Ad}^2 & 0 \\ 0 & 2v_{Lv}^2 |Y_A|^2 + m_{Ad}^2 \end{pmatrix} \quad (261)$$

This matrix is diagonalized by  $B_A^s$ :

$$B_A^s m_{\phi_B^s}^2 B_A^{s,\dagger} = m_{2,\phi_B^s}^{dia} \quad (262)$$

with

$$Ad_s^2 = \sum_j B_{A,j1}^{s,*} \phi_{B,j}^s, \quad Ad_s^3 = \sum_j B_{A,j2}^{s,*} \phi_{B,j}^s \quad (263)$$

#### 4.2.2 Mass Matrices for Fermions

- **Mass matrix for Linking/Ad/K neutral fermion mass eigenstates after AxB breaking** , Basis:

$$\left( \chi_{l1}, \chi_{lt1}, \chi_{l4}, \chi_{lt4}, \tilde{B}_L, \tilde{B}_H, \tilde{B}_L, \tilde{B}_L, \text{Fad1}, K_f \right), \left( \chi_{l1}, \chi_{lt1}, \chi_{l4}, \chi_{lt4}, \tilde{B}_L, \tilde{B}_H, \tilde{B}_L, \tilde{B}_L, \text{Fad1}, K_f \right)$$

$$m_{f_{Po}^0} = \begin{pmatrix} 0 & 0 & 0 & 0 & m_{51} & m_{61} & m_{71} & m_{81} & m_{91} & m_{101} \\ 0 & 0 & 0 & 0 & m_{52} & m_{62} & m_{72} & m_{82} & m_{92} & m_{102} \\ 0 & 0 & 0 & 0 & m_{53} & m_{63} & m_{73} & m_{83} & m_{93} & m_{103} \\ 0 & 0 & 0 & 0 & m_{54} & m_{64} & m_{74} & m_{84} & m_{94} & m_{104} \\ m_{51} & m_{52} & m_{53} & m_{54} & m_{55} & m_{65} & 0 & 0 & 0 & 0 \\ m_{61} & m_{62} & m_{63} & m_{64} & m_{65} & m_{66} & 0 & 0 & 0 & 0 \\ m_{71} & m_{72} & m_{73} & m_{74} & 0 & 0 & m_{77} & m_{87} & 0 & 0 \\ m_{81} & m_{82} & m_{83} & m_{84} & 0 & 0 & m_{87} & m_{88} & 0 & 0 \\ m_{91} & m_{92} & m_{93} & m_{94} & 0 & 0 & 0 & 0 & 0 & 0 \\ m_{101} & m_{102} & m_{103} & m_{104} & 0 & 0 & 0 & 0 & 0 & 0 \end{pmatrix} \quad (264)$$

$$m_{51} = \frac{1}{\sqrt{2}} v_{Lv} \left( -g_{A1} \cos \theta_1 + g_{B1} \sin \theta_1 \right) \quad (265)$$

$$m_{52} = \frac{1}{\sqrt{2}} v_{Lv} (g_{A1} \cos \theta_1 - g_{B1} \sin \theta_1) \quad (266)$$

$$m_{53} = \frac{1}{\sqrt{2}} v_{Lv} (-g_{A1} \cos \theta_1 + g_{B1} \sin \theta_1) \quad (267)$$

$$m_{54} = \frac{1}{\sqrt{2}} v_{Lv} (g_{A1} \cos \theta_1 - g_{B1} \sin \theta_1) \quad (268)$$

$$m_{55} = m_{B_A} \cos^2 \theta_1 + m_{B_B} \sin^2 \theta_1 \quad (269)$$

$$m_{61} = \frac{1}{\sqrt{2}} v_{Lv} (g_{A1} \sin \theta_1 + g_{B1} \cos \theta_1) \quad (270)$$

$$m_{62} = -\frac{1}{\sqrt{2}} v_{Lv} (g_{A1} \sin \theta_1 + g_{B1} \cos \theta_1) \quad (271)$$

$$m_{63} = \frac{1}{\sqrt{2}} v_{Lv} (g_{A1} \sin \theta_1 + g_{B1} \cos \theta_1) \quad (272)$$

$$m_{64} = -\frac{1}{\sqrt{2}} v_{Lv} (g_{A1} \sin \theta_1 + g_{B1} \cos \theta_1) \quad (273)$$

$$m_{65} = (-m_{B_A} + m_{B_B}) \cos \theta_1 \sin \theta_1 \quad (274)$$

$$m_{66} = m_{B_A} \sin^2 \theta_1 + m_{B_B} \cos^2 \theta_1 \quad (275)$$

$$m_{71} = \frac{1}{\sqrt{2}} v_{Lv} (g_{A2} \cos \theta_2 - g_{B2} \sin \theta_2) \quad (276)$$

$$m_{72} = \frac{1}{\sqrt{2}} v_{Lv} (-g_{A2} \cos \theta_2 + g_{B2} \sin \theta_2) \quad (277)$$

$$m_{73} = \frac{1}{\sqrt{2}} v_{Lv} (-g_{A2} \cos \theta_2 + g_{B2} \sin \theta_2) \quad (278)$$

$$m_{74} = \frac{1}{\sqrt{2}} v_{Lv} (g_{A2} \cos \theta_2 - g_{B2} \sin \theta_2) \quad (279)$$

$$m_{77} = m_{W_A} \cos^2 \theta_2 + m_{W_B} \sin^2 \theta_2 \quad (280)$$

$$m_{81} = -\frac{1}{\sqrt{2}} v_{Lv} (g_{A2} \sin \theta_2 + g_{B2} \cos \theta_2) \quad (281)$$

$$m_{82} = \frac{1}{\sqrt{2}} v_{Lv} (g_{A2} \sin \theta_2 + g_{B2} \cos \theta_2) \quad (282)$$

$$m_{83} = \frac{1}{\sqrt{2}} v_{Lv} (g_{A2} \sin \theta_2 + g_{B2} \cos \theta_2) \quad (283)$$

$$m_{84} = -\frac{1}{\sqrt{2}} v_{Lv} (g_{A2} \sin \theta_2 + g_{B2} \cos \theta_2) \quad (284)$$

$$m_{87} = (-m_{W_A} + m_{W_B}) \cos \theta_2 \sin \theta_2 \quad (285)$$

$$m_{88} = m_{W_A} \sin^2 \theta_2 + m_{W_B} \cos^2 \theta_2 \quad (286)$$

$$m_{91} = \frac{1}{\sqrt{2}} v_{Lv} Y_A \quad (287)$$

$$m_{92} = \frac{1}{\sqrt{2}} v_{Lv} Y_A \quad (288)$$

$$m_{93} = -\frac{1}{\sqrt{2}} v_{Lv} Y_A \quad (289)$$

$$m_{94} = -\frac{1}{\sqrt{2}} v_{Lv} Y_A \quad (290)$$

$$m_{101} = \frac{1}{2} v_{Lv} Y_K \quad (291)$$

$$m_{102} = \frac{1}{2} v_{Lv} Y_K \quad (292)$$

$$m_{103} = \frac{1}{2} v_{Lv} Y_K \quad (293)$$

$$m_{104} = \frac{1}{2} v_{Lv} Y_K \quad (294)$$

This matrix is diagonalized by  $Z_{Po}$ :

$$Z_{Po}^* m_{f_{Po}^0} Z_{Po}^\dagger = m_{f_{Po}^0}^{dia} \quad (295)$$

with

$$\chi_{l1} = \sum_j Z_{Po,j1}^* f_{Po,j}^0, \quad \chi_{lt1} = \sum_j Z_{Po,j2}^* f_{Po,j}^0, \quad \chi_{l4} = \sum_j Z_{Po,j3}^* f_{Po,j}^0 \quad (296)$$

$$\chi_{lt4} = \sum_j Z_{Po,j4}^* f_{Po,j}^0, \quad \tilde{B}_L = \sum_j Z_{Po,j5}^* f_{Po,j}^0, \quad \tilde{B}_H = \sum_j Z_{Po,j6}^* f_{Po,j}^0 \quad (297)$$

$$\tilde{B}_L = \sum_j Z_{Po,j7}^* f_{Po,j}^0, \quad \tilde{B}_L = \sum_j Z_{Po,j8}^* f_{Po,j}^0, \quad \text{Fad1} = \sum_j Z_{Po,j9}^* f_{Po,j}^0 \quad (298)$$

$$K_f = \sum_j Z_{Po,j10}^* f_{Po,j}^0 \quad (299)$$

- **Mass matrix for Linking/Ad charged fermion mass eigenstates after AxB breaking ,**

Basis:  $(\chi_{l2}, \chi_{lt2}, \chi_{l3}, \chi_{lt3}, \tilde{B}_L, \tilde{B}_L, \tilde{B}_L, \tilde{B}_L, \text{Fad2}, \text{Fad3}), (\chi_{l2}, \chi_{lt2}, \chi_{l3}, \chi_{lt3}, \tilde{B}_L, \tilde{B}_L, \tilde{B}_L, \tilde{B}_L, \text{Fad2}, \text{Fad3})$

$$m_{f_{Go}^-} = \begin{pmatrix} 0 & 0 & 0 & 0 & m_{51} & m_{61} & m_{71} & m_{81} & 0 & v_{Lv} Y_A \\ 0 & 0 & 0 & 0 & m_{52} & m_{62} & m_{72} & m_{82} & v_{Lv} Y_A & 0 \\ 0 & 0 & 0 & 0 & m_{53} & m_{63} & m_{73} & m_{83} & v_{Lv} Y_A & 0 \\ 0 & 0 & 0 & 0 & m_{54} & m_{64} & m_{74} & m_{84} & 0 & v_{Lv} Y_A \\ m_{51} & m_{52} & m_{53} & m_{54} & m_{55} & m_{65} & 0 & 0 & 0 & 0 \\ m_{61} & m_{62} & m_{63} & m_{64} & m_{65} & m_{66} & 0 & 0 & 0 & 0 \\ m_{71} & m_{72} & m_{73} & m_{74} & 0 & 0 & m_{77} & m_{87} & 0 & 0 \\ m_{81} & m_{82} & m_{83} & m_{84} & 0 & 0 & m_{87} & m_{88} & 0 & 0 \\ 0 & v_{Lv} Y_A & v_{Lv} Y_A & 0 & 0 & 0 & 0 & 0 & 0 & 0 \\ v_{Lv} Y_A & 0 & 0 & v_{Lv} Y_A & 0 & 0 & 0 & 0 & 0 & 0 \end{pmatrix} \quad (300)$$



$$m_{51} = \frac{1}{\sqrt{2}} v_{Lv} \left( g_{A2} \cos \theta_2 - g_{B2} \sin \theta_2 \right) \quad (301)$$

$$m_{52} = \frac{1}{\sqrt{2}} v_{Lv} \left( -g_{A2} \cos \theta_2 + g_{B2} \sin \theta_2 \right) \quad (302)$$

$$m_{53} = \frac{1}{\sqrt{2}} v_{Lv} \left( g_{A2} \cos \theta_2 - g_{B2} \sin \theta_2 \right) \quad (303)$$

$$m_{54} = \frac{1}{\sqrt{2}} v_{Lv} \left( -g_{A2} \cos \theta_2 + g_{B2} \sin \theta_2 \right) \quad (304)$$

$$m_{55} = m_{W_A} \cos^2 \theta_2 + m_{W_B} \sin^2 \theta_2 \quad (305)$$

$$m_{61} = -\frac{1}{\sqrt{2}} v_{Lv} \left( g_{A2} \sin \theta_2 + g_{B2} \cos \theta_2 \right) \quad (306)$$

$$m_{62} = \frac{1}{\sqrt{2}} v_{Lv} \left( g_{A2} \sin \theta_2 + g_{B2} \cos \theta_2 \right) \quad (307)$$

$$m_{63} = -\frac{1}{\sqrt{2}} v_{Lv} \left( g_{A2} \sin \theta_2 + g_{B2} \cos \theta_2 \right) \quad (308)$$

$$m_{64} = \frac{1}{\sqrt{2}} v_{Lv} \left( g_{A2} \sin \theta_2 + g_{B2} \cos \theta_2 \right) \quad (309)$$

$$m_{65} = \left( -m_{W_A} + m_{W_B} \right) \cos \theta_2 \sin \theta_2 \quad (310)$$

$$m_{66} = m_{W_A} \sin^2 \theta_2 + m_{W_B} \cos^2 \theta_2 \quad (311)$$

$$m_{71} = i \frac{1}{\sqrt{2}} v_{Lv} \left( g_{A2} \cos \theta_2 - g_{B2} \sin \theta_2 \right) \quad (312)$$

$$m_{72} = i \frac{1}{\sqrt{2}} v_{Lv} \left( g_{A2} \cos \theta_2 - g_{B2} \sin \theta_2 \right) \quad (313)$$

$$m_{73} = -i \frac{1}{\sqrt{2}} v_{Lv} \left( g_{A2} \cos \theta_2 - g_{B2} \sin \theta_2 \right) \quad (314)$$

$$m_{74} = -i \frac{1}{\sqrt{2}} v_{Lv} \left( g_{A2} \cos \theta_2 - g_{B2} \sin \theta_2 \right) \quad (315)$$

$$m_{77} = m_{W_A} \cos^2 \theta_2 + m_{W_B} \sin^2 \theta_2 \quad (316)$$

$$m_{81} = -i \frac{1}{\sqrt{2}} v_{Lv} \left( g_{A2} \sin \theta_2 + g_{B2} \cos \theta_2 \right) \quad (317)$$

$$m_{82} = -i \frac{1}{\sqrt{2}} v_{Lv} \left( g_{A2} \sin \theta_2 + g_{B2} \cos \theta_2 \right) \quad (318)$$

$$m_{83} = i \frac{1}{\sqrt{2}} v_{Lv} \left( g_{A2} \sin \theta_2 + g_{B2} \cos \theta_2 \right) \quad (319)$$

$$m_{84} = i \frac{1}{\sqrt{2}} v_{Lv} \left( g_{A2} \sin \theta_2 + g_{B2} \cos \theta_2 \right) \quad (320)$$

$$m_{87} = \left( -m_{W_A} + m_{W_B} \right) \cos \theta_2 \sin \theta_2 \quad (321)$$

$$m_{88} = m_{W_A} \sin^2 \theta_2 + m_{W_B} \cos^2 \theta_2 \quad (322)$$

This matrix is diagonalized by  $Z_{Go}$ :

$$Z_{Go}^* m_{f_{Go}^-} Z_{Go}^\dagger = m_{f_{Go}^-}^{dia} \quad (323)$$

with

$$\chi_{l2} = \sum_j Z_{Go,j1}^* f_{Go,j}^+, \quad \chi_{lt2} = \sum_j Z_{Go,j2}^* f_{Go,j}^+, \quad \chi_{l3} = \sum_j Z_{Go,j3}^* f_{Go,j}^+ \quad (324)$$

$$\chi_{lt3} = \sum_j Z_{Go,j4}^* f_{Go,j}^+, \quad \tilde{B}_L = \sum_j Z_{Go,j5}^* f_{Go,j}^+, \quad \tilde{B}_L = \sum_j Z_{Go,j6}^* f_{Go,j}^+ \quad (325)$$

$$\tilde{B}_L = \sum_j Z_{Go,j7}^* f_{Go,j}^+, \quad \tilde{B}_L = \sum_j Z_{Go,j8}^* f_{Go,j}^+, \quad \text{Fad2} = \sum_j Z_{Go,j9}^* f_{Go,j}^+ \quad (326)$$

$$\text{Fad3} = \sum_j Z_{Go,j10}^* f_{Go,j}^+ \quad (327)$$

## 5 Vacuum Expectation Values

$$\varphi_{l1} = i\sigma_{L1} + \phi_{L1} + v_{Lv} \quad (328)$$

$$\varphi_{l4} = i\sigma_{L4} + \phi_{L4} + v_{Lv} \quad (329)$$

$$\tilde{\varphi}_{lt1} = i\sigma_{Lt1} + \phi_{Lt1} + v_{Lv} \quad (330)$$

$$\tilde{\varphi}_{lt4} = i\sigma_{Lt4} + \phi_{Lt4} + v_{Lv} \quad (331)$$

## 6 Tadpole Equations

$$\frac{\partial V}{\partial \phi_{L1}} = \frac{1}{4} v_{Lv} \left( - \left( -4v_{Lv}^2 Y_K + \Omega \right) Y_K^* + 8m_L^2 - \Omega Y_K \right) \quad (332)$$

$$\frac{\partial V}{\partial \phi_{L4}} = \frac{1}{4} v_{Lv} \left( - \left( -4v_{Lv}^2 Y_K + \Omega \right) Y_K^* + 8m_L^2 - \Omega Y_K \right) \quad (333)$$

$$\frac{\partial V}{\partial \phi_{Lt1}} = \frac{1}{4} v_{Lv} \left( - \left( -4v_{Lv}^2 Y_K + \Omega \right) Y_K^* + 8m_L^2 - \Omega Y_K \right) \quad (334)$$

$$\frac{\partial V}{\partial \phi_{Lt4}} = \frac{1}{4} v_{Lv} \left( - \left( -4v_{Lv}^2 Y_K + \Omega \right) Y_K^* + 8m_L^2 - \Omega Y_K \right) \quad (335)$$

## 7 Particle content for eigenstates 'AxBSB'

| Name            | Type   | complex/real | Generations | Indices            |
|-----------------|--------|--------------|-------------|--------------------|
| $\tilde{d}_L$   | Scalar | complex      | 3           | generation, Acolor |
| $\tilde{u}_L$   | Scalar | complex      | 3           | generation, Acolor |
| $\tilde{e}_L$   | Scalar | complex      | 3           | generation         |
| $\tilde{\nu}_L$ | Scalar | complex      | 3           | generation         |

|                 |         |          |    |                    |
|-----------------|---------|----------|----|--------------------|
| $H_d^0$         | Scalar  | complex  | 1  |                    |
| $H_d^-$         | Scalar  | complex  | 1  |                    |
| $H_u^0$         | Scalar  | complex  | 1  |                    |
| $H_u^+$         | Scalar  | complex  | 1  |                    |
| $\tilde{u}_R$   | Scalar  | complex  | 3  | generation, Acolor |
| $\tilde{d}_R$   | Scalar  | complex  | 3  | generation, Acolor |
| $\tilde{e}_R$   | Scalar  | complex  | 3  | generation         |
| $\phi_L^0$      | Scalar  | real     | 4  | generation         |
| $\sigma_L^0$    | Scalar  | real     | 4  | generation         |
| $\sigma_L^\pm$  | Scalar  | complex  | 4  | generation         |
| $\phi_{AK}^s$   | Scalar  | complex  | 2  | generation         |
| $\phi_B^s$      | Scalar  | complex  | 2  | generation         |
| $d_L^D$         | Fermion | Dirac    | 3  | generation, Acolor |
| $u_L^D$         | Fermion | Dirac    | 3  | generation, Acolor |
| $e_L^D$         | Fermion | Dirac    | 3  | generation         |
| $\nu_L^D$       | Fermion | Dirac    | 3  | generation         |
| $\tilde{H}^0$   | Fermion | Dirac    | 1  |                    |
| $\tilde{H}^-$   | Fermion | Dirac    | 1  |                    |
| $u_R^D$         | Fermion | Dirac    | 3  | generation, Acolor |
| $d_R^D$         | Fermion | Dirac    | 3  | generation, Acolor |
| $e_R^D$         | Fermion | Dirac    | 3  | generation         |
| $\tilde{G}_A^D$ | Fermion | Majorana | 1  | adjAcolor          |
| $f_{Po}^0$      | Fermion | Majorana | 10 | generation         |
| $f_{Go}^-$      | Fermion | Majorana | 10 | generation         |
| $g$             | Vector  | real     | 1  | adjAcolor, lorentz |
| $B_L$           | Vector  | real     | 1  | lorentz            |
| $B_H$           | Vector  | real     | 1  | lorentz            |
| $W_L^1$         | Vector  | real     | 1  | lorentz            |
| $W_H^1$         | Vector  | real     | 1  | lorentz            |
| $W_L^2$         | Vector  | real     | 1  | lorentz            |
| $W_H^2$         | Vector  | real     | 1  | lorentz            |
| $W_L^3$         | Vector  | real     | 1  | lorentz            |
| $W_H^3$         | Vector  | real     | 1  | lorentz            |
| $\eta^G$        | Ghost   | real     | 1  | adjAcolor          |
| $\eta B_L$      | Ghost   | real     | 1  |                    |

|              |       |      |   |
|--------------|-------|------|---|
| $\eta B_H$   | Ghost | real | 1 |
| $\eta W_L^1$ | Ghost | real | 1 |
| $\eta W_H^1$ | Ghost | real | 1 |
| $\eta W_L^2$ | Ghost | real | 1 |
| $\eta W_H^2$ | Ghost | real | 1 |
| $\eta W_L^3$ | Ghost | real | 1 |
| $\eta W_H^3$ | Ghost | real | 1 |

## 8 One Loop Self-Energy and One Loop Tadpoles for eigenstates 'AxBSB'

### 8.1 One Loop Self-Energy

- Self-Energy for Linking fields real scalars  $(\phi_L^0)$

$$\begin{aligned}
\Pi_{i,j}(p^2) = & +2B_0(p^2, m_{B_L}^2, m_{B_L}^2) \Gamma_{\check{\phi}^0_L, j, B_L, B_L}^* \Gamma_{\check{\phi}^0_L, i, B_L, B_L} + 4B_0(p^2, m_{B_L}^2, m_{B_H}^2) \Gamma_{\check{\phi}^0_L, j, B_H, B_L}^* \Gamma_{\check{\phi}^0_L, i, B_H, B_L} \\
& + 2B_0(p^2, m_{B_H}^2, m_{B_H}^2) \Gamma_{\check{\phi}^0_L, j, B_H, B_H}^* \Gamma_{\check{\phi}^0_L, i, B_H, B_H} + 2B_0(p^2, m_{W_L^1}^2, m_{W_L^1}^2) \Gamma_{\check{\phi}^0_L, j, W_L^1, W_L^1}^* \Gamma_{\check{\phi}^0_L, i, W_L^1, W_L^1} \\
& + 4B_0(p^2, m_{W_L^1}^2, m_{W_H^1}^2) \Gamma_{\check{\phi}^0_L, j, W_H^1, W_L^1}^* \Gamma_{\check{\phi}^0_L, i, W_H^1, W_L^1} + 2B_0(p^2, m_{W_H^1}^2, m_{W_H^1}^2) \Gamma_{\check{\phi}^0_L, j, W_H^1, W_H^1}^* \Gamma_{\check{\phi}^0_L, i, W_H^1, W_H^1} \\
& + 2B_0(p^2, m_{W_L^2}^2, m_{W_L^2}^2) \Gamma_{\check{\phi}^0_L, j, W_L^2, W_L^2}^* \Gamma_{\check{\phi}^0_L, i, W_L^2, W_L^2} + 4B_0(p^2, m_{W_L^2}^2, m_{W_H^2}^2) \Gamma_{\check{\phi}^0_L, j, W_H^2, W_L^2}^* \Gamma_{\check{\phi}^0_L, i, W_H^2, W_L^2} \\
& + 2B_0(p^2, m_{W_H^2}^2, m_{W_H^2}^2) \Gamma_{\check{\phi}^0_L, j, W_H^2, W_H^2}^* \Gamma_{\check{\phi}^0_L, i, W_H^2, W_H^2} + 4B_0(p^2, m_{B_L}^2, m_{W_L^3}^2) \Gamma_{\check{\phi}^0_L, j, W_L^3, B_L}^* \Gamma_{\check{\phi}^0_L, i, W_L^3, B_L} \\
& + 4B_0(p^2, m_{B_H}^2, m_{W_L^3}^2) \Gamma_{\check{\phi}^0_L, j, W_L^3, B_H}^* \Gamma_{\check{\phi}^0_L, i, W_L^3, B_H} + 2B_0(p^2, m_{W_L^3}^2, m_{W_L^3}^2) \Gamma_{\check{\phi}^0_L, j, W_L^3, W_L^3}^* \Gamma_{\check{\phi}^0_L, i, W_L^3, W_L^3} \\
& + 4B_0(p^2, m_{B_L}^2, m_{W_H^3}^2) \Gamma_{\check{\phi}^0_L, j, W_H^3, B_L}^* \Gamma_{\check{\phi}^0_L, i, W_H^3, B_L} + 4B_0(p^2, m_{B_H}^2, m_{W_H^3}^2) \Gamma_{\check{\phi}^0_L, j, W_H^3, B_H}^* \Gamma_{\check{\phi}^0_L, i, W_H^3, B_H} \\
& + 4B_0(p^2, m_{W_L^3}^2, m_{W_H^3}^2) \Gamma_{\check{\phi}^0_L, j, W_H^3, W_L^3}^* \Gamma_{\check{\phi}^0_L, i, W_H^3, W_L^3} + 2B_0(p^2, m_{W_H^3}^2, m_{W_H^3}^2) \Gamma_{\check{\phi}^0_L, j, W_H^3, W_H^3}^* \Gamma_{\check{\phi}^0_L, i, W_H^3, W_H^3} \\
& - B_0(p^2, m_{\eta B_L}^2, m_{\eta B_L}^2) \Gamma_{\check{\phi}^0_L, j, \eta \bar{B}_L, \eta B_L}^* \Gamma_{\check{\phi}^0_L, i, \eta \bar{B}_L, \eta B_L} - 2B_0(p^2, m_{\eta B_L}^2, m_{\eta B_H}^2) \Gamma_{\check{\phi}^0_L, j, \eta \bar{B}_H, \eta B_L}^* \Gamma_{\check{\phi}^0_L, i, \eta \bar{B}_H, \eta B_L} \\
& - B_0(p^2, m_{\eta B_H}^2, m_{\eta B_H}^2) \Gamma_{\check{\phi}^0_L, j, \eta \bar{B}_H, \eta B_H}^* \Gamma_{\check{\phi}^0_L, i, \eta \bar{B}_H, \eta B_H} - B_0(p^2, m_{\eta W_L^1}^2, m_{\eta W_L^1}^2) \Gamma_{\check{\phi}^0_L, j, \eta \bar{W}_L^1, \eta W_L^1}^* \Gamma_{\check{\phi}^0_L, i, \eta \bar{W}_L^1, \eta W_L^1} \\
& - 2B_0(p^2, m_{\eta W_L^1}^2, m_{\eta W_H^1}^2) \Gamma_{\check{\phi}^0_L, j, \eta \bar{W}_H^1, \eta W_L^1}^* \Gamma_{\check{\phi}^0_L, i, \eta \bar{W}_H^1, \eta W_L^1} - B_0(p^2, m_{\eta W_H^1}^2, m_{\eta W_H^1}^2) \Gamma_{\check{\phi}^0_L, j, \eta \bar{W}_H^1, \eta W_H^1}^* \Gamma_{\check{\phi}^0_L, i, \eta \bar{W}_H^1, \eta W_H^1} \\
& - B_0(p^2, m_{\eta W_L^2}^2, m_{\eta W_L^2}^2) \Gamma_{\check{\phi}^0_L, j, \eta \bar{W}_L^2, \eta W_L^2}^* \Gamma_{\check{\phi}^0_L, i, \eta \bar{W}_L^2, \eta W_L^2} - 2B_0(p^2, m_{\eta W_L^2}^2, m_{\eta W_H^2}^2) \Gamma_{\check{\phi}^0_L, j, \eta \bar{W}_H^2, \eta W_L^2}^* \Gamma_{\check{\phi}^0_L, i, \eta \bar{W}_H^2, \eta W_L^2} \\
& - B_0(p^2, m_{\eta W_H^2}^2, m_{\eta W_H^2}^2) \Gamma_{\check{\phi}^0_L, j, \eta \bar{W}_H^2, \eta W_H^2}^* \Gamma_{\check{\phi}^0_L, i, \eta \bar{W}_H^2, \eta W_H^2} - 2B_0(p^2, m_{\eta B_L}^2, m_{\eta W_L^3}^2) \Gamma_{\check{\phi}^0_L, j, \eta \bar{W}_L^3, \eta B_L}^* \Gamma_{\check{\phi}^0_L, i, \eta \bar{W}_L^3, \eta B_L} \\
& - 2B_0(p^2, m_{\eta B_H}^2, m_{\eta W_L^3}^2) \Gamma_{\check{\phi}^0_L, j, \eta \bar{W}_L^3, \eta B_H}^* \Gamma_{\check{\phi}^0_L, i, \eta \bar{W}_L^3, \eta B_H} - B_0(p^2, m_{\eta W_L^3}^2, m_{\eta W_L^3}^2) \Gamma_{\check{\phi}^0_L, j, \eta \bar{W}_L^3, \eta W_L^3}^* \Gamma_{\check{\phi}^0_L, i, \eta \bar{W}_L^3, \eta W_L^3} \\
& - 2B_0(p^2, m_{\eta B_L}^2, m_{\eta W_H^3}^2) \Gamma_{\check{\phi}^0_L, j, \eta \bar{W}_H^3, \eta B_L}^* \Gamma_{\check{\phi}^0_L, i, \eta \bar{W}_H^3, \eta B_L} - 2B_0(p^2, m_{\eta B_H}^2, m_{\eta W_H^3}^2) \Gamma_{\check{\phi}^0_L, j, \eta \bar{W}_H^3, \eta B_H}^* \Gamma_{\check{\phi}^0_L, i, \eta \bar{W}_H^3, \eta B_H}
\end{aligned}$$

$$\begin{aligned}
& -2B_0\left(p^2, m_{\eta W_L^3}^2, m_{\eta W_H^3}^2\right) \Gamma_{\check{\phi}^{0L,j}, \eta \bar{W}_H^3, \eta W_L^3}^* \Gamma_{\check{\phi}^{0L,i}, \eta \bar{W}_H^3, \eta W_L^3} - B_0\left(p^2, m_{\eta W_H^3}^2, m_{\eta W_H^3}^2\right) \Gamma_{\check{\phi}^{0L,j}, \eta \bar{W}_H^3, \eta W_H^3}^* \Gamma_{\check{\phi}^{0L,i}, \eta \bar{W}_H^3, \eta W_H^3} \\
& + B_0\left(p^2, m_{H_d^0}^2, m_{H_d^0}^2\right) \Gamma_{\check{\phi}^{0L,j}, H_d^{0,*}, H_d^0}^* \Gamma_{\check{\phi}^{0L,i}, H_d^{0,*}, H_d^0} + B_0\left(p^2, m_{H_d^-}^2, m_{H_d^-}^2\right) \Gamma_{\check{\phi}^{0L,j}, H_d^{-,*}, H_d^-}^* \Gamma_{\check{\phi}^{0L,i}, H_d^{-,*}, H_d^-} \\
& + B_0\left(p^2, m_{H_u^0}^2, m_{H_u^0}^2\right) \Gamma_{\check{\phi}^{0L,j}, H_u^{0,*}, H_u^0}^* \Gamma_{\check{\phi}^{0L,i}, H_u^{0,*}, H_u^0} + B_0\left(p^2, m_{H_u^+}^2, m_{H_u^+}^2\right) \Gamma_{\check{\phi}^{0L,j}, H_u^{+,*}, H_u^+}^* \Gamma_{\check{\phi}^{0L,i}, H_u^{+,*}, H_u^+} \\
& + 2A_0\left(m_{B_L}^2\right) \Gamma_{\check{\phi}^{0L,i}, \check{\phi}^{0L,i}, B_L, B_L} + 2A_0\left(m_{B_H}^2\right) \Gamma_{\check{\phi}^{0L,i}, \check{\phi}^{0L,i}, B_H, B_H} + 2A_0\left(m_{W_L^1}^2\right) \Gamma_{\check{\phi}^{0L,i}, \check{\phi}^{0L,i}, W_L^1, W_L^1} \\
& + 2A_0\left(m_{W_H^1}^2\right) \Gamma_{\check{\phi}^{0L,i}, \check{\phi}^{0L,i}, W_H^1, W_H^1} + 2A_0\left(m_{W_L^2}^2\right) \Gamma_{\check{\phi}^{0L,i}, \check{\phi}^{0L,i}, W_L^2, W_L^2} + 2A_0\left(m_{W_H^2}^2\right) \Gamma_{\check{\phi}^{0L,i}, \check{\phi}^{0L,i}, W_H^2, W_H^2} \\
& + 2A_0\left(m_{W_L^3}^2\right) \Gamma_{\check{\phi}^{0L,i}, \check{\phi}^{0L,i}, W_L^3, W_L^3} + 2A_0\left(m_{W_H^3}^2\right) \Gamma_{\check{\phi}^{0L,i}, \check{\phi}^{0L,i}, W_H^3, W_H^3} - A_0\left(m_{H_d^0}^2\right) \Gamma_{\check{\phi}^{0L,i}, \check{\phi}^{0L,i}, H_d^{0,*}, H_d^0} \\
& - A_0\left(m_{H_d^-}^2\right) \Gamma_{\check{\phi}^{0L,i}, \check{\phi}^{0L,i}, H_d^{-,*}, H_d^-} - A_0\left(m_{H_u^0}^2\right) \Gamma_{\check{\phi}^{0L,i}, \check{\phi}^{0L,i}, H_u^{0,*}, H_u^0} - A_0\left(m_{H_u^+}^2\right) \Gamma_{\check{\phi}^{0L,i}, \check{\phi}^{0L,i}, H_u^{+,*}, H_u^+} \\
& - \sum_{a=1}^2 A_0\left(m_{\phi_{B,a}^s}^2\right) \Gamma_{\check{\phi}^{0L,i}, \check{\phi}^{0L,i}, \phi_{B,a}^{s,*}, \phi_{B,a}^s} - \sum_{a=1}^2 A_0\left(m_{\phi_{AK,a}^s}^2\right) \Gamma_{\check{\phi}^{0L,i}, \check{\phi}^{0L,i}, \phi_{AK,a}^{s,*}, \phi_{AK,a}^s} \\
& + \sum_{a=1}^2 \sum_{b=1}^2 B_0\left(p^2, m_{\phi_{B,a}^s}^2, m_{\phi_{B,b}^s}^2\right) \Gamma_{\check{\phi}^{0L,j}, \phi_{B,a}^{s,*}, \phi_{B,b}^s}^* \Gamma_{\check{\phi}^{0L,i}, \phi_{B,a}^{s,*}, \phi_{B,b}^s} \\
& + \sum_{a=1}^2 \sum_{b=1}^2 B_0\left(p^2, m_{\phi_{AK,a}^s}^2, m_{\phi_{AK,b}^s}^2\right) \Gamma_{\check{\phi}^{0L,j}, \phi_{AK,a}^{s,*}, \phi_{AK,b}^s}^* \Gamma_{\check{\phi}^{0L,i}, \phi_{AK,a}^{s,*}, \phi_{AK,b}^s} \\
& + 2 \sum_{a=1}^2 \sum_{b=1}^4 B_0\left(p^2, m_{\phi_{AK,a}^s}^2, m_{\phi_{L,b}^0}^2\right) \Gamma_{\check{\phi}^{0L,j}, \phi_{AK,a}^{s,*}, \phi_{L,b}^0}^* \Gamma_{\check{\phi}^{0L,i}, \phi_{AK,a}^{s,*}, \phi_{L,b}^0} \\
& - 3 \sum_{a=1}^3 A_0\left(m_{\tilde{d}_{L,a}}^2\right) \Gamma_{\check{\phi}^{0L,i}, \check{\phi}^{0L,i}, \tilde{d}_{L,a}^*, \tilde{d}_{L,a}} - 3 \sum_{a=1}^3 A_0\left(m_{\tilde{d}_{R,a}}^2\right) \Gamma_{\check{\phi}^{0L,i}, \check{\phi}^{0L,i}, \tilde{d}_{R,a}^*, \tilde{d}_{R,a}} \\
& - \sum_{a=1}^3 A_0\left(m_{\tilde{e}_{L,a}}^2\right) \Gamma_{\check{\phi}^{0L,i}, \check{\phi}^{0L,i}, \tilde{e}_{L,a}^*, \tilde{e}_{L,a}} - \sum_{a=1}^3 A_0\left(m_{\tilde{e}_{R,a}}^2\right) \Gamma_{\check{\phi}^{0L,i}, \check{\phi}^{0L,i}, \tilde{e}_{R,a}^*, \tilde{e}_{R,a}} \\
& - 3 \sum_{a=1}^3 A_0\left(m_{\tilde{u}_{L,a}}^2\right) \Gamma_{\check{\phi}^{0L,i}, \check{\phi}^{0L,i}, \tilde{u}_{L,a}^*, \tilde{u}_{L,a}} - 3 \sum_{a=1}^3 A_0\left(m_{\tilde{u}_{R,a}}^2\right) \Gamma_{\check{\phi}^{0L,i}, \check{\phi}^{0L,i}, \tilde{u}_{R,a}^*, \tilde{u}_{R,a}} \\
& - \sum_{a=1}^3 A_0\left(m_{\tilde{\nu}_{L,a}}^2\right) \Gamma_{\check{\phi}^{0L,i}, \check{\phi}^{0L,i}, \tilde{\nu}_{L,a}^*, \tilde{\nu}_{L,a}} + 3 \sum_{a=1}^3 \sum_{b=1}^3 B_0\left(p^2, m_{\tilde{d}_{L,a}}^2, m_{\tilde{d}_{L,b}}^2\right) \Gamma_{\check{\phi}^{0L,j}, \tilde{d}_{L,a}^*, \tilde{d}_{L,b}}^* \Gamma_{\check{\phi}^{0L,i}, \tilde{d}_{L,a}^*, \tilde{d}_{L,b}} \\
& + 3 \sum_{a=1}^3 \sum_{b=1}^3 B_0\left(p^2, m_{\tilde{d}_{R,a}}^2, m_{\tilde{d}_{R,b}}^2\right) \Gamma_{\check{\phi}^{0L,j}, \tilde{d}_{R,a}^*, \tilde{d}_{R,b}}^* \Gamma_{\check{\phi}^{0L,i}, \tilde{d}_{R,a}^*, \tilde{d}_{R,b}} \\
& + \sum_{a=1}^3 \sum_{b=1}^3 B_0\left(p^2, m_{\tilde{e}_{L,a}}^2, m_{\tilde{e}_{L,b}}^2\right) \Gamma_{\check{\phi}^{0L,j}, \tilde{e}_{L,a}^*, \tilde{e}_{L,b}}^* \Gamma_{\check{\phi}^{0L,i}, \tilde{e}_{L,a}^*, \tilde{e}_{L,b}} \\
& + \sum_{a=1}^3 \sum_{b=1}^3 B_0\left(p^2, m_{\tilde{e}_{R,a}}^2, m_{\tilde{e}_{R,b}}^2\right) \Gamma_{\check{\phi}^{0L,j}, \tilde{e}_{R,a}^*, \tilde{e}_{R,b}}^* \Gamma_{\check{\phi}^{0L,i}, \tilde{e}_{R,a}^*, \tilde{e}_{R,b}}
\end{aligned}$$

$$\begin{aligned}
& + 3 \sum_{a=1}^3 \sum_{b=1}^3 B_0 \left( p^2, m_{\tilde{u}_{L,a}}^2, m_{\tilde{u}_{L,b}}^2 \right) \Gamma_{\check{\phi}^0_{L,j}, \tilde{u}_{L,a}^*, \tilde{u}_{L,b}}^* \Gamma_{\check{\phi}^0_{L,i}, \tilde{u}_{L,a}^*, \tilde{u}_{L,b}} \\
& + 3 \sum_{a=1}^3 \sum_{b=1}^3 B_0 \left( p^2, m_{\tilde{u}_{R,a}}^2, m_{\tilde{u}_{R,b}}^2 \right) \Gamma_{\check{\phi}^0_{L,j}, \tilde{u}_{R,a}^*, \tilde{u}_{R,b}}^* \Gamma_{\check{\phi}^0_{L,i}, \tilde{u}_{R,a}^*, \tilde{u}_{R,b}} \\
& + \sum_{a=1}^3 \sum_{b=1}^3 B_0 \left( p^2, m_{\tilde{\nu}_{L,a}}^2, m_{\tilde{\nu}_{L,b}}^2 \right) \Gamma_{\check{\phi}^0_{L,j}, \tilde{\nu}_{L,a}^*, \tilde{\nu}_{L,b}}^* \Gamma_{\check{\phi}^0_{L,i}, \tilde{\nu}_{L,a}^*, \tilde{\nu}_{L,b}} - \sum_{a=1}^4 A_0 \left( m_{\sigma_{L,a}^\pm}^2 \right) \Gamma_{\check{\phi}^0_{L,i}, \check{\phi}^0_{L,i}, \sigma_{L,a}^{\pm,*}, \sigma_{L,a}^\pm} \\
& - \frac{1}{2} \sum_{a=1}^4 A_0 \left( m_{\phi_{L,a}^0}^2 \right) \Gamma_{\check{\phi}^0_{L,i}, \check{\phi}^0_{L,i}, \phi_{L,a}^0, \phi_{L,a}^0} - \frac{1}{2} \sum_{a=1}^4 A_0 \left( m_{\sigma_{L,a}^0}^2 \right) \Gamma_{\check{\phi}^0_{L,i}, \check{\phi}^0_{L,i}, \sigma_{L,a}^0, \sigma_{L,a}^0} \\
& + 2 \sum_{a=1}^4 \sum_{b=1}^2 B_0 \left( p^2, m_{\sigma_{L,a}^\pm}^2, m_{\phi_{B,b}^s}^2 \right) \Gamma_{\check{\phi}^0_{L,j}, \sigma_{L,a}^{\pm,*}, \phi_{B,b}^s}^* \Gamma_{\check{\phi}^0_{L,i}, \sigma_{L,a}^{\pm,*}, \phi_{B,b}^s} \\
& + 2 \sum_{a=1}^4 \sum_{b=1}^2 B_0 \left( p^2, m_{\sigma_{L,a}^0}^2, m_{\phi_{AK,b}^s}^2 \right) \Gamma_{\check{\phi}^0_{L,j}, \sigma_{L,a}^0, \phi_{AK,b}^s}^* \Gamma_{\check{\phi}^0_{L,i}, \sigma_{L,a}^0, \phi_{AK,b}^s} \\
& + \sum_{a=1}^4 \sum_{b=1}^4 B_0 \left( p^2, m_{\sigma_{L,a}^\pm}^2, m_{\sigma_{L,b}^\pm}^2 \right) \Gamma_{\check{\phi}^0_{L,j}, \sigma_{L,a}^{\pm,*}, \sigma_{L,b}^\pm}^* \Gamma_{\check{\phi}^0_{L,i}, \sigma_{L,a}^{\pm,*}, \sigma_{L,b}^\pm} \\
& + \frac{1}{2} \sum_{a=1}^4 \sum_{b=1}^4 B_0 \left( p^2, m_{\phi_{L,a}^0}^2, m_{\phi_{L,b}^0}^2 \right) \Gamma_{\check{\phi}^0_{L,j}, \phi_{L,a}^0, \phi_{L,b}^0}^* \Gamma_{\check{\phi}^0_{L,i}, \phi_{L,a}^0, \phi_{L,b}^0} \\
& + \frac{1}{2} \sum_{a=1}^4 \sum_{b=1}^4 B_0 \left( p^2, m_{\sigma_{L,a}^0}^2, m_{\sigma_{L,b}^0}^2 \right) \Gamma_{\check{\phi}^0_{L,j}, \sigma_{L,a}^0, \sigma_{L,b}^0}^* \Gamma_{\check{\phi}^0_{L,i}, \sigma_{L,a}^0, \sigma_{L,b}^0} \\
& - \sum_{a=1}^{10} m_{f_{Go,a}^-} \sum_{b=1}^{10} B_0 \left( p^2, m_{f_{Go,a}^-}^2, m_{f_{Go,b}^-}^2 \right) m_{f_{Go,b}^-} \left( \Gamma_{\check{\phi}^0_{L,j}, f_{Go,a}^-, f_{Go,b}^-}^{L*} \Gamma_{\check{\phi}^0_{L,i}, f_{Go,a}^-, f_{Go,b}^-}^R + \Gamma_{\check{\phi}^0_{L,j}, f_{Go,a}^-, f_{Go,b}^-}^{R*} \Gamma_{\check{\phi}^0_{L,i}, f_{Go,a}^-, f_{Go,b}^-}^L \right) \\
& + \frac{1}{2} \sum_{a=1}^{10} \sum_{b=1}^{10} G_0 \left( p^2, m_{f_{Go,a}^-}^2, m_{f_{Go,b}^-}^2 \right) \left( \Gamma_{\check{\phi}^0_{L,j}, f_{Go,a}^-, f_{Go,b}^-}^{L*} \Gamma_{\check{\phi}^0_{L,i}, f_{Go,a}^-, f_{Go,b}^-}^L + \Gamma_{\check{\phi}^0_{L,j}, f_{Go,a}^-, f_{Go,b}^-}^{R*} \Gamma_{\check{\phi}^0_{L,i}, f_{Go,a}^-, f_{Go,b}^-}^R \right) \\
& - \sum_{a=1}^{10} m_{f_{Po,a}^0} \sum_{b=1}^{10} B_0 \left( p^2, m_{f_{Po,a}^0}^2, m_{f_{Po,b}^0}^2 \right) m_{f_{Po,b}^0} \left( \Gamma_{\check{\phi}^0_{L,j}, f_{Po,a}^0, f_{Po,b}^0}^{L*} \Gamma_{\check{\phi}^0_{L,i}, f_{Po,a}^0, f_{Po,b}^0}^R + \Gamma_{\check{\phi}^0_{L,j}, f_{Po,a}^0, f_{Po,b}^0}^{R*} \Gamma_{\check{\phi}^0_{L,i}, f_{Po,a}^0, f_{Po,b}^0}^L \right) \\
& + \frac{1}{2} \sum_{a=1}^{10} \sum_{b=1}^{10} G_0 \left( p^2, m_{f_{Po,a}^0}^2, m_{f_{Po,b}^0}^2 \right) \left( \Gamma_{\check{\phi}^0_{L,j}, f_{Po,a}^0, f_{Po,b}^0}^{L*} \Gamma_{\check{\phi}^0_{L,i}, f_{Po,a}^0, f_{Po,b}^0}^L + \Gamma_{\check{\phi}^0_{L,j}, f_{Po,a}^0, f_{Po,b}^0}^{R*} \Gamma_{\check{\phi}^0_{L,i}, f_{Po,a}^0, f_{Po,b}^0}^R \right) \\
& + 2 \sum_{b=1}^4 \Gamma_{\check{\phi}^0_{L,j}, W_{L,b}^1, \sigma_{L,b}^\pm}^* \Gamma_{\check{\phi}^0_{L,i}, W_{L,b}^1, \sigma_{L,b}^\pm} F_0 \left( p^2, m_{\sigma_{L,b}^\pm}^2, m_{W_{L,b}^1}^2 \right) \\
& + 2 \sum_{b=1}^4 \Gamma_{\check{\phi}^0_{L,j}, W_{H,b}^1, \sigma_{L,b}^\pm}^* \Gamma_{\check{\phi}^0_{L,i}, W_{H,b}^1, \sigma_{L,b}^\pm} F_0 \left( p^2, m_{\sigma_{L,b}^\pm}^2, m_{W_{H,b}^1}^2 \right)
\end{aligned}$$

$$\begin{aligned}
& + 2 \sum_{b=1}^4 \Gamma_{\check{\phi}^0_{L,j}, W_L^2, \sigma_{L,b}^\pm}^* \Gamma_{\check{\phi}^0_{L,i}, W_L^2, \sigma_{L,b}^\pm} F_0(p^2, m_{\sigma_{L,b}^\pm}^2, m_{W_L^2}^2) \\
& + 2 \sum_{b=1}^4 \Gamma_{\check{\phi}^0_{L,j}, W_H^2, \sigma_{L,b}^\pm}^* \Gamma_{\check{\phi}^0_{L,i}, W_H^2, \sigma_{L,b}^\pm} F_0(p^2, m_{\sigma_{L,b}^\pm}^2, m_{W_H^2}^2) \\
& + \sum_{b=1}^4 \Gamma_{\check{\phi}^0_{L,j}, B_L, \sigma_{L,b}^0}^* \Gamma_{\check{\phi}^0_{L,i}, B_L, \sigma_{L,b}^0} F_0(p^2, m_{\sigma_{L,b}^0}^2, m_{B_L}^2) + \sum_{b=1}^4 \Gamma_{\check{\phi}^0_{L,j}, B_H, \sigma_{L,b}^0}^* \Gamma_{\check{\phi}^0_{L,i}, B_H, \sigma_{L,b}^0} F_0(p^2, m_{\sigma_{L,b}^0}^2, m_{B_H}^2) \\
& + \sum_{b=1}^4 \Gamma_{\check{\phi}^0_{L,j}, W_L^3, \sigma_{L,b}^0}^* \Gamma_{\check{\phi}^0_{L,i}, W_L^3, \sigma_{L,b}^0} F_0(p^2, m_{\sigma_{L,b}^0}^2, m_{W_L^3}^2) \\
& + \sum_{b=1}^4 \Gamma_{\check{\phi}^0_{L,j}, W_H^3, \sigma_{L,b}^0}^* \Gamma_{\check{\phi}^0_{L,i}, W_H^3, \sigma_{L,b}^0} F_0(p^2, m_{\sigma_{L,b}^0}^2, m_{W_H^3}^2) \tag{336}
\end{aligned}$$

• Self-Energy for Heavy B gauge boson ( $\sigma_L^0$ )

$$\begin{aligned}
\Pi_{i,j}(p^2) = & +4B_0(p^2, m_{W_H^1}^2, m_{W_L^2}^2) \Gamma_{\check{\sigma}^0_{L,j}, W_L^2, W_H^1}^* \Gamma_{\check{\sigma}^0_{L,i}, W_L^2, W_H^1} + 4B_0(p^2, m_{W_L^1}^2, m_{W_H^2}^2) \Gamma_{\check{\sigma}^0_{L,j}, W_H^2, W_L^1}^* \Gamma_{\check{\sigma}^0_{L,i}, W_H^2, W_L^1} \\
& - 2B_0(p^2, m_{\eta_{W_H^1}^2}^2, m_{\eta_{W_L^2}^2}^2) \Gamma_{\check{\sigma}^0_{L,j}, \eta_{W_L^2}, \eta_{W_H^1}}^* \Gamma_{\check{\sigma}^0_{L,i}, \eta_{W_L^2}, \eta_{W_H^1}} - 2B_0(p^2, m_{\eta_{W_L^1}^2}^2, m_{\eta_{W_H^2}^2}^2) \Gamma_{\check{\sigma}^0_{L,j}, \eta_{W_H^2}, \eta_{W_L^1}}^* \Gamma_{\check{\sigma}^0_{L,i}, \eta_{W_H^2}, \eta_{W_L^1}} \\
& - 2B_0(p^2, m_{\eta_{W_H^1}^2}^2, m_{\eta_{W_H^2}^2}^2) \Gamma_{\check{\sigma}^0_{L,j}, \eta_{W_H^2}, \eta_{W_H^1}}^* \Gamma_{\check{\sigma}^0_{L,i}, \eta_{W_H^2}, \eta_{W_H^1}} + 2A_0(m_{B_L}^2) \Gamma_{\check{\sigma}^0_{L,i}, \check{\sigma}^0_{L,i}, B_L, B_L} \\
& + 2A_0(m_{B_H}^2) \Gamma_{\check{\sigma}^0_{L,i}, \check{\sigma}^0_{L,i}, B_H, B_H} + 2A_0(m_{W_L^1}^2) \Gamma_{\check{\sigma}^0_{L,i}, \check{\sigma}^0_{L,i}, W_L^1, W_L^1} + 2A_0(m_{W_H^1}^2) \Gamma_{\check{\sigma}^0_{L,i}, \check{\sigma}^0_{L,i}, W_H^1, W_H^1} \\
& + 2A_0(m_{W_L^2}^2) \Gamma_{\check{\sigma}^0_{L,i}, \check{\sigma}^0_{L,i}, W_L^2, W_L^2} + 2A_0(m_{W_H^2}^2) \Gamma_{\check{\sigma}^0_{L,i}, \check{\sigma}^0_{L,i}, W_H^2, W_H^2} + 2A_0(m_{W_L^3}^2) \Gamma_{\check{\sigma}^0_{L,i}, \check{\sigma}^0_{L,i}, W_L^3, W_L^3} \\
& + 2A_0(m_{W_H^3}^2) \Gamma_{\check{\sigma}^0_{L,i}, \check{\sigma}^0_{L,i}, W_H^3, W_H^3} - A_0(m_{H_d^0}^2) \Gamma_{\check{\sigma}^0_{L,i}, \check{\sigma}^0_{L,i}, H_d^0, H_d^0} - A_0(m_{H_d^-}^2) \Gamma_{\check{\sigma}^0_{L,i}, \check{\sigma}^0_{L,i}, H_d^-, H_d^-} \\
& - A_0(m_{H_u^0}^2) \Gamma_{\check{\sigma}^0_{L,i}, \check{\sigma}^0_{L,i}, H_u^0, H_u^0} - A_0(m_{H_u^+}^2) \Gamma_{\check{\sigma}^0_{L,i}, \check{\sigma}^0_{L,i}, H_u^+, H_u^+} \\
& - \sum_{a=1}^2 A_0(m_{\phi_{B,a}^s}^2) \Gamma_{\check{\sigma}^0_{L,i}, \check{\sigma}^0_{L,i}, \phi_{B,a}^{s,*}, \phi_{B,a}^s} - \sum_{a=1}^2 A_0(m_{\phi_{AK,a}^s}^2) \Gamma_{\check{\sigma}^0_{L,i}, \check{\sigma}^0_{L,i}, \phi_{AK,a}^{s,*}, \phi_{AK,a}^s} \\
& + 2 \sum_{a=1}^2 \sum_{b=1}^4 B_0(p^2, m_{\phi_{AK,a}^s}^2, m_{\phi_{L,b}^0}^2) \Gamma_{\check{\sigma}^0_{L,j}, \phi_{AK,a}^{s,*}, \phi_{L,b}^0}^* \Gamma_{\check{\sigma}^0_{L,i}, \phi_{AK,a}^{s,*}, \phi_{L,b}^0} \\
& - 3 \sum_{a=1}^3 A_0(m_{\tilde{d}_{L,a}}^2) \Gamma_{\check{\sigma}^0_{L,i}, \check{\sigma}^0_{L,i}, \tilde{d}_{L,a}^*, \tilde{d}_{L,a}} - 3 \sum_{a=1}^3 A_0(m_{\tilde{d}_{R,a}}^2) \Gamma_{\check{\sigma}^0_{L,i}, \check{\sigma}^0_{L,i}, \tilde{d}_{R,a}^*, \tilde{d}_{R,a}} \\
& - \sum_{a=1}^3 A_0(m_{\tilde{e}_{L,a}}^2) \Gamma_{\check{\sigma}^0_{L,i}, \check{\sigma}^0_{L,i}, \tilde{e}_{L,a}^*, \tilde{e}_{L,a}} - \sum_{a=1}^3 A_0(m_{\tilde{e}_{R,a}}^2) \Gamma_{\check{\sigma}^0_{L,i}, \check{\sigma}^0_{L,i}, \tilde{e}_{R,a}^*, \tilde{e}_{R,a}} \\
& - 3 \sum_{a=1}^3 A_0(m_{\tilde{u}_{L,a}}^2) \Gamma_{\check{\sigma}^0_{L,i}, \check{\sigma}^0_{L,i}, \tilde{u}_{L,a}^*, \tilde{u}_{L,a}} - 3 \sum_{a=1}^3 A_0(m_{\tilde{u}_{R,a}}^2) \Gamma_{\check{\sigma}^0_{L,i}, \check{\sigma}^0_{L,i}, \tilde{u}_{R,a}^*, \tilde{u}_{R,a}}
\end{aligned}$$

$$\begin{aligned}
& - \sum_{a=1}^3 A_0 \left( m_{\tilde{\nu}_{L,a}}^2 \right) \Gamma_{\tilde{\sigma}^0_{L,i}, \tilde{\sigma}^0_{L,i}, \tilde{\nu}_{L,a}^*, \tilde{\nu}_{L,a}} - \sum_{a=1}^4 A_0 \left( m_{\sigma_{L,a}^\pm}^2 \right) \Gamma_{\tilde{\sigma}^0_{L,i}, \tilde{\sigma}^0_{L,i}, \sigma_{L,a}^\pm, \sigma_{L,a}^\pm} \\
& - \frac{1}{2} \sum_{a=1}^4 A_0 \left( m_{\phi_{L,a}^0}^2 \right) \Gamma_{\tilde{\sigma}^0_{L,i}, \tilde{\sigma}^0_{L,i}, \phi_{L,a}^0, \phi_{L,a}^0} - \frac{1}{2} \sum_{a=1}^4 A_0 \left( m_{\sigma_{L,a}^0}^2 \right) \Gamma_{\tilde{\sigma}^0_{L,i}, \tilde{\sigma}^0_{L,i}, \sigma_{L,a}^0, \sigma_{L,a}^0} \\
& + 2 \sum_{a=1}^4 \sum_{b=1}^2 B_0 \left( p^2, m_{\sigma_{L,a}^\pm}^2, m_{\phi_{B,b}^s}^2 \right) \Gamma_{\tilde{\sigma}^0_{L,j}, \sigma_{L,a}^\pm, \phi_{B,b}^s}^* \Gamma_{\tilde{\sigma}^0_{L,i}, \sigma_{L,a}^\pm, \phi_{B,b}^s} \\
& + 2 \sum_{a=1}^4 \sum_{b=1}^2 B_0 \left( p^2, m_{\sigma_{L,a}^0}^2, m_{\phi_{AK,b}^s}^2 \right) \Gamma_{\tilde{\sigma}^0_{L,j}, \sigma_{L,a}^0, \phi_{AK,b}^s}^* \Gamma_{\tilde{\sigma}^0_{L,i}, \sigma_{L,a}^0, \phi_{AK,b}^s} \\
& + \sum_{a=1}^4 \sum_{b=1}^4 B_0 \left( p^2, m_{\sigma_{L,a}^\pm}^2, m_{\sigma_{L,b}^\pm}^2 \right) \Gamma_{\tilde{\sigma}^0_{L,j}, \sigma_{L,a}^\pm, \sigma_{L,b}^\pm}^* \Gamma_{\tilde{\sigma}^0_{L,i}, \sigma_{L,a}^\pm, \sigma_{L,b}^\pm} \\
& + \sum_{a=1}^4 \sum_{b=1}^4 B_0 \left( p^2, m_{\sigma_{L,a}^0}^2, m_{\phi_{L,b}^0}^2 \right) \Gamma_{\tilde{\sigma}^0_{L,j}, \sigma_{L,a}^0, \phi_{L,b}^0}^* \Gamma_{\tilde{\sigma}^0_{L,i}, \sigma_{L,a}^0, \phi_{L,b}^0} \\
& - \sum_{a=1}^{10} m_{f_{Go,a}^-} \sum_{b=1}^{10} B_0 \left( p^2, m_{f_{Go,a}^-}^2, m_{f_{Go,b}^-}^2 \right) m_{f_{Go,b}^-} \left( \Gamma_{\tilde{\sigma}^0_{L,j}, f_{Go,a}^-, f_{Go,b}^-}^{L*} \Gamma_{\tilde{\sigma}^0_{L,i}, f_{Go,a}^-, f_{Go,b}^-}^R + \Gamma_{\tilde{\sigma}^0_{L,j}, f_{Go,a}^-, f_{Go,b}^-}^{R*} \Gamma_{\tilde{\sigma}^0_{L,i}, f_{Go,a}^-, f_{Go,b}^-}^L \right) \\
& + \frac{1}{2} \sum_{a=1}^{10} \sum_{b=1}^{10} G_0 \left( p^2, m_{f_{Go,a}^-}^2, m_{f_{Go,b}^-}^2 \right) \left( \Gamma_{\tilde{\sigma}^0_{L,j}, f_{Go,a}^-, f_{Go,b}^-}^{L*} \Gamma_{\tilde{\sigma}^0_{L,i}, f_{Go,a}^-, f_{Go,b}^-}^L + \Gamma_{\tilde{\sigma}^0_{L,j}, f_{Go,a}^-, f_{Go,b}^-}^{R*} \Gamma_{\tilde{\sigma}^0_{L,i}, f_{Go,a}^-, f_{Go,b}^-}^R \right) \\
& - \sum_{a=1}^{10} m_{f_{Po,a}^0} \sum_{b=1}^{10} B_0 \left( p^2, m_{f_{Po,a}^0}^2, m_{f_{Po,b}^0}^2 \right) m_{f_{Po,b}^0} \left( \Gamma_{\tilde{\sigma}^0_{L,j}, f_{Po,a}^0, f_{Po,b}^0}^{L*} \Gamma_{\tilde{\sigma}^0_{L,i}, f_{Po,a}^0, f_{Po,b}^0}^R + \Gamma_{\tilde{\sigma}^0_{L,j}, f_{Po,a}^0, f_{Po,b}^0}^{R*} \Gamma_{\tilde{\sigma}^0_{L,i}, f_{Po,a}^0, f_{Po,b}^0}^L \right) \\
& + \frac{1}{2} \sum_{a=1}^{10} \sum_{b=1}^{10} G_0 \left( p^2, m_{f_{Po,a}^0}^2, m_{f_{Po,b}^0}^2 \right) \left( \Gamma_{\tilde{\sigma}^0_{L,j}, f_{Po,a}^0, f_{Po,b}^0}^{L*} \Gamma_{\tilde{\sigma}^0_{L,i}, f_{Po,a}^0, f_{Po,b}^0}^L + \Gamma_{\tilde{\sigma}^0_{L,j}, f_{Po,a}^0, f_{Po,b}^0}^{R*} \Gamma_{\tilde{\sigma}^0_{L,i}, f_{Po,a}^0, f_{Po,b}^0}^R \right) \\
& + 2 \sum_{b=1}^4 \Gamma_{\tilde{\sigma}^0_{L,j}, W_L^1, \sigma_{L,b}^\pm}^* \Gamma_{\tilde{\sigma}^0_{L,i}, W_L^1, \sigma_{L,b}^\pm} F_0 \left( p^2, m_{\sigma_{L,b}^\pm}^2, m_{W_L^1}^2 \right) \\
& + 2 \sum_{b=1}^4 \Gamma_{\tilde{\sigma}^0_{L,j}, W_H^1, \sigma_{L,b}^\pm}^* \Gamma_{\tilde{\sigma}^0_{L,i}, W_H^1, \sigma_{L,b}^\pm} F_0 \left( p^2, m_{\sigma_{L,b}^\pm}^2, m_{W_H^1}^2 \right) \\
& + 2 \sum_{b=1}^4 \Gamma_{\tilde{\sigma}^0_{L,j}, W_L^2, \sigma_{L,b}^\pm}^* \Gamma_{\tilde{\sigma}^0_{L,i}, W_L^2, \sigma_{L,b}^\pm} F_0 \left( p^2, m_{\sigma_{L,b}^\pm}^2, m_{W_L^2}^2 \right) \\
& + 2 \sum_{b=1}^4 \Gamma_{\tilde{\sigma}^0_{L,j}, W_H^2, \sigma_{L,b}^\pm}^* \Gamma_{\tilde{\sigma}^0_{L,i}, W_H^2, \sigma_{L,b}^\pm} F_0 \left( p^2, m_{\sigma_{L,b}^\pm}^2, m_{W_H^2}^2 \right) \\
& + \sum_{b=1}^4 \Gamma_{\tilde{\sigma}^0_{L,j}, B_L, \phi_{L,b}^0}^* \Gamma_{\tilde{\sigma}^0_{L,i}, B_L, \phi_{L,b}^0} F_0 \left( p^2, m_{\phi_{L,b}^0}^2, m_{B_L}^2 \right) + \sum_{b=1}^4 \Gamma_{\tilde{\sigma}^0_{L,j}, B_H, \phi_{L,b}^0}^* \Gamma_{\tilde{\sigma}^0_{L,i}, B_H, \phi_{L,b}^0} F_0 \left( p^2, m_{\phi_{L,b}^0}^2, m_{B_H}^2 \right)
\end{aligned}$$



$$\begin{aligned}
& + \sum_{b=1}^4 \Gamma_{\tilde{\sigma}^0_{L,j}, W_L^3, \phi_{L,b}^0}^* \Gamma_{\tilde{\sigma}^0_{L,i}, W_L^3, \phi_{L,b}^0} F_0(p^2, m_{\phi_{L,b}^0}^2, m_{W_L^3}^2) \\
& + \sum_{b=1}^4 \Gamma_{\tilde{\sigma}^0_{L,j}, W_H^3, \phi_{L,b}^0}^* \Gamma_{\tilde{\sigma}^0_{L,i}, W_H^3, \phi_{L,b}^0} F_0(p^2, m_{\phi_{L,b}^0}^2, m_{W_H^3}^2)
\end{aligned} \tag{337}$$

- **Self-Energy for Linking fields charged scalars** ( $\sigma_L^\pm$ )

[illegible]

$$\begin{aligned}
& + B_0 \left( p^2, m_{H_d^-}^2, m_{H_d^0}^2 \right) \Gamma_{\check{\sigma}^\pm, *L, j, H_d^-, *H_d^0}^* \Gamma_{\check{\sigma}^\pm, *L, i, H_d^-, *H_d^0} + B_0 \left( p^2, m_{H_u^0}^2, m_{H_u^+}^2 \right) \Gamma_{\check{\sigma}^\pm, *L, j, H_u^0, *H_u^+}^* \Gamma_{\check{\sigma}^\pm, *L, i, H_u^0, *H_u^+} \\
& + 2A_0 \left( m_{B_L}^2 \right) \Gamma_{\check{\sigma}^\pm L, i, \check{\sigma}^\pm, *L, i, B_L, B_L} + 2A_0 \left( m_{B_H}^2 \right) \Gamma_{\check{\sigma}^\pm L, i, \check{\sigma}^\pm, *L, i, B_H, B_H} + 2A_0 \left( m_{W_L^1}^2 \right) \Gamma_{\check{\sigma}^\pm L, i, \check{\sigma}^\pm, *L, i, W_L^1, W_L^1} \\
& + 2A_0 \left( m_{W_H^1}^2 \right) \Gamma_{\check{\sigma}^\pm L, i, \check{\sigma}^\pm, *L, i, W_H^1, W_H^1} + 2A_0 \left( m_{W_L^2}^2 \right) \Gamma_{\check{\sigma}^\pm L, i, \check{\sigma}^\pm, *L, i, W_L^2, W_L^2} + 2A_0 \left( m_{W_H^2}^2 \right) \Gamma_{\check{\sigma}^\pm L, i, \check{\sigma}^\pm, *L, i, W_H^2, W_H^2} \\
& + 2A_0 \left( m_{W_L^3}^2 \right) \Gamma_{\check{\sigma}^\pm L, i, \check{\sigma}^\pm, *L, i, W_L^3, W_L^3} + 2A_0 \left( m_{W_H^3}^2 \right) \Gamma_{\check{\sigma}^\pm L, i, \check{\sigma}^\pm, *L, i, W_H^3, W_H^3} - A_0 \left( m_{H_d^0}^2 \right) \Gamma_{\check{\sigma}^\pm L, i, \check{\sigma}^\pm, *L, i, H_d^0, *H_d^0} \\
& - A_0 \left( m_{H_d^-}^2 \right) \Gamma_{\check{\sigma}^\pm L, i, \check{\sigma}^\pm, *L, i, H_d^-, *H_d^-} - A_0 \left( m_{H_u^0}^2 \right) \Gamma_{\check{\sigma}^\pm L, i, \check{\sigma}^\pm, *L, i, H_u^0, *H_u^0} \\
& - A_0 \left( m_{H_u^+}^2 \right) \Gamma_{\check{\sigma}^\pm L, i, \check{\sigma}^\pm, *L, i, H_u^+, *H_u^+} - \sum_{a=1}^2 A_0 \left( m_{\phi_{B,a}^s}^2 \right) \Gamma_{\check{\sigma}^\pm L, i, \check{\sigma}^\pm, *L, i, \phi_{B,a}^s, \phi_{B,a}^s} \\
& - \sum_{a=1}^2 A_0 \left( m_{\phi_{AK,a}^s}^2 \right) \Gamma_{\check{\sigma}^\pm L, i, \check{\sigma}^\pm, *L, i, \phi_{AK,a}^s, \phi_{AK,a}^s} \\
& + \sum_{a=1}^2 \sum_{b=1}^2 B_0 \left( p^2, m_{\phi_{AK,a}^s}^2, m_{\phi_{B,b}^s}^2 \right) \Gamma_{\check{\sigma}^\pm, *L, j, \phi_{AK,a}^s, \phi_{B,b}^s}^* \Gamma_{\check{\sigma}^\pm, *L, i, \phi_{AK,a}^s, \phi_{B,b}^s} \\
& + \sum_{a=1}^2 \sum_{b=1}^2 B_0 \left( p^2, m_{\phi_{AK,a}^s}^2, m_{\phi_{B,b}^s}^2 \right) \Gamma_{\check{\sigma}^\pm, *L, j, \phi_{AK,a}^s, \phi_{B,b}^s}^* \Gamma_{\check{\sigma}^\pm, *L, i, \phi_{AK,a}^s, \phi_{B,b}^s} \\
& + \sum_{a=1}^2 \sum_{b=1}^4 B_0 \left( p^2, m_{\phi_{AK,a}^s}^2, m_{\sigma_{L,b}^\pm}^2 \right) \Gamma_{\check{\sigma}^\pm, *L, j, \phi_{AK,a}^s, \sigma_{L,b}^\pm}^* \Gamma_{\check{\sigma}^\pm, *L, i, \phi_{AK,a}^s, \sigma_{L,b}^\pm} \\
& - 3 \sum_{a=1}^3 A_0 \left( m_{\tilde{d}_{L,a}}^2 \right) \Gamma_{\check{\sigma}^\pm L, i, \check{\sigma}^\pm, *L, i, \tilde{d}_{L,a}^*, \tilde{d}_{L,a}} - 3 \sum_{a=1}^3 A_0 \left( m_{\tilde{d}_{R,a}}^2 \right) \Gamma_{\check{\sigma}^\pm L, i, \check{\sigma}^\pm, *L, i, \tilde{d}_{R,a}^*, \tilde{d}_{R,a}} \\
& - \sum_{a=1}^3 A_0 \left( m_{\tilde{e}_{L,a}}^2 \right) \Gamma_{\check{\sigma}^\pm L, i, \check{\sigma}^\pm, *L, i, \tilde{e}_{L,a}^*, \tilde{e}_{L,a}} - \sum_{a=1}^3 A_0 \left( m_{\tilde{e}_{R,a}}^2 \right) \Gamma_{\check{\sigma}^\pm L, i, \check{\sigma}^\pm, *L, i, \tilde{e}_{R,a}^*, \tilde{e}_{R,a}} \\
& - 3 \sum_{a=1}^3 A_0 \left( m_{\tilde{u}_{L,a}}^2 \right) \Gamma_{\check{\sigma}^\pm L, i, \check{\sigma}^\pm, *L, i, \tilde{u}_{L,a}^*, \tilde{u}_{L,a}} - 3 \sum_{a=1}^3 A_0 \left( m_{\tilde{u}_{R,a}}^2 \right) \Gamma_{\check{\sigma}^\pm L, i, \check{\sigma}^\pm, *L, i, \tilde{u}_{R,a}^*, \tilde{u}_{R,a}} \\
& - \sum_{a=1}^3 A_0 \left( m_{\tilde{\nu}_{L,a}}^2 \right) \Gamma_{\check{\sigma}^\pm L, i, \check{\sigma}^\pm, *L, i, \tilde{\nu}_{L,a}^*, \tilde{\nu}_{L,a}} \\
& + 3 \sum_{a=1}^3 \sum_{b=1}^3 B_0 \left( p^2, m_{\tilde{d}_{L,a}}^2, m_{\tilde{u}_{L,b}}^2 \right) \Gamma_{\check{\sigma}^\pm, *L, j, \tilde{d}_{L,a}^*, \tilde{u}_{L,b}}^* \Gamma_{\check{\sigma}^\pm, *L, i, \tilde{d}_{L,a}^*, \tilde{u}_{L,b}} \\
& + \sum_{a=1}^3 \sum_{b=1}^3 B_0 \left( p^2, m_{\tilde{e}_{L,a}}^2, m_{\tilde{\nu}_{L,b}}^2 \right) \Gamma_{\check{\sigma}^\pm, *L, j, \tilde{e}_{L,a}^*, \tilde{\nu}_{L,b}}^* \Gamma_{\check{\sigma}^\pm, *L, i, \tilde{e}_{L,a}^*, \tilde{\nu}_{L,b}} \\
& - \sum_{a=1}^4 A_0 \left( m_{\sigma_{L,a}^\pm}^2 \right) \Gamma_{\check{\sigma}^\pm L, i, \check{\sigma}^\pm, *L, i, \sigma_{L,a}^\pm, \sigma_{L,a}^\pm} - \frac{1}{2} \sum_{a=1}^4 A_0 \left( m_{\phi_{L,a}^0}^2 \right) \Gamma_{\check{\sigma}^\pm L, i, \check{\sigma}^\pm, *L, i, \phi_{L,a}^0, \phi_{L,a}^0}
\end{aligned}$$

$$\begin{aligned}
& -\frac{1}{2} \sum_{a=1}^4 A_0 \left( m_{\sigma_{L,a}^0}^2 \right) \Gamma_{\check{\sigma}^{\pm,L},i,\check{\sigma}^{\pm,*L},i,\sigma_{L,a}^0,\sigma_{L,a}^0} \\
& + \sum_{a=1}^4 \sum_{b=1}^2 B_0 \left( p^2, m_{\phi_{L,a}^0}^2, m_{\phi_{B,b}^s}^2 \right) \Gamma_{\check{\sigma}^{\pm,*L},j,\phi_{L,a}^0,\phi_{B,b}^s}^* \Gamma_{\check{\sigma}^{\pm,*L},i,\phi_{L,a}^0,\phi_{B,b}^s} \\
& + \sum_{a=1}^4 \sum_{b=1}^2 B_0 \left( p^2, m_{\sigma_{L,a}^0}^2, m_{\phi_{B,b}^s}^2 \right) \Gamma_{\check{\sigma}^{\pm,*L},j,\sigma_{L,a}^0,\phi_{B,b}^s}^* \Gamma_{\check{\sigma}^{\pm,*L},i,\sigma_{L,a}^0,\phi_{B,b}^s} \\
& + \sum_{a=1}^4 \sum_{b=1}^4 B_0 \left( p^2, m_{\phi_{L,a}^0}^2, m_{\sigma_{L,b}^{\pm}}^2 \right) \Gamma_{\check{\sigma}^{\pm,*L},j,\phi_{L,a}^0,\sigma_{L,b}^{\pm}}^* \Gamma_{\check{\sigma}^{\pm,*L},i,\phi_{L,a}^0,\sigma_{L,b}^{\pm}} \\
& + \sum_{a=1}^4 \sum_{b=1}^4 B_0 \left( p^2, m_{\sigma_{L,a}^0}^2, m_{\sigma_{L,b}^{\pm}}^2 \right) \Gamma_{\check{\sigma}^{\pm,*L},j,\sigma_{L,a}^0,\sigma_{L,b}^{\pm}}^* \Gamma_{\check{\sigma}^{\pm,*L},i,\sigma_{L,a}^0,\sigma_{L,b}^{\pm}} \\
& - \sum_{a=1}^{10} m_{f_{Po,a}^0} \sum_{b=1}^{10} B_0 \left( p^2, m_{f_{Po,a}^0}^2, m_{f_{Go,b}^-}^2 \right) m_{f_{Go,b}^-} \left( \Gamma_{\check{\sigma}^{\pm,*L},j,f_{Po,a}^0,f_{Go,b}^-}^{L*} \Gamma_{\check{\sigma}^{\pm,*L},i,f_{Po,a}^0,f_{Go,b}^-}^R + \Gamma_{\check{\sigma}^{\pm,*L},j,f_{Po,a}^0,f_{Go,b}^-}^{R*} \Gamma_{\check{\sigma}^{\pm,*L},i,f_{Po,a}^0,f_{Go,b}^-}^L \right) \\
& + \frac{1}{2} \sum_{a=1}^{10} \sum_{b=1}^{10} G_0 \left( p^2, m_{f_{Po,a}^0}^2, m_{f_{Go,b}^-}^2 \right) \left( \Gamma_{\check{\sigma}^{\pm,*L},j,f_{Po,a}^0,f_{Go,b}^-}^{L*} \Gamma_{\check{\sigma}^{\pm,*L},i,f_{Po,a}^0,f_{Go,b}^-}^L + \Gamma_{\check{\sigma}^{\pm,*L},j,f_{Po,a}^0,f_{Go,b}^-}^{R*} \Gamma_{\check{\sigma}^{\pm,*L},i,f_{Po,a}^0,f_{Go,b}^-}^R \right) \\
& + \sum_{b=1}^4 \Gamma_{\check{\sigma}^{\pm,*L},j,B_L,\sigma_{L,b}^{\pm}}^* \Gamma_{\check{\sigma}^{\pm,*L},i,B_L,\sigma_{L,b}^{\pm}} \Gamma_{\check{\sigma}^{\pm,*L},j,B_L,\sigma_{L,b}^{\pm}} F_0 \left( p^2, m_{\sigma_{L,b}^{\pm}}^2, m_{B_L}^2 \right) \\
& + \sum_{b=1}^4 \Gamma_{\check{\sigma}^{\pm,*L},j,B_H,\sigma_{L,b}^{\pm}}^* \Gamma_{\check{\sigma}^{\pm,*L},i,B_H,\sigma_{L,b}^{\pm}} \Gamma_{\check{\sigma}^{\pm,*L},j,B_H,\sigma_{L,b}^{\pm}} F_0 \left( p^2, m_{\sigma_{L,b}^{\pm}}^2, m_{B_H}^2 \right) \\
& + \sum_{b=1}^4 \Gamma_{\check{\sigma}^{\pm,*L},j,W_L^3,\sigma_{L,b}^{\pm}}^* \Gamma_{\check{\sigma}^{\pm,*L},i,W_L^3,\sigma_{L,b}^{\pm}} \Gamma_{\check{\sigma}^{\pm,*L},j,W_L^3,\sigma_{L,b}^{\pm}} F_0 \left( p^2, m_{\sigma_{L,b}^{\pm}}^2, m_{W_L^3}^2 \right) \\
& + \sum_{b=1}^4 \Gamma_{\check{\sigma}^{\pm,*L},j,W_H^3,\sigma_{L,b}^{\pm}}^* \Gamma_{\check{\sigma}^{\pm,*L},i,W_H^3,\sigma_{L,b}^{\pm}} \Gamma_{\check{\sigma}^{\pm,*L},j,W_H^3,\sigma_{L,b}^{\pm}} F_0 \left( p^2, m_{\sigma_{L,b}^{\pm}}^2, m_{W_H^3}^2 \right) \\
& + \frac{1}{2} \sum_{b=1}^4 \Gamma_{\check{\sigma}^{\pm,*L},j,W_L^1,\phi_{L,b}^0}^* \Gamma_{\check{\sigma}^{\pm,*L},i,W_L^1,\phi_{L,b}^0} \Gamma_{\check{\sigma}^{\pm,*L},j,W_L^1,\phi_{L,b}^0} F_0 \left( p^2, m_{\phi_{L,b}^0}^2, m_{W_L^1}^2 \right) \\
& + \frac{1}{2} \sum_{b=1}^4 \Gamma_{\check{\sigma}^{\pm,*L},j,W_H^1,\phi_{L,b}^0}^* \Gamma_{\check{\sigma}^{\pm,*L},i,W_H^1,\phi_{L,b}^0} \Gamma_{\check{\sigma}^{\pm,*L},j,W_H^1,\phi_{L,b}^0} F_0 \left( p^2, m_{\phi_{L,b}^0}^2, m_{W_H^1}^2 \right) \\
& + \frac{1}{2} \sum_{b=1}^4 \Gamma_{\check{\sigma}^{\pm,*L},j,W_L^2,\phi_{L,b}^0}^* \Gamma_{\check{\sigma}^{\pm,*L},i,W_L^2,\phi_{L,b}^0} \Gamma_{\check{\sigma}^{\pm,*L},j,W_L^2,\phi_{L,b}^0} F_0 \left( p^2, m_{\phi_{L,b}^0}^2, m_{W_L^2}^2 \right) \\
& + \frac{1}{2} \sum_{b=1}^4 \Gamma_{\check{\sigma}^{\pm,*L},j,W_H^2,\phi_{L,b}^0}^* \Gamma_{\check{\sigma}^{\pm,*L},i,W_H^2,\phi_{L,b}^0} \Gamma_{\check{\sigma}^{\pm,*L},j,W_H^2,\phi_{L,b}^0} F_0 \left( p^2, m_{\phi_{L,b}^0}^2, m_{W_H^2}^2 \right)
\end{aligned}$$

$$\begin{aligned}
& + \frac{1}{2} \sum_{b=1}^4 \Gamma_{\check{\sigma}^{\pm,*L,j}, W_L^1, \sigma_{L,b}^0}^* \Gamma_{\check{\sigma}^{\pm,*L,i}, W_L^1, \sigma_{L,b}^0} F_0(p^2, m_{\sigma_{L,b}^0}^2, m_{W_L^1}^2) \\
& + \frac{1}{2} \sum_{b=1}^4 \Gamma_{\check{\sigma}^{\pm,*L,j}, W_H^1, \sigma_{L,b}^0}^* \Gamma_{\check{\sigma}^{\pm,*L,i}, W_H^1, \sigma_{L,b}^0} F_0(p^2, m_{\sigma_{L,b}^0}^2, m_{W_H^1}^2) \\
& + \frac{1}{2} \sum_{b=1}^4 \Gamma_{\check{\sigma}^{\pm,*L,j}, W_L^2, \sigma_{L,b}^0}^* \Gamma_{\check{\sigma}^{\pm,*L,i}, W_L^2, \sigma_{L,b}^0} F_0(p^2, m_{\sigma_{L,b}^0}^2, m_{W_L^2}^2) \\
& + \frac{1}{2} \sum_{b=1}^4 \Gamma_{\check{\sigma}^{\pm,*L,j}, W_H^2, \sigma_{L,b}^0}^* \Gamma_{\check{\sigma}^{\pm,*L,i}, W_H^2, \sigma_{L,b}^0} F_0(p^2, m_{\sigma_{L,b}^0}^2, m_{W_H^2}^2)
\end{aligned} \tag{338}$$

• Self-Energy for Final heavy scalars 1 ( $\phi_{AK}^s$ )

$$\begin{aligned}
\Pi_{i,j}(p^2) = & + 2A_0(m_{W_L^1}^2) \Gamma_{\check{\phi}^{s,AK,i}, \check{\phi}^{s,*AK,i}, W_L^1, W_L^1} + 2A_0(m_{W_H^1}^2) \Gamma_{\check{\phi}^{s,AK,i}, \check{\phi}^{s,*AK,i}, W_H^1, W_H^1} + 2A_0(m_{W_L^2}^2) \Gamma_{\check{\phi}^{s,AK,i}, \check{\phi}^{s,*AK,i}, W_L^2, W_L^2} \\
& + 2A_0(m_{W_H^2}^2) \Gamma_{\check{\phi}^{s,AK,i}, \check{\phi}^{s,*AK,i}, W_H^2, W_H^2} - \sum_{a=1}^2 A_0(m_{\phi_{B,a}^s}^2) \Gamma_{\check{\phi}^{s,AK,i}, \check{\phi}^{s,*AK,i}, \phi_{B,a}^{s,*}, \phi_{B,a}^s} \\
& + \sum_{a=1}^2 \Gamma_{\check{\phi}^{s,*AK,j}, \phi_{B,a}^{s,*}, W_L^1}^* \Gamma_{\check{\phi}^{s,*AK,i}, \phi_{B,a}^{s,*}, W_L^1} F_0(p^2, m_{\phi_{B,a}^s}^2, m_{W_L^1}^2) \\
& + \sum_{a=1}^2 \Gamma_{\check{\phi}^{s,*AK,j}, \phi_{B,a}^{s,*}, W_H^1}^* \Gamma_{\check{\phi}^{s,*AK,i}, \phi_{B,a}^{s,*}, W_H^1} F_0(p^2, m_{\phi_{B,a}^s}^2, m_{W_H^1}^2) \\
& + \sum_{a=1}^2 \Gamma_{\check{\phi}^{s,*AK,j}, \phi_{B,a}^{s,*}, W_L^2}^* \Gamma_{\check{\phi}^{s,*AK,i}, \phi_{B,a}^{s,*}, W_L^2} F_0(p^2, m_{\phi_{B,a}^s}^2, m_{W_L^2}^2) \\
& + \sum_{a=1}^2 \Gamma_{\check{\phi}^{s,*AK,j}, \phi_{B,a}^{s,*}, W_H^2}^* \Gamma_{\check{\phi}^{s,*AK,i}, \phi_{B,a}^{s,*}, W_H^2} F_0(p^2, m_{\phi_{B,a}^s}^2, m_{W_H^2}^2) \\
& + \sum_{a=1}^2 \sum_{b=1}^4 B_0(p^2, m_{\phi_{B,a}^s}^2, m_{\sigma_{L,b}^{\pm}}^2) \Gamma_{\check{\phi}^{s,*AK,j}, \phi_{B,a}^{s,*}, \sigma_{L,b}^{\pm}}^* \Gamma_{\check{\phi}^{s,*AK,i}, \phi_{B,a}^{s,*}, \sigma_{L,b}^{\pm}} \\
& + \sum_{a=1}^2 \sum_{b=1}^4 B_0(p^2, m_{\phi_{AK,a}^s}^2, m_{\phi_{L,b}^0}^2) \Gamma_{\check{\phi}^{s,*AK,j}, \phi_{AK,a}^s, \phi_{L,b}^0}^* \Gamma_{\check{\phi}^{s,*AK,i}, \phi_{AK,a}^s, \phi_{L,b}^0} \\
& - \sum_{a=1}^4 A_0(m_{\sigma_{L,a}^{\pm}}^2) \Gamma_{\check{\phi}^{s,AK,i}, \check{\phi}^{s,*AK,i}, \sigma_{L,a}^{\pm,*}, \sigma_{L,a}^{\pm}} - \frac{1}{2} \sum_{a=1}^4 A_0(m_{\phi_{L,a}^0}^2) \Gamma_{\check{\phi}^{s,AK,i}, \check{\phi}^{s,*AK,i}, \phi_{L,a}^0, \phi_{L,a}^0} \\
& - \frac{1}{2} \sum_{a=1}^4 A_0(m_{\sigma_{L,a}^0}^2) \Gamma_{\check{\phi}^{s,AK,i}, \check{\phi}^{s,*AK,i}, \sigma_{L,a}^0, \sigma_{L,a}^0} \\
& + \sum_{a=1}^4 \sum_{b=1}^2 B_0(p^2, m_{\sigma_{L,a}^{\pm}}^2, m_{\phi_{B,b}^s}^2) \Gamma_{\check{\phi}^{s,*AK,j}, \sigma_{L,a}^{\pm,*}, \phi_{B,b}^s}^* \Gamma_{\check{\phi}^{s,*AK,i}, \sigma_{L,a}^{\pm,*}, \phi_{B,b}^s}
\end{aligned}$$

$$\begin{aligned}
& + \frac{1}{2} \sum_{a=1}^4 \sum_{b=1}^4 B_0(p^2, m_{\sigma_{L,a}^\pm}^2, m_{\sigma_{L,b}^\pm}^2) \Gamma_{\check{\phi}^{s,*AK},j,\sigma_{L,a}^\pm,*}^* \Gamma_{\check{\phi}^{s,*AK},i,\sigma_{L,a}^\pm,*} \Gamma_{\sigma_{L,b}^\pm} \\
& + \frac{1}{4} \sum_{a=1}^4 \sum_{b=1}^4 B_0(p^2, m_{\phi_{L,a}^0}^2, m_{\phi_{L,b}^0}^2) \Gamma_{\check{\phi}^{s,*AK},j,\phi_{L,a}^0,\phi_{L,b}^0}^* \Gamma_{\check{\phi}^{s,*AK},i,\phi_{L,a}^0,\phi_{L,b}^0} \\
& + \frac{1}{2} \sum_{a=1}^4 \sum_{b=1}^4 B_0(p^2, m_{\sigma_{L,a}^0}^2, m_{\phi_{L,b}^0}^2) \Gamma_{\check{\phi}^{s,*AK},j,\sigma_{L,a}^0,\phi_{L,b}^0}^* \Gamma_{\check{\phi}^{s,*AK},i,\sigma_{L,a}^0,\phi_{L,b}^0} \\
& + \frac{1}{4} \sum_{a=1}^4 \sum_{b=1}^4 B_0(p^2, m_{\sigma_{L,a}^0}^2, m_{\sigma_{L,b}^0}^2) \Gamma_{\check{\phi}^{s,*AK},j,\sigma_{L,a}^0,\sigma_{L,b}^0}^* \Gamma_{\check{\phi}^{s,*AK},i,\sigma_{L,a}^0,\sigma_{L,b}^0} \\
& - \frac{1}{2} \sum_{a=1}^{10} m_{f_{Go,a}^-} \sum_{b=1}^{10} B_0(p^2, m_{f_{Go,a}^-}^2, m_{f_{Go,b}^-}^2) m_{f_{Go,b}^-} \left( \Gamma_{\check{\phi}^{s,*AK},j,f_{Go,a}^-,f_{Go,b}^-}^{L*} \Gamma_{\check{\phi}^{s,*AK},i,f_{Go,a}^-,f_{Go,b}^-}^R + \Gamma_{\check{\phi}^{s,*AK},j,f_{Go,a}^-,f_{Go,b}^-}^{R*} \Gamma_{\check{\phi}^{s,*AK},i,f_{Go,a}^-,f_{Go,b}^-}^L \right) \\
& + \frac{1}{4} \sum_{a=1}^{10} \sum_{b=1}^{10} G_0(p^2, m_{f_{Go,a}^-}^2, m_{f_{Go,b}^-}^2) \left( \Gamma_{\check{\phi}^{s,*AK},j,f_{Go,a}^-,f_{Go,b}^-}^{L*} \Gamma_{\check{\phi}^{s,*AK},i,f_{Go,a}^-,f_{Go,b}^-}^L + \Gamma_{\check{\phi}^{s,*AK},j,f_{Go,a}^-,f_{Go,b}^-}^{R*} \Gamma_{\check{\phi}^{s,*AK},i,f_{Go,a}^-,f_{Go,b}^-}^R \right) \\
& - \frac{1}{2} \sum_{a=1}^{10} m_{f_{Po,a}^0} \sum_{b=1}^{10} B_0(p^2, m_{f_{Po,a}^0}^2, m_{f_{Po,b}^0}^2) m_{f_{Po,b}^0} \left( \Gamma_{\check{\phi}^{s,*AK},j,f_{Po,a}^0,f_{Po,b}^0}^{L*} \Gamma_{\check{\phi}^{s,*AK},i,f_{Po,a}^0,f_{Po,b}^0}^R + \Gamma_{\check{\phi}^{s,*AK},j,f_{Po,a}^0,f_{Po,b}^0}^{R*} \Gamma_{\check{\phi}^{s,*AK},i,f_{Po,a}^0,f_{Po,b}^0}^L \right) \\
& + \frac{1}{4} \sum_{a=1}^{10} \sum_{b=1}^{10} G_0(p^2, m_{f_{Po,a}^0}^2, m_{f_{Po,b}^0}^2) \left( \Gamma_{\check{\phi}^{s,*AK},j,f_{Po,a}^0,f_{Po,b}^0}^{L*} \Gamma_{\check{\phi}^{s,*AK},i,f_{Po,a}^0,f_{Po,b}^0}^L + \Gamma_{\check{\phi}^{s,*AK},j,f_{Po,a}^0,f_{Po,b}^0}^{R*} \Gamma_{\check{\phi}^{s,*AK},i,f_{Po,a}^0,f_{Po,b}^0}^R \right) \\
& + \sum_{b=1}^2 \Gamma_{\check{\phi}^{s,*AK},j,W_L^1,\phi_{B,b}^s}^* \Gamma_{\check{\phi}^{s,*AK},i,W_L^1,\phi_{B,b}^s} F_0(p^2, m_{\phi_{B,b}^s}^2, m_{W_L^1}^2) \\
& + \sum_{b=1}^2 \Gamma_{\check{\phi}^{s,*AK},j,W_H^1,\phi_{B,b}^s}^* \Gamma_{\check{\phi}^{s,*AK},i,W_H^1,\phi_{B,b}^s} F_0(p^2, m_{\phi_{B,b}^s}^2, m_{W_H^1}^2) \\
& + \sum_{b=1}^2 \Gamma_{\check{\phi}^{s,*AK},j,W_L^2,\phi_{B,b}^s}^* \Gamma_{\check{\phi}^{s,*AK},i,W_L^2,\phi_{B,b}^s} F_0(p^2, m_{\phi_{B,b}^s}^2, m_{W_L^2}^2) \\
& + \sum_{b=1}^2 \Gamma_{\check{\phi}^{s,*AK},j,W_H^2,\phi_{B,b}^s}^* \Gamma_{\check{\phi}^{s,*AK},i,W_H^2,\phi_{B,b}^s} F_0(p^2, m_{\phi_{B,b}^s}^2, m_{W_H^2}^2) \tag{339}
\end{aligned}$$

• Self-Energy for Final heavy scalars 2 ( $\phi_B^s$ )

$$\begin{aligned}
\Pi_{i,j}(p^2) = & + 2A_0(m_{W_L^1}^2) \Gamma_{\check{\phi}^{sB},i,\check{\phi}^{s,*B},i,W_L^1,W_L^1} \Gamma_{\check{\phi}^{sB},i,\check{\phi}^{s,*B},i,W_H^1,W_H^1} + 2A_0(m_{W_L^2}^2) \Gamma_{\check{\phi}^{sB},i,\check{\phi}^{s,*B},i,W_L^2,W_L^2} \\
& + 2A_0(m_{W_H^2}^2) \Gamma_{\check{\phi}^{sB},i,\check{\phi}^{s,*B},i,W_H^2,W_H^2} + 2A_0(m_{W_L^3}^2) \Gamma_{\check{\phi}^{sB},i,\check{\phi}^{s,*B},i,W_L^3,W_L^3} + 2A_0(m_{W_H^3}^2) \Gamma_{\check{\phi}^{sB},i,\check{\phi}^{s,*B},i,W_H^3,W_H^3} \\
& - \sum_{a=1}^2 A_0(m_{\phi_{B,a}^s}^2) \Gamma_{\check{\phi}^{sB},i,\check{\phi}^{s,*B},i,\phi_{B,a}^s,\phi_{B,a}^s} - \sum_{a=1}^2 A_0(m_{\phi_{AK,a}^s}^2) \Gamma_{\check{\phi}^{sB},i,\check{\phi}^{s,*B},i,\phi_{AK,a}^s,\phi_{AK,a}^s}
\end{aligned}$$

$$\begin{aligned}
& + \sum_{a=1}^2 \Gamma_{\check{\phi}^{s,*B,j}, \phi_{AK,a}^s, W_L^1}^* \Gamma_{\check{\phi}^{s,*B,i}, \phi_{AK,a}^s, W_L^1} F_0(p^2, m_{\phi_{AK,a}^s}^2, m_{W_L^1}^2) \\
& + \sum_{a=1}^2 \Gamma_{\check{\phi}^{s,*B,j}, \phi_{AK,a}^s, W_H^1}^* \Gamma_{\check{\phi}^{s,*B,i}, \phi_{AK,a}^s, W_H^1} F_0(p^2, m_{\phi_{AK,a}^s}^2, m_{W_H^1}^2) \\
& + \sum_{a=1}^2 \Gamma_{\check{\phi}^{s,*B,j}, \phi_{AK,a}^s, W_L^2}^* \Gamma_{\check{\phi}^{s,*B,i}, \phi_{AK,a}^s, W_L^2} F_0(p^2, m_{\phi_{AK,a}^s}^2, m_{W_L^2}^2) \\
& + \sum_{a=1}^2 \Gamma_{\check{\phi}^{s,*B,j}, \phi_{AK,a}^s, W_H^2}^* \Gamma_{\check{\phi}^{s,*B,i}, \phi_{AK,a}^s, W_H^2} F_0(p^2, m_{\phi_{AK,a}^s}^2, m_{W_H^2}^2) \\
& + \sum_{a=1}^2 \sum_{b=1}^4 B_0(p^2, m_{\phi_{AK,a}^s}^2, m_{\sigma_{L,b}^\pm}^2) \Gamma_{\check{\phi}^{s,*B,j}, \phi_{AK,a}^s, \sigma_{L,b}^\pm}^* \Gamma_{\check{\phi}^{s,*B,i}, \phi_{AK,a}^s, \sigma_{L,b}^\pm} \\
& + \sum_{a=1}^2 \sum_{b=1}^4 B_0(p^2, m_{\phi_{AK,a}^s}^2, m_{\sigma_{L,b}^\pm}^2) \Gamma_{\check{\phi}^{s,*B,j}, \phi_{AK,a}^s, \sigma_{L,b}^\pm}^* \Gamma_{\check{\phi}^{s,*B,i}, \phi_{AK,a}^s, \sigma_{L,b}^\pm} \\
& - \sum_{a=1}^4 A_0(m_{\sigma_{L,a}^\pm}^2) \Gamma_{\check{\phi}^{sB,i}, \check{\phi}^{s,*B,i}, \sigma_{L,a}^\pm, \sigma_{L,a}^\pm} - \frac{1}{2} \sum_{a=1}^4 A_0(m_{\phi_{L,a}^0}^2) \Gamma_{\check{\phi}^{sB,i}, \check{\phi}^{s,*B,i}, \phi_{L,a}^0, \phi_{L,a}^0} \\
& - \frac{1}{2} \sum_{a=1}^4 A_0(m_{\sigma_{L,a}^0}^2) \Gamma_{\check{\phi}^{sB,i}, \check{\phi}^{s,*B,i}, \sigma_{L,a}^0, \sigma_{L,a}^0} \\
& + \sum_{a=1}^4 \sum_{b=1}^2 B_0(p^2, m_{\phi_{L,a}^0}^2, m_{\phi_{B,b}^s}^2) \Gamma_{\check{\phi}^{s,*B,j}, \phi_{L,a}^0, \phi_{B,b}^s}^* \Gamma_{\check{\phi}^{s,*B,i}, \phi_{L,a}^0, \phi_{B,b}^s} \\
& + \sum_{a=1}^4 \sum_{b=1}^4 B_0(p^2, m_{\phi_{L,a}^0}^2, m_{\sigma_{L,b}^\pm}^2) \Gamma_{\check{\phi}^{s,*B,j}, \phi_{L,a}^0, \sigma_{L,b}^\pm}^* \Gamma_{\check{\phi}^{s,*B,i}, \phi_{L,a}^0, \sigma_{L,b}^\pm} \\
& + \sum_{a=1}^4 \sum_{b=1}^4 B_0(p^2, m_{\sigma_{L,a}^0}^2, m_{\sigma_{L,b}^\pm}^2) \Gamma_{\check{\phi}^{s,*B,j}, \sigma_{L,a}^0, \sigma_{L,b}^\pm}^* \Gamma_{\check{\phi}^{s,*B,i}, \sigma_{L,a}^0, \sigma_{L,b}^\pm} \\
& - \sum_{a=1}^{10} m_{f_{Po,a}^0} \sum_{b=1}^{10} B_0(p^2, m_{f_{Po,a}^0}^2, m_{f_{Go,b}^-}^2) m_{f_{Go,b}^-} \left( \Gamma_{\check{\phi}^{s,*B,j}, f_{Po,a}^0, f_{Go,b}^-}^{L*} \Gamma_{\check{\phi}^{s,*B,i}, f_{Po,a}^0, f_{Go,b}^-}^R + \Gamma_{\check{\phi}^{s,*B,j}, f_{Po,a}^0, f_{Go,b}^-}^{R*} \Gamma_{\check{\phi}^{s,*B,i}, f_{Po,a}^0, f_{Go,b}^-}^L \right) \\
& + \frac{1}{2} \sum_{a=1}^{10} \sum_{b=1}^{10} G_0(p^2, m_{f_{Po,a}^0}^2, m_{f_{Go,b}^-}^2) \left( \Gamma_{\check{\phi}^{s,*B,j}, f_{Po,a}^0, f_{Go,b}^-}^{L*} \Gamma_{\check{\phi}^{s,*B,i}, f_{Po,a}^0, f_{Go,b}^-}^L + \Gamma_{\check{\phi}^{s,*B,j}, f_{Po,a}^0, f_{Go,b}^-}^{R*} \Gamma_{\check{\phi}^{s,*B,i}, f_{Po,a}^0, f_{Go,b}^-}^R \right) \\
& + \sum_{b=1}^2 \Gamma_{\check{\phi}^{s,*B,j}, W_L^3, \phi_{B,b}^s}^* \Gamma_{\check{\phi}^{s,*B,i}, W_L^3, \phi_{B,b}^s} F_0(p^2, m_{\phi_{B,b}^s}^2, m_{W_L^3}^2) \\
& + \sum_{b=1}^2 \Gamma_{\check{\phi}^{s,*B,j}, W_H^3, \phi_{B,b}^s}^* \Gamma_{\check{\phi}^{s,*B,i}, W_H^3, \phi_{B,b}^s} F_0(p^2, m_{\phi_{B,b}^s}^2, m_{W_H^3}^2) \\
& + \sum_{b=1}^2 \Gamma_{\check{\phi}^{s,*B,j}, W_L^1, \phi_{AK,b}^s}^* \Gamma_{\check{\phi}^{s,*B,i}, W_L^1, \phi_{AK,b}^s} F_0(p^2, m_{\phi_{AK,b}^s}^2, m_{W_L^1}^2)
\end{aligned}$$

$$\begin{aligned}
& + \sum_{b=1}^2 \Gamma_{\check{\phi}^{s,*B,j}, W_H^1, \phi_{AK,b}^s}^* \Gamma_{\check{\phi}^{s,*B,i}, W_H^1, \phi_{AK,b}^s} F_0(p^2, m_{\phi_{AK,b}^s}^2, m_{W_H^1}^2) \\
& + \sum_{b=1}^2 \Gamma_{\check{\phi}^{s,*B,j}, W_L^2, \phi_{AK,b}^s}^* \Gamma_{\check{\phi}^{s,*B,i}, W_L^2, \phi_{AK,b}^s} F_0(p^2, m_{\phi_{AK,b}^s}^2, m_{W_L^2}^2) \\
& + \sum_{b=1}^2 \Gamma_{\check{\phi}^{s,*B,j}, W_H^2, \phi_{AK,b}^s}^* \Gamma_{\check{\phi}^{s,*B,i}, W_H^2, \phi_{AK,b}^s} F_0(p^2, m_{\phi_{AK,b}^s}^2, m_{W_H^2}^2)
\end{aligned} \tag{340}$$

• Self-Energy for Linking/Ad/K neutral fermion mass eigenstates after AxB breaking ( $f_{Po}^0$ )

$$\begin{aligned}
\Sigma_{i,j}^S(p^2) = & + \sum_{a=1}^2 \sum_{b=1}^{10} B_0(p^2, m_{f_{Po,b}^0}^2, m_{\phi_{AK,a}^s}^2) \Gamma_{\check{f}^{0Po,j}, \phi_{AK,a}^s, f_{Po,b}^0}^{L*} m_{f_{Po,b}^0} \Gamma_{\check{f}^{0Po,i}, \phi_{AK,a}^s, f_{Po,b}^0}^R \\
& + 3 \sum_{a=1}^3 \sum_{b=1}^3 B_0(p^2, m_{d_{L,b}^D}^2, m_{\tilde{d}_{L,a}^*}^2) \Gamma_{\check{f}^{0Po,j}, \tilde{d}_{L,a}^*, d_{L,b}^D}^{L*} m_{d_{L,b}^D} \Gamma_{\check{f}^{0Po,i}, \tilde{d}_{L,a}^*, d_{L,b}^D}^R \\
& + 3 \sum_{a=1}^3 \sum_{b=1}^3 B_0(p^2, m_{d_{R,b}^D}^2, m_{\tilde{d}_{R,a}^*}^2) \Gamma_{\check{f}^{0Po,j}, \tilde{d}_{R,a}^*, d_{R,b}^D}^{L*} m_{d_{R,b}^D} \Gamma_{\check{f}^{0Po,i}, \tilde{d}_{R,a}^*, d_{R,b}^D}^R \\
& + \sum_{a=1}^3 \sum_{b=1}^3 B_0(p^2, m_{e_{L,b}^D}^2, m_{\tilde{e}_{L,a}^*}^2) \Gamma_{\check{f}^{0Po,j}, \tilde{e}_{L,a}^*, e_{L,b}^D}^{L*} m_{e_{L,b}^D} \Gamma_{\check{f}^{0Po,i}, \tilde{e}_{L,a}^*, e_{L,b}^D}^R \\
& + \sum_{a=1}^3 \sum_{b=1}^3 B_0(p^2, m_{e_{R,b}^D}^2, m_{\tilde{e}_{R,a}^*}^2) \Gamma_{\check{f}^{0Po,j}, \tilde{e}_{R,a}^*, e_{R,b}^D}^{L*} m_{e_{R,b}^D} \Gamma_{\check{f}^{0Po,i}, \tilde{e}_{R,a}^*, e_{R,b}^D}^R \\
& + 3 \sum_{a=1}^3 \sum_{b=1}^3 B_0(p^2, m_{u_{L,b}^D}^2, m_{\tilde{u}_{L,a}^*}^2) \Gamma_{\check{f}^{0Po,j}, \tilde{u}_{L,a}^*, u_{L,b}^D}^{L*} m_{u_{L,b}^D} \Gamma_{\check{f}^{0Po,i}, \tilde{u}_{L,a}^*, u_{L,b}^D}^R \\
& + 3 \sum_{a=1}^3 \sum_{b=1}^3 B_0(p^2, m_{u_{R,b}^D}^2, m_{\tilde{u}_{R,a}^*}^2) \Gamma_{\check{f}^{0Po,j}, \tilde{u}_{R,a}^*, u_{R,b}^D}^{L*} m_{u_{R,b}^D} \Gamma_{\check{f}^{0Po,i}, \tilde{u}_{R,a}^*, u_{R,b}^D}^R \\
& + \sum_{a=1}^3 \sum_{b=1}^3 B_0(p^2, m_{\nu_{L,b}^D}^2, m_{\tilde{\nu}_{L,a}^*}^2) \Gamma_{\check{f}^{0Po,j}, \tilde{\nu}_{L,a}^*, \nu_{L,b}^D}^{L*} m_{\nu_{L,b}^D} \Gamma_{\check{f}^{0Po,i}, \tilde{\nu}_{L,a}^*, \nu_{L,b}^D}^R \\
& + \sum_{a=1}^4 \sum_{b=1}^{10} B_0(p^2, m_{f_{Go,b}^-}^2, m_{\sigma_{L,a}^{\pm}}^2) \Gamma_{\check{f}^{0Po,j}, \sigma_{L,a}^{\pm,*}, f_{Go,b}^-}^{L*} m_{f_{Go,b}^-} \Gamma_{\check{f}^{0Po,i}, \sigma_{L,a}^{\pm,*}, f_{Go,b}^-}^R \\
& + \frac{1}{2} \sum_{a=1}^4 \sum_{b=1}^{10} B_0(p^2, m_{f_{Po,b}^0}^2, m_{\sigma_{L,a}^0}^2) \Gamma_{\check{f}^{0Po,j}, \sigma_{L,a}^0, f_{Po,b}^0}^{L*} m_{f_{Po,b}^0} \Gamma_{\check{f}^{0Po,i}, \sigma_{L,a}^0, f_{Po,b}^0}^R \\
& + \sum_{a=1}^{10} m_{f_{Go,a}^-} \sum_{b=1}^2 B_0(p^2, m_{f_{Go,a}^-}^2, m_{\phi_{B,b}^s}^2) \Gamma_{\check{f}^{0Po,j}, f_{Go,a}^-, \phi_{B,b}^s}^{L*} \Gamma_{\check{f}^{0Po,i}, f_{Go,a}^-, \phi_{B,b}^s}^R
\end{aligned}$$

$$\begin{aligned}
& + \frac{1}{2} \sum_{a=1}^{10} m_{f_{Po,a}^0} \sum_{b=1}^4 B_0(p^2, m_{f_{Po,a}^0}^2, m_{\phi_{L,b}^0}^2) \Gamma_{\tilde{f}^0 Po, j, f_{Po,a}^0, \phi_{L,b}^0}^{L*} \Gamma_{\tilde{f}^0 Po, i, f_{Po,a}^0, \phi_{L,b}^0}^R \\
& - 2 \sum_{b=1}^{10} B_0(p^2, m_{f_{Po,b}^0}^2, m_{B_L}^2) \Gamma_{\tilde{f}^0 Po, j, B_L, f_{Po,b}^0}^{R*} m_{f_{Po,b}^0} \Gamma_{\tilde{f}^0 Po, i, B_L, f_{Po,b}^0}^L \\
& - 2 \sum_{b=1}^{10} B_0(p^2, m_{f_{Po,b}^0}^2, m_{B_H}^2) \Gamma_{\tilde{f}^0 Po, j, B_H, f_{Po,b}^0}^{R*} m_{f_{Po,b}^0} \Gamma_{\tilde{f}^0 Po, i, B_H, f_{Po,b}^0}^L \\
& - 2 \sum_{b=1}^{10} B_0(p^2, m_{f_{Go,b}^-}^2, m_{W_L^1}^2) \Gamma_{\tilde{f}^0 Po, j, W_L^1, f_{Go,b}^-}^{R*} m_{f_{Go,b}^-} \Gamma_{\tilde{f}^0 Po, i, W_L^1, f_{Go,b}^-}^L \\
& - 2 \sum_{b=1}^{10} B_0(p^2, m_{f_{Go,b}^-}^2, m_{W_H^1}^2) \Gamma_{\tilde{f}^0 Po, j, W_H^1, f_{Go,b}^-}^{R*} m_{f_{Go,b}^-} \Gamma_{\tilde{f}^0 Po, i, W_H^1, f_{Go,b}^-}^L \\
& - 2 \sum_{b=1}^{10} B_0(p^2, m_{f_{Go,b}^-}^2, m_{W_L^2}^2) \Gamma_{\tilde{f}^0 Po, j, W_L^2, f_{Go,b}^-}^{R*} m_{f_{Go,b}^-} \Gamma_{\tilde{f}^0 Po, i, W_L^2, f_{Go,b}^-}^L \\
& - 2 \sum_{b=1}^{10} B_0(p^2, m_{f_{Go,b}^-}^2, m_{W_H^2}^2) \Gamma_{\tilde{f}^0 Po, j, W_H^2, f_{Go,b}^-}^{R*} m_{f_{Go,b}^-} \Gamma_{\tilde{f}^0 Po, i, W_H^2, f_{Go,b}^-}^L \\
& - 2 \sum_{b=1}^{10} B_0(p^2, m_{f_{Po,b}^0}^2, m_{W_L^3}^2) \Gamma_{\tilde{f}^0 Po, j, W_L^3, f_{Po,b}^0}^{R*} m_{f_{Po,b}^0} \Gamma_{\tilde{f}^0 Po, i, W_L^3, f_{Po,b}^0}^L \\
& - 2 \sum_{b=1}^{10} B_0(p^2, m_{f_{Po,b}^0}^2, m_{W_H^3}^2) \Gamma_{\tilde{f}^0 Po, j, W_H^3, f_{Po,b}^0}^{R*} m_{f_{Po,b}^0} \Gamma_{\tilde{f}^0 Po, i, W_H^3, f_{Po,b}^0}^L \\
& + B_0(p^2, m_{\tilde{H}^0}^2, m_{H_d^0}^2) \Gamma_{\tilde{f}^0 Po, j, H_d^0, \text{FH0D}(\{1\})}^{L*} m_{\tilde{H}^0} \Gamma_{\tilde{f}^0 Po, i, H_d^0, \text{FH0D}(\{1\})}^R + B_0(p^2, m_{\tilde{H}^-}^2, m_{H_d^-}^2) \Gamma_{\tilde{f}^0 Po, j, H_d^-, \text{FHCD}(\{1\})}^{L*} m_{\tilde{H}^-} \\
& + B_0(p^2, m_{\tilde{H}^0}^2, m_{H_u^0}^2) \Gamma_{\tilde{f}^0 Po, j, H_u^0, \text{FH0D}(\{1\})}^{L*} m_{\tilde{H}^0} \Gamma_{\tilde{f}^0 Po, i, H_u^0, \text{FH0D}(\{1\})}^R \\
& + B_0(p^2, m_{\tilde{H}^-}^2, m_{H_u^+}^2) \Gamma_{\tilde{f}^0 Po, j, H_u^+, \text{FHCD}(\{1\})}^{L*} m_{\tilde{H}^-} \Gamma_{\tilde{f}^0 Po, i, H_u^+, \text{FHCD}(\{1\})}^R \tag{341}
\end{aligned}$$

$$\begin{aligned}
\Sigma_{i,j}^R(p^2) & = + \sum_{a=1}^2 \sum_{b=1}^{10} B_0(p^2, m_{f_{Po,b}^0}^2, m_{\phi_{AK,a}^s}^2) \Gamma_{\tilde{f}^0 Po, j, \phi_{AK,a}^s, f_{Po,b}^0}^{L*} m_{f_{Po,b}^0} \Gamma_{\tilde{f}^0 Po, i, \phi_{AK,a}^s, f_{Po,b}^0}^R \\
& + 3 \sum_{a=1}^3 \sum_{b=1}^3 B_0(p^2, m_{d_{L,b}^D}^2, m_{d_{L,a}^D}^2) \Gamma_{\tilde{f}^0 Po, j, \tilde{d}_{L,a}^*, d_{L,b}^D}^{L*} m_{d_{L,b}^D} \Gamma_{\tilde{f}^0 Po, i, \tilde{d}_{L,a}^*, d_{L,b}^D}^R \\
& + 3 \sum_{a=1}^3 \sum_{b=1}^3 B_0(p^2, m_{d_{R,b}^D}^2, m_{d_{R,a}^D}^2) \Gamma_{\tilde{f}^0 Po, j, \tilde{d}_{R,a}^*, d_{R,b}^D}^{L*} m_{d_{R,b}^D} \Gamma_{\tilde{f}^0 Po, i, \tilde{d}_{R,a}^*, d_{R,b}^D}^R \\
& + \sum_{a=1}^3 \sum_{b=1}^3 B_0(p^2, m_{e_{L,b}^D}^2, m_{e_{L,a}^D}^2) \Gamma_{\tilde{f}^0 Po, j, \tilde{e}_{L,a}^*, e_{L,b}^D}^{L*} m_{e_{L,b}^D} \Gamma_{\tilde{f}^0 Po, i, \tilde{e}_{L,a}^*, e_{L,b}^D}^R
\end{aligned}$$



$$\begin{aligned}
& + \sum_{a=1}^3 \sum_{b=1}^3 B_0 \left( p^2, m_{e_{R,b}^D}^2, m_{\tilde{e}_{R,a}}^2 \right) \Gamma_{\tilde{f}^0 P o, j, \tilde{e}_{R,a}^*, e_{R,b}^D}^{L*} m_{e_{R,b}^D} \Gamma_{\tilde{f}^0 P o, i, \tilde{e}_{R,a}^*, e_{R,b}^D}^R \\
& + 3 \sum_{a=1}^3 \sum_{b=1}^3 B_0 \left( p^2, m_{u_{L,b}^D}^2, m_{\tilde{u}_{L,a}}^2 \right) \Gamma_{\tilde{f}^0 P o, j, \tilde{u}_{L,a}^*, u_{L,b}^D}^{L*} m_{u_{L,b}^D} \Gamma_{\tilde{f}^0 P o, i, \tilde{u}_{L,a}^*, u_{L,b}^D}^R \\
& + 3 \sum_{a=1}^3 \sum_{b=1}^3 B_0 \left( p^2, m_{u_{R,b}^D}^2, m_{\tilde{u}_{R,a}}^2 \right) \Gamma_{\tilde{f}^0 P o, j, \tilde{u}_{R,a}^*, u_{R,b}^D}^{L*} m_{u_{R,b}^D} \Gamma_{\tilde{f}^0 P o, i, \tilde{u}_{R,a}^*, u_{R,b}^D}^R \\
& + \sum_{a=1}^3 \sum_{b=1}^3 B_0 \left( p^2, m_{\nu_{L,b}^D}^2, m_{\tilde{\nu}_{L,a}}^2 \right) \Gamma_{\tilde{f}^0 P o, j, \tilde{\nu}_{L,a}^*, \nu_{L,b}^D}^{L*} m_{\nu_{L,b}^D} \Gamma_{\tilde{f}^0 P o, i, \tilde{\nu}_{L,a}^*, \nu_{L,b}^D}^R \\
& + \sum_{a=1}^4 \sum_{b=1}^{10} B_0 \left( p^2, m_{f_{G o, b}^-}^2, m_{\sigma_{L, a}^{\pm, *}}^2 \right) \Gamma_{\tilde{f}^0 P o, j, \sigma_{L, a}^{\pm, *}, f_{G o, b}^-}^{L*} m_{f_{G o, b}^-} \Gamma_{\tilde{f}^0 P o, i, \sigma_{L, a}^{\pm, *}, f_{G o, b}^-}^R \\
& + \frac{1}{2} \sum_{a=1}^4 \sum_{b=1}^{10} B_0 \left( p^2, m_{f_{P o, b}^0}^2, m_{\sigma_{L, a}^0}^2 \right) \Gamma_{\tilde{f}^0 P o, j, \sigma_{L, a}^0, f_{P o, b}^0}^{L*} m_{f_{P o, b}^0} \Gamma_{\tilde{f}^0 P o, i, \sigma_{L, a}^0, f_{P o, b}^0}^R \\
& + \sum_{a=1}^{10} m_{f_{G o, a}^-} \sum_{b=1}^2 B_0 \left( p^2, m_{f_{G o, a}^-}^2, m_{\phi_{B, b}^s}^2 \right) \Gamma_{\tilde{f}^0 P o, j, f_{G o, a}^-, \phi_{B, b}^s}^{L*} \Gamma_{\tilde{f}^0 P o, i, f_{G o, a}^-, \phi_{B, b}^s}^R \\
& + \frac{1}{2} \sum_{a=1}^{10} m_{f_{P o, a}^0} \sum_{b=1}^4 B_0 \left( p^2, m_{f_{P o, a}^0}^2, m_{\phi_{L, b}^0}^2 \right) \Gamma_{\tilde{f}^0 P o, j, f_{P o, a}^0, \phi_{L, b}^0}^{L*} \Gamma_{\tilde{f}^0 P o, i, f_{P o, a}^0, \phi_{L, b}^0}^R \\
& - 2 \sum_{b=1}^{10} B_0 \left( p^2, m_{f_{P o, b}^0}^2, m_{B_L}^2 \right) \Gamma_{\tilde{f}^0 P o, j, B_L, f_{P o, b}^0}^{R*} m_{f_{P o, b}^0} \Gamma_{\tilde{f}^0 P o, i, B_L, f_{P o, b}^0}^L \\
& - 2 \sum_{b=1}^{10} B_0 \left( p^2, m_{f_{P o, b}^0}^2, m_{B_H}^2 \right) \Gamma_{\tilde{f}^0 P o, j, B_H, f_{P o, b}^0}^{R*} m_{f_{P o, b}^0} \Gamma_{\tilde{f}^0 P o, i, B_H, f_{P o, b}^0}^L \\
& - 2 \sum_{b=1}^{10} B_0 \left( p^2, m_{f_{G o, b}^-}^2, m_{W_L^1}^2 \right) \Gamma_{\tilde{f}^0 P o, j, W_L^1, f_{G o, b}^-}^{R*} m_{f_{G o, b}^-} \Gamma_{\tilde{f}^0 P o, i, W_L^1, f_{G o, b}^-}^L \\
& - 2 \sum_{b=1}^{10} B_0 \left( p^2, m_{f_{G o, b}^-}^2, m_{W_H^1}^2 \right) \Gamma_{\tilde{f}^0 P o, j, W_H^1, f_{G o, b}^-}^{R*} m_{f_{G o, b}^-} \Gamma_{\tilde{f}^0 P o, i, W_H^1, f_{G o, b}^-}^L \\
& - 2 \sum_{b=1}^{10} B_0 \left( p^2, m_{f_{G o, b}^-}^2, m_{W_L^2}^2 \right) \Gamma_{\tilde{f}^0 P o, j, W_L^2, f_{G o, b}^-}^{R*} m_{f_{G o, b}^-} \Gamma_{\tilde{f}^0 P o, i, W_L^2, f_{G o, b}^-}^L \\
& - 2 \sum_{b=1}^{10} B_0 \left( p^2, m_{f_{G o, b}^-}^2, m_{W_H^2}^2 \right) \Gamma_{\tilde{f}^0 P o, j, W_H^2, f_{G o, b}^-}^{R*} m_{f_{G o, b}^-} \Gamma_{\tilde{f}^0 P o, i, W_H^2, f_{G o, b}^-}^L \\
& - 2 \sum_{b=1}^{10} B_0 \left( p^2, m_{f_{P o, b}^0}^2, m_{W_L^3}^2 \right) \Gamma_{\tilde{f}^0 P o, j, W_L^3, f_{P o, b}^0}^{R*} m_{f_{P o, b}^0} \Gamma_{\tilde{f}^0 P o, i, W_L^3, f_{P o, b}^0}^L
\end{aligned}$$

$$\begin{aligned}
& -2 \sum_{b=1}^{10} B_0 \left( p^2, m_{f_{Po,b}^0}^2, m_{W_H^3}^2 \right) \Gamma_{\tilde{f}^0_{Po,j}, W_H^3, f_{Po,b}^0}^{R*} m_{f_{Po,b}^0} \Gamma_{\tilde{f}^0_{Po,i}, W_H^3, f_{Po,b}^0}^L \\
& + B_0 \left( p^2, m_{\tilde{H}^0}^2, m_{H_d^0}^2 \right) \Gamma_{\tilde{f}^0_{Po,j}, H_d^0, \text{FH0D}(\{1\})}^{L*} m_{\tilde{H}^0} \Gamma_{\tilde{f}^0_{Po,i}, H_d^0, \text{FH0D}(\{1\})}^R + B_0 \left( p^2, m_{\tilde{H}^-}^2, m_{H_d^-}^2 \right) \Gamma_{\tilde{f}^0_{Po,j}, H_d^-, \text{FHCD}(\{1\})}^{L*} m_{\tilde{H}^-} \\
& + B_0 \left( p^2, m_{\tilde{H}^0}^2, m_{H_u^0}^2 \right) \Gamma_{\tilde{f}^0_{Po,j}, H_u^0, \text{FH0D}(\{1\})}^{L*} m_{\tilde{H}^0} \Gamma_{\tilde{f}^0_{Po,i}, H_u^0, \text{FH0D}(\{1\})}^R \\
& + B_0 \left( p^2, m_{\tilde{H}^-}^2, m_{H_u^+}^2 \right) \Gamma_{\tilde{f}^0_{Po,j}, H_u^+, \text{FHCD}(\{1\})}^{L*} m_{\tilde{H}^-} \Gamma_{\tilde{f}^0_{Po,i}, H_u^+, \text{FHCD}(\{1\})}^R \tag{342}
\end{aligned}$$

$$\begin{aligned}
\Sigma_{i,j}^L(p^2) = & + \sum_{a=1}^2 \sum_{b=1}^{10} B_0 \left( p^2, m_{f_{Po,b}^0}^2, m_{\phi_{AK,a}^s}^2 \right) \Gamma_{\tilde{f}^0_{Po,j}, \phi_{AK,a}^{s,*}, f_{Po,b}^0}^{L*} m_{f_{Po,b}^0} \Gamma_{\tilde{f}^0_{Po,i}, \phi_{AK,a}^{s,*}, f_{Po,b}^0}^R \\
& + 3 \sum_{a=1}^3 \sum_{b=1}^3 B_0 \left( p^2, m_{d_{L,b}^D}^2, m_{d_{L,a}^D}^2 \right) \Gamma_{\tilde{f}^0_{Po,j}, \tilde{d}_{L,a}^*, d_{L,b}^D}^{L*} m_{d_{L,b}^D} \Gamma_{\tilde{f}^0_{Po,i}, \tilde{d}_{L,a}^*, d_{L,b}^D}^R \\
& + 3 \sum_{a=1}^3 \sum_{b=1}^3 B_0 \left( p^2, m_{d_{R,b}^D}^2, m_{d_{R,a}^D}^2 \right) \Gamma_{\tilde{f}^0_{Po,j}, \tilde{d}_{R,a}^*, d_{R,b}^D}^{L*} m_{d_{R,b}^D} \Gamma_{\tilde{f}^0_{Po,i}, \tilde{d}_{R,a}^*, d_{R,b}^D}^R \\
& + \sum_{a=1}^3 \sum_{b=1}^3 B_0 \left( p^2, m_{e_{L,b}^D}^2, m_{e_{L,a}^D}^2 \right) \Gamma_{\tilde{f}^0_{Po,j}, \tilde{e}_{L,a}^*, e_{L,b}^D}^{L*} m_{e_{L,b}^D} \Gamma_{\tilde{f}^0_{Po,i}, \tilde{e}_{L,a}^*, e_{L,b}^D}^R \\
& + \sum_{a=1}^3 \sum_{b=1}^3 B_0 \left( p^2, m_{e_{R,b}^D}^2, m_{e_{R,a}^D}^2 \right) \Gamma_{\tilde{f}^0_{Po,j}, \tilde{e}_{R,a}^*, e_{R,b}^D}^{L*} m_{e_{R,b}^D} \Gamma_{\tilde{f}^0_{Po,i}, \tilde{e}_{R,a}^*, e_{R,b}^D}^R \\
& + 3 \sum_{a=1}^3 \sum_{b=1}^3 B_0 \left( p^2, m_{u_{L,b}^D}^2, m_{u_{L,a}^D}^2 \right) \Gamma_{\tilde{f}^0_{Po,j}, \tilde{u}_{L,a}^*, u_{L,b}^D}^{L*} m_{u_{L,b}^D} \Gamma_{\tilde{f}^0_{Po,i}, \tilde{u}_{L,a}^*, u_{L,b}^D}^R \\
& + 3 \sum_{a=1}^3 \sum_{b=1}^3 B_0 \left( p^2, m_{u_{R,b}^D}^2, m_{u_{R,a}^D}^2 \right) \Gamma_{\tilde{f}^0_{Po,j}, \tilde{u}_{R,a}^*, u_{R,b}^D}^{L*} m_{u_{R,b}^D} \Gamma_{\tilde{f}^0_{Po,i}, \tilde{u}_{R,a}^*, u_{R,b}^D}^R \\
& + \sum_{a=1}^3 \sum_{b=1}^3 B_0 \left( p^2, m_{\nu_{L,b}^D}^2, m_{\nu_{L,a}^D}^2 \right) \Gamma_{\tilde{f}^0_{Po,j}, \tilde{\nu}_{L,a}^*, \nu_{L,b}^D}^{L*} m_{\nu_{L,b}^D} \Gamma_{\tilde{f}^0_{Po,i}, \tilde{\nu}_{L,a}^*, \nu_{L,b}^D}^R \\
& + \sum_{a=1}^4 \sum_{b=1}^{10} B_0 \left( p^2, m_{f_{Go,b}^-}^2, m_{\sigma_{L,a}^\pm}^2 \right) \Gamma_{\tilde{f}^0_{Po,j}, \sigma_{L,a}^{\pm,*}, f_{Go,b}^-}^{L*} m_{f_{Go,b}^-} \Gamma_{\tilde{f}^0_{Po,i}, \sigma_{L,a}^{\pm,*}, f_{Go,b}^-}^R \\
& + \frac{1}{2} \sum_{a=1}^4 \sum_{b=1}^{10} B_0 \left( p^2, m_{f_{Po,b}^0}^2, m_{\sigma_{L,a}^0}^2 \right) \Gamma_{\tilde{f}^0_{Po,j}, \sigma_{L,a}^0, f_{Po,b}^0}^{L*} m_{f_{Po,b}^0} \Gamma_{\tilde{f}^0_{Po,i}, \sigma_{L,a}^0, f_{Po,b}^0}^R \\
& + \sum_{a=1}^{10} m_{f_{Go,a}^-} \sum_{b=1}^2 B_0 \left( p^2, m_{f_{Go,a}^-}^2, m_{\phi_{B,b}^s}^2 \right) \Gamma_{\tilde{f}^0_{Po,j}, f_{Go,a}^-, \phi_{B,b}^s}^{L*} \Gamma_{\tilde{f}^0_{Po,i}, f_{Go,a}^-, \phi_{B,b}^s}^R \\
& + \frac{1}{2} \sum_{a=1}^{10} m_{f_{Po,a}^0} \sum_{b=1}^4 B_0 \left( p^2, m_{f_{Po,a}^0}^2, m_{\phi_{L,b}^0}^2 \right) \Gamma_{\tilde{f}^0_{Po,j}, f_{Po,a}^0, \phi_{L,b}^0}^{L*} \Gamma_{\tilde{f}^0_{Po,i}, f_{Po,a}^0, \phi_{L,b}^0}^R
\end{aligned}$$

$$\begin{aligned}
& -2 \sum_{b=1}^{10} B_0 \left( p^2, m_{f_{Po,b}^0}^2, m_{B_L}^2 \right) \Gamma_{\tilde{f}^0 Po, j, B_L, f_{Po,b}^0}^{R*} m_{f_{Po,b}^0} \Gamma_{\tilde{f}^0 Po, i, B_L, f_{Po,b}^0}^L \\
& -2 \sum_{b=1}^{10} B_0 \left( p^2, m_{f_{Po,b}^0}^2, m_{B_H}^2 \right) \Gamma_{\tilde{f}^0 Po, j, B_H, f_{Po,b}^0}^{R*} m_{f_{Po,b}^0} \Gamma_{\tilde{f}^0 Po, i, B_H, f_{Po,b}^0}^L \\
& -2 \sum_{b=1}^{10} B_0 \left( p^2, m_{f_{Go,b}^-}^2, m_{W_L^1}^2 \right) \Gamma_{\tilde{f}^0 Po, j, W_L^1, f_{Go,b}^-}^{R*} m_{f_{Go,b}^-} \Gamma_{\tilde{f}^0 Po, i, W_L^1, f_{Go,b}^-}^L \\
& -2 \sum_{b=1}^{10} B_0 \left( p^2, m_{f_{Go,b}^-}^2, m_{W_H^1}^2 \right) \Gamma_{\tilde{f}^0 Po, j, W_H^1, f_{Go,b}^-}^{R*} m_{f_{Go,b}^-} \Gamma_{\tilde{f}^0 Po, i, W_H^1, f_{Go,b}^-}^L \\
& -2 \sum_{b=1}^{10} B_0 \left( p^2, m_{f_{Go,b}^-}^2, m_{W_L^2}^2 \right) \Gamma_{\tilde{f}^0 Po, j, W_L^2, f_{Go,b}^-}^{R*} m_{f_{Go,b}^-} \Gamma_{\tilde{f}^0 Po, i, W_L^2, f_{Go,b}^-}^L \\
& -2 \sum_{b=1}^{10} B_0 \left( p^2, m_{f_{Go,b}^-}^2, m_{W_H^2}^2 \right) \Gamma_{\tilde{f}^0 Po, j, W_H^2, f_{Go,b}^-}^{R*} m_{f_{Go,b}^-} \Gamma_{\tilde{f}^0 Po, i, W_H^2, f_{Go,b}^-}^L \\
& -2 \sum_{b=1}^{10} B_0 \left( p^2, m_{f_{Po,b}^0}^2, m_{W_L^3}^2 \right) \Gamma_{\tilde{f}^0 Po, j, W_L^3, f_{Po,b}^0}^{R*} m_{f_{Po,b}^0} \Gamma_{\tilde{f}^0 Po, i, W_L^3, f_{Po,b}^0}^L \\
& -2 \sum_{b=1}^{10} B_0 \left( p^2, m_{f_{Po,b}^0}^2, m_{W_H^3}^2 \right) \Gamma_{\tilde{f}^0 Po, j, W_H^3, f_{Po,b}^0}^{R*} m_{f_{Po,b}^0} \Gamma_{\tilde{f}^0 Po, i, W_H^3, f_{Po,b}^0}^L \\
& + B_0 \left( p^2, m_{\tilde{H}^0}^2, m_{H_d^0}^2 \right) \Gamma_{\tilde{f}^0 Po, j, H_d^0, \text{FH0D}(\{1\})}^{L*} m_{\tilde{H}^0} \Gamma_{\tilde{f}^0 Po, i, H_d^0, \text{FH0D}(\{1\})}^R + B_0 \left( p^2, m_{\tilde{H}^-}^2, m_{H_d^-}^2 \right) \Gamma_{\tilde{f}^0 Po, j, H_d^-, \text{FHCD}(\{1\})}^{L*} m_{\tilde{H}^-} \\
& + B_0 \left( p^2, m_{\tilde{H}^0}^2, m_{H_u^0}^2 \right) \Gamma_{\tilde{f}^0 Po, j, H_u^0, \text{FH0D}(\{1\})}^{L*} m_{\tilde{H}^0} \Gamma_{\tilde{f}^0 Po, i, H_u^0, \text{FH0D}(\{1\})}^R \\
& + B_0 \left( p^2, m_{\tilde{H}^-}^2, m_{H_u^+}^2 \right) \Gamma_{\tilde{f}^0 Po, j, H_u^+, \text{FHCD}(\{1\})}^{L*} m_{\tilde{H}^-} \Gamma_{\tilde{f}^0 Po, i, H_u^+, \text{FHCD}(\{1\})}^R \tag{343}
\end{aligned}$$

• **Self-Energy for Linking/Ad charged fermion mass eigenstates after AxB breaking** ( $f_{Go}^-$ )

$$\begin{aligned}
\Sigma_{i,j}^S(p^2) = & + \sum_{a=1}^2 \sum_{b=1}^{10} B_0 \left( p^2, m_{f_{Go,b}^-}^2, m_{\phi_{AK,a}^s}^2 \right) \Gamma_{\tilde{f}^- Go, j, \phi_{AK,a}^{s,*}, f_{Go,b}^-}^{L*} m_{f_{Go,b}^-} \Gamma_{\tilde{f}^- Go, i, \phi_{AK,a}^{s,*}, f_{Go,b}^-}^R \\
& + 3 \sum_{a=1}^3 \sum_{b=1}^3 B_0 \left( p^2, m_{u_{L,b}^D}^2, m_{d_{L,a}^D}^2 \right) \Gamma_{\tilde{f}^- Go, j, \tilde{d}_{L,a}^*, u_{L,b}^D}^{L*} m_{u_{L,b}^D} \Gamma_{\tilde{f}^- Go, i, \tilde{d}_{L,a}^*, u_{L,b}^D}^R \\
& + \sum_{a=1}^3 \sum_{b=1}^3 B_0 \left( p^2, m_{\nu_{L,b}^D}^2, m_{\tilde{e}_{L,a}^D}^2 \right) \Gamma_{\tilde{f}^- Go, j, \tilde{e}_{L,a}^*, \nu_{L,b}^D}^{L*} m_{\nu_{L,b}^D} \Gamma_{\tilde{f}^- Go, i, \tilde{e}_{L,a}^*, \nu_{L,b}^D}^R \\
& + 3 \sum_{a=1}^3 \sum_{b=1}^3 B_0 \left( p^2, m_{d_{L,b}^D}^2, m_{\tilde{u}_{L,a}^D}^2 \right) \Gamma_{\tilde{f}^- Go, j, \tilde{u}_{L,a}^*, d_{L,b}^D}^{L*} m_{d_{L,b}^D} \Gamma_{\tilde{f}^- Go, i, \tilde{u}_{L,a}^*, d_{L,b}^D}^R
\end{aligned}$$

$$\begin{aligned}
& + \sum_{a=1}^3 \sum_{b=1}^3 B_0 \left( p^2, m_{e_{L,b}^D}^2, m_{\tilde{\nu}_{L,a}}^2 \right) \Gamma_{\tilde{f}^{-G o, j}, \tilde{\nu}_{L,a}^*, e_{L,b}^D}^{L*} m_{e_{L,b}^D} \Gamma_{\tilde{f}^{-G o, i}, \tilde{\nu}_{L,a}^*, e_{L,b}^D}^R \\
& + \frac{1}{2} \sum_{a=1}^4 \sum_{b=1}^{10} B_0 \left( p^2, m_{f_{G o, b}^-}^2, m_{\phi_{L,a}^0}^2 \right) \Gamma_{\tilde{f}^{-G o, j}, \phi_{L,a}^0, f_{G o, b}^-}^{L*} m_{f_{G o, b}^-} \Gamma_{\tilde{f}^{-G o, i}, \phi_{L,a}^0, f_{G o, b}^-}^R \\
& + \frac{1}{2} \sum_{a=1}^4 \sum_{b=1}^{10} B_0 \left( p^2, m_{f_{G o, b}^-}^2, m_{\sigma_{L,a}^0}^2 \right) \Gamma_{\tilde{f}^{-G o, j}, \sigma_{L,a}^0, f_{G o, b}^-}^{L*} m_{f_{G o, b}^-} \Gamma_{\tilde{f}^{-G o, i}, \sigma_{L,a}^0, f_{G o, b}^-}^R \\
& + \sum_{a=1}^{10} m_{f_{P o, a}^0} \sum_{b=1}^2 B_0 \left( p^2, m_{f_{P o, a}^0}^2, m_{\phi_{B,b}^*}^2 \right) \Gamma_{\tilde{f}^{-G o, j}, f_{P o, a}^0, \phi_{B,b}^*}^{L*} \Gamma_{\tilde{f}^{-G o, i}, f_{P o, a}^0, \phi_{B,b}^*}^R \\
& + \sum_{a=1}^{10} m_{f_{P o, a}^0} \sum_{b=1}^4 B_0 \left( p^2, m_{f_{P o, a}^0}^2, m_{\sigma_{L,b}^\pm}^2 \right) \Gamma_{\tilde{f}^{-G o, j}, f_{P o, a}^0, \sigma_{L,b}^\pm}^{L*} \Gamma_{\tilde{f}^{-G o, i}, f_{P o, a}^0, \sigma_{L,b}^\pm}^R \\
& - 2 \sum_{b=1}^{10} B_0 \left( p^2, m_{f_{G o, b}^-}^2, m_{B_L}^2 \right) \Gamma_{\tilde{f}^{-G o, j}, B_L, f_{G o, b}^-}^{R*} m_{f_{G o, b}^-} \Gamma_{\tilde{f}^{-G o, i}, B_L, f_{G o, b}^-}^L \\
& - 2 \sum_{b=1}^{10} B_0 \left( p^2, m_{f_{G o, b}^-}^2, m_{B_H}^2 \right) \Gamma_{\tilde{f}^{-G o, j}, B_H, f_{G o, b}^-}^{R*} m_{f_{G o, b}^-} \Gamma_{\tilde{f}^{-G o, i}, B_H, f_{G o, b}^-}^L \\
& - 2 \sum_{b=1}^{10} B_0 \left( p^2, m_{f_{P o, b}^0}^2, m_{W_L^1}^2 \right) \Gamma_{\tilde{f}^{-G o, j}, W_L^1, f_{P o, b}^0}^{R*} m_{f_{P o, b}^0} \Gamma_{\tilde{f}^{-G o, i}, W_L^1, f_{P o, b}^0}^L \\
& - 2 \sum_{b=1}^{10} B_0 \left( p^2, m_{f_{P o, b}^0}^2, m_{W_H^1}^2 \right) \Gamma_{\tilde{f}^{-G o, j}, W_H^1, f_{P o, b}^0}^{R*} m_{f_{P o, b}^0} \Gamma_{\tilde{f}^{-G o, i}, W_H^1, f_{P o, b}^0}^L \\
& - 2 \sum_{b=1}^{10} B_0 \left( p^2, m_{f_{P o, b}^0}^2, m_{W_L^2}^2 \right) \Gamma_{\tilde{f}^{-G o, j}, W_L^2, f_{P o, b}^0}^{R*} m_{f_{P o, b}^0} \Gamma_{\tilde{f}^{-G o, i}, W_L^2, f_{P o, b}^0}^L \\
& - 2 \sum_{b=1}^{10} B_0 \left( p^2, m_{f_{P o, b}^0}^2, m_{W_H^2}^2 \right) \Gamma_{\tilde{f}^{-G o, j}, W_H^2, f_{P o, b}^0}^{R*} m_{f_{P o, b}^0} \Gamma_{\tilde{f}^{-G o, i}, W_H^2, f_{P o, b}^0}^L \\
& - 2 \sum_{b=1}^{10} B_0 \left( p^2, m_{f_{G o, b}^-}^2, m_{W_L^3}^2 \right) \Gamma_{\tilde{f}^{-G o, j}, W_L^3, f_{G o, b}^-}^{R*} m_{f_{G o, b}^-} \Gamma_{\tilde{f}^{-G o, i}, W_L^3, f_{G o, b}^-}^L \\
& - 2 \sum_{b=1}^{10} B_0 \left( p^2, m_{f_{G o, b}^-}^2, m_{W_H^3}^2 \right) \Gamma_{\tilde{f}^{-G o, j}, W_H^3, f_{G o, b}^-}^{R*} m_{f_{G o, b}^-} \Gamma_{\tilde{f}^{-G o, i}, W_H^3, f_{G o, b}^-}^L \\
& + B_0 \left( p^2, m_{\tilde{H}^-}^2, m_{H_d^0}^2 \right) \Gamma_{\tilde{f}^{-G o, j}, H_d^0, \text{FHCD}(\{1\})}^{L*} m_{\tilde{H}^-} \Gamma_{\tilde{f}^{-G o, i}, H_d^0, \text{FHCD}(\{1\})}^R + B_0 \left( p^2, m_{\tilde{H}^0}^2, m_{H_d^-}^2 \right) \Gamma_{\tilde{f}^{-G o, j}, H_d^-, \text{FH0D}(\{1\})}^{L*} m_{\tilde{H}^0} \\
& + B_0 \left( p^2, m_{\tilde{H}^-}^2, m_{H_u^0}^2 \right) \Gamma_{\tilde{f}^{-G o, j}, H_u^0, *, \text{FHCD}(\{1\})}^{L*} m_{\tilde{H}^-} \Gamma_{\tilde{f}^{-G o, i}, H_u^0, *, \text{FHCD}(\{1\})}^R \\
& + B_0 \left( p^2, m_{\tilde{H}^0}^2, m_{H_u^+}^2 \right) \Gamma_{\tilde{f}^{-G o, j}, H_u^+, *, \text{FH0D}(\{1\})}^{L*} m_{\tilde{H}^0} \Gamma_{\tilde{f}^{-G o, i}, H_u^+, *, \text{FH0D}(\{1\})}^R
\end{aligned} \tag{344}$$

$$\begin{aligned}
\Sigma_{i,j}^R(p^2) = & + \sum_{a=1}^2 \sum_{b=1}^{10} B_0 \left( p^2, m_{f_{Go,b}^-}^2, m_{\phi_{AK,a}^s}^2 \right) \Gamma_{\tilde{f}^{-Go,j}, \phi_{AK,a}^{s,*}, f_{Go,b}^-}^{L*} m_{f_{Go,b}^-} \Gamma_{\tilde{f}^{-Go,i}, \phi_{AK,a}^{s,*}, f_{Go,b}^-}^R \\
& + 3 \sum_{a=1}^3 \sum_{b=1}^3 B_0 \left( p^2, m_{u_{L,b}^D}^2, m_{\tilde{d}_{L,a}}^2 \right) \Gamma_{\tilde{f}^{-Go,j}, \tilde{d}_{L,a}^*, u_{L,b}^D}^{L*} m_{u_{L,b}^D} \Gamma_{\tilde{f}^{-Go,i}, \tilde{d}_{L,a}^*, u_{L,b}^D}^R \\
& + \sum_{a=1}^3 \sum_{b=1}^3 B_0 \left( p^2, m_{\nu_{L,b}^D}^2, m_{\tilde{e}_{L,a}}^2 \right) \Gamma_{\tilde{f}^{-Go,j}, \tilde{e}_{L,a}^*, \nu_{L,b}^D}^{L*} m_{\nu_{L,b}^D} \Gamma_{\tilde{f}^{-Go,i}, \tilde{e}_{L,a}^*, \nu_{L,b}^D}^R \\
& + 3 \sum_{a=1}^3 \sum_{b=1}^3 B_0 \left( p^2, m_{d_{L,b}^D}^2, m_{\tilde{u}_{L,a}}^2 \right) \Gamma_{\tilde{f}^{-Go,j}, \tilde{u}_{L,a}^*, d_{L,b}^D}^{L*} m_{d_{L,b}^D} \Gamma_{\tilde{f}^{-Go,i}, \tilde{u}_{L,a}^*, d_{L,b}^D}^R \\
& + \sum_{a=1}^3 \sum_{b=1}^3 B_0 \left( p^2, m_{e_{L,b}^D}^2, m_{\tilde{\nu}_{L,a}}^2 \right) \Gamma_{\tilde{f}^{-Go,j}, \tilde{\nu}_{L,a}^*, e_{L,b}^D}^{L*} m_{e_{L,b}^D} \Gamma_{\tilde{f}^{-Go,i}, \tilde{\nu}_{L,a}^*, e_{L,b}^D}^R \\
& + \frac{1}{2} \sum_{a=1}^4 \sum_{b=1}^{10} B_0 \left( p^2, m_{f_{Go,b}^-}^2, m_{\phi_{L,a}^0}^2 \right) \Gamma_{\tilde{f}^{-Go,j}, \phi_{L,a}^0, f_{Go,b}^-}^{L*} m_{f_{Go,b}^-} \Gamma_{\tilde{f}^{-Go,i}, \phi_{L,a}^0, f_{Go,b}^-}^R \\
& + \frac{1}{2} \sum_{a=1}^4 \sum_{b=1}^{10} B_0 \left( p^2, m_{f_{Go,b}^-}^2, m_{\sigma_{L,a}^0}^2 \right) \Gamma_{\tilde{f}^{-Go,j}, \sigma_{L,a}^0, f_{Go,b}^-}^{L*} m_{f_{Go,b}^-} \Gamma_{\tilde{f}^{-Go,i}, \sigma_{L,a}^0, f_{Go,b}^-}^R \\
& + \sum_{a=1}^{10} m_{f_{Po,a}^0} \sum_{b=1}^2 B_0 \left( p^2, m_{f_{Po,a}^0}^2, m_{\phi_{B,b}^s}^2 \right) \Gamma_{\tilde{f}^{-Go,j}, f_{Po,a}^0, \phi_{B,b}^s}^{L*} \Gamma_{\tilde{f}^{-Go,i}, f_{Po,a}^0, \phi_{B,b}^s}^R \\
& + \sum_{a=1}^{10} m_{f_{Po,a}^0} \sum_{b=1}^4 B_0 \left( p^2, m_{f_{Po,a}^0}^2, m_{\sigma_{L,b}^\pm}^2 \right) \Gamma_{\tilde{f}^{-Go,j}, f_{Po,a}^0, \sigma_{L,b}^\pm}^{L*} \Gamma_{\tilde{f}^{-Go,i}, f_{Po,a}^0, \sigma_{L,b}^\pm}^R \\
& - 2 \sum_{b=1}^{10} B_0 \left( p^2, m_{f_{Go,b}^-}^2, m_{B_L}^2 \right) \Gamma_{\tilde{f}^{-Go,j}, B_L, f_{Go,b}^-}^{R*} m_{f_{Go,b}^-} \Gamma_{\tilde{f}^{-Go,i}, B_L, f_{Go,b}^-}^L \\
& - 2 \sum_{b=1}^{10} B_0 \left( p^2, m_{f_{Go,b}^-}^2, m_{B_H}^2 \right) \Gamma_{\tilde{f}^{-Go,j}, B_H, f_{Go,b}^-}^{R*} m_{f_{Go,b}^-} \Gamma_{\tilde{f}^{-Go,i}, B_H, f_{Go,b}^-}^L \\
& - 2 \sum_{b=1}^{10} B_0 \left( p^2, m_{f_{Po,b}^0}^2, m_{W_L^1}^2 \right) \Gamma_{\tilde{f}^{-Go,j}, W_L^1, f_{Po,b}^0}^{R*} m_{f_{Po,b}^0} \Gamma_{\tilde{f}^{-Go,i}, W_L^1, f_{Po,b}^0}^L \\
& - 2 \sum_{b=1}^{10} B_0 \left( p^2, m_{f_{Po,b}^0}^2, m_{W_H^1}^2 \right) \Gamma_{\tilde{f}^{-Go,j}, W_H^1, f_{Po,b}^0}^{R*} m_{f_{Po,b}^0} \Gamma_{\tilde{f}^{-Go,i}, W_H^1, f_{Po,b}^0}^L \\
& - 2 \sum_{b=1}^{10} B_0 \left( p^2, m_{f_{Po,b}^0}^2, m_{W_L^2}^2 \right) \Gamma_{\tilde{f}^{-Go,j}, W_L^2, f_{Po,b}^0}^{R*} m_{f_{Po,b}^0} \Gamma_{\tilde{f}^{-Go,i}, W_L^2, f_{Po,b}^0}^L \\
& - 2 \sum_{b=1}^{10} B_0 \left( p^2, m_{f_{Po,b}^0}^2, m_{W_H^2}^2 \right) \Gamma_{\tilde{f}^{-Go,j}, W_H^2, f_{Po,b}^0}^{R*} m_{f_{Po,b}^0} \Gamma_{\tilde{f}^{-Go,i}, W_H^2, f_{Po,b}^0}^L
\end{aligned}$$

$$\begin{aligned}
& -2 \sum_{b=1}^{10} B_0 \left( p^2, m_{f_{G o, b}^-}^2, m_{W_L^3}^2 \right) \Gamma_{\check{f}^{-G o, j}, W_L^3, f_{G o, b}^-}^{R*} m_{f_{G o, b}^-} \Gamma_{\check{f}^{-G o, i}, W_L^3, f_{G o, b}^-}^L \\
& -2 \sum_{b=1}^{10} B_0 \left( p^2, m_{f_{G o, b}^-}^2, m_{W_H^3}^2 \right) \Gamma_{\check{f}^{-G o, j}, W_H^3, f_{G o, b}^-}^{R*} m_{f_{G o, b}^-} \Gamma_{\check{f}^{-G o, i}, W_H^3, f_{G o, b}^-}^L \\
& + B_0 \left( p^2, m_{\tilde{H}^-}^2, m_{H_d^0}^2 \right) \Gamma_{\check{f}^{-G o, j}, H_d^0, \text{FHCD}(\{1\})}^{L*} m_{\tilde{H}^-} \Gamma_{\check{f}^{-G o, i}, H_d^0, \text{FHCD}(\{1\})}^R + B_0 \left( p^2, m_{\tilde{H}^0}^2, m_{H_d^-}^2 \right) \Gamma_{\check{f}^{-G o, j}, H_d^-, \text{FH0D}(\{1\})}^{L*} m_{\tilde{H}^0} \\
& + B_0 \left( p^2, m_{\tilde{H}^-}^2, m_{H_u^0}^2 \right) \Gamma_{\check{f}^{-G o, j}, H_u^{0,*}, \text{FHCD}(\{1\})}^{L*} m_{\tilde{H}^-} \Gamma_{\check{f}^{-G o, i}, H_u^{0,*}, \text{FHCD}(\{1\})}^R \\
& + B_0 \left( p^2, m_{\tilde{H}^0}^2, m_{H_u^+}^2 \right) \Gamma_{\check{f}^{-G o, j}, H_u^{+,*}, \text{FH0D}(\{1\})}^{L*} m_{\tilde{H}^0} \Gamma_{\check{f}^{-G o, i}, H_u^{+,*}, \text{FH0D}(\{1\})}^R \tag{345}
\end{aligned}$$

$$\begin{aligned}
\Sigma_{i,j}^L(p^2) = & + \sum_{a=1}^2 \sum_{b=1}^{10} B_0 \left( p^2, m_{f_{G o, b}^-}^2, m_{\phi_{AK,a}^s}^2 \right) \Gamma_{\check{f}^{-G o, j}, \phi_{AK,a}^{s,*}, f_{G o, b}^-}^{L*} m_{f_{G o, b}^-} \Gamma_{\check{f}^{-G o, i}, \phi_{AK,a}^{s,*}, f_{G o, b}^-}^R \\
& + 3 \sum_{a=1}^3 \sum_{b=1}^3 B_0 \left( p^2, m_{u_{L,b}^D}^2, m_{\tilde{d}_{L,a}^*}^2 \right) \Gamma_{\check{f}^{-G o, j}, \tilde{d}_{L,a}^*, u_{L,b}^D}^{L*} m_{u_{L,b}^D} \Gamma_{\check{f}^{-G o, i}, \tilde{d}_{L,a}^*, u_{L,b}^D}^R \\
& + \sum_{a=1}^3 \sum_{b=1}^3 B_0 \left( p^2, m_{\nu_{L,b}^D}^2, m_{\tilde{e}_{L,a}^*}^2 \right) \Gamma_{\check{f}^{-G o, j}, \tilde{e}_{L,a}^*, \nu_{L,b}^D}^{L*} m_{\nu_{L,b}^D} \Gamma_{\check{f}^{-G o, i}, \tilde{e}_{L,a}^*, \nu_{L,b}^D}^R \\
& + 3 \sum_{a=1}^3 \sum_{b=1}^3 B_0 \left( p^2, m_{d_{L,b}^D}^2, m_{\tilde{u}_{L,a}^*}^2 \right) \Gamma_{\check{f}^{-G o, j}, \tilde{u}_{L,a}^*, d_{L,b}^D}^{L*} m_{d_{L,b}^D} \Gamma_{\check{f}^{-G o, i}, \tilde{u}_{L,a}^*, d_{L,b}^D}^R \\
& + \sum_{a=1}^3 \sum_{b=1}^3 B_0 \left( p^2, m_{e_{L,b}^D}^2, m_{\tilde{\nu}_{L,a}^*}^2 \right) \Gamma_{\check{f}^{-G o, j}, \tilde{\nu}_{L,a}^*, e_{L,b}^D}^{L*} m_{e_{L,b}^D} \Gamma_{\check{f}^{-G o, i}, \tilde{\nu}_{L,a}^*, e_{L,b}^D}^R \\
& + \frac{1}{2} \sum_{a=1}^4 \sum_{b=1}^{10} B_0 \left( p^2, m_{f_{G o, b}^-}^2, m_{\phi_{L,a}^0}^2 \right) \Gamma_{\check{f}^{-G o, j}, \phi_{L,a}^0, f_{G o, b}^-}^{L*} m_{f_{G o, b}^-} \Gamma_{\check{f}^{-G o, i}, \phi_{L,a}^0, f_{G o, b}^-}^R \\
& + \frac{1}{2} \sum_{a=1}^4 \sum_{b=1}^{10} B_0 \left( p^2, m_{f_{G o, b}^-}^2, m_{\sigma_{L,a}^0}^2 \right) \Gamma_{\check{f}^{-G o, j}, \sigma_{L,a}^0, f_{G o, b}^-}^{L*} m_{f_{G o, b}^-} \Gamma_{\check{f}^{-G o, i}, \sigma_{L,a}^0, f_{G o, b}^-}^R \\
& + \sum_{a=1}^{10} m_{f_{P o, a}^0} \sum_{b=1}^2 B_0 \left( p^2, m_{f_{P o, a}^0}^2, m_{\phi_{B,b}^s}^2 \right) \Gamma_{\check{f}^{-G o, j}, f_{P o, a}^0, \phi_{B,b}^s}^{L*} \Gamma_{\check{f}^{-G o, i}, f_{P o, a}^0, \phi_{B,b}^s}^R \\
& + \sum_{a=1}^{10} m_{f_{P o, a}^0} \sum_{b=1}^4 B_0 \left( p^2, m_{f_{P o, a}^0}^2, m_{\sigma_{L,b}^\pm}^2 \right) \Gamma_{\check{f}^{-G o, j}, f_{P o, a}^0, \sigma_{L,b}^\pm}^{L*} \Gamma_{\check{f}^{-G o, i}, f_{P o, a}^0, \sigma_{L,b}^\pm}^R \\
& - 2 \sum_{b=1}^{10} B_0 \left( p^2, m_{f_{G o, b}^-}^2, m_{B_L}^2 \right) \Gamma_{\check{f}^{-G o, j}, B_L, f_{G o, b}^-}^{R*} m_{f_{G o, b}^-} \Gamma_{\check{f}^{-G o, i}, B_L, f_{G o, b}^-}^L \\
& - 2 \sum_{b=1}^{10} B_0 \left( p^2, m_{f_{G o, b}^-}^2, m_{B_H}^2 \right) \Gamma_{\check{f}^{-G o, j}, B_H, f_{G o, b}^-}^{R*} m_{f_{G o, b}^-} \Gamma_{\check{f}^{-G o, i}, B_H, f_{G o, b}^-}^L
\end{aligned}$$

$$\begin{aligned}
& -2 \sum_{b=1}^{10} B_0(p^2, m_{f_{Po,b}^0}^2, m_{W_L^1}^2) \Gamma_{\tilde{f}^{-Go,j}, W_L^1, f_{Po,b}^0}^{R*} m_{f_{Po,b}^0} \Gamma_{\tilde{f}^{-Go,i}, W_L^1, f_{Po,b}^0}^L \\
& -2 \sum_{b=1}^{10} B_0(p^2, m_{f_{Po,b}^0}^2, m_{W_H^1}^2) \Gamma_{\tilde{f}^{-Go,j}, W_H^1, f_{Po,b}^0}^{R*} m_{f_{Po,b}^0} \Gamma_{\tilde{f}^{-Go,i}, W_H^1, f_{Po,b}^0}^L \\
& -2 \sum_{b=1}^{10} B_0(p^2, m_{f_{Po,b}^0}^2, m_{W_L^2}^2) \Gamma_{\tilde{f}^{-Go,j}, W_L^2, f_{Po,b}^0}^{R*} m_{f_{Po,b}^0} \Gamma_{\tilde{f}^{-Go,i}, W_L^2, f_{Po,b}^0}^L \\
& -2 \sum_{b=1}^{10} B_0(p^2, m_{f_{Po,b}^0}^2, m_{W_H^2}^2) \Gamma_{\tilde{f}^{-Go,j}, W_H^2, f_{Po,b}^0}^{R*} m_{f_{Po,b}^0} \Gamma_{\tilde{f}^{-Go,i}, W_H^2, f_{Po,b}^0}^L \\
& -2 \sum_{b=1}^{10} B_0(p^2, m_{f_{Go,b}^-}^2, m_{W_L^3}^2) \Gamma_{\tilde{f}^{-Go,j}, W_L^3, f_{Go,b}^-}^{R*} m_{f_{Go,b}^-} \Gamma_{\tilde{f}^{-Go,i}, W_L^3, f_{Go,b}^-}^L \\
& -2 \sum_{b=1}^{10} B_0(p^2, m_{f_{Go,b}^-}^2, m_{W_H^3}^2) \Gamma_{\tilde{f}^{-Go,j}, W_H^3, f_{Go,b}^-}^{R*} m_{f_{Go,b}^-} \Gamma_{\tilde{f}^{-Go,i}, W_H^3, f_{Go,b}^-}^L \\
& + B_0(p^2, m_{\tilde{H}^-}^2, m_{H_d^0}^2) \Gamma_{\tilde{f}^{-Go,j}, H_d^0, \text{FHCD}(\{1\})}^{L*} m_{\tilde{H}^-} \Gamma_{\tilde{f}^{-Go,i}, H_d^0, \text{FHCD}(\{1\})}^R + B_0(p^2, m_{\tilde{H}^0}^2, m_{H_d^-}^2) \Gamma_{\tilde{f}^{-Go,j}, H_d^-, \text{FH0D}(\{1\})}^{L*} m_{\tilde{H}^0} \\
& + B_0(p^2, m_{\tilde{H}^-}^2, m_{H_u^0}^2) \Gamma_{\tilde{f}^{-Go,j}, H_u^0, \text{FHCD}(\{1\})}^{L*} m_{\tilde{H}^-} \Gamma_{\tilde{f}^{-Go,i}, H_u^0, \text{FHCD}(\{1\})}^R \\
& + B_0(p^2, m_{\tilde{H}^0}^2, m_{H_u^+}^2) \Gamma_{\tilde{f}^{-Go,j}, H_u^+, \text{FH0D}(\{1\})}^{L*} m_{\tilde{H}^0} \Gamma_{\tilde{f}^{-Go,i}, H_u^+, \text{FH0D}(\{1\})}^R
\end{aligned} \tag{346}$$

• Self-Energy for Neutral higgsino Majorana spinor ( $\tilde{H}^0$ )

$$\begin{aligned}
\Sigma^S(p^2) = & +3 \sum_{a=1}^3 m_{\tilde{d}^{D_R,a}} \sum_{b=1}^3 B_0(p^2, m_{d_{R,a}^D}^2, m_{\tilde{d}_{L,b}}^2) \Gamma_{\text{FH0D}(\{\text{gO2}\}), \tilde{d}^{D_R,a}, \tilde{d}_{L,b}}^{L*} \Gamma_{\text{FH0D}(\{\text{gO1}\}), \tilde{d}^{D_R,a}, \tilde{d}_{L,b}}^R \\
& + \sum_{a=1}^3 m_{\tilde{e}^{D_R,a}} \sum_{b=1}^3 B_0(p^2, m_{e_{R,a}^D}^2, m_{\tilde{e}_{L,b}}^2) \Gamma_{\text{FH0D}(\{\text{gO2}\}), \tilde{e}^{D_R,a}, \tilde{e}_{L,b}}^{L*} \Gamma_{\text{FH0D}(\{\text{gO1}\}), \tilde{e}^{D_R,a}, \tilde{e}_{L,b}}^R \\
& + 3 \sum_{a=1}^3 m_{\tilde{u}^{D_L,a}} \sum_{b=1}^3 B_0(p^2, m_{u_{L,a}^D}^2, m_{\tilde{u}_{R,b}}^2) \Gamma_{\text{FH0D}(\{\text{gO2}\}), \tilde{u}^{D_L,a}, \tilde{u}_{R,b}}^{L*} \Gamma_{\text{FH0D}(\{\text{gO1}\}), \tilde{u}^{D_L,a}, \tilde{u}_{R,b}}^R \\
& + 3 \sum_{a=1}^3 \sum_{b=1}^3 B_0(p^2, m_{d_{L,b}^D}^2, m_{\tilde{d}_{R,a}}^2) \Gamma_{\text{FH0D}(\{\text{gO2}\}), \tilde{d}_{R,a}^*, d_{L,b}^D}^{L*} m_{d_{L,b}^D} \Gamma_{\text{FH0D}(\{\text{gO1}\}), \tilde{d}_{R,a}^*, d_{L,b}^D}^R \\
& + \sum_{a=1}^3 \sum_{b=1}^3 B_0(p^2, m_{e_{L,b}^D}^2, m_{\tilde{e}_{R,a}}^2) \Gamma_{\text{FH0D}(\{\text{gO2}\}), \tilde{e}_{R,a}^*, e_{L,b}^D}^{L*} m_{e_{L,b}^D} \Gamma_{\text{FH0D}(\{\text{gO1}\}), \tilde{e}_{R,a}^*, e_{L,b}^D}^R
\end{aligned}$$

$$\begin{aligned}
& + 3 \sum_{a=1}^3 \sum_{b=1}^3 B_0 \left( p^2, m_{u_{R,b}^D}^2, m_{\tilde{u}_{L,a}}^2 \right) \Gamma_{\text{FH0D}(\{\text{gO2}\}), \tilde{u}_{L,a}^*, u_{R,b}^D}^{L*} m_{u_{R,b}^D} \Gamma_{\text{FH0D}(\{\text{gO1}\}), \tilde{u}_{L,a}^*, u_{R,b}^D}^R \\
& + \sum_{b=1}^{10} B_0 \left( p^2, m_{f_{Po,b}^0}^2, m_{H_u^0}^2 \right) \Gamma_{\text{FH0D}(\{\text{gO2}\}), H_u^0, f_{Po,b}^0}^{L*} m_{f_{Po,b}^0} \Gamma_{\text{FH0D}(\{\text{gO1}\}), H_u^0, f_{Po,b}^0}^R \\
& + \sum_{b=1}^{10} B_0 \left( p^2, m_{f_{Go,b}^-}^2, m_{H_u^+}^2 \right) \Gamma_{\text{FH0D}(\{\text{gO2}\}), H_u^+, f_{Go,b}^-}^{L*} m_{f_{Go,b}^-} \Gamma_{\text{FH0D}(\{\text{gO1}\}), H_u^+, f_{Go,b}^-}^R \\
& + \sum_{b=1}^{10} B_0 \left( p^2, m_{f_{Po,b}^0}^2, m_{H_d^0}^2 \right) \Gamma_{\text{FH0D}(\{\text{gO2}\}), H_d^{0,*}, f_{Po,b}^0}^{L*} m_{f_{Po,b}^0} \Gamma_{\text{FH0D}(\{\text{gO1}\}), H_d^{0,*}, f_{Po,b}^0}^R \\
& + \sum_{b=1}^{10} B_0 \left( p^2, m_{f_{Go,b}^-}^2, m_{H_d^-}^2 \right) \Gamma_{\text{FH0D}(\{\text{gO2}\}), H_d^{-,*}, f_{Go,b}^-}^{L*} m_{f_{Go,b}^-} \Gamma_{\text{FH0D}(\{\text{gO1}\}), H_d^{-,*}, f_{Go,b}^-}^R \\
& - 4B_0 \left( p^2, m_{\tilde{H}^0}^2, m_{B_L}^2 \right) \Gamma_{\text{FH0D}(\{\text{gO2}\}), B_L, \text{FH0D}(\{1\})}^{R*} m_{\tilde{H}^0} \Gamma_{\text{FH0D}(\{\text{gO1}\}), B_L, \text{FH0D}(\{1\})}^L \\
& - 4B_0 \left( p^2, m_{\tilde{H}^0}^2, m_{B_H}^2 \right) \Gamma_{\text{FH0D}(\{\text{gO2}\}), B_H, \text{FH0D}(\{1\})}^{R*} m_{\tilde{H}^0} \Gamma_{\text{FH0D}(\{\text{gO1}\}), B_H, \text{FH0D}(\{1\})}^L \\
& - 4B_0 \left( p^2, m_{\tilde{H}^-}^2, m_{W_L^1}^2 \right) \Gamma_{\text{FH0D}(\{\text{gO2}\}), W_L^1, \text{FHCD}(\{1\})}^{R*} m_{\tilde{H}^-} \Gamma_{\text{FH0D}(\{\text{gO1}\}), W_L^1, \text{FHCD}(\{1\})}^L \\
& - 4B_0 \left( p^2, m_{\tilde{H}^-}^2, m_{W_H^1}^2 \right) \Gamma_{\text{FH0D}(\{\text{gO2}\}), W_H^1, \text{FHCD}(\{1\})}^{R*} m_{\tilde{H}^-} \Gamma_{\text{FH0D}(\{\text{gO1}\}), W_H^1, \text{FHCD}(\{1\})}^L \\
& - 4B_0 \left( p^2, m_{\tilde{H}^-}^2, m_{W_L^2}^2 \right) \Gamma_{\text{FH0D}(\{\text{gO2}\}), W_L^2, \text{FHCD}(\{1\})}^{R*} m_{\tilde{H}^-} \Gamma_{\text{FH0D}(\{\text{gO1}\}), W_L^2, \text{FHCD}(\{1\})}^L \\
& - 4B_0 \left( p^2, m_{\tilde{H}^-}^2, m_{W_H^2}^2 \right) \Gamma_{\text{FH0D}(\{\text{gO2}\}), W_H^2, \text{FHCD}(\{1\})}^{R*} m_{\tilde{H}^-} \Gamma_{\text{FH0D}(\{\text{gO1}\}), W_H^2, \text{FHCD}(\{1\})}^L \\
& - 4B_0 \left( p^2, m_{\tilde{H}^0}^2, m_{W_L^3}^2 \right) \Gamma_{\text{FH0D}(\{\text{gO2}\}), W_L^3, \text{FH0D}(\{1\})}^{R*} m_{\tilde{H}^0} \Gamma_{\text{FH0D}(\{\text{gO1}\}), W_L^3, \text{FH0D}(\{1\})}^L \\
& - 4B_0 \left( p^2, m_{\tilde{H}^0}^2, m_{W_H^3}^2 \right) \Gamma_{\text{FH0D}(\{\text{gO2}\}), W_H^3, \text{FH0D}(\{1\})}^{R*} m_{\tilde{H}^0} \Gamma_{\text{FH0D}(\{\text{gO1}\}), W_H^3, \text{FH0D}(\{1\})}^L \tag{347}
\end{aligned}$$

$$\begin{aligned}
\Sigma^R(p^2) = & + 3 \sum_{a=1}^3 m_{\tilde{d}^{D_{R,a}}} \sum_{b=1}^3 B_0 \left( p^2, m_{d_{R,a}^D}^2, m_{\tilde{d}_{L,b}}^2 \right) \Gamma_{\text{FH0D}(\{\text{gO2}\}), \tilde{d}^{D_{R,a}}, \tilde{d}_{L,b}}^{L*} \Gamma_{\text{FH0D}(\{\text{gO1}\}), \tilde{d}^{D_{R,a}}, \tilde{d}_{L,b}}^R \\
& + \sum_{a=1}^3 m_{\tilde{e}^{D_{R,a}}} \sum_{b=1}^3 B_0 \left( p^2, m_{e_{R,a}^D}^2, m_{\tilde{e}_{L,b}}^2 \right) \Gamma_{\text{FH0D}(\{\text{gO2}\}), \tilde{e}^{D_{R,a}}, \tilde{e}_{L,b}}^{L*} \Gamma_{\text{FH0D}(\{\text{gO1}\}), \tilde{e}^{D_{R,a}}, \tilde{e}_{L,b}}^R
\end{aligned}$$



$$\begin{aligned}
& + 3 \sum_{a=1}^3 m_{\bar{u}^{D_L,a}} \sum_{b=1}^3 B_0(p^2, m_{\bar{u}_{L,a}^D}^2, m_{\bar{u}_{R,b}}^2) \Gamma_{\text{FH0D}(\{\text{gO2}\})}^{L*} \Gamma_{\text{FH0D}(\{\text{gO1}\})}^R, \bar{u}^{D_L,a}, \bar{u}_{R,b} \\
& + 3 \sum_{a=1}^3 \sum_{b=1}^3 B_0(p^2, m_{d_{L,b}^D}^2, m_{d_{R,a}}^2) \Gamma_{\text{FH0D}(\{\text{gO2}\})}^{L*} \Gamma_{\text{FH0D}(\{\text{gO1}\})}^R, \bar{d}_{R,a}^*, d_{L,b}^D, m_{d_{L,b}^D} \Gamma_{\text{FH0D}(\{\text{gO1}\})}^R, \bar{d}_{R,a}^*, d_{L,b}^D \\
& + \sum_{a=1}^3 \sum_{b=1}^3 B_0(p^2, m_{e_{L,b}^D}^2, m_{e_{R,a}}^2) \Gamma_{\text{FH0D}(\{\text{gO2}\})}^{L*} \Gamma_{\text{FH0D}(\{\text{gO1}\})}^R, \bar{e}_{R,a}^*, e_{L,b}^D, m_{e_{L,b}^D} \Gamma_{\text{FH0D}(\{\text{gO1}\})}^R, \bar{e}_{R,a}^*, e_{L,b}^D \\
& + 3 \sum_{a=1}^3 \sum_{b=1}^3 B_0(p^2, m_{u_{R,b}^D}^2, m_{\bar{u}_{L,a}}^2) \Gamma_{\text{FH0D}(\{\text{gO2}\})}^{L*} \Gamma_{\text{FH0D}(\{\text{gO1}\})}^R, \bar{u}_{L,a}^*, u_{R,b}^D, m_{u_{R,b}^D} \Gamma_{\text{FH0D}(\{\text{gO1}\})}^R, \bar{u}_{L,a}^*, u_{R,b}^D \\
& + \sum_{b=1}^{10} B_0(p^2, m_{f_{Po,b}^0}^2, m_{H_u^0}^2) \Gamma_{\text{FH0D}(\{\text{gO2}\})}^{L*} \Gamma_{\text{FH0D}(\{\text{gO1}\})}^R, H_u^0, f_{Po,b}^0, m_{f_{Po,b}^0} \Gamma_{\text{FH0D}(\{\text{gO1}\})}^R, H_u^0, f_{Po,b}^0 \\
& + \sum_{b=1}^{10} B_0(p^2, m_{f_{Go,b}^-}^2, m_{H_u^+}^2) \Gamma_{\text{FH0D}(\{\text{gO2}\})}^{L*} \Gamma_{\text{FH0D}(\{\text{gO1}\})}^R, H_u^+, f_{Go,b}^-, m_{f_{Go,b}^-} \Gamma_{\text{FH0D}(\{\text{gO1}\})}^R, H_u^+, f_{Go,b}^- \\
& + \sum_{b=1}^{10} B_0(p^2, m_{f_{Po,b}^0}^2, m_{H_d^0}^2) \Gamma_{\text{FH0D}(\{\text{gO2}\})}^{L*} \Gamma_{\text{FH0D}(\{\text{gO1}\})}^R, H_d^{0,*}, f_{Po,b}^0, m_{f_{Po,b}^0} \Gamma_{\text{FH0D}(\{\text{gO1}\})}^R, H_d^{0,*}, f_{Po,b}^0 \\
& + \sum_{b=1}^{10} B_0(p^2, m_{f_{Go,b}^-}^2, m_{H_d^-}^2) \Gamma_{\text{FH0D}(\{\text{gO2}\})}^{L*} \Gamma_{\text{FH0D}(\{\text{gO1}\})}^R, H_d^{-,*}, f_{Go,b}^-, m_{f_{Go,b}^-} \Gamma_{\text{FH0D}(\{\text{gO1}\})}^R, H_d^{-,*}, f_{Go,b}^- \\
& - 4B_0(p^2, m_{\bar{H}^0}^2, m_{B_L}^2) \Gamma_{\text{FH0D}(\{\text{gO2}\})}^{R*} \Gamma_{\text{FH0D}(\{\text{gO1}\})}^L, B_L, \text{FH0D}(\{1\}) m_{\bar{H}^0} \Gamma_{\text{FH0D}(\{\text{gO1}\})}^L, B_L, \text{FH0D}(\{1\}) \\
& - 4B_0(p^2, m_{\bar{H}^0}^2, m_{B_H}^2) \Gamma_{\text{FH0D}(\{\text{gO2}\})}^{R*} \Gamma_{\text{FH0D}(\{\text{gO1}\})}^L, B_H, \text{FH0D}(\{1\}) m_{\bar{H}^0} \Gamma_{\text{FH0D}(\{\text{gO1}\})}^L, B_H, \text{FH0D}(\{1\}) \\
& - 4B_0(p^2, m_{\bar{H}^-}^2, m_{W_L^1}^2) \Gamma_{\text{FH0D}(\{\text{gO2}\})}^{R*} \Gamma_{\text{FH0D}(\{\text{gO1}\})}^L, W_L^1, \text{FHCD}(\{1\}) m_{\bar{H}^-} \Gamma_{\text{FH0D}(\{\text{gO1}\})}^L, W_L^1, \text{FHCD}(\{1\}) \\
& - 4B_0(p^2, m_{\bar{H}^-}^2, m_{W_H^1}^2) \Gamma_{\text{FH0D}(\{\text{gO2}\})}^{R*} \Gamma_{\text{FH0D}(\{\text{gO1}\})}^L, W_H^1, \text{FHCD}(\{1\}) m_{\bar{H}^-} \Gamma_{\text{FH0D}(\{\text{gO1}\})}^L, W_H^1, \text{FHCD}(\{1\}) \\
& - 4B_0(p^2, m_{\bar{H}^-}^2, m_{W_L^2}^2) \Gamma_{\text{FH0D}(\{\text{gO2}\})}^{R*} \Gamma_{\text{FH0D}(\{\text{gO1}\})}^L, W_L^2, \text{FHCD}(\{1\}) m_{\bar{H}^-} \Gamma_{\text{FH0D}(\{\text{gO1}\})}^L, W_L^2, \text{FHCD}(\{1\}) \\
& - 4B_0(p^2, m_{\bar{H}^-}^2, m_{W_H^2}^2) \Gamma_{\text{FH0D}(\{\text{gO2}\})}^{R*} \Gamma_{\text{FH0D}(\{\text{gO1}\})}^L, W_H^2, \text{FHCD}(\{1\}) m_{\bar{H}^-} \Gamma_{\text{FH0D}(\{\text{gO1}\})}^L, W_H^2, \text{FHCD}(\{1\}) \\
& - 4B_0(p^2, m_{\bar{H}^0}^2, m_{W_L^3}^2) \Gamma_{\text{FH0D}(\{\text{gO2}\})}^{R*} \Gamma_{\text{FH0D}(\{\text{gO1}\})}^L, W_L^3, \text{FH0D}(\{1\}) m_{\bar{H}^0} \Gamma_{\text{FH0D}(\{\text{gO1}\})}^L, W_L^3, \text{FH0D}(\{1\})
\end{aligned}$$

$$\begin{aligned}
& -4B_0\left(p^2, m_{\tilde{H}^0}^2, m_{W_H^3}^2\right)\Gamma^{R*}_{\text{FH0D}\left(\bar{\{gO2\}}\right), W_H^3, \text{FH0D}\left(\{1\}\right)} m_{\tilde{H}^0}\Gamma^L_{\text{FH0D}\left(\bar{\{gO1\}}\right), W_H^3, \text{FH0D}\left(\{1\}\right)} \quad (348) \\
& \Sigma^L(p^2) = +3 \sum_{a=1}^3 m_{\tilde{d}^{D_{R,a}}} \sum_{b=1}^3 B_0\left(p^2, m_{d_{R,a}^D}^2, m_{\tilde{d}_{L,b}}^2\right)\Gamma^{L*}_{\text{FH0D}\left(\bar{\{gO2\}}\right), \tilde{d}^{D_{R,a}}, \tilde{d}_{L,b}} \Gamma^R_{\text{FH0D}\left(\bar{\{gO1\}}\right), \tilde{d}^{D_{R,a}}, \tilde{d}_{L,b}} \\
& + \sum_{a=1}^3 m_{\tilde{e}^{D_{R,a}}} \sum_{b=1}^3 B_0\left(p^2, m_{e_{R,a}^D}^2, m_{\tilde{e}_{L,b}}^2\right)\Gamma^{L*}_{\text{FH0D}\left(\bar{\{gO2\}}\right), \tilde{e}^{D_{R,a}}, \tilde{e}_{L,b}} \Gamma^R_{\text{FH0D}\left(\bar{\{gO1\}}\right), \tilde{e}^{D_{R,a}}, \tilde{e}_{L,b}} \\
& + 3 \sum_{a=1}^3 m_{\tilde{u}^{D_{L,a}}} \sum_{b=1}^3 B_0\left(p^2, m_{u_{L,a}^D}^2, m_{\tilde{u}_{R,b}}^2\right)\Gamma^{L*}_{\text{FH0D}\left(\bar{\{gO2\}}\right), \tilde{u}^{D_{L,a}}, \tilde{u}_{R,b}} \Gamma^R_{\text{FH0D}\left(\bar{\{gO1\}}\right), \tilde{u}^{D_{L,a}}, \tilde{u}_{R,b}} \\
& + 3 \sum_{a=1}^3 \sum_{b=1}^3 B_0\left(p^2, m_{d_{L,b}^D}^2, m_{\tilde{d}_{R,a}}^2\right)\Gamma^{L*}_{\text{FH0D}\left(\bar{\{gO2\}}\right), \tilde{d}_{R,a}^*, d_{L,b}^D} m_{d_{L,b}^D} \Gamma^R_{\text{FH0D}\left(\bar{\{gO1\}}\right), \tilde{d}_{R,a}^*, d_{L,b}^D} \\
& + \sum_{a=1}^3 \sum_{b=1}^3 B_0\left(p^2, m_{e_{L,b}^D}^2, m_{\tilde{e}_{R,a}}^2\right)\Gamma^{L*}_{\text{FH0D}\left(\bar{\{gO2\}}\right), \tilde{e}_{R,a}^*, e_{L,b}^D} m_{e_{L,b}^D} \Gamma^R_{\text{FH0D}\left(\bar{\{gO1\}}\right), \tilde{e}_{R,a}^*, e_{L,b}^D} \\
& + 3 \sum_{a=1}^3 \sum_{b=1}^3 B_0\left(p^2, m_{u_{R,b}^D}^2, m_{\tilde{u}_{L,a}}^2\right)\Gamma^{L*}_{\text{FH0D}\left(\bar{\{gO2\}}\right), \tilde{u}_{L,a}^*, u_{R,b}^D} m_{u_{R,b}^D} \Gamma^R_{\text{FH0D}\left(\bar{\{gO1\}}\right), \tilde{u}_{L,a}^*, u_{R,b}^D} \\
& + \sum_{b=1}^{10} B_0\left(p^2, m_{f_{Po,b}^0}^2, m_{H_u^0}^2\right)\Gamma^{L*}_{\text{FH0D}\left(\bar{\{gO2\}}\right), H_u^0, f_{Po,b}^0} m_{f_{Po,b}^0} \Gamma^R_{\text{FH0D}\left(\bar{\{gO1\}}\right), H_u^0, f_{Po,b}^0} \\
& + \sum_{b=1}^{10} B_0\left(p^2, m_{f_{Go,b}^-}^2, m_{H_u^+}^2\right)\Gamma^{L*}_{\text{FH0D}\left(\bar{\{gO2\}}\right), H_u^+, f_{Go,b}^-} m_{f_{Go,b}^-} \Gamma^R_{\text{FH0D}\left(\bar{\{gO1\}}\right), H_u^+, f_{Go,b}^-} \\
& + \sum_{b=1}^{10} B_0\left(p^2, m_{f_{Po,b}^0}^2, m_{H_d^0}^2\right)\Gamma^{L*}_{\text{FH0D}\left(\bar{\{gO2\}}\right), H_d^{0,*}, f_{Po,b}^0} m_{f_{Po,b}^0} \Gamma^R_{\text{FH0D}\left(\bar{\{gO1\}}\right), H_d^{0,*}, f_{Po,b}^0} \\
& + \sum_{b=1}^{10} B_0\left(p^2, m_{f_{Go,b}^-}^2, m_{H_d^-}^2\right)\Gamma^{L*}_{\text{FH0D}\left(\bar{\{gO2\}}\right), H_d^{-,*}, f_{Go,b}^-} m_{f_{Go,b}^-} \Gamma^R_{\text{FH0D}\left(\bar{\{gO1\}}\right), H_d^{-,*}, f_{Go,b}^-} \\
& - 4B_0\left(p^2, m_{\tilde{H}^0}^2, m_{B_L}^2\right)\Gamma^{R*}_{\text{FH0D}\left(\bar{\{gO2\}}\right), B_L, \text{FH0D}\left(\{1\}\right)} m_{\tilde{H}^0}\Gamma^L_{\text{FH0D}\left(\bar{\{gO1\}}\right), B_L, \text{FH0D}\left(\{1\}\right)} \\
& - 4B_0\left(p^2, m_{\tilde{H}^0}^2, m_{B_H}^2\right)\Gamma^{R*}_{\text{FH0D}\left(\bar{\{gO2\}}\right), B_H, \text{FH0D}\left(\{1\}\right)} m_{\tilde{H}^0}\Gamma^L_{\text{FH0D}\left(\bar{\{gO1\}}\right), B_H, \text{FH0D}\left(\{1\}\right)} \\
& - 4B_0\left(p^2, m_{\tilde{H}^-}^2, m_{W_L^1}^2\right)\Gamma^{R*}_{\text{FH0D}\left(\bar{\{gO2\}}\right), W_L^1, \text{FHCD}\left(\{1\}\right)} m_{\tilde{H}^-}\Gamma^L_{\text{FH0D}\left(\bar{\{gO1\}}\right), W_L^1, \text{FHCD}\left(\{1\}\right)} \\
& - 4B_0\left(p^2, m_{\tilde{H}^-}^2, m_{W_H^1}^2\right)\Gamma^{R*}_{\text{FH0D}\left(\bar{\{gO2\}}\right), W_H^1, \text{FHCD}\left(\{1\}\right)} m_{\tilde{H}^-}\Gamma^L_{\text{FH0D}\left(\bar{\{gO1\}}\right), W_H^1, \text{FHCD}\left(\{1\}\right)}
\end{aligned}$$

$$\begin{aligned}
& -4B_0(p^2, m_{\tilde{H}^-}^2, m_{W_L^2}^2) \Gamma_{\text{FH0D}(\{\bar{\text{gO2}}\})}^{R*} m_{\tilde{H}^-} \Gamma_{\text{FH0D}(\{\bar{\text{gO1}}\})}^L W_L^2, \text{FHCD}(\{1\}) \\
& -4B_0(p^2, m_{\tilde{H}^-}^2, m_{W_H^2}^2) \Gamma_{\text{FH0D}(\{\bar{\text{gO2}}\})}^{R*} m_{\tilde{H}^-} \Gamma_{\text{FH0D}(\{\bar{\text{gO1}}\})}^L W_H^2, \text{FHCD}(\{1\}) \\
& -4B_0(p^2, m_{\tilde{H}^0}^2, m_{W_L^3}^2) \Gamma_{\text{FH0D}(\{\bar{\text{gO2}}\})}^{R*} m_{\tilde{H}^0} \Gamma_{\text{FH0D}(\{\bar{\text{gO1}}\})}^L W_L^3, \text{FH0D}(\{1\}) \\
& -4B_0(p^2, m_{\tilde{H}^0}^2, m_{W_H^3}^2) \Gamma_{\text{FH0D}(\{\bar{\text{gO2}}\})}^{R*} m_{\tilde{H}^0} \Gamma_{\text{FH0D}(\{\bar{\text{gO1}}\})}^L W_H^3, \text{FH0D}(\{1\})
\end{aligned} \tag{349}$$

• Self-Energy for Charged Higgsino Majorana spinor ( $\tilde{H}^-$ )

$$\begin{aligned}
\Sigma^S(p^2) = & +3 \sum_{a=1}^3 m_{\tilde{d}^{D_L, a}} \sum_{b=1}^3 B_0(p^2, m_{\tilde{d}_{L,a}^D}^2, m_{\tilde{u}_{R,b}}^2) \Gamma_{\text{FHCD}(\{\bar{\text{gO2}}\})}^{L*} \Gamma_{\text{FHCD}(\{\bar{\text{gO1}}\})}^R \tilde{d}^{D_L, a}, \tilde{u}_{R,b} \\
& +3 \sum_{a=1}^3 m_{\tilde{d}^{D_R, a}} \sum_{b=1}^3 B_0(p^2, m_{\tilde{d}_{R,a}^D}^2, m_{\tilde{u}_{L,b}}^2) \Gamma_{\text{FHCD}(\{\bar{\text{gO2}}\})}^{L*} \Gamma_{\text{FHCD}(\{\bar{\text{gO1}}\})}^R \tilde{d}^{D_R, a}, \tilde{u}_{L,b} \\
& + \sum_{a=1}^3 m_{\tilde{e}^{D_R, a}} \sum_{b=1}^3 B_0(p^2, m_{\tilde{e}_{R,a}^D}^2, m_{\tilde{\nu}_{L,b}}^2) \Gamma_{\text{FHCD}(\{\bar{\text{gO2}}\})}^{L*} \Gamma_{\text{FHCD}(\{\bar{\text{gO1}}\})}^R \tilde{e}^{D_R, a}, \tilde{\nu}_{L,b} \\
& +3 \sum_{a=1}^3 \sum_{b=1}^3 B_0(p^2, m_{\tilde{u}_{R,b}^D}^2, m_{\tilde{d}_{L,a}^D}^2) \Gamma_{\text{FHCD}(\{\bar{\text{gO2}}\})}^{L*} m_{\tilde{u}_{R,b}^D} \Gamma_{\text{FHCD}(\{\bar{\text{gO1}}\})}^R \tilde{d}_{L,a}^*, u_{R,b}^D \\
& +3 \sum_{a=1}^3 \sum_{b=1}^3 B_0(p^2, m_{\tilde{u}_{L,b}^D}^2, m_{\tilde{d}_{R,a}^D}^2) \Gamma_{\text{FHCD}(\{\bar{\text{gO2}}\})}^{L*} m_{\tilde{u}_{L,b}^D} \Gamma_{\text{FHCD}(\{\bar{\text{gO1}}\})}^R \tilde{d}_{R,a}^*, u_{L,b}^D \\
& + \sum_{a=1}^3 \sum_{b=1}^3 B_0(p^2, m_{\tilde{\nu}_{L,b}^D}^2, m_{\tilde{e}_{R,a}^D}^2) \Gamma_{\text{FHCD}(\{\bar{\text{gO2}}\})}^{L*} m_{\tilde{\nu}_{L,b}^D} \Gamma_{\text{FHCD}(\{\bar{\text{gO1}}\})}^R \tilde{e}_{R,a}^*, \nu_{L,b}^D \\
& + \sum_{b=1}^{10} B_0(p^2, m_{f_{G^0, b}^-}^2, m_{H_u^0}^2) \Gamma_{\text{FHCD}(\{\bar{\text{gO2}}\})}^{L*} m_{f_{G^0, b}^-} \Gamma_{\text{FHCD}(\{\bar{\text{gO1}}\})}^R H_u^0, f_{G^0, b}^- \\
& + \sum_{b=1}^{10} B_0(p^2, m_{f_{P^0, b}^0}^2, m_{H_u^+}^2) \Gamma_{\text{FHCD}(\{\bar{\text{gO2}}\})}^{L*} m_{f_{P^0, b}^0} \Gamma_{\text{FHCD}(\{\bar{\text{gO1}}\})}^R H_u^+, f_{P^0, b}^0 \\
& + \sum_{b=1}^{10} B_0(p^2, m_{f_{G^0, b}^-}^2, m_{H_d^0}^2) \Gamma_{\text{FHCD}(\{\bar{\text{gO2}}\})}^{L*} m_{f_{G^0, b}^-} \Gamma_{\text{FHCD}(\{\bar{\text{gO1}}\})}^R H_d^{0,*}, f_{G^0, b}^- \\
& + \sum_{b=1}^{10} B_0(p^2, m_{f_{P^0, b}^0}^2, m_{H_d^-}^2) \Gamma_{\text{FHCD}(\{\bar{\text{gO2}}\})}^{L*} m_{f_{P^0, b}^0} \Gamma_{\text{FHCD}(\{\bar{\text{gO1}}\})}^R H_d^{-,*}, f_{P^0, b}^0
\end{aligned}$$

$$\begin{aligned}
& -4B_0\left(p^2, m_{\tilde{H}^-}^2, m_{B_L}^2\right) \Gamma_{\text{FHCD}\left(\bar{\{gO2\}}\right), B_L, \text{FHCD}\left(\{1\}\right)}^{R*} m_{\tilde{H}^-} \Gamma_{\text{FHCD}\left(\bar{\{gO1\}}\right), B_L, \text{FHCD}\left(\{1\}\right)}^L \\
& -4B_0\left(p^2, m_{\tilde{H}^-}^2, m_{B_H}^2\right) \Gamma_{\text{FHCD}\left(\bar{\{gO2\}}\right), B_H, \text{FHCD}\left(\{1\}\right)}^{R*} m_{\tilde{H}^-} \Gamma_{\text{FHCD}\left(\bar{\{gO1\}}\right), B_H, \text{FHCD}\left(\{1\}\right)}^L \\
& -4B_0\left(p^2, m_{\tilde{H}^0}^2, m_{W_L^1}^2\right) \Gamma_{\text{FHCD}\left(\bar{\{gO2\}}\right), W_L^1, \text{FH0D}\left(\{1\}\right)}^{R*} m_{\tilde{H}^0} \Gamma_{\text{FHCD}\left(\bar{\{gO1\}}\right), W_L^1, \text{FH0D}\left(\{1\}\right)}^L \\
& -4B_0\left(p^2, m_{\tilde{H}^0}^2, m_{W_H^1}^2\right) \Gamma_{\text{FHCD}\left(\bar{\{gO2\}}\right), W_H^1, \text{FH0D}\left(\{1\}\right)}^{R*} m_{\tilde{H}^0} \Gamma_{\text{FHCD}\left(\bar{\{gO1\}}\right), W_H^1, \text{FH0D}\left(\{1\}\right)}^L \\
& -4B_0\left(p^2, m_{\tilde{H}^0}^2, m_{W_L^2}^2\right) \Gamma_{\text{FHCD}\left(\bar{\{gO2\}}\right), W_L^2, \text{FH0D}\left(\{1\}\right)}^{R*} m_{\tilde{H}^0} \Gamma_{\text{FHCD}\left(\bar{\{gO1\}}\right), W_L^2, \text{FH0D}\left(\{1\}\right)}^L \\
& -4B_0\left(p^2, m_{\tilde{H}^0}^2, m_{W_H^2}^2\right) \Gamma_{\text{FHCD}\left(\bar{\{gO2\}}\right), W_H^2, \text{FH0D}\left(\{1\}\right)}^{R*} m_{\tilde{H}^0} \Gamma_{\text{FHCD}\left(\bar{\{gO1\}}\right), W_H^2, \text{FH0D}\left(\{1\}\right)}^L \\
& -4B_0\left(p^2, m_{\tilde{H}^-}^2, m_{W_L^3}^2\right) \Gamma_{\text{FHCD}\left(\bar{\{gO2\}}\right), W_L^3, \text{FHCD}\left(\{1\}\right)}^{R*} m_{\tilde{H}^-} \Gamma_{\text{FHCD}\left(\bar{\{gO1\}}\right), W_L^3, \text{FHCD}\left(\{1\}\right)}^L \\
& -4B_0\left(p^2, m_{\tilde{H}^-}^2, m_{W_H^3}^2\right) \Gamma_{\text{FHCD}\left(\bar{\{gO2\}}\right), W_H^3, \text{FHCD}\left(\{1\}\right)}^{R*} m_{\tilde{H}^-} \Gamma_{\text{FHCD}\left(\bar{\{gO1\}}\right), W_H^3, \text{FHCD}\left(\{1\}\right)}^L
\end{aligned} \tag{350}$$

$$\begin{aligned}
\Sigma^R(p^2) = & +3 \sum_{a=1}^3 m_{\tilde{d}^{D_L, a}} \sum_{b=1}^3 B_0\left(p^2, m_{d_{L, a}^D}^2, m_{\tilde{u}_{R, b}}^2\right) \Gamma_{\text{FHCD}\left(\bar{\{gO2\}}\right), \tilde{d}^{D_L, a}, \tilde{u}_{R, b}}^{L*} \Gamma_{\text{FHCD}\left(\bar{\{gO1\}}\right), \tilde{d}^{D_L, a}, \tilde{u}_{R, b}}^R \\
& +3 \sum_{a=1}^3 m_{\tilde{d}^{D_R, a}} \sum_{b=1}^3 B_0\left(p^2, m_{d_{R, a}^D}^2, m_{\tilde{u}_{L, b}}^2\right) \Gamma_{\text{FHCD}\left(\bar{\{gO2\}}\right), \tilde{d}^{D_R, a}, \tilde{u}_{L, b}}^{L*} \Gamma_{\text{FHCD}\left(\bar{\{gO1\}}\right), \tilde{d}^{D_R, a}, \tilde{u}_{L, b}}^R \\
& + \sum_{a=1}^3 m_{\tilde{e}^{D_R, a}} \sum_{b=1}^3 B_0\left(p^2, m_{e_{R, a}^D}^2, m_{\tilde{\nu}_{L, b}}^2\right) \Gamma_{\text{FHCD}\left(\bar{\{gO2\}}\right), \tilde{e}^{D_R, a}, \tilde{\nu}_{L, b}}^{L*} \Gamma_{\text{FHCD}\left(\bar{\{gO1\}}\right), \tilde{e}^{D_R, a}, \tilde{\nu}_{L, b}}^R \\
& +3 \sum_{a=1}^3 \sum_{b=1}^3 B_0\left(p^2, m_{u_{R, b}^D}^2, m_{\tilde{d}_{L, a}}^2\right) \Gamma_{\text{FHCD}\left(\bar{\{gO2\}}\right), \tilde{d}_{L, a}^*, u_{R, b}^D}^{L*} m_{u_{R, b}^D} \Gamma_{\text{FHCD}\left(\bar{\{gO1\}}\right), \tilde{d}_{L, a}^*, u_{R, b}^D}^R \\
& +3 \sum_{a=1}^3 \sum_{b=1}^3 B_0\left(p^2, m_{u_{L, b}^D}^2, m_{\tilde{d}_{R, a}}^2\right) \Gamma_{\text{FHCD}\left(\bar{\{gO2\}}\right), \tilde{d}_{R, a}^*, u_{L, b}^D}^{L*} m_{u_{L, b}^D} \Gamma_{\text{FHCD}\left(\bar{\{gO1\}}\right), \tilde{d}_{R, a}^*, u_{L, b}^D}^R \\
& + \sum_{a=1}^3 \sum_{b=1}^3 B_0\left(p^2, m_{\nu_{L, b}^D}^2, m_{\tilde{e}_{R, a}}^2\right) \Gamma_{\text{FHCD}\left(\bar{\{gO2\}}\right), \tilde{e}_{R, a}^*, \nu_{L, b}^D}^{L*} m_{\nu_{L, b}^D} \Gamma_{\text{FHCD}\left(\bar{\{gO1\}}\right), \tilde{e}_{R, a}^*, \nu_{L, b}^D}^R \\
& + \sum_{b=1}^{10} B_0\left(p^2, m_{f_{G^0, b}^-}^2, m_{H_u^0}^2\right) \Gamma_{\text{FHCD}\left(\bar{\{gO2\}}\right), H_u^0, f_{G^0, b}^-}^{L*} m_{f_{G^0, b}^-} \Gamma_{\text{FHCD}\left(\bar{\{gO1\}}\right), H_u^0, f_{G^0, b}^-}^R
\end{aligned}$$

$$\begin{aligned}
& + \sum_{b=1}^{10} B_0(p^2, m_{f_{Po,b}^0}^2, m_{H_u^+}^2) \Gamma_{\text{FHCD}(\{\text{gO2}\})}^{L*} m_{f_{Po,b}^0} \Gamma_{\text{FHCD}(\{\text{gO1}\})}^R, H_u^+, f_{Po,b}^0 \\
& + \sum_{b=1}^{10} B_0(p^2, m_{f_{Go,b}^-}^2, m_{H_d^0}^2) \Gamma_{\text{FHCD}(\{\text{gO2}\})}^{L*} m_{f_{Go,b}^-} \Gamma_{\text{FHCD}(\{\text{gO1}\})}^R, H_d^{0,*}, f_{Go,b}^- \\
& + \sum_{b=1}^{10} B_0(p^2, m_{f_{Po,b}^0}^2, m_{H_d^-}^2) \Gamma_{\text{FHCD}(\{\text{gO2}\})}^{L*} m_{f_{Po,b}^0} \Gamma_{\text{FHCD}(\{\text{gO1}\})}^R, H_d^{-,*}, f_{Po,b}^0 \\
& - 4B_0(p^2, m_{\tilde{H}^-}^2, m_{B_L}^2) \Gamma_{\text{FHCD}(\{\text{gO2}\})}^{R*} m_{\tilde{H}^-} \Gamma_{\text{FHCD}(\{\text{gO1}\})}^L, B_L, \text{FHCD}(\{1\}) \\
& - 4B_0(p^2, m_{\tilde{H}^-}^2, m_{B_H}^2) \Gamma_{\text{FHCD}(\{\text{gO2}\})}^{R*} m_{\tilde{H}^-} \Gamma_{\text{FHCD}(\{\text{gO1}\})}^L, B_H, \text{FHCD}(\{1\}) \\
& - 4B_0(p^2, m_{\tilde{H}^0}^2, m_{W_L^1}^2) \Gamma_{\text{FHCD}(\{\text{gO2}\})}^{R*} m_{\tilde{H}^0} \Gamma_{\text{FHCD}(\{\text{gO1}\})}^L, W_L^1, \text{FH0D}(\{1\}) \\
& - 4B_0(p^2, m_{\tilde{H}^0}^2, m_{W_H^1}^2) \Gamma_{\text{FHCD}(\{\text{gO2}\})}^{R*} m_{\tilde{H}^0} \Gamma_{\text{FHCD}(\{\text{gO1}\})}^L, W_H^1, \text{FH0D}(\{1\}) \\
& - 4B_0(p^2, m_{\tilde{H}^0}^2, m_{W_L^2}^2) \Gamma_{\text{FHCD}(\{\text{gO2}\})}^{R*} m_{\tilde{H}^0} \Gamma_{\text{FHCD}(\{\text{gO1}\})}^L, W_L^2, \text{FH0D}(\{1\}) \\
& - 4B_0(p^2, m_{\tilde{H}^0}^2, m_{W_H^2}^2) \Gamma_{\text{FHCD}(\{\text{gO2}\})}^{R*} m_{\tilde{H}^0} \Gamma_{\text{FHCD}(\{\text{gO1}\})}^L, W_H^2, \text{FH0D}(\{1\}) \\
& - 4B_0(p^2, m_{\tilde{H}^-}^2, m_{W_L^3}^2) \Gamma_{\text{FHCD}(\{\text{gO2}\})}^{R*} m_{\tilde{H}^-} \Gamma_{\text{FHCD}(\{\text{gO1}\})}^L, W_L^3, \text{FHCD}(\{1\}) \\
& - 4B_0(p^2, m_{\tilde{H}^-}^2, m_{W_H^3}^2) \Gamma_{\text{FHCD}(\{\text{gO2}\})}^{R*} m_{\tilde{H}^-} \Gamma_{\text{FHCD}(\{\text{gO1}\})}^L, W_H^3, \text{FHCD}(\{1\}) \tag{351}
\end{aligned}$$

$$\begin{aligned}
\Sigma^L(p^2) = & + 3 \sum_{a=1}^3 m_{\tilde{d}^{D_L,a}} \sum_{b=1}^3 B_0(p^2, m_{\tilde{d}_{L,a}^D}^2, m_{\tilde{u}_{R,b}}^2) \Gamma_{\text{FHCD}(\{\text{gO2}\})}^{L*} \Gamma_{\text{FHCD}(\{\text{gO1}\})}^R, \tilde{d}^{D_L,a}, \tilde{u}_{R,b} \\
& + 3 \sum_{a=1}^3 m_{\tilde{d}^{D_R,a}} \sum_{b=1}^3 B_0(p^2, m_{\tilde{d}_{R,a}^D}^2, m_{\tilde{u}_{L,b}}^2) \Gamma_{\text{FHCD}(\{\text{gO2}\})}^{L*} \Gamma_{\text{FHCD}(\{\text{gO1}\})}^R, \tilde{d}^{D_R,a}, \tilde{u}_{L,b} \\
& + \sum_{a=1}^3 m_{\tilde{e}^{D_R,a}} \sum_{b=1}^3 B_0(p^2, m_{\tilde{e}_{R,a}^D}^2, m_{\tilde{\nu}_{L,b}}^2) \Gamma_{\text{FHCD}(\{\text{gO2}\})}^{L*} \Gamma_{\text{FHCD}(\{\text{gO1}\})}^R, \tilde{e}^{D_R,a}, \tilde{\nu}_{L,b} \\
& + 3 \sum_{a=1}^3 \sum_{b=1}^3 B_0(p^2, m_{u_{R,b}^D}^2, m_{\tilde{d}_{L,a}}^2) \Gamma_{\text{FHCD}(\{\text{gO2}\})}^{L*} m_{u_{R,b}^D} \Gamma_{\text{FHCD}(\{\text{gO1}\})}^R, \tilde{d}_{L,a}^*, u_{R,b}^D
\end{aligned}$$

$$\begin{aligned}
& + 3 \sum_{a=1}^3 \sum_{b=1}^3 B_0(p^2, m_{u_{L,b}^D}^2, m_{\tilde{d}_{R,a}}^2) \Gamma_{\text{FHCD}(\{\text{gO2}\})}^{L*} \bar{d}_{R,a}^* u_{L,b}^D m_{u_{L,b}^D} \Gamma_{\text{FHCD}(\{\text{gO1}\})}^R \tilde{d}_{R,a}^* u_{L,b}^D \\
& + \sum_{a=1}^3 \sum_{b=1}^3 B_0(p^2, m_{\nu_{L,b}^D}^2, m_{\tilde{e}_{R,a}}^2) \Gamma_{\text{FHCD}(\{\text{gO2}\})}^{L*} \bar{e}_{R,a}^* \nu_{L,b}^D m_{\nu_{L,b}^D} \Gamma_{\text{FHCD}(\{\text{gO1}\})}^R \tilde{e}_{R,a}^* \nu_{L,b}^D \\
& + \sum_{b=1}^{10} B_0(p^2, m_{f_{Go,b}^-}^2, m_{H_u^0}^2) \Gamma_{\text{FHCD}(\{\text{gO2}\})}^{L*} H_u^0 f_{Go,b}^- m_{f_{Go,b}^-} \Gamma_{\text{FHCD}(\{\text{gO1}\})}^R H_u^0 f_{Go,b}^- \\
& + \sum_{b=1}^{10} B_0(p^2, m_{f_{Po,b}^0}^2, m_{H_u^+}^2) \Gamma_{\text{FHCD}(\{\text{gO2}\})}^{L*} H_u^+ f_{Po,b}^0 m_{f_{Po,b}^0} \Gamma_{\text{FHCD}(\{\text{gO1}\})}^R H_u^+ f_{Po,b}^0 \\
& + \sum_{b=1}^{10} B_0(p^2, m_{f_{Go,b}^-}^2, m_{H_d^0}^2) \Gamma_{\text{FHCD}(\{\text{gO2}\})}^{L*} H_d^{0,*} f_{Go,b}^- m_{f_{Go,b}^-} \Gamma_{\text{FHCD}(\{\text{gO1}\})}^R H_d^{0,*} f_{Go,b}^- \\
& + \sum_{b=1}^{10} B_0(p^2, m_{f_{Po,b}^0}^2, m_{H_d^-}^2) \Gamma_{\text{FHCD}(\{\text{gO2}\})}^{L*} H_d^{-,*} f_{Po,b}^0 m_{f_{Po,b}^0} \Gamma_{\text{FHCD}(\{\text{gO1}\})}^R H_d^{-,*} f_{Po,b}^0 \\
& - 4B_0(p^2, m_{\tilde{H}^-}^2, m_{B_L}^2) \Gamma_{\text{FHCD}(\{\text{gO2}\})}^{R*} B_L \Gamma_{\text{FHCD}(\{1\})}^{L*} m_{\tilde{H}^-} \Gamma_{\text{FHCD}(\{\text{gO1}\})}^L B_L \Gamma_{\text{FHCD}(\{1\})}^R \\
& - 4B_0(p^2, m_{\tilde{H}^-}^2, m_{B_H}^2) \Gamma_{\text{FHCD}(\{\text{gO2}\})}^{R*} B_H \Gamma_{\text{FHCD}(\{1\})}^{L*} m_{\tilde{H}^-} \Gamma_{\text{FHCD}(\{\text{gO1}\})}^L B_H \Gamma_{\text{FHCD}(\{1\})}^R \\
& - 4B_0(p^2, m_{\tilde{H}^0}^2, m_{W_L^1}^2) \Gamma_{\text{FHCD}(\{\text{gO2}\})}^{R*} W_L^1 \Gamma_{\text{FH0D}(\{1\})}^{L*} m_{\tilde{H}^0} \Gamma_{\text{FHCD}(\{\text{gO1}\})}^L W_L^1 \Gamma_{\text{FH0D}(\{1\})}^R \\
& - 4B_0(p^2, m_{\tilde{H}^0}^2, m_{W_H^1}^2) \Gamma_{\text{FHCD}(\{\text{gO2}\})}^{R*} W_H^1 \Gamma_{\text{FH0D}(\{1\})}^{L*} m_{\tilde{H}^0} \Gamma_{\text{FHCD}(\{\text{gO1}\})}^L W_H^1 \Gamma_{\text{FH0D}(\{1\})}^R \\
& - 4B_0(p^2, m_{\tilde{H}^0}^2, m_{W_L^2}^2) \Gamma_{\text{FHCD}(\{\text{gO2}\})}^{R*} W_L^2 \Gamma_{\text{FH0D}(\{1\})}^{L*} m_{\tilde{H}^0} \Gamma_{\text{FHCD}(\{\text{gO1}\})}^L W_L^2 \Gamma_{\text{FH0D}(\{1\})}^R \\
& - 4B_0(p^2, m_{\tilde{H}^0}^2, m_{W_H^2}^2) \Gamma_{\text{FHCD}(\{\text{gO2}\})}^{R*} W_H^2 \Gamma_{\text{FH0D}(\{1\})}^{L*} m_{\tilde{H}^0} \Gamma_{\text{FHCD}(\{\text{gO1}\})}^L W_H^2 \Gamma_{\text{FH0D}(\{1\})}^R \\
& - 4B_0(p^2, m_{\tilde{H}^-}^2, m_{W_L^3}^2) \Gamma_{\text{FHCD}(\{\text{gO2}\})}^{R*} W_L^3 \Gamma_{\text{FHCD}(\{1\})}^{L*} m_{\tilde{H}^-} \Gamma_{\text{FHCD}(\{\text{gO1}\})}^L W_L^3 \Gamma_{\text{FHCD}(\{1\})}^R \\
& - 4B_0(p^2, m_{\tilde{H}^-}^2, m_{W_H^3}^2) \Gamma_{\text{FHCD}(\{\text{gO2}\})}^{R*} W_H^3 \Gamma_{\text{FHCD}(\{1\})}^{L*} m_{\tilde{H}^-} \Gamma_{\text{FHCD}(\{\text{gO1}\})}^L W_H^3 \Gamma_{\text{FHCD}(\{1\})}^R \tag{352}
\end{aligned}$$

• Self-Energy for SU(3) A gluino Dirac ( $\tilde{G}_{AD}$ )

$$\Sigma^S(p^2) = + \sum_{a=1}^3 \sum_{b=1}^3 B_0(p^2, m_{d_{L,b}^D}^2, m_{\tilde{d}_{L,a}}^2) \Gamma_{\tilde{G}_{AD,j}}^{L*} \bar{d}_{L,a}^* d_{L,b}^D m_{d_{L,b}^D} \Gamma_{\tilde{G}_{AD,i}}^R \tilde{d}_{L,a}^* d_{L,b}^D$$

$$\begin{aligned}
& + \sum_{a=1}^3 \sum_{b=1}^3 B_0(p^2, m_{d_{R,b}}^2, m_{\tilde{d}_{R,a}}^2) \Gamma_{\tilde{G}_{AD,j}, \tilde{d}_{R,a}^*, d_{R,b}^D}^{L*} m_{d_{R,b}^D} \Gamma_{\tilde{G}_{AD,i}, \tilde{d}_{R,a}^*, d_{R,b}^D}^R \\
& + \sum_{a=1}^3 \sum_{b=1}^3 B_0(p^2, m_{u_{L,b}}^2, m_{\tilde{u}_{L,a}}^2) \Gamma_{\tilde{G}_{AD,j}, \tilde{u}_{L,a}^*, u_{L,b}^D}^{L*} m_{u_{L,b}^D} \Gamma_{\tilde{G}_{AD,i}, \tilde{u}_{L,a}^*, u_{L,b}^D}^R \\
& + \sum_{a=1}^3 \sum_{b=1}^3 B_0(p^2, m_{u_{R,b}}^2, m_{\tilde{u}_{R,a}}^2) \Gamma_{\tilde{G}_{AD,j}, \tilde{u}_{R,a}^*, u_{R,b}^D}^{L*} m_{u_{R,b}^D} \Gamma_{\tilde{G}_{AD,i}, \tilde{u}_{R,a}^*, u_{R,b}^D}^R \\
& - 12B_0(p^2, m_{\tilde{G}_{AD}}^2, 0) \Gamma_{\tilde{G}_{AD,j}, g, \tilde{G}_{AD,1}}^{R*} m_{\tilde{G}_{AD}} \Gamma_{\tilde{G}_{AD,i}, g, \tilde{G}_{AD,1}}^L
\end{aligned} \tag{353}$$

$$\begin{aligned}
\Sigma^R(p^2) = & + \sum_{a=1}^3 \sum_{b=1}^3 B_0(p^2, m_{d_{L,b}^D}^2, m_{\tilde{d}_{L,a}}^2) \Gamma_{\tilde{G}_{AD,j}, \tilde{d}_{L,a}^*, d_{L,b}^D}^{L*} m_{d_{L,b}^D} \Gamma_{\tilde{G}_{AD,i}, \tilde{d}_{L,a}^*, d_{L,b}^D}^R \\
& + \sum_{a=1}^3 \sum_{b=1}^3 B_0(p^2, m_{d_{R,b}}^2, m_{\tilde{d}_{R,a}}^2) \Gamma_{\tilde{G}_{AD,j}, \tilde{d}_{R,a}^*, d_{R,b}^D}^{L*} m_{d_{R,b}^D} \Gamma_{\tilde{G}_{AD,i}, \tilde{d}_{R,a}^*, d_{R,b}^D}^R \\
& + \sum_{a=1}^3 \sum_{b=1}^3 B_0(p^2, m_{u_{L,b}}^2, m_{\tilde{u}_{L,a}}^2) \Gamma_{\tilde{G}_{AD,j}, \tilde{u}_{L,a}^*, u_{L,b}^D}^{L*} m_{u_{L,b}^D} \Gamma_{\tilde{G}_{AD,i}, \tilde{u}_{L,a}^*, u_{L,b}^D}^R \\
& + \sum_{a=1}^3 \sum_{b=1}^3 B_0(p^2, m_{u_{R,b}}^2, m_{\tilde{u}_{R,a}}^2) \Gamma_{\tilde{G}_{AD,j}, \tilde{u}_{R,a}^*, u_{R,b}^D}^{L*} m_{u_{R,b}^D} \Gamma_{\tilde{G}_{AD,i}, \tilde{u}_{R,a}^*, u_{R,b}^D}^R \\
& - 12B_0(p^2, m_{\tilde{G}_{AD}}^2, 0) \Gamma_{\tilde{G}_{AD,j}, g, \tilde{G}_{AD,1}}^{R*} m_{\tilde{G}_{AD}} \Gamma_{\tilde{G}_{AD,i}, g, \tilde{G}_{AD,1}}^L
\end{aligned} \tag{354}$$

$$\begin{aligned}
\Sigma^L(p^2) = & + \sum_{a=1}^3 \sum_{b=1}^3 B_0(p^2, m_{d_{L,b}^D}^2, m_{\tilde{d}_{L,a}}^2) \Gamma_{\tilde{G}_{AD,j}, \tilde{d}_{L,a}^*, d_{L,b}^D}^{L*} m_{d_{L,b}^D} \Gamma_{\tilde{G}_{AD,i}, \tilde{d}_{L,a}^*, d_{L,b}^D}^R \\
& + \sum_{a=1}^3 \sum_{b=1}^3 B_0(p^2, m_{d_{R,b}}^2, m_{\tilde{d}_{R,a}}^2) \Gamma_{\tilde{G}_{AD,j}, \tilde{d}_{R,a}^*, d_{R,b}^D}^{L*} m_{d_{R,b}^D} \Gamma_{\tilde{G}_{AD,i}, \tilde{d}_{R,a}^*, d_{R,b}^D}^R \\
& + \sum_{a=1}^3 \sum_{b=1}^3 B_0(p^2, m_{u_{L,b}}^2, m_{\tilde{u}_{L,a}}^2) \Gamma_{\tilde{G}_{AD,j}, \tilde{u}_{L,a}^*, u_{L,b}^D}^{L*} m_{u_{L,b}^D} \Gamma_{\tilde{G}_{AD,i}, \tilde{u}_{L,a}^*, u_{L,b}^D}^R \\
& + \sum_{a=1}^3 \sum_{b=1}^3 B_0(p^2, m_{u_{R,b}}^2, m_{\tilde{u}_{R,a}}^2) \Gamma_{\tilde{G}_{AD,j}, \tilde{u}_{R,a}^*, u_{R,b}^D}^{L*} m_{u_{R,b}^D} \Gamma_{\tilde{G}_{AD,i}, \tilde{u}_{R,a}^*, u_{R,b}^D}^R \\
& - 12B_0(p^2, m_{\tilde{G}_{AD}}^2, 0) \Gamma_{\tilde{G}_{AD,j}, g, \tilde{G}_{AD,1}}^{R*} m_{\tilde{G}_{AD}} \Gamma_{\tilde{G}_{AD,i}, g, \tilde{G}_{AD,1}}^L
\end{aligned} \tag{355}$$

• Self-Energy for Left Down-Squarks ( $\tilde{d}_L$ )

$$\begin{aligned}
\Pi_{i,j}(p^2) = & + 2A_0(m_{B_L}^2) \Gamma_{\tilde{d}_{L,i}, \tilde{d}_{L,i}^*, B_L, B_L} + 2A_0(m_{B_H}^2) \Gamma_{\tilde{d}_{L,i}, \tilde{d}_{L,i}^*, B_H, B_H} + 2A_0(m_{W_L^1}^2) \Gamma_{\tilde{d}_{L,i}, \tilde{d}_{L,i}^*, W_L^1, W_L^1} \\
& + 2A_0(m_{W_H^1}^2) \Gamma_{\tilde{d}_{L,i}, \tilde{d}_{L,i}^*, W_H^1, W_H^1} + 2A_0(m_{W_L^2}^2) \Gamma_{\tilde{d}_{L,i}, \tilde{d}_{L,i}^*, W_L^2, W_L^2} + 2A_0(m_{W_H^2}^2) \Gamma_{\tilde{d}_{L,i}, \tilde{d}_{L,i}^*, W_H^2, W_H^2} \\
& + 2A_0(m_{W_L^3}^2) \Gamma_{\tilde{d}_{L,i}, \tilde{d}_{L,i}^*, W_L^3, W_L^3} + 2A_0(m_{W_H^3}^2) \Gamma_{\tilde{d}_{L,i}, \tilde{d}_{L,i}^*, W_H^3, W_H^3}
\end{aligned}$$

$$\begin{aligned}
& -A_0\left(m_{H_d^0}^2\right)\Gamma_{\tilde{d}_{L,i},\tilde{d}_{L,i}^*,H_d^{0,*},H_d^0}-A_0\left(m_{H_d^-}^2\right)\Gamma_{\tilde{d}_{L,i},\tilde{d}_{L,i}^*,H_d^{-,*},H_d^-}\\
& -A_0\left(m_{H_u^0}^2\right)\Gamma_{\tilde{d}_{L,i},\tilde{d}_{L,i}^*,H_u^{0,*},H_u^0}-A_0\left(m_{H_u^+}^2\right)\Gamma_{\tilde{d}_{L,i},\tilde{d}_{L,i}^*,H_u^{+,*},H_u^+}\\
& +\sum_{a=1}^3B_0\left(p^2,m_{\tilde{u}_{R,a}}^2,m_{H_d^-}^2\right)\Gamma_{\tilde{d}_{L,j}^*,\tilde{u}_{R,a},H_d^-}^*\Gamma_{\tilde{d}_{L,i},\tilde{u}_{R,a},H_d^-}-C\sum_{a=1}^3A_0\left(m_{\tilde{d}_{L,a}}^2\right)\Gamma_{\tilde{d}_{L,i},\tilde{d}_{L,i}^*,\tilde{d}_{L,a}^*,\tilde{d}_{L,a}}\\
& -C\sum_{a=1}^3A_0\left(m_{\tilde{d}_{R,a}}^2\right)\Gamma_{\tilde{d}_{L,i},\tilde{d}_{L,i}^*,\tilde{d}_{R,a}^*,\tilde{d}_{R,a}}-\sum_{a=1}^3A_0\left(m_{\tilde{e}_{L,a}}^2\right)\Gamma_{\tilde{d}_{L,i},\tilde{d}_{L,i}^*,\tilde{e}_{L,a}^*,\tilde{e}_{L,a}}\\
& -\sum_{a=1}^3A_0\left(m_{\tilde{e}_{R,a}}^2\right)\Gamma_{\tilde{d}_{L,i},\tilde{d}_{L,i}^*,\tilde{e}_{R,a}^*,\tilde{e}_{R,a}}-C\sum_{a=1}^3A_0\left(m_{\tilde{u}_{L,a}}^2\right)\Gamma_{\tilde{d}_{L,i},\tilde{d}_{L,i}^*,\tilde{u}_{L,a}^*,\tilde{u}_{L,a}}\\
& -C\sum_{a=1}^3A_0\left(m_{\tilde{u}_{R,a}}^2\right)\Gamma_{\tilde{d}_{L,i},\tilde{d}_{L,i}^*,\tilde{u}_{R,a}^*,\tilde{u}_{R,a}}-\sum_{a=1}^3A_0\left(m_{\tilde{\nu}_{L,a}}^2\right)\Gamma_{\tilde{d}_{L,i},\tilde{d}_{L,i}^*,\tilde{\nu}_{L,a}^*,\tilde{\nu}_{L,a}}\\
& +\sum_{a=1}^3\sum_{b=1}^4B_0\left(p^2,m_{\tilde{d}_{L,a}}^2,m_{\phi_{L,b}^0}^2\right)\Gamma_{\tilde{d}_{L,j}^*,\tilde{d}_{L,a},\phi_{L,b}^0}^*\Gamma_{\tilde{d}_{L,i},\tilde{d}_{L,a},\phi_{L,b}^0}\\
& -\sum_{a=1}^4A_0\left(m_{\sigma_{L,a}^\pm}^2\right)\Gamma_{\tilde{d}_{L,i},\tilde{d}_{L,i}^*,\sigma_{L,a}^{\pm,*},\sigma_{L,a}^\pm}-\frac{1}{2}\sum_{a=1}^4A_0\left(m_{\phi_{L,a}^0}^2\right)\Gamma_{\tilde{d}_{L,i},\tilde{d}_{L,i}^*,\phi_{L,a}^0,\phi_{L,a}^0}\\
& -\frac{1}{2}\sum_{a=1}^4A_0\left(m_{\sigma_{L,a}^0}^2\right)\Gamma_{\tilde{d}_{L,i},\tilde{d}_{L,i}^*,\sigma_{L,a}^0,\sigma_{L,a}^0}\\
& +\sum_{a=1}^4\sum_{b=1}^3B_0\left(p^2,m_{\sigma_{L,a}^\pm}^2,m_{\tilde{u}_{L,b}}^2\right)\Gamma_{\tilde{d}_{L,j}^*,\sigma_{L,a}^{\pm,*},\tilde{u}_{L,b}}^*\Gamma_{\tilde{d}_{L,i},\sigma_{L,a}^{\pm,*},\tilde{u}_{L,b}}\\
& -2\sum_{a=1}^{10}m_{f_{Go,a}^-}\sum_{b=1}^3B_0\left(p^2,m_{f_{Go,a}^-}^2,m_{u_{L,b}^D}^2\right)m_{u_{L,b}^D}\left(\Gamma_{\tilde{d}_{L,j}^*,f_{Go,a}^-,u_{L,b}^D}^{L*}\Gamma_{\tilde{d}_{L,i},f_{Go,a}^-,u_{L,b}^D}^R+\Gamma_{\tilde{d}_{L,j}^*,f_{Go,a}^-,u_{L,b}^D}^{R*}\Gamma_{\tilde{d}_{L,i},f_{Go,a}^-,u_{L,b}^D}^L\right)\\
& +\sum_{a=1}^{10}\sum_{b=1}^3G_0\left(p^2,m_{f_{Go,a}^-}^2,m_{u_{L,b}^D}^2\right)\left(\Gamma_{\tilde{d}_{L,j}^*,f_{Go,a}^-,u_{L,b}^D}^{L*}\Gamma_{\tilde{d}_{L,i},f_{Go,a}^-,u_{L,b}^D}^L+\Gamma_{\tilde{d}_{L,j}^*,f_{Go,a}^-,u_{L,b}^D}^{R*}\Gamma_{\tilde{d}_{L,i},f_{Go,a}^-,u_{L,b}^D}^R\right)\\
& -2\sum_{a=1}^{10}m_{f_{Po,a}^0}\sum_{b=1}^3B_0\left(p^2,m_{f_{Po,a}^0}^2,m_{d_{L,b}^D}^2\right)m_{d_{L,b}^D}\left(\Gamma_{\tilde{d}_{L,j}^*,f_{Po,a}^0,d_{L,b}^D}^{L*}\Gamma_{\tilde{d}_{L,i},f_{Po,a}^0,d_{L,b}^D}^R+\Gamma_{\tilde{d}_{L,j}^*,f_{Po,a}^0,d_{L,b}^D}^{R*}\Gamma_{\tilde{d}_{L,i},f_{Po,a}^0,d_{L,b}^D}^L\right)\\
& +\sum_{a=1}^{10}\sum_{b=1}^3G_0\left(p^2,m_{f_{Po,a}^0}^2,m_{d_{L,b}^D}^2\right)\left(\Gamma_{\tilde{d}_{L,j}^*,f_{Po,a}^0,d_{L,b}^D}^{L*}\Gamma_{\tilde{d}_{L,i},f_{Po,a}^0,d_{L,b}^D}^L+\Gamma_{\tilde{d}_{L,j}^*,f_{Po,a}^0,d_{L,b}^D}^{R*}\Gamma_{\tilde{d}_{L,i},f_{Po,a}^0,d_{L,b}^D}^R\right)\\
& +\sum_{b=1}^3B_0\left(p^2,m_{H_u^0}^2,m_{\tilde{d}_{R,b}}^2\right)\Gamma_{\tilde{d}_{L,j}^*,H_u^0,\tilde{d}_{R,b}}^*\Gamma_{\tilde{d}_{L,i},H_u^0,\tilde{d}_{R,b}}+\frac{4}{3}\sum_{b=1}^3\Gamma_{\tilde{d}_{L,j}^*,g,\tilde{d}_{L,b}}^*\Gamma_{\tilde{d}_{L,i},g,\tilde{d}_{L,b}}F_0\left(p^2,m_{\tilde{d}_{L,b}}^2,0\right)\\
& +\sum_{b=1}^3\Gamma_{\tilde{d}_{L,j}^*,B_L,\tilde{d}_{L,b}}^*\Gamma_{\tilde{d}_{L,i},B_L,\tilde{d}_{L,b}}F_0\left(p^2,m_{\tilde{d}_{L,b}}^2,m_{B_L}^2\right)
\end{aligned}$$



$$\begin{aligned}
& + \sum_{b=1}^3 \Gamma_{\tilde{d}_{L,j}^*, B_H, \tilde{d}_{L,b}}^* \Gamma_{\tilde{d}_{L,i}^*, B_H, \tilde{d}_{L,b}} F_0(p^2, m_{\tilde{d}_{L,b}}^2, m_{B_H}^2) \\
& + \sum_{b=1}^3 \Gamma_{\tilde{d}_{L,j}^*, W_L^3, \tilde{d}_{L,b}}^* \Gamma_{\tilde{d}_{L,i}^*, W_L^3, \tilde{d}_{L,b}} F_0(p^2, m_{\tilde{d}_{L,b}}^2, m_{W_L^3}^2) \\
& + \sum_{b=1}^3 \Gamma_{\tilde{d}_{L,j}^*, W_H^3, \tilde{d}_{L,b}}^* \Gamma_{\tilde{d}_{L,i}^*, W_H^3, \tilde{d}_{L,b}} F_0(p^2, m_{\tilde{d}_{L,b}}^2, m_{W_H^3}^2) \\
& + \sum_{b=1}^3 \Gamma_{\tilde{d}_{L,j}^*, W_L^1, \tilde{u}_{L,b}}^* \Gamma_{\tilde{d}_{L,i}^*, W_L^1, \tilde{u}_{L,b}} F_0(p^2, m_{\tilde{u}_{L,b}}^2, m_{W_L^1}^2) \\
& + \sum_{b=1}^3 \Gamma_{\tilde{d}_{L,j}^*, W_H^1, \tilde{u}_{L,b}}^* \Gamma_{\tilde{d}_{L,i}^*, W_H^1, \tilde{u}_{L,b}} F_0(p^2, m_{\tilde{u}_{L,b}}^2, m_{W_H^1}^2) \\
& + \sum_{b=1}^3 \Gamma_{\tilde{d}_{L,j}^*, W_L^2, \tilde{u}_{L,b}}^* \Gamma_{\tilde{d}_{L,i}^*, W_L^2, \tilde{u}_{L,b}} F_0(p^2, m_{\tilde{u}_{L,b}}^2, m_{W_L^2}^2) \\
& + \sum_{b=1}^3 \Gamma_{\tilde{d}_{L,j}^*, W_H^2, \tilde{u}_{L,b}}^* \Gamma_{\tilde{d}_{L,i}^*, W_H^2, \tilde{u}_{L,b}} F_0(p^2, m_{\tilde{u}_{L,b}}^2, m_{W_H^2}^2) \\
& - 2m_{\tilde{H}^-} \sum_{b=1}^3 B_0(p^2, m_{\tilde{H}^-}^2, m_{u_{R,b}^D}^2) m_{u_{R,b}^D} \left( \Gamma_{\tilde{d}_{L,j}^*, \text{FHCD}^-(\{1\}), u_{R,b}^D}^{L*} \Gamma_{\tilde{d}_{L,i}^*, \text{FHCD}^-(\{1\}), u_{R,b}^D}^R + \Gamma_{\tilde{d}_{L,j}^*, \text{FHCD}^-(\{1\}), u_{R,b}^D}^{R*} \Gamma_{\tilde{d}_{L,i}^*, \text{FHCD}^-(\{1\}), u_{R,b}^D}^L \right) \\
& + \sum_{b=1}^3 G_0(p^2, m_{\tilde{H}^-}^2, m_{u_{R,b}^D}^2) \left( \Gamma_{\tilde{d}_{L,j}^*, \text{FHCD}^-(\{1\}), u_{R,b}^D}^{L*} \Gamma_{\tilde{d}_{L,i}^*, \text{FHCD}^-(\{1\}), u_{R,b}^D}^L + \Gamma_{\tilde{d}_{L,j}^*, \text{FHCD}^-(\{1\}), u_{R,b}^D}^{R*} \Gamma_{\tilde{d}_{L,i}^*, \text{FHCD}^-(\{1\}), u_{R,b}^D}^R \right) \\
& - \frac{8}{3} m_{\tilde{G}_{AD}} \sum_{b=1}^3 B_0(p^2, m_{\tilde{G}_{AD}}^2, m_{d_{L,b}^D}^2) m_{d_{L,b}^D} \left( \Gamma_{\tilde{d}_{L,j}^*, \tilde{G}_{AD,1}, d_{L,b}^D}^{L*} \Gamma_{\tilde{d}_{L,i}^*, \tilde{G}_{AD,1}, d_{L,b}^D}^R + \Gamma_{\tilde{d}_{L,j}^*, \tilde{G}_{AD,1}, d_{L,b}^D}^{R*} \Gamma_{\tilde{d}_{L,i}^*, \tilde{G}_{AD,1}, d_{L,b}^D}^L \right) \\
& + \frac{4}{3} \sum_{b=1}^3 G_0(p^2, m_{\tilde{G}_{AD}}^2, m_{d_{L,b}^D}^2) \left( \Gamma_{\tilde{d}_{L,j}^*, \tilde{G}_{AD,1}, d_{L,b}^D}^{L*} \Gamma_{\tilde{d}_{L,i}^*, \tilde{G}_{AD,1}, d_{L,b}^D}^L + \Gamma_{\tilde{d}_{L,j}^*, \tilde{G}_{AD,1}, d_{L,b}^D}^{R*} \Gamma_{\tilde{d}_{L,i}^*, \tilde{G}_{AD,1}, d_{L,b}^D}^R \right) \\
& - 2m_{\tilde{H}^0} \sum_{b=1}^3 B_0(p^2, m_{\tilde{H}^0}^2, m_{d_{R,b}^D}^2) m_{d_{R,b}^D} \left( \Gamma_{\tilde{d}_{L,j}^*, \text{FH0D}(\{1\}), d_{R,b}^D}^{L*} \Gamma_{\tilde{d}_{L,i}^*, \text{FH0D}(\{1\}), d_{R,b}^D}^R + \Gamma_{\tilde{d}_{L,j}^*, \text{FH0D}(\{1\}), d_{R,b}^D}^{R*} \Gamma_{\tilde{d}_{L,i}^*, \text{FH0D}(\{1\}), d_{R,b}^D}^L \right) \\
& + \sum_{b=1}^3 G_0(p^2, m_{\tilde{H}^0}^2, m_{d_{R,b}^D}^2) \left( \Gamma_{\tilde{d}_{L,j}^*, \text{FH0D}(\{1\}), d_{R,b}^D}^{L*} \Gamma_{\tilde{d}_{L,i}^*, \text{FH0D}(\{1\}), d_{R,b}^D}^L + \Gamma_{\tilde{d}_{L,j}^*, \text{FH0D}(\{1\}), d_{R,b}^D}^{R*} \Gamma_{\tilde{d}_{L,i}^*, \text{FH0D}(\{1\}), d_{R,b}^D}^R \right)
\end{aligned} \tag{356}$$

(357)

• Self-Energy for Left Up-Squarks ( $\tilde{u}_L$ )

$$\Pi_{i,j}(p^2) = +2A_0(m_{B_L}^2) \Gamma_{\tilde{u}_{L,i}, \tilde{u}_{L,i}^*, B_L, B_L} + 2A_0(m_{B_H}^2) \Gamma_{\tilde{u}_{L,i}, \tilde{u}_{L,i}^*, B_H, B_H} + 2A_0(m_{W_L^1}^2) \Gamma_{\tilde{u}_{L,i}, \tilde{u}_{L,i}^*, W_L^1, W_L^1}$$

$$\begin{aligned}
& + 2A_0(m_{W_H^1}^2)\Gamma_{\tilde{u}_{L,i},\tilde{u}_{L,i}^*,W_H^1,W_H^1} + 2A_0(m_{W_L^2}^2)\Gamma_{\tilde{u}_{L,i},\tilde{u}_{L,i}^*,W_L^2,W_L^2} + 2A_0(m_{W_H^2}^2)\Gamma_{\tilde{u}_{L,i},\tilde{u}_{L,i}^*,W_H^2,W_H^2} \\
& + 2A_0(m_{W_L^3}^2)\Gamma_{\tilde{u}_{L,i},\tilde{u}_{L,i}^*,W_L^3,W_L^3} + 2A_0(m_{W_H^3}^2)\Gamma_{\tilde{u}_{L,i},\tilde{u}_{L,i}^*,W_H^3,W_H^3} \\
& - A_0(m_{H_d^0}^2)\Gamma_{\tilde{u}_{L,i},\tilde{u}_{L,i}^*,H_d^0,H_d^0} - A_0(m_{H_d^-}^2)\Gamma_{\tilde{u}_{L,i},\tilde{u}_{L,i}^*,H_d^-,H_d^-} \\
& - A_0(m_{H_u^0}^2)\Gamma_{\tilde{u}_{L,i},\tilde{u}_{L,i}^*,H_u^0,H_u^0} - A_0(m_{H_u^+}^2)\Gamma_{\tilde{u}_{L,i},\tilde{u}_{L,i}^*,H_u^+,H_u^+} \\
& + \sum_{a=1}^3 B_0(p^2, m_{\tilde{u}_{R,a}}^2, m_{H_d^0}^2)\Gamma_{\tilde{u}_{L,j}^*,\tilde{u}_{R,a},H_d^0}^* \Gamma_{\tilde{u}_{L,i},\tilde{u}_{R,a},H_d^0} - C \sum_{a=1}^3 A_0(m_{\tilde{d}_{L,a}}^2)\Gamma_{\tilde{u}_{L,i},\tilde{u}_{L,i}^*,\tilde{d}_{L,a}^*,\tilde{d}_{L,a}} \\
& - C \sum_{a=1}^3 A_0(m_{\tilde{d}_{R,a}}^2)\Gamma_{\tilde{u}_{L,i},\tilde{u}_{L,i}^*,\tilde{d}_{R,a}^*,\tilde{d}_{R,a}} - \sum_{a=1}^3 A_0(m_{\tilde{e}_{L,a}}^2)\Gamma_{\tilde{u}_{L,i},\tilde{u}_{L,i}^*,\tilde{e}_{L,a}^*,\tilde{e}_{L,a}} \\
& - \sum_{a=1}^3 A_0(m_{\tilde{e}_{R,a}}^2)\Gamma_{\tilde{u}_{L,i},\tilde{u}_{L,i}^*,\tilde{e}_{R,a}^*,\tilde{e}_{R,a}} - C \sum_{a=1}^3 A_0(m_{\tilde{u}_{L,a}}^2)\Gamma_{\tilde{u}_{L,i},\tilde{u}_{L,i}^*,\tilde{u}_{L,a}^*,\tilde{u}_{L,a}} \\
& - C \sum_{a=1}^3 A_0(m_{\tilde{u}_{R,a}}^2)\Gamma_{\tilde{u}_{L,i},\tilde{u}_{L,i}^*,\tilde{u}_{R,a}^*,\tilde{u}_{R,a}} - \sum_{a=1}^3 A_0(m_{\tilde{\nu}_{L,a}}^2)\Gamma_{\tilde{u}_{L,i},\tilde{u}_{L,i}^*,\tilde{\nu}_{L,a}^*,\tilde{\nu}_{L,a}} \\
& + \sum_{a=1}^3 \sum_{b=1}^4 B_0(p^2, m_{\tilde{d}_{L,a}}^2, m_{\sigma_{L,b}^\pm}^2)\Gamma_{\tilde{u}_{L,j}^*,\tilde{d}_{L,a},\sigma_{L,b}^\pm}^* \Gamma_{\tilde{u}_{L,i},\tilde{d}_{L,a},\sigma_{L,b}^\pm} \\
& + \sum_{a=1}^3 \sum_{b=1}^4 B_0(p^2, m_{\tilde{u}_{L,a}}^2, m_{\phi_{L,b}^0}^2)\Gamma_{\tilde{u}_{L,j}^*,\tilde{u}_{L,a},\phi_{L,b}^0}^* \Gamma_{\tilde{u}_{L,i},\tilde{u}_{L,a},\phi_{L,b}^0} \\
& - \frac{8}{3}m_{\tilde{G}_{AD}} \sum_{a=1}^3 B_0(p^2, m_{u_{L,a}^D}^2, m_{\tilde{G}_{AD}}^2)m_{u_{L,a}^D} \left( \Gamma_{\tilde{u}_{L,j}^*,u_{L,a}^D,\tilde{G}_{AD,1}}^{L*} \Gamma_{\tilde{u}_{L,i},u_{L,a}^D,\tilde{G}_{AD,1}}^R + \Gamma_{\tilde{u}_{L,j}^*,u_{L,a}^D,\tilde{G}_{AD,1}}^{R*} \Gamma_{\tilde{u}_{L,i},u_{L,a}^D,\tilde{G}_{AD,1}}^L \right) \\
& + \frac{4}{3} \sum_{a=1}^3 G_0(p^2, m_{u_{L,a}^D}^2, m_{\tilde{G}_{AD}}^2) \left( \Gamma_{\tilde{u}_{L,j}^*,u_{L,a}^D,\tilde{G}_{AD,1}}^{L*} \Gamma_{\tilde{u}_{L,i},u_{L,a}^D,\tilde{G}_{AD,1}}^L + \Gamma_{\tilde{u}_{L,j}^*,u_{L,a}^D,\tilde{G}_{AD,1}}^{R*} \Gamma_{\tilde{u}_{L,i},u_{L,a}^D,\tilde{G}_{AD,1}}^R \right) \\
& - \sum_{a=1}^4 A_0(m_{\sigma_{L,a}^\pm}^2)\Gamma_{\tilde{u}_{L,i},\tilde{u}_{L,i}^*,\sigma_{L,a}^\pm,\sigma_{L,a}^\pm} - \frac{1}{2} \sum_{a=1}^4 A_0(m_{\phi_{L,a}^0}^2)\Gamma_{\tilde{u}_{L,i},\tilde{u}_{L,i}^*,\phi_{L,a}^0,\phi_{L,a}^0} \\
& - \frac{1}{2} \sum_{a=1}^4 A_0(m_{\sigma_{L,a}^0}^2)\Gamma_{\tilde{u}_{L,i},\tilde{u}_{L,i}^*,\sigma_{L,a}^0,\sigma_{L,a}^0} \\
& - 2 \sum_{a=1}^{10} m_{f_{Go,a}^-} \sum_{b=1}^3 B_0(p^2, m_{f_{Go,a}^-}^2, m_{d_{L,b}^D}^2)m_{d_{L,b}^D} \left( \Gamma_{\tilde{u}_{L,j}^*,f_{Go,a}^-,d_{L,b}^D}^{L*} \Gamma_{\tilde{u}_{L,i},f_{Go,a}^-,d_{L,b}^D}^R + \Gamma_{\tilde{u}_{L,j}^*,f_{Go,a}^-,d_{L,b}^D}^{R*} \Gamma_{\tilde{u}_{L,i},f_{Go,a}^-,d_{L,b}^D}^L \right) \\
& + \sum_{a=1}^{10} \sum_{b=1}^3 G_0(p^2, m_{f_{Go,a}^-}^2, m_{d_{L,b}^D}^2) \left( \Gamma_{\tilde{u}_{L,j}^*,f_{Go,a}^-,d_{L,b}^D}^{L*} \Gamma_{\tilde{u}_{L,i},f_{Go,a}^-,d_{L,b}^D}^L + \Gamma_{\tilde{u}_{L,j}^*,f_{Go,a}^-,d_{L,b}^D}^{R*} \Gamma_{\tilde{u}_{L,i},f_{Go,a}^-,d_{L,b}^D}^R \right) \\
& - 2 \sum_{a=1}^{10} m_{f_{Po,a}^0} \sum_{b=1}^3 B_0(p^2, m_{f_{Po,a}^0}^2, m_{u_{L,b}^D}^2)m_{u_{L,b}^D} \left( \Gamma_{\tilde{u}_{L,j}^*,f_{Po,a}^0,u_{L,b}^D}^{L*} \Gamma_{\tilde{u}_{L,i},f_{Po,a}^0,u_{L,b}^D}^R + \Gamma_{\tilde{u}_{L,j}^*,f_{Po,a}^0,u_{L,b}^D}^{R*} \Gamma_{\tilde{u}_{L,i},f_{Po,a}^0,u_{L,b}^D}^L \right)
\end{aligned}$$

$$\begin{aligned}
& + \sum_{a=1}^{10} \sum_{b=1}^3 G_0 \left( p^2, m_{f_{Po,a}^0}^2, m_{u_{L,b}^D}^2 \right) \left( \Gamma_{\tilde{u}_{L,j}^*, f_{Po,a}^0, u_{L,b}^D}^{L*} \Gamma_{\tilde{u}_{L,i}^*, f_{Po,a}^0, u_{L,b}^D}^L + \Gamma_{\tilde{u}_{L,j}^*, f_{Po,a}^0, u_{L,b}^D}^{R*} \Gamma_{\tilde{u}_{L,i}^*, f_{Po,a}^0, u_{L,b}^D}^R \right) \\
& + \sum_{b=1}^3 B_0 \left( p^2, m_{H_u^+}^2, m_{\tilde{d}_{R,b}}^2 \right) \Gamma_{\tilde{u}_{L,j}^*, H_u^+, \tilde{d}_{R,b}}^* \Gamma_{\tilde{u}_{L,i}^*, H_u^+, \tilde{d}_{R,b}} \\
& + \sum_{b=1}^3 \Gamma_{\tilde{u}_{L,j}^*, W_L^1, \tilde{d}_{L,b}}^* \Gamma_{\tilde{u}_{L,i}^*, W_L^1, \tilde{d}_{L,b}} F_0 \left( p^2, m_{\tilde{d}_{L,b}}^2, m_{W_L^1}^2 \right) \\
& + \sum_{b=1}^3 \Gamma_{\tilde{u}_{L,j}^*, W_H^1, \tilde{d}_{L,b}}^* \Gamma_{\tilde{u}_{L,i}^*, W_H^1, \tilde{d}_{L,b}} F_0 \left( p^2, m_{\tilde{d}_{L,b}}^2, m_{W_H^1}^2 \right) \\
& + \sum_{b=1}^3 \Gamma_{\tilde{u}_{L,j}^*, W_L^2, \tilde{d}_{L,b}}^* \Gamma_{\tilde{u}_{L,i}^*, W_L^2, \tilde{d}_{L,b}} F_0 \left( p^2, m_{\tilde{d}_{L,b}}^2, m_{W_L^2}^2 \right) \\
& + \sum_{b=1}^3 \Gamma_{\tilde{u}_{L,j}^*, W_H^2, \tilde{d}_{L,b}}^* \Gamma_{\tilde{u}_{L,i}^*, W_H^2, \tilde{d}_{L,b}} F_0 \left( p^2, m_{\tilde{d}_{L,b}}^2, m_{W_H^2}^2 \right) + \frac{4}{3} \sum_{b=1}^3 \Gamma_{\tilde{u}_{L,j}^*, g, \tilde{u}_{L,b}}^* \Gamma_{\tilde{u}_{L,i}^*, g, \tilde{u}_{L,b}} F_0 \left( p^2, m_{\tilde{u}_{L,b}}^2, 0 \right) \\
& + \sum_{b=1}^3 \Gamma_{\tilde{u}_{L,j}^*, B_L, \tilde{u}_{L,b}}^* \Gamma_{\tilde{u}_{L,i}^*, B_L, \tilde{u}_{L,b}} F_0 \left( p^2, m_{\tilde{u}_{L,b}}^2, m_{B_L}^2 \right) \\
& + \sum_{b=1}^3 \Gamma_{\tilde{u}_{L,j}^*, B_H, \tilde{u}_{L,b}}^* \Gamma_{\tilde{u}_{L,i}^*, B_H, \tilde{u}_{L,b}} F_0 \left( p^2, m_{\tilde{u}_{L,b}}^2, m_{B_H}^2 \right) \\
& + \sum_{b=1}^3 \Gamma_{\tilde{u}_{L,j}^*, W_L^3, \tilde{u}_{L,b}}^* \Gamma_{\tilde{u}_{L,i}^*, W_L^3, \tilde{u}_{L,b}} F_0 \left( p^2, m_{\tilde{u}_{L,b}}^2, m_{W_L^3}^2 \right) \\
& + \sum_{b=1}^3 \Gamma_{\tilde{u}_{L,j}^*, W_H^3, \tilde{u}_{L,b}}^* \Gamma_{\tilde{u}_{L,i}^*, W_H^3, \tilde{u}_{L,b}} F_0 \left( p^2, m_{\tilde{u}_{L,b}}^2, m_{W_H^3}^2 \right) \\
& - 2m_{\tilde{H}^0} \sum_{b=1}^3 B_0 \left( p^2, m_{\tilde{H}^0}^2, m_{u_{R,b}^D}^2 \right) m_{u_{R,b}^D} \left( \Gamma_{\tilde{u}_{L,j}^*, \text{FH0D}(\{1\})}^{L*}, u_{R,b}^D \Gamma_{\tilde{u}_{L,i}^*, \text{FH0D}(\{1\})}^R, u_{R,b}^D + \Gamma_{\tilde{u}_{L,j}^*, \text{FH0D}(\{1\})}^{R*}, u_{R,b}^D \Gamma_{\tilde{u}_{L,i}^*, \text{FH0D}(\{1\})}^L, u_{R,b}^D \right) \\
& + \sum_{b=1}^3 G_0 \left( p^2, m_{\tilde{H}^0}^2, m_{u_{R,b}^D}^2 \right) \left( \Gamma_{\tilde{u}_{L,j}^*, \text{FH0D}(\{1\})}^{L*}, u_{R,b}^D \Gamma_{\tilde{u}_{L,i}^*, \text{FH0D}(\{1\})}^L, u_{R,b}^D + \Gamma_{\tilde{u}_{L,j}^*, \text{FH0D}(\{1\})}^{R*}, u_{R,b}^D \Gamma_{\tilde{u}_{L,i}^*, \text{FH0D}(\{1\})}^R, u_{R,b}^D \right) \\
& - 2m_{\tilde{H}^-} \sum_{b=1}^3 B_0 \left( p^2, m_{\tilde{H}^-}^2, m_{d_{R,b}^D}^2 \right) m_{d_{R,b}^D} \left( \Gamma_{\tilde{u}_{L,j}^*, \text{FHCD}(\{1\})}^{L*}, d_{R,b}^D \Gamma_{\tilde{u}_{L,i}^*, \text{FHCD}(\{1\})}^R, d_{R,b}^D + \Gamma_{\tilde{u}_{L,j}^*, \text{FHCD}(\{1\})}^{R*}, d_{R,b}^D \Gamma_{\tilde{u}_{L,i}^*, \text{FHCD}(\{1\})}^L, d_{R,b}^D \right) \\
& + \sum_{b=1}^3 G_0 \left( p^2, m_{\tilde{H}^-}^2, m_{d_{R,b}^D}^2 \right) \left( \Gamma_{\tilde{u}_{L,j}^*, \text{FHCD}(\{1\})}^{L*}, d_{R,b}^D \Gamma_{\tilde{u}_{L,i}^*, \text{FHCD}(\{1\})}^L, d_{R,b}^D + \Gamma_{\tilde{u}_{L,j}^*, \text{FHCD}(\{1\})}^{R*}, d_{R,b}^D \Gamma_{\tilde{u}_{L,i}^*, \text{FHCD}(\{1\})}^R, d_{R,b}^D \right)
\end{aligned} \tag{358}$$

(359)

• Self-Energy for Left Selectron ( $\tilde{e}_L$ )

$$\begin{aligned}
\Pi_{i,j}(p^2) = & +2A_0(m_{B_L}^2)\Gamma_{\tilde{e}_{L,i},\tilde{e}_{L,i}^*,B_L,B_L} + 2A_0(m_{B_H}^2)\Gamma_{\tilde{e}_{L,i},\tilde{e}_{L,i}^*,B_H,B_H} + 2A_0(m_{W_L^1}^2)\Gamma_{\tilde{e}_{L,i},\tilde{e}_{L,i}^*,W_L^1,W_L^1} \\
& + 2A_0(m_{W_H^1}^2)\Gamma_{\tilde{e}_{L,i},\tilde{e}_{L,i}^*,W_H^1,W_H^1} + 2A_0(m_{W_L^2}^2)\Gamma_{\tilde{e}_{L,i},\tilde{e}_{L,i}^*,W_L^2,W_L^2} + 2A_0(m_{W_H^2}^2)\Gamma_{\tilde{e}_{L,i},\tilde{e}_{L,i}^*,W_H^2,W_H^2} \\
& + 2A_0(m_{W_L^3}^2)\Gamma_{\tilde{e}_{L,i},\tilde{e}_{L,i}^*,W_L^3,W_L^3} + 2A_0(m_{W_H^3}^2)\Gamma_{\tilde{e}_{L,i},\tilde{e}_{L,i}^*,W_H^3,W_H^3} \\
& - A_0(m_{H_d^0}^2)\Gamma_{\tilde{e}_{L,i},\tilde{e}_{L,i}^*,H_d^{0,*},H_d^0} - A_0(m_{H_d^-}^2)\Gamma_{\tilde{e}_{L,i},\tilde{e}_{L,i}^*,H_d^{-,*},H_d^-} \\
& - A_0(m_{H_u^0}^2)\Gamma_{\tilde{e}_{L,i},\tilde{e}_{L,i}^*,H_u^{0,*},H_u^0} - A_0(m_{H_u^+}^2)\Gamma_{\tilde{e}_{L,i},\tilde{e}_{L,i}^*,H_u^{+,*},H_u^+} \\
& - 3\sum_{a=1}^3 A_0(m_{\tilde{d}_{L,a}}^2)\Gamma_{\tilde{e}_{L,i},\tilde{e}_{L,i}^*,\tilde{d}_{L,a}^*,\tilde{d}_{L,a}} - 3\sum_{a=1}^3 A_0(m_{\tilde{d}_{R,a}}^2)\Gamma_{\tilde{e}_{L,i},\tilde{e}_{L,i}^*,\tilde{d}_{R,a}^*,\tilde{d}_{R,a}} \\
& - \sum_{a=1}^3 A_0(m_{\tilde{e}_{L,a}}^2)\Gamma_{\tilde{e}_{L,i},\tilde{e}_{L,i}^*,\tilde{e}_{L,a}^*,\tilde{e}_{L,a}} - \sum_{a=1}^3 A_0(m_{\tilde{e}_{R,a}}^2)\Gamma_{\tilde{e}_{L,i},\tilde{e}_{L,i}^*,\tilde{e}_{R,a}^*,\tilde{e}_{R,a}} \\
& - 3\sum_{a=1}^3 A_0(m_{\tilde{u}_{L,a}}^2)\Gamma_{\tilde{e}_{L,i},\tilde{e}_{L,i}^*,\tilde{u}_{L,a}^*,\tilde{u}_{L,a}} - 3\sum_{a=1}^3 A_0(m_{\tilde{u}_{R,a}}^2)\Gamma_{\tilde{e}_{L,i},\tilde{e}_{L,i}^*,\tilde{u}_{R,a}^*,\tilde{u}_{R,a}} \\
& - \sum_{a=1}^3 A_0(m_{\tilde{\nu}_{L,a}}^2)\Gamma_{\tilde{e}_{L,i},\tilde{e}_{L,i}^*,\tilde{\nu}_{L,a}^*,\tilde{\nu}_{L,a}} \\
& + \sum_{a=1}^3 \sum_{b=1}^4 B_0(p^2, m_{\tilde{e}_{L,a}}^2, m_{\phi_{L,b}^0}^2)\Gamma_{\tilde{e}_{L,j},\tilde{e}_{L,a},\phi_{L,b}^0}^* \Gamma_{\tilde{e}_{L,i},\tilde{e}_{L,a},\phi_{L,b}^0} \\
& - \sum_{a=1}^4 A_0(m_{\sigma_{L,a}^\pm}^2)\Gamma_{\tilde{e}_{L,i},\tilde{e}_{L,i}^*,\sigma_{L,a}^{\pm,*},\sigma_{L,a}^\pm} - \frac{1}{2}\sum_{a=1}^4 A_0(m_{\phi_{L,a}^0}^2)\Gamma_{\tilde{e}_{L,i},\tilde{e}_{L,i}^*,\phi_{L,a}^0,\phi_{L,a}^0} \\
& - \frac{1}{2}\sum_{a=1}^4 A_0(m_{\sigma_{L,a}^0}^2)\Gamma_{\tilde{e}_{L,i},\tilde{e}_{L,i}^*,\sigma_{L,a}^0,\sigma_{L,a}^0} \\
& + \sum_{a=1}^4 \sum_{b=1}^3 B_0(p^2, m_{\sigma_{L,a}^\pm}^2, m_{\tilde{\nu}_{L,b}}^2)\Gamma_{\tilde{e}_{L,j},\sigma_{L,a}^\pm,\tilde{\nu}_{L,b}}^* \Gamma_{\tilde{e}_{L,i},\sigma_{L,a}^\pm,\tilde{\nu}_{L,b}} \\
& - 2\sum_{a=1}^{10} m_{f_{G^0,a}^-} \sum_{b=1}^3 B_0(p^2, m_{f_{G^0,a}^-}^2, m_{\nu_{L,b}^D}^2)m_{\nu_{L,b}^D} \left( \Gamma_{\tilde{e}_{L,j},f_{G^0,a}^-, \nu_{L,b}^D}^{L*} \Gamma_{\tilde{e}_{L,i},f_{G^0,a}^-, \nu_{L,b}^D}^R + \Gamma_{\tilde{e}_{L,j},f_{G^0,a}^-, \nu_{L,b}^D}^{R*} \Gamma_{\tilde{e}_{L,i},f_{G^0,a}^-, \nu_{L,b}^D}^L \right) \\
& + \sum_{a=1}^{10} \sum_{b=1}^3 G_0(p^2, m_{f_{G^0,a}^-}^2, m_{\nu_{L,b}^D}^2) \left( \Gamma_{\tilde{e}_{L,j},f_{G^0,a}^-, \nu_{L,b}^D}^{L*} \Gamma_{\tilde{e}_{L,i},f_{G^0,a}^-, \nu_{L,b}^D}^L + \Gamma_{\tilde{e}_{L,j},f_{G^0,a}^-, \nu_{L,b}^D}^{R*} \Gamma_{\tilde{e}_{L,i},f_{G^0,a}^-, \nu_{L,b}^D}^R \right) \\
& - 2\sum_{a=1}^{10} m_{f_{P^0,a}^0} \sum_{b=1}^3 B_0(p^2, m_{f_{P^0,a}^0}^2, m_{e_{L,b}^D}^2)m_{e_{L,b}^D} \left( \Gamma_{\tilde{e}_{L,j},f_{P^0,a}^0, e_{L,b}^D}^{L*} \Gamma_{\tilde{e}_{L,i},f_{P^0,a}^0, e_{L,b}^D}^R + \Gamma_{\tilde{e}_{L,j},f_{P^0,a}^0, e_{L,b}^D}^{R*} \Gamma_{\tilde{e}_{L,i},f_{P^0,a}^0, e_{L,b}^D}^L \right) \\
& + \sum_{a=1}^{10} \sum_{b=1}^3 G_0(p^2, m_{f_{P^0,a}^0}^2, m_{e_{L,b}^D}^2) \left( \Gamma_{\tilde{e}_{L,j},f_{P^0,a}^0, e_{L,b}^D}^{L*} \Gamma_{\tilde{e}_{L,i},f_{P^0,a}^0, e_{L,b}^D}^L + \Gamma_{\tilde{e}_{L,j},f_{P^0,a}^0, e_{L,b}^D}^{R*} \Gamma_{\tilde{e}_{L,i},f_{P^0,a}^0, e_{L,b}^D}^R \right)
\end{aligned}$$

$$\begin{aligned}
& + \sum_{b=1}^3 B_0 \left( p^2, m_{H_u}^2, m_{\tilde{e}_{R,b}}^2 \right) \Gamma_{\tilde{e}_{L,j}, H_u^0, \tilde{e}_{R,b}}^* \Gamma_{\tilde{e}_{L,i}, H_u^0, \tilde{e}_{R,b}} \\
& + \sum_{b=1}^3 \Gamma_{\tilde{e}_{L,j}, B_L, \tilde{e}_{L,b}}^* \Gamma_{\tilde{e}_{L,i}, B_L, \tilde{e}_{L,b}} F_0 \left( p^2, m_{\tilde{e}_{L,b}}^2, m_{B_L}^2 \right) \\
& + \sum_{b=1}^3 \Gamma_{\tilde{e}_{L,j}, B_H, \tilde{e}_{L,b}}^* \Gamma_{\tilde{e}_{L,i}, B_H, \tilde{e}_{L,b}} F_0 \left( p^2, m_{\tilde{e}_{L,b}}^2, m_{B_H}^2 \right) \\
& + \sum_{b=1}^3 \Gamma_{\tilde{e}_{L,j}, W_L^3, \tilde{e}_{L,b}}^* \Gamma_{\tilde{e}_{L,i}, W_L^3, \tilde{e}_{L,b}} F_0 \left( p^2, m_{\tilde{e}_{L,b}}^2, m_{W_L^3}^2 \right) \\
& + \sum_{b=1}^3 \Gamma_{\tilde{e}_{L,j}, W_H^3, \tilde{e}_{L,b}}^* \Gamma_{\tilde{e}_{L,i}, W_H^3, \tilde{e}_{L,b}} F_0 \left( p^2, m_{\tilde{e}_{L,b}}^2, m_{W_H^3}^2 \right) \\
& + \sum_{b=1}^3 \Gamma_{\tilde{e}_{L,j}, W_L^1, \tilde{\nu}_{L,b}}^* \Gamma_{\tilde{e}_{L,i}, W_L^1, \tilde{\nu}_{L,b}} F_0 \left( p^2, m_{\tilde{\nu}_{L,b}}^2, m_{W_L^1}^2 \right) \\
& + \sum_{b=1}^3 \Gamma_{\tilde{e}_{L,j}, W_H^1, \tilde{\nu}_{L,b}}^* \Gamma_{\tilde{e}_{L,i}, W_H^1, \tilde{\nu}_{L,b}} F_0 \left( p^2, m_{\tilde{\nu}_{L,b}}^2, m_{W_H^1}^2 \right) \\
& + \sum_{b=1}^3 \Gamma_{\tilde{e}_{L,j}, W_L^2, \tilde{\nu}_{L,b}}^* \Gamma_{\tilde{e}_{L,i}, W_L^2, \tilde{\nu}_{L,b}} F_0 \left( p^2, m_{\tilde{\nu}_{L,b}}^2, m_{W_L^2}^2 \right) \\
& + \sum_{b=1}^3 \Gamma_{\tilde{e}_{L,j}, W_H^2, \tilde{\nu}_{L,b}}^* \Gamma_{\tilde{e}_{L,i}, W_H^2, \tilde{\nu}_{L,b}} F_0 \left( p^2, m_{\tilde{\nu}_{L,b}}^2, m_{W_H^2}^2 \right) \\
& - 2m_{\tilde{H}^0} \sum_{b=1}^3 B_0 \left( p^2, m_{\tilde{H}^0}^2, m_{e_{R,b}^D}^2 \right) m_{e_{R,b}^D} \left( \Gamma_{\tilde{e}_{L,j}, \text{FH0D}(\{1\})}^{L*}, e_{R,b}^D \Gamma_{\tilde{e}_{L,i}, \text{FH0D}(\{1\})}^R, e_{R,b}^D + \Gamma_{\tilde{e}_{L,j}, \text{FH0D}(\{1\})}^{R*}, e_{R,b}^D \Gamma_{\tilde{e}_{L,i}, \text{FH0D}(\{1\})}^L, e_{R,b}^D \right) \\
& + \sum_{b=1}^3 G_0 \left( p^2, m_{\tilde{H}^0}^2, m_{e_{R,b}^D}^2 \right) \left( \Gamma_{\tilde{e}_{L,j}, \text{FH0D}(\{1\})}^{L*}, e_{R,b}^D \Gamma_{\tilde{e}_{L,i}, \text{FH0D}(\{1\})}^L, e_{R,b}^D + \Gamma_{\tilde{e}_{L,j}, \text{FH0D}(\{1\})}^{R*}, e_{R,b}^D \Gamma_{\tilde{e}_{L,i}, \text{FH0D}(\{1\})}^R, e_{R,b}^D \right)
\end{aligned}
\tag{360}$$

$$\tag{361}$$

• **Self-Energy for Left Sneutrino** ( $\tilde{\nu}_L$ )

$$\begin{aligned}
\Pi_{i,j}(p^2) = & + 2A_0 \left( m_{B_L}^2 \right) \Gamma_{\tilde{\nu}_{L,i}, \tilde{\nu}_{L,i}^*, B_L, B_L} + 2A_0 \left( m_{B_H}^2 \right) \Gamma_{\tilde{\nu}_{L,i}, \tilde{\nu}_{L,i}^*, B_H, B_H} + 2A_0 \left( m_{W_L^1}^2 \right) \Gamma_{\tilde{\nu}_{L,i}, \tilde{\nu}_{L,i}^*, W_L^1, W_L^1} \\
& + 2A_0 \left( m_{W_H^1}^2 \right) \Gamma_{\tilde{\nu}_{L,i}, \tilde{\nu}_{L,i}^*, W_H^1, W_H^1} + 2A_0 \left( m_{W_L^2}^2 \right) \Gamma_{\tilde{\nu}_{L,i}, \tilde{\nu}_{L,i}^*, W_L^2, W_L^2} + 2A_0 \left( m_{W_H^2}^2 \right) \Gamma_{\tilde{\nu}_{L,i}, \tilde{\nu}_{L,i}^*, W_H^2, W_H^2} \\
& + 2A_0 \left( m_{W_L^3}^2 \right) \Gamma_{\tilde{\nu}_{L,i}, \tilde{\nu}_{L,i}^*, W_L^3, W_L^3} + 2A_0 \left( m_{W_H^3}^2 \right) \Gamma_{\tilde{\nu}_{L,i}, \tilde{\nu}_{L,i}^*, W_H^3, W_H^3} \\
& - A_0 \left( m_{H_d^0}^2 \right) \Gamma_{\tilde{\nu}_{L,i}, \tilde{\nu}_{L,i}^*, H_d^{0,*}, H_d^0} - A_0 \left( m_{H_d^-}^2 \right) \Gamma_{\tilde{\nu}_{L,i}, \tilde{\nu}_{L,i}^*, H_d^{-,*}, H_d^-}
\end{aligned}$$

$$\begin{aligned}
& -A_0\left(m_{H_u^0}^2\right)\Gamma_{\tilde{\nu}_{L,i},\tilde{\nu}_{L,i}^*,H_u^{0,*},H_u^0}-A_0\left(m_{H_u^+}^2\right)\Gamma_{\tilde{\nu}_{L,i},\tilde{\nu}_{L,i}^*,H_u^{+,*},H_u^+}\\
& -3\sum_{a=1}^3A_0\left(m_{\tilde{d}_{L,a}}^2\right)\Gamma_{\tilde{\nu}_{L,i},\tilde{\nu}_{L,i}^*,\tilde{d}_{L,a}^*,\tilde{d}_{L,a}}-3\sum_{a=1}^3A_0\left(m_{\tilde{d}_{R,a}}^2\right)\Gamma_{\tilde{\nu}_{L,i},\tilde{\nu}_{L,i}^*,\tilde{d}_{R,a}^*,\tilde{d}_{R,a}}\\
& -\sum_{a=1}^3A_0\left(m_{\tilde{e}_{L,a}}^2\right)\Gamma_{\tilde{\nu}_{L,i},\tilde{\nu}_{L,i}^*,\tilde{e}_{L,a}^*,\tilde{e}_{L,a}}-\sum_{a=1}^3A_0\left(m_{\tilde{e}_{R,a}}^2\right)\Gamma_{\tilde{\nu}_{L,i},\tilde{\nu}_{L,i}^*,\tilde{e}_{R,a}^*,\tilde{e}_{R,a}}\\
& -3\sum_{a=1}^3A_0\left(m_{\tilde{u}_{L,a}}^2\right)\Gamma_{\tilde{\nu}_{L,i},\tilde{\nu}_{L,i}^*,\tilde{u}_{L,a}^*,\tilde{u}_{L,a}}-3\sum_{a=1}^3A_0\left(m_{\tilde{u}_{R,a}}^2\right)\Gamma_{\tilde{\nu}_{L,i},\tilde{\nu}_{L,i}^*,\tilde{u}_{R,a}^*,\tilde{u}_{R,a}}\\
& -\sum_{a=1}^3A_0\left(m_{\tilde{\nu}_{L,a}}^2\right)\Gamma_{\tilde{\nu}_{L,i},\tilde{\nu}_{L,i}^*,\tilde{\nu}_{L,a}^*,\tilde{\nu}_{L,a}}\\
& +\sum_{a=1}^3\sum_{b=1}^4B_0\left(p^2,m_{\tilde{e}_{L,a}}^2,m_{\sigma_{L,b}^\pm}^2\right)\Gamma_{\tilde{\nu}_{L,j}^*,\tilde{e}_{L,a},\sigma_{L,b}^\pm}^*\Gamma_{\tilde{\nu}_{L,i}^*,\tilde{e}_{L,a},\sigma_{L,b}^\pm}\\
& +\sum_{a=1}^3\sum_{b=1}^4B_0\left(p^2,m_{\tilde{\nu}_{L,a}}^2,m_{\phi_{L,b}^0}^2\right)\Gamma_{\tilde{\nu}_{L,j}^*,\tilde{\nu}_{L,a},\phi_{L,b}^0}^*\Gamma_{\tilde{\nu}_{L,i}^*,\tilde{\nu}_{L,a},\phi_{L,b}^0}\\
& -\sum_{a=1}^4A_0\left(m_{\sigma_{L,a}^\pm}^2\right)\Gamma_{\tilde{\nu}_{L,i},\tilde{\nu}_{L,i}^*,\sigma_{L,a}^\pm,*,\sigma_{L,a}^\pm}-\frac{1}{2}\sum_{a=1}^4A_0\left(m_{\phi_{L,a}^0}^2\right)\Gamma_{\tilde{\nu}_{L,i},\tilde{\nu}_{L,i}^*,\phi_{L,a}^0,\phi_{L,a}^0}\\
& -\frac{1}{2}\sum_{a=1}^4A_0\left(m_{\sigma_{L,a}^0}^2\right)\Gamma_{\tilde{\nu}_{L,i},\tilde{\nu}_{L,i}^*,\sigma_{L,a}^0,\sigma_{L,a}^0}\\
& -2\sum_{a=1}^{10}m_{f_{Go,a}^-}\sum_{b=1}^3B_0\left(p^2,m_{f_{Go,a}^-}^2,m_{e_{L,b}^D}^2\right)m_{e_{L,b}^D}\left(\Gamma_{\tilde{\nu}_{L,j}^*,f_{Go,a}^-,e_{L,b}^D}^{L*}\Gamma_{\tilde{\nu}_{L,i}^*,f_{Go,a}^-,e_{L,b}^D}^R+\Gamma_{\tilde{\nu}_{L,j}^*,f_{Go,a}^-,e_{L,b}^D}^{R*}\Gamma_{\tilde{\nu}_{L,i}^*,f_{Go,a}^-,e_{L,b}^D}^L\right)\\
& +\sum_{a=1}^{10}\sum_{b=1}^3G_0\left(p^2,m_{f_{Go,a}^-}^2,m_{e_{L,b}^D}^2\right)\left(\Gamma_{\tilde{\nu}_{L,j}^*,f_{Go,a}^-,e_{L,b}^D}^{L*}\Gamma_{\tilde{\nu}_{L,i}^*,f_{Go,a}^-,e_{L,b}^D}^L+\Gamma_{\tilde{\nu}_{L,j}^*,f_{Go,a}^-,e_{L,b}^D}^{R*}\Gamma_{\tilde{\nu}_{L,i}^*,f_{Go,a}^-,e_{L,b}^D}^R\right)\\
& -2\sum_{a=1}^{10}m_{f_{Po,a}^0}\sum_{b=1}^3B_0\left(p^2,m_{f_{Po,a}^0}^2,m_{\nu_{L,b}^D}^2\right)m_{\nu_{L,b}^D}\left(\Gamma_{\tilde{\nu}_{L,j}^*,f_{Po,a}^0,\nu_{L,b}^D}^{L*}\Gamma_{\tilde{\nu}_{L,i}^*,f_{Po,a}^0,\nu_{L,b}^D}^R+\Gamma_{\tilde{\nu}_{L,j}^*,f_{Po,a}^0,\nu_{L,b}^D}^{R*}\Gamma_{\tilde{\nu}_{L,i}^*,f_{Po,a}^0,\nu_{L,b}^D}^L\right)\\
& +\sum_{a=1}^{10}\sum_{b=1}^3G_0\left(p^2,m_{f_{Po,a}^0}^2,m_{\nu_{L,b}^D}^2\right)\left(\Gamma_{\tilde{\nu}_{L,j}^*,f_{Po,a}^0,\nu_{L,b}^D}^{L*}\Gamma_{\tilde{\nu}_{L,i}^*,f_{Po,a}^0,\nu_{L,b}^D}^L+\Gamma_{\tilde{\nu}_{L,j}^*,f_{Po,a}^0,\nu_{L,b}^D}^{R*}\Gamma_{\tilde{\nu}_{L,i}^*,f_{Po,a}^0,\nu_{L,b}^D}^R\right)\\
& +\sum_{b=1}^3B_0\left(p^2,m_{H_u^+}^2,m_{\tilde{e}_{R,b}}^2\right)\Gamma_{\tilde{\nu}_{L,j}^*,H_u^+,\tilde{e}_{R,b}}^*\Gamma_{\tilde{\nu}_{L,i}^*,H_u^+,\tilde{e}_{R,b}}\\
& +\sum_{b=1}^3\Gamma_{\tilde{\nu}_{L,j}^*,W_L^1,\tilde{e}_{L,b}}^*\Gamma_{\tilde{\nu}_{L,i}^*,W_L^1,\tilde{e}_{L,b}}F_0\left(p^2,m_{\tilde{e}_{L,b}}^2,m_{W_L^1}^2\right)\\
& +\sum_{b=1}^3\Gamma_{\tilde{\nu}_{L,j}^*,W_H^1,\tilde{e}_{L,b}}^*\Gamma_{\tilde{\nu}_{L,i}^*,W_H^1,\tilde{e}_{L,b}}F_0\left(p^2,m_{\tilde{e}_{L,b}}^2,m_{W_H^1}^2\right)
\end{aligned}$$

$$\begin{aligned}
& + \sum_{b=1}^3 \Gamma_{\tilde{\nu}_{L,j}^*, W_L^2, \tilde{e}_{L,b}}^* \Gamma_{\tilde{\nu}_{L,i}^*, W_L^2, \tilde{e}_{L,b}} F_0(p^2, m_{\tilde{e}_{L,b}}^2, m_{W_L^2}^2) \\
& + \sum_{b=1}^3 \Gamma_{\tilde{\nu}_{L,j}^*, W_H^2, \tilde{e}_{L,b}}^* \Gamma_{\tilde{\nu}_{L,i}^*, W_H^2, \tilde{e}_{L,b}} F_0(p^2, m_{\tilde{e}_{L,b}}^2, m_{W_H^2}^2) \\
& + \sum_{b=1}^3 \Gamma_{\tilde{\nu}_{L,j}^*, B_L, \tilde{\nu}_{L,b}}^* \Gamma_{\tilde{\nu}_{L,i}^*, B_L, \tilde{\nu}_{L,b}} F_0(p^2, m_{\tilde{\nu}_{L,b}}^2, m_{B_L}^2) \\
& + \sum_{b=1}^3 \Gamma_{\tilde{\nu}_{L,j}^*, B_H, \tilde{\nu}_{L,b}}^* \Gamma_{\tilde{\nu}_{L,i}^*, B_H, \tilde{\nu}_{L,b}} F_0(p^2, m_{\tilde{\nu}_{L,b}}^2, m_{B_H}^2) \\
& + \sum_{b=1}^3 \Gamma_{\tilde{\nu}_{L,j}^*, W_L^3, \tilde{\nu}_{L,b}}^* \Gamma_{\tilde{\nu}_{L,i}^*, W_L^3, \tilde{\nu}_{L,b}} F_0(p^2, m_{\tilde{\nu}_{L,b}}^2, m_{W_L^3}^2) \\
& + \sum_{b=1}^3 \Gamma_{\tilde{\nu}_{L,j}^*, W_H^3, \tilde{\nu}_{L,b}}^* \Gamma_{\tilde{\nu}_{L,i}^*, W_H^3, \tilde{\nu}_{L,b}} F_0(p^2, m_{\tilde{\nu}_{L,b}}^2, m_{W_H^3}^2) \\
& - 2m_{\tilde{H}^-} \sum_{b=1}^3 B_0(p^2, m_{\tilde{H}^-}^2, m_{e_{R,b}^D}^2) m_{e_{R,b}^D} \left( \Gamma_{\tilde{\nu}_{L,j}^*, \text{FHCD}(\{1\})}^{L*}, e_{R,b}^D \Gamma_{\tilde{\nu}_{L,i}^*, \text{FHCD}(\{1\})}^R, e_{R,b}^D + \Gamma_{\tilde{\nu}_{L,j}^*, \text{FHCD}(\{1\})}^{R*}, e_{R,b}^D \Gamma_{\tilde{\nu}_{L,i}^*, \text{FHCD}(\{1\})}^L, e_{R,b}^D \right) \\
& + \sum_{b=1}^3 G_0(p^2, m_{\tilde{H}^-}^2, m_{e_{R,b}^D}^2) \left( \Gamma_{\tilde{\nu}_{L,j}^*, \text{FHCD}(\{1\})}^{L*}, e_{R,b}^D \Gamma_{\tilde{\nu}_{L,i}^*, \text{FHCD}(\{1\})}^L, e_{R,b}^D + \Gamma_{\tilde{\nu}_{L,j}^*, \text{FHCD}(\{1\})}^{R*}, e_{R,b}^D \Gamma_{\tilde{\nu}_{L,i}^*, \text{FHCD}(\{1\})}^R, e_{R,b}^D \right)
\end{aligned}
\tag{362}$$

$$\tag{363}$$

• Self-Energy for Neutral Down-Higgs ( $H_d^0$ )

$$\begin{aligned}
\Pi(p^2) = & + 2A_0(m_{B_L}^2) \Gamma_{H_d^0, H_d^{0,*}, B_L, B_L} + 2A_0(m_{B_H}^2) \Gamma_{H_d^0, H_d^{0,*}, B_H, B_H} + 2A_0(m_{W_L^1}^2) \Gamma_{H_d^0, H_d^{0,*}, W_L^1, W_L^1} \\
& + 2A_0(m_{W_H^1}^2) \Gamma_{H_d^0, H_d^{0,*}, W_H^1, W_H^1} + 2A_0(m_{W_L^2}^2) \Gamma_{H_d^0, H_d^{0,*}, W_L^2, W_L^2} + 2A_0(m_{W_H^2}^2) \Gamma_{H_d^0, H_d^{0,*}, W_H^2, W_H^2} \\
& + 2A_0(m_{W_L^3}^2) \Gamma_{H_d^0, H_d^{0,*}, W_L^3, W_L^3} + 2A_0(m_{W_H^3}^2) \Gamma_{H_d^0, H_d^{0,*}, W_H^3, W_H^3} - A_0(m_{H_d^0}^2) \Gamma_{H_d^0, H_d^{0,*}, H_d^{0,*}, H_d^0} \\
& - A_0(m_{H_d^-}^2) \Gamma_{H_d^0, H_d^{0,*}, H_d^{0,*}, H_d^-} - A_0(m_{H_u^0}^2) \Gamma_{H_d^0, H_d^{0,*}, H_u^{0,*}, H_u^0} \\
& - A_0(m_{H_u^+}^2) \Gamma_{H_d^0, H_d^{0,*}, H_u^{0,*}, H_u^+} + |\Gamma_{H_d^{0,*}, B_L, H_d^0}|^2 F_0(p^2, m_{H_d^0}^2, m_{B_L}^2) \\
& + |\Gamma_{H_d^{0,*}, B_H, H_d^0}|^2 F_0(p^2, m_{H_d^0}^2, m_{B_H}^2) + |\Gamma_{H_d^{0,*}, W_L^1, H_d^0}|^2 F_0(p^2, m_{H_d^0}^2, m_{W_L^1}^2) \\
& + |\Gamma_{H_d^{0,*}, W_H^1, H_d^0}|^2 F_0(p^2, m_{H_d^0}^2, m_{W_H^1}^2) + |\Gamma_{H_d^{0,*}, W_L^2, H_d^0}|^2 F_0(p^2, m_{H_d^0}^2, m_{W_L^2}^2) \\
& + |\Gamma_{H_d^{0,*}, W_H^2, H_d^0}|^2 F_0(p^2, m_{H_d^0}^2, m_{W_H^2}^2) + |\Gamma_{H_d^{0,*}, W_L^3, H_d^0}|^2 F_0(p^2, m_{H_d^0}^2, m_{W_L^3}^2) \\
& + |\Gamma_{H_d^{0,*}, W_H^3, H_d^0}|^2 F_0(p^2, m_{H_d^0}^2, m_{W_H^3}^2) - 3 \sum_{a=1}^3 A_0(m_{\tilde{d}_{L,a}}^2) \Gamma_{H_d^0, H_d^{0,*}, \tilde{d}_{L,a}^*, \tilde{d}_{L,a}}
\end{aligned}$$

$$\begin{aligned}
& -3 \sum_{a=1}^3 A_0 \left( m_{\tilde{d}_{R,a}}^2 \right) \Gamma_{H_d^0, H_d^{0,*}, \tilde{d}_{R,a}^*, \tilde{d}_{R,a}} - \sum_{a=1}^3 A_0 \left( m_{\tilde{e}_{L,a}}^2 \right) \Gamma_{H_d^0, H_d^{0,*}, \tilde{e}_{L,a}^*, \tilde{e}_{L,a}} \\
& - \sum_{a=1}^3 A_0 \left( m_{\tilde{e}_{R,a}}^2 \right) \Gamma_{H_d^0, H_d^{0,*}, \tilde{e}_{R,a}^*, \tilde{e}_{R,a}} - 3 \sum_{a=1}^3 A_0 \left( m_{\tilde{u}_{L,a}}^2 \right) \Gamma_{H_d^0, H_d^{0,*}, \tilde{u}_{L,a}^*, \tilde{u}_{L,a}} \\
& - 3 \sum_{a=1}^3 A_0 \left( m_{\tilde{u}_{R,a}}^2 \right) \Gamma_{H_d^0, H_d^{0,*}, \tilde{u}_{R,a}^*, \tilde{u}_{R,a}} - \sum_{a=1}^3 A_0 \left( m_{\tilde{\nu}_{L,a}}^2 \right) \Gamma_{H_d^0, H_d^{0,*}, \tilde{\nu}_{L,a}^*, \tilde{\nu}_{L,a}} \\
& + 3 \sum_{a=1}^3 \sum_{b=1}^3 |\Gamma_{H_d^0, H_d^{0,*}, \tilde{u}_{R,a}^*, \tilde{u}_{L,b}}|^2 B_0 \left( p^2, m_{\tilde{u}_{R,a}}^2, m_{\tilde{u}_{L,b}}^2 \right) \\
& + 3 \sum_{a=1}^3 \sum_{b=1}^3 \left( |\Gamma_{H_d^0, H_d^{0,*}, \bar{d}^{D_L, a}, d_{R,b}^D}|^2 + |\Gamma_{H_d^0, H_d^{0,*}, \bar{d}^{D_L, a}, d_{R,b}^D}|^2 \right) G_0 \left( p^2, m_{d_{L,a}^D}^2, m_{d_{R,b}^D}^2 \right) \\
& + \sum_{a=1}^3 \sum_{b=1}^3 \left( |\Gamma_{H_d^0, H_d^{0,*}, \bar{e}^{D_L, a}, e_{R,b}^D}|^2 + |\Gamma_{H_d^0, H_d^{0,*}, \bar{e}^{D_L, a}, e_{R,b}^D}|^2 \right) G_0 \left( p^2, m_{e_{L,a}^D}^2, m_{e_{R,b}^D}^2 \right) \\
& - 6 \sum_{a=1}^3 m_{\bar{d}^{D_L, a}} \sum_{b=1}^3 B_0 \left( p^2, m_{d_{L,a}^D}^2, m_{d_{R,b}^D}^2 \right) m_{d_{R,b}^D} \left( \Gamma_{H_d^0, H_d^{0,*}, \bar{d}^{D_L, a}, d_{R,b}^D} \Gamma_{H_d^0, H_d^{0,*}, \bar{d}^{D_L, a}, d_{R,b}^D}^R + \Gamma_{H_d^0, H_d^{0,*}, \bar{d}^{D_L, a}, d_{R,b}^D}^{R*} \Gamma_{H_d^0, H_d^{0,*}, \bar{d}^{D_L, a}, d_{R,b}^D}^L \right) \\
& - 2 \sum_{a=1}^3 m_{\bar{e}^{D_L, a}} \sum_{b=1}^3 B_0 \left( p^2, m_{e_{L,a}^D}^2, m_{e_{R,b}^D}^2 \right) m_{e_{R,b}^D} \left( \Gamma_{H_d^0, H_d^{0,*}, \bar{e}^{D_L, a}, e_{R,b}^D} \Gamma_{H_d^0, H_d^{0,*}, \bar{e}^{D_L, a}, e_{R,b}^D}^R + \Gamma_{H_d^0, H_d^{0,*}, \bar{e}^{D_L, a}, e_{R,b}^D}^{R*} \Gamma_{H_d^0, H_d^{0,*}, \bar{e}^{D_L, a}, e_{R,b}^D}^L \right) \\
& - \sum_{a=1}^4 A_0 \left( m_{\sigma_{L,a}^\pm}^2 \right) \Gamma_{H_d^0, H_d^{0,*}, \sigma_{L,a}^\pm, \sigma_{L,a}^\pm} - \frac{1}{2} \sum_{a=1}^4 A_0 \left( m_{\phi_{L,a}^0}^2 \right) \Gamma_{H_d^0, H_d^{0,*}, \phi_{L,a}^0, \phi_{L,a}^0} \\
& - \frac{1}{2} \sum_{a=1}^4 A_0 \left( m_{\sigma_{L,a}^0}^2 \right) \Gamma_{H_d^0, H_d^{0,*}, \sigma_{L,a}^0, \sigma_{L,a}^0} + \sum_{b=1}^4 |\Gamma_{H_d^0, H_d^{0,*}, \phi_{L,b}^0}|^2 B_0 \left( p^2, m_{H_d^0}^2, m_{\phi_{L,b}^0}^2 \right) \\
& + \sum_{b=1}^4 |\Gamma_{H_d^0, H_d^{0,*}, H_d^-, \sigma_{L,b}^\pm}|^2 B_0 \left( p^2, m_{H_d^-}^2, m_{\sigma_{L,b}^\pm}^2 \right) \\
& + \sum_{b=1}^{10} \left( |\Gamma_{H_d^0, H_d^{0,*}, \text{FH0D}^-(\{1\}), f_{P_{o,b}}^0}|^2 + |\Gamma_{H_d^0, H_d^{0,*}, \text{FH0D}^-(\{1\}), f_{P_{o,b}}^0}|^2 \right) G_0 \left( p^2, m_{\tilde{H}^0}^2, m_{f_{P_{o,b}}^0}^2 \right) \\
& + \sum_{b=1}^{10} \left( |\Gamma_{H_d^0, H_d^{0,*}, \text{FHCD}^-(\{1\}), f_{G_{o,b}}^-}|^2 + |\Gamma_{H_d^0, H_d^{0,*}, \text{FHCD}^-(\{1\}), f_{G_{o,b}}^-}|^2 \right) G_0 \left( p^2, m_{\tilde{H}^-}^2, m_{f_{G_{o,b}}^-}^2 \right) \\
& - 2m_{\tilde{H}^0} \sum_{b=1}^{10} B_0 \left( p^2, m_{\tilde{H}^0}^2, m_{f_{P_{o,b}}^0}^2 \right) m_{f_{P_{o,b}}^0} \left( \Gamma_{H_d^0, H_d^{0,*}, \text{FH0D}^-(\{1\}), f_{P_{o,b}}^0} \Gamma_{H_d^0, H_d^{0,*}, \text{FH0D}^-(\{1\}), f_{P_{o,b}}^0}^R + \Gamma_{H_d^0, H_d^{0,*}, \text{FH0D}^-(\{1\}), f_{P_{o,b}}^0}^{R*} \Gamma_{H_d^0, H_d^{0,*}, \text{FH0D}^-(\{1\}), f_{P_{o,b}}^0}^L \right) \\
& - 2m_{\tilde{H}^-} \sum_{b=1}^{10} B_0 \left( p^2, m_{\tilde{H}^-}^2, m_{f_{G_{o,b}}^-}^2 \right) m_{f_{G_{o,b}}^-} \left( \Gamma_{H_d^0, H_d^{0,*}, \text{FHCD}^-(\{1\}), f_{G_{o,b}}^-} \Gamma_{H_d^0, H_d^{0,*}, \text{FHCD}^-(\{1\}), f_{G_{o,b}}^-}^R + \Gamma_{H_d^0, H_d^{0,*}, \text{FHCD}^-(\{1\}), f_{G_{o,b}}^-}^{R*} \Gamma_{H_d^0, H_d^{0,*}, \text{FHCD}^-(\{1\}), f_{G_{o,b}}^-}^L \right)
\end{aligned}$$

(364)



• Self-Energy for Charged Down-Higgs ( $H_d^-$ )

$$\begin{aligned}
\Pi(p^2) = & +2A_0(m_{B_L}^2)\Gamma_{H_d^-, H_d^-, *, B_L, B_L} + 2A_0(m_{B_H}^2)\Gamma_{H_d^-, H_d^-, *, B_H, B_H} + 2A_0(m_{W_L^1}^2)\Gamma_{H_d^-, H_d^-, *, W_L^1, W_L^1} \\
& + 2A_0(m_{W_H^1}^2)\Gamma_{H_d^-, H_d^-, *, W_H^1, W_H^1} + 2A_0(m_{W_L^2}^2)\Gamma_{H_d^-, H_d^-, *, W_L^2, W_L^2} + 2A_0(m_{W_H^2}^2)\Gamma_{H_d^-, H_d^-, *, W_H^2, W_H^2} \\
& + 2A_0(m_{W_L^3}^2)\Gamma_{H_d^-, H_d^-, *, W_L^3, W_L^3} + 2A_0(m_{W_H^3}^2)\Gamma_{H_d^-, H_d^-, *, W_H^3, W_H^3} - A_0(m_{H_d^0}^2)\Gamma_{H_d^-, H_d^-, *, H_d^0, *, H_d^0} \\
& - A_0(m_{H_u^-}^2)\Gamma_{H_d^-, H_d^-, *, H_d^-, *, H_d^-} - A_0(m_{H_u^0}^2)\Gamma_{H_d^-, H_d^-, *, H_u^0, *, H_u^0} - A_0(m_{H_u^+}^2)\Gamma_{H_d^-, H_d^-, *, H_u^+, *, H_u^+} \\
& + |\Gamma_{H_d^-, *, W_L^1, H_d^0}|^2 F_0(p^2, m_{H_d^0}^2, m_{W_L^1}^2) + |\Gamma_{H_d^-, *, W_H^1, H_d^0}|^2 F_0(p^2, m_{H_d^0}^2, m_{W_H^1}^2) \\
& + |\Gamma_{H_d^-, *, W_L^2, H_d^0}|^2 F_0(p^2, m_{H_d^0}^2, m_{W_L^2}^2) + |\Gamma_{H_d^-, *, W_H^2, H_d^0}|^2 F_0(p^2, m_{H_d^0}^2, m_{W_H^2}^2) \\
& + |\Gamma_{H_d^-, *, B_L, H_d^-}|^2 F_0(p^2, m_{H_d^-}^2, m_{B_L}^2) + |\Gamma_{H_d^-, *, B_H, H_d^-}|^2 F_0(p^2, m_{H_d^-}^2, m_{B_H}^2) + |\Gamma_{H_d^-, *, W_L^3, H_d^-}|^2 F_0(p^2, m_{H_d^-}^2, m_{W_L^3}^2) \\
& + |\Gamma_{H_d^-, *, W_H^3, H_d^-}|^2 F_0(p^2, m_{H_d^-}^2, m_{W_H^3}^2) - 3 \sum_{a=1}^3 A_0(m_{\tilde{d}_{L,a}}^2)\Gamma_{H_d^-, H_d^-, *, \tilde{d}_{L,a}^*, \tilde{d}_{L,a}} \\
& - 3 \sum_{a=1}^3 A_0(m_{\tilde{d}_{R,a}}^2)\Gamma_{H_d^-, H_d^-, *, \tilde{d}_{R,a}^*, \tilde{d}_{R,a}} - \sum_{a=1}^3 A_0(m_{\tilde{e}_{L,a}}^2)\Gamma_{H_d^-, H_d^-, *, \tilde{e}_{L,a}^*, \tilde{e}_{L,a}} \\
& - \sum_{a=1}^3 A_0(m_{\tilde{e}_{R,a}}^2)\Gamma_{H_d^-, H_d^-, *, \tilde{e}_{R,a}^*, \tilde{e}_{R,a}} - 3 \sum_{a=1}^3 A_0(m_{\tilde{u}_{L,a}}^2)\Gamma_{H_d^-, H_d^-, *, \tilde{u}_{L,a}^*, \tilde{u}_{L,a}} \\
& - 3 \sum_{a=1}^3 A_0(m_{\tilde{u}_{R,a}}^2)\Gamma_{H_d^-, H_d^-, *, \tilde{u}_{R,a}^*, \tilde{u}_{R,a}} - \sum_{a=1}^3 A_0(m_{\tilde{\nu}_{L,a}}^2)\Gamma_{H_d^-, H_d^-, *, \tilde{\nu}_{L,a}^*, \tilde{\nu}_{L,a}} \\
& + 3 \sum_{a=1}^3 \sum_{b=1}^3 |\Gamma_{H_d^-, *, \tilde{u}_{R,a}^*, \tilde{d}_{L,b}}|^2 B_0(p^2, m_{\tilde{u}_{R,a}}^2, m_{\tilde{d}_{L,b}}^2) \\
& + 3 \sum_{a=1}^3 \sum_{b=1}^3 \left( |\Gamma_{H_d^-, *, \tilde{u}^{D_{L,a}}, d_{R,b}^D}|^2 + |\Gamma_{H_d^-, *, \tilde{u}^{D_{L,a}}, d_{R,b}^D}|^2 \right) G_0(p^2, m_{\tilde{u}_{L,a}^D}^2, m_{d_{R,b}^D}^2) \\
& + \sum_{a=1}^3 \sum_{b=1}^3 \left( |\Gamma_{H_d^-, *, \tilde{\nu}^{D_{L,a}}, e_{R,b}^D}|^2 + |\Gamma_{H_d^-, *, \tilde{\nu}^{D_{L,a}}, e_{R,b}^D}|^2 \right) G_0(p^2, m_{\tilde{\nu}_{L,a}^D}^2, m_{e_{R,b}^D}^2) \\
& - 6 \sum_{a=1}^3 m_{\tilde{u}^{D_{L,a}}} \sum_{b=1}^3 B_0(p^2, m_{\tilde{u}_{L,a}^D}^2, m_{d_{R,b}^D}^2) m_{d_{R,b}^D} \left( \Gamma_{H_d^-, *, \tilde{u}^{D_{L,a}}, d_{R,b}^D}^{L*} \Gamma_{H_d^-, *, \tilde{u}^{D_{L,a}}, d_{R,b}^D}^R + \Gamma_{H_d^-, *, \tilde{u}^{D_{L,a}}, d_{R,b}^D}^{R*} \Gamma_{H_d^-, *, \tilde{u}^{D_{L,a}}, d_{R,b}^D}^L \right) \\
& - 2 \sum_{a=1}^3 m_{\tilde{\nu}^{D_{L,a}}} \sum_{b=1}^3 B_0(p^2, m_{\tilde{\nu}_{L,a}^D}^2, m_{e_{R,b}^D}^2) m_{e_{R,b}^D} \left( \Gamma_{H_d^-, *, \tilde{\nu}^{D_{L,a}}, e_{R,b}^D}^{L*} \Gamma_{H_d^-, *, \tilde{\nu}^{D_{L,a}}, e_{R,b}^D}^R + \Gamma_{H_d^-, *, \tilde{\nu}^{D_{L,a}}, e_{R,b}^D}^{R*} \Gamma_{H_d^-, *, \tilde{\nu}^{D_{L,a}}, e_{R,b}^D}^L \right) \\
& + \sum_{a=1}^4 |\Gamma_{H_d^-, *, \sigma_{L,a}^\pm, H_d^0}|^2 B_0(p^2, m_{\sigma_{L,a}^\pm}^2, m_{H_d^0}^2) - \sum_{a=1}^4 A_0(m_{\sigma_{L,a}^\pm}^2)\Gamma_{H_d^-, H_d^-, *, \sigma_{L,a}^\pm, *, \sigma_{L,a}^\pm}
\end{aligned}$$

$$\begin{aligned}
& -\frac{1}{2} \sum_{a=1}^4 A_0(m_{\phi_{L,a}^0}^2) \Gamma_{H_d^-, H_d^-, *, \phi_{L,a}^0, \phi_{L,a}^0} - \frac{1}{2} \sum_{a=1}^4 A_0(m_{\sigma_{L,a}^0}^2) \Gamma_{H_d^-, H_d^-, *, \sigma_{L,a}^0, \sigma_{L,a}^0} \\
& + \sum_{b=1}^4 |\Gamma_{H_d^-, *, H_d^-, \phi_{L,b}^0}|^2 B_0(p^2, m_{H_d^-}^2, m_{\phi_{L,b}^0}^2) \\
& + \sum_{b=1}^{10} \left( |\Gamma_{H_d^-, *, \text{FHOD}}^L(\{1\}, f_{G_{o,b}}^-)|^2 + |\Gamma_{H_d^-, *, \text{FHOD}}^R(\{1\}, f_{G_{o,b}}^-)|^2 \right) G_0(p^2, m_{\tilde{H}^0}^2, m_{f_{G_{o,b}}^-}^2) \\
& + \sum_{b=1}^{10} \left( |\Gamma_{H_d^-, *, \text{FHCD}}^L(\{1\}, f_{P_{o,b}}^0)|^2 + |\Gamma_{H_d^-, *, \text{FHCD}}^R(\{1\}, f_{P_{o,b}}^0)|^2 \right) G_0(p^2, m_{\tilde{H}^-}^2, m_{f_{P_{o,b}}^0}^2) \\
& - 2m_{\tilde{H}^0} \sum_{b=1}^{10} B_0(p^2, m_{\tilde{H}^0}^2, m_{f_{G_{o,b}}^-}^2) m_{f_{G_{o,b}}^-} \left( \Gamma_{H_d^-, *, \text{FHOD}}^{L*}(\{1\}, f_{G_{o,b}}^-) \Gamma_{H_d^-, *, \text{FHOD}}^R(\{1\}, f_{G_{o,b}}^-) + \Gamma_{H_d^-, *, \text{FHOD}}^{R*}(\{1\}, f_{G_{o,b}}^-) \Gamma_{H_d^-, *, \text{FHOD}}^L(\{1\}, f_{G_{o,b}}^-) \right) \\
& - 2m_{\tilde{H}^-} \sum_{b=1}^{10} B_0(p^2, m_{\tilde{H}^-}^2, m_{f_{P_{o,b}}^0}^2) m_{f_{P_{o,b}}^0} \left( \Gamma_{H_d^-, *, \text{FHCD}}^{L*}(\{1\}, f_{P_{o,b}}^0) \Gamma_{H_d^-, *, \text{FHCD}}^R(\{1\}, f_{P_{o,b}}^0) + \Gamma_{H_d^-, *, \text{FHCD}}^{R*}(\{1\}, f_{P_{o,b}}^0) \Gamma_{H_d^-, *, \text{FHCD}}^L(\{1\}, f_{P_{o,b}}^0) \right)
\end{aligned} \tag{365}$$

• **Self-Energy for Neutral Up-Higgs** ( $H_u^0$ )

$$\begin{aligned}
\Pi(p^2) = & +2A_0(m_{B_L}^2) \Gamma_{H_u^0, H_u^0, *, B_L, B_L} + 2A_0(m_{B_H}^2) \Gamma_{H_u^0, H_u^0, *, B_H, B_H} + 2A_0(m_{W_L^1}^2) \Gamma_{H_u^0, H_u^0, *, W_L^1, W_L^1} \\
& + 2A_0(m_{W_H^1}^2) \Gamma_{H_u^0, H_u^0, *, W_H^1, W_H^1} + 2A_0(m_{W_L^2}^2) \Gamma_{H_u^0, H_u^0, *, W_L^2, W_L^2} + 2A_0(m_{W_H^2}^2) \Gamma_{H_u^0, H_u^0, *, W_H^2, W_H^2} \\
& + 2A_0(m_{W_L^3}^2) \Gamma_{H_u^0, H_u^0, *, W_L^3, W_L^3} + 2A_0(m_{W_H^3}^2) \Gamma_{H_u^0, H_u^0, *, W_H^3, W_H^3} - A_0(m_{H_d^0}^2) \Gamma_{H_u^0, H_u^0, *, H_d^0, *, H_d^0} \\
& - A_0(m_{H_d^-}^2) \Gamma_{H_u^0, H_u^0, *, H_d^-, *, H_d^-} - A_0(m_{H_u^0}^2) \Gamma_{H_u^0, H_u^0, *, H_u^0, *, H_u^0} - A_0(m_{H_u^+}^2) \Gamma_{H_u^0, H_u^0, *, H_u^+, *, H_u^+} \\
& + |\Gamma_{H_u^0, *, B_L, H_u^0}|^2 F_0(p^2, m_{H_u^0}^2, m_{B_L}^2) + |\Gamma_{H_u^0, *, B_H, H_u^0}|^2 F_0(p^2, m_{H_u^0}^2, m_{B_H}^2) + |\Gamma_{H_u^0, *, W_L^3, H_u^0}|^2 F_0(p^2, m_{H_u^0}^2, m_{W_L^3}^2) \\
& + |\Gamma_{H_u^0, *, W_H^3, H_u^0}|^2 F_0(p^2, m_{H_u^0}^2, m_{W_H^3}^2) + |\Gamma_{H_u^0, *, W_L^1, H_u^+}|^2 F_0(p^2, m_{H_u^+}^2, m_{W_L^1}^2) \\
& + |\Gamma_{H_u^0, *, W_H^1, H_u^+}|^2 F_0(p^2, m_{H_u^+}^2, m_{W_H^1}^2) + |\Gamma_{H_u^0, *, W_L^2, H_u^+}|^2 F_0(p^2, m_{H_u^+}^2, m_{W_L^2}^2) \\
& + |\Gamma_{H_u^0, *, W_H^2, H_u^+}|^2 F_0(p^2, m_{H_u^+}^2, m_{W_H^2}^2) - 3 \sum_{a=1}^3 A_0(m_{\tilde{d}_{L,a}}^2) \Gamma_{H_u^0, H_u^0, *, \tilde{d}_{L,a}^*, \tilde{d}_{L,a}} \\
& - 3 \sum_{a=1}^3 A_0(m_{\tilde{d}_{R,a}}^2) \Gamma_{H_u^0, H_u^0, *, \tilde{d}_{R,a}^*, \tilde{d}_{R,a}} - \sum_{a=1}^3 A_0(m_{\tilde{e}_{L,a}}^2) \Gamma_{H_u^0, H_u^0, *, \tilde{e}_{L,a}^*, \tilde{e}_{L,a}} \\
& - \sum_{a=1}^3 A_0(m_{\tilde{e}_{R,a}}^2) \Gamma_{H_u^0, H_u^0, *, \tilde{e}_{R,a}^*, \tilde{e}_{R,a}} - 3 \sum_{a=1}^3 A_0(m_{\tilde{u}_{L,a}}^2) \Gamma_{H_u^0, H_u^0, *, \tilde{u}_{L,a}^*, \tilde{u}_{L,a}}
\end{aligned}$$

$$\begin{aligned}
& -3 \sum_{a=1}^3 A_0 \left( m_{\tilde{u}_{R,a}}^2 \right) \Gamma_{H_u^0, H_u^{0,*}, \tilde{u}_{R,a}^*, \tilde{u}_{R,a}} - \sum_{a=1}^3 A_0 \left( m_{\tilde{\nu}_{L,a}}^2 \right) \Gamma_{H_u^0, H_u^{0,*}, \tilde{\nu}_{L,a}^*, \tilde{\nu}_{L,a}} \\
& + 3 \sum_{a=1}^3 \sum_{b=1}^3 |\Gamma_{H_u^{0,*}, \tilde{d}_{R,a}^*, \tilde{d}_{L,b}}|^2 B_0 \left( p^2, m_{\tilde{d}_{R,a}}^2, m_{\tilde{d}_{L,b}}^2 \right) + \sum_{a=1}^3 \sum_{b=1}^3 |\Gamma_{H_u^{0,*}, \tilde{e}_{R,a}^*, \tilde{e}_{L,b}}|^2 B_0 \left( p^2, m_{\tilde{e}_{R,a}}^2, m_{\tilde{e}_{L,b}}^2 \right) \\
& + 3 \sum_{a=1}^3 \sum_{b=1}^3 \left( |\Gamma_{H_u^{0,*}, \tilde{u}^{D_L,a}, u_{R,b}^D}|^2 + |\Gamma_{H_u^{0,*}, \tilde{u}^{D_L,a}, u_{R,b}^D}|^2 \right) G_0 \left( p^2, m_{u_{L,a}^D}^2, m_{u_{R,b}^D}^2 \right) \\
& - 6 \sum_{a=1}^3 m_{\tilde{u}^{D_L,a}} \sum_{b=1}^3 B_0 \left( p^2, m_{u_{L,a}^D}^2, m_{u_{R,b}^D}^2 \right) m_{u_{R,b}^D} \left( \Gamma_{H_u^{0,*}, \tilde{u}^{D_L,a}, u_{R,b}^D} \Gamma_{H_u^{0,*}, \tilde{u}^{D_L,a}, u_{R,b}^D}^R + \Gamma_{H_u^{0,*}, \tilde{u}^{D_L,a}, u_{R,b}^D}^{R*} \Gamma_{H_u^{0,*}, \tilde{u}^{D_L,a}, u_{R,b}^D}^L \right) \\
& + \sum_{a=1}^4 |\Gamma_{H_u^{0,*}, \sigma_{L,a}^{\pm}, H_u^+}|^2 B_0 \left( p^2, m_{\sigma_{L,a}^{\pm}}^2, m_{H_u^+}^2 \right) - \sum_{a=1}^4 A_0 \left( m_{\sigma_{L,a}^{\pm}}^2 \right) \Gamma_{H_u^0, H_u^{0,*}, \sigma_{L,a}^{\pm}, \sigma_{L,a}^{\pm}} \\
& - \frac{1}{2} \sum_{a=1}^4 A_0 \left( m_{\phi_{L,a}^0}^2 \right) \Gamma_{H_u^0, H_u^{0,*}, \phi_{L,a}^0, \phi_{L,a}^0} - \frac{1}{2} \sum_{a=1}^4 A_0 \left( m_{\sigma_{L,a}^0}^2 \right) \Gamma_{H_u^0, H_u^{0,*}, \sigma_{L,a}^0, \sigma_{L,a}^0} \\
& + \sum_{a=1}^{10} \left( |\Gamma_{H_u^{0,*}, f_{G^0,a}^-, \text{FHCD}(\{1\})}^L|^2 + |\Gamma_{H_u^{0,*}, f_{G^0,a}^-, \text{FHCD}(\{1\})}^R|^2 \right) G_0 \left( p^2, m_{f_{G^0,a}^-}^2, m_{\tilde{H}^-}^2 \right) \\
& + \sum_{a=1}^{10} \left( |\Gamma_{H_u^{0,*}, f_{P^0,a}^0, \text{FH0D}(\{1\})}^L|^2 + |\Gamma_{H_u^{0,*}, f_{P^0,a}^0, \text{FH0D}(\{1\})}^R|^2 \right) G_0 \left( p^2, m_{f_{P^0,a}^0}^2, m_{\tilde{H}^0}^2 \right) \\
& - 2m_{\tilde{H}^-} \sum_{a=1}^{10} B_0 \left( p^2, m_{f_{G^0,a}^-}^2, m_{\tilde{H}^-}^2 \right) m_{f_{G^0,a}^-} \left( \Gamma_{H_u^{0,*}, f_{G^0,a}^-, \text{FHCD}(\{1\})}^{L*} \Gamma_{H_u^{0,*}, f_{G^0,a}^-, \text{FHCD}(\{1\})}^R + \Gamma_{H_u^{0,*}, f_{G^0,a}^-, \text{FHCD}(\{1\})}^{R*} \Gamma_{H_u^{0,*}, f_{G^0,a}^-, \text{FHCD}(\{1\})}^L \right) \\
& - 2m_{\tilde{H}^0} \sum_{a=1}^{10} B_0 \left( p^2, m_{f_{P^0,a}^0}^2, m_{\tilde{H}^0}^2 \right) m_{f_{P^0,a}^0} \left( \Gamma_{H_u^{0,*}, f_{P^0,a}^0, \text{FH0D}(\{1\})}^{L*} \Gamma_{H_u^{0,*}, f_{P^0,a}^0, \text{FH0D}(\{1\})}^R + \Gamma_{H_u^{0,*}, f_{P^0,a}^0, \text{FH0D}(\{1\})}^{R*} \Gamma_{H_u^{0,*}, f_{P^0,a}^0, \text{FH0D}(\{1\})}^L \right) \\
& + \sum_{b=1}^4 |\Gamma_{H_u^{0,*}, H_u^0, \phi_{L,b}^0}|^2 B_0 \left( p^2, m_{H_u^0}^2, m_{\phi_{L,b}^0}^2 \right) \tag{366}
\end{aligned}$$

• **Self-Energy for Charged Up-Higgs ( $H_u^+$ )**

$$\begin{aligned}
\Pi(p^2) = & +2A_0 \left( m_{B_L}^2 \right) \Gamma_{H_u^+, H_u^{+,*}, B_L, B_L} + 2A_0 \left( m_{B_H}^2 \right) \Gamma_{H_u^+, H_u^{+,*}, B_H, B_H} + 2A_0 \left( m_{W_L^1}^2 \right) \Gamma_{H_u^+, H_u^{+,*}, W_L^1, W_L^1} \\
& + 2A_0 \left( m_{W_H^1}^2 \right) \Gamma_{H_u^+, H_u^{+,*}, W_H^1, W_H^1} + 2A_0 \left( m_{W_L^2}^2 \right) \Gamma_{H_u^+, H_u^{+,*}, W_L^2, W_L^2} + 2A_0 \left( m_{W_H^2}^2 \right) \Gamma_{H_u^+, H_u^{+,*}, W_H^2, W_H^2} \\
& + 2A_0 \left( m_{W_L^3}^2 \right) \Gamma_{H_u^+, H_u^{+,*}, W_L^3, W_L^3} + 2A_0 \left( m_{W_H^3}^2 \right) \Gamma_{H_u^+, H_u^{+,*}, W_H^3, W_H^3} - A_0 \left( m_{H_d^0}^2 \right) \Gamma_{H_u^+, H_u^{+,*}, H_d^{0,*}, H_d^0} \\
& - A_0 \left( m_{H_d^-}^2 \right) \Gamma_{H_u^+, H_u^{+,*}, H_d^{-,*}, H_d^-} - A_0 \left( m_{H_u^0}^2 \right) \Gamma_{H_u^+, H_u^{+,*}, H_u^0, H_u^0} - A_0 \left( m_{H_u^+}^2 \right) \Gamma_{H_u^+, H_u^{+,*}, H_u^+, H_u^+} \\
& + |\Gamma_{H_u^+, H_u^0, W_L^1}|^2 F_0 \left( p^2, m_{H_u^0}^2, m_{W_L^1}^2 \right) + |\Gamma_{H_u^+, H_u^0, W_H^1}|^2 F_0 \left( p^2, m_{H_u^0}^2, m_{W_H^1}^2 \right)
\end{aligned}$$

$$\begin{aligned}
& + |\Gamma_{H_u^+,*,W_L^2,H_u^0}|^2 F_0(p^2, m_{H_u^0}^2, m_{W_L^2}^2) + |\Gamma_{H_u^+,*,W_H^2,H_u^0}|^2 F_0(p^2, m_{H_u^0}^2, m_{W_H^2}^2) \\
& + |\Gamma_{H_u^+,*,B_L,H_u^+}|^2 F_0(p^2, m_{H_u^+}^2, m_{B_L}^2) + |\Gamma_{H_u^+,*,B_H,H_u^+}|^2 F_0(p^2, m_{H_u^+}^2, m_{B_H}^2) + |\Gamma_{H_u^+,*,W_L^3,H_u^+}|^2 F_0(p^2, m_{H_u^+}^2, m_{W_L^3}^2) \\
& + |\Gamma_{H_u^+,*,W_H^3,H_u^+}|^2 F_0(p^2, m_{H_u^+}^2, m_{W_H^3}^2) - 3 \sum_{a=1}^3 A_0(m_{\tilde{d}_{L,a}}^2) \Gamma_{H_u^+,H_u^+,*} \tilde{d}_{L,a}^* \tilde{d}_{L,a} \\
& - 3 \sum_{a=1}^3 A_0(m_{\tilde{d}_{R,a}}^2) \Gamma_{H_u^+,H_u^+,*} \tilde{d}_{R,a}^* \tilde{d}_{R,a} - \sum_{a=1}^3 A_0(m_{\tilde{e}_{L,a}}^2) \Gamma_{H_u^+,H_u^+,*} \tilde{e}_{L,a}^* \tilde{e}_{L,a} \\
& - \sum_{a=1}^3 A_0(m_{\tilde{e}_{R,a}}^2) \Gamma_{H_u^+,H_u^+,*} \tilde{e}_{R,a}^* \tilde{e}_{R,a} - 3 \sum_{a=1}^3 A_0(m_{\tilde{u}_{L,a}}^2) \Gamma_{H_u^+,H_u^+,*} \tilde{u}_{L,a}^* \tilde{u}_{L,a} \\
& - 3 \sum_{a=1}^3 A_0(m_{\tilde{u}_{R,a}}^2) \Gamma_{H_u^+,H_u^+,*} \tilde{u}_{R,a}^* \tilde{u}_{R,a} - \sum_{a=1}^3 A_0(m_{\tilde{\nu}_{L,a}}^2) \Gamma_{H_u^+,H_u^+,*} \tilde{\nu}_{L,a}^* \tilde{\nu}_{L,a} \\
& + 3 \sum_{a=1}^3 \sum_{b=1}^3 |\Gamma_{H_u^+,*,\tilde{d}_{R,a}^*,\tilde{u}_{L,b}}|^2 B_0(p^2, m_{\tilde{d}_{R,a}}^2, m_{\tilde{u}_{L,b}}^2) + \sum_{a=1}^3 \sum_{b=1}^3 |\Gamma_{H_u^+,*,\tilde{e}_{R,a}^*,\tilde{\nu}_{L,b}}|^2 B_0(p^2, m_{\tilde{e}_{R,a}}^2, m_{\tilde{\nu}_{L,b}}^2) \\
& + 3 \sum_{a=1}^3 \sum_{b=1}^3 \left( |\Gamma_{H_u^+,*,\bar{d}^{DL,a},u_{R,b}^D}|^2 + |\Gamma_{H_u^+,*,\bar{d}^{DL,a},u_{R,b}^D}|^2 \right) G_0(p^2, m_{\bar{d}_{L,a}^D}^2, m_{u_{R,b}^D}^2) \\
& - 6 \sum_{a=1}^3 m_{\bar{d}^{DL,a}} \sum_{b=1}^3 B_0(p^2, m_{\bar{d}_{L,a}^D}^2, m_{u_{R,b}^D}^2) m_{u_{R,b}^D} \left( \Gamma_{H_u^+,*,\bar{d}^{DL,a},u_{R,b}^D}^{L*} \Gamma_{H_u^+,*,\bar{d}^{DL,a},u_{R,b}^D}^R + \Gamma_{H_u^+,*,\bar{d}^{DL,a},u_{R,b}^D}^{R*} \Gamma_{H_u^+,*,\bar{d}^{DL,a},u_{R,b}^D}^L \right) \\
& - \sum_{a=1}^4 A_0(m_{\sigma_{L,a}^\pm}^2) \Gamma_{H_u^+,H_u^+,*} \sigma_{L,a}^{\pm,*} \sigma_{L,a}^\pm - \frac{1}{2} \sum_{a=1}^4 A_0(m_{\phi_{L,a}^0}^2) \Gamma_{H_u^+,H_u^+,*} \phi_{L,a}^0 \phi_{L,a}^0 \\
& - \frac{1}{2} \sum_{a=1}^4 A_0(m_{\sigma_{L,a}^0}^2) \Gamma_{H_u^+,H_u^+,*} \sigma_{L,a}^0 \sigma_{L,a}^0 \\
& + \sum_{a=1}^{10} \left( |\Gamma_{H_u^+,*,f_{Go,a}^-,FH0D}^L(\{1\})|^2 + |\Gamma_{H_u^+,*,f_{Go,a}^-,FH0D}^R(\{1\})|^2 \right) G_0(p^2, m_{f_{Go,a}^-}^2, m_{\tilde{H}^0}^2) \\
& + \sum_{a=1}^{10} \left( |\Gamma_{H_u^+,*,f_{Po,a}^0,FHCD}^L(\{1\})|^2 + |\Gamma_{H_u^+,*,f_{Po,a}^0,FHCD}^R(\{1\})|^2 \right) G_0(p^2, m_{f_{Po,a}^0}^2, m_{\tilde{H}^-}^2) \\
& - 2m_{\tilde{H}^0} \sum_{a=1}^{10} B_0(p^2, m_{f_{Go,a}^-}^2, m_{\tilde{H}^0}^2) m_{f_{Go,a}^-} \left( \Gamma_{H_u^+,*,f_{Go,a}^-,FH0D}^{L*}(\{1\}) \Gamma_{H_u^+,*,f_{Go,a}^-,FH0D}^R(\{1\}) + \Gamma_{H_u^+,*,f_{Go,a}^-,FH0D}^{R*}(\{1\}) \Gamma_{H_u^+,*,f_{Go,a}^-,FH0D}^L(\{1\}) \right) \\
& - 2m_{\tilde{H}^-} \sum_{a=1}^{10} B_0(p^2, m_{f_{Po,a}^0}^2, m_{\tilde{H}^-}^2) m_{f_{Po,a}^0} \left( \Gamma_{H_u^+,*,f_{Po,a}^0,FHCD}^{L*}(\{1\}) \Gamma_{H_u^+,*,f_{Po,a}^0,FHCD}^R(\{1\}) + \Gamma_{H_u^+,*,f_{Po,a}^0,FHCD}^{R*}(\{1\}) \Gamma_{H_u^+,*,f_{Po,a}^0,FHCD}^L(\{1\}) \right) \\
& + \sum_{b=1}^4 |\Gamma_{H_u^+,*,H_u^0,\sigma_{L,b}^\pm}|^2 B_0(p^2, m_{H_u^0}^2, m_{\sigma_{L,b}^\pm}^2) + \sum_{b=1}^4 |\Gamma_{H_u^+,*,H_u^+,\phi_{L,b}^0}|^2 B_0(p^2, m_{H_u^+}^2, m_{\phi_{L,b}^0}^2) \tag{367}
\end{aligned}$$

• Self-Energy for Right Up-Squarks ( $\tilde{u}_R$ )

$$\begin{aligned}
\Pi_{i,j}(p^2) = & +2A_0(m_{B_L}^2)\Gamma_{\tilde{u}_{R,i},\tilde{u}_{R,i}^*,B_L,B_L} + 2A_0(m_{B_H}^2)\Gamma_{\tilde{u}_{R,i},\tilde{u}_{R,i}^*,B_H,B_H} - A_0(m_{H_d^0}^2)\Gamma_{\tilde{u}_{R,i},\tilde{u}_{R,i}^*,H_d^{0,*},H_d^0} \\
& - A_0(m_{H_d^-}^2)\Gamma_{\tilde{u}_{R,i},\tilde{u}_{R,i}^*,H_d^{-,*},H_d^-} - A_0(m_{H_u^0}^2)\Gamma_{\tilde{u}_{R,i},\tilde{u}_{R,i}^*,H_u^{0,*},H_u^0} \\
& - A_0(m_{H_u^+}^2)\Gamma_{\tilde{u}_{R,i},\tilde{u}_{R,i}^*,H_u^{+,*},H_u^+} - C\sum_{a=1}^3 A_0(m_{\tilde{d}_{L,a}}^2)\Gamma_{\tilde{u}_{R,i},\tilde{u}_{R,i}^*,\tilde{d}_{L,a}^*,\tilde{d}_{L,a}} \\
& - C\sum_{a=1}^3 A_0(m_{\tilde{d}_{R,a}}^2)\Gamma_{\tilde{u}_{R,i},\tilde{u}_{R,i}^*,\tilde{d}_{R,a}^*,\tilde{d}_{R,a}} - \sum_{a=1}^3 A_0(m_{\tilde{e}_{L,a}}^2)\Gamma_{\tilde{u}_{R,i},\tilde{u}_{R,i}^*,\tilde{e}_{L,a}^*,\tilde{e}_{L,a}} \\
& - \sum_{a=1}^3 A_0(m_{\tilde{e}_{R,a}}^2)\Gamma_{\tilde{u}_{R,i},\tilde{u}_{R,i}^*,\tilde{e}_{R,a}^*,\tilde{e}_{R,a}} - C\sum_{a=1}^3 A_0(m_{\tilde{u}_{L,a}}^2)\Gamma_{\tilde{u}_{R,i},\tilde{u}_{R,i}^*,\tilde{u}_{L,a}^*,\tilde{u}_{L,a}} \\
& - C\sum_{a=1}^3 A_0(m_{\tilde{u}_{R,a}}^2)\Gamma_{\tilde{u}_{R,i},\tilde{u}_{R,i}^*,\tilde{u}_{R,a}^*,\tilde{u}_{R,a}} - \sum_{a=1}^3 A_0(m_{\tilde{\nu}_{L,a}}^2)\Gamma_{\tilde{u}_{R,i},\tilde{u}_{R,i}^*,\tilde{\nu}_{L,a}^*,\tilde{\nu}_{L,a}} \\
& + \sum_{a=1}^3 \sum_{b=1}^4 B_0(p^2, m_{\tilde{u}_{R,a}}^2, m_{\phi_{L,b}^0}^2)\Gamma_{\tilde{u}_{R,j}^*,\tilde{u}_{R,a},\phi_{L,b}^0}^* \Gamma_{\tilde{u}_{R,i}^*,\tilde{u}_{R,a},\phi_{L,b}^0} \\
& - 2m_{\tilde{H}^0} \sum_{a=1}^3 B_0(p^2, m_{u_{L,a}^D}^2, m_{\tilde{H}^0}^2)m_{u_{L,a}^D} \left( \Gamma_{\tilde{u}_{R,j}^*,u_{L,a}^D,\text{FH0D}(\{1\})}^{L*} \Gamma_{\tilde{u}_{R,i}^*,u_{L,a}^D,\text{FH0D}(\{1\})}^R + \Gamma_{\tilde{u}_{R,j}^*,u_{L,a}^D,\text{FH0D}(\{1\})}^{R*} \Gamma_{\tilde{u}_{R,i}^*,u_{L,a}^D,\text{FH0D}(\{1\})}^L \right) \\
& + \sum_{a=1}^3 G_0(p^2, m_{u_{L,a}^D}^2, m_{\tilde{H}^0}^2) \left( \Gamma_{\tilde{u}_{R,j}^*,u_{L,a}^D,\text{FH0D}(\{1\})}^{L*} \Gamma_{\tilde{u}_{R,i}^*,u_{L,a}^D,\text{FH0D}(\{1\})}^L + \Gamma_{\tilde{u}_{R,j}^*,u_{L,a}^D,\text{FH0D}(\{1\})}^{R*} \Gamma_{\tilde{u}_{R,i}^*,u_{L,a}^D,\text{FH0D}(\{1\})}^R \right) \\
& - \frac{8}{3}m_{\tilde{G}_{AD}} \sum_{a=1}^3 B_0(p^2, m_{u_{R,a}^D}^2, m_{\tilde{G}_{AD}}^2)m_{u_{R,a}^D} \left( \Gamma_{\tilde{u}_{R,j}^*,u_{R,a}^D,\tilde{G}_{AD,1}}^{L*} \Gamma_{\tilde{u}_{R,i}^*,u_{R,a}^D,\tilde{G}_{AD,1}}^R + \Gamma_{\tilde{u}_{R,j}^*,u_{R,a}^D,\tilde{G}_{AD,1}}^{R*} \Gamma_{\tilde{u}_{R,i}^*,u_{R,a}^D,\tilde{G}_{AD,1}}^L \right) \\
& + \frac{4}{3} \sum_{a=1}^3 G_0(p^2, m_{u_{R,a}^D}^2, m_{\tilde{G}_{AD}}^2) \left( \Gamma_{\tilde{u}_{R,j}^*,u_{R,a}^D,\tilde{G}_{AD,1}}^{L*} \Gamma_{\tilde{u}_{R,i}^*,u_{R,a}^D,\tilde{G}_{AD,1}}^L + \Gamma_{\tilde{u}_{R,j}^*,u_{R,a}^D,\tilde{G}_{AD,1}}^{R*} \Gamma_{\tilde{u}_{R,i}^*,u_{R,a}^D,\tilde{G}_{AD,1}}^R \right) \\
& - \sum_{a=1}^4 A_0(m_{\sigma_{L,a}^\pm}^2)\Gamma_{\tilde{u}_{R,i},\tilde{u}_{R,i}^*,\sigma_{L,a}^{\pm,*},\sigma_{L,a}^\pm} - \frac{1}{2} \sum_{a=1}^4 A_0(m_{\phi_{L,a}^0}^2)\Gamma_{\tilde{u}_{R,i},\tilde{u}_{R,i}^*,\phi_{L,a}^0,\phi_{L,a}^0} \\
& - \frac{1}{2} \sum_{a=1}^4 A_0(m_{\sigma_{L,a}^0}^2)\Gamma_{\tilde{u}_{R,i},\tilde{u}_{R,i}^*,\sigma_{L,a}^0,\sigma_{L,a}^0} \\
& - 2 \sum_{a=1}^{10} m_{f_{Po,a}^0} \sum_{b=1}^3 B_0(p^2, m_{f_{Po,a}^0}^2, m_{u_{R,b}^D}^2)m_{u_{R,b}^D} \left( \Gamma_{\tilde{u}_{R,j}^*,f_{Po,a}^0,u_{R,b}^D}^{L*} \Gamma_{\tilde{u}_{R,i}^*,f_{Po,a}^0,u_{R,b}^D}^R + \Gamma_{\tilde{u}_{R,j}^*,f_{Po,a}^0,u_{R,b}^D}^{R*} \Gamma_{\tilde{u}_{R,i}^*,f_{Po,a}^0,u_{R,b}^D}^L \right) \\
& + \sum_{a=1}^{10} \sum_{b=1}^3 G_0(p^2, m_{f_{Po,a}^0}^2, m_{u_{R,b}^D}^2) \left( \Gamma_{\tilde{u}_{R,j}^*,f_{Po,a}^0,u_{R,b}^D}^{L*} \Gamma_{\tilde{u}_{R,i}^*,f_{Po,a}^0,u_{R,b}^D}^L + \Gamma_{\tilde{u}_{R,j}^*,f_{Po,a}^0,u_{R,b}^D}^{R*} \Gamma_{\tilde{u}_{R,i}^*,f_{Po,a}^0,u_{R,b}^D}^R \right)
\end{aligned}$$

$$\begin{aligned}
& + \sum_{b=1}^3 B_0(p^2, m_{H_d^0}^2, m_{\tilde{u}_{L,b}}^2) \Gamma_{\tilde{u}_{R,j}, H_d^{0,*}, \tilde{u}_{L,b}}^* \Gamma_{\tilde{u}_{R,i}, H_d^{0,*}, \tilde{u}_{L,b}} \\
& + \sum_{b=1}^3 B_0(p^2, m_{H_d^-}^2, m_{\tilde{d}_{L,b}}^2) \Gamma_{\tilde{u}_{R,j}, H_d^{-,*}, \tilde{d}_{L,b}}^* \Gamma_{\tilde{u}_{R,i}, H_d^{-,*}, \tilde{d}_{L,b}} \\
& + \frac{4}{3} \sum_{b=1}^3 \Gamma_{\tilde{u}_{R,j}, g, \tilde{u}_{R,b}}^* \Gamma_{\tilde{u}_{R,i}, g, \tilde{u}_{R,b}} F_0(p^2, m_{\tilde{u}_{R,b}}^2, 0) + \sum_{b=1}^3 \Gamma_{\tilde{u}_{R,j}, B_L, \tilde{u}_{R,b}}^* \Gamma_{\tilde{u}_{R,i}, B_L, \tilde{u}_{R,b}} F_0(p^2, m_{\tilde{u}_{R,b}}^2, m_{B_L}^2) \\
& + \sum_{b=1}^3 \Gamma_{\tilde{u}_{R,j}, B_H, \tilde{u}_{R,b}}^* \Gamma_{\tilde{u}_{R,i}, B_H, \tilde{u}_{R,b}} F_0(p^2, m_{\tilde{u}_{R,b}}^2, m_{B_H}^2) \\
& - 2m_{\tilde{H}^-} \sum_{b=1}^3 B_0(p^2, m_{\tilde{H}^-}^2, m_{\tilde{d}_{L,b}^D}^2) m_{\tilde{d}_{L,b}^D} \left( \Gamma_{\tilde{u}_{R,j}, \text{FHCD}(\{1\})}^{L*} \Gamma_{\tilde{u}_{R,i}, \text{FHCD}(\{1\})}^R \right)_{, d_{L,b}^D} + \Gamma_{\tilde{u}_{R,j}, \text{FHCD}(\{1\})}^{R*} \Gamma_{\tilde{u}_{R,i}, \text{FHCD}(\{1\})}^L \left( \right)_{, d_{L,b}^D} \\
& + \sum_{b=1}^3 G_0(p^2, m_{\tilde{H}^-}^2, m_{\tilde{d}_{L,b}^D}^2) \left( \Gamma_{\tilde{u}_{R,j}, \text{FHCD}(\{1\})}^{L*} \Gamma_{\tilde{u}_{R,i}, \text{FHCD}(\{1\})}^L \right)_{, d_{L,b}^D} + \Gamma_{\tilde{u}_{R,j}, \text{FHCD}(\{1\})}^{R*} \Gamma_{\tilde{u}_{R,i}, \text{FHCD}(\{1\})}^R \left( \right)_{, d_{L,b}^D}
\end{aligned} \tag{368}$$

$$\tag{369}$$

• Self-Energy for Right Down-Squarks ( $\tilde{d}_R$ )

$$\begin{aligned}
\Pi_{i,j}(p^2) = & + 2A_0(m_{B_L}^2) \Gamma_{\tilde{d}_{R,i}, \tilde{d}_{R,i}^*, B_L, B_L} + 2A_0(m_{B_H}^2) \Gamma_{\tilde{d}_{R,i}, \tilde{d}_{R,i}^*, B_H, B_H} - A_0(m_{H_d^0}^2) \Gamma_{\tilde{d}_{R,i}, \tilde{d}_{R,i}^*, H_d^{0,*}, H_d^0} \\
& - A_0(m_{H_d^-}^2) \Gamma_{\tilde{d}_{R,i}, \tilde{d}_{R,i}^*, H_d^{-,*}, H_d^-} - A_0(m_{H_u^0}^2) \Gamma_{\tilde{d}_{R,i}, \tilde{d}_{R,i}^*, H_u^{0,*}, H_u^0} \\
& - A_0(m_{H_u^+}^2) \Gamma_{\tilde{d}_{R,i}, \tilde{d}_{R,i}^*, H_u^{+,*}, H_u^+} - C \sum_{a=1}^3 A_0(m_{\tilde{d}_{L,a}}^2) \Gamma_{\tilde{d}_{R,i}, \tilde{d}_{R,i}^*, \tilde{d}_{L,a}^*, \tilde{d}_{L,a}} \\
& - C \sum_{a=1}^3 A_0(m_{\tilde{d}_{R,a}}^2) \Gamma_{\tilde{d}_{R,i}, \tilde{d}_{R,i}^*, \tilde{d}_{R,a}^*, \tilde{d}_{R,a}} - \sum_{a=1}^3 A_0(m_{\tilde{e}_{L,a}}^2) \Gamma_{\tilde{d}_{R,i}, \tilde{d}_{R,i}^*, \tilde{e}_{L,a}^*, \tilde{e}_{L,a}} \\
& - \sum_{a=1}^3 A_0(m_{\tilde{e}_{R,a}}^2) \Gamma_{\tilde{d}_{R,i}, \tilde{d}_{R,i}^*, \tilde{e}_{R,a}^*, \tilde{e}_{R,a}} - C \sum_{a=1}^3 A_0(m_{\tilde{u}_{L,a}}^2) \Gamma_{\tilde{d}_{R,i}, \tilde{d}_{R,i}^*, \tilde{u}_{L,a}^*, \tilde{u}_{L,a}} \\
& - C \sum_{a=1}^3 A_0(m_{\tilde{u}_{R,a}}^2) \Gamma_{\tilde{d}_{R,i}, \tilde{d}_{R,i}^*, \tilde{u}_{R,a}^*, \tilde{u}_{R,a}} - \sum_{a=1}^3 A_0(m_{\tilde{\nu}_{L,a}}^2) \Gamma_{\tilde{d}_{R,i}, \tilde{d}_{R,i}^*, \tilde{\nu}_{L,a}^*, \tilde{\nu}_{L,a}} \\
& + \sum_{a=1}^3 \sum_{b=1}^4 B_0(p^2, m_{\tilde{d}_{R,a}}^2, m_{\phi_{L,b}^0}^2) \Gamma_{\tilde{d}_{R,j}, \tilde{d}_{R,a}, \phi_{L,b}^0}^* \Gamma_{\tilde{d}_{R,i}, \tilde{d}_{R,a}, \phi_{L,b}^0} \\
& - \sum_{a=1}^4 A_0(m_{\sigma_{L,a}^\pm}^2) \Gamma_{\tilde{d}_{R,i}, \tilde{d}_{R,i}^*, \sigma_{L,a}^{\pm,*}, \sigma_{L,a}^\pm} - \frac{1}{2} \sum_{a=1}^4 A_0(m_{\phi_{L,a}^0}^2) \Gamma_{\tilde{d}_{R,i}, \tilde{d}_{R,i}^*, \phi_{L,a}^0, \phi_{L,a}^0}
\end{aligned}$$

$$\begin{aligned}
& -\frac{1}{2} \sum_{a=1}^4 A_0(m_{\sigma_{L,a}^0}^2) \Gamma_{\tilde{d}_{R,i}, \tilde{d}_{R,i}^*, \sigma_{L,a}^0, \sigma_{L,a}^0} \\
& -2 \sum_{a=1}^{10} m_{f_{Po,a}^0} \sum_{b=1}^3 B_0(p^2, m_{f_{Po,a}^0}^2, m_{d_{R,b}^D}^2) m_{d_{R,b}^D} \left( \Gamma_{\tilde{d}_{R,j}, f_{Po,a}^0, d_{R,b}^D}^{L*} \Gamma_{\tilde{d}_{R,i}, f_{Po,a}^0, d_{R,b}^D}^R + \Gamma_{\tilde{d}_{R,j}, f_{Po,a}^0, d_{R,b}^D}^{R*} \Gamma_{\tilde{d}_{R,i}, f_{Po,a}^0, d_{R,b}^D}^L \right) \\
& + \sum_{a=1}^{10} \sum_{b=1}^3 G_0(p^2, m_{f_{Po,a}^0}^2, m_{d_{R,b}^D}^2) \left( \Gamma_{\tilde{d}_{R,j}, f_{Po,a}^0, d_{R,b}^D}^{L*} \Gamma_{\tilde{d}_{R,i}, f_{Po,a}^0, d_{R,b}^D}^L + \Gamma_{\tilde{d}_{R,j}, f_{Po,a}^0, d_{R,b}^D}^{R*} \Gamma_{\tilde{d}_{R,i}, f_{Po,a}^0, d_{R,b}^D}^R \right) \\
& + \sum_{b=1}^3 B_0(p^2, m_{H_u^0}^2, m_{\tilde{d}_{L,b}}^2) \Gamma_{\tilde{d}_{R,j}, H_u^0, *, \tilde{d}_{L,b}}^* \Gamma_{\tilde{d}_{R,i}, H_u^0, *, \tilde{d}_{L,b}} \\
& + \sum_{b=1}^3 B_0(p^2, m_{H_u^+}^2, m_{\tilde{u}_{L,b}}^2) \Gamma_{\tilde{d}_{R,j}, H_u^+, *, \tilde{u}_{L,b}}^* \Gamma_{\tilde{d}_{R,i}, H_u^+, *, \tilde{u}_{L,b}} \\
& + \frac{4}{3} \sum_{b=1}^3 \Gamma_{\tilde{d}_{R,j}, g, \tilde{d}_{R,b}}^* \Gamma_{\tilde{d}_{R,i}, g, \tilde{d}_{R,b}} F_0(p^2, m_{\tilde{d}_{R,b}}^2, 0) + \sum_{b=1}^3 \Gamma_{\tilde{d}_{R,j}, B_L, \tilde{d}_{R,b}}^* \Gamma_{\tilde{d}_{R,i}, B_L, \tilde{d}_{R,b}} F_0(p^2, m_{\tilde{d}_{R,b}}^2, m_{B_L}^2) \\
& + \sum_{b=1}^3 \Gamma_{\tilde{d}_{R,j}, B_H, \tilde{d}_{R,b}}^* \Gamma_{\tilde{d}_{R,i}, B_H, \tilde{d}_{R,b}} F_0(p^2, m_{\tilde{d}_{R,b}}^2, m_{B_H}^2) \\
& - 2m_{\tilde{H}^0} \sum_{b=1}^3 B_0(p^2, m_{\tilde{H}^0}^2, m_{d_{L,b}^D}^2) m_{d_{L,b}^D} \left( \Gamma_{\tilde{d}_{R,j}, \text{FH0D}^-(\{1\}), d_{L,b}^D}^{L*} \Gamma_{\tilde{d}_{R,i}, \text{FH0D}^-(\{1\}), d_{L,b}^D}^R + \Gamma_{\tilde{d}_{R,j}, \text{FH0D}^-(\{1\}), d_{L,b}^D}^{R*} \Gamma_{\tilde{d}_{R,i}, \text{FH0D}^-(\{1\}), d_{L,b}^D}^L \right) \\
& + \sum_{b=1}^3 G_0(p^2, m_{\tilde{H}^0}^2, m_{d_{L,b}^D}^2) \left( \Gamma_{\tilde{d}_{R,j}, \text{FH0D}^-(\{1\}), d_{L,b}^D}^{L*} \Gamma_{\tilde{d}_{R,i}, \text{FH0D}^-(\{1\}), d_{L,b}^D}^L + \Gamma_{\tilde{d}_{R,j}, \text{FH0D}^-(\{1\}), d_{L,b}^D}^{R*} \Gamma_{\tilde{d}_{R,i}, \text{FH0D}^-(\{1\}), d_{L,b}^D}^R \right) \\
& - 2m_{\tilde{H}^-} \sum_{b=1}^3 B_0(p^2, m_{\tilde{H}^-}^2, m_{u_{L,b}^D}^2) m_{u_{L,b}^D} \left( \Gamma_{\tilde{d}_{R,j}, \text{FHCD}^-(\{1\}), u_{L,b}^D}^{L*} \Gamma_{\tilde{d}_{R,i}, \text{FHCD}^-(\{1\}), u_{L,b}^D}^R + \Gamma_{\tilde{d}_{R,j}, \text{FHCD}^-(\{1\}), u_{L,b}^D}^{R*} \Gamma_{\tilde{d}_{R,i}, \text{FHCD}^-(\{1\}), u_{L,b}^D}^L \right) \\
& + \sum_{b=1}^3 G_0(p^2, m_{\tilde{H}^-}^2, m_{u_{L,b}^D}^2) \left( \Gamma_{\tilde{d}_{R,j}, \text{FHCD}^-(\{1\}), u_{L,b}^D}^{L*} \Gamma_{\tilde{d}_{R,i}, \text{FHCD}^-(\{1\}), u_{L,b}^D}^L + \Gamma_{\tilde{d}_{R,j}, \text{FHCD}^-(\{1\}), u_{L,b}^D}^{R*} \Gamma_{\tilde{d}_{R,i}, \text{FHCD}^-(\{1\}), u_{L,b}^D}^R \right) \\
& - \frac{8}{3} \tilde{m}_{\tilde{G}_{AD}} \sum_{b=1}^3 B_0(p^2, m_{\tilde{G}_{AD}}^2, m_{d_{R,b}^D}^2) m_{d_{R,b}^D} \left( \Gamma_{\tilde{d}_{R,j}, \tilde{G}_{AD,1}, d_{R,b}^D}^{L*} \Gamma_{\tilde{d}_{R,i}, \tilde{G}_{AD,1}, d_{R,b}^D}^R + \Gamma_{\tilde{d}_{R,j}, \tilde{G}_{AD,1}, d_{R,b}^D}^{R*} \Gamma_{\tilde{d}_{R,i}, \tilde{G}_{AD,1}, d_{R,b}^D}^L \right) \\
& + \frac{4}{3} \sum_{b=1}^3 G_0(p^2, m_{\tilde{G}_{AD}}^2, m_{d_{R,b}^D}^2) \left( \Gamma_{\tilde{d}_{R,j}, \tilde{G}_{AD,1}, d_{R,b}^D}^{L*} \Gamma_{\tilde{d}_{R,i}, \tilde{G}_{AD,1}, d_{R,b}^D}^L + \Gamma_{\tilde{d}_{R,j}, \tilde{G}_{AD,1}, d_{R,b}^D}^{R*} \Gamma_{\tilde{d}_{R,i}, \tilde{G}_{AD,1}, d_{R,b}^D}^R \right) \quad (370)
\end{aligned}$$

(371)

• **Self-Energy for Right Selectron** ( $\tilde{e}_R$ )

$$\Pi_{i,j}(p^2) = +2A_0(m_{B_L}^2) \Gamma_{\tilde{e}_{R,i}, \tilde{e}_{R,i}^*, B_L, B_L} + 2A_0(m_{B_H}^2) \Gamma_{\tilde{e}_{R,i}, \tilde{e}_{R,i}^*, B_H, B_H} - A_0(m_{H_d^0}^2) \Gamma_{\tilde{e}_{R,i}, \tilde{e}_{R,i}^*, H_d^0, H_d^0}$$

$$\begin{aligned}
& -A_0\left(m_{H_d^-}^2\right)\Gamma_{\tilde{e}_{R,i},\tilde{e}_{R,i}^*,H_d^-,*,H_d^-}-A_0\left(m_{H_u^0}^2\right)\Gamma_{\tilde{e}_{R,i},\tilde{e}_{R,i}^*,H_u^{0,*},H_u^0}\\
& -A_0\left(m_{H_u^+}^2\right)\Gamma_{\tilde{e}_{R,i},\tilde{e}_{R,i}^*,H_u^{+,*},H_u^+}-3\sum_{a=1}^3A_0\left(m_{\tilde{d}_{L,a}}^2\right)\Gamma_{\tilde{e}_{R,i},\tilde{e}_{R,i}^*,\tilde{d}_{L,a}^*,\tilde{d}_{L,a}}\\
& -3\sum_{a=1}^3A_0\left(m_{\tilde{d}_{R,a}}^2\right)\Gamma_{\tilde{e}_{R,i},\tilde{e}_{R,i}^*,\tilde{d}_{R,a}^*,\tilde{d}_{R,a}}-\sum_{a=1}^3A_0\left(m_{\tilde{e}_{L,a}}^2\right)\Gamma_{\tilde{e}_{R,i},\tilde{e}_{R,i}^*,\tilde{e}_{L,a}^*,\tilde{e}_{L,a}}\\
& -\sum_{a=1}^3A_0\left(m_{\tilde{e}_{R,a}}^2\right)\Gamma_{\tilde{e}_{R,i},\tilde{e}_{R,i}^*,\tilde{e}_{R,a}^*,\tilde{e}_{R,a}}-3\sum_{a=1}^3A_0\left(m_{\tilde{u}_{L,a}}^2\right)\Gamma_{\tilde{e}_{R,i},\tilde{e}_{R,i}^*,\tilde{u}_{L,a}^*,\tilde{u}_{L,a}}\\
& -3\sum_{a=1}^3A_0\left(m_{\tilde{u}_{R,a}}^2\right)\Gamma_{\tilde{e}_{R,i},\tilde{e}_{R,i}^*,\tilde{u}_{R,a}^*,\tilde{u}_{R,a}}-\sum_{a=1}^3A_0\left(m_{\tilde{\nu}_{L,a}}^2\right)\Gamma_{\tilde{e}_{R,i},\tilde{e}_{R,i}^*,\tilde{\nu}_{L,a}^*,\tilde{\nu}_{L,a}}\\
& +\sum_{a=1}^3\sum_{b=1}^4B_0\left(p^2,m_{\tilde{e}_{R,a}}^2,m_{\phi_{L,b}^0}^2\right)\Gamma_{\tilde{e}_{R,j},\tilde{e}_{R,a},\phi_{L,b}^0}^*\Gamma_{\tilde{e}_{R,i},\tilde{e}_{R,a},\phi_{L,b}^0}\\
& -\sum_{a=1}^4A_0\left(m_{\sigma_{L,a}^\pm}^2\right)\Gamma_{\tilde{e}_{R,i},\tilde{e}_{R,i}^*,\sigma_{L,a}^\pm,*,\sigma_{L,a}^\pm}-\frac{1}{2}\sum_{a=1}^4A_0\left(m_{\phi_{L,a}^0}^2\right)\Gamma_{\tilde{e}_{R,i},\tilde{e}_{R,i}^*,\phi_{L,a}^0,\phi_{L,a}^0}\\
& -\frac{1}{2}\sum_{a=1}^4A_0\left(m_{\sigma_{L,a}^0}^2\right)\Gamma_{\tilde{e}_{R,i},\tilde{e}_{R,i}^*,\sigma_{L,a}^0,\sigma_{L,a}^0}\\
& -2\sum_{a=1}^{10}m_{f_{Po,a}^0}\sum_{b=1}^3B_0\left(p^2,m_{f_{Po,a}^0}^2,m_{e_{R,b}^D}^2\right)m_{e_{R,b}^D}\left(\Gamma_{\tilde{e}_{R,j},f_{Po,a}^0,e_{R,b}^D}^{L*}\Gamma_{\tilde{e}_{R,i},f_{Po,a}^0,e_{R,b}^D}^R+\Gamma_{\tilde{e}_{R,j},f_{Po,a}^0,e_{R,b}^D}^{R*}\Gamma_{\tilde{e}_{R,i},f_{Po,a}^0,e_{R,b}^D}^L\right)\\
& +\sum_{a=1}^{10}\sum_{b=1}^3G_0\left(p^2,m_{f_{Po,a}^0}^2,m_{e_{R,b}^D}^2\right)\left(\Gamma_{\tilde{e}_{R,j},f_{Po,a}^0,e_{R,b}^D}^{L*}\Gamma_{\tilde{e}_{R,i},f_{Po,a}^0,e_{R,b}^D}^L+\Gamma_{\tilde{e}_{R,j},f_{Po,a}^0,e_{R,b}^D}^{R*}\Gamma_{\tilde{e}_{R,i},f_{Po,a}^0,e_{R,b}^D}^R\right)\\
& +\sum_{b=1}^3B_0\left(p^2,m_{H_u^0}^2,m_{\tilde{e}_{L,b}}^2\right)\Gamma_{\tilde{e}_{R,j},H_u^{0,*},\tilde{e}_{L,b}}^*\Gamma_{\tilde{e}_{R,i},H_u^{0,*},\tilde{e}_{L,b}}\\
& +\sum_{b=1}^3B_0\left(p^2,m_{H_u^+}^2,m_{\tilde{\nu}_{L,b}}^2\right)\Gamma_{\tilde{e}_{R,j},H_u^{+,*},\tilde{\nu}_{L,b}}^*\Gamma_{\tilde{e}_{R,i},H_u^{+,*},\tilde{\nu}_{L,b}}\\
& +\sum_{b=1}^3\Gamma_{\tilde{e}_{R,j},B_L,\tilde{e}_{R,b}}^*\Gamma_{\tilde{e}_{R,i},B_L,\tilde{e}_{R,b}}F_0\left(p^2,m_{\tilde{e}_{R,b}}^2,m_{B_L}^2\right)\\
& +\sum_{b=1}^3\Gamma_{\tilde{e}_{R,j},B_H,\tilde{e}_{R,b}}^*\Gamma_{\tilde{e}_{R,i},B_H,\tilde{e}_{R,b}}F_0\left(p^2,m_{\tilde{e}_{R,b}}^2,m_{B_H}^2\right)\\
& -2m_{\tilde{H}^0}\sum_{b=1}^3B_0\left(p^2,m_{\tilde{H}^0}^2,m_{e_{L,b}^D}^2\right)m_{e_{L,b}^D}\left(\Gamma_{\tilde{e}_{R,j},\text{FH0D}\left(\{1\}\right),e_{L,b}^D}^{L*}\Gamma_{\tilde{e}_{R,i},\text{FH0D}\left(\{1\}\right),e_{L,b}^D}^R+\Gamma_{\tilde{e}_{R,j},\text{FH0D}\left(\{1\}\right),e_{L,b}^D}^{R*}\Gamma_{\tilde{e}_{R,i},\text{FH0D}\left(\{1\}\right),e_{L,b}^D}^L\right)\\
& +\sum_{b=1}^3G_0\left(p^2,m_{\tilde{H}^0}^2,m_{e_{L,b}^D}^2\right)\left(\Gamma_{\tilde{e}_{R,j},\text{FH0D}\left(\{1\}\right),e_{L,b}^D}^{L*}\Gamma_{\tilde{e}_{R,i},\text{FH0D}\left(\{1\}\right),e_{L,b}^D}^L+\Gamma_{\tilde{e}_{R,j},\text{FH0D}\left(\{1\}\right),e_{L,b}^D}^{R*}\Gamma_{\tilde{e}_{R,i},\text{FH0D}\left(\{1\}\right),e_{L,b}^D}^R\right)
\end{aligned}$$



$$\begin{aligned}
& -2m_{\tilde{H}^-} \sum_{b=1}^3 B_0(p^2, m_{\tilde{H}^-}^2, m_{\nu_{L,b}^D}^2) m_{\nu_{L,b}^D} \left( \Gamma_{\tilde{e}_{R,j}^*, \text{FHCD}(\{1\})}^{L*} \Gamma_{\nu_{L,b}^D, \tilde{e}_{R,i}^*, \text{FHCD}(\{1\})}^R + \Gamma_{\tilde{e}_{R,j}^*, \text{FHCD}(\{1\})}^{R*} \Gamma_{\nu_{L,b}^D, \tilde{e}_{R,i}^*, \text{FHCD}(\{1\})}^L \right) \\
& + \sum_{b=1}^3 G_0(p^2, m_{\tilde{H}^-}^2, m_{\nu_{L,b}^D}^2) \left( \Gamma_{\tilde{e}_{R,j}^*, \text{FHCD}(\{1\})}^{L*} \Gamma_{\nu_{L,b}^D, \tilde{e}_{R,i}^*, \text{FHCD}(\{1\})}^L + \Gamma_{\tilde{e}_{R,j}^*, \text{FHCD}(\{1\})}^{R*} \Gamma_{\nu_{L,b}^D, \tilde{e}_{R,i}^*, \text{FHCD}(\{1\})}^R \right)
\end{aligned} \tag{372}$$

$$\tag{373}$$

• Self-Energy for Light B gauge boson ( $B_L$ )

$$\begin{aligned}
\Pi(p^2) = & |\Gamma_{B_L, H_d^{0,*}, H_d^0}|^2 \left( -2A_0(m_{H_d^0}^2) - 4B_{22}(p^2, m_{H_d^0}^2, m_{H_d^0}^2) \right) \\
& + |\Gamma_{B_L, H_d^-, *, H_d^-}|^2 \left( -2A_0(m_{H_d^-}^2) - 4B_{22}(p^2, m_{H_d^-}^2, m_{H_d^-}^2) \right) \\
& + |\Gamma_{B_L, H_u^{0,*}, H_u^0}|^2 \left( -2A_0(m_{H_u^0}^2) - 4B_{22}(p^2, m_{H_u^0}^2, m_{H_u^0}^2) \right) \\
& + |\Gamma_{B_L, H_u^+, *, H_u^+}|^2 \left( -2A_0(m_{H_u^+}^2) - 4B_{22}(p^2, m_{H_u^+}^2, m_{H_u^+}^2) \right) + A_0(m_{H_d^0}^2) \Gamma_{B_L, B_L, H_d^{0,*}, H_d^0} \\
& + A_0(m_{H_d^-}^2) \Gamma_{B_L, B_L, H_d^-, *, H_d^-} + A_0(m_{H_u^0}^2) \Gamma_{B_L, B_L, H_u^{0,*}, H_u^0} + A_0(m_{H_u^+}^2) \Gamma_{B_L, B_L, H_u^+, *, H_u^+} \\
& + \frac{1}{2} \left( 4B_0(p^2, m_{\tilde{H}^0}^2, m_{\tilde{H}^0}^2) m_{\tilde{H}^0} m_{\tilde{H}^0} \Re \left( \Gamma_{B_L, \text{FH0D}(\{1\})}^{L*} \Gamma_{B_L, \text{FH0D}(\{1\})}^R \right) + \left( |\Gamma_{B_L, \text{FH0D}(\{1\})}^L| \Gamma_{B_L, \text{FH0D}(\{1\})}^R \right) \right) \\
& + \frac{1}{2} \left( 4B_0(p^2, m_{\tilde{H}^-}^2, m_{\tilde{H}^-}^2) m_{\tilde{H}^-} m_{\tilde{H}^-} \Re \left( \Gamma_{B_L, \text{FHCD}(\{1\})}^{L*} \Gamma_{B_L, \text{FHCD}(\{1\})}^R \right) + \left( |\Gamma_{B_L, \text{FHCD}(\{1\})}^L| \Gamma_{B_L, \text{FHCD}(\{1\})}^R \right) \right) \\
& + 3 \sum_{a=1}^3 A_0(m_{\tilde{d}_{L,a}}^2) \Gamma_{B_L, B_L, \tilde{d}_{L,a}^*, \tilde{d}_{L,a}} + 3 \sum_{a=1}^3 A_0(m_{\tilde{d}_{R,a}}^2) \Gamma_{B_L, B_L, \tilde{d}_{R,a}^*, \tilde{d}_{R,a}} \\
& + \sum_{a=1}^3 A_0(m_{\tilde{e}_{L,a}}^2) \Gamma_{B_L, B_L, \tilde{e}_{L,a}^*, \tilde{e}_{L,a}} + \sum_{a=1}^3 A_0(m_{\tilde{e}_{R,a}}^2) \Gamma_{B_L, B_L, \tilde{e}_{R,a}^*, \tilde{e}_{R,a}} \\
& + 3 \sum_{a=1}^3 A_0(m_{\tilde{u}_{L,a}}^2) \Gamma_{B_L, B_L, \tilde{u}_{L,a}^*, \tilde{u}_{L,a}} + 3 \sum_{a=1}^3 A_0(m_{\tilde{u}_{R,a}}^2) \Gamma_{B_L, B_L, \tilde{u}_{R,a}^*, \tilde{u}_{R,a}} \\
& + \sum_{a=1}^3 A_0(m_{\tilde{\nu}_{L,a}}^2) \Gamma_{B_L, B_L, \tilde{\nu}_{L,a}^*, \tilde{\nu}_{L,a}} \\
& + 3 \sum_{a=1}^3 \sum_{b=1}^3 |\Gamma_{B_L, \tilde{d}_{L,a}^*, \tilde{d}_{L,b}}|^2 \left( -4B_{22}(p^2, m_{\tilde{d}_{L,a}}^2, m_{\tilde{d}_{L,b}}^2) - A_0(m_{\tilde{d}_{L,a}}^2) - A_0(m_{\tilde{d}_{L,b}}^2) \right) \\
& + 3 \sum_{a=1}^3 \sum_{b=1}^3 |\Gamma_{B_L, \tilde{d}_{R,a}^*, \tilde{d}_{R,b}}|^2 \left( -4B_{22}(p^2, m_{\tilde{d}_{R,a}}^2, m_{\tilde{d}_{R,b}}^2) - A_0(m_{\tilde{d}_{R,a}}^2) - A_0(m_{\tilde{d}_{R,b}}^2) \right)
\end{aligned}$$

$$\begin{aligned}
& + \sum_{a=1}^3 \sum_{b=1}^3 |\Gamma_{B_L, \tilde{e}_{L,a}^*, \tilde{e}_{L,b}}|^2 \left( -4B_{22}(p^2, m_{\tilde{e}_{L,a}}^2, m_{\tilde{e}_{L,b}}^2) - A_0(m_{\tilde{e}_{L,a}}^2) - A_0(m_{\tilde{e}_{L,b}}^2) \right) \\
& + \sum_{a=1}^3 \sum_{b=1}^3 |\Gamma_{B_L, \tilde{e}_{R,a}^*, \tilde{e}_{R,b}}|^2 \left( -4B_{22}(p^2, m_{\tilde{e}_{R,a}}^2, m_{\tilde{e}_{R,b}}^2) - A_0(m_{\tilde{e}_{R,a}}^2) - A_0(m_{\tilde{e}_{R,b}}^2) \right) \\
& + 3 \sum_{a=1}^3 \sum_{b=1}^3 |\Gamma_{B_L, \tilde{u}_{L,a}^*, \tilde{u}_{L,b}}|^2 \left( -4B_{22}(p^2, m_{\tilde{u}_{L,a}}^2, m_{\tilde{u}_{L,b}}^2) - A_0(m_{\tilde{u}_{L,a}}^2) - A_0(m_{\tilde{u}_{L,b}}^2) \right) \\
& + 3 \sum_{a=1}^3 \sum_{b=1}^3 |\Gamma_{B_L, \tilde{u}_{R,a}^*, \tilde{u}_{R,b}}|^2 \left( -4B_{22}(p^2, m_{\tilde{u}_{R,a}}^2, m_{\tilde{u}_{R,b}}^2) - A_0(m_{\tilde{u}_{R,a}}^2) - A_0(m_{\tilde{u}_{R,b}}^2) \right) \\
& + \sum_{a=1}^3 \sum_{b=1}^3 |\Gamma_{B_L, \tilde{\nu}_{L,a}^*, \tilde{\nu}_{L,b}}|^2 \left( -4B_{22}(p^2, m_{\tilde{\nu}_{L,a}}^2, m_{\tilde{\nu}_{L,b}}^2) - A_0(m_{\tilde{\nu}_{L,a}}^2) - A_0(m_{\tilde{\nu}_{L,b}}^2) \right) \\
& + \frac{3}{2} \sum_{a=1}^3 \sum_{b=1}^3 \left[ \left( |\Gamma_{B_L, \bar{d}^{D_L,a}, d_{L,b}^D}|^2 + |\Gamma_{B_L, \bar{d}^{D_L,a}, d_{L,b}^D}|^2 \right) H_0(p^2, m_{d_{L,a}^D}^2, m_{d_{L,b}^D}^2) \right. \\
& + 4B_0(p^2, m_{d_{L,a}^D}^2, m_{d_{L,b}^D}^2) m_{\bar{d}^{D_L,a}} m_{d_{L,b}^D} \Re \left( \Gamma_{B_L, \bar{d}^{D_L,a}, d_{L,b}^D}^{L*} \Gamma_{B_L, \bar{d}^{D_L,a}, d_{L,b}^D}^R \right) \Big] \\
& + \frac{3}{2} \sum_{a=1}^3 \sum_{b=1}^3 \left[ \left( |\Gamma_{B_L, \bar{d}^{D_R,a}, d_{R,b}^D}|^2 + |\Gamma_{B_L, \bar{d}^{D_R,a}, d_{R,b}^D}|^2 \right) H_0(p^2, m_{d_{R,a}^D}^2, m_{d_{R,b}^D}^2) \right. \\
& + 4B_0(p^2, m_{d_{R,a}^D}^2, m_{d_{R,b}^D}^2) m_{\bar{d}^{D_R,a}} m_{d_{R,b}^D} \Re \left( \Gamma_{B_L, \bar{d}^{D_R,a}, d_{R,b}^D}^{L*} \Gamma_{B_L, \bar{d}^{D_R,a}, d_{R,b}^D}^R \right) \Big] \\
& + \frac{1}{2} \sum_{a=1}^3 \sum_{b=1}^3 \left[ \left( |\Gamma_{B_L, \bar{e}^{D_L,a}, e_{L,b}^D}|^2 + |\Gamma_{B_L, \bar{e}^{D_L,a}, e_{L,b}^D}|^2 \right) H_0(p^2, m_{e_{L,a}^D}^2, m_{e_{L,b}^D}^2) \right. \\
& + 4B_0(p^2, m_{e_{L,a}^D}^2, m_{e_{L,b}^D}^2) m_{\bar{e}^{D_L,a}} m_{e_{L,b}^D} \Re \left( \Gamma_{B_L, \bar{e}^{D_L,a}, e_{L,b}^D}^{L*} \Gamma_{B_L, \bar{e}^{D_L,a}, e_{L,b}^D}^R \right) \Big] \\
& + \frac{1}{2} \sum_{a=1}^3 \sum_{b=1}^3 \left[ \left( |\Gamma_{B_L, \bar{e}^{D_R,a}, e_{R,b}^D}|^2 + |\Gamma_{B_L, \bar{e}^{D_R,a}, e_{R,b}^D}|^2 \right) H_0(p^2, m_{e_{R,a}^D}^2, m_{e_{R,b}^D}^2) \right. \\
& + 4B_0(p^2, m_{e_{R,a}^D}^2, m_{e_{R,b}^D}^2) m_{\bar{e}^{D_R,a}} m_{e_{R,b}^D} \Re \left( \Gamma_{B_L, \bar{e}^{D_R,a}, e_{R,b}^D}^{L*} \Gamma_{B_L, \bar{e}^{D_R,a}, e_{R,b}^D}^R \right) \Big] \\
& + \frac{3}{2} \sum_{a=1}^3 \sum_{b=1}^3 \left[ \left( |\Gamma_{B_L, \bar{u}^{D_L,a}, u_{L,b}^D}|^2 + |\Gamma_{B_L, \bar{u}^{D_L,a}, u_{L,b}^D}|^2 \right) H_0(p^2, m_{u_{L,a}^D}^2, m_{u_{L,b}^D}^2) \right. \\
& + 4B_0(p^2, m_{u_{L,a}^D}^2, m_{u_{L,b}^D}^2) m_{\bar{u}^{D_L,a}} m_{u_{L,b}^D} \Re \left( \Gamma_{B_L, \bar{u}^{D_L,a}, u_{L,b}^D}^{L*} \Gamma_{B_L, \bar{u}^{D_L,a}, u_{L,b}^D}^R \right) \Big] \\
& + \frac{3}{2} \sum_{a=1}^3 \sum_{b=1}^3 \left[ \left( |\Gamma_{B_L, \bar{u}^{D_R,a}, u_{R,b}^D}|^2 + |\Gamma_{B_L, \bar{u}^{D_R,a}, u_{R,b}^D}|^2 \right) H_0(p^2, m_{u_{R,a}^D}^2, m_{u_{R,b}^D}^2) \right. \\
& + 4B_0(p^2, m_{u_{R,a}^D}^2, m_{u_{R,b}^D}^2) m_{\bar{u}^{D_R,a}} m_{u_{R,b}^D} \Re \left( \Gamma_{B_L, \bar{u}^{D_R,a}, u_{R,b}^D}^{L*} \Gamma_{B_L, \bar{u}^{D_R,a}, u_{R,b}^D}^R \right) \Big] \\
& + \frac{1}{2} \sum_{a=1}^3 \sum_{b=1}^3 \left[ \left( |\Gamma_{B_L, \bar{\nu}^{D_L,a}, \nu_{L,b}^D}|^2 + |\Gamma_{B_L, \bar{\nu}^{D_L,a}, \nu_{L,b}^D}|^2 \right) H_0(p^2, m_{\nu_{L,a}^D}^2, m_{\nu_{L,b}^D}^2) \right.
\end{aligned}$$

$$\begin{aligned}
& + 4B_0 \left( p^2, m_{\nu_{L,a}^D}^2, m_{\nu_{L,b}^D}^2 \right) m_{\bar{\nu}^{D_L,a}} m_{\nu_{L,b}^D} \Re \left( \Gamma_{B_L, \bar{\nu}^{D_L,a}, \nu_{L,b}^D}^{L*} \Gamma_{B_L, \bar{\nu}^{D_L,a}, \nu_{L,b}^D}^R \right) \Big] \\
& + \sum_{a=1}^4 A_0 \left( m_{\sigma_{L,a}^\pm}^2 \right) \Gamma_{B_L, B_L, \sigma_{L,a}^\pm, *} \sigma_{L,a}^\pm + \frac{1}{2} \sum_{a=1}^4 A_0 \left( m_{\phi_{L,a}^0}^2 \right) \Gamma_{B_L, B_L, \phi_{L,a}^0, \phi_{L,a}^0} \\
& + \frac{1}{2} \sum_{a=1}^4 A_0 \left( m_{\sigma_{L,a}^0}^2 \right) \Gamma_{B_L, B_L, \sigma_{L,a}^0, \sigma_{L,a}^0} \\
& + \sum_{a=1}^4 \sum_{b=1}^4 |\Gamma_{B_L, \sigma_{L,a}^\pm, *} \sigma_{L,b}^\pm|^2 \left( -4B_{22} \left( p^2, m_{\sigma_{L,a}^\pm}^2, m_{\sigma_{L,b}^\pm}^2 \right) - A_0 \left( m_{\sigma_{L,a}^\pm}^2 \right) - A_0 \left( m_{\sigma_{L,b}^\pm}^2 \right) \right) \\
& + \sum_{a=1}^4 \sum_{b=1}^4 |\Gamma_{B_L, \sigma_{L,a}^0, \phi_{L,b}^0}|^2 \left( -4B_{22} \left( p^2, m_{\phi_{L,a}^0}^2, m_{\sigma_{L,b}^0}^2 \right) - A_0 \left( m_{\phi_{L,a}^0}^2 \right) - A_0 \left( m_{\sigma_{L,b}^0}^2 \right) \right) \\
& + \frac{1}{4} \sum_{a=1}^{10} \sum_{b=1}^{10} \left[ \left( |\Gamma_{B_L, f_{G^0,a}^-, f_{G^0,b}^-}^L|^2 + |\Gamma_{B_L, f_{G^0,a}^-, f_{G^0,b}^-}^R|^2 \right) H_0 \left( p^2, m_{f_{G^0,a}^-}^2, m_{f_{G^0,b}^-}^2 \right) \right. \\
& \left. + 4B_0 \left( p^2, m_{f_{G^0,a}^-}^2, m_{f_{G^0,b}^-}^2 \right) m_{f_{G^0,a}^-} m_{f_{G^0,b}^-} \Re \left( \Gamma_{B_L, f_{G^0,a}^-, f_{G^0,b}^-}^{L*} \Gamma_{B_L, f_{G^0,a}^-, f_{G^0,b}^-}^R \right) \right] \\
& + \frac{1}{4} \sum_{a=1}^{10} \sum_{b=1}^{10} \left[ \left( |\Gamma_{B_L, f_{P^0,a}^0, f_{P^0,b}^0}^L|^2 + |\Gamma_{B_L, f_{P^0,a}^0, f_{P^0,b}^0}^R|^2 \right) H_0 \left( p^2, m_{f_{P^0,a}^0}^2, m_{f_{P^0,b}^0}^2 \right) \right. \\
& \left. + 4B_0 \left( p^2, m_{f_{P^0,a}^0}^2, m_{f_{P^0,b}^0}^2 \right) m_{f_{P^0,a}^0} m_{f_{P^0,b}^0} \Re \left( \Gamma_{B_L, f_{P^0,a}^0, f_{P^0,b}^0}^{L*} \Gamma_{B_L, f_{P^0,a}^0, f_{P^0,b}^0}^R \right) \right] \\
& + \sum_{b=1}^4 |\Gamma_{B_L, B_L, \phi_{L,b}^0}|^2 B_0 \left( p^2, m_{B_L}^2, m_{\phi_{L,b}^0}^2 \right) + \sum_{b=1}^4 |\Gamma_{B_L, B_H, \phi_{L,b}^0}|^2 B_0 \left( p^2, m_{B_H}^2, m_{\phi_{L,b}^0}^2 \right) \\
& + 2 \sum_{b=1}^4 |\Gamma_{B_L, W_L^1, \sigma_{L,b}^\pm}|^2 B_0 \left( p^2, m_{W_L^1}^2, m_{\sigma_{L,b}^\pm}^2 \right) + 2 \sum_{b=1}^4 |\Gamma_{B_L, W_H^1, \sigma_{L,b}^\pm}|^2 B_0 \left( p^2, m_{W_H^1}^2, m_{\sigma_{L,b}^\pm}^2 \right) \\
& + 2 \sum_{b=1}^4 |\Gamma_{B_L, W_L^2, \sigma_{L,b}^\pm}|^2 B_0 \left( p^2, m_{W_L^2}^2, m_{\sigma_{L,b}^\pm}^2 \right) + 2 \sum_{b=1}^4 |\Gamma_{B_L, W_H^2, \sigma_{L,b}^\pm}|^2 B_0 \left( p^2, m_{W_H^2}^2, m_{\sigma_{L,b}^\pm}^2 \right) \\
& + \sum_{b=1}^4 |\Gamma_{B_L, W_L^3, \phi_{L,b}^0}|^2 B_0 \left( p^2, m_{W_L^3}^2, m_{\phi_{L,b}^0}^2 \right) + \sum_{b=1}^4 |\Gamma_{B_L, W_H^3, \phi_{L,b}^0}|^2 B_0 \left( p^2, m_{W_H^3}^2, m_{\phi_{L,b}^0}^2 \right) \tag{374}
\end{aligned}$$

• **Self-Energy for Heavy B gauge boson ( $B_H$ )**

$$\begin{aligned}
\Pi(p^2) = & |\Gamma_{B_H, H_d^{0,*}, H_d^0}|^2 \left( -2A_0 \left( m_{H_d^0}^2 \right) - 4B_{22} \left( p^2, m_{H_d^0}^2, m_{H_d^0}^2 \right) \right) \\
& + |\Gamma_{B_H, H_d^{-,*}, H_d^-}|^2 \left( -2A_0 \left( m_{H_d^-}^2 \right) - 4B_{22} \left( p^2, m_{H_d^-}^2, m_{H_d^-}^2 \right) \right) \\
& + |\Gamma_{B_H, H_u^{0,*}, H_u^0}|^2 \left( -2A_0 \left( m_{H_u^0}^2 \right) - 4B_{22} \left( p^2, m_{H_u^0}^2, m_{H_u^0}^2 \right) \right) \\
& + |\Gamma_{B_H, H_u^{+,*}, H_u^+}|^2 \left( -2A_0 \left( m_{H_u^+}^2 \right) - 4B_{22} \left( p^2, m_{H_u^+}^2, m_{H_u^+}^2 \right) \right) + A_0 \left( m_{H_d^0}^2 \right) \Gamma_{B_H, B_H, H_d^{0,*}, H_d^0}
\end{aligned}$$

$$\begin{aligned}
& + A_0 \left( m_{H_d^-}^2 \right) \Gamma_{B_H, B_H, H_d^-, *, H_d^-} + A_0 \left( m_{H_u^0}^2 \right) \Gamma_{B_H, B_H, H_u^0, *, H_u^0} + A_0 \left( m_{H_u^+}^2 \right) \Gamma_{B_H, B_H, H_u^+, *, H_u^+} \\
& + \frac{1}{2} \left( 4B_0 \left( p^2, m_{\tilde{H}^0}^2, m_{\tilde{H}^0}^2 \right) m_{\tilde{H}^0} m_{\tilde{H}^0} \Re \left( \Gamma_{B_H, \text{FH0D}}^{L*} \left( \{1\} \right), \text{FH0D} \left( \{1\} \right) \Gamma_{B_H, \text{FH0D}}^R \left( \{1\} \right), \text{FH0D} \left( \{1\} \right) \right) + \left( \Gamma_{B_H, \text{FH0D}}^L \left( \{1\} \right), \text{FH0D} \left( \{1\} \right) \right) \right) \\
& + \frac{1}{2} \left( 4B_0 \left( p^2, m_{\tilde{H}^-}^2, m_{\tilde{H}^-}^2 \right) m_{\tilde{H}^-} m_{\tilde{H}^-} \Re \left( \Gamma_{B_H, \text{FHCD}}^{L*} \left( \{1\} \right), \text{FHCD} \left( \{1\} \right) \Gamma_{B_H, \text{FHCD}}^R \left( \{1\} \right), \text{FHCD} \left( \{1\} \right) \right) + \left( \Gamma_{B_H, \text{FHCD}}^L \left( \{1\} \right), \text{FHCD} \left( \{1\} \right) \right) \right) \\
& + 3 \sum_{a=1}^3 A_0 \left( m_{\tilde{d}_{L,a}}^2 \right) \Gamma_{B_H, B_H, \tilde{d}_{L,a}^*, \tilde{d}_{L,a}} + 3 \sum_{a=1}^3 A_0 \left( m_{\tilde{d}_{R,a}}^2 \right) \Gamma_{B_H, B_H, \tilde{d}_{R,a}^*, \tilde{d}_{R,a}} \\
& + \sum_{a=1}^3 A_0 \left( m_{\tilde{e}_{L,a}}^2 \right) \Gamma_{B_H, B_H, \tilde{e}_{L,a}^*, \tilde{e}_{L,a}} + \sum_{a=1}^3 A_0 \left( m_{\tilde{e}_{R,a}}^2 \right) \Gamma_{B_H, B_H, \tilde{e}_{R,a}^*, \tilde{e}_{R,a}} \\
& + 3 \sum_{a=1}^3 A_0 \left( m_{\tilde{u}_{L,a}}^2 \right) \Gamma_{B_H, B_H, \tilde{u}_{L,a}^*, \tilde{u}_{L,a}} + 3 \sum_{a=1}^3 A_0 \left( m_{\tilde{u}_{R,a}}^2 \right) \Gamma_{B_H, B_H, \tilde{u}_{R,a}^*, \tilde{u}_{R,a}} \\
& + \sum_{a=1}^3 A_0 \left( m_{\tilde{\nu}_{L,a}}^2 \right) \Gamma_{B_H, B_H, \tilde{\nu}_{L,a}^*, \tilde{\nu}_{L,a}} \\
& + 3 \sum_{a=1}^3 \sum_{b=1}^3 |\Gamma_{B_H, \tilde{d}_{L,a}^*, \tilde{d}_{L,b}}|^2 \left( -4B_{22} \left( p^2, m_{\tilde{d}_{L,a}}^2, m_{\tilde{d}_{L,b}}^2 \right) - A_0 \left( m_{\tilde{d}_{L,a}}^2 \right) - A_0 \left( m_{\tilde{d}_{L,b}}^2 \right) \right) \\
& + 3 \sum_{a=1}^3 \sum_{b=1}^3 |\Gamma_{B_H, \tilde{d}_{R,a}^*, \tilde{d}_{R,b}}|^2 \left( -4B_{22} \left( p^2, m_{\tilde{d}_{R,a}}^2, m_{\tilde{d}_{R,b}}^2 \right) - A_0 \left( m_{\tilde{d}_{R,a}}^2 \right) - A_0 \left( m_{\tilde{d}_{R,b}}^2 \right) \right) \\
& + \sum_{a=1}^3 \sum_{b=1}^3 |\Gamma_{B_H, \tilde{e}_{L,a}^*, \tilde{e}_{L,b}}|^2 \left( -4B_{22} \left( p^2, m_{\tilde{e}_{L,a}}^2, m_{\tilde{e}_{L,b}}^2 \right) - A_0 \left( m_{\tilde{e}_{L,a}}^2 \right) - A_0 \left( m_{\tilde{e}_{L,b}}^2 \right) \right) \\
& + \sum_{a=1}^3 \sum_{b=1}^3 |\Gamma_{B_H, \tilde{e}_{R,a}^*, \tilde{e}_{R,b}}|^2 \left( -4B_{22} \left( p^2, m_{\tilde{e}_{R,a}}^2, m_{\tilde{e}_{R,b}}^2 \right) - A_0 \left( m_{\tilde{e}_{R,a}}^2 \right) - A_0 \left( m_{\tilde{e}_{R,b}}^2 \right) \right) \\
& + 3 \sum_{a=1}^3 \sum_{b=1}^3 |\Gamma_{B_H, \tilde{u}_{L,a}^*, \tilde{u}_{L,b}}|^2 \left( -4B_{22} \left( p^2, m_{\tilde{u}_{L,a}}^2, m_{\tilde{u}_{L,b}}^2 \right) - A_0 \left( m_{\tilde{u}_{L,a}}^2 \right) - A_0 \left( m_{\tilde{u}_{L,b}}^2 \right) \right) \\
& + 3 \sum_{a=1}^3 \sum_{b=1}^3 |\Gamma_{B_H, \tilde{u}_{R,a}^*, \tilde{u}_{R,b}}|^2 \left( -4B_{22} \left( p^2, m_{\tilde{u}_{R,a}}^2, m_{\tilde{u}_{R,b}}^2 \right) - A_0 \left( m_{\tilde{u}_{R,a}}^2 \right) - A_0 \left( m_{\tilde{u}_{R,b}}^2 \right) \right) \\
& + \sum_{a=1}^3 \sum_{b=1}^3 |\Gamma_{B_H, \tilde{\nu}_{L,a}^*, \tilde{\nu}_{L,b}}|^2 \left( -4B_{22} \left( p^2, m_{\tilde{\nu}_{L,a}}^2, m_{\tilde{\nu}_{L,b}}^2 \right) - A_0 \left( m_{\tilde{\nu}_{L,a}}^2 \right) - A_0 \left( m_{\tilde{\nu}_{L,b}}^2 \right) \right) \\
& + \frac{3}{2} \sum_{a=1}^3 \sum_{b=1}^3 \left[ \left( |\Gamma_{B_H, \bar{d}^{D_L}, a, d_{L,b}^D}|^2 + |\Gamma_{B_H, \bar{d}^{D_L}, a, d_{L,b}^D}|^2 \right) H_0 \left( p^2, m_{d_{L,a}^D}^2, m_{d_{L,b}^D}^2 \right) \right. \\
& \left. + 4B_0 \left( p^2, m_{d_{L,a}^D}^2, m_{d_{L,b}^D}^2 \right) m_{\bar{d}^{D_L}, a} m_{d_{L,b}^D} \Re \left( \Gamma_{B_H, \bar{d}^{D_L}, a, d_{L,b}^D}^{L*} \Gamma_{B_H, \bar{d}^{D_L}, a, d_{L,b}^D}^R \right) \right]
\end{aligned}$$

$$\begin{aligned}
& + \frac{3}{2} \sum_{a=1}^3 \sum_{b=1}^3 \left[ \left( |\Gamma_{B_H, \bar{d}^{D_R, a}, d_{R, b}^D}|^2 + |\Gamma_{B_H, \bar{d}^{D_R, a}, d_{R, b}^D}|^2 \right) H_0 \left( p^2, m_{d_{R, a}^D}^2, m_{d_{R, b}^D}^2 \right) \right. \\
& + 4B_0 \left( p^2, m_{d_{R, a}^D}^2, m_{d_{R, b}^D}^2 \right) m_{\bar{d}^{D_R, a}} m_{d_{R, b}^D} \Re \left( \Gamma_{B_H, \bar{d}^{D_R, a}, d_{R, b}^D}^{L*} \Gamma_{B_H, \bar{d}^{D_R, a}, d_{R, b}^D}^R \right) \Big] \\
& + \frac{1}{2} \sum_{a=1}^3 \sum_{b=1}^3 \left[ \left( |\Gamma_{B_H, \bar{e}^{D_L, a}, e_{L, b}^D}|^2 + |\Gamma_{B_H, \bar{e}^{D_L, a}, e_{L, b}^D}|^2 \right) H_0 \left( p^2, m_{e_{L, a}^D}^2, m_{e_{L, b}^D}^2 \right) \right. \\
& + 4B_0 \left( p^2, m_{e_{L, a}^D}^2, m_{e_{L, b}^D}^2 \right) m_{\bar{e}^{D_L, a}} m_{e_{L, b}^D} \Re \left( \Gamma_{B_H, \bar{e}^{D_L, a}, e_{L, b}^D}^{L*} \Gamma_{B_H, \bar{e}^{D_L, a}, e_{L, b}^D}^R \right) \Big] \\
& + \frac{1}{2} \sum_{a=1}^3 \sum_{b=1}^3 \left[ \left( |\Gamma_{B_H, \bar{e}^{D_R, a}, e_{R, b}^D}|^2 + |\Gamma_{B_H, \bar{e}^{D_R, a}, e_{R, b}^D}|^2 \right) H_0 \left( p^2, m_{e_{R, a}^D}^2, m_{e_{R, b}^D}^2 \right) \right. \\
& + 4B_0 \left( p^2, m_{e_{R, a}^D}^2, m_{e_{R, b}^D}^2 \right) m_{\bar{e}^{D_R, a}} m_{e_{R, b}^D} \Re \left( \Gamma_{B_H, \bar{e}^{D_R, a}, e_{R, b}^D}^{L*} \Gamma_{B_H, \bar{e}^{D_R, a}, e_{R, b}^D}^R \right) \Big] \\
& + \frac{3}{2} \sum_{a=1}^3 \sum_{b=1}^3 \left[ \left( |\Gamma_{B_H, \bar{u}^{D_L, a}, u_{L, b}^D}|^2 + |\Gamma_{B_H, \bar{u}^{D_L, a}, u_{L, b}^D}|^2 \right) H_0 \left( p^2, m_{u_{L, a}^D}^2, m_{u_{L, b}^D}^2 \right) \right. \\
& + 4B_0 \left( p^2, m_{u_{L, a}^D}^2, m_{u_{L, b}^D}^2 \right) m_{\bar{u}^{D_L, a}} m_{u_{L, b}^D} \Re \left( \Gamma_{B_H, \bar{u}^{D_L, a}, u_{L, b}^D}^{L*} \Gamma_{B_H, \bar{u}^{D_L, a}, u_{L, b}^D}^R \right) \Big] \\
& + \frac{3}{2} \sum_{a=1}^3 \sum_{b=1}^3 \left[ \left( |\Gamma_{B_H, \bar{u}^{D_R, a}, u_{R, b}^D}|^2 + |\Gamma_{B_H, \bar{u}^{D_R, a}, u_{R, b}^D}|^2 \right) H_0 \left( p^2, m_{u_{R, a}^D}^2, m_{u_{R, b}^D}^2 \right) \right. \\
& + 4B_0 \left( p^2, m_{u_{R, a}^D}^2, m_{u_{R, b}^D}^2 \right) m_{\bar{u}^{D_R, a}} m_{u_{R, b}^D} \Re \left( \Gamma_{B_H, \bar{u}^{D_R, a}, u_{R, b}^D}^{L*} \Gamma_{B_H, \bar{u}^{D_R, a}, u_{R, b}^D}^R \right) \Big] \\
& + \frac{1}{2} \sum_{a=1}^3 \sum_{b=1}^3 \left[ \left( |\Gamma_{B_H, \bar{\nu}^{D_L, a}, \nu_{L, b}^D}|^2 + |\Gamma_{B_H, \bar{\nu}^{D_L, a}, \nu_{L, b}^D}|^2 \right) H_0 \left( p^2, m_{\nu_{L, a}^D}^2, m_{\nu_{L, b}^D}^2 \right) \right. \\
& + 4B_0 \left( p^2, m_{\nu_{L, a}^D}^2, m_{\nu_{L, b}^D}^2 \right) m_{\bar{\nu}^{D_L, a}} m_{\nu_{L, b}^D} \Re \left( \Gamma_{B_H, \bar{\nu}^{D_L, a}, \nu_{L, b}^D}^{L*} \Gamma_{B_H, \bar{\nu}^{D_L, a}, \nu_{L, b}^D}^R \right) \Big] \\
& + \sum_{a=1}^4 A_0 \left( m_{\sigma_{L, a}^\pm}^2 \right) \Gamma_{B_H, B_H, \sigma_{L, a}^\pm, *} \sigma_{L, a}^\pm + \frac{1}{2} \sum_{a=1}^4 A_0 \left( m_{\phi_{L, a}^0}^2 \right) \Gamma_{B_H, B_H, \phi_{L, a}^0, \phi_{L, a}^0} \\
& + \frac{1}{2} \sum_{a=1}^4 A_0 \left( m_{\sigma_{L, a}^0}^2 \right) \Gamma_{B_H, B_H, \sigma_{L, a}^0, \sigma_{L, a}^0} \\
& + \sum_{a=1}^4 \sum_{b=1}^4 |\Gamma_{B_H, \sigma_{L, a}^\pm, *} \sigma_{L, b}^\pm|^2 \left( -4B_{22} \left( p^2, m_{\sigma_{L, a}^\pm}^2, m_{\sigma_{L, b}^\pm}^2 \right) - A_0 \left( m_{\sigma_{L, a}^\pm}^2 \right) - A_0 \left( m_{\sigma_{L, b}^\pm}^2 \right) \right) \\
& + \sum_{a=1}^4 \sum_{b=1}^4 |\Gamma_{B_H, \sigma_{L, a}^0, \phi_{L, b}^0}|^2 \left( -4B_{22} \left( p^2, m_{\phi_{L, a}^0}^2, m_{\sigma_{L, b}^0}^2 \right) - A_0 \left( m_{\phi_{L, a}^0}^2 \right) - A_0 \left( m_{\sigma_{L, b}^0}^2 \right) \right) \\
& + \frac{1}{4} \sum_{a=1}^{10} \sum_{b=1}^{10} \left[ \left( |\Gamma_{B_H, f_{G^0, a}^-, f_{G^0, b}^-}|^2 + |\Gamma_{B_H, f_{G^0, a}^-, f_{G^0, b}^-}|^2 \right) H_0 \left( p^2, m_{f_{G^0, a}^-}^2, m_{f_{G^0, b}^-}^2 \right) \right. \\
& + 4B_0 \left( p^2, m_{f_{G^0, a}^-}^2, m_{f_{G^0, b}^-}^2 \right) m_{f_{G^0, a}^-} m_{f_{G^0, b}^-} \Re \left( \Gamma_{B_H, f_{G^0, a}^-, f_{G^0, b}^-}^{L*} \Gamma_{B_H, f_{G^0, a}^-, f_{G^0, b}^-}^R \right) \Big]
\end{aligned}$$

$$\begin{aligned}
& + \frac{1}{4} \sum_{a=1}^{10} \sum_{b=1}^{10} \left[ \left( |\Gamma_{BH, f_{Po,a}^0, f_{Po,b}^0}^L|^2 + |\Gamma_{BH, f_{Po,a}^0, f_{Po,b}^0}^R|^2 \right) H_0 \left( p^2, m_{f_{Po,a}^0}^2, m_{f_{Po,b}^0}^2 \right) \right. \\
& + 4B_0 \left( p^2, m_{f_{Po,a}^0}^2, m_{f_{Po,b}^0}^2 \right) m_{f_{Po,a}^0} m_{f_{Po,b}^0} \Re \left( \Gamma_{BH, f_{Po,a}^0, f_{Po,b}^0}^{L*} \Gamma_{BH, f_{Po,a}^0, f_{Po,b}^0}^R \right) \left. \right] \\
& + \sum_{b=1}^4 |\Gamma_{BH, BL, \phi_{L,b}^0}|^2 B_0 \left( p^2, m_{BL}^2, m_{\phi_{L,b}^0}^2 \right) + \sum_{b=1}^4 |\Gamma_{BH, BH, \phi_{L,b}^0}|^2 B_0 \left( p^2, m_{BH}^2, m_{\phi_{L,b}^0}^2 \right) \\
& + 2 \sum_{b=1}^4 |\Gamma_{BH, WL, \sigma_{L,b}^\pm}|^2 B_0 \left( p^2, m_{WL}^2, m_{\sigma_{L,b}^\pm}^2 \right) + 2 \sum_{b=1}^4 |\Gamma_{BH, WH, \sigma_{L,b}^\pm}|^2 B_0 \left( p^2, m_{WH}^2, m_{\sigma_{L,b}^\pm}^2 \right) \\
& + 2 \sum_{b=1}^4 |\Gamma_{BH, WL, \sigma_{L,b}^\pm}|^2 B_0 \left( p^2, m_{WL}^2, m_{\sigma_{L,b}^\pm}^2 \right) + 2 \sum_{b=1}^4 |\Gamma_{BH, WH, \sigma_{L,b}^\pm}|^2 B_0 \left( p^2, m_{WH}^2, m_{\sigma_{L,b}^\pm}^2 \right) \\
& + \sum_{b=1}^4 |\Gamma_{BH, WL, \phi_{L,b}^0}|^2 B_0 \left( p^2, m_{WL}^2, m_{\phi_{L,b}^0}^2 \right) + \sum_{b=1}^4 |\Gamma_{BH, WH, \phi_{L,b}^0}|^2 B_0 \left( p^2, m_{WH}^2, m_{\phi_{L,b}^0}^2 \right) \tag{375}
\end{aligned}$$

• Self-Energy for Light W1 gauge boson ( $W_L^1$ )

$$\begin{aligned}
\Pi(p^2) = & + 2|\Gamma_{W_L^1, \eta \bar{W}_L^3, \eta W_L^2}|^2 B_{00} \left( p^2, m_{\eta W_L^2}^2, m_{\eta W_L^3}^2 \right) + 2|\Gamma_{W_L^1, \eta \bar{W}_H^3, \eta W_L^2}|^2 B_{00} \left( p^2, m_{\eta W_L^2}^2, m_{\eta W_H^3}^2 \right) \\
& + 2|\Gamma_{W_L^1, \eta \bar{W}_L^3, \eta W_H^2}|^2 B_{00} \left( p^2, m_{\eta W_H^2}^2, m_{\eta W_L^3}^2 \right) + 2|\Gamma_{W_L^1, \eta \bar{W}_H^3, \eta W_H^2}|^2 B_{00} \left( p^2, m_{\eta W_H^2}^2, m_{\eta W_H^3}^2 \right) \\
& + 2|\Gamma_{W_L^1, H_d^{0,*}, H_d^0}|^2 \left( -4B_{22} \left( p^2, m_{H_d^0}^2, m_{H_d^-}^2 \right) - A_0 \left( m_{H_d^-}^2 \right) - A_0 \left( m_{H_d^0}^2 \right) \right) \\
& + 2|\Gamma_{W_L^1, H_u^{0,*}, H_u^0}|^2 \left( -4B_{22} \left( p^2, m_{H_u^0}^2, m_{H_u^+}^2 \right) - A_0 \left( m_{H_u^+}^2 \right) - A_0 \left( m_{H_u^0}^2 \right) \right) \\
& + A_0 \left( m_{H_d^0}^2 \right) \Gamma_{W_L^1, W_L^1, H_d^{0,*}, H_d^0} + A_0 \left( m_{H_d^-}^2 \right) \Gamma_{W_L^1, W_L^1, H_d^{0,*}, H_d^-} + A_0 \left( m_{H_u^0}^2 \right) \Gamma_{W_L^1, W_L^1, H_u^{0,*}, H_u^0} \\
& + A_0 \left( m_{H_u^+}^2 \right) \Gamma_{W_L^1, W_L^1, H_u^{0,*}, H_u^+} + \left( |\Gamma_{W_L^1, \text{FHCD}^-(\{1\}), \text{FH0D}(\{1\})}^L|^2 + |\Gamma_{W_L^1, \text{FHCD}^-(\{1\}), \text{FH0D}(\{1\})}^R|^2 \right) H_0 \left( p^2, m_{H^-}^2, m_{H^0}^2 \right) \\
& - |\Gamma_{W_L^1, W_L^3, W_L^2}|^2 \left( 10B_{00} \left( p^2, m_{W_L^3}^2, m_{W_L^2}^2 \right) + B_0 \left( p^2, m_{W_L^3}^2, m_{W_L^2}^2 \right) \left( 4p^2 + m_{W_L^2}^2 + m_{W_L^3}^2 \right) + A_0 \left( m_{W_L^2}^2 \right) + A_0 \left( m_{W_L^3}^2 \right) \right) \\
& - |\Gamma_{W_L^1, W_L^3, W_H^2}|^2 \left( 10B_{00} \left( p^2, m_{W_L^3}^2, m_{W_H^2}^2 \right) + B_0 \left( p^2, m_{W_L^3}^2, m_{W_H^2}^2 \right) \left( 4p^2 + m_{W_H^2}^2 + m_{W_L^3}^2 \right) + A_0 \left( m_{W_H^2}^2 \right) + A_0 \left( m_{W_L^3}^2 \right) \right) \\
& - |\Gamma_{W_L^1, W_H^3, W_L^2}|^2 \left( 10B_{00} \left( p^2, m_{W_H^3}^2, m_{W_L^2}^2 \right) + B_0 \left( p^2, m_{W_H^3}^2, m_{W_L^2}^2 \right) \left( 4p^2 + m_{W_L^2}^2 + m_{W_H^3}^2 \right) + A_0 \left( m_{W_L^2}^2 \right) + A_0 \left( m_{W_H^3}^2 \right) \right) \\
& - |\Gamma_{W_L^1, W_H^3, W_H^2}|^2 \left( 10B_{00} \left( p^2, m_{W_H^3}^2, m_{W_H^2}^2 \right) + B_0 \left( p^2, m_{W_H^3}^2, m_{W_H^2}^2 \right) \left( 4p^2 + m_{W_H^2}^2 + m_{W_H^3}^2 \right) + A_0 \left( m_{W_H^2}^2 \right) + A_0 \left( m_{W_H^3}^2 \right) \right) \\
& + 4B_0 \left( p^2, m_{H^-}^2, m_{H^0}^2 \right) m_{H^0} m_{H^-} \Re \left( \Gamma_{W_L^1, \text{FHCD}^-(\{1\}), \text{FH0D}(\{1\})}^{L*} \Gamma_{W_L^1, \text{FHCD}^-(\{1\}), \text{FH0D}(\{1\})}^R \right) + \sum_{a=1}^2 A_0 \left( m_{\phi_{B,a}^s}^2 \right) \Gamma_{W_L^1, W_L^1, \phi_{B,a}^s} \\
& + \sum_{a=1}^2 A_0 \left( m_{\phi_{AK,a}^s}^2 \right) \Gamma_{W_L^1, W_L^1, \phi_{AK,a}^{s,*}, \phi_{AK,a}^s}
\end{aligned}$$

$$\begin{aligned}
& + 2 \sum_{a=1}^2 \sum_{b=1}^2 |\Gamma_{W_L^1, \phi_{AK,a}^{s,*}, \phi_{B,b}^s}|^2 \left( -4B_{22} \left( p^2, m_{\phi_{B,a}^s}^2, m_{\phi_{AK,b}^s}^2 \right) - A_0 \left( m_{\phi_{AK,b}^s}^2 \right) - A_0 \left( m_{\phi_{B,a}^s}^2 \right) \right) \\
& + 2 \sum_{a=1}^2 \sum_{b=1}^2 |\Gamma_{W_L^1, \phi_{AK,a}^s, \phi_{B,b}^s}|^2 \left( -4B_{22} \left( p^2, m_{\phi_{B,a}^s}^2, m_{\phi_{AK,b}^s}^2 \right) - A_0 \left( m_{\phi_{AK,b}^s}^2 \right) - A_0 \left( m_{\phi_{B,a}^s}^2 \right) \right) \\
& + 3 \sum_{a=1}^3 A_0 \left( m_{\tilde{d}_{L,a}}^2 \right) \Gamma_{W_L^1, W_L^1, \tilde{d}_{L,a}^*, \tilde{d}_{L,a}} + \sum_{a=1}^3 A_0 \left( m_{\tilde{e}_{L,a}}^2 \right) \Gamma_{W_L^1, W_L^1, \tilde{e}_{L,a}^*, \tilde{e}_{L,a}} \\
& + 3 \sum_{a=1}^3 A_0 \left( m_{\tilde{u}_{L,a}}^2 \right) \Gamma_{W_L^1, W_L^1, \tilde{u}_{L,a}^*, \tilde{u}_{L,a}} + \sum_{a=1}^3 A_0 \left( m_{\tilde{\nu}_{L,a}}^2 \right) \Gamma_{W_L^1, W_L^1, \tilde{\nu}_{L,a}^*, \tilde{\nu}_{L,a}} \\
& + 6 \sum_{a=1}^3 \sum_{b=1}^3 |\Gamma_{W_L^1, \tilde{u}_{L,a}^*, \tilde{d}_{L,b}}|^2 \left( -4B_{22} \left( p^2, m_{\tilde{d}_{L,a}}^2, m_{\tilde{u}_{L,b}}^2 \right) - A_0 \left( m_{\tilde{d}_{L,a}}^2 \right) - A_0 \left( m_{\tilde{u}_{L,b}}^2 \right) \right) \\
& + 2 \sum_{a=1}^3 \sum_{b=1}^3 |\Gamma_{W_L^1, \tilde{\nu}_{L,a}^*, \tilde{e}_{L,b}}|^2 \left( -4B_{22} \left( p^2, m_{\tilde{e}_{L,a}}^2, m_{\tilde{\nu}_{L,b}}^2 \right) - A_0 \left( m_{\tilde{e}_{L,a}}^2 \right) - A_0 \left( m_{\tilde{\nu}_{L,b}}^2 \right) \right) \\
& + 3 \sum_{a=1}^3 \sum_{b=1}^3 \left[ \left( |\Gamma_{W_L^1, \bar{u}^{D_L,a}, d_{L,b}^D}|^2 + |\Gamma_{W_L^1, \bar{u}^{D_L,a}, d_{L,b}^D}|^2 \right) H_0 \left( p^2, m_{u_{L,a}^D}^2, m_{d_{L,b}^D}^2 \right) \right. \\
& \quad \left. + 4B_0 \left( p^2, m_{u_{L,a}^D}^2, m_{d_{L,b}^D}^2 \right) m_{\bar{u}^{D_L,a}} m_{d_{L,b}^D} \Re \left( \Gamma_{W_L^1, \bar{u}^{D_L,a}, d_{L,b}^D}^{L*} \Gamma_{W_L^1, \bar{u}^{D_L,a}, d_{L,b}^D}^R \right) \right] \\
& + \sum_{a=1}^3 \sum_{b=1}^3 \left[ \left( |\Gamma_{W_L^1, \bar{\nu}^{D_L,a}, e_{L,b}^D}|^2 + |\Gamma_{W_L^1, \bar{\nu}^{D_L,a}, e_{L,b}^D}|^2 \right) H_0 \left( p^2, m_{\nu_{L,a}^D}^2, m_{e_{L,b}^D}^2 \right) \right. \\
& \quad \left. + 4B_0 \left( p^2, m_{\nu_{L,a}^D}^2, m_{e_{L,b}^D}^2 \right) m_{\bar{\nu}^{D_L,a}} m_{e_{L,b}^D} \Re \left( \Gamma_{W_L^1, \bar{\nu}^{D_L,a}, e_{L,b}^D}^{L*} \Gamma_{W_L^1, \bar{\nu}^{D_L,a}, e_{L,b}^D}^R \right) \right] \\
& + \sum_{a=1}^4 A_0 \left( m_{\sigma_{L,a}^\pm}^2 \right) \Gamma_{W_L^1, W_L^1, \sigma_{L,a}^{\pm,*}, \sigma_{L,a}^\pm} + \frac{1}{2} \sum_{a=1}^4 A_0 \left( m_{\phi_{L,a}^0}^2 \right) \Gamma_{W_L^1, W_L^1, \phi_{L,a}^0, \phi_{L,a}^0} \\
& + \frac{1}{2} \sum_{a=1}^4 A_0 \left( m_{\sigma_{L,a}^0}^2 \right) \Gamma_{W_L^1, W_L^1, \sigma_{L,a}^0, \sigma_{L,a}^0} \\
& + 2 \sum_{a=1}^4 \sum_{b=1}^4 |\Gamma_{W_L^1, \phi_{L,a}^0, \sigma_{L,b}^\pm}|^2 \left( -4B_{22} \left( p^2, m_{\sigma_{L,a}^\pm}^2, m_{\phi_{L,b}^0}^2 \right) - A_0 \left( m_{\phi_{L,b}^0}^2 \right) - A_0 \left( m_{\sigma_{L,a}^\pm}^2 \right) \right) \\
& + 2 \sum_{a=1}^4 \sum_{b=1}^4 |\Gamma_{W_L^1, \sigma_{L,a}^0, \sigma_{L,b}^\pm}|^2 \left( -4B_{22} \left( p^2, m_{\sigma_{L,a}^\pm}^2, m_{\sigma_{L,b}^0}^2 \right) - A_0 \left( m_{\sigma_{L,b}^0}^2 \right) - A_0 \left( m_{\sigma_{L,a}^\pm}^2 \right) \right) \\
& + \frac{1}{2} \sum_{a=1}^{10} \sum_{b=1}^{10} \left[ \left( |\Gamma_{W_L^1, f_{Po,a}^0, f_{Go,b}^-}|^2 + |\Gamma_{W_L^1, f_{Po,a}^0, f_{Go,b}^-}|^2 \right) H_0 \left( p^2, m_{f_{Po,a}^0}^2, m_{f_{Go,b}^-}^2 \right) \right. \\
& \quad \left. + 4B_0 \left( p^2, m_{f_{Po,a}^0}^2, m_{f_{Go,b}^-}^2 \right) m_{f_{Go,b}^-} m_{f_{Po,a}^0} \Re \left( \Gamma_{W_L^1, f_{Po,a}^0, f_{Go,b}^-}^{L*} \Gamma_{W_L^1, f_{Po,a}^0, f_{Go,b}^-}^R \right) \right] \\
& + 2 \sum_{b=1}^4 |\Gamma_{W_L^1, B_L, \sigma_{L,b}^\pm}|^2 B_0 \left( p^2, m_{B_L}^2, m_{\sigma_{L,b}^\pm}^2 \right) + 2 \sum_{b=1}^4 |\Gamma_{W_L^1, B_H, \sigma_{L,b}^\pm}|^2 B_0 \left( p^2, m_{B_H}^2, m_{\sigma_{L,b}^\pm}^2 \right)
\end{aligned}$$

$$\begin{aligned}
& + \sum_{b=1}^4 |\Gamma_{W_L^1, W_L^1, \phi_{L,b}^0}|^2 B_0(p^2, m_{W_L^1}^2, m_{\phi_{L,b}^0}^2) + \sum_{b=1}^4 |\Gamma_{W_L^1, W_H^1, \phi_{L,b}^0}|^2 B_0(p^2, m_{W_H^1}^2, m_{\phi_{L,b}^0}^2) \\
& + \sum_{b=1}^4 |\Gamma_{W_L^1, W_H^2, \sigma_{L,b}^0}|^2 B_0(p^2, m_{W_H^2}^2, m_{\sigma_{L,b}^0}^2) + 2 \sum_{b=1}^4 |\Gamma_{W_L^1, W_H^3, \sigma_{L,b}^\pm}|^2 B_0(p^2, m_{W_H^3}^2, m_{\sigma_{L,b}^\pm}^2) \\
& - \frac{1}{2} A_0(m_{W_L^2}^2) \left( 4\Gamma_{W_L^1, W_L^1, W_L^2, W_L^2}^1 + \Gamma_{W_L^1, W_L^1, W_L^2, W_L^2}^2 + \Gamma_{W_L^1, W_L^1, W_L^2, W_L^2}^3 \right) - \frac{1}{2} A_0(m_{W_H^2}^2) \left( 4\Gamma_{W_L^1, W_L^1, W_H^2, W_H^2}^1 + \Gamma_{W_L^1, W_L^1, W_H^2, W_H^2}^2 \right) \\
& \hspace{15em} (376)
\end{aligned}$$

• Self-Energy for Heavy W1 gauge boson ( $W_H^1$ )

$$\begin{aligned}
\Pi(p^2) = & 2|\Gamma_{W_H^1, \eta \bar{W}_L^3, \eta W_L^2}|^2 B_{00}(p^2, m_{\eta W_L^2}^2, m_{\eta W_L^3}^2) + 2|\Gamma_{W_H^1, \eta \bar{W}_H^3, \eta W_L^2}|^2 B_{00}(p^2, m_{\eta W_L^2}^2, m_{\eta W_H^3}^2) \\
& + 2|\Gamma_{W_H^1, \eta \bar{W}_L^3, \eta W_H^2}|^2 B_{00}(p^2, m_{\eta W_H^2}^2, m_{\eta W_L^3}^2) + 2|\Gamma_{W_H^1, \eta \bar{W}_H^3, \eta W_H^2}|^2 B_{00}(p^2, m_{\eta W_H^2}^2, m_{\eta W_H^3}^2) \\
& + 2|\Gamma_{W_H^1, H_d^{0,*}, H_d^0}|^2 \left( -4B_{22}(p^2, m_{H_d^0}^2, m_{H_d^-}^2) - A_0(m_{H_d^-}^2) - A_0(m_{H_d^0}^2) \right) \\
& + 2|\Gamma_{W_H^1, H_u^{0,*}, H_u^0}|^2 \left( -4B_{22}(p^2, m_{H_u^0}^2, m_{H_u^+}^2) - A_0(m_{H_u^+}^2) - A_0(m_{H_u^0}^2) \right) \\
& + A_0(m_{H_d^0}^2) \Gamma_{W_H^1, W_H^1, H_d^{0,*}, H_d^0} + A_0(m_{H_d^-}^2) \Gamma_{W_H^1, W_H^1, H_d^{0,*}, H_d^-} + A_0(m_{H_u^0}^2) \Gamma_{W_H^1, W_H^1, H_u^{0,*}, H_u^0} \\
& + A_0(m_{H_u^+}^2) \Gamma_{W_H^1, W_H^1, H_u^{0,*}, H_u^+} + \left( |\Gamma_{W_H^1, \text{FHCD}(\{1\}), \text{FH0D}(\{1\})}^L|^2 + |\Gamma_{W_H^1, \text{FHCD}(\{1\}), \text{FH0D}(\{1\})}^R|^2 \right) H_0(p^2, m_{\bar{H}^-}^2, m_{\bar{H}^0}^2) \\
& - |\Gamma_{W_H^1, W_L^3, W_L^2}|^2 \left( 10B_{00}(p^2, m_{W_L^3}^2, m_{W_L^2}^2) + B_0(p^2, m_{W_L^3}^2, m_{W_L^2}^2) (4p^2 + m_{W_L^2}^2 + m_{W_L^3}^2) + A_0(m_{W_L^2}^2) + A_0(m_{W_L^3}^2) \right) \\
& - |\Gamma_{W_H^1, W_L^3, W_H^2}|^2 \left( 10B_{00}(p^2, m_{W_L^3}^2, m_{W_H^2}^2) + B_0(p^2, m_{W_L^3}^2, m_{W_H^2}^2) (4p^2 + m_{W_H^2}^2 + m_{W_L^3}^2) + A_0(m_{W_H^2}^2) + A_0(m_{W_L^3}^2) \right) \\
& - |\Gamma_{W_H^1, W_H^3, W_L^2}|^2 \left( 10B_{00}(p^2, m_{W_H^3}^2, m_{W_L^2}^2) + B_0(p^2, m_{W_H^3}^2, m_{W_L^2}^2) (4p^2 + m_{W_L^2}^2 + m_{W_H^3}^2) + A_0(m_{W_L^2}^2) + A_0(m_{W_H^3}^2) \right) \\
& - |\Gamma_{W_H^1, W_H^3, W_H^2}|^2 \left( 10B_{00}(p^2, m_{W_H^3}^2, m_{W_H^2}^2) + B_0(p^2, m_{W_H^3}^2, m_{W_H^2}^2) (4p^2 + m_{W_H^2}^2 + m_{W_H^3}^2) + A_0(m_{W_H^2}^2) + A_0(m_{W_H^3}^2) \right) \\
& + 4B_0(p^2, m_{\bar{H}^-}^2, m_{\bar{H}^0}^2) m_{\bar{H}^0} m_{\bar{H}^-} \Re \left( \Gamma_{W_H^1, \text{FHCD}(\{1\}), \text{FH0D}(\{1\})}^{L*} \Gamma_{W_H^1, \text{FHCD}(\{1\}), \text{FH0D}(\{1\})}^R \right) + \sum_{a=1}^2 A_0(m_{\phi_{B,a}^s}^2) \Gamma_{W_H^1, W_H^1, \phi_{AK,a}^s} \\
& + \sum_{a=1}^2 A_0(m_{\phi_{AK,a}^s}^2) \Gamma_{W_H^1, W_H^1, \phi_{AK,a}^{s,*}, \phi_{AK,a}^s} \\
& + 2 \sum_{a=1}^2 \sum_{b=1}^2 |\Gamma_{W_H^1, \phi_{AK,a}^{s,*}, \phi_{B,b}^s}|^2 \left( -4B_{22}(p^2, m_{\phi_{B,a}^s}^2, m_{\phi_{AK,b}^s}^2) - A_0(m_{\phi_{AK,b}^s}^2) - A_0(m_{\phi_{B,a}^s}^2) \right) \\
& + 2 \sum_{a=1}^2 \sum_{b=1}^2 |\Gamma_{W_H^1, \phi_{AK,a}^s, \phi_{B,b}^{s,*}}|^2 \left( -4B_{22}(p^2, m_{\phi_{B,a}^s}^2, m_{\phi_{AK,b}^s}^2) - A_0(m_{\phi_{AK,b}^s}^2) - A_0(m_{\phi_{B,a}^s}^2) \right) \\
& + 3 \sum_{a=1}^3 A_0(m_{\tilde{d}_{L,a}^2}^2) \Gamma_{W_H^1, W_H^1, \tilde{d}_{L,a}^*, \tilde{d}_{L,a}} + \sum_{a=1}^3 A_0(m_{\tilde{e}_{L,a}^2}^2) \Gamma_{W_H^1, W_H^1, \tilde{e}_{L,a}^*, \tilde{e}_{L,a}}
\end{aligned}$$



$$\begin{aligned}
& + 3 \sum_{a=1}^3 A_0 \left( m_{\tilde{u}_{L,a}}^2 \right) \Gamma_{W_H^1, W_H^1, \tilde{u}_{L,a}^*, \tilde{u}_{L,a}} + \sum_{a=1}^3 A_0 \left( m_{\tilde{\nu}_{L,a}}^2 \right) \Gamma_{W_H^1, W_H^1, \tilde{\nu}_{L,a}^*, \tilde{\nu}_{L,a}} \\
& + 6 \sum_{a=1}^3 \sum_{b=1}^3 |\Gamma_{W_H^1, \tilde{u}_{L,a}^*, \tilde{d}_{L,b}}|^2 \left( -4B_{22} \left( p^2, m_{\tilde{d}_{L,a}}^2, m_{\tilde{u}_{L,b}}^2 \right) - A_0 \left( m_{\tilde{d}_{L,a}}^2 \right) - A_0 \left( m_{\tilde{u}_{L,b}}^2 \right) \right) \\
& + 2 \sum_{a=1}^3 \sum_{b=1}^3 |\Gamma_{W_H^1, \tilde{\nu}_{L,a}^*, \tilde{e}_{L,b}}|^2 \left( -4B_{22} \left( p^2, m_{\tilde{e}_{L,a}}^2, m_{\tilde{\nu}_{L,b}}^2 \right) - A_0 \left( m_{\tilde{e}_{L,a}}^2 \right) - A_0 \left( m_{\tilde{\nu}_{L,b}}^2 \right) \right) \\
& + 3 \sum_{a=1}^3 \sum_{b=1}^3 \left[ \left( |\Gamma_{W_H^1, \tilde{u}^{D_{L,a}}, d_{L,b}^D}|^2 + |\Gamma_{W_H^1, \tilde{u}^{D_{L,a}}, d_{L,b}^D}|^2 \right) H_0 \left( p^2, m_{u_{L,a}^D}^2, m_{d_{L,b}^D}^2 \right) \right. \\
& \left. + 4B_0 \left( p^2, m_{u_{L,a}^D}^2, m_{d_{L,b}^D}^2 \right) m_{\tilde{u}^{D_{L,a}}} m_{d_{L,b}^D} \Re \left( \Gamma_{W_H^1, \tilde{u}^{D_{L,a}}, d_{L,b}^D}^{L*} \Gamma_{W_H^1, \tilde{u}^{D_{L,a}}, d_{L,b}^D}^R \right) \right] \\
& + \sum_{a=1}^3 \sum_{b=1}^3 \left[ \left( |\Gamma_{W_H^1, \tilde{\nu}^{D_{L,a}}, e_{L,b}^D}|^2 + |\Gamma_{W_H^1, \tilde{\nu}^{D_{L,a}}, e_{L,b}^D}|^2 \right) H_0 \left( p^2, m_{\nu_{L,a}^D}^2, m_{e_{L,b}^D}^2 \right) \right. \\
& \left. + 4B_0 \left( p^2, m_{\nu_{L,a}^D}^2, m_{e_{L,b}^D}^2 \right) m_{\tilde{\nu}^{D_{L,a}}} m_{e_{L,b}^D} \Re \left( \Gamma_{W_H^1, \tilde{\nu}^{D_{L,a}}, e_{L,b}^D}^{L*} \Gamma_{W_H^1, \tilde{\nu}^{D_{L,a}}, e_{L,b}^D}^R \right) \right] \\
& + \sum_{a=1}^4 A_0 \left( m_{\sigma_{L,a}^\pm}^2 \right) \Gamma_{W_H^1, W_H^1, \sigma_{L,a}^\pm, \sigma_{L,a}^\pm} + \frac{1}{2} \sum_{a=1}^4 A_0 \left( m_{\phi_{L,a}^0}^2 \right) \Gamma_{W_H^1, W_H^1, \phi_{L,a}^0, \phi_{L,a}^0} \\
& + \frac{1}{2} \sum_{a=1}^4 A_0 \left( m_{\sigma_{L,a}^0}^2 \right) \Gamma_{W_H^1, W_H^1, \sigma_{L,a}^0, \sigma_{L,a}^0} \\
& + 2 \sum_{a=1}^4 \sum_{b=1}^4 |\Gamma_{W_H^1, \phi_{L,a}^0, \sigma_{L,b}^\pm}|^2 \left( -4B_{22} \left( p^2, m_{\sigma_{L,a}^\pm}^2, m_{\phi_{L,b}^0}^2 \right) - A_0 \left( m_{\phi_{L,b}^0}^2 \right) - A_0 \left( m_{\sigma_{L,a}^\pm}^2 \right) \right) \\
& + 2 \sum_{a=1}^4 \sum_{b=1}^4 |\Gamma_{W_H^1, \sigma_{L,a}^0, \sigma_{L,b}^\pm}|^2 \left( -4B_{22} \left( p^2, m_{\sigma_{L,a}^\pm}^2, m_{\sigma_{L,b}^0}^2 \right) - A_0 \left( m_{\sigma_{L,b}^0}^2 \right) - A_0 \left( m_{\sigma_{L,a}^\pm}^2 \right) \right) \\
& + \frac{1}{2} \sum_{a=1}^{10} \sum_{b=1}^{10} \left[ \left( |\Gamma_{W_H^1, f_{Po,a}^0, f_{Go,b}^-}|^2 + |\Gamma_{W_H^1, f_{Po,a}^0, f_{Go,b}^-}|^2 \right) H_0 \left( p^2, m_{f_{Po,a}^0}^2, m_{f_{Go,b}^-}^2 \right) \right. \\
& \left. + 4B_0 \left( p^2, m_{f_{Po,a}^0}^2, m_{f_{Go,b}^-}^2 \right) m_{f_{Go,b}^-} m_{f_{Po,a}^0} \Re \left( \Gamma_{W_H^1, f_{Po,a}^0, f_{Go,b}^-}^{L*} \Gamma_{W_H^1, f_{Po,a}^0, f_{Go,b}^-}^R \right) \right] \\
& + 2 \sum_{b=1}^4 |\Gamma_{W_H^1, B_L, \sigma_{L,b}^\pm}|^2 B_0 \left( p^2, m_{B_L}^2, m_{\sigma_{L,b}^\pm}^2 \right) + 2 \sum_{b=1}^4 |\Gamma_{W_H^1, B_H, \sigma_{L,b}^\pm}|^2 B_0 \left( p^2, m_{B_H}^2, m_{\sigma_{L,b}^\pm}^2 \right) \\
& + \sum_{b=1}^4 |\Gamma_{W_H^1, W_L^1, \phi_{L,b}^0}|^2 B_0 \left( p^2, m_{W_L^1}^2, m_{\phi_{L,b}^0}^2 \right) + \sum_{b=1}^4 |\Gamma_{W_H^1, W_H^1, \phi_{L,b}^0}|^2 B_0 \left( p^2, m_{W_H^1}^2, m_{\phi_{L,b}^0}^2 \right) \\
& + \sum_{b=1}^4 |\Gamma_{W_H^1, W_L^2, \sigma_{L,b}^0}|^2 B_0 \left( p^2, m_{W_L^2}^2, m_{\sigma_{L,b}^0}^2 \right) + 2 \sum_{b=1}^4 |\Gamma_{W_H^1, W_L^3, \sigma_{L,b}^\pm}|^2 B_0 \left( p^2, m_{W_L^3}^2, m_{\sigma_{L,b}^\pm}^2 \right) \\
& - \frac{1}{2} A_0 \left( m_{W_L^2}^2 \right) \left( 4\Gamma_{W_H^1, W_H^1, W_L^2, W_L^2}^1 + \Gamma_{W_H^1, W_H^1, W_L^2, W_L^2}^2 + \Gamma_{W_H^1, W_H^1, W_L^2, W_L^2}^3 \right) - \frac{1}{2} A_0 \left( m_{W_H^2}^2 \right) \left( 4\Gamma_{W_H^1, W_H^1, W_H^2, W_H^2}^1 + \Gamma_{W_H^1, W_H^1, W_H^2, W_H^2}^2 \right) \\
\end{aligned} \tag{377}$$

• Self-Energy for Light W2 gauge boson ( $W_L^2$ )

$$\begin{aligned}
\Pi(p^2) = & +2|\Gamma_{W_L^2, \eta \bar{W}_L^3, \eta W_L^1}|^2 B_{00}(p^2, m_{\eta W_L^1}^2, m_{\eta W_L^3}^2) + 2|\Gamma_{W_L^2, \eta \bar{W}_H^3, \eta W_L^1}|^2 B_{00}(p^2, m_{\eta W_L^1}^2, m_{\eta W_H^3}^2) \\
& + 2|\Gamma_{W_L^2, \eta \bar{W}_L^3, \eta W_H^1}|^2 B_{00}(p^2, m_{\eta W_H^1}^2, m_{\eta W_L^3}^2) + 2|\Gamma_{W_L^2, \eta \bar{W}_H^3, \eta W_H^1}|^2 B_{00}(p^2, m_{\eta W_H^1}^2, m_{\eta W_H^3}^2) \\
& + 2|\Gamma_{W_L^2, H_d^-, *, H_d^0}|^2 \left( -4B_{22}(p^2, m_{H_d^0}^2, m_{H_d^-}^2) - A_0(m_{H_d^-}^2) - A_0(m_{H_d^0}^2) \right) \\
& + 2|\Gamma_{W_L^2, H_u^+, *, H_u^0}|^2 \left( -4B_{22}(p^2, m_{H_u^0}^2, m_{H_u^+}^2) - A_0(m_{H_u^+}^2) - A_0(m_{H_u^0}^2) \right) \\
& + A_0(m_{H_d^0}^2) \Gamma_{W_L^2, W_L^2, H_d^0, *, H_d^0} + A_0(m_{H_d^-}^2) \Gamma_{W_L^2, W_L^2, H_d^-, *, H_d^-} + A_0(m_{H_u^0}^2) \Gamma_{W_L^2, W_L^2, H_u^0, *, H_u^0} \\
& + A_0(m_{H_u^+}^2) \Gamma_{W_L^2, W_L^2, H_u^+, *, H_u^+} + \left( |\Gamma_{W_L^2, \text{FHCD}^-(\{1\}), \text{FH0D}(\{1\})}^L|^2 + |\Gamma_{W_L^2, \text{FHCD}^-(\{1\}), \text{FH0D}(\{1\})}^R|^2 \right) H_0(p^2, m_{\tilde{H}^-}^2, m_{\tilde{H}^0}^2) \\
& - |\Gamma_{W_L^2, W_L^3, W_L^1}|^2 \left( 10B_{00}(p^2, m_{W_L^3}^2, m_{W_L^1}^2) + B_0(p^2, m_{W_L^3}^2, m_{W_L^1}^2) (4p^2 + m_{W_L^1}^2 + m_{W_L^3}^2) + A_0(m_{W_L^1}^2) + A_0(m_{W_L^3}^2) \right) \\
& - |\Gamma_{W_L^2, W_L^3, W_H^1}|^2 \left( 10B_{00}(p^2, m_{W_L^3}^2, m_{W_H^1}^2) + B_0(p^2, m_{W_L^3}^2, m_{W_H^1}^2) (4p^2 + m_{W_H^1}^2 + m_{W_L^3}^2) + A_0(m_{W_H^1}^2) + A_0(m_{W_L^3}^2) \right) \\
& - |\Gamma_{W_L^2, W_H^3, W_L^1}|^2 \left( 10B_{00}(p^2, m_{W_H^3}^2, m_{W_L^1}^2) + B_0(p^2, m_{W_H^3}^2, m_{W_L^1}^2) (4p^2 + m_{W_L^1}^2 + m_{W_H^3}^2) + A_0(m_{W_L^1}^2) + A_0(m_{W_H^3}^2) \right) \\
& - |\Gamma_{W_L^2, W_H^3, W_H^1}|^2 \left( 10B_{00}(p^2, m_{W_H^3}^2, m_{W_H^1}^2) + B_0(p^2, m_{W_H^3}^2, m_{W_H^1}^2) (4p^2 + m_{W_H^1}^2 + m_{W_H^3}^2) + A_0(m_{W_H^1}^2) + A_0(m_{W_H^3}^2) \right) \\
& + 4B_0(p^2, m_{\tilde{H}^-}^2, m_{\tilde{H}^0}^2) m_{\tilde{H}^0} m_{\tilde{H}^-} \Re \left( \Gamma_{W_L^2, \text{FHCD}^-(\{1\}), \text{FH0D}(\{1\})}^{L*} \Gamma_{W_L^2, \text{FHCD}^-(\{1\}), \text{FH0D}(\{1\})}^R \right) + \sum_{a=1}^2 A_0(m_{\phi_{B,a}^s}^2) \Gamma_{W_L^2, W_L^2, \phi_{B,a}^s} \\
& + \sum_{a=1}^2 A_0(m_{\phi_{AK,a}^s}^2) \Gamma_{W_L^2, W_L^2, \phi_{AK,a}^{s,*}, \phi_{AK,a}^s} \\
& + 2 \sum_{a=1}^2 \sum_{b=1}^2 |\Gamma_{W_L^2, \phi_{AK,a}^{s,*}, \phi_{B,b}^s}|^2 \left( -4B_{22}(p^2, m_{\phi_{B,a}^s}^2, m_{\phi_{AK,b}^s}^2) - A_0(m_{\phi_{AK,b}^s}^2) - A_0(m_{\phi_{B,a}^s}^2) \right) \\
& + 2 \sum_{a=1}^2 \sum_{b=1}^2 |\Gamma_{W_L^2, \phi_{AK,a}^s, \phi_{B,b}^{s,*}}|^2 \left( -4B_{22}(p^2, m_{\phi_{B,a}^s}^2, m_{\phi_{AK,b}^s}^2) - A_0(m_{\phi_{AK,b}^s}^2) - A_0(m_{\phi_{B,a}^s}^2) \right) \\
& + 3 \sum_{a=1}^3 A_0(m_{\tilde{d}_{L,a}}^2) \Gamma_{W_L^2, W_L^2, \tilde{d}_{L,a}^*, \tilde{d}_{L,a}} + \sum_{a=1}^3 A_0(m_{\tilde{e}_{L,a}}^2) \Gamma_{W_L^2, W_L^2, \tilde{e}_{L,a}^*, \tilde{e}_{L,a}} \\
& + 3 \sum_{a=1}^3 A_0(m_{\tilde{u}_{L,a}}^2) \Gamma_{W_L^2, W_L^2, \tilde{u}_{L,a}^*, \tilde{u}_{L,a}} + \sum_{a=1}^3 A_0(m_{\tilde{\nu}_{L,a}}^2) \Gamma_{W_L^2, W_L^2, \tilde{\nu}_{L,a}^*, \tilde{\nu}_{L,a}} \\
& + 6 \sum_{a=1}^3 \sum_{b=1}^3 |\Gamma_{W_L^2, \tilde{u}_{L,a}^*, \tilde{d}_{L,b}}|^2 \left( -4B_{22}(p^2, m_{\tilde{d}_{L,a}}^2, m_{\tilde{u}_{L,b}}^2) - A_0(m_{\tilde{d}_{L,a}}^2) - A_0(m_{\tilde{u}_{L,b}}^2) \right)
\end{aligned}$$

$$\begin{aligned}
& + 2 \sum_{a=1}^3 \sum_{b=1}^3 |\Gamma_{W_L^2, \tilde{\nu}_{L,a}^*, \tilde{e}_{L,b}}|^2 \left( -4B_{22}(p^2, m_{\tilde{e}_{L,a}}^2, m_{\tilde{\nu}_{L,b}}^2) - A_0(m_{\tilde{e}_{L,a}}^2) - A_0(m_{\tilde{\nu}_{L,b}}^2) \right) \\
& + 3 \sum_{a=1}^3 \sum_{b=1}^3 \left[ \left( |\Gamma_{W_L^2, \bar{u}^{D_L,a}, d_{L,b}^D}|^2 + |\Gamma_{W_L^2, \bar{u}^{D_L,a}, d_{L,b}^D}|^2 \right) H_0(p^2, m_{u_{L,a}^D}^2, m_{d_{L,b}^D}^2) \right. \\
& + 4B_0(p^2, m_{u_{L,a}^D}^2, m_{d_{L,b}^D}^2) m_{\bar{u}^{D_L,a}} m_{d_{L,b}^D} \Re \left( \Gamma_{W_L^2, \bar{u}^{D_L,a}, d_{L,b}^D}^{L*} \Gamma_{W_L^2, \bar{u}^{D_L,a}, d_{L,b}^D}^R \right) \Big] \\
& + \sum_{a=1}^3 \sum_{b=1}^3 \left[ \left( |\Gamma_{W_L^2, \bar{\nu}^{D_L,a}, e_{L,b}^D}|^2 + |\Gamma_{W_L^2, \bar{\nu}^{D_L,a}, e_{L,b}^D}|^2 \right) H_0(p^2, m_{\nu_{L,a}^D}^2, m_{e_{L,b}^D}^2) \right. \\
& + 4B_0(p^2, m_{\nu_{L,a}^D}^2, m_{e_{L,b}^D}^2) m_{\bar{\nu}^{D_L,a}} m_{e_{L,b}^D} \Re \left( \Gamma_{W_L^2, \bar{\nu}^{D_L,a}, e_{L,b}^D}^{L*} \Gamma_{W_L^2, \bar{\nu}^{D_L,a}, e_{L,b}^D}^R \right) \Big] \\
& + \sum_{a=1}^4 A_0(m_{\sigma_{L,a}^\pm}^2) \Gamma_{W_L^2, W_L^2, \sigma_{L,a}^\pm, *} \sigma_{L,a}^\pm + \frac{1}{2} \sum_{a=1}^4 A_0(m_{\phi_{L,a}^0}^2) \Gamma_{W_L^2, W_L^2, \phi_{L,a}^0, \phi_{L,a}^0} \\
& + \frac{1}{2} \sum_{a=1}^4 A_0(m_{\sigma_{L,a}^0}^2) \Gamma_{W_L^2, W_L^2, \sigma_{L,a}^0, \sigma_{L,a}^0} \\
& + 2 \sum_{a=1}^4 \sum_{b=1}^4 |\Gamma_{W_L^2, \phi_{L,a}^0, \sigma_{L,b}^\pm}|^2 \left( -4B_{22}(p^2, m_{\sigma_{L,a}^\pm}^2, m_{\phi_{L,b}^0}^2) - A_0(m_{\phi_{L,b}^0}^2) - A_0(m_{\sigma_{L,a}^\pm}^2) \right) \\
& + 2 \sum_{a=1}^4 \sum_{b=1}^4 |\Gamma_{W_L^2, \sigma_{L,a}^0, \sigma_{L,b}^\pm}|^2 \left( -4B_{22}(p^2, m_{\sigma_{L,a}^\pm}^2, m_{\sigma_{L,b}^0}^2) - A_0(m_{\sigma_{L,b}^0}^2) - A_0(m_{\sigma_{L,a}^\pm}^2) \right) \\
& + \frac{1}{2} \sum_{a=1}^{10} \sum_{b=1}^{10} \left[ \left( |\Gamma_{W_L^2, f_{P_{o,a}}^0, f_{G_{o,b}}^-}|^2 + |\Gamma_{W_L^2, f_{P_{o,a}}^0, f_{G_{o,b}}^-}|^2 \right) H_0(p^2, m_{f_{P_{o,a}}^0}^2, m_{f_{G_{o,b}}^-}^2) \right. \\
& + 4B_0(p^2, m_{f_{P_{o,a}}^0}^2, m_{f_{G_{o,b}}^-}^2) m_{f_{G_{o,b}}^-} m_{f_{P_{o,a}}^0} \Re \left( \Gamma_{W_L^2, f_{P_{o,a}}^0, f_{G_{o,b}}^-}^{L*} \Gamma_{W_L^2, f_{P_{o,a}}^0, f_{G_{o,b}}^-}^R \right) \Big] \\
& + 2 \sum_{b=1}^4 |\Gamma_{W_L^2, B_L, \sigma_{L,b}^\pm}|^2 B_0(p^2, m_{B_L}^2, m_{\sigma_{L,b}^\pm}^2) + 2 \sum_{b=1}^4 |\Gamma_{W_L^2, B_H, \sigma_{L,b}^\pm}|^2 B_0(p^2, m_{B_H}^2, m_{\sigma_{L,b}^\pm}^2) \\
& + \sum_{b=1}^4 |\Gamma_{W_L^2, W_H^1, \sigma_{L,b}^0}|^2 B_0(p^2, m_{W_H^1}^2, m_{\sigma_{L,b}^0}^2) + \sum_{b=1}^4 |\Gamma_{W_L^2, W_L^2, \phi_{L,b}^0}|^2 B_0(p^2, m_{W_L^2}^2, m_{\phi_{L,b}^0}^2) \\
& + \sum_{b=1}^4 |\Gamma_{W_L^2, W_H^2, \phi_{L,b}^0}|^2 B_0(p^2, m_{W_H^2}^2, m_{\phi_{L,b}^0}^2) + 2 \sum_{b=1}^4 |\Gamma_{W_L^2, W_H^3, \sigma_{L,b}^\pm}|^2 B_0(p^2, m_{W_H^3}^2, m_{\sigma_{L,b}^\pm}^2) \\
& - \frac{1}{2} A_0(m_{W_L^1}^2) \left( 4\Gamma_{W_L^2, W_L^2, W_L^1, W_L^1}^1 + \Gamma_{W_L^2, W_L^2, W_L^1, W_L^1}^2 + \Gamma_{W_L^2, W_L^2, W_L^1, W_L^1}^3 \right) - \frac{1}{2} A_0(m_{W_H^1}^2) \left( 4\Gamma_{W_L^2, W_L^2, W_H^1, W_H^1}^1 + \Gamma_{W_L^2, W_L^2, W_H^1, W_H^1}^2 \right. \\
& \quad \left. (378) \right)
\end{aligned}$$

• Self-Energy for Heavy W2 gauge boson ( $W_H^2$ )

$$\Pi(p^2) = +2|\Gamma_{W_H^2, \eta \bar{W}_L^3, \eta W_L^1}|^2 B_{00}(p^2, m_{\eta W_L^1}^2, m_{\eta W_L^3}^2) + 2|\Gamma_{W_H^2, \eta \bar{W}_H^3, \eta W_L^1}|^2 B_{00}(p^2, m_{\eta W_L^1}^2, m_{\eta W_H^3}^2)$$

$$\begin{aligned}
& + 2|\Gamma_{W_H^2, \eta \bar{W}_L^3, \eta W_H^1}|^2 B_{00}(p^2, m_{\eta W_H^1}^2, m_{\eta W_L^3}^2) + 2|\Gamma_{W_H^2, \eta \bar{W}_H^3, \eta W_H^1}|^2 B_{00}(p^2, m_{\eta W_H^1}^2, m_{\eta W_H^3}^2) \\
& + 2|\Gamma_{W_H^2, H_d^-, *, H_d^0}|^2 \left( -4B_{22}(p^2, m_{H_d^0}^2, m_{H_d^-}^2) - A_0(m_{H_d^-}^2) - A_0(m_{H_d^0}^2) \right) \\
& + 2|\Gamma_{W_H^2, H_u^+, *, H_u^0}|^2 \left( -4B_{22}(p^2, m_{H_u^0}^2, m_{H_u^+}^2) - A_0(m_{H_u^+}^2) - A_0(m_{H_u^0}^2) \right) \\
& + A_0(m_{H_d^0}^2) \Gamma_{W_H^2, W_H^2, H_d^0, *, H_d^0} + A_0(m_{H_d^-}^2) \Gamma_{W_H^2, W_H^2, H_d^-, *, H_d^-} + A_0(m_{H_u^0}^2) \Gamma_{W_H^2, W_H^2, H_u^0, *, H_u^0} \\
& + A_0(m_{H_u^+}^2) \Gamma_{W_H^2, W_H^2, H_u^+, *, H_u^+} + \left( |\Gamma_{W_H^2, \text{FHCD}^-(\{1\}), \text{FH0D}(\{1\})}^L|^2 + |\Gamma_{W_H^2, \text{FHCD}^-(\{1\}), \text{FH0D}(\{1\})}^R|^2 \right) H_0(p^2, m_{H^-}^2, m_{H^0}^2) \\
& - |\Gamma_{W_H^2, W_L^3, W_L^1}|^2 \left( 10B_{00}(p^2, m_{W_L^3}^2, m_{W_L^1}^2) + B_0(p^2, m_{W_L^3}^2, m_{W_L^1}^2) (4p^2 + m_{W_L^1}^2 + m_{W_L^3}^2) + A_0(m_{W_L^1}^2) + A_0(m_{W_L^3}^2) \right) \\
& - |\Gamma_{W_H^2, W_L^3, W_H^1}|^2 \left( 10B_{00}(p^2, m_{W_L^3}^2, m_{W_H^1}^2) + B_0(p^2, m_{W_L^3}^2, m_{W_H^1}^2) (4p^2 + m_{W_H^1}^2 + m_{W_L^3}^2) + A_0(m_{W_H^1}^2) + A_0(m_{W_L^3}^2) \right) \\
& - |\Gamma_{W_H^2, W_H^3, W_L^1}|^2 \left( 10B_{00}(p^2, m_{W_H^3}^2, m_{W_L^1}^2) + B_0(p^2, m_{W_H^3}^2, m_{W_L^1}^2) (4p^2 + m_{W_L^1}^2 + m_{W_H^3}^2) + A_0(m_{W_L^1}^2) + A_0(m_{W_H^3}^2) \right) \\
& - |\Gamma_{W_H^2, W_H^3, W_H^1}|^2 \left( 10B_{00}(p^2, m_{W_H^3}^2, m_{W_H^1}^2) + B_0(p^2, m_{W_H^3}^2, m_{W_H^1}^2) (4p^2 + m_{W_H^1}^2 + m_{W_H^3}^2) + A_0(m_{W_H^1}^2) + A_0(m_{W_H^3}^2) \right) \\
& + 4B_0(p^2, m_{H^-}^2, m_{H^0}^2) m_{H^0} m_{H^-} \Re \left( \Gamma_{W_H^2, \text{FHCD}^-(\{1\}), \text{FH0D}(\{1\})}^{L*} \Gamma_{W_H^2, \text{FHCD}^-(\{1\}), \text{FH0D}(\{1\})}^R \right) + \sum_{a=1}^2 A_0(m_{\phi_{B,a}^s}^2) \Gamma_{W_H^2, W_H^2, \phi_{B,a}^s} \\
& + \sum_{a=1}^2 A_0(m_{\phi_{AK,a}^s}^2) \Gamma_{W_H^2, W_H^2, \phi_{AK,a}^{s,*}, \phi_{AK,a}^s} \\
& + 2 \sum_{a=1}^2 \sum_{b=1}^2 |\Gamma_{W_H^2, \phi_{AK,a}^{s,*}, \phi_{B,b}^s}|^2 \left( -4B_{22}(p^2, m_{\phi_{B,a}^s}^2, m_{\phi_{AK,b}^s}^2) - A_0(m_{\phi_{AK,b}^s}^2) - A_0(m_{\phi_{B,a}^s}^2) \right) \\
& + 2 \sum_{a=1}^2 \sum_{b=1}^2 |\Gamma_{W_H^2, \phi_{AK,a}^s, \phi_{B,b}^s}|^2 \left( -4B_{22}(p^2, m_{\phi_{B,a}^s}^2, m_{\phi_{AK,b}^s}^2) - A_0(m_{\phi_{AK,b}^s}^2) - A_0(m_{\phi_{B,a}^s}^2) \right) \\
& + 3 \sum_{a=1}^3 A_0(m_{\tilde{d}_{L,a}}^2) \Gamma_{W_H^2, W_H^2, \tilde{d}_{L,a}^*, \tilde{d}_{L,a}} + \sum_{a=1}^3 A_0(m_{\tilde{e}_{L,a}}^2) \Gamma_{W_H^2, W_H^2, \tilde{e}_{L,a}^*, \tilde{e}_{L,a}} \\
& + 3 \sum_{a=1}^3 A_0(m_{\tilde{u}_{L,a}}^2) \Gamma_{W_H^2, W_H^2, \tilde{u}_{L,a}^*, \tilde{u}_{L,a}} + \sum_{a=1}^3 A_0(m_{\tilde{\nu}_{L,a}}^2) \Gamma_{W_H^2, W_H^2, \tilde{\nu}_{L,a}^*, \tilde{\nu}_{L,a}} \\
& + 6 \sum_{a=1}^3 \sum_{b=1}^3 |\Gamma_{W_H^2, \tilde{u}_{L,a}^*, \tilde{d}_{L,b}}|^2 \left( -4B_{22}(p^2, m_{\tilde{d}_{L,a}}^2, m_{\tilde{u}_{L,b}}^2) - A_0(m_{\tilde{d}_{L,a}}^2) - A_0(m_{\tilde{u}_{L,b}}^2) \right) \\
& + 2 \sum_{a=1}^3 \sum_{b=1}^3 |\Gamma_{W_H^2, \tilde{\nu}_{L,a}^*, \tilde{e}_{L,b}}|^2 \left( -4B_{22}(p^2, m_{\tilde{e}_{L,a}}^2, m_{\tilde{\nu}_{L,b}}^2) - A_0(m_{\tilde{e}_{L,a}}^2) - A_0(m_{\tilde{\nu}_{L,b}}^2) \right) \\
& + 3 \sum_{a=1}^3 \sum_{b=1}^3 \left[ \left( |\Gamma_{W_H^2, \tilde{u}^{DL,a}, d_{L,b}^D}|^2 + |\Gamma_{W_H^2, \tilde{u}^{DL,a}, d_{L,b}^D}|^2 \right) H_0(p^2, m_{u_{L,a}^D}^2, m_{d_{L,b}^D}^2) \right. \\
& \left. + 4B_0(p^2, m_{u_{L,a}^D}^2, m_{d_{L,b}^D}^2) m_{\tilde{u}^{DL,a}} m_{d_{L,b}^D} \Re \left( \Gamma_{W_H^2, \tilde{u}^{DL,a}, d_{L,b}^D}^{L*} \Gamma_{W_H^2, \tilde{u}^{DL,a}, d_{L,b}^D}^R \right) \right]
\end{aligned}$$

$$\begin{aligned}
& + \sum_{a=1}^3 \sum_{b=1}^3 \left[ \left( |\Gamma_{W_H^2, \bar{\nu}^{D_L, a}, e_{L, b}^D}|^2 + |\Gamma_{W_H^2, \bar{\nu}^{D_L, a}, e_{L, b}^D}|^2 \right) H_0 \left( p^2, m_{\nu_{L, a}^D}^2, m_{e_{L, b}^D}^2 \right) \right. \\
& + 4B_0 \left( p^2, m_{\nu_{L, a}^D}^2, m_{e_{L, b}^D}^2 \right) m_{\bar{\nu}^{D_L, a}} m_{e_{L, b}^D} \Re \left( \Gamma_{W_H^2, \bar{\nu}^{D_L, a}, e_{L, b}^D}^{L*} \Gamma_{W_H^2, \bar{\nu}^{D_L, a}, e_{L, b}^D}^R \right) \Big] \\
& + \sum_{a=1}^4 A_0 \left( m_{\sigma_{L, a}^\pm}^2 \right) \Gamma_{W_H^2, W_H^2, \sigma_{L, a}^\pm, *} + \frac{1}{2} \sum_{a=1}^4 A_0 \left( m_{\phi_{L, a}^0}^2 \right) \Gamma_{W_H^2, W_H^2, \phi_{L, a}^0, \phi_{L, a}^0} \\
& + \frac{1}{2} \sum_{a=1}^4 A_0 \left( m_{\sigma_{L, a}^0}^2 \right) \Gamma_{W_H^2, W_H^2, \sigma_{L, a}^0, \sigma_{L, a}^0} \\
& + 2 \sum_{a=1}^4 \sum_{b=1}^4 |\Gamma_{W_H^2, \phi_{L, a}^0, \sigma_{L, b}^\pm}|^2 \left( -4B_{22} \left( p^2, m_{\sigma_{L, a}^\pm}^2, m_{\phi_{L, b}^0}^2 \right) - A_0 \left( m_{\phi_{L, b}^0}^2 \right) - A_0 \left( m_{\sigma_{L, a}^\pm}^2 \right) \right) \\
& + 2 \sum_{a=1}^4 \sum_{b=1}^4 |\Gamma_{W_H^2, \sigma_{L, a}^0, \sigma_{L, b}^\pm}|^2 \left( -4B_{22} \left( p^2, m_{\sigma_{L, a}^\pm}^2, m_{\sigma_{L, b}^0}^2 \right) - A_0 \left( m_{\sigma_{L, b}^0}^2 \right) - A_0 \left( m_{\sigma_{L, a}^\pm}^2 \right) \right) \\
& + \frac{1}{2} \sum_{a=1}^{10} \sum_{b=1}^{10} \left[ \left( |\Gamma_{W_H^2, f_{P o, a}^0, f_{G o, b}^-}|^2 + |\Gamma_{W_H^2, f_{P o, a}^0, f_{G o, b}^-}|^2 \right) H_0 \left( p^2, m_{f_{P o, a}^0}^2, m_{f_{G o, b}^-}^2 \right) \right. \\
& + 4B_0 \left( p^2, m_{f_{P o, a}^0}^2, m_{f_{G o, b}^-}^2 \right) m_{f_{G o, b}^-} m_{f_{P o, a}^0} \Re \left( \Gamma_{W_H^2, f_{P o, a}^0, f_{G o, b}^-}^{L*} \Gamma_{W_H^2, f_{P o, a}^0, f_{G o, b}^-}^R \right) \Big] \\
& + 2 \sum_{b=1}^4 |\Gamma_{W_H^2, B_L, \sigma_{L, b}^\pm}|^2 B_0 \left( p^2, m_{B_L}^2, m_{\sigma_{L, b}^\pm}^2 \right) + 2 \sum_{b=1}^4 |\Gamma_{W_H^2, B_H, \sigma_{L, b}^\pm}|^2 B_0 \left( p^2, m_{B_H}^2, m_{\sigma_{L, b}^\pm}^2 \right) \\
& + \sum_{b=1}^4 |\Gamma_{W_H^2, W_L^1, \sigma_{L, b}^0}|^2 B_0 \left( p^2, m_{W_L^1}^2, m_{\sigma_{L, b}^0}^2 \right) + \sum_{b=1}^4 |\Gamma_{W_H^2, W_L^2, \phi_{L, b}^0}|^2 B_0 \left( p^2, m_{W_L^2}^2, m_{\phi_{L, b}^0}^2 \right) \\
& + \sum_{b=1}^4 |\Gamma_{W_H^2, W_H^2, \phi_{L, b}^0}|^2 B_0 \left( p^2, m_{W_H^2}^2, m_{\phi_{L, b}^0}^2 \right) + 2 \sum_{b=1}^4 |\Gamma_{W_H^2, W_L^3, \sigma_{L, b}^\pm}|^2 B_0 \left( p^2, m_{W_L^3}^2, m_{\sigma_{L, b}^\pm}^2 \right) \\
& - \frac{1}{2} A_0 \left( m_{W_L^1}^2 \right) \left( 4\Gamma_{W_H^2, W_H^2, W_L^1, W_L^1}^1 + \Gamma_{W_H^2, W_H^2, W_L^1, W_L^1}^2 + \Gamma_{W_H^2, W_H^2, W_L^1, W_L^1}^3 \right) - \frac{1}{2} A_0 \left( m_{W_H^1}^2 \right) \left( 4\Gamma_{W_H^2, W_H^2, W_H^1, W_H^1}^1 + \Gamma_{W_H^2, W_H^2, W_H^1, W_H^1}^2 \right) \\
& \hspace{15cm} (379)
\end{aligned}$$

• Self-Energy for Light W3 gauge boson ( $W_L^3$ )

$$\begin{aligned}
\Pi(p^2) = & 2|\Gamma_{W_L^3, \eta \bar{W}_L^2, \eta W_L^1}|^2 B_{00} \left( p^2, m_{\eta W_L^1}^2, m_{\eta W_L^2}^2 \right) + 2|\Gamma_{W_L^3, \eta \bar{W}_H^2, \eta W_L^1}|^2 B_{00} \left( p^2, m_{\eta W_L^1}^2, m_{\eta W_H^2}^2 \right) \\
& + 2|\Gamma_{W_L^3, \eta \bar{W}_L^2, \eta W_H^1}|^2 B_{00} \left( p^2, m_{\eta W_H^1}^2, m_{\eta W_L^2}^2 \right) + 2|\Gamma_{W_L^3, \eta \bar{W}_H^2, \eta W_H^1}|^2 B_{00} \left( p^2, m_{\eta W_H^1}^2, m_{\eta W_H^2}^2 \right) \\
& + |\Gamma_{W_L^3, H_d^{0,*}, H_d^0}|^2 \left( -2A_0 \left( m_{H_d^0}^2 \right) - 4B_{22} \left( p^2, m_{H_d^0}^2, m_{H_d^0}^2 \right) \right) \\
& + |\Gamma_{W_L^3, H_d^{0,*}, H_d^-}|^2 \left( -2A_0 \left( m_{H_d^-}^2 \right) - 4B_{22} \left( p^2, m_{H_d^-}^2, m_{H_d^-}^2 \right) \right) \\
& + |\Gamma_{W_L^3, H_u^{0,*}, H_u^0}|^2 \left( -2A_0 \left( m_{H_u^0}^2 \right) - 4B_{22} \left( p^2, m_{H_u^0}^2, m_{H_u^0}^2 \right) \right)
\end{aligned}$$

$$\begin{aligned}
& + |\Gamma_{W_L^3, H_u^+, *, H_u^+}|^2 \left( -2A_0(m_{H_u^+}^2) - 4B_{22}(p^2, m_{H_u^+}^2, m_{H_u^+}^2) \right) + A_0(m_{H_d^0}^2) \Gamma_{W_L^3, W_L^3, H_d^0, *, H_d^0} \\
& + A_0(m_{H_d^-}^2) \Gamma_{W_L^3, W_L^3, H_d^-, *, H_d^-} + A_0(m_{H_u^0}^2) \Gamma_{W_L^3, W_L^3, H_u^0, *, H_u^0} + A_0(m_{H_u^+}^2) \Gamma_{W_L^3, W_L^3, H_u^+, *, H_u^+} \\
& - |\Gamma_{W_L^3, W_L^2, W_L^1}|^2 \left( 10B_{00}(p^2, m_{W_L^2}^2, m_{W_L^1}^2) + B_0(p^2, m_{W_L^2}^2, m_{W_L^1}^2) (4p^2 + m_{W_L^1}^2 + m_{W_L^2}^2) + A_0(m_{W_L^1}^2) + A_0(m_{W_L^2}^2) \right) \\
& - |\Gamma_{W_L^3, W_L^2, W_H^1}|^2 \left( 10B_{00}(p^2, m_{W_L^2}^2, m_{W_H^1}^2) + B_0(p^2, m_{W_L^2}^2, m_{W_H^1}^2) (4p^2 + m_{W_H^1}^2 + m_{W_L^2}^2) + A_0(m_{W_H^1}^2) + A_0(m_{W_L^2}^2) \right) \\
& - |\Gamma_{W_L^3, W_H^2, W_L^1}|^2 \left( 10B_{00}(p^2, m_{W_H^2}^2, m_{W_L^1}^2) + B_0(p^2, m_{W_H^2}^2, m_{W_L^1}^2) (4p^2 + m_{W_L^1}^2 + m_{W_H^2}^2) + A_0(m_{W_L^1}^2) + A_0(m_{W_H^2}^2) \right) \\
& - |\Gamma_{W_L^3, W_H^2, W_H^1}|^2 \left( 10B_{00}(p^2, m_{W_H^2}^2, m_{W_H^1}^2) + B_0(p^2, m_{W_H^2}^2, m_{W_H^1}^2) (4p^2 + m_{W_H^1}^2 + m_{W_H^2}^2) + A_0(m_{W_H^1}^2) + A_0(m_{W_H^2}^2) \right) \\
& + \frac{1}{2} \left( 4B_0(p^2, m_{\tilde{H}^0}^2, m_{\tilde{H}^0}^2) m_{\tilde{H}^0} m_{\tilde{H}^0} \Re \left( \Gamma_{W_L^3, \text{FH0D}}^{L*}(\{1\}) \Gamma_{W_L^3, \text{FH0D}}^R(\{1\}) \right) + \left( |\Gamma_{W_L^3, \text{FH0D}}^L(\{1\})| \Gamma_{W_L^3, \text{FH0D}}^R(\{1\}) \right) \right. \\
& + \frac{1}{2} \left( 4B_0(p^2, m_{\tilde{H}^-}^2, m_{\tilde{H}^-}^2) m_{\tilde{H}^-} m_{\tilde{H}^-} \Re \left( \Gamma_{W_L^3, \text{FHCD}}^{L*}(\{1\}) \Gamma_{W_L^3, \text{FHCD}}^R(\{1\}) \right) + \left( |\Gamma_{W_L^3, \text{FHCD}}^L(\{1\})| \Gamma_{W_L^3, \text{FHCD}}^R(\{1\}) \right) \right. \\
& + \sum_{a=1}^2 A_0(m_{\phi_{B,a}^s}^2) \Gamma_{W_L^3, W_L^3, \phi_{B,a}^s, *, \phi_{B,a}^s} \\
& + \sum_{a=1}^2 \sum_{b=1}^2 |\Gamma_{W_L^3, \phi_{B,a}^s, *, \phi_{B,b}^s}|^2 \left( -4B_{22}(p^2, m_{\phi_{B,a}^s}^2, m_{\phi_{B,b}^s}^2) - A_0(m_{\phi_{B,a}^s}^2) - A_0(m_{\phi_{B,b}^s}^2) \right) \\
& + 3 \sum_{a=1}^3 A_0(m_{\tilde{d}_{L,a}}^2) \Gamma_{W_L^3, W_L^3, \tilde{d}_{L,a}^*, \tilde{d}_{L,a}} + \sum_{a=1}^3 A_0(m_{\tilde{e}_{L,a}}^2) \Gamma_{W_L^3, W_L^3, \tilde{e}_{L,a}^*, \tilde{e}_{L,a}} \\
& + 3 \sum_{a=1}^3 A_0(m_{\tilde{u}_{L,a}}^2) \Gamma_{W_L^3, W_L^3, \tilde{u}_{L,a}^*, \tilde{u}_{L,a}} + \sum_{a=1}^3 A_0(m_{\tilde{\nu}_{L,a}}^2) \Gamma_{W_L^3, W_L^3, \tilde{\nu}_{L,a}^*, \tilde{\nu}_{L,a}} \\
& + 3 \sum_{a=1}^3 \sum_{b=1}^3 |\Gamma_{W_L^3, \tilde{d}_{L,a}^*, \tilde{d}_{L,b}}|^2 \left( -4B_{22}(p^2, m_{\tilde{d}_{L,a}}^2, m_{\tilde{d}_{L,b}}^2) - A_0(m_{\tilde{d}_{L,a}}^2) - A_0(m_{\tilde{d}_{L,b}}^2) \right) \\
& + \sum_{a=1}^3 \sum_{b=1}^3 |\Gamma_{W_L^3, \tilde{e}_{L,a}^*, \tilde{e}_{L,b}}|^2 \left( -4B_{22}(p^2, m_{\tilde{e}_{L,a}}^2, m_{\tilde{e}_{L,b}}^2) - A_0(m_{\tilde{e}_{L,a}}^2) - A_0(m_{\tilde{e}_{L,b}}^2) \right) \\
& + 3 \sum_{a=1}^3 \sum_{b=1}^3 |\Gamma_{W_L^3, \tilde{u}_{L,a}^*, \tilde{u}_{L,b}}|^2 \left( -4B_{22}(p^2, m_{\tilde{u}_{L,a}}^2, m_{\tilde{u}_{L,b}}^2) - A_0(m_{\tilde{u}_{L,a}}^2) - A_0(m_{\tilde{u}_{L,b}}^2) \right) \\
& + \sum_{a=1}^3 \sum_{b=1}^3 |\Gamma_{W_L^3, \tilde{\nu}_{L,a}^*, \tilde{\nu}_{L,b}}|^2 \left( -4B_{22}(p^2, m_{\tilde{\nu}_{L,a}}^2, m_{\tilde{\nu}_{L,b}}^2) - A_0(m_{\tilde{\nu}_{L,a}}^2) - A_0(m_{\tilde{\nu}_{L,b}}^2) \right) \\
& + \frac{3}{2} \sum_{a=1}^3 \sum_{b=1}^3 \left[ \left( |\Gamma_{W_L^3, \tilde{d}^D, a, d_{L,b}^D}|^2 + |\Gamma_{W_L^3, \tilde{d}^D, a, d_{L,b}^D}|^2 \right) H_0(p^2, m_{d_{L,a}^D}^2, m_{d_{L,b}^D}^2) \right. \\
& + 4B_0(p^2, m_{d_{L,a}^D}^2, m_{d_{L,b}^D}^2) m_{\tilde{d}^D, a} m_{d_{L,b}^D} \Re \left( \Gamma_{W_L^3, \tilde{d}^D, a, d_{L,b}^D}^{L*} \Gamma_{W_L^3, \tilde{d}^D, a, d_{L,b}^D}^R \right) \left. \right]
\end{aligned}$$

$$\begin{aligned}
& + \frac{1}{2} \sum_{a=1}^3 \sum_{b=1}^3 \left[ \left( |\Gamma_{W_L^3, \bar{e}^{D_L, a}, e_{L, b}^D}|^2 + |\Gamma_{W_L^3, \bar{e}^{D_L, a}, e_{L, b}^D}|^2 \right) H_0(p^2, m_{e_{L, a}^D}^2, m_{e_{L, b}^D}^2) \right. \\
& + 4B_0(p^2, m_{e_{L, a}^D}^2, m_{e_{L, b}^D}^2) m_{\bar{e}^{D_L, a}} m_{e_{L, b}^D} \Re \left( \Gamma_{W_L^3, \bar{e}^{D_L, a}, e_{L, b}^D}^{L*} \Gamma_{W_L^3, \bar{e}^{D_L, a}, e_{L, b}^D}^R \right) \Big] \\
& + \frac{3}{2} \sum_{a=1}^3 \sum_{b=1}^3 \left[ \left( |\Gamma_{W_L^3, \bar{u}^{D_L, a}, u_{L, b}^D}|^2 + |\Gamma_{W_L^3, \bar{u}^{D_L, a}, u_{L, b}^D}|^2 \right) H_0(p^2, m_{u_{L, a}^D}^2, m_{u_{L, b}^D}^2) \right. \\
& + 4B_0(p^2, m_{u_{L, a}^D}^2, m_{u_{L, b}^D}^2) m_{\bar{u}^{D_L, a}} m_{u_{L, b}^D} \Re \left( \Gamma_{W_L^3, \bar{u}^{D_L, a}, u_{L, b}^D}^{L*} \Gamma_{W_L^3, \bar{u}^{D_L, a}, u_{L, b}^D}^R \right) \Big] \\
& + \frac{1}{2} \sum_{a=1}^3 \sum_{b=1}^3 \left[ \left( |\Gamma_{W_L^3, \bar{\nu}^{D_L, a}, \nu_{L, b}^D}|^2 + |\Gamma_{W_L^3, \bar{\nu}^{D_L, a}, \nu_{L, b}^D}|^2 \right) H_0(p^2, m_{\nu_{L, a}^D}^2, m_{\nu_{L, b}^D}^2) \right. \\
& + 4B_0(p^2, m_{\nu_{L, a}^D}^2, m_{\nu_{L, b}^D}^2) m_{\bar{\nu}^{D_L, a}} m_{\nu_{L, b}^D} \Re \left( \Gamma_{W_L^3, \bar{\nu}^{D_L, a}, \nu_{L, b}^D}^{L*} \Gamma_{W_L^3, \bar{\nu}^{D_L, a}, \nu_{L, b}^D}^R \right) \Big] \\
& + \sum_{a=1}^4 A_0(m_{\sigma_{L, a}^\pm}^2) \Gamma_{W_L^3, W_L^3, \sigma_{L, a}^\pm, *} \sigma_{L, a}^\pm + \frac{1}{2} \sum_{a=1}^4 A_0(m_{\phi_{L, a}^0}^2) \Gamma_{W_L^3, W_L^3, \phi_{L, a}^0, \phi_{L, a}^0} \\
& + \frac{1}{2} \sum_{a=1}^4 A_0(m_{\sigma_{L, a}^0}^2) \Gamma_{W_L^3, W_L^3, \sigma_{L, a}^0, \sigma_{L, a}^0} \\
& + \sum_{a=1}^4 \sum_{b=1}^4 |\Gamma_{W_L^3, \sigma_{L, a}^\pm, *} \sigma_{L, b}^\pm|^2 \left( -4B_{22}(p^2, m_{\sigma_{L, a}^\pm}^2, m_{\sigma_{L, b}^\pm}^2) - A_0(m_{\sigma_{L, a}^\pm}^2) - A_0(m_{\sigma_{L, b}^\pm}^2) \right) \\
& + \sum_{a=1}^4 \sum_{b=1}^4 |\Gamma_{W_L^3, \sigma_{L, a}^0, \phi_{L, b}^0}|^2 \left( -4B_{22}(p^2, m_{\phi_{L, a}^0}^2, m_{\sigma_{L, b}^0}^2) - A_0(m_{\phi_{L, a}^0}^2) - A_0(m_{\sigma_{L, b}^0}^2) \right) \\
& + \frac{1}{4} \sum_{a=1}^{10} \sum_{b=1}^{10} \left[ \left( |\Gamma_{W_L^3, f_{G^0, a}^-, f_{G^0, b}^-}|^2 + |\Gamma_{W_L^3, f_{G^0, a}^-, f_{G^0, b}^-}|^2 \right) H_0(p^2, m_{f_{G^0, a}^-}^2, m_{f_{G^0, b}^-}^2) \right. \\
& + 4B_0(p^2, m_{f_{G^0, a}^-}^2, m_{f_{G^0, b}^-}^2) m_{f_{G^0, a}^-} m_{f_{G^0, b}^-} \Re \left( \Gamma_{W_L^3, f_{G^0, a}^-, f_{G^0, b}^-}^{L*} \Gamma_{W_L^3, f_{G^0, a}^-, f_{G^0, b}^-}^R \right) \Big] \\
& + \frac{1}{4} \sum_{a=1}^{10} \sum_{b=1}^{10} \left[ \left( |\Gamma_{W_L^3, f_{P^0, a}^0, f_{P^0, b}^0}|^2 + |\Gamma_{W_L^3, f_{P^0, a}^0, f_{P^0, b}^0}|^2 \right) H_0(p^2, m_{f_{P^0, a}^0}^2, m_{f_{P^0, b}^0}^2) \right. \\
& + 4B_0(p^2, m_{f_{P^0, a}^0}^2, m_{f_{P^0, b}^0}^2) m_{f_{P^0, a}^0} m_{f_{P^0, b}^0} \Re \left( \Gamma_{W_L^3, f_{P^0, a}^0, f_{P^0, b}^0}^{L*} \Gamma_{W_L^3, f_{P^0, a}^0, f_{P^0, b}^0}^R \right) \Big] \\
& + \sum_{b=1}^4 |\Gamma_{W_L^3, B_L, \phi_{L, b}^0}|^2 B_0(p^2, m_{B_L}^2, m_{\phi_{L, b}^0}^2) + \sum_{b=1}^4 |\Gamma_{W_L^3, B_H, \phi_{L, b}^0}|^2 B_0(p^2, m_{B_H}^2, m_{\phi_{L, b}^0}^2) \\
& + 2 \sum_{b=1}^4 |\Gamma_{W_L^3, W_H^1, \sigma_{L, b}^\pm}|^2 B_0(p^2, m_{W_H^1}^2, m_{\sigma_{L, b}^\pm}^2) + 2 \sum_{b=1}^4 |\Gamma_{W_L^3, W_H^2, \sigma_{L, b}^\pm}|^2 B_0(p^2, m_{W_H^2}^2, m_{\sigma_{L, b}^\pm}^2) \\
& + \sum_{b=1}^4 |\Gamma_{W_L^3, W_L^3, \phi_{L, b}^0}|^2 B_0(p^2, m_{W_L^3}^2, m_{\phi_{L, b}^0}^2) + \sum_{b=1}^4 |\Gamma_{W_L^3, W_H^3, \phi_{L, b}^0}|^2 B_0(p^2, m_{W_H^3}^2, m_{\phi_{L, b}^0}^2)
\end{aligned}$$

$$-\frac{1}{2}A_0\left(m_{W_L^1}^2\right)\left(4\Gamma_{W_L^3,W_L^3,W_L^1,W_L^1}^1+\Gamma_{W_L^3,W_L^3,W_L^1,W_L^1}^2+\Gamma_{W_L^3,W_L^3,W_L^1,W_L^1}^3\right)-\frac{1}{2}A_0\left(m_{W_H^1}^2\right)\left(4\Gamma_{W_L^3,W_L^3,W_H^1,W_H^1}^1+\Gamma_{W_L^3,W_L^3,W_H^1,W_H^1}^2\right. \\ \left.(380)\right)$$

• Self-Energy for Heavy W3 gauge boson ( $W_H^3$ )

$$\begin{aligned} \Pi(p^2) = & +2|\Gamma_{W_H^3,\eta\bar{W}_L^2,\eta W_L^1}|^2 B_{00}\left(p^2, m_{\eta W_L^1}^2, m_{\eta W_L^2}^2\right) + 2|\Gamma_{W_H^3,\eta\bar{W}_H^2,\eta W_L^1}|^2 B_{00}\left(p^2, m_{\eta W_L^1}^2, m_{\eta W_H^2}^2\right) \\ & + 2|\Gamma_{W_H^3,\eta\bar{W}_L^2,\eta W_H^1}|^2 B_{00}\left(p^2, m_{\eta W_H^1}^2, m_{\eta W_L^2}^2\right) + 2|\Gamma_{W_H^3,\eta\bar{W}_H^2,\eta W_H^1}|^2 B_{00}\left(p^2, m_{\eta W_H^1}^2, m_{\eta W_H^2}^2\right) \\ & + |\Gamma_{W_H^3,H_d^{0,*},H_d^0}|^2 \left(-2A_0\left(m_{H_d^0}^2\right) - 4B_{22}\left(p^2, m_{H_d^0}^2, m_{H_d^0}^2\right)\right) \\ & + |\Gamma_{W_H^3,H_d^{-,*},H_d^-}|^2 \left(-2A_0\left(m_{H_d^-}^2\right) - 4B_{22}\left(p^2, m_{H_d^-}^2, m_{H_d^-}^2\right)\right) \\ & + |\Gamma_{W_H^3,H_u^{0,*},H_u^0}|^2 \left(-2A_0\left(m_{H_u^0}^2\right) - 4B_{22}\left(p^2, m_{H_u^0}^2, m_{H_u^0}^2\right)\right) \\ & + |\Gamma_{W_H^3,H_u^{+,*},H_u^+}|^2 \left(-2A_0\left(m_{H_u^+}^2\right) - 4B_{22}\left(p^2, m_{H_u^+}^2, m_{H_u^+}^2\right)\right) + A_0\left(m_{H_d^0}^2\right)\Gamma_{W_H^3,W_H^3,H_d^{0,*},H_d^0} \\ & + A_0\left(m_{H_d^-}^2\right)\Gamma_{W_H^3,W_H^3,H_d^{-,*},H_d^-} + A_0\left(m_{H_u^0}^2\right)\Gamma_{W_H^3,W_H^3,H_u^{0,*},H_u^0} + A_0\left(m_{H_u^+}^2\right)\Gamma_{W_H^3,W_H^3,H_u^{+,*},H_u^+} \\ & - |\Gamma_{W_H^3,W_L^2,W_L^1}|^2 \left(10B_{00}\left(p^2, m_{W_L^2}^2, m_{W_L^1}^2\right) + B_0\left(p^2, m_{W_L^2}^2, m_{W_L^1}^2\right)\left(4p^2 + m_{W_L^1}^2 + m_{W_L^2}^2\right) + A_0\left(m_{W_L^1}^2\right) + A_0\left(m_{W_L^2}^2\right)\right) \\ & - |\Gamma_{W_H^3,W_L^2,W_H^1}|^2 \left(10B_{00}\left(p^2, m_{W_L^2}^2, m_{W_H^1}^2\right) + B_0\left(p^2, m_{W_L^2}^2, m_{W_H^1}^2\right)\left(4p^2 + m_{W_H^1}^2 + m_{W_L^2}^2\right) + A_0\left(m_{W_H^1}^2\right) + A_0\left(m_{W_L^2}^2\right)\right) \\ & - |\Gamma_{W_H^3,W_H^2,W_L^1}|^2 \left(10B_{00}\left(p^2, m_{W_H^2}^2, m_{W_L^1}^2\right) + B_0\left(p^2, m_{W_H^2}^2, m_{W_L^1}^2\right)\left(4p^2 + m_{W_L^1}^2 + m_{W_H^2}^2\right) + A_0\left(m_{W_L^1}^2\right) + A_0\left(m_{W_H^2}^2\right)\right) \\ & - |\Gamma_{W_H^3,W_H^2,W_H^1}|^2 \left(10B_{00}\left(p^2, m_{W_H^2}^2, m_{W_H^1}^2\right) + B_0\left(p^2, m_{W_H^2}^2, m_{W_H^1}^2\right)\left(4p^2 + m_{W_H^1}^2 + m_{W_H^2}^2\right) + A_0\left(m_{W_H^1}^2\right) + A_0\left(m_{W_H^2}^2\right)\right) \\ & + \frac{1}{2}\left(4B_0\left(p^2, m_{H^0}^2, m_{H^0}^2\right)m_{H^0}m_{H^0}\Re\left(\Gamma_{W_H^3,\text{FH0D}}^{L*}\left(\{1\}\right),\text{FH0D}\left(\{1\}\right)\Gamma_{W_H^3,\text{FH0D}}^R\left(\{1\}\right),\text{FH0D}\left(\{1\}\right)\right) + \left(|\Gamma_{W_H^3,\text{FH0D}}^L\left(\{1\}\right),\text{FH0D}\left(\{1\}\right)\right| \right. \\ & + \frac{1}{2}\left(4B_0\left(p^2, m_{H^-}^2, m_{H^-}^2\right)m_{H^-}m_{H^-}\Re\left(\Gamma_{W_H^3,\text{FHCD}}^{L*}\left(\{1\}\right),\text{FHCD}\left(\{1\}\right)\Gamma_{W_H^3,\text{FHCD}}^R\left(\{1\}\right),\text{FHCD}\left(\{1\}\right)\right) + \left(|\Gamma_{W_H^3,\text{FHCD}}^L\left(\{1\}\right),\text{FHCD}\left(\{1\}\right)\right| \right. \\ & + \sum_{a=1}^2 A_0\left(m_{\phi_{B,a}^s}^2\right)\Gamma_{W_H^3,W_H^3,\phi_{B,a}^{s,*},\phi_{B,a}^s} \\ & + \sum_{a=1}^2 \sum_{b=1}^2 |\Gamma_{W_H^3,\phi_{B,a}^{s,*},\phi_{B,b}^s}|^2 \left(-4B_{22}\left(p^2, m_{\phi_{B,a}^s}^2, m_{\phi_{B,b}^s}^2\right) - A_0\left(m_{\phi_{B,a}^s}^2\right) - A_0\left(m_{\phi_{B,b}^s}^2\right)\right) \\ & + 3 \sum_{a=1}^3 A_0\left(m_{\tilde{d}_{L,a}}^2\right)\Gamma_{W_H^3,W_H^3,\tilde{d}_{L,a}^*,\tilde{d}_{L,a}} + \sum_{a=1}^3 A_0\left(m_{\tilde{e}_{L,a}}^2\right)\Gamma_{W_H^3,W_H^3,\tilde{e}_{L,a}^*,\tilde{e}_{L,a}} \\ & + 3 \sum_{a=1}^3 A_0\left(m_{\tilde{u}_{L,a}}^2\right)\Gamma_{W_H^3,W_H^3,\tilde{u}_{L,a}^*,\tilde{u}_{L,a}} + \sum_{a=1}^3 A_0\left(m_{\tilde{\nu}_{L,a}}^2\right)\Gamma_{W_H^3,W_H^3,\tilde{\nu}_{L,a}^*,\tilde{\nu}_{L,a}} \\ & + 3 \sum_{a=1}^3 \sum_{b=1}^3 |\Gamma_{W_H^3,\tilde{d}_{L,a}^*,\tilde{d}_{L,b}}|^2 \left(-4B_{22}\left(p^2, m_{\tilde{d}_{L,a}}^2, m_{\tilde{d}_{L,b}}^2\right) - A_0\left(m_{\tilde{d}_{L,a}}^2\right) - A_0\left(m_{\tilde{d}_{L,b}}^2\right)\right) \end{aligned}$$



$$\begin{aligned}
& + \sum_{a=1}^3 \sum_{b=1}^3 |\Gamma_{W_H^3, \tilde{e}_{L,a}^*, \tilde{e}_{L,b}}|^2 \left( -4B_{22} \left( p^2, m_{\tilde{e}_{L,a}}^2, m_{\tilde{e}_{L,b}}^2 \right) - A_0 \left( m_{\tilde{e}_{L,a}}^2 \right) - A_0 \left( m_{\tilde{e}_{L,b}}^2 \right) \right) \\
& + 3 \sum_{a=1}^3 \sum_{b=1}^3 |\Gamma_{W_H^3, \tilde{u}_{L,a}^*, \tilde{u}_{L,b}}|^2 \left( -4B_{22} \left( p^2, m_{\tilde{u}_{L,a}}^2, m_{\tilde{u}_{L,b}}^2 \right) - A_0 \left( m_{\tilde{u}_{L,a}}^2 \right) - A_0 \left( m_{\tilde{u}_{L,b}}^2 \right) \right) \\
& + \sum_{a=1}^3 \sum_{b=1}^3 |\Gamma_{W_H^3, \tilde{\nu}_{L,a}^*, \tilde{\nu}_{L,b}}|^2 \left( -4B_{22} \left( p^2, m_{\tilde{\nu}_{L,a}}^2, m_{\tilde{\nu}_{L,b}}^2 \right) - A_0 \left( m_{\tilde{\nu}_{L,a}}^2 \right) - A_0 \left( m_{\tilde{\nu}_{L,b}}^2 \right) \right) \\
& + \frac{3}{2} \sum_{a=1}^3 \sum_{b=1}^3 \left[ \left( |\Gamma_{W_H^3, \bar{d}^{D_L,a}, d_{L,b}^D}|^2 + |\Gamma_{W_H^3, \bar{d}^{D_L,a}, d_{L,b}^D}|^2 \right) H_0 \left( p^2, m_{d_{L,a}^D}^2, m_{d_{L,b}^D}^2 \right) \right. \\
& \left. + 4B_0 \left( p^2, m_{d_{L,a}^D}^2, m_{d_{L,b}^D}^2 \right) m_{\bar{d}^{D_L,a}} m_{d_{L,b}^D} \Re \left( \Gamma_{W_H^3, \bar{d}^{D_L,a}, d_{L,b}^D}^{L*} \Gamma_{W_H^3, \bar{d}^{D_L,a}, d_{L,b}^D}^R \right) \right] \\
& + \frac{1}{2} \sum_{a=1}^3 \sum_{b=1}^3 \left[ \left( |\Gamma_{W_H^3, \bar{e}^{D_L,a}, e_{L,b}^D}|^2 + |\Gamma_{W_H^3, \bar{e}^{D_L,a}, e_{L,b}^D}|^2 \right) H_0 \left( p^2, m_{e_{L,a}^D}^2, m_{e_{L,b}^D}^2 \right) \right. \\
& \left. + 4B_0 \left( p^2, m_{e_{L,a}^D}^2, m_{e_{L,b}^D}^2 \right) m_{\bar{e}^{D_L,a}} m_{e_{L,b}^D} \Re \left( \Gamma_{W_H^3, \bar{e}^{D_L,a}, e_{L,b}^D}^{L*} \Gamma_{W_H^3, \bar{e}^{D_L,a}, e_{L,b}^D}^R \right) \right] \\
& + \frac{3}{2} \sum_{a=1}^3 \sum_{b=1}^3 \left[ \left( |\Gamma_{W_H^3, \bar{u}^{D_L,a}, u_{L,b}^D}|^2 + |\Gamma_{W_H^3, \bar{u}^{D_L,a}, u_{L,b}^D}|^2 \right) H_0 \left( p^2, m_{u_{L,a}^D}^2, m_{u_{L,b}^D}^2 \right) \right. \\
& \left. + 4B_0 \left( p^2, m_{u_{L,a}^D}^2, m_{u_{L,b}^D}^2 \right) m_{\bar{u}^{D_L,a}} m_{u_{L,b}^D} \Re \left( \Gamma_{W_H^3, \bar{u}^{D_L,a}, u_{L,b}^D}^{L*} \Gamma_{W_H^3, \bar{u}^{D_L,a}, u_{L,b}^D}^R \right) \right] \\
& + \frac{1}{2} \sum_{a=1}^3 \sum_{b=1}^3 \left[ \left( |\Gamma_{W_H^3, \bar{\nu}^{D_L,a}, \nu_{L,b}^D}|^2 + |\Gamma_{W_H^3, \bar{\nu}^{D_L,a}, \nu_{L,b}^D}|^2 \right) H_0 \left( p^2, m_{\nu_{L,a}^D}^2, m_{\nu_{L,b}^D}^2 \right) \right. \\
& \left. + 4B_0 \left( p^2, m_{\nu_{L,a}^D}^2, m_{\nu_{L,b}^D}^2 \right) m_{\bar{\nu}^{D_L,a}} m_{\nu_{L,b}^D} \Re \left( \Gamma_{W_H^3, \bar{\nu}^{D_L,a}, \nu_{L,b}^D}^{L*} \Gamma_{W_H^3, \bar{\nu}^{D_L,a}, \nu_{L,b}^D}^R \right) \right] \\
& + \sum_{a=1}^4 A_0 \left( m_{\sigma_{L,a}^\pm}^2 \right) \Gamma_{W_H^3, W_H^3, \sigma_{L,a}^\pm, *} \sigma_{L,a}^\pm + \frac{1}{2} \sum_{a=1}^4 A_0 \left( m_{\phi_{L,a}^0}^2 \right) \Gamma_{W_H^3, W_H^3, \phi_{L,a}^0, \phi_{L,a}^0} \\
& + \frac{1}{2} \sum_{a=1}^4 A_0 \left( m_{\sigma_{L,a}^0}^2 \right) \Gamma_{W_H^3, W_H^3, \sigma_{L,a}^0, \sigma_{L,a}^0} \\
& + \sum_{a=1}^4 \sum_{b=1}^4 |\Gamma_{W_H^3, \sigma_{L,a}^\pm, *} \sigma_{L,b}^\pm|^2 \left( -4B_{22} \left( p^2, m_{\sigma_{L,a}^\pm}^2, m_{\sigma_{L,b}^\pm}^2 \right) - A_0 \left( m_{\sigma_{L,a}^\pm}^2 \right) - A_0 \left( m_{\sigma_{L,b}^\pm}^2 \right) \right) \\
& + \sum_{a=1}^4 \sum_{b=1}^4 |\Gamma_{W_H^3, \sigma_{L,a}^0, \phi_{L,b}^0}|^2 \left( -4B_{22} \left( p^2, m_{\phi_{L,a}^0}^2, m_{\sigma_{L,b}^0}^2 \right) - A_0 \left( m_{\phi_{L,a}^0}^2 \right) - A_0 \left( m_{\sigma_{L,b}^0}^2 \right) \right) \\
& + \frac{1}{4} \sum_{a=1}^{10} \sum_{b=1}^{10} \left[ \left( |\Gamma_{W_H^3, f_{G^0,a}^-, f_{G^0,b}^-}|^2 + |\Gamma_{W_H^3, f_{G^0,a}^-, f_{G^0,b}^-}|^2 \right) H_0 \left( p^2, m_{f_{G^0,a}^-}^2, m_{f_{G^0,b}^-}^2 \right) \right. \\
& \left. + 4B_0 \left( p^2, m_{f_{G^0,a}^-}^2, m_{f_{G^0,b}^-}^2 \right) m_{f_{G^0,a}^-} m_{f_{G^0,b}^-} \Re \left( \Gamma_{W_H^3, f_{G^0,a}^-, f_{G^0,b}^-}^{L*} \Gamma_{W_H^3, f_{G^0,a}^-, f_{G^0,b}^-}^R \right) \right]
\end{aligned}$$

$$\begin{aligned}
& + \frac{1}{4} \sum_{a=1}^{10} \sum_{b=1}^{10} \left[ \left( |\Gamma_{W_H^3, f_{Po,a}^0, f_{Po,b}^0}^L|^2 + |\Gamma_{W_H^3, f_{Po,a}^0, f_{Po,b}^0}^R|^2 \right) H_0(p^2, m_{f_{Po,a}^0}^2, m_{f_{Po,b}^0}^2) \right. \\
& + 4B_0(p^2, m_{f_{Po,a}^0}^2, m_{f_{Po,b}^0}^2) m_{f_{Po,a}^0} m_{f_{Po,b}^0} \Re \left( \Gamma_{W_H^3, f_{Po,a}^0, f_{Po,b}^0}^{L*} \Gamma_{W_H^3, f_{Po,a}^0, f_{Po,b}^0}^R \right) \left. \right] \\
& + \sum_{b=1}^4 |\Gamma_{W_H^3, B_L, \phi_{L,b}^0}|^2 B_0(p^2, m_{B_L}^2, m_{\phi_{L,b}^0}^2) + \sum_{b=1}^4 |\Gamma_{W_H^3, B_H, \phi_{L,b}^0}|^2 B_0(p^2, m_{B_H}^2, m_{\phi_{L,b}^0}^2) \\
& + 2 \sum_{b=1}^4 |\Gamma_{W_H^3, W_L^1, \sigma_{L,b}^\pm}|^2 B_0(p^2, m_{W_L^1}^2, m_{\sigma_{L,b}^\pm}^2) + 2 \sum_{b=1}^4 |\Gamma_{W_H^3, W_L^2, \sigma_{L,b}^\pm}|^2 B_0(p^2, m_{W_L^2}^2, m_{\sigma_{L,b}^\pm}^2) \\
& + \sum_{b=1}^4 |\Gamma_{W_H^3, W_L^3, \phi_{L,b}^0}|^2 B_0(p^2, m_{W_L^3}^2, m_{\phi_{L,b}^0}^2) + \sum_{b=1}^4 |\Gamma_{W_H^3, W_H^3, \phi_{L,b}^0}|^2 B_0(p^2, m_{W_H^3}^2, m_{\phi_{L,b}^0}^2) \\
& - \frac{1}{2} A_0(m_{W_L^1}^2) \left( 4\Gamma_{W_H^3, W_H^3, W_L^1, W_L^1}^1 + \Gamma_{W_H^3, W_H^3, W_L^1, W_L^1}^2 + \Gamma_{W_H^3, W_H^3, W_L^1, W_L^1}^3 \right) - \frac{1}{2} A_0(m_{W_H^1}^2) \left( 4\Gamma_{W_H^3, W_H^3, W_H^1, W_H^1}^1 + \Gamma_{W_H^3, W_H^3, W_H^1, W_H^1}^2 + \Gamma_{W_H^3, W_H^3, W_H^1, W_H^1}^3 \right) \\
& \hspace{15em} (381)
\end{aligned}$$

## 8.2 Tadpoles

$$\begin{aligned}
\delta t_{\phi_L^0}^{(1)} = & + \frac{1}{2} A_0(m_{B_L}^2) \Gamma_{\check{\phi}^0_L, i, B_L, B_L} + \frac{1}{2} A_0(m_{B_H}^2) \Gamma_{\check{\phi}^0_L, i, B_H, B_H} + \frac{1}{2} A_0(m_{W_L^1}^2) \Gamma_{\check{\phi}^0_L, i, W_L^1, W_L^1} \\
& + \frac{1}{2} A_0(m_{W_H^1}^2) \Gamma_{\check{\phi}^0_L, i, W_H^1, W_H^1} + \frac{1}{2} A_0(m_{W_L^2}^2) \Gamma_{\check{\phi}^0_L, i, W_L^2, W_L^2} + \frac{1}{2} A_0(m_{W_H^2}^2) \Gamma_{\check{\phi}^0_L, i, W_H^2, W_H^2} \\
& + \frac{1}{2} A_0(m_{W_L^3}^2) \Gamma_{\check{\phi}^0_L, i, W_L^3, W_L^3} + \frac{1}{2} A_0(m_{W_H^3}^2) \Gamma_{\check{\phi}^0_L, i, W_H^3, W_H^3} - 2A_0(m_{\eta B_L}^2) \Gamma_{\check{\phi}^0_L, i, \eta B_L, \eta B_L} \\
& - 2A_0(m_{\eta B_H}^2) \Gamma_{\check{\phi}^0_L, i, \eta \bar{B}_H, \eta B_H} - 2A_0(m_{\eta W_L^1}^2) \Gamma_{\check{\phi}^0_L, i, \eta \bar{W}_L^1, \eta W_L^1} - 2A_0(m_{\eta W_H^1}^2) \Gamma_{\check{\phi}^0_L, i, \eta \bar{W}_H^1, \eta W_H^1} \\
& - 2A_0(m_{\eta W_L^2}^2) \Gamma_{\check{\phi}^0_L, i, \eta \bar{W}_L^2, \eta W_L^2} - 2A_0(m_{\eta W_H^2}^2) \Gamma_{\check{\phi}^0_L, i, \eta \bar{W}_H^2, \eta W_H^2} - 2A_0(m_{\eta W_L^3}^2) \Gamma_{\check{\phi}^0_L, i, \eta \bar{W}_L^3, \eta W_L^3} \\
& - 2A_0(m_{\eta W_H^3}^2) \Gamma_{\check{\phi}^0_L, i, \eta \bar{W}_H^3, \eta W_H^3} - A_0(m_{H_d^0}^2) \Gamma_{\check{\phi}^0_L, i, H_d^0, * , H_d^0} - A_0(m_{H_d^-}^2) \Gamma_{\check{\phi}^0_L, i, H_d^-, * , H_d^-} \\
& - A_0(m_{H_u^0}^2) \Gamma_{\check{\phi}^0_L, i, H_u^0, * , H_u^0} - A_0(m_{H_u^+}^2) \Gamma_{\check{\phi}^0_L, i, H_u^+, * , H_u^+} - \sum_{a=1}^2 A_0(m_{\phi_{B,a}^s}^2) \Gamma_{\check{\phi}^0_L, i, \phi_{B,a}^s, * , \phi_{B,a}^s} \\
& - \sum_{a=1}^2 A_0(m_{\phi_{AK,a}^s}^2) \Gamma_{\check{\phi}^0_L, i, \phi_{AK,a}^s, * , \phi_{AK,a}^s} - 3 \sum_{a=1}^3 A_0(m_{\tilde{d}_{L,a}}^2) \Gamma_{\check{\phi}^0_L, i, \tilde{d}_{L,a}^*, \tilde{d}_{L,a}} \\
& - 3 \sum_{a=1}^3 A_0(m_{\tilde{d}_{R,a}}^2) \Gamma_{\check{\phi}^0_L, i, \tilde{d}_{R,a}^*, \tilde{d}_{R,a}} - \sum_{a=1}^3 A_0(m_{\tilde{e}_{L,a}}^2) \Gamma_{\check{\phi}^0_L, i, \tilde{e}_{L,a}^*, \tilde{e}_{L,a}} \\
& - \sum_{a=1}^3 A_0(m_{\tilde{e}_{R,a}}^2) \Gamma_{\check{\phi}^0_L, i, \tilde{e}_{R,a}^*, \tilde{e}_{R,a}} - 3 \sum_{a=1}^3 A_0(m_{\tilde{u}_{L,a}}^2) \Gamma_{\check{\phi}^0_L, i, \tilde{u}_{L,a}^*, \tilde{u}_{L,a}} \\
& - 3 \sum_{a=1}^3 A_0(m_{\tilde{u}_{R,a}}^2) \Gamma_{\check{\phi}^0_L, i, \tilde{u}_{R,a}^*, \tilde{u}_{R,a}} - \sum_{a=1}^3 A_0(m_{\tilde{\nu}_{L,a}}^2) \Gamma_{\check{\phi}^0_L, i, \tilde{\nu}_{L,a}^*, \tilde{\nu}_{L,a}}
\end{aligned}$$

$$\begin{aligned}
& - \sum_{a=1}^4 A_0(m_{\sigma_{L,a}^\pm}^2) \Gamma_{\check{\phi}^0_{L,i}, \sigma_{L,a}^{\pm,*}, \sigma_{L,a}^\pm} - \frac{1}{2} \sum_{a=1}^4 A_0(m_{\phi_{L,a}^0}^2) \Gamma_{\check{\phi}^0_{L,i}, \phi_{L,a}^0, \phi_{L,a}^0} \\
& - \frac{1}{2} \sum_{a=1}^4 A_0(m_{\sigma_{L,a}^0}^2) \Gamma_{\check{\phi}^0_{L,i}, \sigma_{L,a}^0, \sigma_{L,a}^0} + \sum_{a=1}^{10} A_0(m_{f_{Go,a}^-}^2) m_{f_{Go,a}^-}^2 \left( \Gamma_{\check{\phi}^0_{L,i}, f_{Go,a}^-, f_{Go,a}^-}^L + \Gamma_{\check{\phi}^0_{L,i}, f_{Go,a}^-, f_{Go,a}^-}^R \right) \\
& + \sum_{a=1}^{10} A_0(m_{f_{Po,a}^0}^2) m_{f_{Po,a}^0}^2 \left( \Gamma_{\check{\phi}^0_{L,i}, f_{Po,a}^0, f_{Po,a}^0}^L + \Gamma_{\check{\phi}^0_{L,i}, f_{Po,a}^0, f_{Po,a}^0}^R \right)
\end{aligned} \tag{382}$$

## 9 Interactions for eigenstates 'AxBSB'

### 9.1 Three Scalar-Interaction

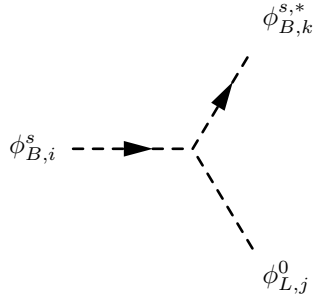

$$\begin{aligned}
& i v_{Lv} \left( B_{A,i1}^{s,*} \left( \left( -2|Y_A|^2 + g_{B2}^2 \right) Z_{Ls,j1}^{DR,*} - 2|Y_A|^2 Z_{Ls,j4}^{DR,*} - g_{B2}^2 Z_{Ls,j2}^{DR,*} - g_{B2}^2 Z_{Ls,j3}^{DR,*} + g_{B2}^2 Z_{Ls,j4}^{DR,*} \right) B_{A,k1}^s \right. \\
& \left. - B_{A,i2}^{s,*} \left( - \left( -2|Y_A|^2 + g_{B2}^2 \right) Z_{Ls,j2}^{DR,*} + 2|Y_A|^2 Z_{Ls,j3}^{DR,*} + g_{B2}^2 Z_{Ls,j1}^{DR,*} - g_{B2}^2 Z_{Ls,j3}^{DR,*} + g_{B2}^2 Z_{Ls,j4}^{DR,*} \right) B_{A,k2}^s \right)
\end{aligned} \tag{383}$$

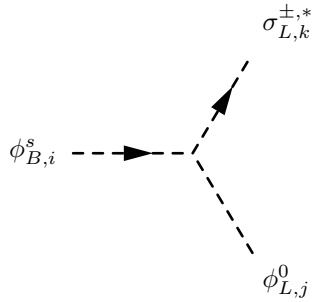

$$- i \left( B_{A,i1}^{s,*} T_A \left( Z_{Ls,j1}^{DR,*} Z_{Ls,k3}^{od} + Z_{Ls,j4}^{DR,*} Z_{Ls,k4}^{od} \right) + T_A^* B_{A,i2}^{s,*} \left( Z_{Ls,j2}^{DR,*} Z_{Ls,k1}^{od} + Z_{Ls,j3}^{DR,*} Z_{Ls,k2}^{od} \right) \right) \tag{384}$$

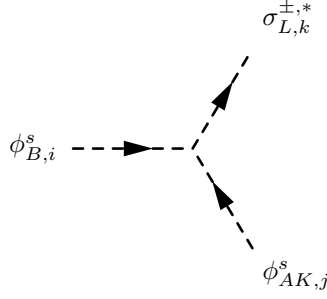

$$\begin{aligned}
& -\frac{i}{2}v_{Lv}B_{A,i2}^{s,*}\left(\sqrt{2}g_{B2}^2Z_{AK,j2}^{s,*}\left(-Z_{Ls,k1}^{od}-Z_{Ls,k4}^{od}+Z_{Ls,k2}^{od}+Z_{Ls,k3}^{od}\right)\right. \\
& \left.+Y_A^*\left(\sqrt{2}Y_AZ_{AK,j2}^{s,*}\left(-Z_{Ls,k2}^{od}-Z_{Ls,k3}^{od}+Z_{Ls,k1}^{od}+Z_{Ls,k4}^{od}\right)+Y_KZ_{AK,j1}^{s,*}\left(Z_{Ls,k1}^{od}+Z_{Ls,k2}^{od}+Z_{Ls,k3}^{od}+Z_{Ls,k4}^{od}\right)\right)\right)
\end{aligned} \tag{385}$$


---

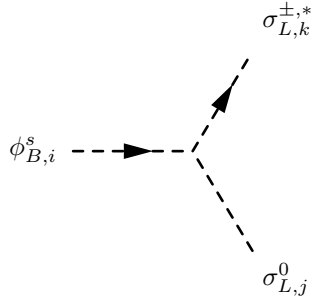

$$B_{A,i1}^{s,*}T_A\left(Z_{Ls,j1}^{Di,*}Z_{Ls,k3}^{od}+Z_{Ls,j4}^{Di,*}Z_{Ls,k4}^{od}\right)-T_A^*B_{A,i2}^{s,*}\left(Z_{Ls,j2}^{Di,*}Z_{Ls,k1}^{od}+Z_{Ls,j3}^{Di,*}Z_{Ls,k2}^{od}\right) \tag{386}$$


---

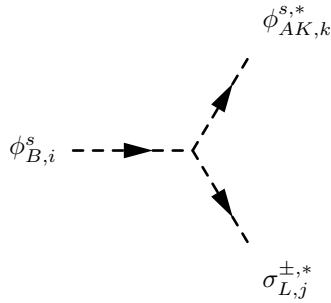

$$-\frac{i}{2}v_{Lv}B_{A,i1}^{s,*}\left(\sqrt{2}\left(-|Y_A|^2+g_{B2}^2\right)Z_{AK,k2}^s\left(-Z_{Ls,j2}^{od}-Z_{Ls,j3}^{od}+Z_{Ls,j1}^{od}+Z_{Ls,j4}^{od}\right)+Y_A Y_K^*Z_{AK,k1}^s\left(Z_{Ls,j1}^{od}+Z_{Ls,j2}^{od}+Z_{Ls,j3}^{od}+Z_{Ls,j4}^{od}\right)\right) \tag{387}$$


---

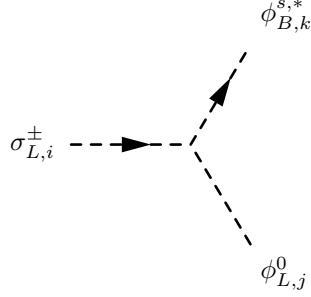

$$-i \left( T_A^* \left( Z_{Ls,i3}^{od,*} Z_{Ls,j1}^{DR,*} + Z_{Ls,i4}^{od,*} Z_{Ls,j4}^{DR,*} \right) B_{A,k1}^s + \left( Z_{Ls,i1}^{od,*} Z_{Ls,j2}^{DR,*} + Z_{Ls,i2}^{od,*} Z_{Ls,j3}^{DR,*} \right) T_A B_{A,k2}^s \right) \quad (388)$$

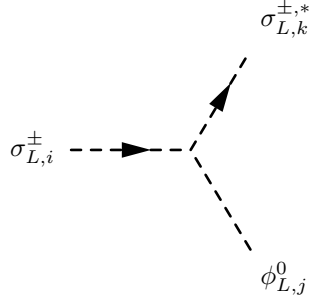

$$\begin{aligned} & -\frac{i}{4} v_{Lv} \left( -2g_{B2}^2 Z_{Ls,i3}^{od,*} Z_{Ls,j1}^{DR,*} Z_{Ls,k1}^{od} - 2|Y_A|^2 Z_{Ls,i3}^{od,*} Z_{Ls,j1}^{DR,*} Z_{Ls,k1}^{od} + |Y_K|^2 Z_{Ls,i3}^{od,*} Z_{Ls,j1}^{DR,*} Z_{Ls,k1}^{od} \right. \\ & + 2g_{A2}^2 Z_{Ls,i4}^{od,*} Z_{Ls,j1}^{DR,*} Z_{Ls,k1}^{od} + 2g_{B2}^2 Z_{Ls,i4}^{od,*} Z_{Ls,j1}^{DR,*} Z_{Ls,k1}^{od} - 2g_{B2}^2 Z_{Ls,i3}^{od,*} Z_{Ls,j2}^{DR,*} Z_{Ls,k1}^{od} \\ & - 2|Y_A|^2 Z_{Ls,i3}^{od,*} Z_{Ls,j2}^{DR,*} Z_{Ls,k1}^{od} + |Y_K|^2 Z_{Ls,i3}^{od,*} Z_{Ls,j2}^{DR,*} Z_{Ls,k1}^{od} - 2g_{A2}^2 Z_{Ls,i3}^{od,*} Z_{Ls,j3}^{DR,*} Z_{Ls,k1}^{od} \\ & + 2|Y_A|^2 Z_{Ls,i3}^{od,*} Z_{Ls,j3}^{DR,*} Z_{Ls,k1}^{od} + |Y_K|^2 Z_{Ls,i3}^{od,*} Z_{Ls,j3}^{DR,*} Z_{Ls,k1}^{od} + 2g_{A2}^2 Z_{Ls,i4}^{od,*} Z_{Ls,j3}^{DR,*} Z_{Ls,k1}^{od} \\ & + 2g_{B2}^2 Z_{Ls,i4}^{od,*} Z_{Ls,j3}^{DR,*} Z_{Ls,k1}^{od} - 2g_{A2}^2 Z_{Ls,i3}^{od,*} Z_{Ls,j4}^{DR,*} Z_{Ls,k1}^{od} + 2|Y_A|^2 Z_{Ls,i3}^{od,*} Z_{Ls,j4}^{DR,*} Z_{Ls,k1}^{od} \\ & + |Y_K|^2 Z_{Ls,i3}^{od,*} Z_{Ls,j4}^{DR,*} Z_{Ls,k1}^{od} - 2g_{A2}^2 Z_{Ls,i4}^{od,*} Z_{Ls,j1}^{DR,*} Z_{Ls,k2}^{od} + 2|Y_A|^2 Z_{Ls,i4}^{od,*} Z_{Ls,j1}^{DR,*} Z_{Ls,k2}^{od} \\ & + |Y_K|^2 Z_{Ls,i4}^{od,*} Z_{Ls,j1}^{DR,*} Z_{Ls,k2}^{od} + 2g_{A2}^2 Z_{Ls,i3}^{od,*} Z_{Ls,j2}^{DR,*} Z_{Ls,k2}^{od} + 2g_{B2}^2 Z_{Ls,i3}^{od,*} Z_{Ls,j2}^{DR,*} Z_{Ls,k2}^{od} \\ & - 2g_{A2}^2 Z_{Ls,i4}^{od,*} Z_{Ls,j2}^{DR,*} Z_{Ls,k2}^{od} + 2|Y_A|^2 Z_{Ls,i4}^{od,*} Z_{Ls,j2}^{DR,*} Z_{Ls,k2}^{od} + |Y_K|^2 Z_{Ls,i4}^{od,*} Z_{Ls,j2}^{DR,*} Z_{Ls,k2}^{od} \\ & - 2g_{B2}^2 Z_{Ls,i4}^{od,*} Z_{Ls,j3}^{DR,*} Z_{Ls,k2}^{od} - 2|Y_A|^2 Z_{Ls,i4}^{od,*} Z_{Ls,j3}^{DR,*} Z_{Ls,k2}^{od} + |Y_K|^2 Z_{Ls,i4}^{od,*} Z_{Ls,j3}^{DR,*} Z_{Ls,k2}^{od} \\ & + 2g_{A2}^2 Z_{Ls,i3}^{od,*} Z_{Ls,j4}^{DR,*} Z_{Ls,k2}^{od} + 2g_{B2}^2 Z_{Ls,i3}^{od,*} Z_{Ls,j4}^{DR,*} Z_{Ls,k2}^{od} - 2g_{B2}^2 Z_{Ls,i4}^{od,*} Z_{Ls,j4}^{DR,*} Z_{Ls,k2}^{od} \\ & - 2|Y_A|^2 Z_{Ls,i4}^{od,*} Z_{Ls,j4}^{DR,*} Z_{Ls,k2}^{od} + |Y_K|^2 Z_{Ls,i4}^{od,*} Z_{Ls,j4}^{DR,*} Z_{Ls,k2}^{od} - 2g_{A1}^2 Z_{Ls,i3}^{od,*} Z_{Ls,j1}^{DR,*} Z_{Ls,k3}^{od} \\ & - 2g_{A2}^2 Z_{Ls,i3}^{od,*} Z_{Ls,j1}^{DR,*} Z_{Ls,k3}^{od} - 2g_{B1}^2 Z_{Ls,i3}^{od,*} Z_{Ls,j1}^{DR,*} Z_{Ls,k3}^{od} + 2g_{B2}^2 Z_{Ls,i3}^{od,*} Z_{Ls,j1}^{DR,*} Z_{Ls,k3}^{od} \\ & + 8|Y_A|^2 Z_{Ls,i3}^{od,*} Z_{Ls,j1}^{DR,*} Z_{Ls,k3}^{od} - 2g_{A2}^2 Z_{Ls,i4}^{od,*} Z_{Ls,j1}^{DR,*} Z_{Ls,k3}^{od} + 4|Y_A|^2 Z_{Ls,i4}^{od,*} Z_{Ls,j1}^{DR,*} Z_{Ls,k3}^{od} \\ & + 2g_{A1}^2 Z_{Ls,i3}^{od,*} Z_{Ls,j2}^{DR,*} Z_{Ls,k3}^{od} + 2g_{A2}^2 Z_{Ls,i3}^{od,*} Z_{Ls,j2}^{DR,*} Z_{Ls,k3}^{od} + 2g_{B1}^2 Z_{Ls,i3}^{od,*} Z_{Ls,j2}^{DR,*} Z_{Ls,k3}^{od} \end{aligned}$$

$$\begin{aligned}
& + 2g_{B2}^2 Z_{Ls,i3}^{od,*} Z_{Ls,j2}^{DR,*} Z_{Ls,k3}^{od} - 2g_{B2}^2 Z_{Ls,i4}^{od,*} Z_{Ls,j2}^{DR,*} Z_{Ls,k3}^{od} - 2g_{A1}^2 Z_{Ls,i3}^{od,*} Z_{Ls,j3}^{DR,*} Z_{Ls,k3}^{od} \\
& + 2g_{A2}^2 Z_{Ls,i3}^{od,*} Z_{Ls,j3}^{DR,*} Z_{Ls,k3}^{od} - 2g_{B1}^2 Z_{Ls,i3}^{od,*} Z_{Ls,j3}^{DR,*} Z_{Ls,k3}^{od} - 2g_{B2}^2 Z_{Ls,i3}^{od,*} Z_{Ls,j3}^{DR,*} Z_{Ls,k3}^{od} \\
& - 2g_{B2}^2 Z_{Ls,i4}^{od,*} Z_{Ls,j3}^{DR,*} Z_{Ls,k3}^{od} + 2g_{A1}^2 Z_{Ls,i3}^{od,*} Z_{Ls,j4}^{DR,*} Z_{Ls,k3}^{od} + 2g_{A2}^2 Z_{Ls,i3}^{od,*} Z_{Ls,j4}^{DR,*} Z_{Ls,k3}^{od} \\
& + 2g_{B1}^2 Z_{Ls,i3}^{od,*} Z_{Ls,j4}^{DR,*} Z_{Ls,k3}^{od} + 2g_{B2}^2 Z_{Ls,i3}^{od,*} Z_{Ls,j4}^{DR,*} Z_{Ls,k3}^{od} - 2g_{A2}^2 Z_{Ls,i4}^{od,*} Z_{Ls,j4}^{DR,*} Z_{Ls,k3}^{od} \\
& + 4|Y_A|^2 Z_{Ls,i4}^{od,*} Z_{Ls,j4}^{DR,*} Z_{Ls,k3}^{od} - 2g_{A2}^2 Z_{Ls,i3}^{od,*} Z_{Ls,j1}^{DR,*} Z_{Ls,k4}^{od} + 4|Y_A|^2 Z_{Ls,i3}^{od,*} Z_{Ls,j1}^{DR,*} Z_{Ls,k4}^{od} \\
& + 2g_{A1}^2 Z_{Ls,i4}^{od,*} Z_{Ls,j1}^{DR,*} Z_{Ls,k4}^{od} + 2g_{A2}^2 Z_{Ls,i4}^{od,*} Z_{Ls,j1}^{DR,*} Z_{Ls,k4}^{od} + 2g_{B1}^2 Z_{Ls,i4}^{od,*} Z_{Ls,j1}^{DR,*} Z_{Ls,k4}^{od} \\
& + 2g_{B2}^2 Z_{Ls,i4}^{od,*} Z_{Ls,j1}^{DR,*} Z_{Ls,k4}^{od} - 2g_{B2}^2 Z_{Ls,i3}^{od,*} Z_{Ls,j2}^{DR,*} Z_{Ls,k4}^{od} - 2g_{A1}^2 Z_{Ls,i4}^{od,*} Z_{Ls,j2}^{DR,*} Z_{Ls,k4}^{od} \\
& + 2g_{A2}^2 Z_{Ls,i4}^{od,*} Z_{Ls,j2}^{DR,*} Z_{Ls,k4}^{od} - 2g_{B1}^2 Z_{Ls,i4}^{od,*} Z_{Ls,j2}^{DR,*} Z_{Ls,k4}^{od} - 2g_{B2}^2 Z_{Ls,i4}^{od,*} Z_{Ls,j2}^{DR,*} Z_{Ls,k4}^{od} \\
& - 2g_{B2}^2 Z_{Ls,i3}^{od,*} Z_{Ls,j3}^{DR,*} Z_{Ls,k4}^{od} + 2g_{A1}^2 Z_{Ls,i4}^{od,*} Z_{Ls,j3}^{DR,*} Z_{Ls,k4}^{od} + 2g_{A2}^2 Z_{Ls,i4}^{od,*} Z_{Ls,j3}^{DR,*} Z_{Ls,k4}^{od} \\
& + 2g_{B1}^2 Z_{Ls,i4}^{od,*} Z_{Ls,j3}^{DR,*} Z_{Ls,k4}^{od} + 2g_{B2}^2 Z_{Ls,i4}^{od,*} Z_{Ls,j3}^{DR,*} Z_{Ls,k4}^{od} - 2g_{A2}^2 Z_{Ls,i3}^{od,*} Z_{Ls,j4}^{DR,*} Z_{Ls,k4}^{od} \\
& + 4|Y_A|^2 Z_{Ls,i3}^{od,*} Z_{Ls,j4}^{DR,*} Z_{Ls,k4}^{od} - 2g_{A1}^2 Z_{Ls,i4}^{od,*} Z_{Ls,j4}^{DR,*} Z_{Ls,k4}^{od} - 2g_{A2}^2 Z_{Ls,i4}^{od,*} Z_{Ls,j4}^{DR,*} Z_{Ls,k4}^{od} \\
& - 2g_{B1}^2 Z_{Ls,i4}^{od,*} Z_{Ls,j4}^{DR,*} Z_{Ls,k4}^{od} + 2g_{B2}^2 Z_{Ls,i4}^{od,*} Z_{Ls,j4}^{DR,*} Z_{Ls,k4}^{od} + 8|Y_A|^2 Z_{Ls,i4}^{od,*} Z_{Ls,j4}^{DR,*} Z_{Ls,k4}^{od} \\
& + Z_{Ls,i1}^{od,*} \left( 2g_{A1}^2 Z_{Ls,j3}^{DR,*} Z_{Ls,k1}^{od} + 2g_{A2}^2 Z_{Ls,j3}^{DR,*} Z_{Ls,k1}^{od} + 2g_{B1}^2 Z_{Ls,j3}^{DR,*} Z_{Ls,k1}^{od} + 2g_{B2}^2 Z_{Ls,j3}^{DR,*} Z_{Ls,k1}^{od} \right. \\
& - 2g_{A1}^2 Z_{Ls,j4}^{DR,*} Z_{Ls,k1}^{od} + 2g_{A2}^2 Z_{Ls,j4}^{DR,*} Z_{Ls,k1}^{od} - 2g_{B1}^2 Z_{Ls,j4}^{DR,*} Z_{Ls,k1}^{od} - 2g_{B2}^2 Z_{Ls,j4}^{DR,*} Z_{Ls,k1}^{od} \\
& - 2g_{A2}^2 Z_{Ls,j3}^{DR,*} Z_{Ls,k2}^{od} + 4|Y_A|^2 Z_{Ls,j3}^{DR,*} Z_{Ls,k2}^{od} - 2g_{B2}^2 Z_{Ls,j4}^{DR,*} Z_{Ls,k2}^{od} - 2g_{A2}^2 Z_{Ls,j3}^{DR,*} Z_{Ls,k3}^{od} \\
& + 2|Y_A|^2 Z_{Ls,j3}^{DR,*} Z_{Ls,k3}^{od} + |Y_K|^2 Z_{Ls,j3}^{DR,*} Z_{Ls,k3}^{od} - 2g_{A2}^2 Z_{Ls,j4}^{DR,*} Z_{Ls,k3}^{od} + 2|Y_A|^2 Z_{Ls,j4}^{DR,*} Z_{Ls,k3}^{od} \\
& + |Y_K|^2 Z_{Ls,j4}^{DR,*} Z_{Ls,k3}^{od} \\
& + Z_{Ls,j2}^{DR,*} \left( -2 \left( -4|Y_A|^2 - g_{B2}^2 + g_{A1}^2 + g_{A2}^2 + g_{B1}^2 \right) Z_{Ls,k1}^{od} - 2 \left( -2|Y_A|^2 + g_{A2}^2 \right) Z_{Ls,k2}^{od} \right. \\
& + \left( -2g_{B2}^2 - 2|Y_A|^2 + |Y_K|^2 \right) Z_{Ls,k3}^{od} \Big) \\
& + 2g_{A2}^2 Z_{Ls,j3}^{DR,*} Z_{Ls,k4}^{od} + 2g_{B2}^2 Z_{Ls,j3}^{DR,*} Z_{Ls,k4}^{od} \\
& + Z_{Ls,j1}^{DR,*} \left( 2 \left( g_{A1}^2 + g_{A2}^2 + g_{B1}^2 + g_{B2}^2 \right) Z_{Ls,k1}^{od} - 2g_{B2}^2 Z_{Ls,k2}^{od} - 2g_{B2}^2 Z_{Ls,k3}^{od} - 2|Y_A|^2 Z_{Ls,k3}^{od} + |Y_K|^2 Z_{Ls,k3}^{od} \right. \\
& + 2g_{A2}^2 Z_{Ls,k4}^{od} + 2g_{B2}^2 Z_{Ls,k4}^{od} \Big) \\
& + Z_{Ls,i2}^{od,*} \left( -2g_{A2}^2 Z_{Ls,j3}^{DR,*} Z_{Ls,k1}^{od} + 4|Y_A|^2 Z_{Ls,j3}^{DR,*} Z_{Ls,k1}^{od} - 2g_{B2}^2 Z_{Ls,j4}^{DR,*} Z_{Ls,k1}^{od} - 2g_{A1}^2 Z_{Ls,j3}^{DR,*} Z_{Ls,k2}^{od} \right. \\
& - 2g_{A2}^2 Z_{Ls,j3}^{DR,*} Z_{Ls,k2}^{od} - 2g_{B1}^2 Z_{Ls,j3}^{DR,*} Z_{Ls,k2}^{od} + 2g_{B2}^2 Z_{Ls,j3}^{DR,*} Z_{Ls,k2}^{od} + 8|Y_A|^2 Z_{Ls,j3}^{DR,*} Z_{Ls,k2}^{od} \\
& + 2g_{A1}^2 Z_{Ls,j4}^{DR,*} Z_{Ls,k2}^{od} + 2g_{A2}^2 Z_{Ls,j4}^{DR,*} Z_{Ls,k2}^{od} + 2g_{B1}^2 Z_{Ls,j4}^{DR,*} Z_{Ls,k2}^{od} + 2g_{B2}^2 Z_{Ls,j4}^{DR,*} Z_{Ls,k2}^{od} \\
& + 2g_{A2}^2 Z_{Ls,j4}^{DR,*} Z_{Ls,k3}^{od} + 2g_{B2}^2 Z_{Ls,j4}^{DR,*} Z_{Ls,k3}^{od} - 2g_{B2}^2 Z_{Ls,j3}^{DR,*} Z_{Ls,k4}^{od} - 2|Y_A|^2 Z_{Ls,j3}^{DR,*} Z_{Ls,k4}^{od} \\
& + |Y_K|^2 Z_{Ls,j3}^{DR,*} Z_{Ls,k4}^{od} - 2g_{B2}^2 Z_{Ls,j4}^{DR,*} Z_{Ls,k4}^{od} - 2|Y_A|^2 Z_{Ls,j4}^{DR,*} Z_{Ls,k4}^{od} + |Y_K|^2 Z_{Ls,j4}^{DR,*} Z_{Ls,k4}^{od} \\
& + Z_{Ls,j2}^{DR,*} \left( -2 \left( -2|Y_A|^2 + g_{A2}^2 \right) Z_{Ls,k1}^{od} + 2 \left( g_{A1}^2 + g_{A2}^2 + g_{B1}^2 + g_{B2}^2 \right) Z_{Ls,k2}^{od} + 2g_{A2}^2 Z_{Ls,k3}^{od} + 2g_{B2}^2 Z_{Ls,k3}^{od} - 2g_{A2}^2 Z_{Ls,k4}^{od} \right. \\
& + 2|Y_A|^2 Z_{Ls,k4}^{od} + |Y_K|^2 Z_{Ls,k4}^{od} \Big)
\end{aligned}$$

$$+ Z_{Ls,j1}^{DR,*} \left( \left( -2g_{A2}^2 + 2|Y_A|^2 + |Y_K|^2 \right) Z_{Ls,k4}^{od} - 2 \left( -g_{A2}^2 + g_{A1}^2 + g_{B1}^2 + g_{B2}^2 \right) Z_{Ls,k2}^{od} - 2g_{B2}^2 Z_{Ls,k1}^{od} \right) \right) \quad (389)$$


---

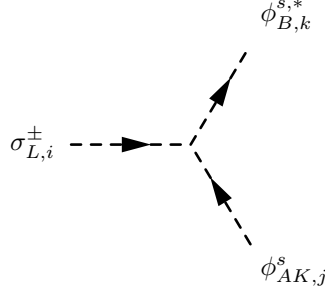

$$- \frac{i}{2} v_{Lv} \left( \sqrt{2} g_{B2}^2 Z_{AK,j2}^{s,*} \left( -Z_{Ls,i2}^{od,*} - Z_{Ls,i3}^{od,*} + Z_{Ls,i1}^{od,*} + Z_{Ls,i4}^{od,*} \right) \right. \\ \left. + Y_A^* \left( \sqrt{2} Y_A Z_{AK,j2}^{s,*} \left( -Z_{Ls,i1}^{od,*} - Z_{Ls,i4}^{od,*} + Z_{Ls,i2}^{od,*} + Z_{Ls,i3}^{od,*} \right) + Y_K Z_{AK,j1}^{s,*} \left( Z_{Ls,i1}^{od,*} + Z_{Ls,i2}^{od,*} + Z_{Ls,i3}^{od,*} + Z_{Ls,i4}^{od,*} \right) \right) \right) B_{A,k1}^s \quad (390)$$


---

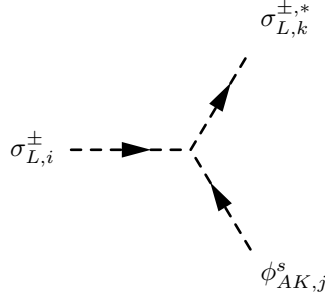

$$\frac{i}{2} \left( \sqrt{2} Z_{AK,j2}^{s,*} T_A \left( Z_{Ls,i1}^{od,*} Z_{Ls,k3}^{od} - Z_{Ls,i2}^{od,*} Z_{Ls,k4}^{od} \right) - Z_{AK,j1}^{s,*} T_K \left( Z_{Ls,i1}^{od,*} Z_{Ls,k3}^{od} + Z_{Ls,i2}^{od,*} Z_{Ls,k4}^{od} \right) \right) \quad (391)$$


---

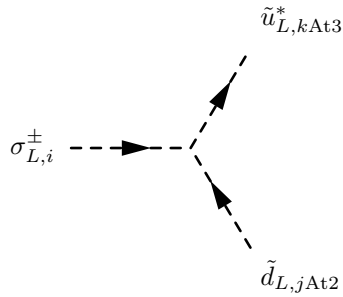

$$-\frac{i}{2}g_{A2}^2v_{Lv}\left(-Z_{Ls,i2}^{od,*}-Z_{Ls,i3}^{od,*}+Z_{Ls,i1}^{od,*}+Z_{Ls,i4}^{od,*}\right)\delta_{At2At3}\delta_{jk} \quad (392)$$


---

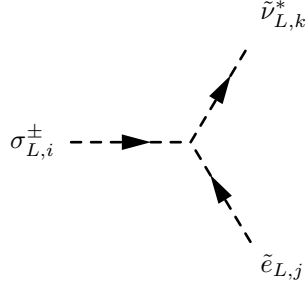

$$-\frac{i}{2}g_{A2}^2v_{Lv}\left(-Z_{Ls,i2}^{od,*}-Z_{Ls,i3}^{od,*}+Z_{Ls,i1}^{od,*}+Z_{Ls,i4}^{od,*}\right)\delta_{jk} \quad (393)$$


---

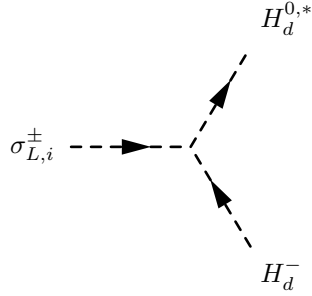

$$-\frac{i}{2}g_{A2}^2v_{Lv}\left(-Z_{Ls,i2}^{od,*}-Z_{Ls,i3}^{od,*}+Z_{Ls,i1}^{od,*}+Z_{Ls,i4}^{od,*}\right) \quad (394)$$


---

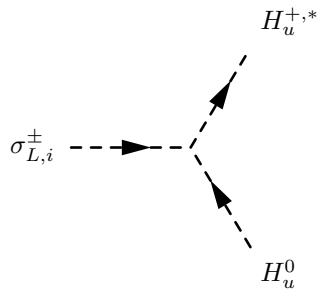

$$-\frac{i}{2}g_{A2}^2v_{Lv}\left(-Z_{Ls,i2}^{od,*}-Z_{Ls,i3}^{od,*}+Z_{Ls,i1}^{od,*}+Z_{Ls,i4}^{od,*}\right) \quad (395)$$


---



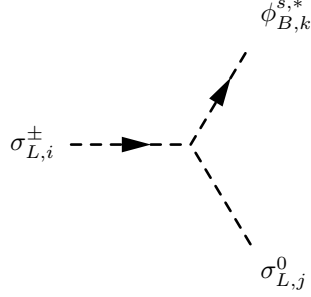

$$-T_A^* \left( Z_{Ls,i3}^{od,*} Z_{Ls,j1}^{Di,*} + Z_{Ls,i4}^{od,*} Z_{Ls,j4}^{Di,*} \right) B_{A,k1}^s + \left( Z_{Ls,i1}^{od,*} Z_{Ls,j2}^{Di,*} + Z_{Ls,i2}^{od,*} Z_{Ls,j3}^{Di,*} \right) T_A B_{A,k2}^s \quad (396)$$

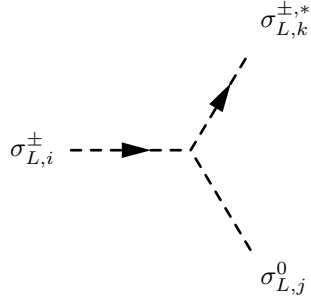

$$\begin{aligned} & \frac{1}{4} v_{Lv} \left( 2g_{A2}^2 Z_{Ls,i4}^{od,*} Z_{Ls,j1}^{Di,*} Z_{Ls,k1}^{od} + 2g_{B2}^2 Z_{Ls,i4}^{od,*} Z_{Ls,j1}^{Di,*} Z_{Ls,k1}^{od} + 2g_{A2}^2 Z_{Ls,i4}^{od,*} Z_{Ls,j3}^{Di,*} Z_{Ls,k1}^{od} \right. \\ & + 2g_{B2}^2 Z_{Ls,i4}^{od,*} Z_{Ls,j3}^{Di,*} Z_{Ls,k1}^{od} + 2g_{B2}^2 Z_{Ls,i1}^{od,*} Z_{Ls,j1}^{Di,*} Z_{Ls,k2}^{od} - 2g_{A2}^2 Z_{Ls,i4}^{od,*} Z_{Ls,j1}^{Di,*} Z_{Ls,k2}^{od} \\ & + 2|Y_A|^2 Z_{Ls,i4}^{od,*} Z_{Ls,j1}^{Di,*} Z_{Ls,k2}^{od} + |Y_K|^2 Z_{Ls,i4}^{od,*} Z_{Ls,j1}^{Di,*} Z_{Ls,k2}^{od} - 2g_{A2}^2 Z_{Ls,i1}^{od,*} Z_{Ls,j2}^{Di,*} Z_{Ls,k2}^{od} \\ & + 4|Y_A|^2 Z_{Ls,i1}^{od,*} Z_{Ls,j2}^{Di,*} Z_{Ls,k2}^{od} - 2g_{A2}^2 Z_{Ls,i4}^{od,*} Z_{Ls,j2}^{Di,*} Z_{Ls,k2}^{od} + 2|Y_A|^2 Z_{Ls,i4}^{od,*} Z_{Ls,j2}^{Di,*} Z_{Ls,k2}^{od} \\ & + |Y_K|^2 Z_{Ls,i4}^{od,*} Z_{Ls,j2}^{Di,*} Z_{Ls,k2}^{od} + 2g_{A2}^2 Z_{Ls,i1}^{od,*} Z_{Ls,j3}^{Di,*} Z_{Ls,k2}^{od} - 4|Y_A|^2 Z_{Ls,i1}^{od,*} Z_{Ls,j3}^{Di,*} Z_{Ls,k2}^{od} \\ & - 2g_{B2}^2 Z_{Ls,i4}^{od,*} Z_{Ls,j3}^{Di,*} Z_{Ls,k2}^{od} - 2|Y_A|^2 Z_{Ls,i4}^{od,*} Z_{Ls,j3}^{Di,*} Z_{Ls,k2}^{od} + |Y_K|^2 Z_{Ls,i4}^{od,*} Z_{Ls,j3}^{Di,*} Z_{Ls,k2}^{od} \\ & - 2g_{B2}^2 Z_{Ls,i1}^{od,*} Z_{Ls,j4}^{Di,*} Z_{Ls,k2}^{od} - 2g_{B2}^2 Z_{Ls,i4}^{od,*} Z_{Ls,j4}^{Di,*} Z_{Ls,k2}^{od} - 2|Y_A|^2 Z_{Ls,i4}^{od,*} Z_{Ls,j4}^{Di,*} Z_{Ls,k2}^{od} \\ & + |Y_K|^2 Z_{Ls,i4}^{od,*} Z_{Ls,j4}^{Di,*} Z_{Ls,k2}^{od} + 2g_{B2}^2 Z_{Ls,i1}^{od,*} Z_{Ls,j1}^{Di,*} Z_{Ls,k3}^{od} + 2|Y_A|^2 Z_{Ls,i1}^{od,*} Z_{Ls,j1}^{Di,*} Z_{Ls,k3}^{od} \\ & - |Y_K|^2 Z_{Ls,i1}^{od,*} Z_{Ls,j1}^{Di,*} Z_{Ls,k3}^{od} - 2g_{A2}^2 Z_{Ls,i4}^{od,*} Z_{Ls,j1}^{Di,*} Z_{Ls,k3}^{od} + 4|Y_A|^2 Z_{Ls,i4}^{od,*} Z_{Ls,j1}^{Di,*} Z_{Ls,k3}^{od} \\ & + 2g_{B2}^2 Z_{Ls,i1}^{od,*} Z_{Ls,j2}^{Di,*} Z_{Ls,k3}^{od} + 2|Y_A|^2 Z_{Ls,i1}^{od,*} Z_{Ls,j2}^{Di,*} Z_{Ls,k3}^{od} - |Y_K|^2 Z_{Ls,i1}^{od,*} Z_{Ls,j2}^{Di,*} Z_{Ls,k3}^{od} \\ & + 2g_{B2}^2 Z_{Ls,i4}^{od,*} Z_{Ls,j2}^{Di,*} Z_{Ls,k3}^{od} + 2g_{A2}^2 Z_{Ls,i1}^{od,*} Z_{Ls,j3}^{Di,*} Z_{Ls,k3}^{od} - 2|Y_A|^2 Z_{Ls,i1}^{od,*} Z_{Ls,j3}^{Di,*} Z_{Ls,k3}^{od} \\ & - |Y_K|^2 Z_{Ls,i1}^{od,*} Z_{Ls,j3}^{Di,*} Z_{Ls,k3}^{od} - 2g_{B2}^2 Z_{Ls,i4}^{od,*} Z_{Ls,j3}^{Di,*} Z_{Ls,k3}^{od} + 2g_{A2}^2 Z_{Ls,i1}^{od,*} Z_{Ls,j4}^{Di,*} Z_{Ls,k3}^{od} \\ & - 2|Y_A|^2 Z_{Ls,i1}^{od,*} Z_{Ls,j4}^{Di,*} Z_{Ls,k3}^{od} - |Y_K|^2 Z_{Ls,i1}^{od,*} Z_{Ls,j4}^{Di,*} Z_{Ls,k3}^{od} + 2g_{A2}^2 Z_{Ls,i4}^{od,*} Z_{Ls,j4}^{Di,*} Z_{Ls,k3}^{od} \\ & - 4|Y_A|^2 Z_{Ls,i4}^{od,*} Z_{Ls,j4}^{Di,*} Z_{Ls,k3}^{od} - 2g_{A2}^2 Z_{Ls,i1}^{od,*} Z_{Ls,j1}^{Di,*} Z_{Ls,k4}^{od} - 2g_{B2}^2 Z_{Ls,i1}^{od,*} Z_{Ls,j1}^{Di,*} Z_{Ls,k4}^{od} \end{aligned}$$

$$\begin{aligned}
& -2g_{A2}^2 Z_{Ls,i1}^{od,*} Z_{Ls,j3}^{Di,*} Z_{Ls,k4}^{od} - 2g_{B2}^2 Z_{Ls,i1}^{od,*} Z_{Ls,j3}^{Di,*} Z_{Ls,k4}^{od} \\
& - Z_{Ls,i2}^{od,*} \left( 2g_{A2}^2 Z_{Ls,j3}^{Di,*} Z_{Ls,k1}^{od} - 4|Y_A|^2 Z_{Ls,j3}^{Di,*} Z_{Ls,k1}^{od} - 2g_{B2}^2 Z_{Ls,j4}^{Di,*} Z_{Ls,k1}^{od} + 2g_{A2}^2 Z_{Ls,j4}^{Di,*} Z_{Ls,k3}^{od} \right. \\
& + 2g_{B2}^2 Z_{Ls,j4}^{Di,*} Z_{Ls,k3}^{od} - 2g_{B2}^2 Z_{Ls,j3}^{Di,*} Z_{Ls,k4}^{od} - 2|Y_A|^2 Z_{Ls,j3}^{Di,*} Z_{Ls,k4}^{od} + |Y_K|^2 Z_{Ls,j3}^{Di,*} Z_{Ls,k4}^{od} \\
& - 2g_{B2}^2 Z_{Ls,j4}^{Di,*} Z_{Ls,k4}^{od} - 2|Y_A|^2 Z_{Ls,j4}^{Di,*} Z_{Ls,k4}^{od} + |Y_K|^2 Z_{Ls,j4}^{Di,*} Z_{Ls,k4}^{od} \\
& + Z_{Ls,j1}^{Di,*} \left( \left( -2g_{A2}^2 + 2|Y_A|^2 + |Y_K|^2 \right) Z_{Ls,k4}^{od} + 2g_{B2}^2 Z_{Ls,k1}^{od} \right) \\
& + Z_{Ls,j2}^{Di,*} \left( -2 \left( -2|Y_A|^2 + g_{A2}^2 \right) Z_{Ls,k1}^{od} + \left( -2g_{A2}^2 + 2|Y_A|^2 + |Y_K|^2 \right) Z_{Ls,k4}^{od} + 2 \left( g_{A2}^2 + g_{B2}^2 \right) Z_{Ls,k3}^{od} \right) \\
& + Z_{Ls,i3}^{od,*} \left( -2g_{A2}^2 Z_{Ls,j3}^{Di,*} Z_{Ls,k1}^{od} + 2|Y_A|^2 Z_{Ls,j3}^{Di,*} Z_{Ls,k1}^{od} + |Y_K|^2 Z_{Ls,j3}^{Di,*} Z_{Ls,k1}^{od} - 2g_{A2}^2 Z_{Ls,j4}^{Di,*} Z_{Ls,k1}^{od} \right. \\
& + 2|Y_A|^2 Z_{Ls,j4}^{Di,*} Z_{Ls,k1}^{od} + |Y_K|^2 Z_{Ls,j4}^{Di,*} Z_{Ls,k1}^{od} + 2g_{A2}^2 Z_{Ls,j4}^{Di,*} Z_{Ls,k2}^{od} + 2g_{B2}^2 Z_{Ls,j4}^{Di,*} Z_{Ls,k2}^{od} \\
& + 2g_{B2}^2 Z_{Ls,j3}^{Di,*} Z_{Ls,k4}^{od} - 2g_{A2}^2 Z_{Ls,j4}^{Di,*} Z_{Ls,k4}^{od} + 4|Y_A|^2 Z_{Ls,j4}^{Di,*} Z_{Ls,k4}^{od} \\
& + Z_{Ls,j1}^{Di,*} \left( 2 \left( -2|Y_A|^2 + g_{A2}^2 \right) Z_{Ls,k4}^{od} + \left( -2g_{B2}^2 - 2|Y_A|^2 + |Y_K|^2 \right) Z_{Ls,k1}^{od} \right) \\
& \left. + Z_{Ls,j2}^{Di,*} \left( 2 \left( \left( g_{A2}^2 + g_{B2}^2 \right) Z_{Ls,k2}^{od} - g_{B2}^2 Z_{Ls,k4}^{od} \right) + \left( -2g_{B2}^2 - 2|Y_A|^2 + |Y_K|^2 \right) Z_{Ls,k1}^{od} \right) \right) \quad (397)
\end{aligned}$$


---

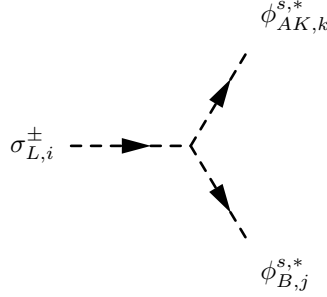

$$\begin{aligned}
& -\frac{i}{2} v_L \left( Y_A Y_K^* \left( Z_{Ls,i1}^{od,*} + Z_{Ls,i2}^{od,*} + Z_{Ls,i3}^{od,*} + Z_{Ls,i4}^{od,*} \right) Z_{AK,k1}^s \right. \\
& \left. - \sqrt{2} \left( -|Y_A|^2 + g_{B2}^2 \right) \left( -Z_{Ls,i2}^{od,*} - Z_{Ls,i3}^{od,*} + Z_{Ls,i1}^{od,*} + Z_{Ls,i4}^{od,*} \right) Z_{AK,k2}^s \right) B_{A,j2}^s \quad (398)
\end{aligned}$$


---

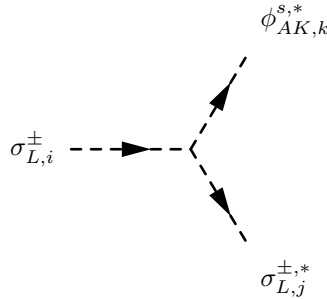

$$-\frac{i}{2}\left(\sqrt{2}T_A^*Z_{AK,k2}^s\left(-Z_{Ls,i3}^{od,*}Z_{Ls,j1}^{od}+Z_{Ls,i4}^{od,*}Z_{Ls,j2}^{od}\right)+T_K^*Z_{AK,k1}^s\left(Z_{Ls,i3}^{od,*}Z_{Ls,j1}^{od}+Z_{Ls,i4}^{od,*}Z_{Ls,j2}^{od}\right)\right) \quad (399)$$

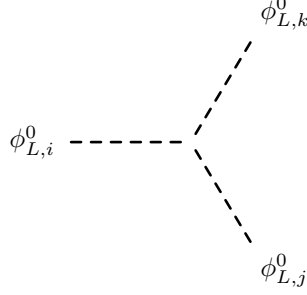

$$\begin{aligned} & -\frac{i}{2}v_{Lv}\left(2g_{A1}^2Z_{Ls,i3}^{DR,*}Z_{Ls,j1}^{DR,*}Z_{Ls,k1}^{DR,*}-2g_{A2}^2Z_{Ls,i3}^{DR,*}Z_{Ls,j1}^{DR,*}Z_{Ls,k1}^{DR,*}+2g_{B1}^2Z_{Ls,i3}^{DR,*}Z_{Ls,j1}^{DR,*}Z_{Ls,k1}^{DR,*}\right. \\ & -2g_{B2}^2Z_{Ls,i3}^{DR,*}Z_{Ls,j1}^{DR,*}Z_{Ls,k1}^{DR,*}-2g_{A1}^2Z_{Ls,i4}^{DR,*}Z_{Ls,j1}^{DR,*}Z_{Ls,k1}^{DR,*}+2g_{A2}^2Z_{Ls,i4}^{DR,*}Z_{Ls,j1}^{DR,*}Z_{Ls,k1}^{DR,*} \\ & -2g_{B1}^2Z_{Ls,i4}^{DR,*}Z_{Ls,j1}^{DR,*}Z_{Ls,k1}^{DR,*}+2g_{B2}^2Z_{Ls,i4}^{DR,*}Z_{Ls,j1}^{DR,*}Z_{Ls,k1}^{DR,*}-2|Y_A|^2Z_{Ls,i3}^{DR,*}Z_{Ls,j2}^{DR,*}Z_{Ls,k1}^{DR,*} \\ & +|Y_K|^2Z_{Ls,i3}^{DR,*}Z_{Ls,j2}^{DR,*}Z_{Ls,k1}^{DR,*}-2|Y_A|^2Z_{Ls,i4}^{DR,*}Z_{Ls,j2}^{DR,*}Z_{Ls,k1}^{DR,*}+|Y_K|^2Z_{Ls,i4}^{DR,*}Z_{Ls,j2}^{DR,*}Z_{Ls,k1}^{DR,*} \\ & +2g_{A1}^2Z_{Ls,i3}^{DR,*}Z_{Ls,j3}^{DR,*}Z_{Ls,k1}^{DR,*}-2g_{A2}^2Z_{Ls,i3}^{DR,*}Z_{Ls,j3}^{DR,*}Z_{Ls,k1}^{DR,*}+2g_{B1}^2Z_{Ls,i3}^{DR,*}Z_{Ls,j3}^{DR,*}Z_{Ls,k1}^{DR,*} \\ & -2g_{B2}^2Z_{Ls,i3}^{DR,*}Z_{Ls,j3}^{DR,*}Z_{Ls,k1}^{DR,*}-2|Y_A|^2Z_{Ls,i4}^{DR,*}Z_{Ls,j3}^{DR,*}Z_{Ls,k1}^{DR,*}+|Y_K|^2Z_{Ls,i4}^{DR,*}Z_{Ls,j3}^{DR,*}Z_{Ls,k1}^{DR,*} \\ & -2|Y_A|^2Z_{Ls,i3}^{DR,*}Z_{Ls,j4}^{DR,*}Z_{Ls,k1}^{DR,*}+|Y_K|^2Z_{Ls,i3}^{DR,*}Z_{Ls,j4}^{DR,*}Z_{Ls,k1}^{DR,*}-2g_{A1}^2Z_{Ls,i4}^{DR,*}Z_{Ls,j4}^{DR,*}Z_{Ls,k1}^{DR,*} \\ & +2g_{A2}^2Z_{Ls,i4}^{DR,*}Z_{Ls,j4}^{DR,*}Z_{Ls,k1}^{DR,*}-2g_{B1}^2Z_{Ls,i4}^{DR,*}Z_{Ls,j4}^{DR,*}Z_{Ls,k1}^{DR,*}+2g_{B2}^2Z_{Ls,i4}^{DR,*}Z_{Ls,j4}^{DR,*}Z_{Ls,k1}^{DR,*} \\ & -2|Y_A|^2Z_{Ls,i3}^{DR,*}Z_{Ls,j1}^{DR,*}Z_{Ls,k2}^{DR,*}+|Y_K|^2Z_{Ls,i3}^{DR,*}Z_{Ls,j1}^{DR,*}Z_{Ls,k2}^{DR,*}-2|Y_A|^2Z_{Ls,i4}^{DR,*}Z_{Ls,j1}^{DR,*}Z_{Ls,k2}^{DR,*} \\ & +|Y_K|^2Z_{Ls,i4}^{DR,*}Z_{Ls,j1}^{DR,*}Z_{Ls,k2}^{DR,*}-2g_{A1}^2Z_{Ls,i3}^{DR,*}Z_{Ls,j2}^{DR,*}Z_{Ls,k2}^{DR,*}+2g_{A2}^2Z_{Ls,i3}^{DR,*}Z_{Ls,j2}^{DR,*}Z_{Ls,k2}^{DR,*} \\ & -2g_{B1}^2Z_{Ls,i3}^{DR,*}Z_{Ls,j2}^{DR,*}Z_{Ls,k2}^{DR,*}+2g_{B2}^2Z_{Ls,i3}^{DR,*}Z_{Ls,j2}^{DR,*}Z_{Ls,k2}^{DR,*}-2g_{A1}^2Z_{Ls,i4}^{DR,*}Z_{Ls,j2}^{DR,*}Z_{Ls,k2}^{DR,*} \\ & +2g_{A2}^2Z_{Ls,i4}^{DR,*}Z_{Ls,j2}^{DR,*}Z_{Ls,k2}^{DR,*}-2g_{B1}^2Z_{Ls,i4}^{DR,*}Z_{Ls,j2}^{DR,*}Z_{Ls,k2}^{DR,*}+2g_{B2}^2Z_{Ls,i4}^{DR,*}Z_{Ls,j2}^{DR,*}Z_{Ls,k2}^{DR,*} \\ & -2g_{A1}^2Z_{Ls,i3}^{DR,*}Z_{Ls,j3}^{DR,*}Z_{Ls,k2}^{DR,*}+2g_{A2}^2Z_{Ls,i3}^{DR,*}Z_{Ls,j3}^{DR,*}Z_{Ls,k2}^{DR,*}-2g_{B1}^2Z_{Ls,i3}^{DR,*}Z_{Ls,j3}^{DR,*}Z_{Ls,k2}^{DR,*} \\ & +2g_{B2}^2Z_{Ls,i3}^{DR,*}Z_{Ls,j3}^{DR,*}Z_{Ls,k2}^{DR,*}-2|Y_A|^2Z_{Ls,i4}^{DR,*}Z_{Ls,j3}^{DR,*}Z_{Ls,k2}^{DR,*}+|Y_K|^2Z_{Ls,i4}^{DR,*}Z_{Ls,j3}^{DR,*}Z_{Ls,k2}^{DR,*} \\ & -2|Y_A|^2Z_{Ls,i3}^{DR,*}Z_{Ls,j4}^{DR,*}Z_{Ls,k2}^{DR,*}+|Y_K|^2Z_{Ls,i3}^{DR,*}Z_{Ls,j4}^{DR,*}Z_{Ls,k2}^{DR,*}+2g_{A1}^2Z_{Ls,i4}^{DR,*}Z_{Ls,j4}^{DR,*}Z_{Ls,k2}^{DR,*} \\ & -2g_{A2}^2Z_{Ls,i4}^{DR,*}Z_{Ls,j4}^{DR,*}Z_{Ls,k2}^{DR,*}+2g_{B1}^2Z_{Ls,i4}^{DR,*}Z_{Ls,j4}^{DR,*}Z_{Ls,k2}^{DR,*}-2g_{B2}^2Z_{Ls,i4}^{DR,*}Z_{Ls,j4}^{DR,*}Z_{Ls,k2}^{DR,*} \\ & +2g_{A1}^2Z_{Ls,i3}^{DR,*}Z_{Ls,j1}^{DR,*}Z_{Ls,k3}^{DR,*}-2g_{A2}^2Z_{Ls,i3}^{DR,*}Z_{Ls,j1}^{DR,*}Z_{Ls,k3}^{DR,*}+2g_{B1}^2Z_{Ls,i3}^{DR,*}Z_{Ls,j1}^{DR,*}Z_{Ls,k3}^{DR,*} \\ & -2g_{B2}^2Z_{Ls,i3}^{DR,*}Z_{Ls,j1}^{DR,*}Z_{Ls,k3}^{DR,*}-2|Y_A|^2Z_{Ls,i4}^{DR,*}Z_{Ls,j1}^{DR,*}Z_{Ls,k3}^{DR,*}+|Y_K|^2Z_{Ls,i4}^{DR,*}Z_{Ls,j1}^{DR,*}Z_{Ls,k3}^{DR,*} \\ & -2g_{A1}^2Z_{Ls,i3}^{DR,*}Z_{Ls,j2}^{DR,*}Z_{Ls,k3}^{DR,*}+2g_{A2}^2Z_{Ls,i3}^{DR,*}Z_{Ls,j2}^{DR,*}Z_{Ls,k3}^{DR,*}-2g_{B1}^2Z_{Ls,i3}^{DR,*}Z_{Ls,j2}^{DR,*}Z_{Ls,k3}^{DR,*} \\ & +2g_{B2}^2Z_{Ls,i3}^{DR,*}Z_{Ls,j2}^{DR,*}Z_{Ls,k3}^{DR,*}-2|Y_A|^2Z_{Ls,i4}^{DR,*}Z_{Ls,j2}^{DR,*}Z_{Ls,k3}^{DR,*}+|Y_K|^2Z_{Ls,i4}^{DR,*}Z_{Ls,j2}^{DR,*}Z_{Ls,k3}^{DR,*} \\ & +6g_{A1}^2Z_{Ls,i3}^{DR,*}Z_{Ls,j3}^{DR,*}Z_{Ls,k3}^{DR,*}+6g_{A2}^2Z_{Ls,i3}^{DR,*}Z_{Ls,j3}^{DR,*}Z_{Ls,k3}^{DR,*}+6g_{B1}^2Z_{Ls,i3}^{DR,*}Z_{Ls,j3}^{DR,*}Z_{Ls,k3}^{DR,*} \end{aligned}$$

$$\begin{aligned}
& + 6g_{B2}^2 Z_{Ls,i3}^{DR,*} Z_{Ls,j3}^{DR,*} Z_{Ls,k3}^{DR,*} - 2g_{A1}^2 Z_{Ls,i4}^{DR,*} Z_{Ls,j3}^{DR,*} Z_{Ls,k3}^{DR,*} - 2g_{A2}^2 Z_{Ls,i4}^{DR,*} Z_{Ls,j3}^{DR,*} Z_{Ls,k3}^{DR,*} \\
& - 2g_{B1}^2 Z_{Ls,i4}^{DR,*} Z_{Ls,j3}^{DR,*} Z_{Ls,k3}^{DR,*} - 2g_{B2}^2 Z_{Ls,i4}^{DR,*} Z_{Ls,j3}^{DR,*} Z_{Ls,k3}^{DR,*} + 4|Y_A|^2 Z_{Ls,i4}^{DR,*} Z_{Ls,j3}^{DR,*} Z_{Ls,k3}^{DR,*} \\
& + 2|Y_K|^2 Z_{Ls,i4}^{DR,*} Z_{Ls,j3}^{DR,*} Z_{Ls,k3}^{DR,*} - 2g_{A1}^2 Z_{Ls,i3}^{DR,*} Z_{Ls,j4}^{DR,*} Z_{Ls,k3}^{DR,*} - 2g_{A2}^2 Z_{Ls,i3}^{DR,*} Z_{Ls,j4}^{DR,*} Z_{Ls,k3}^{DR,*} \\
& - 2g_{B1}^2 Z_{Ls,i3}^{DR,*} Z_{Ls,j4}^{DR,*} Z_{Ls,k3}^{DR,*} - 2g_{B2}^2 Z_{Ls,i3}^{DR,*} Z_{Ls,j4}^{DR,*} Z_{Ls,k3}^{DR,*} + 4|Y_A|^2 Z_{Ls,i3}^{DR,*} Z_{Ls,j4}^{DR,*} Z_{Ls,k3}^{DR,*} \\
& + 2|Y_K|^2 Z_{Ls,i3}^{DR,*} Z_{Ls,j4}^{DR,*} Z_{Ls,k3}^{DR,*} - 2g_{A1}^2 Z_{Ls,i4}^{DR,*} Z_{Ls,j4}^{DR,*} Z_{Ls,k3}^{DR,*} - 2g_{A2}^2 Z_{Ls,i4}^{DR,*} Z_{Ls,j4}^{DR,*} Z_{Ls,k3}^{DR,*} \\
& - 2g_{B1}^2 Z_{Ls,i4}^{DR,*} Z_{Ls,j4}^{DR,*} Z_{Ls,k3}^{DR,*} - 2g_{B2}^2 Z_{Ls,i4}^{DR,*} Z_{Ls,j4}^{DR,*} Z_{Ls,k3}^{DR,*} + 4|Y_A|^2 Z_{Ls,i4}^{DR,*} Z_{Ls,j4}^{DR,*} Z_{Ls,k3}^{DR,*} \\
& + 2|Y_K|^2 Z_{Ls,i4}^{DR,*} Z_{Ls,j4}^{DR,*} Z_{Ls,k3}^{DR,*} - 2|Y_A|^2 Z_{Ls,i3}^{DR,*} Z_{Ls,j1}^{DR,*} Z_{Ls,k4}^{DR,*} + |Y_K|^2 Z_{Ls,i3}^{DR,*} Z_{Ls,j1}^{DR,*} Z_{Ls,k4}^{DR,*} \\
& - 2g_{A1}^2 Z_{Ls,i4}^{DR,*} Z_{Ls,j1}^{DR,*} Z_{Ls,k4}^{DR,*} + 2g_{A2}^2 Z_{Ls,i4}^{DR,*} Z_{Ls,j1}^{DR,*} Z_{Ls,k4}^{DR,*} - 2g_{B1}^2 Z_{Ls,i4}^{DR,*} Z_{Ls,j1}^{DR,*} Z_{Ls,k4}^{DR,*} \\
& + 2g_{B2}^2 Z_{Ls,i4}^{DR,*} Z_{Ls,j1}^{DR,*} Z_{Ls,k4}^{DR,*} - 2|Y_A|^2 Z_{Ls,i3}^{DR,*} Z_{Ls,j2}^{DR,*} Z_{Ls,k4}^{DR,*} + |Y_K|^2 Z_{Ls,i3}^{DR,*} Z_{Ls,j2}^{DR,*} Z_{Ls,k4}^{DR,*} \\
& + 2g_{A1}^2 Z_{Ls,i4}^{DR,*} Z_{Ls,j2}^{DR,*} Z_{Ls,k4}^{DR,*} - 2g_{A2}^2 Z_{Ls,i4}^{DR,*} Z_{Ls,j2}^{DR,*} Z_{Ls,k4}^{DR,*} + 2g_{B1}^2 Z_{Ls,i4}^{DR,*} Z_{Ls,j2}^{DR,*} Z_{Ls,k4}^{DR,*} \\
& - 2g_{B2}^2 Z_{Ls,i4}^{DR,*} Z_{Ls,j2}^{DR,*} Z_{Ls,k4}^{DR,*} - 2g_{A1}^2 Z_{Ls,i3}^{DR,*} Z_{Ls,j3}^{DR,*} Z_{Ls,k4}^{DR,*} - 2g_{A2}^2 Z_{Ls,i3}^{DR,*} Z_{Ls,j3}^{DR,*} Z_{Ls,k4}^{DR,*} \\
& - 2g_{B1}^2 Z_{Ls,i3}^{DR,*} Z_{Ls,j3}^{DR,*} Z_{Ls,k4}^{DR,*} - 2g_{B2}^2 Z_{Ls,i3}^{DR,*} Z_{Ls,j3}^{DR,*} Z_{Ls,k4}^{DR,*} + 4|Y_A|^2 Z_{Ls,i3}^{DR,*} Z_{Ls,j3}^{DR,*} Z_{Ls,k4}^{DR,*} \\
& + 2|Y_K|^2 Z_{Ls,i3}^{DR,*} Z_{Ls,j3}^{DR,*} Z_{Ls,k4}^{DR,*} - 2g_{A1}^2 Z_{Ls,i4}^{DR,*} Z_{Ls,j3}^{DR,*} Z_{Ls,k4}^{DR,*} - 2g_{A2}^2 Z_{Ls,i4}^{DR,*} Z_{Ls,j3}^{DR,*} Z_{Ls,k4}^{DR,*} \\
& - 2g_{B1}^2 Z_{Ls,i4}^{DR,*} Z_{Ls,j3}^{DR,*} Z_{Ls,k4}^{DR,*} - 2g_{B2}^2 Z_{Ls,i4}^{DR,*} Z_{Ls,j3}^{DR,*} Z_{Ls,k4}^{DR,*} + 4|Y_A|^2 Z_{Ls,i4}^{DR,*} Z_{Ls,j3}^{DR,*} Z_{Ls,k4}^{DR,*} \\
& + 2|Y_K|^2 Z_{Ls,i4}^{DR,*} Z_{Ls,j3}^{DR,*} Z_{Ls,k4}^{DR,*} - 2g_{A1}^2 Z_{Ls,i3}^{DR,*} Z_{Ls,j4}^{DR,*} Z_{Ls,k4}^{DR,*} - 2g_{A2}^2 Z_{Ls,i3}^{DR,*} Z_{Ls,j4}^{DR,*} Z_{Ls,k4}^{DR,*} \\
& - 2g_{B1}^2 Z_{Ls,i3}^{DR,*} Z_{Ls,j4}^{DR,*} Z_{Ls,k4}^{DR,*} - 2g_{B2}^2 Z_{Ls,i3}^{DR,*} Z_{Ls,j4}^{DR,*} Z_{Ls,k4}^{DR,*} + 4|Y_A|^2 Z_{Ls,i3}^{DR,*} Z_{Ls,j4}^{DR,*} Z_{Ls,k4}^{DR,*} \\
& + 2|Y_K|^2 Z_{Ls,i3}^{DR,*} Z_{Ls,j4}^{DR,*} Z_{Ls,k4}^{DR,*} + 6g_{A1}^2 Z_{Ls,i4}^{DR,*} Z_{Ls,j4}^{DR,*} Z_{Ls,k4}^{DR,*} + 6g_{A2}^2 Z_{Ls,i4}^{DR,*} Z_{Ls,j4}^{DR,*} Z_{Ls,k4}^{DR,*} \\
& + 6g_{B1}^2 Z_{Ls,i4}^{DR,*} Z_{Ls,j4}^{DR,*} Z_{Ls,k4}^{DR,*} + 6g_{B2}^2 Z_{Ls,i4}^{DR,*} Z_{Ls,j4}^{DR,*} Z_{Ls,k4}^{DR,*} \\
& + Z_{Ls,i2}^{DR,*} \left( -2|Y_A|^2 Z_{Ls,j3}^{DR,*} Z_{Ls,k1}^{DR,*} + |Y_K|^2 Z_{Ls,j3}^{DR,*} Z_{Ls,k1}^{DR,*} - 2|Y_A|^2 Z_{Ls,j4}^{DR,*} Z_{Ls,k1}^{DR,*} + |Y_K|^2 Z_{Ls,j4}^{DR,*} Z_{Ls,k1}^{DR,*} \right. \\
& - 2g_{A1}^2 Z_{Ls,j3}^{DR,*} Z_{Ls,k2}^{DR,*} + 2g_{A2}^2 Z_{Ls,j3}^{DR,*} Z_{Ls,k2}^{DR,*} - 2g_{B1}^2 Z_{Ls,j3}^{DR,*} Z_{Ls,k2}^{DR,*} + 2g_{B2}^2 Z_{Ls,j3}^{DR,*} Z_{Ls,k2}^{DR,*} \\
& + 2g_{A1}^2 Z_{Ls,j4}^{DR,*} Z_{Ls,k2}^{DR,*} - 2g_{A2}^2 Z_{Ls,j4}^{DR,*} Z_{Ls,k2}^{DR,*} + 2g_{B1}^2 Z_{Ls,j4}^{DR,*} Z_{Ls,k2}^{DR,*} - 2g_{B2}^2 Z_{Ls,j4}^{DR,*} Z_{Ls,k2}^{DR,*} \\
& - 2g_{A1}^2 Z_{Ls,j3}^{DR,*} Z_{Ls,k3}^{DR,*} + 2g_{A2}^2 Z_{Ls,j3}^{DR,*} Z_{Ls,k3}^{DR,*} - 2g_{B1}^2 Z_{Ls,j3}^{DR,*} Z_{Ls,k3}^{DR,*} + 2g_{B2}^2 Z_{Ls,j3}^{DR,*} Z_{Ls,k3}^{DR,*} \\
& \left. - 2|Y_A|^2 Z_{Ls,j4}^{DR,*} Z_{Ls,k3}^{DR,*} + |Y_K|^2 Z_{Ls,j4}^{DR,*} Z_{Ls,k3}^{DR,*} \right) \\
& - 2Z_{Ls,j2}^{DR,*} \left( \left( -2|Y_A|^2 - |Y_K|^2 + g_{A1}^2 + g_{A2}^2 + g_{B1}^2 + g_{B2}^2 \right) Z_{Ls,k1}^{DR,*} - 3 \left( g_{A1}^2 + g_{A2}^2 + g_{B1}^2 + g_{B2}^2 \right) Z_{Ls,k2}^{DR,*} \right. \\
& + \left( -g_{A2}^2 - g_{B2}^2 + g_{A1}^2 + g_{B1}^2 \right) \left( -Z_{Ls,k4}^{DR,*} + Z_{Ls,k3}^{DR,*} \right) \\
& - 2|Y_A|^2 Z_{Ls,j3}^{DR,*} Z_{Ls,k4}^{DR,*} + |Y_K|^2 Z_{Ls,j3}^{DR,*} Z_{Ls,k4}^{DR,*} + 2g_{A1}^2 Z_{Ls,j4}^{DR,*} Z_{Ls,k4}^{DR,*} - 2g_{A2}^2 Z_{Ls,j4}^{DR,*} Z_{Ls,k4}^{DR,*} \\
& + 2g_{B1}^2 Z_{Ls,j4}^{DR,*} Z_{Ls,k4}^{DR,*} - 2g_{B2}^2 Z_{Ls,j4}^{DR,*} Z_{Ls,k4}^{DR,*} \\
& \left. - Z_{Ls,j1}^{DR,*} \left( 2 \left( -2|Y_A|^2 - |Y_K|^2 + g_{A1}^2 + g_{A2}^2 + g_{B1}^2 + g_{B2}^2 \right) Z_{Ls,k1}^{DR,*} \right. \right. \\
& \left. \left. + 2 \left( -2|Y_A|^2 - |Y_K|^2 + g_{A1}^2 + g_{A2}^2 + g_{B1}^2 + g_{B2}^2 \right) Z_{Ls,k2}^{DR,*} + \left( 2|Y_A|^2 - |Y_K|^2 \right) \left( Z_{Ls,k3}^{DR,*} + Z_{Ls,k4}^{DR,*} \right) \right) \right)
\end{aligned}$$

$$\begin{aligned}
& + Z_{Ls,i1}^{DR,*} \left( 2g_{A1}^2 Z_{Ls,j3}^{DR,*} Z_{Ls,k1}^{DR,*} - 2g_{A2}^2 Z_{Ls,j3}^{DR,*} Z_{Ls,k1}^{DR,*} + 2g_{B1}^2 Z_{Ls,j3}^{DR,*} Z_{Ls,k1}^{DR,*} - 2g_{B2}^2 Z_{Ls,j3}^{DR,*} Z_{Ls,k1}^{DR,*} \right. \\
& - 2g_{A1}^2 Z_{Ls,j4}^{DR,*} Z_{Ls,k1}^{DR,*} + 2g_{A2}^2 Z_{Ls,j4}^{DR,*} Z_{Ls,k1}^{DR,*} - 2g_{B1}^2 Z_{Ls,j4}^{DR,*} Z_{Ls,k1}^{DR,*} + 2g_{B2}^2 Z_{Ls,j4}^{DR,*} Z_{Ls,k1}^{DR,*} \\
& - 2|Y_A|^2 Z_{Ls,j3}^{DR,*} Z_{Ls,k2}^{DR,*} + |Y_K|^2 Z_{Ls,j3}^{DR,*} Z_{Ls,k2}^{DR,*} - 2|Y_A|^2 Z_{Ls,j4}^{DR,*} Z_{Ls,k2}^{DR,*} + |Y_K|^2 Z_{Ls,j4}^{DR,*} Z_{Ls,k2}^{DR,*} \\
& + 2g_{A1}^2 Z_{Ls,j3}^{DR,*} Z_{Ls,k3}^{DR,*} - 2g_{A2}^2 Z_{Ls,j3}^{DR,*} Z_{Ls,k3}^{DR,*} + 2g_{B1}^2 Z_{Ls,j3}^{DR,*} Z_{Ls,k3}^{DR,*} - 2g_{B2}^2 Z_{Ls,j3}^{DR,*} Z_{Ls,k3}^{DR,*} \\
& - 2|Y_A|^2 Z_{Ls,j4}^{DR,*} Z_{Ls,k3}^{DR,*} + |Y_K|^2 Z_{Ls,j4}^{DR,*} Z_{Ls,k3}^{DR,*} \\
& + 2Z_{Ls,j1}^{DR,*} \left( 3 \left( g_{A1}^2 + g_{A2}^2 + g_{B1}^2 + g_{B2}^2 \right) Z_{Ls,k1}^{DR,*} - \left( -2|Y_A|^2 - |Y_K|^2 + g_{A1}^2 + g_{A2}^2 + g_{B1}^2 + g_{B2}^2 \right) Z_{Ls,k2}^{DR,*} \right. \\
& + \left( -g_{A2}^2 - g_{B2}^2 + g_{A1}^2 + g_{B1}^2 \right) \left( -Z_{Ls,k4}^{DR,*} + Z_{Ls,k3}^{DR,*} \right) \\
& - 2|Y_A|^2 Z_{Ls,j3}^{DR,*} Z_{Ls,k4}^{DR,*} + |Y_K|^2 Z_{Ls,j3}^{DR,*} Z_{Ls,k4}^{DR,*} - 2g_{A1}^2 Z_{Ls,j4}^{DR,*} Z_{Ls,k4}^{DR,*} + 2g_{A2}^2 Z_{Ls,j4}^{DR,*} Z_{Ls,k4}^{DR,*} \\
& - 2g_{B1}^2 Z_{Ls,j4}^{DR,*} Z_{Ls,k4}^{DR,*} + 2g_{B2}^2 Z_{Ls,j4}^{DR,*} Z_{Ls,k4}^{DR,*} \\
& - Z_{Ls,j2}^{DR,*} \left( 2 \left( -2|Y_A|^2 - |Y_K|^2 + g_{A1}^2 + g_{A2}^2 + g_{B1}^2 + g_{B2}^2 \right) Z_{Ls,k1}^{DR,*} \right. \\
& \left. \left. + 2 \left( -2|Y_A|^2 - |Y_K|^2 + g_{A1}^2 + g_{A2}^2 + g_{B1}^2 + g_{B2}^2 \right) Z_{Ls,k2}^{DR,*} + \left( 2|Y_A|^2 - |Y_K|^2 \right) \left( Z_{Ls,k3}^{DR,*} + Z_{Ls,k4}^{DR,*} \right) \right) \right) \quad (400)
\end{aligned}$$


---

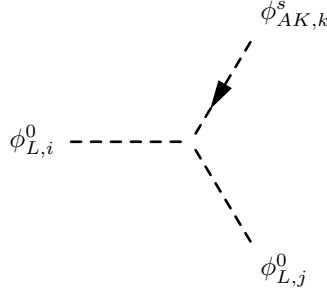

$$\begin{aligned}
& - \frac{i}{2} \left( \sqrt{2} Z_{AK,k2}^{s,*} \left( Z_{Ls,i1}^{DR,*} Z_{Ls,j2}^{DR,*} + Z_{Ls,i2}^{DR,*} Z_{Ls,j1}^{DR,*} - Z_{Ls,i3}^{DR,*} Z_{Ls,j4}^{DR,*} - Z_{Ls,i4}^{DR,*} Z_{Ls,j3}^{DR,*} \right) T_A \right. \\
& \left. + Z_{AK,k1}^{s,*} \left( Z_{Ls,i1}^{DR,*} Z_{Ls,j2}^{DR,*} + Z_{Ls,i2}^{DR,*} Z_{Ls,j1}^{DR,*} + Z_{Ls,i3}^{DR,*} Z_{Ls,j4}^{DR,*} + Z_{Ls,i4}^{DR,*} Z_{Ls,j3}^{DR,*} \right) T_K \right) \quad (401)
\end{aligned}$$


---

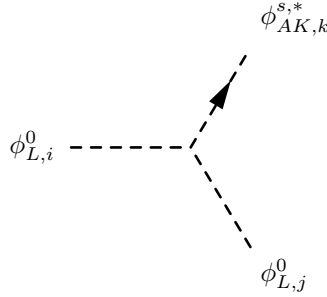

$$\begin{aligned}
& -\frac{i}{2} \left( T_K^* \left( Z_{Ls,i1}^{DR,*} Z_{Ls,j2}^{DR,*} + Z_{Ls,i2}^{DR,*} Z_{Ls,j1}^{DR,*} + Z_{Ls,i3}^{DR,*} Z_{Ls,j4}^{DR,*} + Z_{Ls,i4}^{DR,*} Z_{Ls,j3}^{DR,*} \right) Z_{AK,k1}^s \right. \\
& \left. + \sqrt{2} T_A^* \left( Z_{Ls,i1}^{DR,*} Z_{Ls,j2}^{DR,*} + Z_{Ls,i2}^{DR,*} Z_{Ls,j1}^{DR,*} - Z_{Ls,i3}^{DR,*} Z_{Ls,j4}^{DR,*} - Z_{Ls,i4}^{DR,*} Z_{Ls,j3}^{DR,*} \right) Z_{AK,k2}^s \right)
\end{aligned} \tag{402}$$


---

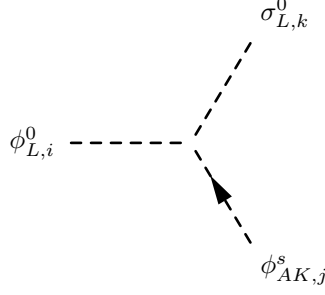

$$\begin{aligned}
& \frac{1}{2} \left( \sqrt{2} Z_{AK,j2}^{s,*} \left( Z_{Ls,i1}^{DR,*} Z_{Ls,k2}^{Di,*} + Z_{Ls,i2}^{DR,*} Z_{Ls,k1}^{Di,*} - Z_{Ls,i3}^{DR,*} Z_{Ls,k4}^{Di,*} - Z_{Ls,i4}^{DR,*} Z_{Ls,k3}^{Di,*} \right) T_A \right. \\
& \left. + Z_{AK,j1}^{s,*} \left( Z_{Ls,i1}^{DR,*} Z_{Ls,k2}^{Di,*} + Z_{Ls,i2}^{DR,*} Z_{Ls,k1}^{Di,*} + Z_{Ls,i3}^{DR,*} Z_{Ls,k4}^{Di,*} + Z_{Ls,i4}^{DR,*} Z_{Ls,k3}^{Di,*} \right) T_K \right)
\end{aligned} \tag{403}$$


---

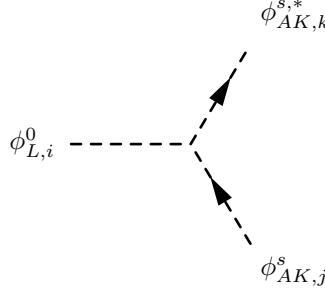

$$\begin{aligned}
& -\frac{i}{2} v_{Lv} \left( Y_K^* \left( \sqrt{2} Y_A Z_{AK,j2}^{s,*} \left( -Z_{Ls,i3}^{DR,*} - Z_{Ls,i4}^{DR,*} + Z_{Ls,i1}^{DR,*} + Z_{Ls,i2}^{DR,*} \right) + Y_K Z_{AK,j1}^{s,*} \left( Z_{Ls,i1}^{DR,*} + Z_{Ls,i2}^{DR,*} + Z_{Ls,i3}^{DR,*} + Z_{Ls,i4}^{DR,*} \right) \right) Z_{AK,k1}^s \right. \\
& \left. + Y_A^* \left( 2 Y_A Z_{AK,j2}^{s,*} \left( Z_{Ls,i1}^{DR,*} + Z_{Ls,i2}^{DR,*} + Z_{Ls,i3}^{DR,*} + Z_{Ls,i4}^{DR,*} \right) + \sqrt{2} Y_K Z_{AK,j1}^{s,*} \left( -Z_{Ls,i3}^{DR,*} - Z_{Ls,i4}^{DR,*} + Z_{Ls,i1}^{DR,*} + Z_{Ls,i2}^{DR,*} \right) \right) Z_{AK,k2}^s \right)
\end{aligned} \tag{404}$$


---

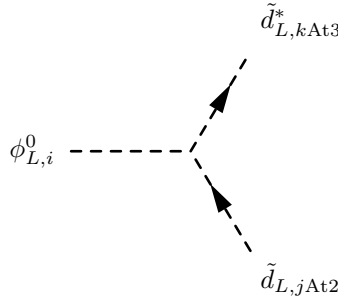

$$\frac{i}{6}v_{Lv}\left(\left(3g_{A2}^2+g_{A1}^2\right)Z_{Ls,i1}^{DR,*}-\left(3g_{A2}^2+g_{A1}^2\right)Z_{Ls,i2}^{DR,*}+\left(-3g_{A2}^2+g_{A1}^2\right)\left(-Z_{Ls,i4}^{DR,*}+Z_{Ls,i3}^{DR,*}\right)\right)\delta_{\text{At2At3}}\delta_{jk} \quad (405)$$


---

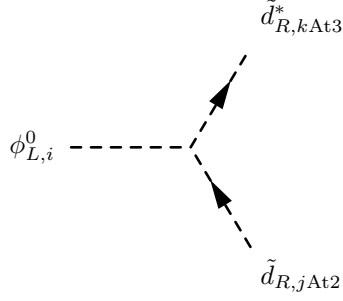

$$\frac{i}{3}g_{A1}^2v_{Lv}\left(-Z_{Ls,i2}^{DR,*}-Z_{Ls,i4}^{DR,*}+Z_{Ls,i1}^{DR,*}+Z_{Ls,i3}^{DR,*}\right)\delta_{\text{At2At3}}\delta_{jk} \quad (406)$$


---

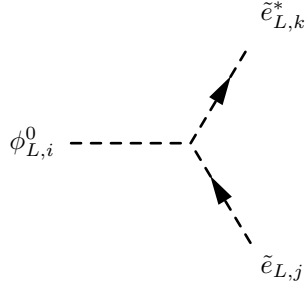

$$-\frac{i}{2}v_{Lv}\left(\left(-g_{A1}^2+g_{A2}^2\right)Z_{Ls,i2}^{DR,*}+\left(g_{A1}^2+g_{A2}^2\right)\left(-Z_{Ls,i4}^{DR,*}+Z_{Ls,i3}^{DR,*}\right)+\left(-g_{A2}^2+g_{A1}^2\right)Z_{Ls,i1}^{DR,*}\right)\delta_{jk} \quad (407)$$


---

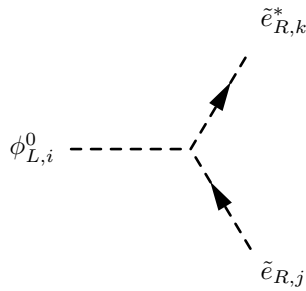

$$ig_{A1}^2v_{Lv}\left(-Z_{Ls,i2}^{DR,*}-Z_{Ls,i4}^{DR,*}+Z_{Ls,i1}^{DR,*}+Z_{Ls,i3}^{DR,*}\right)\delta_{jk} \quad (408)$$


---

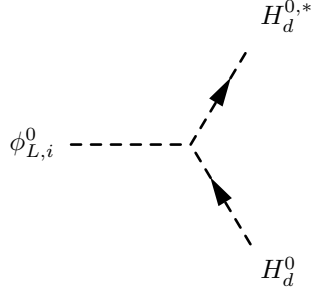

$$-\frac{i}{2}v_{Lv}\left(\left(g_{A1}^2+g_{A2}^2\right)Z_{Ls,i1}^{DR,*}-\left(g_{A1}^2+g_{A2}^2\right)Z_{Ls,i2}^{DR,*}+\left(-g_{A2}^2+g_{A1}^2\right)\left(-Z_{Ls,i4}^{DR,*}+Z_{Ls,i3}^{DR,*}\right)\right) \quad (409)$$


---

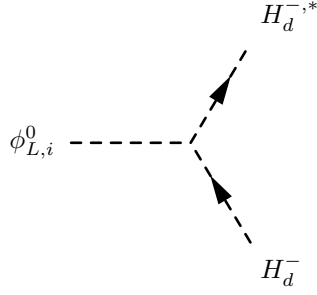

$$-\frac{i}{2}v_{Lv}\left(\left(-g_{A1}^2+g_{A2}^2\right)Z_{Ls,i2}^{DR,*}+\left(g_{A1}^2+g_{A2}^2\right)\left(-Z_{Ls,i4}^{DR,*}+Z_{Ls,i3}^{DR,*}\right)+\left(-g_{A2}^2+g_{A1}^2\right)Z_{Ls,i1}^{DR,*}\right) \quad (410)$$


---

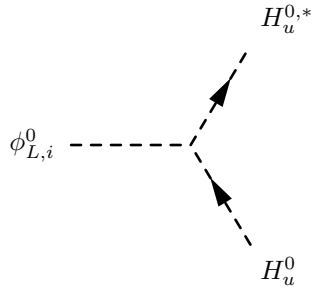

$$\frac{i}{2}v_{Lv}\left(\left(g_{A1}^2+g_{A2}^2\right)Z_{Ls,i1}^{DR,*}-\left(g_{A1}^2+g_{A2}^2\right)Z_{Ls,i2}^{DR,*}+\left(-g_{A2}^2+g_{A1}^2\right)\left(-Z_{Ls,i4}^{DR,*}+Z_{Ls,i3}^{DR,*}\right)\right) \quad (411)$$


---



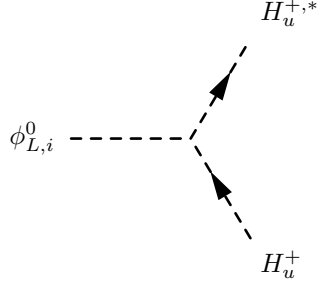

$$\frac{i}{2} v_{Lv} \left( \left( -g_{A1}^2 + g_{A2}^2 \right) Z_{Ls,i2}^{DR,*} + \left( g_{A1}^2 + g_{A2}^2 \right) \left( -Z_{Ls,i4}^{DR,*} + Z_{Ls,i3}^{DR,*} \right) + \left( -g_{A2}^2 + g_{A1}^2 \right) Z_{Ls,i1}^{DR,*} \right) \quad (412)$$

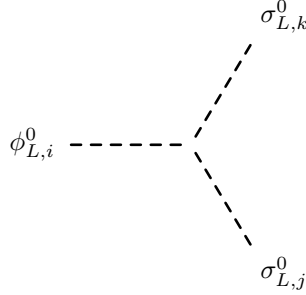

$$\begin{aligned} & -\frac{i}{2} v_{Lv} \left( 2g_{A1}^2 Z_{Ls,i3}^{DR,*} Z_{Ls,j1}^{Di,*} Z_{Ls,k1}^{Di,*} - 2g_{A2}^2 Z_{Ls,i3}^{DR,*} Z_{Ls,j1}^{Di,*} Z_{Ls,k1}^{Di,*} + 2g_{B1}^2 Z_{Ls,i3}^{DR,*} Z_{Ls,j1}^{Di,*} Z_{Ls,k1}^{Di,*} \right. \\ & - 2g_{B2}^2 Z_{Ls,i3}^{DR,*} Z_{Ls,j1}^{Di,*} Z_{Ls,k1}^{Di,*} - 2g_{A1}^2 Z_{Ls,i4}^{DR,*} Z_{Ls,j1}^{Di,*} Z_{Ls,k1}^{Di,*} + 2g_{A2}^2 Z_{Ls,i4}^{DR,*} Z_{Ls,j1}^{Di,*} Z_{Ls,k1}^{Di,*} \\ & - 2g_{B1}^2 Z_{Ls,i4}^{DR,*} Z_{Ls,j1}^{Di,*} Z_{Ls,k1}^{Di,*} + 2g_{B2}^2 Z_{Ls,i4}^{DR,*} Z_{Ls,j1}^{Di,*} Z_{Ls,k1}^{Di,*} + 2|Y_A|^2 Z_{Ls,i3}^{DR,*} Z_{Ls,j2}^{Di,*} Z_{Ls,k1}^{Di,*} \\ & - |Y_K|^2 Z_{Ls,i3}^{DR,*} Z_{Ls,j2}^{Di,*} Z_{Ls,k1}^{Di,*} + 2|Y_A|^2 Z_{Ls,i4}^{DR,*} Z_{Ls,j2}^{Di,*} Z_{Ls,k1}^{Di,*} - |Y_K|^2 Z_{Ls,i4}^{DR,*} Z_{Ls,j2}^{Di,*} Z_{Ls,k1}^{Di,*} \\ & - 2|Y_A|^2 Z_{Ls,i4}^{DR,*} Z_{Ls,j3}^{Di,*} Z_{Ls,k1}^{Di,*} + |Y_K|^2 Z_{Ls,i4}^{DR,*} Z_{Ls,j3}^{Di,*} Z_{Ls,k1}^{Di,*} - 2|Y_A|^2 Z_{Ls,i3}^{DR,*} Z_{Ls,j4}^{Di,*} Z_{Ls,k1}^{Di,*} \\ & + |Y_K|^2 Z_{Ls,i3}^{DR,*} Z_{Ls,j4}^{Di,*} Z_{Ls,k1}^{Di,*} + 2|Y_A|^2 Z_{Ls,i3}^{DR,*} Z_{Ls,j1}^{Di,*} Z_{Ls,k2}^{Di,*} - |Y_K|^2 Z_{Ls,i3}^{DR,*} Z_{Ls,j1}^{Di,*} Z_{Ls,k2}^{Di,*} \\ & + 2|Y_A|^2 Z_{Ls,i4}^{DR,*} Z_{Ls,j1}^{Di,*} Z_{Ls,k2}^{Di,*} - |Y_K|^2 Z_{Ls,i4}^{DR,*} Z_{Ls,j1}^{Di,*} Z_{Ls,k2}^{Di,*} - 2g_{A1}^2 Z_{Ls,i3}^{DR,*} Z_{Ls,j2}^{Di,*} Z_{Ls,k2}^{Di,*} \\ & + 2g_{A2}^2 Z_{Ls,i3}^{DR,*} Z_{Ls,j2}^{Di,*} Z_{Ls,k2}^{Di,*} - 2g_{B1}^2 Z_{Ls,i3}^{DR,*} Z_{Ls,j2}^{Di,*} Z_{Ls,k2}^{Di,*} + 2g_{B2}^2 Z_{Ls,i3}^{DR,*} Z_{Ls,j2}^{Di,*} Z_{Ls,k2}^{Di,*} \\ & + 2g_{A1}^2 Z_{Ls,i4}^{DR,*} Z_{Ls,j2}^{Di,*} Z_{Ls,k2}^{Di,*} - 2g_{A2}^2 Z_{Ls,i4}^{DR,*} Z_{Ls,j2}^{Di,*} Z_{Ls,k2}^{Di,*} + 2g_{B1}^2 Z_{Ls,i4}^{DR,*} Z_{Ls,j2}^{Di,*} Z_{Ls,k2}^{Di,*} \\ & - 2g_{B2}^2 Z_{Ls,i4}^{DR,*} Z_{Ls,j2}^{Di,*} Z_{Ls,k2}^{Di,*} - 2|Y_A|^2 Z_{Ls,i4}^{DR,*} Z_{Ls,j3}^{Di,*} Z_{Ls,k2}^{Di,*} + |Y_K|^2 Z_{Ls,i4}^{DR,*} Z_{Ls,j3}^{Di,*} Z_{Ls,k2}^{Di,*} \\ & - 2|Y_A|^2 Z_{Ls,i3}^{DR,*} Z_{Ls,j4}^{Di,*} Z_{Ls,k2}^{Di,*} + |Y_K|^2 Z_{Ls,i3}^{DR,*} Z_{Ls,j4}^{Di,*} Z_{Ls,k2}^{Di,*} - 2|Y_A|^2 Z_{Ls,i4}^{DR,*} Z_{Ls,j1}^{Di,*} Z_{Ls,k3}^{Di,*} \\ & + |Y_K|^2 Z_{Ls,i4}^{DR,*} Z_{Ls,j1}^{Di,*} Z_{Ls,k3}^{Di,*} - 2|Y_A|^2 Z_{Ls,i4}^{DR,*} Z_{Ls,j2}^{Di,*} Z_{Ls,k3}^{Di,*} + |Y_K|^2 Z_{Ls,i4}^{DR,*} Z_{Ls,j2}^{Di,*} Z_{Ls,k3}^{Di,*} \\ & + 2g_{A1}^2 Z_{Ls,i3}^{DR,*} Z_{Ls,j3}^{Di,*} Z_{Ls,k3}^{Di,*} + 2g_{A2}^2 Z_{Ls,i3}^{DR,*} Z_{Ls,j3}^{Di,*} Z_{Ls,k3}^{Di,*} + 2g_{B1}^2 Z_{Ls,i3}^{DR,*} Z_{Ls,j3}^{Di,*} Z_{Ls,k3}^{Di,*} \end{aligned}$$

$$\begin{aligned}
& + 2g_{B2}^2 Z_{Ls,i3}^{DR,*} Z_{Ls,j3}^{Di,*} Z_{Ls,k3}^{Di,*} - 2g_{A1}^2 Z_{Ls,i4}^{DR,*} Z_{Ls,j3}^{Di,*} Z_{Ls,k3}^{Di,*} - 2g_{A2}^2 Z_{Ls,i4}^{DR,*} Z_{Ls,j3}^{Di,*} Z_{Ls,k3}^{Di,*} \\
& - 2g_{B1}^2 Z_{Ls,i4}^{DR,*} Z_{Ls,j3}^{Di,*} Z_{Ls,k3}^{Di,*} - 2g_{B2}^2 Z_{Ls,i4}^{DR,*} Z_{Ls,j3}^{Di,*} Z_{Ls,k3}^{Di,*} + 4|Y_A|^2 Z_{Ls,i4}^{DR,*} Z_{Ls,j3}^{Di,*} Z_{Ls,k3}^{Di,*} \\
& + 2|Y_K|^2 Z_{Ls,i4}^{DR,*} Z_{Ls,j3}^{Di,*} Z_{Ls,k3}^{Di,*} - 2|Y_A|^2 Z_{Ls,i3}^{DR,*} Z_{Ls,j1}^{Di,*} Z_{Ls,k4}^{Di,*} + |Y_K|^2 Z_{Ls,i3}^{DR,*} Z_{Ls,j1}^{Di,*} Z_{Ls,k4}^{Di,*} \\
& - 2|Y_A|^2 Z_{Ls,i3}^{DR,*} Z_{Ls,j2}^{Di,*} Z_{Ls,k4}^{Di,*} + |Y_K|^2 Z_{Ls,i3}^{DR,*} Z_{Ls,j2}^{Di,*} Z_{Ls,k4}^{Di,*} - 2g_{A1}^2 Z_{Ls,i3}^{DR,*} Z_{Ls,j4}^{Di,*} Z_{Ls,k4}^{Di,*} \\
& - 2g_{A2}^2 Z_{Ls,i3}^{DR,*} Z_{Ls,j4}^{Di,*} Z_{Ls,k4}^{Di,*} - 2g_{B1}^2 Z_{Ls,i3}^{DR,*} Z_{Ls,j4}^{Di,*} Z_{Ls,k4}^{Di,*} - 2g_{B2}^2 Z_{Ls,i3}^{DR,*} Z_{Ls,j4}^{Di,*} Z_{Ls,k4}^{Di,*} \\
& + 4|Y_A|^2 Z_{Ls,i4}^{DR,*} Z_{Ls,j4}^{Di,*} Z_{Ls,k4}^{Di,*} + 2|Y_K|^2 Z_{Ls,i4}^{DR,*} Z_{Ls,j4}^{Di,*} Z_{Ls,k4}^{Di,*} + 2g_{A1}^2 Z_{Ls,i4}^{DR,*} Z_{Ls,j4}^{Di,*} Z_{Ls,k4}^{Di,*} \\
& + 2g_{A2}^2 Z_{Ls,i4}^{DR,*} Z_{Ls,j4}^{Di,*} Z_{Ls,k4}^{Di,*} + 2g_{B1}^2 Z_{Ls,i4}^{DR,*} Z_{Ls,j4}^{Di,*} Z_{Ls,k4}^{Di,*} + 2g_{B2}^2 Z_{Ls,i4}^{DR,*} Z_{Ls,j4}^{Di,*} Z_{Ls,k4}^{Di,*} \\
& + Z_{Ls,i2}^{DR,*} \left( |Y_K|^2 Z_{Ls,j3}^{Di,*} Z_{Ls,k1}^{Di,*} + |Y_K|^2 Z_{Ls,j4}^{Di,*} Z_{Ls,k1}^{Di,*} + 2g_{A1}^2 Z_{Ls,j2}^{Di,*} Z_{Ls,k2}^{Di,*} + 2g_{A2}^2 Z_{Ls,j2}^{Di,*} Z_{Ls,k2}^{Di,*} \right. \\
& + 2g_{B1}^2 Z_{Ls,j2}^{Di,*} Z_{Ls,k2}^{Di,*} + 2g_{B2}^2 Z_{Ls,j2}^{Di,*} Z_{Ls,k2}^{Di,*} - 2g_{A1}^2 Z_{Ls,j3}^{Di,*} Z_{Ls,k3}^{Di,*} + 2g_{A2}^2 Z_{Ls,j3}^{Di,*} Z_{Ls,k3}^{Di,*} \\
& - 2g_{B1}^2 Z_{Ls,j3}^{Di,*} Z_{Ls,k3}^{Di,*} + 2g_{B2}^2 Z_{Ls,j3}^{Di,*} Z_{Ls,k3}^{Di,*} - |Y_K|^2 Z_{Ls,j4}^{Di,*} Z_{Ls,k3}^{Di,*} \\
& \left. - 2|Y_A|^2 \left( Z_{Ls,j3}^{Di,*} \left( -Z_{Ls,k4}^{Di,*} + Z_{Ls,k1}^{Di,*} \right) + Z_{Ls,j4}^{Di,*} \left( -Z_{Ls,k3}^{Di,*} + Z_{Ls,k1}^{Di,*} \right) \right) - |Y_K|^2 Z_{Ls,j3}^{Di,*} Z_{Ls,k4}^{Di,*} \right. \\
& + 2g_{A1}^2 Z_{Ls,j4}^{Di,*} Z_{Ls,k4}^{Di,*} - 2g_{A2}^2 Z_{Ls,j4}^{Di,*} Z_{Ls,k4}^{Di,*} + 2g_{B1}^2 Z_{Ls,j4}^{Di,*} Z_{Ls,k4}^{Di,*} - 2g_{B2}^2 Z_{Ls,j4}^{Di,*} Z_{Ls,k4}^{Di,*} \\
& + Z_{Ls,j1}^{Di,*} \left( -2 \left( -2|Y_A|^2 - |Y_K|^2 + g_{A1}^2 + g_{A2}^2 + g_{B1}^2 + g_{B2}^2 \right) Z_{Ls,k1}^{Di,*} - \left( 2|Y_A|^2 - |Y_K|^2 \right) \left( Z_{Ls,k3}^{Di,*} + Z_{Ls,k4}^{Di,*} \right) \right) \\
& + Z_{Ls,i1}^{DR,*} \left( 2 \left( g_{A1}^2 + g_{A2}^2 + g_{B1}^2 + g_{B2}^2 \right) Z_{Ls,j1}^{Di,*} Z_{Ls,k1}^{Di,*} - 2|Y_A|^2 Z_{Ls,j3}^{Di,*} Z_{Ls,k2}^{Di,*} + |Y_K|^2 Z_{Ls,j3}^{Di,*} Z_{Ls,k2}^{Di,*} \right. \\
& - 2|Y_A|^2 Z_{Ls,j4}^{Di,*} Z_{Ls,k2}^{Di,*} + |Y_K|^2 Z_{Ls,j4}^{Di,*} Z_{Ls,k2}^{Di,*} + 2g_{A1}^2 Z_{Ls,j3}^{Di,*} Z_{Ls,k3}^{Di,*} - 2g_{A2}^2 Z_{Ls,j3}^{Di,*} Z_{Ls,k3}^{Di,*} \\
& + 2g_{B1}^2 Z_{Ls,j3}^{Di,*} Z_{Ls,k3}^{Di,*} - 2g_{B2}^2 Z_{Ls,j3}^{Di,*} Z_{Ls,k3}^{Di,*} + 2|Y_A|^2 Z_{Ls,j4}^{Di,*} Z_{Ls,k3}^{Di,*} - |Y_K|^2 Z_{Ls,j4}^{Di,*} Z_{Ls,k3}^{Di,*} \\
& + 2|Y_A|^2 Z_{Ls,j3}^{Di,*} Z_{Ls,k4}^{Di,*} - |Y_K|^2 Z_{Ls,j3}^{Di,*} Z_{Ls,k4}^{Di,*} - 2g_{A1}^2 Z_{Ls,j4}^{Di,*} Z_{Ls,k4}^{Di,*} + 2g_{A2}^2 Z_{Ls,j4}^{Di,*} Z_{Ls,k4}^{Di,*} \\
& - 2g_{B1}^2 Z_{Ls,j4}^{Di,*} Z_{Ls,k4}^{Di,*} + 2g_{B2}^2 Z_{Ls,j4}^{Di,*} Z_{Ls,k4}^{Di,*} \\
& \left. + Z_{Ls,j2}^{Di,*} \left( -2 \left( -2|Y_A|^2 - |Y_K|^2 + g_{A1}^2 + g_{A2}^2 + g_{B1}^2 + g_{B2}^2 \right) Z_{Ls,k2}^{Di,*} - \left( 2|Y_A|^2 - |Y_K|^2 \right) \left( Z_{Ls,k3}^{Di,*} + Z_{Ls,k4}^{Di,*} \right) \right) \right) \quad (413)
\end{aligned}$$

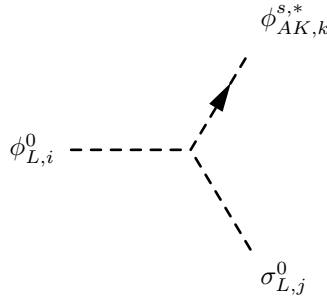

$$\begin{aligned}
& \frac{1}{2} \left( -T_K^* \left( Z_{Ls,i1}^{DR,*} Z_{Ls,j2}^{Di,*} + Z_{Ls,i2}^{DR,*} Z_{Ls,j1}^{Di,*} + Z_{Ls,i3}^{DR,*} Z_{Ls,j4}^{Di,*} + Z_{Ls,i4}^{DR,*} Z_{Ls,j3}^{Di,*} \right) Z_{AK,k1}^s \right. \\
& \left. + \sqrt{2} T_A^* \left( -Z_{Ls,i1}^{DR,*} Z_{Ls,j2}^{Di,*} - Z_{Ls,i2}^{DR,*} Z_{Ls,j1}^{Di,*} + Z_{Ls,i3}^{DR,*} Z_{Ls,j4}^{Di,*} + Z_{Ls,i4}^{DR,*} Z_{Ls,j3}^{Di,*} \right) Z_{AK,k2}^s \right) \quad (414)
\end{aligned}$$

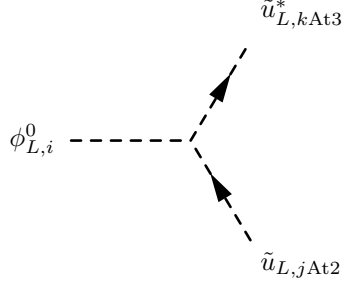

$$\frac{i}{6}v_{Lv}\left(\left(-3g_{A2}^2+g_{A1}^2\right)Z_{Ls,i1}^{DR,*}-\left(-3g_{A2}^2+g_{A1}^2\right)Z_{Ls,i2}^{DR,*}+\left(3g_{A2}^2+g_{A1}^2\right)\left(-Z_{Ls,i4}^{DR,*}+Z_{Ls,i3}^{DR,*}\right)\right)\delta_{\text{At}2\text{At}3}\delta_{jk} \quad (415)$$


---

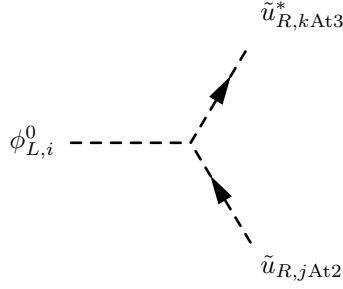

$$-\frac{2i}{3}g_{A1}^2v_{Lv}\left(-Z_{Ls,i2}^{DR,*}-Z_{Ls,i4}^{DR,*}+Z_{Ls,i1}^{DR,*}+Z_{Ls,i3}^{DR,*}\right)\delta_{\text{At}2\text{At}3}\delta_{jk} \quad (416)$$


---

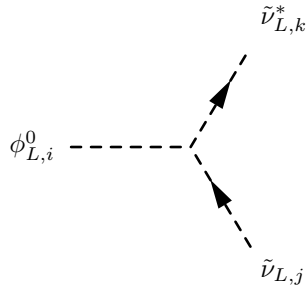

$$-\frac{i}{2}v_{Lv}\left(\left(g_{A1}^2+g_{A2}^2\right)Z_{Ls,i1}^{DR,*}-\left(g_{A1}^2+g_{A2}^2\right)Z_{Ls,i2}^{DR,*}+\left(-g_{A2}^2+g_{A1}^2\right)\left(-Z_{Ls,i4}^{DR,*}+Z_{Ls,i3}^{DR,*}\right)\right)\delta_{jk} \quad (417)$$


---

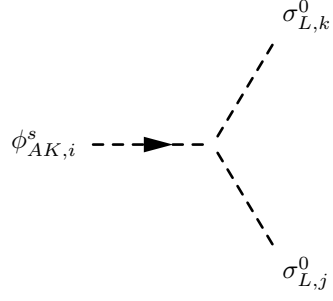

$$\begin{aligned}
& \frac{i}{2} \left( \sqrt{2} Z_{AK,i2}^{s,*} \left( Z_{Ls,j1}^{Di,*} Z_{Ls,k2}^{Di,*} + Z_{Ls,j2}^{Di,*} Z_{Ls,k1}^{Di,*} - Z_{Ls,j3}^{Di,*} Z_{Ls,k4}^{Di,*} - Z_{Ls,j4}^{Di,*} Z_{Ls,k3}^{Di,*} \right) T_A \right. \\
& \left. + Z_{AK,i1}^{s,*} \left( Z_{Ls,j1}^{Di,*} Z_{Ls,k2}^{Di,*} + Z_{Ls,j2}^{Di,*} Z_{Ls,k1}^{Di,*} + Z_{Ls,j3}^{Di,*} Z_{Ls,k4}^{Di,*} + Z_{Ls,j4}^{Di,*} Z_{Ls,k3}^{Di,*} \right) T_K \right)
\end{aligned} \tag{418}$$


---

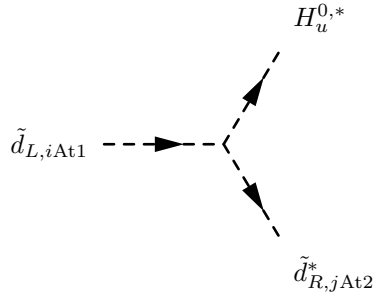

$$i\mu^* \delta_{At1At2} Y_{d,ji} \tag{419}$$


---

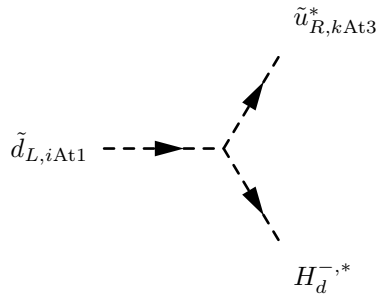

$$i\mu^* \delta_{At1At3} Y_{u,ki} \tag{420}$$


---

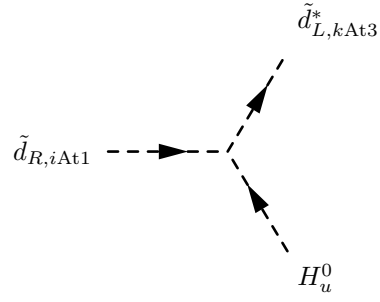

$$i\mu Y_{d,ik}^* \delta_{At1At3} \quad (421)$$


---

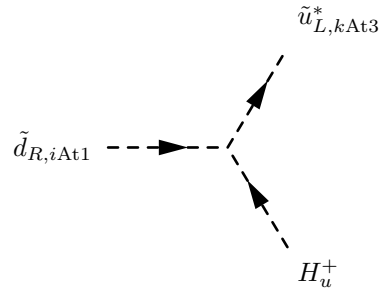

$$i\mu Y_{d,ik}^* \delta_{At1At3} \quad (422)$$


---

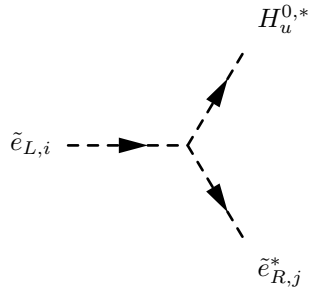

$$i\mu^* Y_{e,ji} \quad (423)$$


---

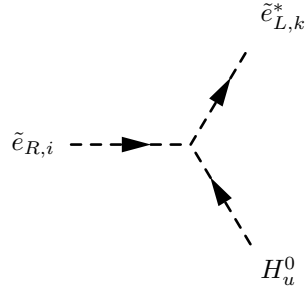

$$i\mu Y_{e,ik}^* \quad (424)$$


---

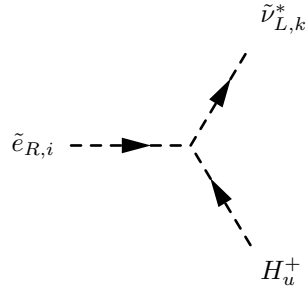

$$i\mu Y_{e,ik}^* \quad (425)$$


---

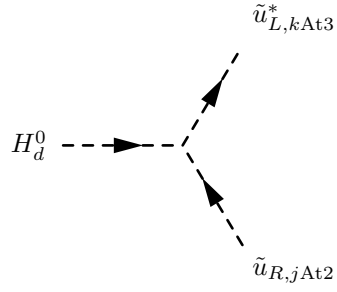

$$i\mu Y_{u,jk}^* \delta_{\text{At}2\text{At}3} \quad (426)$$


---

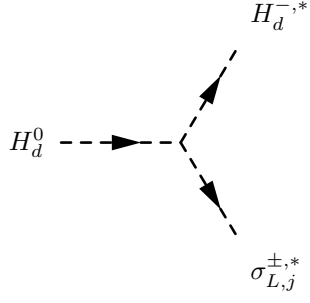

$$-\frac{i}{2}g_{A2}^2v_{Lv}\left(-Z_{Ls,j2}^{od}-Z_{Ls,j3}^{od}+Z_{Ls,j1}^{od}+Z_{Ls,j4}^{od}\right) \quad (427)$$


---

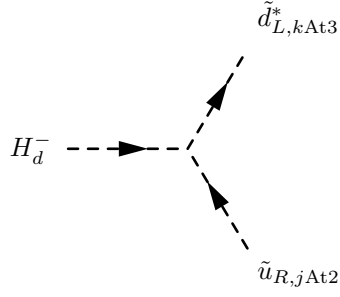

$$i\mu Y_{u,jk}^*\delta_{At2At3} \quad (428)$$


---

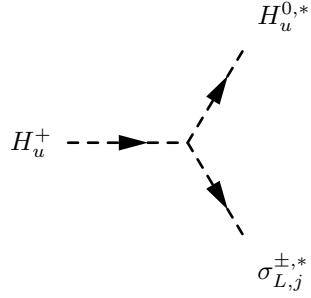

$$-\frac{i}{2}g_{A2}^2v_{Lv}\left(-Z_{Ls,j2}^{od}-Z_{Ls,j3}^{od}+Z_{Ls,j1}^{od}+Z_{Ls,j4}^{od}\right) \quad (429)$$


---

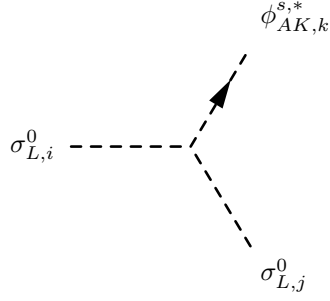

$$\begin{aligned}
& \frac{i}{2} \left( T_K^* \left( Z_{Ls,i1}^{Di,*} Z_{Ls,j2}^{Di,*} + Z_{Ls,i2}^{Di,*} Z_{Ls,j1}^{Di,*} + Z_{Ls,i3}^{Di,*} Z_{Ls,j4}^{Di,*} + Z_{Ls,i4}^{Di,*} Z_{Ls,j3}^{Di,*} \right) Z_{AK,k1}^s \right. \\
& \left. + \sqrt{2} T_A^* \left( Z_{Ls,i1}^{Di,*} Z_{Ls,j2}^{Di,*} + Z_{Ls,i2}^{Di,*} Z_{Ls,j1}^{Di,*} - Z_{Ls,i3}^{Di,*} Z_{Ls,j4}^{Di,*} - Z_{Ls,i4}^{Di,*} Z_{Ls,j3}^{Di,*} \right) Z_{AK,k2}^s \right)
\end{aligned} \tag{430}$$


---

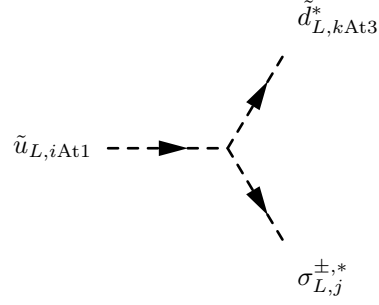

$$-\frac{i}{2} g_{A2}^2 v_{Lv} \delta_{At1At3} \delta_{ik} \left( -Z_{Ls,j2}^{od} - Z_{Ls,j3}^{od} + Z_{Ls,j1}^{od} + Z_{Ls,j4}^{od} \right) \tag{431}$$


---

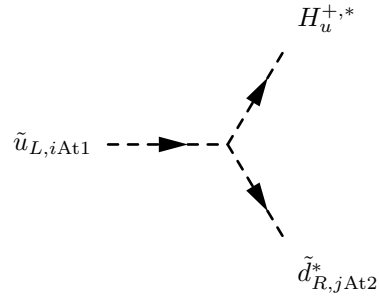

$$i\mu^* \delta_{At1At2} Y_{d,ji} \tag{432}$$


---



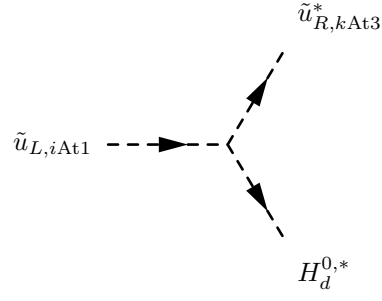

$$i\mu^* \delta_{\text{At}1\text{At}3} Y_{u,ki} \quad (433)$$


---

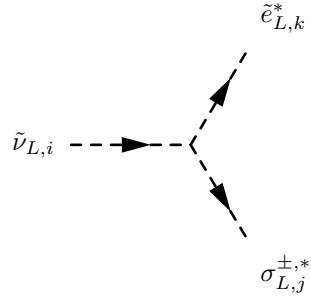

$$-\frac{i}{2} g_{A2}^2 v_{Lv} \delta_{ik} \left( -Z_{Ls,j2}^{od} - Z_{Ls,j3}^{od} + Z_{Ls,j1}^{od} + Z_{Ls,j4}^{od} \right) \quad (434)$$


---

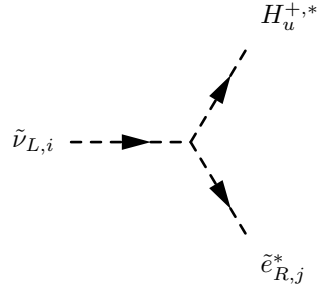

$$i\mu^* Y_{e,ji} \quad (435)$$


---

## 9.2 Two Scalar-One Vector Boson-Interaction

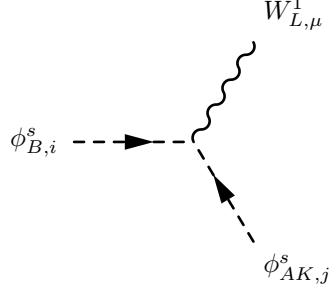

$$i \frac{1}{\sqrt{2}} g_{B2} \sqrt{\frac{g_A 2^2}{g_A 2^2 + g_B 2^2}} Z_{AK,j2}^{s,*} B_{A,i2}^{s,*} \left( -p_\mu^{\phi_{AK,j}^s} + p_\mu^{\phi_{B,i}^s} \right) \quad (436)$$


---

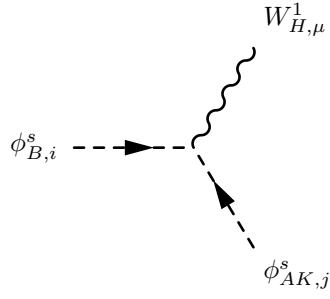

$$i \frac{1}{\sqrt{2}} g_{B2}^2 \frac{1}{\sqrt{g_A 2^2 + g_B 2^2}} Z_{AK,j2}^{s,*} B_{A,i2}^{s,*} \left( -p_\mu^{\phi_{AK,j}^s} + p_\mu^{\phi_{B,i}^s} \right) \quad (437)$$


---

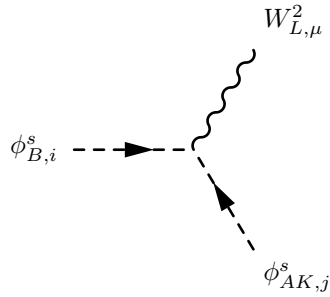

$$- \frac{1}{\sqrt{2}} g_{B2} \sqrt{\frac{g_A 2^2}{g_A 2^2 + g_B 2^2}} Z_{AK,j2}^{s,*} B_{A,i2}^{s,*} \left( -p_\mu^{\phi_{AK,j}^s} + p_\mu^{\phi_{B,i}^s} \right) \quad (438)$$


---

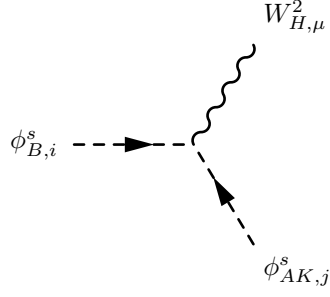

$$-\frac{1}{\sqrt{2}}g_{B2}^2\frac{1}{\sqrt{gA2^2+gB2^2}}Z_{AK,j2}^{s,*}B_{A,i2}^{s,*}\left(-p_{\mu}^{\phi_{AK,j}^s}+p_{\mu}^{\phi_{B,i}^s}\right) \quad (439)$$


---

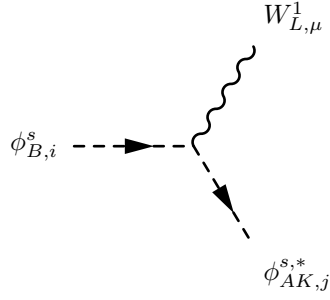

$$i\frac{1}{\sqrt{2}}g_{B2}\sqrt{\frac{gA2^2}{gA2^2+gB2^2}}B_{A,i1}^{s,*}Z_{AK,j2}^s\left(-p_{\mu}^{\phi_{AK,j}^{s,*}}+p_{\mu}^{\phi_{B,i}^s}\right) \quad (440)$$


---

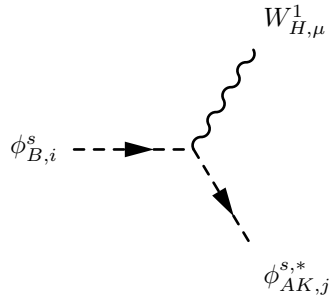

$$i\frac{1}{\sqrt{2}}g_{B2}^2\frac{1}{\sqrt{gA2^2+gB2^2}}B_{A,i1}^{s,*}Z_{AK,j2}^s\left(-p_{\mu}^{\phi_{AK,j}^{s,*}}+p_{\mu}^{\phi_{B,i}^s}\right) \quad (441)$$


---

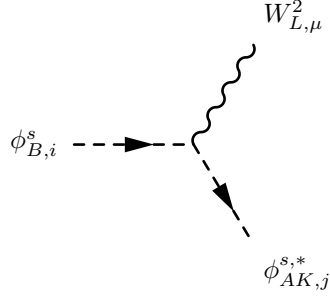

$$-\frac{1}{\sqrt{2}}g_{B2}\sqrt{\frac{gA2^2}{gA2^2+gB2^2}}B_{A,i1}^{s,*}Z_{AK,j2}^s\left(-p_\mu^{\phi_{AK,j}^{s,*}}+p_\mu^{\phi_{B,i}^s}\right) \quad (442)$$


---

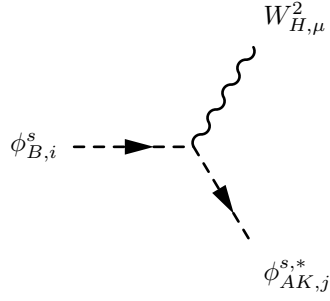

$$-\frac{1}{\sqrt{2}}g_{B2}^2\frac{1}{\sqrt{gA2^2+gB2^2}}B_{A,i1}^{s,*}Z_{AK,j2}^s\left(-p_\mu^{\phi_{AK,j}^{s,*}}+p_\mu^{\phi_{B,i}^s}\right) \quad (443)$$


---

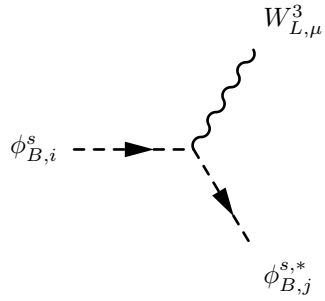

$$-ig_{B2}\sqrt{\frac{gA2^2}{gA2^2+gB2^2}}\left(B_{A,i1}^{s,*}B_{A,j1}^s+B_{A,i2}^{s,*}B_{A,j2}^s\right)\left(-p_\mu^{\phi_{B,j}^{s,*}}+p_\mu^{\phi_{B,i}^s}\right) \quad (444)$$


---

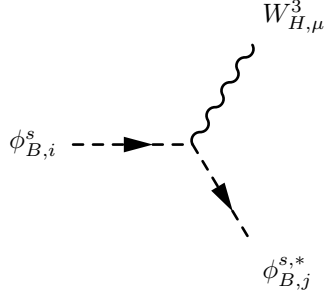

$$-ig_{B2}^2 \frac{1}{\sqrt{gA2^2 + gB2^2}} \left( B_{A,i1}^{s,*} B_{A,j1}^s + B_{A,i2}^{s,*} B_{A,j2}^s \right) \left( -p_\mu^{\phi_{B,j}^{s,*}} + p_\mu^{\phi_{B,i}^s} \right) \quad (445)$$


---

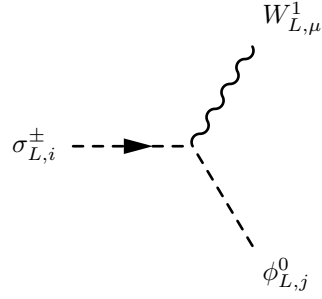

$$\begin{aligned} & \frac{i}{2} g_{B2} \frac{1}{\sqrt{gA2^2 + gB2^2}} \left( g_{A2} Z_{Ls,i2}^{od,*} Z_{Ls,j2}^{DR,*} + \sqrt{\frac{gA2^2}{gA2^2 + gB2^2}} \sqrt{gA2^2 + gB2^2} Z_{Ls,i3}^{od,*} Z_{Ls,j2}^{DR,*} \right. \\ & + Z_{Ls,i1}^{od,*} \left( -g_{A2} Z_{Ls,j3}^{DR,*} + \sqrt{\frac{gA2^2}{gA2^2 + gB2^2}} \sqrt{gA2^2 + gB2^2} Z_{Ls,j1}^{DR,*} \right) \\ & + Z_{Ls,i4}^{od,*} \left( g_{A2} Z_{Ls,j1}^{DR,*} - \sqrt{\frac{gA2^2}{gA2^2 + gB2^2}} \sqrt{gA2^2 + gB2^2} Z_{Ls,j3}^{DR,*} \right) \\ & \left. - \sqrt{\frac{gA2^2}{gA2^2 + gB2^2}} \sqrt{gA2^2 + gB2^2} Z_{Ls,i2}^{od,*} Z_{Ls,j4}^{DR,*} - g_{A2} Z_{Ls,i3}^{od,*} Z_{Ls,j4}^{DR,*} \right) \left( -p_\mu^{\phi_{L,j}^0} + p_\mu^{\sigma_{L,i}^\pm} \right) \quad (446) \end{aligned}$$


---

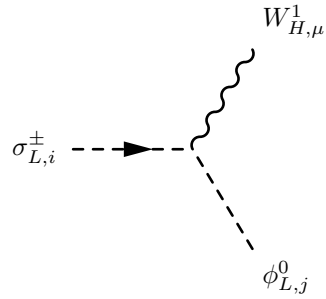

$$\begin{aligned}
& \frac{i}{2} \frac{1}{\sqrt{gA^2 + gB^2}} \left( -g_{A2} \sqrt{\frac{gA^2}{gA^2 + gB^2}} \sqrt{gA^2 + gB^2} Z_{Ls,i2}^{od,*} Z_{Ls,j2}^{DR,*} + g_{B2}^2 Z_{Ls,i3}^{od,*} Z_{Ls,j2}^{DR,*} \right. \\
& - Z_{Ls,i4}^{od,*} \left( g_{A2} \sqrt{\frac{gA^2}{gA^2 + gB^2}} \sqrt{gA^2 + gB^2} Z_{Ls,j1}^{DR,*} + g_{B2}^2 Z_{Ls,j3}^{DR,*} \right) \\
& + Z_{Ls,i1}^{od,*} \left( g_{A2} \sqrt{\frac{gA^2}{gA^2 + gB^2}} \sqrt{gA^2 + gB^2} Z_{Ls,j3}^{DR,*} + g_{B2}^2 Z_{Ls,j1}^{DR,*} \right) - g_{B2}^2 Z_{Ls,i2}^{od,*} Z_{Ls,j4}^{DR,*} \\
& \left. + g_{A2} \sqrt{\frac{gA^2}{gA^2 + gB^2}} \sqrt{gA^2 + gB^2} Z_{Ls,i3}^{od,*} Z_{Ls,j4}^{DR,*} \right) \left( -p_\mu^{\phi_{L,j}^0} + p_\mu^{\sigma_{L,i}^\pm} \right) \quad (447)
\end{aligned}$$


---

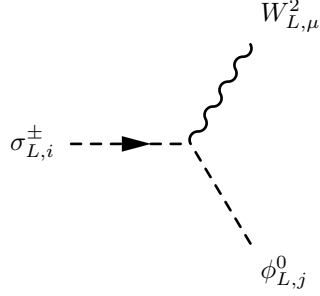

$$\begin{aligned}
& \frac{1}{2} g_{B2} \frac{1}{\sqrt{gA^2 + gB^2}} \left( -g_{A2} Z_{Ls,i2}^{od,*} Z_{Ls,j2}^{DR,*} - \sqrt{\frac{gA^2}{gA^2 + gB^2}} \sqrt{gA^2 + gB^2} Z_{Ls,i3}^{od,*} Z_{Ls,j2}^{DR,*} \right. \\
& + Z_{Ls,i1}^{od,*} \left( g_{A2} Z_{Ls,j3}^{DR,*} - \sqrt{\frac{gA^2}{gA^2 + gB^2}} \sqrt{gA^2 + gB^2} Z_{Ls,j1}^{DR,*} \right) \\
& + Z_{Ls,i4}^{od,*} \left( -g_{A2} Z_{Ls,j1}^{DR,*} + \sqrt{\frac{gA^2}{gA^2 + gB^2}} \sqrt{gA^2 + gB^2} Z_{Ls,j3}^{DR,*} \right) \\
& \left. + \sqrt{\frac{gA^2}{gA^2 + gB^2}} \sqrt{gA^2 + gB^2} Z_{Ls,i2}^{od,*} Z_{Ls,j4}^{DR,*} + g_{A2} Z_{Ls,i3}^{od,*} Z_{Ls,j4}^{DR,*} \right) \left( -p_\mu^{\phi_{L,j}^0} + p_\mu^{\sigma_{L,i}^\pm} \right) \quad (448)
\end{aligned}$$


---

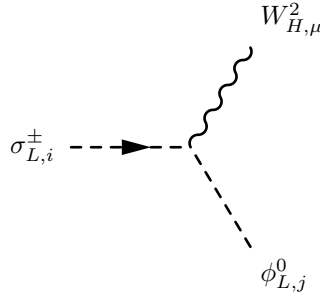

$$\begin{aligned}
& \frac{1}{2} \frac{1}{\sqrt{gA^2 + gB^2}} \left( gA^2 \sqrt{\frac{gA^2}{gA^2 + gB^2}} \sqrt{gA^2 + gB^2} Z_{Ls,i2}^{od,*} Z_{Ls,j2}^{DR,*} - g_{B2}^2 Z_{Ls,i3}^{od,*} Z_{Ls,j2}^{DR,*} \right. \\
& + Z_{Ls,i4}^{od,*} \left( gA^2 \sqrt{\frac{gA^2}{gA^2 + gB^2}} \sqrt{gA^2 + gB^2} Z_{Ls,j1}^{DR,*} + g_{B2}^2 Z_{Ls,j3}^{DR,*} \right) \\
& - Z_{Ls,i1}^{od,*} \left( gA^2 \sqrt{\frac{gA^2}{gA^2 + gB^2}} \sqrt{gA^2 + gB^2} Z_{Ls,j3}^{DR,*} + g_{B2}^2 Z_{Ls,j1}^{DR,*} \right) + g_{B2}^2 Z_{Ls,i2}^{od,*} Z_{Ls,j4}^{DR,*} \\
& \left. - gA^2 \sqrt{\frac{gA^2}{gA^2 + gB^2}} \sqrt{gA^2 + gB^2} Z_{Ls,i3}^{od,*} Z_{Ls,j4}^{DR,*} \right) \left( -p_\mu^{\phi_{L,j}^0} + p_\mu^{\sigma_{L,i}^\pm} \right)
\end{aligned} \tag{449}$$


---

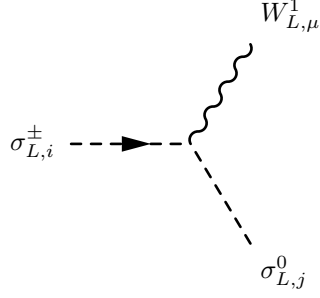

$$\begin{aligned}
& \frac{1}{2} g_{B2} \frac{1}{\sqrt{gA^2 + gB^2}} \left( gA^2 Z_{Ls,i2}^{od,*} Z_{Ls,j2}^{Di,*} - \sqrt{\frac{gA^2}{gA^2 + gB^2}} \sqrt{gA^2 + gB^2} Z_{Ls,i3}^{od,*} Z_{Ls,j2}^{Di,*} \right. \\
& + Z_{Ls,i1}^{od,*} \left( -gA^2 Z_{Ls,j3}^{Di,*} + \sqrt{\frac{gA^2}{gA^2 + gB^2}} \sqrt{gA^2 + gB^2} Z_{Ls,j1}^{Di,*} \right) \\
& + Z_{Ls,i4}^{od,*} \left( -gA^2 Z_{Ls,j1}^{Di,*} + \sqrt{\frac{gA^2}{gA^2 + gB^2}} \sqrt{gA^2 + gB^2} Z_{Ls,j3}^{Di,*} \right) \\
& \left. - \sqrt{\frac{gA^2}{gA^2 + gB^2}} \sqrt{gA^2 + gB^2} Z_{Ls,i2}^{od,*} Z_{Ls,j4}^{Di,*} + gA^2 Z_{Ls,i3}^{od,*} Z_{Ls,j4}^{Di,*} \right) \left( -p_\mu^{\sigma_{L,j}^0} + p_\mu^{\sigma_{L,i}^\pm} \right)
\end{aligned} \tag{450}$$


---

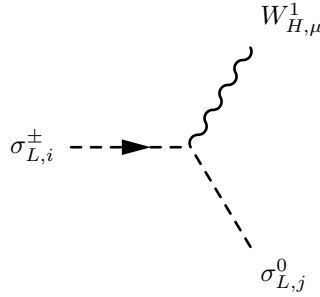

$$\begin{aligned}
& \frac{1}{2} \frac{1}{\sqrt{gA2^2 + gB2^2}} \left( -g_{A2} \sqrt{\frac{gA2^2}{gA2^2 + gB2^2}} \sqrt{gA2^2 + gB2^2} Z_{Ls,i2}^{od,*} Z_{Ls,j2}^{Di,*} - g_{B2}^2 Z_{Ls,i3}^{od,*} Z_{Ls,j2}^{Di,*} \right. \\
& + Z_{Ls,i4}^{od,*} \left( g_{A2} \sqrt{\frac{gA2^2}{gA2^2 + gB2^2}} \sqrt{gA2^2 + gB2^2} Z_{Ls,j1}^{Di,*} + g_{B2}^2 Z_{Ls,j3}^{Di,*} \right) \\
& + Z_{Ls,i1}^{od,*} \left( g_{A2} \sqrt{\frac{gA2^2}{gA2^2 + gB2^2}} \sqrt{gA2^2 + gB2^2} Z_{Ls,j3}^{Di,*} + g_{B2}^2 Z_{Ls,j1}^{Di,*} \right) - g_{B2}^2 Z_{Ls,i2}^{od,*} Z_{Ls,j4}^{Di,*} \\
& \left. - g_{A2} \sqrt{\frac{gA2^2}{gA2^2 + gB2^2}} \sqrt{gA2^2 + gB2^2} Z_{Ls,i3}^{od,*} Z_{Ls,j4}^{Di,*} \right) \left( -p_\mu^{\sigma_{L,j}^0} + p_\mu^{\sigma_{L,i}^\pm} \right)
\end{aligned} \tag{451}$$


---

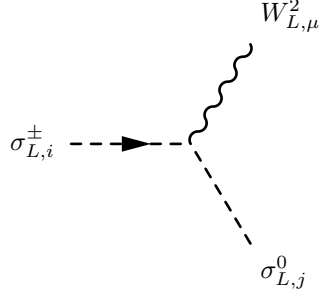

$$\begin{aligned}
& \frac{i}{2} g_{B2} \frac{1}{\sqrt{gA2^2 + gB2^2}} \left( g_{A2} Z_{Ls,i2}^{od,*} Z_{Ls,j2}^{Di,*} - \sqrt{\frac{gA2^2}{gA2^2 + gB2^2}} \sqrt{gA2^2 + gB2^2} Z_{Ls,i3}^{od,*} Z_{Ls,j2}^{Di,*} \right. \\
& + Z_{Ls,i1}^{od,*} \left( -g_{A2} Z_{Ls,j3}^{Di,*} + \sqrt{\frac{gA2^2}{gA2^2 + gB2^2}} \sqrt{gA2^2 + gB2^2} Z_{Ls,j1}^{Di,*} \right) \\
& + Z_{Ls,i4}^{od,*} \left( -g_{A2} Z_{Ls,j1}^{Di,*} + \sqrt{\frac{gA2^2}{gA2^2 + gB2^2}} \sqrt{gA2^2 + gB2^2} Z_{Ls,j3}^{Di,*} \right) \\
& \left. - \sqrt{\frac{gA2^2}{gA2^2 + gB2^2}} \sqrt{gA2^2 + gB2^2} Z_{Ls,i2}^{od,*} Z_{Ls,j4}^{Di,*} + g_{A2} Z_{Ls,i3}^{od,*} Z_{Ls,j4}^{Di,*} \right) \left( -p_\mu^{\sigma_{L,j}^0} + p_\mu^{\sigma_{L,i}^\pm} \right)
\end{aligned} \tag{452}$$


---

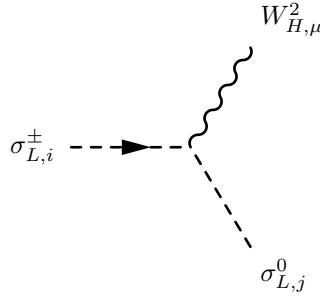



$$\begin{aligned}
& \frac{i}{2} \frac{1}{\sqrt{gA2^2 + gB2^2}} \left( -g_{A2} \sqrt{\frac{gA2^2}{gA2^2 + gB2^2}} \sqrt{gA2^2 + gB2^2} Z_{Ls,i2}^{od,*} Z_{Ls,j2}^{Di,*} - g_{B2}^2 Z_{Ls,i3}^{od,*} Z_{Ls,j2}^{Di,*} \right. \\
& + Z_{Ls,i4}^{od,*} \left( g_{A2} \sqrt{\frac{gA2^2}{gA2^2 + gB2^2}} \sqrt{gA2^2 + gB2^2} Z_{Ls,j1}^{Di,*} + g_{B2}^2 Z_{Ls,j3}^{Di,*} \right) \\
& + Z_{Ls,i1}^{od,*} \left( g_{A2} \sqrt{\frac{gA2^2}{gA2^2 + gB2^2}} \sqrt{gA2^2 + gB2^2} Z_{Ls,j3}^{Di,*} + g_{B2}^2 Z_{Ls,j1}^{Di,*} \right) - g_{B2}^2 Z_{Ls,i2}^{od,*} Z_{Ls,j4}^{Di,*} \\
& \left. - g_{A2} \sqrt{\frac{gA2^2}{gA2^2 + gB2^2}} \sqrt{gA2^2 + gB2^2} Z_{Ls,i3}^{od,*} Z_{Ls,j4}^{Di,*} \right) \left( -p_\mu^{\sigma_{L,j}^0} + p_\mu^{\sigma_{L,i}^\pm} \right)
\end{aligned} \tag{453}$$


---

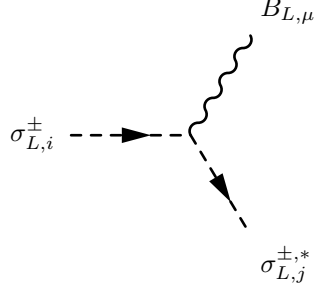

$$-\frac{i}{2} g_{B1} \frac{1}{\sqrt{gA1^2 + gB1^2}} \left( -g_{A1} + \sqrt{\frac{gA1^2}{gA1^2 + gB1^2}} \sqrt{gA1^2 + gB1^2} \right) \left( Z_{Ls,i1}^{od,*} Z_{Ls,j1}^{od} - Z_{Ls,i2}^{od,*} Z_{Ls,j2}^{od} + Z_{Ls,i3}^{od,*} Z_{Ls,j3}^{od} - Z_{Ls,i4}^{od,*} Z_{Ls,j4}^{od} \right) \left( -p_\mu^{\sigma_{L,j}^0} + p_\mu^{\sigma_{L,i}^\pm} \right) \tag{454}$$


---

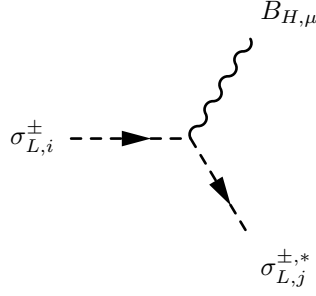

$$-\frac{i}{2} \frac{1}{\sqrt{gA1^2 + gB1^2}} \left( g_{A1} \sqrt{\frac{gA1^2}{gA1^2 + gB1^2}} \sqrt{gA1^2 + gB1^2} + g_{B1}^2 \right) \left( Z_{Ls,i1}^{od,*} Z_{Ls,j1}^{od} - Z_{Ls,i2}^{od,*} Z_{Ls,j2}^{od} + Z_{Ls,i3}^{od,*} Z_{Ls,j3}^{od} - Z_{Ls,i4}^{od,*} Z_{Ls,j4}^{od} \right) \left( -p_\mu^{\sigma_{L,j}^0} + p_\mu^{\sigma_{L,i}^\pm} \right) \tag{455}$$


---

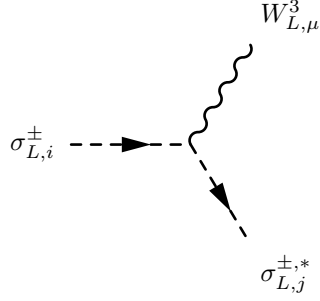

$$-\frac{i}{2}g_{B2}\frac{1}{\sqrt{g_{A2}^2+g_{B2}^2}}\left(\sqrt{\frac{g_{A2}^2}{g_{A2}^2+g_{B2}^2}}\sqrt{g_{A2}^2+g_{B2}^2}+g_{A2}\right)\left(Z_{Ls,i1}^{od,*}Z_{Ls,j1}^{od}+Z_{Ls,i2}^{od,*}Z_{Ls,j2}^{od}+Z_{Ls,i3}^{od,*}Z_{Ls,j3}^{od}+Z_{Ls,i4}^{od,*}Z_{Ls,j4}^{od}\right)\left(-p_{\mu}^{\sigma_{L,i}^{\pm},\sigma_{L,j}^{\pm,*}}\right) \quad (456)$$


---

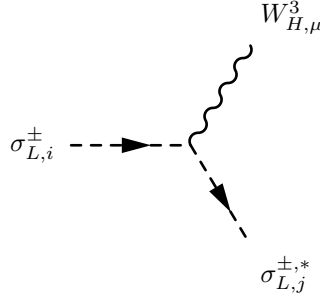

$$\frac{i}{2}\frac{1}{\sqrt{g_{A2}^2+g_{B2}^2}}\left(g_{A2}\sqrt{\frac{g_{A2}^2}{g_{A2}^2+g_{B2}^2}}\sqrt{g_{A2}^2+g_{B2}^2}-g_{B2}^2\right)\left(Z_{Ls,i1}^{od,*}Z_{Ls,j1}^{od}+Z_{Ls,i2}^{od,*}Z_{Ls,j2}^{od}+Z_{Ls,i3}^{od,*}Z_{Ls,j3}^{od}+Z_{Ls,i4}^{od,*}Z_{Ls,j4}^{od}\right)\left(-p_{\mu}^{\sigma_{L,i}^{\pm},\sigma_{L,j}^{\pm,*}}\right) \quad (457)$$


---

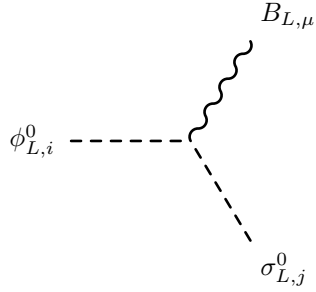

$$-g_{B1}\frac{1}{\sqrt{g_{A1}^2+g_{B1}^2}}\left(-g_{A1}+\sqrt{\frac{g_{A1}^2}{g_{A1}^2+g_{B1}^2}}\sqrt{g_{A1}^2+g_{B1}^2}\right)\left(Z_{Ls,i1}^{DR,*}Z_{Ls,j1}^{Di,*}-Z_{Ls,i2}^{DR,*}Z_{Ls,j2}^{Di,*}+Z_{Ls,i3}^{DR,*}Z_{Ls,j3}^{Di,*}-Z_{Ls,i4}^{DR,*}Z_{Ls,j4}^{Di,*}\right)\left(-p_{\mu}^{\phi_{L,i}^0,\sigma_{L,j}^0}\right) \quad (458)$$


---

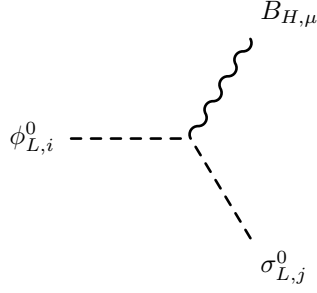

$$- \frac{1}{\sqrt{gA1^2 + gB1^2}} \left( gA1 \sqrt{\frac{gA1^2}{gA1^2 + gB1^2}} \sqrt{gA1^2 + gB1^2 + g_{B1}^2} \right) \left( Z_{Ls,i1}^{DR,*} Z_{Ls,j1}^{Di,*} - Z_{Ls,i2}^{DR,*} Z_{Ls,j2}^{Di,*} + Z_{Ls,i3}^{DR,*} Z_{Ls,j3}^{Di,*} - Z_{Ls,i4}^{DR,*} Z_{Ls,j4}^{Di,*} \right) \left( -p_\mu^{\sigma_{L,j}^0} \right) \quad (459)$$


---

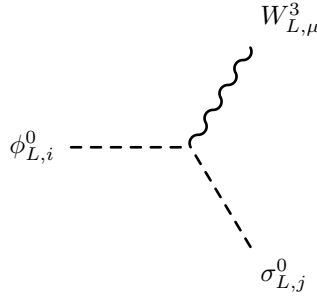

$$g_{B2} \frac{1}{\sqrt{gA2^2 + gB2^2}} \left( -g_{A2} + \sqrt{\frac{gA2^2}{gA2^2 + gB2^2}} \sqrt{gA2^2 + gB2^2} \right) \left( Z_{Ls,i1}^{DR,*} Z_{Ls,j1}^{Di,*} - Z_{Ls,i2}^{DR,*} Z_{Ls,j2}^{Di,*} - Z_{Ls,i3}^{DR,*} Z_{Ls,j3}^{Di,*} + Z_{Ls,i4}^{DR,*} Z_{Ls,j4}^{Di,*} \right) \left( -p_\mu^{\sigma_{L,j}^0} \right) \quad (460)$$


---

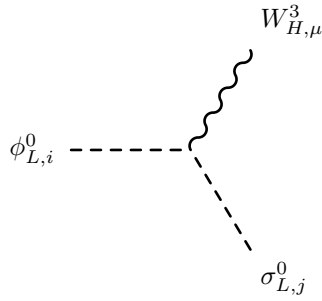

$$\frac{1}{\sqrt{gA2^2 + gB2^2}} \left( g_{A2} \sqrt{\frac{gA2^2}{gA2^2 + gB2^2}} \sqrt{gA2^2 + gB2^2 + g_{B2}^2} \right) \left( Z_{Ls,i1}^{DR,*} Z_{Ls,j1}^{Di,*} - Z_{Ls,i2}^{DR,*} Z_{Ls,j2}^{Di,*} - Z_{Ls,i3}^{DR,*} Z_{Ls,j3}^{Di,*} + Z_{Ls,i4}^{DR,*} Z_{Ls,j4}^{Di,*} \right) \left( -p_\mu^{\sigma_{L,j}^0} + \right) \quad (461)$$


---

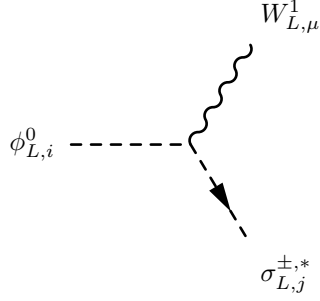

$$\begin{aligned}
& \frac{i}{2} g_{B2} \frac{1}{\sqrt{gA2^2 + gB2^2}} \left( g_{A2} Z_{Ls,i2}^{DR,*} Z_{Ls,j2}^{od} - \sqrt{\frac{gA2^2}{gA2^2 + gB2^2}} \sqrt{gA2^2 + gB2^2} Z_{Ls,i4}^{DR,*} Z_{Ls,j2}^{od} \right. \\
& + \sqrt{\frac{gA2^2}{gA2^2 + gB2^2}} \sqrt{gA2^2 + gB2^2} Z_{Ls,i2}^{DR,*} Z_{Ls,j3}^{od} - g_{A2} Z_{Ls,i4}^{DR,*} Z_{Ls,j3}^{od} \\
& + Z_{Ls,i1}^{DR,*} \left( g_{A2} Z_{Ls,j4}^{od} + \sqrt{\frac{gA2^2}{gA2^2 + gB2^2}} \sqrt{gA2^2 + gB2^2} Z_{Ls,j1}^{od} \right) \\
& \left. - Z_{Ls,i3}^{DR,*} \left( g_{A2} Z_{Ls,j1}^{od} + \sqrt{\frac{gA2^2}{gA2^2 + gB2^2}} \sqrt{gA2^2 + gB2^2} Z_{Ls,j4}^{od} \right) \right) \left( -p_{\mu}^{\sigma_{L,j}^{\pm,*}} + p_{\mu}^{\phi_{L,i}^0} \right) \quad (462)
\end{aligned}$$


---

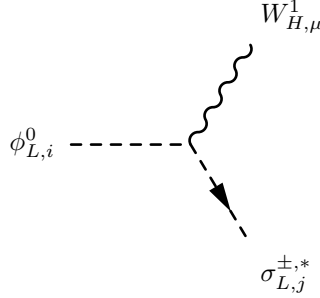

$$\begin{aligned}
& \frac{i}{2} \frac{1}{\sqrt{gA2^2 + gB2^2}} \left( -g_{A2} \sqrt{\frac{gA2^2}{gA2^2 + gB2^2}} \sqrt{gA2^2 + gB2^2} Z_{Ls,i2}^{DR,*} Z_{Ls,j2}^{od} - g_{B2}^2 Z_{Ls,i4}^{DR,*} Z_{Ls,j2}^{od} + g_{B2}^2 Z_{Ls,i2}^{DR,*} Z_{Ls,j3}^{od} \right. \\
& + g_{A2} \sqrt{\frac{gA2^2}{gA2^2 + gB2^2}} \sqrt{gA2^2 + gB2^2} Z_{Ls,i4}^{DR,*} Z_{Ls,j3}^{od} \\
& + Z_{Ls,i3}^{DR,*} \left( g_{A2} \sqrt{\frac{gA2^2}{gA2^2 + gB2^2}} \sqrt{gA2^2 + gB2^2} Z_{Ls,j1}^{od} - g_{B2}^2 Z_{Ls,j4}^{od} \right) \\
& \left. + Z_{Ls,i1}^{DR,*} \left( -g_{A2} \sqrt{\frac{gA2^2}{gA2^2 + gB2^2}} \sqrt{gA2^2 + gB2^2} Z_{Ls,j4}^{od} + g_{B2}^2 Z_{Ls,j1}^{od} \right) \right) \left( -p_{\mu}^{\sigma_{L,j}^{\pm,*}} + p_{\mu}^{\phi_{L,i}^0} \right) \quad (463)
\end{aligned}$$


---

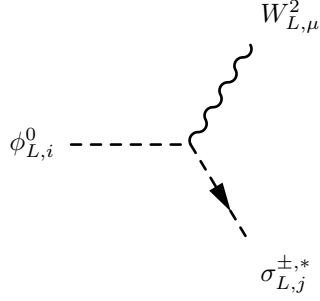

$$\begin{aligned}
& \frac{1}{2} g_{B2} \frac{1}{\sqrt{gA2^2 + gB2^2}} \left( g_{A2} Z_{Ls,i2}^{DR,*} Z_{Ls,j2}^{od} - \sqrt{\frac{gA2^2}{gA2^2 + gB2^2}} \sqrt{gA2^2 + gB2^2} Z_{Ls,i4}^{DR,*} Z_{Ls,j2}^{od} \right. \\
& + \sqrt{\frac{gA2^2}{gA2^2 + gB2^2}} \sqrt{gA2^2 + gB2^2} Z_{Ls,i2}^{DR,*} Z_{Ls,j3}^{od} - g_{A2} Z_{Ls,i4}^{DR,*} Z_{Ls,j3}^{od} \\
& + Z_{Ls,i1}^{DR,*} \left( g_{A2} Z_{Ls,j4}^{od} + \sqrt{\frac{gA2^2}{gA2^2 + gB2^2}} \sqrt{gA2^2 + gB2^2} Z_{Ls,j1}^{od} \right) \\
& \left. - Z_{Ls,i3}^{DR,*} \left( g_{A2} Z_{Ls,j1}^{od} + \sqrt{\frac{gA2^2}{gA2^2 + gB2^2}} \sqrt{gA2^2 + gB2^2} Z_{Ls,j4}^{od} \right) \right) \left( -p_{\mu}^{\sigma_{L,j}^{\pm,*}} + p_{\mu}^{\phi_{L,i}^0} \right) \quad (464)
\end{aligned}$$


---

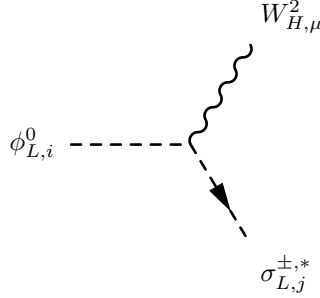

$$\begin{aligned}
& \frac{1}{2} \frac{1}{\sqrt{gA2^2 + gB2^2}} \left( -g_{A2} \sqrt{\frac{gA2^2}{gA2^2 + gB2^2}} \sqrt{gA2^2 + gB2^2} Z_{Ls,i2}^{DR,*} Z_{Ls,j2}^{od} - g_{B2}^2 Z_{Ls,i4}^{DR,*} Z_{Ls,j2}^{od} + g_{B2}^2 Z_{Ls,i2}^{DR,*} Z_{Ls,j3}^{od} \right. \\
& + g_{A2} \sqrt{\frac{gA2^2}{gA2^2 + gB2^2}} \sqrt{gA2^2 + gB2^2} Z_{Ls,i4}^{DR,*} Z_{Ls,j3}^{od} \\
& + Z_{Ls,i3}^{DR,*} \left( g_{A2} \sqrt{\frac{gA2^2}{gA2^2 + gB2^2}} \sqrt{gA2^2 + gB2^2} Z_{Ls,j1}^{od} - g_{B2}^2 Z_{Ls,j4}^{od} \right) \\
& \left. + Z_{Ls,i1}^{DR,*} \left( -g_{A2} \sqrt{\frac{gA2^2}{gA2^2 + gB2^2}} \sqrt{gA2^2 + gB2^2} Z_{Ls,j4}^{od} + g_{B2}^2 Z_{Ls,j1}^{od} \right) \right) \left( -p_{\mu}^{\sigma_{L,j}^{\pm,*}} + p_{\mu}^{\phi_{L,i}^0} \right) \quad (465)
\end{aligned}$$


---

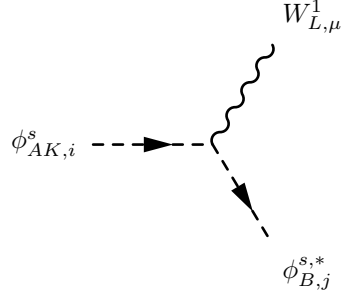

$$i \frac{1}{\sqrt{2}} g_{B2} \sqrt{\frac{g_{A2}^2}{g_{A2}^2 + g_{B2}^2}} Z_{AK,i2}^{s,*} B_{A,j1}^s \left( -p_\mu^{\phi_{B,j}^{s,*}} + p_\mu^{\phi_{AK,i}^s} \right) \quad (466)$$


---

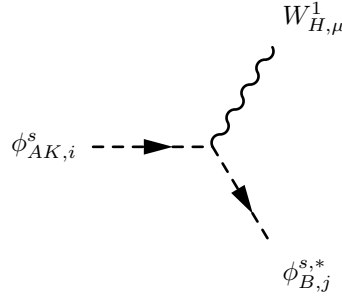

$$i \frac{1}{\sqrt{2}} g_{B2}^2 \frac{1}{\sqrt{g_{A2}^2 + g_{B2}^2}} Z_{AK,i2}^{s,*} B_{A,j1}^s \left( -p_\mu^{\phi_{B,j}^{s,*}} + p_\mu^{\phi_{AK,i}^s} \right) \quad (467)$$


---

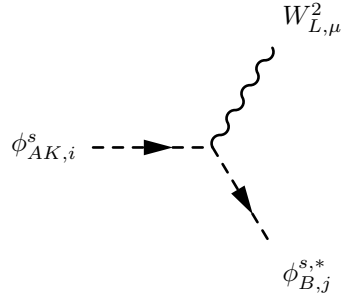

$$\frac{1}{\sqrt{2}} g_{B2} \sqrt{\frac{g_{A2}^2}{g_{A2}^2 + g_{B2}^2}} Z_{AK,i2}^{s,*} B_{A,j1}^s \left( -p_\mu^{\phi_{B,j}^{s,*}} + p_\mu^{\phi_{AK,i}^s} \right) \quad (468)$$


---

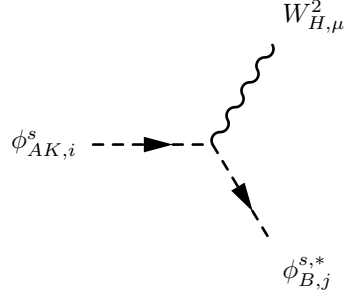

$$\frac{1}{\sqrt{2}}g_{B2}^2\frac{1}{\sqrt{gA2^2+gB2^2}}Z_{AK,i2}^{s,*}B_{A,j1}^s\left(-p_\mu^{\phi_{B,j}^{s,*}}+p_\mu^{\phi_{AK,i}^s}\right) \quad (469)$$


---

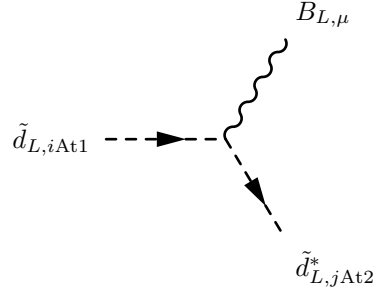

$$-\frac{i}{6}g_{A1}g_{B1}\frac{1}{\sqrt{gA1^2+gB1^2}}\delta_{At1At2}\delta_{ij}\left(-p_\mu^{\tilde{d}_{L,jAt2}^*}+p_\mu^{\tilde{d}_{L,iAt1}}\right) \quad (470)$$


---

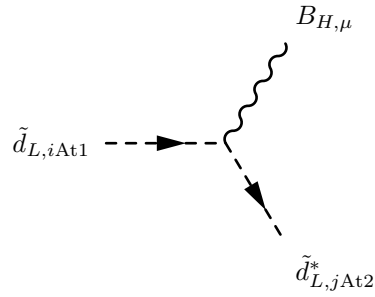

$$\frac{i}{6}g_{A1}\sqrt{\frac{gA1^2}{gA1^2+gB1^2}}\delta_{At1At2}\delta_{ij}\left(-p_\mu^{\tilde{d}_{L,jAt2}^*}+p_\mu^{\tilde{d}_{L,iAt1}}\right) \quad (471)$$


---

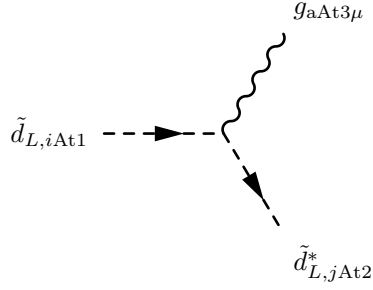

$$-\frac{i}{2}g_3\delta_{ij}\lambda_{\text{At}2,\text{At}1}^{\text{aAt}3}\left(-p_\mu^{\tilde{d}_{L,j\text{At}2}^*}+p_\mu^{\tilde{d}_{L,i\text{At}1}}\right) \quad (472)$$


---

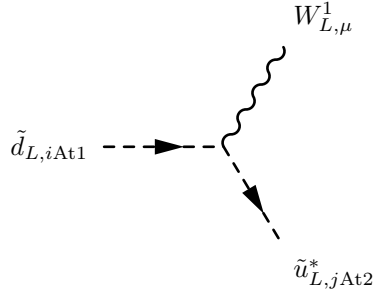

$$-\frac{i}{2}g_{A2}g_{B2}\frac{1}{\sqrt{g_{A2}^2+g_{B2}^2}}\delta_{\text{At}1\text{At}2}\delta_{ij}\left(-p_\mu^{\tilde{u}_{L,j\text{At}2}^*}+p_\mu^{\tilde{d}_{L,i\text{At}1}}\right) \quad (473)$$


---

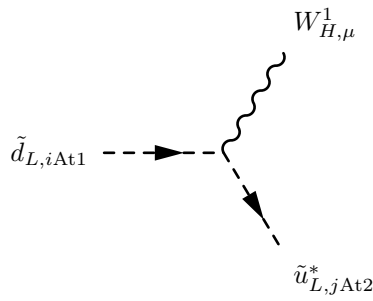

$$\frac{i}{2}g_{A2}\sqrt{\frac{g_{A2}^2}{g_{A2}^2+g_{B2}^2}}\delta_{\text{At}1\text{At}2}\delta_{ij}\left(-p_\mu^{\tilde{u}_{L,j\text{At}2}^*}+p_\mu^{\tilde{d}_{L,i\text{At}1}}\right) \quad (474)$$


---



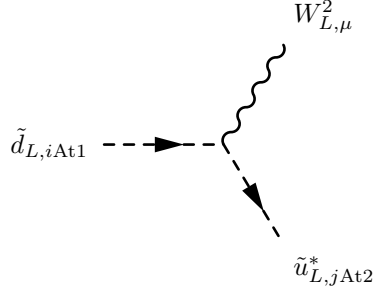

$$-\frac{1}{2}g_{A2}g_{B2}\frac{1}{\sqrt{g_{A2}^2+g_{B2}^2}}\delta_{At1At2}\delta_{ij}\left(-p_{\mu}^{\tilde{u}_{L,jAt2}^*}+p_{\mu}^{\tilde{d}_{L,iAt1}}\right) \quad (475)$$


---

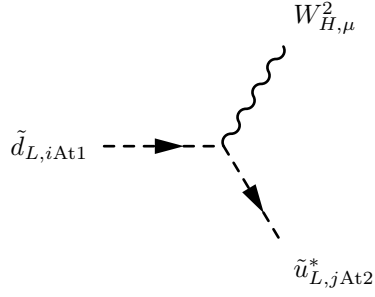

$$\frac{1}{2}g_{A2}\sqrt{\frac{g_{A2}^2}{g_{A2}^2+g_{B2}^2}}\delta_{At1At2}\delta_{ij}\left(-p_{\mu}^{\tilde{u}_{L,jAt2}^*}+p_{\mu}^{\tilde{d}_{L,iAt1}}\right) \quad (476)$$


---

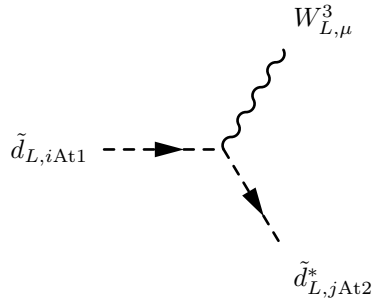

$$\frac{i}{2}g_{A2}g_{B2}\frac{1}{\sqrt{g_{A2}^2+g_{B2}^2}}\delta_{At1At2}\delta_{ij}\left(-p_{\mu}^{\tilde{d}_{L,jAt2}^*}+p_{\mu}^{\tilde{d}_{L,iAt1}}\right) \quad (477)$$


---

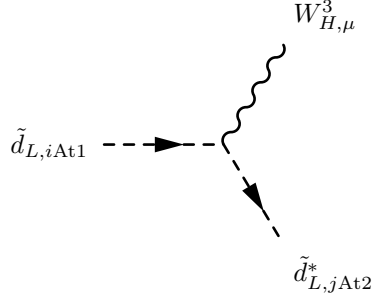

$$-\frac{i}{2}g_{A2}\sqrt{\frac{g_{A2}^2}{g_{A2}^2+g_{B2}^2}}\delta_{At1At2}\delta_{ij}\left(-p_\mu^{\tilde{d}_{L,jAt2}^*}+p_\mu^{\tilde{d}_{L,iAt1}}\right) \quad (478)$$


---

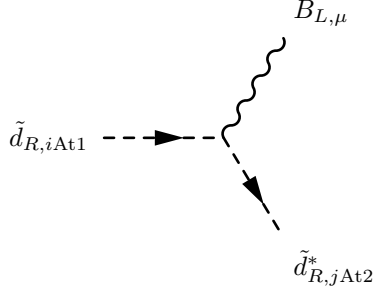

$$\frac{i}{3}g_{A1}g_{B1}\frac{1}{\sqrt{g_{A1}^2+g_{B1}^2}}\delta_{At1At2}\delta_{ij}\left(-p_\mu^{\tilde{d}_{R,jAt2}^*}+p_\mu^{\tilde{d}_{R,iAt1}}\right) \quad (479)$$


---

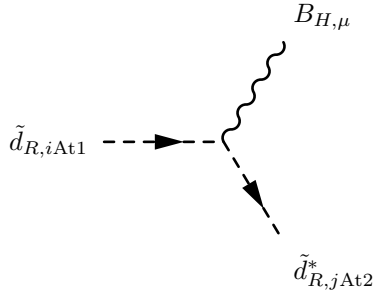

$$-\frac{i}{3}g_{A1}\sqrt{\frac{g_{A1}^2}{g_{A1}^2+g_{B1}^2}}\delta_{At1At2}\delta_{ij}\left(-p_\mu^{\tilde{d}_{R,jAt2}^*}+p_\mu^{\tilde{d}_{R,iAt1}}\right) \quad (480)$$


---

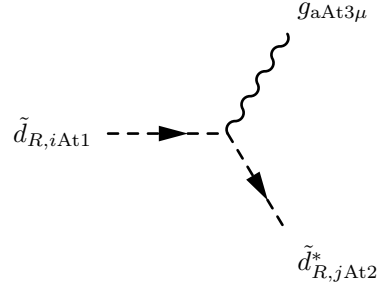

$$-\frac{i}{2}g_3\delta_{ij}\lambda_{\text{At}2,\text{At}1}^{\text{aAt}3}\left(-p_\mu^{\tilde{d}_{R,j\text{At}2}^*}+p_\mu^{\tilde{d}_{R,i\text{At}1}}\right) \quad (481)$$


---

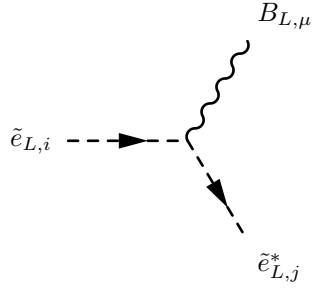

$$\frac{i}{2}g_{A1}g_{B1}\frac{1}{\sqrt{g_{A1}^2+g_{B1}^2}}\delta_{ij}\left(-p_\mu^{\tilde{e}_{L,j}^*}+p_\mu^{\tilde{e}_{L,i}}\right) \quad (482)$$


---

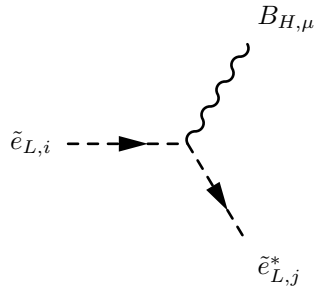

$$-\frac{i}{2}g_{A1}\sqrt{\frac{g_{A1}^2}{g_{A1}^2+g_{B1}^2}}\delta_{ij}\left(-p_\mu^{\tilde{e}_{L,j}^*}+p_\mu^{\tilde{e}_{L,i}}\right) \quad (483)$$


---

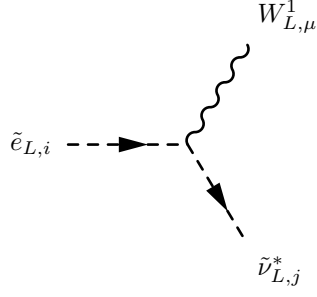

$$-\frac{i}{2}g_{A2}g_{B2}\frac{1}{\sqrt{gA2^2+gB2^2}}\delta_{ij}\left(-p_{\mu}^{\tilde{\nu}_{L,j}^*}+p_{\mu}^{\tilde{e}_{L,i}}\right) \quad (484)$$


---

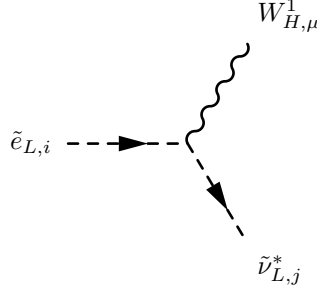

$$\frac{i}{2}g_{A2}\sqrt{\frac{gA2^2}{gA2^2+gB2^2}}\delta_{ij}\left(-p_{\mu}^{\tilde{\nu}_{L,j}^*}+p_{\mu}^{\tilde{e}_{L,i}}\right) \quad (485)$$


---

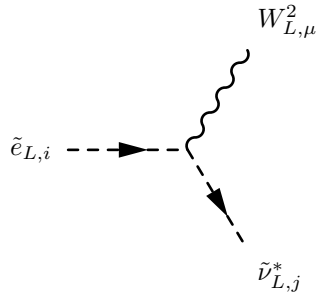

$$-\frac{1}{2}g_{A2}g_{B2}\frac{1}{\sqrt{gA2^2+gB2^2}}\delta_{ij}\left(-p_{\mu}^{\tilde{\nu}_{L,j}^*}+p_{\mu}^{\tilde{e}_{L,i}}\right) \quad (486)$$


---

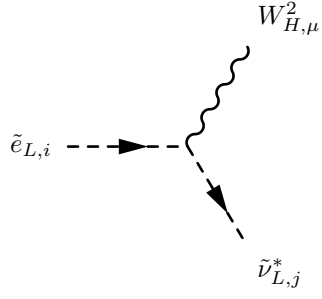

$$\frac{1}{2}g_{A2}\sqrt{\frac{gA2^2}{gA2^2+gB2^2}}\delta_{ij}\left(-p_{\mu}^{\tilde{\nu}_{L,j}^*}+p_{\mu}^{\tilde{e}_{L,i}}\right) \quad (487)$$


---

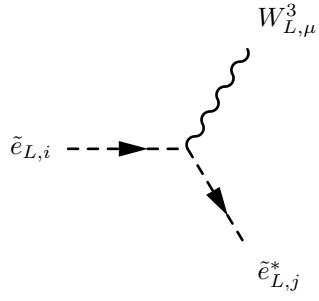

$$\frac{i}{2}g_{A2}g_{B2}\frac{1}{\sqrt{gA2^2+gB2^2}}\delta_{ij}\left(-p_{\mu}^{\tilde{e}_{L,j}^*}+p_{\mu}^{\tilde{e}_{L,i}}\right) \quad (488)$$


---

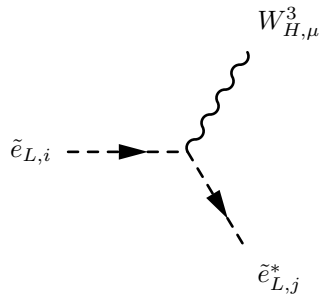

$$-\frac{i}{2}g_{A2}\sqrt{\frac{gA2^2}{gA2^2+gB2^2}}\delta_{ij}\left(-p_{\mu}^{\tilde{e}_{L,j}^*}+p_{\mu}^{\tilde{e}_{L,i}}\right) \quad (489)$$


---

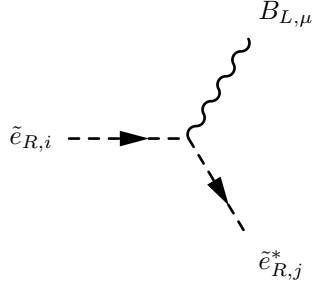

$$ig_{A1}g_{B1}\frac{1}{\sqrt{g_{A1}^2+g_{B1}^2}}\delta_{ij}\left(-p_{\mu}^{\tilde{e}_{R,j}^*}+p_{\mu}^{\tilde{e}_{R,i}}\right) \quad (490)$$


---

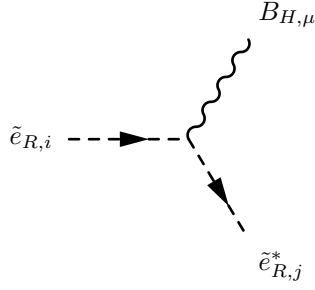

$$-ig_{A1}\sqrt{\frac{g_{A1}^2}{g_{A1}^2+g_{B1}^2}}\delta_{ij}\left(-p_{\mu}^{\tilde{e}_{R,j}^*}+p_{\mu}^{\tilde{e}_{R,i}}\right) \quad (491)$$


---

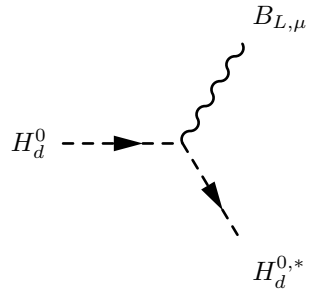

$$\frac{i}{2}g_{A1}g_{B1}\frac{1}{\sqrt{g_{A1}^2+g_{B1}^2}}\left(-p_{\mu}^{H_d^{0,*}}+p_{\mu}^{H_d^0}\right) \quad (492)$$


---

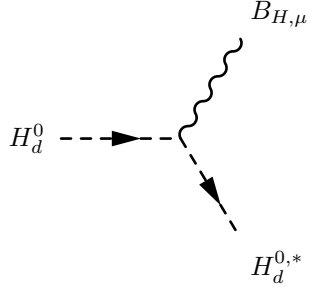

$$-\frac{i}{2}g_{A1}\sqrt{\frac{gA1^2}{gA1^2+gB1^2}}\left(-p_\mu^{H_d^{0,*}}+p_\mu^{H_d^0}\right) \quad (493)$$


---

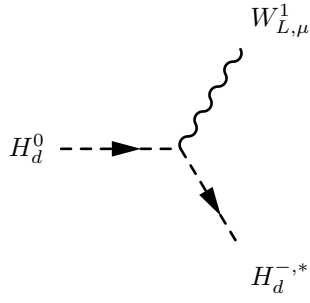

$$-\frac{i}{2}g_{A2}g_{B2}\frac{1}{\sqrt{gA2^2+gB2^2}}\left(-p_\mu^{H_d^{-,*}}+p_\mu^{H_d^0}\right) \quad (494)$$


---

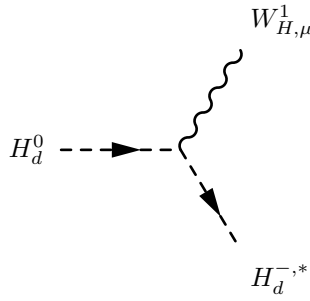

$$\frac{i}{2}g_{A2}\sqrt{\frac{gA2^2}{gA2^2+gB2^2}}\left(-p_\mu^{H_d^{-,*}}+p_\mu^{H_d^0}\right) \quad (495)$$


---

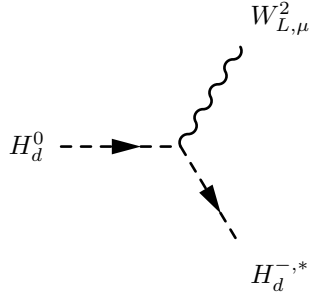

$$\frac{1}{2}g_{A2}g_{B2}\frac{1}{\sqrt{gA2^2+gB2^2}}\left(-p_\mu^{H_d^{-,*}}+p_\mu^{H_d^0}\right) \quad (496)$$


---

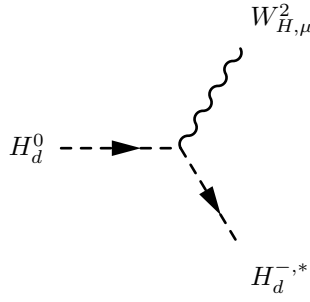

$$-\frac{1}{2}g_{A2}\sqrt{\frac{gA2^2}{gA2^2+gB2^2}}\left(-p_\mu^{H_d^{-,*}}+p_\mu^{H_d^0}\right) \quad (497)$$


---

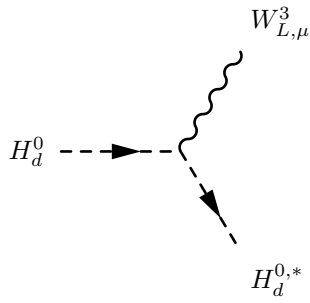

$$-\frac{i}{2}g_{A2}g_{B2}\frac{1}{\sqrt{gA2^2+gB2^2}}\left(-p_\mu^{H_d^{0,*}}+p_\mu^{H_d^0}\right) \quad (498)$$


---



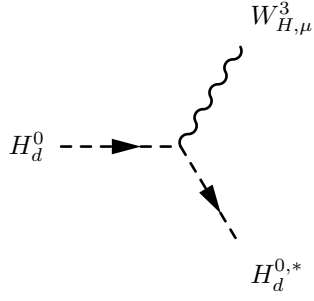

$$\frac{i}{2}g_{A2}\sqrt{\frac{g_{A2}^2}{g_{A2}^2+g_{B2}^2}}\left(-p_\mu^{H_d^{0,*}}+p_\mu^{H_d^0}\right) \quad (499)$$


---

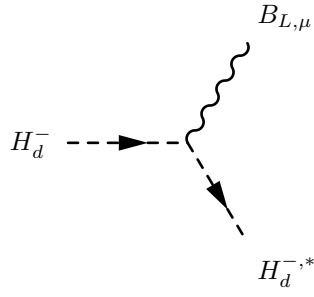

$$\frac{i}{2}g_{A1}g_{B1}\frac{1}{\sqrt{g_{A1}^2+g_{B1}^2}}\left(-p_\mu^{H_d^{-,*}}+p_\mu^{H_d^-}\right) \quad (500)$$


---

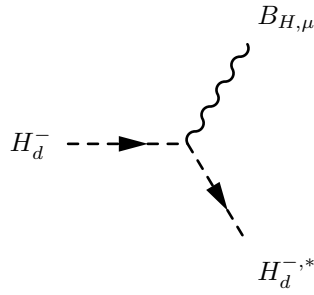

$$-\frac{i}{2}g_{A1}\sqrt{\frac{g_{A1}^2}{g_{A1}^2+g_{B1}^2}}\left(-p_\mu^{H_d^{-,*}}+p_\mu^{H_d^-}\right) \quad (501)$$


---

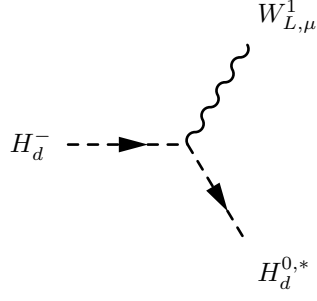

$$-\frac{i}{2}g_{A2}g_{B2}\frac{1}{\sqrt{gA2^2+gB2^2}}\left(-p_\mu^{H_d^{0,*}}+p_\mu^{H_d^-}\right) \quad (502)$$


---

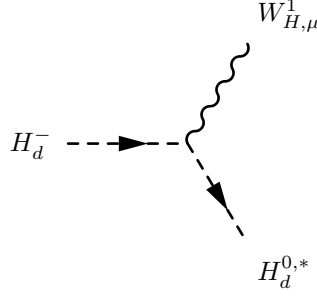

$$\frac{i}{2}g_{A2}\sqrt{\frac{gA2^2}{gA2^2+gB2^2}}\left(-p_\mu^{H_d^{0,*}}+p_\mu^{H_d^-}\right) \quad (503)$$


---

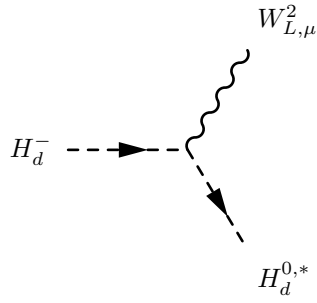

$$-\frac{1}{2}g_{A2}g_{B2}\frac{1}{\sqrt{gA2^2+gB2^2}}\left(-p_\mu^{H_d^{0,*}}+p_\mu^{H_d^-}\right) \quad (504)$$


---

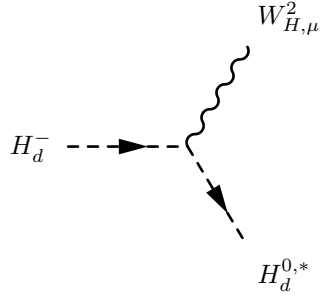

$$\frac{1}{2}g_{A2}\sqrt{\frac{gA2^2}{gA2^2+gB2^2}}\left(-p_\mu^{H_d^{0,*}}+p_\mu^{H_d^-}\right) \quad (505)$$


---

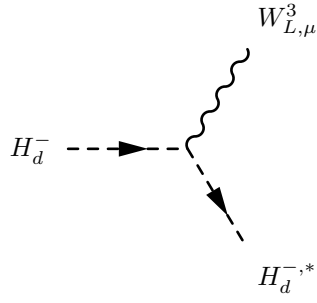

$$\frac{i}{2}g_{A2}g_{B2}\frac{1}{\sqrt{gA2^2+gB2^2}}\left(-p_\mu^{H_d^{-,*}}+p_\mu^{H_d^-}\right) \quad (506)$$


---

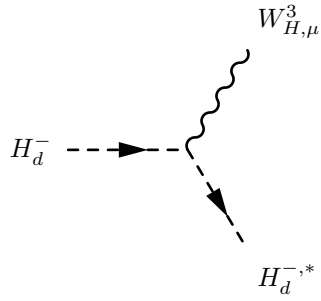

$$-\frac{i}{2}g_{A2}\sqrt{\frac{gA2^2}{gA2^2+gB2^2}}\left(-p_\mu^{H_d^{-,*}}+p_\mu^{H_d^-}\right) \quad (507)$$


---

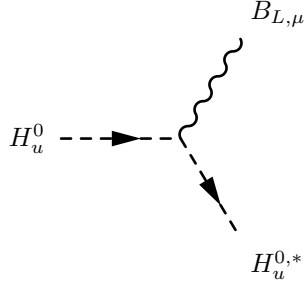

$$-\frac{i}{2}g_{A1}g_{B1}\frac{1}{\sqrt{g_{A1}^2+g_{B1}^2}}\left(-p_\mu^{H_u^{0,*}}+p_\mu^{H_u^0}\right) \quad (508)$$


---

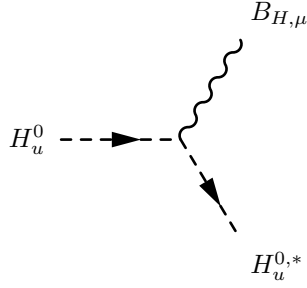

$$\frac{i}{2}g_{A1}\sqrt{\frac{g_{A1}^2}{g_{A1}^2+g_{B1}^2}}\left(-p_\mu^{H_u^{0,*}}+p_\mu^{H_u^0}\right) \quad (509)$$


---

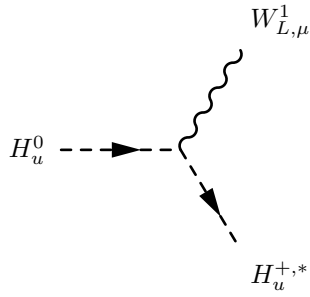

$$-\frac{i}{2}g_{A2}g_{B2}\frac{1}{\sqrt{g_{A2}^2+g_{B2}^2}}\left(-p_\mu^{H_u^{+,*}}+p_\mu^{H_u^0}\right) \quad (510)$$


---

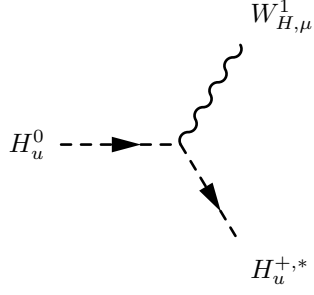

$$\frac{i}{2}g_{A2}\sqrt{\frac{gA2^2}{gA2^2+gB2^2}}\left(-p_\mu^{H_u^{+,*}}+p_\mu^{H_u^0}\right) \quad (511)$$


---

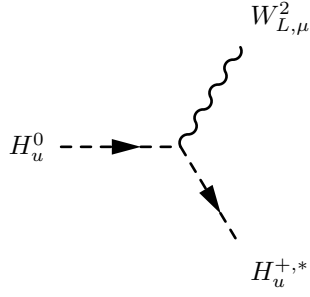

$$-\frac{1}{2}g_{A2}g_{B2}\frac{1}{\sqrt{gA2^2+gB2^2}}\left(-p_\mu^{H_u^{+,*}}+p_\mu^{H_u^0}\right) \quad (512)$$


---

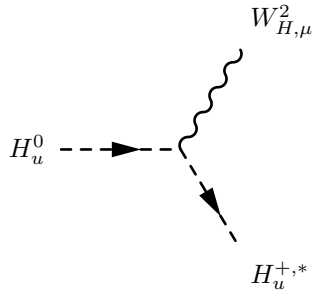

$$\frac{1}{2}g_{A2}\sqrt{\frac{gA2^2}{gA2^2+gB2^2}}\left(-p_\mu^{H_u^{+,*}}+p_\mu^{H_u^0}\right) \quad (513)$$


---

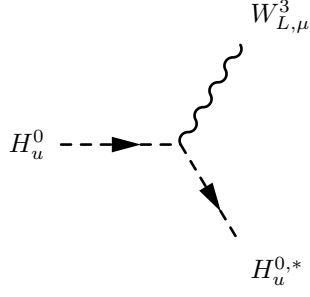

$$\frac{i}{2} g_{A2} g_{B2} \frac{1}{\sqrt{g_{A2}^2 + g_{B2}^2}} \left( -p_\mu^{H_u^{0,*}} + p_\mu^{H_u^0} \right) \quad (514)$$


---

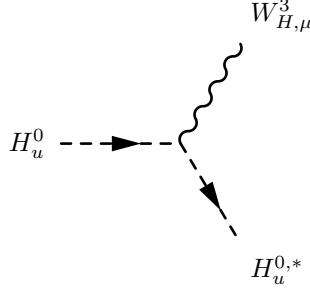

$$-\frac{i}{2} g_{A2} \sqrt{\frac{g_{A2}^2}{g_{A2}^2 + g_{B2}^2}} \left( -p_\mu^{H_u^{0,*}} + p_\mu^{H_u^0} \right) \quad (515)$$


---

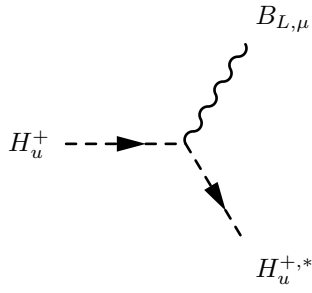

$$-\frac{i}{2} g_{A1} g_{B1} \frac{1}{\sqrt{g_{A1}^2 + g_{B1}^2}} \left( -p_\mu^{H_u^{+,*}} + p_\mu^{H_u^+} \right) \quad (516)$$


---

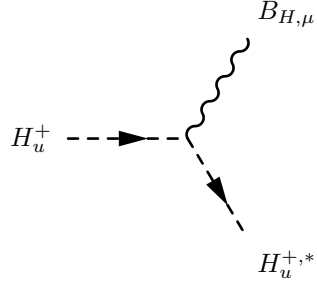

$$\frac{i}{2}g_{A1}\sqrt{\frac{gA1^2}{gA1^2+gB1^2}}\left(-p_\mu^{H_u^{+,*}}+p_\mu^{H_u^+}\right) \quad (517)$$


---

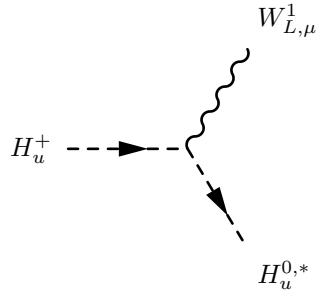

$$-\frac{i}{2}g_{A2}g_{B2}\frac{1}{\sqrt{gA2^2+gB2^2}}\left(-p_\mu^{H_u^{0,*}}+p_\mu^{H_u^+}\right) \quad (518)$$


---

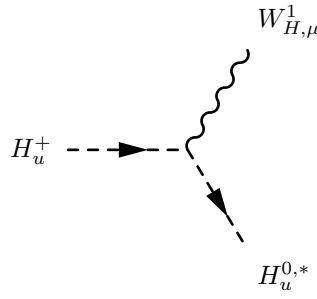

$$\frac{i}{2}g_{A2}\sqrt{\frac{gA2^2}{gA2^2+gB2^2}}\left(-p_\mu^{H_u^{0,*}}+p_\mu^{H_u^+}\right) \quad (519)$$


---

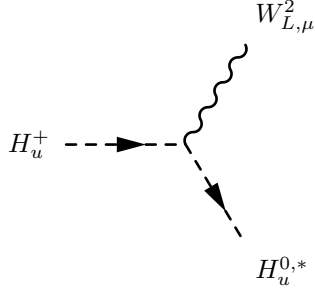

$$\frac{1}{2}g_{A2}g_{B2}\frac{1}{\sqrt{gA2^2+gB2^2}}\left(-p_\mu^{H_u^{0,*}}+p_\mu^{H_u^+}\right) \quad (520)$$


---

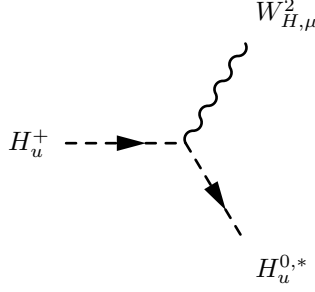

$$-\frac{1}{2}g_{A2}\sqrt{\frac{gA2^2}{gA2^2+gB2^2}}\left(-p_\mu^{H_u^{0,*}}+p_\mu^{H_u^+}\right) \quad (521)$$


---

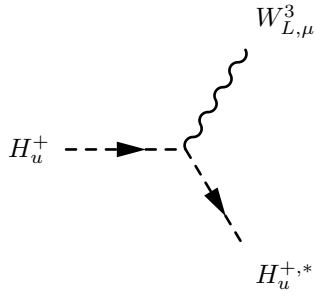

$$-\frac{i}{2}g_{A2}g_{B2}\frac{1}{\sqrt{gA2^2+gB2^2}}\left(-p_\mu^{H_u^{+,*}}+p_\mu^{H_u^+}\right) \quad (522)$$


---



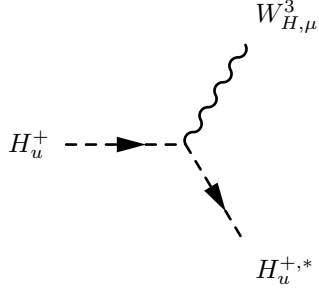

$$\frac{i}{2} g_{A2} \sqrt{\frac{gA2^2}{gA2^2 + gB2^2}} \left( -p_\mu^{H_u^{+,*}} + p_\mu^{H_u^+} \right) \quad (523)$$


---

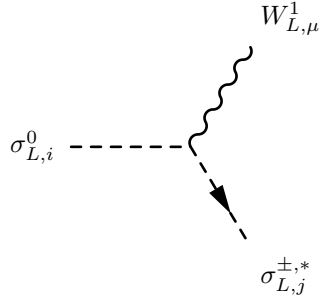

$$\begin{aligned}
 & \frac{1}{2} g_{B2} \frac{1}{\sqrt{gA2^2 + gB2^2}} \left( -g_{A2} Z_{Ls,i2}^{Di,*} Z_{Ls,j2}^{od} + \sqrt{\frac{gA2^2}{gA2^2 + gB2^2}} \sqrt{gA2^2 + gB2^2} Z_{Ls,i4}^{Di,*} Z_{Ls,j2}^{od} \right. \\
 & + \sqrt{\frac{gA2^2}{gA2^2 + gB2^2}} \sqrt{gA2^2 + gB2^2} Z_{Ls,i2}^{Di,*} Z_{Ls,j3}^{od} - g_{A2} Z_{Ls,i4}^{Di,*} Z_{Ls,j3}^{od} \\
 & + Z_{Ls,i1}^{Di,*} \left( g_{A2} Z_{Ls,j4}^{od} - \sqrt{\frac{gA2^2}{gA2^2 + gB2^2}} \sqrt{gA2^2 + gB2^2} Z_{Ls,j1}^{od} \right) \\
 & \left. + Z_{Ls,i3}^{Di,*} \left( g_{A2} Z_{Ls,j1}^{od} - \sqrt{\frac{gA2^2}{gA2^2 + gB2^2}} \sqrt{gA2^2 + gB2^2} Z_{Ls,j4}^{od} \right) \right) \left( -p_\mu^{\sigma_{L,j}^{\pm,*}} + p_\mu^{\sigma_{L,i}^0} \right) \quad (524)
 \end{aligned}$$


---

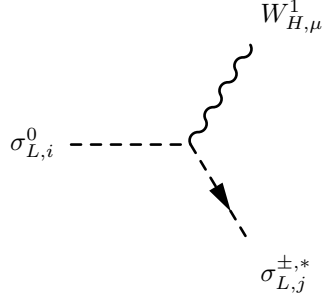

$$\begin{aligned}
& \frac{1}{2} \frac{1}{\sqrt{gA^2 + gB^2}} \left( gA^2 \sqrt{\frac{gA^2}{gA^2 + gB^2}} \sqrt{gA^2 + gB^2} Z_{Ls,i2}^{Di,*} Z_{Ls,j2}^{od} + g_{B2}^2 Z_{Ls,i4}^{Di,*} Z_{Ls,j2}^{od} + g_{B2}^2 Z_{Ls,i2}^{Di,*} Z_{Ls,j3}^{od} \right. \\
& + gA^2 \sqrt{\frac{gA^2}{gA^2 + gB^2}} \sqrt{gA^2 + gB^2} Z_{Ls,i4}^{Di,*} Z_{Ls,j3}^{od} \\
& - Z_{Ls,i3}^{Di,*} \left( gA^2 \sqrt{\frac{gA^2}{gA^2 + gB^2}} \sqrt{gA^2 + gB^2} Z_{Ls,j1}^{od} + g_{B2}^2 Z_{Ls,j4}^{od} \right) \\
& \left. - Z_{Ls,i1}^{Di,*} \left( gA^2 \sqrt{\frac{gA^2}{gA^2 + gB^2}} \sqrt{gA^2 + gB^2} Z_{Ls,j4}^{od} + g_{B2}^2 Z_{Ls,j1}^{od} \right) \right) \left( -p_\mu^{\sigma_{L,j}^{\pm,*}} + p_\mu^{\sigma_{L,i}^0} \right) \quad (525)
\end{aligned}$$


---

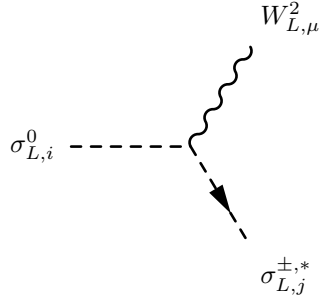

$$\begin{aligned}
& \frac{i}{2} g_{B2} \frac{1}{\sqrt{gA^2 + gB^2}} \left( gA^2 Z_{Ls,i2}^{Di,*} Z_{Ls,j2}^{od} - \sqrt{\frac{gA^2}{gA^2 + gB^2}} \sqrt{gA^2 + gB^2} Z_{Ls,i4}^{Di,*} Z_{Ls,j2}^{od} \right. \\
& - \sqrt{\frac{gA^2}{gA^2 + gB^2}} \sqrt{gA^2 + gB^2} Z_{Ls,i2}^{Di,*} Z_{Ls,j3}^{od} + gA^2 Z_{Ls,i4}^{Di,*} Z_{Ls,j3}^{od} \\
& + Z_{Ls,i1}^{Di,*} \left( -gA^2 Z_{Ls,j4}^{od} + \sqrt{\frac{gA^2}{gA^2 + gB^2}} \sqrt{gA^2 + gB^2} Z_{Ls,j1}^{od} \right) \\
& \left. + Z_{Ls,i3}^{Di,*} \left( -gA^2 Z_{Ls,j1}^{od} + \sqrt{\frac{gA^2}{gA^2 + gB^2}} \sqrt{gA^2 + gB^2} Z_{Ls,j4}^{od} \right) \right) \left( -p_\mu^{\sigma_{L,j}^{\pm,*}} + p_\mu^{\sigma_{L,i}^0} \right) \quad (526)
\end{aligned}$$


---

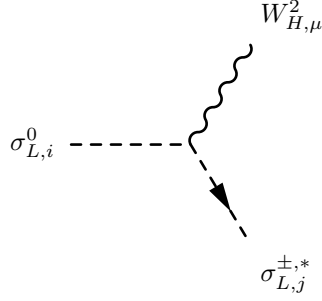

$$\begin{aligned}
& \frac{i}{2} \frac{1}{\sqrt{gA2^2 + gB2^2}} \left( -gA2 \sqrt{\frac{gA2^2}{gA2^2 + gB2^2}} \sqrt{gA2^2 + gB2^2} Z_{Ls,i2}^{Di,*} Z_{Ls,j2}^{od} - g_{B2}^2 Z_{Ls,i4}^{Di,*} Z_{Ls,j2}^{od} - g_{B2}^2 Z_{Ls,i2}^{Di,*} Z_{Ls,j3}^{od} \right. \\
& - gA2 \sqrt{\frac{gA2^2}{gA2^2 + gB2^2}} \sqrt{gA2^2 + gB2^2} Z_{Ls,i4}^{Di,*} Z_{Ls,j3}^{od} \\
& + Z_{Ls,i3}^{Di,*} \left( gA2 \sqrt{\frac{gA2^2}{gA2^2 + gB2^2}} \sqrt{gA2^2 + gB2^2} Z_{Ls,j1}^{od} + g_{B2}^2 Z_{Ls,j4}^{od} \right) \\
& \left. + Z_{Ls,i1}^{Di,*} \left( gA2 \sqrt{\frac{gA2^2}{gA2^2 + gB2^2}} \sqrt{gA2^2 + gB2^2} Z_{Ls,j4}^{od} + g_{B2}^2 Z_{Ls,j1}^{od} \right) \right) \left( -p_{\mu}^{\sigma_{L,j}^{\pm,*}} + p_{\mu}^{\sigma_{L,i}^0} \right) \quad (527)
\end{aligned}$$


---

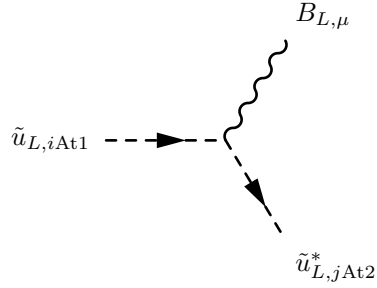

$$-\frac{i}{6} g_{A1} g_{B1} \frac{1}{\sqrt{gA1^2 + gB1^2}} \delta_{At1At2} \delta_{ij} \left( -p_{\mu}^{\tilde{u}_{L,jAt2}^*} + p_{\mu}^{\tilde{u}_{L,iAt1}} \right) \quad (528)$$


---

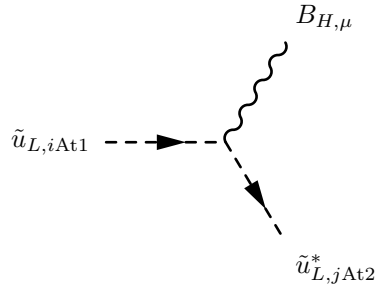

$$\frac{i}{6}g_{A1}\sqrt{\frac{g_{A1}^2}{g_{A1}^2+g_{B1}^2}}\delta_{At1At2}\delta_{ij}\left(-p_\mu^{\tilde{u}_{L,jAt2}^*}+p_\mu^{\tilde{u}_{L,iAt1}}\right) \quad (529)$$


---

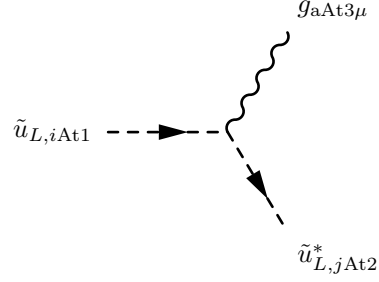

$$-\frac{i}{2}g_3\delta_{ij}\lambda_{At2,At1}^{aAt3}\left(-p_\mu^{\tilde{u}_{L,jAt2}^*}+p_\mu^{\tilde{u}_{L,iAt1}}\right) \quad (530)$$


---

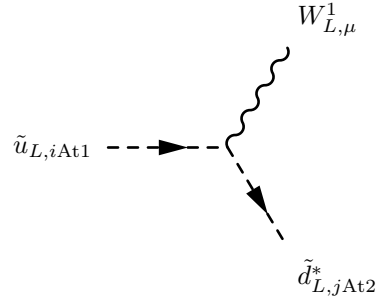

$$-\frac{i}{2}g_{A2}g_{B2}\frac{1}{\sqrt{g_{A2}^2+g_{B2}^2}}\delta_{At1At2}\delta_{ij}\left(-p_\mu^{\tilde{d}_{L,jAt2}^*}+p_\mu^{\tilde{u}_{L,iAt1}}\right) \quad (531)$$


---

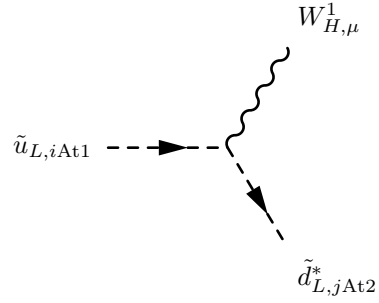

$$\frac{i}{2}g_{A2}\sqrt{\frac{g_{A2}^2}{g_{A2}^2+g_{B2}^2}}\delta_{At1At2}\delta_{ij}\left(-p_\mu^{\tilde{d}_{L,jAt2}^*}+p_\mu^{\tilde{u}_{L,iAt1}}\right) \quad (532)$$


---

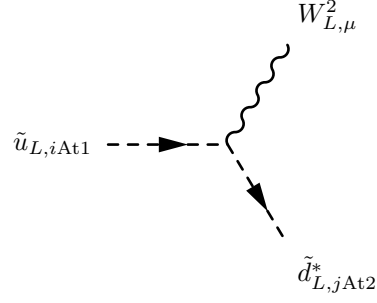

$$\frac{1}{2}g_{A2}g_{B2}\frac{1}{\sqrt{g_{A2}^2+g_{B2}^2}}\delta_{\text{At}1\text{At}2}\delta_{ij}\left(-p_{\mu}^{\tilde{d}_{L,j\text{At}2}^*}+p_{\mu}^{\tilde{u}_{L,i\text{At}1}}\right) \quad (533)$$


---

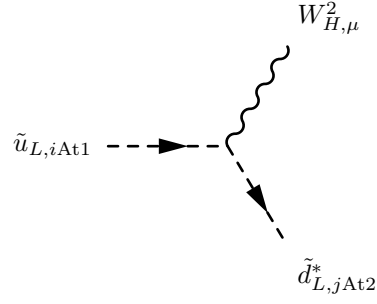

$$-\frac{1}{2}g_{A2}\sqrt{\frac{g_{A2}^2}{g_{A2}^2+g_{B2}^2}}\delta_{\text{At}1\text{At}2}\delta_{ij}\left(-p_{\mu}^{\tilde{d}_{L,j\text{At}2}^*}+p_{\mu}^{\tilde{u}_{L,i\text{At}1}}\right) \quad (534)$$


---

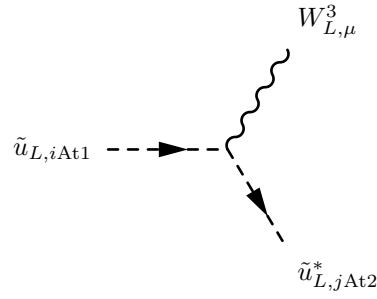

$$-\frac{i}{2}g_{A2}g_{B2}\frac{1}{\sqrt{g_{A2}^2+g_{B2}^2}}\delta_{\text{At}1\text{At}2}\delta_{ij}\left(-p_{\mu}^{\tilde{u}_{L,j\text{At}2}^*}+p_{\mu}^{\tilde{u}_{L,i\text{At}1}}\right) \quad (535)$$


---

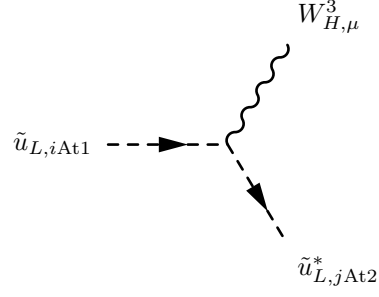

$$\frac{i}{2} g_{A2} \sqrt{\frac{g_{A2}^2}{g_{A2}^2 + g_{B2}^2}} \delta_{At1At2} \delta_{ij} \left( -p_\mu^{\tilde{u}_{L,jAt2}^*} + p_\mu^{\tilde{u}_{L,iAt1}} \right) \quad (536)$$


---

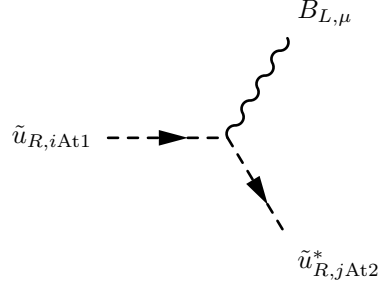

$$-\frac{2i}{3} g_{A1} g_{B1} \frac{1}{\sqrt{g_{A1}^2 + g_{B1}^2}} \delta_{At1At2} \delta_{ij} \left( -p_\mu^{\tilde{u}_{R,jAt2}^*} + p_\mu^{\tilde{u}_{R,iAt1}} \right) \quad (537)$$


---

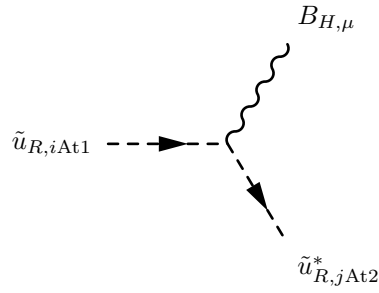

$$\frac{2i}{3} g_{A1} \sqrt{\frac{g_{A1}^2}{g_{A1}^2 + g_{B1}^2}} \delta_{At1At2} \delta_{ij} \left( -p_\mu^{\tilde{u}_{R,jAt2}^*} + p_\mu^{\tilde{u}_{R,iAt1}} \right) \quad (538)$$


---

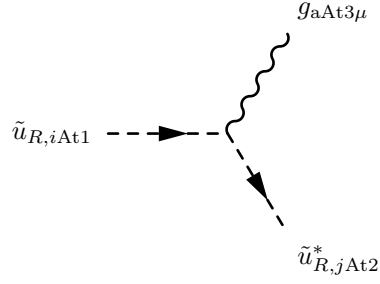

$$-\frac{i}{2}g_3\delta_{ij}\lambda_{\text{At}2,\text{At}1}^{\text{aAt}3}\left(-p_\mu^{\tilde{u}_{R,j\text{At}2}^*}+p_\mu^{\tilde{u}_{R,i\text{At}1}}\right) \quad (539)$$


---

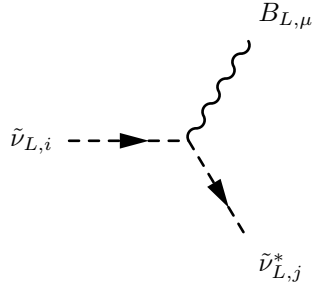

$$\frac{i}{2}g_{A1}g_{B1}\frac{1}{\sqrt{g_{A1}^2+g_{B1}^2}}\delta_{ij}\left(-p_\mu^{\tilde{\nu}_{L,j}^*}+p_\mu^{\tilde{\nu}_{L,i}}\right) \quad (540)$$


---

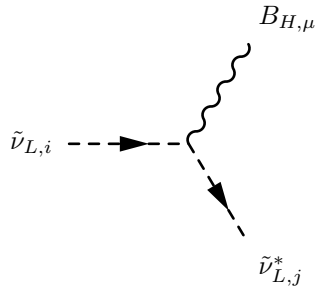

$$-\frac{i}{2}g_{A1}\sqrt{\frac{g_{A1}^2}{g_{A1}^2+g_{B1}^2}}\delta_{ij}\left(-p_\mu^{\tilde{\nu}_{L,j}^*}+p_\mu^{\tilde{\nu}_{L,i}}\right) \quad (541)$$


---

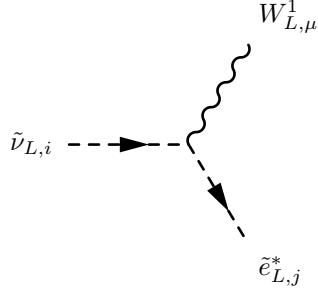

$$-\frac{i}{2}g_{A2}g_{B2}\frac{1}{\sqrt{gA2^2+gB2^2}}\delta_{ij}\left(-p_{\mu}^{\tilde{e}_{L,j}^*}+p_{\mu}^{\tilde{\nu}_{L,i}}\right) \quad (542)$$


---

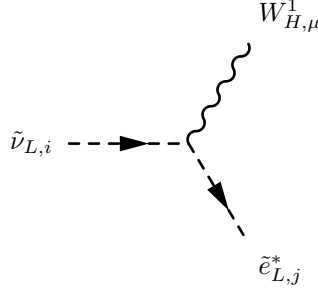

$$\frac{i}{2}g_{A2}\sqrt{\frac{gA2^2}{gA2^2+gB2^2}}\delta_{ij}\left(-p_{\mu}^{\tilde{e}_{L,j}^*}+p_{\mu}^{\tilde{\nu}_{L,i}}\right) \quad (543)$$


---

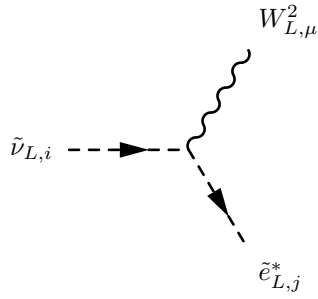

$$\frac{1}{2}g_{A2}g_{B2}\frac{1}{\sqrt{gA2^2+gB2^2}}\delta_{ij}\left(-p_{\mu}^{\tilde{e}_{L,j}^*}+p_{\mu}^{\tilde{\nu}_{L,i}}\right) \quad (544)$$


---



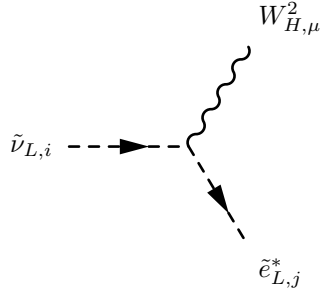

$$-\frac{1}{2}g_{A2}\sqrt{\frac{gA2^2}{gA2^2+gB2^2}}\delta_{ij}\left(-p_{\mu}^{\tilde{e}_{L,j}^*}+p_{\mu}^{\tilde{\nu}_{L,i}}\right) \quad (545)$$


---

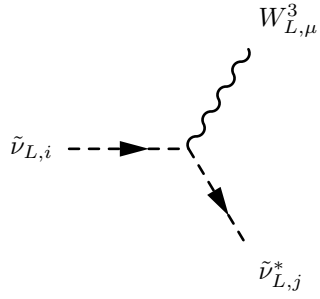

$$-\frac{i}{2}g_{A2}g_{B2}\frac{1}{\sqrt{gA2^2+gB2^2}}\delta_{ij}\left(-p_{\mu}^{\tilde{\nu}_{L,j}^*}+p_{\mu}^{\tilde{\nu}_{L,i}}\right) \quad (546)$$


---

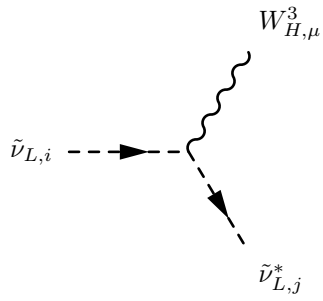

$$\frac{i}{2}g_{A2}\sqrt{\frac{gA2^2}{gA2^2+gB2^2}}\delta_{ij}\left(-p_{\mu}^{\tilde{\nu}_{L,j}^*}+p_{\mu}^{\tilde{\nu}_{L,i}}\right) \quad (547)$$


---

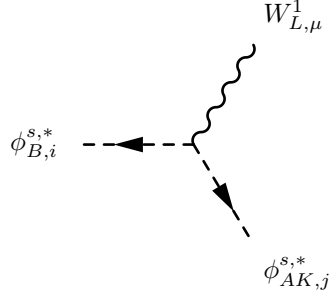

$$-i \frac{1}{\sqrt{2}} g_{B2} \sqrt{\frac{gA2^2}{gA2^2 + gB2^2}} Z_{AK,j2}^s B_{A,i2}^s \left( -p_\mu^{\phi_{AK,j}^{s,*}} + p_\mu^{\phi_{B,i}^{s,*}} \right) \quad (548)$$


---

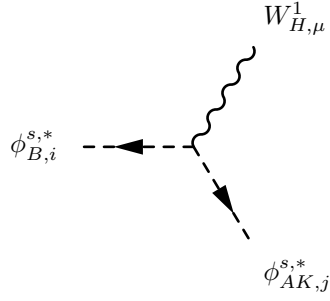

$$-i \frac{1}{\sqrt{2}} g_{B2}^2 \frac{1}{\sqrt{gA2^2 + gB2^2}} Z_{AK,j2}^s B_{A,i2}^s \left( -p_\mu^{\phi_{AK,j}^{s,*}} + p_\mu^{\phi_{B,i}^{s,*}} \right) \quad (549)$$


---

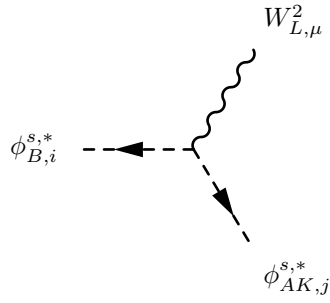

$$- \frac{1}{\sqrt{2}} g_{B2} \sqrt{\frac{gA2^2}{gA2^2 + gB2^2}} Z_{AK,j2}^s B_{A,i2}^s \left( -p_\mu^{\phi_{AK,j}^{s,*}} + p_\mu^{\phi_{B,i}^{s,*}} \right) \quad (550)$$


---

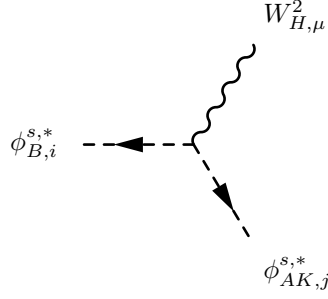

$$-\frac{1}{\sqrt{2}}g_{B2}^2\frac{1}{\sqrt{g_{A2}^2+g_{B2}^2}}Z_{AK,j2}^sB_{A,i2}^s\left(-p_\mu^{\phi_{AK,j}^{s,*}}+p_\mu^{\phi_{B,i}^{s,*}}\right) \quad (551)$$


---

### 9.3 One Scalar-Two Vector Boson-Interaction

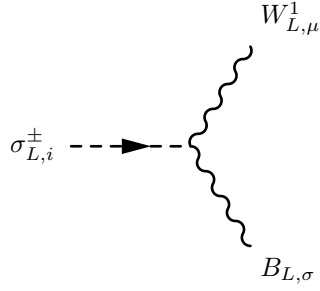

$$-\frac{i}{2}g_{B1}\frac{1}{\sqrt{g_{A1}^2+g_{B1}^2}}\left(-g_{A1}+\sqrt{\frac{g_{A1}^2}{g_{A1}^2+g_{B1}^2}}\sqrt{g_{A1}^2+g_{B1}^2}\right)g_{B2}\frac{1}{\sqrt{g_{A2}^2+g_{B2}^2}}\left(-g_{A2}+\sqrt{\frac{g_{A2}^2}{g_{A2}^2+g_{B2}^2}}\sqrt{g_{A2}^2+g_{B2}^2}\right)v_{Lv}\left(Z_{Ls,i1}^{od,*}+Z_{Ls,i2}^{od,*}\right) \quad (552)$$


---

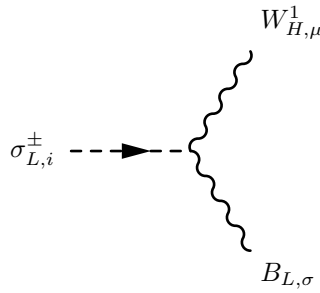

$$-\frac{i}{2}g_{B1}\frac{1}{\sqrt{g_{A1}^2+g_{B1}^2}}\left(-g_{A1}+\sqrt{\frac{g_{A1}^2}{g_{A1}^2+g_{B1}^2}}\sqrt{g_{A1}^2+g_{B1}^2}\right)\frac{1}{\sqrt{g_{A2}^2+g_{B2}^2}}\left(g_{A2}\sqrt{\frac{g_{A2}^2}{g_{A2}^2+g_{B2}^2}}\sqrt{g_{A2}^2+g_{B2}^2}+g_{B2}\right)v_{Lv}\left(Z_{Ls,i1}^{od,*}+Z_{Ls,i2}^{od,*}+Z_{Ls,i3}^{od,*}\right) \quad (553)$$


---

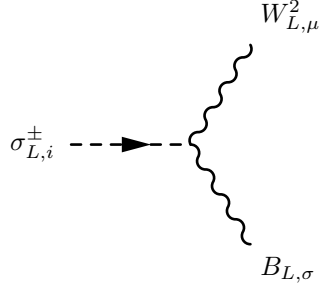

$$\frac{1}{2}g_{B1}\frac{1}{\sqrt{g_{A1}^2+g_{B1}^2}}\left(-g_{A1}+\sqrt{\frac{g_{A1}^2}{g_{A1}^2+g_{B1}^2}}\sqrt{g_{A1}^2+g_{B1}^2}\right)g_{B2}\frac{1}{\sqrt{g_{A2}^2+g_{B2}^2}}\left(-g_{A2}+\sqrt{\frac{g_{A2}^2}{g_{A2}^2+g_{B2}^2}}\sqrt{g_{A2}^2+g_{B2}^2}\right)v_{Lv}\left(Z_{Ls,i1}^{od,*}+Z_{Ls,i2}^{od,*}+Z_{Ls,i3}^{od,*}\right) \quad (554)$$


---

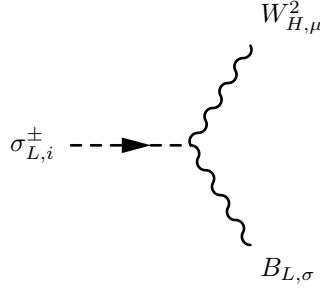

$$\frac{1}{2}g_{B1}\frac{1}{\sqrt{g_{A1}^2+g_{B1}^2}}\left(-g_{A1}+\sqrt{\frac{g_{A1}^2}{g_{A1}^2+g_{B1}^2}}\sqrt{g_{A1}^2+g_{B1}^2}\right)\frac{1}{\sqrt{g_{A2}^2+g_{B2}^2}}\left(g_{A2}\sqrt{\frac{g_{A2}^2}{g_{A2}^2+g_{B2}^2}}\sqrt{g_{A2}^2+g_{B2}^2}+g_{B2}^2\right)v_{Lv}\left(Z_{Ls,i1}^{od,*}+Z_{Ls,i2}^{od,*}+Z_{Ls,i3}^{od,*}\right) \quad (555)$$


---

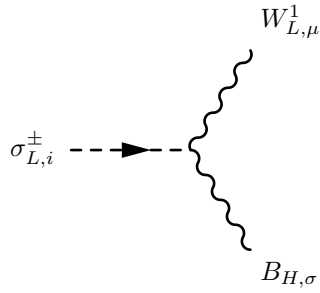

$$-\frac{i}{2}\frac{1}{\sqrt{g_{A1}^2+g_{B1}^2}}\left(g_{A1}\sqrt{\frac{g_{A1}^2}{g_{A1}^2+g_{B1}^2}}\sqrt{g_{A1}^2+g_{B1}^2}+g_{B1}^2\right)g_{B2}\frac{1}{\sqrt{g_{A2}^2+g_{B2}^2}}\left(-g_{A2}+\sqrt{\frac{g_{A2}^2}{g_{A2}^2+g_{B2}^2}}\sqrt{g_{A2}^2+g_{B2}^2}\right)v_{Lv}\left(Z_{Ls,i1}^{od,*}+Z_{Ls,i2}^{od,*}+Z_{Ls,i3}^{od,*}\right) \quad (556)$$


---

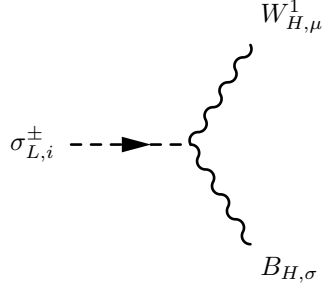

$$-\frac{i}{2} \frac{1}{\sqrt{g_{A1}^2 + g_{B1}^2}} \left( g_{A1} \sqrt{\frac{g_{A1}^2}{g_{A1}^2 + g_{B1}^2}} \sqrt{g_{A1}^2 + g_{B1}^2 + g_{B1}^2} \right) \frac{1}{\sqrt{g_{A2}^2 + g_{B2}^2}} \left( g_{A2} \sqrt{\frac{g_{A2}^2}{g_{A2}^2 + g_{B2}^2}} \sqrt{g_{A2}^2 + g_{B2}^2 + g_{B2}^2} \right) v_{Lv} \left( Z_{Ls,i1}^{od,*} + Z_{Ls,i2}^{od,*} + Z_{Ls}^{od,*} \right) \quad (557)$$


---

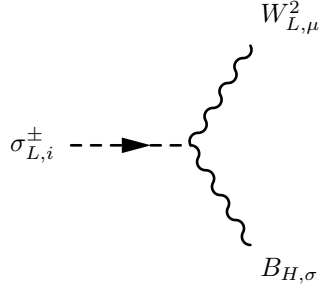

$$\frac{1}{2} \frac{1}{\sqrt{g_{A1}^2 + g_{B1}^2}} \left( g_{A1} \sqrt{\frac{g_{A1}^2}{g_{A1}^2 + g_{B1}^2}} \sqrt{g_{A1}^2 + g_{B1}^2 + g_{B1}^2} \right) g_{B2} \frac{1}{\sqrt{g_{A2}^2 + g_{B2}^2}} \left( -g_{A2} + \sqrt{\frac{g_{A2}^2}{g_{A2}^2 + g_{B2}^2}} \sqrt{g_{A2}^2 + g_{B2}^2 + g_{B2}^2} \right) v_{Lv} \left( Z_{Ls,i1}^{od,*} + Z_{Ls,i2}^{od,*} + Z_{Ls}^{od,*} \right) \quad (558)$$


---

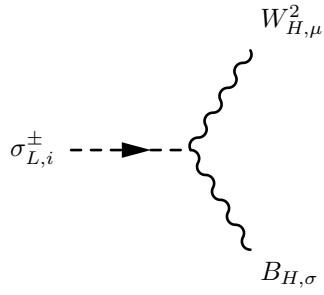

$$\frac{1}{2} \frac{1}{\sqrt{g_{A1}^2 + g_{B1}^2}} \left( g_{A1} \sqrt{\frac{g_{A1}^2}{g_{A1}^2 + g_{B1}^2}} \sqrt{g_{A1}^2 + g_{B1}^2 + g_{B1}^2} \right) \frac{1}{\sqrt{g_{A2}^2 + g_{B2}^2}} \left( g_{A2} \sqrt{\frac{g_{A2}^2}{g_{A2}^2 + g_{B2}^2}} \sqrt{g_{A2}^2 + g_{B2}^2 + g_{B2}^2} \right) v_{Lv} \left( Z_{Ls,i1}^{od,*} + Z_{Ls,i2}^{od,*} + Z_{Ls,i3}^{od,*} \right) \quad (559)$$


---

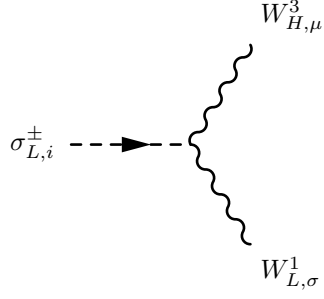

$$\frac{i}{2} g_{A2} g_{B2} v_{Lv} \left( -Z_{Ls,i2}^{od,*} - Z_{Ls,i4}^{od,*} + Z_{Ls,i1}^{od,*} + Z_{Ls,i3}^{od,*} \right) (g_{\sigma\mu}) \quad (560)$$


---

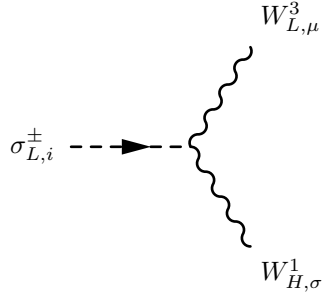

$$-\frac{i}{2} g_{A2} g_{B2} v_{Lv} \left( -Z_{Ls,i2}^{od,*} - Z_{Ls,i4}^{od,*} + Z_{Ls,i1}^{od,*} + Z_{Ls,i3}^{od,*} \right) (g_{\sigma\mu}) \quad (561)$$


---

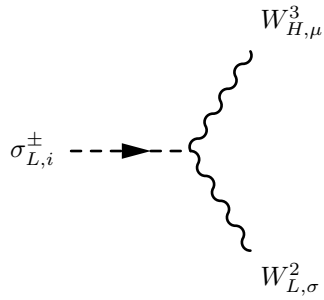

$$\frac{1}{2} g_{A2} g_{B2} v_{Lv} \left( -Z_{Ls,i1}^{od,*} - Z_{Ls,i3}^{od,*} + Z_{Ls,i2}^{od,*} + Z_{Ls,i4}^{od,*} \right) (g_{\sigma\mu}) \quad (562)$$


---

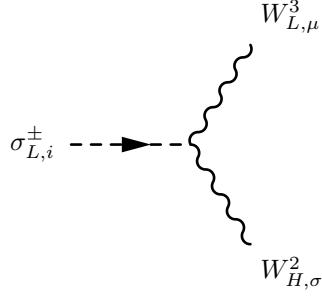

$$\frac{1}{2} g_{A2} g_{B2} v_{Lv} \left( -Z_{Ls,i2}^{od,*} - Z_{Ls,i4}^{od,*} + Z_{Ls,i1}^{od,*} + Z_{Ls,i3}^{od,*} \right) (g_{\sigma\mu}) \quad (563)$$


---

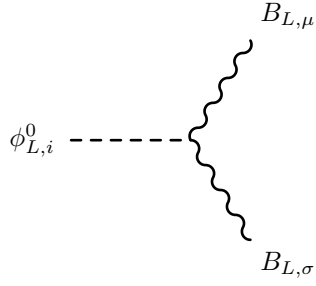

$$-2ig_{A1}g_{B1}^2 \frac{1}{\left(g_{A1}^2 + g_{B1}^2\right)^{3/2}} \left( g_{A1}^2 \sqrt{\frac{g_{A1}^2}{g_{A1}^2 + g_{B1}^2}} - g_{A1} \sqrt{g_{A1}^2 + g_{B1}^2} + g_{B1}^2 \sqrt{\frac{g_{A1}^2}{g_{A1}^2 + g_{B1}^2}} \right) v_{Lv} \left( Z_{Ls,i1}^{DR,*} + Z_{Ls,i2}^{DR,*} + Z_{Ls,i3}^{DR,*} + Z_{Ls,i4}^{DR,*} \right) (g_{\sigma\mu}) \quad (564)$$


---

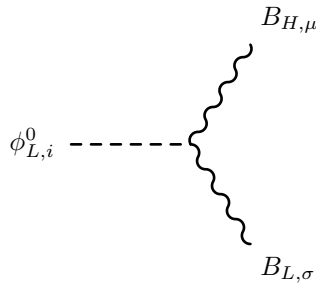

$$ig_{B1} \left( -g_{A1}^2 + g_{B1}^2 \right) \frac{1}{\left(g_{A1}^2 + g_{B1}^2\right)^{3/2}} \left( g_{A1}^2 \sqrt{\frac{g_{A1}^2}{g_{A1}^2 + g_{B1}^2}} - g_{A1} \sqrt{g_{A1}^2 + g_{B1}^2} + g_{B1}^2 \sqrt{\frac{g_{A1}^2}{g_{A1}^2 + g_{B1}^2}} \right) v_{Lv} \left( Z_{Ls,i1}^{DR,*} + Z_{Ls,i2}^{DR,*} + Z_{Ls,i3}^{DR,*} + Z_{Ls,i4}^{DR,*} \right) (g_{\sigma\mu}) \quad (565)$$


---

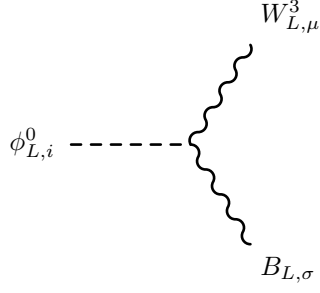

$$-ig_{B1} \frac{1}{\sqrt{g_{A1}^2 + g_{B1}^2}} \left( -g_{A1} + \sqrt{\frac{g_{A1}^2}{g_{A1}^2 + g_{B1}^2}} \sqrt{g_{A1}^2 + g_{B1}^2} \right) g_{B2} \frac{1}{\sqrt{g_{A2}^2 + g_{B2}^2}} \left( -g_{A2} + \sqrt{\frac{g_{A2}^2}{g_{A2}^2 + g_{B2}^2}} \sqrt{g_{A2}^2 + g_{B2}^2} \right) v_{Lv} \left( -Z_{Ls,i3}^{DR,*} - Z_{Ls,i4}^{DR,*} \right) \quad (566)$$


---

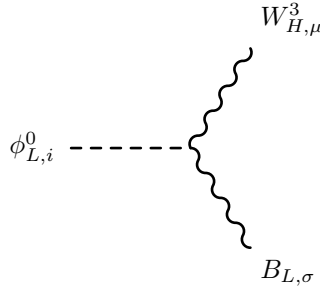

$$-ig_{B1} \frac{1}{\sqrt{g_{A1}^2 + g_{B1}^2}} \left( -g_{A1} + \sqrt{\frac{g_{A1}^2}{g_{A1}^2 + g_{B1}^2}} \sqrt{g_{A1}^2 + g_{B1}^2} \right) \frac{1}{\sqrt{g_{A2}^2 + g_{B2}^2}} \left( g_{A2} \sqrt{\frac{g_{A2}^2}{g_{A2}^2 + g_{B2}^2}} \sqrt{g_{A2}^2 + g_{B2}^2} + g_{B2}^2 \right) v_{Lv} \left( -Z_{Ls,i3}^{DR,*} - Z_{Ls,i4}^{DR,*} \right) \quad (567)$$


---

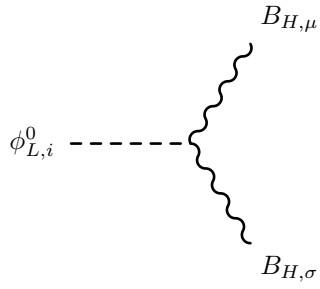

$$i \frac{1}{\left( g_{A1}^2 + g_{B1}^2 \right)^{3/2}} \left( 2g_{A1}^3 g_{B1}^2 \sqrt{\frac{g_{A1}^2}{g_{A1}^2 + g_{B1}^2}} + 2g_{A1} g_{B1}^4 \sqrt{\frac{g_{A1}^2}{g_{A1}^2 + g_{B1}^2}} + g_{A1}^4 \sqrt{g_{A1}^2 + g_{B1}^2} \right)$$



$$+ g_{B1}^4 \sqrt{g_{A1}^2 + g_{B1}^2} \Big) v_{Lv} \Big( Z_{Ls,i1}^{DR,*} + Z_{Ls,i2}^{DR,*} + Z_{Ls,i3}^{DR,*} + Z_{Ls,i4}^{DR,*} \Big) \Big( g_{\sigma\mu} \Big) \quad (568)$$


---

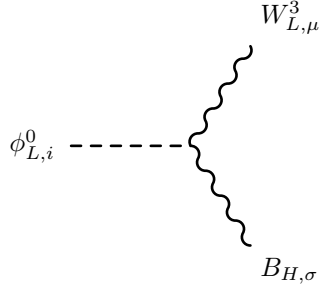

$$- i \frac{1}{\sqrt{g_{A1}^2 + g_{B1}^2}} \Big( g_{A1} \sqrt{\frac{g_{A1}^2}{g_{A1}^2 + g_{B1}^2}} \sqrt{g_{A1}^2 + g_{B1}^2} + g_{B1}^2 \Big) g_{B2} \frac{1}{\sqrt{g_{A2}^2 + g_{B2}^2}} \Big( -g_{A2} + \sqrt{\frac{g_{A2}^2}{g_{A2}^2 + g_{B2}^2}} \sqrt{g_{A2}^2 + g_{B2}^2} \Big) v_{Lv} \Big( -Z_{Ls,i3}^{DR,*} - Z_{Ls,i4}^{DR,*} \Big) \quad (569)$$


---

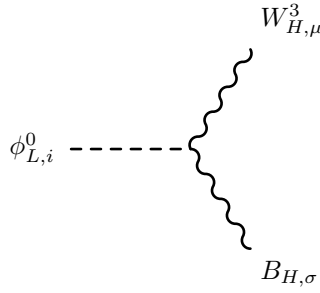

$$- i \frac{1}{\sqrt{g_{A1}^2 + g_{B1}^2}} \Big( g_{A1} \sqrt{\frac{g_{A1}^2}{g_{A1}^2 + g_{B1}^2}} \sqrt{g_{A1}^2 + g_{B1}^2} + g_{B1}^2 \Big) \frac{1}{\sqrt{g_{A2}^2 + g_{B2}^2}} \Big( g_{A2} \sqrt{\frac{g_{A2}^2}{g_{A2}^2 + g_{B2}^2}} \sqrt{g_{A2}^2 + g_{B2}^2} + g_{B2}^2 \Big) v_{Lv} \Big( -Z_{Ls,i3}^{DR,*} - Z_{Ls,i4}^{DR,*} + Z_{Ls,i1}^{DR,*} + Z_{Ls,i2}^{DR,*} \Big) \quad (570)$$


---

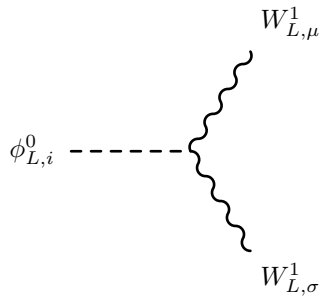

$$-2ig_{A2}g_{B2}^2 \frac{1}{\left(g_{A2}^2 + g_{B2}^2\right)^{3/2}} \left(g_{A2}^2 \sqrt{\frac{g_{A2}^2}{g_{A2}^2 + g_{B2}^2}} - g_{A2} \sqrt{g_{A2}^2 + g_{B2}^2} + g_{B2}^2 \sqrt{\frac{g_{A2}^2}{g_{A2}^2 + g_{B2}^2}}\right) v_{Lv} \left(Z_{Ls,i1}^{DR,*} + Z_{Ls,i2}^{DR,*} + Z_{Ls,i3}^{DR,*} + Z_{Ls,i4}^{DR,*}\right) (g_{\sigma\mu})$$


---

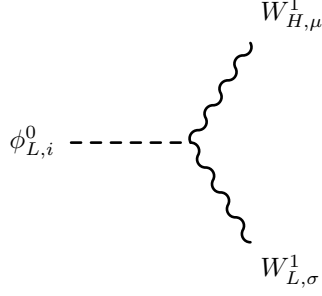

$$ig_{B2} \left(-g_{A2}^2 + g_{B2}^2\right) \frac{1}{\left(g_{A2}^2 + g_{B2}^2\right)^{3/2}} \left(g_{A2}^2 \sqrt{\frac{g_{A2}^2}{g_{A2}^2 + g_{B2}^2}} - g_{A2} \sqrt{g_{A2}^2 + g_{B2}^2} + g_{B2}^2 \sqrt{\frac{g_{A2}^2}{g_{A2}^2 + g_{B2}^2}}\right) v_{Lv} \left(Z_{Ls,i1}^{DR,*} + Z_{Ls,i2}^{DR,*} + Z_{Ls,i3}^{DR,*} + Z_{Ls,i4}^{DR,*}\right)$$


---

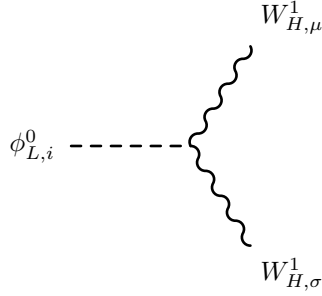

$$i \frac{1}{\left(g_{A2}^2 + g_{B2}^2\right)^{3/2}} \left(2g_{A2}^3 g_{B2}^2 \sqrt{\frac{g_{A2}^2}{g_{A2}^2 + g_{B2}^2}} + 2g_{A2} g_{B2}^4 \sqrt{\frac{g_{A2}^2}{g_{A2}^2 + g_{B2}^2}} + g_{A2}^4 \sqrt{g_{A2}^2 + g_{B2}^2} + g_{B2}^4 \sqrt{g_{A2}^2 + g_{B2}^2}\right) v_{Lv} \left(Z_{Ls,i1}^{DR,*} + Z_{Ls,i2}^{DR,*} + Z_{Ls,i3}^{DR,*} + Z_{Ls,i4}^{DR,*}\right) (g_{\sigma\mu})$$


---

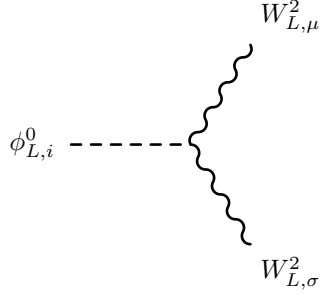

$$-2ig_{A2}g_{B2}^2 \frac{1}{(g_{A2}^2 + g_{B2}^2)^{3/2}} \left( g_{A2}^2 \sqrt{\frac{g_{A2}^2}{g_{A2}^2 + g_{B2}^2}} - g_{A2} \sqrt{g_{A2}^2 + g_{B2}^2} + g_{B2}^2 \sqrt{\frac{g_{A2}^2}{g_{A2}^2 + g_{B2}^2}} \right) v_{Lv} \left( Z_{Ls,i1}^{DR,*} + Z_{Ls,i2}^{DR,*} + Z_{Ls,i3}^{DR,*} + Z_{Ls,i4}^{DR,*} \right) (g_{\sigma\mu})$$

(574)

---

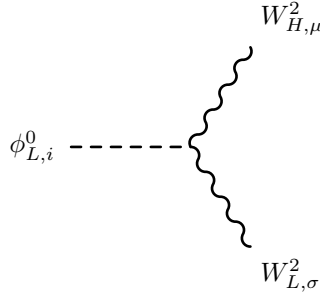

$$ig_{B2} \left( -g_{A2}^2 + g_{B2}^2 \right) \frac{1}{(g_{A2}^2 + g_{B2}^2)^{3/2}} \left( g_{A2}^2 \sqrt{\frac{g_{A2}^2}{g_{A2}^2 + g_{B2}^2}} - g_{A2} \sqrt{g_{A2}^2 + g_{B2}^2} + g_{B2}^2 \sqrt{\frac{g_{A2}^2}{g_{A2}^2 + g_{B2}^2}} \right) v_{Lv} \left( Z_{Ls,i1}^{DR,*} + Z_{Ls,i2}^{DR,*} + Z_{Ls,i3}^{DR,*} + Z_{Ls,i4}^{DR,*} \right)$$

(575)

---

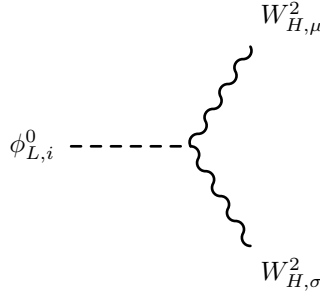

$$\begin{aligned}
& i \frac{1}{\left(g_{A2}^2 + g_{B2}^2\right)^{3/2}} \left( 2g_{A2}^3 g_{B2}^2 \sqrt{\frac{g_{A2}^2}{g_{A2}^2 + g_{B2}^2}} + 2g_{A2} g_{B2}^4 \sqrt{\frac{g_{A2}^2}{g_{A2}^2 + g_{B2}^2}} + g_{A2}^4 \sqrt{g_{A2}^2 + g_{B2}^2} \right. \\
& \left. + g_{B2}^4 \sqrt{g_{A2}^2 + g_{B2}^2} \right) v_{Lv} \left( Z_{Ls,i1}^{DR,*} + Z_{Ls,i2}^{DR,*} + Z_{Ls,i3}^{DR,*} + Z_{Ls,i4}^{DR,*} \right) (g_{\sigma\mu})
\end{aligned} \tag{576}$$


---

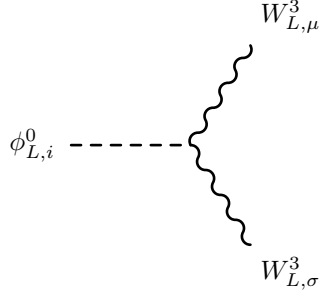

$$\begin{aligned}
& -2ig_{A2} g_{B2}^2 \frac{1}{\left(g_{A2}^2 + g_{B2}^2\right)^{3/2}} \left( g_{A2}^2 \sqrt{\frac{g_{A2}^2}{g_{A2}^2 + g_{B2}^2}} - g_{A2} \sqrt{g_{A2}^2 + g_{B2}^2} + g_{B2}^2 \sqrt{\frac{g_{A2}^2}{g_{A2}^2 + g_{B2}^2}} \right) v_{Lv} \left( Z_{Ls,i1}^{DR,*} + Z_{Ls,i2}^{DR,*} + Z_{Ls,i3}^{DR,*} + Z_{Ls,i4}^{DR,*} \right) (g_{\sigma\mu})
\end{aligned} \tag{577}$$


---

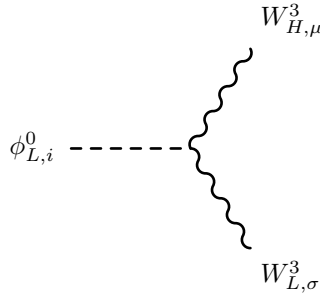

$$\begin{aligned}
& ig_{B2} \left( -g_{A2}^2 + g_{B2}^2 \right) \frac{1}{\left(g_{A2}^2 + g_{B2}^2\right)^{3/2}} \left( g_{A2}^2 \sqrt{\frac{g_{A2}^2}{g_{A2}^2 + g_{B2}^2}} - g_{A2} \sqrt{g_{A2}^2 + g_{B2}^2} + g_{B2}^2 \sqrt{\frac{g_{A2}^2}{g_{A2}^2 + g_{B2}^2}} \right) v_{Lv} \left( Z_{Ls,i1}^{DR,*} + Z_{Ls,i2}^{DR,*} + Z_{Ls,i3}^{DR,*} + Z_{Ls,i4}^{DR,*} \right) (g_{\sigma\mu})
\end{aligned} \tag{578}$$


---

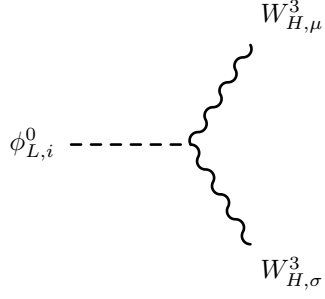

$$\begin{aligned}
& i \frac{1}{\left(g_{A2}^2 + g_{B2}^2\right)^{3/2}} \left( 2g_{A2}^3 g_{B2}^2 \sqrt{\frac{g_{A2}^2}{g_{A2}^2 + g_{B2}^2}} + 2g_{A2} g_{B2}^4 \sqrt{\frac{g_{A2}^2}{g_{A2}^2 + g_{B2}^2}} + g_{A2}^4 \sqrt{g_{A2}^2 + g_{B2}^2} \right. \\
& \left. + g_{B2}^4 \sqrt{g_{A2}^2 + g_{B2}^2} \right) v_{Lv} \left( Z_{Ls,i1}^{DR,*} + Z_{Ls,i2}^{DR,*} + Z_{Ls,i3}^{DR,*} + Z_{Ls,i4}^{DR,*} \right) (g_{\sigma\mu})
\end{aligned} \tag{579}$$


---

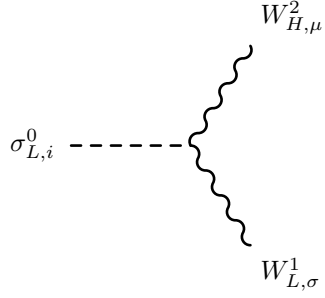

$$-ig_{A2}g_{B2}v_{Lv} \left( -Z_{Ls,i2}^{Di,*} - Z_{Ls,i3}^{Di,*} + Z_{Ls,i1}^{Di,*} + Z_{Ls,i4}^{Di,*} \right) (g_{\sigma\mu}) \tag{580}$$


---

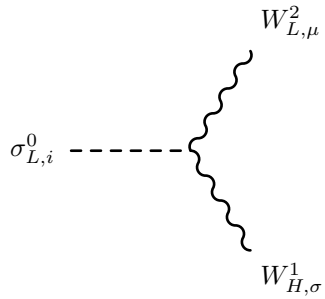

$$ig_{A2}g_{B2}v_{Lv} \left( -Z_{Ls,i2}^{Di,*} - Z_{Ls,i3}^{Di,*} + Z_{Ls,i1}^{Di,*} + Z_{Ls,i4}^{Di,*} \right) (g_{\sigma\mu}) \tag{581}$$


---

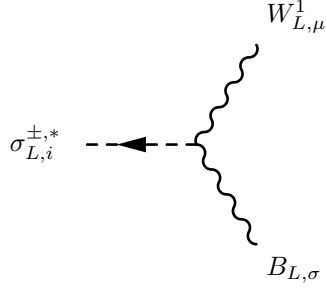

$$-\frac{i}{2}g_{B1}\frac{1}{\sqrt{g_{A1}^2+g_{B1}^2}}\left(-g_{A1}+\sqrt{\frac{g_{A1}^2}{g_{A1}^2+g_{B1}^2}}\sqrt{g_{A1}^2+g_{B1}^2}\right)g_{B2}\frac{1}{\sqrt{g_{A2}^2+g_{B2}^2}}\left(-g_{A2}+\sqrt{\frac{g_{A2}^2}{g_{A2}^2+g_{B2}^2}}\sqrt{g_{A2}^2+g_{B2}^2}\right)v_{Lv}\left(Z_{Ls,i1}^{od}+Z_{Ls,i2}^{od}\right) \quad (582)$$


---

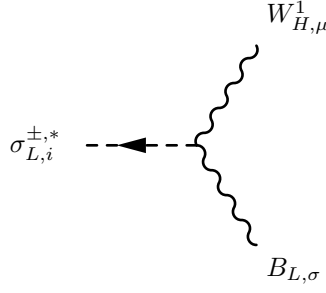

$$-\frac{i}{2}g_{B1}\frac{1}{\sqrt{g_{A1}^2+g_{B1}^2}}\left(-g_{A1}+\sqrt{\frac{g_{A1}^2}{g_{A1}^2+g_{B1}^2}}\sqrt{g_{A1}^2+g_{B1}^2}\right)\frac{1}{\sqrt{g_{A2}^2+g_{B2}^2}}\left(g_{A2}\sqrt{\frac{g_{A2}^2}{g_{A2}^2+g_{B2}^2}}\sqrt{g_{A2}^2+g_{B2}^2}+g_{B2}^2\right)v_{Lv}\left(Z_{Ls,i1}^{od}+Z_{Ls,i2}^{od}+Z_{Ls,i3}^{od}\right) \quad (583)$$


---

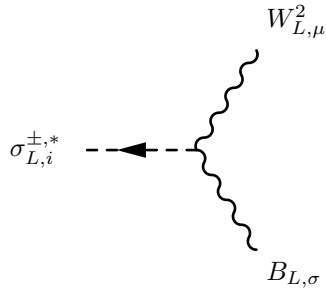

$$-\frac{1}{2}g_{B1}\frac{1}{\sqrt{g_{A1}^2+g_{B1}^2}}\left(-g_{A1}+\sqrt{\frac{g_{A1}^2}{g_{A1}^2+g_{B1}^2}}\sqrt{g_{A1}^2+g_{B1}^2}\right)g_{B2}\frac{1}{\sqrt{g_{A2}^2+g_{B2}^2}}\left(-g_{A2}+\sqrt{\frac{g_{A2}^2}{g_{A2}^2+g_{B2}^2}}\sqrt{g_{A2}^2+g_{B2}^2}\right)v_{Lv}\left(Z_{Ls,i1}^{od}+Z_{Ls,i2}^{od}\right) \quad (584)$$


---

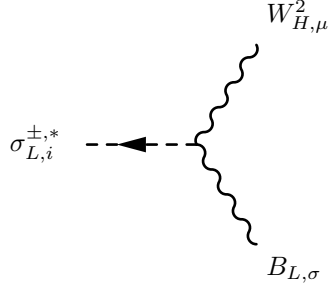

$$-\frac{1}{2}g_{B1}\frac{1}{\sqrt{g_{A1}^2+g_{B1}^2}}\left(-g_{A1}+\sqrt{\frac{g_{A1}^2}{g_{A1}^2+g_{B1}^2}}\sqrt{g_{A1}^2+g_{B1}^2}\right)\frac{1}{\sqrt{g_{A2}^2+g_{B2}^2}}\left(g_{A2}\sqrt{\frac{g_{A2}^2}{g_{A2}^2+g_{B2}^2}}\sqrt{g_{A2}^2+g_{B2}^2}+g_{B2}^2\right)v_{Lv}\left(Z_{Ls,i1}^{od}+Z_{Ls,i2}^{od}+Z_{Ls,i3}^{od}\right) \quad (585)$$


---

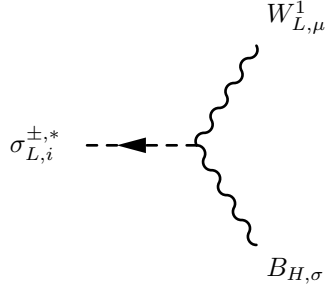

$$-\frac{i}{2}\frac{1}{\sqrt{g_{A1}^2+g_{B1}^2}}\left(g_{A1}\sqrt{\frac{g_{A1}^2}{g_{A1}^2+g_{B1}^2}}\sqrt{g_{A1}^2+g_{B1}^2}+g_{B1}^2\right)g_{B2}\frac{1}{\sqrt{g_{A2}^2+g_{B2}^2}}\left(-g_{A2}+\sqrt{\frac{g_{A2}^2}{g_{A2}^2+g_{B2}^2}}\sqrt{g_{A2}^2+g_{B2}^2}\right)v_{Lv}\left(Z_{Ls,i1}^{od}+Z_{Ls,i2}^{od}+Z_{Ls,i3}^{od}\right) \quad (586)$$


---

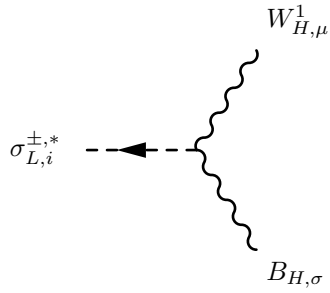

$$-\frac{i}{2}\frac{1}{\sqrt{g_{A1}^2+g_{B1}^2}}\left(g_{A1}\sqrt{\frac{g_{A1}^2}{g_{A1}^2+g_{B1}^2}}\sqrt{g_{A1}^2+g_{B1}^2}+g_{B1}^2\right)\frac{1}{\sqrt{g_{A2}^2+g_{B2}^2}}\left(g_{A2}\sqrt{\frac{g_{A2}^2}{g_{A2}^2+g_{B2}^2}}\sqrt{g_{A2}^2+g_{B2}^2}+g_{B2}^2\right)v_{Lv}\left(Z_{Ls,i1}^{od}+Z_{Ls,i2}^{od}+Z_{Ls,i3}^{od}\right) \quad (587)$$


---

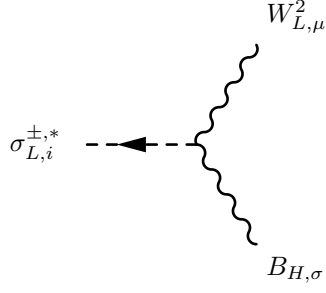

$$-\frac{1}{2} \frac{1}{\sqrt{g_{A1}^2 + g_{B1}^2}} \left( g_{A1} \sqrt{\frac{g_{A1}^2}{g_{A1}^2 + g_{B1}^2}} \sqrt{g_{A1}^2 + g_{B1}^2 + g_{B1}^2} \right) g_{B2} \frac{1}{\sqrt{g_{A2}^2 + 2}} \left( -g_{A2} + \sqrt{\frac{g_{A2}^2}{g_{A2}^2 + g_{B2}^2}} \sqrt{g_{A2}^2 + g_{B2}^2} \right) v_{Lv} \left( Z_{Ls,i1}^{od} + Z_{Ls,i2}^{od} + Z_{Ls,i3}^{od} \right) \quad (588)$$


---

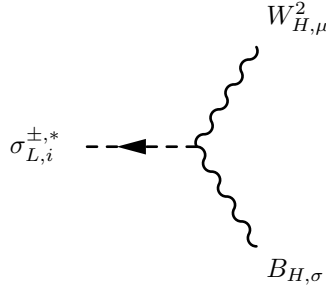

$$-\frac{1}{2} \frac{1}{\sqrt{g_{A1}^2 + g_{B1}^2}} \left( g_{A1} \sqrt{\frac{g_{A1}^2}{g_{A1}^2 + g_{B1}^2}} \sqrt{g_{A1}^2 + g_{B1}^2 + g_{B1}^2} \right) \frac{1}{\sqrt{g_{A2}^2 + g_{B2}^2}} \left( g_{A2} \sqrt{\frac{g_{A2}^2}{g_{A2}^2 + g_{B2}^2}} \sqrt{g_{A2}^2 + g_{B2}^2 + g_{B2}^2} \right) v_{Lv} \left( Z_{Ls,i1}^{od} + Z_{Ls,i2}^{od} + Z_{Ls,i3}^{od} \right) \quad (589)$$


---

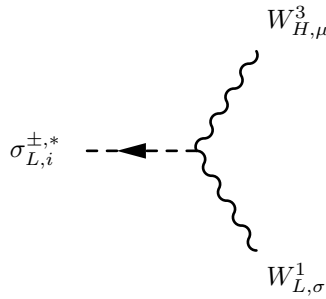

$$\frac{i}{2} g_{A2} g_{B2} v_{Lv} \left( -Z_{Ls,i2}^{od} - Z_{Ls,i4}^{od} + Z_{Ls,i1}^{od} + Z_{Ls,i3}^{od} \right) \left( g_{\sigma\mu} \right) \quad (590)$$


---



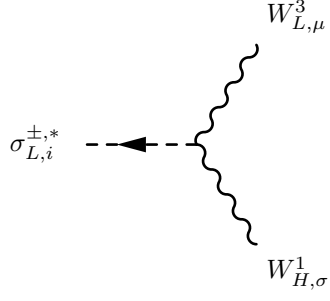

$$-\frac{i}{2}g_{A2}g_{B2}v_{Lv}\left(-Z_{Ls,i2}^{od}-Z_{Ls,i4}^{od}+Z_{Ls,i1}^{od}+Z_{Ls,i3}^{od}\right)\left(g_{\sigma\mu}\right) \quad (591)$$


---

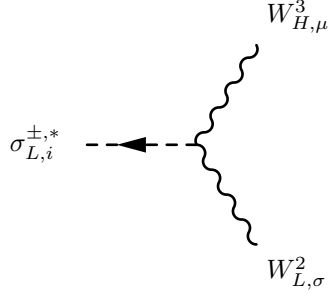

$$\frac{1}{2}g_{A2}g_{B2}v_{Lv}\left(-Z_{Ls,i2}^{od}-Z_{Ls,i4}^{od}+Z_{Ls,i1}^{od}+Z_{Ls,i3}^{od}\right)\left(g_{\sigma\mu}\right) \quad (592)$$


---

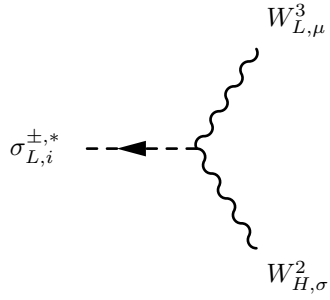

$$\frac{1}{2}g_{A2}g_{B2}v_{Lv}\left(-Z_{Ls,i1}^{od}-Z_{Ls,i3}^{od}+Z_{Ls,i2}^{od}+Z_{Ls,i4}^{od}\right)\left(g_{\sigma\mu}\right) \quad (593)$$


---

## 9.4 Two Fermion-One Vector Boson-Interaction

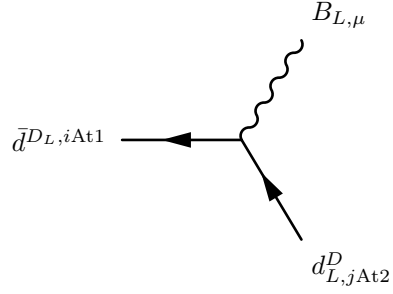

$$-\frac{i}{6}g_{A1}g_{B1}\frac{1}{\sqrt{g_{A1}^2+g_{B1}^2}}\delta_{At1At2}\delta_{ij}\left(\gamma_\mu\cdot\frac{1-\gamma_5}{2}\right) \quad (594)$$


---

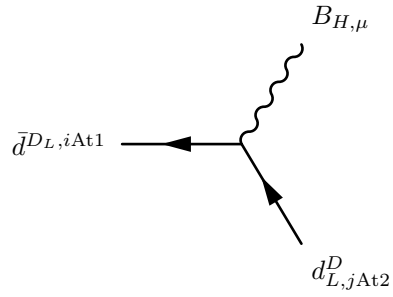

$$\frac{i}{6}g_{A1}\sqrt{\frac{g_{A1}^2}{g_{A1}^2+g_{B1}^2}}\delta_{At1At2}\delta_{ij}\left(\gamma_\mu\cdot\frac{1-\gamma_5}{2}\right) \quad (595)$$


---

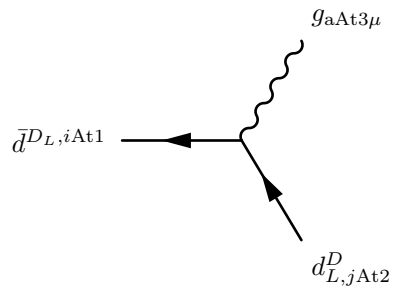

$$-\frac{i}{2}g_3\delta_{ij}\lambda_{At1,At2}^{aAt3}\left(\gamma_\mu\cdot\frac{1-\gamma_5}{2}\right) \quad (596)$$


---

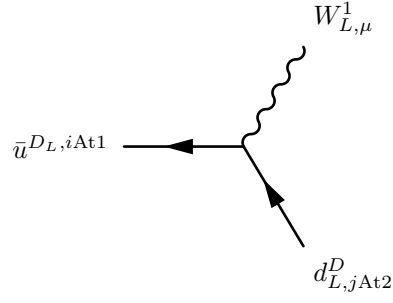

$$-\frac{i}{2}g_{A2}g_{B2}\frac{1}{\sqrt{g_{A2}^2+g_{B2}^2}}\delta_{\text{At}1\text{At}2}\delta_{ij}\left(\gamma_\mu\cdot\frac{1-\gamma_5}{2}\right) \quad (597)$$


---

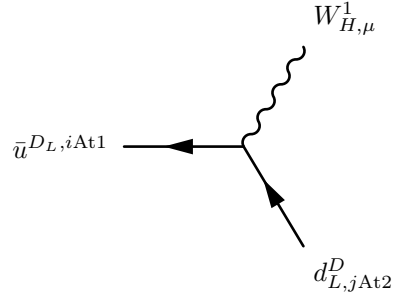

$$\frac{i}{2}g_{A2}\sqrt{\frac{g_{A2}^2}{g_{A2}^2+g_{B2}^2}}\delta_{\text{At}1\text{At}2}\delta_{ij}\left(\gamma_\mu\cdot\frac{1-\gamma_5}{2}\right) \quad (598)$$


---

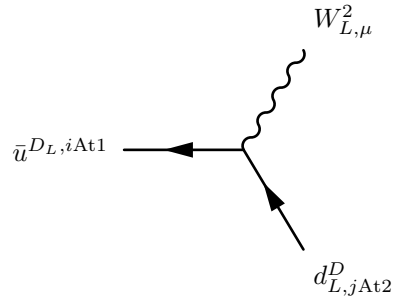

$$-\frac{1}{2}g_{A2}g_{B2}\frac{1}{\sqrt{g_{A2}^2+g_{B2}^2}}\delta_{\text{At}1\text{At}2}\delta_{ij}\left(\gamma_\mu\cdot\frac{1-\gamma_5}{2}\right) \quad (599)$$


---

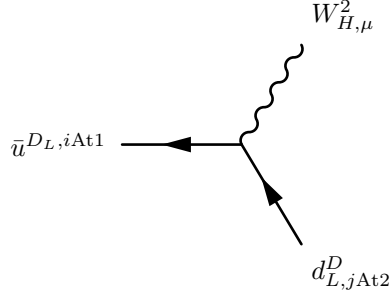

$$\frac{1}{2}g_{A2}\sqrt{\frac{gA2^2}{gA2^2 + gB2^2}}\delta_{\text{At}1\text{At}2}\delta_{ij}\left(\gamma_\mu \cdot \frac{1 - \gamma_5}{2}\right) \quad (600)$$


---

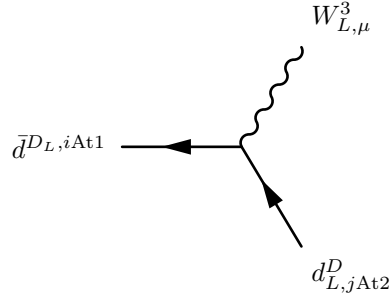

$$\frac{i}{2}g_{A2}g_{B2}\frac{1}{\sqrt{gA2^2 + gB2^2}}\delta_{\text{At}1\text{At}2}\delta_{ij}\left(\gamma_\mu \cdot \frac{1 - \gamma_5}{2}\right) \quad (601)$$


---

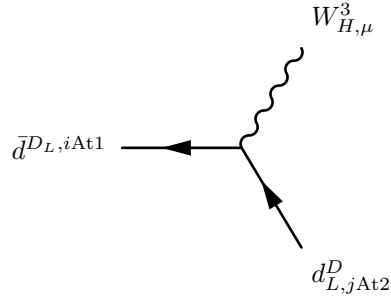

$$-\frac{i}{2}g_{A2}\sqrt{\frac{gA2^2}{gA2^2 + gB2^2}}\delta_{\text{At}1\text{At}2}\delta_{ij}\left(\gamma_\mu \cdot \frac{1 - \gamma_5}{2}\right) \quad (602)$$


---

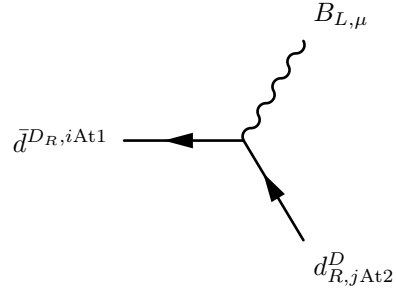

(603)

$$+ \frac{i}{3} g_{A1} g_{B1} \frac{1}{\sqrt{g_{A1}^2 + g_{B1}^2}} \delta_{At1At2} \delta_{ij} \left( \gamma_\mu \cdot \frac{1 + \gamma_5}{2} \right) \quad (604)$$


---

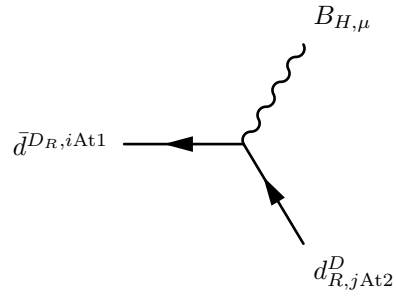

(605)

$$+ -\frac{i}{3} g_{A1} \sqrt{\frac{g_{A1}^2}{g_{A1}^2 + g_{B1}^2}} \delta_{At1At2} \delta_{ij} \left( \gamma_\mu \cdot \frac{1 + \gamma_5}{2} \right) \quad (606)$$


---

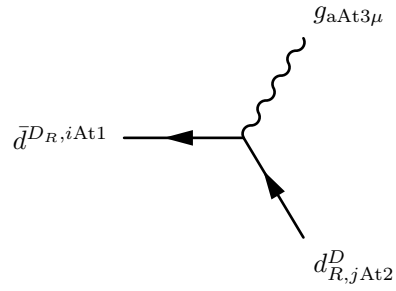

(607)

$$+ -\frac{i}{2} g_3 \delta_{ij} \lambda_{At1, At2}^{aAt3} \left( \gamma_\mu \cdot \frac{1 + \gamma_5}{2} \right) \quad (608)$$


---

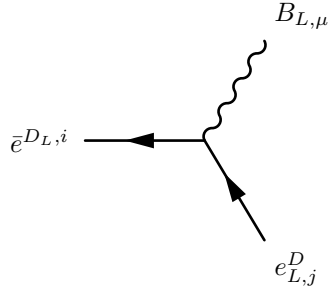

$$\frac{i}{2}g_{A1}g_{B1}\frac{1}{\sqrt{g_{A1}^2+g_{B1}^2}}\delta_{ij}\left(\gamma_\mu\cdot\frac{1-\gamma_5}{2}\right) \quad (609)$$


---

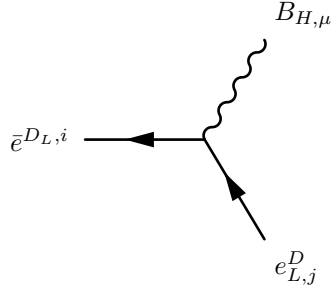

$$-\frac{i}{2}g_{A1}\sqrt{\frac{g_{A1}^2}{g_{A1}^2+g_{B1}^2}}\delta_{ij}\left(\gamma_\mu\cdot\frac{1-\gamma_5}{2}\right) \quad (610)$$


---

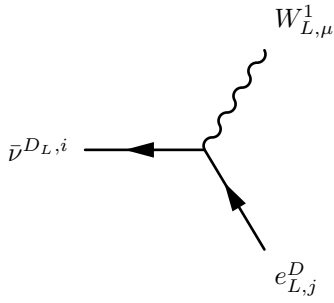

$$-\frac{i}{2}g_{A2}g_{B2}\frac{1}{\sqrt{g_{A2}^2+g_{B2}^2}}\delta_{ij}\left(\gamma_\mu\cdot\frac{1-\gamma_5}{2}\right) \quad (611)$$


---

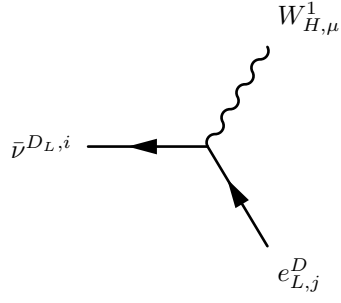

$$\frac{i}{2}g_{A2}\sqrt{\frac{g_{A2}^2}{g_{A2}^2+g_{B2}^2}}\delta_{ij}\left(\gamma_\mu\cdot\frac{1-\gamma_5}{2}\right) \quad (612)$$


---

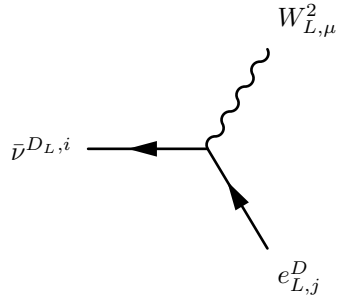

$$-\frac{1}{2}g_{A2}g_{B2}\frac{1}{\sqrt{g_{A2}^2+g_{B2}^2}}\delta_{ij}\left(\gamma_\mu\cdot\frac{1-\gamma_5}{2}\right) \quad (613)$$


---

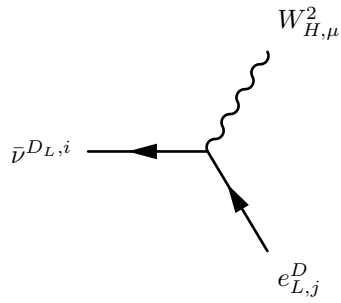

$$\frac{1}{2}g_{A2}\sqrt{\frac{g_{A2}^2}{g_{A2}^2+g_{B2}^2}}\delta_{ij}\left(\gamma_\mu\cdot\frac{1-\gamma_5}{2}\right) \quad (614)$$


---

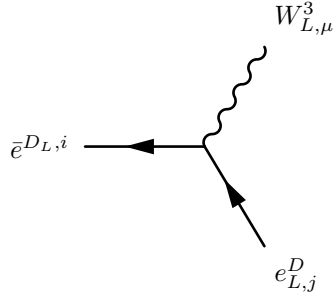

$$\frac{i}{2} g_{A2} g_{B2} \frac{1}{\sqrt{g_{A2}^2 + g_{B2}^2}} \delta_{ij} \left( \gamma_\mu \cdot \frac{1 - \gamma_5}{2} \right) \quad (615)$$


---

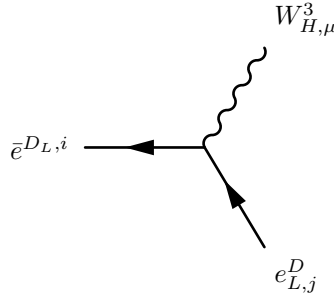

$$- \frac{i}{2} g_{A2} \sqrt{\frac{g_{A2}^2}{g_{A2}^2 + g_{B2}^2}} \delta_{ij} \left( \gamma_\mu \cdot \frac{1 - \gamma_5}{2} \right) \quad (616)$$


---

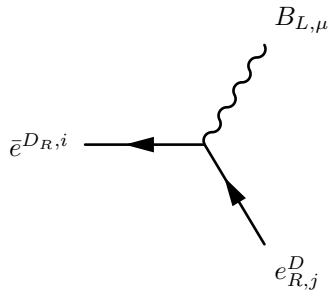

$$(617)$$

$$+ i g_{A1} g_{B1} \frac{1}{\sqrt{g_{A1}^2 + g_{B1}^2}} \delta_{ij} \left( \gamma_\mu \cdot \frac{1 + \gamma_5}{2} \right) \quad (618)$$


---



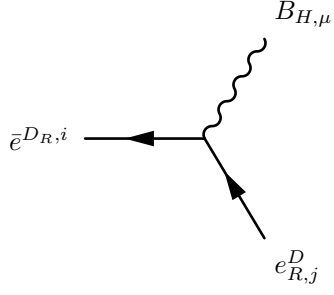

(619)

$$+ -ig_{A1}\sqrt{\frac{g_{A1}^2}{g_{A1}^2+g_{B1}^2}}\delta_{ij}\left(\gamma_\mu\cdot\frac{1+\gamma_5}{2}\right) \quad (620)$$


---

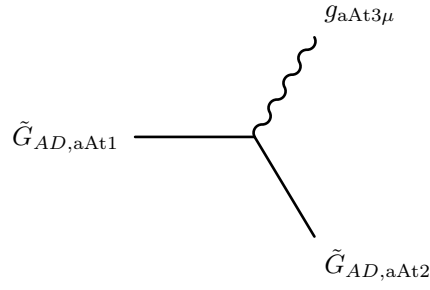

$$-g_3f_{aAt1,aAt2,aAt3}\left(\gamma_\mu\cdot\frac{1-\gamma_5}{2}\right) \quad (621)$$

$$+ -g_3f_{aAt1,aAt2,aAt3}\left(\gamma_\mu\cdot\frac{1+\gamma_5}{2}\right) \quad (622)$$


---

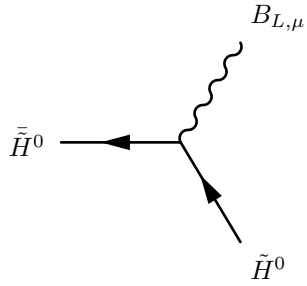

$$-\frac{i}{2}g_{A1}g_{B1}\frac{1}{\sqrt{g_{A1}^2+g_{B1}^2}}\left(\gamma_\mu\cdot\frac{1-\gamma_5}{2}\right) \quad (623)$$

$$+ -\frac{i}{2}g_{A1}g_{B1}\frac{1}{\sqrt{g_{A1}^2+g_{B1}^2}}\left(\gamma_\mu\cdot\frac{1+\gamma_5}{2}\right) \quad (624)$$


---

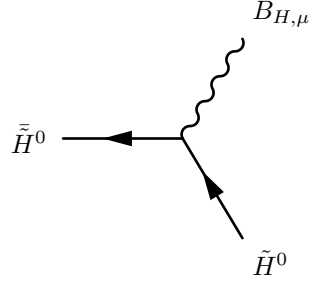

$$\frac{i}{2}g_{A1}\sqrt{\frac{g_{A1}^2}{g_{A1}^2+g_{B1}^2}}\left(\gamma_\mu\cdot\frac{1-\gamma_5}{2}\right) \quad (625)$$

$$+ \frac{i}{2}g_{A1}\sqrt{\frac{g_{A1}^2}{g_{A1}^2+g_{B1}^2}}\left(\gamma_\mu\cdot\frac{1+\gamma_5}{2}\right) \quad (626)$$


---

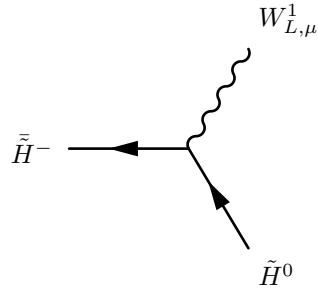

$$- \frac{i}{2}g_{A2}g_{B2}\frac{1}{\sqrt{g_{A2}^2+g_{B2}^2}}\left(\gamma_\mu\cdot\frac{1-\gamma_5}{2}\right) \quad (627)$$

$$+ \frac{i}{2}g_{A2}g_{B2}\frac{1}{\sqrt{g_{A2}^2+g_{B2}^2}}\left(\gamma_\mu\cdot\frac{1+\gamma_5}{2}\right) \quad (628)$$


---

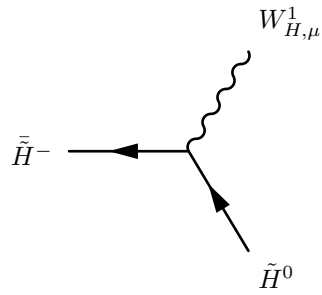

$$\frac{i}{2}g_{A2}\sqrt{\frac{g_{A2}^2}{g_{A2}^2+g_{B2}^2}}\left(\gamma_\mu\cdot\frac{1-\gamma_5}{2}\right) \quad (629)$$

$$+ -\frac{i}{2}g_{A2}\sqrt{\frac{g_{A2}^2}{g_{A2}^2+g_{B2}^2}}\left(\gamma_\mu\cdot\frac{1+\gamma_5}{2}\right) \quad (630)$$


---

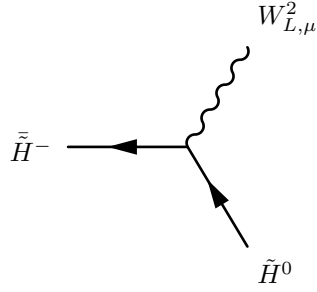

$$- \frac{1}{2}g_{A2}g_{B2}\frac{1}{\sqrt{g_{A2}^2+g_{B2}^2}}\left(\gamma_\mu\cdot\frac{1-\gamma_5}{2}\right) \quad (631)$$

$$+ \frac{1}{2}g_{A2}g_{B2}\frac{1}{\sqrt{g_{A2}^2+g_{B2}^2}}\left(\gamma_\mu\cdot\frac{1+\gamma_5}{2}\right) \quad (632)$$


---

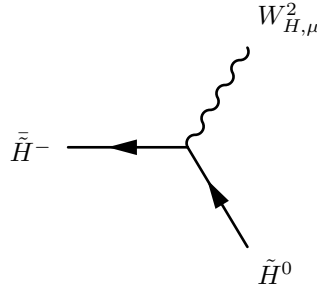

$$\frac{1}{2}g_{A2}\sqrt{\frac{g_{A2}^2}{g_{A2}^2+g_{B2}^2}}\left(\gamma_\mu\cdot\frac{1-\gamma_5}{2}\right) \quad (633)$$

$$+ -\frac{1}{2}g_{A2}\sqrt{\frac{g_{A2}^2}{g_{A2}^2+g_{B2}^2}}\left(\gamma_\mu\cdot\frac{1+\gamma_5}{2}\right) \quad (634)$$


---

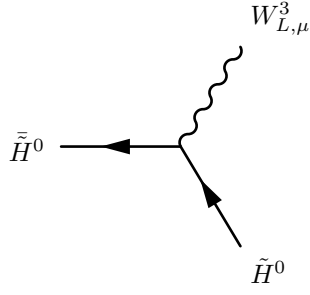

$$\frac{i}{2} g_{A2} g_{B2} \frac{1}{\sqrt{g_{A2}^2 + g_{B2}^2}} \left( \gamma_\mu \cdot \frac{1 - \gamma_5}{2} \right) \quad (635)$$

$$+ \frac{i}{2} g_{A2} g_{B2} \frac{1}{\sqrt{g_{A2}^2 + g_{B2}^2}} \left( \gamma_\mu \cdot \frac{1 + \gamma_5}{2} \right) \quad (636)$$


---

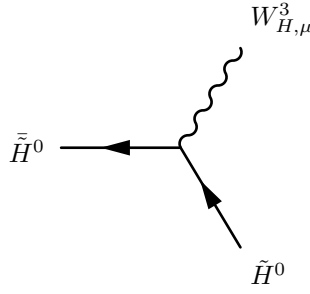

$$- \frac{i}{2} g_{A2} \sqrt{\frac{g_{A2}^2}{g_{A2}^2 + g_{B2}^2}} \left( \gamma_\mu \cdot \frac{1 - \gamma_5}{2} \right) \quad (637)$$

$$+ - \frac{i}{2} g_{A2} \sqrt{\frac{g_{A2}^2}{g_{A2}^2 + g_{B2}^2}} \left( \gamma_\mu \cdot \frac{1 + \gamma_5}{2} \right) \quad (638)$$


---

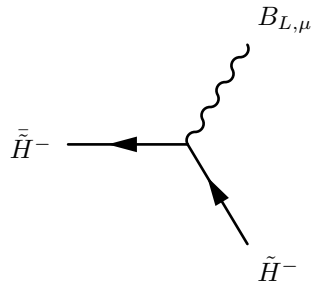

$$-\frac{i}{2}g_{A1}g_{B1}\frac{1}{\sqrt{g_{A1}^2+g_{B1}^2}}\left(\gamma_\mu\cdot\frac{1-\gamma_5}{2}\right) \quad (639)$$

$$+\frac{i}{2}g_{A1}g_{B1}\frac{1}{\sqrt{g_{A1}^2+g_{B1}^2}}\left(\gamma_\mu\cdot\frac{1+\gamma_5}{2}\right) \quad (640)$$


---

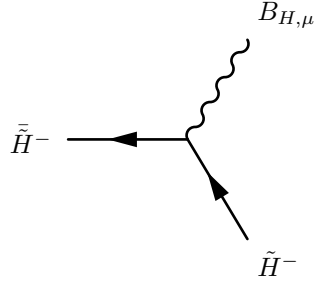

$$\frac{i}{2}g_{A1}\sqrt{\frac{g_{A1}^2}{g_{A1}^2+g_{B1}^2}}\left(\gamma_\mu\cdot\frac{1-\gamma_5}{2}\right) \quad (641)$$

$$+\frac{i}{2}g_{A1}\sqrt{\frac{g_{A1}^2}{g_{A1}^2+g_{B1}^2}}\left(\gamma_\mu\cdot\frac{1+\gamma_5}{2}\right) \quad (642)$$


---

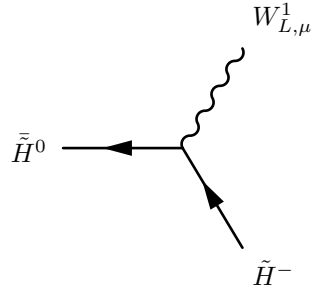

$$-\frac{i}{2}g_{A2}g_{B2}\frac{1}{\sqrt{g_{A2}^2+g_{B2}^2}}\left(\gamma_\mu\cdot\frac{1-\gamma_5}{2}\right) \quad (643)$$

$$+\frac{i}{2}g_{A2}g_{B2}\frac{1}{\sqrt{g_{A2}^2+g_{B2}^2}}\left(\gamma_\mu\cdot\frac{1+\gamma_5}{2}\right) \quad (644)$$


---

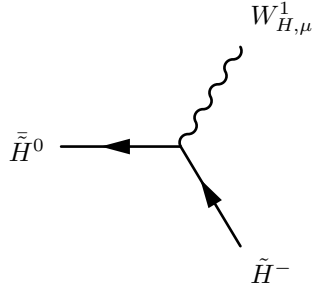

$$\frac{i}{2}g_{A2}\sqrt{\frac{gA2^2}{gA2^2+gB2^2}}\left(\gamma_\mu\cdot\frac{1-\gamma_5}{2}\right) \quad (645)$$

$$+ \frac{-i}{2}g_{A2}\sqrt{\frac{gA2^2}{gA2^2+gB2^2}}\left(\gamma_\mu\cdot\frac{1+\gamma_5}{2}\right) \quad (646)$$


---

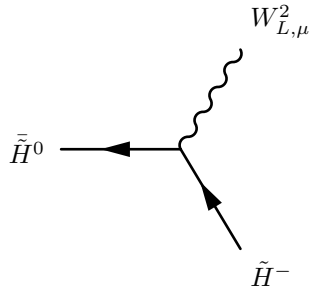

$$\frac{1}{2}g_{A2}g_{B2}\frac{1}{\sqrt{gA2^2+gB2^2}}\left(\gamma_\mu\cdot\frac{1-\gamma_5}{2}\right) \quad (647)$$

$$+ \frac{-1}{2}g_{A2}g_{B2}\frac{1}{\sqrt{gA2^2+gB2^2}}\left(\gamma_\mu\cdot\frac{1+\gamma_5}{2}\right) \quad (648)$$


---

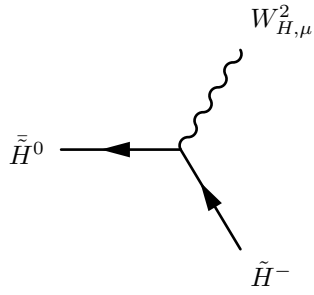

$$-\frac{1}{2}g_{A2}\sqrt{\frac{gA2^2}{gA2^2+gB2^2}}\left(\gamma_\mu\cdot\frac{1-\gamma_5}{2}\right) \quad (649)$$

$$+\frac{1}{2}g_{A2}\sqrt{\frac{gA2^2}{gA2^2+gB2^2}}\left(\gamma_\mu\cdot\frac{1+\gamma_5}{2}\right) \quad (650)$$


---

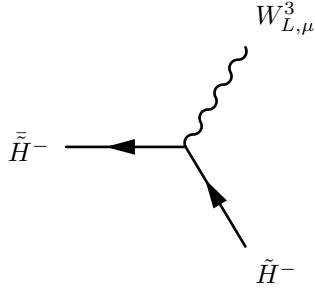

$$-\frac{i}{2}g_{A2}g_{B2}\frac{1}{\sqrt{gA2^2+gB2^2}}\left(\gamma_\mu\cdot\frac{1-\gamma_5}{2}\right) \quad (651)$$

$$+\frac{i}{2}g_{A2}g_{B2}\frac{1}{\sqrt{gA2^2+gB2^2}}\left(\gamma_\mu\cdot\frac{1+\gamma_5}{2}\right) \quad (652)$$


---

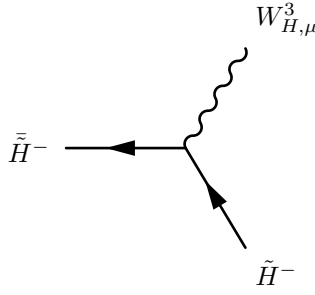

$$\frac{i}{2}g_{A2}\sqrt{\frac{gA2^2}{gA2^2+gB2^2}}\left(\gamma_\mu\cdot\frac{1-\gamma_5}{2}\right) \quad (653)$$

$$+\frac{i}{2}g_{A2}\sqrt{\frac{gA2^2}{gA2^2+gB2^2}}\left(\gamma_\mu\cdot\frac{1+\gamma_5}{2}\right) \quad (654)$$


---

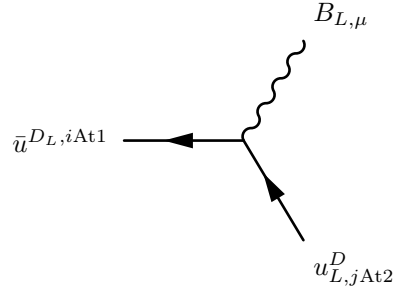

$$-\frac{i}{6}g_{A1}g_{B1}\frac{1}{\sqrt{g_{A1}^2+g_{B1}^2}}\delta_{\text{At}1\text{At}2}\delta_{ij}\left(\gamma_\mu\cdot\frac{1-\gamma_5}{2}\right) \quad (655)$$


---

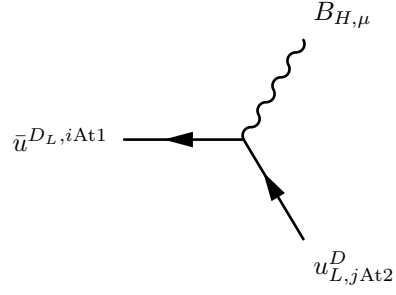

$$\frac{i}{6}g_{A1}\sqrt{\frac{g_{A1}^2}{g_{A1}^2+g_{B1}^2}}\delta_{\text{At}1\text{At}2}\delta_{ij}\left(\gamma_\mu\cdot\frac{1-\gamma_5}{2}\right) \quad (656)$$


---

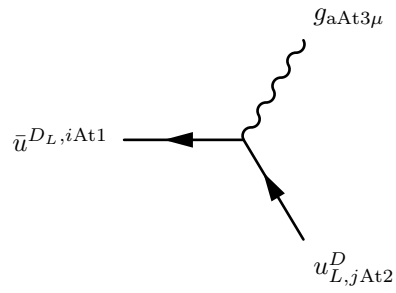

$$-\frac{i}{2}g_3\delta_{ij}\lambda_{\text{At}1,\text{At}2}^{\text{aAt}3}\left(\gamma_\mu\cdot\frac{1-\gamma_5}{2}\right) \quad (657)$$


---



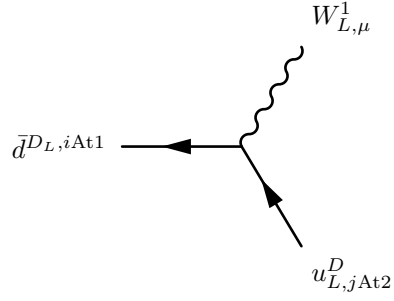

$$-\frac{i}{2}g_{A2}g_{B2}\frac{1}{\sqrt{g_{A2}^2+g_{B2}^2}}\delta_{At1At2}\delta_{ij}\left(\gamma_\mu\cdot\frac{1-\gamma_5}{2}\right) \quad (658)$$


---

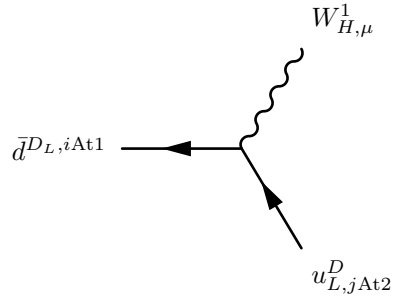

$$\frac{i}{2}g_{A2}\sqrt{\frac{g_{A2}^2}{g_{A2}^2+g_{B2}^2}}\delta_{At1At2}\delta_{ij}\left(\gamma_\mu\cdot\frac{1-\gamma_5}{2}\right) \quad (659)$$


---

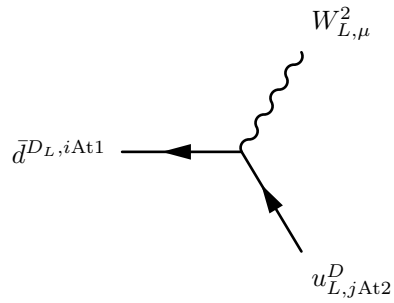

$$\frac{1}{2}g_{A2}g_{B2}\frac{1}{\sqrt{g_{A2}^2+g_{B2}^2}}\delta_{At1At2}\delta_{ij}\left(\gamma_\mu\cdot\frac{1-\gamma_5}{2}\right) \quad (660)$$


---

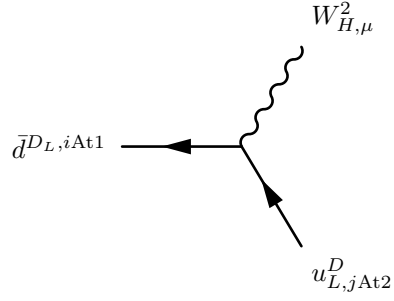

$$-\frac{1}{2}g_{A2}\sqrt{\frac{g_{A2}^2}{g_{A2}^2+g_{B2}^2}}\delta_{\text{At}1\text{At}2}\delta_{ij}\left(\gamma_\mu\cdot\frac{1-\gamma_5}{2}\right) \quad (661)$$


---

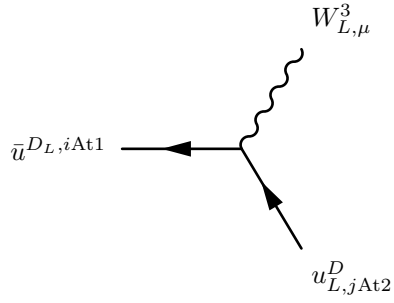

$$-\frac{i}{2}g_{A2}g_{B2}\frac{1}{\sqrt{g_{A2}^2+g_{B2}^2}}\delta_{\text{At}1\text{At}2}\delta_{ij}\left(\gamma_\mu\cdot\frac{1-\gamma_5}{2}\right) \quad (662)$$


---

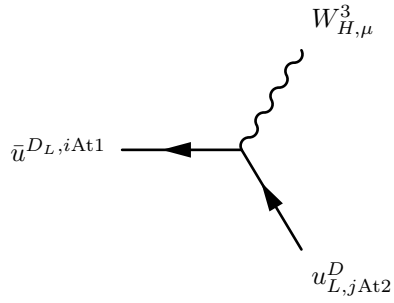

$$\frac{i}{2}g_{A2}\sqrt{\frac{g_{A2}^2}{g_{A2}^2+g_{B2}^2}}\delta_{\text{At}1\text{At}2}\delta_{ij}\left(\gamma_\mu\cdot\frac{1-\gamma_5}{2}\right) \quad (663)$$


---

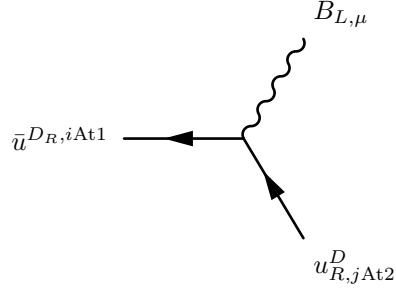

(664)

$$+ -\frac{2i}{3}g_{A1}g_{B1}\frac{1}{\sqrt{g_{A1}^2+g_{B1}^2}}\delta_{\text{At}1\text{At}2}\delta_{ij}\left(\gamma_\mu\cdot\frac{1+\gamma_5}{2}\right) \quad (665)$$


---

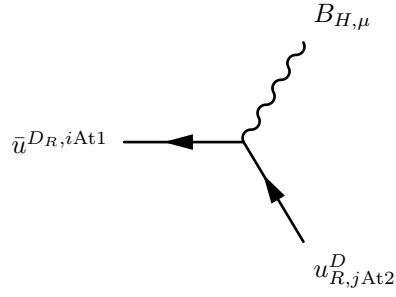

(666)

$$+ \frac{2i}{3}g_{A1}\sqrt{\frac{g_{A1}^2}{g_{A1}^2+g_{B1}^2}}\delta_{\text{At}1\text{At}2}\delta_{ij}\left(\gamma_\mu\cdot\frac{1+\gamma_5}{2}\right) \quad (667)$$


---

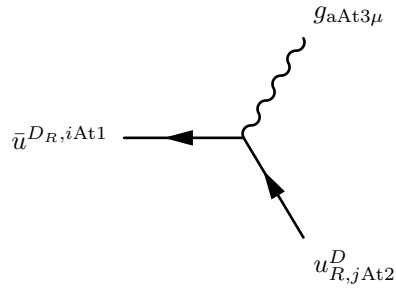

(668)

$$+ -\frac{i}{2}g_3\delta_{ij}\lambda_{\text{At}1,\text{At}2}^{\text{aAt}3}\left(\gamma_\mu\cdot\frac{1+\gamma_5}{2}\right) \quad (669)$$


---

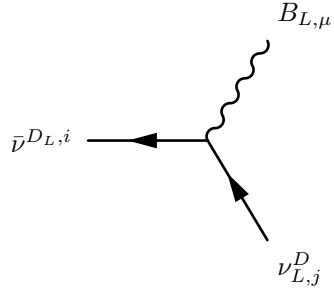

$$\frac{i}{2} g_{A1} g_{B1} \frac{1}{\sqrt{g_{A1}^2 + g_{B1}^2}} \delta_{ij} \left( \gamma_\mu \cdot \frac{1 - \gamma_5}{2} \right) \quad (670)$$


---

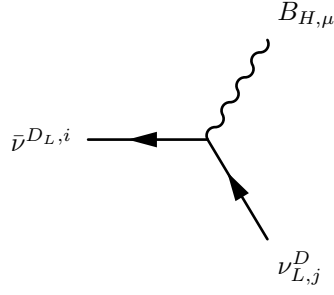

$$- \frac{i}{2} g_{A1} \sqrt{\frac{g_{A1}^2}{g_{A1}^2 + g_{B1}^2}} \delta_{ij} \left( \gamma_\mu \cdot \frac{1 - \gamma_5}{2} \right) \quad (671)$$


---

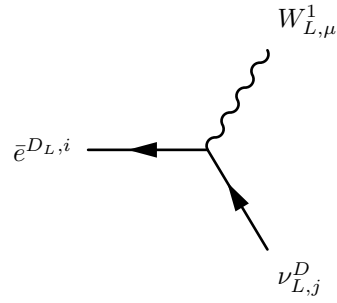

$$- \frac{i}{2} g_{A2} g_{B2} \frac{1}{\sqrt{g_{A2}^2 + g_{B2}^2}} \delta_{ij} \left( \gamma_\mu \cdot \frac{1 - \gamma_5}{2} \right) \quad (672)$$


---

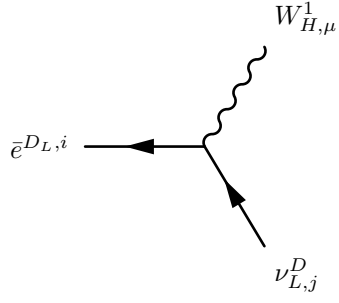

$$\frac{i}{2}g_{A2}\sqrt{\frac{g_{A2}^2}{g_{A2}^2+g_{B2}^2}}\delta_{ij}\left(\gamma_\mu\cdot\frac{1-\gamma_5}{2}\right) \quad (673)$$


---

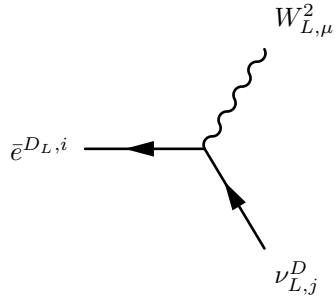

$$\frac{1}{2}g_{A2}g_{B2}\frac{1}{\sqrt{g_{A2}^2+g_{B2}^2}}\delta_{ij}\left(\gamma_\mu\cdot\frac{1-\gamma_5}{2}\right) \quad (674)$$


---

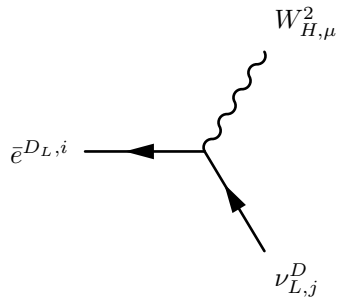

$$-\frac{1}{2}g_{A2}\sqrt{\frac{g_{A2}^2}{g_{A2}^2+g_{B2}^2}}\delta_{ij}\left(\gamma_\mu\cdot\frac{1-\gamma_5}{2}\right) \quad (675)$$


---

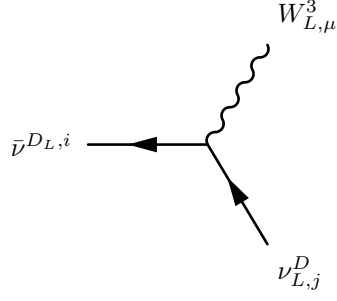

$$-\frac{i}{2}g_{A2}g_{B2}\frac{1}{\sqrt{g_{A2}^2+g_{B2}^2}}\delta_{ij}\left(\gamma_\mu\cdot\frac{1-\gamma_5}{2}\right) \quad (676)$$


---

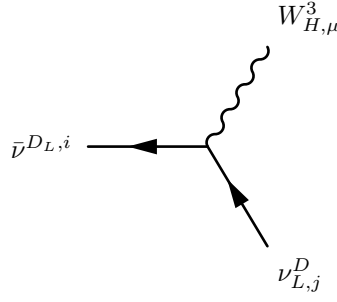

$$\frac{i}{2}g_{A2}\sqrt{\frac{g_{A2}^2}{g_{A2}^2+g_{B2}^2}}\delta_{ij}\left(\gamma_\mu\cdot\frac{1-\gamma_5}{2}\right) \quad (677)$$


---

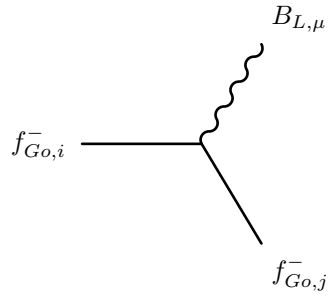

$$-\frac{i}{2}g_{B1}\frac{1}{\sqrt{g_{A1}^2+g_{B1}^2}}\left(-g_{A1}+\sqrt{\frac{g_{A1}^2}{g_{A1}^2+g_{B1}^2}}\sqrt{g_{A1}^2+g_{B1}^2}\right)\left(Z_{Go,j1}^*Z_{Go,i1}-Z_{Go,j2}^*Z_{Go,i2}+Z_{Go,j3}^*Z_{Go,i3}-Z_{Go,j4}^*Z_{Go,i4}\right)\left(\gamma_\mu\right) \quad (678)$$

$$+ \frac{i}{2} g_{B1} \frac{1}{\sqrt{gA1^2 + gB1^2}} \left( -g_{A1} + \sqrt{\frac{gA1^2}{gA1^2 + gB1^2}} \sqrt{gA1^2 + gB1^2} \right) \left( Z_{Go,i1}^* Z_{Go,j1} - Z_{Go,i2}^* Z_{Go,j2} + Z_{Go,i3}^* Z_{Go,j3} - Z_{Go,i4}^* Z_{Go,j4} \right) \left( \gamma_\mu \cdot \right. \quad (679)$$


---

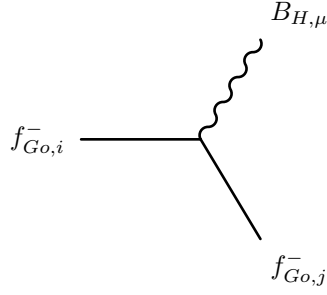

$$- \frac{i}{2} \frac{1}{\sqrt{gA1^2 + gB1^2}} \left( g_{A1} \sqrt{\frac{gA1^2}{gA1^2 + gB1^2}} \sqrt{gA1^2 + gB1^2} + g_{B1}^2 \right) \left( Z_{Go,j1}^* Z_{Go,i1} - Z_{Go,j2}^* Z_{Go,i2} + Z_{Go,j3}^* Z_{Go,i3} - Z_{Go,j4}^* Z_{Go,i4} \right) \left( \gamma_\mu \cdot \right. \quad (680)$$

$$+ \frac{i}{2} \frac{1}{\sqrt{gA1^2 + gB1^2}} \left( g_{A1} \sqrt{\frac{gA1^2}{gA1^2 + gB1^2}} \sqrt{gA1^2 + gB1^2} + g_{B1}^2 \right) \left( Z_{Go,i1}^* Z_{Go,j1} - Z_{Go,i2}^* Z_{Go,j2} + Z_{Go,i3}^* Z_{Go,j3} - Z_{Go,i4}^* Z_{Go,j4} \right) \left( \gamma_\mu \cdot \right. \quad (681)$$


---

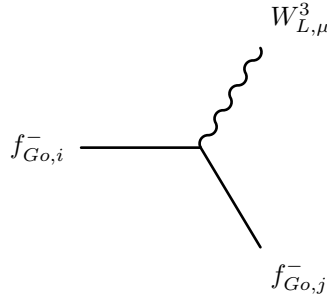

$$\frac{1}{2} g_{B2} \frac{1}{\left( gA2^2 + gB2^2 \right)^{3/2}} \left( -i \left( g_{A2}^2 + g_{B2}^2 \right) \left( \sqrt{\frac{gA2^2}{gA2^2 + gB2^2}} \sqrt{gA2^2 + gB2^2} + g_{A2} \right) Z_{Go,j1}^* Z_{Go,i1} \right. \\ + i \left( g_{A2}^2 + g_{B2}^2 \right) \left( \sqrt{\frac{gA2^2}{gA2^2 + gB2^2}} \sqrt{gA2^2 + gB2^2} + g_{A2} \right) Z_{Go,j2}^* Z_{Go,i2} + i g_{A2}^3 Z_{Go,j3}^* Z_{Go,i3} \\ \left. + i g_{A2} g_{B2}^2 Z_{Go,j3}^* Z_{Go,i3} + i g_{B2}^2 \sqrt{\frac{gA2^2}{gA2^2 + gB2^2}} \sqrt{gA2^2 + gB2^2} Z_{Go,j3}^* Z_{Go,i3} \right)$$

$$\begin{aligned}
& + i \left( \frac{gA^2}{gA^2 + gB^2} \right)^{3/2} \left( gA^2 + gB^2 \right)^{3/2} Z_{Go,j3}^* Z_{Go,i3} - ig_{A2}^3 Z_{Go,j4}^* Z_{Go,i4} - ig_{A2} g_{B2}^2 Z_{Go,j4}^* Z_{Go,i4} \\
& - ig_{B2}^2 \sqrt{\frac{gA^2}{gA^2 + gB^2}} \sqrt{gA^2 + gB^2} Z_{Go,j4}^* Z_{Go,i4} \\
& - i \left( \frac{gA^2}{gA^2 + gB^2} \right)^{3/2} \left( gA^2 + gB^2 \right)^{3/2} Z_{Go,j4}^* Z_{Go,i4} - 2g_{A2} g_{B2}^2 Z_{Go,j7}^* Z_{Go,i5} \\
& - 2 \left( \frac{gA^2}{gA^2 + gB^2} \right)^{3/2} \left( gA^2 + gB^2 \right)^{3/2} Z_{Go,j7}^* Z_{Go,i5} - 2g_{A2}^2 g_{B2} Z_{Go,j8}^* Z_{Go,i5} \\
& + 2g_{A2} g_{B2} \sqrt{\frac{gA^2}{gA^2 + gB^2}} \sqrt{gA^2 + gB^2} Z_{Go,j8}^* Z_{Go,i5} - 2g_{A2}^2 g_{B2} Z_{Go,j7}^* Z_{Go,i6} \\
& + 2g_{A2} g_{B2} \sqrt{\frac{gA^2}{gA^2 + gB^2}} \sqrt{gA^2 + gB^2} Z_{Go,j7}^* Z_{Go,i6} - 2g_{A2}^3 Z_{Go,j8}^* Z_{Go,i6} \\
& - 2g_{B2}^2 \sqrt{\frac{gA^2}{gA^2 + gB^2}} \sqrt{gA^2 + gB^2} Z_{Go,j8}^* Z_{Go,i6} + 2g_{A2} g_{B2}^2 Z_{Go,j5}^* Z_{Go,i7} \\
& + 2 \left( \frac{gA^2}{gA^2 + gB^2} \right)^{3/2} \left( gA^2 + gB^2 \right)^{3/2} Z_{Go,j5}^* Z_{Go,i7} + 2g_{A2}^2 g_{B2} Z_{Go,j6}^* Z_{Go,i7} \\
& - 2g_{A2} g_{B2} \sqrt{\frac{gA^2}{gA^2 + gB^2}} \sqrt{gA^2 + gB^2} Z_{Go,j6}^* Z_{Go,i7} + 2g_{A2}^2 g_{B2} Z_{Go,j5}^* Z_{Go,i8} \\
& - 2g_{A2} g_{B2} \sqrt{\frac{gA^2}{gA^2 + gB^2}} \sqrt{gA^2 + gB^2} Z_{Go,j5}^* Z_{Go,i8} + 2g_{A2}^3 Z_{Go,j6}^* Z_{Go,i8} \\
& + 2g_{B2}^2 \sqrt{\frac{gA^2}{gA^2 + gB^2}} \sqrt{gA^2 + gB^2} Z_{Go,j6}^* Z_{Go,i8} \\
& - 2ig_{B2}^2 \sqrt{\frac{gA^2}{gA^2 + gB^2}} \sqrt{gA^2 + gB^2} Z_{Go,j9}^* Z_{Go,i9} \\
& - 2i \left( \frac{gA^2}{gA^2 + gB^2} \right)^{3/2} \left( gA^2 + gB^2 \right)^{3/2} Z_{Go,j9}^* Z_{Go,i9} \\
& + 2ig_{B2}^2 \sqrt{\frac{gA^2}{gA^2 + gB^2}} \sqrt{gA^2 + gB^2} Z_{Go,j10}^* Z_{Go,i10} \\
& + 2i \left( \frac{gA^2}{gA^2 + gB^2} \right)^{3/2} \left( gA^2 + gB^2 \right)^{3/2} Z_{Go,j10}^* Z_{Go,i10} \left( \gamma_\mu \cdot \frac{1 - \gamma_5}{2} \right) \\
& + \frac{1}{2} g_{B2} \frac{1}{\left( gA^2 + gB^2 \right)^{3/2}} \left( i \left( g_{A2}^2 + g_{B2}^2 \right) \left( \sqrt{\frac{gA^2}{gA^2 + gB^2}} \sqrt{gA^2 + gB^2} + g_{A2} \right) Z_{Go,i1}^* Z_{Go,j1} \right)
\end{aligned} \tag{682}$$



$$\begin{aligned}
& -i\left(g_{A2}^2 + g_{B2}^2\right)\left(\sqrt{\frac{gA2^2}{gA2^2 + gB2^2}}\sqrt{gA2^2 + gB2^2} + g_{A2}\right)Z_{Go,i2}^*Z_{Go,j2} - ig_{A2}^3Z_{Go,i3}^*Z_{Go,j3} \\
& - ig_{A2}g_{B2}^2Z_{Go,i3}^*Z_{Go,j3} - ig_{B2}^2\sqrt{\frac{gA2^2}{gA2^2 + gB2^2}}\sqrt{gA2^2 + gB2^2}Z_{Go,i3}^*Z_{Go,j3} \\
& - i\left(\frac{gA2^2}{gA2^2 + gB2^2}\right)^{3/2}\left(gA2^2 + gB2^2\right)^{3/2}Z_{Go,i3}^*Z_{Go,j3} + ig_{A2}^3Z_{Go,i4}^*Z_{Go,j4} + ig_{A2}g_{B2}^2Z_{Go,i4}^*Z_{Go,j4} \\
& + ig_{B2}^2\sqrt{\frac{gA2^2}{gA2^2 + gB2^2}}\sqrt{gA2^2 + gB2^2}Z_{Go,i4}^*Z_{Go,j4} \\
& + i\left(\frac{gA2^2}{gA2^2 + gB2^2}\right)^{3/2}\left(gA2^2 + gB2^2\right)^{3/2}Z_{Go,i4}^*Z_{Go,j4} + 2g_{A2}g_{B2}^2Z_{Go,i7}^*Z_{Go,j5} \\
& + 2\left(\frac{gA2^2}{gA2^2 + gB2^2}\right)^{3/2}\left(gA2^2 + gB2^2\right)^{3/2}Z_{Go,i7}^*Z_{Go,j5} + 2g_{A2}^2g_{B2}Z_{Go,i8}^*Z_{Go,j5} \\
& - 2g_{A2}g_{B2}\sqrt{\frac{gA2^2}{gA2^2 + gB2^2}}\sqrt{gA2^2 + gB2^2}Z_{Go,i8}^*Z_{Go,j5} + 2g_{A2}^2g_{B2}Z_{Go,i7}^*Z_{Go,j6} \\
& - 2g_{A2}g_{B2}\sqrt{\frac{gA2^2}{gA2^2 + gB2^2}}\sqrt{gA2^2 + gB2^2}Z_{Go,i7}^*Z_{Go,j6} + 2g_{A2}^3Z_{Go,i8}^*Z_{Go,j6} \\
& + 2g_{B2}^2\sqrt{\frac{gA2^2}{gA2^2 + gB2^2}}\sqrt{gA2^2 + gB2^2}Z_{Go,i8}^*Z_{Go,j6} - 2g_{A2}g_{B2}^2Z_{Go,i5}^*Z_{Go,j7} \\
& - 2\left(\frac{gA2^2}{gA2^2 + gB2^2}\right)^{3/2}\left(gA2^2 + gB2^2\right)^{3/2}Z_{Go,i5}^*Z_{Go,j7} - 2g_{A2}^2g_{B2}Z_{Go,i6}^*Z_{Go,j7} \\
& + 2g_{A2}g_{B2}\sqrt{\frac{gA2^2}{gA2^2 + gB2^2}}\sqrt{gA2^2 + gB2^2}Z_{Go,i6}^*Z_{Go,j7} - 2g_{A2}^2g_{B2}Z_{Go,i5}^*Z_{Go,j8} \\
& + 2g_{A2}g_{B2}\sqrt{\frac{gA2^2}{gA2^2 + gB2^2}}\sqrt{gA2^2 + gB2^2}Z_{Go,i5}^*Z_{Go,j8} - 2g_{A2}^3Z_{Go,i6}^*Z_{Go,j8} \\
& - 2g_{B2}^2\sqrt{\frac{gA2^2}{gA2^2 + gB2^2}}\sqrt{gA2^2 + gB2^2}Z_{Go,i6}^*Z_{Go,j8} \\
& + 2ig_{B2}^2\sqrt{\frac{gA2^2}{gA2^2 + gB2^2}}\sqrt{gA2^2 + gB2^2}Z_{Go,i9}^*Z_{Go,j9} \\
& + 2i\left(\frac{gA2^2}{gA2^2 + gB2^2}\right)^{3/2}\left(gA2^2 + gB2^2\right)^{3/2}Z_{Go,i9}^*Z_{Go,j9} \\
& - 2ig_{B2}^2\sqrt{\frac{gA2^2}{gA2^2 + gB2^2}}\sqrt{gA2^2 + gB2^2}Z_{Go,i10}^*Z_{Go,j10} \\
& - 2i\left(\frac{gA2^2}{gA2^2 + gB2^2}\right)^{3/2}\left(gA2^2 + gB2^2\right)^{3/2}Z_{Go,i10}^*Z_{Go,j10}\left(\gamma_\mu \cdot \frac{1 + \gamma_5}{2}\right)
\end{aligned} \tag{683}$$

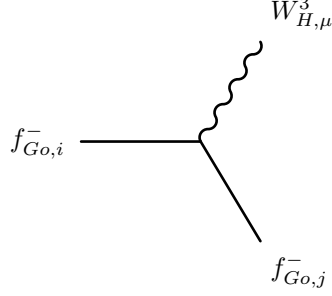

$$\begin{aligned}
& \frac{1}{2} \frac{1}{\left(gA^2 + gB^2\right)^{3/2}} \left( i \left( g_{A2}^2 + g_{B2}^2 \right) \left( g_{A2} \sqrt{\frac{gA^2}{gA^2 + gB^2}} \sqrt{gA^2 + gB^2 - g_{B2}^2} \right) Z_{Go,j1}^* Z_{Go,i1} \right. \\
& - i \left( g_{A2}^2 + g_{B2}^2 \right) \left( g_{A2} \sqrt{\frac{gA^2}{gA^2 + gB^2}} \sqrt{gA^2 + gB^2 - g_{B2}^2} \right) Z_{Go,j2}^* Z_{Go,i2} + i g_{A2}^2 g_{B2}^2 Z_{Go,j3}^* Z_{Go,i3} \\
& + i g_{B2}^4 Z_{Go,j3}^* Z_{Go,i3} - i g_{A2} g_{B2}^2 \sqrt{\frac{gA^2}{gA^2 + gB^2}} \sqrt{gA^2 + gB^2} Z_{Go,j3}^* Z_{Go,i3} \\
& - i g_{A2} \left( \frac{gA^2}{gA^2 + gB^2} \right)^{3/2} \left( gA^2 + gB^2 \right)^{3/2} Z_{Go,j3}^* Z_{Go,i3} - i g_{A2}^2 g_{B2}^2 Z_{Go,j4}^* Z_{Go,i4} - i g_{B2}^4 Z_{Go,j4}^* Z_{Go,i4} \\
& + i g_{A2} g_{B2}^2 \sqrt{\frac{gA^2}{gA^2 + gB^2}} \sqrt{gA^2 + gB^2} Z_{Go,j4}^* Z_{Go,i4} \\
& + i g_{A2} \left( \frac{gA^2}{gA^2 + gB^2} \right)^{3/2} \left( gA^2 + gB^2 \right)^{3/2} Z_{Go,j4}^* Z_{Go,i4} - 2 g_{A2}^2 g_{B2}^2 Z_{Go,j7}^* Z_{Go,i5} \\
& + 2 g_{A2} g_{B2}^2 \sqrt{\frac{gA^2}{gA^2 + gB^2}} \sqrt{gA^2 + gB^2} Z_{Go,j7}^* Z_{Go,i5} - 2 g_{A2}^3 g_{B2} Z_{Go,j8}^* Z_{Go,i5} \\
& - 2 g_{B2}^3 \sqrt{\frac{gA^2}{gA^2 + gB^2}} \sqrt{gA^2 + gB^2} Z_{Go,j8}^* Z_{Go,i5} - 2 g_{A2}^3 g_{B2} Z_{Go,j7}^* Z_{Go,i6} \\
& - 2 g_{B2}^3 \sqrt{\frac{gA^2}{gA^2 + gB^2}} \sqrt{gA^2 + gB^2} Z_{Go,j7}^* Z_{Go,i6} - 2 g_{B2}^4 Z_{Go,j8}^* Z_{Go,i6} \\
& + 2 g_{A2} \left( \frac{gA^2}{gA^2 + gB^2} \right)^{3/2} \left( gA^2 + gB^2 \right)^{3/2} Z_{Go,j8}^* Z_{Go,i6} + 2 g_{A2}^2 g_{B2}^2 Z_{Go,j5}^* Z_{Go,i7} \\
& - 2 g_{A2} g_{B2}^2 \sqrt{\frac{gA^2}{gA^2 + gB^2}} \sqrt{gA^2 + gB^2} Z_{Go,j5}^* Z_{Go,i7} + 2 g_{A2}^3 g_{B2} Z_{Go,j6}^* Z_{Go,i7} \\
& + 2 g_{B2}^3 \sqrt{\frac{gA^2}{gA^2 + gB^2}} \sqrt{gA^2 + gB^2} Z_{Go,j6}^* Z_{Go,i7} + 2 g_{A2}^3 g_{B2} Z_{Go,j5}^* Z_{Go,i8}
\end{aligned}$$

$$\begin{aligned}
& + 2g_{B2}^3 \sqrt{\frac{gA2^2}{gA2^2 + gB2^2}} \sqrt{gA2^2 + gB2^2} Z_{Go,j5}^* Z_{Go,i8} + 2g_{B2}^4 Z_{Go,j6}^* Z_{Go,i8} \\
& - 2g_{A2} \left( \frac{gA2^2}{gA2^2 + gB2^2} \right)^{3/2} (gA2^2 + gB2^2)^{3/2} Z_{Go,j6}^* Z_{Go,i8} - 2ig_{A2}^2 g_{B2}^2 Z_{Go,j9}^* Z_{Go,i9} - 2ig_{B2}^4 Z_{Go,j9}^* Z_{Go,i9} \\
& + 2ig_{A2}^2 g_{B2}^2 Z_{Go,j10}^* Z_{Go,i10} + 2ig_{B2}^4 Z_{Go,j10}^* Z_{Go,i10} \left( \gamma_\mu \cdot \frac{1 - \gamma_5}{2} \right) \tag{684} \\
& + \frac{1}{2} \frac{1}{(gA2^2 + gB2^2)^{3/2}} \left( -i(g_{A2}^2 + g_{B2}^2) \left( g_{A2} \sqrt{\frac{gA2^2}{gA2^2 + gB2^2}} \sqrt{gA2^2 + gB2^2} - g_{B2}^2 \right) Z_{Go,i1}^* Z_{Go,j1} \right. \\
& + i(g_{A2}^2 + g_{B2}^2) \left( g_{A2} \sqrt{\frac{gA2^2}{gA2^2 + gB2^2}} \sqrt{gA2^2 + gB2^2} - g_{B2}^2 \right) Z_{Go,i2}^* Z_{Go,j2} - ig_{A2}^2 g_{B2}^2 Z_{Go,i3}^* Z_{Go,j3} \\
& - ig_{B2}^4 Z_{Go,i3}^* Z_{Go,j3} + ig_{A2} g_{B2}^2 \sqrt{\frac{gA2^2}{gA2^2 + gB2^2}} \sqrt{gA2^2 + gB2^2} Z_{Go,i3}^* Z_{Go,j3} \\
& + ig_{A2} \left( \frac{gA2^2}{gA2^2 + gB2^2} \right)^{3/2} (gA2^2 + gB2^2)^{3/2} Z_{Go,i3}^* Z_{Go,j3} + ig_{A2}^2 g_{B2}^2 Z_{Go,i4}^* Z_{Go,j4} + ig_{B2}^4 Z_{Go,i4}^* Z_{Go,j4} \\
& - ig_{A2} g_{B2}^2 \sqrt{\frac{gA2^2}{gA2^2 + gB2^2}} \sqrt{gA2^2 + gB2^2} Z_{Go,i4}^* Z_{Go,j4} \\
& - ig_{A2} \left( \frac{gA2^2}{gA2^2 + gB2^2} \right)^{3/2} (gA2^2 + gB2^2)^{3/2} Z_{Go,i4}^* Z_{Go,j4} + 2g_{A2}^2 g_{B2}^2 Z_{Go,i7}^* Z_{Go,j5} \\
& - 2g_{A2} g_{B2}^2 \sqrt{\frac{gA2^2}{gA2^2 + gB2^2}} \sqrt{gA2^2 + gB2^2} Z_{Go,i7}^* Z_{Go,j5} + 2g_{A2}^3 g_{B2} Z_{Go,i8}^* Z_{Go,j5} \\
& + 2g_{B2}^3 \sqrt{\frac{gA2^2}{gA2^2 + gB2^2}} \sqrt{gA2^2 + gB2^2} Z_{Go,i8}^* Z_{Go,j5} + 2g_{A2}^3 g_{B2} Z_{Go,i7}^* Z_{Go,j6} \\
& + 2g_{B2}^3 \sqrt{\frac{gA2^2}{gA2^2 + gB2^2}} \sqrt{gA2^2 + gB2^2} Z_{Go,i7}^* Z_{Go,j6} + 2g_{B2}^4 Z_{Go,i8}^* Z_{Go,j6} \\
& - 2g_{A2} \left( \frac{gA2^2}{gA2^2 + gB2^2} \right)^{3/2} (gA2^2 + gB2^2)^{3/2} Z_{Go,i8}^* Z_{Go,j6} - 2g_{A2}^2 g_{B2}^2 Z_{Go,i5}^* Z_{Go,j7} \\
& + 2g_{A2} g_{B2}^2 \sqrt{\frac{gA2^2}{gA2^2 + gB2^2}} \sqrt{gA2^2 + gB2^2} Z_{Go,i5}^* Z_{Go,j7} - 2g_{A2}^3 g_{B2} Z_{Go,i6}^* Z_{Go,j7} \\
& - 2g_{B2}^3 \sqrt{\frac{gA2^2}{gA2^2 + gB2^2}} \sqrt{gA2^2 + gB2^2} Z_{Go,i6}^* Z_{Go,j7} - 2g_{A2}^3 g_{B2} Z_{Go,i5}^* Z_{Go,j8} \\
& - 2g_{B2}^3 \sqrt{\frac{gA2^2}{gA2^2 + gB2^2}} \sqrt{gA2^2 + gB2^2} Z_{Go,i5}^* Z_{Go,j8} - 2g_{B2}^4 Z_{Go,i6}^* Z_{Go,j8} \\
& + 2g_{A2} \left( \frac{gA2^2}{gA2^2 + gB2^2} \right)^{3/2} (gA2^2 + gB2^2)^{3/2} Z_{Go,i6}^* Z_{Go,j8} + 2ig_{A2}^2 g_{B2}^2 Z_{Go,i9}^* Z_{Go,j9} + 2ig_{B2}^4 Z_{Go,i9}^* Z_{Go,j9}
\end{aligned}$$

$$-2ig_{A2}^2g_{B2}^2Z_{Go,i10}^*Z_{Go,j10}-2ig_{B2}^4Z_{Go,i10}^*Z_{Go,j10}\Big)\Big(\gamma_\mu\cdot\frac{1+\gamma_5}{2}\Big) \quad (685)$$

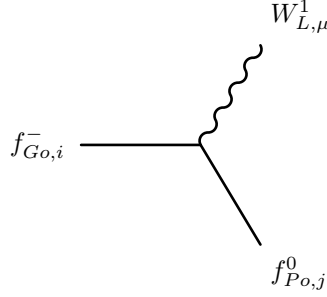

$$\begin{aligned} & \frac{1}{2}g_{B2}\Big(-i\sqrt{\frac{gA2^2}{gA2^2+gB2^2}}Z_{Po,j2}^*Z_{Go,i2}+ig_{A2}\frac{1}{\sqrt{gA2^2+gB2^2}}Z_{Po,j4}^*Z_{Go,i2} \\ & +Z_{Po,j3}^*\Big(-ig_{A2}\frac{1}{\sqrt{gA2^2+gB2^2}}Z_{Go,i1}+i\sqrt{\frac{gA2^2}{gA2^2+gB2^2}}Z_{Go,i3}\Big) \\ & +iZ_{Po,j1}^*\Big(-g_{A2}\frac{1}{\sqrt{gA2^2+gB2^2}}Z_{Go,i3}+\sqrt{\frac{gA2^2}{gA2^2+gB2^2}}Z_{Go,i1}\Big)+ig_{A2}\frac{1}{\sqrt{gA2^2+gB2^2}}Z_{Po,j2}^*Z_{Go,i4} \\ & -i\sqrt{\frac{gA2^2}{gA2^2+gB2^2}}Z_{Po,j4}^*Z_{Go,i4}-2\sqrt{\frac{gA2^2}{gA2^2+gB2^2}}Z_{Po,j7}^*Z_{Go,i7} \\ & +2g_{A2}^{-2}g_{B2}^2\left(\frac{gA2^2}{gA2^2+gB2^2}\right)^{3/2}Z_{Po,j7}^*Z_{Go,i7}-2g_{A2}g_{B2}^2\frac{1}{\left(gA2^2+gB2^2\right)^{3/2}}Z_{Po,j7}^*Z_{Go,i7} \\ & +2g_{A2}^{-1}g_{B2}\left(\frac{gA2^2}{gA2^2+gB2^2}\right)^{3/2}Z_{Po,j8}^*Z_{Go,i7}+2g_{B2}^3\frac{1}{\left(gA2^2+gB2^2\right)^{3/2}}Z_{Po,j8}^*Z_{Go,i7} \\ & -2g_{B2}\frac{1}{\sqrt{gA2^2+gB2^2}}Z_{Po,j8}^*Z_{Go,i7}+2g_{A2}^{-1}g_{B2}\left(\frac{gA2^2}{gA2^2+gB2^2}\right)^{3/2}Z_{Po,j7}^*Z_{Go,i8} \\ & +2g_{B2}^3\frac{1}{\left(gA2^2+gB2^2\right)^{3/2}}Z_{Po,j7}^*Z_{Go,i8}-2g_{B2}\frac{1}{\sqrt{gA2^2+gB2^2}}Z_{Po,j7}^*Z_{Go,i8} \\ & -2g_{A2}^{-2}g_{B2}^2\left(\frac{gA2^2}{gA2^2+gB2^2}\right)^{3/2}Z_{Po,j8}^*Z_{Go,i8}+2g_{A2}g_{B2}^2\frac{1}{\left(gA2^2+gB2^2\right)^{3/2}}Z_{Po,j8}^*Z_{Go,i8} \\ & -2g_{A2}\frac{1}{\sqrt{gA2^2+gB2^2}}Z_{Po,j8}^*Z_{Go,i8}+i\sqrt{2}\sqrt{\frac{gA2^2}{gA2^2+gB2^2}}Z_{Po,j9}^*Z_{Go,i9} \\ & -i\sqrt{2}\sqrt{\frac{gA2^2}{gA2^2+gB2^2}}Z_{Po,j9}^*Z_{Go,i10}\Big)\Big(\gamma_\mu\cdot\frac{1-\gamma_5}{2}\Big) \end{aligned} \quad (686)$$

$$\begin{aligned}
& + \frac{1}{2}g_{B2} \left( i\sqrt{\frac{gA2^2}{gA2^2 + gB2^2}} Z_{Go,i2}^* Z_{Po,j2} - ig_{A2} \frac{1}{\sqrt{gA2^2 + gB2^2}} Z_{Go,i4}^* Z_{Po,j2} \right. \\
& + iZ_{Go,i3}^* \left( g_{A2} \frac{1}{\sqrt{gA2^2 + gB2^2}} Z_{Po,j1} - \sqrt{\frac{gA2^2}{gA2^2 + gB2^2}} Z_{Po,j3} \right) \\
& + Z_{Go,i1}^* \left( ig_{A2} \frac{1}{\sqrt{gA2^2 + gB2^2}} Z_{Po,j3} - i\sqrt{\frac{gA2^2}{gA2^2 + gB2^2}} Z_{Po,j1} \right) - ig_{A2} \frac{1}{\sqrt{gA2^2 + gB2^2}} Z_{Go,i2}^* Z_{Po,j4} \\
& + i\sqrt{\frac{gA2^2}{gA2^2 + gB2^2}} Z_{Go,i4}^* Z_{Po,j4} - 2\sqrt{\frac{gA2^2}{gA2^2 + gB2^2}} Z_{Go,i7}^* Z_{Po,j7} \\
& + 2g_{A2}^{-2} g_{B2}^2 \left( \frac{gA2^2}{gA2^2 + gB2^2} \right)^{3/2} Z_{Go,i7}^* Z_{Po,j7} - 2g_{A2} g_{B2}^2 \frac{1}{(gA2^2 + gB2^2)^{3/2}} Z_{Go,i7}^* Z_{Po,j7} \\
& + 2g_{A2}^{-1} g_{B2} \left( \frac{gA2^2}{gA2^2 + gB2^2} \right)^{3/2} Z_{Go,i8}^* Z_{Po,j7} + 2g_{B2}^3 \frac{1}{(gA2^2 + gB2^2)^{3/2}} Z_{Go,i8}^* Z_{Po,j7} \\
& - 2g_{B2} \frac{1}{\sqrt{gA2^2 + gB2^2}} Z_{Go,i8}^* Z_{Po,j7} + 2g_{A2}^{-1} g_{B2} \left( \frac{gA2^2}{gA2^2 + gB2^2} \right)^{3/2} Z_{Go,i7}^* Z_{Po,j8} \\
& + 2g_{B2}^3 \frac{1}{(gA2^2 + gB2^2)^{3/2}} Z_{Go,i7}^* Z_{Po,j8} - 2g_{B2} \frac{1}{\sqrt{gA2^2 + gB2^2}} Z_{Go,i7}^* Z_{Po,j8} \\
& - 2g_{A2}^{-2} g_{B2}^2 \left( \frac{gA2^2}{gA2^2 + gB2^2} \right)^{3/2} Z_{Go,i8}^* Z_{Po,j8} + 2g_{A2} g_{B2}^2 \frac{1}{(gA2^2 + gB2^2)^{3/2}} Z_{Go,i8}^* Z_{Po,j8} \\
& - 2g_{A2} \frac{1}{\sqrt{gA2^2 + gB2^2}} Z_{Go,i8}^* Z_{Po,j8} - i\sqrt{2} \sqrt{\frac{gA2^2}{gA2^2 + gB2^2}} Z_{Go,i9}^* Z_{Po,j9} \\
& + i\sqrt{2} \sqrt{\frac{gA2^2}{gA2^2 + gB2^2}} Z_{Go,i10}^* Z_{Po,j9} \Big) \left( \gamma_\mu \cdot \frac{1 + \gamma_5}{2} \right)
\end{aligned} \tag{687}$$

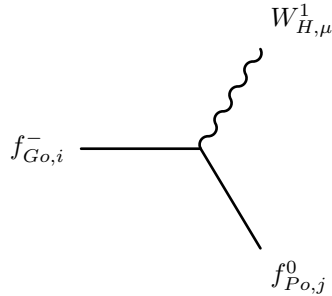

$$\begin{aligned}
& \frac{1}{2} \frac{1}{\left(gA^2 + gB^2\right)^{3/2}} \left( -ig_{A2}^2 g_{B2}^2 Z_{Po,j2}^* Z_{Go,i2} - ig_{B2}^4 Z_{Po,j2}^* Z_{Go,i2} \right. \\
& - ig_{A2} g_{B2}^2 \sqrt{\frac{gA^2}{gA^2 + gB^2}} \sqrt{gA^2 + gB^2} Z_{Po,j4}^* Z_{Go,i2} \\
& - ig_{A2} \left( \frac{gA^2}{gA^2 + gB^2} \right)^{3/2} \left( gA^2 + gB^2 \right)^{3/2} Z_{Po,j4}^* Z_{Go,i2} \\
& + i \left( g_{A2}^2 + g_{B2}^2 \right) Z_{Po,j3}^* \left( g_{A2} \sqrt{\frac{gA^2}{gA^2 + gB^2}} \sqrt{gA^2 + gB^2} Z_{Go,i1} + g_{B2}^2 Z_{Go,i3} \right) \\
& + i \left( g_{A2}^2 + g_{B2}^2 \right) Z_{Po,j1}^* \left( g_{A2} \sqrt{\frac{gA^2}{gA^2 + gB^2}} \sqrt{gA^2 + gB^2} Z_{Go,i3} + g_{B2}^2 Z_{Go,i1} \right) \\
& - ig_{A2} g_{B2}^2 \sqrt{\frac{gA^2}{gA^2 + gB^2}} \sqrt{gA^2 + gB^2} Z_{Po,j2}^* Z_{Go,i4} \\
& - ig_{A2} \left( \frac{gA^2}{gA^2 + gB^2} \right)^{3/2} \left( gA^2 + gB^2 \right)^{3/2} Z_{Po,j2}^* Z_{Go,i4} - ig_{A2}^2 g_{B2}^2 Z_{Po,j4}^* Z_{Go,i4} - ig_{B2}^4 Z_{Po,j4}^* Z_{Go,i4} \\
& - 2g_{A2}^2 g_{B2}^2 Z_{Po,j7}^* Z_{Go,i7} + 2g_{A2} g_{B2}^2 \sqrt{\frac{gA^2}{gA^2 + gB^2}} \sqrt{gA^2 + gB^2} Z_{Po,j7}^* Z_{Go,i7} \\
& - 2g_{A2}^3 g_{B2} Z_{Po,j8}^* Z_{Go,i7} - 2g_{B2}^3 \sqrt{\frac{gA^2}{gA^2 + gB^2}} \sqrt{gA^2 + gB^2} Z_{Po,j8}^* Z_{Go,i7} \\
& - 2g_{A2}^3 g_{B2} Z_{Po,j7}^* Z_{Go,i8} - 2g_{B2}^3 \sqrt{\frac{gA^2}{gA^2 + gB^2}} \sqrt{gA^2 + gB^2} Z_{Po,j7}^* Z_{Go,i8} - 2g_{B2}^4 Z_{Po,j8}^* Z_{Go,i8} \\
& + 2g_{A2} \left( \frac{gA^2}{gA^2 + gB^2} \right)^{3/2} \left( gA^2 + gB^2 \right)^{3/2} Z_{Po,j8}^* Z_{Go,i8} + i\sqrt{2} g_{A2}^2 g_{B2}^2 Z_{Po,j9}^* Z_{Go,i9} \\
& + i\sqrt{2} g_{B2}^4 Z_{Po,j9}^* Z_{Go,i9} - i\sqrt{2} g_{A2}^2 g_{B2}^2 Z_{Po,j9}^* Z_{Go,i10} - i\sqrt{2} g_{B2}^4 Z_{Po,j9}^* Z_{Go,i10} \left( \gamma_\mu \cdot \frac{1 - \gamma_5}{2} \right) \\
& + \frac{1}{2} \frac{1}{\left(gA^2 + gB^2\right)^{3/2}} \left( ig_{A2}^2 g_{B2}^2 Z_{Go,i2}^* Z_{Po,j2} + ig_{B2}^4 Z_{Go,i2}^* Z_{Po,j2} \right. \\
& + ig_{A2} g_{B2}^2 \sqrt{\frac{gA^2}{gA^2 + gB^2}} \sqrt{gA^2 + gB^2} Z_{Go,i4}^* Z_{Po,j2} \\
& + ig_{A2} \left( \frac{gA^2}{gA^2 + gB^2} \right)^{3/2} \left( gA^2 + gB^2 \right)^{3/2} Z_{Go,i4}^* Z_{Po,j2} \\
& \left. - i \left( g_{A2}^2 + g_{B2}^2 \right) Z_{Go,i3}^* \left( g_{A2} \sqrt{\frac{gA^2}{gA^2 + gB^2}} \sqrt{gA^2 + gB^2} Z_{Po,j1} + g_{B2}^2 Z_{Po,j3} \right) \right)
\end{aligned} \tag{688}$$

$$\begin{aligned}
& -i(g_{A2}^2 + g_{B2}^2)Z_{Go,i1}^* \left( g_{A2} \sqrt{\frac{gA2^2}{gA2^2 + gB2^2}} \sqrt{gA2^2 + gB2^2} Z_{Po,j3} + g_{B2}^2 Z_{Po,j1} \right) \\
& + ig_{A2}g_{B2}^2 \sqrt{\frac{gA2^2}{gA2^2 + gB2^2}} \sqrt{gA2^2 + gB2^2} Z_{Go,i2}^* Z_{Po,j4} \\
& + ig_{A2} \left( \frac{gA2^2}{gA2^2 + gB2^2} \right)^{3/2} (gA2^2 + gB2^2)^{3/2} Z_{Go,i2}^* Z_{Po,j4} + ig_{A2}^2 g_{B2}^2 Z_{Go,i4}^* Z_{Po,j4} + ig_{B2}^4 Z_{Go,i4}^* Z_{Po,j4} \\
& - 2g_{A2}^2 g_{B2}^2 Z_{Go,i7}^* Z_{Po,j7} + 2g_{A2}g_{B2}^2 \sqrt{\frac{gA2^2}{gA2^2 + gB2^2}} \sqrt{gA2^2 + gB2^2} Z_{Go,i7}^* Z_{Po,j7} \\
& - 2g_{A2}^3 g_{B2} Z_{Go,i8}^* Z_{Po,j7} - 2g_{B2}^3 \sqrt{\frac{gA2^2}{gA2^2 + gB2^2}} \sqrt{gA2^2 + gB2^2} Z_{Go,i8}^* Z_{Po,j7} \\
& - 2g_{A2}^3 g_{B2} Z_{Go,i7}^* Z_{Po,j8} - 2g_{B2}^3 \sqrt{\frac{gA2^2}{gA2^2 + gB2^2}} \sqrt{gA2^2 + gB2^2} Z_{Go,i7}^* Z_{Po,j8} - 2g_{B2}^4 Z_{Go,i8}^* Z_{Po,j8} \\
& + 2g_{A2} \left( \frac{gA2^2}{gA2^2 + gB2^2} \right)^{3/2} (gA2^2 + gB2^2)^{3/2} Z_{Go,i8}^* Z_{Po,j8} - i\sqrt{2}g_{A2}^2 g_{B2}^2 Z_{Go,i9}^* Z_{Po,j9} \\
& - i\sqrt{2}g_{B2}^4 Z_{Go,i9}^* Z_{Po,j9} + i\sqrt{2}g_{A2}^2 g_{B2}^2 Z_{Go,i10}^* Z_{Po,j9} + i\sqrt{2}g_{B2}^4 Z_{Go,i10}^* Z_{Po,j9} \left( \gamma_\mu \cdot \frac{1 + \gamma_5}{2} \right)
\end{aligned} \tag{689}$$


---

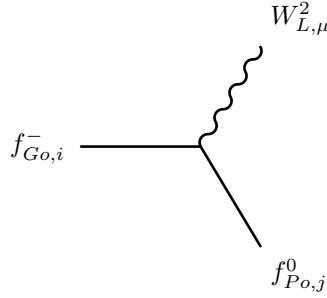

$$\begin{aligned}
& \frac{1}{2}g_{B2} \frac{1}{(gA2^2 + gB2^2)^{3/2}} \left( g_{B2}^2 \sqrt{\frac{gA2^2}{gA2^2 + gB2^2}} \sqrt{gA2^2 + gB2^2} Z_{Po,j2}^* Z_{Go,i2} \right. \\
& + \left( \frac{gA2^2}{gA2^2 + gB2^2} \right)^{3/2} (gA2^2 + gB2^2)^{3/2} Z_{Po,j2}^* Z_{Go,i2} - g_{A2}^3 Z_{Po,j4}^* Z_{Go,i2} - g_{A2}g_{B2}^2 Z_{Po,j4}^* Z_{Go,i2} \\
& + (g_{A2}^2 + g_{B2}^2) Z_{Po,j1}^* \left( g_{A2} Z_{Go,i3} + \sqrt{\frac{gA2^2}{gA2^2 + gB2^2}} \sqrt{gA2^2 + gB2^2} Z_{Go,i1} \right) \\
& \left. - (g_{A2}^2 + g_{B2}^2) Z_{Po,j3}^* \left( g_{A2} Z_{Go,i1} + \sqrt{\frac{gA2^2}{gA2^2 + gB2^2}} \sqrt{gA2^2 + gB2^2} Z_{Go,i3} \right) + g_{A2}^3 Z_{Po,j2}^* Z_{Go,i4} \right)
\end{aligned}$$

$$\begin{aligned}
& + g_{A2} g_{B2}^2 Z_{Po,j2}^* Z_{Go,i4} - g_{B2}^2 \sqrt{\frac{gA2^2}{gA2^2 + gB2^2}} \sqrt{gA2^2 + gB2^2} Z_{Po,j4}^* Z_{Go,i4} \\
& - \left( \frac{gA2^2}{gA2^2 + gB2^2} \right)^{3/2} (gA2^2 + gB2^2)^{3/2} Z_{Po,j4}^* Z_{Go,i4} + 2g_{A2} g_{B2}^2 Z_{Po,j7}^* Z_{Go,i5} \\
& + 2 \left( \frac{gA2^2}{gA2^2 + gB2^2} \right)^{3/2} (gA2^2 + gB2^2)^{3/2} Z_{Po,j7}^* Z_{Go,i5} + 2g_{A2}^2 g_{B2} Z_{Po,j8}^* Z_{Go,i5} \\
& - 2g_{A2} g_{B2} \sqrt{\frac{gA2^2}{gA2^2 + gB2^2}} \sqrt{gA2^2 + gB2^2} Z_{Po,j8}^* Z_{Go,i5} + 2g_{A2}^2 g_{B2} Z_{Po,j7}^* Z_{Go,i6} \\
& - 2g_{A2} g_{B2} \sqrt{\frac{gA2^2}{gA2^2 + gB2^2}} \sqrt{gA2^2 + gB2^2} Z_{Po,j7}^* Z_{Go,i6} + 2g_{A2}^3 Z_{Po,j8}^* Z_{Go,i6} \\
& + 2g_{B2}^2 \sqrt{\frac{gA2^2}{gA2^2 + gB2^2}} \sqrt{gA2^2 + gB2^2} Z_{Po,j8}^* Z_{Go,i6} \\
& + \sqrt{2} g_{B2}^2 \sqrt{\frac{gA2^2}{gA2^2 + gB2^2}} \sqrt{gA2^2 + gB2^2} Z_{Po,j9}^* Z_{Go,i9} \\
& + \sqrt{2} \left( \frac{gA2^2}{gA2^2 + gB2^2} \right)^{3/2} (gA2^2 + gB2^2)^{3/2} Z_{Po,j9}^* Z_{Go,i9} \\
& + \sqrt{2} g_{B2}^2 \sqrt{\frac{gA2^2}{gA2^2 + gB2^2}} \sqrt{gA2^2 + gB2^2} Z_{Po,j9}^* Z_{Go,i10} \\
& + \sqrt{2} \left( \frac{gA2^2}{gA2^2 + gB2^2} \right)^{3/2} (gA2^2 + gB2^2)^{3/2} Z_{Po,j9}^* Z_{Go,i10} \left( \gamma_\mu \cdot \frac{1 - \gamma_5}{2} \right) \\
& + \frac{1}{2} g_{B2} \frac{1}{(gA2^2 + gB2^2)^{3/2}} \left( g_{B2}^2 \sqrt{\frac{gA2^2}{gA2^2 + gB2^2}} \sqrt{gA2^2 + gB2^2} Z_{Go,i2}^* Z_{Po,j2} \right. \\
& + \left( \frac{gA2^2}{gA2^2 + gB2^2} \right)^{3/2} (gA2^2 + gB2^2)^{3/2} Z_{Go,i2}^* Z_{Po,j2} + g_{A2}^3 Z_{Go,i4}^* Z_{Po,j2} + g_{A2} g_{B2}^2 Z_{Go,i4}^* Z_{Po,j2} \\
& + (g_{A2}^2 + g_{B2}^2) Z_{Go,i1}^* \left( -g_{A2} Z_{Po,j3} + \sqrt{\frac{gA2^2}{gA2^2 + gB2^2}} \sqrt{gA2^2 + gB2^2} Z_{Po,j1} \right) \\
& + (g_{A2}^2 + g_{B2}^2) Z_{Go,i3}^* \left( g_{A2} Z_{Po,j1} - \sqrt{\frac{gA2^2}{gA2^2 + gB2^2}} \sqrt{gA2^2 + gB2^2} Z_{Po,j3} \right) - g_{A2}^3 Z_{Go,i2}^* Z_{Po,j4} \\
& - g_{A2} g_{B2}^2 Z_{Go,i2}^* Z_{Po,j4} - g_{B2}^2 \sqrt{\frac{gA2^2}{gA2^2 + gB2^2}} \sqrt{gA2^2 + gB2^2} Z_{Go,i4}^* Z_{Po,j4} \\
& - \left( \frac{gA2^2}{gA2^2 + gB2^2} \right)^{3/2} (gA2^2 + gB2^2)^{3/2} Z_{Go,i4}^* Z_{Po,j4} + 2g_{A2} g_{B2}^2 Z_{Go,i5}^* Z_{Po,j7} \\
& + 2 \left( \frac{gA2^2}{gA2^2 + gB2^2} \right)^{3/2} (gA2^2 + gB2^2)^{3/2} Z_{Go,i5}^* Z_{Po,j7} + 2g_{A2}^2 g_{B2} Z_{Go,i6}^* Z_{Po,j7}
\end{aligned} \tag{690}$$



$$\begin{aligned}
& -2g_{A2}g_{B2}\sqrt{\frac{gA2^2}{gA2^2+gB2^2}}\sqrt{gA2^2+gB2^2}Z_{Go,i6}^*Z_{Po,j7}+2g_{A2}^2g_{B2}Z_{Go,i5}^*Z_{Po,j8} \\
& -2g_{A2}g_{B2}\sqrt{\frac{gA2^2}{gA2^2+gB2^2}}\sqrt{gA2^2+gB2^2}Z_{Go,i5}^*Z_{Po,j8}+2g_{A2}^3Z_{Go,i6}^*Z_{Po,j8} \\
& +2g_{B2}^2\sqrt{\frac{gA2^2}{gA2^2+gB2^2}}\sqrt{gA2^2+gB2^2}Z_{Go,i6}^*Z_{Po,j8} \\
& +\sqrt{2}g_{B2}^2\sqrt{\frac{gA2^2}{gA2^2+gB2^2}}\sqrt{gA2^2+gB2^2}Z_{Go,i9}^*Z_{Po,j9} \\
& +\sqrt{2}\left(\frac{gA2^2}{gA2^2+gB2^2}\right)^{3/2}\left(gA2^2+gB2^2\right)^{3/2}Z_{Go,i9}^*Z_{Po,j9} \\
& +\sqrt{2}g_{B2}^2\sqrt{\frac{gA2^2}{gA2^2+gB2^2}}\sqrt{gA2^2+gB2^2}Z_{Go,i10}^*Z_{Po,j9} \\
& +\sqrt{2}\left(\frac{gA2^2}{gA2^2+gB2^2}\right)^{3/2}\left(gA2^2+gB2^2\right)^{3/2}Z_{Go,i10}^*Z_{Po,j9}\left(\gamma_\mu\cdot\frac{1+\gamma_5}{2}\right)
\end{aligned} \tag{691}$$


---

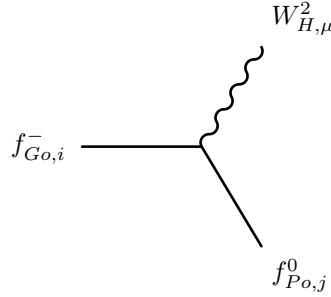

$$\begin{aligned}
& \frac{1}{2}\frac{1}{\left(gA2^2+gB2^2\right)^{3/2}}\left(g_{A2}^2g_{B2}^2Z_{Po,j2}^*Z_{Go,i2}+g_{B2}^4Z_{Po,j2}^*Z_{Go,i2}+g_{A2}g_{B2}^2\sqrt{\frac{gA2^2}{gA2^2+gB2^2}}\sqrt{gA2^2+gB2^2}Z_{Po,j4}^*Z_{Go,i2}\right. \\
& +g_{A2}\left(\frac{gA2^2}{gA2^2+gB2^2}\right)^{3/2}\left(gA2^2+gB2^2\right)^{3/2}Z_{Po,j4}^*Z_{Go,i2} \\
& +\left(g_{A2}^2+g_{B2}^2\right)Z_{Po,j3}^*\left(g_{A2}\sqrt{\frac{gA2^2}{gA2^2+gB2^2}}\sqrt{gA2^2+gB2^2}Z_{Go,i1}-g_{B2}^2Z_{Go,i3}\right) \\
& -\left(g_{A2}^2+g_{B2}^2\right)Z_{Po,j1}^*\left(g_{A2}\sqrt{\frac{gA2^2}{gA2^2+gB2^2}}\sqrt{gA2^2+gB2^2}Z_{Go,i3}-g_{B2}^2Z_{Go,i1}\right) \\
& \left.-g_{A2}g_{B2}^2\sqrt{\frac{gA2^2}{gA2^2+gB2^2}}\sqrt{gA2^2+gB2^2}Z_{Po,j2}^*Z_{Go,i4}\right)
\end{aligned}$$

$$\begin{aligned}
& -g_{A2} \left( \frac{gA2^2}{gA2^2 + gB2^2} \right)^{3/2} \left( gA2^2 + gB2^2 \right)^{3/2} Z_{Po,j2}^* Z_{Go,i4} - g_{A2}^2 g_{B2}^2 Z_{Po,j4}^* Z_{Go,i4} - g_{B2}^4 Z_{Po,j4}^* Z_{Go,i4} \\
& + 2g_{A2}^2 g_{B2}^2 Z_{Po,j7}^* Z_{Go,i5} - 2g_{A2} g_{B2}^2 \sqrt{\frac{gA2^2}{gA2^2 + gB2^2}} \sqrt{gA2^2 + gB2^2} Z_{Po,j7}^* Z_{Go,i5} \\
& + 2g_{A2}^3 g_{B2} Z_{Po,j8}^* Z_{Go,i5} + 2g_{B2}^3 \sqrt{\frac{gA2^2}{gA2^2 + gB2^2}} \sqrt{gA2^2 + gB2^2} Z_{Po,j8}^* Z_{Go,i5} \\
& + 2g_{A2}^3 g_{B2} Z_{Po,j7}^* Z_{Go,i6} + 2g_{B2}^3 \sqrt{\frac{gA2^2}{gA2^2 + gB2^2}} \sqrt{gA2^2 + gB2^2} Z_{Po,j7}^* Z_{Go,i6} + 2g_{B2}^4 Z_{Po,j8}^* Z_{Go,i6} \\
& - 2g_{A2} \left( \frac{gA2^2}{gA2^2 + gB2^2} \right)^{3/2} \left( gA2^2 + gB2^2 \right)^{3/2} Z_{Po,j8}^* Z_{Go,i6} + \sqrt{2} g_{A2}^2 g_{B2}^2 Z_{Po,j9}^* Z_{Go,i9} \\
& + \sqrt{2} g_{B2}^4 Z_{Po,j9}^* Z_{Go,i9} + \sqrt{2} g_{A2}^2 g_{B2}^2 Z_{Po,j9}^* Z_{Go,i10} + \sqrt{2} g_{B2}^4 Z_{Po,j9}^* Z_{Go,i10} \left( \gamma_\mu \cdot \frac{1 - \gamma_5}{2} \right) \\
& + \frac{1}{2} \frac{1}{\left( gA2^2 + gB2^2 \right)^{3/2}} \left( g_{A2}^2 g_{B2}^2 Z_{Go,i2}^* Z_{Po,j2} + g_{B2}^4 Z_{Go,i2}^* Z_{Po,j2} \right. \\
& - g_{A2} g_{B2}^2 \sqrt{\frac{gA2^2}{gA2^2 + gB2^2}} \sqrt{gA2^2 + gB2^2} Z_{Go,i4}^* Z_{Po,j2} \\
& - g_{A2} \left( \frac{gA2^2}{gA2^2 + gB2^2} \right)^{3/2} \left( gA2^2 + gB2^2 \right)^{3/2} Z_{Go,i4}^* Z_{Po,j2} \\
& - \left( g_{A2}^2 + g_{B2}^2 \right) Z_{Go,i3}^* \left( g_{A2} \sqrt{\frac{gA2^2}{gA2^2 + gB2^2}} \sqrt{gA2^2 + gB2^2} Z_{Po,j1} + g_{B2}^2 Z_{Po,j3} \right) \\
& + \left( g_{A2}^2 + g_{B2}^2 \right) Z_{Go,i1}^* \left( g_{A2} \sqrt{\frac{gA2^2}{gA2^2 + gB2^2}} \sqrt{gA2^2 + gB2^2} Z_{Po,j3} + g_{B2}^2 Z_{Po,j1} \right) \\
& + g_{A2} g_{B2}^2 \sqrt{\frac{gA2^2}{gA2^2 + gB2^2}} \sqrt{gA2^2 + gB2^2} Z_{Go,i2}^* Z_{Po,j4} \\
& + g_{A2} \left( \frac{gA2^2}{gA2^2 + gB2^2} \right)^{3/2} \left( gA2^2 + gB2^2 \right)^{3/2} Z_{Go,i2}^* Z_{Po,j4} - g_{A2}^2 g_{B2}^2 Z_{Go,i4}^* Z_{Po,j4} - g_{B2}^4 Z_{Go,i4}^* Z_{Po,j4} \\
& + 2g_{A2}^2 g_{B2}^2 Z_{Go,i5}^* Z_{Po,j7} - 2g_{A2} g_{B2}^2 \sqrt{\frac{gA2^2}{gA2^2 + gB2^2}} \sqrt{gA2^2 + gB2^2} Z_{Go,i5}^* Z_{Po,j7} \\
& + 2g_{A2}^3 g_{B2} Z_{Go,i6}^* Z_{Po,j7} + 2g_{B2}^3 \sqrt{\frac{gA2^2}{gA2^2 + gB2^2}} \sqrt{gA2^2 + gB2^2} Z_{Go,i6}^* Z_{Po,j7} \\
& + 2g_{A2}^3 g_{B2} Z_{Go,i5}^* Z_{Po,j8} + 2g_{B2}^3 \sqrt{\frac{gA2^2}{gA2^2 + gB2^2}} \sqrt{gA2^2 + gB2^2} Z_{Go,i5}^* Z_{Po,j8} + 2g_{B2}^4 Z_{Go,i6}^* Z_{Po,j8} \\
& - 2g_{A2} \left( \frac{gA2^2}{gA2^2 + gB2^2} \right)^{3/2} \left( gA2^2 + gB2^2 \right)^{3/2} Z_{Go,i6}^* Z_{Po,j8} + \sqrt{2} g_{A2}^2 g_{B2}^2 Z_{Go,i9}^* Z_{Po,j9}
\end{aligned} \tag{692}$$

$$+ \sqrt{2}g_{B2}^4 Z_{Go,i9}^* Z_{Po,j9} + \sqrt{2}g_{A2}^2 g_{B2}^2 Z_{Go,i10}^* Z_{Po,j9} + \sqrt{2}g_{B2}^4 Z_{Go,i10}^* Z_{Po,j9} \Big) \left( \gamma_\mu \cdot \frac{1+\gamma_5}{2} \right) \quad (693)$$


---

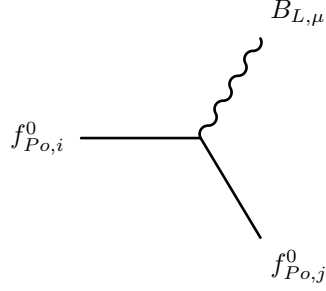

$$- \frac{i}{2} g_{B1} \frac{1}{\sqrt{gA1^2 + gB1^2}} \left( -g_{A1} + \sqrt{\frac{gA1^2}{gA1^2 + gB1^2}} \sqrt{gA1^2 + gB1^2} \right) \left( Z_{Po,j1}^* Z_{Po,i1} - Z_{Po,j2}^* Z_{Po,i2} + Z_{Po,j3}^* Z_{Po,i3} - Z_{Po,j4}^* Z_{Po,i4} \right) \left( \gamma_\mu \cdot \frac{1+\gamma_5}{2} \right) \quad (694)$$

$$+ \frac{i}{2} g_{B1} \frac{1}{\sqrt{gA1^2 + gB1^2}} \left( -g_{A1} + \sqrt{\frac{gA1^2}{gA1^2 + gB1^2}} \sqrt{gA1^2 + gB1^2} \right) \left( Z_{Po,i1}^* Z_{Po,j1} - Z_{Po,i2}^* Z_{Po,j2} + Z_{Po,i3}^* Z_{Po,j3} - Z_{Po,i4}^* Z_{Po,j4} \right) \left( \gamma_\mu \cdot \frac{1+\gamma_5}{2} \right) \quad (695)$$


---

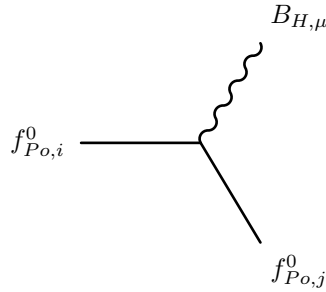

$$- \frac{i}{2} \frac{1}{\sqrt{gA1^2 + gB1^2}} \left( g_{A1} \sqrt{\frac{gA1^2}{gA1^2 + gB1^2}} \sqrt{gA1^2 + gB1^2} + g_{B1}^2 \right) \left( Z_{Po,j1}^* Z_{Po,i1} - Z_{Po,j2}^* Z_{Po,i2} + Z_{Po,j3}^* Z_{Po,i3} - Z_{Po,j4}^* Z_{Po,i4} \right) \left( \gamma_\mu \cdot \frac{1+\gamma_5}{2} \right) \quad (696)$$

$$+ \frac{i}{2} \frac{1}{\sqrt{gA1^2 + gB1^2}} \left( g_{A1} \sqrt{\frac{gA1^2}{gA1^2 + gB1^2}} \sqrt{gA1^2 + gB1^2} + g_{B1}^2 \right) \left( Z_{Po,i1}^* Z_{Po,j1} - Z_{Po,i2}^* Z_{Po,j2} + Z_{Po,i3}^* Z_{Po,j3} - Z_{Po,i4}^* Z_{Po,j4} \right) \left( \gamma_\mu \cdot \frac{1+\gamma_5}{2} \right) \quad (697)$$


---

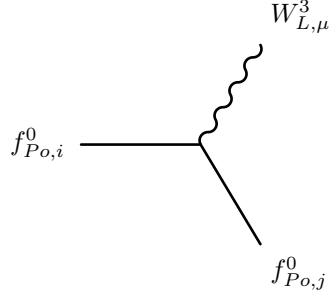

$$\frac{i}{2} g_{B2} \frac{1}{\sqrt{gA2^2 + gB2^2}} \left( -g_{A2} + \sqrt{\frac{gA2^2}{gA2^2 + gB2^2}} \sqrt{gA2^2 + gB2^2} \right) \left( Z_{Po,j1}^* Z_{Po,i1} - Z_{Po,j2}^* Z_{Po,i2} - Z_{Po,j3}^* Z_{Po,i3} + Z_{Po,j4}^* Z_{Po,i4} \right) \left( \gamma_\mu \cdot \frac{1}{2} \right. \\ \left. (698) \right)$$

$$+ -\frac{i}{2} g_{B2} \frac{1}{\sqrt{gA2^2 + gB2^2}} \left( -g_{A2} + \sqrt{\frac{gA2^2}{gA2^2 + gB2^2}} \sqrt{gA2^2 + gB2^2} \right) \left( Z_{Po,i1}^* Z_{Po,j1} - Z_{Po,i2}^* Z_{Po,j2} - Z_{Po,i3}^* Z_{Po,j3} + Z_{Po,i4}^* Z_{Po,j4} \right) \left( \gamma_\mu \cdot \frac{1}{2} \right) \\ \left. (699) \right)$$


---

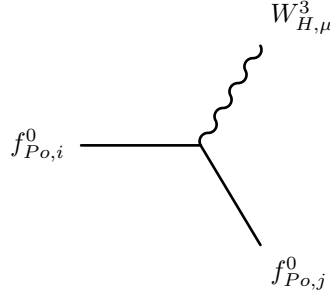

$$\frac{i}{2} \frac{1}{\sqrt{gA2^2 + gB2^2}} \left( g_{A2} \sqrt{\frac{gA2^2}{gA2^2 + gB2^2}} \sqrt{gA2^2 + gB2^2} + g_{B2}^2 \right) \left( Z_{Po,j1}^* Z_{Po,i1} - Z_{Po,j2}^* Z_{Po,i2} - Z_{Po,j3}^* Z_{Po,i3} + Z_{Po,j4}^* Z_{Po,i4} \right) \left( \gamma_\mu \cdot \frac{1}{2} \right. \\ \left. (700) \right)$$

$$+ -\frac{i}{2} \frac{1}{\sqrt{gA2^2 + gB2^2}} \left( g_{A2} \sqrt{\frac{gA2^2}{gA2^2 + gB2^2}} \sqrt{gA2^2 + gB2^2} + g_{B2}^2 \right) \left( Z_{Po,i1}^* Z_{Po,j1} - Z_{Po,i2}^* Z_{Po,j2} - Z_{Po,i3}^* Z_{Po,j3} + Z_{Po,i4}^* Z_{Po,j4} \right) \left( \gamma_\mu \cdot \frac{1}{2} \right) \\ \left. (701) \right)$$


---

## 9.5 Two Fermion-One Scalar Boson-Interaction

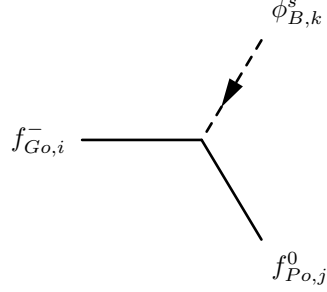

$$\begin{aligned}
& \frac{1}{\sqrt{gA^2 + gB^2}} \left( -i\sqrt{gA^2 + gB^2} Y_A B_{A,k1}^{s,*} \left( Z_{Go,i2}^* Z_{Po,j1}^* + Z_{Go,i3}^* Z_{Po,j4}^* \right) \right. \\
& + g_{B2} B_{A,k2}^{s,*} \left( i\sqrt{2} Z_{Go,i10}^* \left( g_{B2} Z_{Po,j8}^* + \sqrt{\frac{gA^2}{gA^2 + gB^2}} \sqrt{gA^2 + gB^2} Z_{Po,j7}^* \right) \right. \\
& + \left( -i\sqrt{\frac{gA^2}{gA^2 + gB^2}} \sqrt{gA^2 + gB^2} Z_{Go,i5}^* - ig_{B2} Z_{Go,i6}^* \right. \\
& \left. \left. + \sqrt{\frac{gA^2}{gA^2 + gB^2}} \sqrt{gA^2 + gB^2} Z_{Go,i7}^* + g_{B2} Z_{Go,i8}^* \right) Z_{Po,j9}^* \right) \left( \frac{1 - \gamma_5}{2} \right) \quad (702)
\end{aligned}$$

$$\begin{aligned}
& + -i \frac{1}{\sqrt{gA^2 + gB^2}} \left( \sqrt{gA^2 + gB^2} Y_A^* B_{A,k2}^{s,*} \left( Z_{Go,i1} Z_{Po,j2} + Z_{Go,i4} Z_{Po,j3} \right) \right. \\
& + g_{B2} B_{A,k1}^{s,*} \left( \sqrt{2} Z_{Go,i9} \left( g_{B2} Z_{Po,j8} + \sqrt{\frac{gA^2}{gA^2 + gB^2}} \sqrt{gA^2 + gB^2} Z_{Po,j7} \right) \right. \\
& - \left( \sqrt{\frac{gA^2}{gA^2 + gB^2}} \sqrt{gA^2 + gB^2} Z_{Go,i5} + g_{B2} Z_{Go,i6} \right. \\
& \left. \left. + i \left( g_{B2} Z_{Go,i8} + \sqrt{\frac{gA^2}{gA^2 + gB^2}} \sqrt{gA^2 + gB^2} Z_{Go,i7} \right) \right) Z_{Po,j9} \right) \left( \frac{1 + \gamma_5}{2} \right) \quad (703)
\end{aligned}$$

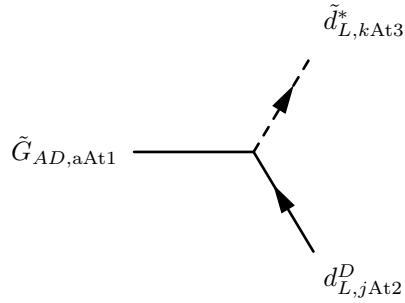

$$-i \frac{1}{\sqrt{2}} g_3 \delta_{jk} \lambda_{\text{At}3, \text{At}2}^{\text{aAt}1} \left( \frac{1 - \gamma_5}{2} \right) \quad (704)$$


---

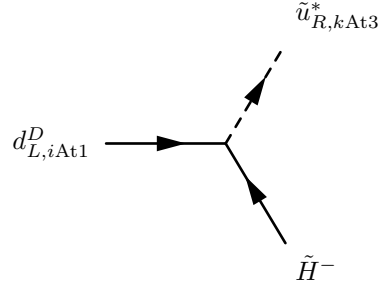

$$i \delta_{\text{At}1 \text{At}3} Y_{u,ki} \left( \frac{1 - \gamma_5}{2} \right) \quad (705)$$


---

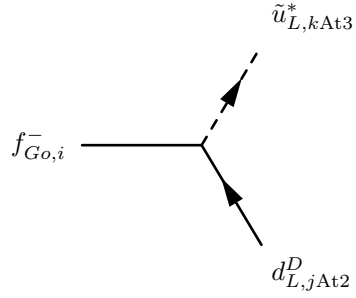

$$\begin{aligned} & \frac{1}{\sqrt{2}} g_{A2} \frac{1}{\sqrt{g_{A2}^2 + g_{B2}^2}} \left( -i g_{B2} Z_{Go,i5}^* + i \sqrt{\frac{g_{A2}^2}{g_{A2}^2 + g_{B2}^2}} \sqrt{g_{A2}^2 + g_{B2}^2} Z_{Go,i6}^* - g_{B2} Z_{Go,i7}^* \right. \\ & \left. + \sqrt{\frac{g_{A2}^2}{g_{A2}^2 + g_{B2}^2}} \sqrt{g_{A2}^2 + g_{B2}^2} Z_{Go,i8}^* \right) \delta_{\text{At}2 \text{At}3} \delta_{jk} \left( \frac{1 - \gamma_5}{2} \right) \end{aligned} \quad (706)$$


---

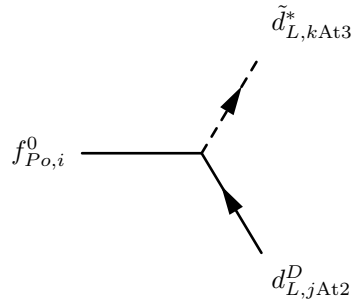

$$\begin{aligned}
& -\frac{i}{3}\frac{1}{\sqrt{2}}\left(g_{A1}g_{B1}\frac{1}{\sqrt{g_{A1}^2+g_{B1}^2}}Z_{Po,i5}^*-g_{A1}\sqrt{\frac{g_{A1}^2}{g_{A1}^2+g_{B1}^2}}Z_{Po,i6}^*-3g_{A2}g_{B2}\frac{1}{\sqrt{g_{A2}^2+g_{B2}^2}}Z_{Po,i7}^*\right. \\
& \left.+3g_{A2}\sqrt{\frac{g_{A2}^2}{g_{A2}^2+g_{B2}^2}}Z_{Po,i8}^*\right)\delta_{At2At3}\delta_{jk}\left(\frac{1-\gamma_5}{2}\right)
\end{aligned} \tag{707}$$


---

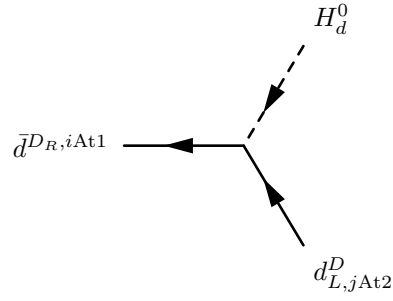

$$-i\delta_{At1At2}Y_{d,ij}\left(\frac{1-\gamma_5}{2}\right) \tag{708}$$


---

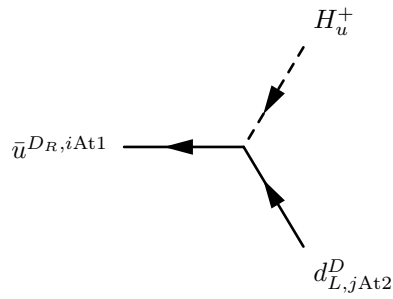

$$i\delta_{At1At2}Y_{u,ij}\left(\frac{1-\gamma_5}{2}\right) \tag{709}$$


---

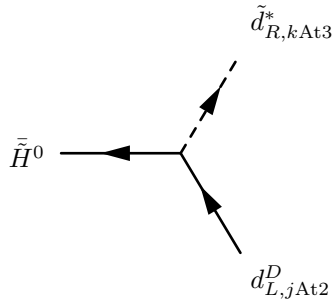

$$-i\delta_{\text{At}2\text{At}3}Y_{d,kj}\left(\frac{1-\gamma_5}{2}\right) \quad (710)$$


---

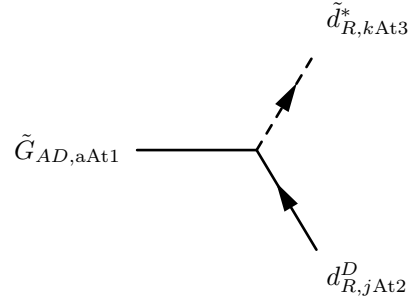

(711)

$$+i\frac{1}{\sqrt{2}}g_3\delta_{jk}\lambda_{\text{At}3,\text{At}2}^{\text{aAt}1}\left(\frac{1+\gamma_5}{2}\right) \quad (712)$$


---

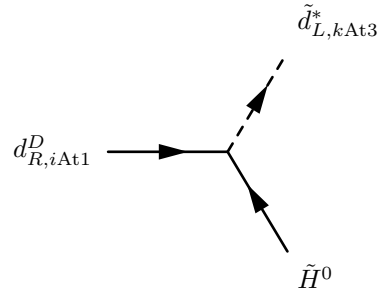

(713)

$$+ -iY_{d,ik}^*\delta_{\text{At}1\text{At}3}\left(\frac{1+\gamma_5}{2}\right) \quad (714)$$


---

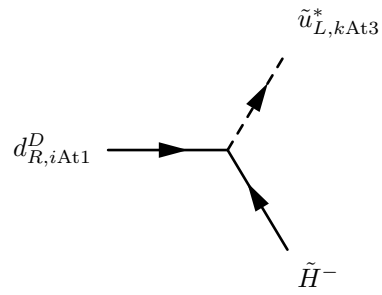



(715)

$$+ iY_{d,ik}^* \delta_{\text{At1At3}} \left( \frac{1 + \gamma_5}{2} \right) \quad (716)$$

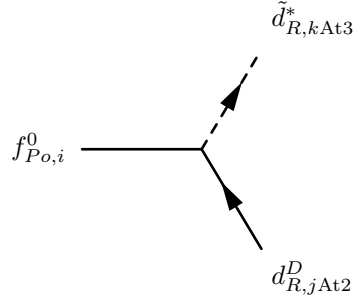

(717)

$$+ \frac{i}{3} \sqrt{2} g_{A1} \frac{1}{\sqrt{g_{A1}^2 + g_{B1}^2}} \delta_{\text{At2At3}} \delta_{jk} \left( -g_{B1} Z_{Po,i5} + \sqrt{\frac{g_{A1}^2}{g_{A1}^2 + g_{B1}^2}} \sqrt{g_{A1}^2 + g_{B1}^2} Z_{Po,i6} \right) \left( \frac{1 + \gamma_5}{2} \right) \quad (718)$$

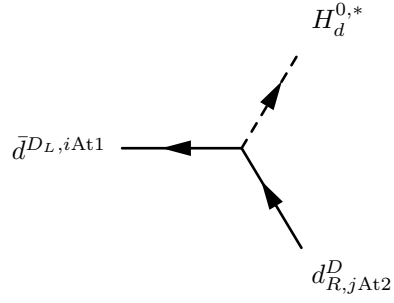

(719)

$$+ -iY_{d,ji}^* \delta_{\text{At1At2}} \left( \frac{1 + \gamma_5}{2} \right) \quad (720)$$

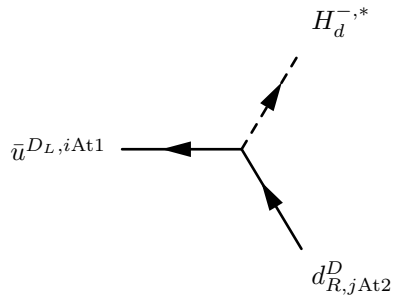

(721)

$$+ iY_{d,ji}^* \delta_{At1At2} \left( \frac{1 + \gamma_5}{2} \right) \quad (722)$$

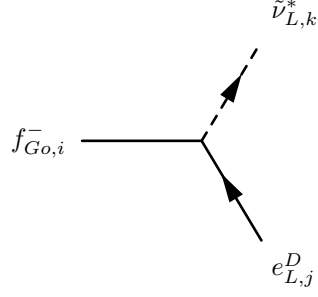

$$\begin{aligned} & \frac{1}{\sqrt{2}} g_{A2} \frac{1}{\sqrt{g_{A2}^2 + g_{B2}^2}} \left( -ig_{B2} Z_{Go,i5}^* + i \sqrt{\frac{g_{A2}^2}{g_{A2}^2 + g_{B2}^2}} \sqrt{g_{A2}^2 + g_{B2}^2} Z_{Go,i6}^* - g_{B2} Z_{Go,i7}^* \right. \\ & \left. + \sqrt{\frac{g_{A2}^2}{g_{A2}^2 + g_{B2}^2}} \sqrt{g_{A2}^2 + g_{B2}^2} Z_{Go,i8}^* \right) \delta_{jk} \left( \frac{1 - \gamma_5}{2} \right) \end{aligned} \quad (723)$$

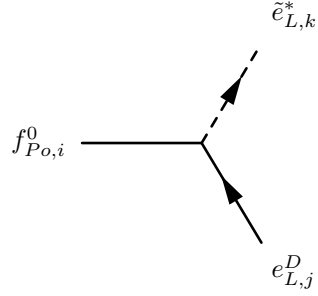

$$\begin{aligned} & i \frac{1}{\sqrt{2}} \left( g_{A1} g_{B1} \frac{1}{\sqrt{g_{A1}^2 + g_{B1}^2}} Z_{Po,i5}^* - g_{A1} \sqrt{\frac{g_{A1}^2}{g_{A1}^2 + g_{B1}^2}} Z_{Po,i6}^* + g_{A2} g_{B2} \frac{1}{\sqrt{g_{A2}^2 + g_{B2}^2}} Z_{Po,i7}^* \right. \\ & \left. - g_{A2} \sqrt{\frac{g_{A2}^2}{g_{A2}^2 + g_{B2}^2}} Z_{Po,i8}^* \right) \delta_{jk} \left( \frac{1 - \gamma_5}{2} \right) \end{aligned} \quad (724)$$

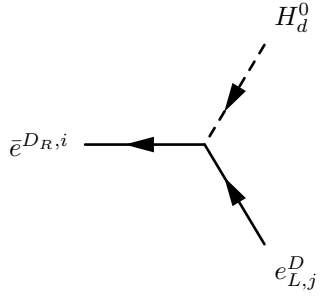

$$-iY_{e,ij}\left(\frac{1-\gamma_5}{2}\right) \quad (725)$$


---

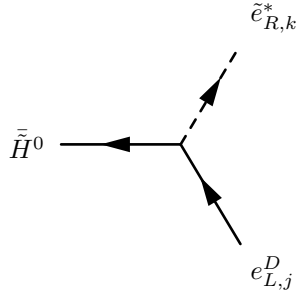

$$-iY_{e,kj}\left(\frac{1-\gamma_5}{2}\right) \quad (726)$$


---

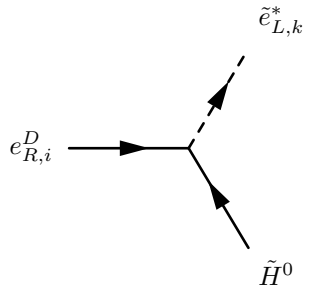

$$+ -iY_{e,ik}^*\left(\frac{1+\gamma_5}{2}\right) \quad (727)$$

$$(728)$$


---

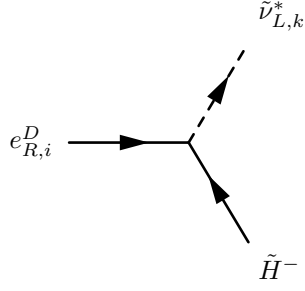

(729)

$$+ iY_{e,ik}^* \left( \frac{1 + \gamma_5}{2} \right)$$

(730)

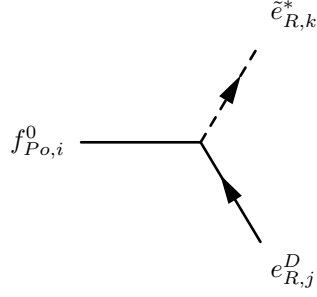

(731)

$$+ -i\sqrt{2}g_{A1}\delta_{jk} \left( g_{B1} \frac{1}{\sqrt{g_{A1}^2 + g_{B1}^2}} Z_{Po,i5} - \sqrt{\frac{g_{A1}^2}{g_{A1}^2 + g_{B1}^2}} Z_{Po,i6} \right) \left( \frac{1 + \gamma_5}{2} \right)$$

(732)

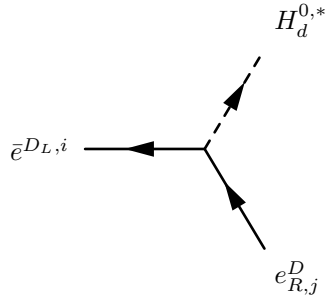

(733)

$$+ -iY_{e,ji}^* \left( \frac{1 + \gamma_5}{2} \right)$$

(734)

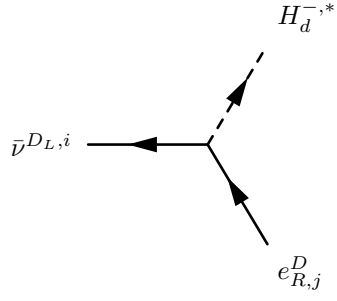

(735)

$$+ iY_{e,j}^* \left( \frac{1 + \gamma_5}{2} \right)$$

(736)

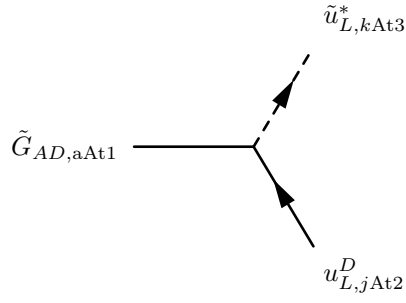

$$- i \frac{1}{\sqrt{2}} g_3 \delta_{jk} \lambda_{At3,At2}^{aAt1} \left( \frac{1 - \gamma_5}{2} \right)$$

(737)

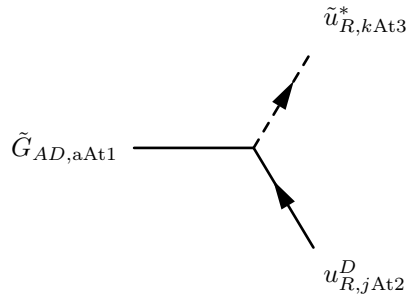

(738)

$$+ i \frac{1}{\sqrt{2}} g_3 \delta_{jk} \lambda_{At3,At2}^{aAt1} \left( \frac{1 + \gamma_5}{2} \right)$$

(739)

(740)

$$+ -i \frac{1}{\sqrt{2}} g_3 \delta_{ik} \lambda_{\text{At}1, \text{At}3}^{\text{aAt}2} \left( \frac{1 + \gamma_5}{2} \right) \quad (741)$$


---

(742)

$$i \frac{1}{\sqrt{2}} g_3 \delta_{ik} \lambda_{\text{At}1, \text{At}3}^{\text{aAt}2} \left( \frac{1 - \gamma_5}{2} \right) \quad (743)$$


---

(743)

$$+ -i \frac{1}{\sqrt{2}} g_3 \delta_{ik} \lambda_{\text{At}1, \text{At}3}^{\text{aAt}2} \left( \frac{1 + \gamma_5}{2} \right) \quad (744)$$


---

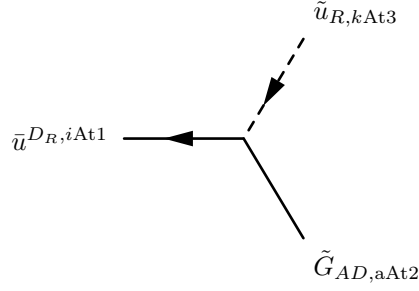

$$i \frac{1}{\sqrt{2}} g_3 \delta_{ik} \lambda_{\text{At}1, \text{At}3}^{\text{aAt}2} \left( \frac{1 - \gamma_5}{2} \right) \quad (745)$$


---

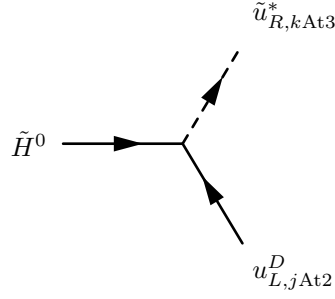

$$- i \delta_{\text{At}2 \text{At}3} Y_{u, kj} \left( \frac{1 - \gamma_5}{2} \right) \quad (746)$$


---

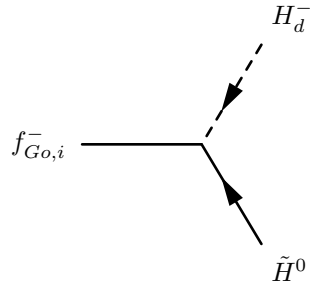

$$(747)$$

$$+ \frac{1}{\sqrt{2}} g_{A2} \frac{1}{\sqrt{g_{A2}^2 + g_{B2}^2}} \left( -i g_{B2} Z_{Go, i5} + i \sqrt{\frac{g_{A2}^2}{g_{A2}^2 + g_{B2}^2}} \sqrt{g_{A2}^2 + g_{B2}^2} Z_{Go, i6} - g_{B2} Z_{Go, i7} \right. \\ \left. + \sqrt{\frac{g_{A2}^2}{g_{A2}^2 + g_{B2}^2}} \sqrt{g_{A2}^2 + g_{B2}^2} Z_{Go, i8} \right) \left( \frac{1 + \gamma_5}{2} \right) \quad (748)$$


---

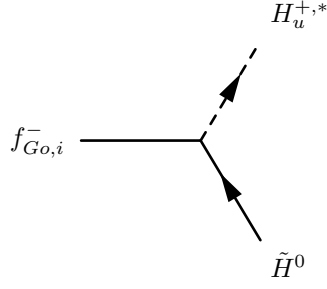

$$\begin{aligned} & \frac{1}{\sqrt{2}} g_{A2} \frac{1}{\sqrt{g_{A2}^2 + g_{B2}^2}} \left( -ig_{B2} Z_{Go,i5}^* + i \sqrt{\frac{g_{A2}^2}{g_{A2}^2 + g_{B2}^2}} \sqrt{g_{A2}^2 + g_{B2}^2} Z_{Go,i6}^* - g_{B2} Z_{Go,i7}^* \right. \\ & \left. + \sqrt{\frac{g_{A2}^2}{g_{A2}^2 + g_{B2}^2}} \sqrt{g_{A2}^2 + g_{B2}^2} Z_{Go,i8}^* \right) \left( \frac{1 - \gamma_5}{2} \right) \end{aligned} \quad (749)$$


---

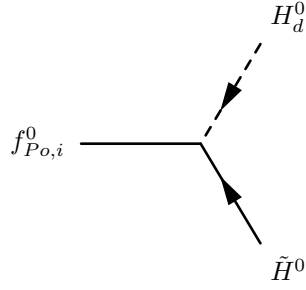

(750)

$$\begin{aligned} & + i \frac{1}{\sqrt{2}} \left( g_{A1} g_{B1} \frac{1}{\sqrt{g_{A1}^2 + g_{B1}^2}} Z_{Po,i5} - g_{A1} \sqrt{\frac{g_{A1}^2}{g_{A1}^2 + g_{B1}^2}} Z_{Po,i6} - g_{A2} g_{B2} \frac{1}{\sqrt{g_{A2}^2 + g_{B2}^2}} Z_{Po,i7} \right. \\ & \left. + g_{A2} \sqrt{\frac{g_{A2}^2}{g_{A2}^2 + g_{B2}^2}} Z_{Po,i8} \right) \left( \frac{1 + \gamma_5}{2} \right) \end{aligned} \quad (751)$$


---

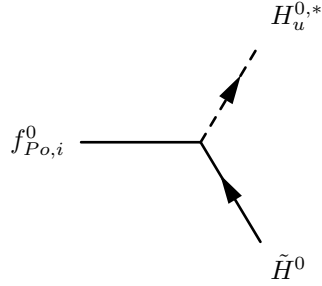



$$\begin{aligned}
& -i\frac{1}{\sqrt{2}}\left(g_{A1}g_{B1}\frac{1}{\sqrt{g_{A1}^2+g_{B1}^2}}Z_{Po,i5}^*-g_{A1}\sqrt{\frac{g_{A1}^2}{g_{A1}^2+g_{B1}^2}}Z_{Po,i6}^*-g_{A2}g_{B2}\frac{1}{\sqrt{g_{A2}^2+g_{B2}^2}}Z_{Po,i7}^*\right. \\
& \left.+g_{A2}\sqrt{\frac{g_{A2}^2}{g_{A2}^2+g_{B2}^2}}Z_{Po,i8}^*\right)\left(\frac{1-\gamma_5}{2}\right)
\end{aligned} \tag{752}$$


---

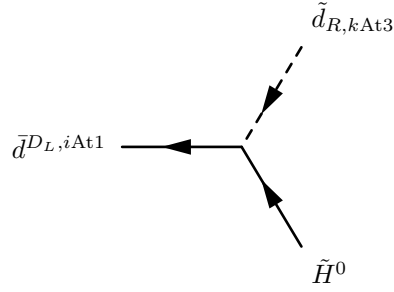

(753)

$$+ -iY_{d,ki}^*\delta_{At1At3}\left(\frac{1+\gamma_5}{2}\right) \tag{754}$$


---

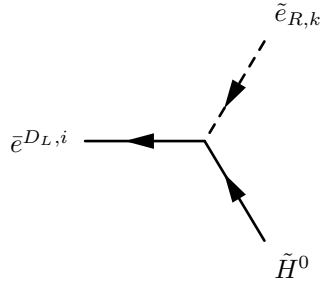

(755)

$$+ -iY_{e,ki}^*\left(\frac{1+\gamma_5}{2}\right) \tag{756}$$


---

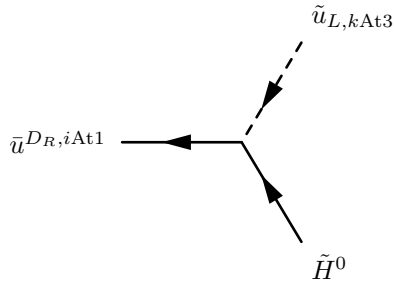

$$-i\delta_{\text{At1At3}}Y_{u,ik}\left(\frac{1-\gamma_5}{2}\right) \quad (757)$$


---

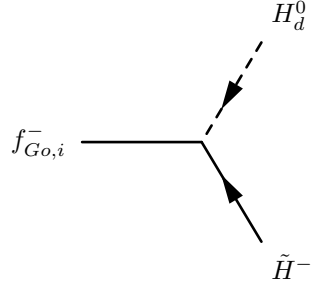

$$(758)$$

$$\begin{aligned} & + \frac{1}{\sqrt{2}}g_{A2}\frac{1}{\sqrt{g_{A2}^2+g_{B2}^2}}\left(-ig_{B2}Z_{Go,i5}+i\sqrt{\frac{g_{A2}^2}{g_{A2}^2+g_{B2}^2}}\sqrt{g_{A2}^2+g_{B2}^2}Z_{Go,i6}+g_{B2}Z_{Go,i7}\right. \\ & \left.-\sqrt{\frac{g_{A2}^2}{g_{A2}^2+g_{B2}^2}}\sqrt{g_{A2}^2+g_{B2}^2}Z_{Go,i8}\right)\left(\frac{1+\gamma_5}{2}\right) \end{aligned} \quad (759)$$


---

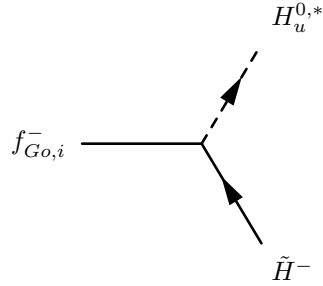

$$\begin{aligned} & \frac{1}{\sqrt{2}}g_{A2}\frac{1}{\sqrt{g_{A2}^2+g_{B2}^2}}\left(-ig_{B2}Z_{Go,i5}^*+i\sqrt{\frac{g_{A2}^2}{g_{A2}^2+g_{B2}^2}}\sqrt{g_{A2}^2+g_{B2}^2}Z_{Go,i6}^*+g_{B2}Z_{Go,i7}^*\right. \\ & \left.-\sqrt{\frac{g_{A2}^2}{g_{A2}^2+g_{B2}^2}}\sqrt{g_{A2}^2+g_{B2}^2}Z_{Go,i8}^*\right)\left(\frac{1-\gamma_5}{2}\right) \end{aligned} \quad (760)$$


---

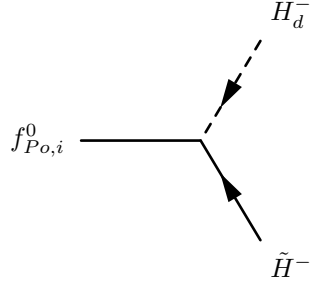

(761)

$$\begin{aligned}
& + i \frac{1}{\sqrt{2}} \left( g_{A1} g_{B1} \frac{1}{\sqrt{g_{A1}^2 + g_{B1}^2}} Z_{Po,i5} - g_{A1} \sqrt{\frac{g_{A1}^2}{g_{A1}^2 + g_{B1}^2}} Z_{Po,i6} + g_{A2} g_{B2} \frac{1}{\sqrt{g_{A2}^2 + g_{B2}^2}} Z_{Po,i7} \right. \\
& \left. - g_{A2} \sqrt{\frac{g_{A2}^2}{g_{A2}^2 + g_{B2}^2}} Z_{Po,i8} \right) \left( \frac{1 + \gamma_5}{2} \right)
\end{aligned} \tag{762}$$


---

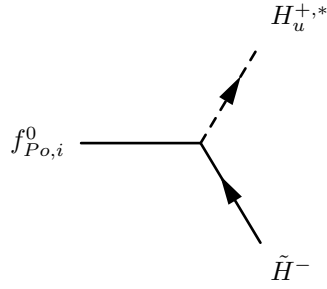

(763)

$$\begin{aligned}
& - i \frac{1}{\sqrt{2}} \left( g_{A1} g_{B1} \frac{1}{\sqrt{g_{A1}^2 + g_{B1}^2}} Z_{Po,i5}^* - g_{A1} \sqrt{\frac{g_{A1}^2}{g_{A1}^2 + g_{B1}^2}} Z_{Po,i6}^* + g_{A2} g_{B2} \frac{1}{\sqrt{g_{A2}^2 + g_{B2}^2}} Z_{Po,i7}^* \right. \\
& \left. - g_{A2} \sqrt{\frac{g_{A2}^2}{g_{A2}^2 + g_{B2}^2}} Z_{Po,i8}^* \right) \left( \frac{1 - \gamma_5}{2} \right)
\end{aligned} \tag{763}$$


---

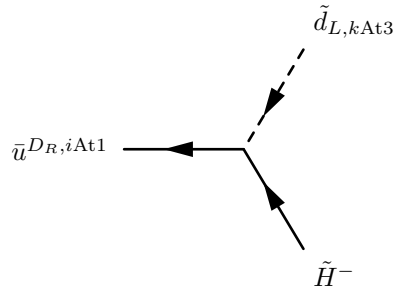

$$i\delta_{\text{At1At3}}Y_{u,ik}\left(\frac{1-\gamma_5}{2}\right) \quad (764)$$


---

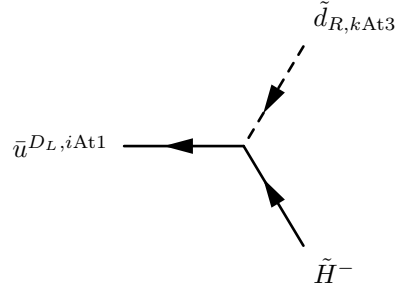

(765)

$$+ iY_{d,ki}^*\delta_{\text{At1At3}}\left(\frac{1+\gamma_5}{2}\right) \quad (766)$$


---

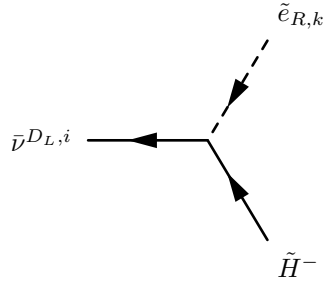

(767)

$$+ iY_{e,ki}^*\left(\frac{1+\gamma_5}{2}\right) \quad (768)$$


---

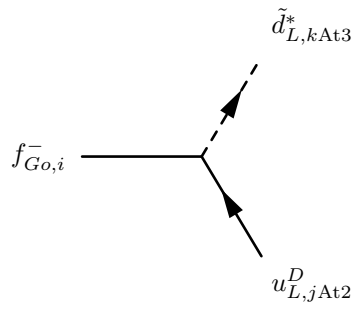

$$\begin{aligned}
& \frac{1}{\sqrt{2}} g_{A2} \frac{1}{\sqrt{g_{A2}^2 + g_{B2}^2}} \left( -i g_{B2} Z_{Go,i5}^* + i \sqrt{\frac{g_{A2}^2}{g_{A2}^2 + g_{B2}^2}} \sqrt{g_{A2}^2 + g_{B2}^2} Z_{Go,i6}^* + g_{B2} Z_{Go,i7}^* \right. \\
& \left. - \sqrt{\frac{g_{A2}^2}{g_{A2}^2 + g_{B2}^2}} \sqrt{g_{A2}^2 + g_{B2}^2} Z_{Go,i8}^* \right) \delta_{At2At3} \delta_{jk} \left( \frac{1 - \gamma_5}{2} \right)
\end{aligned} \tag{769}$$


---

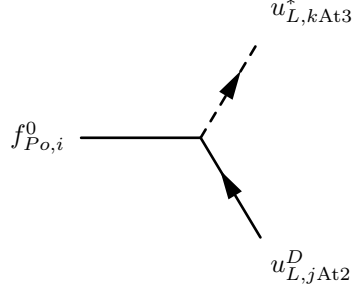

$$\begin{aligned}
& - \frac{i}{3} \frac{1}{\sqrt{2}} \left( g_{A1} g_{B1} \frac{1}{\sqrt{g_{A1}^2 + g_{B1}^2}} Z_{Po,i5}^* - g_{A1} \sqrt{\frac{g_{A1}^2}{g_{A1}^2 + g_{B1}^2}} Z_{Po,i6}^* + 3 g_{A2} g_{B2} \frac{1}{\sqrt{g_{A2}^2 + g_{B2}^2}} Z_{Po,i7}^* \right. \\
& \left. - 3 g_{A2} \sqrt{\frac{g_{A2}^2}{g_{A2}^2 + g_{B2}^2}} Z_{Po,i8}^* \right) \delta_{At2At3} \delta_{jk} \left( \frac{1 - \gamma_5}{2} \right)
\end{aligned} \tag{770}$$


---

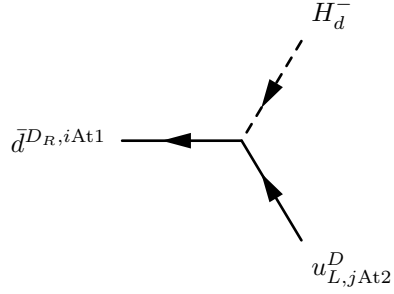

$$i \delta_{At1At2} Y_{d,ij} \left( \frac{1 - \gamma_5}{2} \right) \tag{771}$$


---

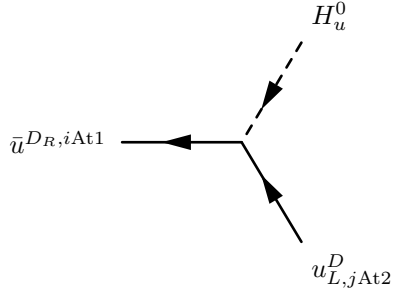

$$-i\delta_{\text{At1At2}}Y_{u,ij}\left(\frac{1-\gamma_5}{2}\right) \quad (772)$$


---

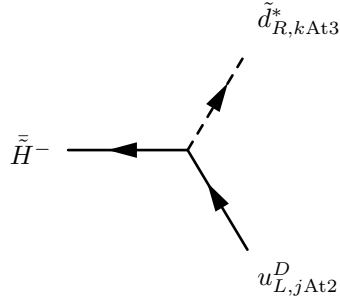

$$i\delta_{\text{At2At3}}Y_{d,kj}\left(\frac{1-\gamma_5}{2}\right) \quad (773)$$


---

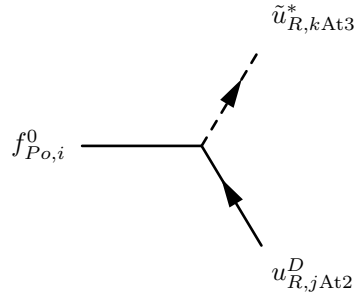

$$(774)$$

$$+ \frac{2i}{3}\sqrt{2}g_{A1}\frac{1}{\sqrt{g_{A1}^2+g_{B1}^2}}\delta_{\text{At2At3}}\delta_{jk}\left(g_{B1}Z_{Po,i5}-\sqrt{\frac{g_{A1}^2}{g_{A1}^2+g_{B1}^2}}\sqrt{g_{A1}^2+g_{B1}^2}Z_{Po,i6}\right)\left(\frac{1+\gamma_5}{2}\right) \quad (775)$$


---

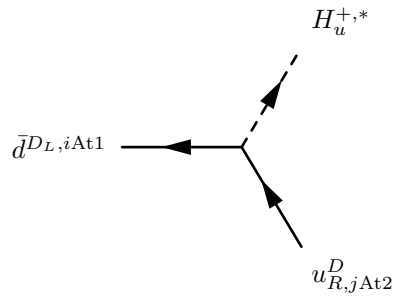

(776)

$$+ iY_{u,ji}^* \delta_{\text{At1At2}} \left( \frac{1 + \gamma_5}{2} \right) \quad (777)$$

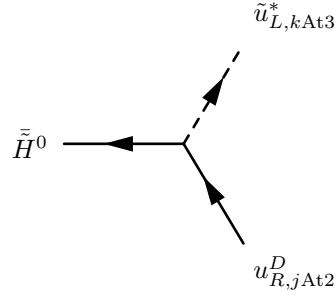

(778)

$$+ -iY_{u,jk}^* \delta_{\text{At2At3}} \left( \frac{1 + \gamma_5}{2} \right) \quad (779)$$

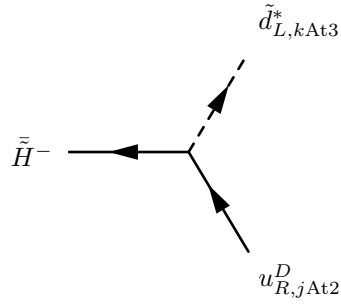

(780)

$$+ iY_{u,jk}^* \delta_{\text{At2At3}} \left( \frac{1 + \gamma_5}{2} \right) \quad (781)$$

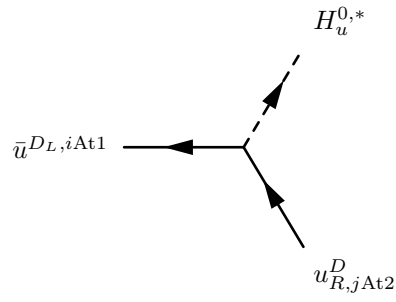

(782)

$$+ -iY_{u,ji}^* \delta_{At1At2} \left( \frac{1+\gamma_5}{2} \right) \quad (783)$$

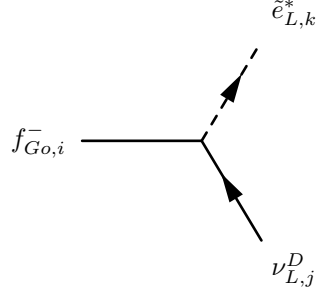

$$\begin{aligned} & \frac{1}{\sqrt{2}} g_{A2} \frac{1}{\sqrt{g_{A2}^2 + g_{B2}^2}} \left( -ig_{B2} Z_{Go,i5}^* + i \sqrt{\frac{g_{A2}^2}{g_{A2}^2 + g_{B2}^2}} \sqrt{g_{A2}^2 + g_{B2}^2} Z_{Go,i6}^* + g_{B2} Z_{Go,i7}^* \right. \\ & \left. - \sqrt{\frac{g_{A2}^2}{g_{A2}^2 + g_{B2}^2}} \sqrt{g_{A2}^2 + g_{B2}^2} Z_{Go,i8}^* \right) \delta_{jk} \left( \frac{1-\gamma_5}{2} \right) \end{aligned} \quad (784)$$

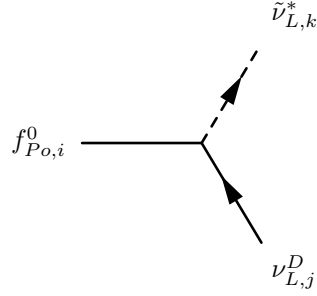

$$\begin{aligned} & i \frac{1}{\sqrt{2}} \left( g_{A1} g_{B1} \frac{1}{\sqrt{g_{A1}^2 + g_{B1}^2}} Z_{Po,i5}^* - g_{A1} \sqrt{\frac{g_{A1}^2}{g_{A1}^2 + g_{B1}^2}} Z_{Po,i6}^* - g_{A2} g_{B2} \frac{1}{\sqrt{g_{A2}^2 + g_{B2}^2}} Z_{Po,i7}^* \right. \\ & \left. + g_{A2} \sqrt{\frac{g_{A2}^2}{g_{A2}^2 + g_{B2}^2}} Z_{Po,i8}^* \right) \delta_{jk} \left( \frac{1-\gamma_5}{2} \right) \end{aligned} \quad (785)$$



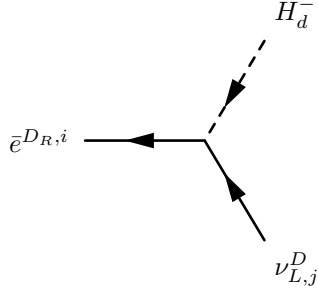

$$iY_{e,ij}\left(\frac{1-\gamma_5}{2}\right) \quad (786)$$


---

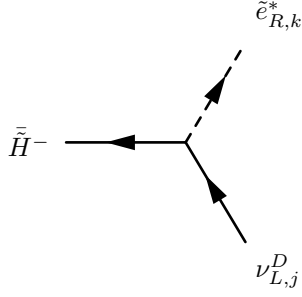

$$iY_{e,kj}\left(\frac{1-\gamma_5}{2}\right) \quad (787)$$


---

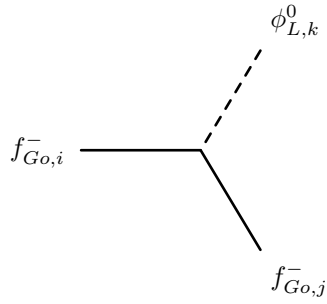

$$\begin{aligned} & \frac{1}{2} \frac{1}{\sqrt{gA^2 + gB^2}} \left( -\sqrt{2}g_{B2} \sqrt{\frac{gA^2}{gA^2 + gB^2}} \sqrt{gA^2 + gB^2} Z_{Go,i7}^* Z_{Go,j1}^* Z_{Ls,k1}^{DR,*} - \sqrt{2}g_{B2}^2 Z_{Go,i8}^* Z_{Go,j1}^* Z_{Ls,k1}^{DR,*} \right. \\ & \left. - 2i \sqrt{gA^2 + gB^2} Y_A Z_{Go,i9}^* Z_{Go,j2}^* Z_{Ls,k1}^{DR,*} - \sqrt{2}g_{A2}g_{B2} Z_{Go,i7}^* Z_{Go,j3}^* Z_{Ls,k1}^{DR,*} \right) \end{aligned}$$

$$\begin{aligned}
& + \sqrt{2}g_{A2}\sqrt{\frac{gA2^2}{gA2^2 + gB2^2}}\sqrt{gA2^2 + gB2^2}Z_{Go,i8}^*Z_{Go,j3}^*Z_{Ls,k1}^{DR,*} \\
& + i\sqrt{2}g_{B2}\sqrt{\frac{gA2^2}{gA2^2 + gB2^2}}\sqrt{gA2^2 + gB2^2}Z_{Go,i1}^*Z_{Go,j5}^*Z_{Ls,k1}^{DR,*} - i\sqrt{2}g_{A2}g_{B2}Z_{Go,i3}^*Z_{Go,j5}^*Z_{Ls,k1}^{DR,*} \\
& + i\sqrt{2}g_{B2}^2Z_{Go,i1}^*Z_{Go,j6}^*Z_{Ls,k1}^{DR,*} + i\sqrt{2}g_{A2}\sqrt{\frac{gA2^2}{gA2^2 + gB2^2}}\sqrt{gA2^2 + gB2^2}Z_{Go,i3}^*Z_{Go,j6}^*Z_{Ls,k1}^{DR,*} \\
& - \sqrt{2}g_{B2}\sqrt{\frac{gA2^2}{gA2^2 + gB2^2}}\sqrt{gA2^2 + gB2^2}Z_{Go,i1}^*Z_{Go,j7}^*Z_{Ls,k1}^{DR,*} - \sqrt{2}g_{A2}g_{B2}Z_{Go,i3}^*Z_{Go,j7}^*Z_{Ls,k1}^{DR,*} \\
& - \sqrt{2}g_{B2}^2Z_{Go,i1}^*Z_{Go,j8}^*Z_{Ls,k1}^{DR,*} + \sqrt{2}g_{A2}\sqrt{\frac{gA2^2}{gA2^2 + gB2^2}}\sqrt{gA2^2 + gB2^2}Z_{Go,i3}^*Z_{Go,j8}^*Z_{Ls,k1}^{DR,*} \\
& - 2i\sqrt{gA2^2 + gB2^2}Y_AZ_{Go,i2}^*Z_{Go,j9}^*Z_{Ls,k1}^{DR,*} - 2i\sqrt{gA2^2 + gB2^2}Y_AZ_{Go,i10}^*Z_{Go,j1}^*Z_{Ls,k2}^{DR,*} \\
& - \sqrt{2}g_{B2}\sqrt{\frac{gA2^2}{gA2^2 + gB2^2}}\sqrt{gA2^2 + gB2^2}Z_{Go,i7}^*Z_{Go,j2}^*Z_{Ls,k2}^{DR,*} - \sqrt{2}g_{B2}^2Z_{Go,i8}^*Z_{Go,j2}^*Z_{Ls,k2}^{DR,*} \\
& - \sqrt{2}g_{A2}g_{B2}Z_{Go,i7}^*Z_{Go,j4}^*Z_{Ls,k2}^{DR,*} + \sqrt{2}g_{A2}\sqrt{\frac{gA2^2}{gA2^2 + gB2^2}}\sqrt{gA2^2 + gB2^2}Z_{Go,i8}^*Z_{Go,j4}^*Z_{Ls,k2}^{DR,*} \\
& - i\sqrt{2}g_{B2}\sqrt{\frac{gA2^2}{gA2^2 + gB2^2}}\sqrt{gA2^2 + gB2^2}Z_{Go,i2}^*Z_{Go,j5}^*Z_{Ls,k2}^{DR,*} + i\sqrt{2}g_{A2}g_{B2}Z_{Go,i4}^*Z_{Go,j5}^*Z_{Ls,k2}^{DR,*} \\
& - i\sqrt{2}g_{B2}^2Z_{Go,i2}^*Z_{Go,j6}^*Z_{Ls,k2}^{DR,*} - i\sqrt{2}g_{A2}\sqrt{\frac{gA2^2}{gA2^2 + gB2^2}}\sqrt{gA2^2 + gB2^2}Z_{Go,i4}^*Z_{Go,j6}^*Z_{Ls,k2}^{DR,*} \\
& - \sqrt{2}g_{B2}\sqrt{\frac{gA2^2}{gA2^2 + gB2^2}}\sqrt{gA2^2 + gB2^2}Z_{Go,i2}^*Z_{Go,j7}^*Z_{Ls,k2}^{DR,*} - \sqrt{2}g_{A2}g_{B2}Z_{Go,i4}^*Z_{Go,j7}^*Z_{Ls,k2}^{DR,*} \\
& - \sqrt{2}g_{B2}^2Z_{Go,i2}^*Z_{Go,j8}^*Z_{Ls,k2}^{DR,*} + \sqrt{2}g_{A2}\sqrt{\frac{gA2^2}{gA2^2 + gB2^2}}\sqrt{gA2^2 + gB2^2}Z_{Go,i4}^*Z_{Go,j8}^*Z_{Ls,k2}^{DR,*} \\
& - 2i\sqrt{gA2^2 + gB2^2}Y_AZ_{Go,i1}^*Z_{Go,j10}^*Z_{Ls,k2}^{DR,*} + \sqrt{2}g_{A2}g_{B2}Z_{Go,i7}^*Z_{Go,j1}^*Z_{Ls,k3}^{DR,*} \\
& - \sqrt{2}g_{A2}\sqrt{\frac{gA2^2}{gA2^2 + gB2^2}}\sqrt{gA2^2 + gB2^2}Z_{Go,i8}^*Z_{Go,j1}^*Z_{Ls,k3}^{DR,*} \\
& + \sqrt{2}g_{B2}\sqrt{\frac{gA2^2}{gA2^2 + gB2^2}}\sqrt{gA2^2 + gB2^2}Z_{Go,i7}^*Z_{Go,j3}^*Z_{Ls,k3}^{DR,*} + \sqrt{2}g_{B2}^2Z_{Go,i8}^*Z_{Go,j3}^*Z_{Ls,k3}^{DR,*} \\
& - 2i\sqrt{gA2^2 + gB2^2}Y_AZ_{Go,i10}^*Z_{Go,j4}^*Z_{Ls,k3}^{DR,*} - i\sqrt{2}g_{A2}g_{B2}Z_{Go,i1}^*Z_{Go,j5}^*Z_{Ls,k3}^{DR,*} \\
& + i\sqrt{2}g_{B2}\sqrt{\frac{gA2^2}{gA2^2 + gB2^2}}\sqrt{gA2^2 + gB2^2}Z_{Go,i3}^*Z_{Go,j5}^*Z_{Ls,k3}^{DR,*}
\end{aligned}$$

$$\begin{aligned}
& + i\sqrt{2}g_{A2}\sqrt{\frac{gA^2}{gA^2 + gB^2}}\sqrt{gA^2 + gB^2}Z_{Go,i1}^*Z_{Go,j6}^*Z_{Ls,k3}^{DR,*} + i\sqrt{2}g_{B2}^2Z_{Go,i3}^*Z_{Go,j6}^*Z_{Ls,k3}^{DR,*} \\
& + \sqrt{2}g_{A2}g_{B2}Z_{Go,i1}^*Z_{Go,j7}^*Z_{Ls,k3}^{DR,*} + \sqrt{2}g_{B2}\sqrt{\frac{gA^2}{gA^2 + gB^2}}\sqrt{gA^2 + gB^2}Z_{Go,i3}^*Z_{Go,j7}^*Z_{Ls,k3}^{DR,*} \\
& - \sqrt{2}g_{A2}\sqrt{\frac{gA^2}{gA^2 + gB^2}}\sqrt{gA^2 + gB^2}Z_{Go,i1}^*Z_{Go,j8}^*Z_{Ls,k3}^{DR,*} + \sqrt{2}g_{B2}^2Z_{Go,i3}^*Z_{Go,j8}^*Z_{Ls,k3}^{DR,*} \\
& - 2i\sqrt{gA^2 + gB^2}Y_AZ_{Go,i4}^*Z_{Go,j10}^*Z_{Ls,k3}^{DR,*} + \sqrt{2}g_{A2}g_{B2}Z_{Go,i7}^*Z_{Go,j2}^*Z_{Ls,k4}^{DR,*} \\
& - \sqrt{2}g_{A2}\sqrt{\frac{gA^2}{gA^2 + gB^2}}\sqrt{gA^2 + gB^2}Z_{Go,i8}^*Z_{Go,j2}^*Z_{Ls,k4}^{DR,*} \\
& - 2i\sqrt{gA^2 + gB^2}Y_AZ_{Go,i9}^*Z_{Go,j3}^*Z_{Ls,k4}^{DR,*} \\
& + \sqrt{2}g_{B2}\sqrt{\frac{gA^2}{gA^2 + gB^2}}\sqrt{gA^2 + gB^2}Z_{Go,i7}^*Z_{Go,j4}^*Z_{Ls,k4}^{DR,*} + \sqrt{2}g_{B2}^2Z_{Go,i8}^*Z_{Go,j4}^*Z_{Ls,k4}^{DR,*} \\
& + i\sqrt{2}g_{A2}g_{B2}Z_{Go,i2}^*Z_{Go,j5}^*Z_{Ls,k4}^{DR,*} - i\sqrt{2}g_{B2}\sqrt{\frac{gA^2}{gA^2 + gB^2}}\sqrt{gA^2 + gB^2}Z_{Go,i4}^*Z_{Go,j5}^*Z_{Ls,k4}^{DR,*} \\
& - i\sqrt{2}g_{A2}\sqrt{\frac{gA^2}{gA^2 + gB^2}}\sqrt{gA^2 + gB^2}Z_{Go,i2}^*Z_{Go,j6}^*Z_{Ls,k4}^{DR,*} - i\sqrt{2}g_{B2}^2Z_{Go,i4}^*Z_{Go,j6}^*Z_{Ls,k4}^{DR,*} \\
& + \sqrt{2}g_{A2}g_{B2}Z_{Go,i2}^*Z_{Go,j7}^*Z_{Ls,k4}^{DR,*} + \sqrt{2}g_{B2}\sqrt{\frac{gA^2}{gA^2 + gB^2}}\sqrt{gA^2 + gB^2}Z_{Go,i4}^*Z_{Go,j7}^*Z_{Ls,k4}^{DR,*} \\
& - \sqrt{2}g_{A2}\sqrt{\frac{gA^2}{gA^2 + gB^2}}\sqrt{gA^2 + gB^2}Z_{Go,i2}^*Z_{Go,j8}^*Z_{Ls,k4}^{DR,*} + \sqrt{2}g_{B2}^2Z_{Go,i4}^*Z_{Go,j8}^*Z_{Ls,k4}^{DR,*} \\
& - 2i\sqrt{gA^2 + gB^2}Y_AZ_{Go,i3}^*Z_{Go,j9}^*Z_{Ls,k4}^{DR,*} \\
& + i\sqrt{2}Z_{Go,i6}^*\left(-g_{B2}^2Z_{Go,j2}^*Z_{Ls,k2}^{DR,*} - g_{A2}\sqrt{\frac{gA^2}{gA^2 + gB^2}}\sqrt{gA^2 + gB^2}Z_{Go,j4}^*Z_{Ls,k2}^{DR,*}\right. \\
& + Z_{Go,j3}^*\left(g_{A2}\sqrt{\frac{gA^2}{gA^2 + gB^2}}\sqrt{gA^2 + gB^2}Z_{Ls,k1}^{DR,*} + g_{B2}^2Z_{Ls,k3}^{DR,*}\right) \\
& + Z_{Go,j1}^*\left(g_{A2}\sqrt{\frac{gA^2}{gA^2 + gB^2}}\sqrt{gA^2 + gB^2}Z_{Ls,k3}^{DR,*} + g_{B2}^2Z_{Ls,k1}^{DR,*}\right) \\
& - g_{A2}\sqrt{\frac{gA^2}{gA^2 + gB^2}}\sqrt{gA^2 + gB^2}Z_{Go,j2}^*Z_{Ls,k4}^{DR,*} - g_{B2}^2Z_{Go,j4}^*Z_{Ls,k4}^{DR,*}) \\
& + i\sqrt{2}g_{B2}Z_{Go,i5}^*\left(-\sqrt{\frac{gA^2}{gA^2 + gB^2}}\sqrt{gA^2 + gB^2}Z_{Go,j2}^*Z_{Ls,k2}^{DR,*} + g_{A2}Z_{Go,j4}^*Z_{Ls,k2}^{DR,*}\right.
\end{aligned}$$

$$\begin{aligned}
& + Z_{Go,j1}^* \left( -g_{A2} Z_{Ls,k3}^{DR,*} + \sqrt{\frac{gA2^2}{gA2^2 + gB2^2}} \sqrt{gA2^2 + gB2^2} Z_{Ls,k1}^{DR,*} \right) \\
& + Z_{Go,j3}^* \left( -g_{A2} Z_{Ls,k1}^{DR,*} + \sqrt{\frac{gA2^2}{gA2^2 + gB2^2}} \sqrt{gA2^2 + gB2^2} Z_{Ls,k3}^{DR,*} \right) + g_{A2} Z_{Go,j2}^* Z_{Ls,k4}^{DR,*} \\
& - \sqrt{\frac{gA2^2}{gA2^2 + gB2^2}} \sqrt{gA2^2 + gB2^2} Z_{Go,j4}^* Z_{Ls,k4}^{DR,*} \left( \frac{1 - \gamma_5}{2} \right) \\
& + \frac{1}{2} \frac{1}{\sqrt{gA2^2 + gB2^2}} \left( -2i \sqrt{gA2^2 + gB2^2} Y_A^* Z_{Ls,k2}^{DR,*} Z_{Go,i10} Z_{Go,j1} \right. \\
& - i\sqrt{2} g_{B2} \sqrt{\frac{gA2^2}{gA2^2 + gB2^2}} \sqrt{gA2^2 + gB2^2} Z_{Ls,k2}^{DR,*} Z_{Go,i5} Z_{Go,j2} + i\sqrt{2} g_{A2} g_{B2} Z_{Ls,k4}^{DR,*} Z_{Go,i5} Z_{Go,j2} \\
& - i\sqrt{2} g_{B2}^2 Z_{Ls,k2}^{DR,*} Z_{Go,i6} Z_{Go,j2} - i\sqrt{2} g_{A2} \sqrt{\frac{gA2^2}{gA2^2 + gB2^2}} \sqrt{gA2^2 + gB2^2} Z_{Ls,k4}^{DR,*} Z_{Go,i6} Z_{Go,j2} \\
& + \sqrt{2} g_{B2} \sqrt{\frac{gA2^2}{gA2^2 + gB2^2}} \sqrt{gA2^2 + gB2^2} Z_{Ls,k2}^{DR,*} Z_{Go,i7} Z_{Go,j2} - \sqrt{2} g_{A2} g_{B2} Z_{Ls,k4}^{DR,*} Z_{Go,i7} Z_{Go,j2} \\
& + \sqrt{2} g_{B2}^2 Z_{Ls,k2}^{DR,*} Z_{Go,i8} Z_{Go,j2} + \sqrt{2} g_{A2} \sqrt{\frac{gA2^2}{gA2^2 + gB2^2}} \sqrt{gA2^2 + gB2^2} Z_{Ls,k4}^{DR,*} Z_{Go,i8} Z_{Go,j2} \\
& - 2i \sqrt{gA2^2 + gB2^2} Y_A^* Z_{Ls,k4}^{DR,*} Z_{Go,i9} Z_{Go,j3} + i\sqrt{2} g_{A2} g_{B2} Z_{Ls,k2}^{DR,*} Z_{Go,i5} Z_{Go,j4} \\
& - i\sqrt{2} g_{B2} \sqrt{\frac{gA2^2}{gA2^2 + gB2^2}} \sqrt{gA2^2 + gB2^2} Z_{Ls,k4}^{DR,*} Z_{Go,i5} Z_{Go,j4} \\
& - i\sqrt{2} g_{A2} \sqrt{\frac{gA2^2}{gA2^2 + gB2^2}} \sqrt{gA2^2 + gB2^2} Z_{Ls,k2}^{DR,*} Z_{Go,i6} Z_{Go,j4} - i\sqrt{2} g_{B2}^2 Z_{Ls,k4}^{DR,*} Z_{Go,i6} Z_{Go,j4} \\
& + \sqrt{2} g_{A2} g_{B2} Z_{Ls,k2}^{DR,*} Z_{Go,i7} Z_{Go,j4} - \sqrt{2} g_{B2} \sqrt{\frac{gA2^2}{gA2^2 + gB2^2}} \sqrt{gA2^2 + gB2^2} Z_{Ls,k4}^{DR,*} Z_{Go,i7} Z_{Go,j4} \\
& - \sqrt{2} g_{A2} \sqrt{\frac{gA2^2}{gA2^2 + gB2^2}} \sqrt{gA2^2 + gB2^2} Z_{Ls,k2}^{DR,*} Z_{Go,i8} Z_{Go,j4} - \sqrt{2} g_{B2}^2 Z_{Ls,k4}^{DR,*} Z_{Go,i8} Z_{Go,j4} \\
& - i\sqrt{2} g_{B2} \sqrt{\frac{gA2^2}{gA2^2 + gB2^2}} \sqrt{gA2^2 + gB2^2} Z_{Ls,k2}^{DR,*} Z_{Go,i2} Z_{Go,j5} + i\sqrt{2} g_{A2} g_{B2} Z_{Ls,k4}^{DR,*} Z_{Go,i2} Z_{Go,j5} \\
& + i\sqrt{2} g_{A2} g_{B2} Z_{Ls,k2}^{DR,*} Z_{Go,i4} Z_{Go,j5} - i\sqrt{2} g_{B2} \sqrt{\frac{gA2^2}{gA2^2 + gB2^2}} \sqrt{gA2^2 + gB2^2} Z_{Ls,k4}^{DR,*} Z_{Go,i4} Z_{Go,j5} \\
& - i\sqrt{2} g_{B2}^2 Z_{Ls,k2}^{DR,*} Z_{Go,i2} Z_{Go,j6} - i\sqrt{2} g_{A2} \sqrt{\frac{gA2^2}{gA2^2 + gB2^2}} \sqrt{gA2^2 + gB2^2} Z_{Ls,k4}^{DR,*} Z_{Go,i2} Z_{Go,j6}
\end{aligned} \tag{788}$$

$$\begin{aligned}
& -i\sqrt{2}g_{A2}\sqrt{\frac{gA^2}{gA^2+gB^2}}\sqrt{gA^2+gB^2}Z_{Ls,k2}^{DR,*}Z_{Go,i4}Z_{Go,j6}-i\sqrt{2}g_{B2}^2Z_{Ls,k4}^{DR,*}Z_{Go,i4}Z_{Go,j6} \\
& +\sqrt{2}g_{B2}\sqrt{\frac{gA^2}{gA^2+gB^2}}\sqrt{gA^2+gB^2}Z_{Ls,k2}^{DR,*}Z_{Go,i2}Z_{Go,j7}-\sqrt{2}g_{A2}g_{B2}Z_{Ls,k4}^{DR,*}Z_{Go,i2}Z_{Go,j7} \\
& +\sqrt{2}g_{A2}g_{B2}Z_{Ls,k2}^{DR,*}Z_{Go,i4}Z_{Go,j7}-\sqrt{2}g_{B2}\sqrt{\frac{gA^2}{gA^2+gB^2}}\sqrt{gA^2+gB^2}Z_{Ls,k4}^{DR,*}Z_{Go,i4}Z_{Go,j7} \\
& +\sqrt{2}g_{B2}^2Z_{Ls,k2}^{DR,*}Z_{Go,i2}Z_{Go,j8}+\sqrt{2}g_{A2}\sqrt{\frac{gA^2}{gA^2+gB^2}}\sqrt{gA^2+gB^2}Z_{Ls,k4}^{DR,*}Z_{Go,i2}Z_{Go,j8} \\
& -\sqrt{2}g_{A2}\sqrt{\frac{gA^2}{gA^2+gB^2}}\sqrt{gA^2+gB^2}Z_{Ls,k2}^{DR,*}Z_{Go,i4}Z_{Go,j8}-\sqrt{2}g_{B2}^2Z_{Ls,k4}^{DR,*}Z_{Go,i4}Z_{Go,j8} \\
& -2i\sqrt{gA^2+gB^2}Y_A^*Z_{Ls,k4}^{DR,*}Z_{Go,i3}Z_{Go,j9} \\
& +Z_{Ls,k1}^{DR,*}\left(\sqrt{2}g_{B2}\sqrt{\frac{gA^2}{gA^2+gB^2}}\sqrt{gA^2+gB^2}Z_{Go,i7}Z_{Go,j1}+\sqrt{2}g_{B2}^2Z_{Go,i8}Z_{Go,j1}\right. \\
& \left.-2i\sqrt{gA^2+gB^2}Y_A^*Z_{Go,i9}Z_{Go,j2}+\sqrt{2}g_{A2}g_{B2}Z_{Go,i7}Z_{Go,j3}\right. \\
& \left.-\sqrt{2}g_{A2}\sqrt{\frac{gA^2}{gA^2+gB^2}}\sqrt{gA^2+gB^2}Z_{Go,i8}Z_{Go,j3}\right. \\
& \left.+i\sqrt{2}g_{B2}Z_{Go,i5}\left(-g_{A2}Z_{Go,j3}+\sqrt{\frac{gA^2}{gA^2+gB^2}}\sqrt{gA^2+gB^2}Z_{Go,j1}\right)\right. \\
& \left.+i\sqrt{2}Z_{Go,i6}\left(g_{A2}\sqrt{\frac{gA^2}{gA^2+gB^2}}\sqrt{gA^2+gB^2}Z_{Go,j3}+g_{B2}^2Z_{Go,j1}\right)\right. \\
& \left.+i\sqrt{2}g_{B2}\sqrt{\frac{gA^2}{gA^2+gB^2}}\sqrt{gA^2+gB^2}Z_{Go,i1}Z_{Go,j5}-i\sqrt{2}g_{A2}g_{B2}Z_{Go,i3}Z_{Go,j5}\right. \\
& \left.+i\sqrt{2}g_{B2}^2Z_{Go,i1}Z_{Go,j6}+i\sqrt{2}g_{A2}\sqrt{\frac{gA^2}{gA^2+gB^2}}\sqrt{gA^2+gB^2}Z_{Go,i3}Z_{Go,j6}\right. \\
& \left.+\sqrt{2}g_{B2}\sqrt{\frac{gA^2}{gA^2+gB^2}}\sqrt{gA^2+gB^2}Z_{Go,i1}Z_{Go,j7}+\sqrt{2}g_{A2}g_{B2}Z_{Go,i3}Z_{Go,j7}+\sqrt{2}g_{B2}^2Z_{Go,i1}Z_{Go,j8}\right. \\
& \left.-\sqrt{2}g_{A2}\sqrt{\frac{gA^2}{gA^2+gB^2}}\sqrt{gA^2+gB^2}Z_{Go,i3}Z_{Go,j8}-2i\sqrt{gA^2+gB^2}Y_A^*Z_{Go,i2}Z_{Go,j9}\right) \\
& -2i\sqrt{gA^2+gB^2}Y_A^*Z_{Ls,k2}^{DR,*}Z_{Go,i1}Z_{Go,j10} \\
& +Z_{Ls,k3}^{DR,*}\left(-\sqrt{2}g_{A2}g_{B2}Z_{Go,i7}Z_{Go,j1}+\sqrt{2}g_{A2}\sqrt{\frac{gA^2}{gA^2+gB^2}}\sqrt{gA^2+gB^2}Z_{Go,i8}Z_{Go,j1}\right.
\end{aligned}$$

$$\begin{aligned}
& -\sqrt{2}g_{B2}\sqrt{\frac{gA2^2}{gA2^2+gB2^2}}\sqrt{gA2^2+gB2^2}Z_{Go,i7}Z_{Go,j3}-\sqrt{2}g_{B2}^2Z_{Go,i8}Z_{Go,j3} \\
& +i\sqrt{2}Z_{Go,i6}\left(g_{A2}\sqrt{\frac{gA2^2}{gA2^2+gB2^2}}\sqrt{gA2^2+gB2^2}Z_{Go,j1}+g_{B2}^2Z_{Go,j3}\right) \\
& -i\sqrt{2}g_{B2}Z_{Go,i5}\left(g_{A2}Z_{Go,j1}-\sqrt{\frac{gA2^2}{gA2^2+gB2^2}}\sqrt{gA2^2+gB2^2}Z_{Go,j3}\right) \\
& -2i\sqrt{gA2^2+gB2^2}Y_A^*Z_{Go,i10}Z_{Go,j4}-i\sqrt{2}g_{A2}g_{B2}Z_{Go,i1}Z_{Go,j5} \\
& +i\sqrt{2}g_{B2}\sqrt{\frac{gA2^2}{gA2^2+gB2^2}}\sqrt{gA2^2+gB2^2}Z_{Go,i3}Z_{Go,j5} \\
& +i\sqrt{2}g_{A2}\sqrt{\frac{gA2^2}{gA2^2+gB2^2}}\sqrt{gA2^2+gB2^2}Z_{Go,i1}Z_{Go,j6}+i\sqrt{2}g_{B2}^2Z_{Go,i3}Z_{Go,j6} \\
& -\sqrt{2}g_{A2}g_{B2}Z_{Go,i1}Z_{Go,j7}-\sqrt{2}g_{B2}\sqrt{\frac{gA2^2}{gA2^2+gB2^2}}\sqrt{gA2^2+gB2^2}Z_{Go,i3}Z_{Go,j7} \\
& +\sqrt{2}g_{A2}\sqrt{\frac{gA2^2}{gA2^2+gB2^2}}\sqrt{gA2^2+gB2^2}Z_{Go,i1}Z_{Go,j8}-\sqrt{2}g_{B2}^2Z_{Go,i3}Z_{Go,j8} \\
& -2i\sqrt{gA2^2+gB2^2}Y_A^*Z_{Go,i4}Z_{Go,j10}\Big)\Big)\left(\frac{1+\gamma_5}{2}\right)
\end{aligned} \tag{789}$$


---

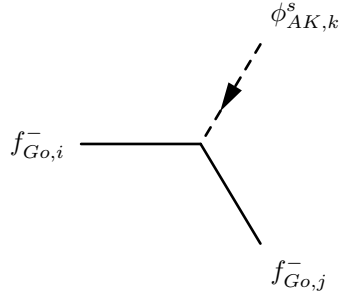

$$\begin{aligned}
& -\frac{i}{2}\left(\sqrt{2}Y_AZ_{AK,k2}^{s,*}\left(-Z_{Go,i1}^*Z_{Go,j2}^*-Z_{Go,i2}^*Z_{Go,j1}^*+Z_{Go,i3}^*Z_{Go,j4}^*+Z_{Go,i4}^*Z_{Go,j3}^*\right)\right. \\
& \left.+Y_KZ_{AK,k1}^{s,*}\left(Z_{Go,i1}^*Z_{Go,j2}^*+Z_{Go,i2}^*Z_{Go,j1}^*+Z_{Go,i3}^*Z_{Go,j4}^*+Z_{Go,i4}^*Z_{Go,j3}^*\right)\right)\left(\frac{1-\gamma_5}{2}\right) \\
& +g_{B2}\frac{1}{\sqrt{gA2^2+gB2^2}}Z_{AK,k2}^{s,*}\left(Z_{Go,i10}\left(-i\sqrt{\frac{gA2^2}{gA2^2+gB2^2}}\sqrt{gA2^2+gB2^2}Z_{Go,j5}-ig_{B2}Z_{Go,j6}+\sqrt{\frac{gA2^2}{gA2^2+gB2^2}}\sqrt{gA2^2+gB2^2}Z_{Go,j7}\right.\right. \\
& \left.\left.+g_{B2}Z_{Go,j8}\right)\right)
\end{aligned} \tag{790}$$

$$\begin{aligned}
& + Z_{Go,i9} \left( i \sqrt{\frac{gA^2}{gA^2 + gB^2}} \sqrt{gA^2 + gB^2} Z_{Go,j5} + i g_{B2} Z_{Go,j6} + \sqrt{\frac{gA^2}{gA^2 + gB^2}} \sqrt{gA^2 + gB^2} Z_{Go,j7} \right. \\
& \left. + g_{B2} Z_{Go,j8} \right) \\
& + i \sqrt{\frac{gA^2}{gA^2 + gB^2}} \sqrt{gA^2 + gB^2} Z_{Go,i5} Z_{Go,j9} + i g_{B2} Z_{Go,i6} Z_{Go,j9} \\
& + \sqrt{\frac{gA^2}{gA^2 + gB^2}} \sqrt{gA^2 + gB^2} Z_{Go,i7} Z_{Go,j9} + g_{B2} Z_{Go,i8} Z_{Go,j9} \\
& - i \sqrt{\frac{gA^2}{gA^2 + gB^2}} \sqrt{gA^2 + gB^2} Z_{Go,i5} Z_{Go,j10} - i g_{B2} Z_{Go,i6} Z_{Go,j10} \\
& + \sqrt{\frac{gA^2}{gA^2 + gB^2}} \sqrt{gA^2 + gB^2} Z_{Go,i7} Z_{Go,j10} + g_{B2} Z_{Go,i8} Z_{Go,j10} \Big) \left( \frac{1 + \gamma_5}{2} \right)
\end{aligned} \tag{791}$$


---

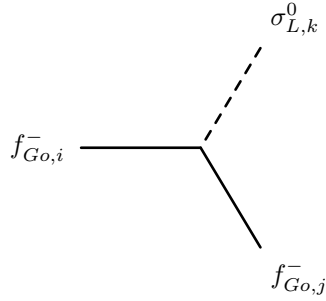

$$\begin{aligned}
& \frac{1}{2} \frac{1}{\sqrt{gA^2 + gB^2}} \left( i \sqrt{2} g_{B2} \sqrt{\frac{gA^2}{gA^2 + gB^2}} \sqrt{gA^2 + gB^2} Z_{Go,i7}^* Z_{Go,j1}^* Z_{Ls,k1}^{Di,*} + i \sqrt{2} g_{B2}^2 Z_{Go,i8}^* Z_{Go,j1}^* Z_{Ls,k1}^{Di,*} \right. \\
& + 2 \sqrt{gA^2 + gB^2} Y_A Z_{Go,i9}^* Z_{Go,j2}^* Z_{Ls,k1}^{Di,*} + i \sqrt{2} g_{A2} g_{B2} Z_{Go,i7}^* Z_{Go,j3}^* Z_{Ls,k1}^{Di,*} \\
& - i \sqrt{2} g_{A2} \sqrt{\frac{gA^2}{gA^2 + gB^2}} \sqrt{gA^2 + gB^2} Z_{Go,i8}^* Z_{Go,j3}^* Z_{Ls,k1}^{Di,*} \\
& + \sqrt{2} g_{B2} \sqrt{\frac{gA^2}{gA^2 + gB^2}} \sqrt{gA^2 + gB^2} Z_{Go,i1}^* Z_{Go,j5}^* Z_{Ls,k1}^{Di,*} - \sqrt{2} g_{A2} g_{B2} Z_{Go,i3}^* Z_{Go,j5}^* Z_{Ls,k1}^{Di,*} \\
& + \sqrt{2} g_{B2}^2 Z_{Go,i1}^* Z_{Go,j6}^* Z_{Ls,k1}^{Di,*} + \sqrt{2} g_{A2} \sqrt{\frac{gA^2}{gA^2 + gB^2}} \sqrt{gA^2 + gB^2} Z_{Go,i3}^* Z_{Go,j6}^* Z_{Ls,k1}^{Di,*} \\
& + i \sqrt{2} g_{B2} \sqrt{\frac{gA^2}{gA^2 + gB^2}} \sqrt{gA^2 + gB^2} Z_{Go,i1}^* Z_{Go,j7}^* Z_{Ls,k1}^{Di,*} + i \sqrt{2} g_{A2} g_{B2} Z_{Go,i3}^* Z_{Go,j7}^* Z_{Ls,k1}^{Di,*} \\
& \left. + i \sqrt{2} g_{B2}^2 Z_{Go,i1}^* Z_{Go,j8}^* Z_{Ls,k1}^{Di,*} - i \sqrt{2} g_{A2} \sqrt{\frac{gA^2}{gA^2 + gB^2}} \sqrt{gA^2 + gB^2} Z_{Go,i3}^* Z_{Go,j8}^* Z_{Ls,k1}^{Di,*} \right)
\end{aligned}$$

$$\begin{aligned}
& + 2\sqrt{gA^2 + gB^2} Y_A Z_{Go,i2}^* Z_{Go,j9}^* Z_{Ls,k1}^{Di,*} + 2\sqrt{gA^2 + gB^2} Y_A Z_{Go,i10}^* Z_{Go,j1}^* Z_{Ls,k2}^{Di,*} \\
& + i\sqrt{2} g_{B2} \sqrt{\frac{gA^2}{gA^2 + gB^2}} \sqrt{gA^2 + gB^2} Z_{Go,i7}^* Z_{Go,j2}^* Z_{Ls,k2}^{Di,*} + i\sqrt{2} g_{B2}^2 Z_{Go,i8}^* Z_{Go,j2}^* Z_{Ls,k2}^{Di,*} \\
& + i\sqrt{2} g_{A2} g_{B2} Z_{Go,i7}^* Z_{Go,j4}^* Z_{Ls,k2}^{Di,*} - i\sqrt{2} g_{A2} \sqrt{\frac{gA^2}{gA^2 + gB^2}} \sqrt{gA^2 + gB^2} Z_{Go,i8}^* Z_{Go,j4}^* Z_{Ls,k2}^{Di,*} \\
& - \sqrt{2} g_{B2} \sqrt{\frac{gA^2}{gA^2 + gB^2}} \sqrt{gA^2 + gB^2} Z_{Go,i2}^* Z_{Go,j5}^* Z_{Ls,k2}^{Di,*} + \sqrt{2} g_{A2} g_{B2} Z_{Go,i4}^* Z_{Go,j5}^* Z_{Ls,k2}^{Di,*} \\
& - \sqrt{2} g_{B2}^2 Z_{Go,i2}^* Z_{Go,j6}^* Z_{Ls,k2}^{Di,*} - \sqrt{2} g_{A2} \sqrt{\frac{gA^2}{gA^2 + gB^2}} \sqrt{gA^2 + gB^2} Z_{Go,i4}^* Z_{Go,j6}^* Z_{Ls,k2}^{Di,*} \\
& + i\sqrt{2} g_{B2} \sqrt{\frac{gA^2}{gA^2 + gB^2}} \sqrt{gA^2 + gB^2} Z_{Go,i2}^* Z_{Go,j7}^* Z_{Ls,k2}^{Di,*} + i\sqrt{2} g_{A2} g_{B2} Z_{Go,i4}^* Z_{Go,j7}^* Z_{Ls,k2}^{Di,*} \\
& + i\sqrt{2} g_{B2}^2 Z_{Go,i2}^* Z_{Go,j8}^* Z_{Ls,k2}^{Di,*} - i\sqrt{2} g_{A2} \sqrt{\frac{gA^2}{gA^2 + gB^2}} \sqrt{gA^2 + gB^2} Z_{Go,i4}^* Z_{Go,j8}^* Z_{Ls,k2}^{Di,*} \\
& + 2\sqrt{gA^2 + gB^2} Y_A Z_{Go,i1}^* Z_{Go,j10}^* Z_{Ls,k2}^{Di,*} - i\sqrt{2} g_{A2} g_{B2} Z_{Go,i7}^* Z_{Go,j1}^* Z_{Ls,k3}^{Di,*} \\
& + i\sqrt{2} g_{A2} \sqrt{\frac{gA^2}{gA^2 + gB^2}} \sqrt{gA^2 + gB^2} Z_{Go,i8}^* Z_{Go,j1}^* Z_{Ls,k3}^{Di,*} \\
& - i\sqrt{2} g_{B2} \sqrt{\frac{gA^2}{gA^2 + gB^2}} \sqrt{gA^2 + gB^2} Z_{Go,i7}^* Z_{Go,j3}^* Z_{Ls,k3}^{Di,*} - i\sqrt{2} g_{B2}^2 Z_{Go,i8}^* Z_{Go,j3}^* Z_{Ls,k3}^{Di,*} \\
& + 2\sqrt{gA^2 + gB^2} Y_A Z_{Go,i10}^* Z_{Go,j4}^* Z_{Ls,k3}^{Di,*} - \sqrt{2} g_{A2} g_{B2} Z_{Go,i1}^* Z_{Go,j5}^* Z_{Ls,k3}^{Di,*} \\
& + \sqrt{2} g_{B2} \sqrt{\frac{gA^2}{gA^2 + gB^2}} \sqrt{gA^2 + gB^2} Z_{Go,i3}^* Z_{Go,j5}^* Z_{Ls,k3}^{Di,*} \\
& + \sqrt{2} g_{A2} \sqrt{\frac{gA^2}{gA^2 + gB^2}} \sqrt{gA^2 + gB^2} Z_{Go,i1}^* Z_{Go,j6}^* Z_{Ls,k3}^{Di,*} + \sqrt{2} g_{B2}^2 Z_{Go,i3}^* Z_{Go,j6}^* Z_{Ls,k3}^{Di,*} \\
& - i\sqrt{2} g_{A2} g_{B2} Z_{Go,i1}^* Z_{Go,j7}^* Z_{Ls,k3}^{Di,*} - i\sqrt{2} g_{B2} \sqrt{\frac{gA^2}{gA^2 + gB^2}} \sqrt{gA^2 + gB^2} Z_{Go,i3}^* Z_{Go,j7}^* Z_{Ls,k3}^{Di,*} \\
& + i\sqrt{2} g_{A2} \sqrt{\frac{gA^2}{gA^2 + gB^2}} \sqrt{gA^2 + gB^2} Z_{Go,i1}^* Z_{Go,j8}^* Z_{Ls,k3}^{Di,*} - i\sqrt{2} g_{B2}^2 Z_{Go,i3}^* Z_{Go,j8}^* Z_{Ls,k3}^{Di,*} \\
& + 2\sqrt{gA^2 + gB^2} Y_A Z_{Go,i4}^* Z_{Go,j10}^* Z_{Ls,k3}^{Di,*} - i\sqrt{2} g_{A2} g_{B2} Z_{Go,i7}^* Z_{Go,j2}^* Z_{Ls,k4}^{Di,*} \\
& + i\sqrt{2} g_{A2} \sqrt{\frac{gA^2}{gA^2 + gB^2}} \sqrt{gA^2 + gB^2} Z_{Go,i8}^* Z_{Go,j2}^* Z_{Ls,k4}^{Di,*}
\end{aligned}$$



$$\begin{aligned}
& + 2\sqrt{gA^2 + gB^2}Y_A Z_{Go,i9}^* Z_{Go,j3}^* Z_{Ls,k4}^{Di,*} \\
& - i\sqrt{2}g_{B2}\sqrt{\frac{gA^2}{gA^2 + gB^2}}\sqrt{gA^2 + gB^2}Z_{Go,i7}^* Z_{Go,j4}^* Z_{Ls,k4}^{Di,*} - i\sqrt{2}g_{B2}^2 Z_{Go,i8}^* Z_{Go,j4}^* Z_{Ls,k4}^{Di,*} \\
& + \sqrt{2}g_{A2}g_{B2}Z_{Go,i2}^* Z_{Go,j5}^* Z_{Ls,k4}^{Di,*} - \sqrt{2}g_{B2}\sqrt{\frac{gA^2}{gA^2 + gB^2}}\sqrt{gA^2 + gB^2}Z_{Go,i4}^* Z_{Go,j5}^* Z_{Ls,k4}^{Di,*} \\
& - \sqrt{2}g_{A2}\sqrt{\frac{gA^2}{gA^2 + gB^2}}\sqrt{gA^2 + gB^2}Z_{Go,i2}^* Z_{Go,j6}^* Z_{Ls,k4}^{Di,*} - \sqrt{2}g_{B2}^2 Z_{Go,i4}^* Z_{Go,j6}^* Z_{Ls,k4}^{Di,*} \\
& - i\sqrt{2}g_{A2}g_{B2}Z_{Go,i2}^* Z_{Go,j7}^* Z_{Ls,k4}^{Di,*} - i\sqrt{2}g_{B2}\sqrt{\frac{gA^2}{gA^2 + gB^2}}\sqrt{gA^2 + gB^2}Z_{Go,i4}^* Z_{Go,j7}^* Z_{Ls,k4}^{Di,*} \\
& + i\sqrt{2}g_{A2}\sqrt{\frac{gA^2}{gA^2 + gB^2}}\sqrt{gA^2 + gB^2}Z_{Go,i2}^* Z_{Go,j8}^* Z_{Ls,k4}^{Di,*} - i\sqrt{2}g_{B2}^2 Z_{Go,i4}^* Z_{Go,j8}^* Z_{Ls,k4}^{Di,*} \\
& + 2\sqrt{gA^2 + gB^2}Y_A Z_{Go,i3}^* Z_{Go,j9}^* Z_{Ls,k4}^{Di,*} \\
& + \sqrt{2}Z_{Go,i6}^* \left( -g_{B2}^2 Z_{Go,j2}^* Z_{Ls,k2}^{Di,*} - g_{A2}\sqrt{\frac{gA^2}{gA^2 + gB^2}}\sqrt{gA^2 + gB^2}Z_{Go,j4}^* Z_{Ls,k2}^{Di,*} \right. \\
& + Z_{Go,j3}^* \left( g_{A2}\sqrt{\frac{gA^2}{gA^2 + gB^2}}\sqrt{gA^2 + gB^2}Z_{Ls,k1}^{Di,*} + g_{B2}^2 Z_{Ls,k3}^{Di,*} \right) \\
& + Z_{Go,j1}^* \left( g_{A2}\sqrt{\frac{gA^2}{gA^2 + gB^2}}\sqrt{gA^2 + gB^2}Z_{Ls,k3}^{Di,*} + g_{B2}^2 Z_{Ls,k1}^{Di,*} \right) \\
& \left. - g_{A2}\sqrt{\frac{gA^2}{gA^2 + gB^2}}\sqrt{gA^2 + gB^2}Z_{Go,j2}^* Z_{Ls,k4}^{Di,*} - g_{B2}^2 Z_{Go,j4}^* Z_{Ls,k4}^{Di,*} \right) \\
& + \sqrt{2}g_{B2}Z_{Go,i5}^* \left( -\sqrt{\frac{gA^2}{gA^2 + gB^2}}\sqrt{gA^2 + gB^2}Z_{Go,j2}^* Z_{Ls,k2}^{Di,*} + g_{A2}Z_{Go,j4}^* Z_{Ls,k2}^{Di,*} \right. \\
& + Z_{Go,j1}^* \left( -g_{A2}Z_{Ls,k3}^{Di,*} + \sqrt{\frac{gA^2}{gA^2 + gB^2}}\sqrt{gA^2 + gB^2}Z_{Ls,k1}^{Di,*} \right) \\
& + Z_{Go,j3}^* \left( -g_{A2}Z_{Ls,k1}^{Di,*} + \sqrt{\frac{gA^2}{gA^2 + gB^2}}\sqrt{gA^2 + gB^2}Z_{Ls,k3}^{Di,*} \right) + g_{A2}Z_{Go,j2}^* Z_{Ls,k4}^{Di,*} \\
& \left. - \sqrt{\frac{gA^2}{gA^2 + gB^2}}\sqrt{gA^2 + gB^2}Z_{Go,j4}^* Z_{Ls,k4}^{Di,*} \right) \left( \frac{1-\gamma_5}{2} \right) \\
& + \frac{1}{2}\frac{1}{\sqrt{gA^2 + gB^2}} \left( -2\sqrt{gA^2 + gB^2}Y_A^* Z_{Ls,k2}^{Di,*} Z_{Go,i10} Z_{Go,j1} \right. \\
& \left. + \sqrt{2}g_{B2}\sqrt{\frac{gA^2}{gA^2 + gB^2}}\sqrt{gA^2 + gB^2}Z_{Ls,k2}^{Di,*} Z_{Go,i5} Z_{Go,j2} - \sqrt{2}g_{A2}g_{B2}Z_{Ls,k4}^{Di,*} Z_{Go,i5} Z_{Go,j2} \right)
\end{aligned} \tag{792}$$

$$\begin{aligned}
& + \sqrt{2}g_{B2}^2 Z_{Ls,k2}^{Di,*} Z_{Go,i6} Z_{Go,j2} + \sqrt{2}g_{A2} \sqrt{\frac{gA2^2}{gA2^2 + gB2^2}} \sqrt{gA2^2 + gB2^2} Z_{Ls,k4}^{Di,*} Z_{Go,i6} Z_{Go,j2} \\
& + i\sqrt{2}g_{B2} \sqrt{\frac{gA2^2}{gA2^2 + gB2^2}} \sqrt{gA2^2 + gB2^2} Z_{Ls,k2}^{Di,*} Z_{Go,i7} Z_{Go,j2} - i\sqrt{2}g_{A2}g_{B2} Z_{Ls,k4}^{Di,*} Z_{Go,i7} Z_{Go,j2} \\
& + i\sqrt{2}g_{B2}^2 Z_{Ls,k2}^{Di,*} Z_{Go,i8} Z_{Go,j2} + i\sqrt{2}g_{A2} \sqrt{\frac{gA2^2}{gA2^2 + gB2^2}} \sqrt{gA2^2 + gB2^2} Z_{Ls,k4}^{Di,*} Z_{Go,i8} Z_{Go,j2} \\
& - 2\sqrt{gA2^2 + gB2^2} Y_A^* Z_{Ls,k4}^{Di,*} Z_{Go,i9} Z_{Go,j3} - \sqrt{2}g_{A2}g_{B2} Z_{Ls,k2}^{Di,*} Z_{Go,i5} Z_{Go,j4} \\
& + \sqrt{2}g_{B2} \sqrt{\frac{gA2^2}{gA2^2 + gB2^2}} \sqrt{gA2^2 + gB2^2} Z_{Ls,k4}^{Di,*} Z_{Go,i5} Z_{Go,j4} \\
& + \sqrt{2}g_{A2} \sqrt{\frac{gA2^2}{gA2^2 + gB2^2}} \sqrt{gA2^2 + gB2^2} Z_{Ls,k2}^{Di,*} Z_{Go,i6} Z_{Go,j4} + \sqrt{2}g_{B2}^2 Z_{Ls,k4}^{Di,*} Z_{Go,i6} Z_{Go,j4} \\
& + i\sqrt{2}g_{A2}g_{B2} Z_{Ls,k2}^{Di,*} Z_{Go,i7} Z_{Go,j4} - i\sqrt{2}g_{B2} \sqrt{\frac{gA2^2}{gA2^2 + gB2^2}} \sqrt{gA2^2 + gB2^2} Z_{Ls,k4}^{Di,*} Z_{Go,i7} Z_{Go,j4} \\
& - i\sqrt{2}g_{A2} \sqrt{\frac{gA2^2}{gA2^2 + gB2^2}} \sqrt{gA2^2 + gB2^2} Z_{Ls,k2}^{Di,*} Z_{Go,i8} Z_{Go,j4} - i\sqrt{2}g_{B2}^2 Z_{Ls,k4}^{Di,*} Z_{Go,i8} Z_{Go,j4} \\
& + \sqrt{2}g_{B2} \sqrt{\frac{gA2^2}{gA2^2 + gB2^2}} \sqrt{gA2^2 + gB2^2} Z_{Ls,k2}^{Di,*} Z_{Go,i2} Z_{Go,j5} - \sqrt{2}g_{A2}g_{B2} Z_{Ls,k4}^{Di,*} Z_{Go,i2} Z_{Go,j5} \\
& - \sqrt{2}g_{A2}g_{B2} Z_{Ls,k2}^{Di,*} Z_{Go,i4} Z_{Go,j5} + \sqrt{2}g_{B2} \sqrt{\frac{gA2^2}{gA2^2 + gB2^2}} \sqrt{gA2^2 + gB2^2} Z_{Ls,k4}^{Di,*} Z_{Go,i4} Z_{Go,j5} \\
& + \sqrt{2}g_{B2}^2 Z_{Ls,k2}^{Di,*} Z_{Go,i2} Z_{Go,j6} + \sqrt{2}g_{A2} \sqrt{\frac{gA2^2}{gA2^2 + gB2^2}} \sqrt{gA2^2 + gB2^2} Z_{Ls,k4}^{Di,*} Z_{Go,i2} Z_{Go,j6} \\
& + \sqrt{2}g_{A2} \sqrt{\frac{gA2^2}{gA2^2 + gB2^2}} \sqrt{gA2^2 + gB2^2} Z_{Ls,k2}^{Di,*} Z_{Go,i4} Z_{Go,j6} + \sqrt{2}g_{B2}^2 Z_{Ls,k4}^{Di,*} Z_{Go,i4} Z_{Go,j6} \\
& + i\sqrt{2}g_{B2} \sqrt{\frac{gA2^2}{gA2^2 + gB2^2}} \sqrt{gA2^2 + gB2^2} Z_{Ls,k2}^{Di,*} Z_{Go,i2} Z_{Go,j7} - i\sqrt{2}g_{A2}g_{B2} Z_{Ls,k4}^{Di,*} Z_{Go,i2} Z_{Go,j7} \\
& + i\sqrt{2}g_{A2}g_{B2} Z_{Ls,k2}^{Di,*} Z_{Go,i4} Z_{Go,j7} - i\sqrt{2}g_{B2} \sqrt{\frac{gA2^2}{gA2^2 + gB2^2}} \sqrt{gA2^2 + gB2^2} Z_{Ls,k4}^{Di,*} Z_{Go,i4} Z_{Go,j7} \\
& + i\sqrt{2}g_{B2}^2 Z_{Ls,k2}^{Di,*} Z_{Go,i2} Z_{Go,j8} + i\sqrt{2}g_{A2} \sqrt{\frac{gA2^2}{gA2^2 + gB2^2}} \sqrt{gA2^2 + gB2^2} Z_{Ls,k4}^{Di,*} Z_{Go,i2} Z_{Go,j8} \\
& - i\sqrt{2}g_{A2} \sqrt{\frac{gA2^2}{gA2^2 + gB2^2}} \sqrt{gA2^2 + gB2^2} Z_{Ls,k2}^{Di,*} Z_{Go,i4} Z_{Go,j8} - i\sqrt{2}g_{B2}^2 Z_{Ls,k4}^{Di,*} Z_{Go,i4} Z_{Go,j8}
\end{aligned}$$

$$\begin{aligned}
& -2\sqrt{gA^2 + gB^2}Y_A^*Z_{Ls,k4}^{Di,*}Z_{Go,i3}Z_{Go,j9} \\
& -Z_{Ls,k1}^{Di,*}\left(-i\sqrt{2}g_{B2}\sqrt{\frac{gA^2}{gA^2 + gB^2}}\sqrt{gA^2 + gB^2}Z_{Go,i7}Z_{Go,j1} - i\sqrt{2}g_{B2}^2Z_{Go,i8}Z_{Go,j1}\right. \\
& + 2\sqrt{gA^2 + gB^2}Y_A^*Z_{Go,i9}Z_{Go,j2} - i\sqrt{2}g_{A2}g_{B2}Z_{Go,i7}Z_{Go,j3} \\
& + i\sqrt{2}g_{A2}\sqrt{\frac{gA^2}{gA^2 + gB^2}}\sqrt{gA^2 + gB^2}Z_{Go,i8}Z_{Go,j3} \\
& + \sqrt{2}g_{B2}Z_{Go,i5}\left(-g_{A2}Z_{Go,j3} + \sqrt{\frac{gA^2}{gA^2 + gB^2}}\sqrt{gA^2 + gB^2}Z_{Go,j1}\right) \\
& + \sqrt{2}Z_{Go,i6}\left(g_{A2}\sqrt{\frac{gA^2}{gA^2 + gB^2}}\sqrt{gA^2 + gB^2}Z_{Go,j3} + g_{B2}^2Z_{Go,j1}\right) \\
& + \sqrt{2}g_{B2}\sqrt{\frac{gA^2}{gA^2 + gB^2}}\sqrt{gA^2 + gB^2}Z_{Go,i1}Z_{Go,j5} - \sqrt{2}g_{A2}g_{B2}Z_{Go,i3}Z_{Go,j5} + \sqrt{2}g_{B2}^2Z_{Go,i1}Z_{Go,j6} \\
& + \sqrt{2}g_{A2}\sqrt{\frac{gA^2}{gA^2 + gB^2}}\sqrt{gA^2 + gB^2}Z_{Go,i3}Z_{Go,j6} \\
& - i\sqrt{2}g_{B2}\sqrt{\frac{gA^2}{gA^2 + gB^2}}\sqrt{gA^2 + gB^2}Z_{Go,i1}Z_{Go,j7} - i\sqrt{2}g_{A2}g_{B2}Z_{Go,i3}Z_{Go,j7} \\
& - i\sqrt{2}g_{B2}^2Z_{Go,i1}Z_{Go,j8} + i\sqrt{2}g_{A2}\sqrt{\frac{gA^2}{gA^2 + gB^2}}\sqrt{gA^2 + gB^2}Z_{Go,i3}Z_{Go,j8} \\
& + 2\sqrt{gA^2 + gB^2}Y_A^*Z_{Go,i2}Z_{Go,j9}\Big) \\
& - 2\sqrt{gA^2 + gB^2}Y_A^*Z_{Ls,k2}^{Di,*}Z_{Go,i1}Z_{Go,j10} \\
& - Z_{Ls,k3}^{Di,*}\left(i\sqrt{2}g_{A2}g_{B2}Z_{Go,i7}Z_{Go,j1} - i\sqrt{2}g_{A2}\sqrt{\frac{gA^2}{gA^2 + gB^2}}\sqrt{gA^2 + gB^2}Z_{Go,i8}Z_{Go,j1}\right. \\
& + i\sqrt{2}g_{B2}\sqrt{\frac{gA^2}{gA^2 + gB^2}}\sqrt{gA^2 + gB^2}Z_{Go,i7}Z_{Go,j3} + i\sqrt{2}g_{B2}^2Z_{Go,i8}Z_{Go,j3} \\
& + \sqrt{2}Z_{Go,i6}\left(g_{A2}\sqrt{\frac{gA^2}{gA^2 + gB^2}}\sqrt{gA^2 + gB^2}Z_{Go,j1} + g_{B2}^2Z_{Go,j3}\right) \\
& + \sqrt{2}g_{B2}Z_{Go,i5}\left(-g_{A2}Z_{Go,j1} + \sqrt{\frac{gA^2}{gA^2 + gB^2}}\sqrt{gA^2 + gB^2}Z_{Go,j3}\right) + 2\sqrt{gA^2 + gB^2}Y_A^*Z_{Go,i10}Z_{Go,j4} \\
& - \sqrt{2}g_{A2}g_{B2}Z_{Go,i1}Z_{Go,j5} + \sqrt{2}g_{B2}\sqrt{\frac{gA^2}{gA^2 + gB^2}}\sqrt{gA^2 + gB^2}Z_{Go,i3}Z_{Go,j5}
\end{aligned}$$

$$\begin{aligned}
& + \sqrt{2}g_{A2}\sqrt{\frac{gA2^2}{gA2^2 + gB2^2}}\sqrt{gA2^2 + gB2^2}Z_{Go,i1}Z_{Go,j6} + \sqrt{2}g_{B2}^2Z_{Go,i3}Z_{Go,j6} + i\sqrt{2}g_{A2}g_{B2}Z_{Go,i1}Z_{Go,j7} \\
& + i\sqrt{2}g_{B2}\sqrt{\frac{gA2^2}{gA2^2 + gB2^2}}\sqrt{gA2^2 + gB2^2}Z_{Go,i3}Z_{Go,j7} \\
& - i\sqrt{2}g_{A2}\sqrt{\frac{gA2^2}{gA2^2 + gB2^2}}\sqrt{gA2^2 + gB2^2}Z_{Go,i1}Z_{Go,j8} + i\sqrt{2}g_{B2}^2Z_{Go,i3}Z_{Go,j8} \\
& + 2\sqrt{gA2^2 + gB2^2}Y_A^*Z_{Go,i4}Z_{Go,j10}\Big)\Big)\Big(\frac{1+\gamma_5}{2}\Big)
\end{aligned} \tag{793}$$


---

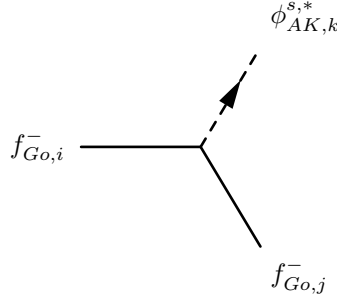

$$\begin{aligned}
& ig_{B2}\frac{1}{\sqrt{gA2^2 + gB2^2}}\Big(-Z_{Go,i10}^*\Big(\sqrt{\frac{gA2^2}{gA2^2 + gB2^2}}\sqrt{gA2^2 + gB2^2}Z_{Go,j5}^* + g_{B2}Z_{Go,j6}^* \\
& - i\Big(g_{B2}Z_{Go,j8}^* + \sqrt{\frac{gA2^2}{gA2^2 + gB2^2}}\sqrt{gA2^2 + gB2^2}Z_{Go,j7}^*\Big)\Big) \\
& + Z_{Go,i9}^*\Big(\sqrt{\frac{gA2^2}{gA2^2 + gB2^2}}\sqrt{gA2^2 + gB2^2}Z_{Go,j5}^* + g_{B2}Z_{Go,j6}^* \\
& + i\Big(g_{B2}Z_{Go,j8}^* + \sqrt{\frac{gA2^2}{gA2^2 + gB2^2}}\sqrt{gA2^2 + gB2^2}Z_{Go,j7}^*\Big)\Big) \\
& + \sqrt{\frac{gA2^2}{gA2^2 + gB2^2}}\sqrt{gA2^2 + gB2^2}Z_{Go,i5}^*Z_{Go,j9}^* + g_{B2}Z_{Go,i6}^*Z_{Go,j9}^* \\
& + i\sqrt{\frac{gA2^2}{gA2^2 + gB2^2}}\sqrt{gA2^2 + gB2^2}Z_{Go,i7}^*Z_{Go,j9}^* + ig_{B2}Z_{Go,i8}^*Z_{Go,j9}^* \\
& - \sqrt{\frac{gA2^2}{gA2^2 + gB2^2}}\sqrt{gA2^2 + gB2^2}Z_{Go,i5}^*Z_{Go,j10}^* - g_{B2}Z_{Go,i6}^*Z_{Go,j10}^* \\
& + i\sqrt{\frac{gA2^2}{gA2^2 + gB2^2}}\sqrt{gA2^2 + gB2^2}Z_{Go,i7}^*Z_{Go,j10}^* + ig_{B2}Z_{Go,i8}^*Z_{Go,j10}^*\Big)Z_{AK,k2}^s\Big(\frac{1-\gamma_5}{2}\Big)
\end{aligned} \tag{794}$$

$$\begin{aligned}
& + \frac{i}{2} \left( \sqrt{2} Y_A^* Z_{AK,k2}^s \left( -Z_{Go,i1} Z_{Go,j2} - Z_{Go,i2} Z_{Go,j1} + Z_{Go,i3} Z_{Go,j4} + Z_{Go,i4} Z_{Go,j3} \right) \right. \\
& \left. + Y_K^* Z_{AK,k1}^s \left( Z_{Go,i1} Z_{Go,j2} + Z_{Go,i2} Z_{Go,j1} + Z_{Go,i3} Z_{Go,j4} + Z_{Go,i4} Z_{Go,j3} \right) \right) \left( \frac{1+\gamma_5}{2} \right)
\end{aligned} \tag{795}$$


---

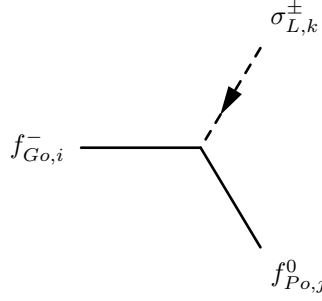

$$\begin{aligned}
& \frac{1}{2} \left( \sqrt{2} g_{A2} g_{B2} \frac{1}{\sqrt{g_{A2}^2 + g_{B2}^2}} Z_{Go,i7}^* Z_{Ls,k4}^{od,*} Z_{Po,j1}^* - \sqrt{2} g_{A2} \sqrt{\frac{g_{A2}^2}{g_{A2}^2 + g_{B2}^2}} Z_{Go,i8}^* Z_{Ls,k4}^{od,*} Z_{Po,j1}^* \right. \\
& - 2i Y_A Z_{Go,i10}^* Z_{Ls,k1}^{od,*} Z_{Po,j2}^* + \sqrt{2} g_{B2} \sqrt{\frac{g_{A2}^2}{g_{A2}^2 + g_{B2}^2}} Z_{Go,i7}^* Z_{Ls,k3}^{od,*} Z_{Po,j2}^* \\
& + \sqrt{2} g_{B2}^2 \frac{1}{\sqrt{g_{A2}^2 + g_{B2}^2}} Z_{Go,i8}^* Z_{Ls,k3}^{od,*} Z_{Po,j2}^* - 2i Y_A Z_{Go,i10}^* Z_{Ls,k2}^{od,*} Z_{Po,j3}^* \\
& - \sqrt{2} g_{B2} \sqrt{\frac{g_{A2}^2}{g_{A2}^2 + g_{B2}^2}} Z_{Go,i7}^* Z_{Ls,k4}^{od,*} Z_{Po,j3}^* - \sqrt{2} g_{B2}^2 \frac{1}{\sqrt{g_{A2}^2 + g_{B2}^2}} Z_{Go,i8}^* Z_{Ls,k4}^{od,*} Z_{Po,j3}^* \\
& - \sqrt{2} g_{A2} g_{B2} \frac{1}{\sqrt{g_{A2}^2 + g_{B2}^2}} Z_{Go,i7}^* Z_{Ls,k3}^{od,*} Z_{Po,j4}^* + \sqrt{2} g_{A2} \sqrt{\frac{g_{A2}^2}{g_{A2}^2 + g_{B2}^2}} Z_{Go,i8}^* Z_{Ls,k3}^{od,*} Z_{Po,j4}^* \\
& + i\sqrt{2} g_{B2} \frac{1}{\sqrt{g_{A2}^2 + g_{B2}^2}} Z_{Go,i5}^* \left( Z_{Ls,k4}^{od,*} \left( -g_{A2} Z_{Po,j1}^* + \sqrt{\frac{g_{A2}^2}{g_{A2}^2 + g_{B2}^2}} \sqrt{g_{A2}^2 + g_{B2}^2} Z_{Po,j3}^* \right) \right. \\
& \left. + Z_{Ls,k3}^{od,*} \left( g_{A2} Z_{Po,j4}^* - \sqrt{\frac{g_{A2}^2}{g_{A2}^2 + g_{B2}^2}} \sqrt{g_{A2}^2 + g_{B2}^2} Z_{Po,j2}^* \right) \right) \\
& + i\sqrt{2} \frac{1}{\sqrt{g_{A2}^2 + g_{B2}^2}} Z_{Go,i6}^* \left( Z_{Ls,k4}^{od,*} \left( g_{A2} \sqrt{\frac{g_{A2}^2}{g_{A2}^2 + g_{B2}^2}} \sqrt{g_{A2}^2 + g_{B2}^2} Z_{Po,j1}^* + g_{B2}^2 Z_{Po,j3}^* \right) \right. \\
& \left. - Z_{Ls,k3}^{od,*} \left( g_{A2} \sqrt{\frac{g_{A2}^2}{g_{A2}^2 + g_{B2}^2}} \sqrt{g_{A2}^2 + g_{B2}^2} Z_{Po,j4}^* + g_{B2}^2 Z_{Po,j2}^* \right) \right) \\
& + i\sqrt{2} g_{B1} \sqrt{\frac{g_{A1}^2}{g_{A1}^2 + g_{B1}^2}} Z_{Go,i2}^* Z_{Ls,k3}^{od,*} Z_{Po,j5}^* - i\sqrt{2} g_{A1} g_{B1} \frac{1}{\sqrt{g_{A1}^2 + g_{B1}^2}} Z_{Go,i2}^* Z_{Ls,k3}^{od,*} Z_{Po,j5}^* \\
& - i\sqrt{2} g_{B1} \sqrt{\frac{g_{A1}^2}{g_{A1}^2 + g_{B1}^2}} Z_{Go,i3}^* Z_{Ls,k4}^{od,*} Z_{Po,j5}^* + i\sqrt{2} g_{A1} g_{B1} \frac{1}{\sqrt{g_{A1}^2 + g_{B1}^2}} Z_{Go,i3}^* Z_{Ls,k4}^{od,*} Z_{Po,j5}^*
\end{aligned}$$

$$\begin{aligned}
& + i\sqrt{2}g_{A1}\sqrt{\frac{gA1^2}{gA1^2 + gB1^2}}Z_{Go,i2}^*Z_{Ls,k3}^{od,*}Z_{Po,j6}^* + i\sqrt{2}g_{B1}^2\frac{1}{\sqrt{gA1^2 + gB1^2}}Z_{Go,i2}^*Z_{Ls,k3}^{od,*}Z_{Po,j6}^* \\
& - i\sqrt{2}g_{A1}\sqrt{\frac{gA1^2}{gA1^2 + gB1^2}}Z_{Go,i3}^*Z_{Ls,k4}^{od,*}Z_{Po,j6}^* - i\sqrt{2}g_{B1}^2\frac{1}{\sqrt{gA1^2 + gB1^2}}Z_{Go,i3}^*Z_{Ls,k4}^{od,*}Z_{Po,j6}^* \\
& + i\sqrt{2}g_{B2}\sqrt{\frac{gA2^2}{gA2^2 + gB2^2}}Z_{Go,i2}^*Z_{Ls,k3}^{od,*}Z_{Po,j7}^* + i\sqrt{2}g_{A2}g_{B2}\frac{1}{\sqrt{gA2^2 + gB2^2}}Z_{Go,i2}^*Z_{Ls,k3}^{od,*}Z_{Po,j7}^* \\
& + i\sqrt{2}g_{B2}\sqrt{\frac{gA2^2}{gA2^2 + gB2^2}}Z_{Go,i3}^*Z_{Ls,k4}^{od,*}Z_{Po,j7}^* + i\sqrt{2}g_{A2}g_{B2}\frac{1}{\sqrt{gA2^2 + gB2^2}}Z_{Go,i3}^*Z_{Ls,k4}^{od,*}Z_{Po,j7}^* \\
& - i\sqrt{2}g_{A2}\sqrt{\frac{gA2^2}{gA2^2 + gB2^2}}Z_{Go,i2}^*Z_{Ls,k3}^{od,*}Z_{Po,j8}^* + i\sqrt{2}g_{B2}^2\frac{1}{\sqrt{gA2^2 + gB2^2}}Z_{Go,i2}^*Z_{Ls,k3}^{od,*}Z_{Po,j8}^* \\
& - i\sqrt{2}g_{A2}\sqrt{\frac{gA2^2}{gA2^2 + gB2^2}}Z_{Go,i3}^*Z_{Ls,k4}^{od,*}Z_{Po,j8}^* + i\sqrt{2}g_{B2}^2\frac{1}{\sqrt{gA2^2 + gB2^2}}Z_{Go,i3}^*Z_{Ls,k4}^{od,*}Z_{Po,j8}^* \\
& + i\sqrt{2}Y_A Z_{Go,i2}^*Z_{Ls,k1}^{od,*}Z_{Po,j9}^* - i\sqrt{2}Y_A Z_{Go,i3}^*Z_{Ls,k2}^{od,*}Z_{Po,j9}^* - iY_K Z_{Go,i2}^*Z_{Ls,k1}^{od,*}Z_{Po,j10}^* \\
& - iY_K Z_{Go,i3}^*Z_{Ls,k2}^{od,*}Z_{Po,j10}^* \left( \frac{1 - \gamma_5}{2} \right) \tag{796} \\
& + \frac{1}{2} \left( i\sqrt{2}g_{A2}g_{B2}\frac{1}{\sqrt{gA2^2 + gB2^2}}Z_{Ls,k2}^{od,*}Z_{Go,i5}Z_{Po,j2} - i\sqrt{2}g_{A2}\sqrt{\frac{gA2^2}{gA2^2 + gB2^2}}Z_{Ls,k2}^{od,*}Z_{Go,i6}Z_{Po,j2} \right. \\
& - \sqrt{2}g_{A2}g_{B2}\frac{1}{\sqrt{gA2^2 + gB2^2}}Z_{Ls,k2}^{od,*}Z_{Go,i7}Z_{Po,j2} + \sqrt{2}g_{A2}\sqrt{\frac{gA2^2}{gA2^2 + gB2^2}}Z_{Ls,k2}^{od,*}Z_{Go,i8}Z_{Po,j2} \\
& - i\sqrt{2}g_{B2}\sqrt{\frac{gA2^2}{gA2^2 + gB2^2}}Z_{Ls,k2}^{od,*}Z_{Go,i5}Z_{Po,j4} - i\sqrt{2}g_{B2}^2\frac{1}{\sqrt{gA2^2 + gB2^2}}Z_{Ls,k2}^{od,*}Z_{Go,i6}Z_{Po,j4} \\
& + \sqrt{2}g_{B2}\sqrt{\frac{gA2^2}{gA2^2 + gB2^2}}Z_{Ls,k2}^{od,*}Z_{Go,i7}Z_{Po,j4} + \sqrt{2}g_{B2}^2\frac{1}{\sqrt{gA2^2 + gB2^2}}Z_{Ls,k2}^{od,*}Z_{Go,i8}Z_{Po,j4} \\
& + i\sqrt{2}g_{B1}\sqrt{\frac{gA1^2}{gA1^2 + gB1^2}}Z_{Ls,k2}^{od,*}Z_{Go,i4}Z_{Po,j5} - i\sqrt{2}g_{A1}g_{B1}\frac{1}{\sqrt{gA1^2 + gB1^2}}Z_{Ls,k2}^{od,*}Z_{Go,i4}Z_{Po,j5} \\
& + i\sqrt{2}g_{A1}\sqrt{\frac{gA1^2}{gA1^2 + gB1^2}}Z_{Ls,k2}^{od,*}Z_{Go,i4}Z_{Po,j6} + i\sqrt{2}g_{B1}^2\frac{1}{\sqrt{gA1^2 + gB1^2}}Z_{Ls,k2}^{od,*}Z_{Go,i4}Z_{Po,j6} \\
& - i\sqrt{2}g_{B2}\sqrt{\frac{gA2^2}{gA2^2 + gB2^2}}Z_{Ls,k2}^{od,*}Z_{Go,i4}Z_{Po,j7} - i\sqrt{2}g_{A2}g_{B2}\frac{1}{\sqrt{gA2^2 + gB2^2}}Z_{Ls,k2}^{od,*}Z_{Go,i4}Z_{Po,j7} \\
& + i\sqrt{2}g_{A2}\sqrt{\frac{gA2^2}{gA2^2 + gB2^2}}Z_{Ls,k2}^{od,*}Z_{Go,i4}Z_{Po,j8} - i\sqrt{2}g_{B2}^2\frac{1}{\sqrt{gA2^2 + gB2^2}}Z_{Ls,k2}^{od,*}Z_{Go,i4}Z_{Po,j8}
\end{aligned}$$

$$\begin{aligned}
& + \sqrt{2} Z_{Ls,k1}^{od,*} \left( -g_{B2} \sqrt{\frac{gA2^2}{gA2^2 + gB2^2}} Z_{Go,i7} Z_{Po,j1} - g_{B2}^2 \frac{1}{\sqrt{gA2^2 + gB2^2}} Z_{Go,i8} Z_{Po,j1} \right. \\
& + g_{A2} g_{B2} \frac{1}{\sqrt{gA2^2 + gB2^2}} Z_{Go,i7} Z_{Po,j3} - g_{A2} \sqrt{\frac{gA2^2}{gA2^2 + gB2^2}} Z_{Go,i8} Z_{Po,j3} \\
& + i Z_{Go,i6} \left( g_{A2} \sqrt{\frac{gA2^2}{gA2^2 + gB2^2}} Z_{Po,j3} + g_{B2}^2 \frac{1}{\sqrt{gA2^2 + gB2^2}} Z_{Po,j1} \right) \\
& + i g_{B2} Z_{Go,i5} \left( -g_{A2} \frac{1}{\sqrt{gA2^2 + gB2^2}} Z_{Po,j3} + \sqrt{\frac{gA2^2}{gA2^2 + gB2^2}} Z_{Po,j1} \right) \\
& - i g_{B1} \sqrt{\frac{gA1^2}{gA1^2 + gB1^2}} Z_{Go,i1} Z_{Po,j5} + i g_{A1} g_{B1} \frac{1}{\sqrt{gA1^2 + gB1^2}} Z_{Go,i1} Z_{Po,j5} \\
& - i g_{A1} \sqrt{\frac{gA1^2}{gA1^2 + gB1^2}} Z_{Go,i1} Z_{Po,j6} - i g_{B1}^2 \frac{1}{\sqrt{gA1^2 + gB1^2}} Z_{Go,i1} Z_{Po,j6} \\
& - i g_{B2} \sqrt{\frac{gA2^2}{gA2^2 + gB2^2}} Z_{Go,i1} Z_{Po,j7} - i g_{A2} g_{B2} \frac{1}{\sqrt{gA2^2 + gB2^2}} Z_{Go,i1} Z_{Po,j7} \\
& + i g_{A2} \sqrt{\frac{gA2^2}{gA2^2 + gB2^2}} Z_{Go,i1} Z_{Po,j8} - i g_{B2}^2 \frac{1}{\sqrt{gA2^2 + gB2^2}} Z_{Go,i1} Z_{Po,j8} \Big) \\
& - i Y_A^* \left( Z_{Ls,k3}^{od,*} \left( 2 Z_{Go,i9} Z_{Po,j1} - \sqrt{2} Z_{Go,i1} Z_{Po,j9} \right) + Z_{Ls,k4}^{od,*} \left( 2 Z_{Go,i9} Z_{Po,j4} + \sqrt{2} Z_{Go,i4} Z_{Po,j9} \right) \right) \\
& - i Y_K^* Z_{Ls,k3}^{od,*} Z_{Go,i1} Z_{Po,j10} - i Y_K^* Z_{Ls,k4}^{od,*} Z_{Go,i4} Z_{Po,j10} \Big) \left( \frac{1 + \gamma_5}{2} \right) \tag{797}
\end{aligned}$$


---

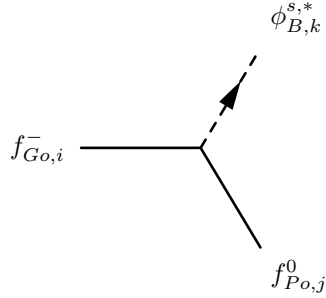

$$\begin{aligned}
& \left( -i \sqrt{2} g_{B2} \frac{1}{\sqrt{gA2^2 + gB2^2}} Z_{Go,i9}^* \left( g_{B2} Z_{Po,j8}^* + \sqrt{\frac{gA2^2}{gA2^2 + gB2^2}} \sqrt{gA2^2 + gB2^2} Z_{Po,j7}^* \right) B_{A,k1}^s \right. \\
& + i g_{B2} \sqrt{\frac{gA2^2}{gA2^2 + gB2^2}} Z_{Go,i5}^* Z_{Po,j9}^* B_{A,k1}^s + i g_{B2}^2 \frac{1}{\sqrt{gA2^2 + gB2^2}} Z_{Go,i6}^* Z_{Po,j9}^* B_{A,k1}^s
\end{aligned}$$

$$\begin{aligned}
& + g_{B2} \sqrt{\frac{gA2^2}{gA2^2 + gB2^2}} Z_{Go,i7}^* Z_{Po,j9}^* B_{A,k1}^s + g_{B2}^2 \frac{1}{\sqrt{gA2^2 + gB2^2}} Z_{Go,i8}^* Z_{Po,j9}^* B_{A,k1}^s \\
& - i Y_A Z_{Go,i1}^* Z_{Po,j2}^* B_{A,k2}^s - i Y_A Z_{Go,i4}^* Z_{Po,j3}^* B_{A,k2}^s \left( \frac{1 - \gamma_5}{2} \right) \tag{798}
\end{aligned}$$

$$\begin{aligned}
& + i \frac{1}{\sqrt{gA2^2 + gB2^2}} \left( - \sqrt{gA2^2 + gB2^2} Y_A^* B_{A,k1}^s \left( Z_{Go,i2} Z_{Po,j1} + Z_{Go,i3} Z_{Po,j4} \right) \right. \\
& + g_{B2} B_{A,k2}^s \left( \sqrt{2} Z_{Go,i10} \left( g_{B2} Z_{Po,j8} + \sqrt{\frac{gA2^2}{gA2^2 + gB2^2}} \sqrt{gA2^2 + gB2^2} Z_{Po,j7} \right) \right. \\
& - \left( \sqrt{\frac{gA2^2}{gA2^2 + gB2^2}} \sqrt{gA2^2 + gB2^2} Z_{Go,i5} + g_{B2} Z_{Go,i6} \right. \\
& \left. \left. \left. - i \left( g_{B2} Z_{Go,i8} + \sqrt{\frac{gA2^2}{gA2^2 + gB2^2}} \sqrt{gA2^2 + gB2^2} Z_{Go,i7} \right) Z_{Po,j9} \right) \right) \right) \left( \frac{1 + \gamma_5}{2} \right) \tag{799}
\end{aligned}$$

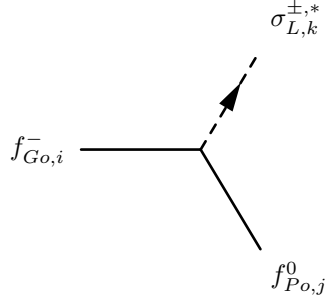

$$\begin{aligned}
& \frac{1}{2} \left( \sqrt{2} g_{B2} \sqrt{\frac{gA2^2}{gA2^2 + gB2^2}} Z_{Go,i7}^* Z_{Po,j1}^* Z_{Ls,k1}^{od} + \sqrt{2} g_{B2}^2 \frac{1}{\sqrt{gA2^2 + gB2^2}} Z_{Go,i8}^* Z_{Po,j1}^* Z_{Ls,k1}^{od} \right. \\
& - \sqrt{2} g_{A2} g_{B2} \frac{1}{\sqrt{gA2^2 + gB2^2}} Z_{Go,i7}^* Z_{Po,j3}^* Z_{Ls,k1}^{od} + \sqrt{2} g_{A2} \sqrt{\frac{gA2^2}{gA2^2 + gB2^2}} Z_{Go,i8}^* Z_{Po,j3}^* Z_{Ls,k1}^{od} \\
& - i \sqrt{2} g_{B1} \sqrt{\frac{gA1^2}{gA1^2 + gB1^2}} Z_{Go,i1}^* Z_{Po,j5}^* Z_{Ls,k1}^{od} + i \sqrt{2} g_{A1} g_{B1} \frac{1}{\sqrt{gA1^2 + gB1^2}} Z_{Go,i1}^* Z_{Po,j5}^* Z_{Ls,k1}^{od} \\
& - i \sqrt{2} g_{A1} \sqrt{\frac{gA1^2}{gA1^2 + gB1^2}} Z_{Go,i1}^* Z_{Po,j6}^* Z_{Ls,k1}^{od} - i \sqrt{2} g_{B1}^2 \frac{1}{\sqrt{gA1^2 + gB1^2}} Z_{Go,i1}^* Z_{Po,j6}^* Z_{Ls,k1}^{od} \\
& - i \sqrt{2} g_{B2} \sqrt{\frac{gA2^2}{gA2^2 + gB2^2}} Z_{Go,i1}^* Z_{Po,j7}^* Z_{Ls,k1}^{od} - i \sqrt{2} g_{A2} g_{B2} \frac{1}{\sqrt{gA2^2 + gB2^2}} Z_{Go,i1}^* Z_{Po,j7}^* Z_{Ls,k1}^{od} \\
& \left. + i \sqrt{2} g_{A2} \sqrt{\frac{gA2^2}{gA2^2 + gB2^2}} Z_{Go,i1}^* Z_{Po,j8}^* Z_{Ls,k1}^{od} - i \sqrt{2} g_{B2}^2 \frac{1}{\sqrt{gA2^2 + gB2^2}} Z_{Go,i1}^* Z_{Po,j8}^* Z_{Ls,k1}^{od} \right)
\end{aligned}$$



$$\begin{aligned}
& + \sqrt{2}g_{A2}g_{B2} \frac{1}{\sqrt{gA2^2 + gB2^2}} Z_{Go,i7}^* Z_{Po,j2}^* Z_{Ls,k2}^{od} - \sqrt{2}g_{A2} \sqrt{\frac{gA2^2}{gA2^2 + gB2^2}} Z_{Go,i8}^* Z_{Po,j2}^* Z_{Ls,k2}^{od} \\
& - \sqrt{2}g_{B2} \sqrt{\frac{gA2^2}{gA2^2 + gB2^2}} Z_{Go,i7}^* Z_{Po,j4}^* Z_{Ls,k2}^{od} - \sqrt{2}g_{B2}^2 \frac{1}{\sqrt{gA2^2 + gB2^2}} Z_{Go,i8}^* Z_{Po,j4}^* Z_{Ls,k2}^{od} \\
& + i\sqrt{2}g_{B1} \sqrt{\frac{gA1^2}{gA1^2 + gB1^2}} Z_{Go,i4}^* Z_{Po,j5}^* Z_{Ls,k2}^{od} - i\sqrt{2}g_{A1}g_{B1} \frac{1}{\sqrt{gA1^2 + gB1^2}} Z_{Go,i4}^* Z_{Po,j5}^* Z_{Ls,k2}^{od} \\
& + i\sqrt{2}g_{A1} \sqrt{\frac{gA1^2}{gA1^2 + gB1^2}} Z_{Go,i4}^* Z_{Po,j6}^* Z_{Ls,k2}^{od} + i\sqrt{2}g_{B1}^2 \frac{1}{\sqrt{gA1^2 + gB1^2}} Z_{Go,i4}^* Z_{Po,j6}^* Z_{Ls,k2}^{od} \\
& - i\sqrt{2}g_{B2} \sqrt{\frac{gA2^2}{gA2^2 + gB2^2}} Z_{Go,i4}^* Z_{Po,j7}^* Z_{Ls,k2}^{od} - i\sqrt{2}g_{A2}g_{B2} \frac{1}{\sqrt{gA2^2 + gB2^2}} Z_{Go,i4}^* Z_{Po,j7}^* Z_{Ls,k2}^{od} \\
& + i\sqrt{2}g_{A2} \sqrt{\frac{gA2^2}{gA2^2 + gB2^2}} Z_{Go,i4}^* Z_{Po,j8}^* Z_{Ls,k2}^{od} - i\sqrt{2}g_{B2}^2 \frac{1}{\sqrt{gA2^2 + gB2^2}} Z_{Go,i4}^* Z_{Po,j8}^* Z_{Ls,k2}^{od} \\
& + i\sqrt{2} \frac{1}{\sqrt{gA2^2 + gB2^2}} Z_{Go,i6}^* \left( g_{B2}^2 Z_{Po,j1}^* Z_{Ls,k1}^{od} + g_{A2} \sqrt{\frac{gA2^2}{gA2^2 + gB2^2}} \sqrt{gA2^2 + gB2^2} Z_{Po,j3}^* Z_{Ls,k1}^{od} \right. \\
& \left. - \left( g_{A2} \sqrt{\frac{gA2^2}{gA2^2 + gB2^2}} \sqrt{gA2^2 + gB2^2} Z_{Po,j2}^* + g_{B2}^2 Z_{Po,j4}^* \right) Z_{Ls,k2}^{od} \right) \\
& + i\sqrt{2}g_{B2} \frac{1}{\sqrt{gA2^2 + gB2^2}} Z_{Go,i5}^* \left( \sqrt{\frac{gA2^2}{gA2^2 + gB2^2}} \sqrt{gA2^2 + gB2^2} Z_{Po,j1}^* Z_{Ls,k1}^{od} - g_{A2} Z_{Po,j3}^* Z_{Ls,k1}^{od} \right. \\
& \left. + \left( g_{A2} Z_{Po,j2}^* - \sqrt{\frac{gA2^2}{gA2^2 + gB2^2}} \sqrt{gA2^2 + gB2^2} Z_{Po,j4}^* \right) Z_{Ls,k2}^{od} \right) \\
& - 2iY_A Z_{Go,i9}^* Z_{Po,j1}^* Z_{Ls,k3}^{od} + i\sqrt{2}Y_A Z_{Go,i1}^* Z_{Po,j9}^* Z_{Ls,k3}^{od} - iY_K Z_{Go,i1}^* Z_{Po,j10}^* Z_{Ls,k3}^{od} \\
& - 2iY_A Z_{Go,i9}^* Z_{Po,j4}^* Z_{Ls,k4}^{od} - i\sqrt{2}Y_A Z_{Go,i4}^* Z_{Po,j9}^* Z_{Ls,k4}^{od} - iY_K Z_{Go,i4}^* Z_{Po,j10}^* Z_{Ls,k4}^{od} \Big) \left( \frac{1 - \gamma_5}{2} \right) \tag{800} \\
& + \frac{1}{2} \left( -\sqrt{2}g_{A2}g_{B2} \frac{1}{\sqrt{gA2^2 + gB2^2}} Z_{Go,i7}^* Z_{Ls,k4}^{od} Z_{Po,j1} + \sqrt{2}g_{A2} \sqrt{\frac{gA2^2}{gA2^2 + gB2^2}} Z_{Go,i8}^* Z_{Ls,k4}^{od} Z_{Po,j1} \right. \\
& - 2iY_A^* Z_{Go,i10}^* Z_{Ls,k1}^{od} Z_{Po,j2} - \sqrt{2}g_{B2} \sqrt{\frac{gA2^2}{gA2^2 + gB2^2}} Z_{Go,i7}^* Z_{Ls,k3}^{od} Z_{Po,j2} \\
& - \sqrt{2}g_{B2}^2 \frac{1}{\sqrt{gA2^2 + gB2^2}} Z_{Go,i8}^* Z_{Ls,k3}^{od} Z_{Po,j2} - 2iY_A^* Z_{Go,i10}^* Z_{Ls,k2}^{od} Z_{Po,j3} \\
& + \sqrt{2}g_{B2} \sqrt{\frac{gA2^2}{gA2^2 + gB2^2}} Z_{Go,i7}^* Z_{Ls,k4}^{od} Z_{Po,j3} + \sqrt{2}g_{B2}^2 \frac{1}{\sqrt{gA2^2 + gB2^2}} Z_{Go,i8}^* Z_{Ls,k4}^{od} Z_{Po,j3} \\
& \left. + \sqrt{2}g_{A2}g_{B2} \frac{1}{\sqrt{gA2^2 + gB2^2}} Z_{Go,i7}^* Z_{Ls,k3}^{od} Z_{Po,j4} - \sqrt{2}g_{A2} \sqrt{\frac{gA2^2}{gA2^2 + gB2^2}} Z_{Go,i8}^* Z_{Ls,k3}^{od} Z_{Po,j4} \right)
\end{aligned}$$

$$\begin{aligned}
& + i\sqrt{2}g_{B2}\frac{1}{\sqrt{gA2^2 + gB2^2}}Z_{Go,i5}\left(Z_{Ls,k4}^{od}\left(-g_{A2}Z_{Po,j1} + \sqrt{\frac{gA2^2}{gA2^2 + gB2^2}}\sqrt{gA2^2 + gB2^2}Z_{Po,j3}\right)\right. \\
& + Z_{Ls,k3}^{od}\left(g_{A2}Z_{Po,j4} - \sqrt{\frac{gA2^2}{gA2^2 + gB2^2}}\sqrt{gA2^2 + gB2^2}Z_{Po,j2}\right)\left.\right) \\
& + i\sqrt{2}\frac{1}{\sqrt{gA2^2 + gB2^2}}Z_{Go,i6}\left(Z_{Ls,k4}^{od}\left(g_{A2}\sqrt{\frac{gA2^2}{gA2^2 + gB2^2}}\sqrt{gA2^2 + gB2^2}Z_{Po,j1} + g_{B2}^2Z_{Po,j3}\right)\right. \\
& - Z_{Ls,k3}^{od}\left(g_{A2}\sqrt{\frac{gA2^2}{gA2^2 + gB2^2}}\sqrt{gA2^2 + gB2^2}Z_{Po,j4} + g_{B2}^2Z_{Po,j2}\right)\left.\right) \\
& + i\sqrt{2}g_{B1}\sqrt{\frac{gA1^2}{gA1^2 + gB1^2}}Z_{Go,i2}Z_{Ls,k3}^{od}Z_{Po,j5} - i\sqrt{2}g_{A1}g_{B1}\frac{1}{\sqrt{gA1^2 + gB1^2}}Z_{Go,i2}Z_{Ls,k3}^{od}Z_{Po,j5} \\
& - i\sqrt{2}g_{B1}\sqrt{\frac{gA1^2}{gA1^2 + gB1^2}}Z_{Go,i3}Z_{Ls,k4}^{od}Z_{Po,j5} + i\sqrt{2}g_{A1}g_{B1}\frac{1}{\sqrt{gA1^2 + gB1^2}}Z_{Go,i3}Z_{Ls,k4}^{od}Z_{Po,j5} \\
& + i\sqrt{2}g_{A1}\sqrt{\frac{gA1^2}{gA1^2 + gB1^2}}Z_{Go,i2}Z_{Ls,k3}^{od}Z_{Po,j6} + i\sqrt{2}g_{B1}^2\frac{1}{\sqrt{gA1^2 + gB1^2}}Z_{Go,i2}Z_{Ls,k3}^{od}Z_{Po,j6} \\
& - i\sqrt{2}g_{A1}\sqrt{\frac{gA1^2}{gA1^2 + gB1^2}}Z_{Go,i3}Z_{Ls,k4}^{od}Z_{Po,j6} - i\sqrt{2}g_{B1}^2\frac{1}{\sqrt{gA1^2 + gB1^2}}Z_{Go,i3}Z_{Ls,k4}^{od}Z_{Po,j6} \\
& + i\sqrt{2}g_{B2}\sqrt{\frac{gA2^2}{gA2^2 + gB2^2}}Z_{Go,i2}Z_{Ls,k3}^{od}Z_{Po,j7} + i\sqrt{2}g_{A2}g_{B2}\frac{1}{\sqrt{gA2^2 + gB2^2}}Z_{Go,i2}Z_{Ls,k3}^{od}Z_{Po,j7} \\
& + i\sqrt{2}g_{B2}\sqrt{\frac{gA2^2}{gA2^2 + gB2^2}}Z_{Go,i3}Z_{Ls,k4}^{od}Z_{Po,j7} + i\sqrt{2}g_{A2}g_{B2}\frac{1}{\sqrt{gA2^2 + gB2^2}}Z_{Go,i3}Z_{Ls,k4}^{od}Z_{Po,j7} \\
& - i\sqrt{2}g_{A2}\sqrt{\frac{gA2^2}{gA2^2 + gB2^2}}Z_{Go,i2}Z_{Ls,k3}^{od}Z_{Po,j8} + i\sqrt{2}g_{B2}^2\frac{1}{\sqrt{gA2^2 + gB2^2}}Z_{Go,i2}Z_{Ls,k3}^{od}Z_{Po,j8} \\
& - i\sqrt{2}g_{A2}\sqrt{\frac{gA2^2}{gA2^2 + gB2^2}}Z_{Go,i3}Z_{Ls,k4}^{od}Z_{Po,j8} + i\sqrt{2}g_{B2}^2\frac{1}{\sqrt{gA2^2 + gB2^2}}Z_{Go,i3}Z_{Ls,k4}^{od}Z_{Po,j8} \\
& + i\sqrt{2}Y_A^*Z_{Go,i2}Z_{Ls,k1}^{od}Z_{Po,j9} - i\sqrt{2}Y_A^*Z_{Go,i3}Z_{Ls,k2}^{od}Z_{Po,j9} - iY_K^*Z_{Go,i2}Z_{Ls,k1}^{od}Z_{Po,j10} \\
& - iY_K^*Z_{Go,i3}Z_{Ls,k2}^{od}Z_{Po,j10}\left)\left(\frac{1+\gamma_5}{2}\right)
\end{aligned} \tag{801}$$


---

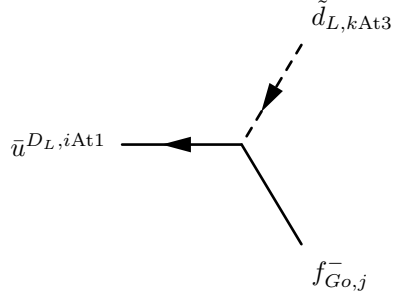

(802)

$$\begin{aligned}
& + \frac{1}{\sqrt{2}} g_{A2} \frac{1}{\sqrt{g_{A2}^2 + g_{B2}^2}} \delta_{\text{At}1\text{At}3} \delta_{ik} \left( -ig_{B2} Z_{Go,j5} + i \sqrt{\frac{g_{A2}^2}{g_{A2}^2 + g_{B2}^2}} \sqrt{g_{A2}^2 + g_{B2}^2} Z_{Go,j6} - g_{B2} Z_{Go,j7} \right. \\
& \left. + \sqrt{\frac{g_{A2}^2}{g_{A2}^2 + g_{B2}^2}} \sqrt{g_{A2}^2 + g_{B2}^2} Z_{Go,j8} \right) \left( \frac{1 + \gamma_5}{2} \right)
\end{aligned}
\tag{803}$$


---

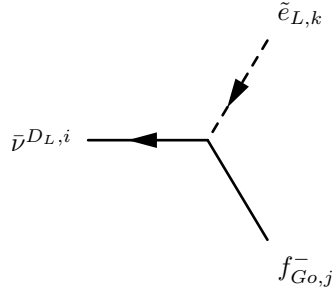

(804)

$$\begin{aligned}
& + \frac{1}{\sqrt{2}} g_{A2} \frac{1}{\sqrt{g_{A2}^2 + g_{B2}^2}} \delta_{ik} \left( -ig_{B2} Z_{Go,j5} + i \sqrt{\frac{g_{A2}^2}{g_{A2}^2 + g_{B2}^2}} \sqrt{g_{A2}^2 + g_{B2}^2} Z_{Go,j6} - g_{B2} Z_{Go,j7} \right. \\
& \left. + \sqrt{\frac{g_{A2}^2}{g_{A2}^2 + g_{B2}^2}} \sqrt{g_{A2}^2 + g_{B2}^2} Z_{Go,j8} \right) \left( \frac{1 + \gamma_5}{2} \right)
\end{aligned}
\tag{805}$$


---

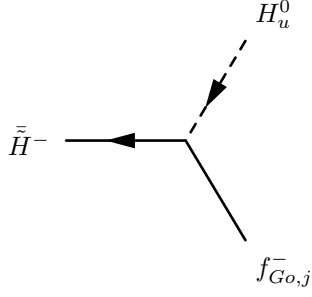

(806)

$$\begin{aligned}
& + \frac{1}{\sqrt{2}} g_{A2} \frac{1}{\sqrt{g_{A2}^2 + g_{B2}^2}} \left( -ig_{B2} Z_{Go,j5} + i \sqrt{\frac{g_{A2}^2}{g_{A2}^2 + g_{B2}^2}} \sqrt{g_{A2}^2 + g_{B2}^2} Z_{Go,j6} - g_{B2} Z_{Go,j7} \right. \\
& \left. + \sqrt{\frac{g_{A2}^2}{g_{A2}^2 + g_{B2}^2}} \sqrt{g_{A2}^2 + g_{B2}^2} Z_{Go,j8} \right) \left( \frac{1 + \gamma_5}{2} \right)
\end{aligned}$$

(807)

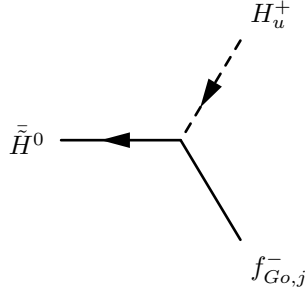

(808)

$$\begin{aligned}
& + \frac{1}{\sqrt{2}} g_{A2} \frac{1}{\sqrt{g_{A2}^2 + g_{B2}^2}} \left( -ig_{B2} Z_{Go,j5} + i \sqrt{\frac{g_{A2}^2}{g_{A2}^2 + g_{B2}^2}} \sqrt{g_{A2}^2 + g_{B2}^2} Z_{Go,j6} + g_{B2} Z_{Go,j7} \right. \\
& \left. - \sqrt{\frac{g_{A2}^2}{g_{A2}^2 + g_{B2}^2}} \sqrt{g_{A2}^2 + g_{B2}^2} Z_{Go,j8} \right) \left( \frac{1 + \gamma_5}{2} \right)
\end{aligned}$$

(809)

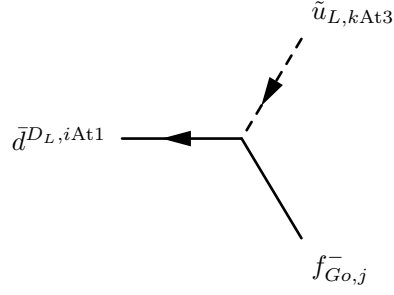

(810)

$$\begin{aligned}
& + \frac{1}{\sqrt{2}} g_{A2} \frac{1}{\sqrt{g_{A2}^2 + g_{B2}^2}} \delta_{\text{At}1\text{At}3} \delta_{ik} \left( -ig_{B2} Z_{Go, j5} + i \sqrt{\frac{g_{A2}^2}{g_{A2}^2 + g_{B2}^2}} \sqrt{g_{A2}^2 + g_{B2}^2} Z_{Go, j6} + g_{B2} Z_{Go, j7} \right. \\
& \left. - \sqrt{\frac{g_{A2}^2}{g_{A2}^2 + g_{B2}^2}} \sqrt{g_{A2}^2 + g_{B2}^2} Z_{Go, j8} \right) \left( \frac{1 + \gamma_5}{2} \right)
\end{aligned} \tag{811}$$


---

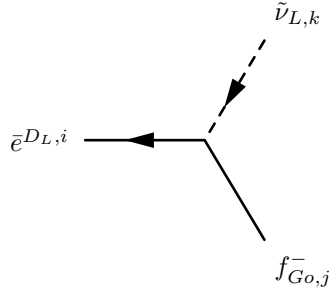

(812)

$$\begin{aligned}
& + \frac{1}{\sqrt{2}} g_{A2} \frac{1}{\sqrt{g_{A2}^2 + g_{B2}^2}} \delta_{ik} \left( -ig_{B2} Z_{Go, j5} + i \sqrt{\frac{g_{A2}^2}{g_{A2}^2 + g_{B2}^2}} \sqrt{g_{A2}^2 + g_{B2}^2} Z_{Go, j6} + g_{B2} Z_{Go, j7} \right. \\
& \left. - \sqrt{\frac{g_{A2}^2}{g_{A2}^2 + g_{B2}^2}} \sqrt{g_{A2}^2 + g_{B2}^2} Z_{Go, j8} \right) \left( \frac{1 + \gamma_5}{2} \right)
\end{aligned} \tag{813}$$


---

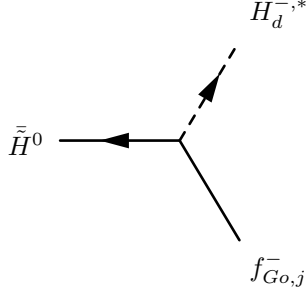

$$\begin{aligned} & \frac{1}{\sqrt{2}} g_{A2} \frac{1}{\sqrt{g_{A2}^2 + g_{B2}^2}} \left( -ig_{B2} Z_{Go,j5}^* + i \sqrt{\frac{g_{A2}^2}{g_{A2}^2 + g_{B2}^2}} \sqrt{g_{A2}^2 + g_{B2}^2} Z_{Go,j6}^* + g_{B2} Z_{Go,j7}^* \right. \\ & \left. - \sqrt{\frac{g_{A2}^2}{g_{A2}^2 + g_{B2}^2}} \sqrt{g_{A2}^2 + g_{B2}^2} Z_{Go,j8}^* \right) \left( \frac{1 - \gamma_5}{2} \right) \end{aligned} \quad (814)$$


---

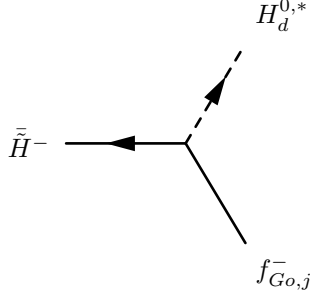

$$\begin{aligned} & \frac{1}{\sqrt{2}} g_{A2} \frac{1}{\sqrt{g_{A2}^2 + g_{B2}^2}} \left( -ig_{B2} Z_{Go,j5}^* + i \sqrt{\frac{g_{A2}^2}{g_{A2}^2 + g_{B2}^2}} \sqrt{g_{A2}^2 + g_{B2}^2} Z_{Go,j6}^* - g_{B2} Z_{Go,j7}^* \right. \\ & \left. + \sqrt{\frac{g_{A2}^2}{g_{A2}^2 + g_{B2}^2}} \sqrt{g_{A2}^2 + g_{B2}^2} Z_{Go,j8}^* \right) \left( \frac{1 - \gamma_5}{2} \right) \end{aligned} \quad (815)$$


---

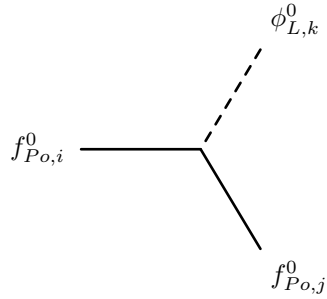

$$\begin{aligned}
& -\frac{i}{2} \left( \sqrt{2} g_{B1} \sqrt{\frac{gA1^2}{gA1^2 + gB1^2}} Z_{Ls,k3}^{DR,*} Z_{Po,i5}^* Z_{Po,j3}^* - \sqrt{2} g_{A1} g_{B1} \frac{1}{\sqrt{gA1^2 + gB1^2}} Z_{Ls,k3}^{DR,*} Z_{Po,i5}^* Z_{Po,j3}^* \right. \\
& + \sqrt{2} g_{A1} \sqrt{\frac{gA1^2}{gA1^2 + gB1^2}} Z_{Ls,k3}^{DR,*} Z_{Po,i6}^* Z_{Po,j3}^* + \sqrt{2} g_{B1}^2 \frac{1}{\sqrt{gA1^2 + gB1^2}} Z_{Ls,k3}^{DR,*} Z_{Po,i6}^* Z_{Po,j3}^* \\
& + \sqrt{2} g_{B2} \sqrt{\frac{gA2^2}{gA2^2 + gB2^2}} Z_{Ls,k3}^{DR,*} Z_{Po,i7}^* Z_{Po,j3}^* - \sqrt{2} g_{A2} g_{B2} \frac{1}{\sqrt{gA2^2 + gB2^2}} Z_{Ls,k3}^{DR,*} Z_{Po,i7}^* Z_{Po,j3}^* \\
& + \sqrt{2} g_{A2} \sqrt{\frac{gA2^2}{gA2^2 + gB2^2}} Z_{Ls,k3}^{DR,*} Z_{Po,i8}^* Z_{Po,j3}^* + \sqrt{2} g_{B2}^2 \frac{1}{\sqrt{gA2^2 + gB2^2}} Z_{Ls,k3}^{DR,*} Z_{Po,i8}^* Z_{Po,j3}^* \\
& - \sqrt{2} Y_A Z_{Ls,k4}^{DR,*} Z_{Po,i9}^* Z_{Po,j3}^* + Y_K Z_{Ls,k4}^{DR,*} Z_{Po,i10}^* Z_{Po,j3}^* \\
& - \sqrt{2} g_{B1} \sqrt{\frac{gA1^2}{gA1^2 + gB1^2}} Z_{Ls,k4}^{DR,*} Z_{Po,i5}^* Z_{Po,j4}^* + \sqrt{2} g_{A1} g_{B1} \frac{1}{\sqrt{gA1^2 + gB1^2}} Z_{Ls,k4}^{DR,*} Z_{Po,i5}^* Z_{Po,j4}^* \\
& - \sqrt{2} g_{A1} \sqrt{\frac{gA1^2}{gA1^2 + gB1^2}} Z_{Ls,k4}^{DR,*} Z_{Po,i6}^* Z_{Po,j4}^* - \sqrt{2} g_{B1}^2 \frac{1}{\sqrt{gA1^2 + gB1^2}} Z_{Ls,k4}^{DR,*} Z_{Po,i6}^* Z_{Po,j4}^* \\
& - \sqrt{2} g_{B2} \sqrt{\frac{gA2^2}{gA2^2 + gB2^2}} Z_{Ls,k4}^{DR,*} Z_{Po,i7}^* Z_{Po,j4}^* + \sqrt{2} g_{A2} g_{B2} \frac{1}{\sqrt{gA2^2 + gB2^2}} Z_{Ls,k4}^{DR,*} Z_{Po,i7}^* Z_{Po,j4}^* \\
& - \sqrt{2} g_{A2} \sqrt{\frac{gA2^2}{gA2^2 + gB2^2}} Z_{Ls,k4}^{DR,*} Z_{Po,i8}^* Z_{Po,j4}^* - \sqrt{2} g_{B2}^2 \frac{1}{\sqrt{gA2^2 + gB2^2}} Z_{Ls,k4}^{DR,*} Z_{Po,i8}^* Z_{Po,j4}^* \\
& - \sqrt{2} Y_A Z_{Ls,k3}^{DR,*} Z_{Po,i9}^* Z_{Po,j4}^* + Y_K Z_{Ls,k3}^{DR,*} Z_{Po,i10}^* Z_{Po,j4}^* \\
& + \sqrt{2} g_{B1} \sqrt{\frac{gA1^2}{gA1^2 + gB1^2}} Z_{Ls,k3}^{DR,*} Z_{Po,i3}^* Z_{Po,j5}^* - \sqrt{2} g_{A1} g_{B1} \frac{1}{\sqrt{gA1^2 + gB1^2}} Z_{Ls,k3}^{DR,*} Z_{Po,i3}^* Z_{Po,j5}^* \\
& - \sqrt{2} g_{B1} \sqrt{\frac{gA1^2}{gA1^2 + gB1^2}} Z_{Ls,k4}^{DR,*} Z_{Po,i4}^* Z_{Po,j5}^* + \sqrt{2} g_{A1} g_{B1} \frac{1}{\sqrt{gA1^2 + gB1^2}} Z_{Ls,k4}^{DR,*} Z_{Po,i4}^* Z_{Po,j5}^* \\
& + \sqrt{2} g_{A1} \sqrt{\frac{gA1^2}{gA1^2 + gB1^2}} Z_{Ls,k3}^{DR,*} Z_{Po,i3}^* Z_{Po,j6}^* + \sqrt{2} g_{B1}^2 \frac{1}{\sqrt{gA1^2 + gB1^2}} Z_{Ls,k3}^{DR,*} Z_{Po,i3}^* Z_{Po,j6}^* \\
& - \sqrt{2} g_{A1} \sqrt{\frac{gA1^2}{gA1^2 + gB1^2}} Z_{Ls,k4}^{DR,*} Z_{Po,i4}^* Z_{Po,j6}^* - \sqrt{2} g_{B1}^2 \frac{1}{\sqrt{gA1^2 + gB1^2}} Z_{Ls,k4}^{DR,*} Z_{Po,i4}^* Z_{Po,j6}^* \\
& + \sqrt{2} g_{B2} \sqrt{\frac{gA2^2}{gA2^2 + gB2^2}} Z_{Ls,k3}^{DR,*} Z_{Po,i3}^* Z_{Po,j7}^* - \sqrt{2} g_{A2} g_{B2} \frac{1}{\sqrt{gA2^2 + gB2^2}} Z_{Ls,k3}^{DR,*} Z_{Po,i3}^* Z_{Po,j7}^* \\
& - \sqrt{2} g_{B2} \sqrt{\frac{gA2^2}{gA2^2 + gB2^2}} Z_{Ls,k4}^{DR,*} Z_{Po,i4}^* Z_{Po,j7}^* + \sqrt{2} g_{A2} g_{B2} \frac{1}{\sqrt{gA2^2 + gB2^2}} Z_{Ls,k4}^{DR,*} Z_{Po,i4}^* Z_{Po,j7}^* \\
& + \sqrt{2} g_{A2} \sqrt{\frac{gA2^2}{gA2^2 + gB2^2}} Z_{Ls,k3}^{DR,*} Z_{Po,i3}^* Z_{Po,j8}^* + \sqrt{2} g_{B2}^2 \frac{1}{\sqrt{gA2^2 + gB2^2}} Z_{Ls,k3}^{DR,*} Z_{Po,i3}^* Z_{Po,j8}^*
\end{aligned}$$

$$\begin{aligned}
& -\sqrt{2}g_{A2}\sqrt{\frac{gA2^2}{gA2^2+gB2^2}}Z_{Ls,k4}^{DR,*}Z_{Po,i4}^*Z_{Po,j8}^* - \sqrt{2}g_{B2}^2\frac{1}{\sqrt{gA2^2+gB2^2}}Z_{Ls,k4}^{DR,*}Z_{Po,i4}^*Z_{Po,j8}^* \\
& -\sqrt{2}Y_AZ_{Ls,k4}^{DR,*}Z_{Po,i3}^*Z_{Po,j9}^* - \sqrt{2}Y_AZ_{Ls,k3}^{DR,*}Z_{Po,i4}^*Z_{Po,j9}^* + Y_KZ_{Ls,k4}^{DR,*}Z_{Po,i3}^*Z_{Po,j10}^* \\
& + Y_KZ_{Ls,k3}^{DR,*}Z_{Po,i4}^*Z_{Po,j10}^* \\
& + Z_{Ls,k2}^{DR,*}\left(\sqrt{2}Y_AZ_{Po,i9}^*Z_{Po,j1}^* + Y_KZ_{Po,i10}^*Z_{Po,j1}^* - \sqrt{2}g_{B1}\sqrt{\frac{gA1^2}{gA1^2+gB1^2}}Z_{Po,i5}^*Z_{Po,j2}^* \right. \\
& + \sqrt{2}g_{A1}g_{B1}\frac{1}{\sqrt{gA1^2+gB1^2}}Z_{Po,i5}^*Z_{Po,j2}^* - \sqrt{2}g_{A1}\sqrt{\frac{gA1^2}{gA1^2+gB1^2}}Z_{Po,i6}^*Z_{Po,j2}^* \\
& - \sqrt{2}g_{B1}^2\frac{1}{\sqrt{gA1^2+gB1^2}}Z_{Po,i6}^*Z_{Po,j2}^* + \sqrt{2}g_{B2}\sqrt{\frac{gA2^2}{gA2^2+gB2^2}}Z_{Po,i7}^*Z_{Po,j2}^* \\
& - \sqrt{2}g_{A2}g_{B2}\frac{1}{\sqrt{gA2^2+gB2^2}}Z_{Po,i7}^*Z_{Po,j2}^* + \sqrt{2}g_{A2}\sqrt{\frac{gA2^2}{gA2^2+gB2^2}}Z_{Po,i8}^*Z_{Po,j2}^* \\
& + \sqrt{2}g_{B2}^2\frac{1}{\sqrt{gA2^2+gB2^2}}Z_{Po,i8}^*Z_{Po,j2}^* - \sqrt{2}g_{B1}\sqrt{\frac{gA1^2}{gA1^2+gB1^2}}Z_{Po,i2}^*Z_{Po,j5}^* \\
& + \sqrt{2}g_{A1}g_{B1}\frac{1}{\sqrt{gA1^2+gB1^2}}Z_{Po,i2}^*Z_{Po,j5}^* - \sqrt{2}g_{A1}\sqrt{\frac{gA1^2}{gA1^2+gB1^2}}Z_{Po,i2}^*Z_{Po,j6}^* \\
& - \sqrt{2}g_{B1}^2\frac{1}{\sqrt{gA1^2+gB1^2}}Z_{Po,i2}^*Z_{Po,j6}^* + \sqrt{2}g_{B2}\sqrt{\frac{gA2^2}{gA2^2+gB2^2}}Z_{Po,i2}^*Z_{Po,j7}^* \\
& - \sqrt{2}g_{A2}g_{B2}\frac{1}{\sqrt{gA2^2+gB2^2}}Z_{Po,i2}^*Z_{Po,j7}^* + \sqrt{2}g_{A2}\sqrt{\frac{gA2^2}{gA2^2+gB2^2}}Z_{Po,i2}^*Z_{Po,j8}^* \\
& + \sqrt{2}g_{B2}^2\frac{1}{\sqrt{gA2^2+gB2^2}}Z_{Po,i2}^*Z_{Po,j8}^* + \sqrt{2}Y_AZ_{Po,i1}^*Z_{Po,j9}^* + Y_KZ_{Po,i1}^*Z_{Po,j10}^*) \\
& + Z_{Ls,k1}^{DR,*}\left(\sqrt{2}g_{B1}\left(-g_{A1}\frac{1}{\sqrt{gA1^2+gB1^2}} + \sqrt{\frac{gA1^2}{gA1^2+gB1^2}}\right)Z_{Po,i5}^*Z_{Po,j1}^* \right. \\
& + \sqrt{2}\left(g_{A1}\sqrt{\frac{gA1^2}{gA1^2+gB1^2}} + g_{B1}^2\frac{1}{\sqrt{gA1^2+gB1^2}}\right)Z_{Po,i6}^*Z_{Po,j1}^* \\
& - \sqrt{2}g_{B2}\sqrt{\frac{gA2^2}{gA2^2+gB2^2}}Z_{Po,i7}^*Z_{Po,j1}^* + \sqrt{2}g_{A2}g_{B2}\frac{1}{\sqrt{gA2^2+gB2^2}}Z_{Po,i7}^*Z_{Po,j1}^* \\
& - \sqrt{2}g_{A2}\sqrt{\frac{gA2^2}{gA2^2+gB2^2}}Z_{Po,i8}^*Z_{Po,j1}^* - \sqrt{2}g_{B2}^2\frac{1}{\sqrt{gA2^2+gB2^2}}Z_{Po,i8}^*Z_{Po,j1}^* \\
& \left. + \sqrt{2}Y_AZ_{Po,i9}^*Z_{Po,j2}^* + Y_KZ_{Po,i10}^*Z_{Po,j2}^* + \sqrt{2}g_{B1}\sqrt{\frac{gA1^2}{gA1^2+gB1^2}}Z_{Po,i1}^*Z_{Po,j5}^*\right)
\end{aligned}$$



$$\begin{aligned}
& -\sqrt{2}g_{A1}g_{B1}\frac{1}{\sqrt{gA1^2+gB1^2}}Z_{Po,i1}^*Z_{Po,j5}^*+\sqrt{2}g_{A1}\sqrt{\frac{gA1^2}{gA1^2+gB1^2}}Z_{Po,i1}^*Z_{Po,j6}^* \\
& +\sqrt{2}g_{B1}^2\frac{1}{\sqrt{gA1^2+gB1^2}}Z_{Po,i1}^*Z_{Po,j6}^*-\sqrt{2}g_{B2}\sqrt{\frac{gA2^2}{gA2^2+gB2^2}}Z_{Po,i1}^*Z_{Po,j7}^* \\
& +\sqrt{2}g_{A2}g_{B2}\frac{1}{\sqrt{gA2^2+gB2^2}}Z_{Po,i1}^*Z_{Po,j7}^*-\sqrt{2}g_{A2}\sqrt{\frac{gA2^2}{gA2^2+gB2^2}}Z_{Po,i1}^*Z_{Po,j8}^* \\
& -\sqrt{2}g_{B2}^2\frac{1}{\sqrt{gA2^2+gB2^2}}Z_{Po,i1}^*Z_{Po,j8}^*+\sqrt{2}Y_AZ_{Po,i2}^*Z_{Po,j9}^*+Y_KZ_{Po,i2}^*Z_{Po,j10}^*)\left(\frac{1-\gamma_5}{2}\right) \\
& +\frac{i}{2}\left(Y_K^*Z_{Ls,k2}^{DR,*}Z_{Po,i10}Z_{Po,j1}-\sqrt{2}g_{B1}\sqrt{\frac{gA1^2}{gA1^2+gB1^2}}Z_{Ls,k2}^{DR,*}Z_{Po,i5}Z_{Po,j2}\right. \\
& +\sqrt{2}g_{A1}g_{B1}\frac{1}{\sqrt{gA1^2+gB1^2}}Z_{Ls,k2}^{DR,*}Z_{Po,i5}Z_{Po,j2}-\sqrt{2}g_{A1}\sqrt{\frac{gA1^2}{gA1^2+gB1^2}}Z_{Ls,k2}^{DR,*}Z_{Po,i6}Z_{Po,j2} \\
& -\sqrt{2}g_{B1}^2\frac{1}{\sqrt{gA1^2+gB1^2}}Z_{Ls,k2}^{DR,*}Z_{Po,i6}Z_{Po,j2}+\sqrt{2}g_{B2}\sqrt{\frac{gA2^2}{gA2^2+gB2^2}}Z_{Ls,k2}^{DR,*}Z_{Po,i7}Z_{Po,j2} \\
& -\sqrt{2}g_{A2}g_{B2}\frac{1}{\sqrt{gA2^2+gB2^2}}Z_{Ls,k2}^{DR,*}Z_{Po,i7}Z_{Po,j2}+\sqrt{2}g_{A2}\sqrt{\frac{gA2^2}{gA2^2+gB2^2}}Z_{Ls,k2}^{DR,*}Z_{Po,i8}Z_{Po,j2} \\
& +\sqrt{2}g_{B2}^2\frac{1}{\sqrt{gA2^2+gB2^2}}Z_{Ls,k2}^{DR,*}Z_{Po,i8}Z_{Po,j2}+\sqrt{2}g_{B1}\sqrt{\frac{gA1^2}{gA1^2+gB1^2}}Z_{Ls,k3}^{DR,*}Z_{Po,i5}Z_{Po,j3} \\
& -\sqrt{2}g_{A1}g_{B1}\frac{1}{\sqrt{gA1^2+gB1^2}}Z_{Ls,k3}^{DR,*}Z_{Po,i5}Z_{Po,j3}+\sqrt{2}g_{A1}\sqrt{\frac{gA1^2}{gA1^2+gB1^2}}Z_{Ls,k3}^{DR,*}Z_{Po,i6}Z_{Po,j3} \\
& +\sqrt{2}g_{B1}^2\frac{1}{\sqrt{gA1^2+gB1^2}}Z_{Ls,k3}^{DR,*}Z_{Po,i6}Z_{Po,j3}+\sqrt{2}g_{B2}\sqrt{\frac{gA2^2}{gA2^2+gB2^2}}Z_{Ls,k3}^{DR,*}Z_{Po,i7}Z_{Po,j3} \\
& -\sqrt{2}g_{A2}g_{B2}\frac{1}{\sqrt{gA2^2+gB2^2}}Z_{Ls,k3}^{DR,*}Z_{Po,i7}Z_{Po,j3}+\sqrt{2}g_{A2}\sqrt{\frac{gA2^2}{gA2^2+gB2^2}}Z_{Ls,k3}^{DR,*}Z_{Po,i8}Z_{Po,j3} \\
& +\sqrt{2}g_{B2}^2\frac{1}{\sqrt{gA2^2+gB2^2}}Z_{Ls,k3}^{DR,*}Z_{Po,i8}Z_{Po,j3}+Y_K^*Z_{Ls,k4}^{DR,*}Z_{Po,i10}Z_{Po,j3} \\
& -\sqrt{2}g_{B1}\sqrt{\frac{gA1^2}{gA1^2+gB1^2}}Z_{Ls,k4}^{DR,*}Z_{Po,i5}Z_{Po,j4}+\sqrt{2}g_{A1}g_{B1}\frac{1}{\sqrt{gA1^2+gB1^2}}Z_{Ls,k4}^{DR,*}Z_{Po,i5}Z_{Po,j4} \\
& -\sqrt{2}g_{A1}\sqrt{\frac{gA1^2}{gA1^2+gB1^2}}Z_{Ls,k4}^{DR,*}Z_{Po,i6}Z_{Po,j4}-\sqrt{2}g_{B1}^2\frac{1}{\sqrt{gA1^2+gB1^2}}Z_{Ls,k4}^{DR,*}Z_{Po,i6}Z_{Po,j4} \\
& -\sqrt{2}g_{B2}\sqrt{\frac{gA2^2}{gA2^2+gB2^2}}Z_{Ls,k4}^{DR,*}Z_{Po,i7}Z_{Po,j4}+\sqrt{2}g_{A2}g_{B2}\frac{1}{\sqrt{gA2^2+gB2^2}}Z_{Ls,k4}^{DR,*}Z_{Po,i7}Z_{Po,j4}
\end{aligned} \tag{816}$$

$$\begin{aligned}
& -\sqrt{2}g_{A2}\sqrt{\frac{gA2^2}{gA2^2+gB2^2}}Z_{Ls,k4}^{DR,*}Z_{Po,i8}Z_{Po,j4}-\sqrt{2}g_{B2}^2\frac{1}{\sqrt{gA2^2+gB2^2}}Z_{Ls,k4}^{DR,*}Z_{Po,i8}Z_{Po,j4} \\
& +Y_K^*Z_{Ls,k3}^{DR,*}Z_{Po,i10}Z_{Po,j4}-\sqrt{2}g_{B1}\sqrt{\frac{gA1^2}{gA1^2+gB1^2}}Z_{Ls,k2}^{DR,*}Z_{Po,i2}Z_{Po,j5} \\
& +\sqrt{2}g_{A1}g_{B1}\frac{1}{\sqrt{gA1^2+gB1^2}}Z_{Ls,k2}^{DR,*}Z_{Po,i2}Z_{Po,j5}+\sqrt{2}g_{B1}\sqrt{\frac{gA1^2}{gA1^2+gB1^2}}Z_{Ls,k3}^{DR,*}Z_{Po,i3}Z_{Po,j5} \\
& -\sqrt{2}g_{A1}g_{B1}\frac{1}{\sqrt{gA1^2+gB1^2}}Z_{Ls,k3}^{DR,*}Z_{Po,i3}Z_{Po,j5}-\sqrt{2}g_{B1}\sqrt{\frac{gA1^2}{gA1^2+gB1^2}}Z_{Ls,k4}^{DR,*}Z_{Po,i4}Z_{Po,j5} \\
& +\sqrt{2}g_{A1}g_{B1}\frac{1}{\sqrt{gA1^2+gB1^2}}Z_{Ls,k4}^{DR,*}Z_{Po,i4}Z_{Po,j5}-\sqrt{2}g_{A1}\sqrt{\frac{gA1^2}{gA1^2+gB1^2}}Z_{Ls,k2}^{DR,*}Z_{Po,i2}Z_{Po,j6} \\
& -\sqrt{2}g_{B1}^2\frac{1}{\sqrt{gA1^2+gB1^2}}Z_{Ls,k2}^{DR,*}Z_{Po,i2}Z_{Po,j6}+\sqrt{2}g_{A1}\sqrt{\frac{gA1^2}{gA1^2+gB1^2}}Z_{Ls,k3}^{DR,*}Z_{Po,i3}Z_{Po,j6} \\
& +\sqrt{2}g_{B1}^2\frac{1}{\sqrt{gA1^2+gB1^2}}Z_{Ls,k3}^{DR,*}Z_{Po,i3}Z_{Po,j6}-\sqrt{2}g_{A1}\sqrt{\frac{gA1^2}{gA1^2+gB1^2}}Z_{Ls,k4}^{DR,*}Z_{Po,i4}Z_{Po,j6} \\
& -\sqrt{2}g_{B1}^2\frac{1}{\sqrt{gA1^2+gB1^2}}Z_{Ls,k4}^{DR,*}Z_{Po,i4}Z_{Po,j6}+\sqrt{2}g_{B2}\sqrt{\frac{gA2^2}{gA2^2+gB2^2}}Z_{Ls,k2}^{DR,*}Z_{Po,i2}Z_{Po,j7} \\
& -\sqrt{2}g_{A2}g_{B2}\frac{1}{\sqrt{gA2^2+gB2^2}}Z_{Ls,k2}^{DR,*}Z_{Po,i2}Z_{Po,j7}+\sqrt{2}g_{B2}\sqrt{\frac{gA2^2}{gA2^2+gB2^2}}Z_{Ls,k3}^{DR,*}Z_{Po,i3}Z_{Po,j7} \\
& -\sqrt{2}g_{A2}g_{B2}\frac{1}{\sqrt{gA2^2+gB2^2}}Z_{Ls,k3}^{DR,*}Z_{Po,i3}Z_{Po,j7}-\sqrt{2}g_{B2}\sqrt{\frac{gA2^2}{gA2^2+gB2^2}}Z_{Ls,k4}^{DR,*}Z_{Po,i4}Z_{Po,j7} \\
& +\sqrt{2}g_{A2}g_{B2}\frac{1}{\sqrt{gA2^2+gB2^2}}Z_{Ls,k4}^{DR,*}Z_{Po,i4}Z_{Po,j7}+\sqrt{2}g_{A2}\sqrt{\frac{gA2^2}{gA2^2+gB2^2}}Z_{Ls,k2}^{DR,*}Z_{Po,i2}Z_{Po,j8} \\
& +\sqrt{2}g_{B2}^2\frac{1}{\sqrt{gA2^2+gB2^2}}Z_{Ls,k2}^{DR,*}Z_{Po,i2}Z_{Po,j8}+\sqrt{2}g_{A2}\sqrt{\frac{gA2^2}{gA2^2+gB2^2}}Z_{Ls,k3}^{DR,*}Z_{Po,i3}Z_{Po,j8} \\
& +\sqrt{2}g_{B2}^2\frac{1}{\sqrt{gA2^2+gB2^2}}Z_{Ls,k3}^{DR,*}Z_{Po,i3}Z_{Po,j8}-\sqrt{2}g_{A2}\sqrt{\frac{gA2^2}{gA2^2+gB2^2}}Z_{Ls,k4}^{DR,*}Z_{Po,i4}Z_{Po,j8} \\
& -\sqrt{2}g_{B2}^2\frac{1}{\sqrt{gA2^2+gB2^2}}Z_{Ls,k4}^{DR,*}Z_{Po,i4}Z_{Po,j8} \\
& -\sqrt{2}Y_A^*\left(-Z_{Ls,k2}^{DR,*}\left(Z_{Po,i1}Z_{Po,j9}+Z_{Po,i9}Z_{Po,j1}\right)+Z_{Ls,k3}^{DR,*}\left(Z_{Po,i4}Z_{Po,j9}+Z_{Po,i9}Z_{Po,j4}\right)+Z_{Ls,k4}^{DR,*}\left(Z_{Po,i3}Z_{Po,j9}+Z_{Po,i9}Z_{Po,j3}\right)\right) \\
& +Y_K^*Z_{Ls,k2}^{DR,*}Z_{Po,i1}Z_{Po,j10}+Y_K^*Z_{Ls,k3}^{DR,*}Z_{Po,i3}Z_{Po,j10}+Y_K^*Z_{Ls,k4}^{DR,*}Z_{Po,i4}Z_{Po,j10} \\
& +Z_{Ls,k1}^{DR,*}\left(\sqrt{2}g_{B1}\left(-g_{A1}\frac{1}{\sqrt{gA1^2+gB1^2}}+\sqrt{\frac{gA1^2}{gA1^2+gB1^2}}\right)Z_{Po,i5}Z_{Po,j1}\right)
\end{aligned}$$

$$\begin{aligned}
& + \sqrt{2} \left( g_{A1} \sqrt{\frac{gA1^2}{gA1^2 + gB1^2}} + g_{B1}^2 \frac{1}{\sqrt{gA1^2 + gB1^2}} \right) Z_{Po,i6} Z_{Po,j1} \\
& - \sqrt{2} g_{B2} \sqrt{\frac{gA2^2}{gA2^2 + gB2^2}} Z_{Po,i7} Z_{Po,j1} + \sqrt{2} g_{A2} g_{B2} \frac{1}{\sqrt{gA2^2 + gB2^2}} Z_{Po,i7} Z_{Po,j1} \\
& - \sqrt{2} g_{A2} \sqrt{\frac{gA2^2}{gA2^2 + gB2^2}} Z_{Po,i8} Z_{Po,j1} - \sqrt{2} g_{B2}^2 \frac{1}{\sqrt{gA2^2 + gB2^2}} Z_{Po,i8} Z_{Po,j1} + \sqrt{2} Y_A^* Z_{Po,i9} Z_{Po,j2} \\
& + Y_K^* Z_{Po,i10} Z_{Po,j2} + \sqrt{2} g_{B1} \sqrt{\frac{gA1^2}{gA1^2 + gB1^2}} Z_{Po,i1} Z_{Po,j5} - \sqrt{2} g_{A1} g_{B1} \frac{1}{\sqrt{gA1^2 + gB1^2}} Z_{Po,i1} Z_{Po,j5} \\
& + \sqrt{2} g_{A1} \sqrt{\frac{gA1^2}{gA1^2 + gB1^2}} Z_{Po,i1} Z_{Po,j6} + \sqrt{2} g_{B1}^2 \frac{1}{\sqrt{gA1^2 + gB1^2}} Z_{Po,i1} Z_{Po,j6} \\
& - \sqrt{2} g_{B2} \sqrt{\frac{gA2^2}{gA2^2 + gB2^2}} Z_{Po,i1} Z_{Po,j7} + \sqrt{2} g_{A2} g_{B2} \frac{1}{\sqrt{gA2^2 + gB2^2}} Z_{Po,i1} Z_{Po,j7} \\
& - \sqrt{2} g_{A2} \sqrt{\frac{gA2^2}{gA2^2 + gB2^2}} Z_{Po,i1} Z_{Po,j8} - \sqrt{2} g_{B2}^2 \frac{1}{\sqrt{gA2^2 + gB2^2}} Z_{Po,i1} Z_{Po,j8} + \sqrt{2} Y_A^* Z_{Po,i2} Z_{Po,j9} \\
& + Y_K^* Z_{Po,i2} Z_{Po,j10} \Big) \Big) \left( \frac{1 + \gamma_5}{2} \right)
\end{aligned} \tag{817}$$


---

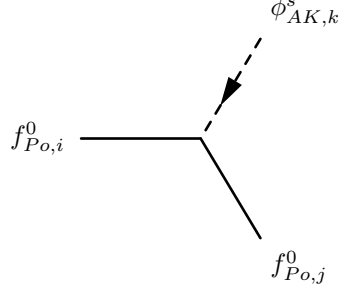

$$\begin{aligned}
& - \frac{i}{2} \left( \sqrt{2} Y_A Z_{AK,k2}^{s,*} \left( Z_{Po,i1}^* Z_{Po,j2}^* + Z_{Po,i2}^* Z_{Po,j1}^* - Z_{Po,i3}^* Z_{Po,j4}^* - Z_{Po,i4}^* Z_{Po,j3}^* \right) \right. \\
& \left. + Y_K Z_{AK,k1}^{s,*} \left( Z_{Po,i1}^* Z_{Po,j2}^* + Z_{Po,i2}^* Z_{Po,j1}^* + Z_{Po,i3}^* Z_{Po,j4}^* + Z_{Po,i4}^* Z_{Po,j3}^* \right) \right) \left( \frac{1 - \gamma_5}{2} \right)
\end{aligned} \tag{818}$$


---

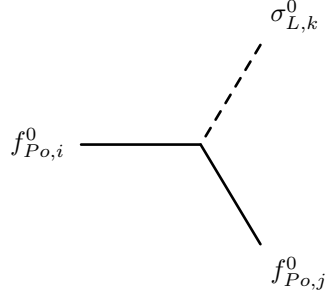

$$\begin{aligned}
& \frac{1}{2} \left( \sqrt{2} g_{B2} \sqrt{\frac{gA2^2}{gA2^2 + gB2^2}} Z_{Po,i7}^* Z_{Po,j1}^* Z_{Ls,k1}^{Di,*} - \sqrt{2} g_{A2} g_{B2} \frac{1}{\sqrt{gA2^2 + gB2^2}} Z_{Po,i7}^* Z_{Po,j1}^* Z_{Ls,k1}^{Di,*} \right. \\
& + \sqrt{2} g_{A2} \sqrt{\frac{gA2^2}{gA2^2 + gB2^2}} Z_{Po,i8}^* Z_{Po,j1}^* Z_{Ls,k1}^{Di,*} + \sqrt{2} g_{B2}^2 \frac{1}{\sqrt{gA2^2 + gB2^2}} Z_{Po,i8}^* Z_{Po,j1}^* Z_{Ls,k1}^{Di,*} \\
& + \sqrt{2} Y_A Z_{Po,i9}^* Z_{Po,j2}^* Z_{Ls,k1}^{Di,*} + Y_K Z_{Po,i10}^* Z_{Po,j2}^* Z_{Ls,k1}^{Di,*} \\
& - \sqrt{2} g_{B1} \sqrt{\frac{gA1^2}{gA1^2 + gB1^2}} Z_{Po,i1}^* Z_{Po,j5}^* Z_{Ls,k1}^{Di,*} + \sqrt{2} g_{A1} g_{B1} \frac{1}{\sqrt{gA1^2 + gB1^2}} Z_{Po,i1}^* Z_{Po,j5}^* Z_{Ls,k1}^{Di,*} \\
& - \sqrt{2} g_{A1} \sqrt{\frac{gA1^2}{gA1^2 + gB1^2}} Z_{Po,i1}^* Z_{Po,j6}^* Z_{Ls,k1}^{Di,*} - \sqrt{2} g_{B1}^2 \frac{1}{\sqrt{gA1^2 + gB1^2}} Z_{Po,i1}^* Z_{Po,j6}^* Z_{Ls,k1}^{Di,*} \\
& + \sqrt{2} g_{B2} \sqrt{\frac{gA2^2}{gA2^2 + gB2^2}} Z_{Po,i1}^* Z_{Po,j7}^* Z_{Ls,k1}^{Di,*} - \sqrt{2} g_{A2} g_{B2} \frac{1}{\sqrt{gA2^2 + gB2^2}} Z_{Po,i1}^* Z_{Po,j7}^* Z_{Ls,k1}^{Di,*} \\
& + \sqrt{2} g_{A2} \sqrt{\frac{gA2^2}{gA2^2 + gB2^2}} Z_{Po,i1}^* Z_{Po,j8}^* Z_{Ls,k1}^{Di,*} + \sqrt{2} g_{B2}^2 \frac{1}{\sqrt{gA2^2 + gB2^2}} Z_{Po,i1}^* Z_{Po,j8}^* Z_{Ls,k1}^{Di,*} \\
& + \sqrt{2} Y_A Z_{Po,i2}^* Z_{Po,j9}^* Z_{Ls,k1}^{Di,*} + Y_K Z_{Po,i2}^* Z_{Po,j10}^* Z_{Ls,k1}^{Di,*} + \sqrt{2} Y_A Z_{Po,i9}^* Z_{Po,j1}^* Z_{Ls,k2}^{Di,*} \\
& + Y_K Z_{Po,i10}^* Z_{Po,j1}^* Z_{Ls,k2}^{Di,*} - \sqrt{2} g_{B2} \sqrt{\frac{gA2^2}{gA2^2 + gB2^2}} Z_{Po,i7}^* Z_{Po,j2}^* Z_{Ls,k2}^{Di,*} \\
& + \sqrt{2} g_{A2} g_{B2} \frac{1}{\sqrt{gA2^2 + gB2^2}} Z_{Po,i7}^* Z_{Po,j2}^* Z_{Ls,k2}^{Di,*} - \sqrt{2} g_{A2} \sqrt{\frac{gA2^2}{gA2^2 + gB2^2}} Z_{Po,i8}^* Z_{Po,j2}^* Z_{Ls,k2}^{Di,*} \\
& - \sqrt{2} g_{B2}^2 \frac{1}{\sqrt{gA2^2 + gB2^2}} Z_{Po,i8}^* Z_{Po,j2}^* Z_{Ls,k2}^{Di,*} + \sqrt{2} g_{B1} \sqrt{\frac{gA1^2}{gA1^2 + gB1^2}} Z_{Po,i2}^* Z_{Po,j5}^* Z_{Ls,k2}^{Di,*} \\
& - \sqrt{2} g_{A1} g_{B1} \frac{1}{\sqrt{gA1^2 + gB1^2}} Z_{Po,i2}^* Z_{Po,j5}^* Z_{Ls,k2}^{Di,*} + \sqrt{2} g_{A1} \sqrt{\frac{gA1^2}{gA1^2 + gB1^2}} Z_{Po,i2}^* Z_{Po,j6}^* Z_{Ls,k2}^{Di,*} \\
& + \sqrt{2} g_{B1}^2 \frac{1}{\sqrt{gA1^2 + gB1^2}} Z_{Po,i2}^* Z_{Po,j6}^* Z_{Ls,k2}^{Di,*} - \sqrt{2} g_{B2} \sqrt{\frac{gA2^2}{gA2^2 + gB2^2}} Z_{Po,i2}^* Z_{Po,j7}^* Z_{Ls,k2}^{Di,*} \Big)
\end{aligned}$$

$$\begin{aligned}
& + \sqrt{2}g_{A2}g_{B2} \frac{1}{\sqrt{g_{A2}^2 + g_{B2}^2}} Z_{Po,i2}^* Z_{Po,j7}^* Z_{Ls,k2}^{Di,*} - \sqrt{2}g_{A2} \sqrt{\frac{g_{A2}^2}{g_{A2}^2 + g_{B2}^2}} Z_{Po,i2}^* Z_{Po,j8}^* Z_{Ls,k2}^{Di,*} \\
& - \sqrt{2}g_{B2}^2 \frac{1}{\sqrt{g_{A2}^2 + g_{B2}^2}} Z_{Po,i2}^* Z_{Po,j8}^* Z_{Ls,k2}^{Di,*} + \sqrt{2}Y_A Z_{Po,i1}^* Z_{Po,j9}^* Z_{Ls,k2}^{Di,*} + Y_K Z_{Po,i1}^* Z_{Po,j10}^* Z_{Ls,k2}^{Di,*} \\
& - \sqrt{2}g_{B2} \sqrt{\frac{g_{A2}^2}{g_{A2}^2 + g_{B2}^2}} Z_{Po,i7}^* Z_{Po,j3}^* Z_{Ls,k3}^{Di,*} + \sqrt{2}g_{A2}g_{B2} \frac{1}{\sqrt{g_{A2}^2 + g_{B2}^2}} Z_{Po,i7}^* Z_{Po,j3}^* Z_{Ls,k3}^{Di,*} \\
& - \sqrt{2}g_{A2} \sqrt{\frac{g_{A2}^2}{g_{A2}^2 + g_{B2}^2}} Z_{Po,i8}^* Z_{Po,j3}^* Z_{Ls,k3}^{Di,*} - \sqrt{2}g_{B2}^2 \frac{1}{\sqrt{g_{A2}^2 + g_{B2}^2}} Z_{Po,i8}^* Z_{Po,j3}^* Z_{Ls,k3}^{Di,*} \\
& - \sqrt{2}Y_A Z_{Po,i9}^* Z_{Po,j4}^* Z_{Ls,k3}^{Di,*} + Y_K Z_{Po,i10}^* Z_{Po,j4}^* Z_{Ls,k3}^{Di,*} \\
& - \sqrt{2}g_{B1} \sqrt{\frac{g_{A1}^2}{g_{A1}^2 + g_{B1}^2}} Z_{Po,i3}^* Z_{Po,j5}^* Z_{Ls,k3}^{Di,*} + \sqrt{2}g_{A1}g_{B1} \frac{1}{\sqrt{g_{A1}^2 + g_{B1}^2}} Z_{Po,i3}^* Z_{Po,j5}^* Z_{Ls,k3}^{Di,*} \\
& - \sqrt{2}g_{A1} \sqrt{\frac{g_{A1}^2}{g_{A1}^2 + g_{B1}^2}} Z_{Po,i3}^* Z_{Po,j6}^* Z_{Ls,k3}^{Di,*} - \sqrt{2}g_{B1}^2 \frac{1}{\sqrt{g_{A1}^2 + g_{B1}^2}} Z_{Po,i3}^* Z_{Po,j6}^* Z_{Ls,k3}^{Di,*} \\
& - \sqrt{2}g_{B2} \sqrt{\frac{g_{A2}^2}{g_{A2}^2 + g_{B2}^2}} Z_{Po,i3}^* Z_{Po,j7}^* Z_{Ls,k3}^{Di,*} + \sqrt{2}g_{A2}g_{B2} \frac{1}{\sqrt{g_{A2}^2 + g_{B2}^2}} Z_{Po,i3}^* Z_{Po,j7}^* Z_{Ls,k3}^{Di,*} \\
& - \sqrt{2}g_{A2} \sqrt{\frac{g_{A2}^2}{g_{A2}^2 + g_{B2}^2}} Z_{Po,i3}^* Z_{Po,j8}^* Z_{Ls,k3}^{Di,*} - \sqrt{2}g_{B2}^2 \frac{1}{\sqrt{g_{A2}^2 + g_{B2}^2}} Z_{Po,i3}^* Z_{Po,j8}^* Z_{Ls,k3}^{Di,*} \\
& - \sqrt{2}Y_A Z_{Po,i4}^* Z_{Po,j9}^* Z_{Ls,k3}^{Di,*} + Y_K Z_{Po,i4}^* Z_{Po,j10}^* Z_{Ls,k3}^{Di,*} - \sqrt{2}Y_A Z_{Po,i9}^* Z_{Po,j3}^* Z_{Ls,k4}^{Di,*} \\
& + Y_K Z_{Po,i10}^* Z_{Po,j3}^* Z_{Ls,k4}^{Di,*} + \sqrt{2}g_{B2} \sqrt{\frac{g_{A2}^2}{g_{A2}^2 + g_{B2}^2}} Z_{Po,i7}^* Z_{Po,j4}^* Z_{Ls,k4}^{Di,*} \\
& - \sqrt{2}g_{A2}g_{B2} \frac{1}{\sqrt{g_{A2}^2 + g_{B2}^2}} Z_{Po,i7}^* Z_{Po,j4}^* Z_{Ls,k4}^{Di,*} + \sqrt{2}g_{A2} \sqrt{\frac{g_{A2}^2}{g_{A2}^2 + g_{B2}^2}} Z_{Po,i8}^* Z_{Po,j4}^* Z_{Ls,k4}^{Di,*} \\
& + \sqrt{2}g_{B2}^2 \frac{1}{\sqrt{g_{A2}^2 + g_{B2}^2}} Z_{Po,i8}^* Z_{Po,j4}^* Z_{Ls,k4}^{Di,*} + \sqrt{2}g_{B1} \sqrt{\frac{g_{A1}^2}{g_{A1}^2 + g_{B1}^2}} Z_{Po,i4}^* Z_{Po,j5}^* Z_{Ls,k4}^{Di,*} \\
& - \sqrt{2}g_{A1}g_{B1} \frac{1}{\sqrt{g_{A1}^2 + g_{B1}^2}} Z_{Po,i4}^* Z_{Po,j5}^* Z_{Ls,k4}^{Di,*} + \sqrt{2}g_{A1} \sqrt{\frac{g_{A1}^2}{g_{A1}^2 + g_{B1}^2}} Z_{Po,i4}^* Z_{Po,j6}^* Z_{Ls,k4}^{Di,*} \\
& + \sqrt{2}g_{B1}^2 \frac{1}{\sqrt{g_{A1}^2 + g_{B1}^2}} Z_{Po,i4}^* Z_{Po,j6}^* Z_{Ls,k4}^{Di,*} + \sqrt{2}g_{B2} \sqrt{\frac{g_{A2}^2}{g_{A2}^2 + g_{B2}^2}} Z_{Po,i4}^* Z_{Po,j7}^* Z_{Ls,k4}^{Di,*} \\
& - \sqrt{2}g_{A2}g_{B2} \frac{1}{\sqrt{g_{A2}^2 + g_{B2}^2}} Z_{Po,i4}^* Z_{Po,j7}^* Z_{Ls,k4}^{Di,*} + \sqrt{2}g_{A2} \sqrt{\frac{g_{A2}^2}{g_{A2}^2 + g_{B2}^2}} Z_{Po,i4}^* Z_{Po,j8}^* Z_{Ls,k4}^{Di,*} \\
& + \sqrt{2}g_{B2}^2 \frac{1}{\sqrt{g_{A2}^2 + g_{B2}^2}} Z_{Po,i4}^* Z_{Po,j8}^* Z_{Ls,k4}^{Di,*} - \sqrt{2}Y_A Z_{Po,i3}^* Z_{Po,j9}^* Z_{Ls,k4}^{Di,*} + Y_K Z_{Po,i3}^* Z_{Po,j10}^* Z_{Ls,k4}^{Di,*}
\end{aligned}$$

$$\begin{aligned}
& -\sqrt{2}g_{B1}\frac{1}{\sqrt{gA1^2+gB1^2}}\left(-g_{A1}+\sqrt{\frac{gA1^2}{gA1^2+gB1^2}}\sqrt{gA1^2+gB1^2}\right)Z_{Po,i5}^*\left(Z_{Po,j1}^*Z_{Ls,k1}^{Di,*}-Z_{Po,j2}^*Z_{Ls,k2}^{Di,*}+Z_{Po,j3}^*Z_{Ls,k3}^{Di,*}-Z_{Po,j4}^*Z_{Ls,k4}^{Di,*}\right) \\
& -\sqrt{2}\frac{1}{\sqrt{gA1^2+gB1^2}}\left(g_{A1}\sqrt{\frac{gA1^2}{gA1^2+gB1^2}}\sqrt{gA1^2+gB1^2}+g_{B1}^2\right)Z_{Po,i6}^*\left(Z_{Po,j1}^*Z_{Ls,k1}^{Di,*}-Z_{Po,j2}^*Z_{Ls,k2}^{Di,*}+Z_{Po,j3}^*Z_{Ls,k3}^{Di,*}-Z_{Po,j4}^*Z_{Ls,k4}^{Di,*}\right) \\
& \quad (819) \\
& +\frac{1}{2}\left(-Y_K^*Z_{Ls,k2}^{Di,*}Z_{Po,i10}Z_{Po,j1}-\sqrt{2}g_{B1}\sqrt{\frac{gA1^2}{gA1^2+gB1^2}}Z_{Ls,k2}^{Di,*}Z_{Po,i5}Z_{Po,j2}\right. \\
& +\sqrt{2}g_{A1}g_{B1}\frac{1}{\sqrt{gA1^2+gB1^2}}Z_{Ls,k2}^{Di,*}Z_{Po,i5}Z_{Po,j2}-\sqrt{2}g_{A1}\sqrt{\frac{gA1^2}{gA1^2+gB1^2}}Z_{Ls,k2}^{Di,*}Z_{Po,i6}Z_{Po,j2} \\
& -\sqrt{2}g_{B1}^2\frac{1}{\sqrt{gA1^2+gB1^2}}Z_{Ls,k2}^{Di,*}Z_{Po,i6}Z_{Po,j2}+\sqrt{2}g_{B2}\sqrt{\frac{gA2^2}{gA2^2+gB2^2}}Z_{Ls,k2}^{Di,*}Z_{Po,i7}Z_{Po,j2} \\
& -\sqrt{2}g_{A2}g_{B2}\frac{1}{\sqrt{gA2^2+gB2^2}}Z_{Ls,k2}^{Di,*}Z_{Po,i7}Z_{Po,j2}+\sqrt{2}g_{A2}\sqrt{\frac{gA2^2}{gA2^2+gB2^2}}Z_{Ls,k2}^{Di,*}Z_{Po,i8}Z_{Po,j2} \\
& +\sqrt{2}g_{B2}^2\frac{1}{\sqrt{gA2^2+gB2^2}}Z_{Ls,k2}^{Di,*}Z_{Po,i8}Z_{Po,j2}+\sqrt{2}g_{B1}\sqrt{\frac{gA1^2}{gA1^2+gB1^2}}Z_{Ls,k3}^{Di,*}Z_{Po,i5}Z_{Po,j3} \\
& -\sqrt{2}g_{A1}g_{B1}\frac{1}{\sqrt{gA1^2+gB1^2}}Z_{Ls,k3}^{Di,*}Z_{Po,i5}Z_{Po,j3}+\sqrt{2}g_{A1}\sqrt{\frac{gA1^2}{gA1^2+gB1^2}}Z_{Ls,k3}^{Di,*}Z_{Po,i6}Z_{Po,j3} \\
& +\sqrt{2}g_{B1}^2\frac{1}{\sqrt{gA1^2+gB1^2}}Z_{Ls,k3}^{Di,*}Z_{Po,i6}Z_{Po,j3}+\sqrt{2}g_{B2}\sqrt{\frac{gA2^2}{gA2^2+gB2^2}}Z_{Ls,k3}^{Di,*}Z_{Po,i7}Z_{Po,j3} \\
& -\sqrt{2}g_{A2}g_{B2}\frac{1}{\sqrt{gA2^2+gB2^2}}Z_{Ls,k3}^{Di,*}Z_{Po,i7}Z_{Po,j3}+\sqrt{2}g_{A2}\sqrt{\frac{gA2^2}{gA2^2+gB2^2}}Z_{Ls,k3}^{Di,*}Z_{Po,i8}Z_{Po,j3} \\
& +\sqrt{2}g_{B2}^2\frac{1}{\sqrt{gA2^2+gB2^2}}Z_{Ls,k3}^{Di,*}Z_{Po,i8}Z_{Po,j3}-Y_K^*Z_{Ls,k4}^{Di,*}Z_{Po,i10}Z_{Po,j3} \\
& -\sqrt{2}g_{B1}\sqrt{\frac{gA1^2}{gA1^2+gB1^2}}Z_{Ls,k4}^{Di,*}Z_{Po,i5}Z_{Po,j4}+\sqrt{2}g_{A1}g_{B1}\frac{1}{\sqrt{gA1^2+gB1^2}}Z_{Ls,k4}^{Di,*}Z_{Po,i5}Z_{Po,j4} \\
& -\sqrt{2}g_{A1}\sqrt{\frac{gA1^2}{gA1^2+gB1^2}}Z_{Ls,k4}^{Di,*}Z_{Po,i6}Z_{Po,j4}-\sqrt{2}g_{B1}^2\frac{1}{\sqrt{gA1^2+gB1^2}}Z_{Ls,k4}^{Di,*}Z_{Po,i6}Z_{Po,j4} \\
& -\sqrt{2}g_{B2}\sqrt{\frac{gA2^2}{gA2^2+gB2^2}}Z_{Ls,k4}^{Di,*}Z_{Po,i7}Z_{Po,j4}+\sqrt{2}g_{A2}g_{B2}\frac{1}{\sqrt{gA2^2+gB2^2}}Z_{Ls,k4}^{Di,*}Z_{Po,i7}Z_{Po,j4} \\
& -\sqrt{2}g_{A2}\sqrt{\frac{gA2^2}{gA2^2+gB2^2}}Z_{Ls,k4}^{Di,*}Z_{Po,i8}Z_{Po,j4}-\sqrt{2}g_{B2}^2\frac{1}{\sqrt{gA2^2+gB2^2}}Z_{Ls,k4}^{Di,*}Z_{Po,i8}Z_{Po,j4}
\end{aligned}$$

$$\begin{aligned}
& -Y_K^* Z_{Ls,k3}^{Di,*} Z_{Po,i10} Z_{Po,j4} - \sqrt{2} g_{B1} \sqrt{\frac{gA1^2}{gA1^2 + gB1^2}} Z_{Ls,k2}^{Di,*} Z_{Po,i2} Z_{Po,j5} \\
& + \sqrt{2} g_{A1} g_{B1} \frac{1}{\sqrt{gA1^2 + gB1^2}} Z_{Ls,k2}^{Di,*} Z_{Po,i2} Z_{Po,j5} + \sqrt{2} g_{B1} \sqrt{\frac{gA1^2}{gA1^2 + gB1^2}} Z_{Ls,k3}^{Di,*} Z_{Po,i3} Z_{Po,j5} \\
& - \sqrt{2} g_{A1} g_{B1} \frac{1}{\sqrt{gA1^2 + gB1^2}} Z_{Ls,k3}^{Di,*} Z_{Po,i3} Z_{Po,j5} - \sqrt{2} g_{B1} \sqrt{\frac{gA1^2}{gA1^2 + gB1^2}} Z_{Ls,k4}^{Di,*} Z_{Po,i4} Z_{Po,j5} \\
& + \sqrt{2} g_{A1} g_{B1} \frac{1}{\sqrt{gA1^2 + gB1^2}} Z_{Ls,k4}^{Di,*} Z_{Po,i4} Z_{Po,j5} - \sqrt{2} g_{A1} \sqrt{\frac{gA1^2}{gA1^2 + gB1^2}} Z_{Ls,k2}^{Di,*} Z_{Po,i2} Z_{Po,j6} \\
& - \sqrt{2} g_{B1}^2 \frac{1}{\sqrt{gA1^2 + gB1^2}} Z_{Ls,k2}^{Di,*} Z_{Po,i2} Z_{Po,j6} + \sqrt{2} g_{A1} \sqrt{\frac{gA1^2}{gA1^2 + gB1^2}} Z_{Ls,k3}^{Di,*} Z_{Po,i3} Z_{Po,j6} \\
& + \sqrt{2} g_{B1}^2 \frac{1}{\sqrt{gA1^2 + gB1^2}} Z_{Ls,k3}^{Di,*} Z_{Po,i3} Z_{Po,j6} - \sqrt{2} g_{A1} \sqrt{\frac{gA1^2}{gA1^2 + gB1^2}} Z_{Ls,k4}^{Di,*} Z_{Po,i4} Z_{Po,j6} \\
& - \sqrt{2} g_{B1}^2 \frac{1}{\sqrt{gA1^2 + gB1^2}} Z_{Ls,k4}^{Di,*} Z_{Po,i4} Z_{Po,j6} + \sqrt{2} g_{B2} \sqrt{\frac{gA2^2}{gA2^2 + gB2^2}} Z_{Ls,k2}^{Di,*} Z_{Po,i2} Z_{Po,j7} \\
& - \sqrt{2} g_{A2} g_{B2} \frac{1}{\sqrt{gA2^2 + gB2^2}} Z_{Ls,k2}^{Di,*} Z_{Po,i2} Z_{Po,j7} + \sqrt{2} g_{B2} \sqrt{\frac{gA2^2}{gA2^2 + gB2^2}} Z_{Ls,k3}^{Di,*} Z_{Po,i3} Z_{Po,j7} \\
& - \sqrt{2} g_{A2} g_{B2} \frac{1}{\sqrt{gA2^2 + gB2^2}} Z_{Ls,k3}^{Di,*} Z_{Po,i3} Z_{Po,j7} - \sqrt{2} g_{B2} \sqrt{\frac{gA2^2}{gA2^2 + gB2^2}} Z_{Ls,k4}^{Di,*} Z_{Po,i4} Z_{Po,j7} \\
& + \sqrt{2} g_{A2} g_{B2} \frac{1}{\sqrt{gA2^2 + gB2^2}} Z_{Ls,k4}^{Di,*} Z_{Po,i4} Z_{Po,j7} + \sqrt{2} g_{A2} \sqrt{\frac{gA2^2}{gA2^2 + gB2^2}} Z_{Ls,k2}^{Di,*} Z_{Po,i2} Z_{Po,j8} \\
& + \sqrt{2} g_{B2}^2 \frac{1}{\sqrt{gA2^2 + gB2^2}} Z_{Ls,k2}^{Di,*} Z_{Po,i2} Z_{Po,j8} + \sqrt{2} g_{A2} \sqrt{\frac{gA2^2}{gA2^2 + gB2^2}} Z_{Ls,k3}^{Di,*} Z_{Po,i3} Z_{Po,j8} \\
& + \sqrt{2} g_{B2}^2 \frac{1}{\sqrt{gA2^2 + gB2^2}} Z_{Ls,k3}^{Di,*} Z_{Po,i3} Z_{Po,j8} - \sqrt{2} g_{A2} \sqrt{\frac{gA2^2}{gA2^2 + gB2^2}} Z_{Ls,k4}^{Di,*} Z_{Po,i4} Z_{Po,j8} \\
& - \sqrt{2} g_{B2}^2 \frac{1}{\sqrt{gA2^2 + gB2^2}} Z_{Ls,k4}^{Di,*} Z_{Po,i4} Z_{Po,j8} \\
& + \sqrt{2} Y_A^* \left( -Z_{Ls,k2}^{Di,*} \left( Z_{Po,i1} Z_{Po,j9} + Z_{Po,i9} Z_{Po,j1} \right) + Z_{Ls,k3}^{Di,*} \left( Z_{Po,i4} Z_{Po,j9} + Z_{Po,i9} Z_{Po,j4} \right) + Z_{Ls,k4}^{Di,*} \left( Z_{Po,i3} Z_{Po,j9} + Z_{Po,i9} Z_{Po,j3} \right) \right) \\
& - Y_K^* Z_{Ls,k2}^{Di,*} Z_{Po,i1} Z_{Po,j10} - Y_K^* Z_{Ls,k4}^{Di,*} Z_{Po,i3} Z_{Po,j10} - Y_K^* Z_{Ls,k3}^{Di,*} Z_{Po,i4} Z_{Po,j10} \\
& + Z_{Ls,k1}^{Di,*} \left( \sqrt{2} g_{B1} \left( -g_{A1} \frac{1}{\sqrt{gA1^2 + gB1^2}} + \sqrt{\frac{gA1^2}{gA1^2 + gB1^2}} \right) Z_{Po,i5} Z_{Po,j1} \right. \\
& \left. + \sqrt{2} \left( g_{A1} \sqrt{\frac{gA1^2}{gA1^2 + gB1^2}} + g_{B1}^2 \frac{1}{\sqrt{gA1^2 + gB1^2}} \right) Z_{Po,i6} Z_{Po,j1} \right)
\end{aligned}$$

$$\begin{aligned}
& -\sqrt{2}g_{B2}\sqrt{\frac{gA2^2}{gA2^2+gB2^2}}Z_{Po,i7}Z_{Po,j1}+\sqrt{2}g_{A2}g_{B2}\frac{1}{\sqrt{gA2^2+gB2^2}}Z_{Po,i7}Z_{Po,j1} \\
& -\sqrt{2}g_{A2}\sqrt{\frac{gA2^2}{gA2^2+gB2^2}}Z_{Po,i8}Z_{Po,j1}-\sqrt{2}g_{B2}^2\frac{1}{\sqrt{gA2^2+gB2^2}}Z_{Po,i8}Z_{Po,j1} \\
& -\sqrt{2}Y_A^*Z_{Po,i9}Z_{Po,j2}-Y_K^*Z_{Po,i10}Z_{Po,j2}+\sqrt{2}g_{B1}\sqrt{\frac{gA1^2}{gA1^2+gB1^2}}Z_{Po,i1}Z_{Po,j5} \\
& -\sqrt{2}g_{A1}g_{B1}\frac{1}{\sqrt{gA1^2+gB1^2}}Z_{Po,i1}Z_{Po,j5}+\sqrt{2}g_{A1}\sqrt{\frac{gA1^2}{gA1^2+gB1^2}}Z_{Po,i1}Z_{Po,j6} \\
& +\sqrt{2}g_{B1}^2\frac{1}{\sqrt{gA1^2+gB1^2}}Z_{Po,i1}Z_{Po,j6}-\sqrt{2}g_{B2}\sqrt{\frac{gA2^2}{gA2^2+gB2^2}}Z_{Po,i1}Z_{Po,j7} \\
& +\sqrt{2}g_{A2}g_{B2}\frac{1}{\sqrt{gA2^2+gB2^2}}Z_{Po,i1}Z_{Po,j7}-\sqrt{2}g_{A2}\sqrt{\frac{gA2^2}{gA2^2+gB2^2}}Z_{Po,i1}Z_{Po,j8} \\
& -\sqrt{2}g_{B2}^2\frac{1}{\sqrt{gA2^2+gB2^2}}Z_{Po,i1}Z_{Po,j8}-\sqrt{2}Y_A^*Z_{Po,i2}Z_{Po,j9}-Y_K^*Z_{Po,i2}Z_{Po,j10}\Big)\Big(\frac{1+\gamma_5}{2}\Big)
\end{aligned} \tag{820}$$


---

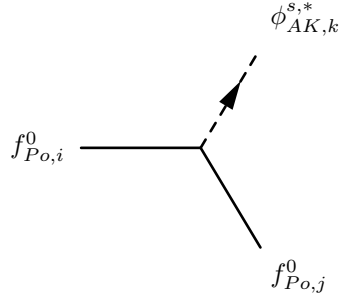

(821)

$$\begin{aligned}
& +-\frac{i}{2}\Big(\sqrt{2}Y_A^*Z_{AK,k2}^s\Big(Z_{Po,i1}Z_{Po,j2}+Z_{Po,i2}Z_{Po,j1}-Z_{Po,i3}Z_{Po,j4}-Z_{Po,i4}Z_{Po,j3}\Big) \\
& +Y_K^*Z_{AK,k1}^s\Big(Z_{Po,i1}Z_{Po,j2}+Z_{Po,i2}Z_{Po,j1}+Z_{Po,i3}Z_{Po,j4}+Z_{Po,i4}Z_{Po,j3}\Big)\Big)\Big(\frac{1+\gamma_5}{2}\Big)
\end{aligned} \tag{822}$$


---



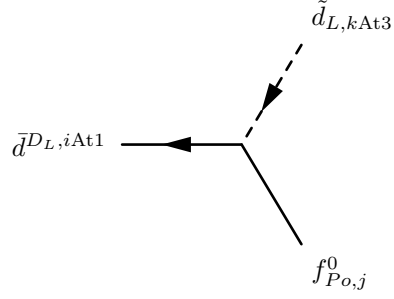

(823)

$$\begin{aligned}
& + -\frac{i}{3} \frac{1}{\sqrt{2}} \delta_{\text{At}1\text{At}3} \delta_{ik} \left( g_{A1} g_{B1} \frac{1}{\sqrt{g_{A1}^2 + g_{B1}^2}} Z_{Po, j5} - g_{A1} \sqrt{\frac{g_{A1}^2}{g_{A1}^2 + g_{B1}^2}} Z_{Po, j6} - 3g_{A2} g_{B2} \frac{1}{\sqrt{g_{A2}^2 + g_{B2}^2}} Z_{Po, j7} \right. \\
& \left. + 3g_{A2} \sqrt{\frac{g_{A2}^2}{g_{A2}^2 + g_{B2}^2}} Z_{Po, j8} \right) \left( \frac{1 + \gamma_5}{2} \right)
\end{aligned} \tag{824}$$


---

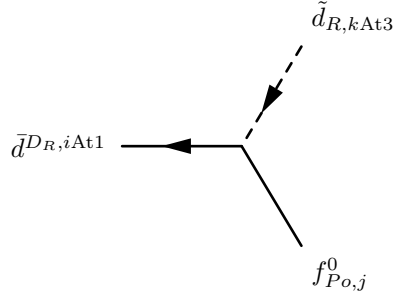

$$\frac{i}{3} \sqrt{2} g_{A1} \frac{1}{\sqrt{g_{A1}^2 + g_{B1}^2}} \left( -g_{B1} Z_{Po, j5}^* + \sqrt{\frac{g_{A1}^2}{g_{A1}^2 + g_{B1}^2}} \sqrt{g_{A1}^2 + g_{B1}^2} Z_{Po, j6}^* \right) \delta_{\text{At}1\text{At}3} \delta_{ik} \left( \frac{1 - \gamma_5}{2} \right) \tag{825}$$


---

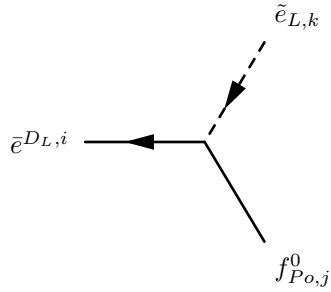

(826)

$$\begin{aligned}
& + i \frac{1}{\sqrt{2}} \delta_{ik} \left( g_{A1} g_{B1} \frac{1}{\sqrt{g_{A1}^2 + g_{B1}^2}} Z_{Po,j5} - g_{A1} \sqrt{\frac{g_{A1}^2}{g_{A1}^2 + g_{B1}^2}} Z_{Po,j6} + g_{A2} g_{B2} \frac{1}{\sqrt{g_{A2}^2 + g_{B2}^2}} Z_{Po,j7} \right. \\
& \left. - g_{A2} \sqrt{\frac{g_{A2}^2}{g_{A2}^2 + g_{B2}^2}} Z_{Po,j8} \right) \left( \frac{1 + \gamma_5}{2} \right)
\end{aligned} \tag{827}$$


---

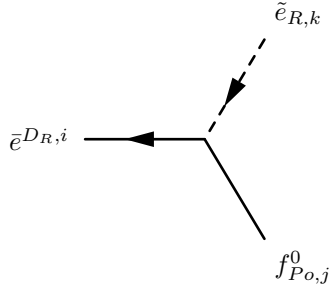

$$- i \sqrt{2} g_{A1} \left( g_{B1} \frac{1}{\sqrt{g_{A1}^2 + g_{B1}^2}} Z_{Po,j5}^* - \sqrt{\frac{g_{A1}^2}{g_{A1}^2 + g_{B1}^2}} Z_{Po,j6}^* \right) \delta_{ik} \left( \frac{1 - \gamma_5}{2} \right) \tag{828}$$


---

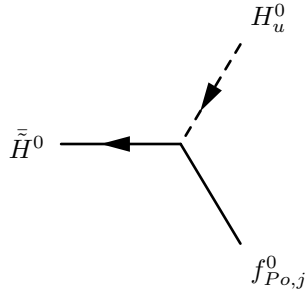

(829)

$$\begin{aligned}
& + -i \frac{1}{\sqrt{2}} \left( g_{A1} g_{B1} \frac{1}{\sqrt{g_{A1}^2 + g_{B1}^2}} Z_{Po,j5} - g_{A1} \sqrt{\frac{g_{A1}^2}{g_{A1}^2 + g_{B1}^2}} Z_{Po,j6} - g_{A2} g_{B2} \frac{1}{\sqrt{g_{A2}^2 + g_{B2}^2}} Z_{Po,j7} \right. \\
& \left. + g_{A2} \sqrt{\frac{g_{A2}^2}{g_{A2}^2 + g_{B2}^2}} Z_{Po,j8} \right) \left( \frac{1 + \gamma_5}{2} \right)
\end{aligned} \tag{830}$$


---

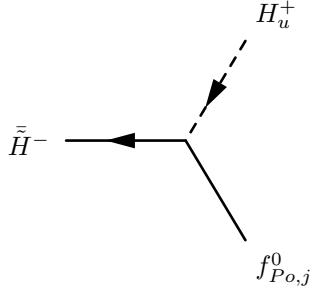

(831)

$$\begin{aligned}
& + -i \frac{1}{\sqrt{2}} \left( g_{A1} g_{B1} \frac{1}{\sqrt{g_{A1}^2 + g_{B1}^2}} Z_{Po,j5} - g_{A1} \sqrt{\frac{g_{A1}^2}{g_{A1}^2 + g_{B1}^2}} Z_{Po,j6} + g_{A2} g_{B2} \frac{1}{\sqrt{g_{A2}^2 + g_{B2}^2}} Z_{Po,j7} \right. \\
& \left. - g_{A2} \sqrt{\frac{g_{A2}^2}{g_{A2}^2 + g_{B2}^2}} Z_{Po,j8} \right) \left( \frac{1 + \gamma_5}{2} \right)
\end{aligned}
\tag{832}$$


---

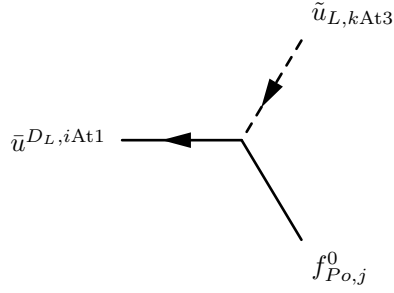

(833)

$$\begin{aligned}
& + -\frac{i}{3} \frac{1}{\sqrt{2}} \delta_{At1At3} \delta_{ik} \left( g_{A1} g_{B1} \frac{1}{\sqrt{g_{A1}^2 + g_{B1}^2}} Z_{Po,j5} - g_{A1} \sqrt{\frac{g_{A1}^2}{g_{A1}^2 + g_{B1}^2}} Z_{Po,j6} + 3g_{A2} g_{B2} \frac{1}{\sqrt{g_{A2}^2 + g_{B2}^2}} Z_{Po,j7} \right. \\
& \left. - 3g_{A2} \sqrt{\frac{g_{A2}^2}{g_{A2}^2 + g_{B2}^2}} Z_{Po,j8} \right) \left( \frac{1 + \gamma_5}{2} \right)
\end{aligned}
\tag{834}$$


---

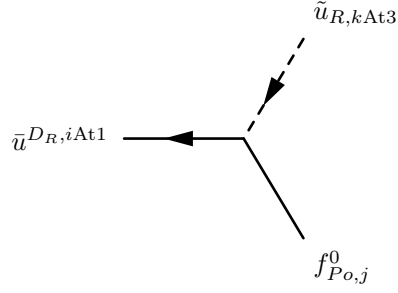

$$\frac{2i}{3}\sqrt{2}g_{A1}\frac{1}{\sqrt{g_{A1}^2 + g_{B1}^2}}\left(g_{B1}Z_{Po, j5}^* - \sqrt{\frac{g_{A1}^2}{g_{A1}^2 + g_{B1}^2}}\sqrt{g_{A1}^2 + g_{B1}^2}Z_{Po, j6}^*\right)\delta_{\text{At}1\text{At}3}\delta_{ik}\left(\frac{1 - \gamma_5}{2}\right) \quad (835)$$


---

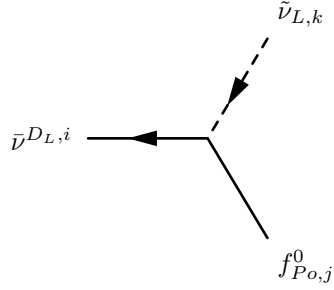

$$(836)$$

$$\begin{aligned} &+ i\frac{1}{\sqrt{2}}\delta_{ik}\left(g_{A1}g_{B1}\frac{1}{\sqrt{g_{A1}^2 + g_{B1}^2}}Z_{Po, j5} - g_{A1}\sqrt{\frac{g_{A1}^2}{g_{A1}^2 + g_{B1}^2}}Z_{Po, j6} - g_{A2}g_{B2}\frac{1}{\sqrt{g_{A2}^2 + g_{B2}^2}}Z_{Po, j7}\right. \\ &\left.+ g_{A2}\sqrt{\frac{g_{A2}^2}{g_{A2}^2 + g_{B2}^2}}Z_{Po, j8}\right)\left(\frac{1 + \gamma_5}{2}\right) \end{aligned} \quad (837)$$


---

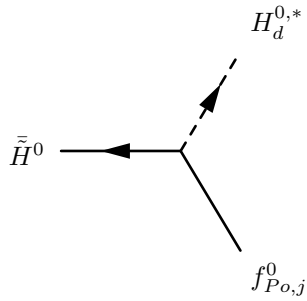

$$\begin{aligned}
& i \frac{1}{\sqrt{2}} \left( g_{A1} g_{B1} \frac{1}{\sqrt{g_{A1}^2 + g_{B1}^2}} Z_{Po,j5}^* - g_{A1} \sqrt{\frac{g_{A1}^2}{g_{A1}^2 + g_{B1}^2}} Z_{Po,j6}^* - g_{A2} g_{B2} \frac{1}{\sqrt{g_{A2}^2 + g_{B2}^2}} Z_{Po,j7}^* \right. \\
& \left. + g_{A2} \sqrt{\frac{g_{A2}^2}{g_{A2}^2 + g_{B2}^2}} Z_{Po,j8}^* \right) \left( \frac{1 - \gamma_5}{2} \right)
\end{aligned} \tag{838}$$


---

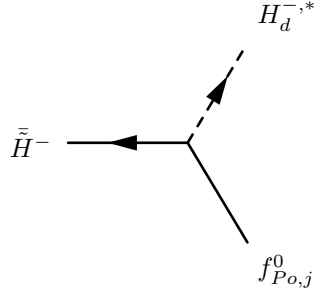

$$\begin{aligned}
& i \frac{1}{\sqrt{2}} \left( g_{A1} g_{B1} \frac{1}{\sqrt{g_{A1}^2 + g_{B1}^2}} Z_{Po,j5}^* - g_{A1} \sqrt{\frac{g_{A1}^2}{g_{A1}^2 + g_{B1}^2}} Z_{Po,j6}^* + g_{A2} g_{B2} \frac{1}{\sqrt{g_{A2}^2 + g_{B2}^2}} Z_{Po,j7}^* \right. \\
& \left. - g_{A2} \sqrt{\frac{g_{A2}^2}{g_{A2}^2 + g_{B2}^2}} Z_{Po,j8}^* \right) \left( \frac{1 - \gamma_5}{2} \right)
\end{aligned} \tag{839}$$


---

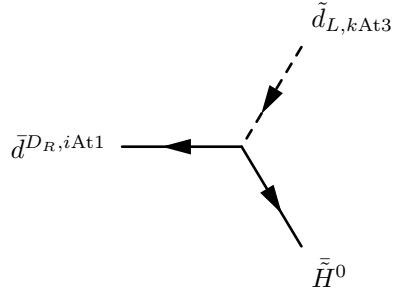

$$- i \delta_{At1At3} Y_{d,ik} \left( \frac{1 - \gamma_5}{2} \right) \tag{840}$$


---

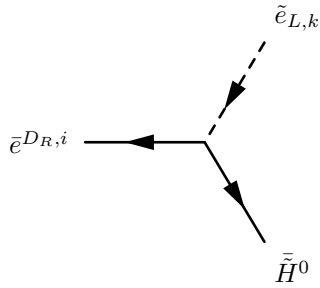

$$-iY_{e,ik}\left(\frac{1-\gamma_5}{2}\right) \quad (841)$$


---

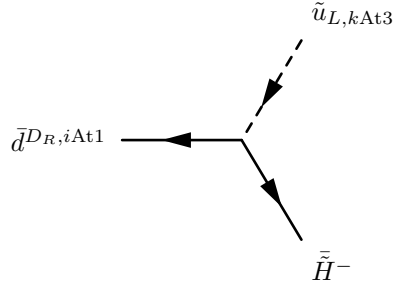

$$i\delta_{\text{At}1\text{At}3}Y_{d,ik}\left(\frac{1-\gamma_5}{2}\right) \quad (842)$$


---

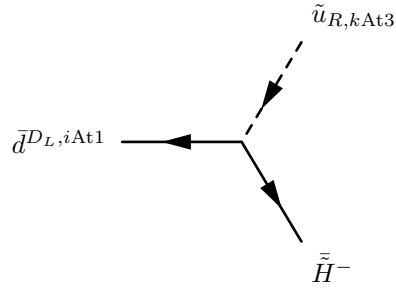

$$(843)$$

$$+iY_{u,ki}^*\delta_{\text{At}1\text{At}3}\left(\frac{1+\gamma_5}{2}\right) \quad (844)$$


---

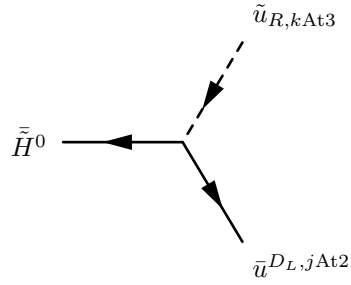

(845)

$$+ -iY_{u,kj}^* \delta_{\text{At}2\text{At}3} \left( \frac{1+\gamma_5}{2} \right) \quad (846)$$

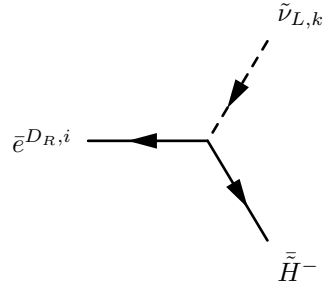

$$iY_{e,ik} \left( \frac{1-\gamma_5}{2} \right) \quad (847)$$

## 9.6 Three Vector Boson-Interaction

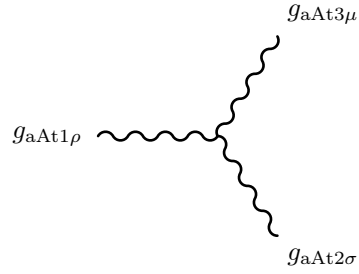

$$g_3 f_{a\text{At}1,a\text{At}2,a\text{At}3} \left( g_{\rho\mu} \left( -p_\sigma^{g_{a\text{At}3\mu}} + p_\sigma^{g_{a\text{At}1\rho}} \right) + g_{\rho\sigma} \left( -p_\mu^{g_{a\text{At}1\rho}} + p_\mu^{g_{a\text{At}2\sigma}} \right) + g_{\sigma\mu} \left( -p_\rho^{g_{a\text{At}2\sigma}} + p_\rho^{g_{a\text{At}3\mu}} \right) \right) \quad (848)$$

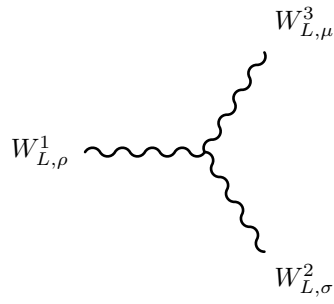

$$g_{A2}g_{B2}\frac{1}{\left(gA2^2+gB2^2\right)^{3/2}}\left(g_{A2}\sqrt{\frac{gA2^2}{gA2^2+gB2^2}}\sqrt{gA2^2+gB2^2}+g_{B2}^2\right)\left(g_{\rho\mu}\left(-p_{\sigma}^{W_{L,\mu}^3}+p_{\sigma}^{W_{L,\rho}^1}\right)+g_{\rho\sigma}\left(-p_{\mu}^{W_{L,\rho}^1}+p_{\mu}^{W_{L,\sigma}^2}\right)+g_{\sigma\mu}\left(-p_{\rho}^{W_{L,\rho}^1}+p_{\rho}^{W_{L,\sigma}^2}\right)\right) \quad (849)$$


---

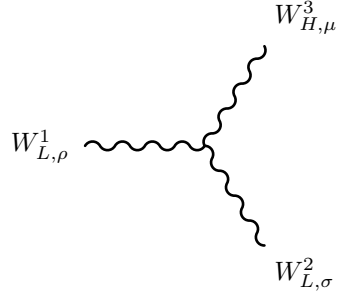

$$-g_{A2}g_{B2}^2\frac{1}{\left(gA2^2+gB2^2\right)^{3/2}}\left(-g_{A2}+\sqrt{\frac{gA2^2}{gA2^2+gB2^2}}\sqrt{gA2^2+gB2^2}\right)\left(g_{\rho\mu}\left(-p_{\sigma}^{W_{H,\mu}^3}+p_{\sigma}^{W_{L,\rho}^1}\right)+g_{\rho\sigma}\left(-p_{\mu}^{W_{L,\rho}^1}+p_{\mu}^{W_{L,\sigma}^2}\right)+g_{\sigma\mu}\left(-p_{\rho}^{W_{L,\rho}^1}+p_{\rho}^{W_{L,\sigma}^2}\right)\right) \quad (850)$$


---

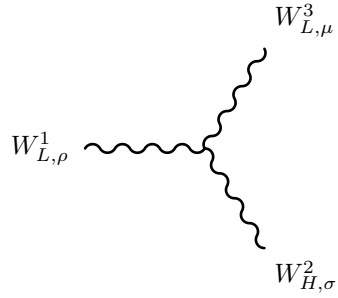

$$-g_{A2}g_{B2}^2\frac{1}{\left(gA2^2+gB2^2\right)^{3/2}}\left(-g_{A2}+\sqrt{\frac{gA2^2}{gA2^2+gB2^2}}\sqrt{gA2^2+gB2^2}\right)\left(g_{\rho\mu}\left(-p_{\sigma}^{W_{L,\mu}^3}+p_{\sigma}^{W_{L,\rho}^1}\right)+g_{\rho\sigma}\left(-p_{\mu}^{W_{L,\rho}^1}+p_{\mu}^{W_{H,\sigma}^2}\right)+g_{\sigma\mu}\left(-p_{\rho}^{W_{L,\rho}^1}+p_{\rho}^{W_{H,\sigma}^2}\right)\right) \quad (851)$$


---



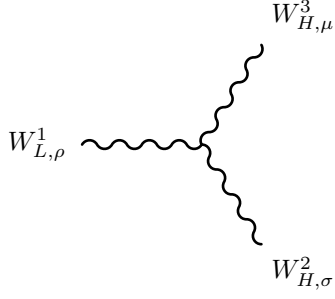

$$\left(g_{A2}^{-2}g_{B2}^3\left(\frac{gA2^2}{gA2^2+gB2^2}\right)^{3/2}+g_{A2}^3g_{B2}\frac{1}{\left(gA2^2+gB2^2\right)^{3/2}}\right)\left(g_{\rho\mu}\left(-p_{\sigma}^{W_{H,\mu}^3}+p_{\sigma}^{W_{L,\rho}^1}\right)+g_{\rho\sigma}\left(-p_{\mu}^{W_{L,\rho}^1}+p_{\mu}^{W_{H,\sigma}^2}\right)+g_{\sigma\mu}\left(-p_{\rho}^{W_{H,\sigma}^2}+p_{\rho}^{W_{L,\rho}^1}\right)\right) \quad (852)$$


---

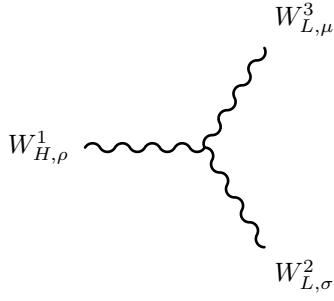

$$-g_{A2}g_{B2}^2\frac{1}{\left(gA2^2+gB2^2\right)^{3/2}}\left(-g_{A2}+\sqrt{\frac{gA2^2}{gA2^2+gB2^2}}\sqrt{gA2^2+gB2^2}\right)\left(g_{\rho\mu}\left(-p_{\sigma}^{W_{L,\mu}^3}+p_{\sigma}^{W_{H,\rho}^1}\right)+g_{\rho\sigma}\left(-p_{\mu}^{W_{H,\rho}^1}+p_{\mu}^{W_{L,\sigma}^2}\right)+g_{\sigma\mu}\left(-p_{\rho}^{W_{L,\sigma}^2}+p_{\rho}^{W_{H,\rho}^1}\right)\right) \quad (853)$$


---

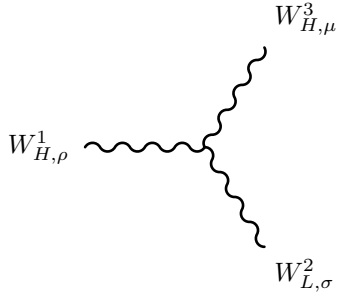

$$\left(g_{A2}^{-2}g_{B2}^3\left(\frac{gA2^2}{gA2^2+gB2^2}\right)^{3/2}+g_{A2}^3g_{B2}\frac{1}{\left(gA2^2+gB2^2\right)^{3/2}}\right)\left(g_{\rho\mu}\left(-p_{\sigma}^{W_{H,\mu}^3}+p_{\sigma}^{W_{H,\rho}^1}\right)+g_{\rho\sigma}\left(-p_{\mu}^{W_{H,\rho}^1}+p_{\mu}^{W_{L,\sigma}^2}\right)+g_{\sigma\mu}\left(-p_{\rho}^{W_{L,\sigma}^2}+p_{\rho}^{W_{H,\mu}^3}\right)\right) \quad (854)$$


---

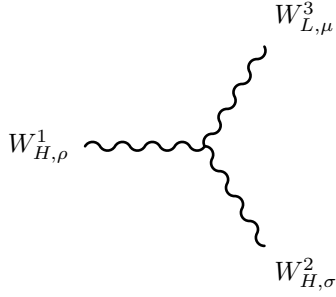

$$\left(g_{A2}^{-2}g_{B2}^3\left(\frac{gA2^2}{gA2^2+gB2^2}\right)^{3/2}+g_{A2}^3g_{B2}\frac{1}{\left(gA2^2+gB2^2\right)^{3/2}}\right)\left(g_{\rho\mu}\left(-p_{\sigma}^{W_{L,\mu}^3}+p_{\sigma}^{W_{H,\rho}^1}\right)+g_{\rho\sigma}\left(-p_{\mu}^{W_{H,\rho}^1}+p_{\mu}^{W_{H,\sigma}^2}\right)+g_{\sigma\mu}\left(-p_{\rho}^{W_{H,\sigma}^2}+p_{\rho}^{W_{L,\mu}^3}\right)\right) \quad (855)$$


---

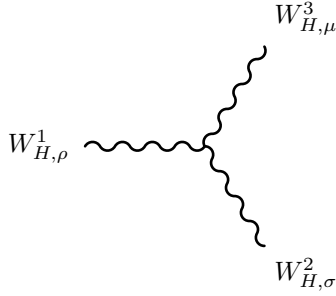

$$\frac{1}{\left(gA2^2+gB2^2\right)^{3/2}}\left(-g_{A2}\left(\frac{gA2^2}{gA2^2+gB2^2}\right)^{3/2}\left(gA2^2+gB2^2\right)^{3/2}+g_{B2}^4\right)\left(g_{\rho\mu}\left(-p_{\sigma}^{W_{H,\mu}^3}+p_{\sigma}^{W_{H,\rho}^1}\right)+g_{\rho\sigma}\left(-p_{\mu}^{W_{H,\rho}^1}+p_{\mu}^{W_{H,\sigma}^2}\right)+g_{\sigma\mu}\left(-p_{\rho}^{W_{H,\sigma}^2}+p_{\rho}^{W_{H,\mu}^3}\right)\right) \quad (856)$$


---

## 9.7 Four Scalar-Interaction

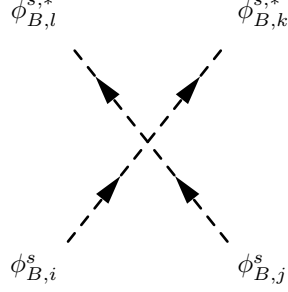

$$\begin{aligned}
& -ig_{B2}^2 \left( -B_{A,i2}^{s,*} \left( -2B_{A,j2}^{s,*} B_{A,k2}^s B_{A,l2}^s + B_{A,j1}^{s,*} \left( B_{A,k1}^s B_{A,l2}^s + B_{A,k2}^s B_{A,l1}^s \right) \right) \right. \\
& \left. + B_{A,i1}^{s,*} \left( 2B_{A,j1}^{s,*} B_{A,k1}^s B_{A,l1}^s - B_{A,j2}^{s,*} \left( B_{A,k1}^s B_{A,l2}^s + B_{A,k2}^s B_{A,l1}^s \right) \right) \right) \quad (857)
\end{aligned}$$


---

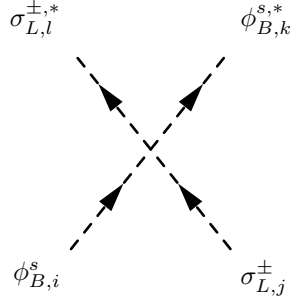

$$\begin{aligned}
& -\frac{i}{2} \left( B_{A,i2}^{s,*} B_{A,k2}^s \left( - \left( -2|Y_A|^2 + g_{B2}^2 \right) Z_{Ls,j1}^{od,*} Z_{Ls,l1}^{od} - \left( -2|Y_A|^2 + g_{B2}^2 \right) Z_{Ls,j2}^{od,*} Z_{Ls,l2}^{od} \right. \right. \\
& \left. \left. + g_{B2}^2 \left( Z_{Ls,j3}^{od,*} Z_{Ls,l3}^{od} + Z_{Ls,j4}^{od,*} Z_{Ls,l4}^{od} \right) \right) \right) \\
& + B_{A,i1}^{s,*} B_{A,k1}^s \left( - \left( -2|Y_A|^2 + g_{B2}^2 \right) \left( Z_{Ls,j3}^{od,*} Z_{Ls,l3}^{od} + Z_{Ls,j4}^{od,*} Z_{Ls,l4}^{od} \right) + g_{B2}^2 Z_{Ls,j1}^{od,*} Z_{Ls,l1}^{od} + g_{B2}^2 Z_{Ls,j2}^{od,*} Z_{Ls,l2}^{od} \right) \quad (858)
\end{aligned}$$


---

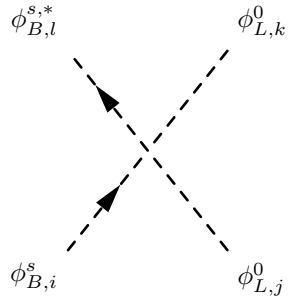

$$\begin{aligned}
& i \left( B_{A,i1}^{s,*} \left( \left( -2|Y_A|^2 + g_{B2}^2 \right) Z_{Ls,j1}^{DR,*} Z_{Ls,k1}^{DR,*} - g_{B2}^2 Z_{Ls,j2}^{DR,*} Z_{Ls,k2}^{DR,*} - g_{B2}^2 Z_{Ls,j3}^{DR,*} Z_{Ls,k3}^{DR,*} + g_{B2}^2 Z_{Ls,j4}^{DR,*} Z_{Ls,k4}^{DR,*} \right. \right. \\
& \quad \left. \left. - 2|Y_A|^2 Z_{Ls,j4}^{DR,*} Z_{Ls,k4}^{DR,*} \right) B_{A,l1}^s \right. \\
& \quad \left. - B_{A,i2}^{s,*} \left( g_{B2}^2 Z_{Ls,j1}^{DR,*} Z_{Ls,k1}^{DR,*} - \left( -2|Y_A|^2 + g_{B2}^2 \right) Z_{Ls,j2}^{DR,*} Z_{Ls,k2}^{DR,*} - g_{B2}^2 Z_{Ls,j3}^{DR,*} Z_{Ls,k3}^{DR,*} \right. \right. \\
& \quad \left. \left. + 2|Y_A|^2 Z_{Ls,j3}^{DR,*} Z_{Ls,k3}^{DR,*} + g_{B2}^2 Z_{Ls,j4}^{DR,*} Z_{Ls,k4}^{DR,*} \right) B_{A,l2}^s \right) \quad (859)
\end{aligned}$$


---

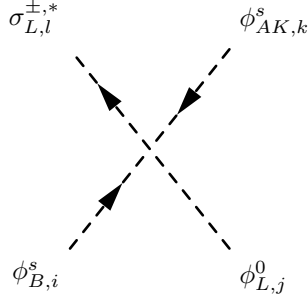

$$\begin{aligned}
& -\frac{i}{2} B_{A,i2}^{s,*} \left( \sqrt{2} g_{B2}^2 Z_{AK,k2}^{s,*} \left( -Z_{Ls,j1}^{DR,*} Z_{Ls,l1}^{od} + Z_{Ls,j2}^{DR,*} Z_{Ls,l3}^{od} - Z_{Ls,j3}^{DR,*} Z_{Ls,l4}^{od} + Z_{Ls,j4}^{DR,*} Z_{Ls,l2}^{od} \right) \right. \\
& \quad + Y_A^* \left( \sqrt{2} Y_A Z_{AK,k2}^{s,*} \left( Z_{Ls,j1}^{DR,*} Z_{Ls,l1}^{od} - Z_{Ls,j2}^{DR,*} Z_{Ls,l3}^{od} + Z_{Ls,j3}^{DR,*} Z_{Ls,l4}^{od} - Z_{Ls,j4}^{DR,*} Z_{Ls,l2}^{od} \right) \right. \\
& \quad \left. \left. + Y_K Z_{AK,k1}^{s,*} \left( Z_{Ls,j1}^{DR,*} Z_{Ls,l1}^{od} + Z_{Ls,j2}^{DR,*} Z_{Ls,l3}^{od} + Z_{Ls,j3}^{DR,*} Z_{Ls,l4}^{od} + Z_{Ls,j4}^{DR,*} Z_{Ls,l2}^{od} \right) \right) \right) \quad (860)
\end{aligned}$$


---

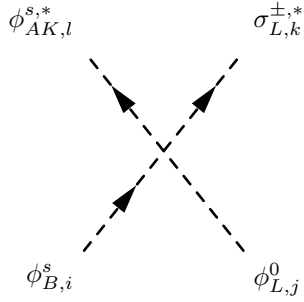

$$\begin{aligned}
& -\frac{i}{2} B_{A,i1}^{s,*} \left( \sqrt{2} \left( -|Y_A|^2 + g_{B2}^2 \right) Z_{AK,l2}^s \left( Z_{Ls,j1}^{DR,*} Z_{Ls,k1}^{od} - Z_{Ls,j2}^{DR,*} Z_{Ls,k3}^{od} + Z_{Ls,j3}^{DR,*} Z_{Ls,k4}^{od} - Z_{Ls,j4}^{DR,*} Z_{Ls,k2}^{od} \right) \right. \\
& \quad \left. + Y_A Y_K^* Z_{AK,l1}^s \left( Z_{Ls,j1}^{DR,*} Z_{Ls,k1}^{od} + Z_{Ls,j2}^{DR,*} Z_{Ls,k3}^{od} + Z_{Ls,j3}^{DR,*} Z_{Ls,k4}^{od} + Z_{Ls,j4}^{DR,*} Z_{Ls,k2}^{od} \right) \right) \quad (861)
\end{aligned}$$


---

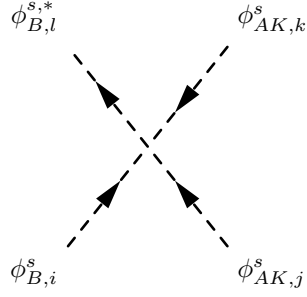

$$2ig_{B2}^2 Z_{AK,j2}^{s,*} Z_{AK,k2}^{s,*} B_{A,i2}^{s,*} B_{A,l1}^s \quad (862)$$


---

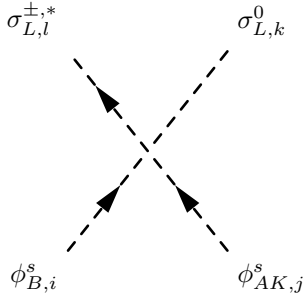

$$\begin{aligned} & \frac{1}{2} B_{A,i2}^{s,*} \left( \sqrt{2} g_{B2}^2 Z_{AK,j2}^{s,*} \left( -Z_{Ls,k1}^{Di,*} Z_{Ls,l1}^{od} - Z_{Ls,k2}^{Di,*} Z_{Ls,l3}^{od} + Z_{Ls,k3}^{Di,*} Z_{Ls,l4}^{od} + Z_{Ls,k4}^{Di,*} Z_{Ls,l2}^{od} \right) \right. \\ & + Y_A^* \left( Y_K Z_{AK,j1}^{s,*} \left( Z_{Ls,k1}^{Di,*} Z_{Ls,l1}^{od} - Z_{Ls,k2}^{Di,*} Z_{Ls,l3}^{od} - Z_{Ls,k3}^{Di,*} Z_{Ls,l4}^{od} + Z_{Ls,k4}^{Di,*} Z_{Ls,l2}^{od} \right) \right. \\ & \left. \left. + \sqrt{2} Y_A Z_{AK,j2}^{s,*} \left( Z_{Ls,k1}^{Di,*} Z_{Ls,l1}^{od} + Z_{Ls,k2}^{Di,*} Z_{Ls,l3}^{od} - Z_{Ls,k3}^{Di,*} Z_{Ls,l4}^{od} - Z_{Ls,k4}^{Di,*} Z_{Ls,l2}^{od} \right) \right) \right) \quad (863) \end{aligned}$$


---

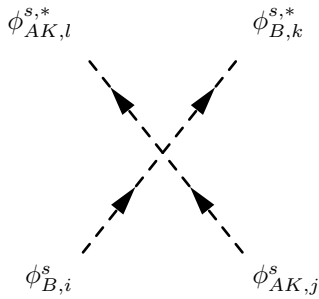

$$-ig_{B2}^2 Z_{AK,j2}^{s,*} Z_{AK,l2}^s \left( B_{A,i1}^{s,*} B_{A,k1}^s + B_{A,i2}^{s,*} B_{A,k2}^s \right) \quad (864)$$


---

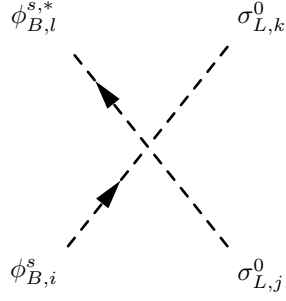

$$\begin{aligned}
& i \left( B_{A,i1}^{s,*} \left( \left( -2|Y_A|^2 + g_{B2}^2 \right) Z_{Ls,j1}^{Di,*} Z_{Ls,k1}^{Di,*} - g_{B2}^2 Z_{Ls,j2}^{Di,*} Z_{Ls,k2}^{Di,*} - g_{B2}^2 Z_{Ls,j3}^{Di,*} Z_{Ls,k3}^{Di,*} + g_{B2}^2 Z_{Ls,j4}^{Di,*} Z_{Ls,k4}^{Di,*} \right. \right. \\
& \quad \left. \left. - 2|Y_A|^2 Z_{Ls,j4}^{Di,*} Z_{Ls,k4}^{Di,*} \right) B_{A,l1}^s \right. \\
& \quad \left. - B_{A,i2}^{s,*} \left( g_{B2}^2 Z_{Ls,j1}^{Di,*} Z_{Ls,k1}^{Di,*} - \left( -2|Y_A|^2 + g_{B2}^2 \right) Z_{Ls,j2}^{Di,*} Z_{Ls,k2}^{Di,*} - g_{B2}^2 Z_{Ls,j3}^{Di,*} Z_{Ls,k3}^{Di,*} \right. \right. \\
& \quad \left. \left. + 2|Y_A|^2 Z_{Ls,j3}^{Di,*} Z_{Ls,k3}^{Di,*} + g_{B2}^2 Z_{Ls,j4}^{Di,*} Z_{Ls,k4}^{Di,*} \right) B_{A,l2}^s \right) \quad (865)
\end{aligned}$$


---

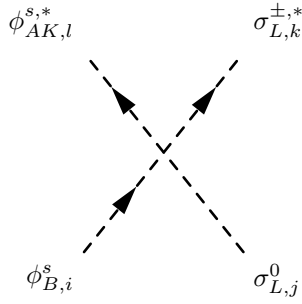

$$\begin{aligned}
& \frac{1}{2} B_{A,i1}^{s,*} \left( Y_A Y_K^* Z_{AK,l1}^s \left( Z_{Ls,j1}^{Di,*} Z_{Ls,k1}^{od} - Z_{Ls,j2}^{Di,*} Z_{Ls,k3}^{od} - Z_{Ls,j3}^{Di,*} Z_{Ls,k4}^{od} + Z_{Ls,j4}^{Di,*} Z_{Ls,k2}^{od} \right) \right. \\
& \quad \left. + \sqrt{2} \left( -|Y_A|^2 + g_{B2}^2 \right) Z_{AK,l2}^s \left( Z_{Ls,j1}^{Di,*} Z_{Ls,k1}^{od} + Z_{Ls,j2}^{Di,*} Z_{Ls,k3}^{od} - Z_{Ls,j3}^{Di,*} Z_{Ls,k4}^{od} - Z_{Ls,j4}^{Di,*} Z_{Ls,k2}^{od} \right) \right) \quad (866)
\end{aligned}$$


---

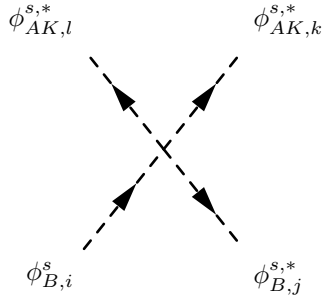

$$2ig_{B2}^2 B_{A,i1}^{s,*} Z_{AK,k2}^s Z_{AK,l2}^s B_{A,j2}^s \quad (867)$$

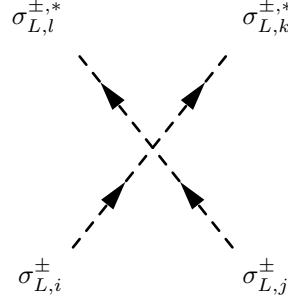

$$\begin{aligned}
& \frac{i}{4} \left( g_{A1}^2 Z_{Ls,i3}^{od,*} Z_{Ls,j1}^{od,*} Z_{Ls,k3}^{od} Z_{Ls,l1}^{od} + g_{A2}^2 Z_{Ls,i3}^{od,*} Z_{Ls,j1}^{od,*} Z_{Ls,k3}^{od} Z_{Ls,l1}^{od} \right. \\
& + g_{B1}^2 Z_{Ls,i3}^{od,*} Z_{Ls,j1}^{od,*} Z_{Ls,k3}^{od} Z_{Ls,l1}^{od} + g_{B2}^2 Z_{Ls,i3}^{od,*} Z_{Ls,j1}^{od,*} Z_{Ls,k3}^{od} Z_{Ls,l1}^{od} \\
& - 2|Y_A|^2 Z_{Ls,i3}^{od,*} Z_{Ls,j1}^{od,*} Z_{Ls,k3}^{od} Z_{Ls,l1}^{od} - |Y_K|^2 Z_{Ls,i3}^{od,*} Z_{Ls,j1}^{od,*} Z_{Ls,k3}^{od} Z_{Ls,l1}^{od} \\
& - g_{A1}^2 Z_{Ls,i4}^{od,*} Z_{Ls,j1}^{od,*} Z_{Ls,k4}^{od} Z_{Ls,l1}^{od} + g_{A2}^2 Z_{Ls,i4}^{od,*} Z_{Ls,j1}^{od,*} Z_{Ls,k4}^{od} Z_{Ls,l1}^{od} \\
& - g_{B1}^2 Z_{Ls,i4}^{od,*} Z_{Ls,j1}^{od,*} Z_{Ls,k4}^{od} Z_{Ls,l1}^{od} + g_{B2}^2 Z_{Ls,i4}^{od,*} Z_{Ls,j1}^{od,*} Z_{Ls,k4}^{od} Z_{Ls,l1}^{od} \\
& + 2|Y_A|^2 Z_{Ls,i3}^{od,*} Z_{Ls,j2}^{od,*} Z_{Ls,k4}^{od} Z_{Ls,l1}^{od} - |Y_K|^2 Z_{Ls,i3}^{od,*} Z_{Ls,j2}^{od,*} Z_{Ls,k4}^{od} Z_{Ls,l1}^{od} \\
& + 2|Y_A|^2 Z_{Ls,i4}^{od,*} Z_{Ls,j1}^{od,*} Z_{Ls,k3}^{od} Z_{Ls,l2}^{od} - |Y_K|^2 Z_{Ls,i4}^{od,*} Z_{Ls,j1}^{od,*} Z_{Ls,k3}^{od} Z_{Ls,l2}^{od} \\
& - g_{A1}^2 Z_{Ls,i3}^{od,*} Z_{Ls,j2}^{od,*} Z_{Ls,k3}^{od} Z_{Ls,l2}^{od} + g_{A2}^2 Z_{Ls,i3}^{od,*} Z_{Ls,j2}^{od,*} Z_{Ls,k3}^{od} Z_{Ls,l2}^{od} \\
& - g_{B1}^2 Z_{Ls,i3}^{od,*} Z_{Ls,j2}^{od,*} Z_{Ls,k3}^{od} Z_{Ls,l2}^{od} + g_{B2}^2 Z_{Ls,i3}^{od,*} Z_{Ls,j2}^{od,*} Z_{Ls,k3}^{od} Z_{Ls,l2}^{od} \\
& + g_{A1}^2 Z_{Ls,i4}^{od,*} Z_{Ls,j2}^{od,*} Z_{Ls,k4}^{od} Z_{Ls,l2}^{od} + g_{A2}^2 Z_{Ls,i4}^{od,*} Z_{Ls,j2}^{od,*} Z_{Ls,k4}^{od} Z_{Ls,l2}^{od} \\
& + g_{B1}^2 Z_{Ls,i4}^{od,*} Z_{Ls,j2}^{od,*} Z_{Ls,k4}^{od} Z_{Ls,l2}^{od} + g_{B2}^2 Z_{Ls,i4}^{od,*} Z_{Ls,j2}^{od,*} Z_{Ls,k4}^{od} Z_{Ls,l2}^{od} \\
& - 2|Y_A|^2 Z_{Ls,i4}^{od,*} Z_{Ls,j2}^{od,*} Z_{Ls,k4}^{od} Z_{Ls,l2}^{od} - |Y_K|^2 Z_{Ls,i4}^{od,*} Z_{Ls,j2}^{od,*} Z_{Ls,k4}^{od} Z_{Ls,l2}^{od} \\
& + g_{A1}^2 Z_{Ls,i3}^{od,*} Z_{Ls,j1}^{od,*} Z_{Ls,k1}^{od} Z_{Ls,l3}^{od} + g_{A2}^2 Z_{Ls,i3}^{od,*} Z_{Ls,j1}^{od,*} Z_{Ls,k1}^{od} Z_{Ls,l3}^{od} \\
& + g_{B1}^2 Z_{Ls,i3}^{od,*} Z_{Ls,j1}^{od,*} Z_{Ls,k1}^{od} Z_{Ls,l3}^{od} + g_{B2}^2 Z_{Ls,i3}^{od,*} Z_{Ls,j1}^{od,*} Z_{Ls,k1}^{od} Z_{Ls,l3}^{od} \\
& - 2|Y_A|^2 Z_{Ls,i3}^{od,*} Z_{Ls,j1}^{od,*} Z_{Ls,k1}^{od} Z_{Ls,l3}^{od} - |Y_K|^2 Z_{Ls,i3}^{od,*} Z_{Ls,j1}^{od,*} Z_{Ls,k1}^{od} Z_{Ls,l3}^{od} \\
& + 2|Y_A|^2 Z_{Ls,i4}^{od,*} Z_{Ls,j1}^{od,*} Z_{Ls,k2}^{od} Z_{Ls,l3}^{od} - |Y_K|^2 Z_{Ls,i4}^{od,*} Z_{Ls,j1}^{od,*} Z_{Ls,k2}^{od} Z_{Ls,l3}^{od} \\
& - g_{A1}^2 Z_{Ls,i3}^{od,*} Z_{Ls,j2}^{od,*} Z_{Ls,k2}^{od} Z_{Ls,l3}^{od} + g_{A2}^2 Z_{Ls,i3}^{od,*} Z_{Ls,j2}^{od,*} Z_{Ls,k2}^{od} Z_{Ls,l3}^{od} \\
& - g_{B1}^2 Z_{Ls,i3}^{od,*} Z_{Ls,j2}^{od,*} Z_{Ls,k2}^{od} Z_{Ls,l3}^{od} + g_{B2}^2 Z_{Ls,i3}^{od,*} Z_{Ls,j2}^{od,*} Z_{Ls,k2}^{od} Z_{Ls,l3}^{od} \\
& - 2g_{A1}^2 Z_{Ls,i3}^{od,*} Z_{Ls,j3}^{od,*} Z_{Ls,k3}^{od} Z_{Ls,l3}^{od} - 2g_{A2}^2 Z_{Ls,i3}^{od,*} Z_{Ls,j3}^{od,*} Z_{Ls,k3}^{od} Z_{Ls,l3}^{od} \\
& - 2g_{B1}^2 Z_{Ls,i3}^{od,*} Z_{Ls,j3}^{od,*} Z_{Ls,k3}^{od} Z_{Ls,l3}^{od} - 2g_{B2}^2 Z_{Ls,i3}^{od,*} Z_{Ls,j3}^{od,*} Z_{Ls,k3}^{od} Z_{Ls,l3}^{od} \\
& + g_{A1}^2 Z_{Ls,i4}^{od,*} Z_{Ls,j3}^{od,*} Z_{Ls,k4}^{od} Z_{Ls,l3}^{od} - g_{A2}^2 Z_{Ls,i4}^{od,*} Z_{Ls,j3}^{od,*} Z_{Ls,k4}^{od} Z_{Ls,l3}^{od}
\end{aligned}$$

$$\begin{aligned}
& + g_{B1}^2 Z_{Ls,i4}^{od,*} Z_{Ls,j3}^{od,*} Z_{Ls,k4}^{od} Z_{Ls,l3}^{od} - g_{B2}^2 Z_{Ls,i4}^{od,*} Z_{Ls,j3}^{od,*} Z_{Ls,k4}^{od} Z_{Ls,l3}^{od} \\
& + g_{A1}^2 Z_{Ls,i3}^{od,*} Z_{Ls,j4}^{od,*} Z_{Ls,k4}^{od} Z_{Ls,l3}^{od} - g_{A2}^2 Z_{Ls,i3}^{od,*} Z_{Ls,j4}^{od,*} Z_{Ls,k4}^{od} Z_{Ls,l3}^{od} \\
& + g_{B1}^2 Z_{Ls,i3}^{od,*} Z_{Ls,j4}^{od,*} Z_{Ls,k4}^{od} Z_{Ls,l3}^{od} - g_{B2}^2 Z_{Ls,i3}^{od,*} Z_{Ls,j4}^{od,*} Z_{Ls,k4}^{od} Z_{Ls,l3}^{od} \\
& - g_{A1}^2 Z_{Ls,i4}^{od,*} Z_{Ls,j2}^{od,*} Z_{Ls,k1}^{od} Z_{Ls,l4}^{od} + g_{A2}^2 Z_{Ls,i4}^{od,*} Z_{Ls,j1}^{od,*} Z_{Ls,k1}^{od} Z_{Ls,l4}^{od} \\
& - g_{B1}^2 Z_{Ls,i4}^{od,*} Z_{Ls,j1}^{od,*} Z_{Ls,k1}^{od} Z_{Ls,l4}^{od} + g_{B2}^2 Z_{Ls,i4}^{od,*} Z_{Ls,j1}^{od,*} Z_{Ls,k1}^{od} Z_{Ls,l4}^{od} \\
& + 2|Y_A|^2 Z_{Ls,i3}^{od,*} Z_{Ls,j2}^{od,*} Z_{Ls,k1}^{od} Z_{Ls,l4}^{od} - |Y_K|^2 Z_{Ls,i3}^{od,*} Z_{Ls,j2}^{od,*} Z_{Ls,k1}^{od} Z_{Ls,l4}^{od} \\
& + g_{A1}^2 Z_{Ls,i4}^{od,*} Z_{Ls,j2}^{od,*} Z_{Ls,k2}^{od} Z_{Ls,l4}^{od} + g_{A2}^2 Z_{Ls,i4}^{od,*} Z_{Ls,j2}^{od,*} Z_{Ls,k2}^{od} Z_{Ls,l4}^{od} \\
& + g_{B1}^2 Z_{Ls,i4}^{od,*} Z_{Ls,j2}^{od,*} Z_{Ls,k2}^{od} Z_{Ls,l4}^{od} + g_{B2}^2 Z_{Ls,i4}^{od,*} Z_{Ls,j2}^{od,*} Z_{Ls,k2}^{od} Z_{Ls,l4}^{od} \\
& - 2|Y_A|^2 Z_{Ls,i4}^{od,*} Z_{Ls,j2}^{od,*} Z_{Ls,k2}^{od} Z_{Ls,l4}^{od} - |Y_K|^2 Z_{Ls,i4}^{od,*} Z_{Ls,j2}^{od,*} Z_{Ls,k2}^{od} Z_{Ls,l4}^{od} \\
& + g_{A1}^2 Z_{Ls,i4}^{od,*} Z_{Ls,j3}^{od,*} Z_{Ls,k3}^{od} Z_{Ls,l4}^{od} - g_{A2}^2 Z_{Ls,i4}^{od,*} Z_{Ls,j3}^{od,*} Z_{Ls,k3}^{od} Z_{Ls,l4}^{od} \\
& + g_{B1}^2 Z_{Ls,i4}^{od,*} Z_{Ls,j3}^{od,*} Z_{Ls,k3}^{od} Z_{Ls,l4}^{od} - g_{B2}^2 Z_{Ls,i4}^{od,*} Z_{Ls,j3}^{od,*} Z_{Ls,k3}^{od} Z_{Ls,l4}^{od} \\
& + g_{A1}^2 Z_{Ls,i3}^{od,*} Z_{Ls,j4}^{od,*} Z_{Ls,k3}^{od} Z_{Ls,l4}^{od} - g_{A2}^2 Z_{Ls,i3}^{od,*} Z_{Ls,j4}^{od,*} Z_{Ls,k3}^{od} Z_{Ls,l4}^{od} \\
& + g_{B1}^2 Z_{Ls,i3}^{od,*} Z_{Ls,j4}^{od,*} Z_{Ls,k3}^{od} Z_{Ls,l4}^{od} - g_{B2}^2 Z_{Ls,i3}^{od,*} Z_{Ls,j4}^{od,*} Z_{Ls,k3}^{od} Z_{Ls,l4}^{od} \\
& - 2g_{A1}^2 Z_{Ls,i4}^{od,*} Z_{Ls,j4}^{od,*} Z_{Ls,k4}^{od} Z_{Ls,l4}^{od} - 2g_{A2}^2 Z_{Ls,i4}^{od,*} Z_{Ls,j4}^{od,*} Z_{Ls,k4}^{od} Z_{Ls,l4}^{od} \\
& - 2g_{B1}^2 Z_{Ls,i4}^{od,*} Z_{Ls,j4}^{od,*} Z_{Ls,k4}^{od} Z_{Ls,l4}^{od} - 2g_{B2}^2 Z_{Ls,i4}^{od,*} Z_{Ls,j4}^{od,*} Z_{Ls,k4}^{od} Z_{Ls,l4}^{od} \\
& + Z_{Ls,i1}^{od,*} \left( -2 \left( g_{A1}^2 + g_{A2}^2 + g_{B1}^2 + g_{B2}^2 \right) Z_{Ls,j1}^{od,*} Z_{Ls,k1}^{od} Z_{Ls,l1}^{od} + g_{A1}^2 Z_{Ls,j3}^{od,*} Z_{Ls,k3}^{od} Z_{Ls,l1}^{od} + g_{A2}^2 Z_{Ls,j3}^{od,*} Z_{Ls,k3}^{od} Z_{Ls,l1}^{od} \right. \\
& + g_{B1}^2 Z_{Ls,j3}^{od,*} Z_{Ls,k3}^{od} Z_{Ls,l1}^{od} + g_{B2}^2 Z_{Ls,j3}^{od,*} Z_{Ls,k3}^{od} Z_{Ls,l1}^{od} - 2|Y_A|^2 Z_{Ls,j3}^{od,*} Z_{Ls,k3}^{od} Z_{Ls,l1}^{od} \\
& - |Y_K|^2 Z_{Ls,j3}^{od,*} Z_{Ls,k3}^{od} Z_{Ls,l1}^{od} - g_{A1}^2 Z_{Ls,j4}^{od,*} Z_{Ls,k4}^{od} Z_{Ls,l1}^{od} + g_{A2}^2 Z_{Ls,j4}^{od,*} Z_{Ls,k4}^{od} Z_{Ls,l1}^{od} \\
& - g_{B1}^2 Z_{Ls,j4}^{od,*} Z_{Ls,k4}^{od} Z_{Ls,l1}^{od} + g_{B2}^2 Z_{Ls,j4}^{od,*} Z_{Ls,k4}^{od} Z_{Ls,l1}^{od} + 2|Y_A|^2 Z_{Ls,j4}^{od,*} Z_{Ls,k3}^{od} Z_{Ls,l2}^{od} \\
& - |Y_K|^2 Z_{Ls,j4}^{od,*} Z_{Ls,k3}^{od} Z_{Ls,l2}^{od} + \left( -g_{A2}^2 - g_{B2}^2 + g_{A1}^2 + g_{B1}^2 \right) Z_{Ls,j2}^{od,*} \left( Z_{Ls,k1}^{od} Z_{Ls,l2}^{od} + Z_{Ls,k2}^{od} Z_{Ls,l1}^{od} \right) \\
& + g_{A1}^2 Z_{Ls,j3}^{od,*} Z_{Ls,k1}^{od} Z_{Ls,l3}^{od} + g_{A2}^2 Z_{Ls,j3}^{od,*} Z_{Ls,k1}^{od} Z_{Ls,l3}^{od} + g_{B1}^2 Z_{Ls,j3}^{od,*} Z_{Ls,k1}^{od} Z_{Ls,l3}^{od} \\
& + g_{B2}^2 Z_{Ls,j3}^{od,*} Z_{Ls,k1}^{od} Z_{Ls,l3}^{od} - 2|Y_A|^2 Z_{Ls,j3}^{od,*} Z_{Ls,k1}^{od} Z_{Ls,l3}^{od} - |Y_K|^2 Z_{Ls,j3}^{od,*} Z_{Ls,k1}^{od} Z_{Ls,l3}^{od} \\
& + 2|Y_A|^2 Z_{Ls,j4}^{od,*} Z_{Ls,k2}^{od} Z_{Ls,l3}^{od} - |Y_K|^2 Z_{Ls,j4}^{od,*} Z_{Ls,k2}^{od} Z_{Ls,l3}^{od} - g_{A1}^2 Z_{Ls,j4}^{od,*} Z_{Ls,k1}^{od} Z_{Ls,l4}^{od} \\
& + g_{A2}^2 Z_{Ls,j4}^{od,*} Z_{Ls,k1}^{od} Z_{Ls,l4}^{od} - g_{B1}^2 Z_{Ls,j4}^{od,*} Z_{Ls,k1}^{od} Z_{Ls,l4}^{od} + g_{B2}^2 Z_{Ls,j4}^{od,*} Z_{Ls,k1}^{od} Z_{Ls,l4}^{od} \left. \right) \\
& + Z_{Ls,i2}^{od,*} \left( -|Y_K|^2 Z_{Ls,j3}^{od,*} Z_{Ls,k4}^{od} Z_{Ls,l1}^{od} - 2g_{A1}^2 Z_{Ls,j2}^{od,*} Z_{Ls,k2}^{od} Z_{Ls,l2}^{od} - 2g_{A2}^2 Z_{Ls,j2}^{od,*} Z_{Ls,k2}^{od} Z_{Ls,l2}^{od} \right. \\
& - 2g_{B1}^2 Z_{Ls,j2}^{od,*} Z_{Ls,k2}^{od} Z_{Ls,l2}^{od} - 2g_{B2}^2 Z_{Ls,j2}^{od,*} Z_{Ls,k2}^{od} Z_{Ls,l2}^{od} - g_{A1}^2 Z_{Ls,j3}^{od,*} Z_{Ls,k3}^{od} Z_{Ls,l2}^{od} \\
& + g_{A2}^2 Z_{Ls,j3}^{od,*} Z_{Ls,k3}^{od} Z_{Ls,l2}^{od} - g_{B1}^2 Z_{Ls,j3}^{od,*} Z_{Ls,k3}^{od} Z_{Ls,l2}^{od} + g_{B2}^2 Z_{Ls,j3}^{od,*} Z_{Ls,k3}^{od} Z_{Ls,l2}^{od} \\
& + g_{A1}^2 Z_{Ls,j4}^{od,*} Z_{Ls,k4}^{od} Z_{Ls,l2}^{od} + g_{A2}^2 Z_{Ls,j4}^{od,*} Z_{Ls,k4}^{od} Z_{Ls,l2}^{od} + g_{B1}^2 Z_{Ls,j4}^{od,*} Z_{Ls,k4}^{od} Z_{Ls,l2}^{od} \\
& \left. + g_{B2}^2 Z_{Ls,j4}^{od,*} Z_{Ls,k4}^{od} Z_{Ls,l2}^{od} - |Y_K|^2 Z_{Ls,j4}^{od,*} Z_{Ls,k4}^{od} Z_{Ls,l2}^{od} \right)
\end{aligned}$$



$$\begin{aligned}
& + \left( -g_{A2}^2 - g_{B2}^2 + g_{A1}^2 + g_{B1}^2 \right) Z_{Ls,j1}^{od,*} \left( Z_{Ls,k1}^{od} Z_{Ls,l2}^{od} + Z_{Ls,k2}^{od} Z_{Ls,l1}^{od} \right) - g_{A1}^2 Z_{Ls,j3}^{od,*} Z_{Ls,k2}^{od} Z_{Ls,l3}^{od} \\
& + g_{A2}^2 Z_{Ls,j3}^{od,*} Z_{Ls,k2}^{od} Z_{Ls,l3}^{od} - g_{B1}^2 Z_{Ls,j3}^{od,*} Z_{Ls,k2}^{od} Z_{Ls,l3}^{od} + g_{B2}^2 Z_{Ls,j3}^{od,*} Z_{Ls,k2}^{od} Z_{Ls,l3}^{od} \\
& - |Y_K|^2 Z_{Ls,j3}^{od,*} Z_{Ls,k1}^{od} Z_{Ls,l4}^{od} + g_{A1}^2 Z_{Ls,j4}^{od,*} Z_{Ls,k2}^{od} Z_{Ls,l4}^{od} + g_{A2}^2 Z_{Ls,j4}^{od,*} Z_{Ls,k2}^{od} Z_{Ls,l4}^{od} \\
& + g_{B1}^2 Z_{Ls,j4}^{od,*} Z_{Ls,k2}^{od} Z_{Ls,l4}^{od} + g_{B2}^2 Z_{Ls,j4}^{od,*} Z_{Ls,k2}^{od} Z_{Ls,l4}^{od} - |Y_K|^2 Z_{Ls,j4}^{od,*} Z_{Ls,k2}^{od} Z_{Ls,l4}^{od} \\
& + 2|Y_A|^2 \left( Z_{Ls,j3}^{od,*} \left( Z_{Ls,k1}^{od} Z_{Ls,l4}^{od} + Z_{Ls,k4}^{od} Z_{Ls,l1}^{od} \right) - Z_{Ls,j4}^{od,*} \left( Z_{Ls,k2}^{od} Z_{Ls,l4}^{od} + Z_{Ls,k4}^{od} Z_{Ls,l2}^{od} \right) \right) \Big) \Big) \quad (868)
\end{aligned}$$

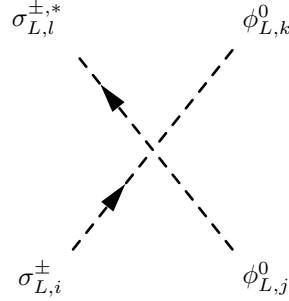

$$\begin{aligned}
& - \frac{i}{4} \left( 2g_{A2}^2 Z_{Ls,i4}^{od,*} Z_{Ls,j3}^{DR,*} Z_{Ls,k1}^{DR,*} Z_{Ls,l1}^{od} + 2g_{B2}^2 Z_{Ls,i4}^{od,*} Z_{Ls,j3}^{DR,*} Z_{Ls,k1}^{DR,*} Z_{Ls,l1}^{od} \right. \\
& - 2g_{B2}^2 Z_{Ls,i2}^{od,*} Z_{Ls,j4}^{DR,*} Z_{Ls,k1}^{DR,*} Z_{Ls,l1}^{od} - 2g_{A2}^2 Z_{Ls,i2}^{od,*} Z_{Ls,j3}^{DR,*} Z_{Ls,k2}^{DR,*} Z_{Ls,l1}^{od} \\
& + 4|Y_A|^2 Z_{Ls,i2}^{od,*} Z_{Ls,j3}^{DR,*} Z_{Ls,k2}^{DR,*} Z_{Ls,l1}^{od} + 2g_{A2}^2 Z_{Ls,i4}^{od,*} Z_{Ls,j1}^{DR,*} Z_{Ls,k3}^{DR,*} Z_{Ls,l1}^{od} \\
& + 2g_{B2}^2 Z_{Ls,i4}^{od,*} Z_{Ls,j1}^{DR,*} Z_{Ls,k3}^{DR,*} Z_{Ls,l1}^{od} - 2g_{A2}^2 Z_{Ls,i2}^{od,*} Z_{Ls,j2}^{DR,*} Z_{Ls,k3}^{DR,*} Z_{Ls,l1}^{od} \\
& + 4|Y_A|^2 Z_{Ls,i2}^{od,*} Z_{Ls,j2}^{DR,*} Z_{Ls,k3}^{DR,*} Z_{Ls,l1}^{od} - 2g_{B2}^2 Z_{Ls,i2}^{od,*} Z_{Ls,j1}^{DR,*} Z_{Ls,k4}^{DR,*} Z_{Ls,l1}^{od} \\
& - 2g_{A1}^2 Z_{Ls,i2}^{od,*} Z_{Ls,j1}^{DR,*} Z_{Ls,k1}^{DR,*} Z_{Ls,l2}^{od} + 2g_{A2}^2 Z_{Ls,i2}^{od,*} Z_{Ls,j1}^{DR,*} Z_{Ls,k1}^{DR,*} Z_{Ls,l2}^{od} \\
& - 2g_{B1}^2 Z_{Ls,i2}^{od,*} Z_{Ls,j1}^{DR,*} Z_{Ls,k1}^{DR,*} Z_{Ls,l2}^{od} - 2g_{B2}^2 Z_{Ls,i2}^{od,*} Z_{Ls,j1}^{DR,*} Z_{Ls,k1}^{DR,*} Z_{Ls,l2}^{od} \\
& - 2g_{A2}^2 Z_{Ls,i4}^{od,*} Z_{Ls,j2}^{DR,*} Z_{Ls,k1}^{DR,*} Z_{Ls,l2}^{od} + 2|Y_A|^2 Z_{Ls,i4}^{od,*} Z_{Ls,j2}^{DR,*} Z_{Ls,k1}^{DR,*} Z_{Ls,l2}^{od} \\
& + |Y_K|^2 Z_{Ls,i4}^{od,*} Z_{Ls,j2}^{DR,*} Z_{Ls,k1}^{DR,*} Z_{Ls,l2}^{od} - 2g_{A2}^2 Z_{Ls,i4}^{od,*} Z_{Ls,j1}^{DR,*} Z_{Ls,k2}^{DR,*} Z_{Ls,l2}^{od} \\
& + 2|Y_A|^2 Z_{Ls,i4}^{od,*} Z_{Ls,j1}^{DR,*} Z_{Ls,k2}^{DR,*} Z_{Ls,l2}^{od} + |Y_K|^2 Z_{Ls,i4}^{od,*} Z_{Ls,j1}^{DR,*} Z_{Ls,k2}^{DR,*} Z_{Ls,l2}^{od} \\
& + 2g_{A1}^2 Z_{Ls,i2}^{od,*} Z_{Ls,j2}^{DR,*} Z_{Ls,k2}^{DR,*} Z_{Ls,l2}^{od} + 2g_{A2}^2 Z_{Ls,i2}^{od,*} Z_{Ls,j2}^{DR,*} Z_{Ls,k2}^{DR,*} Z_{Ls,l2}^{od} \\
& + 2g_{B1}^2 Z_{Ls,i2}^{od,*} Z_{Ls,j2}^{DR,*} Z_{Ls,k2}^{DR,*} Z_{Ls,l2}^{od} + 2g_{B2}^2 Z_{Ls,i2}^{od,*} Z_{Ls,j2}^{DR,*} Z_{Ls,k2}^{DR,*} Z_{Ls,l2}^{od} \\
& - 2g_{A1}^2 Z_{Ls,i2}^{od,*} Z_{Ls,j3}^{DR,*} Z_{Ls,k3}^{DR,*} Z_{Ls,l2}^{od} - 2g_{A2}^2 Z_{Ls,i2}^{od,*} Z_{Ls,j3}^{DR,*} Z_{Ls,k3}^{DR,*} Z_{Ls,l2}^{od} \\
& - 2g_{B1}^2 Z_{Ls,i2}^{od,*} Z_{Ls,j3}^{DR,*} Z_{Ls,k3}^{DR,*} Z_{Ls,l2}^{od} + 2g_{B2}^2 Z_{Ls,i2}^{od,*} Z_{Ls,j3}^{DR,*} Z_{Ls,k3}^{DR,*} Z_{Ls,l2}^{od} \\
& + 8|Y_A|^2 Z_{Ls,i2}^{od,*} Z_{Ls,j3}^{DR,*} Z_{Ls,k3}^{DR,*} Z_{Ls,l2}^{od} - 2g_{B2}^2 Z_{Ls,i4}^{od,*} Z_{Ls,j4}^{DR,*} Z_{Ls,k3}^{DR,*} Z_{Ls,l2}^{od} \\
& - 2|Y_A|^2 Z_{Ls,i4}^{od,*} Z_{Ls,j4}^{DR,*} Z_{Ls,k3}^{DR,*} Z_{Ls,l2}^{od} + |Y_K|^2 Z_{Ls,i4}^{od,*} Z_{Ls,j4}^{DR,*} Z_{Ls,k3}^{DR,*} Z_{Ls,l2}^{od} \\
& - 2g_{B2}^2 Z_{Ls,i4}^{od,*} Z_{Ls,j3}^{DR,*} Z_{Ls,k4}^{DR,*} Z_{Ls,l2}^{od} - 2|Y_A|^2 Z_{Ls,i4}^{od,*} Z_{Ls,j3}^{DR,*} Z_{Ls,k4}^{DR,*} Z_{Ls,l2}^{od}
\end{aligned}$$

$$\begin{aligned}
& + |Y_K|^2 Z_{Ls,i4}^{od,*} Z_{Ls,j3}^{DR,*} Z_{Ls,k4}^{DR,*} Z_{Ls,l2}^{od} + 2g_{A1}^2 Z_{Ls,i2}^{od,*} Z_{Ls,j4}^{DR,*} Z_{Ls,k4}^{DR,*} Z_{Ls,l2}^{od} \\
& + 2g_{A2}^2 Z_{Ls,i2}^{od,*} Z_{Ls,j4}^{DR,*} Z_{Ls,k4}^{DR,*} Z_{Ls,l2}^{od} + 2g_{B1}^2 Z_{Ls,i2}^{od,*} Z_{Ls,j4}^{DR,*} Z_{Ls,k4}^{DR,*} Z_{Ls,l2}^{od} \\
& + 2g_{B2}^2 Z_{Ls,i2}^{od,*} Z_{Ls,j4}^{DR,*} Z_{Ls,k4}^{DR,*} Z_{Ls,l2}^{od} - 2g_{A2}^2 Z_{Ls,i4}^{od,*} Z_{Ls,j4}^{DR,*} Z_{Ls,k1}^{DR,*} Z_{Ls,l3}^{od} \\
& + 4|Y_A|^2 Z_{Ls,i4}^{od,*} Z_{Ls,j4}^{DR,*} Z_{Ls,k1}^{DR,*} Z_{Ls,l3}^{od} - 2g_{B2}^2 Z_{Ls,i4}^{od,*} Z_{Ls,j3}^{DR,*} Z_{Ls,k2}^{DR,*} Z_{Ls,l3}^{od} \\
& + 2g_{A2}^2 Z_{Ls,i2}^{od,*} Z_{Ls,j4}^{DR,*} Z_{Ls,k2}^{DR,*} Z_{Ls,l3}^{od} + 2g_{B2}^2 Z_{Ls,i2}^{od,*} Z_{Ls,j4}^{DR,*} Z_{Ls,k2}^{DR,*} Z_{Ls,l3}^{od} \\
& - 2g_{B2}^2 Z_{Ls,i4}^{od,*} Z_{Ls,j4}^{DR,*} Z_{Ls,k3}^{DR,*} Z_{Ls,l3}^{od} - 2g_{A2}^2 Z_{Ls,i4}^{od,*} Z_{Ls,j1}^{DR,*} Z_{Ls,k4}^{DR,*} Z_{Ls,l3}^{od} \\
& + 4|Y_A|^2 Z_{Ls,i4}^{od,*} Z_{Ls,j1}^{DR,*} Z_{Ls,k4}^{DR,*} Z_{Ls,l3}^{od} + 2g_{A2}^2 Z_{Ls,i2}^{od,*} Z_{Ls,j2}^{DR,*} Z_{Ls,k4}^{DR,*} Z_{Ls,l3}^{od} \\
& + 2g_{B2}^2 Z_{Ls,i2}^{od,*} Z_{Ls,j2}^{DR,*} Z_{Ls,k4}^{DR,*} Z_{Ls,l3}^{od} + 2g_{A1}^2 Z_{Ls,i4}^{od,*} Z_{Ls,j1}^{DR,*} Z_{Ls,k1}^{DR,*} Z_{Ls,l4}^{od} \\
& + 2g_{A2}^2 Z_{Ls,i4}^{od,*} Z_{Ls,j1}^{DR,*} Z_{Ls,k1}^{DR,*} Z_{Ls,l4}^{od} + 2g_{B1}^2 Z_{Ls,i4}^{od,*} Z_{Ls,j1}^{DR,*} Z_{Ls,k1}^{DR,*} Z_{Ls,l4}^{od} \\
& + 2g_{B2}^2 Z_{Ls,i4}^{od,*} Z_{Ls,j1}^{DR,*} Z_{Ls,k1}^{DR,*} Z_{Ls,l4}^{od} - 2g_{A2}^2 Z_{Ls,i2}^{od,*} Z_{Ls,j2}^{DR,*} Z_{Ls,k1}^{DR,*} Z_{Ls,l4}^{od} \\
& + 2|Y_A|^2 Z_{Ls,i2}^{od,*} Z_{Ls,j2}^{DR,*} Z_{Ls,k1}^{DR,*} Z_{Ls,l4}^{od} + |Y_K|^2 Z_{Ls,i2}^{od,*} Z_{Ls,j2}^{DR,*} Z_{Ls,k1}^{DR,*} Z_{Ls,l4}^{od} \\
& - 2g_{A2}^2 Z_{Ls,i2}^{od,*} Z_{Ls,j1}^{DR,*} Z_{Ls,k2}^{DR,*} Z_{Ls,l4}^{od} + 2|Y_A|^2 Z_{Ls,i2}^{od,*} Z_{Ls,j1}^{DR,*} Z_{Ls,k2}^{DR,*} Z_{Ls,l4}^{od} \\
& + |Y_K|^2 Z_{Ls,i2}^{od,*} Z_{Ls,j1}^{DR,*} Z_{Ls,k2}^{DR,*} Z_{Ls,l4}^{od} - 2g_{A1}^2 Z_{Ls,i4}^{od,*} Z_{Ls,j2}^{DR,*} Z_{Ls,k2}^{DR,*} Z_{Ls,l4}^{od} \\
& + 2g_{A2}^2 Z_{Ls,i4}^{od,*} Z_{Ls,j2}^{DR,*} Z_{Ls,k2}^{DR,*} Z_{Ls,l4}^{od} - 2g_{B1}^2 Z_{Ls,i4}^{od,*} Z_{Ls,j2}^{DR,*} Z_{Ls,k2}^{DR,*} Z_{Ls,l4}^{od} \\
& - 2g_{B2}^2 Z_{Ls,i4}^{od,*} Z_{Ls,j2}^{DR,*} Z_{Ls,k2}^{DR,*} Z_{Ls,l4}^{od} + 2g_{A1}^2 Z_{Ls,i4}^{od,*} Z_{Ls,j3}^{DR,*} Z_{Ls,k3}^{DR,*} Z_{Ls,l4}^{od} \\
& + 2g_{A2}^2 Z_{Ls,i4}^{od,*} Z_{Ls,j3}^{DR,*} Z_{Ls,k3}^{DR,*} Z_{Ls,l4}^{od} + 2g_{B1}^2 Z_{Ls,i4}^{od,*} Z_{Ls,j3}^{DR,*} Z_{Ls,k3}^{DR,*} Z_{Ls,l4}^{od} \\
& + 2g_{B2}^2 Z_{Ls,i4}^{od,*} Z_{Ls,j3}^{DR,*} Z_{Ls,k3}^{DR,*} Z_{Ls,l4}^{od} - 2g_{B2}^2 Z_{Ls,i2}^{od,*} Z_{Ls,j4}^{DR,*} Z_{Ls,k3}^{DR,*} Z_{Ls,l4}^{od} \\
& - 2|Y_A|^2 Z_{Ls,i2}^{od,*} Z_{Ls,j3}^{DR,*} Z_{Ls,k3}^{DR,*} Z_{Ls,l4}^{od} + |Y_K|^2 Z_{Ls,i2}^{od,*} Z_{Ls,j4}^{DR,*} Z_{Ls,k3}^{DR,*} Z_{Ls,l4}^{od} \\
& - 2g_{B2}^2 Z_{Ls,i2}^{od,*} Z_{Ls,j3}^{DR,*} Z_{Ls,k4}^{DR,*} Z_{Ls,l4}^{od} - 2|Y_A|^2 Z_{Ls,i2}^{od,*} Z_{Ls,j3}^{DR,*} Z_{Ls,k4}^{DR,*} Z_{Ls,l4}^{od} \\
& + |Y_K|^2 Z_{Ls,i2}^{od,*} Z_{Ls,j3}^{DR,*} Z_{Ls,k4}^{DR,*} Z_{Ls,l4}^{od} - 2g_{A1}^2 Z_{Ls,i4}^{od,*} Z_{Ls,j4}^{DR,*} Z_{Ls,k4}^{DR,*} Z_{Ls,l4}^{od} \\
& - 2g_{A2}^2 Z_{Ls,i4}^{od,*} Z_{Ls,j4}^{DR,*} Z_{Ls,k4}^{DR,*} Z_{Ls,l4}^{od} - 2g_{B1}^2 Z_{Ls,i4}^{od,*} Z_{Ls,j4}^{DR,*} Z_{Ls,k4}^{DR,*} Z_{Ls,l4}^{od} \\
& + 2g_{B2}^2 Z_{Ls,i4}^{od,*} Z_{Ls,j4}^{DR,*} Z_{Ls,k4}^{DR,*} Z_{Ls,l4}^{od} + 8|Y_A|^2 Z_{Ls,i4}^{od,*} Z_{Ls,j4}^{DR,*} Z_{Ls,k4}^{DR,*} Z_{Ls,l4}^{od} \\
& + Z_{Ls,i1}^{od,*} \left( 2g_{A1}^2 Z_{Ls,j3}^{DR,*} Z_{Ls,k3}^{DR,*} Z_{Ls,l1}^{od} + 2g_{A2}^2 Z_{Ls,j3}^{DR,*} Z_{Ls,k3}^{DR,*} Z_{Ls,l1}^{od} + 2g_{B1}^2 Z_{Ls,j3}^{DR,*} Z_{Ls,k3}^{DR,*} Z_{Ls,l1}^{od} \right. \\
& + 2g_{B2}^2 Z_{Ls,j3}^{DR,*} Z_{Ls,k3}^{DR,*} Z_{Ls,l1}^{od} - 2g_{A1}^2 Z_{Ls,j4}^{DR,*} Z_{Ls,k4}^{DR,*} Z_{Ls,l1}^{od} + 2g_{A2}^2 Z_{Ls,j4}^{DR,*} Z_{Ls,k4}^{DR,*} Z_{Ls,l1}^{od} \\
& - 2g_{B1}^2 Z_{Ls,j4}^{DR,*} Z_{Ls,k4}^{DR,*} Z_{Ls,l1}^{od} - 2g_{B2}^2 Z_{Ls,j4}^{DR,*} Z_{Ls,k4}^{DR,*} Z_{Ls,l1}^{od} - 2g_{B2}^2 Z_{Ls,j4}^{DR,*} Z_{Ls,k1}^{DR,*} Z_{Ls,l2}^{od} \\
& - 2g_{A2}^2 Z_{Ls,j3}^{DR,*} Z_{Ls,k2}^{DR,*} Z_{Ls,l2}^{od} + 4|Y_A|^2 Z_{Ls,j3}^{DR,*} Z_{Ls,k2}^{DR,*} Z_{Ls,l2}^{od} - 2g_{A2}^2 Z_{Ls,j4}^{DR,*} Z_{Ls,k3}^{DR,*} Z_{Ls,l3}^{od} \\
& + 2|Y_A|^2 Z_{Ls,j4}^{DR,*} Z_{Ls,k3}^{DR,*} Z_{Ls,l3}^{od} + |Y_K|^2 Z_{Ls,j4}^{DR,*} Z_{Ls,k3}^{DR,*} Z_{Ls,l3}^{od} - 2g_{A2}^2 Z_{Ls,j3}^{DR,*} Z_{Ls,k4}^{DR,*} Z_{Ls,l3}^{od} \\
& + 2|Y_A|^2 Z_{Ls,j3}^{DR,*} Z_{Ls,k4}^{DR,*} Z_{Ls,l3}^{od} + |Y_K|^2 Z_{Ls,j3}^{DR,*} Z_{Ls,k4}^{DR,*} Z_{Ls,l3}^{od} \\
& + Z_{Ls,j2}^{DR,*} \left( -2 \left( -4|Y_A|^2 - g_{B2}^2 + g_{A1}^2 + g_{A2}^2 + g_{B1}^2 \right) Z_{Ls,k2}^{DR,*} Z_{Ls,l1}^{od} - 2 \left( -2|Y_A|^2 + g_{A2}^2 \right) Z_{Ls,k3}^{DR,*} Z_{Ls,l2}^{od} \right. \\
& \left. + \left( -2g_{B2}^2 - 2|Y_A|^2 + |Y_K|^2 \right) Z_{Ls,k1}^{DR,*} Z_{Ls,l3}^{od} \right)
\end{aligned}$$

$$\begin{aligned}
& + 2g_{A2}^2 Z_{Ls,j3}^{DR,*} Z_{Ls,k1}^{DR,*} Z_{Ls,l4}^{od} + 2g_{B2}^2 Z_{Ls,j3}^{DR,*} Z_{Ls,k1}^{DR,*} Z_{Ls,l4}^{od} \\
& + Z_{Ls,j1}^{DR,*} \left( 2 \left( g_{A1}^2 + g_{A2}^2 + g_{B1}^2 + g_{B2}^2 \right) Z_{Ls,k1}^{DR,*} Z_{Ls,l1}^{od} - 2g_{B2}^2 Z_{Ls,k4}^{DR,*} Z_{Ls,l2}^{od} - 2g_{B2}^2 Z_{Ls,k2}^{DR,*} Z_{Ls,l3}^{od} \right. \\
& \left. - 2|Y_A|^2 Z_{Ls,k2}^{DR,*} Z_{Ls,l3}^{od} + |Y_K|^2 Z_{Ls,k2}^{DR,*} Z_{Ls,l3}^{od} + 2g_{A2}^2 Z_{Ls,k3}^{DR,*} Z_{Ls,l4}^{od} + 2g_{B2}^2 Z_{Ls,k3}^{DR,*} Z_{Ls,l4}^{od} \right) \\
& + Z_{Ls,i3}^{od,*} \left( - 2g_{A2}^2 Z_{Ls,j4}^{DR,*} Z_{Ls,k3}^{DR,*} Z_{Ls,l1}^{od} + 2|Y_A|^2 Z_{Ls,j4}^{DR,*} Z_{Ls,k3}^{DR,*} Z_{Ls,l1}^{od} + |Y_K|^2 Z_{Ls,j4}^{DR,*} Z_{Ls,k3}^{DR,*} Z_{Ls,l1}^{od} \right. \\
& \left. - 2g_{A2}^2 Z_{Ls,j3}^{DR,*} Z_{Ls,k4}^{DR,*} Z_{Ls,l1}^{od} + 2|Y_A|^2 Z_{Ls,j3}^{DR,*} Z_{Ls,k4}^{DR,*} Z_{Ls,l1}^{od} + |Y_K|^2 Z_{Ls,j3}^{DR,*} Z_{Ls,k4}^{DR,*} Z_{Ls,l1}^{od} \right. \\
& + 2g_{A2}^2 Z_{Ls,j4}^{DR,*} Z_{Ls,k2}^{DR,*} Z_{Ls,l2}^{od} + 2g_{B2}^2 Z_{Ls,j4}^{DR,*} Z_{Ls,k2}^{DR,*} Z_{Ls,l2}^{od} - 2g_{A1}^2 Z_{Ls,j3}^{DR,*} Z_{Ls,k3}^{DR,*} Z_{Ls,l3}^{od} \\
& + 2g_{A2}^2 Z_{Ls,j3}^{DR,*} Z_{Ls,k3}^{DR,*} Z_{Ls,l3}^{od} - 2g_{B1}^2 Z_{Ls,j3}^{DR,*} Z_{Ls,k3}^{DR,*} Z_{Ls,l3}^{od} - 2g_{B2}^2 Z_{Ls,j3}^{DR,*} Z_{Ls,k3}^{DR,*} Z_{Ls,l3}^{od} \\
& + 2g_{A1}^2 Z_{Ls,j4}^{DR,*} Z_{Ls,k4}^{DR,*} Z_{Ls,l3}^{od} + 2g_{A2}^2 Z_{Ls,j4}^{DR,*} Z_{Ls,k4}^{DR,*} Z_{Ls,l3}^{od} + 2g_{B1}^2 Z_{Ls,j4}^{DR,*} Z_{Ls,k4}^{DR,*} Z_{Ls,l3}^{od} \\
& + 2g_{B2}^2 Z_{Ls,j4}^{DR,*} Z_{Ls,k4}^{DR,*} Z_{Ls,l3}^{od} - 2g_{A2}^2 Z_{Ls,j4}^{DR,*} Z_{Ls,k1}^{DR,*} Z_{Ls,l4}^{od} + 4|Y_A|^2 Z_{Ls,j4}^{DR,*} Z_{Ls,k1}^{DR,*} Z_{Ls,l4}^{od} \\
& - 2g_{B2}^2 Z_{Ls,j3}^{DR,*} Z_{Ls,k2}^{DR,*} Z_{Ls,l4}^{od} \\
& + Z_{Ls,j2}^{DR,*} \left( \left( - 2g_{B2}^2 - 2|Y_A|^2 + |Y_K|^2 \right) Z_{Ls,k1}^{DR,*} Z_{Ls,l1}^{od} \right. \\
& + 2 \left( \left( g_{A1}^2 + g_{A2}^2 + g_{B1}^2 + g_{B2}^2 \right) Z_{Ls,k2}^{DR,*} Z_{Ls,l3}^{od} + \left( g_{A2}^2 + g_{B2}^2 \right) Z_{Ls,k4}^{DR,*} Z_{Ls,l2}^{od} - g_{B2}^2 Z_{Ls,k3}^{DR,*} Z_{Ls,l4}^{od} \right) \\
& + Z_{Ls,j1}^{DR,*} \left( \left( - 2g_{B2}^2 - 2|Y_A|^2 + |Y_K|^2 \right) Z_{Ls,k2}^{DR,*} Z_{Ls,l1}^{od} \right. \\
& \left. \left. - 2 \left( \left( - 2|Y_A|^2 + g_{A2}^2 \right) Z_{Ls,k4}^{DR,*} Z_{Ls,l4}^{od} + \left( - 4|Y_A|^2 - g_{B2}^2 + g_{A1}^2 + g_{A2}^2 + g_{B1}^2 \right) Z_{Ls,k1}^{DR,*} Z_{Ls,l3}^{od} \right) \right) \right) \quad (869)
\end{aligned}$$

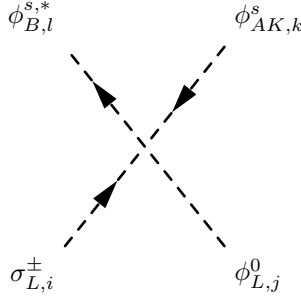

$$\begin{aligned}
& - \frac{i}{2} \left( \sqrt{2} g_{B2}^2 Z_{AK,k2}^{s,*} \left( Z_{Ls,i1}^{od,*} Z_{Ls,j1}^{DR,*} - Z_{Ls,i2}^{od,*} Z_{Ls,j4}^{DR,*} - Z_{Ls,i3}^{od,*} Z_{Ls,j2}^{DR,*} + Z_{Ls,i4}^{od,*} Z_{Ls,j3}^{DR,*} \right) \right. \\
& + Y_A^* \left( \sqrt{2} Y_A Z_{AK,k2}^{s,*} \left( - Z_{Ls,i1}^{od,*} Z_{Ls,j1}^{DR,*} + Z_{Ls,i2}^{od,*} Z_{Ls,j4}^{DR,*} + Z_{Ls,i3}^{od,*} Z_{Ls,j2}^{DR,*} - Z_{Ls,i4}^{od,*} Z_{Ls,j3}^{DR,*} \right) \right. \\
& \left. \left. + Y_K Z_{AK,k1}^{s,*} \left( Z_{Ls,i1}^{od,*} Z_{Ls,j1}^{DR,*} + Z_{Ls,i2}^{od,*} Z_{Ls,j4}^{DR,*} + Z_{Ls,i3}^{od,*} Z_{Ls,j2}^{DR,*} + Z_{Ls,i4}^{od,*} Z_{Ls,j3}^{DR,*} \right) \right) \right) B_{A,l1}^s \quad (870)
\end{aligned}$$

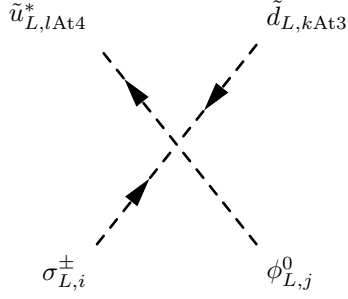

$$-\frac{i}{2}g_{A2}^2\left(Z_{Ls,i1}^{od,*}Z_{Ls,j3}^{DR,*}-Z_{Ls,i2}^{od,*}Z_{Ls,j2}^{DR,*}-Z_{Ls,i3}^{od,*}Z_{Ls,j4}^{DR,*}+Z_{Ls,i4}^{od,*}Z_{Ls,j1}^{DR,*}\right)\delta_{At3At4}\delta_{kl} \quad (871)$$


---

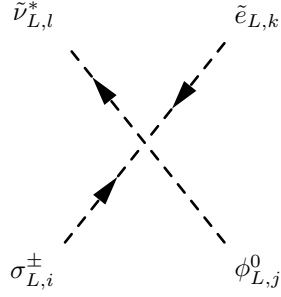

$$-\frac{i}{2}g_{A2}^2\left(Z_{Ls,i1}^{od,*}Z_{Ls,j3}^{DR,*}-Z_{Ls,i2}^{od,*}Z_{Ls,j2}^{DR,*}-Z_{Ls,i3}^{od,*}Z_{Ls,j4}^{DR,*}+Z_{Ls,i4}^{od,*}Z_{Ls,j1}^{DR,*}\right)\delta_{kl} \quad (872)$$


---

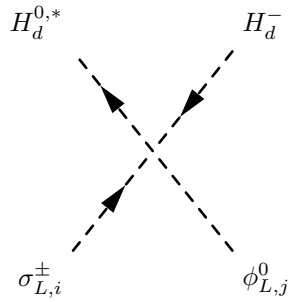

$$-\frac{i}{2}g_{A2}^2\left(Z_{Ls,i1}^{od,*}Z_{Ls,j3}^{DR,*}-Z_{Ls,i2}^{od,*}Z_{Ls,j2}^{DR,*}-Z_{Ls,i3}^{od,*}Z_{Ls,j4}^{DR,*}+Z_{Ls,i4}^{od,*}Z_{Ls,j1}^{DR,*}\right) \quad (873)$$


---

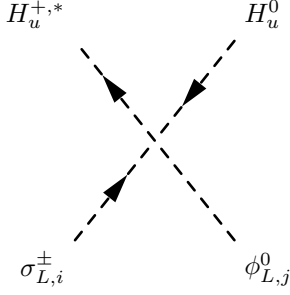

$$-\frac{i}{2}g_{A2}^2 \left( Z_{Ls,i1}^{od,*} Z_{Ls,j3}^{DR,*} - Z_{Ls,i2}^{od,*} Z_{Ls,j2}^{DR,*} - Z_{Ls,i3}^{od,*} Z_{Ls,j4}^{DR,*} + Z_{Ls,i4}^{od,*} Z_{Ls,j1}^{DR,*} \right) \quad (874)$$


---

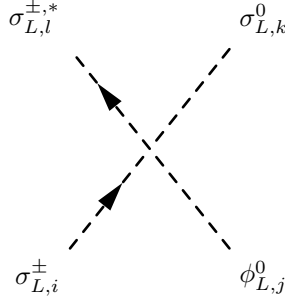

$$\begin{aligned} & \frac{1}{4} \left( -2g_{B2}^2 Z_{Ls,i2}^{od,*} Z_{Ls,j4}^{DR,*} Z_{Ls,k1}^{Di,*} Z_{Ls,l1}^{od} + 2g_{A2}^2 Z_{Ls,i2}^{od,*} Z_{Ls,j3}^{DR,*} Z_{Ls,k2}^{Di,*} Z_{Ls,l1}^{od} \right. \\ & - 4|Y_A|^2 Z_{Ls,i2}^{od,*} Z_{Ls,j3}^{DR,*} Z_{Ls,k2}^{Di,*} Z_{Ls,l1}^{od} - 2g_{A2}^2 Z_{Ls,i2}^{od,*} Z_{Ls,j2}^{DR,*} Z_{Ls,k3}^{Di,*} Z_{Ls,l1}^{od} \\ & + 4|Y_A|^2 Z_{Ls,i2}^{od,*} Z_{Ls,j2}^{DR,*} Z_{Ls,k3}^{Di,*} Z_{Ls,l1}^{od} + 2g_{B2}^2 Z_{Ls,i2}^{od,*} Z_{Ls,j1}^{DR,*} Z_{Ls,k4}^{Di,*} Z_{Ls,l1}^{od} \\ & + 2g_{B2}^2 Z_{Ls,i1}^{od,*} Z_{Ls,j4}^{DR,*} Z_{Ls,k1}^{Di,*} Z_{Ls,l2}^{od} - 2g_{A2}^2 Z_{Ls,i1}^{od,*} Z_{Ls,j3}^{DR,*} Z_{Ls,k2}^{Di,*} Z_{Ls,l2}^{od} \\ & + 4|Y_A|^2 Z_{Ls,i1}^{od,*} Z_{Ls,j3}^{DR,*} Z_{Ls,k2}^{Di,*} Z_{Ls,l2}^{od} + 2g_{A2}^2 Z_{Ls,i1}^{od,*} Z_{Ls,j2}^{DR,*} Z_{Ls,k3}^{Di,*} Z_{Ls,l2}^{od} \\ & - 4|Y_A|^2 Z_{Ls,i1}^{od,*} Z_{Ls,j2}^{DR,*} Z_{Ls,k3}^{Di,*} Z_{Ls,l2}^{od} - 2g_{B2}^2 Z_{Ls,i1}^{od,*} Z_{Ls,j1}^{DR,*} Z_{Ls,k4}^{Di,*} Z_{Ls,l2}^{od} \\ & + 2g_{B2}^2 Z_{Ls,i1}^{od,*} Z_{Ls,j2}^{DR,*} Z_{Ls,k1}^{Di,*} Z_{Ls,l3}^{od} + 2|Y_A|^2 Z_{Ls,i1}^{od,*} Z_{Ls,j2}^{DR,*} Z_{Ls,k1}^{Di,*} Z_{Ls,l3}^{od} \\ & - |Y_K|^2 Z_{Ls,i1}^{od,*} Z_{Ls,j2}^{DR,*} Z_{Ls,k1}^{Di,*} Z_{Ls,l3}^{od} + 2g_{B2}^2 Z_{Ls,i1}^{od,*} Z_{Ls,j1}^{DR,*} Z_{Ls,k2}^{Di,*} Z_{Ls,l3}^{od} \\ & + 2|Y_A|^2 Z_{Ls,i1}^{od,*} Z_{Ls,j1}^{DR,*} Z_{Ls,k2}^{Di,*} Z_{Ls,l3}^{od} - |Y_K|^2 Z_{Ls,i1}^{od,*} Z_{Ls,j1}^{DR,*} Z_{Ls,k2}^{Di,*} Z_{Ls,l3}^{od} \\ & - 2g_{A2}^2 Z_{Ls,i2}^{od,*} Z_{Ls,j4}^{DR,*} Z_{Ls,k2}^{Di,*} Z_{Ls,l3}^{od} - 2g_{B2}^2 Z_{Ls,i2}^{od,*} Z_{Ls,j4}^{DR,*} Z_{Ls,k2}^{Di,*} Z_{Ls,l3}^{od} \\ & + 2g_{A2}^2 Z_{Ls,i1}^{od,*} Z_{Ls,j4}^{DR,*} Z_{Ls,k3}^{Di,*} Z_{Ls,l3}^{od} - 2|Y_A|^2 Z_{Ls,i1}^{od,*} Z_{Ls,j4}^{DR,*} Z_{Ls,k3}^{Di,*} Z_{Ls,l3}^{od} \\ & - |Y_K|^2 Z_{Ls,i1}^{od,*} Z_{Ls,j4}^{DR,*} Z_{Ls,k3}^{Di,*} Z_{Ls,l3}^{od} - 2g_{A2}^2 Z_{Ls,i2}^{od,*} Z_{Ls,j2}^{DR,*} Z_{Ls,k4}^{Di,*} Z_{Ls,l3}^{od} \\ & \left. - 2g_{B2}^2 Z_{Ls,i2}^{od,*} Z_{Ls,j2}^{DR,*} Z_{Ls,k4}^{Di,*} Z_{Ls,l3}^{od} + 2g_{A2}^2 Z_{Ls,i1}^{od,*} Z_{Ls,j3}^{DR,*} Z_{Ls,k4}^{Di,*} Z_{Ls,l3}^{od} \right) \end{aligned}$$

$$\begin{aligned}
& -2|Y_A|^2 Z_{Ls,i1}^{od,*} Z_{Ls,j3}^{DR,*} Z_{Ls,k4}^{Di,*} Z_{Ls,l3}^{od} - |Y_K|^2 Z_{Ls,i1}^{od,*} Z_{Ls,j3}^{DR,*} Z_{Ls,k4}^{Di,*} Z_{Ls,l3}^{od} \\
& + Z_{Ls,i4}^{od,*} \left( -2g_{A2}^2 Z_{Ls,j2}^{DR,*} Z_{Ls,k1}^{Di,*} Z_{Ls,l2}^{od} + 2|Y_A|^2 Z_{Ls,j2}^{DR,*} Z_{Ls,k1}^{Di,*} Z_{Ls,l2}^{od} + |Y_K|^2 Z_{Ls,j2}^{DR,*} Z_{Ls,k1}^{Di,*} Z_{Ls,l2}^{od} \right. \\
& - 2g_{B2}^2 Z_{Ls,j4}^{DR,*} Z_{Ls,k3}^{Di,*} Z_{Ls,l2}^{od} - 2|Y_A|^2 Z_{Ls,j4}^{DR,*} Z_{Ls,k3}^{Di,*} Z_{Ls,l2}^{od} + |Y_K|^2 Z_{Ls,j4}^{DR,*} Z_{Ls,k3}^{Di,*} Z_{Ls,l2}^{od} \\
& - 2g_{A2}^2 Z_{Ls,j4}^{DR,*} Z_{Ls,k1}^{Di,*} Z_{Ls,l3}^{od} + 4|Y_A|^2 Z_{Ls,j4}^{DR,*} Z_{Ls,k1}^{Di,*} Z_{Ls,l3}^{od} - 2g_{B2}^2 Z_{Ls,j2}^{DR,*} Z_{Ls,k3}^{Di,*} Z_{Ls,l3}^{od} \\
& + Z_{Ls,j3}^{DR,*} \left( 2(g_{A2}^2 + g_{B2}^2) Z_{Ls,k1}^{Di,*} Z_{Ls,l1}^{od} + \left( -2g_{B2}^2 - 2|Y_A|^2 + |Y_K|^2 \right) Z_{Ls,k4}^{Di,*} Z_{Ls,l2}^{od} + 2g_{B2}^2 Z_{Ls,k2}^{Di,*} Z_{Ls,l3}^{od} \right) \\
& + Z_{Ls,j1}^{DR,*} \left( 2(-2|Y_A|^2 + g_{A2}^2) Z_{Ls,k4}^{Di,*} Z_{Ls,l3}^{od} + \left( -2g_{A2}^2 + 2|Y_A|^2 + |Y_K|^2 \right) Z_{Ls,k2}^{Di,*} Z_{Ls,l2}^{od} + 2(g_{A2}^2 + g_{B2}^2) Z_{Ls,k3}^{Di,*} Z_{Ls,l1}^{od} \right) \\
& + 2g_{A2}^2 Z_{Ls,i2}^{od,*} Z_{Ls,j2}^{DR,*} Z_{Ls,k1}^{Di,*} Z_{Ls,l4}^{od} - 2|Y_A|^2 Z_{Ls,i2}^{od,*} Z_{Ls,j2}^{DR,*} Z_{Ls,k1}^{Di,*} Z_{Ls,l4}^{od} \\
& - |Y_K|^2 Z_{Ls,i2}^{od,*} Z_{Ls,j2}^{DR,*} Z_{Ls,k1}^{Di,*} Z_{Ls,l4}^{od} - 2g_{A2}^2 Z_{Ls,i1}^{od,*} Z_{Ls,j3}^{DR,*} Z_{Ls,k1}^{Di,*} Z_{Ls,l4}^{od} \\
& - 2g_{B2}^2 Z_{Ls,i1}^{od,*} Z_{Ls,j3}^{DR,*} Z_{Ls,k1}^{Di,*} Z_{Ls,l4}^{od} + 2g_{A2}^2 Z_{Ls,i2}^{od,*} Z_{Ls,j1}^{DR,*} Z_{Ls,k2}^{Di,*} Z_{Ls,l4}^{od} \\
& - 2|Y_A|^2 Z_{Ls,i2}^{od,*} Z_{Ls,j1}^{DR,*} Z_{Ls,k2}^{Di,*} Z_{Ls,l4}^{od} - |Y_K|^2 Z_{Ls,i2}^{od,*} Z_{Ls,j1}^{DR,*} Z_{Ls,k2}^{Di,*} Z_{Ls,l4}^{od} \\
& - 2g_{A2}^2 Z_{Ls,i1}^{od,*} Z_{Ls,j1}^{DR,*} Z_{Ls,k3}^{Di,*} Z_{Ls,l4}^{od} - 2g_{B2}^2 Z_{Ls,i1}^{od,*} Z_{Ls,j1}^{DR,*} Z_{Ls,k3}^{Di,*} Z_{Ls,l4}^{od} \\
& + 2g_{B2}^2 Z_{Ls,i2}^{od,*} Z_{Ls,j4}^{DR,*} Z_{Ls,k3}^{Di,*} Z_{Ls,l4}^{od} + 2|Y_A|^2 Z_{Ls,i2}^{od,*} Z_{Ls,j4}^{DR,*} Z_{Ls,k3}^{Di,*} Z_{Ls,l4}^{od} \\
& - |Y_K|^2 Z_{Ls,i2}^{od,*} Z_{Ls,j4}^{DR,*} Z_{Ls,k3}^{Di,*} Z_{Ls,l4}^{od} + 2g_{B2}^2 Z_{Ls,i2}^{od,*} Z_{Ls,j3}^{DR,*} Z_{Ls,k4}^{Di,*} Z_{Ls,l4}^{od} \\
& + 2|Y_A|^2 Z_{Ls,i2}^{od,*} Z_{Ls,j3}^{DR,*} Z_{Ls,k4}^{Di,*} Z_{Ls,l4}^{od} - |Y_K|^2 Z_{Ls,i2}^{od,*} Z_{Ls,j3}^{DR,*} Z_{Ls,k4}^{Di,*} Z_{Ls,l4}^{od} \\
& + Z_{Ls,i3}^{od,*} \left( -2g_{A2}^2 Z_{Ls,j4}^{DR,*} Z_{Ls,k3}^{Di,*} Z_{Ls,l1}^{od} + 2|Y_A|^2 Z_{Ls,j4}^{DR,*} Z_{Ls,k3}^{Di,*} Z_{Ls,l1}^{od} + |Y_K|^2 Z_{Ls,j4}^{DR,*} Z_{Ls,k3}^{Di,*} Z_{Ls,l1}^{od} \right. \\
& - 2g_{A2}^2 Z_{Ls,j3}^{DR,*} Z_{Ls,k4}^{Di,*} Z_{Ls,l1}^{od} + 2|Y_A|^2 Z_{Ls,j3}^{DR,*} Z_{Ls,k4}^{Di,*} Z_{Ls,l1}^{od} + |Y_K|^2 Z_{Ls,j3}^{DR,*} Z_{Ls,k4}^{Di,*} Z_{Ls,l1}^{od} \\
& + 2g_{A2}^2 Z_{Ls,j4}^{DR,*} Z_{Ls,k2}^{Di,*} Z_{Ls,l2}^{od} + 2g_{B2}^2 Z_{Ls,j4}^{DR,*} Z_{Ls,k2}^{Di,*} Z_{Ls,l2}^{od} + 2g_{A2}^2 Z_{Ls,j4}^{DR,*} Z_{Ls,k1}^{Di,*} Z_{Ls,l4}^{od} \\
& - 4|Y_A|^2 Z_{Ls,j4}^{DR,*} Z_{Ls,k1}^{Di,*} Z_{Ls,l4}^{od} - 2g_{B2}^2 Z_{Ls,j3}^{DR,*} Z_{Ls,k2}^{Di,*} Z_{Ls,l4}^{od} \\
& + Z_{Ls,j1}^{DR,*} \left( -2(-2|Y_A|^2 + g_{A2}^2) Z_{Ls,k4}^{Di,*} Z_{Ls,l4}^{od} + \left( -2g_{B2}^2 - 2|Y_A|^2 + |Y_K|^2 \right) Z_{Ls,k2}^{Di,*} Z_{Ls,l1}^{od} \right) \\
& + Z_{Ls,j2}^{DR,*} \left( 2\left( (g_{A2}^2 + g_{B2}^2) Z_{Ls,k4}^{Di,*} Z_{Ls,l2}^{od} + g_{B2}^2 Z_{Ls,k3}^{Di,*} Z_{Ls,l4}^{od} \right) + \left( -2g_{B2}^2 - 2|Y_A|^2 + |Y_K|^2 \right) Z_{Ls,k1}^{Di,*} Z_{Ls,l1}^{od} \right) \Big) \quad (875)
\end{aligned}$$

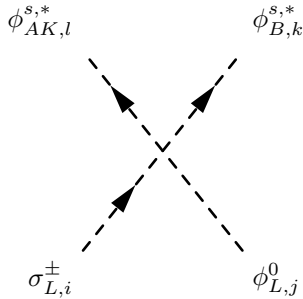

$$- \frac{i}{2} \left( Y_A Y_K^* \left( Z_{Ls,i1}^{od,*} Z_{Ls,j1}^{DR,*} + Z_{Ls,i2}^{od,*} Z_{Ls,j4}^{DR,*} + Z_{Ls,i3}^{od,*} Z_{Ls,j2}^{DR,*} + Z_{Ls,i4}^{od,*} Z_{Ls,j3}^{DR,*} \right) Z_{AK,l1}^s \right.$$

$$- \sqrt{2} \left( -|Y_A|^2 + g_{B2}^2 \right) \left( Z_{Ls,i1}^{od,*} Z_{Ls,j1}^{DR,*} - Z_{Ls,i2}^{od,*} Z_{Ls,j4}^{DR,*} - Z_{Ls,i3}^{od,*} Z_{Ls,j2}^{DR,*} + Z_{Ls,i4}^{od,*} Z_{Ls,j3}^{DR,*} \right) Z_{AK,l2}^s B_{A,k2}^s \quad (876)$$


---

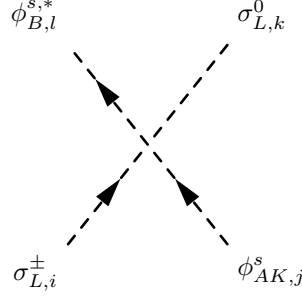

$$\begin{aligned} & \frac{1}{2} \left( \sqrt{2} g_{B2}^2 Z_{AK,j2}^{s,*} \left( -Z_{Ls,i1}^{od,*} Z_{Ls,k1}^{Di,*} + Z_{Ls,i2}^{od,*} Z_{Ls,k4}^{Di,*} - Z_{Ls,i3}^{od,*} Z_{Ls,k2}^{Di,*} + Z_{Ls,i4}^{od,*} Z_{Ls,k3}^{Di,*} \right) \right. \\ & + Y_A^* \left( \sqrt{2} Y_A Z_{AK,j2}^{s,*} \left( Z_{Ls,i1}^{od,*} Z_{Ls,k1}^{Di,*} - Z_{Ls,i2}^{od,*} Z_{Ls,k4}^{Di,*} + Z_{Ls,i3}^{od,*} Z_{Ls,k2}^{Di,*} - Z_{Ls,i4}^{od,*} Z_{Ls,k3}^{Di,*} \right) \right. \\ & \left. \left. + Y_K Z_{AK,j1}^{s,*} \left( -Z_{Ls,i1}^{od,*} Z_{Ls,k1}^{Di,*} - Z_{Ls,i2}^{od,*} Z_{Ls,k4}^{Di,*} + Z_{Ls,i3}^{od,*} Z_{Ls,k2}^{Di,*} + Z_{Ls,i4}^{od,*} Z_{Ls,k3}^{Di,*} \right) \right) \right) B_{A,l1}^s \end{aligned} \quad (877)$$


---

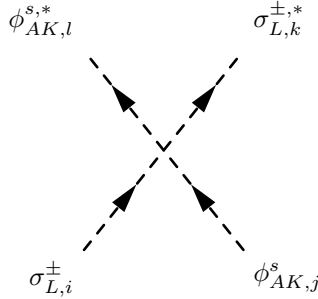

$$\begin{aligned} & -\frac{i}{4} \left( Y_K^* Z_{AK,l1}^s \left( \sqrt{2} Y_A Z_{AK,j2}^{s,*} \left( -Z_{Ls,i1}^{od,*} Z_{Ls,k1}^{od} + Z_{Ls,i2}^{od,*} Z_{Ls,k2}^{od} - Z_{Ls,i3}^{od,*} Z_{Ls,k3}^{od} + Z_{Ls,i4}^{od,*} Z_{Ls,k4}^{od} \right) \right. \right. \\ & + Y_K Z_{AK,j1}^{s,*} \left( Z_{Ls,i1}^{od,*} Z_{Ls,k1}^{od} + Z_{Ls,i2}^{od,*} Z_{Ls,k2}^{od} + Z_{Ls,i3}^{od,*} Z_{Ls,k3}^{od} + Z_{Ls,i4}^{od,*} Z_{Ls,k4}^{od} \right) \left. \right) \\ & + Y_A^* Z_{AK,l2}^s \left( \sqrt{2} Y_K Z_{AK,j1}^{s,*} \left( -Z_{Ls,i1}^{od,*} Z_{Ls,k1}^{od} + Z_{Ls,i2}^{od,*} Z_{Ls,k2}^{od} - Z_{Ls,i3}^{od,*} Z_{Ls,k3}^{od} + Z_{Ls,i4}^{od,*} Z_{Ls,k4}^{od} \right) \right. \\ & \left. \left. + 2 Y_A Z_{AK,j2}^{s,*} \left( Z_{Ls,i1}^{od,*} Z_{Ls,k1}^{od} + Z_{Ls,i2}^{od,*} Z_{Ls,k2}^{od} + Z_{Ls,i3}^{od,*} Z_{Ls,k3}^{od} + Z_{Ls,i4}^{od,*} Z_{Ls,k4}^{od} \right) \right) \right) \end{aligned} \quad (878)$$


---

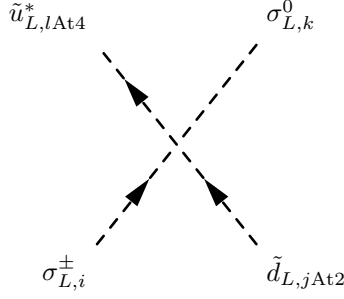

$$\frac{1}{2}g_{A2}^2 \left( -Z_{Ls,i1}^{od,*} Z_{Ls,k3}^{Di,*} + Z_{Ls,i2}^{od,*} Z_{Ls,k2}^{Di,*} - Z_{Ls,i3}^{od,*} Z_{Ls,k4}^{Di,*} + Z_{Ls,i4}^{od,*} Z_{Ls,k1}^{Di,*} \right) \delta_{At2At4} \delta_{jl} \quad (879)$$


---

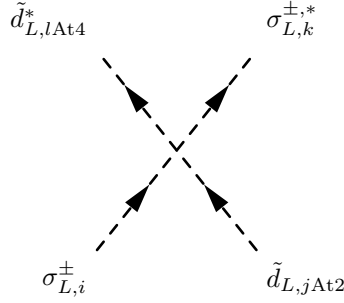

$$\begin{aligned} \frac{i}{12} \delta_{At2At4} \delta_{jl} & \left( \left( 3g_{A2}^2 + g_{A1}^2 \right) Z_{Ls,i1}^{od,*} Z_{Ls,k1}^{od} - \left( -3g_{A2}^2 + g_{A1}^2 \right) Z_{Ls,i2}^{od,*} Z_{Ls,k2}^{od} - g_{A1}^2 Z_{Ls,i3}^{od,*} Z_{Ls,k3}^{od} \right. \\ & \left. - 3g_{A2}^2 Z_{Ls,i3}^{od,*} Z_{Ls,k3}^{od} + g_{A1}^2 Z_{Ls,i4}^{od,*} Z_{Ls,k4}^{od} - 3g_{A2}^2 Z_{Ls,i4}^{od,*} Z_{Ls,k4}^{od} \right) \end{aligned} \quad (880)$$


---

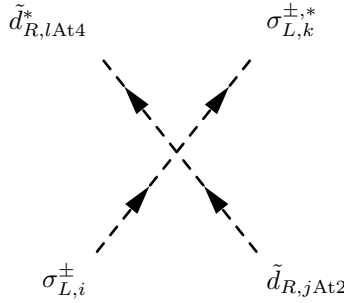

$$\frac{i}{6} g_{A1}^2 \delta_{At2At4} \delta_{jl} \left( Z_{Ls,i1}^{od,*} Z_{Ls,k1}^{od} - Z_{Ls,i2}^{od,*} Z_{Ls,k2}^{od} - Z_{Ls,i3}^{od,*} Z_{Ls,k3}^{od} + Z_{Ls,i4}^{od,*} Z_{Ls,k4}^{od} \right) \quad (881)$$


---



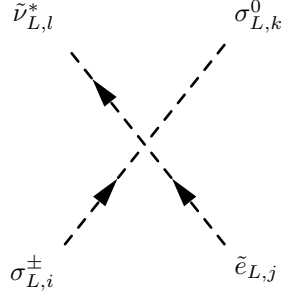

$$\frac{1}{2}g_{A2}^2 \left( -Z_{Ls,i1}^{od,*} Z_{Ls,k3}^{Di,*} + Z_{Ls,i2}^{od,*} Z_{Ls,k2}^{Di,*} - Z_{Ls,i3}^{od,*} Z_{Ls,k4}^{Di,*} + Z_{Ls,i4}^{od,*} Z_{Ls,k1}^{Di,*} \right) \delta_{jl} \quad (882)$$


---

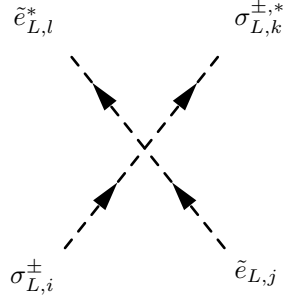

$$-\frac{i}{4}\delta_{jl} \left( \left( -g_{A2}^2 + g_{A1}^2 \right) Z_{Ls,i1}^{od,*} Z_{Ls,k1}^{od} - \left( g_{A1}^2 + g_{A2}^2 \right) Z_{Ls,i2}^{od,*} Z_{Ls,k2}^{od} - g_{A1}^2 Z_{Ls,i3}^{od,*} Z_{Ls,k3}^{od} + g_{A2}^2 Z_{Ls,i3}^{od,*} Z_{Ls,k3}^{od} \right. \\ \left. + g_{A1}^2 Z_{Ls,i4}^{od,*} Z_{Ls,k4}^{od} + g_{A2}^2 Z_{Ls,i4}^{od,*} Z_{Ls,k4}^{od} \right) \quad (883)$$


---

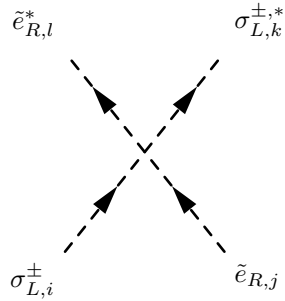

$$\frac{i}{2}g_{A1}^2 \delta_{jl} \left( Z_{Ls,i1}^{od,*} Z_{Ls,k1}^{od} - Z_{Ls,i2}^{od,*} Z_{Ls,k2}^{od} - Z_{Ls,i3}^{od,*} Z_{Ls,k3}^{od} + Z_{Ls,i4}^{od,*} Z_{Ls,k4}^{od} \right) \quad (884)$$


---

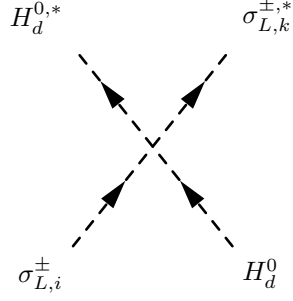

$$\begin{aligned}
& -\frac{i}{4} \left( (g_{A1}^2 + g_{A2}^2) Z_{Ls,i1}^{od,*} Z_{Ls,k1}^{od} + (-g_{A1}^2 + g_{A2}^2) Z_{Ls,i2}^{od,*} Z_{Ls,k2}^{od} - g_{A1}^2 Z_{Ls,i3}^{od,*} Z_{Ls,k3}^{od} - g_{A2}^2 Z_{Ls,i3}^{od,*} Z_{Ls,k3}^{od} \right. \\
& \left. + g_{A1}^2 Z_{Ls,i4}^{od,*} Z_{Ls,k4}^{od} - g_{A2}^2 Z_{Ls,i4}^{od,*} Z_{Ls,k4}^{od} \right) \quad (885)
\end{aligned}$$


---

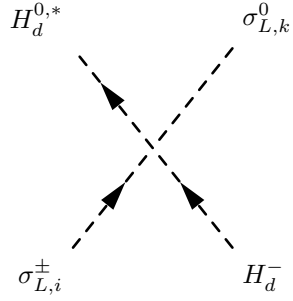

$$\frac{1}{2} g_{A2}^2 \left( -Z_{Ls,i1}^{od,*} Z_{Ls,k3}^{Di,*} + Z_{Ls,i2}^{od,*} Z_{Ls,k2}^{Di,*} - Z_{Ls,i3}^{od,*} Z_{Ls,k4}^{Di,*} + Z_{Ls,i4}^{od,*} Z_{Ls,k1}^{Di,*} \right) \quad (886)$$


---

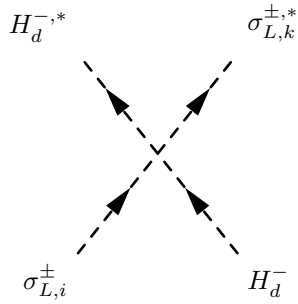

$$\begin{aligned}
& -\frac{i}{4} \left( (-g_{A2}^2 + g_{A1}^2) Z_{Ls,i1}^{od,*} Z_{Ls,k1}^{od} - (g_{A1}^2 + g_{A2}^2) Z_{Ls,i2}^{od,*} Z_{Ls,k2}^{od} - g_{A1}^2 Z_{Ls,i3}^{od,*} Z_{Ls,k3}^{od} + g_{A2}^2 Z_{Ls,i3}^{od,*} Z_{Ls,k3}^{od} \right. \\
& \left. + g_{A1}^2 Z_{Ls,i4}^{od,*} Z_{Ls,k4}^{od} + g_{A2}^2 Z_{Ls,i4}^{od,*} Z_{Ls,k4}^{od} \right) \quad (887)
\end{aligned}$$


---

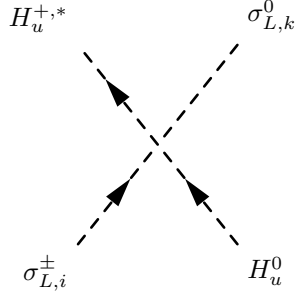

$$\frac{1}{2}g_{A2}^2 \left( -Z_{Ls,i1}^{od,*} Z_{Ls,k3}^{Di,*} + Z_{Ls,i2}^{od,*} Z_{Ls,k2}^{Di,*} - Z_{Ls,i3}^{od,*} Z_{Ls,k4}^{Di,*} + Z_{Ls,i4}^{od,*} Z_{Ls,k1}^{Di,*} \right) \quad (888)$$


---

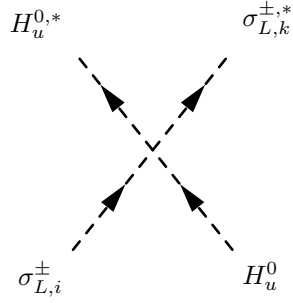

$$\begin{aligned} & \frac{i}{4} \left( (g_{A1}^2 + g_{A2}^2) Z_{Ls,i1}^{od,*} Z_{Ls,k1}^{od} + (-g_{A1}^2 + g_{A2}^2) Z_{Ls,i2}^{od,*} Z_{Ls,k2}^{od} - g_{A1}^2 Z_{Ls,i3}^{od,*} Z_{Ls,k3}^{od} - g_{A2}^2 Z_{Ls,i3}^{od,*} Z_{Ls,k3}^{od} \right. \\ & \left. + g_{A1}^2 Z_{Ls,i4}^{od,*} Z_{Ls,k4}^{od} - g_{A2}^2 Z_{Ls,i4}^{od,*} Z_{Ls,k4}^{od} \right) \end{aligned} \quad (889)$$


---

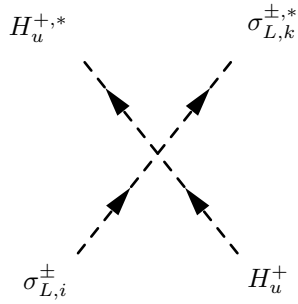

$$\begin{aligned} & \frac{i}{4} \left( (-g_{A2}^2 + g_{A1}^2) Z_{Ls,i1}^{od,*} Z_{Ls,k1}^{od} - (g_{A1}^2 + g_{A2}^2) Z_{Ls,i2}^{od,*} Z_{Ls,k2}^{od} - g_{A1}^2 Z_{Ls,i3}^{od,*} Z_{Ls,k3}^{od} + g_{A2}^2 Z_{Ls,i3}^{od,*} Z_{Ls,k3}^{od} \right. \\ & \left. + g_{A1}^2 Z_{Ls,i4}^{od,*} Z_{Ls,k4}^{od} + g_{A2}^2 Z_{Ls,i4}^{od,*} Z_{Ls,k4}^{od} \right) \end{aligned} \quad (890)$$


---

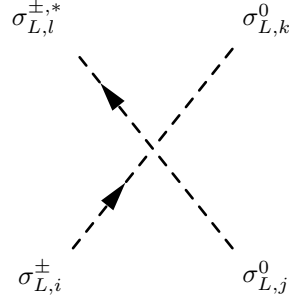

$$\begin{aligned}
& \frac{i}{4} \left( 2g_{A2}^2 Z_{L,i4}^{od,*} Z_{L,j3}^{Di,*} Z_{L,k1}^{Di,*} Z_{L,l1}^{od} + 2g_{B2}^2 Z_{L,i4}^{od,*} Z_{L,j3}^{Di,*} Z_{L,k1}^{Di,*} Z_{L,l1}^{od} \right. \\
& + 2g_{B2}^2 Z_{L,i2}^{od,*} Z_{L,j4}^{Di,*} Z_{L,k1}^{Di,*} Z_{L,l1}^{od} + 2g_{A2}^2 Z_{L,i2}^{od,*} Z_{L,j3}^{Di,*} Z_{L,k2}^{Di,*} Z_{L,l1}^{od} \\
& - 4|Y_A|^2 Z_{L,i2}^{od,*} Z_{L,j3}^{Di,*} Z_{L,k2}^{Di,*} Z_{L,l1}^{od} + 2g_{A2}^2 Z_{L,i4}^{od,*} Z_{L,j1}^{Di,*} Z_{L,k3}^{Di,*} Z_{L,l1}^{od} \\
& + 2g_{B2}^2 Z_{L,i4}^{od,*} Z_{L,j1}^{Di,*} Z_{L,k3}^{Di,*} Z_{L,l1}^{od} + 2g_{A2}^2 Z_{L,i2}^{od,*} Z_{L,j2}^{Di,*} Z_{L,k3}^{Di,*} Z_{L,l1}^{od} \\
& - 4|Y_A|^2 Z_{L,i2}^{od,*} Z_{L,j2}^{Di,*} Z_{L,k3}^{Di,*} Z_{L,l1}^{od} + 2g_{B2}^2 Z_{L,i2}^{od,*} Z_{L,j1}^{Di,*} Z_{L,k4}^{Di,*} Z_{L,l1}^{od} \\
& + 2g_{A1}^2 Z_{L,i2}^{od,*} Z_{L,j1}^{Di,*} Z_{L,k1}^{Di,*} Z_{L,l2}^{od} - 2g_{A2}^2 Z_{L,i2}^{od,*} Z_{L,j1}^{Di,*} Z_{L,k1}^{Di,*} Z_{L,l2}^{od} \\
& + 2g_{B1}^2 Z_{L,i2}^{od,*} Z_{L,j1}^{Di,*} Z_{L,k1}^{Di,*} Z_{L,l2}^{od} + 2g_{B2}^2 Z_{L,i2}^{od,*} Z_{L,j1}^{Di,*} Z_{L,k1}^{Di,*} Z_{L,l2}^{od} \\
& - 2g_{A2}^2 Z_{L,i4}^{od,*} Z_{L,j2}^{Di,*} Z_{L,k1}^{Di,*} Z_{L,l2}^{od} + 2|Y_A|^2 Z_{L,i4}^{od,*} Z_{L,j2}^{Di,*} Z_{L,k1}^{Di,*} Z_{L,l2}^{od} \\
& + |Y_K|^2 Z_{L,i4}^{od,*} Z_{L,j2}^{Di,*} Z_{L,k1}^{Di,*} Z_{L,l2}^{od} - 2g_{A2}^2 Z_{L,i4}^{od,*} Z_{L,j1}^{Di,*} Z_{L,k2}^{Di,*} Z_{L,l2}^{od} \\
& + 2|Y_A|^2 Z_{L,i4}^{od,*} Z_{L,j1}^{Di,*} Z_{L,k2}^{Di,*} Z_{L,l2}^{od} + |Y_K|^2 Z_{L,i4}^{od,*} Z_{L,j1}^{Di,*} Z_{L,k2}^{Di,*} Z_{L,l2}^{od} \\
& - 2g_{A1}^2 Z_{L,i2}^{od,*} Z_{L,j2}^{Di,*} Z_{L,k2}^{Di,*} Z_{L,l2}^{od} - 2g_{A2}^2 Z_{L,i2}^{od,*} Z_{L,j2}^{Di,*} Z_{L,k2}^{Di,*} Z_{L,l2}^{od} \\
& - 2g_{B1}^2 Z_{L,i2}^{od,*} Z_{L,j2}^{Di,*} Z_{L,k2}^{Di,*} Z_{L,l2}^{od} - 2g_{B2}^2 Z_{L,i2}^{od,*} Z_{L,j2}^{Di,*} Z_{L,k2}^{Di,*} Z_{L,l2}^{od} \\
& + 2g_{A1}^2 Z_{L,i2}^{od,*} Z_{L,j3}^{Di,*} Z_{L,k3}^{Di,*} Z_{L,l2}^{od} + 2g_{A2}^2 Z_{L,i2}^{od,*} Z_{L,j3}^{Di,*} Z_{L,k3}^{Di,*} Z_{L,l2}^{od} \\
& + 2g_{B1}^2 Z_{L,i2}^{od,*} Z_{L,j3}^{Di,*} Z_{L,k3}^{Di,*} Z_{L,l2}^{od} - 2g_{B2}^2 Z_{L,i2}^{od,*} Z_{L,j3}^{Di,*} Z_{L,k3}^{Di,*} Z_{L,l2}^{od} \\
& - 8|Y_A|^2 Z_{L,i2}^{od,*} Z_{L,j3}^{Di,*} Z_{L,k3}^{Di,*} Z_{L,l2}^{od} - 2g_{B2}^2 Z_{L,i4}^{od,*} Z_{L,j4}^{Di,*} Z_{L,k3}^{Di,*} Z_{L,l2}^{od} \\
& - 2|Y_A|^2 Z_{L,i4}^{od,*} Z_{L,j4}^{Di,*} Z_{L,k3}^{Di,*} Z_{L,l2}^{od} + |Y_K|^2 Z_{L,i4}^{od,*} Z_{L,j4}^{Di,*} Z_{L,k3}^{Di,*} Z_{L,l2}^{od} \\
& - 2g_{B2}^2 Z_{L,i4}^{od,*} Z_{L,j3}^{Di,*} Z_{L,k4}^{Di,*} Z_{L,l2}^{od} - 2|Y_A|^2 Z_{L,i4}^{od,*} Z_{L,j3}^{Di,*} Z_{L,k4}^{Di,*} Z_{L,l2}^{od} \\
& + |Y_K|^2 Z_{L,i4}^{od,*} Z_{L,j3}^{Di,*} Z_{L,k4}^{Di,*} Z_{L,l2}^{od} - 2g_{A1}^2 Z_{L,i2}^{od,*} Z_{L,j4}^{Di,*} Z_{L,k4}^{Di,*} Z_{L,l2}^{od} \\
& - 2g_{A2}^2 Z_{L,i2}^{od,*} Z_{L,j4}^{Di,*} Z_{L,k4}^{Di,*} Z_{L,l2}^{od} - 2g_{B1}^2 Z_{L,i2}^{od,*} Z_{L,j4}^{Di,*} Z_{L,k4}^{Di,*} Z_{L,l2}^{od} \\
& - 2g_{B2}^2 Z_{L,i2}^{od,*} Z_{L,j4}^{Di,*} Z_{L,k4}^{Di,*} Z_{L,l2}^{od} + 2g_{A2}^2 Z_{L,i4}^{od,*} Z_{L,j4}^{Di,*} Z_{L,k1}^{Di,*} Z_{L,l3}^{od} \\
& - 4|Y_A|^2 Z_{L,i4}^{od,*} Z_{L,j4}^{Di,*} Z_{L,k1}^{Di,*} Z_{L,l3}^{od} + 2g_{B2}^2 Z_{L,i4}^{od,*} Z_{L,j3}^{Di,*} Z_{L,k2}^{Di,*} Z_{L,l3}^{od} \\
& + 2g_{A2}^2 Z_{L,i2}^{od,*} Z_{L,j4}^{Di,*} Z_{L,k2}^{Di,*} Z_{L,l3}^{od} + 2g_{B2}^2 Z_{L,i2}^{od,*} Z_{L,j4}^{Di,*} Z_{L,k2}^{Di,*} Z_{L,l3}^{od} \\
& + 2g_{B2}^2 Z_{L,i4}^{od,*} Z_{L,j2}^{Di,*} Z_{L,k3}^{Di,*} Z_{L,l3}^{od} + 2g_{A2}^2 Z_{L,i4}^{od,*} Z_{L,j1}^{Di,*} Z_{L,k4}^{Di,*} Z_{L,l3}^{od} \Big)
\end{aligned}$$

$$\begin{aligned}
& -4|Y_A|^2 Z_{Ls,i4}^{od,*} Z_{Ls,j1}^{Di,*} Z_{Ls,k4}^{Di,*} Z_{Ls,l3}^{od} + 2g_{A2}^2 Z_{Ls,i2}^{od,*} Z_{Ls,j2}^{Di,*} Z_{Ls,k4}^{Di,*} Z_{Ls,l3}^{od} \\
& + 2g_{B2}^2 Z_{Ls,i2}^{od,*} Z_{Ls,j2}^{Di,*} Z_{Ls,k4}^{Di,*} Z_{Ls,l3}^{od} - 2g_{A1}^2 Z_{Ls,i4}^{od,*} Z_{Ls,j1}^{Di,*} Z_{Ls,k1}^{Di,*} Z_{Ls,l4}^{od} \\
& - 2g_{A2}^2 Z_{Ls,i4}^{od,*} Z_{Ls,j1}^{Di,*} Z_{Ls,k1}^{Di,*} Z_{Ls,l4}^{od} - 2g_{B1}^2 Z_{Ls,i4}^{od,*} Z_{Ls,j1}^{Di,*} Z_{Ls,k1}^{Di,*} Z_{Ls,l4}^{od} \\
& - 2g_{B2}^2 Z_{Ls,i4}^{od,*} Z_{Ls,j1}^{Di,*} Z_{Ls,k1}^{Di,*} Z_{Ls,l4}^{od} - 2g_{A2}^2 Z_{Ls,i2}^{od,*} Z_{Ls,j2}^{Di,*} Z_{Ls,k1}^{Di,*} Z_{Ls,l4}^{od} \\
& + 2|Y_A|^2 Z_{Ls,i2}^{od,*} Z_{Ls,j2}^{Di,*} Z_{Ls,k1}^{Di,*} Z_{Ls,l4}^{od} + |Y_K|^2 Z_{Ls,i2}^{od,*} Z_{Ls,j2}^{Di,*} Z_{Ls,k1}^{Di,*} Z_{Ls,l4}^{od} \\
& - 2g_{A2}^2 Z_{Ls,i2}^{od,*} Z_{Ls,j1}^{Di,*} Z_{Ls,k2}^{Di,*} Z_{Ls,l4}^{od} + 2|Y_A|^2 Z_{Ls,i2}^{od,*} Z_{Ls,j1}^{Di,*} Z_{Ls,k2}^{Di,*} Z_{Ls,l4}^{od} \\
& + |Y_K|^2 Z_{Ls,i2}^{od,*} Z_{Ls,j1}^{Di,*} Z_{Ls,k2}^{Di,*} Z_{Ls,l4}^{od} + 2g_{A1}^2 Z_{Ls,i4}^{od,*} Z_{Ls,j2}^{Di,*} Z_{Ls,k2}^{Di,*} Z_{Ls,l4}^{od} \\
& - 2g_{A2}^2 Z_{Ls,i4}^{od,*} Z_{Ls,j2}^{Di,*} Z_{Ls,k2}^{Di,*} Z_{Ls,l4}^{od} + 2g_{B1}^2 Z_{Ls,i4}^{od,*} Z_{Ls,j2}^{Di,*} Z_{Ls,k2}^{Di,*} Z_{Ls,l4}^{od} \\
& + 2g_{B2}^2 Z_{Ls,i4}^{od,*} Z_{Ls,j2}^{Di,*} Z_{Ls,k2}^{Di,*} Z_{Ls,l4}^{od} - 2g_{A1}^2 Z_{Ls,i4}^{od,*} Z_{Ls,j3}^{Di,*} Z_{Ls,k3}^{Di,*} Z_{Ls,l4}^{od} \\
& - 2g_{A2}^2 Z_{Ls,i4}^{od,*} Z_{Ls,j3}^{Di,*} Z_{Ls,k3}^{Di,*} Z_{Ls,l4}^{od} - 2g_{B1}^2 Z_{Ls,i4}^{od,*} Z_{Ls,j3}^{Di,*} Z_{Ls,k3}^{Di,*} Z_{Ls,l4}^{od} \\
& - 2g_{B2}^2 Z_{Ls,i4}^{od,*} Z_{Ls,j3}^{Di,*} Z_{Ls,k3}^{Di,*} Z_{Ls,l4}^{od} - 2g_{B2}^2 Z_{Ls,i2}^{od,*} Z_{Ls,j4}^{Di,*} Z_{Ls,k3}^{Di,*} Z_{Ls,l4}^{od} \\
& - 2|Y_A|^2 Z_{Ls,i2}^{od,*} Z_{Ls,j4}^{Di,*} Z_{Ls,k3}^{Di,*} Z_{Ls,l4}^{od} + |Y_K|^2 Z_{Ls,i2}^{od,*} Z_{Ls,j4}^{Di,*} Z_{Ls,k3}^{Di,*} Z_{Ls,l4}^{od} \\
& - 2g_{B2}^2 Z_{Ls,i2}^{od,*} Z_{Ls,j3}^{Di,*} Z_{Ls,k4}^{Di,*} Z_{Ls,l4}^{od} - 2|Y_A|^2 Z_{Ls,i2}^{od,*} Z_{Ls,j3}^{Di,*} Z_{Ls,k4}^{Di,*} Z_{Ls,l4}^{od} \\
& + |Y_K|^2 Z_{Ls,i2}^{od,*} Z_{Ls,j3}^{Di,*} Z_{Ls,k4}^{Di,*} Z_{Ls,l4}^{od} + 2g_{A1}^2 Z_{Ls,i4}^{od,*} Z_{Ls,j4}^{Di,*} Z_{Ls,k4}^{Di,*} Z_{Ls,l4}^{od} \\
& + 2g_{A2}^2 Z_{Ls,i4}^{od,*} Z_{Ls,j4}^{Di,*} Z_{Ls,k4}^{Di,*} Z_{Ls,l4}^{od} + 2g_{B1}^2 Z_{Ls,i4}^{od,*} Z_{Ls,j4}^{Di,*} Z_{Ls,k4}^{Di,*} Z_{Ls,l4}^{od} \\
& - 2g_{B2}^2 Z_{Ls,i4}^{od,*} Z_{Ls,j4}^{Di,*} Z_{Ls,k4}^{Di,*} Z_{Ls,l4}^{od} - 8|Y_A|^2 Z_{Ls,i4}^{od,*} Z_{Ls,j4}^{Di,*} Z_{Ls,k4}^{Di,*} Z_{Ls,l4}^{od} \\
& + Z_{Ls,i1}^{od,*} \left( -2g_{A1}^2 Z_{Ls,j3}^{Di,*} Z_{Ls,k3}^{Di,*} Z_{Ls,l1}^{od} - 2g_{A2}^2 Z_{Ls,j3}^{Di,*} Z_{Ls,k3}^{Di,*} Z_{Ls,l1}^{od} - 2g_{B1}^2 Z_{Ls,j3}^{Di,*} Z_{Ls,k3}^{Di,*} Z_{Ls,l1}^{od} \right. \\
& - 2g_{B2}^2 Z_{Ls,j3}^{Di,*} Z_{Ls,k3}^{Di,*} Z_{Ls,l1}^{od} + 2g_{A1}^2 Z_{Ls,j4}^{Di,*} Z_{Ls,k4}^{Di,*} Z_{Ls,l1}^{od} - 2g_{A2}^2 Z_{Ls,j4}^{Di,*} Z_{Ls,k4}^{Di,*} Z_{Ls,l1}^{od} \\
& + 2g_{B1}^2 Z_{Ls,j4}^{Di,*} Z_{Ls,k4}^{Di,*} Z_{Ls,l1}^{od} + 2g_{B2}^2 Z_{Ls,j4}^{Di,*} Z_{Ls,k4}^{Di,*} Z_{Ls,l1}^{od} + 2g_{B2}^2 Z_{Ls,j4}^{Di,*} Z_{Ls,k1}^{Di,*} Z_{Ls,l2}^{od} \\
& + 2g_{A2}^2 Z_{Ls,j3}^{Di,*} Z_{Ls,k2}^{Di,*} Z_{Ls,l2}^{od} - 4|Y_A|^2 Z_{Ls,j3}^{Di,*} Z_{Ls,k2}^{Di,*} Z_{Ls,l2}^{od} - 2g_{A2}^2 Z_{Ls,j4}^{Di,*} Z_{Ls,k3}^{Di,*} Z_{Ls,l3}^{od} \\
& + 2|Y_A|^2 Z_{Ls,j4}^{Di,*} Z_{Ls,k3}^{Di,*} Z_{Ls,l3}^{od} + |Y_K|^2 Z_{Ls,j4}^{Di,*} Z_{Ls,k3}^{Di,*} Z_{Ls,l3}^{od} - 2g_{A2}^2 Z_{Ls,j3}^{Di,*} Z_{Ls,k4}^{Di,*} Z_{Ls,l3}^{od} \\
& + 2|Y_A|^2 Z_{Ls,j3}^{Di,*} Z_{Ls,k4}^{Di,*} Z_{Ls,l3}^{od} + |Y_K|^2 Z_{Ls,j3}^{Di,*} Z_{Ls,k4}^{Di,*} Z_{Ls,l3}^{od} \\
& + Z_{Ls,j2}^{Di,*} \left( 2 \left( -4|Y_A|^2 - g_{B2}^2 + g_{A1}^2 + g_{A2}^2 + g_{B1}^2 \right) Z_{Ls,k2}^{Di,*} Z_{Ls,l1}^{od} + 2 \left( -2|Y_A|^2 + g_{A2}^2 \right) Z_{Ls,k3}^{Di,*} Z_{Ls,l2}^{od} \right. \\
& + \left. \left( -2g_{B2}^2 - 2|Y_A|^2 + |Y_K|^2 \right) Z_{Ls,k1}^{Di,*} Z_{Ls,l3}^{od} \right) \\
& + 2g_{A2}^2 Z_{Ls,j3}^{Di,*} Z_{Ls,k1}^{Di,*} Z_{Ls,l4}^{od} + 2g_{B2}^2 Z_{Ls,j3}^{Di,*} Z_{Ls,k1}^{Di,*} Z_{Ls,l4}^{od} \\
& + Z_{Ls,j1}^{Di,*} \left( -2 \left( g_{A1}^2 + g_{A2}^2 + g_{B1}^2 + g_{B2}^2 \right) Z_{Ls,k1}^{Di,*} Z_{Ls,l1}^{od} + 2g_{B2}^2 Z_{Ls,k4}^{Di,*} Z_{Ls,l2}^{od} - 2g_{B2}^2 Z_{Ls,k2}^{Di,*} Z_{Ls,l3}^{od} \right. \\
& - 2|Y_A|^2 Z_{Ls,k2}^{Di,*} Z_{Ls,l3}^{od} + |Y_K|^2 Z_{Ls,k2}^{Di,*} Z_{Ls,l3}^{od} + 2g_{A2}^2 Z_{Ls,k3}^{Di,*} Z_{Ls,l4}^{od} + 2g_{B2}^2 Z_{Ls,k3}^{Di,*} Z_{Ls,l4}^{od} \left. \right) \\
& + Z_{Ls,i3}^{od,*} \left( -2g_{A2}^2 Z_{Ls,j4}^{Di,*} Z_{Ls,k3}^{Di,*} Z_{Ls,l1}^{od} + 2|Y_A|^2 Z_{Ls,j4}^{Di,*} Z_{Ls,k3}^{Di,*} Z_{Ls,l1}^{od} + |Y_K|^2 Z_{Ls,j4}^{Di,*} Z_{Ls,k3}^{Di,*} Z_{Ls,l1}^{od} \right. \\
& - 2g_{A2}^2 Z_{Ls,j3}^{Di,*} Z_{Ls,k4}^{Di,*} Z_{Ls,l1}^{od} + 2|Y_A|^2 Z_{Ls,j3}^{Di,*} Z_{Ls,k4}^{Di,*} Z_{Ls,l1}^{od} + |Y_K|^2 Z_{Ls,j3}^{Di,*} Z_{Ls,k4}^{Di,*} Z_{Ls,l1}^{od}
\end{aligned}$$

$$\begin{aligned}
& + 2g_{A2}^2 Z_{Ls,j4}^{Di,*} Z_{Ls,k2}^{Di,*} Z_{Ls,l2}^{od} + 2g_{B2}^2 Z_{Ls,j4}^{Di,*} Z_{Ls,k2}^{Di,*} Z_{Ls,l2}^{od} + 2g_{A1}^2 Z_{Ls,j3}^{Di,*} Z_{Ls,k3}^{Di,*} Z_{Ls,l3}^{od} \\
& - 2g_{A2}^2 Z_{Ls,j3}^{Di,*} Z_{Ls,k3}^{Di,*} Z_{Ls,l3}^{od} + 2g_{B1}^2 Z_{Ls,j3}^{Di,*} Z_{Ls,k3}^{Di,*} Z_{Ls,l3}^{od} + 2g_{B2}^2 Z_{Ls,j3}^{Di,*} Z_{Ls,k3}^{Di,*} Z_{Ls,l3}^{od} \\
& - 2g_{A1}^2 Z_{Ls,j4}^{Di,*} Z_{Ls,k4}^{Di,*} Z_{Ls,l3}^{od} - 2g_{A2}^2 Z_{Ls,j4}^{Di,*} Z_{Ls,k4}^{Di,*} Z_{Ls,l3}^{od} - 2g_{B1}^2 Z_{Ls,j4}^{Di,*} Z_{Ls,k4}^{Di,*} Z_{Ls,l3}^{od} \\
& - 2g_{B2}^2 Z_{Ls,j4}^{Di,*} Z_{Ls,k4}^{Di,*} Z_{Ls,l3}^{od} + 2g_{A2}^2 Z_{Ls,j4}^{Di,*} Z_{Ls,k1}^{Di,*} Z_{Ls,l4}^{od} - 4|Y_A|^2 Z_{Ls,j4}^{Di,*} Z_{Ls,k1}^{Di,*} Z_{Ls,l4}^{od} \\
& + 2g_{B2}^2 Z_{Ls,j3}^{Di,*} Z_{Ls,k2}^{Di,*} Z_{Ls,l4}^{od} \\
& + Z_{Ls,j2}^{Di,*} \left( \left( -2g_{B2}^2 - 2|Y_A|^2 + |Y_K|^2 \right) Z_{Ls,k1}^{Di,*} Z_{Ls,l1}^{od} \right. \\
& + 2 \left( - \left( g_{A1}^2 + g_{A2}^2 + g_{B1}^2 + g_{B2}^2 \right) Z_{Ls,k2}^{Di,*} Z_{Ls,l3}^{od} + \left( g_{A2}^2 + g_{B2}^2 \right) Z_{Ls,k4}^{Di,*} Z_{Ls,l2}^{od} + g_{B2}^2 Z_{Ls,k3}^{Di,*} Z_{Ls,l4}^{od} \right) \\
& + Z_{Ls,j1}^{Di,*} \left( \left( -2g_{B2}^2 - 2|Y_A|^2 + |Y_K|^2 \right) Z_{Ls,k2}^{Di,*} Z_{Ls,l1}^{od} \right. \\
& \left. \left. + 2 \left( \left( -2|Y_A|^2 + g_{A2}^2 \right) Z_{Ls,k4}^{Di,*} Z_{Ls,l4}^{od} + \left( -4|Y_A|^2 - g_{B2}^2 + g_{A1}^2 + g_{A2}^2 + g_{B1}^2 \right) Z_{Ls,k1}^{Di,*} Z_{Ls,l3}^{od} \right) \right) \right) \quad (891)
\end{aligned}$$


---

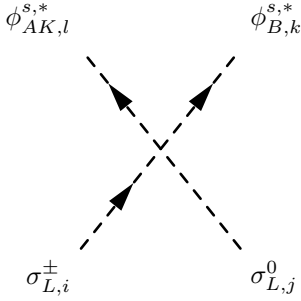

$$\begin{aligned}
& \frac{1}{2} \left( Y_A Y_K^* \left( -Z_{Ls,i1}^{od,*} Z_{Ls,j1}^{Di,*} - Z_{Ls,i2}^{od,*} Z_{Ls,j4}^{Di,*} + Z_{Ls,i3}^{od,*} Z_{Ls,j2}^{Di,*} + Z_{Ls,i4}^{od,*} Z_{Ls,j3}^{Di,*} \right) Z_{AK,l1}^s \right. \\
& \left. + \sqrt{2} \left( -|Y_A|^2 + g_{B2}^2 \right) \left( Z_{Ls,i1}^{od,*} Z_{Ls,j1}^{Di,*} - Z_{Ls,i2}^{od,*} Z_{Ls,j4}^{Di,*} + Z_{Ls,i3}^{od,*} Z_{Ls,j2}^{Di,*} - Z_{Ls,i4}^{od,*} Z_{Ls,j3}^{Di,*} \right) Z_{AK,l2}^s \right) B_{A,k2}^s \quad (892)
\end{aligned}$$


---

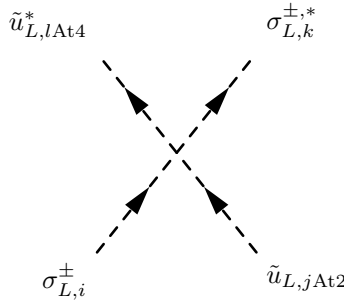

$$\begin{aligned}
& \frac{i}{12} \delta_{At2At4} \delta_{jl} \left( \left( -3g_{A2}^2 + g_{A1}^2 \right) Z_{Ls,i1}^{od,*} Z_{Ls,k1}^{od} - \left( 3g_{A2}^2 + g_{A1}^2 \right) Z_{Ls,i2}^{od,*} Z_{Ls,k2}^{od} - g_{A1}^2 Z_{Ls,i3}^{od,*} Z_{Ls,k3}^{od} + 3g_{A2}^2 Z_{Ls,i3}^{od,*} Z_{Ls,k3}^{od} \right. \\
& \left. + g_{A1}^2 Z_{Ls,i4}^{od,*} Z_{Ls,k4}^{od} + 3g_{A2}^2 Z_{Ls,i4}^{od,*} Z_{Ls,k4}^{od} \right) \quad (893)
\end{aligned}$$


---

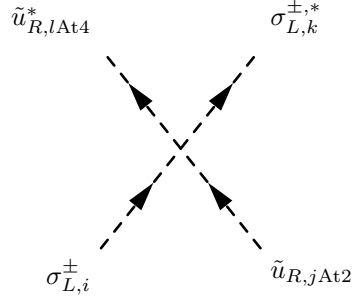

$$-\frac{i}{3}g_{A1}^2\delta_{At2At4}\delta_{jl}\left(Z_{Ls,i1}^{od,*}Z_{Ls,k1}^{od}-Z_{Ls,i2}^{od,*}Z_{Ls,k2}^{od}-Z_{Ls,i3}^{od,*}Z_{Ls,k3}^{od}+Z_{Ls,i4}^{od,*}Z_{Ls,k4}^{od}\right) \quad (894)$$


---

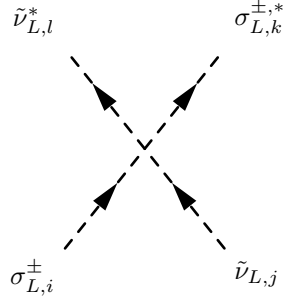

$$-\frac{i}{4}\delta_{jl}\left(\left(g_{A1}^2+g_{A2}^2\right)Z_{Ls,i1}^{od,*}Z_{Ls,k1}^{od}+\left(-g_{A1}^2+g_{A2}^2\right)Z_{Ls,i2}^{od,*}Z_{Ls,k2}^{od}-g_{A1}^2Z_{Ls,i3}^{od,*}Z_{Ls,k3}^{od}-g_{A2}^2Z_{Ls,i3}^{od,*}Z_{Ls,k3}^{od}\right. \\ \left.+g_{A1}^2Z_{Ls,i4}^{od,*}Z_{Ls,k4}^{od}-g_{A2}^2Z_{Ls,i4}^{od,*}Z_{Ls,k4}^{od}\right) \quad (895)$$


---

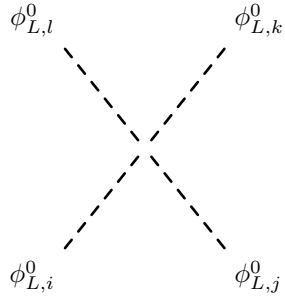

$$-\frac{i}{2}\left(2g_{A1}^2Z_{Ls,i3}^{DR,*}Z_{Ls,j3}^{DR,*}Z_{Ls,k1}^{DR,*}Z_{Ls,l1}^{DR,*}-2g_{A2}^2Z_{Ls,i3}^{DR,*}Z_{Ls,j3}^{DR,*}Z_{Ls,k1}^{DR,*}Z_{Ls,l1}^{DR,*}\right. \\ \left.+2g_{B1}^2Z_{Ls,i3}^{DR,*}Z_{Ls,j3}^{DR,*}Z_{Ls,k1}^{DR,*}Z_{Ls,l1}^{DR,*}-2g_{B2}^2Z_{Ls,i3}^{DR,*}Z_{Ls,j3}^{DR,*}Z_{Ls,k1}^{DR,*}Z_{Ls,l1}^{DR,*}\right)$$

[illegible]



[illegible]

$$\begin{aligned}
& + 2g_{A2}^2 Z_{Ls,j3}^{DR,*} Z_{Ls,k2}^{DR,*} Z_{Ls,l3}^{DR,*} - 2g_{B1}^2 Z_{Ls,j3}^{DR,*} Z_{Ls,k2}^{DR,*} Z_{Ls,l3}^{DR,*} + 2g_{B2}^2 Z_{Ls,j3}^{DR,*} Z_{Ls,k2}^{DR,*} Z_{Ls,l3}^{DR,*} \\
& - 2|Y_A|^2 Z_{Ls,j3}^{DR,*} Z_{Ls,k1}^{DR,*} Z_{Ls,l4}^{DR,*} + |Y_K|^2 Z_{Ls,j3}^{DR,*} Z_{Ls,k1}^{DR,*} Z_{Ls,l4}^{DR,*} + 2g_{A1}^2 Z_{Ls,j4}^{DR,*} Z_{Ls,k2}^{DR,*} Z_{Ls,l4}^{DR,*} \\
& - 2g_{A2}^2 Z_{Ls,j4}^{DR,*} Z_{Ls,k2}^{DR,*} Z_{Ls,l4}^{DR,*} + 2g_{B1}^2 Z_{Ls,j4}^{DR,*} Z_{Ls,k2}^{DR,*} Z_{Ls,l4}^{DR,*} - 2g_{B2}^2 Z_{Ls,j4}^{DR,*} Z_{Ls,k2}^{DR,*} Z_{Ls,l4}^{DR,*} \\
& - Z_{Ls,j1}^{DR,*} \left( 2 \left( -2|Y_A|^2 - |Y_K|^2 + g_{A1}^2 + g_{A2}^2 + g_{B1}^2 + g_{B2}^2 \right) Z_{Ls,k2}^{DR,*} Z_{Ls,l1}^{DR,*} \right. \\
& + 2 \left( -2|Y_A|^2 - |Y_K|^2 + g_{A1}^2 + g_{A2}^2 + g_{B1}^2 + g_{B2}^2 \right) Z_{Ls,k1}^{DR,*} Z_{Ls,l2}^{DR,*} \\
& + \left( 2|Y_A|^2 - |Y_K|^2 \right) \left( Z_{Ls,k3}^{DR,*} Z_{Ls,l4}^{DR,*} + Z_{Ls,k4}^{DR,*} Z_{Ls,l3}^{DR,*} \right) \Big) \\
& - 2Z_{Ls,j2}^{DR,*} \left( \left( -2|Y_A|^2 - |Y_K|^2 + g_{A1}^2 + g_{A2}^2 + g_{B1}^2 + g_{B2}^2 \right) Z_{Ls,k1}^{DR,*} Z_{Ls,l1}^{DR,*} - 3 \left( g_{A1}^2 + g_{A2}^2 + g_{B1}^2 + g_{B2}^2 \right) Z_{Ls,k2}^{DR,*} Z_{Ls,l2}^{DR,*} \right. \\
& + \left( -g_{A2}^2 - g_{B2}^2 + g_{A1}^2 + g_{B1}^2 \right) \left( Z_{Ls,k3}^{DR,*} Z_{Ls,l3}^{DR,*} - Z_{Ls,k4}^{DR,*} Z_{Ls,l4}^{DR,*} \right) \Big) \\
& + Z_{Ls,i1}^{DR,*} \left( -2g_{A1}^2 Z_{Ls,j2}^{DR,*} Z_{Ls,k2}^{DR,*} Z_{Ls,l1}^{DR,*} - 2g_{A2}^2 Z_{Ls,j2}^{DR,*} Z_{Ls,k2}^{DR,*} Z_{Ls,l1}^{DR,*} - 2g_{B1}^2 Z_{Ls,j2}^{DR,*} Z_{Ls,k2}^{DR,*} Z_{Ls,l1}^{DR,*} \right. \\
& - 2g_{B2}^2 Z_{Ls,j2}^{DR,*} Z_{Ls,k2}^{DR,*} Z_{Ls,l1}^{DR,*} + 4|Y_A|^2 Z_{Ls,j2}^{DR,*} Z_{Ls,k2}^{DR,*} Z_{Ls,l1}^{DR,*} + 2|Y_K|^2 Z_{Ls,j2}^{DR,*} Z_{Ls,k2}^{DR,*} Z_{Ls,l1}^{DR,*} \\
& + 2g_{A1}^2 Z_{Ls,j3}^{DR,*} Z_{Ls,k3}^{DR,*} Z_{Ls,l1}^{DR,*} - 2g_{A2}^2 Z_{Ls,j3}^{DR,*} Z_{Ls,k3}^{DR,*} Z_{Ls,l1}^{DR,*} + 2g_{B1}^2 Z_{Ls,j3}^{DR,*} Z_{Ls,k3}^{DR,*} Z_{Ls,l1}^{DR,*} \\
& - 2g_{B2}^2 Z_{Ls,j3}^{DR,*} Z_{Ls,k3}^{DR,*} Z_{Ls,l1}^{DR,*} - 2g_{A1}^2 Z_{Ls,j4}^{DR,*} Z_{Ls,k4}^{DR,*} Z_{Ls,l1}^{DR,*} + 2g_{A2}^2 Z_{Ls,j4}^{DR,*} Z_{Ls,k4}^{DR,*} Z_{Ls,l1}^{DR,*} \\
& - 2g_{B1}^2 Z_{Ls,j4}^{DR,*} Z_{Ls,k4}^{DR,*} Z_{Ls,l1}^{DR,*} + 2g_{B2}^2 Z_{Ls,j4}^{DR,*} Z_{Ls,k4}^{DR,*} Z_{Ls,l1}^{DR,*} - 2g_{A1}^2 Z_{Ls,j2}^{DR,*} Z_{Ls,k1}^{DR,*} Z_{Ls,l2}^{DR,*} \\
& - 2g_{A2}^2 Z_{Ls,j2}^{DR,*} Z_{Ls,k1}^{DR,*} Z_{Ls,l2}^{DR,*} - 2g_{B1}^2 Z_{Ls,j2}^{DR,*} Z_{Ls,k1}^{DR,*} Z_{Ls,l2}^{DR,*} - 2g_{B2}^2 Z_{Ls,j2}^{DR,*} Z_{Ls,k1}^{DR,*} Z_{Ls,l2}^{DR,*} \\
& + 4|Y_A|^2 Z_{Ls,j2}^{DR,*} Z_{Ls,k1}^{DR,*} Z_{Ls,l2}^{DR,*} + 2|Y_K|^2 Z_{Ls,j2}^{DR,*} Z_{Ls,k1}^{DR,*} Z_{Ls,l2}^{DR,*} - 2|Y_A|^2 Z_{Ls,j4}^{DR,*} Z_{Ls,k3}^{DR,*} Z_{Ls,l2}^{DR,*} \\
& + |Y_K|^2 Z_{Ls,j4}^{DR,*} Z_{Ls,k3}^{DR,*} Z_{Ls,l2}^{DR,*} - 2|Y_A|^2 Z_{Ls,j3}^{DR,*} Z_{Ls,k4}^{DR,*} Z_{Ls,l2}^{DR,*} + |Y_K|^2 Z_{Ls,j3}^{DR,*} Z_{Ls,k4}^{DR,*} Z_{Ls,l2}^{DR,*} \\
& + 2g_{A1}^2 Z_{Ls,j3}^{DR,*} Z_{Ls,k1}^{DR,*} Z_{Ls,l3}^{DR,*} - 2g_{A2}^2 Z_{Ls,j3}^{DR,*} Z_{Ls,k1}^{DR,*} Z_{Ls,l3}^{DR,*} + 2g_{B1}^2 Z_{Ls,j3}^{DR,*} Z_{Ls,k1}^{DR,*} Z_{Ls,l3}^{DR,*} \\
& - 2g_{B2}^2 Z_{Ls,j3}^{DR,*} Z_{Ls,k1}^{DR,*} Z_{Ls,l3}^{DR,*} - 2|Y_A|^2 Z_{Ls,j4}^{DR,*} Z_{Ls,k2}^{DR,*} Z_{Ls,l3}^{DR,*} + |Y_K|^2 Z_{Ls,j4}^{DR,*} Z_{Ls,k2}^{DR,*} Z_{Ls,l3}^{DR,*} \\
& - 2|Y_A|^2 Z_{Ls,j2}^{DR,*} Z_{Ls,k4}^{DR,*} Z_{Ls,l3}^{DR,*} + |Y_K|^2 Z_{Ls,j2}^{DR,*} Z_{Ls,k4}^{DR,*} Z_{Ls,l3}^{DR,*} - 2g_{A1}^2 Z_{Ls,j4}^{DR,*} Z_{Ls,k1}^{DR,*} Z_{Ls,l4}^{DR,*} \\
& + 2g_{A2}^2 Z_{Ls,j4}^{DR,*} Z_{Ls,k1}^{DR,*} Z_{Ls,l4}^{DR,*} - 2g_{B1}^2 Z_{Ls,j4}^{DR,*} Z_{Ls,k1}^{DR,*} Z_{Ls,l4}^{DR,*} + 2g_{B2}^2 Z_{Ls,j4}^{DR,*} Z_{Ls,k1}^{DR,*} Z_{Ls,l4}^{DR,*} \\
& - 2|Y_A|^2 Z_{Ls,j3}^{DR,*} Z_{Ls,k2}^{DR,*} Z_{Ls,l4}^{DR,*} + |Y_K|^2 Z_{Ls,j3}^{DR,*} Z_{Ls,k2}^{DR,*} Z_{Ls,l4}^{DR,*} - 2|Y_A|^2 Z_{Ls,j2}^{DR,*} Z_{Ls,k3}^{DR,*} Z_{Ls,l4}^{DR,*} \\
& + |Y_K|^2 Z_{Ls,j2}^{DR,*} Z_{Ls,k3}^{DR,*} Z_{Ls,l4}^{DR,*} \\
& + 2Z_{Ls,j1}^{DR,*} \left( 3 \left( g_{A1}^2 + g_{A2}^2 + g_{B1}^2 + g_{B2}^2 \right) Z_{Ls,k1}^{DR,*} Z_{Ls,l1}^{DR,*} - \left( -2|Y_A|^2 - |Y_K|^2 + g_{A1}^2 + g_{A2}^2 + g_{B1}^2 + g_{B2}^2 \right) Z_{Ls,k2}^{DR,*} Z_{Ls,l2}^{DR,*} \right. \\
& + \left( -g_{A2}^2 - g_{B2}^2 + g_{A1}^2 + g_{B1}^2 \right) \left( Z_{Ls,k3}^{DR,*} Z_{Ls,l3}^{DR,*} - Z_{Ls,k4}^{DR,*} Z_{Ls,l4}^{DR,*} \right) \Big) \Big) \quad (896)
\end{aligned}$$

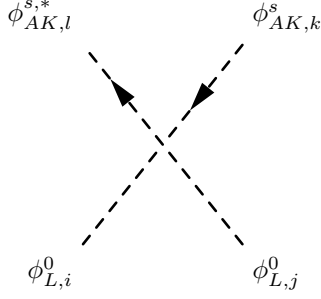

$$\begin{aligned}
& -\frac{i}{2} \left( Y_K^* \left( \sqrt{2} Y_A Z_{AK,k2}^{s,*} \left( Z_{Ls,i1}^{DR,*} Z_{Ls,j1}^{DR,*} + Z_{Ls,i2}^{DR,*} Z_{Ls,j2}^{DR,*} - Z_{Ls,i3}^{DR,*} Z_{Ls,j3}^{DR,*} - Z_{Ls,i4}^{DR,*} Z_{Ls,j4}^{DR,*} \right) \right. \right. \\
& + Y_K Z_{AK,k1}^{s,*} \left( Z_{Ls,i1}^{DR,*} Z_{Ls,j1}^{DR,*} + Z_{Ls,i2}^{DR,*} Z_{Ls,j2}^{DR,*} + Z_{Ls,i3}^{DR,*} Z_{Ls,j3}^{DR,*} + Z_{Ls,i4}^{DR,*} Z_{Ls,j4}^{DR,*} \right) \left. \right) Z_{AK,l1}^s \\
& + Y_A^* \left( \sqrt{2} Y_K Z_{AK,k1}^{s,*} \left( Z_{Ls,i1}^{DR,*} Z_{Ls,j1}^{DR,*} + Z_{Ls,i2}^{DR,*} Z_{Ls,j2}^{DR,*} - Z_{Ls,i3}^{DR,*} Z_{Ls,j3}^{DR,*} - Z_{Ls,i4}^{DR,*} Z_{Ls,j4}^{DR,*} \right) \right. \\
& \left. \left. + 2 Y_A Z_{AK,k2}^{s,*} \left( Z_{Ls,i1}^{DR,*} Z_{Ls,j1}^{DR,*} + Z_{Ls,i2}^{DR,*} Z_{Ls,j2}^{DR,*} + Z_{Ls,i3}^{DR,*} Z_{Ls,j3}^{DR,*} + Z_{Ls,i4}^{DR,*} Z_{Ls,j4}^{DR,*} \right) \right) Z_{AK,l2}^s \right) \quad (897)
\end{aligned}$$


---

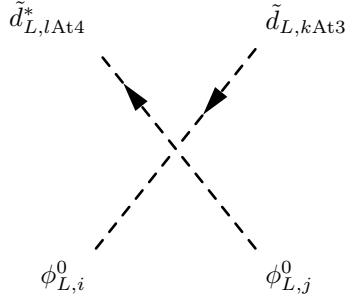

$$\begin{aligned}
& \frac{i}{6} \left( \left( 3g_{A2}^2 + g_{A1}^2 \right) Z_{Ls,i1}^{DR,*} Z_{Ls,j1}^{DR,*} - \left( 3g_{A2}^2 + g_{A1}^2 \right) Z_{Ls,i2}^{DR,*} Z_{Ls,j2}^{DR,*} \right. \\
& \left. + \left( -3g_{A2}^2 + g_{A1}^2 \right) \left( Z_{Ls,i3}^{DR,*} Z_{Ls,j3}^{DR,*} - Z_{Ls,i4}^{DR,*} Z_{Ls,j4}^{DR,*} \right) \right) \delta_{At3At4} \delta_{kl} \quad (898)
\end{aligned}$$


---

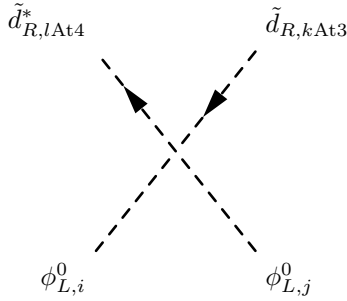

$$\frac{i}{3}g_{A1}^2 \left( Z_{Ls,i1}^{DR,*} Z_{Ls,j1}^{DR,*} - Z_{Ls,i2}^{DR,*} Z_{Ls,j2}^{DR,*} + Z_{Ls,i3}^{DR,*} Z_{Ls,j3}^{DR,*} - Z_{Ls,i4}^{DR,*} Z_{Ls,j4}^{DR,*} \right) \delta_{\text{At}3\text{At}4} \delta_{kl} \quad (899)$$


---

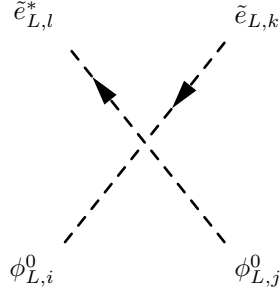

$$\begin{aligned} & -\frac{i}{2} \left( \left( -g_{A2}^2 + g_{A1}^2 \right) Z_{Ls,i1}^{DR,*} Z_{Ls,j1}^{DR,*} + \left( -g_{A1}^2 + g_{A2}^2 \right) Z_{Ls,i2}^{DR,*} Z_{Ls,j2}^{DR,*} \right. \\ & \left. + \left( g_{A1}^2 + g_{A2}^2 \right) \left( Z_{Ls,i3}^{DR,*} Z_{Ls,j3}^{DR,*} - Z_{Ls,i4}^{DR,*} Z_{Ls,j4}^{DR,*} \right) \right) \delta_{kl} \end{aligned} \quad (900)$$


---

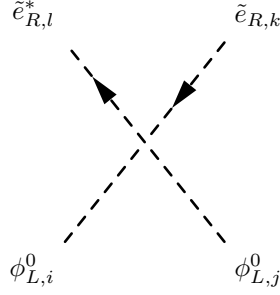

$$ig_{A1}^2 \left( Z_{Ls,i1}^{DR,*} Z_{Ls,j1}^{DR,*} - Z_{Ls,i2}^{DR,*} Z_{Ls,j2}^{DR,*} + Z_{Ls,i3}^{DR,*} Z_{Ls,j3}^{DR,*} - Z_{Ls,i4}^{DR,*} Z_{Ls,j4}^{DR,*} \right) \delta_{kl} \quad (901)$$


---

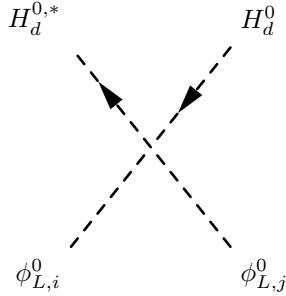

$$\begin{aligned}
& -\frac{i}{2} \left( (g_{A1}^2 + g_{A2}^2) Z_{Ls,i1}^{DR,*} Z_{Ls,j1}^{DR,*} - (g_{A1}^2 + g_{A2}^2) Z_{Ls,i2}^{DR,*} Z_{Ls,j2}^{DR,*} \right. \\
& \left. + (-g_{A2}^2 + g_{A1}^2) (Z_{Ls,i3}^{DR,*} Z_{Ls,j3}^{DR,*} - Z_{Ls,i4}^{DR,*} Z_{Ls,j4}^{DR,*}) \right)
\end{aligned} \tag{902}$$


---

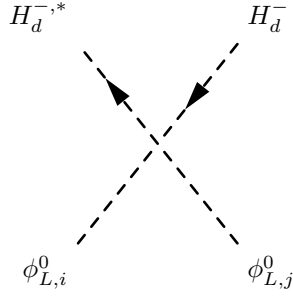

$$\begin{aligned}
& -\frac{i}{2} \left( (-g_{A2}^2 + g_{A1}^2) Z_{Ls,i1}^{DR,*} Z_{Ls,j1}^{DR,*} + (-g_{A1}^2 + g_{A2}^2) Z_{Ls,i2}^{DR,*} Z_{Ls,j2}^{DR,*} \right. \\
& \left. + (g_{A1}^2 + g_{A2}^2) (Z_{Ls,i3}^{DR,*} Z_{Ls,j3}^{DR,*} - Z_{Ls,i4}^{DR,*} Z_{Ls,j4}^{DR,*}) \right)
\end{aligned} \tag{903}$$


---

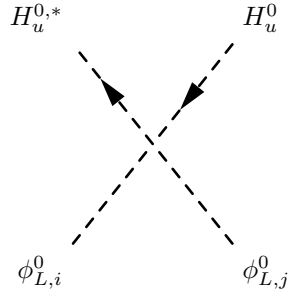

$$\begin{aligned}
& \frac{i}{2} \left( (g_{A1}^2 + g_{A2}^2) Z_{Ls,i1}^{DR,*} Z_{Ls,j1}^{DR,*} - (g_{A1}^2 + g_{A2}^2) Z_{Ls,i2}^{DR,*} Z_{Ls,j2}^{DR,*} \right. \\
& \left. + (-g_{A2}^2 + g_{A1}^2) (Z_{Ls,i3}^{DR,*} Z_{Ls,j3}^{DR,*} - Z_{Ls,i4}^{DR,*} Z_{Ls,j4}^{DR,*}) \right)
\end{aligned} \tag{904}$$


---

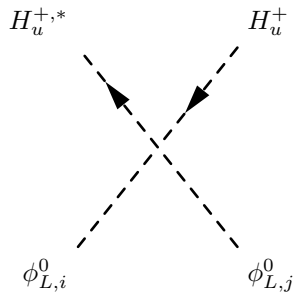

$$\begin{aligned}
& \frac{i}{2} \left( \left( -g_{A2}^2 + g_{A1}^2 \right) Z_{Ls,i1}^{DR,*} Z_{Ls,j1}^{DR,*} + \left( -g_{A1}^2 + g_{A2}^2 \right) Z_{Ls,i2}^{DR,*} Z_{Ls,j2}^{DR,*} \right. \\
& \left. + \left( g_{A1}^2 + g_{A2}^2 \right) \left( Z_{Ls,i3}^{DR,*} Z_{Ls,j3}^{DR,*} - Z_{Ls,i4}^{DR,*} Z_{Ls,j4}^{DR,*} \right) \right) \quad (905)
\end{aligned}$$


---

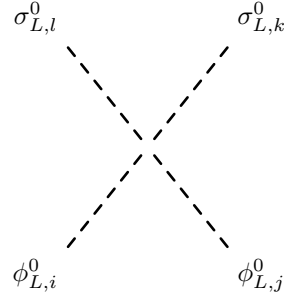

$$\begin{aligned}
& -\frac{i}{2} \left( 2g_{A1}^2 Z_{Ls,i3}^{DR,*} Z_{Ls,j3}^{DR,*} Z_{Ls,k1}^{Di,*} Z_{Ls,l1}^{Di,*} - 2g_{A2}^2 Z_{Ls,i3}^{DR,*} Z_{Ls,j3}^{DR,*} Z_{Ls,k1}^{Di,*} Z_{Ls,l1}^{Di,*} \right. \\
& + 2g_{B1}^2 Z_{Ls,i3}^{DR,*} Z_{Ls,j3}^{DR,*} Z_{Ls,k1}^{Di,*} Z_{Ls,l1}^{Di,*} - 2g_{B2}^2 Z_{Ls,i3}^{DR,*} Z_{Ls,j3}^{DR,*} Z_{Ls,k1}^{Di,*} Z_{Ls,l1}^{Di,*} \\
& - 2g_{A1}^2 Z_{Ls,i4}^{DR,*} Z_{Ls,j4}^{DR,*} Z_{Ls,k1}^{Di,*} Z_{Ls,l1}^{Di,*} + 2g_{A2}^2 Z_{Ls,i4}^{DR,*} Z_{Ls,j4}^{DR,*} Z_{Ls,k1}^{Di,*} Z_{Ls,l1}^{Di,*} \\
& - 2g_{B1}^2 Z_{Ls,i4}^{DR,*} Z_{Ls,j4}^{DR,*} Z_{Ls,k1}^{Di,*} Z_{Ls,l1}^{Di,*} + 2g_{B2}^2 Z_{Ls,i4}^{DR,*} Z_{Ls,j4}^{DR,*} Z_{Ls,k1}^{Di,*} Z_{Ls,l1}^{Di,*} \\
& + 2|Y_A|^2 Z_{Ls,i4}^{DR,*} Z_{Ls,j3}^{DR,*} Z_{Ls,k2}^{Di,*} Z_{Ls,l1}^{Di,*} - |Y_K|^2 Z_{Ls,i4}^{DR,*} Z_{Ls,j3}^{DR,*} Z_{Ls,k2}^{Di,*} Z_{Ls,l1}^{Di,*} \\
& + 2|Y_A|^2 Z_{Ls,i3}^{DR,*} Z_{Ls,j4}^{DR,*} Z_{Ls,k2}^{Di,*} Z_{Ls,l1}^{Di,*} - |Y_K|^2 Z_{Ls,i3}^{DR,*} Z_{Ls,j4}^{DR,*} Z_{Ls,k2}^{Di,*} Z_{Ls,l1}^{Di,*} \\
& - 2|Y_A|^2 Z_{Ls,i4}^{DR,*} Z_{Ls,j3}^{DR,*} Z_{Ls,k3}^{Di,*} Z_{Ls,l1}^{Di,*} + |Y_K|^2 Z_{Ls,i4}^{DR,*} Z_{Ls,j3}^{DR,*} Z_{Ls,k3}^{Di,*} Z_{Ls,l1}^{Di,*} \\
& - 2|Y_A|^2 Z_{Ls,i3}^{DR,*} Z_{Ls,j2}^{DR,*} Z_{Ls,k4}^{Di,*} Z_{Ls,l1}^{Di,*} + |Y_K|^2 Z_{Ls,i3}^{DR,*} Z_{Ls,j2}^{DR,*} Z_{Ls,k4}^{Di,*} Z_{Ls,l1}^{Di,*} \\
& + 2|Y_A|^2 Z_{Ls,i4}^{DR,*} Z_{Ls,j3}^{DR,*} Z_{Ls,k1}^{Di,*} Z_{Ls,l2}^{Di,*} - |Y_K|^2 Z_{Ls,i4}^{DR,*} Z_{Ls,j3}^{DR,*} Z_{Ls,k1}^{Di,*} Z_{Ls,l2}^{Di,*} \\
& + 2|Y_A|^2 Z_{Ls,i3}^{DR,*} Z_{Ls,j4}^{DR,*} Z_{Ls,k1}^{Di,*} Z_{Ls,l2}^{Di,*} - |Y_K|^2 Z_{Ls,i3}^{DR,*} Z_{Ls,j4}^{DR,*} Z_{Ls,k1}^{Di,*} Z_{Ls,l2}^{Di,*} \\
& - 2g_{A1}^2 Z_{Ls,i3}^{DR,*} Z_{Ls,j3}^{DR,*} Z_{Ls,k2}^{Di,*} Z_{Ls,l2}^{Di,*} + 2g_{A2}^2 Z_{Ls,i3}^{DR,*} Z_{Ls,j3}^{DR,*} Z_{Ls,k2}^{Di,*} Z_{Ls,l2}^{Di,*} \\
& - 2g_{B1}^2 Z_{Ls,i3}^{DR,*} Z_{Ls,j3}^{DR,*} Z_{Ls,k2}^{Di,*} Z_{Ls,l2}^{Di,*} + 2g_{B2}^2 Z_{Ls,i3}^{DR,*} Z_{Ls,j3}^{DR,*} Z_{Ls,k2}^{Di,*} Z_{Ls,l2}^{Di,*} \\
& + 2g_{A1}^2 Z_{Ls,i4}^{DR,*} Z_{Ls,j4}^{DR,*} Z_{Ls,k2}^{Di,*} Z_{Ls,l2}^{Di,*} - 2g_{A2}^2 Z_{Ls,i4}^{DR,*} Z_{Ls,j4}^{DR,*} Z_{Ls,k2}^{Di,*} Z_{Ls,l2}^{Di,*} \\
& + 2g_{B1}^2 Z_{Ls,i4}^{DR,*} Z_{Ls,j4}^{DR,*} Z_{Ls,k2}^{Di,*} Z_{Ls,l2}^{Di,*} - 2g_{B2}^2 Z_{Ls,i4}^{DR,*} Z_{Ls,j4}^{DR,*} Z_{Ls,k2}^{Di,*} Z_{Ls,l2}^{Di,*} \\
& - 2|Y_A|^2 Z_{Ls,i4}^{DR,*} Z_{Ls,j1}^{DR,*} Z_{Ls,k3}^{Di,*} Z_{Ls,l2}^{Di,*} + |Y_K|^2 Z_{Ls,i4}^{DR,*} Z_{Ls,j1}^{DR,*} Z_{Ls,k3}^{Di,*} Z_{Ls,l2}^{Di,*} \\
& - 2|Y_A|^2 Z_{Ls,i3}^{DR,*} Z_{Ls,j1}^{DR,*} Z_{Ls,k4}^{Di,*} Z_{Ls,l2}^{Di,*} + |Y_K|^2 Z_{Ls,i3}^{DR,*} Z_{Ls,j1}^{DR,*} Z_{Ls,k4}^{Di,*} Z_{Ls,l2}^{Di,*} \\
& - 2|Y_A|^2 Z_{Ls,i4}^{DR,*} Z_{Ls,j2}^{DR,*} Z_{Ls,k1}^{Di,*} Z_{Ls,l3}^{Di,*} + |Y_K|^2 Z_{Ls,i4}^{DR,*} Z_{Ls,j2}^{DR,*} Z_{Ls,k1}^{Di,*} Z_{Ls,l3}^{Di,*} \\
& - 2|Y_A|^2 Z_{Ls,i4}^{DR,*} Z_{Ls,j1}^{DR,*} Z_{Ls,k2}^{Di,*} Z_{Ls,l3}^{Di,*} + |Y_K|^2 Z_{Ls,i4}^{DR,*} Z_{Ls,j1}^{DR,*} Z_{Ls,k2}^{Di,*} Z_{Ls,l3}^{Di,*} \\
& + 2g_{A1}^2 Z_{Ls,i3}^{DR,*} Z_{Ls,j3}^{DR,*} Z_{Ls,k3}^{Di,*} Z_{Ls,l3}^{Di,*} + 2g_{A2}^2 Z_{Ls,i3}^{DR,*} Z_{Ls,j3}^{DR,*} Z_{Ls,k3}^{Di,*} Z_{Ls,l3}^{Di,*} \\
& + 2g_{B1}^2 Z_{Ls,i3}^{DR,*} Z_{Ls,j3}^{DR,*} Z_{Ls,k3}^{Di,*} Z_{Ls,l3}^{Di,*} + 2g_{B2}^2 Z_{Ls,i3}^{DR,*} Z_{Ls,j3}^{DR,*} Z_{Ls,k3}^{Di,*} Z_{Ls,l3}^{Di,*}
\end{aligned}$$

$$\begin{aligned}
& -2g_{A1}^2 Z_{Ls,i4}^{DR,*} Z_{Ls,j4}^{DR,*} Z_{Ls,k3}^{Di,*} Z_{Ls,l3}^{Di,*} - 2g_{A2}^2 Z_{Ls,i4}^{DR,*} Z_{Ls,j4}^{DR,*} Z_{Ls,k3}^{Di,*} Z_{Ls,l3}^{Di,*} \\
& -2g_{B1}^2 Z_{Ls,i4}^{DR,*} Z_{Ls,j4}^{DR,*} Z_{Ls,k3}^{Di,*} Z_{Ls,l3}^{Di,*} - 2g_{B2}^2 Z_{Ls,i4}^{DR,*} Z_{Ls,j4}^{DR,*} Z_{Ls,k3}^{Di,*} Z_{Ls,l3}^{Di,*} \\
& + 4|Y_A|^2 Z_{Ls,i4}^{DR,*} Z_{Ls,j4}^{DR,*} Z_{Ls,k3}^{Di,*} Z_{Ls,l3}^{Di,*} + 2|Y_K|^2 Z_{Ls,i4}^{DR,*} Z_{Ls,j4}^{DR,*} Z_{Ls,k3}^{Di,*} Z_{Ls,l3}^{Di,*} \\
& - 2|Y_A|^2 Z_{Ls,i3}^{DR,*} Z_{Ls,j2}^{DR,*} Z_{Ls,k1}^{Di,*} Z_{Ls,l4}^{Di,*} + |Y_K|^2 Z_{Ls,i3}^{DR,*} Z_{Ls,j2}^{DR,*} Z_{Ls,k1}^{Di,*} Z_{Ls,l4}^{Di,*} \\
& - 2|Y_A|^2 Z_{Ls,i3}^{DR,*} Z_{Ls,j1}^{DR,*} Z_{Ls,k2}^{Di,*} Z_{Ls,l4}^{Di,*} + |Y_K|^2 Z_{Ls,i3}^{DR,*} Z_{Ls,j1}^{DR,*} Z_{Ls,k2}^{Di,*} Z_{Ls,l4}^{Di,*} \\
& - 2g_{A1}^2 Z_{Ls,i3}^{DR,*} Z_{Ls,j3}^{DR,*} Z_{Ls,k4}^{Di,*} Z_{Ls,l4}^{Di,*} - 2g_{A2}^2 Z_{Ls,i3}^{DR,*} Z_{Ls,j3}^{DR,*} Z_{Ls,k4}^{Di,*} Z_{Ls,l4}^{Di,*} \\
& - 2g_{B1}^2 Z_{Ls,i3}^{DR,*} Z_{Ls,j3}^{DR,*} Z_{Ls,k4}^{Di,*} Z_{Ls,l4}^{Di,*} - 2g_{B2}^2 Z_{Ls,i3}^{DR,*} Z_{Ls,j3}^{DR,*} Z_{Ls,k4}^{Di,*} Z_{Ls,l4}^{Di,*} \\
& + 4|Y_A|^2 Z_{Ls,i3}^{DR,*} Z_{Ls,j3}^{DR,*} Z_{Ls,k4}^{Di,*} Z_{Ls,l4}^{Di,*} + 2|Y_K|^2 Z_{Ls,i3}^{DR,*} Z_{Ls,j3}^{DR,*} Z_{Ls,k4}^{Di,*} Z_{Ls,l4}^{Di,*} \\
& + 2g_{A1}^2 Z_{Ls,i4}^{DR,*} Z_{Ls,j4}^{DR,*} Z_{Ls,k4}^{Di,*} Z_{Ls,l4}^{Di,*} + 2g_{A2}^2 Z_{Ls,i4}^{DR,*} Z_{Ls,j4}^{DR,*} Z_{Ls,k4}^{Di,*} Z_{Ls,l4}^{Di,*} \\
& + 2g_{B1}^2 Z_{Ls,i4}^{DR,*} Z_{Ls,j4}^{DR,*} Z_{Ls,k4}^{Di,*} Z_{Ls,l4}^{Di,*} + 2g_{B2}^2 Z_{Ls,i4}^{DR,*} Z_{Ls,j4}^{DR,*} Z_{Ls,k4}^{Di,*} Z_{Ls,l4}^{Di,*} \\
& + Z_{Ls,i2}^{DR,*} \left( - \left( 2|Y_A|^2 - |Y_K|^2 \right) \left( Z_{Ls,j4}^{DR,*} \left( Z_{Ls,k1}^{Di,*} Z_{Ls,l3}^{Di,*} + Z_{Ls,k3}^{Di,*} Z_{Ls,l1}^{Di,*} \right) + Z_{Ls,j3}^{DR,*} \left( Z_{Ls,k1}^{Di,*} Z_{Ls,l4}^{Di,*} + Z_{Ls,k4}^{Di,*} Z_{Ls,l1}^{Di,*} \right) \right. \right. \\
& \left. \left. - Z_{Ls,j1}^{DR,*} \left( Z_{Ls,k3}^{Di,*} Z_{Ls,l4}^{Di,*} + Z_{Ls,k4}^{Di,*} Z_{Ls,l3}^{Di,*} \right) \right) \right. \\
& \left. - 2Z_{Ls,j2}^{DR,*} \left( \left( -2|Y_A|^2 - |Y_K|^2 + g_{A1}^2 + g_{A2}^2 + g_{B1}^2 + g_{B2}^2 \right) Z_{Ls,k1}^{Di,*} Z_{Ls,l1}^{Di,*} - \left( g_{A1}^2 + g_{A2}^2 + g_{B1}^2 + g_{B2}^2 \right) Z_{Ls,k2}^{Di,*} Z_{Ls,l2}^{Di,*} \right. \right. \\
& \left. \left. + \left( -g_{A2}^2 - g_{B2}^2 + g_{A1}^2 + g_{B1}^2 \right) \left( Z_{Ls,k3}^{Di,*} Z_{Ls,l3}^{Di,*} - Z_{Ls,k4}^{Di,*} Z_{Ls,l4}^{Di,*} \right) \right) \right) \\
& + Z_{Ls,i1}^{DR,*} \left( - \left( 2|Y_A|^2 - |Y_K|^2 \right) \left( Z_{Ls,j4}^{DR,*} \left( Z_{Ls,k2}^{Di,*} Z_{Ls,l3}^{Di,*} + Z_{Ls,k3}^{Di,*} Z_{Ls,l2}^{Di,*} \right) + Z_{Ls,j3}^{DR,*} \left( Z_{Ls,k2}^{Di,*} Z_{Ls,l4}^{Di,*} + Z_{Ls,k4}^{Di,*} Z_{Ls,l2}^{Di,*} \right) \right. \right. \\
& \left. \left. - Z_{Ls,j2}^{DR,*} \left( Z_{Ls,k3}^{Di,*} Z_{Ls,l4}^{Di,*} + Z_{Ls,k4}^{Di,*} Z_{Ls,l3}^{Di,*} \right) \right) \right. \\
& \left. + 2Z_{Ls,j1}^{DR,*} \left( \left( g_{A1}^2 + g_{A2}^2 + g_{B1}^2 + g_{B2}^2 \right) Z_{Ls,k1}^{Di,*} Z_{Ls,l1}^{Di,*} - \left( -2|Y_A|^2 - |Y_K|^2 + g_{A1}^2 + g_{A2}^2 + g_{B1}^2 + g_{B2}^2 \right) Z_{Ls,k2}^{Di,*} Z_{Ls,l2}^{Di,*} \right. \right. \\
& \left. \left. + \left( -g_{A2}^2 - g_{B2}^2 + g_{A1}^2 + g_{B1}^2 \right) \left( Z_{Ls,k3}^{Di,*} Z_{Ls,l3}^{Di,*} - Z_{Ls,k4}^{Di,*} Z_{Ls,l4}^{Di,*} \right) \right) \right) \right) \quad (906)
\end{aligned}$$

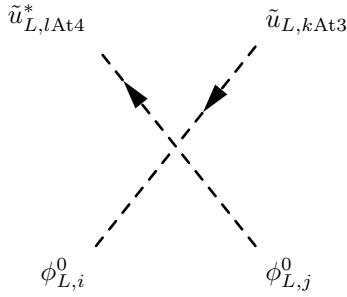

$$\begin{aligned}
& \frac{i}{6} \left( \left( -3g_{A2}^2 + g_{A1}^2 \right) Z_{Ls,i1}^{DR,*} Z_{Ls,j1}^{DR,*} - \left( -3g_{A2}^2 + g_{A1}^2 \right) Z_{Ls,i2}^{DR,*} Z_{Ls,j2}^{DR,*} \right. \\
& \left. + \left( 3g_{A2}^2 + g_{A1}^2 \right) \left( Z_{Ls,i3}^{DR,*} Z_{Ls,j3}^{DR,*} - Z_{Ls,i4}^{DR,*} Z_{Ls,j4}^{DR,*} \right) \right) \delta_{At3At4} \delta_{kl} \quad (907)
\end{aligned}$$

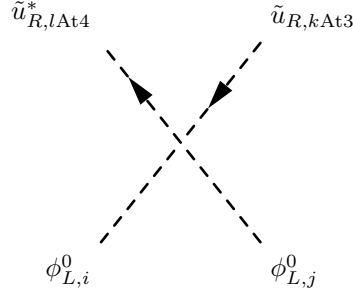

$$-\frac{2i}{3}g_{A1}^2\left(Z_{Ls,i1}^{DR,*}Z_{Ls,j1}^{DR,*}-Z_{Ls,i2}^{DR,*}Z_{Ls,j2}^{DR,*}+Z_{Ls,i3}^{DR,*}Z_{Ls,j3}^{DR,*}-Z_{Ls,i4}^{DR,*}Z_{Ls,j4}^{DR,*}\right)\delta_{At3At4}\delta_{kl} \quad (908)$$


---

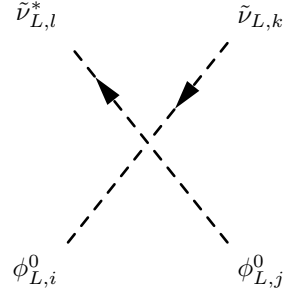

$$-\frac{i}{2}\left((g_{A1}^2+g_{A2}^2)Z_{Ls,i1}^{DR,*}Z_{Ls,j1}^{DR,*}-\left(g_{A1}^2+g_{A2}^2\right)Z_{Ls,i2}^{DR,*}Z_{Ls,j2}^{DR,*}\right. \\ \left.+(-g_{A2}^2+g_{A1}^2)\left(Z_{Ls,i3}^{DR,*}Z_{Ls,j3}^{DR,*}-Z_{Ls,i4}^{DR,*}Z_{Ls,j4}^{DR,*}\right)\right)\delta_{kl} \quad (909)$$


---

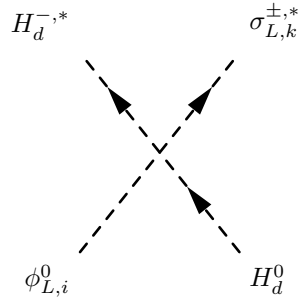

$$-\frac{i}{2}g_{A2}^2\left(Z_{Ls,i1}^{DR,*}Z_{Ls,k4}^{od}-Z_{Ls,i2}^{DR,*}Z_{Ls,k2}^{od}+Z_{Ls,i3}^{DR,*}Z_{Ls,k1}^{od}-Z_{Ls,i4}^{DR,*}Z_{Ls,k3}^{od}\right) \quad (910)$$


---



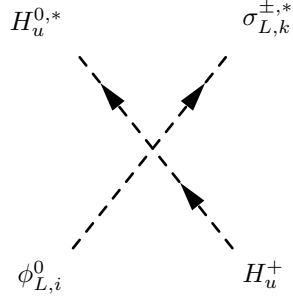

$$-\frac{i}{2}g_{A2}^2\left(Z_{Ls,i1}^{DR,*}Z_{Ls,k4}^{od}-Z_{Ls,i2}^{DR,*}Z_{Ls,k2}^{od}+Z_{Ls,i3}^{DR,*}Z_{Ls,k1}^{od}-Z_{Ls,i4}^{DR,*}Z_{Ls,k3}^{od}\right) \quad (911)$$


---

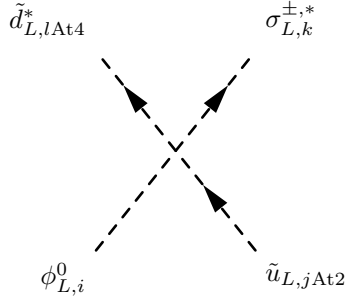

$$-\frac{i}{2}g_{A2}^2\delta_{At2At4}\delta_{jl}\left(Z_{Ls,i1}^{DR,*}Z_{Ls,k4}^{od}-Z_{Ls,i2}^{DR,*}Z_{Ls,k2}^{od}+Z_{Ls,i3}^{DR,*}Z_{Ls,k1}^{od}-Z_{Ls,i4}^{DR,*}Z_{Ls,k3}^{od}\right) \quad (912)$$


---

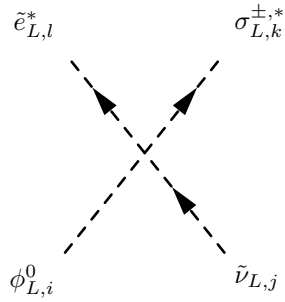

$$-\frac{i}{2}g_{A2}^2\delta_{jl}\left(Z_{Ls,i1}^{DR,*}Z_{Ls,k4}^{od}-Z_{Ls,i2}^{DR,*}Z_{Ls,k2}^{od}+Z_{Ls,i3}^{DR,*}Z_{Ls,k1}^{od}-Z_{Ls,i4}^{DR,*}Z_{Ls,k3}^{od}\right) \quad (913)$$


---

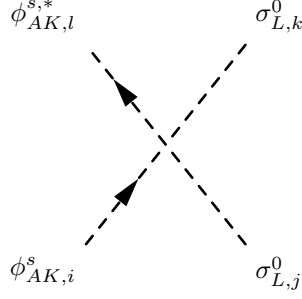

$$\begin{aligned}
& -\frac{i}{2} \left( Y_K^* \left( \sqrt{2} Y_A Z_{AK,i2}^{s,*} \left( Z_{Ls,j1}^{Di,*} Z_{Ls,k1}^{Di,*} + Z_{Ls,j2}^{Di,*} Z_{Ls,k2}^{Di,*} - Z_{Ls,j3}^{Di,*} Z_{Ls,k3}^{Di,*} - Z_{Ls,j4}^{Di,*} Z_{Ls,k4}^{Di,*} \right) \right. \right. \\
& + Y_K Z_{AK,i1}^{s,*} \left( Z_{Ls,j1}^{Di,*} Z_{Ls,k1}^{Di,*} + Z_{Ls,j2}^{Di,*} Z_{Ls,k2}^{Di,*} + Z_{Ls,j3}^{Di,*} Z_{Ls,k3}^{Di,*} + Z_{Ls,j4}^{Di,*} Z_{Ls,k4}^{Di,*} \right) \left. \right) Z_{AK,l1}^s \\
& + Y_A^* \left( \sqrt{2} Y_K Z_{AK,i1}^{s,*} \left( Z_{Ls,j1}^{Di,*} Z_{Ls,k1}^{Di,*} + Z_{Ls,j2}^{Di,*} Z_{Ls,k2}^{Di,*} - Z_{Ls,j3}^{Di,*} Z_{Ls,k3}^{Di,*} - Z_{Ls,j4}^{Di,*} Z_{Ls,k4}^{Di,*} \right) \right. \\
& \left. \left. + 2 Y_A Z_{AK,i2}^{s,*} \left( Z_{Ls,j1}^{Di,*} Z_{Ls,k1}^{Di,*} + Z_{Ls,j2}^{Di,*} Z_{Ls,k2}^{Di,*} + Z_{Ls,j3}^{Di,*} Z_{Ls,k3}^{Di,*} + Z_{Ls,j4}^{Di,*} Z_{Ls,k4}^{Di,*} \right) \right) Z_{AK,l2}^s \right) \quad (914)
\end{aligned}$$


---

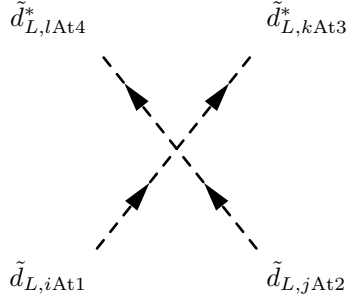

$$\begin{aligned}
& \frac{i}{36} \left( \delta_{At1At4} \delta_{At2At3} \left( -18 g_3^2 \delta_{ik} \delta_{jl} + \left( 6 g_3^2 - 9 g_{A2}^2 - g_{A1}^2 \right) \delta_{il} \delta_{jk} \right) \right. \\
& \left. - \delta_{At1At3} \delta_{At2At4} \left( 18 g_3^2 \delta_{il} \delta_{jk} + \left( -6 g_3^2 + 9 g_{A2}^2 + g_{A1}^2 \right) \delta_{ik} \delta_{jl} \right) \right) \quad (915)
\end{aligned}$$


---

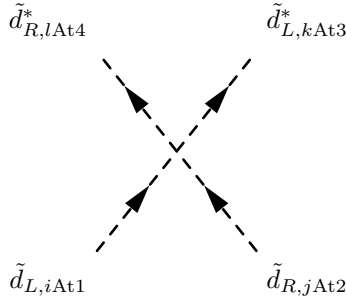

$$\frac{i}{18} \left( - \left( 3g_3^2 + g_{A1}^2 \right) \delta_{\text{At1At3}} \delta_{\text{At2At4}} \delta_{ik} \delta_{jl} + 9 \delta_{\text{At1At4}} \delta_{\text{At2At3}} \left( - 2Y_{d,jk}^* Y_{d,li} + g_3^2 \delta_{ik} \delta_{jl} \right) \right) \quad (916)$$


---

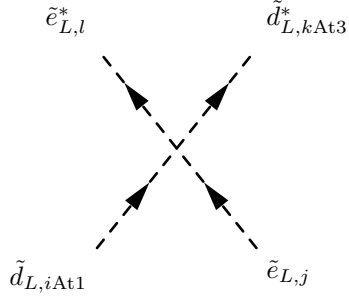

$$\frac{i}{12} \left( - 3g_{A2}^2 + g_{A1}^2 \right) \delta_{\text{At1At3}} \delta_{ik} \delta_{jl} \quad (917)$$


---

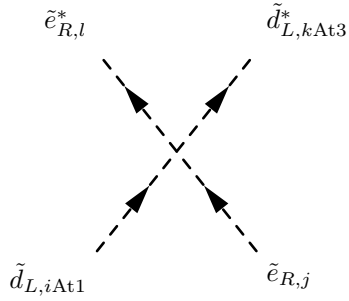

$$- \frac{i}{6} g_{A1}^2 \delta_{\text{At1At3}} \delta_{ik} \delta_{jl} \quad (918)$$


---

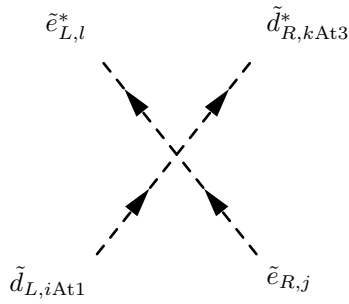

$$- i Y_{e,jl}^* \delta_{\text{At1At3}} V_{d,ki} \quad (919)$$


---

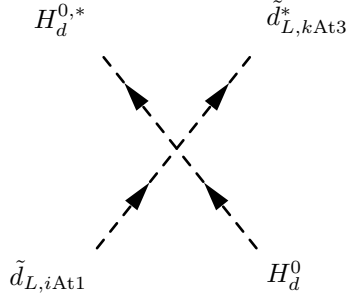

$$\frac{i}{12}\delta_{\text{At}1\text{At}3}\left(-12\sum_{a=1}^3Y_{d,ak}^*Y_{d,ai}+\left(3g_{A2}^2+g_{A1}^2\right)\delta_{ik}\right) \quad (920)$$


---

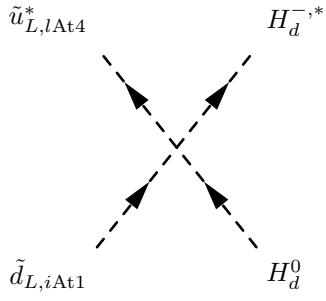

$$-\frac{i}{2}\delta_{\text{At}1\text{At}4}\left(-2\sum_{a=1}^3Y_{d,al}^*Y_{d,ai}+g_{A2}^2\delta_{il}\right) \quad (921)$$


---

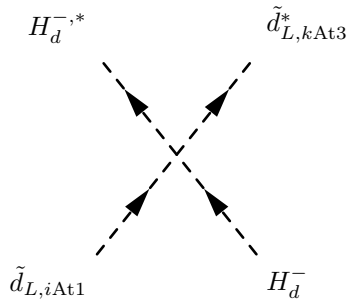

$$\frac{i}{12}\left(-3g_{A2}^2+g_{A1}^2\right)\delta_{\text{At}1\text{At}3}\delta_{ik} \quad (922)$$


---

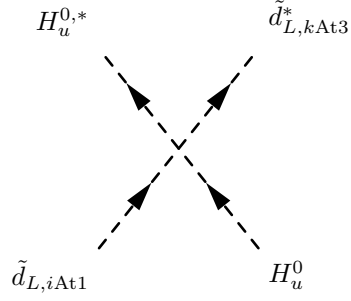

$$- \frac{i}{12} (3g_{A2}^2 + g_{A1}^2) \delta_{\text{At}1\text{At}3} \delta_{ik} \quad (923)$$


---

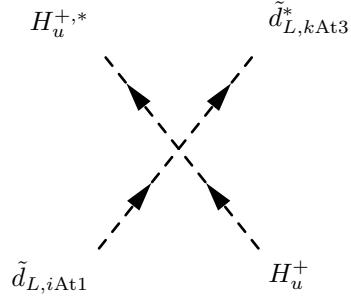

$$- \frac{i}{12} \delta_{\text{At}1\text{At}3} \left( 12 \sum_{a=1}^3 Y_{u,ak}^* Y_{u,ai} + \left( -3g_{A2}^2 + g_{A1}^2 \right) \delta_{ik} \right) \quad (924)$$


---

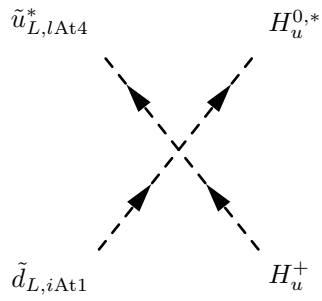

$$- \frac{i}{2} \delta_{\text{At}1\text{At}4} \left( -2 \sum_{a=1}^3 Y_{u,al}^* Y_{u,ai} + g_{A2}^2 \delta_{il} \right) \quad (925)$$


---

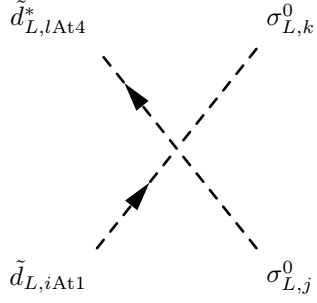

$$\begin{aligned} & \frac{i}{6} \left( (3g_{A2}^2 + g_{A1}^2) Z_{Ls,j1}^{Di,*} Z_{Ls,k1}^{Di,*} - (3g_{A2}^2 + g_{A1}^2) Z_{Ls,j2}^{Di,*} Z_{Ls,k2}^{Di,*} \right. \\ & \left. + (-3g_{A2}^2 + g_{A1}^2) (Z_{Ls,j3}^{Di,*} Z_{Ls,k3}^{Di,*} - Z_{Ls,j4}^{Di,*} Z_{Ls,k4}^{Di,*}) \right) \delta_{At1At4} \delta_{il} \end{aligned} \quad (926)$$


---

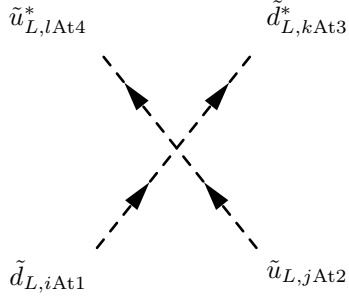

$$\frac{i}{36} \left( -18 \delta_{At1At4} \delta_{At2At3} (g_3^2 \delta_{ik} \delta_{jl} + g_{A2}^2 \delta_{il} \delta_{jk}) + (6g_3^2 + 9g_{A2}^2 - g_{A1}^2) \delta_{At1At3} \delta_{At2At4} \delta_{ik} \delta_{jl} \right) \quad (927)$$


---

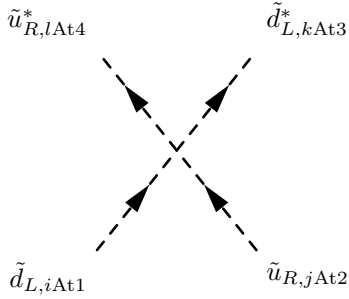

$$\frac{i}{18} \left( (2g_{A1}^2 - 3g_3^2) \delta_{At1At3} \delta_{At2At4} \delta_{ik} \delta_{jl} + 9 \delta_{At1At4} \delta_{At2At3} (-2Y_{u,jk}^* Y_{u,li} + g_3^2 \delta_{ik} \delta_{jl}) \right) \quad (928)$$


---

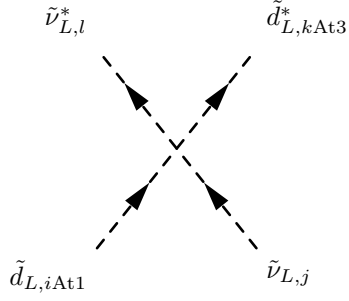

$$\frac{i}{12} \left( 3g_{A2}^2 + g_{A1}^2 \right) \delta_{\text{At}1\text{At}3} \delta_{ik} \delta_{jl} \quad (929)$$


---

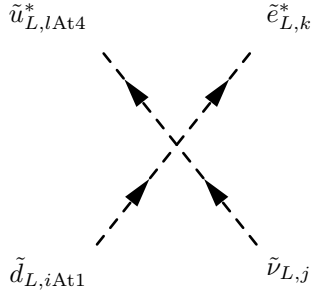

$$- \frac{i}{2} g_{A2}^2 \delta_{\text{At}1\text{At}4} \delta_{il} \delta_{jk} \quad (930)$$


---

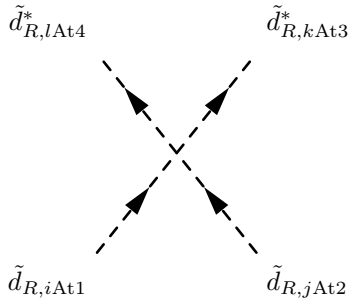

$$\begin{aligned} & \frac{i}{18} \left( \delta_{\text{At}1\text{At}4} \delta_{\text{At}2\text{At}3} \left( \left( -2g_{A1}^2 + 3g_3^2 \right) \delta_{il} \delta_{jk} - 9g_3^2 \delta_{ik} \delta_{jl} \right) \right. \\ & \left. + \delta_{\text{At}1\text{At}3} \delta_{\text{At}2\text{At}4} \left( \left( -2g_{A1}^2 + 3g_3^2 \right) \delta_{ik} \delta_{jl} - 9g_3^2 \delta_{il} \delta_{jk} \right) \right) \quad (931) \end{aligned}$$


---

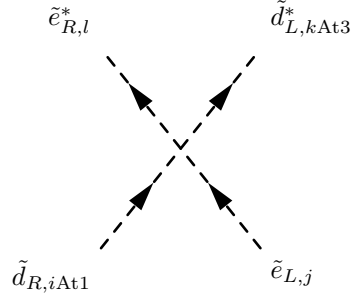

$$-iY_{d,ik}^*\delta_{\text{At}1\text{At}3}Y_{e,lj} \quad (932)$$


---

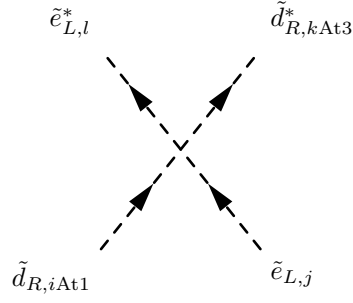

$$\frac{i}{6}g_{A1}^2\delta_{\text{At}1\text{At}3}\delta_{ik}\delta_{jl} \quad (933)$$


---

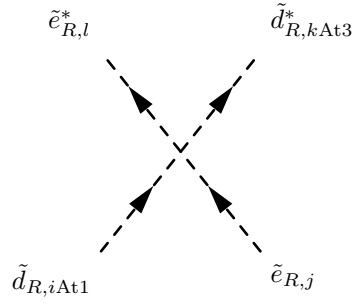

$$-\frac{i}{3}g_{A1}^2\delta_{\text{At}1\text{At}3}\delta_{ik}\delta_{jl} \quad (934)$$


---



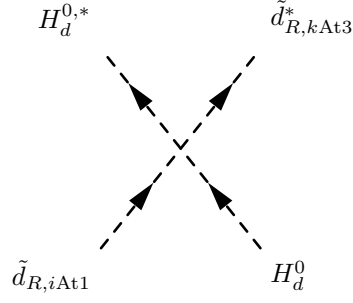

$$\frac{i}{6}\delta_{\text{At}1\text{At}3}\left(-6\sum_{a=1}^3Y_{d,ia}^*Y_{d,ka}+g_{A1}^2\delta_{ik}\right) \quad (935)$$


---

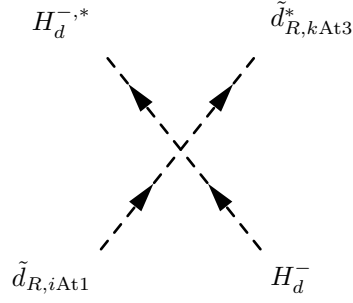

$$\frac{i}{6}\delta_{\text{At}1\text{At}3}\left(-6\sum_{a=1}^3Y_{d,ia}^*Y_{d,ka}+g_{A1}^2\delta_{ik}\right) \quad (936)$$


---

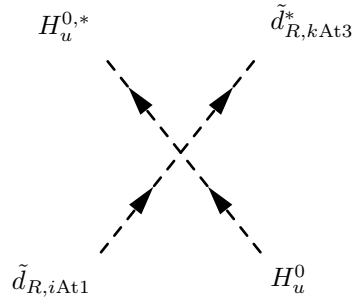

$$-\frac{i}{6}g_{A1}^2\delta_{\text{At}1\text{At}3}\delta_{ik} \quad (937)$$


---

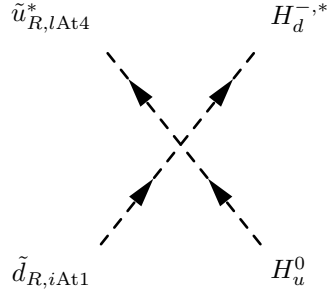

$$i\delta_{At1At4} \sum_{a=1}^3 Y_{d,ia}^* Y_{u,la} \quad (938)$$


---

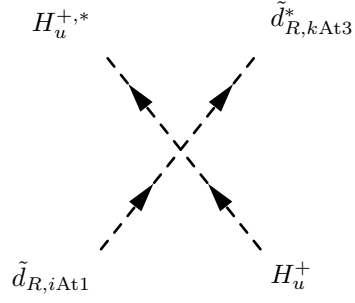

$$-\frac{i}{6} g_{A1}^2 \delta_{At1At3} \delta_{ik} \quad (939)$$


---

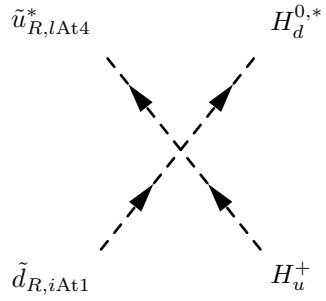

$$i\delta_{At1At4} \sum_{a=1}^3 Y_{d,ia}^* Y_{u,la} \quad (940)$$


---

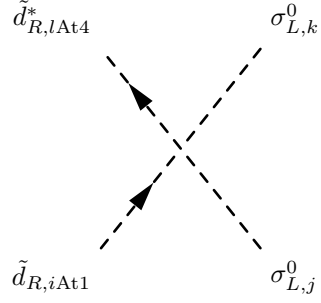

$$\frac{i}{3}g_{A1}^2 \left( Z_{Ls,j1}^{Di,*} Z_{Ls,k1}^{Di,*} - Z_{Ls,j2}^{Di,*} Z_{Ls,k2}^{Di,*} + Z_{Ls,j3}^{Di,*} Z_{Ls,k3}^{Di,*} - Z_{Ls,j4}^{Di,*} Z_{Ls,k4}^{Di,*} \right) \delta_{At1At4} \delta_{il} \quad (941)$$


---

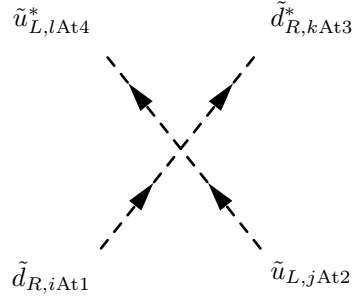

$$\frac{i}{18} \left( - \left( 3g_3^2 + g_{A1}^2 \right) \delta_{At1At3} \delta_{At2At4} \delta_{ik} \delta_{jl} + 9 \delta_{At1At4} \delta_{At2At3} \left( - 2Y_{d,il}^* Y_{d,kj} + g_3^2 \delta_{ik} \delta_{jl} \right) \right) \quad (942)$$


---

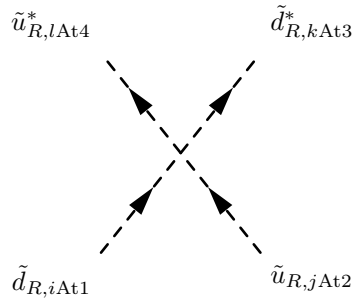

$$\frac{i}{18} \left( \left( 3g_3^2 + 4g_{A1}^2 \right) \delta_{At1At3} \delta_{At2At4} - 9g_3^2 \delta_{At1At4} \delta_{At2At3} \right) \delta_{ik} \delta_{jl} \quad (943)$$


---

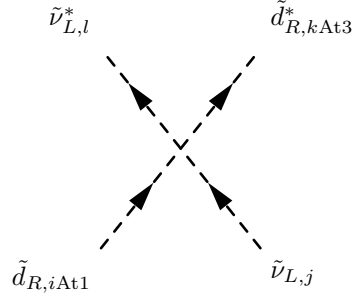

$$\frac{i}{6} g_{A1}^2 \delta_{\text{At}1\text{At}3} \delta_{ik} \delta_{jl} \quad (944)$$


---

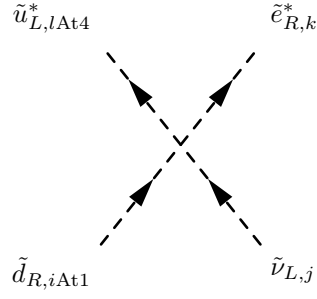

$$-i Y_{d,il}^* \delta_{\text{At}1\text{At}4} Y_{e,kj} \quad (945)$$


---

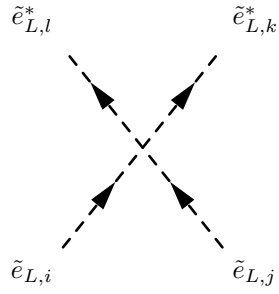

$$-\frac{i}{4} (g_{A1}^2 + g_{A2}^2) (\delta_{ik} \delta_{jl} + \delta_{il} \delta_{jk}) \quad (946)$$


---

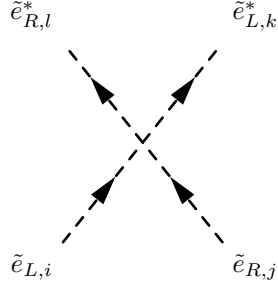

$$\frac{i}{2} \left( -2Y_{e,jk}^* Y_{e,li} + g_{A1}^2 \delta_{ik} \delta_{jl} \right) \quad (947)$$


---

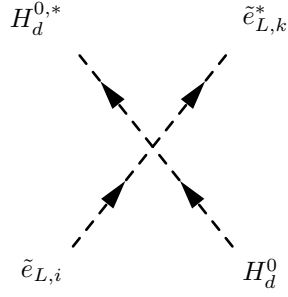

$$-\frac{i}{4} \left( 4 \sum_{a=1}^3 Y_{e,ak}^* Y_{e,ai} + \left( -g_{A2}^2 + g_{A1}^2 \right) \delta_{ik} \right) \quad (948)$$


---

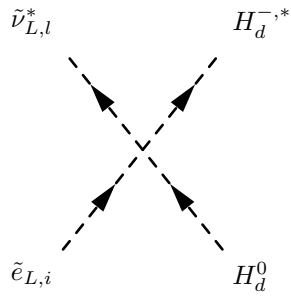

$$-\frac{i}{2} \left( -2 \sum_{a=1}^3 Y_{e,al}^* Y_{e,ai} + g_{A2}^2 \delta_{il} \right) \quad (949)$$


---

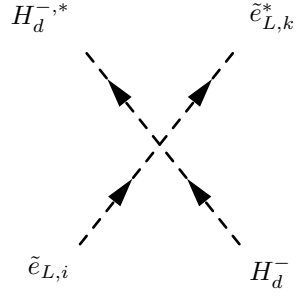

$$-\frac{i}{4}\left(g_{A1}^2+g_{A2}^2\right)\delta_{ik} \quad (950)$$


---

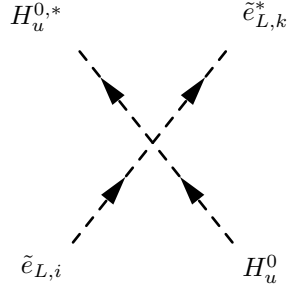

$$\frac{i}{4}\left(-g_{A2}^2+g_{A1}^2\right)\delta_{ik} \quad (951)$$


---

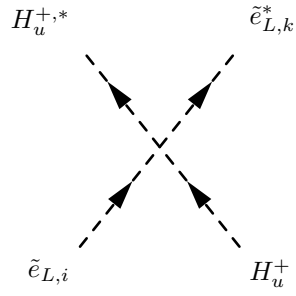

$$\frac{i}{4}\left(g_{A1}^2+g_{A2}^2\right)\delta_{ik} \quad (952)$$


---

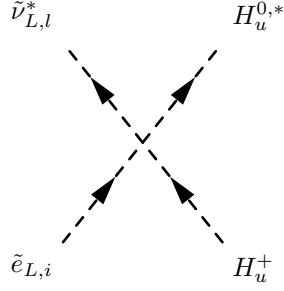

$$-\frac{i}{2}g_{A2}^2\delta_{il} \quad (953)$$


---

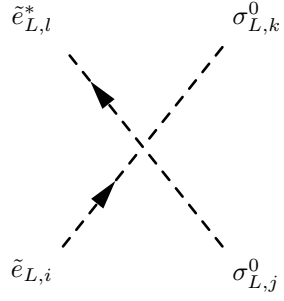

$$\begin{aligned} & -\frac{i}{2}\left(\left(-g_{A2}^2+g_{A1}^2\right)Z_{Ls,j1}^{Di,*}Z_{Ls,k1}^{Di,*}+\left(-g_{A1}^2+g_{A2}^2\right)Z_{Ls,j2}^{Di,*}Z_{Ls,k2}^{Di,*}\right. \\ & \left.+ \left(g_{A1}^2+g_{A2}^2\right)\left(Z_{Ls,j3}^{Di,*}Z_{Ls,k3}^{Di,*}-Z_{Ls,j4}^{Di,*}Z_{Ls,k4}^{Di,*}\right)\right)\delta_{il} \end{aligned} \quad (954)$$


---

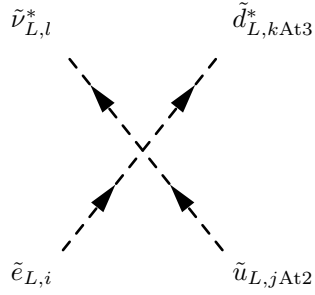

$$-\frac{i}{2}g_{A2}^2\delta_{At2At3}\delta_{il}\delta_{jk} \quad (955)$$


---

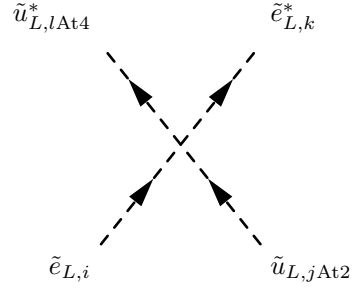

$$\frac{i}{12} \left( 3g_{A2}^2 + g_{A1}^2 \right) \delta_{At2At4} \delta_{ik} \delta_{jl} \quad (956)$$


---

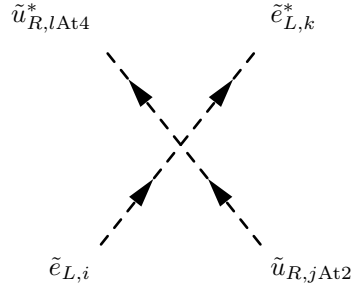

$$-\frac{i}{3} g_{A1}^2 \delta_{At2At4} \delta_{ik} \delta_{jl} \quad (957)$$


---

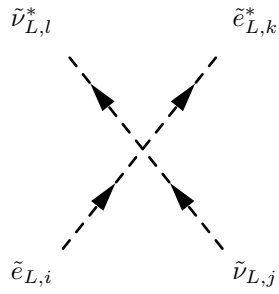

$$-\frac{i}{4} \left( 2g_{A2}^2 \delta_{il} \delta_{jk} + \left( -g_{A2}^2 + g_{A1}^2 \right) \delta_{ik} \delta_{jl} \right) \quad (958)$$


---



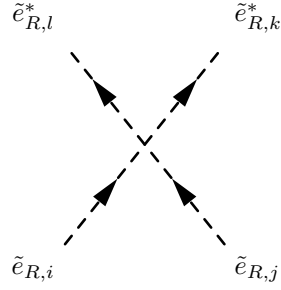

$$-ig_{A1}^2\left(\delta_{ik}\delta_{jl}+\delta_{il}\delta_{jk}\right) \quad (959)$$


---

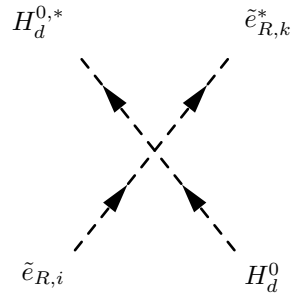

$$\frac{i}{2}\left(-2\sum_{a=1}^3Y_{e,ia}^*Y_{e,ka}+g_{A1}^2\delta_{ik}\right) \quad (960)$$


---

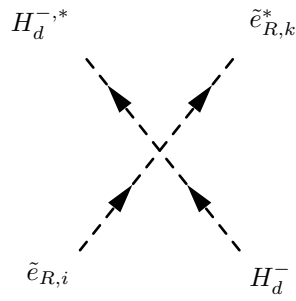

$$\frac{i}{2}\left(-2\sum_{a=1}^3Y_{e,ia}^*Y_{e,ka}+g_{A1}^2\delta_{ik}\right) \quad (961)$$


---

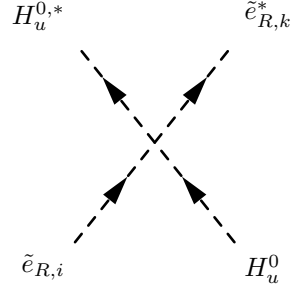

$$-\frac{i}{2}g_{A1}^2\delta_{ik} \quad (962)$$


---

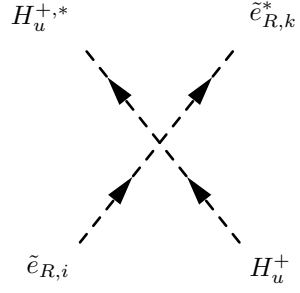

$$-\frac{i}{2}g_{A1}^2\delta_{ik} \quad (963)$$


---

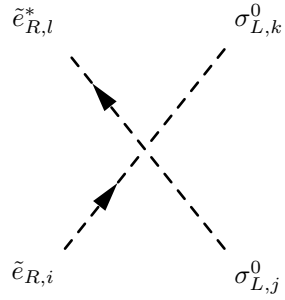

$$ig_{A1}^2 \left( Z_{Ls,j1}^{Di,*} Z_{Ls,k1}^{Di,*} - Z_{Ls,j2}^{Di,*} Z_{Ls,k2}^{Di,*} + Z_{Ls,j3}^{Di,*} Z_{Ls,k3}^{Di,*} - Z_{Ls,j4}^{Di,*} Z_{Ls,k4}^{Di,*} \right) \delta_{il} \quad (964)$$


---

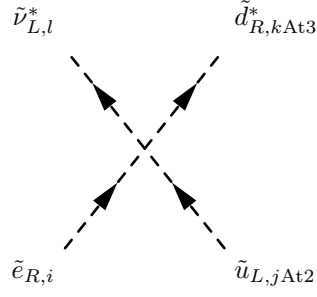

$$-iY_{e,il}^*\delta_{\text{At}2\text{At}3}Y_{d,kj} \quad (965)$$


---

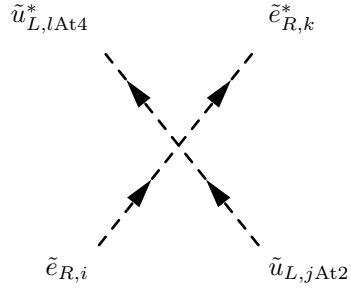

$$-\frac{i}{6}g_{A1}^2\delta_{\text{At}2\text{At}4}\delta_{ik}\delta_{jl} \quad (966)$$


---

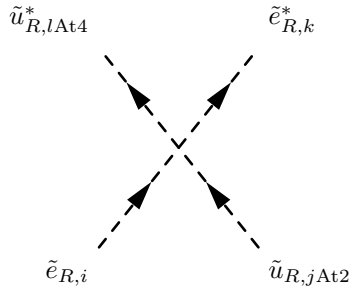

$$\frac{2i}{3}g_{A1}^2\delta_{\text{At}2\text{At}4}\delta_{ik}\delta_{jl} \quad (967)$$


---

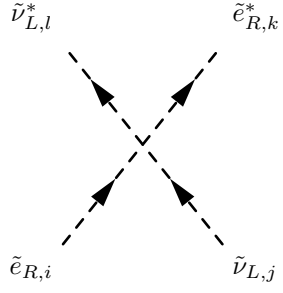

$$\frac{i}{2} \left( -2Y_{e,il}^* Y_{e,kj} + g_{A1}^2 \delta_{ik} \delta_{jl} \right) \quad (968)$$


---

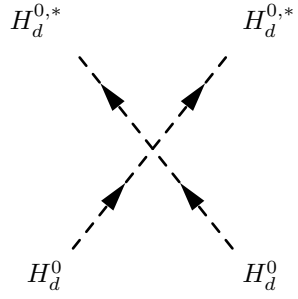

$$-\frac{i}{2} \left( g_{A1}^2 + g_{A2}^2 \right) \quad (969)$$


---

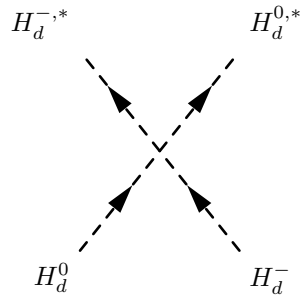

$$-\frac{i}{4} \left( g_{A1}^2 + g_{A2}^2 \right) \quad (970)$$


---

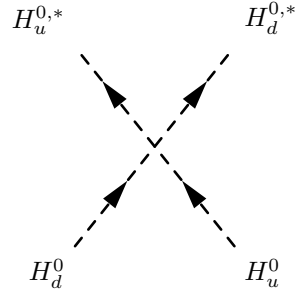

$$\frac{i}{4} \left( g_{A1}^2 + g_{A2}^2 \right) \quad (971)$$


---

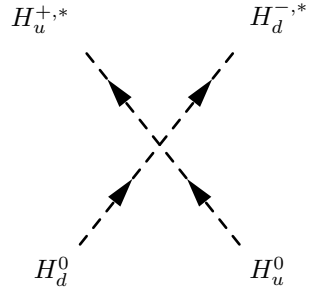

$$-\frac{i}{2} g_{A2}^2 \quad (972)$$


---

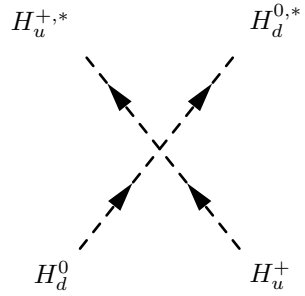

$$\frac{i}{4} \left( -g_{A2}^2 + g_{A1}^2 \right) \quad (973)$$


---

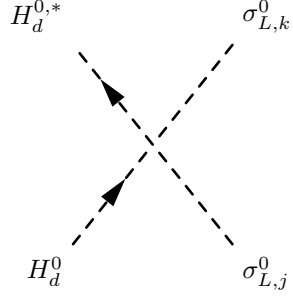

$$\begin{aligned}
& -\frac{i}{2} \left( (g_{A1}^2 + g_{A2}^2) Z_{Ls,j1}^{Di,*} Z_{Ls,k1}^{Di,*} - (g_{A1}^2 + g_{A2}^2) Z_{Ls,j2}^{Di,*} Z_{Ls,k2}^{Di,*} \right. \\
& \left. + (-g_{A2}^2 + g_{A1}^2) (Z_{Ls,j3}^{Di,*} Z_{Ls,k3}^{Di,*} - Z_{Ls,j4}^{Di,*} Z_{Ls,k4}^{Di,*}) \right)
\end{aligned} \tag{974}$$


---

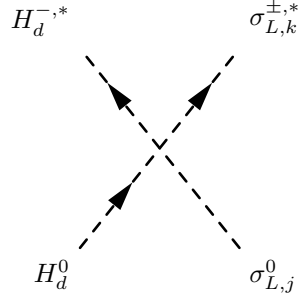

$$\frac{1}{2} g_{A2}^2 \left( -Z_{Ls,j1}^{Di,*} Z_{Ls,k4}^{od} - Z_{Ls,j2}^{Di,*} Z_{Ls,k2}^{od} + Z_{Ls,j3}^{Di,*} Z_{Ls,k1}^{od} + Z_{Ls,j4}^{Di,*} Z_{Ls,k3}^{od} \right) \tag{975}$$


---

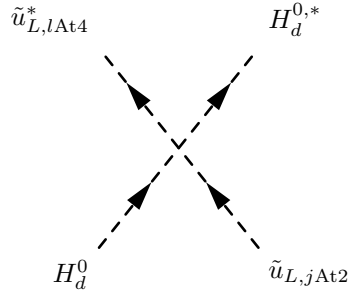

$$\frac{i}{12} \left( -3g_{A2}^2 + g_{A1}^2 \right) \delta_{At2At4} \delta_{jl} \tag{976}$$


---

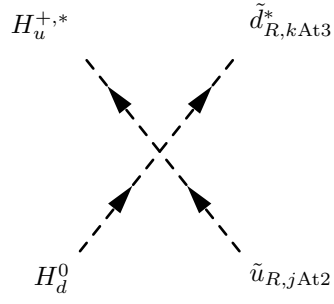

$$i\delta_{\text{At}2\text{At}3} \sum_{a=1}^3 Y_{u,ja}^* Y_{d,ka} \quad (977)$$


---

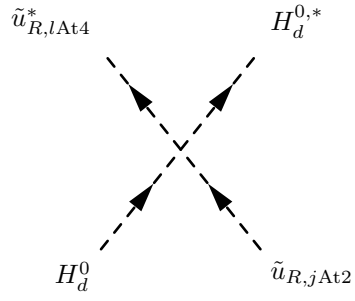

$$-\frac{i}{3} g_{A1}^2 \delta_{\text{At}2\text{At}4} \delta_{jl} \quad (978)$$


---

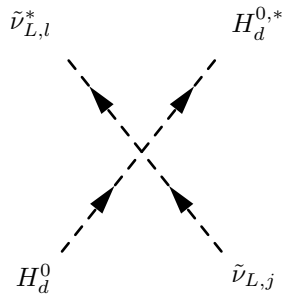

$$-\frac{i}{4} (g_{A1}^2 + g_{A2}^2) \delta_{jl} \quad (979)$$


---

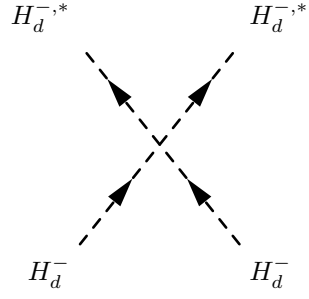

$$-\frac{i}{2}(g_{A1}^2 + g_{A2}^2) \quad (980)$$


---

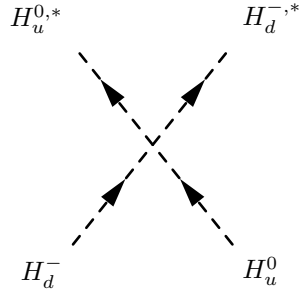

$$\frac{i}{4}(-g_{A2}^2 + g_{A1}^2) \quad (981)$$


---

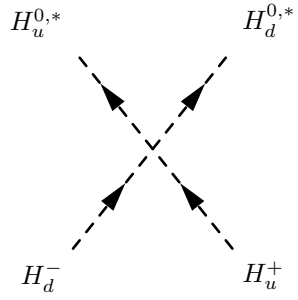

$$-\frac{i}{2}g_{A2}^2 \quad (982)$$


---



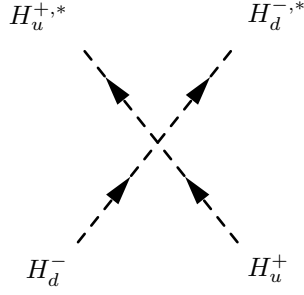

$$\frac{i}{4} \left( g_{A1}^2 + g_{A2}^2 \right) \quad (983)$$


---

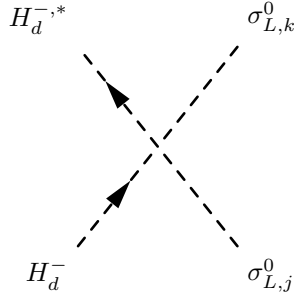

$$\begin{aligned} & -\frac{i}{2} \left( \left( -g_{A2}^2 + g_{A1}^2 \right) Z_{Ls,j1}^{Di,*} Z_{Ls,k1}^{Di,*} + \left( -g_{A1}^2 + g_{A2}^2 \right) Z_{Ls,j2}^{Di,*} Z_{Ls,k2}^{Di,*} \right. \\ & \left. + \left( g_{A1}^2 + g_{A2}^2 \right) \left( Z_{Ls,j3}^{Di,*} Z_{Ls,k3}^{Di,*} - Z_{Ls,j4}^{Di,*} Z_{Ls,k4}^{Di,*} \right) \right) \end{aligned} \quad (984)$$


---

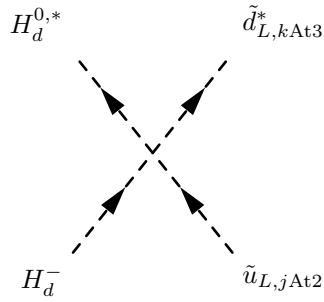

$$-\frac{i}{2} \delta_{\text{At}2\text{At}3} \left( -2 \sum_{a=1}^3 Y_{d,ak}^* Y_{d,aj} + g_{A2}^2 \delta_{jk} \right) \quad (985)$$


---

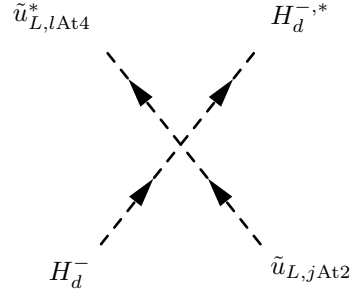

$$\frac{i}{12}\delta_{\text{At}2\text{At}4}\left(-12\sum_{a=1}^3Y_{d,al}^*Y_{d,aj}+\left(3g_{A2}^2+g_{A1}^2\right)\delta_{jl}\right) \quad (986)$$


---

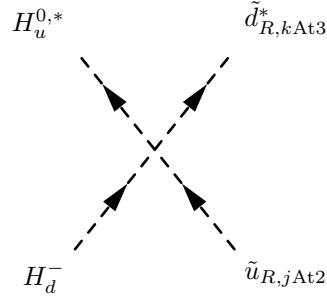

$$i\delta_{\text{At}2\text{At}3}\sum_{a=1}^3Y_{u,ja}^*Y_{d,ka} \quad (987)$$


---

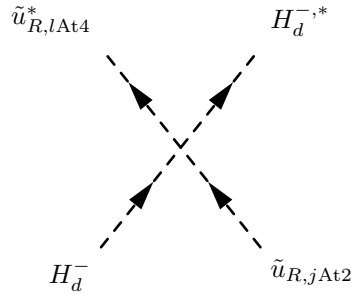

$$-\frac{i}{3}g_{A1}^2\delta_{\text{At}2\text{At}4}\delta_{jl} \quad (988)$$


---

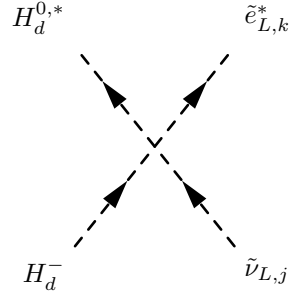

$$-\frac{i}{2}\left(-2\sum_{a=1}^3Y_{e,ak}^*Y_{e,aj}+g_{A2}^2\delta_{jk}\right) \quad (989)$$


---

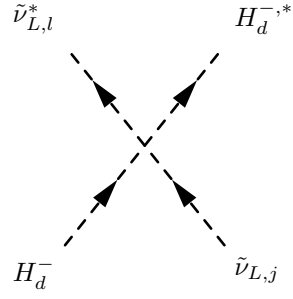

$$-\frac{i}{4}\left(4\sum_{a=1}^3Y_{e,al}^*Y_{e,aj}+\left(-g_{A2}^2+g_{A1}^2\right)\delta_{jl}\right) \quad (990)$$


---

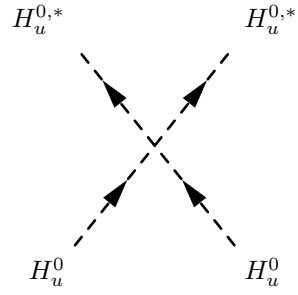

$$-\frac{i}{2}\left(g_{A1}^2+g_{A2}^2\right) \quad (991)$$


---

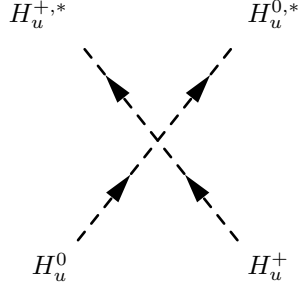

$$-\frac{i}{4}(g_{A1}^2 + g_{A2}^2) \quad (992)$$


---

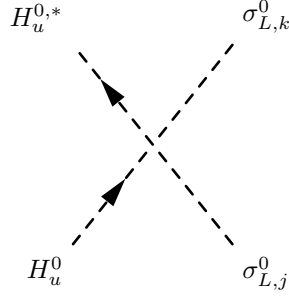

$$\begin{aligned} & \frac{i}{2} \left( (g_{A1}^2 + g_{A2}^2) Z_{Ls,j1}^{Di,*} Z_{Ls,k1}^{Di,*} - (g_{A1}^2 + g_{A2}^2) Z_{Ls,j2}^{Di,*} Z_{Ls,k2}^{Di,*} \right. \\ & \left. + (-g_{A2}^2 + g_{A1}^2) (Z_{Ls,j3}^{Di,*} Z_{Ls,k3}^{Di,*} - Z_{Ls,j4}^{Di,*} Z_{Ls,k4}^{Di,*}) \right) \end{aligned} \quad (993)$$


---

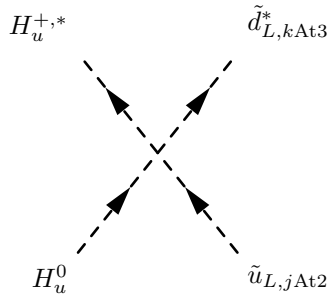

$$-\frac{i}{2} \delta_{\text{At}2\text{At}3} \left( -2 \sum_{a=1}^3 Y_{u,ak}^* Y_{u,aj} + g_{A2}^2 \delta_{jk} \right) \quad (994)$$


---

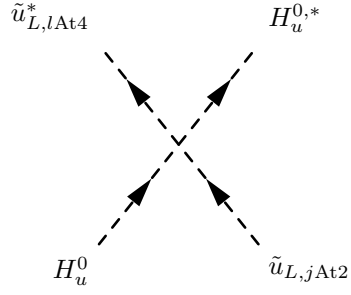

$$-\frac{i}{12}\delta_{\text{At}2\text{At}4}\left(12\sum_{a=1}^3Y_{u,al}^*Y_{u,aj}+\left(-3g_{A2}^2+g_{A1}^2\right)\delta_{jl}\right) \quad (995)$$


---

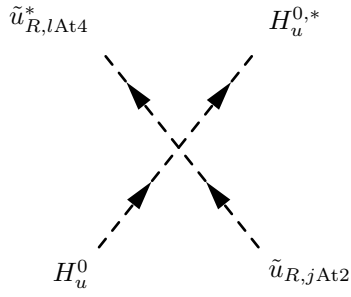

$$\frac{i}{3}\delta_{\text{At}2\text{At}4}\left(-3\sum_{a=1}^3Y_{u,ja}^*Y_{u,la}+g_{A1}^2\delta_{jl}\right) \quad (996)$$


---

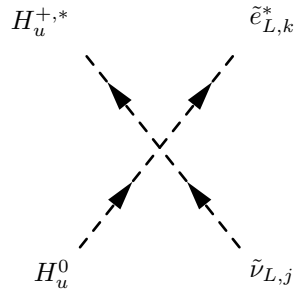

$$-\frac{i}{2}g_{A2}^2\delta_{jk} \quad (997)$$


---

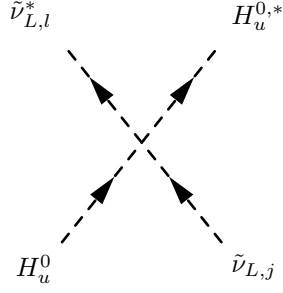

$$\frac{i}{4} \left( g_{A1}^2 + g_{A2}^2 \right) \delta_{jl} \quad (998)$$


---

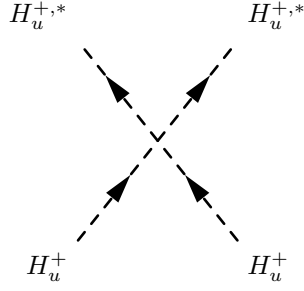

$$-\frac{i}{2} \left( g_{A1}^2 + g_{A2}^2 \right) \quad (999)$$


---

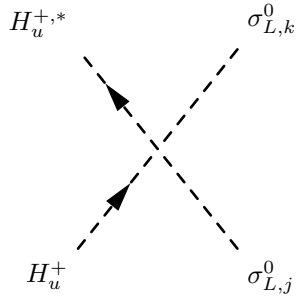

$$\begin{aligned} & \frac{i}{2} \left( \left( -g_{A2}^2 + g_{A1}^2 \right) Z_{Ls,j1}^{Di,*} Z_{Ls,k1}^{Di,*} + \left( -g_{A1}^2 + g_{A2}^2 \right) Z_{Ls,j2}^{Di,*} Z_{Ls,k2}^{Di,*} \right. \\ & \left. + \left( g_{A1}^2 + g_{A2}^2 \right) \left( Z_{Ls,j3}^{Di,*} Z_{Ls,k3}^{Di,*} - Z_{Ls,j4}^{Di,*} Z_{Ls,k4}^{Di,*} \right) \right) \quad (1000) \end{aligned}$$


---

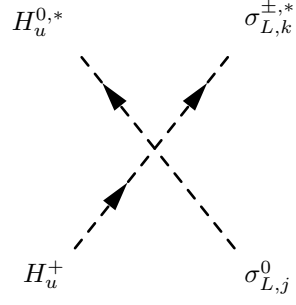

$$\frac{1}{2}g_{A2}^2 \left( -Z_{Ls,j1}^{Di,*} Z_{Ls,k4}^{od} - Z_{Ls,j2}^{Di,*} Z_{Ls,k2}^{od} + Z_{Ls,j3}^{Di,*} Z_{Ls,k1}^{od} + Z_{Ls,j4}^{Di,*} Z_{Ls,k3}^{od} \right) \quad (1001)$$


---

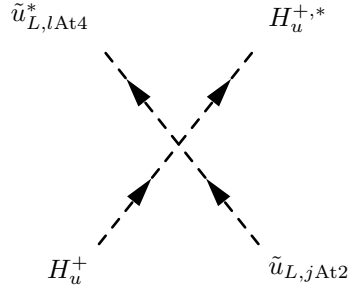

$$- \frac{i}{12} (3g_{A2}^2 + g_{A1}^2) \delta_{At2At4} \delta_{jl} \quad (1002)$$


---

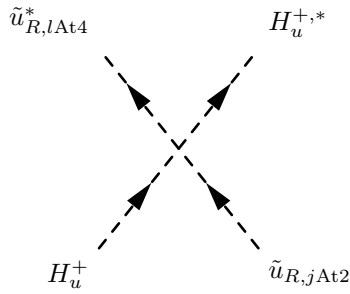

$$\frac{i}{3} \delta_{At2At4} \left( -3 \sum_{a=1}^3 Y_{u,ja}^* Y_{u,la} + g_{A1}^2 \delta_{jl} \right) \quad (1003)$$


---

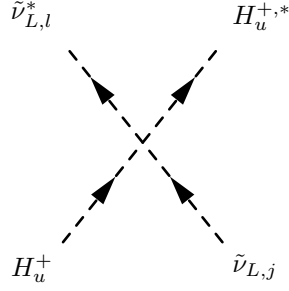

$$\frac{i}{4} \left( -g_{A2}^2 + g_{A1}^2 \right) \delta_{jl} \quad (1004)$$

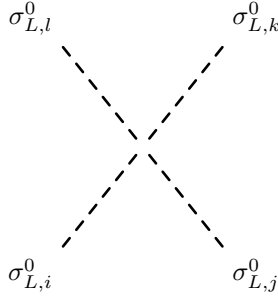

$$\begin{aligned}
& -\frac{i}{2} \left( 2g_{A1}^2 Z_{Ls,i3}^{Di,*} Z_{Ls,j3}^{Di,*} Z_{Ls,k1}^{Di,*} Z_{Ls,l1}^{Di,*} - 2g_{A2}^2 Z_{Ls,i3}^{Di,*} Z_{Ls,j3}^{Di,*} Z_{Ls,k1}^{Di,*} Z_{Ls,l1}^{Di,*} \right. \\
& + 2g_{B1}^2 Z_{Ls,i3}^{Di,*} Z_{Ls,j3}^{Di,*} Z_{Ls,k1}^{Di,*} Z_{Ls,l1}^{Di,*} - 2g_{B2}^2 Z_{Ls,i3}^{Di,*} Z_{Ls,j3}^{Di,*} Z_{Ls,k1}^{Di,*} Z_{Ls,l1}^{Di,*} \\
& - 2g_{A1}^2 Z_{Ls,i4}^{Di,*} Z_{Ls,j4}^{Di,*} Z_{Ls,k1}^{Di,*} Z_{Ls,l1}^{Di,*} + 2g_{A2}^2 Z_{Ls,i4}^{Di,*} Z_{Ls,j4}^{Di,*} Z_{Ls,k1}^{Di,*} Z_{Ls,l1}^{Di,*} \\
& - 2g_{B1}^2 Z_{Ls,i4}^{Di,*} Z_{Ls,j4}^{Di,*} Z_{Ls,k1}^{Di,*} Z_{Ls,l1}^{Di,*} + 2g_{B2}^2 Z_{Ls,i4}^{Di,*} Z_{Ls,j4}^{Di,*} Z_{Ls,k1}^{Di,*} Z_{Ls,l1}^{Di,*} \\
& - 2|Y_A|^2 Z_{Ls,i4}^{Di,*} Z_{Ls,j3}^{Di,*} Z_{Ls,k2}^{Di,*} Z_{Ls,l1}^{Di,*} + |Y_K|^2 Z_{Ls,i4}^{Di,*} Z_{Ls,j3}^{Di,*} Z_{Ls,k2}^{Di,*} Z_{Ls,l1}^{Di,*} \\
& - 2|Y_A|^2 Z_{Ls,i3}^{Di,*} Z_{Ls,j4}^{Di,*} Z_{Ls,k2}^{Di,*} Z_{Ls,l1}^{Di,*} + |Y_K|^2 Z_{Ls,i3}^{Di,*} Z_{Ls,j4}^{Di,*} Z_{Ls,k2}^{Di,*} Z_{Ls,l1}^{Di,*} \\
& + 2g_{A1}^2 Z_{Ls,i3}^{Di,*} Z_{Ls,j1}^{Di,*} Z_{Ls,k3}^{Di,*} Z_{Ls,l1}^{Di,*} - 2g_{A2}^2 Z_{Ls,i3}^{Di,*} Z_{Ls,j1}^{Di,*} Z_{Ls,k3}^{Di,*} Z_{Ls,l1}^{Di,*} \\
& + 2g_{B1}^2 Z_{Ls,i3}^{Di,*} Z_{Ls,j1}^{Di,*} Z_{Ls,k3}^{Di,*} Z_{Ls,l1}^{Di,*} - 2g_{B2}^2 Z_{Ls,i3}^{Di,*} Z_{Ls,j1}^{Di,*} Z_{Ls,k3}^{Di,*} Z_{Ls,l1}^{Di,*} \\
& - 2|Y_A|^2 Z_{Ls,i4}^{Di,*} Z_{Ls,j2}^{Di,*} Z_{Ls,k3}^{Di,*} Z_{Ls,l1}^{Di,*} + |Y_K|^2 Z_{Ls,i4}^{Di,*} Z_{Ls,j2}^{Di,*} Z_{Ls,k3}^{Di,*} Z_{Ls,l1}^{Di,*} \\
& - 2g_{A1}^2 Z_{Ls,i4}^{Di,*} Z_{Ls,j1}^{Di,*} Z_{Ls,k4}^{Di,*} Z_{Ls,l1}^{Di,*} + 2g_{A2}^2 Z_{Ls,i4}^{Di,*} Z_{Ls,j1}^{Di,*} Z_{Ls,k4}^{Di,*} Z_{Ls,l1}^{Di,*} \\
& - 2g_{B1}^2 Z_{Ls,i4}^{Di,*} Z_{Ls,j1}^{Di,*} Z_{Ls,k4}^{Di,*} Z_{Ls,l1}^{Di,*} + 2g_{B2}^2 Z_{Ls,i4}^{Di,*} Z_{Ls,j1}^{Di,*} Z_{Ls,k4}^{Di,*} Z_{Ls,l1}^{Di,*} \\
& - 2|Y_A|^2 Z_{Ls,i3}^{Di,*} Z_{Ls,j2}^{Di,*} Z_{Ls,k4}^{Di,*} Z_{Ls,l1}^{Di,*} + |Y_K|^2 Z_{Ls,i3}^{Di,*} Z_{Ls,j2}^{Di,*} Z_{Ls,k4}^{Di,*} Z_{Ls,l1}^{Di,*} \\
& - 2|Y_A|^2 Z_{Ls,i4}^{Di,*} Z_{Ls,j3}^{Di,*} Z_{Ls,k1}^{Di,*} Z_{Ls,l2}^{Di,*} + |Y_K|^2 Z_{Ls,i4}^{Di,*} Z_{Ls,j3}^{Di,*} Z_{Ls,k1}^{Di,*} Z_{Ls,l2}^{Di,*}
\end{aligned}$$



[illegible]

$$\begin{aligned}
& -2|Y_A|^2 Z_{Ls,i3}^{Di,*} Z_{Ls,j1}^{Di,*} Z_{Ls,k2}^{Di,*} Z_{Ls,l4}^{Di,*} + |Y_K|^2 Z_{Ls,i3}^{Di,*} Z_{Ls,j1}^{Di,*} Z_{Ls,k2}^{Di,*} Z_{Ls,l4}^{Di,*} \\
& + 2g_{A1}^2 Z_{Ls,i4}^{Di,*} Z_{Ls,j2}^{Di,*} Z_{Ls,k2}^{Di,*} Z_{Ls,l4}^{Di,*} - 2g_{A2}^2 Z_{Ls,i4}^{Di,*} Z_{Ls,j2}^{Di,*} Z_{Ls,k2}^{Di,*} Z_{Ls,l4}^{Di,*} \\
& + 2g_{B1}^2 Z_{Ls,i4}^{Di,*} Z_{Ls,j2}^{Di,*} Z_{Ls,k2}^{Di,*} Z_{Ls,l4}^{Di,*} - 2g_{B2}^2 Z_{Ls,i4}^{Di,*} Z_{Ls,j2}^{Di,*} Z_{Ls,k2}^{Di,*} Z_{Ls,l4}^{Di,*} \\
& - 2g_{A1}^2 Z_{Ls,i4}^{Di,*} Z_{Ls,j3}^{Di,*} Z_{Ls,k3}^{Di,*} Z_{Ls,l4}^{Di,*} - 2g_{A2}^2 Z_{Ls,i4}^{Di,*} Z_{Ls,j3}^{Di,*} Z_{Ls,k3}^{Di,*} Z_{Ls,l4}^{Di,*} \\
& - 2g_{B1}^2 Z_{Ls,i4}^{Di,*} Z_{Ls,j3}^{Di,*} Z_{Ls,k3}^{Di,*} Z_{Ls,l4}^{Di,*} - 2g_{B2}^2 Z_{Ls,i4}^{Di,*} Z_{Ls,j3}^{Di,*} Z_{Ls,k3}^{Di,*} Z_{Ls,l4}^{Di,*} \\
& + 4|Y_A|^2 Z_{Ls,i4}^{Di,*} Z_{Ls,j3}^{Di,*} Z_{Ls,k3}^{Di,*} Z_{Ls,l4}^{Di,*} + 2|Y_K|^2 Z_{Ls,i4}^{Di,*} Z_{Ls,j3}^{Di,*} Z_{Ls,k3}^{Di,*} Z_{Ls,l4}^{Di,*} \\
& - 2g_{A1}^2 Z_{Ls,i3}^{Di,*} Z_{Ls,j4}^{Di,*} Z_{Ls,k3}^{Di,*} Z_{Ls,l4}^{Di,*} - 2g_{A2}^2 Z_{Ls,i3}^{Di,*} Z_{Ls,j4}^{Di,*} Z_{Ls,k3}^{Di,*} Z_{Ls,l4}^{Di,*} \\
& - 2g_{B1}^2 Z_{Ls,i3}^{Di,*} Z_{Ls,j4}^{Di,*} Z_{Ls,k3}^{Di,*} Z_{Ls,l4}^{Di,*} - 2g_{B2}^2 Z_{Ls,i3}^{Di,*} Z_{Ls,j4}^{Di,*} Z_{Ls,k3}^{Di,*} Z_{Ls,l4}^{Di,*} \\
& + 4|Y_A|^2 Z_{Ls,i3}^{Di,*} Z_{Ls,j4}^{Di,*} Z_{Ls,k3}^{Di,*} Z_{Ls,l4}^{Di,*} + 2|Y_K|^2 Z_{Ls,i3}^{Di,*} Z_{Ls,j4}^{Di,*} Z_{Ls,k3}^{Di,*} Z_{Ls,l4}^{Di,*} \\
& - 2g_{A1}^2 Z_{Ls,i3}^{Di,*} Z_{Ls,j3}^{Di,*} Z_{Ls,k4}^{Di,*} Z_{Ls,l4}^{Di,*} - 2g_{A2}^2 Z_{Ls,i3}^{Di,*} Z_{Ls,j3}^{Di,*} Z_{Ls,k4}^{Di,*} Z_{Ls,l4}^{Di,*} \\
& - 2g_{B1}^2 Z_{Ls,i3}^{Di,*} Z_{Ls,j3}^{Di,*} Z_{Ls,k4}^{Di,*} Z_{Ls,l4}^{Di,*} - 2g_{B2}^2 Z_{Ls,i3}^{Di,*} Z_{Ls,j3}^{Di,*} Z_{Ls,k4}^{Di,*} Z_{Ls,l4}^{Di,*} \\
& + 4|Y_A|^2 Z_{Ls,i3}^{Di,*} Z_{Ls,j4}^{Di,*} Z_{Ls,k4}^{Di,*} Z_{Ls,l4}^{Di,*} + 2|Y_K|^2 Z_{Ls,i3}^{Di,*} Z_{Ls,j4}^{Di,*} Z_{Ls,k4}^{Di,*} Z_{Ls,l4}^{Di,*} \\
& + 6g_{A1}^2 Z_{Ls,i4}^{Di,*} Z_{Ls,j4}^{Di,*} Z_{Ls,k4}^{Di,*} Z_{Ls,l4}^{Di,*} + 6g_{A2}^2 Z_{Ls,i4}^{Di,*} Z_{Ls,j4}^{Di,*} Z_{Ls,k4}^{Di,*} Z_{Ls,l4}^{Di,*} \\
& + 6g_{B1}^2 Z_{Ls,i4}^{Di,*} Z_{Ls,j4}^{Di,*} Z_{Ls,k4}^{Di,*} Z_{Ls,l4}^{Di,*} + 6g_{B2}^2 Z_{Ls,i4}^{Di,*} Z_{Ls,j4}^{Di,*} Z_{Ls,k4}^{Di,*} Z_{Ls,l4}^{Di,*} \\
& + Z_{Ls,i2}^{Di,*} \left( -2|Y_A|^2 Z_{Ls,j4}^{Di,*} Z_{Ls,k3}^{Di,*} Z_{Ls,l1}^{Di,*} + |Y_K|^2 Z_{Ls,j4}^{Di,*} Z_{Ls,k3}^{Di,*} Z_{Ls,l1}^{Di,*} - 2|Y_A|^2 Z_{Ls,j3}^{Di,*} Z_{Ls,k4}^{Di,*} Z_{Ls,l1}^{Di,*} \right. \\
& + |Y_K|^2 Z_{Ls,j3}^{Di,*} Z_{Ls,k4}^{Di,*} Z_{Ls,l1}^{Di,*} - 2g_{A1}^2 Z_{Ls,j3}^{Di,*} Z_{Ls,k3}^{Di,*} Z_{Ls,l2}^{Di,*} + 2g_{A2}^2 Z_{Ls,j3}^{Di,*} Z_{Ls,k3}^{Di,*} Z_{Ls,l2}^{Di,*} \\
& - 2g_{B1}^2 Z_{Ls,j3}^{Di,*} Z_{Ls,k3}^{Di,*} Z_{Ls,l2}^{Di,*} + 2g_{B2}^2 Z_{Ls,j3}^{Di,*} Z_{Ls,k3}^{Di,*} Z_{Ls,l2}^{Di,*} + 2g_{A1}^2 Z_{Ls,j4}^{Di,*} Z_{Ls,k4}^{Di,*} Z_{Ls,l2}^{Di,*} \\
& - 2g_{A2}^2 Z_{Ls,j4}^{Di,*} Z_{Ls,k4}^{Di,*} Z_{Ls,l2}^{Di,*} + 2g_{B1}^2 Z_{Ls,j4}^{Di,*} Z_{Ls,k4}^{Di,*} Z_{Ls,l2}^{Di,*} - 2g_{B2}^2 Z_{Ls,j4}^{Di,*} Z_{Ls,k4}^{Di,*} Z_{Ls,l2}^{Di,*} \\
& - 2|Y_A|^2 Z_{Ls,j4}^{Di,*} Z_{Ls,k1}^{Di,*} Z_{Ls,l3}^{Di,*} + |Y_K|^2 Z_{Ls,j4}^{Di,*} Z_{Ls,k1}^{Di,*} Z_{Ls,l3}^{Di,*} - 2g_{A1}^2 Z_{Ls,j3}^{Di,*} Z_{Ls,k2}^{Di,*} Z_{Ls,l3}^{Di,*} \\
& + 2g_{A2}^2 Z_{Ls,j3}^{Di,*} Z_{Ls,k2}^{Di,*} Z_{Ls,l3}^{Di,*} - 2g_{B1}^2 Z_{Ls,j3}^{Di,*} Z_{Ls,k2}^{Di,*} Z_{Ls,l3}^{Di,*} + 2g_{B2}^2 Z_{Ls,j3}^{Di,*} Z_{Ls,k2}^{Di,*} Z_{Ls,l3}^{Di,*} \\
& - 2|Y_A|^2 Z_{Ls,j3}^{Di,*} Z_{Ls,k1}^{Di,*} Z_{Ls,l4}^{Di,*} + |Y_K|^2 Z_{Ls,j3}^{Di,*} Z_{Ls,k1}^{Di,*} Z_{Ls,l4}^{Di,*} + 2g_{A1}^2 Z_{Ls,j4}^{Di,*} Z_{Ls,k2}^{Di,*} Z_{Ls,l4}^{Di,*} \\
& - 2g_{A2}^2 Z_{Ls,j4}^{Di,*} Z_{Ls,k2}^{Di,*} Z_{Ls,l4}^{Di,*} + 2g_{B1}^2 Z_{Ls,j4}^{Di,*} Z_{Ls,k2}^{Di,*} Z_{Ls,l4}^{Di,*} - 2g_{B2}^2 Z_{Ls,j4}^{Di,*} Z_{Ls,k2}^{Di,*} Z_{Ls,l4}^{Di,*} \\
& \left. - Z_{Ls,j1}^{Di,*} \left( 2 \left( -2|Y_A|^2 - |Y_K|^2 + g_{A1}^2 + g_{A2}^2 + g_{B1}^2 + g_{B2}^2 \right) Z_{Ls,k2}^{Di,*} Z_{Ls,l1}^{Di,*} \right. \right. \\
& + 2 \left( -2|Y_A|^2 - |Y_K|^2 + g_{A1}^2 + g_{A2}^2 + g_{B1}^2 + g_{B2}^2 \right) Z_{Ls,k1}^{Di,*} Z_{Ls,l2}^{Di,*} \\
& + \left( 2|Y_A|^2 - |Y_K|^2 \right) \left( Z_{Ls,k3}^{Di,*} Z_{Ls,l4}^{Di,*} + Z_{Ls,k4}^{Di,*} Z_{Ls,l3}^{Di,*} \right) \Big) \\
& - 2Z_{Ls,j2}^{Di,*} \left( \left( -2|Y_A|^2 - |Y_K|^2 + g_{A1}^2 + g_{A2}^2 + g_{B1}^2 + g_{B2}^2 \right) Z_{Ls,k1}^{Di,*} Z_{Ls,l1}^{Di,*} - 3 \left( g_{A1}^2 + g_{A2}^2 + g_{B1}^2 + g_{B2}^2 \right) Z_{Ls,k2}^{Di,*} Z_{Ls,l2}^{Di,*} \right. \\
& + \left( -g_{A2}^2 - g_{B2}^2 + g_{A1}^2 + g_{B1}^2 \right) \left( Z_{Ls,k3}^{Di,*} Z_{Ls,l3}^{Di,*} - Z_{Ls,k4}^{Di,*} Z_{Ls,l4}^{Di,*} \right) \Big) \\
& + Z_{Ls,i1}^{Di,*} \left( -2g_{A1}^2 Z_{Ls,j2}^{Di,*} Z_{Ls,k2}^{Di,*} Z_{Ls,l1}^{Di,*} - 2g_{A2}^2 Z_{Ls,j2}^{Di,*} Z_{Ls,k2}^{Di,*} Z_{Ls,l1}^{Di,*} - 2g_{B1}^2 Z_{Ls,j2}^{Di,*} Z_{Ls,k2}^{Di,*} Z_{Ls,l1}^{Di,*} \right. \\
& \left. - 2g_{B2}^2 Z_{Ls,j2}^{Di,*} Z_{Ls,k2}^{Di,*} Z_{Ls,l1}^{Di,*} + 4|Y_A|^2 Z_{Ls,j2}^{Di,*} Z_{Ls,k2}^{Di,*} Z_{Ls,l1}^{Di,*} + 2|Y_K|^2 Z_{Ls,j2}^{Di,*} Z_{Ls,k2}^{Di,*} Z_{Ls,l1}^{Di,*} \right)
\end{aligned}$$

$$\begin{aligned}
& + 2g_{A1}^2 Z_{Ls,j3}^{Di,*} Z_{Ls,k3}^{Di,*} Z_{Ls,l1}^{Di,*} - 2g_{A2}^2 Z_{Ls,j3}^{Di,*} Z_{Ls,k3}^{Di,*} Z_{Ls,l1}^{Di,*} + 2g_{B1}^2 Z_{Ls,j3}^{Di,*} Z_{Ls,k3}^{Di,*} Z_{Ls,l1}^{Di,*} \\
& - 2g_{B2}^2 Z_{Ls,j3}^{Di,*} Z_{Ls,k3}^{Di,*} Z_{Ls,l1}^{Di,*} - 2g_{A1}^2 Z_{Ls,j4}^{Di,*} Z_{Ls,k4}^{Di,*} Z_{Ls,l1}^{Di,*} + 2g_{A2}^2 Z_{Ls,j4}^{Di,*} Z_{Ls,k4}^{Di,*} Z_{Ls,l1}^{Di,*} \\
& - 2g_{B1}^2 Z_{Ls,j4}^{Di,*} Z_{Ls,k4}^{Di,*} Z_{Ls,l1}^{Di,*} + 2g_{B2}^2 Z_{Ls,j4}^{Di,*} Z_{Ls,k4}^{Di,*} Z_{Ls,l1}^{Di,*} - 2g_{A1}^2 Z_{Ls,j2}^{Di,*} Z_{Ls,k1}^{Di,*} Z_{Ls,l2}^{Di,*} \\
& - 2g_{A2}^2 Z_{Ls,j2}^{Di,*} Z_{Ls,k1}^{Di,*} Z_{Ls,l2}^{Di,*} - 2g_{B1}^2 Z_{Ls,j2}^{Di,*} Z_{Ls,k1}^{Di,*} Z_{Ls,l2}^{Di,*} - 2g_{B2}^2 Z_{Ls,j2}^{Di,*} Z_{Ls,k1}^{Di,*} Z_{Ls,l2}^{Di,*} \\
& + 4|Y_A|^2 Z_{Ls,j2}^{Di,*} Z_{Ls,k1}^{Di,*} Z_{Ls,l2}^{Di,*} + 2|Y_K|^2 Z_{Ls,j2}^{Di,*} Z_{Ls,k1}^{Di,*} Z_{Ls,l2}^{Di,*} - 2|Y_A|^2 Z_{Ls,j4}^{Di,*} Z_{Ls,k3}^{Di,*} Z_{Ls,l2}^{Di,*} \\
& + |Y_K|^2 Z_{Ls,j4}^{Di,*} Z_{Ls,k3}^{Di,*} Z_{Ls,l2}^{Di,*} - 2|Y_A|^2 Z_{Ls,j3}^{Di,*} Z_{Ls,k4}^{Di,*} Z_{Ls,l2}^{Di,*} + |Y_K|^2 Z_{Ls,j3}^{Di,*} Z_{Ls,k4}^{Di,*} Z_{Ls,l2}^{Di,*} \\
& + 2g_{A1}^2 Z_{Ls,j3}^{Di,*} Z_{Ls,k1}^{Di,*} Z_{Ls,l3}^{Di,*} - 2g_{A2}^2 Z_{Ls,j3}^{Di,*} Z_{Ls,k1}^{Di,*} Z_{Ls,l3}^{Di,*} + 2g_{B1}^2 Z_{Ls,j3}^{Di,*} Z_{Ls,k1}^{Di,*} Z_{Ls,l3}^{Di,*} \\
& - 2g_{B2}^2 Z_{Ls,j3}^{Di,*} Z_{Ls,k1}^{Di,*} Z_{Ls,l3}^{Di,*} - 2|Y_A|^2 Z_{Ls,j4}^{Di,*} Z_{Ls,k2}^{Di,*} Z_{Ls,l3}^{Di,*} + |Y_K|^2 Z_{Ls,j4}^{Di,*} Z_{Ls,k2}^{Di,*} Z_{Ls,l3}^{Di,*} \\
& - 2|Y_A|^2 Z_{Ls,j2}^{Di,*} Z_{Ls,k4}^{Di,*} Z_{Ls,l3}^{Di,*} + |Y_K|^2 Z_{Ls,j2}^{Di,*} Z_{Ls,k4}^{Di,*} Z_{Ls,l3}^{Di,*} - 2g_{A1}^2 Z_{Ls,j4}^{Di,*} Z_{Ls,k1}^{Di,*} Z_{Ls,l4}^{Di,*} \\
& + 2g_{A2}^2 Z_{Ls,j4}^{Di,*} Z_{Ls,k1}^{Di,*} Z_{Ls,l4}^{Di,*} - 2g_{B1}^2 Z_{Ls,j4}^{Di,*} Z_{Ls,k1}^{Di,*} Z_{Ls,l4}^{Di,*} + 2g_{B2}^2 Z_{Ls,j4}^{Di,*} Z_{Ls,k1}^{Di,*} Z_{Ls,l4}^{Di,*} \\
& - 2|Y_A|^2 Z_{Ls,j3}^{Di,*} Z_{Ls,k2}^{Di,*} Z_{Ls,l4}^{Di,*} + |Y_K|^2 Z_{Ls,j3}^{Di,*} Z_{Ls,k2}^{Di,*} Z_{Ls,l4}^{Di,*} - 2|Y_A|^2 Z_{Ls,j2}^{Di,*} Z_{Ls,k3}^{Di,*} Z_{Ls,l4}^{Di,*} \\
& + |Y_K|^2 Z_{Ls,j2}^{Di,*} Z_{Ls,k3}^{Di,*} Z_{Ls,l4}^{Di,*} \\
& + 2Z_{Ls,j1}^{Di,*} \left( 3 \left( g_{A1}^2 + g_{A2}^2 + g_{B1}^2 + g_{B2}^2 \right) Z_{Ls,k1}^{Di,*} Z_{Ls,l1}^{Di,*} - \left( -2|Y_A|^2 - |Y_K|^2 + g_{A1}^2 + g_{A2}^2 + g_{B1}^2 + g_{B2}^2 \right) Z_{Ls,k2}^{Di,*} Z_{Ls,l2}^{Di,*} \right. \\
& \left. + \left( -g_{A2}^2 - g_{B2}^2 + g_{A1}^2 + g_{B1}^2 \right) \left( Z_{Ls,k3}^{Di,*} Z_{Ls,l3}^{Di,*} - Z_{Ls,k4}^{Di,*} Z_{Ls,l4}^{Di,*} \right) \right) \quad (1005)
\end{aligned}$$

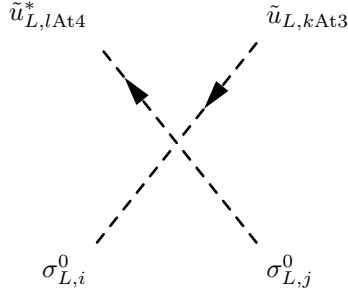

$$\begin{aligned}
& \frac{i}{6} \left( \left( -3g_{A2}^2 + g_{A1}^2 \right) Z_{Ls,i1}^{Di,*} Z_{Ls,j1}^{Di,*} - \left( -3g_{A2}^2 + g_{A1}^2 \right) Z_{Ls,i2}^{Di,*} Z_{Ls,j2}^{Di,*} \right. \\
& \left. + \left( 3g_{A2}^2 + g_{A1}^2 \right) \left( Z_{Ls,i3}^{Di,*} Z_{Ls,j3}^{Di,*} - Z_{Ls,i4}^{Di,*} Z_{Ls,j4}^{Di,*} \right) \right) \delta_{At3At4} \delta_{kl} \quad (1006)
\end{aligned}$$

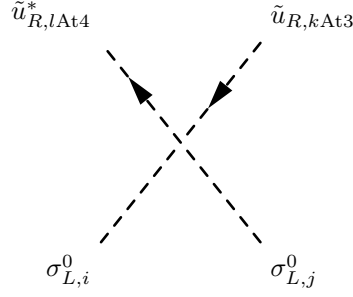

$$-\frac{2i}{3}g_{A1}^2 \left( Z_{Ls,i1}^{Di,*} Z_{Ls,j1}^{Di,*} - Z_{Ls,i2}^{Di,*} Z_{Ls,j2}^{Di,*} + Z_{Ls,i3}^{Di,*} Z_{Ls,j3}^{Di,*} - Z_{Ls,i4}^{Di,*} Z_{Ls,j4}^{Di,*} \right) \delta_{At3At4} \delta_{kl} \quad (1007)$$


---

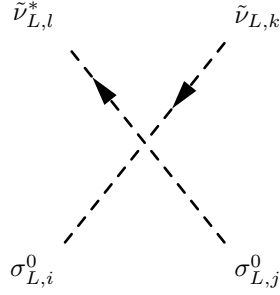

$$-\frac{i}{2} \left( \left( g_{A1}^2 + g_{A2}^2 \right) Z_{Ls,i1}^{Di,*} Z_{Ls,j1}^{Di,*} - \left( g_{A1}^2 + g_{A2}^2 \right) Z_{Ls,i2}^{Di,*} Z_{Ls,j2}^{Di,*} \right. \\ \left. + \left( -g_{A2}^2 + g_{A1}^2 \right) \left( Z_{Ls,i3}^{Di,*} Z_{Ls,j3}^{Di,*} - Z_{Ls,i4}^{Di,*} Z_{Ls,j4}^{Di,*} \right) \right) \delta_{kl} \quad (1008)$$


---

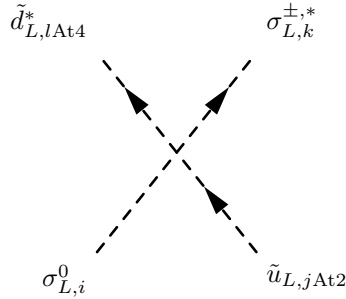

$$\frac{1}{2}g_{A2}^2 \delta_{At2At4} \delta_{jl} \left( -Z_{Ls,i1}^{Di,*} Z_{Ls,k4}^{od} - Z_{Ls,i2}^{Di,*} Z_{Ls,k2}^{od} + Z_{Ls,i3}^{Di,*} Z_{Ls,k1}^{od} + Z_{Ls,i4}^{Di,*} Z_{Ls,k3}^{od} \right) \quad (1009)$$


---

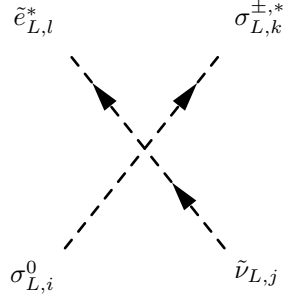

$$\frac{1}{2}g_{A2}^2\delta_{jl}\left(-Z_{Ls,i1}^{Di,*}Z_{Ls,k4}^{od}-Z_{Ls,i2}^{Di,*}Z_{Ls,k2}^{od}+Z_{Ls,i3}^{Di,*}Z_{Ls,k1}^{od}+Z_{Ls,i4}^{Di,*}Z_{Ls,k3}^{od}\right) \quad (1010)$$


---

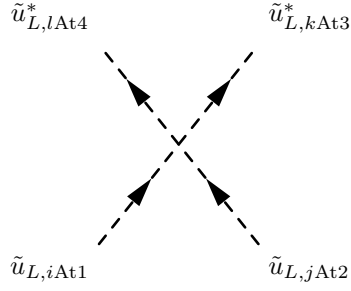

$$\begin{aligned} &\frac{i}{36}\left(\delta_{At1At4}\delta_{At2At3}\left(-18g_3^2\delta_{ik}\delta_{jl}+\left(6g_3^2-9g_{A2}^2-g_{A1}^2\right)\delta_{il}\delta_{jk}\right)\right. \\ &\quad \left.-\delta_{At1At3}\delta_{At2At4}\left(18g_3^2\delta_{il}\delta_{jk}+\left(-6g_3^2+9g_{A2}^2+g_{A1}^2\right)\delta_{ik}\delta_{jl}\right)\right) \end{aligned} \quad (1011)$$


---

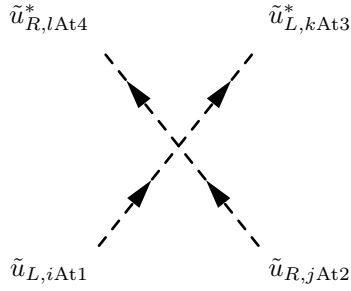

$$\frac{i}{18}\left(\left(2g_{A1}^2-3g_3^2\right)\delta_{At1At3}\delta_{At2At4}\delta_{ik}\delta_{jl}+9\delta_{At1At4}\delta_{At2At3}\left(-2Y_{u,jk}^*Y_{u,li}+g_3^2\delta_{ik}\delta_{jl}\right)\right) \quad (1012)$$


---

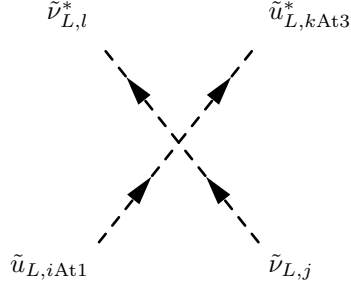

$$\frac{i}{12} \left( -3g_{A2}^2 + g_{A1}^2 \right) \delta_{\text{At}1\text{At}3} \delta_{ik} \delta_{jl} \quad (1013)$$


---

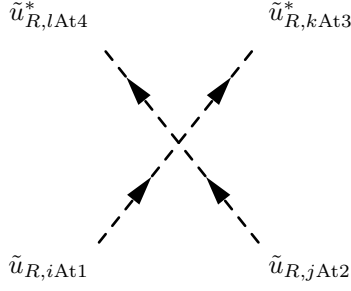

$$\begin{aligned} & \frac{i}{18} \left( \delta_{\text{At}1\text{At}4} \delta_{\text{At}2\text{At}3} \left( \left( 3g_3^2 - 8g_{A1}^2 \right) \delta_{il} \delta_{jk} - 9g_3^2 \delta_{ik} \delta_{jl} \right) \right. \\ & \left. + \delta_{\text{At}1\text{At}3} \delta_{\text{At}2\text{At}4} \left( \left( 3g_3^2 - 8g_{A1}^2 \right) \delta_{ik} \delta_{jl} - 9g_3^2 \delta_{il} \delta_{jk} \right) \right) \end{aligned} \quad (1014)$$


---

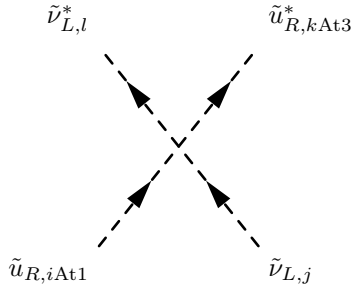

$$- \frac{i}{3} g_{A1}^2 \delta_{\text{At}1\text{At}3} \delta_{ik} \delta_{jl} \quad (1015)$$


---

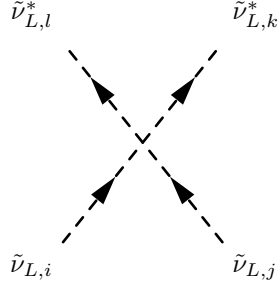

$$-\frac{i}{4}\left(g_{A1}^2 + g_{A2}^2\right)\left(\delta_{ik}\delta_{jl} + \delta_{il}\delta_{jk}\right) \quad (1016)$$


---

## 9.8 Two Scalar-Two Vector Boson-Interaction

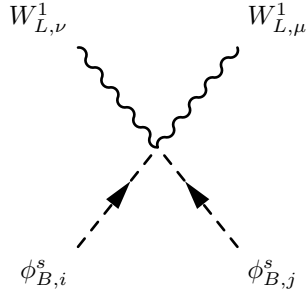

$$-ig_{A2}^2 g_{B2}^2 \left(g_{A2}^2 + g_{B2}^2\right)^{-1} \left(B_{A,i1}^{s,*} B_{A,j2}^{s,*} + B_{A,i2}^{s,*} B_{A,j1}^{s,*}\right) \left(g_{\mu\nu}\right) \quad (1017)$$


---

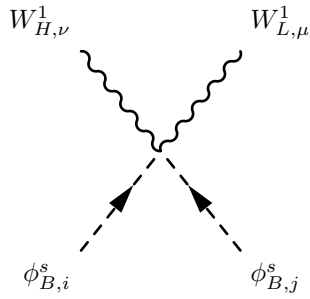

$$-ig_{B2}^3 \sqrt{\frac{g_{A2}^2}{g_{A2}^2 + g_{B2}^2}} \frac{1}{\sqrt{g_{A2}^2 + g_{B2}^2}} \left(B_{A,i1}^{s,*} B_{A,j2}^{s,*} + B_{A,i2}^{s,*} B_{A,j1}^{s,*}\right) \left(g_{\mu\nu}\right) \quad (1018)$$


---

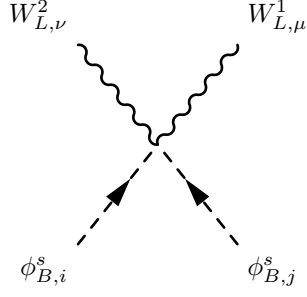

$$g_{A2}^2 g_{B2}^2 (g_{A2}^2 + g_{B2}^2)^{-1} (B_{A,i1}^{s,*} B_{A,j2}^{s,*} + B_{A,i2}^{s,*} B_{A,j1}^{s,*}) (g_{\mu\nu}) \quad (1019)$$


---

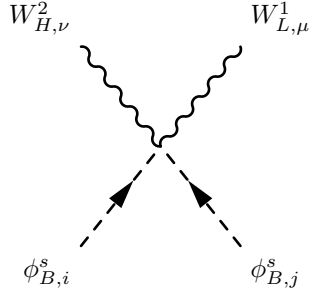

$$g_{B2}^3 \sqrt{\frac{g_{A2}^2}{g_{A2}^2 + g_{B2}^2}} \frac{1}{\sqrt{g_{A2}^2 + g_{B2}^2}} (B_{A,i1}^{s,*} B_{A,j2}^{s,*} + B_{A,i2}^{s,*} B_{A,j1}^{s,*}) (g_{\mu\nu}) \quad (1020)$$


---

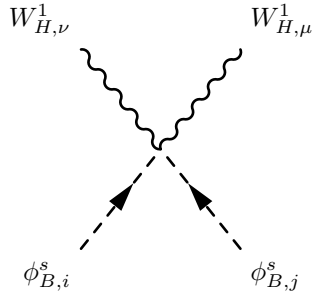

$$-i g_{B2}^4 (g_{A2}^2 + g_{B2}^2)^{-1} (B_{A,i1}^{s,*} B_{A,j2}^{s,*} + B_{A,i2}^{s,*} B_{A,j1}^{s,*}) (g_{\mu\nu}) \quad (1021)$$


---



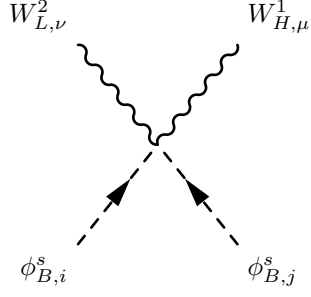

$$g_{B2}^3 \sqrt{\frac{gA2^2}{gA2^2 + gB2^2}} \frac{1}{\sqrt{gA2^2 + gB2^2}} \left( B_{A,i1}^{s,*} B_{A,j2}^{s,*} + B_{A,i2}^{s,*} B_{A,j1}^{s,*} \right) (g_{\mu\nu}) \quad (1022)$$


---

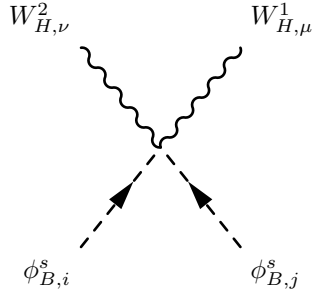

$$g_{B2}^4 \left( g_{A2}^2 + g_{B2}^2 \right)^{-1} \left( B_{A,i1}^{s,*} B_{A,j2}^{s,*} + B_{A,i2}^{s,*} B_{A,j1}^{s,*} \right) (g_{\mu\nu}) \quad (1023)$$


---

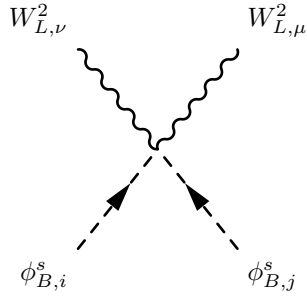

$$ig_{A2}^2 g_{B2}^2 \left( g_{A2}^2 + g_{B2}^2 \right)^{-1} \left( B_{A,i1}^{s,*} B_{A,j2}^{s,*} + B_{A,i2}^{s,*} B_{A,j1}^{s,*} \right) (g_{\mu\nu}) \quad (1024)$$


---

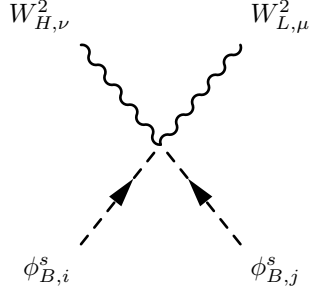

$$ig_{B2}^3 \sqrt{\frac{gA2^2}{gA2^2 + gB2^2}} \frac{1}{\sqrt{gA2^2 + gB2^2}} \left( B_{A,i1}^{s,*} B_{A,j2}^{s,*} + B_{A,i2}^{s,*} B_{A,j1}^{s,*} \right) (g_{\mu\nu}) \quad (1025)$$


---

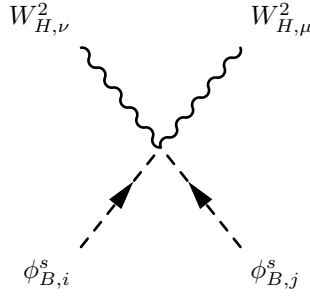

$$ig_{B2}^4 (g_{A2}^2 + g_{B2}^2)^{-1} \left( B_{A,i1}^{s,*} B_{A,j2}^{s,*} + B_{A,i2}^{s,*} B_{A,j1}^{s,*} \right) (g_{\mu\nu}) \quad (1026)$$


---

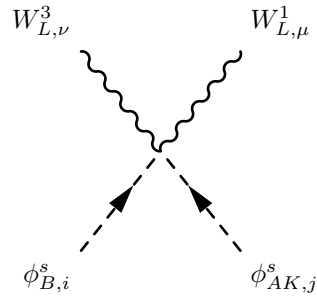

$$-i \frac{1}{\sqrt{2}} g_{A2}^2 g_{B2}^2 (g_{A2}^2 + g_{B2}^2)^{-1} Z_{AK,j2}^{s,*} B_{A,i2}^{s,*} (g_{\mu\nu}) \quad (1027)$$


---

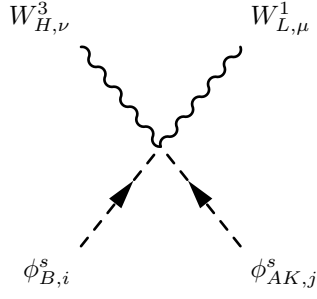

$$-i \frac{1}{\sqrt{2}} g_{B2}^3 \sqrt{\frac{gA2^2}{gA2^2 + gB2^2}} \frac{1}{\sqrt{gA2^2 + gB2^2}} Z_{AK,j2}^{s,*} B_{A,i2}^{s,*} (g_{\mu\nu}) \quad (1028)$$


---

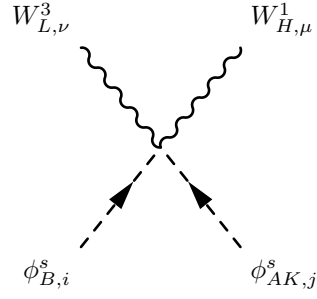

$$-i \frac{1}{\sqrt{2}} g_{B2}^3 \sqrt{\frac{gA2^2}{gA2^2 + gB2^2}} \frac{1}{\sqrt{gA2^2 + gB2^2}} Z_{AK,j2}^{s,*} B_{A,i2}^{s,*} (g_{\mu\nu}) \quad (1029)$$


---

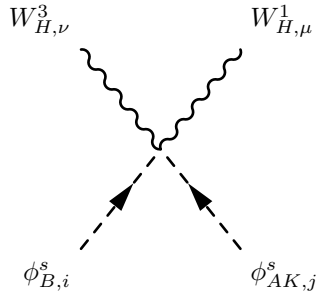

$$-i \frac{1}{\sqrt{2}} g_{B2}^4 (g_{A2}^2 + g_{B2}^2)^{-1} Z_{AK,j2}^{s,*} B_{A,i2}^{s,*} (g_{\mu\nu}) \quad (1030)$$


---

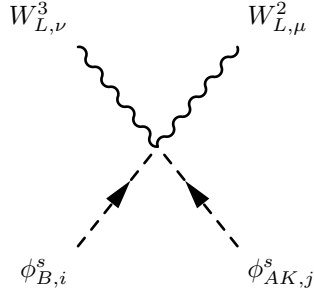

$$\frac{1}{\sqrt{2}} g_{A2}^2 g_{B2}^2 \left( g_{A2}^2 + g_{B2}^2 \right)^{-1} Z_{AK,j2}^{s,*} B_{A,i2}^{s,*} \left( g_{\mu\nu} \right) \quad (1031)$$


---

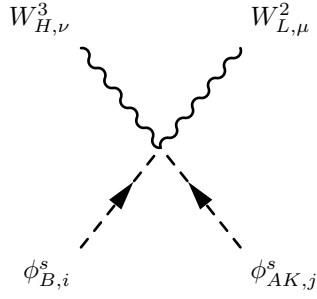

$$\frac{1}{\sqrt{2}} g_{B2}^3 \sqrt{\frac{g_{A2}^2}{g_{A2}^2 + g_{B2}^2}} \frac{1}{\sqrt{g_{A2}^2 + g_{B2}^2}} Z_{AK,j2}^{s,*} B_{A,i2}^{s,*} \left( g_{\mu\nu} \right) \quad (1032)$$


---

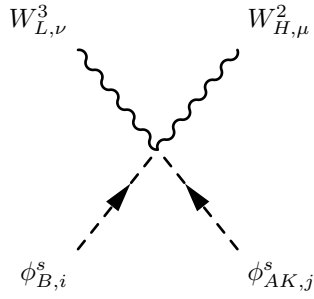

$$\frac{1}{\sqrt{2}} g_{B2}^3 \sqrt{\frac{g_{A2}^2}{g_{A2}^2 + g_{B2}^2}} \frac{1}{\sqrt{g_{A2}^2 + g_{B2}^2}} Z_{AK,j2}^{s,*} B_{A,i2}^{s,*} \left( g_{\mu\nu} \right) \quad (1033)$$


---

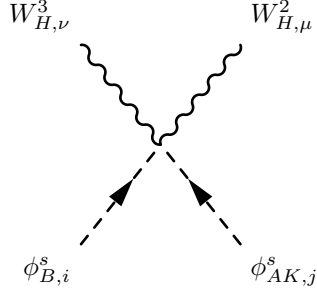

$$\frac{1}{\sqrt{2}} g_{B2}^4 \left( g_{A2}^2 + g_{B2}^2 \right)^{-1} Z_{AK,j2}^{s,*} B_{A,i2}^{s,*} \left( g_{\mu\nu} \right) \quad (1034)$$


---

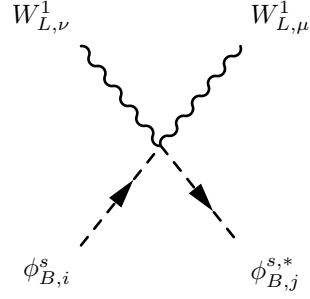

$$i g_{A2}^2 g_{B2}^2 \left( g_{A2}^2 + g_{B2}^2 \right)^{-1} \left( B_{A,i1}^{s,*} B_{A,j1}^s + B_{A,i2}^{s,*} B_{A,j2}^s \right) \left( g_{\mu\nu} \right) \quad (1035)$$


---

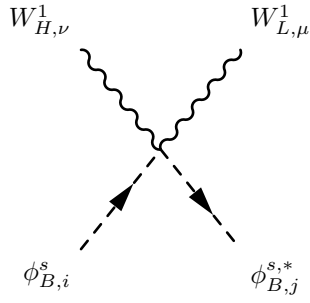

$$i g_{B2}^3 \sqrt{\frac{g_{A2}^2}{g_{A2}^2 + g_{B2}^2}} \frac{1}{\sqrt{g_{A2}^2 + g_{B2}^2}} \left( B_{A,i1}^{s,*} B_{A,j1}^s + B_{A,i2}^{s,*} B_{A,j2}^s \right) \left( g_{\mu\nu} \right) \quad (1036)$$


---

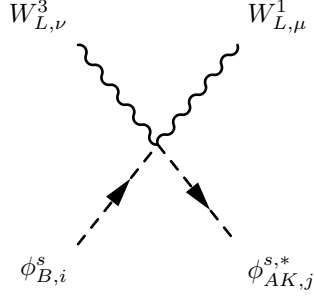

$$-i \frac{1}{\sqrt{2}} g_{A2}^2 g_{B2}^2 (g_{A2}^2 + g_{B2}^2)^{-1} B_{A,i1}^{s,*} Z_{AK,j2}^s (g_{\mu\nu}) \quad (1037)$$


---

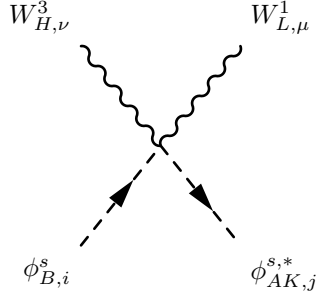

$$-i \frac{1}{\sqrt{2}} g_{B2}^3 \sqrt{\frac{g_{A2}^2}{g_{A2}^2 + g_{B2}^2}} \frac{1}{\sqrt{g_{A2}^2 + g_{B2}^2}} B_{A,i1}^{s,*} Z_{AK,j2}^s (g_{\mu\nu}) \quad (1038)$$


---

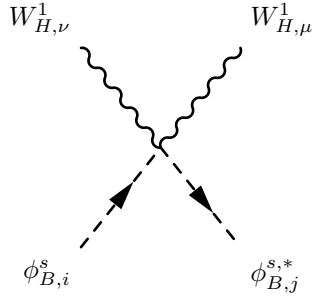

$$i g_{B2}^4 (g_{A2}^2 + g_{B2}^2)^{-1} (B_{A,i1}^{s,*} B_{A,j1}^s + B_{A,i2}^{s,*} B_{A,j2}^s) (g_{\mu\nu}) \quad (1039)$$


---

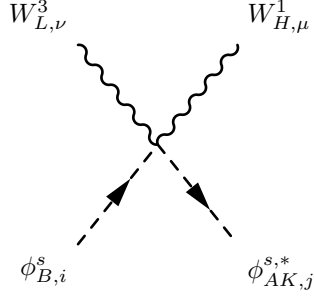

$$-i \frac{1}{\sqrt{2}} g_{B2}^3 \sqrt{\frac{g_{A2}^2}{g_{A2}^2 + g_{B2}^2}} \frac{1}{\sqrt{g_{A2}^2 + g_{B2}^2}} B_{A,i1}^{s,*} Z_{AK,j2}^s (g_{\mu\nu}) \quad (1040)$$


---

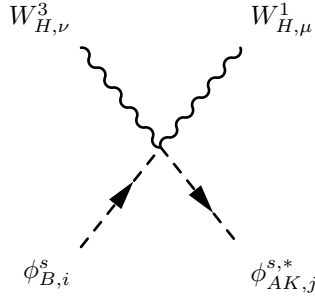

$$-i \frac{1}{\sqrt{2}} g_{B2}^4 (g_{A2}^2 + g_{B2}^2)^{-1} B_{A,i1}^{s,*} Z_{AK,j2}^s (g_{\mu\nu}) \quad (1041)$$


---

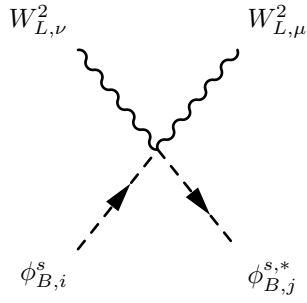

$$i g_{A2}^2 g_{B2}^2 (g_{A2}^2 + g_{B2}^2)^{-1} (B_{A,i1}^{s,*} B_{A,j1}^s + B_{A,i2}^{s,*} B_{A,j2}^s) (g_{\mu\nu}) \quad (1042)$$


---

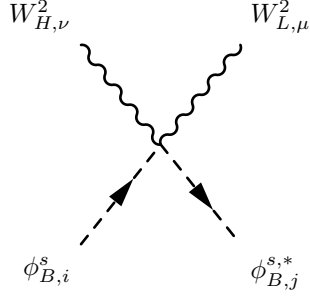

$$ig_{B2}^3 \sqrt{\frac{gA2^2}{gA2^2 + gB2^2}} \frac{1}{\sqrt{gA2^2 + gB2^2}} \left( B_{A,i1}^{s,*} B_{A,j1}^s + B_{A,i2}^{s,*} B_{A,j2}^s \right) (g_{\mu\nu}) \quad (1043)$$


---

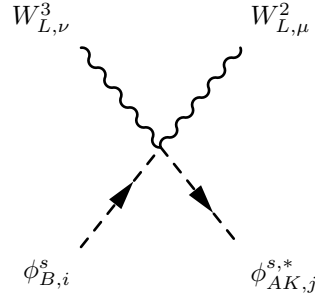

$$\frac{1}{\sqrt{2}} g_{A2}^2 g_{B2}^2 \left( g_{A2}^2 + g_{B2}^2 \right)^{-1} B_{A,i1}^{s,*} Z_{AK,j2}^s (g_{\mu\nu}) \quad (1044)$$


---

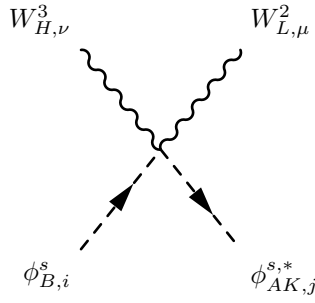

$$\frac{1}{\sqrt{2}} g_{B2}^3 \sqrt{\frac{gA2^2}{gA2^2 + gB2^2}} \frac{1}{\sqrt{gA2^2 + gB2^2}} B_{A,i1}^{s,*} Z_{AK,j2}^s (g_{\mu\nu}) \quad (1045)$$


---



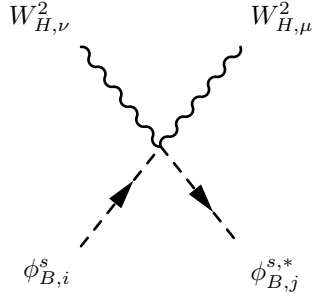

$$ig_{B2}^4 \left( g_{A2}^2 + g_{B2}^2 \right)^{-1} \left( B_{A,i1}^{s,*} B_{A,j1}^s + B_{A,i2}^{s,*} B_{A,j2}^s \right) (g_{\mu\nu}) \quad (1046)$$


---

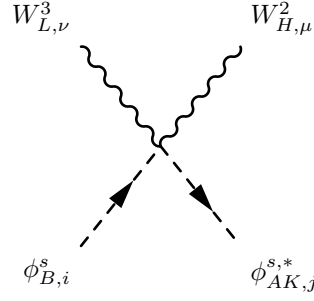

$$\frac{1}{\sqrt{2}} g_{B2}^3 \sqrt{\frac{g_{A2}^2}{g_{A2}^2 + g_{B2}^2}} \frac{1}{\sqrt{g_{A2}^2 + g_{B2}^2}} B_{A,i1}^{s,*} Z_{AK,j2}^s (g_{\mu\nu}) \quad (1047)$$


---

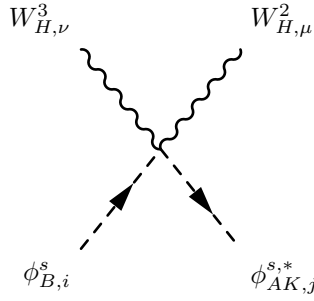

$$\frac{1}{\sqrt{2}} g_{B2}^4 \left( g_{A2}^2 + g_{B2}^2 \right)^{-1} B_{A,i1}^{s,*} Z_{AK,j2}^s (g_{\mu\nu}) \quad (1048)$$


---

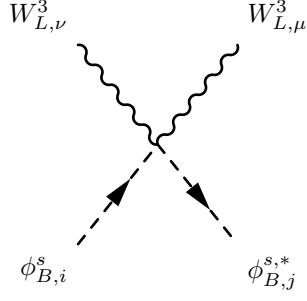

$$2ig_{A2}^2g_{B2}^2\left(g_{A2}^2+g_{B2}^2\right)^{-1}\left(B_{A,i1}^{s,*}B_{A,j1}^s+B_{A,i2}^{s,*}B_{A,j2}^s\right)\left(g_{\mu\nu}\right) \quad (1049)$$


---

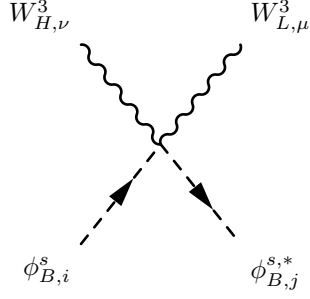

$$2ig_{B2}^3\sqrt{\frac{gA2^2}{gA2^2+gB2^2}}\frac{1}{\sqrt{gA2^2+gB2^2}}\left(B_{A,i1}^{s,*}B_{A,j1}^s+B_{A,i2}^{s,*}B_{A,j2}^s\right)\left(g_{\mu\nu}\right) \quad (1050)$$


---

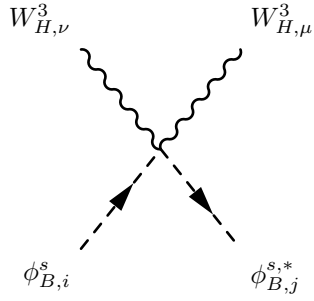

$$2ig_{B2}^4\left(g_{A2}^2+g_{B2}^2\right)^{-1}\left(B_{A,i1}^{s,*}B_{A,j1}^s+B_{A,i2}^{s,*}B_{A,j2}^s\right)\left(g_{\mu\nu}\right) \quad (1051)$$


---

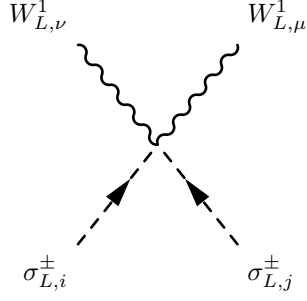

$$-ig_{A2}g_{B2}^2\sqrt{\frac{gA2^2}{gA2^2+gB2^2}}\frac{1}{\sqrt{gA2^2+gB2^2}}\left(Z_{Ls,i1}^{od,*}Z_{Ls,j4}^{od,*}+Z_{Ls,i2}^{od,*}Z_{Ls,j3}^{od,*}+Z_{Ls,i3}^{od,*}Z_{Ls,j2}^{od,*}+Z_{Ls,i4}^{od,*}Z_{Ls,j1}^{od,*}\right)\left(g_{\mu\nu}\right) \quad (1052)$$


---

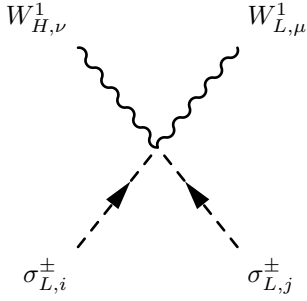

$$\frac{i}{2}g_{A2}g_{B2}\left(-g_{B2}^2+g_{A2}^2\right)\left(g_{A2}^2+g_{B2}^2\right)^{-1}\left(Z_{Ls,i1}^{od,*}Z_{Ls,j4}^{od,*}+Z_{Ls,i2}^{od,*}Z_{Ls,j3}^{od,*}+Z_{Ls,i3}^{od,*}Z_{Ls,j2}^{od,*}+Z_{Ls,i4}^{od,*}Z_{Ls,j1}^{od,*}\right)\left(g_{\mu\nu}\right) \quad (1053)$$


---

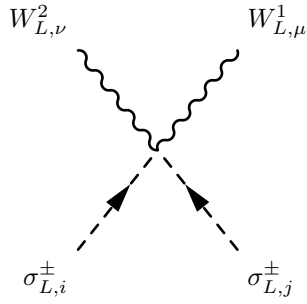

$$g_{A2}g_{B2}^2\sqrt{\frac{gA2^2}{gA2^2+gB2^2}}\frac{1}{\sqrt{gA2^2+gB2^2}}\left(Z_{Ls,i1}^{od,*}Z_{Ls,j4}^{od,*}+Z_{Ls,i2}^{od,*}Z_{Ls,j3}^{od,*}+Z_{Ls,i3}^{od,*}Z_{Ls,j2}^{od,*}+Z_{Ls,i4}^{od,*}Z_{Ls,j1}^{od,*}\right)\left(g_{\mu\nu}\right) \quad (1054)$$


---

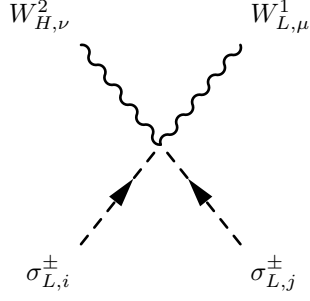

$$-\frac{1}{2}g_{A2}g_{B2}\left(-g_{B2}^2+g_{A2}^2\right)\left(g_{A2}^2+g_{B2}^2\right)^{-1}\left(Z_{Ls,i1}^{od,*}Z_{Ls,j4}^{od,*}+Z_{Ls,i2}^{od,*}Z_{Ls,j3}^{od,*}+Z_{Ls,i3}^{od,*}Z_{Ls,j2}^{od,*}+Z_{Ls,i4}^{od,*}Z_{Ls,j1}^{od,*}\right)\left(g_{\mu\nu}\right) \quad (1055)$$


---

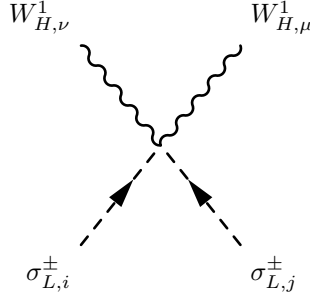

$$ig_{A2}g_{B2}^2\sqrt{\frac{g_{A2}^2}{g_{A2}^2+g_{B2}^2}}\frac{1}{\sqrt{g_{A2}^2+g_{B2}^2}}\left(Z_{Ls,i1}^{od,*}Z_{Ls,j4}^{od,*}+Z_{Ls,i2}^{od,*}Z_{Ls,j3}^{od,*}+Z_{Ls,i3}^{od,*}Z_{Ls,j2}^{od,*}+Z_{Ls,i4}^{od,*}Z_{Ls,j1}^{od,*}\right)\left(g_{\mu\nu}\right) \quad (1056)$$


---

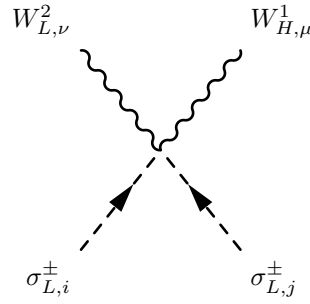

$$-\frac{1}{2}g_{A2}g_{B2}\left(-g_{B2}^2+g_{A2}^2\right)\left(g_{A2}^2+g_{B2}^2\right)^{-1}\left(Z_{Ls,i1}^{od,*}Z_{Ls,j4}^{od,*}+Z_{Ls,i2}^{od,*}Z_{Ls,j3}^{od,*}+Z_{Ls,i3}^{od,*}Z_{Ls,j2}^{od,*}+Z_{Ls,i4}^{od,*}Z_{Ls,j1}^{od,*}\right)\left(g_{\mu\nu}\right) \quad (1057)$$


---

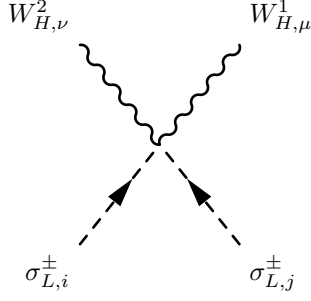

$$-g_{A2}g_{B2}^2\sqrt{\frac{gA2^2}{gA2^2+gB2^2}}\frac{1}{\sqrt{gA2^2+gB2^2}}\left(Z_{Ls,i1}^{od,*}Z_{Ls,j4}^{od,*}+Z_{Ls,i2}^{od,*}Z_{Ls,j3}^{od,*}+Z_{Ls,i3}^{od,*}Z_{Ls,j2}^{od,*}+Z_{Ls,i4}^{od,*}Z_{Ls,j1}^{od,*}\right)\left(g_{\mu\nu}\right) \quad (1058)$$


---

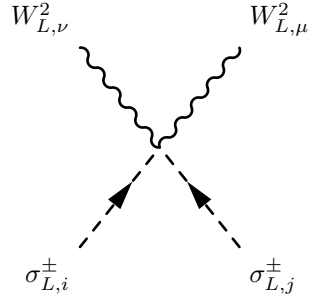

$$ig_{A2}g_{B2}^2\sqrt{\frac{gA2^2}{gA2^2+gB2^2}}\frac{1}{\sqrt{gA2^2+gB2^2}}\left(Z_{Ls,i1}^{od,*}Z_{Ls,j4}^{od,*}+Z_{Ls,i2}^{od,*}Z_{Ls,j3}^{od,*}+Z_{Ls,i3}^{od,*}Z_{Ls,j2}^{od,*}+Z_{Ls,i4}^{od,*}Z_{Ls,j1}^{od,*}\right)\left(g_{\mu\nu}\right) \quad (1059)$$


---

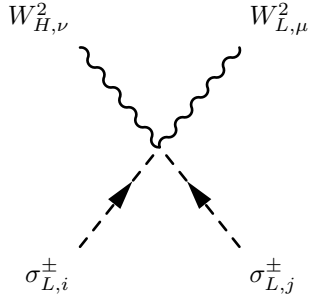

$$-\frac{i}{2}g_{A2}g_{B2}\left(-g_{B2}^2+g_{A2}^2\right)\left(g_{A2}^2+g_{B2}^2\right)^{-1}\left(Z_{Ls,i1}^{od,*}Z_{Ls,j4}^{od,*}+Z_{Ls,i2}^{od,*}Z_{Ls,j3}^{od,*}+Z_{Ls,i3}^{od,*}Z_{Ls,j2}^{od,*}+Z_{Ls,i4}^{od,*}Z_{Ls,j1}^{od,*}\right)\left(g_{\mu\nu}\right) \quad (1060)$$


---

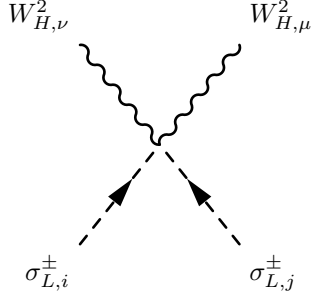

$$-ig_{A2}g_{B2}^2\sqrt{\frac{gA2^2}{gA2^2+gB2^2}}\frac{1}{\sqrt{gA2^2+gB2^2}}\left(Z_{Ls,i1}^{od,*}Z_{Ls,j4}^{od,*}+Z_{Ls,i2}^{od,*}Z_{Ls,j3}^{od,*}+Z_{Ls,i3}^{od,*}Z_{Ls,j2}^{od,*}+Z_{Ls,i4}^{od,*}Z_{Ls,j1}^{od,*}\right)\left(g_{\mu\nu}\right) \quad (1061)$$


---

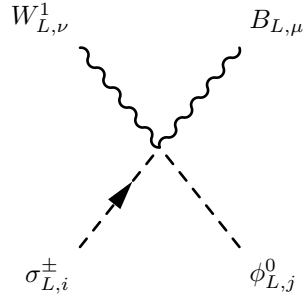

$$\begin{aligned} & -\frac{i}{2}g_{B1}\frac{1}{\sqrt{gA1^2+gB1^2}}\left(-g_{A1}+\sqrt{\frac{gA1^2}{gA1^2+gB1^2}}\sqrt{gA1^2+gB1^2}\right)g_{B2}\frac{1}{\sqrt{gA2^2+gB2^2}}\left(-g_{A2}Z_{Ls,i2}^{od,*}Z_{Ls,j2}^{DR,*}+\sqrt{\frac{gA2^2}{gA2^2+gB2^2}}\sqrt{gA2^2+gB2^2}\right. \\ & +Z_{Ls,i1}^{od,*}\left(-g_{A2}Z_{Ls,j3}^{DR,*}+\sqrt{\frac{gA2^2}{gA2^2+gB2^2}}\sqrt{gA2^2+gB2^2}Z_{Ls,j1}^{DR,*}\right) \\ & +Z_{Ls,i4}^{od,*}\left(-g_{A2}Z_{Ls,j1}^{DR,*}+\sqrt{\frac{gA2^2}{gA2^2+gB2^2}}\sqrt{gA2^2+gB2^2}Z_{Ls,j3}^{DR,*}\right) \\ & \left.+\sqrt{\frac{gA2^2}{gA2^2+gB2^2}}\sqrt{gA2^2+gB2^2}Z_{Ls,i2}^{od,*}Z_{Ls,j4}^{DR,*}-g_{A2}Z_{Ls,i3}^{od,*}Z_{Ls,j4}^{DR,*}\right)\left(g_{\mu\nu}\right) \end{aligned} \quad (1062)$$


---

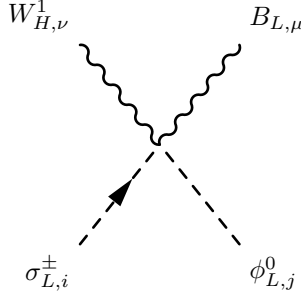

$$\begin{aligned}
& -\frac{i}{2}g_{B1}\frac{1}{\sqrt{gA1^2+gB1^2}}\left(-g_{A1}+\sqrt{\frac{gA1^2}{gA1^2+gB1^2}}\sqrt{gA1^2+gB1^2}\right)\frac{1}{\sqrt{gA2^2+gB2^2}}\left(g_{A2}\sqrt{\frac{gA2^2}{gA2^2+gB2^2}}\sqrt{gA2^2+gB2^2}Z_{Ls,i2}^{od,*}Z_{Ls,j2}^{DR,*}\right. \\
& + Z_{Ls,i4}^{od,*}\left(g_{A2}\sqrt{\frac{gA2^2}{gA2^2+gB2^2}}\sqrt{gA2^2+gB2^2}Z_{Ls,j1}^{DR,*}+g_{B2}^2Z_{Ls,j3}^{DR,*}\right) \\
& + Z_{Ls,i1}^{od,*}\left(g_{A2}\sqrt{\frac{gA2^2}{gA2^2+gB2^2}}\sqrt{gA2^2+gB2^2}Z_{Ls,j3}^{DR,*}+g_{B2}^2Z_{Ls,j1}^{DR,*}\right)+g_{B2}^2Z_{Ls,i2}^{od,*}Z_{Ls,j4}^{DR,*} \\
& \left.+g_{A2}\sqrt{\frac{gA2^2}{gA2^2+gB2^2}}\sqrt{gA2^2+gB2^2}Z_{Ls,i3}^{od,*}Z_{Ls,j4}^{DR,*}\right)(g_{\mu\nu})
\end{aligned} \tag{1063}$$

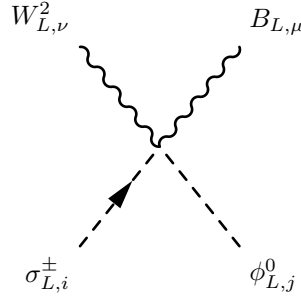

$$\begin{aligned}
& \frac{1}{2}g_{B1}\frac{1}{\sqrt{gA1^2+gB1^2}}\left(-g_{A1}+\sqrt{\frac{gA1^2}{gA1^2+gB1^2}}\sqrt{gA1^2+gB1^2}\right)g_{B2}\frac{1}{\sqrt{gA2^2+gB2^2}}\left(-g_{A2}Z_{Ls,i2}^{od,*}Z_{Ls,j2}^{DR,*}+\sqrt{\frac{gA2^2}{gA2^2+gB2^2}}\sqrt{gA2^2+gB2^2}\right. \\
& + Z_{Ls,i1}^{od,*}\left(-g_{A2}Z_{Ls,j3}^{DR,*}+\sqrt{\frac{gA2^2}{gA2^2+gB2^2}}\sqrt{gA2^2+gB2^2}Z_{Ls,j1}^{DR,*}\right) \\
& + Z_{Ls,i4}^{od,*}\left(-g_{A2}Z_{Ls,j1}^{DR,*}+\sqrt{\frac{gA2^2}{gA2^2+gB2^2}}\sqrt{gA2^2+gB2^2}Z_{Ls,j3}^{DR,*}\right) \\
& \left.+\sqrt{\frac{gA2^2}{gA2^2+gB2^2}}\sqrt{gA2^2+gB2^2}Z_{Ls,i2}^{od,*}Z_{Ls,j4}^{DR,*}-g_{A2}Z_{Ls,i3}^{od,*}Z_{Ls,j4}^{DR,*}\right)(g_{\mu\nu})
\end{aligned} \tag{1064}$$

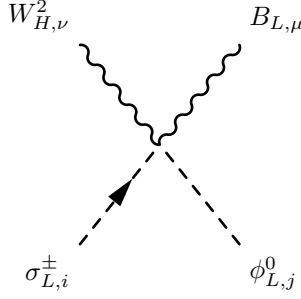

$$\begin{aligned}
& \frac{1}{2} g_{B1} \frac{1}{\sqrt{gA1^2 + gB1^2}} \left( -g_{A1} + \sqrt{\frac{gA1^2}{gA1^2 + gB1^2}} \sqrt{gA1^2 + gB1^2} \right) \frac{1}{\sqrt{gA2^2 + gB2^2}} \left( g_{A2} \sqrt{\frac{gA2^2}{gA2^2 + gB2^2}} \sqrt{gA2^2 + gB2^2} Z_{Ls,i2}^{od,*} Z_{Ls,j2}^{DR,*} + g_{B2} \sqrt{\frac{gA2^2}{gA2^2 + gB2^2}} \sqrt{gA2^2 + gB2^2} Z_{Ls,i2}^{od,*} Z_{Ls,j2}^{DR,*} \right. \\
& + Z_{Ls,i4}^{od,*} \left( g_{A2} \sqrt{\frac{gA2^2}{gA2^2 + gB2^2}} \sqrt{gA2^2 + gB2^2} Z_{Ls,j1}^{DR,*} + g_{B2}^2 Z_{Ls,j3}^{DR,*} \right) \\
& + Z_{Ls,i1}^{od,*} \left( g_{A2} \sqrt{\frac{gA2^2}{gA2^2 + gB2^2}} \sqrt{gA2^2 + gB2^2} Z_{Ls,j3}^{DR,*} + g_{B2}^2 Z_{Ls,j1}^{DR,*} \right) + g_{B2}^2 Z_{Ls,i2}^{od,*} Z_{Ls,j4}^{DR,*} \\
& \left. + g_{A2} \sqrt{\frac{gA2^2}{gA2^2 + gB2^2}} \sqrt{gA2^2 + gB2^2} Z_{Ls,i3}^{od,*} Z_{Ls,j4}^{DR,*} \right) (g_{\mu\nu}) \tag{1065}
\end{aligned}$$

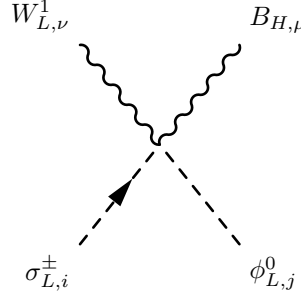

$$\begin{aligned}
& -\frac{i}{2} \frac{1}{\sqrt{gA1^2 + gB1^2}} \left( g_{A1} \sqrt{\frac{gA1^2}{gA1^2 + gB1^2}} \sqrt{gA1^2 + gB1^2} + g_{B1}^2 \right) g_{B2} \frac{1}{\sqrt{gA2^2 + gB2^2}} \left( -g_{A2} Z_{Ls,i2}^{od,*} Z_{Ls,j2}^{DR,*} + \sqrt{\frac{gA2^2}{gA2^2 + gB2^2}} \sqrt{gA2^2 + gB2^2} Z_{Ls,i2}^{od,*} Z_{Ls,j2}^{DR,*} \right. \\
& + Z_{Ls,i1}^{od,*} \left( -g_{A2} Z_{Ls,j3}^{DR,*} + \sqrt{\frac{gA2^2}{gA2^2 + gB2^2}} \sqrt{gA2^2 + gB2^2} Z_{Ls,j1}^{DR,*} \right) \\
& + Z_{Ls,i4}^{od,*} \left( -g_{A2} Z_{Ls,j1}^{DR,*} + \sqrt{\frac{gA2^2}{gA2^2 + gB2^2}} \sqrt{gA2^2 + gB2^2} Z_{Ls,j3}^{DR,*} \right) \\
& \left. + \sqrt{\frac{gA2^2}{gA2^2 + gB2^2}} \sqrt{gA2^2 + gB2^2} Z_{Ls,i2}^{od,*} Z_{Ls,j4}^{DR,*} - g_{A2} Z_{Ls,i3}^{od,*} Z_{Ls,j4}^{DR,*} \right) (g_{\mu\nu}) \tag{1066}
\end{aligned}$$



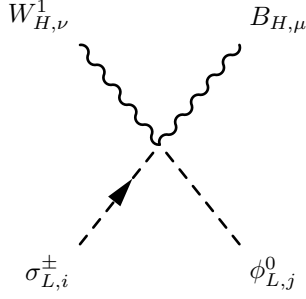

$$\begin{aligned}
& -\frac{i}{2} \frac{1}{\sqrt{gA1^2 + gB1^2}} \left( g_{A1} \sqrt{\frac{gA1^2}{gA1^2 + gB1^2}} \sqrt{gA1^2 + gB1^2} + g_{B1}^2 \right) \frac{1}{\sqrt{gA2^2 + gB2^2}} \left( g_{A2} \sqrt{\frac{gA2^2}{gA2^2 + gB2^2}} \sqrt{gA2^2 + gB2^2} Z_{Ls,i2}^{od,*} Z_{Ls,j2}^{DR,*} + g_{B2}^2 Z_{Ls,i2}^{od,*} Z_{Ls,j2}^{DR,*} \right. \\
& + Z_{Ls,i4}^{od,*} \left( g_{A2} \sqrt{\frac{gA2^2}{gA2^2 + gB2^2}} \sqrt{gA2^2 + gB2^2} Z_{Ls,j1}^{DR,*} + g_{B2}^2 Z_{Ls,j3}^{DR,*} \right) \\
& + Z_{Ls,i1}^{od,*} \left( g_{A2} \sqrt{\frac{gA2^2}{gA2^2 + gB2^2}} \sqrt{gA2^2 + gB2^2} Z_{Ls,j3}^{DR,*} + g_{B2}^2 Z_{Ls,j1}^{DR,*} \right) + g_{B2}^2 Z_{Ls,i2}^{od,*} Z_{Ls,j4}^{DR,*} \\
& \left. + g_{A2} \sqrt{\frac{gA2^2}{gA2^2 + gB2^2}} \sqrt{gA2^2 + gB2^2} Z_{Ls,i3}^{od,*} Z_{Ls,j4}^{DR,*} \right) (g_{\mu\nu}) \tag{1067}
\end{aligned}$$

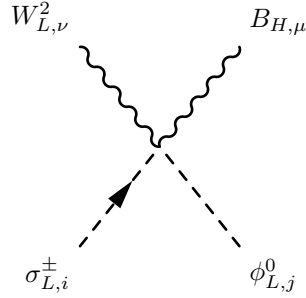

$$\begin{aligned}
& \frac{1}{2} \frac{1}{\sqrt{gA1^2 + gB1^2}} \left( g_{A1} \sqrt{\frac{gA1^2}{gA1^2 + gB1^2}} \sqrt{gA1^2 + gB1^2} + g_{B1}^2 \right) g_{B2} \frac{1}{\sqrt{gA2^2 + gB2^2}} \left( -g_{A2} Z_{Ls,i2}^{od,*} Z_{Ls,j2}^{DR,*} + \sqrt{\frac{gA2^2}{gA2^2 + gB2^2}} \sqrt{gA2^2 + gB2^2} Z_{Ls,i2}^{od,*} Z_{Ls,j2}^{DR,*} \right. \\
& + Z_{Ls,i1}^{od,*} \left( -g_{A2} Z_{Ls,j3}^{DR,*} + \sqrt{\frac{gA2^2}{gA2^2 + gB2^2}} \sqrt{gA2^2 + gB2^2} Z_{Ls,j1}^{DR,*} \right) \\
& + Z_{Ls,i4}^{od,*} \left( -g_{A2} Z_{Ls,j1}^{DR,*} + \sqrt{\frac{gA2^2}{gA2^2 + gB2^2}} \sqrt{gA2^2 + gB2^2} Z_{Ls,j3}^{DR,*} \right) \\
& \left. + \sqrt{\frac{gA2^2}{gA2^2 + gB2^2}} \sqrt{gA2^2 + gB2^2} Z_{Ls,i2}^{od,*} Z_{Ls,j4}^{DR,*} - g_{A2} Z_{Ls,i3}^{od,*} Z_{Ls,j4}^{DR,*} \right) (g_{\mu\nu}) \tag{1068}
\end{aligned}$$

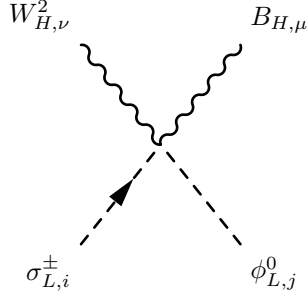

$$\begin{aligned}
& \frac{1}{2} \frac{1}{\sqrt{gA1^2 + gB1^2}} \left( g_{A1} \sqrt{\frac{gA1^2}{gA1^2 + gB1^2}} \sqrt{gA1^2 + gB1^2} + g_{B1}^2 \right) \frac{1}{\sqrt{gA2^2 + gB2^2}} \left( g_{A2} \sqrt{\frac{gA2^2}{gA2^2 + gB2^2}} \sqrt{gA2^2 + gB2^2} Z_{Ls,i2}^{od,*} Z_{Ls,j2}^{DR,*} + g_{B2}^2 \right. \\
& + Z_{Ls,i4}^{od,*} \left( g_{A2} \sqrt{\frac{gA2^2}{gA2^2 + gB2^2}} \sqrt{gA2^2 + gB2^2} Z_{Ls,j1}^{DR,*} + g_{B2}^2 Z_{Ls,j3}^{DR,*} \right) \\
& + Z_{Ls,i1}^{od,*} \left( g_{A2} \sqrt{\frac{gA2^2}{gA2^2 + gB2^2}} \sqrt{gA2^2 + gB2^2} Z_{Ls,j3}^{DR,*} + g_{B2}^2 Z_{Ls,j1}^{DR,*} \right) + g_{B2}^2 Z_{Ls,i2}^{od,*} Z_{Ls,j4}^{DR,*} \\
& \left. + g_{A2} \sqrt{\frac{gA2^2}{gA2^2 + gB2^2}} \sqrt{gA2^2 + gB2^2} Z_{Ls,i3}^{od,*} Z_{Ls,j4}^{DR,*} \right) (g_{\mu\nu}) \tag{1069}
\end{aligned}$$


---

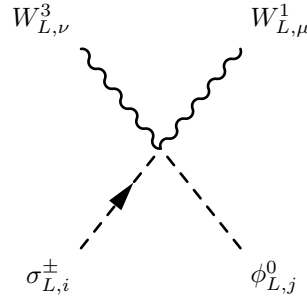

$$\begin{aligned}
& - \frac{i}{2} g_{A2} g_{B2}^2 \sqrt{\frac{gA2^2}{gA2^2 + gB2^2}} \frac{1}{\sqrt{gA2^2 + gB2^2}} \left( Z_{Ls,i1}^{od,*} \left( -Z_{Ls,j3}^{DR,*} + Z_{Ls,j1}^{DR,*} \right) + \left( Z_{Ls,i2}^{od,*} + Z_{Ls,i3}^{od,*} \right) \left( -Z_{Ls,j4}^{DR,*} + Z_{Ls,j2}^{DR,*} \right) + Z_{Ls,i4}^{od,*} \left( -Z_{Ls,j3}^{DR,*} \right. \right. \\
& \left. \left. + Z_{Ls,j1}^{DR,*} \right) \right) \tag{1070}
\end{aligned}$$


---

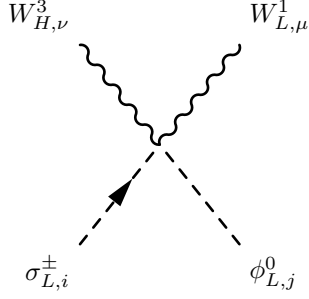

$$\begin{aligned} & \frac{i}{2} g_{A2} g_{B2} \left( g_{A2}^2 + g_{B2}^2 \right)^{-1} \left( -g_{B2}^2 Z_{Ls,i2}^{od,*} Z_{Ls,j2}^{DR,*} + g_{A2}^2 Z_{Ls,i3}^{od,*} Z_{Ls,j2}^{DR,*} - Z_{Ls,i4}^{od,*} \left( g_{A2}^2 Z_{Ls,j3}^{DR,*} + g_{B2}^2 Z_{Ls,j1}^{DR,*} \right) \right. \\ & \left. + Z_{Ls,i1}^{od,*} \left( g_{A2}^2 Z_{Ls,j1}^{DR,*} + g_{B2}^2 Z_{Ls,j3}^{DR,*} \right) - g_{A2}^2 Z_{Ls,i2}^{od,*} Z_{Ls,j4}^{DR,*} + g_{B2}^2 Z_{Ls,i3}^{od,*} Z_{Ls,j4}^{DR,*} \right) (g_{\mu\nu}) \end{aligned} \quad (1071)$$


---

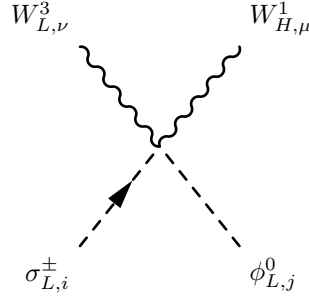

$$\begin{aligned} & \frac{i}{2} g_{A2} g_{B2} \left( g_{A2}^2 + g_{B2}^2 \right)^{-1} \left( g_{A2}^2 Z_{Ls,i2}^{od,*} Z_{Ls,j2}^{DR,*} - g_{B2}^2 Z_{Ls,i3}^{od,*} Z_{Ls,j2}^{DR,*} - Z_{Ls,i1}^{od,*} \left( g_{A2}^2 Z_{Ls,j3}^{DR,*} + g_{B2}^2 Z_{Ls,j1}^{DR,*} \right) \right. \\ & \left. + Z_{Ls,i4}^{od,*} \left( g_{A2}^2 Z_{Ls,j1}^{DR,*} + g_{B2}^2 Z_{Ls,j3}^{DR,*} \right) + g_{B2}^2 Z_{Ls,i2}^{od,*} Z_{Ls,j4}^{DR,*} - g_{A2}^2 Z_{Ls,i3}^{od,*} Z_{Ls,j4}^{DR,*} \right) (g_{\mu\nu}) \end{aligned} \quad (1072)$$


---

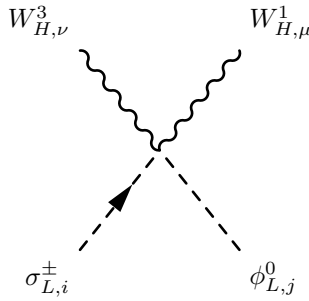

$$\frac{i}{2} g_{A2} g_{B2}^2 \sqrt{\frac{g_{A2}^2}{g_{A2}^2 + g_{B2}^2}} \frac{1}{\sqrt{g_{A2}^2 + g_{B2}^2}} \left( Z_{Ls,i1}^{od,*} \left( -Z_{Ls,j3}^{DR,*} + Z_{Ls,j1}^{DR,*} \right) + \left( Z_{Ls,i2}^{od,*} + Z_{Ls,i3}^{od,*} \right) \left( -Z_{Ls,j4}^{DR,*} + Z_{Ls,j2}^{DR,*} \right) + Z_{Ls,i4}^{od,*} \left( -Z_{Ls,j3}^{DR,*} + \right. \right. \\ \left. \left. + Z_{Ls,j1}^{DR,*} \right) \right) (g_{\mu\nu}) \quad (1073)$$


---

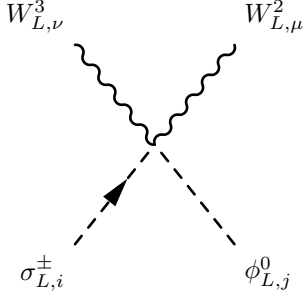

$$\frac{1}{2}g_{A2}g_{B2}^2\sqrt{\frac{g_{A2}^2}{g_{A2}^2+g_{B2}^2}}\frac{1}{\sqrt{g_{A2}^2+g_{B2}^2}}\left(Z_{Ls,i1}^{od,*}\left(-Z_{Ls,j3}^{DR,*}+Z_{Ls,j1}^{DR,*}\right)+\left(Z_{Ls,i2}^{od,*}+Z_{Ls,i3}^{od,*}\right)\left(-Z_{Ls,j4}^{DR,*}+Z_{Ls,j2}^{DR,*}\right)+Z_{Ls,i4}^{od,*}\left(-Z_{Ls,j3}^{DR,*}+Z_{Ls,j1}^{DR,*}\right)\right) \quad (1074)$$


---

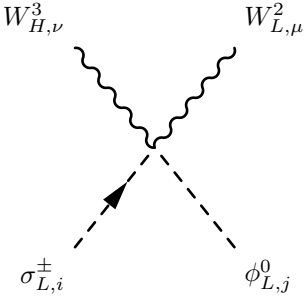

$$\frac{1}{2}g_{A2}g_{B2}\left(g_{A2}^2+g_{B2}^2\right)^{-1}\left(g_{B2}^2Z_{Ls,i2}^{od,*}Z_{Ls,j2}^{DR,*}-g_{A2}^2Z_{Ls,i3}^{od,*}Z_{Ls,j2}^{DR,*}+Z_{Ls,i4}^{od,*}\left(g_{A2}^2Z_{Ls,j3}^{DR,*}+g_{B2}^2Z_{Ls,j1}^{DR,*}\right)-Z_{Ls,i1}^{od,*}\left(g_{A2}^2Z_{Ls,j1}^{DR,*}+g_{B2}^2Z_{Ls,j3}^{DR,*}\right)+g_{A2}^2Z_{Ls,i2}^{od,*}Z_{Ls,j4}^{DR,*}-g_{B2}^2Z_{Ls,i3}^{od,*}Z_{Ls,j4}^{DR,*}\right)\left(g_{\mu\nu}\right) \quad (1075)$$


---

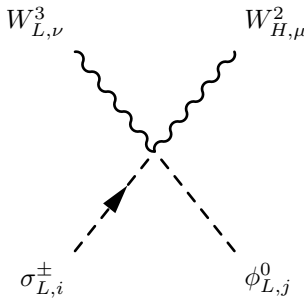

$$\frac{1}{2}g_{A2}g_{B2}\left(g_{A2}^2+g_{B2}^2\right)^{-1}\left(-g_{A2}^2Z_{Ls,i2}^{od,*}Z_{Ls,j2}^{DR,*}+g_{B2}^2Z_{Ls,i3}^{od,*}Z_{Ls,j2}^{DR,*}+Z_{Ls,i1}^{od,*}\left(g_{A2}^2Z_{Ls,j3}^{DR,*}+g_{B2}^2Z_{Ls,j1}^{DR,*}\right)-Z_{Ls,i4}^{od,*}\left(g_{A2}^2Z_{Ls,j1}^{DR,*}+g_{B2}^2Z_{Ls,j3}^{DR,*}\right)-g_{B2}^2Z_{Ls,i2}^{od,*}Z_{Ls,j4}^{DR,*}+g_{A2}^2Z_{Ls,i3}^{od,*}Z_{Ls,j4}^{DR,*}\right)\left(g_{\mu\nu}\right) \quad (1076)$$


---

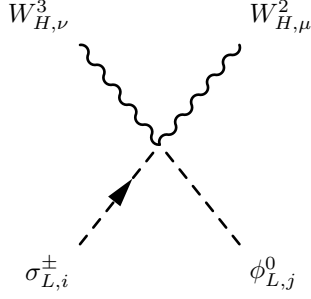

$$-\frac{1}{2}g_{A2}g_{B2}^2\sqrt{\frac{gA2^2}{gA2^2+gB2^2}}\frac{1}{\sqrt{gA2^2+gB2^2}}\left(Z_{Ls,i1}^{od,*}\left(-Z_{Ls,j3}^{DR,*}+Z_{Ls,j1}^{DR,*}\right)+\left(Z_{Ls,i2}^{od,*}+Z_{Ls,i3}^{od,*}\right)\left(-Z_{Ls,j4}^{DR,*}+Z_{Ls,j2}^{DR,*}\right)+Z_{Ls,i4}^{od,*}\left(-Z_{Ls,j3}^{DR,*}\right.\right. \\ \left.\left. (1077) \right.\right.$$


---

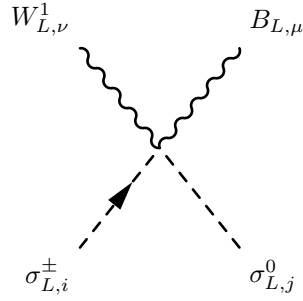

$$-\frac{1}{2}g_{B1}\frac{1}{\sqrt{gA1^2+gB1^2}}\left(-g_{A1}+\sqrt{\frac{gA1^2}{gA1^2+gB1^2}}\sqrt{gA1^2+gB1^2}\right)g_{B2}\frac{1}{\sqrt{gA2^2+gB2^2}}\left(-g_{A2}Z_{Ls,i2}^{od,*}Z_{Ls,j2}^{Di,*}-\sqrt{\frac{gA2^2}{gA2^2+gB2^2}}\sqrt{gA2^2+gB2^2}\right. \\ +Z_{Ls,i1}^{od,*}\left(-g_{A2}Z_{Ls,j3}^{Di,*}+\sqrt{\frac{gA2^2}{gA2^2+gB2^2}}\sqrt{gA2^2+gB2^2}Z_{Ls,j1}^{Di,*}\right) \\ +Z_{Ls,i4}^{od,*}\left(g_{A2}Z_{Ls,j1}^{Di,*}-\sqrt{\frac{gA2^2}{gA2^2+gB2^2}}\sqrt{gA2^2+gB2^2}Z_{Ls,j3}^{Di,*}\right) \\ \left. +\sqrt{\frac{gA2^2}{gA2^2+gB2^2}}\sqrt{gA2^2+gB2^2}Z_{Ls,i2}^{od,*}Z_{Ls,j4}^{Di,*}+g_{A2}Z_{Ls,i3}^{od,*}Z_{Ls,j4}^{Di,*}\right)\left(g_{\mu\nu}\right) \\ (1078)$$


---

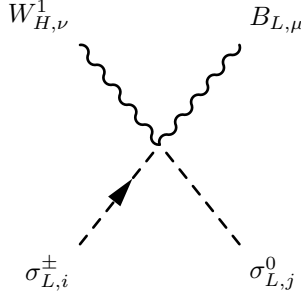

$$\begin{aligned}
& -\frac{1}{2}g_{B1}\frac{1}{\sqrt{gA1^2+gB1^2}}\left(-g_{A1}+\sqrt{\frac{gA1^2}{gA1^2+gB1^2}}\sqrt{gA1^2+gB1^2}\right)\frac{1}{\sqrt{gA2^2+gB2^2}}\left(g_{A2}\sqrt{\frac{gA2^2}{gA2^2+gB2^2}}\sqrt{gA2^2+gB2^2}Z_{Ls,i2}^{od,*}Z_{Ls,j2}^{Di,*}\right. \\
& -Z_{Ls,i4}^{od,*}\left(g_{A2}\sqrt{\frac{gA2^2}{gA2^2+gB2^2}}\sqrt{gA2^2+gB2^2}Z_{Ls,j1}^{Di,*}+g_{B2}^2Z_{Ls,j3}^{Di,*}\right) \\
& +Z_{Ls,i1}^{od,*}\left(g_{A2}\sqrt{\frac{gA2^2}{gA2^2+gB2^2}}\sqrt{gA2^2+gB2^2}Z_{Ls,j3}^{Di,*}+g_{B2}^2Z_{Ls,j1}^{Di,*}\right)+g_{B2}^2Z_{Ls,i2}^{od,*}Z_{Ls,j4}^{Di,*} \\
& \left.-g_{A2}\sqrt{\frac{gA2^2}{gA2^2+gB2^2}}\sqrt{gA2^2+gB2^2}Z_{Ls,i3}^{od,*}Z_{Ls,j4}^{Di,*}\right)(g_{\mu\nu})
\end{aligned} \tag{1079}$$

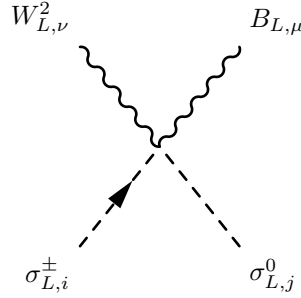

$$\begin{aligned}
& -\frac{i}{2}g_{B1}\frac{1}{\sqrt{gA1^2+gB1^2}}\left(-g_{A1}+\sqrt{\frac{gA1^2}{gA1^2+gB1^2}}\sqrt{gA1^2+gB1^2}\right)g_{B2}\frac{1}{\sqrt{gA2^2+gB2^2}}\left(-g_{A2}Z_{Ls,i2}^{od,*}Z_{Ls,j2}^{Di,*}-\sqrt{\frac{gA2^2}{gA2^2+gB2^2}}\sqrt{gA2^2+gB2^2}\right. \\
& +Z_{Ls,i1}^{od,*}\left(-g_{A2}Z_{Ls,j3}^{Di,*}+\sqrt{\frac{gA2^2}{gA2^2+gB2^2}}\sqrt{gA2^2+gB2^2}Z_{Ls,j1}^{Di,*}\right) \\
& +Z_{Ls,i4}^{od,*}\left(g_{A2}Z_{Ls,j1}^{Di,*}-\sqrt{\frac{gA2^2}{gA2^2+gB2^2}}\sqrt{gA2^2+gB2^2}Z_{Ls,j3}^{Di,*}\right) \\
& \left.+\sqrt{\frac{gA2^2}{gA2^2+gB2^2}}\sqrt{gA2^2+gB2^2}Z_{Ls,i2}^{od,*}Z_{Ls,j4}^{Di,*}+g_{A2}Z_{Ls,i3}^{od,*}Z_{Ls,j4}^{Di,*}\right)(g_{\mu\nu})
\end{aligned} \tag{1080}$$

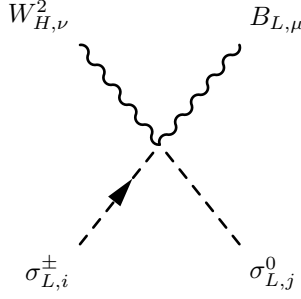

$$\begin{aligned}
& -\frac{i}{2}g_{B1}\frac{1}{\sqrt{gA1^2+gB1^2}}\left(-g_{A1}+\sqrt{\frac{gA1^2}{gA1^2+gB1^2}}\sqrt{gA1^2+gB1^2}\right)\frac{1}{\sqrt{gA2^2+gB2^2}}\left(g_{A2}\sqrt{\frac{gA2^2}{gA2^2+gB2^2}}\sqrt{gA2^2+gB2^2}Z_{Ls,i2}^{od,*}Z_{Ls,j2}^{Di,*}\right. \\
& -Z_{Ls,i4}^{od,*}\left(g_{A2}\sqrt{\frac{gA2^2}{gA2^2+gB2^2}}\sqrt{gA2^2+gB2^2}Z_{Ls,j1}^{Di,*}+g_{B2}^2Z_{Ls,j3}^{Di,*}\right) \\
& +Z_{Ls,i1}^{od,*}\left(g_{A2}\sqrt{\frac{gA2^2}{gA2^2+gB2^2}}\sqrt{gA2^2+gB2^2}Z_{Ls,j3}^{Di,*}+g_{B2}^2Z_{Ls,j1}^{Di,*}\right)+g_{B2}^2Z_{Ls,i2}^{od,*}Z_{Ls,j4}^{Di,*} \\
& \left.-g_{A2}\sqrt{\frac{gA2^2}{gA2^2+gB2^2}}\sqrt{gA2^2+gB2^2}Z_{Ls,i3}^{od,*}Z_{Ls,j4}^{Di,*}\right)(g_{\mu\nu})
\end{aligned} \tag{1081}$$

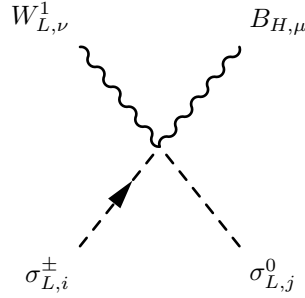

$$\begin{aligned}
& -\frac{1}{2}\frac{1}{\sqrt{gA1^2+gB1^2}}\left(g_{A1}\sqrt{\frac{gA1^2}{gA1^2+gB1^2}}\sqrt{gA1^2+gB1^2}+g_{B1}^2\right)g_{B2}\frac{1}{\sqrt{gA2^2+gB2^2}}\left(-g_{A2}Z_{Ls,i2}^{od,*}Z_{Ls,j2}^{Di,*}-\sqrt{\frac{gA2^2}{gA2^2+gB2^2}}\sqrt{gA2^2+gB2^2}\right. \\
& +Z_{Ls,i1}^{od,*}\left(-g_{A2}Z_{Ls,j3}^{Di,*}+\sqrt{\frac{gA2^2}{gA2^2+gB2^2}}\sqrt{gA2^2+gB2^2}Z_{Ls,j1}^{Di,*}\right) \\
& +Z_{Ls,i4}^{od,*}\left(g_{A2}Z_{Ls,j1}^{Di,*}-\sqrt{\frac{gA2^2}{gA2^2+gB2^2}}\sqrt{gA2^2+gB2^2}Z_{Ls,j3}^{Di,*}\right) \\
& \left.+\sqrt{\frac{gA2^2}{gA2^2+gB2^2}}\sqrt{gA2^2+gB2^2}Z_{Ls,i2}^{od,*}Z_{Ls,j4}^{Di,*}+g_{A2}Z_{Ls,i3}^{od,*}Z_{Ls,j4}^{Di,*}\right)(g_{\mu\nu})
\end{aligned} \tag{1082}$$

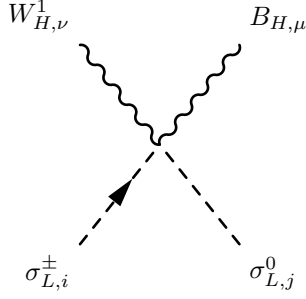

$$\begin{aligned}
& -\frac{1}{2} \frac{1}{\sqrt{gA1^2 + gB1^2}} \left( g_{A1} \sqrt{\frac{gA1^2}{gA1^2 + gB1^2}} \sqrt{gA1^2 + gB1^2} + g_{B1}^2 \right) \frac{1}{\sqrt{gA2^2 + gB2^2}} \left( g_{A2} \sqrt{\frac{gA2^2}{gA2^2 + gB2^2}} \sqrt{gA2^2 + gB2^2} Z_{Ls,i2}^{od,*} Z_{Ls,j2}^{Di,*} - g_{B2}^2 Z_{Ls,i2}^{od,*} Z_{Ls,j2}^{Di,*} \right) \\
& - Z_{Ls,i4}^{od,*} \left( g_{A2} \sqrt{\frac{gA2^2}{gA2^2 + gB2^2}} \sqrt{gA2^2 + gB2^2} Z_{Ls,j1}^{Di,*} + g_{B2}^2 Z_{Ls,j3}^{Di,*} \right) \\
& + Z_{Ls,i1}^{od,*} \left( g_{A2} \sqrt{\frac{gA2^2}{gA2^2 + gB2^2}} \sqrt{gA2^2 + gB2^2} Z_{Ls,j3}^{Di,*} + g_{B2}^2 Z_{Ls,j1}^{Di,*} \right) + g_{B2}^2 Z_{Ls,i2}^{od,*} Z_{Ls,j4}^{Di,*} \\
& - g_{A2} \sqrt{\frac{gA2^2}{gA2^2 + gB2^2}} \sqrt{gA2^2 + gB2^2} Z_{Ls,i3}^{od,*} Z_{Ls,j4}^{Di,*} \Big) (g_{\mu\nu}) \tag{1083}
\end{aligned}$$

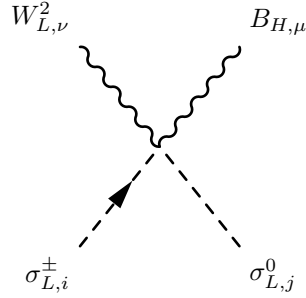

$$\begin{aligned}
& -\frac{i}{2} \frac{1}{\sqrt{gA1^2 + gB1^2}} \left( g_{A1} \sqrt{\frac{gA1^2}{gA1^2 + gB1^2}} \sqrt{gA1^2 + gB1^2} + g_{B1}^2 \right) g_{B2} \frac{1}{\sqrt{gA2^2 + gB2^2}} \left( -g_{A2} Z_{Ls,i2}^{od,*} Z_{Ls,j2}^{Di,*} - \sqrt{\frac{gA2^2}{gA2^2 + gB2^2}} \sqrt{gA2^2 + gB2^2} Z_{Ls,i2}^{od,*} Z_{Ls,j2}^{Di,*} \right) \\
& + Z_{Ls,i1}^{od,*} \left( -g_{A2} Z_{Ls,j3}^{Di,*} + \sqrt{\frac{gA2^2}{gA2^2 + gB2^2}} \sqrt{gA2^2 + gB2^2} Z_{Ls,j1}^{Di,*} \right) \\
& + Z_{Ls,i4}^{od,*} \left( g_{A2} Z_{Ls,j1}^{Di,*} - \sqrt{\frac{gA2^2}{gA2^2 + gB2^2}} \sqrt{gA2^2 + gB2^2} Z_{Ls,j3}^{Di,*} \right) \\
& + \sqrt{\frac{gA2^2}{gA2^2 + gB2^2}} \sqrt{gA2^2 + gB2^2} Z_{Ls,i2}^{od,*} Z_{Ls,j4}^{Di,*} + g_{A2} Z_{Ls,i3}^{od,*} Z_{Ls,j4}^{Di,*} \Big) (g_{\mu\nu}) \tag{1084}
\end{aligned}$$



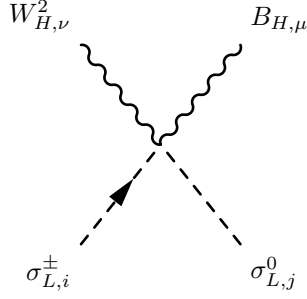

$$\begin{aligned}
& -\frac{i}{2} \frac{1}{\sqrt{gA1^2 + gB1^2}} \left( g_{A1} \sqrt{\frac{gA1^2}{gA1^2 + gB1^2}} \sqrt{gA1^2 + gB1^2} + g_{B1}^2 \right) \frac{1}{\sqrt{gA2^2 + gB2^2}} \left( g_{A2} \sqrt{\frac{gA2^2}{gA2^2 + gB2^2}} \sqrt{gA2^2 + gB2^2} Z_{L,i2}^{od,*} Z_{L,j2}^{Di,*} - g_{B2}^2 Z_{L,i2}^{od,*} Z_{L,j2}^{Di,*} \right) \\
& - Z_{L,i4}^{od,*} \left( g_{A2} \sqrt{\frac{gA2^2}{gA2^2 + gB2^2}} \sqrt{gA2^2 + gB2^2} Z_{L,j1}^{Di,*} + g_{B2}^2 Z_{L,j3}^{Di,*} \right) \\
& + Z_{L,i1}^{od,*} \left( g_{A2} \sqrt{\frac{gA2^2}{gA2^2 + gB2^2}} \sqrt{gA2^2 + gB2^2} Z_{L,j3}^{Di,*} + g_{B2}^2 Z_{L,j1}^{Di,*} \right) + g_{B2}^2 Z_{L,i2}^{od,*} Z_{L,j4}^{Di,*} \\
& - g_{A2} \sqrt{\frac{gA2^2}{gA2^2 + gB2^2}} \sqrt{gA2^2 + gB2^2} Z_{L,i3}^{od,*} Z_{L,j4}^{Di,*} \left( g_{\mu\nu} \right)
\end{aligned} \tag{1085}$$

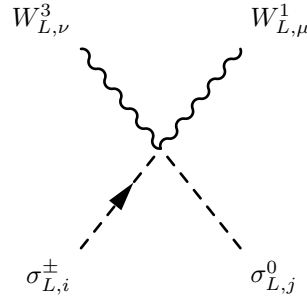

$$\begin{aligned}
& \frac{1}{2} g_{A2} g_{B2}^2 \sqrt{\frac{gA2^2}{gA2^2 + gB2^2}} \frac{1}{\sqrt{gA2^2 + gB2^2}} \left( Z_{L,i1}^{od,*} \left( -Z_{L,j1}^{Di,*} + Z_{L,j3}^{Di,*} \right) - \left( -Z_{L,i3}^{od,*} + Z_{L,i2}^{od,*} \right) \left( -Z_{L,j4}^{Di,*} + Z_{L,j2}^{Di,*} \right) + Z_{L,i4}^{od,*} \left( -Z_{L,j3}^{Di,*} \right) \right)
\end{aligned} \tag{1086}$$

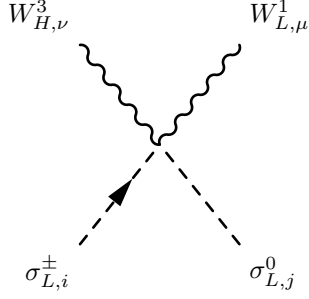

$$\begin{aligned} & \frac{1}{2} g_{A2} g_{B2} (g_{A2}^2 + g_{B2}^2)^{-1} \left( -g_{B2}^2 Z_{Ls,i2}^{od,*} Z_{Ls,j2}^{Di,*} - g_{A2}^2 Z_{Ls,i3}^{od,*} Z_{Ls,j2}^{Di,*} + Z_{Ls,i4}^{od,*} (g_{A2}^2 Z_{Ls,j3}^{Di,*} + g_{B2}^2 Z_{Ls,j1}^{Di,*}) \right. \\ & \left. + Z_{Ls,i1}^{od,*} (g_{A2}^2 Z_{Ls,j1}^{Di,*} + g_{B2}^2 Z_{Ls,j3}^{Di,*}) - g_{A2}^2 Z_{Ls,i2}^{od,*} Z_{Ls,j4}^{Di,*} - g_{B2}^2 Z_{Ls,i3}^{od,*} Z_{Ls,j4}^{Di,*} \right) (g_{\mu\nu}) \end{aligned} \quad (1087)$$


---

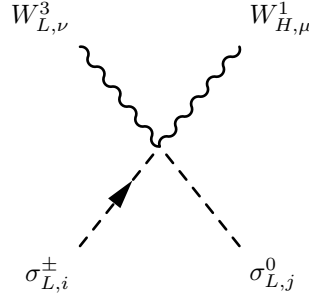

$$\begin{aligned} & \frac{1}{2} g_{A2} g_{B2} (g_{A2}^2 + g_{B2}^2)^{-1} \left( g_{A2}^2 Z_{Ls,i2}^{od,*} Z_{Ls,j2}^{Di,*} + g_{B2}^2 Z_{Ls,i3}^{od,*} Z_{Ls,j2}^{Di,*} - Z_{Ls,i1}^{od,*} (g_{A2}^2 Z_{Ls,j3}^{Di,*} + g_{B2}^2 Z_{Ls,j1}^{Di,*}) \right. \\ & \left. - Z_{Ls,i4}^{od,*} (g_{A2}^2 Z_{Ls,j1}^{Di,*} + g_{B2}^2 Z_{Ls,j3}^{Di,*}) + g_{B2}^2 Z_{Ls,i2}^{od,*} Z_{Ls,j4}^{Di,*} + g_{A2}^2 Z_{Ls,i3}^{od,*} Z_{Ls,j4}^{Di,*} \right) (g_{\mu\nu}) \end{aligned} \quad (1088)$$


---

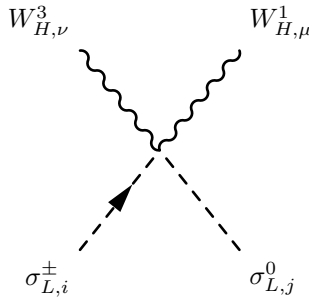

$$\begin{aligned} & \frac{1}{2} g_{A2} g_{B2}^2 \sqrt{\frac{g_{A2}^2}{g_{A2}^2 + g_{B2}^2}} \frac{1}{\sqrt{g_{A2}^2 + g_{B2}^2}} \left( Z_{Ls,i1}^{od,*} (-Z_{Ls,j3}^{Di,*} + Z_{Ls,j1}^{Di,*}) + (-Z_{Ls,i3}^{od,*} + Z_{Ls,i2}^{od,*}) (-Z_{Ls,j4}^{Di,*} + Z_{Ls,j2}^{Di,*}) + Z_{Ls,i4}^{od,*} (-Z_{Ls,j1}^{Di,*} \right. \\ & \left. + Z_{Ls,j3}^{Di,*}) \right) (g_{\mu\nu}) \end{aligned} \quad (1089)$$


---

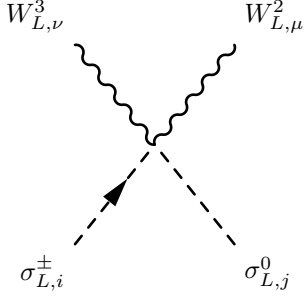

$$-\frac{i}{2}g_{A2}g_{B2}^2\sqrt{\frac{g_{A2}^2}{g_{A2}^2+g_{B2}^2}}\frac{1}{\sqrt{g_{A2}^2+g_{B2}^2}}\left(Z_{Ls,i1}^{od,*}\left(-Z_{Ls,j3}^{Di,*}+Z_{Ls,j1}^{Di,*}\right)+\left(-Z_{Ls,i3}^{od,*}+Z_{Ls,i2}^{od,*}\right)\left(-Z_{Ls,j4}^{Di,*}+Z_{Ls,j2}^{Di,*}\right)+Z_{Ls,i4}^{od,*}\left(-Z_{Ls,j1}^{Di,*}+Z_{Ls,j3}^{Di,*}\right)\right) \quad (1090)$$


---

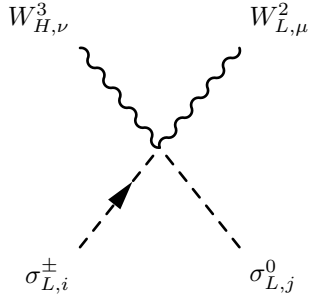

$$\frac{i}{2}g_{A2}g_{B2}\left(g_{A2}^2+g_{B2}^2\right)^{-1}\left(-g_{B2}^2Z_{Ls,i2}^{od,*}Z_{Ls,j2}^{Di,*}-g_{A2}^2Z_{Ls,i3}^{od,*}Z_{Ls,j2}^{Di,*}+Z_{Ls,i4}^{od,*}\left(g_{A2}^2Z_{Ls,j3}^{Di,*}+g_{B2}^2Z_{Ls,j1}^{Di,*}\right)+Z_{Ls,i1}^{od,*}\left(g_{A2}^2Z_{Ls,j1}^{Di,*}+g_{B2}^2Z_{Ls,j3}^{Di,*}\right)-g_{A2}^2Z_{Ls,i2}^{od,*}Z_{Ls,j4}^{Di,*}-g_{B2}^2Z_{Ls,i3}^{od,*}Z_{Ls,j4}^{Di,*}\right)\left(g_{\mu\nu}\right) \quad (1091)$$


---

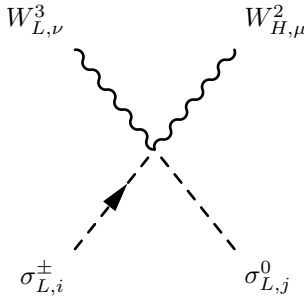

$$\frac{i}{2}g_{A2}g_{B2}\left(g_{A2}^2+g_{B2}^2\right)^{-1}\left(g_{A2}^2Z_{Ls,i2}^{od,*}Z_{Ls,j2}^{Di,*}+g_{B2}^2Z_{Ls,i3}^{od,*}Z_{Ls,j2}^{Di,*}-Z_{Ls,i1}^{od,*}\left(g_{A2}^2Z_{Ls,j3}^{Di,*}+g_{B2}^2Z_{Ls,j1}^{Di,*}\right)-Z_{Ls,i4}^{od,*}\left(g_{A2}^2Z_{Ls,j1}^{Di,*}+g_{B2}^2Z_{Ls,j3}^{Di,*}\right)+g_{B2}^2Z_{Ls,i2}^{od,*}Z_{Ls,j4}^{Di,*}+g_{A2}^2Z_{Ls,i3}^{od,*}Z_{Ls,j4}^{Di,*}\right)\left(g_{\mu\nu}\right) \quad (1092)$$


---

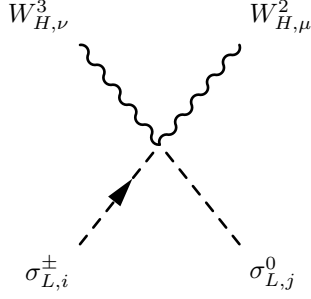

$$\frac{i}{2}g_{A2}g_{B2}^2\sqrt{\frac{gA2^2}{gA2^2+gB2^2}}\frac{1}{\sqrt{gA2^2+gB2^2}}\left(Z_{Ls,i1}^{od,*}\left(-Z_{Ls,j3}^{Di,*}+Z_{Ls,j1}^{Di,*}\right)+\left(-Z_{Ls,i3}^{od,*}+Z_{Ls,i2}^{od,*}\right)\left(-Z_{Ls,j4}^{Di,*}+Z_{Ls,j2}^{Di,*}\right)+Z_{Ls,i4}^{od,*}\left(-Z_{Ls,j1}^{Di,*}\right.\right. \\ \left.\left.\right)\right) \quad (1093)$$


---

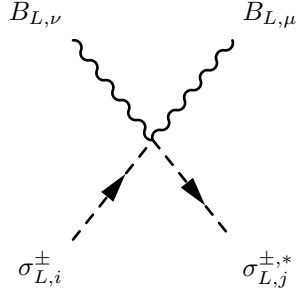

$$-ig_{A1}g_{B1}^2\frac{1}{\left(gA1^2+gB1^2\right)^{3/2}}\left(g_{A1}^2\sqrt{\frac{gA1^2}{gA1^2+gB1^2}}-g_{A1}\sqrt{gA1^2+gB1^2}+g_{B1}^2\sqrt{\frac{gA1^2}{gA1^2+gB1^2}}\right)\left(Z_{Ls,i1}^{od,*}Z_{Ls,j1}^{od}+Z_{Ls,i2}^{od,*}Z_{Ls,j2}^{od}+Z_{Ls,i3}^{od,*}Z_{Ls,j3}^{od}+Z_{Ls,i4}^{od,*}Z_{Ls,j4}^{od}\right) \\ \left.\right) \quad (1094)$$


---

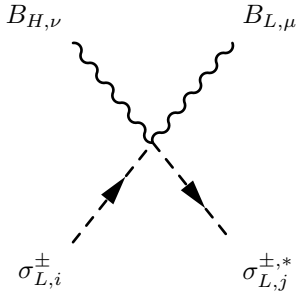

$$\frac{i}{2}g_{B1}\left(-g_{A1}^2+g_{B1}^2\right)\frac{1}{\left(gA1^2+gB1^2\right)^{3/2}}\left(g_{A1}^2\sqrt{\frac{gA1^2}{gA1^2+gB1^2}}-g_{A1}\sqrt{gA1^2+gB1^2}+g_{B1}^2\sqrt{\frac{gA1^2}{gA1^2+gB1^2}}\right)\left(Z_{Ls,i1}^{od,*}Z_{Ls,j1}^{od}+Z_{Ls,i2}^{od,*}Z_{Ls,j2}^{od}+Z_{Ls,i3}^{od,*}Z_{Ls,j3}^{od}+Z_{Ls,i4}^{od,*}Z_{Ls,j4}^{od}\right) \\ \left.\right) \quad (1095)$$

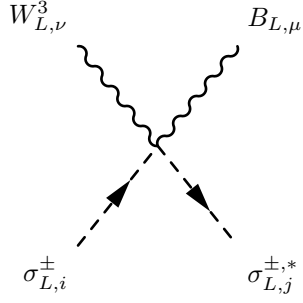

$$\frac{i}{2}g_{B1}\frac{1}{\sqrt{gA1^2+gB1^2}}\Big(-g_{A1}+\sqrt{\frac{gA1^2}{gA1^2+gB1^2}}\sqrt{gA1^2+gB1^2}\Big)g_{B2}\frac{1}{\sqrt{gA2^2+gB2^2}}\Big(\sqrt{\frac{gA2^2}{gA2^2+gB2^2}}\sqrt{gA2^2+gB2^2}+g_{A2}\Big)\Big(Z_{Ls,i1}^{od,*}Z_{Ls,i2}^{od,*}\Big) \quad (1096)$$


---

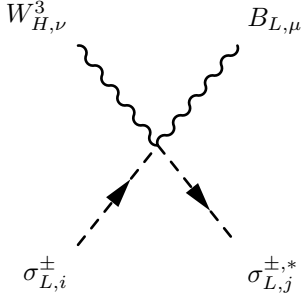

$$\frac{i}{2}g_{B1}\frac{1}{\sqrt{gA1^2+gB1^2}}\Big(-g_{A1}+\sqrt{\frac{gA1^2}{gA1^2+gB1^2}}\sqrt{gA1^2+gB1^2}\Big)\frac{1}{\sqrt{gA2^2+gB2^2}}\Big(-g_{A2}\sqrt{\frac{gA2^2}{gA2^2+gB2^2}}\sqrt{gA2^2+gB2^2}+g_{B2}^2\Big)\Big(Z_{Ls,i1}^{od,*}Z_{Ls,i2}^{od,*}\Big) \quad (1097)$$


---

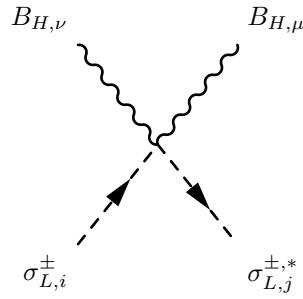

$$\begin{aligned}
& \frac{i}{2} \frac{1}{\left(gA1^2 + gB1^2\right)^{3/2}} \left( 2g_{A1}^3 g_{B1}^2 \sqrt{\frac{gA1^2}{gA1^2 + gB1^2}} + 2g_{A1} g_{B1}^4 \sqrt{\frac{gA1^2}{gA1^2 + gB1^2}} + g_{A1}^4 \sqrt{gA1^2 + gB1^2} \right. \\
& \left. + g_{B1}^4 \sqrt{gA1^2 + gB1^2} \right) \left( Z_{Ls,i1}^{od,*} Z_{Ls,j1}^{od} + Z_{Ls,i2}^{od,*} Z_{Ls,j2}^{od} + Z_{Ls,i3}^{od,*} Z_{Ls,j3}^{od} + Z_{Ls,i4}^{od,*} Z_{Ls,j4}^{od} \right) \left( g_{\mu\nu} \right)
\end{aligned} \tag{1098}$$


---

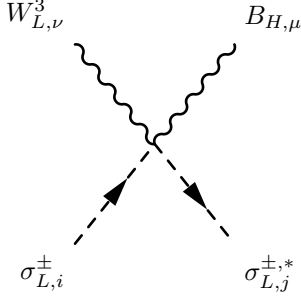

$$\begin{aligned}
& \frac{i}{2} \frac{1}{\sqrt{gA1^2 + gB1^2}} \left( g_{A1} \sqrt{\frac{gA1^2}{gA1^2 + gB1^2}} \sqrt{gA1^2 + gB1^2} + g_{B1}^2 \right) g_{B2} \frac{1}{\sqrt{gA2^2 + gB2^2}} \left( \sqrt{\frac{gA2^2}{gA2^2 + gB2^2}} \sqrt{gA2^2 + gB2^2} + g_{A2} \right) \left( Z_{Ls,i1}^{od,*} Z_{Ls,j1}^{od} \right. \\
& \left. + Z_{Ls,i2}^{od,*} Z_{Ls,j2}^{od} + Z_{Ls,i3}^{od,*} Z_{Ls,j3}^{od} + Z_{Ls,i4}^{od,*} Z_{Ls,j4}^{od} \right)
\end{aligned} \tag{1099}$$


---

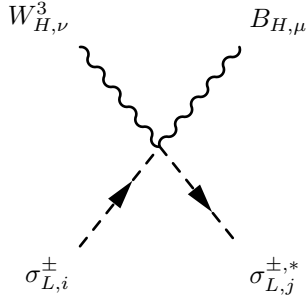

$$\begin{aligned}
& \frac{i}{2} \frac{1}{\sqrt{gA1^2 + gB1^2}} \left( g_{A1} \sqrt{\frac{gA1^2}{gA1^2 + gB1^2}} \sqrt{gA1^2 + gB1^2} + g_{B1}^2 \right) \frac{1}{\sqrt{gA2^2 + gB2^2}} \left( -g_{A2} \sqrt{\frac{gA2^2}{gA2^2 + gB2^2}} \sqrt{gA2^2 + gB2^2} + g_{B2}^2 \right) \left( Z_{Ls,i1}^{od,*} Z_{Ls,j1}^{od} \right. \\
& \left. + Z_{Ls,i2}^{od,*} Z_{Ls,j2}^{od} + Z_{Ls,i3}^{od,*} Z_{Ls,j3}^{od} + Z_{Ls,i4}^{od,*} Z_{Ls,j4}^{od} \right)
\end{aligned} \tag{1100}$$


---

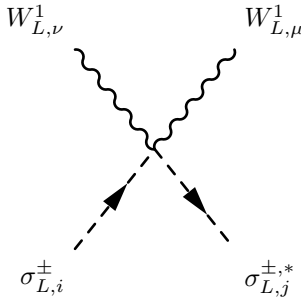

$$ig_{A2}^2 g_{B2}^2 (g_{A2}^2 + g_{B2}^2)^{-1} \left( Z_{Ls,i1}^{od,*} Z_{Ls,j1}^{od} + Z_{Ls,i2}^{od,*} Z_{Ls,j2}^{od} + Z_{Ls,i3}^{od,*} Z_{Ls,j3}^{od} + Z_{Ls,i4}^{od,*} Z_{Ls,j4}^{od} \right) (g_{\mu\nu}) \quad (1101)$$


---

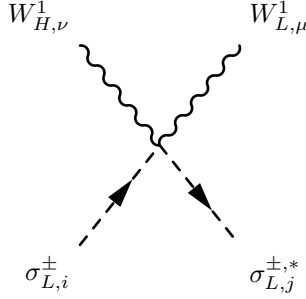

$$-\frac{i}{2} g_{B2} \left( -g_{B2}^2 + g_{A2}^2 \right) \sqrt{\frac{g_{A2}^2}{g_{A2}^2 + g_{B2}^2}} \frac{1}{\sqrt{g_{A2}^2 + g_{B2}^2}} \left( Z_{Ls,i1}^{od,*} Z_{Ls,j1}^{od} + Z_{Ls,i2}^{od,*} Z_{Ls,j2}^{od} + Z_{Ls,i3}^{od,*} Z_{Ls,j3}^{od} + Z_{Ls,i4}^{od,*} Z_{Ls,j4}^{od} \right) (g_{\mu\nu}) \quad (1102)$$


---

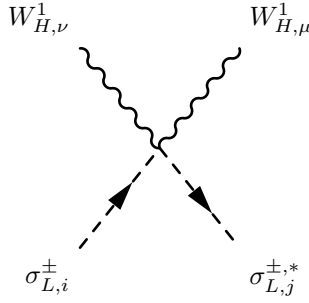

$$\frac{i}{2} (g_{A2}^2 + g_{B2}^2)^{-1} (g_{A2}^4 + g_{B2}^4) \left( Z_{Ls,i1}^{od,*} Z_{Ls,j1}^{od} + Z_{Ls,i2}^{od,*} Z_{Ls,j2}^{od} + Z_{Ls,i3}^{od,*} Z_{Ls,j3}^{od} + Z_{Ls,i4}^{od,*} Z_{Ls,j4}^{od} \right) (g_{\mu\nu}) \quad (1103)$$


---

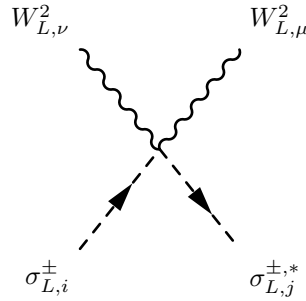

$$ig_{A2}^2 g_{B2}^2 (g_{A2}^2 + g_{B2}^2)^{-1} \left( Z_{Ls,i1}^{od,*} Z_{Ls,j1}^{od} + Z_{Ls,i2}^{od,*} Z_{Ls,j2}^{od} + Z_{Ls,i3}^{od,*} Z_{Ls,j3}^{od} + Z_{Ls,i4}^{od,*} Z_{Ls,j4}^{od} \right) (g_{\mu\nu}) \quad (1104)$$


---

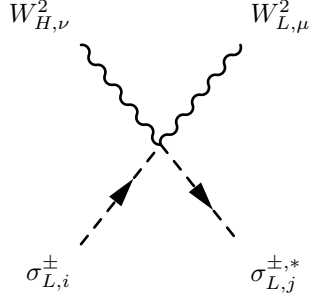

$$-\frac{i}{2}g_{B2}\left(-g_{B2}^2+g_{A2}^2\right)\sqrt{\frac{gA2^2}{gA2^2+gB2^2}}\frac{1}{\sqrt{gA2^2+gB2^2}}\left(Z_{Ls,i1}^{od,*}Z_{Ls,j1}^{od}+Z_{Ls,i2}^{od,*}Z_{Ls,j2}^{od}+Z_{Ls,i3}^{od,*}Z_{Ls,j3}^{od}+Z_{Ls,i4}^{od,*}Z_{Ls,j4}^{od}\right)\left(g_{\mu\nu}\right) \quad (1105)$$


---

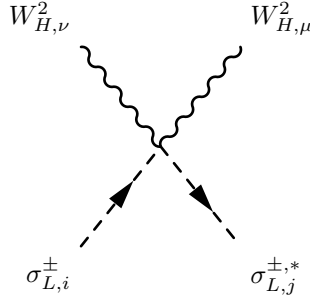

$$\frac{i}{2}\left(g_{A2}^2+g_{B2}^2\right)^{-1}\left(g_{A2}^4+g_{B2}^4\right)\left(Z_{Ls,i1}^{od,*}Z_{Ls,j1}^{od}+Z_{Ls,i2}^{od,*}Z_{Ls,j2}^{od}+Z_{Ls,i3}^{od,*}Z_{Ls,j3}^{od}+Z_{Ls,i4}^{od,*}Z_{Ls,j4}^{od}\right)\left(g_{\mu\nu}\right) \quad (1106)$$


---

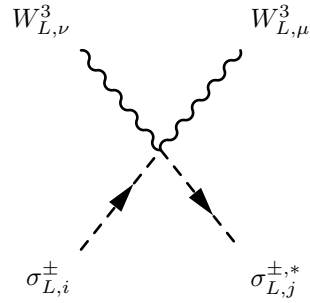

$$ig_{A2}g_{B2}^2\frac{1}{\left(gA2^2+gB2^2\right)^{3/2}}\left(g_{A2}^2\sqrt{\frac{gA2^2}{gA2^2+gB2^2}}+g_{A2}\sqrt{gA2^2+gB2^2}+g_{B2}^2\sqrt{\frac{gA2^2}{gA2^2+gB2^2}}\right)\left(Z_{Ls,i1}^{od,*}Z_{Ls,j1}^{od}+Z_{Ls,i2}^{od,*}Z_{Ls,j2}^{od}+Z_{Ls,i3}^{od,*}Z_{Ls,j3}^{od}+Z_{Ls,i4}^{od,*}Z_{Ls,j4}^{od}\right)\left(g_{\mu\nu}\right) \quad (1107)$$


---



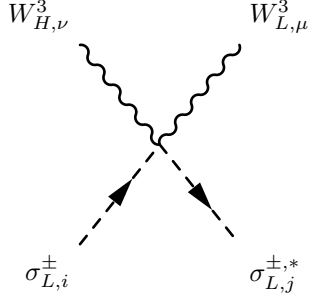

$$\frac{i}{2}g_{B2}\left(-g_{A2}^2+g_{B2}^2\right)\frac{1}{\left(gA2^2+gB2^2\right)^{3/2}}\left(g_{A2}^2\sqrt{\frac{gA2^2}{gA2^2+gB2^2}}+g_{A2}\sqrt{gA2^2+gB2^2}+g_{B2}^2\sqrt{\frac{gA2^2}{gA2^2+gB2^2}}\right)\left(Z_{Ls,i1}^{od,*}Z_{Ls,j1}^{od}+Z_{Ls,i2}^{od,*}Z_{Ls,j2}^{od}+Z_{Ls,i3}^{od,*}Z_{Ls,j3}^{od}+Z_{Ls,i4}^{od,*}Z_{Ls,j4}^{od}\right)\left(g_{\mu\nu}\right) \quad (1108)$$


---

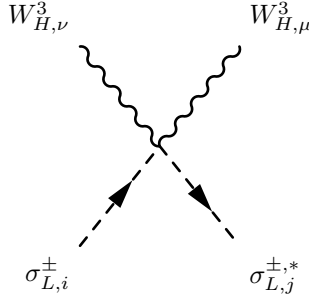

$$\frac{i}{2}\frac{1}{\left(gA2^2+gB2^2\right)^{3/2}}\left(-2g_{A2}^3g_{B2}^2\sqrt{\frac{gA2^2}{gA2^2+gB2^2}}-2g_{A2}g_{B2}^4\sqrt{\frac{gA2^2}{gA2^2+gB2^2}}+g_{A2}^4\sqrt{gA2^2+gB2^2}+g_{B2}^4\sqrt{gA2^2+gB2^2}\right)\left(Z_{Ls,i1}^{od,*}Z_{Ls,j1}^{od}+Z_{Ls,i2}^{od,*}Z_{Ls,j2}^{od}+Z_{Ls,i3}^{od,*}Z_{Ls,j3}^{od}+Z_{Ls,i4}^{od,*}Z_{Ls,j4}^{od}\right)\left(g_{\mu\nu}\right) \quad (1109)$$


---

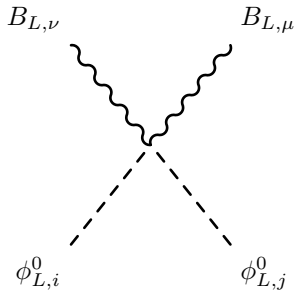

$$-2ig_{A1}g_{B1}^2\frac{1}{\left(gA1^2+gB1^2\right)^{3/2}}\left(g_{A1}^2\sqrt{\frac{gA1^2}{gA1^2+gB1^2}}-g_{A1}\sqrt{gA1^2+gB1^2}+g_{B1}^2\sqrt{\frac{gA1^2}{gA1^2+gB1^2}}\right)\left(Z_{Ls,i1}^{DR,*}Z_{Ls,j1}^{DR,*}+Z_{Ls,i2}^{DR,*}Z_{Ls,j2}^{DR,*}+Z_{Ls,i3}^{DR,*}Z_{Ls,j3}^{DR,*}\right)$$


---

(1110)

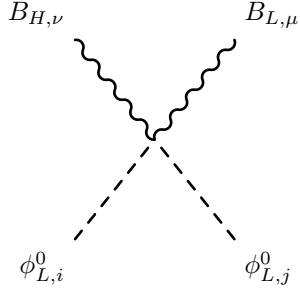

$$ig_{B1}\left(-g_{A1}^2+g_{B1}^2\right)\frac{1}{\left(gA1^2+gB1^2\right)^{3/2}}\left(g_{A1}^2\sqrt{\frac{gA1^2}{gA1^2+gB1^2}}-g_{A1}\sqrt{gA1^2+gB1^2}+g_{B1}^2\sqrt{\frac{gA1^2}{gA1^2+gB1^2}}\right)\left(Z_{Ls,i1}^{DR,*}Z_{Ls,j1}^{DR,*}+Z_{Ls,i2}^{DR,*}Z_{Ls,j2}^{DR,*}+Z_{Ls,i3}^{DR,*}Z_{Ls,j3}^{DR,*}\right)$$


---

(1111)

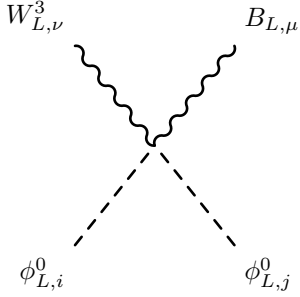

$$-ig_{B1}\frac{1}{\sqrt{gA1^2+gB1^2}}\left(-g_{A1}+\sqrt{\frac{gA1^2}{gA1^2+gB1^2}}\sqrt{gA1^2+gB1^2}\right)g_{B2}\frac{1}{\sqrt{gA2^2+gB2^2}}\left(-g_{A2}+\sqrt{\frac{gA2^2}{gA2^2+gB2^2}}\sqrt{gA2^2+gB2^2}\right)\left(Z_{Ls,i1}^{DR,*}Z_{Ls,j1}^{DR,*}+Z_{Ls,i2}^{DR,*}Z_{Ls,j2}^{DR,*}+Z_{Ls,i3}^{DR,*}Z_{Ls,j3}^{DR,*}\right)$$


---

(1112)

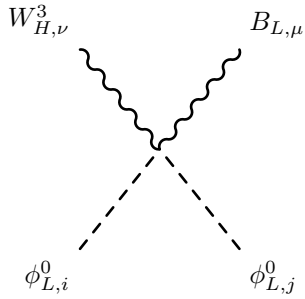

$$-ig_{B1} \frac{1}{\sqrt{gA1^2 + gB1^2}} \left( -g_{A1} + \sqrt{\frac{gA1^2}{gA1^2 + gB1^2}} \sqrt{gA1^2 + gB1^2} \right) \frac{1}{\sqrt{gA2^2 + gB2^2}} \left( g_{A2} \sqrt{\frac{gA2^2}{gA2^2 + gB2^2}} \sqrt{gA2^2 + gB2^2} + g_{B2}^2 \right) \left( Z_{Ls,i}^{DR,*} \right) \quad (1113)$$


---

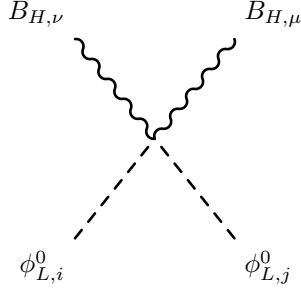

$$i \frac{1}{(gA1^2 + gB1^2)^{3/2}} \left( 2g_{A1}^3 g_{B1}^2 \sqrt{\frac{gA1^2}{gA1^2 + gB1^2}} + 2g_{A1} g_{B1}^4 \sqrt{\frac{gA1^2}{gA1^2 + gB1^2}} + g_{A1}^4 \sqrt{gA1^2 + gB1^2} \right. \\ \left. + g_{B1}^4 \sqrt{gA1^2 + gB1^2} \right) \left( Z_{Ls,i1}^{DR,*} Z_{Ls,j1}^{DR,*} + Z_{Ls,i2}^{DR,*} Z_{Ls,j2}^{DR,*} + Z_{Ls,i3}^{DR,*} Z_{Ls,j3}^{DR,*} + Z_{Ls,i4}^{DR,*} Z_{Ls,j4}^{DR,*} \right) (g_{\mu\nu}) \quad (1114)$$


---

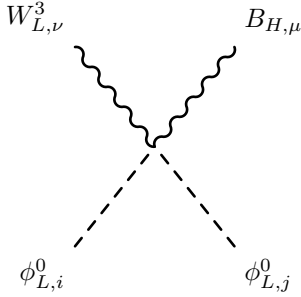

$$-i \frac{1}{\sqrt{gA1^2 + gB1^2}} \left( g_{A1} \sqrt{\frac{gA1^2}{gA1^2 + gB1^2}} \sqrt{gA1^2 + gB1^2} + g_{B1}^2 \right) g_{B2} \frac{1}{\sqrt{gA2^2 + gB2^2}} \left( -g_{A2} + \sqrt{\frac{gA2^2}{gA2^2 + gB2^2}} \sqrt{gA2^2 + gB2^2} \right) \left( Z_{Ls,i}^{DR,*} \right) \quad (1115)$$


---

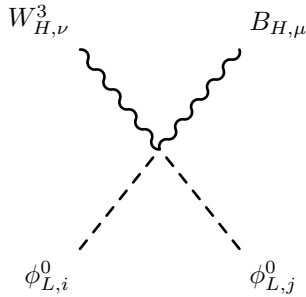

$$-i \frac{1}{\sqrt{gA1^2 + gB1^2}} \left( g_{A1} \sqrt{\frac{gA1^2}{gA1^2 + gB1^2}} \sqrt{gA1^2 + gB1^2} + g_{B1}^2 \right) \frac{1}{\sqrt{gA2^2 + gB2^2}} \left( g_{A2} \sqrt{\frac{gA2^2}{gA2^2 + gB2^2}} \sqrt{gA2^2 + gB2^2} + g_{B2}^2 \right) \left( Z_{Ls,i1}^{DR,*} Z_{Ls,j1}^{DR,*} \right. \\ \left. (1116) \right)$$


---

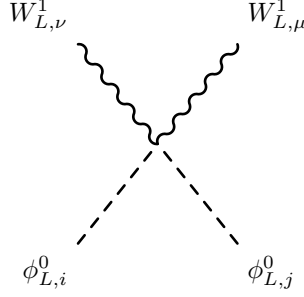

$$2ig_{B2}^2 \sqrt{\frac{gA2^2}{gA2^2 + gB2^2}} \frac{1}{\sqrt{gA2^2 + gB2^2}} \left( \sqrt{\frac{gA2^2}{gA2^2 + gB2^2}} \sqrt{gA2^2 + gB2^2} Z_{Ls,i2}^{DR,*} Z_{Ls,j2}^{DR,*} - g_{A2} Z_{Ls,i4}^{DR,*} Z_{Ls,j2}^{DR,*} \right. \\ \left. + Z_{Ls,i1}^{DR,*} \left( -g_{A2} Z_{Ls,j3}^{DR,*} + \sqrt{\frac{gA2^2}{gA2^2 + gB2^2}} \sqrt{gA2^2 + gB2^2} Z_{Ls,j1}^{DR,*} \right) \right. \\ \left. + Z_{Ls,i3}^{DR,*} \left( -g_{A2} Z_{Ls,j1}^{DR,*} + \sqrt{\frac{gA2^2}{gA2^2 + gB2^2}} \sqrt{gA2^2 + gB2^2} Z_{Ls,j3}^{DR,*} \right) - g_{A2} Z_{Ls,i2}^{DR,*} Z_{Ls,j4}^{DR,*} \right. \\ \left. + \sqrt{\frac{gA2^2}{gA2^2 + gB2^2}} \sqrt{gA2^2 + gB2^2} Z_{Ls,i4}^{DR,*} Z_{Ls,j4}^{DR,*} \right) (g_{\mu\nu}) \quad (1117)$$


---

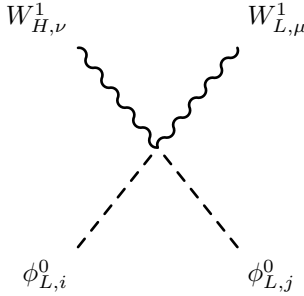

$$ig_{A2}g_{B2} \left( -g_{B2}^2 + g_{A2}^2 \right) \frac{1}{\sqrt{\frac{gA2^2}{gA2^2 + gB2^2}}} \frac{1}{(gA2^2 + gB2^2)^{3/2}} \left( -g_{A2} Z_{Ls,i2}^{DR,*} Z_{Ls,j2}^{DR,*} + \sqrt{\frac{gA2^2}{gA2^2 + gB2^2}} \sqrt{gA2^2 + gB2^2} Z_{Ls,i4}^{DR,*} Z_{Ls,j2}^{DR,*} \right. \\ \left. + Z_{Ls,i3}^{DR,*} \left( -g_{A2} Z_{Ls,j3}^{DR,*} + \sqrt{\frac{gA2^2}{gA2^2 + gB2^2}} \sqrt{gA2^2 + gB2^2} Z_{Ls,j1}^{DR,*} \right) \right)$$

$$\begin{aligned}
& + Z_{Ls,i1}^{DR,*} \left( -g_{A2} Z_{Ls,j1}^{DR,*} + \sqrt{\frac{gA2^2}{gA2^2 + gB2^2}} \sqrt{gA2^2 + gB2^2} Z_{Ls,j3}^{DR,*} \right) \\
& + \sqrt{\frac{gA2^2}{gA2^2 + gB2^2}} \sqrt{gA2^2 + gB2^2} Z_{Ls,i2}^{DR,*} Z_{Ls,j4}^{DR,*} - g_{A2} Z_{Ls,i4}^{DR,*} Z_{Ls,j4}^{DR,*} \Big) (g_{\mu\nu})
\end{aligned} \tag{1118}$$


---

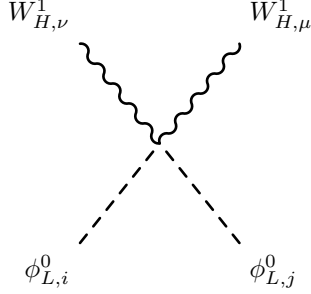

$$\begin{aligned}
& i \frac{1}{\sqrt{\frac{gA2^2}{gA2^2 + gB2^2}}} \frac{1}{\left( gA2^2 + gB2^2 \right)^{3/2}} \left( g_{A2}^4 \sqrt{\frac{gA2^2}{gA2^2 + gB2^2}} \sqrt{gA2^2 + gB2^2} Z_{Ls,i2}^{DR,*} Z_{Ls,j2}^{DR,*} \right. \\
& + g_{B2}^4 \sqrt{\frac{gA2^2}{gA2^2 + gB2^2}} \sqrt{gA2^2 + gB2^2} Z_{Ls,i2}^{DR,*} Z_{Ls,j2}^{DR,*} + 2g_{A2}^3 g_{B2}^2 Z_{Ls,i4}^{DR,*} Z_{Ls,j2}^{DR,*} \\
& + Z_{Ls,i1}^{DR,*} \left( 2g_{A2}^3 g_{B2}^2 Z_{Ls,j3}^{DR,*} + \sqrt{\frac{gA2^2}{gA2^2 + gB2^2}} \sqrt{gA2^2 + gB2^2} (g_{A2}^4 + g_{B2}^4) Z_{Ls,j1}^{DR,*} \right) \\
& + Z_{Ls,i3}^{DR,*} \left( 2g_{A2}^3 g_{B2}^2 Z_{Ls,j1}^{DR,*} + \sqrt{\frac{gA2^2}{gA2^2 + gB2^2}} \sqrt{gA2^2 + gB2^2} (g_{A2}^4 + g_{B2}^4) Z_{Ls,j3}^{DR,*} \right) \\
& + 2g_{A2}^3 g_{B2}^2 Z_{Ls,i2}^{DR,*} Z_{Ls,j4}^{DR,*} + g_{A2}^4 \sqrt{\frac{gA2^2}{gA2^2 + gB2^2}} \sqrt{gA2^2 + gB2^2} Z_{Ls,i4}^{DR,*} Z_{Ls,j4}^{DR,*} \\
& \left. + g_{B2}^4 \sqrt{\frac{gA2^2}{gA2^2 + gB2^2}} \sqrt{gA2^2 + gB2^2} Z_{Ls,i4}^{DR,*} Z_{Ls,j4}^{DR,*} \right) (g_{\mu\nu})
\end{aligned} \tag{1119}$$


---

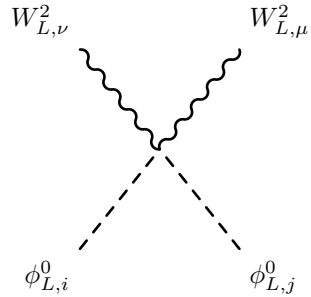

$$\begin{aligned}
& 2ig_B^2 \sqrt{\frac{gA^2}{gA^2 + gB^2}} \frac{1}{\sqrt{gA^2 + gB^2}} \left( \sqrt{\frac{gA^2}{gA^2 + gB^2}} \sqrt{gA^2 + gB^2} Z_{Ls,i2}^{DR,*} Z_{Ls,j2}^{DR,*} - g_{A2} Z_{Ls,i4}^{DR,*} Z_{Ls,j2}^{DR,*} \right. \\
& + Z_{Ls,i1}^{DR,*} \left( -g_{A2} Z_{Ls,j3}^{DR,*} + \sqrt{\frac{gA^2}{gA^2 + gB^2}} \sqrt{gA^2 + gB^2} Z_{Ls,j1}^{DR,*} \right) \\
& + Z_{Ls,i3}^{DR,*} \left( -g_{A2} Z_{Ls,j1}^{DR,*} + \sqrt{\frac{gA^2}{gA^2 + gB^2}} \sqrt{gA^2 + gB^2} Z_{Ls,j3}^{DR,*} \right) - g_{A2} Z_{Ls,i2}^{DR,*} Z_{Ls,j4}^{DR,*} \\
& \left. + \sqrt{\frac{gA^2}{gA^2 + gB^2}} \sqrt{gA^2 + gB^2} Z_{Ls,i4}^{DR,*} Z_{Ls,j4}^{DR,*} \right) (g_{\mu\nu})
\end{aligned} \tag{1120}$$


---

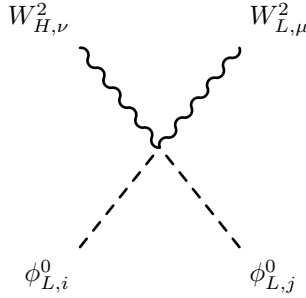

$$\begin{aligned}
& ig_{A2} g_{B2} \left( -g_{B2}^2 + g_{A2}^2 \right) \frac{1}{\sqrt{\frac{gA^2}{gA^2 + gB^2}}} \frac{1}{(gA^2 + gB^2)^{3/2}} \left( -g_{A2} Z_{Ls,i2}^{DR,*} Z_{Ls,j2}^{DR,*} + \sqrt{\frac{gA^2}{gA^2 + gB^2}} \sqrt{gA^2 + gB^2} Z_{Ls,i4}^{DR,*} Z_{Ls,j2}^{DR,*} \right. \\
& + Z_{Ls,i3}^{DR,*} \left( -g_{A2} Z_{Ls,j3}^{DR,*} + \sqrt{\frac{gA^2}{gA^2 + gB^2}} \sqrt{gA^2 + gB^2} Z_{Ls,j1}^{DR,*} \right) \\
& + Z_{Ls,i1}^{DR,*} \left( -g_{A2} Z_{Ls,j1}^{DR,*} + \sqrt{\frac{gA^2}{gA^2 + gB^2}} \sqrt{gA^2 + gB^2} Z_{Ls,j3}^{DR,*} \right) \\
& \left. + \sqrt{\frac{gA^2}{gA^2 + gB^2}} \sqrt{gA^2 + gB^2} Z_{Ls,i2}^{DR,*} Z_{Ls,j4}^{DR,*} - g_{A2} Z_{Ls,i4}^{DR,*} Z_{Ls,j4}^{DR,*} \right) (g_{\mu\nu})
\end{aligned} \tag{1121}$$


---

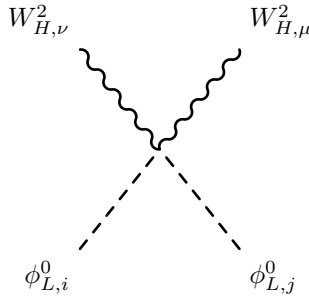

$$\begin{aligned}
& i \frac{1}{\sqrt{\frac{gA^2}{gA^2+gB^2}}} \frac{1}{\left(gA^2+gB^2\right)^{3/2}} \left( g_{A2}^4 \sqrt{\frac{gA^2}{gA^2+gB^2}} \sqrt{gA^2+gB^2} Z_{Ls,i2}^{DR,*} Z_{Ls,j2}^{DR,*} \right. \\
& + g_{B2}^4 \sqrt{\frac{gA^2}{gA^2+gB^2}} \sqrt{gA^2+gB^2} Z_{Ls,i2}^{DR,*} Z_{Ls,j2}^{DR,*} + 2g_{A2}^3 g_{B2}^2 Z_{Ls,i4}^{DR,*} Z_{Ls,j2}^{DR,*} \\
& + Z_{Ls,i1}^{DR,*} \left( 2g_{A2}^3 g_{B2}^2 Z_{Ls,j3}^{DR,*} + \sqrt{\frac{gA^2}{gA^2+gB^2}} \sqrt{gA^2+gB^2} (g_{A2}^4 + g_{B2}^4) Z_{Ls,j1}^{DR,*} \right) \\
& + Z_{Ls,i3}^{DR,*} \left( 2g_{A2}^3 g_{B2}^2 Z_{Ls,j1}^{DR,*} + \sqrt{\frac{gA^2}{gA^2+gB^2}} \sqrt{gA^2+gB^2} (g_{A2}^4 + g_{B2}^4) Z_{Ls,j3}^{DR,*} \right) \\
& + 2g_{A2}^3 g_{B2}^2 Z_{Ls,i2}^{DR,*} Z_{Ls,j4}^{DR,*} + g_{A2}^4 \sqrt{\frac{gA^2}{gA^2+gB^2}} \sqrt{gA^2+gB^2} Z_{Ls,i4}^{DR,*} Z_{Ls,j4}^{DR,*} \\
& \left. + g_{B2}^4 \sqrt{\frac{gA^2}{gA^2+gB^2}} \sqrt{gA^2+gB^2} Z_{Ls,i4}^{DR,*} Z_{Ls,j4}^{DR,*} \right) (g_{\mu\nu}) \tag{1122}
\end{aligned}$$


---

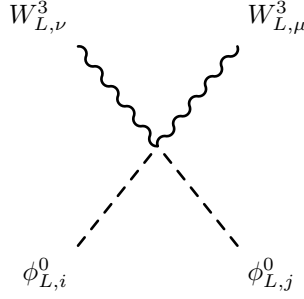

$$-2ig_{A2}g_{B2}^2 \frac{1}{\left(gA^2+gB^2\right)^{3/2}} \left( g_{A2}^2 \sqrt{\frac{gA^2}{gA^2+gB^2}} - g_{A2} \sqrt{gA^2+gB^2} + g_{B2}^2 \sqrt{\frac{gA^2}{gA^2+gB^2}} \right) \left( Z_{Ls,i1}^{DR,*} Z_{Ls,j1}^{DR,*} + Z_{Ls,i2}^{DR,*} Z_{Ls,j2}^{DR,*} + Z_{Ls,i3}^{DR,*} Z_{Ls,j3}^{DR,*} + Z_{Ls,i4}^{DR,*} Z_{Ls,j4}^{DR,*} \right) \tag{1123}$$


---

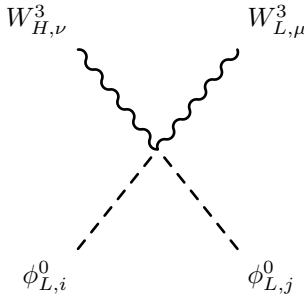

$$ig_{B2}(-g_{A2}^2 + g_{B2}^2) \frac{1}{(gA2^2 + gB2^2)^{3/2}} \left( g_{A2}^2 \sqrt{\frac{gA2^2}{gA2^2 + gB2^2}} - g_{A2} \sqrt{gA2^2 + gB2^2} + g_{B2}^2 \sqrt{\frac{gA2^2}{gA2^2 + gB2^2}} \right) (Z_{Ls,i1}^{DR,*} Z_{Ls,j1}^{DR,*} + Z_{Ls,i2}^{DR,*} Z_{Ls,j2}^{DR,*}) \quad (1124)$$


---

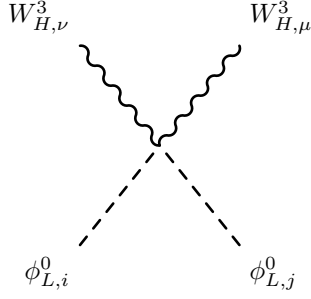

$$i \frac{1}{(gA2^2 + gB2^2)^{3/2}} \left( 2g_{A2}^3 g_{B2}^2 \sqrt{\frac{gA2^2}{gA2^2 + gB2^2}} + 2g_{A2} g_{B2}^4 \sqrt{\frac{gA2^2}{gA2^2 + gB2^2}} + g_{A2}^4 \sqrt{gA2^2 + gB2^2} \right. \\ \left. + g_{B2}^4 \sqrt{gA2^2 + gB2^2} \right) (Z_{Ls,i1}^{DR,*} Z_{Ls,j1}^{DR,*} + Z_{Ls,i2}^{DR,*} Z_{Ls,j2}^{DR,*} + Z_{Ls,i3}^{DR,*} Z_{Ls,j3}^{DR,*} + Z_{Ls,i4}^{DR,*} Z_{Ls,j4}^{DR,*}) (g_{\mu\nu}) \quad (1125)$$


---

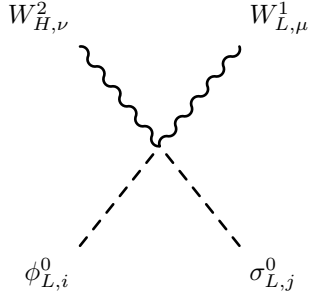

$$-ig_{A2} g_{B2} \left( -Z_{Ls,i1}^{DR,*} Z_{Ls,j3}^{Di,*} + Z_{Ls,i2}^{DR,*} Z_{Ls,j4}^{Di,*} + Z_{Ls,i3}^{DR,*} Z_{Ls,j1}^{Di,*} - Z_{Ls,i4}^{DR,*} Z_{Ls,j2}^{Di,*} \right) (g_{\mu\nu}) \quad (1126)$$


---

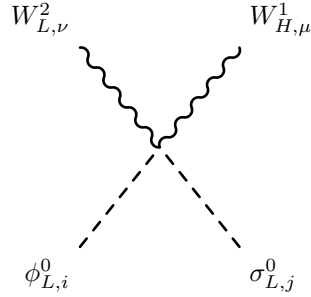



$$ig_{A2}g_{B2}\left(-Z_{Ls,i1}^{DR,*}Z_{Ls,j3}^{Di,*}+Z_{Ls,i2}^{DR,*}Z_{Ls,j4}^{Di,*}+Z_{Ls,i3}^{DR,*}Z_{Ls,j1}^{Di,*}-Z_{Ls,i4}^{DR,*}Z_{Ls,j2}^{Di,*}\right)(g_{\mu\nu}) \quad (1127)$$

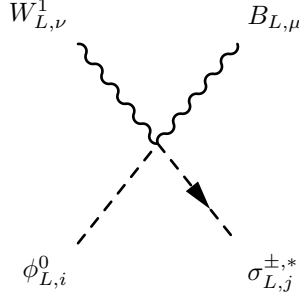

$$\begin{aligned} & -\frac{i}{2}g_{B1}\frac{1}{\sqrt{gA1^2+gB1^2}}\left(-g_{A1}+\sqrt{\frac{gA1^2}{gA1^2+gB1^2}}\sqrt{gA1^2+gB1^2}\right)g_{B2}\frac{1}{\sqrt{gA2^2+gB2^2}}\left(-g_{A2}Z_{Ls,i2}^{DR,*}Z_{Ls,j2}^{od}+\sqrt{\frac{gA2^2}{gA2^2+gB2^2}}\sqrt{gA2^2+gB2^2}\right. \\ & +\sqrt{\frac{gA2^2}{gA2^2+gB2^2}}\sqrt{gA2^2+gB2^2}Z_{Ls,i2}^{DR,*}Z_{Ls,j3}^{od}-g_{A2}Z_{Ls,i4}^{DR,*}Z_{Ls,j3}^{od} \\ & +Z_{Ls,i1}^{DR,*}\left(-g_{A2}Z_{Ls,j4}^{od}+\sqrt{\frac{gA2^2}{gA2^2+gB2^2}}\sqrt{gA2^2+gB2^2}Z_{Ls,j1}^{od}\right) \\ & \left.+Z_{Ls,i3}^{DR,*}\left(-g_{A2}Z_{Ls,j1}^{od}+\sqrt{\frac{gA2^2}{gA2^2+gB2^2}}\sqrt{gA2^2+gB2^2}Z_{Ls,j4}^{od}\right)\right)(g_{\mu\nu}) \quad (1128) \end{aligned}$$

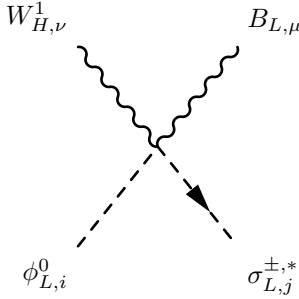

$$\begin{aligned} & -\frac{i}{2}g_{B1}\frac{1}{\sqrt{gA1^2+gB1^2}}\left(-g_{A1}+\sqrt{\frac{gA1^2}{gA1^2+gB1^2}}\sqrt{gA1^2+gB1^2}\right)\frac{1}{\sqrt{gA2^2+gB2^2}}\left(g_{A2}\sqrt{\frac{gA2^2}{gA2^2+gB2^2}}\sqrt{gA2^2+gB2^2}Z_{Ls,i2}^{DR,*}Z_{Ls,j2}^{od}\right. \\ & +g_{A2}\sqrt{\frac{gA2^2}{gA2^2+gB2^2}}\sqrt{gA2^2+gB2^2}Z_{Ls,i4}^{DR,*}Z_{Ls,j3}^{od} \\ & \left.+Z_{Ls,i3}^{DR,*}\left(g_{A2}\sqrt{\frac{gA2^2}{gA2^2+gB2^2}}\sqrt{gA2^2+gB2^2}Z_{Ls,j1}^{od}+g_{B2}^2Z_{Ls,j4}^{od}\right)\right) \end{aligned}$$

$$+ Z_{Ls,i1}^{DR,*} \left( g_{A2} \sqrt{\frac{gA2^2}{gA2^2 + gB2^2}} \sqrt{gA2^2 + gB2^2} Z_{Ls,j4}^{od} + g_{B2}^2 Z_{Ls,j1}^{od} \right) (g_{\mu\nu}) \quad (1129)$$


---

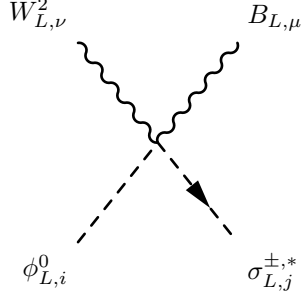

$$\begin{aligned} & -\frac{1}{2} g_{B1} \frac{1}{\sqrt{gA1^2 + gB1^2}} \left( -g_{A1} + \sqrt{\frac{gA1^2}{gA1^2 + gB1^2}} \sqrt{gA1^2 + gB1^2} \right) g_{B2} \frac{1}{\sqrt{gA2^2 + gB2^2}} \left( -g_{A2} Z_{Ls,i2}^{DR,*} Z_{Ls,j2}^{od} + \sqrt{\frac{gA2^2}{gA2^2 + gB2^2}} \sqrt{gA2^2 + gB2^2} \right. \\ & + \sqrt{\frac{gA2^2}{gA2^2 + gB2^2}} \sqrt{gA2^2 + gB2^2} Z_{Ls,i2}^{DR,*} Z_{Ls,j3}^{od} - g_{A2} Z_{Ls,i4}^{DR,*} Z_{Ls,j3}^{od} \\ & + Z_{Ls,i1}^{DR,*} \left( -g_{A2} Z_{Ls,j4}^{od} + \sqrt{\frac{gA2^2}{gA2^2 + gB2^2}} \sqrt{gA2^2 + gB2^2} Z_{Ls,j1}^{od} \right) \\ & \left. + Z_{Ls,i3}^{DR,*} \left( -g_{A2} Z_{Ls,j1}^{od} + \sqrt{\frac{gA2^2}{gA2^2 + gB2^2}} \sqrt{gA2^2 + gB2^2} Z_{Ls,j4}^{od} \right) \right) (g_{\mu\nu}) \quad (1130) \end{aligned}$$


---

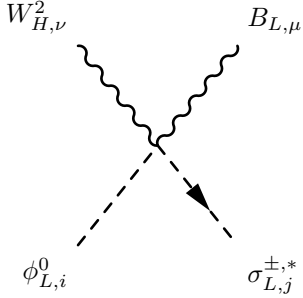

$$\begin{aligned} & -\frac{1}{2} g_{B1} \frac{1}{\sqrt{gA1^2 + gB1^2}} \left( -g_{A1} + \sqrt{\frac{gA1^2}{gA1^2 + gB1^2}} \sqrt{gA1^2 + gB1^2} \right) \frac{1}{\sqrt{gA2^2 + gB2^2}} \left( g_{A2} \sqrt{\frac{gA2^2}{gA2^2 + gB2^2}} \sqrt{gA2^2 + gB2^2} Z_{Ls,i2}^{DR,*} Z_{Ls,j2}^{od} \right. \\ & \left. + g_{A2} \sqrt{\frac{gA2^2}{gA2^2 + gB2^2}} \sqrt{gA2^2 + gB2^2} Z_{Ls,i4}^{DR,*} Z_{Ls,j3}^{od} \right) \end{aligned}$$

$$\begin{aligned}
& + Z_{Ls,i3}^{DR,*} \left( g_{A2} \sqrt{\frac{gA2^2}{gA2^2 + gB2^2}} \sqrt{gA2^2 + gB2^2} Z_{Ls,j1}^{od} + g_{B2}^2 Z_{Ls,j4}^{od} \right) \\
& + Z_{Ls,i1}^{DR,*} \left( g_{A2} \sqrt{\frac{gA2^2}{gA2^2 + gB2^2}} \sqrt{gA2^2 + gB2^2} Z_{Ls,j4}^{od} + g_{B2}^2 Z_{Ls,j1}^{od} \right) \left( g_{\mu\nu} \right)
\end{aligned} \tag{1131}$$


---

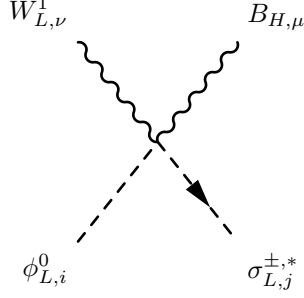

$$\begin{aligned}
& - \frac{i}{2} \frac{1}{\sqrt{gA1^2 + gB1^2}} \left( g_{A1} \sqrt{\frac{gA1^2}{gA1^2 + gB1^2}} \sqrt{gA1^2 + gB1^2} + g_{B1}^2 \right) g_{B2} \frac{1}{\sqrt{gA2^2 + gB2^2}} \left( -g_{A2} Z_{Ls,i2}^{DR,*} Z_{Ls,j2}^{od} + \sqrt{\frac{gA2^2}{gA2^2 + gB2^2}} \sqrt{gA2^2 + gB2^2} \right. \\
& + \sqrt{\frac{gA2^2}{gA2^2 + gB2^2}} \sqrt{gA2^2 + gB2^2} Z_{Ls,i2}^{DR,*} Z_{Ls,j3}^{od} - g_{A2} Z_{Ls,i4}^{DR,*} Z_{Ls,j3}^{od} \\
& + Z_{Ls,i1}^{DR,*} \left( -g_{A2} Z_{Ls,j4}^{od} + \sqrt{\frac{gA2^2}{gA2^2 + gB2^2}} \sqrt{gA2^2 + gB2^2} Z_{Ls,j1}^{od} \right) \\
& \left. + Z_{Ls,i3}^{DR,*} \left( -g_{A2} Z_{Ls,j1}^{od} + \sqrt{\frac{gA2^2}{gA2^2 + gB2^2}} \sqrt{gA2^2 + gB2^2} Z_{Ls,j4}^{od} \right) \right) \left( g_{\mu\nu} \right)
\end{aligned} \tag{1132}$$


---

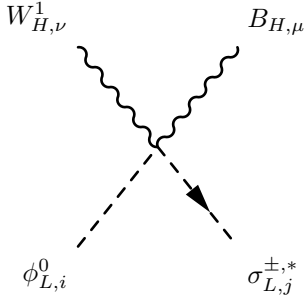

$$- \frac{i}{2} \frac{1}{\sqrt{gA1^2 + gB1^2}} \left( g_{A1} \sqrt{\frac{gA1^2}{gA1^2 + gB1^2}} \sqrt{gA1^2 + gB1^2} + g_{B1}^2 \right) \frac{1}{\sqrt{gA2^2 + gB2^2}} \left( g_{A2} \sqrt{\frac{gA2^2}{gA2^2 + gB2^2}} \sqrt{gA2^2 + gB2^2} Z_{Ls,i2}^{DR,*} Z_{Ls,j2}^{od} + g_{B2}^2 Z_{Ls,i2}^{DR,*} Z_{Ls,j2}^{od} \right)$$

$$\begin{aligned}
& + g_{A2} \sqrt{\frac{gA2^2}{gA2^2 + gB2^2}} \sqrt{gA2^2 + gB2^2} Z_{Ls,i4}^{DR,*} Z_{Ls,j3}^{od} \\
& + Z_{Ls,i3}^{DR,*} \left( g_{A2} \sqrt{\frac{gA2^2}{gA2^2 + gB2^2}} \sqrt{gA2^2 + gB2^2} Z_{Ls,j1}^{od} + g_{B2}^2 Z_{Ls,j4}^{od} \right) \\
& + Z_{Ls,i1}^{DR,*} \left( g_{A2} \sqrt{\frac{gA2^2}{gA2^2 + gB2^2}} \sqrt{gA2^2 + gB2^2} Z_{Ls,j4}^{od} + g_{B2}^2 Z_{Ls,j1}^{od} \right) \left( g_{\mu\nu} \right)
\end{aligned} \tag{1133}$$


---

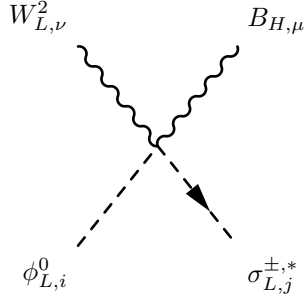

$$\begin{aligned}
& - \frac{1}{2} \frac{1}{\sqrt{gA1^2 + gB1^2}} \left( g_{A1} \sqrt{\frac{gA1^2}{gA1^2 + gB1^2}} \sqrt{gA1^2 + gB1^2} + g_{B1}^2 \right) g_{B2} \frac{1}{\sqrt{gA2^2 + gB2^2}} \left( -g_{A2} Z_{Ls,i2}^{DR,*} Z_{Ls,j2}^{od} + \sqrt{\frac{gA2^2}{gA2^2 + gB2^2}} \sqrt{gA2^2 + gB2^2} \right. \\
& + \sqrt{\frac{gA2^2}{gA2^2 + gB2^2}} \sqrt{gA2^2 + gB2^2} Z_{Ls,i2}^{DR,*} Z_{Ls,j3}^{od} - g_{A2} Z_{Ls,i4}^{DR,*} Z_{Ls,j3}^{od} \\
& + Z_{Ls,i1}^{DR,*} \left( -g_{A2} Z_{Ls,j4}^{od} + \sqrt{\frac{gA2^2}{gA2^2 + gB2^2}} \sqrt{gA2^2 + gB2^2} Z_{Ls,j1}^{od} \right) \\
& + Z_{Ls,i3}^{DR,*} \left( -g_{A2} Z_{Ls,j1}^{od} + \sqrt{\frac{gA2^2}{gA2^2 + gB2^2}} \sqrt{gA2^2 + gB2^2} Z_{Ls,j4}^{od} \right) \left( g_{\mu\nu} \right)
\end{aligned} \tag{1134}$$


---

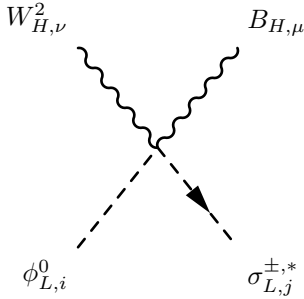

$$- \frac{1}{2} \frac{1}{\sqrt{gA1^2 + gB1^2}} \left( g_{A1} \sqrt{\frac{gA1^2}{gA1^2 + gB1^2}} \sqrt{gA1^2 + gB1^2} + g_{B1}^2 \right) \frac{1}{\sqrt{gA2^2 + gB2^2}} \left( g_{A2} \sqrt{\frac{gA2^2}{gA2^2 + gB2^2}} \sqrt{gA2^2 + gB2^2} Z_{Ls,i2}^{DR,*} Z_{Ls,j2}^{od} + g_{B2}^2 Z_{Ls,i2}^{DR,*} Z_{Ls,j2}^{od} \right)$$

$$\begin{aligned}
& + g_{A2} \sqrt{\frac{gA^2}{gA^2 + gB^2}} \sqrt{gA^2 + gB^2} Z_{Ls,i4}^{DR,*} Z_{Ls,j3}^{od} \\
& + Z_{Ls,i3}^{DR,*} \left( g_{A2} \sqrt{\frac{gA^2}{gA^2 + gB^2}} \sqrt{gA^2 + gB^2} Z_{Ls,j1}^{od} + g_{B2}^2 Z_{Ls,j4}^{od} \right) \\
& + Z_{Ls,i1}^{DR,*} \left( g_{A2} \sqrt{\frac{gA^2}{gA^2 + gB^2}} \sqrt{gA^2 + gB^2} Z_{Ls,j4}^{od} + g_{B2}^2 Z_{Ls,j1}^{od} \right) \left( g_{\mu\nu} \right)
\end{aligned} \tag{1135}$$


---

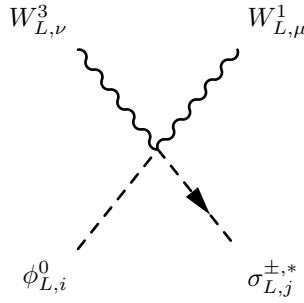

$$-\frac{i}{2} g_{A2} g_{B2}^2 \sqrt{\frac{gA^2}{gA^2 + gB^2}} \frac{1}{\sqrt{gA^2 + gB^2}} \left( Z_{Ls,i1}^{DR,*} \left( Z_{Ls,j1}^{od} + Z_{Ls,j4}^{od} \right) - Z_{Ls,i3}^{DR,*} \left( Z_{Ls,j1}^{od} + Z_{Ls,j4}^{od} \right) + \left( -Z_{Ls,i4}^{DR,*} + Z_{Ls,i2}^{DR,*} \right) \left( Z_{Ls,j2}^{od} + Z_{Ls,j3}^{od} \right) \right) \left( g_{\mu\nu} \right) \tag{1136}$$


---

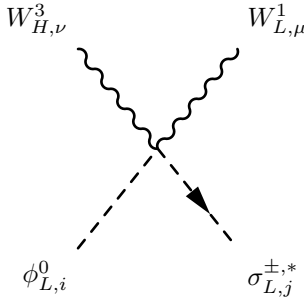

$$\begin{aligned}
& \frac{i}{2} g_{A2} g_{B2} \left( g_{A2}^2 + g_{B2}^2 \right)^{-1} \left( -g_{B2}^2 Z_{Ls,i2}^{DR,*} Z_{Ls,j2}^{od} - g_{A2}^2 Z_{Ls,i4}^{DR,*} Z_{Ls,j2}^{od} + g_{A2}^2 Z_{Ls,i2}^{DR,*} Z_{Ls,j3}^{od} + g_{B2}^2 Z_{Ls,i4}^{DR,*} Z_{Ls,j3}^{od} \right. \\
& \left. + Z_{Ls,i3}^{DR,*} \left( -g_{A2}^2 Z_{Ls,j4}^{od} + g_{B2}^2 Z_{Ls,j1}^{od} \right) + Z_{Ls,i1}^{DR,*} \left( g_{A2}^2 Z_{Ls,j1}^{od} - g_{B2}^2 Z_{Ls,j4}^{od} \right) \right) \left( g_{\mu\nu} \right)
\end{aligned} \tag{1137}$$


---

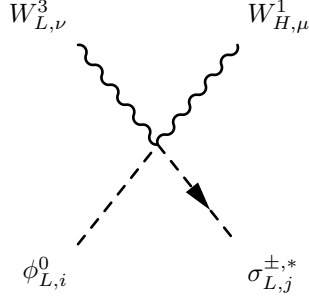

$$\begin{aligned} & \frac{i}{2} g_{A2} g_{B2} \left( g_{A2}^2 + g_{B2}^2 \right)^{-1} \left( g_{A2}^2 Z_{Ls,i2}^{DR,*} Z_{Ls,j2}^{od} + g_{B2}^2 Z_{Ls,i4}^{DR,*} Z_{Ls,j2}^{od} - g_{B2}^2 Z_{Ls,i2}^{DR,*} Z_{Ls,j3}^{od} - g_{A2}^2 Z_{Ls,i4}^{DR,*} Z_{Ls,j3}^{od} \right. \\ & \left. + Z_{Ls,i1}^{DR,*} \left( g_{A2}^2 Z_{Ls,j4}^{od} - g_{B2}^2 Z_{Ls,j1}^{od} \right) + Z_{Ls,i3}^{DR,*} \left( -g_{A2}^2 Z_{Ls,j1}^{od} + g_{B2}^2 Z_{Ls,j4}^{od} \right) \right) \left( g_{\mu\nu} \right) \end{aligned} \quad (1138)$$


---

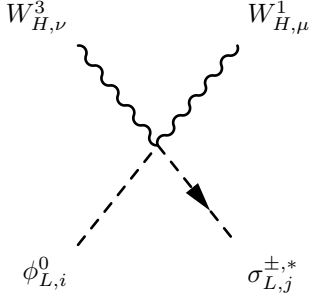

$$\frac{i}{2} g_{A2} g_{B2}^2 \sqrt{\frac{g_{A2}^2}{g_{A2}^2 + g_{B2}^2}} \frac{1}{\sqrt{g_{A2}^2 + g_{B2}^2}} \left( Z_{Ls,i1}^{DR,*} \left( Z_{Ls,j1}^{od} + Z_{Ls,j4}^{od} \right) - Z_{Ls,i3}^{DR,*} \left( Z_{Ls,j1}^{od} + Z_{Ls,j4}^{od} \right) + \left( -Z_{Ls,i4}^{DR,*} + Z_{Ls,i2}^{DR,*} \right) \left( Z_{Ls,j2}^{od} + Z_{Ls,j3}^{od} \right) \right) \quad (1139)$$


---

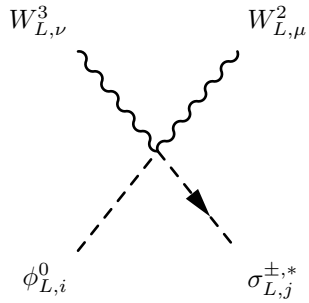

$$- \frac{1}{2} g_{A2} g_{B2}^2 \sqrt{\frac{g_{A2}^2}{g_{A2}^2 + g_{B2}^2}} \frac{1}{\sqrt{g_{A2}^2 + g_{B2}^2}} \left( Z_{Ls,i1}^{DR,*} \left( Z_{Ls,j1}^{od} + Z_{Ls,j4}^{od} \right) - Z_{Ls,i3}^{DR,*} \left( Z_{Ls,j1}^{od} + Z_{Ls,j4}^{od} \right) + \left( -Z_{Ls,i4}^{DR,*} + Z_{Ls,i2}^{DR,*} \right) \left( Z_{Ls,j2}^{od} + Z_{Ls,j3}^{od} \right) \right) \quad (1140)$$


---

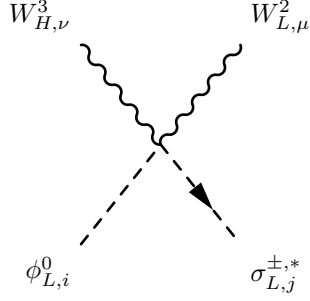

$$\frac{1}{2}g_{A2}g_{B2}\left(g_{A2}^2+g_{B2}^2\right)^{-1}\left(-g_{B2}^2Z_{Ls,i2}^{DR,*}Z_{Ls,j2}^{od}-g_{A2}^2Z_{Ls,i4}^{DR,*}Z_{Ls,j2}^{od}+g_{A2}^2Z_{Ls,i2}^{DR,*}Z_{Ls,j3}^{od}+g_{B2}^2Z_{Ls,i4}^{DR,*}Z_{Ls,j3}^{od}\right. \\ \left.+Z_{Ls,i3}^{DR,*}\left(-g_{A2}^2Z_{Ls,j4}^{od}+g_{B2}^2Z_{Ls,j1}^{od}\right)+Z_{Ls,i1}^{DR,*}\left(g_{A2}^2Z_{Ls,j1}^{od}-g_{B2}^2Z_{Ls,j4}^{od}\right)\right)\left(g_{\mu\nu}\right) \quad (1141)$$


---

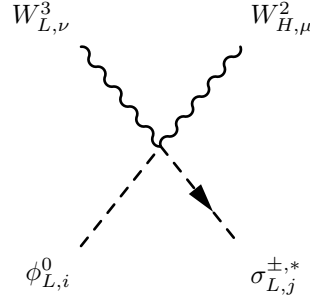

$$\frac{1}{2}g_{A2}g_{B2}\left(g_{A2}^2+g_{B2}^2\right)^{-1}\left(g_{A2}^2Z_{Ls,i2}^{DR,*}Z_{Ls,j2}^{od}+g_{B2}^2Z_{Ls,i4}^{DR,*}Z_{Ls,j2}^{od}-g_{B2}^2Z_{Ls,i2}^{DR,*}Z_{Ls,j3}^{od}-g_{A2}^2Z_{Ls,i4}^{DR,*}Z_{Ls,j3}^{od}\right. \\ \left.+Z_{Ls,i1}^{DR,*}\left(g_{A2}^2Z_{Ls,j4}^{od}-g_{B2}^2Z_{Ls,j1}^{od}\right)+Z_{Ls,i3}^{DR,*}\left(-g_{A2}^2Z_{Ls,j1}^{od}+g_{B2}^2Z_{Ls,j4}^{od}\right)\right)\left(g_{\mu\nu}\right) \quad (1142)$$


---

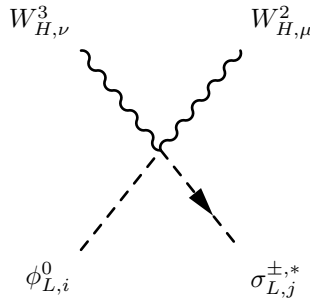

$$\frac{1}{2}g_{A2}g_{B2}^2\sqrt{\frac{g_{A2}^2}{g_{A2}^2+g_{B2}^2}}\frac{1}{\sqrt{g_{A2}^2+g_{B2}^2}}\left(Z_{Ls,i1}^{DR,*}\left(Z_{Ls,j1}^{od}+Z_{Ls,j4}^{od}\right)-Z_{Ls,i3}^{DR,*}\left(Z_{Ls,j1}^{od}+Z_{Ls,j4}^{od}\right)+\left(-Z_{Ls,i4}^{DR,*}+Z_{Ls,i2}^{DR,*}\right)\left(Z_{Ls,j2}^{od}+Z_{Ls,j3}^{od}\right)\right) \quad (1143)$$


---

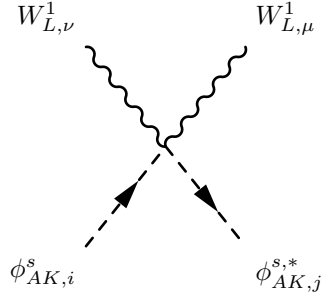

$$2ig_{A2}^2g_{B2}^2\left(g_{A2}^2+g_{B2}^2\right)^{-1}Z_{AK,i2}^{s,*}Z_{AK,j2}^s\left(g_{\mu\nu}\right) \quad (1144)$$


---

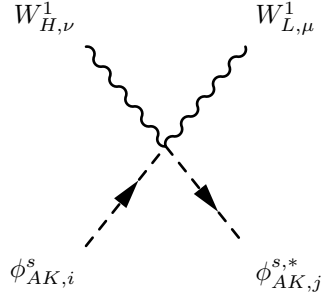

$$2ig_{B2}^3\sqrt{\frac{g_{A2}^2}{g_{A2}^2+g_{B2}^2}}\frac{1}{\sqrt{g_{A2}^2+g_{B2}^2}}Z_{AK,i2}^{s,*}Z_{AK,j2}^s\left(g_{\mu\nu}\right) \quad (1145)$$


---

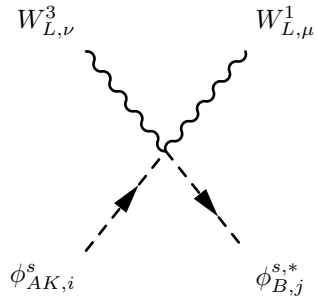

$$-i\frac{1}{\sqrt{2}}g_{A2}^2g_{B2}^2\left(g_{A2}^2+g_{B2}^2\right)^{-1}Z_{AK,i2}^{s,*}B_{A,j1}^s\left(g_{\mu\nu}\right) \quad (1146)$$


---



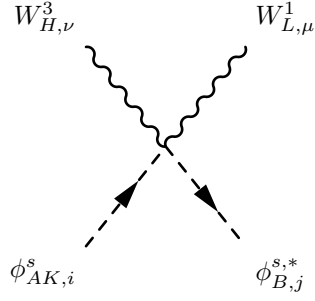

$$-i \frac{1}{\sqrt{2}} g_{B2}^3 \sqrt{\frac{gA2^2}{gA2^2 + gB2^2}} \frac{1}{\sqrt{gA2^2 + gB2^2}} Z_{AK,i2}^{s,*} B_{A,j1}^s (g_{\mu\nu}) \quad (1147)$$


---

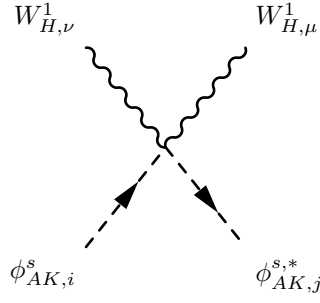

$$2ig_{B2}^4 (g_{A2}^2 + g_{B2}^2)^{-1} Z_{AK,i2}^{s,*} Z_{AK,j2}^s (g_{\mu\nu}) \quad (1148)$$


---

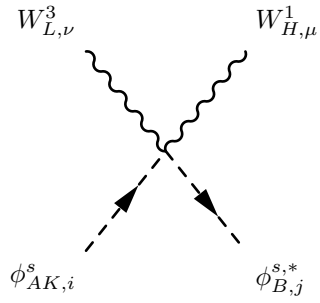

$$-i \frac{1}{\sqrt{2}} g_{B2}^3 \sqrt{\frac{gA2^2}{gA2^2 + gB2^2}} \frac{1}{\sqrt{gA2^2 + gB2^2}} Z_{AK,i2}^{s,*} B_{A,j1}^s (g_{\mu\nu}) \quad (1149)$$


---

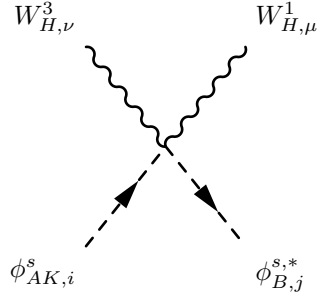

$$-i \frac{1}{\sqrt{2}} g_{B2}^4 \left( g_{A2}^2 + g_{B2}^2 \right)^{-1} Z_{AK,i2}^{s,*} B_{A,j1}^s \left( g_{\mu\nu} \right) \quad (1150)$$


---

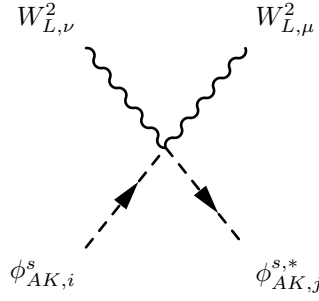

$$2i g_{A2}^2 g_{B2}^2 \left( g_{A2}^2 + g_{B2}^2 \right)^{-1} Z_{AK,i2}^{s,*} Z_{AK,j2}^s \left( g_{\mu\nu} \right) \quad (1151)$$


---

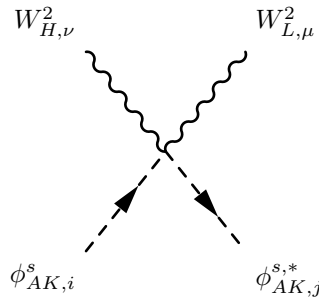

$$2i g_{B2}^3 \sqrt{\frac{g_{A2}^2}{g_{A2}^2 + g_{B2}^2}} \frac{1}{\sqrt{g_{A2}^2 + g_{B2}^2}} Z_{AK,i2}^{s,*} Z_{AK,j2}^s \left( g_{\mu\nu} \right) \quad (1152)$$


---

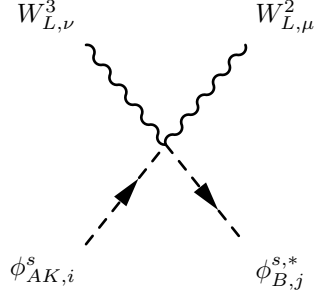

$$- \frac{1}{\sqrt{2}} g_{A2}^2 g_{B2}^2 (g_{A2}^2 + g_{B2}^2)^{-1} Z_{AK,i2}^{s,*} B_{A,j1}^s (g_{\mu\nu}) \quad (1153)$$


---

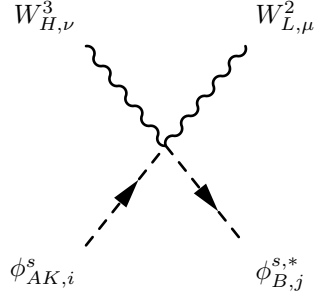

$$- \frac{1}{\sqrt{2}} g_{B2}^3 \sqrt{\frac{g_{A2}^2}{g_{A2}^2 + g_{B2}^2}} \frac{1}{\sqrt{g_{A2}^2 + g_{B2}^2}} Z_{AK,i2}^{s,*} B_{A,j1}^s (g_{\mu\nu}) \quad (1154)$$


---

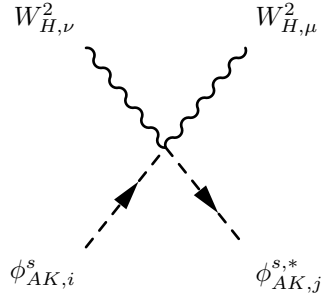

$$2i g_{B2}^4 (g_{A2}^2 + g_{B2}^2)^{-1} Z_{AK,i2}^{s,*} Z_{AK,j2}^s (g_{\mu\nu}) \quad (1155)$$


---

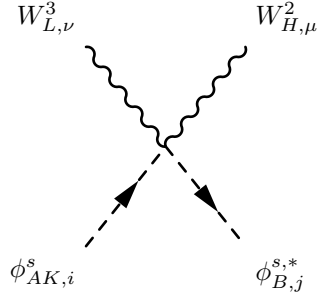

$$-\frac{1}{\sqrt{2}}g_{B2}^3\sqrt{\frac{g_{A2}^2}{g_{A2}^2+g_{B2}^2}}\frac{1}{\sqrt{g_{A2}^2+g_{B2}^2}}Z_{AK,i2}^{s,*}B_{A,j1}^s\left(g_{\mu\nu}\right) \quad (1156)$$


---

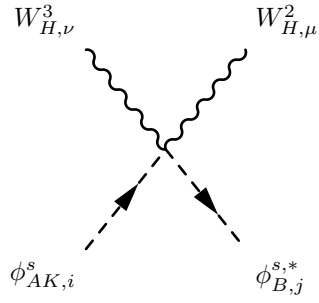

$$-\frac{1}{\sqrt{2}}g_{B2}^4\left(g_{A2}^2+g_{B2}^2\right)^{-1}Z_{AK,i2}^{s,*}B_{A,j1}^s\left(g_{\mu\nu}\right) \quad (1157)$$


---

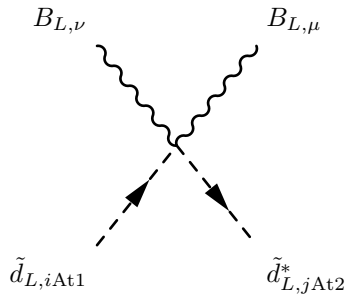

$$\frac{i}{18}g_{A1}^2g_{B1}^2\left(g_{A1}^2+g_{B1}^2\right)^{-1}\delta_{At1At2}\delta_{ij}\left(g_{\mu\nu}\right) \quad (1158)$$


---

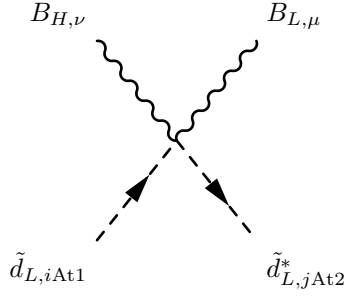

$$-\frac{i}{18}g_{B1}\left(\frac{gA1^2}{gA1^2+gB1^2}\right)^{3/2}\sqrt{gA1^2+gB1^2}\delta_{At1At2}\delta_{ij}\left(g_{\mu\nu}\right) \quad (1159)$$


---

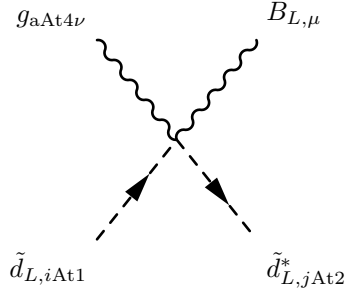

$$\frac{i}{6}g_3g_{A1}g_{B1}\frac{1}{\sqrt{gA1^2+gB1^2}}\delta_{ij}\lambda_{At2,At1}^{aAt4}\left(g_{\mu\nu}\right) \quad (1160)$$


---

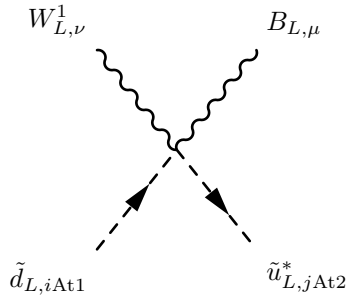

$$\frac{i}{6}g_{A1}g_{A2}g_{B1}\frac{1}{\sqrt{gA1^2+gB1^2}}g_{B2}\frac{1}{\sqrt{gA2^2+gB2^2}}\delta_{At1At2}\delta_{ij}\left(g_{\mu\nu}\right) \quad (1161)$$


---

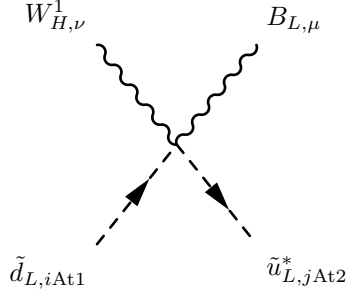

$$-\frac{i}{6}g_{A1}g_{A2}g_{B1}\frac{1}{\sqrt{g_{A1}^2+g_{B1}^2}}\sqrt{\frac{g_{A2}^2}{g_{A2}^2+g_{B2}^2}}\delta_{\text{At}1\text{At}2}\delta_{ij}\left(g_{\mu\nu}\right) \quad (1162)$$


---

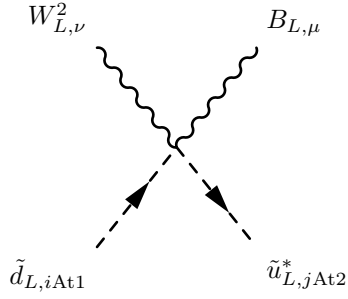

$$\frac{1}{6}g_{A1}g_{A2}g_{B1}\frac{1}{\sqrt{g_{A1}^2+g_{B1}^2}}g_{B2}\frac{1}{\sqrt{g_{A2}^2+g_{B2}^2}}\delta_{\text{At}1\text{At}2}\delta_{ij}\left(g_{\mu\nu}\right) \quad (1163)$$


---

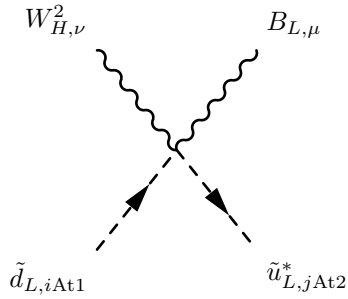

$$-\frac{1}{6}g_{A1}g_{A2}g_{B1}\frac{1}{\sqrt{g_{A1}^2+g_{B1}^2}}\sqrt{\frac{g_{A2}^2}{g_{A2}^2+g_{B2}^2}}\delta_{\text{At}1\text{At}2}\delta_{ij}\left(g_{\mu\nu}\right) \quad (1164)$$


---

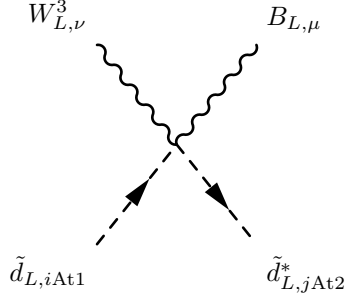

$$-\frac{i}{6}g_{A1}g_{A2}g_{B1}\frac{1}{\sqrt{g_{A1}^2+g_{B1}^2}}g_{B2}\frac{1}{\sqrt{g_{A2}^2+g_{B2}^2}}\delta_{\text{At}1\text{At}2}\delta_{ij}\left(g_{\mu\nu}\right) \quad (1165)$$


---

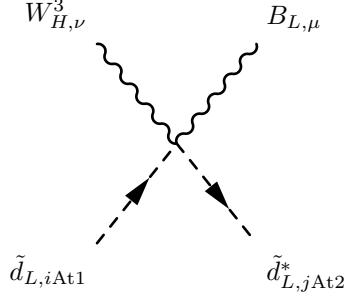

$$\frac{i}{6}g_{A1}g_{A2}g_{B1}\frac{1}{\sqrt{g_{A1}^2+g_{B1}^2}}\sqrt{\frac{g_{A2}^2}{g_{A2}^2+g_{B2}^2}}\delta_{\text{At}1\text{At}2}\delta_{ij}\left(g_{\mu\nu}\right) \quad (1166)$$


---

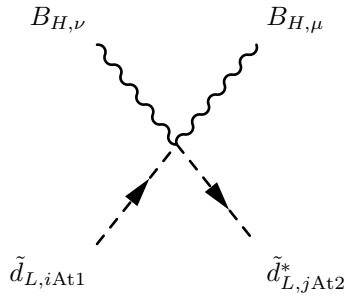

$$\frac{i}{18}g_{A1}^4\left(g_{A1}^2+g_{B1}^2\right)^{-1}\delta_{\text{At}1\text{At}2}\delta_{ij}\left(g_{\mu\nu}\right) \quad (1167)$$


---

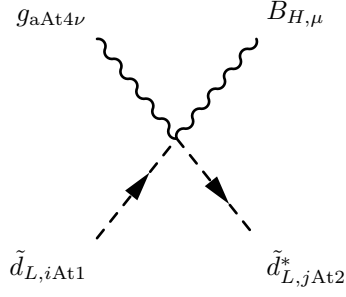

$$-\frac{i}{6}g_3g_{A1}\sqrt{\frac{g_{A1}^2}{g_{A1}^2+g_{B1}^2}}\delta_{ij}\lambda_{At2,At1}^{aAt4}\left(g_{\mu\nu}\right) \quad (1168)$$


---

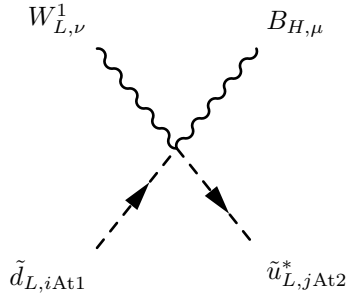

$$-\frac{i}{6}g_{A1}g_{A2}\sqrt{\frac{g_{A1}^2}{g_{A1}^2+g_{B1}^2}}g_{B2}\frac{1}{\sqrt{g_{A2}^2+g_{B2}^2}}\delta_{At1At2}\delta_{ij}\left(g_{\mu\nu}\right) \quad (1169)$$


---

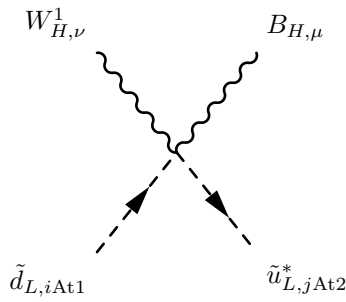

$$\frac{i}{6}g_{A1}g_{A2}\sqrt{\frac{g_{A1}^2}{g_{A1}^2+g_{B1}^2}}\sqrt{\frac{g_{A2}^2}{g_{A2}^2+g_{B2}^2}}\delta_{At1At2}\delta_{ij}\left(g_{\mu\nu}\right) \quad (1170)$$


---



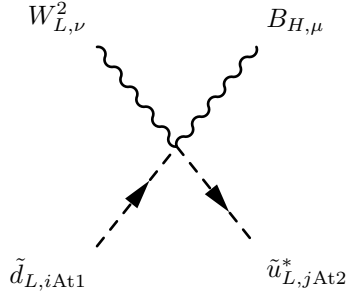

$$-\frac{1}{6}g_{A1}g_{A2}\sqrt{\frac{g_{A1}^2}{g_{A1}^2+g_{B1}^2}g_{B2}}\frac{1}{\sqrt{g_{A2}^2+g_{B2}^2}}\delta_{\text{At}1\text{At}2}\delta_{ij}\left(g_{\mu\nu}\right) \quad (1171)$$


---

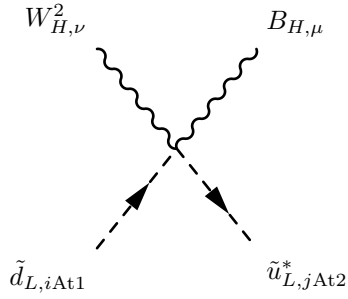

$$\frac{1}{6}g_{A1}g_{A2}\sqrt{\frac{g_{A1}^2}{g_{A1}^2+g_{B1}^2}}\sqrt{\frac{g_{A2}^2}{g_{A2}^2+g_{B2}^2}}\delta_{\text{At}1\text{At}2}\delta_{ij}\left(g_{\mu\nu}\right) \quad (1172)$$


---

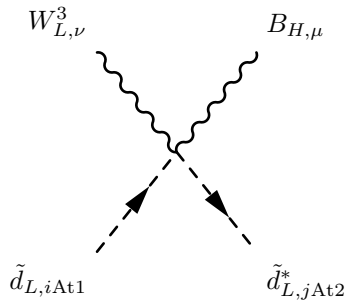

$$\frac{i}{6}g_{A1}g_{A2}\sqrt{\frac{g_{A1}^2}{g_{A1}^2+g_{B1}^2}g_{B2}}\frac{1}{\sqrt{g_{A2}^2+g_{B2}^2}}\delta_{\text{At}1\text{At}2}\delta_{ij}\left(g_{\mu\nu}\right) \quad (1173)$$


---

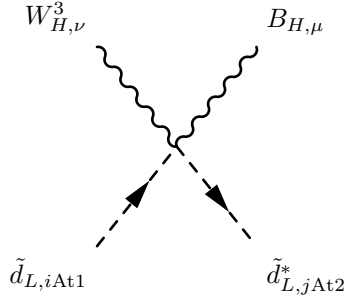

$$-\frac{i}{6}g_{A1}g_{A2}\sqrt{\frac{g_{A1}^2}{g_{A1}^2+g_{B1}^2}}\sqrt{\frac{g_{A2}^2}{g_{A2}^2+g_{B2}^2}}\delta_{\text{At}1\text{At}2}\delta_{ij}\left(g_{\mu\nu}\right) \quad (1174)$$


---

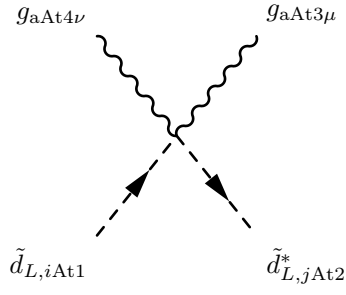

$$\frac{i}{4}g_3^2\delta_{ij}\left(\sum_{a=1}^3\lambda_{a,\text{At}1}^{\text{aAt}3}\lambda_{\text{At}2,a}^{\text{aAt}4}+\sum_{a=1}^3\lambda_{\text{At}2,a}^{\text{aAt}3}\lambda_{a,\text{At}1}^{\text{aAt}4}\right)\left(g_{\mu\nu}\right) \quad (1175)$$


---

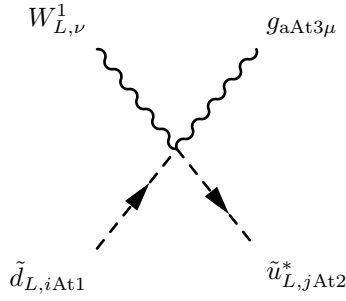

$$\frac{i}{2}g_3g_{A2}g_{B2}\frac{1}{\sqrt{g_{A2}^2+g_{B2}^2}}\delta_{ij}\lambda_{\text{At}2,\text{At}1}^{\text{aAt}3}\left(g_{\mu\nu}\right) \quad (1176)$$


---

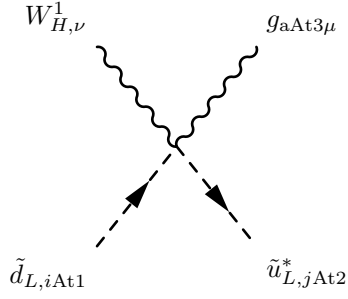

$$-\frac{i}{2}g_3g_{A2}\sqrt{\frac{g_{A2}^2}{g_{A2}^2+g_{B2}^2}}\delta_{ij}\lambda_{At2,At1}^{aAt3}\left(g_{\mu\nu}\right) \quad (1177)$$


---

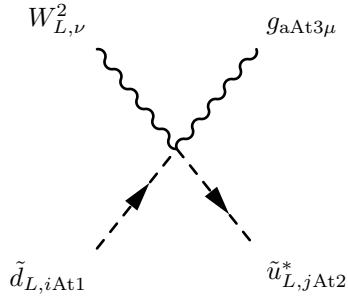

$$\frac{1}{2}g_3g_{A2}g_{B2}\frac{1}{\sqrt{g_{A2}^2+g_{B2}^2}}\delta_{ij}\lambda_{At2,At1}^{aAt3}\left(g_{\mu\nu}\right) \quad (1178)$$


---

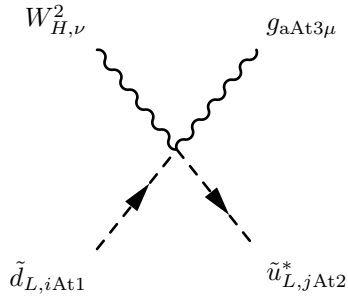

$$-\frac{1}{2}g_3g_{A2}\sqrt{\frac{g_{A2}^2}{g_{A2}^2+g_{B2}^2}}\delta_{ij}\lambda_{At2,At1}^{aAt3}\left(g_{\mu\nu}\right) \quad (1179)$$


---

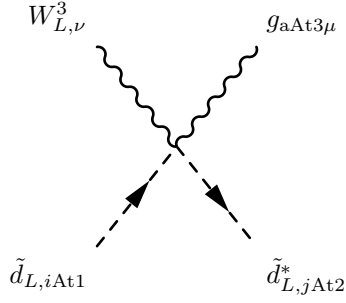

$$-\frac{i}{2}g_3g_{A2}g_{B2}\frac{1}{\sqrt{g_{A2}^2+g_{B2}^2}}\delta_{ij}\lambda_{At2,At1}^{aAt3}\left(g_{\mu\nu}\right) \quad (1180)$$


---

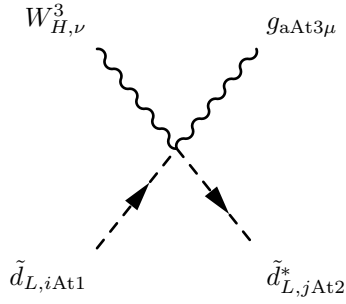

$$\frac{i}{2}g_3g_{A2}\sqrt{\frac{g_{A2}^2}{g_{A2}^2+g_{B2}^2}}\delta_{ij}\lambda_{At2,At1}^{aAt3}\left(g_{\mu\nu}\right) \quad (1181)$$


---

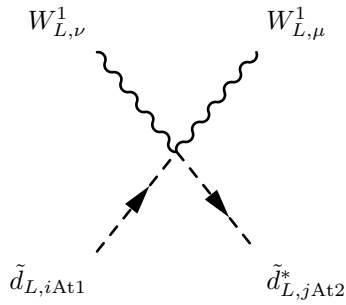

$$\frac{i}{2}g_{A2}^2g_{B2}^2\left(g_{A2}^2+g_{B2}^2\right)^{-1}\delta_{At1At2}\delta_{ij}\left(g_{\mu\nu}\right) \quad (1182)$$


---

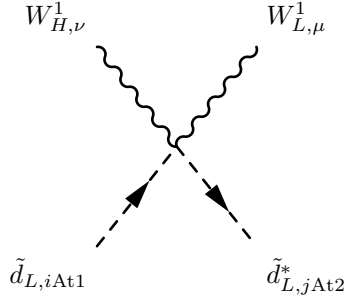

$$-\frac{i}{2}g_{B2}\left(\frac{g_{A2}^2}{g_{A2}^2+g_{B2}^2}\right)^{3/2}\sqrt{g_{A2}^2+g_{B2}^2}\delta_{\text{At}1\text{At}2}\delta_{ij}\left(g_{\mu\nu}\right) \quad (1183)$$


---

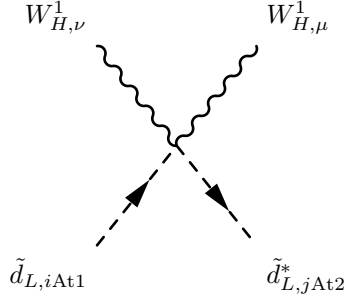

$$\frac{i}{2}g_{A2}^4\left(g_{A2}^2+g_{B2}^2\right)^{-1}\delta_{\text{At}1\text{At}2}\delta_{ij}\left(g_{\mu\nu}\right) \quad (1184)$$


---

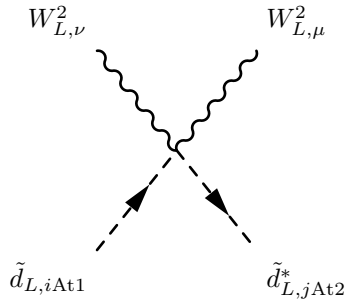

$$\frac{i}{2}g_{A2}^2g_{B2}^2\left(g_{A2}^2+g_{B2}^2\right)^{-1}\delta_{\text{At}1\text{At}2}\delta_{ij}\left(g_{\mu\nu}\right) \quad (1185)$$


---

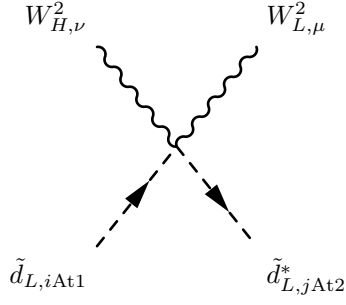

$$-\frac{i}{2}g_{B2}\left(\frac{g_{A2}^2}{g_{A2}^2+g_{B2}^2}\right)^{3/2}\sqrt{g_{A2}^2+g_{B2}^2}\delta_{At1At2}\delta_{ij}\left(g_{\mu\nu}\right) \quad (1186)$$


---

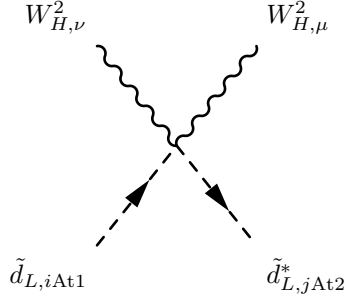

$$\frac{i}{2}g_{A2}^4\left(g_{A2}^2+g_{B2}^2\right)^{-1}\delta_{At1At2}\delta_{ij}\left(g_{\mu\nu}\right) \quad (1187)$$


---

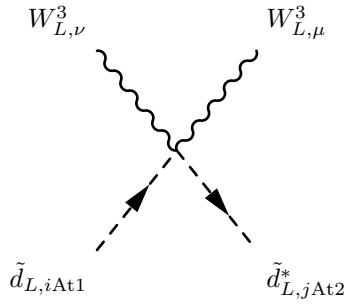

$$\frac{i}{2}g_{A2}^2g_{B2}^2\left(g_{A2}^2+g_{B2}^2\right)^{-1}\delta_{At1At2}\delta_{ij}\left(g_{\mu\nu}\right) \quad (1188)$$


---

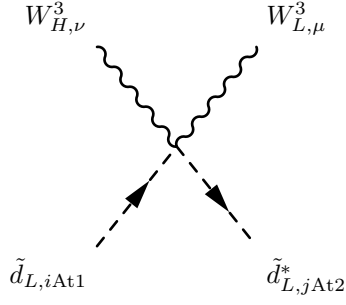

$$-\frac{i}{2}g_{B2}\left(\frac{g_{A2}^2}{g_{A2}^2+g_{B2}^2}\right)^{3/2}\sqrt{g_{A2}^2+g_{B2}^2}\delta_{\text{At}1\text{At}2}\delta_{ij}\left(g_{\mu\nu}\right) \quad (1189)$$


---

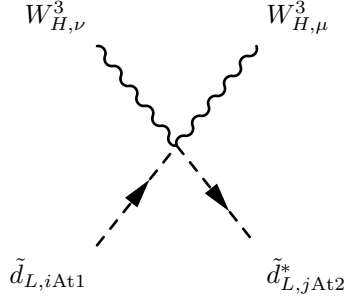

$$\frac{i}{2}g_{A2}^4\left(g_{A2}^2+g_{B2}^2\right)^{-1}\delta_{\text{At}1\text{At}2}\delta_{ij}\left(g_{\mu\nu}\right) \quad (1190)$$


---

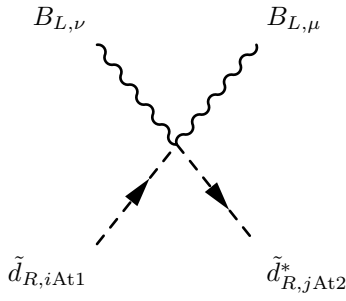

$$\frac{2i}{9}g_{A1}^2g_{B1}^2\left(g_{A1}^2+g_{B1}^2\right)^{-1}\delta_{\text{At}1\text{At}2}\delta_{ij}\left(g_{\mu\nu}\right) \quad (1191)$$


---

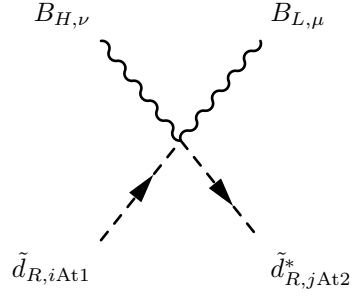

$$-\frac{2i}{9}g_{B1}\left(\frac{g_{A1}^2}{g_{A1}^2+g_{B1}^2}\right)^{3/2}\sqrt{g_{A1}^2+g_{B1}^2}\delta_{At1At2}\delta_{ij}\left(g_{\mu\nu}\right) \quad (1192)$$


---

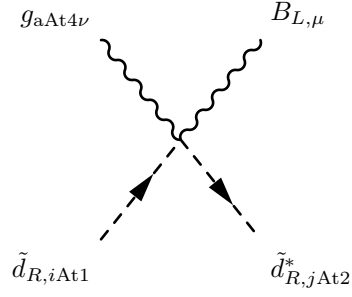

$$-\frac{i}{3}g_3g_{A1}g_{B1}\frac{1}{\sqrt{g_{A1}^2+g_{B1}^2}}\delta_{ij}\lambda_{At2,At1}^{aAt4}\left(g_{\mu\nu}\right) \quad (1193)$$


---

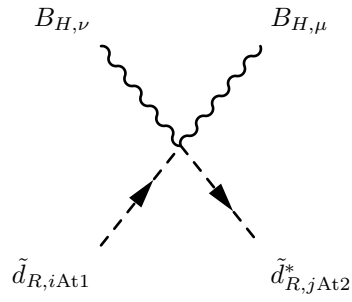

$$\frac{2i}{9}g_{A1}^4\left(g_{A1}^2+g_{B1}^2\right)^{-1}\delta_{At1At2}\delta_{ij}\left(g_{\mu\nu}\right) \quad (1194)$$


---



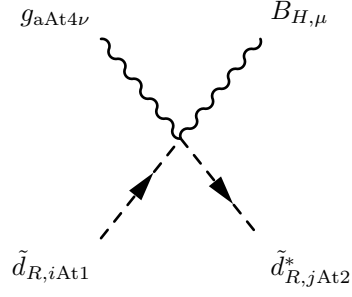

$$\frac{i}{3} g_3 g_{A1} \sqrt{\frac{g_{A1}^2}{g_{A1}^2 + g_{B1}^2}} \delta_{ij} \lambda_{At2,At1}^{aAt4} (g_{\mu\nu}) \quad (1195)$$


---

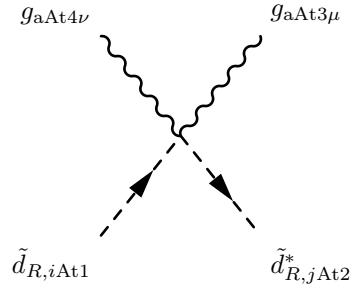

$$\frac{i}{4} g_3^2 \delta_{ij} \left( \sum_{a=1}^3 \lambda_{a,At1}^{aAt3} \lambda_{At2,a}^{aAt4} + \sum_{a=1}^3 \lambda_{At2,a}^{aAt3} \lambda_{a,At1}^{aAt4} \right) (g_{\mu\nu}) \quad (1196)$$


---

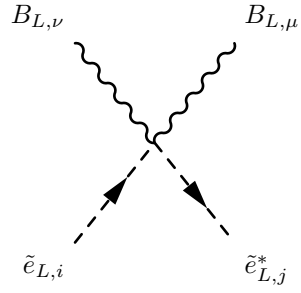

$$\frac{i}{2} g_{A1}^2 g_{B1}^2 (g_{A1}^2 + g_{B1}^2)^{-1} \delta_{ij} (g_{\mu\nu}) \quad (1197)$$


---

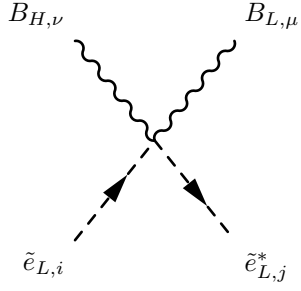

$$-\frac{i}{2}g_{B1}\left(\frac{gA1^2}{gA1^2+gB1^2}\right)^{3/2}\sqrt{gA1^2+gB1^2}\delta_{ij}\left(g_{\mu\nu}\right) \quad (1198)$$


---

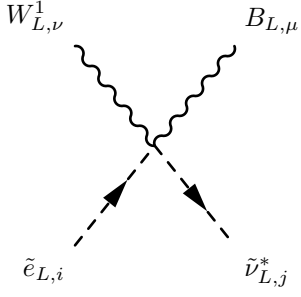

$$-\frac{i}{2}g_{A1}g_{A2}g_{B1}\frac{1}{\sqrt{gA1^2+gB1^2}}g_{B2}\frac{1}{\sqrt{gA2^2+gB2^2}}\delta_{ij}\left(g_{\mu\nu}\right) \quad (1199)$$


---

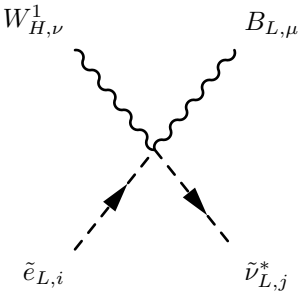

$$\frac{i}{2}g_{A1}g_{A2}g_{B1}\frac{1}{\sqrt{gA1^2+gB1^2}}\sqrt{\frac{gA2^2}{gA2^2+gB2^2}}\delta_{ij}\left(g_{\mu\nu}\right) \quad (1200)$$


---

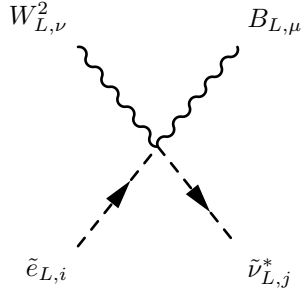

$$-\frac{1}{2}g_{A1}g_{A2}g_{B1}\frac{1}{\sqrt{g_{A1}^2+g_{B1}^2}}g_{B2}\frac{1}{\sqrt{g_{A2}^2+g_{B2}^2}}\delta_{ij}\left(g_{\mu\nu}\right) \quad (1201)$$


---

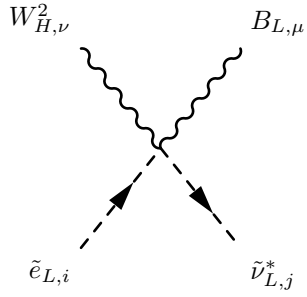

$$\frac{1}{2}g_{A1}g_{A2}g_{B1}\frac{1}{\sqrt{g_{A1}^2+g_{B1}^2}}\sqrt{\frac{g_{A2}^2}{g_{A2}^2+g_{B2}^2}}\delta_{ij}\left(g_{\mu\nu}\right) \quad (1202)$$


---

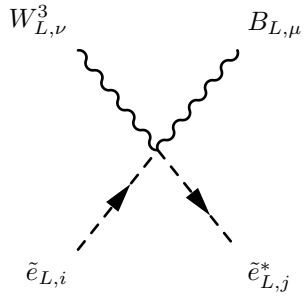

$$\frac{i}{2}g_{A1}g_{A2}g_{B1}\frac{1}{\sqrt{g_{A1}^2+g_{B1}^2}}g_{B2}\frac{1}{\sqrt{g_{A2}^2+g_{B2}^2}}\delta_{ij}\left(g_{\mu\nu}\right) \quad (1203)$$


---

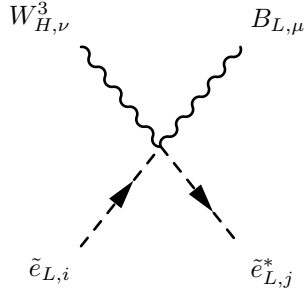

$$-\frac{i}{2}g_{A1}g_{A2}g_{B1}\frac{1}{\sqrt{g_{A1}^2+g_{B1}^2}}\sqrt{\frac{g_{A2}^2}{g_{A2}^2+g_{B2}^2}}\delta_{ij}\left(g_{\mu\nu}\right) \quad (1204)$$


---

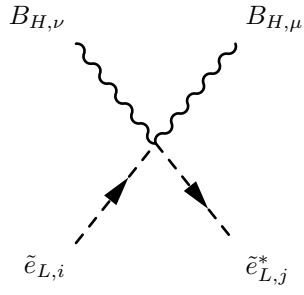

$$\frac{i}{2}g_{A1}^4\left(g_{A1}^2+g_{B1}^2\right)^{-1}\delta_{ij}\left(g_{\mu\nu}\right) \quad (1205)$$


---

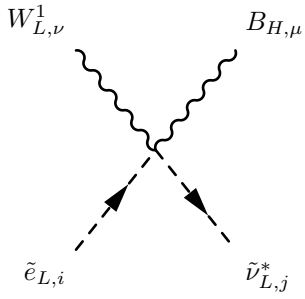

$$\frac{i}{2}g_{A1}g_{A2}\sqrt{\frac{g_{A1}^2}{g_{A1}^2+g_{B1}^2}}g_{B2}\frac{1}{\sqrt{g_{A2}^2+g_{B2}^2}}\delta_{ij}\left(g_{\mu\nu}\right) \quad (1206)$$


---

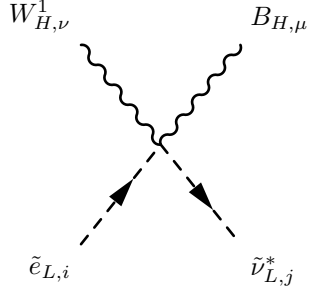

$$-\frac{i}{2}g_{A1}g_{A2}\sqrt{\frac{gA1^2}{gA1^2+gB1^2}}\sqrt{\frac{gA2^2}{gA2^2+gB2^2}}\delta_{ij}\left(g_{\mu\nu}\right) \quad (1207)$$


---

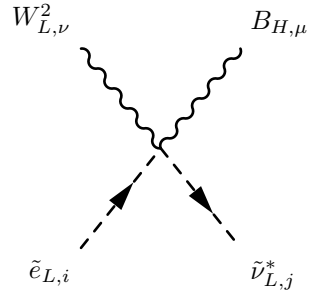

$$\frac{1}{2}g_{A1}g_{A2}\sqrt{\frac{gA1^2}{gA1^2+gB1^2}}\frac{1}{\sqrt{gA2^2+gB2^2}}\delta_{ij}\left(g_{\mu\nu}\right) \quad (1208)$$


---

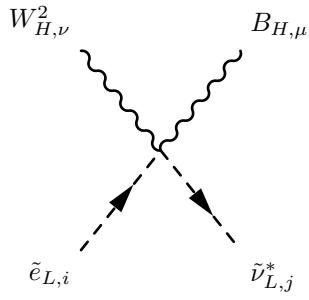

$$-\frac{1}{2}g_{A1}g_{A2}\sqrt{\frac{gA1^2}{gA1^2+gB1^2}}\sqrt{\frac{gA2^2}{gA2^2+gB2^2}}\delta_{ij}\left(g_{\mu\nu}\right) \quad (1209)$$


---

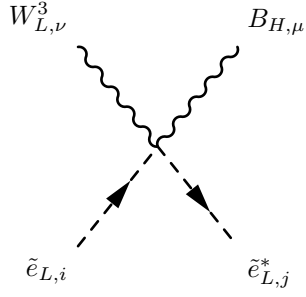

$$-\frac{i}{2}g_{A1}g_{A2}\sqrt{\frac{g_{A1}^2}{g_{A1}^2+g_{B1}^2}g_{B2}}\frac{1}{\sqrt{g_{A2}^2+g_{B2}^2}}\delta_{ij}\left(g_{\mu\nu}\right) \quad (1210)$$


---

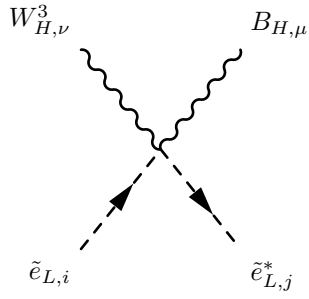

$$\frac{i}{2}g_{A1}g_{A2}\sqrt{\frac{g_{A1}^2}{g_{A1}^2+g_{B1}^2}}\sqrt{\frac{g_{A2}^2}{g_{A2}^2+g_{B2}^2}}\delta_{ij}\left(g_{\mu\nu}\right) \quad (1211)$$


---

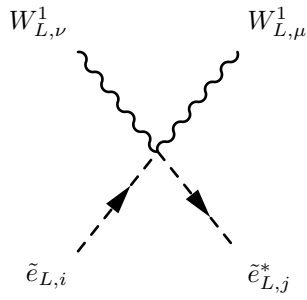

$$\frac{i}{2}g_{A2}^2g_{B2}^2\left(g_{A2}^2+g_{B2}^2\right)^{-1}\delta_{ij}\left(g_{\mu\nu}\right) \quad (1212)$$


---

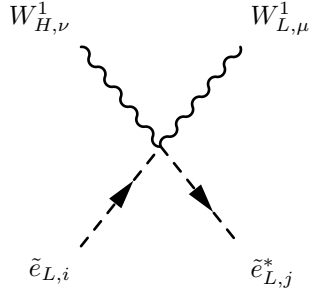

$$-\frac{i}{2}g_{B2}\left(\frac{gA2^2}{gA2^2+gB2^2}\right)^{3/2}\sqrt{gA2^2+gB2^2}\delta_{ij}\left(g_{\mu\nu}\right) \quad (1213)$$


---

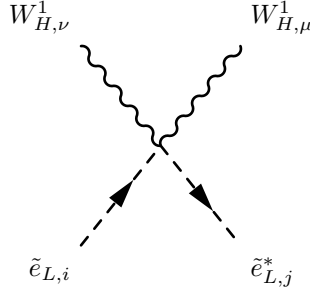

$$\frac{i}{2}g_{A2}^4\left(g_{A2}^2+g_{B2}^2\right)^{-1}\delta_{ij}\left(g_{\mu\nu}\right) \quad (1214)$$


---

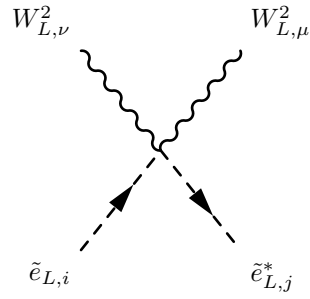

$$\frac{i}{2}g_{A2}^2g_{B2}^2\left(g_{A2}^2+g_{B2}^2\right)^{-1}\delta_{ij}\left(g_{\mu\nu}\right) \quad (1215)$$


---

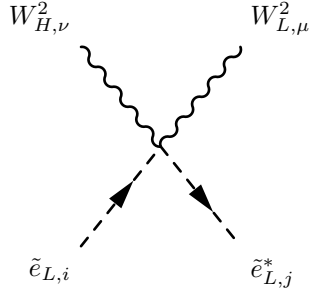

$$-\frac{i}{2}g_{B2}\left(\frac{gA2^2}{gA2^2+gB2^2}\right)^{3/2}\sqrt{gA2^2+gB2^2}\delta_{ij}\left(g_{\mu\nu}\right) \quad (1216)$$


---

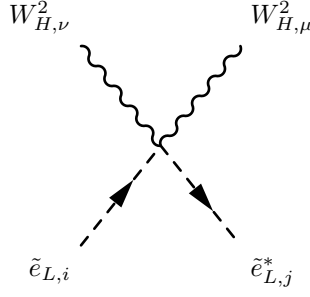

$$\frac{i}{2}g_{A2}^4\left(g_{A2}^2+g_{B2}^2\right)^{-1}\delta_{ij}\left(g_{\mu\nu}\right) \quad (1217)$$


---

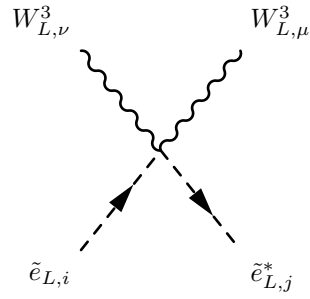

$$\frac{i}{2}g_{A2}^2g_{B2}^2\left(g_{A2}^2+g_{B2}^2\right)^{-1}\delta_{ij}\left(g_{\mu\nu}\right) \quad (1218)$$


---



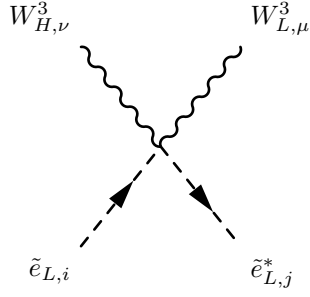

$$-\frac{i}{2}g_{B2}\left(\frac{gA2^2}{gA2^2+gB2^2}\right)^{3/2}\sqrt{gA2^2+gB2^2}\delta_{ij}\left(g_{\mu\nu}\right) \quad (1219)$$


---

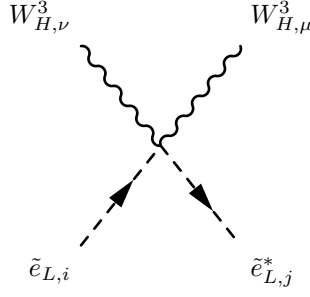

$$\frac{i}{2}g_{A2}^4\left(g_{A2}^2+g_{B2}^2\right)^{-1}\delta_{ij}\left(g_{\mu\nu}\right) \quad (1220)$$


---

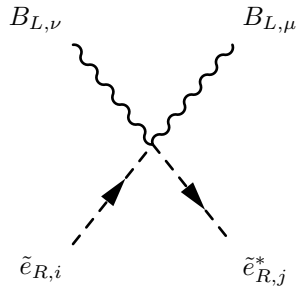

$$2ig_{A1}^2g_{B1}^2\left(g_{A1}^2+g_{B1}^2\right)^{-1}\delta_{ij}\left(g_{\mu\nu}\right) \quad (1221)$$


---

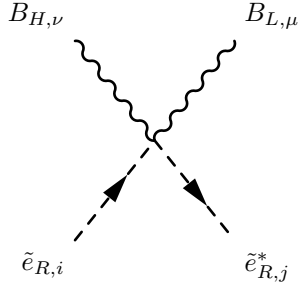

$$-2ig_{B1} \left( \frac{gA1^2}{gA1^2 + gB1^2} \right)^{3/2} \sqrt{gA1^2 + gB1^2} \delta_{ij} (g_{\mu\nu}) \quad (1222)$$


---

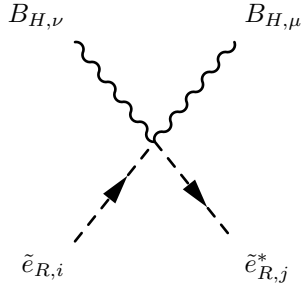

$$2ig_{A1}^4 (g_{A1}^2 + g_{B1}^2)^{-1} \delta_{ij} (g_{\mu\nu}) \quad (1223)$$


---

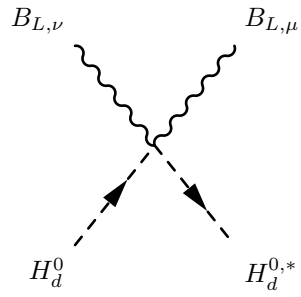

$$\frac{i}{2} g_{A1}^2 g_{B1}^2 (g_{A1}^2 + g_{B1}^2)^{-1} (g_{\mu\nu}) \quad (1224)$$


---

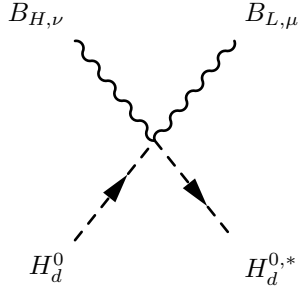

$$-\frac{i}{2}g_{B1}\left(\frac{gA1^2}{gA1^2+gB1^2}\right)^{3/2}\sqrt{gA1^2+gB1^2}(g_{\mu\nu}) \quad (1225)$$


---

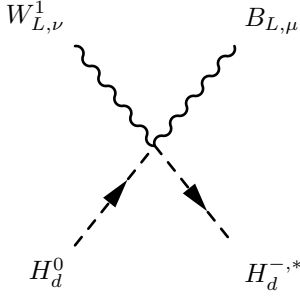

$$-\frac{i}{2}g_{A1}g_{A2}g_{B1}\frac{1}{\sqrt{gA1^2+gB1^2}}g_{B2}\frac{1}{\sqrt{gA2^2+gB2^2}}(g_{\mu\nu}) \quad (1226)$$


---

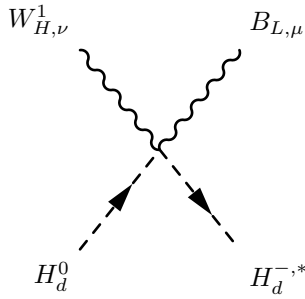

$$\frac{i}{2}g_{A1}g_{A2}g_{B1}\frac{1}{\sqrt{gA1^2+gB1^2}}\sqrt{\frac{gA2^2}{gA2^2+gB2^2}}(g_{\mu\nu}) \quad (1227)$$


---

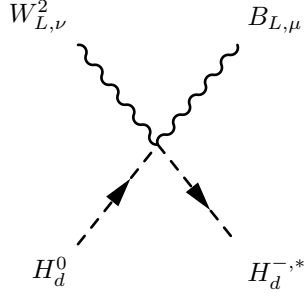

$$\frac{1}{2}g_{A1}g_{A2}g_{B1}\frac{1}{\sqrt{g_{A1}^2+g_{B1}^2}}g_{B2}\frac{1}{\sqrt{g_{A2}^2+g_{B2}^2}}(g_{\mu\nu}) \quad (1228)$$


---

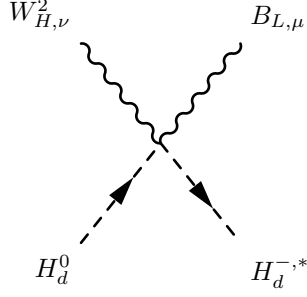

$$-\frac{1}{2}g_{A1}g_{A2}g_{B1}\frac{1}{\sqrt{g_{A1}^2+g_{B1}^2}}\sqrt{\frac{g_{A2}^2}{g_{A2}^2+g_{B2}^2}}(g_{\mu\nu}) \quad (1229)$$


---

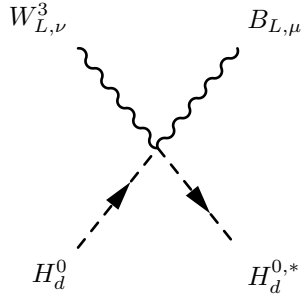

$$-\frac{i}{2}g_{A1}g_{A2}g_{B1}\frac{1}{\sqrt{g_{A1}^2+g_{B1}^2}}g_{B2}\frac{1}{\sqrt{g_{A2}^2+g_{B2}^2}}(g_{\mu\nu}) \quad (1230)$$


---

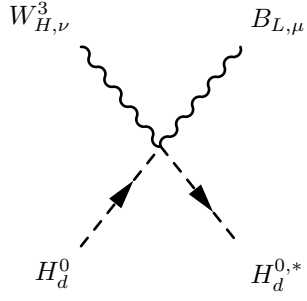

$$\frac{i}{2} g_{A1} g_{A2} g_{B1} \frac{1}{\sqrt{g_{A1}^2 + g_{B1}^2}} \sqrt{\frac{g_{A2}^2}{g_{A2}^2 + g_{B2}^2}} (g_{\mu\nu}) \quad (1231)$$


---

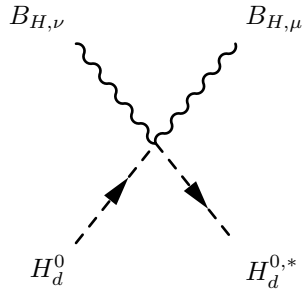

$$\frac{i}{2} g_{A1}^4 (g_{A1}^2 + g_{B1}^2)^{-1} (g_{\mu\nu}) \quad (1232)$$


---

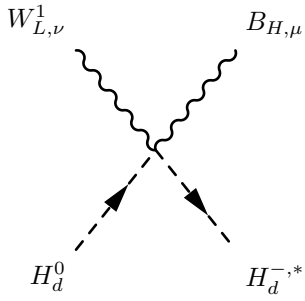

$$\frac{i}{2} g_{A1} g_{A2} \sqrt{\frac{g_{A1}^2}{g_{A1}^2 + g_{B1}^2}} g_{B2} \frac{1}{\sqrt{g_{A2}^2 + g_{B2}^2}} (g_{\mu\nu}) \quad (1233)$$


---

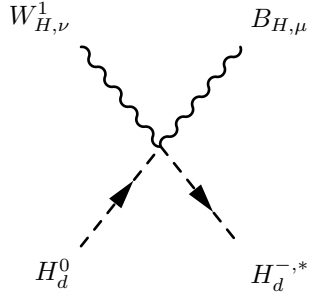

$$-\frac{i}{2}g_{A1}g_{A2}\sqrt{\frac{gA1^2}{gA1^2+gB1^2}}\sqrt{\frac{gA2^2}{gA2^2+gB2^2}}(g_{\mu\nu}) \quad (1234)$$


---

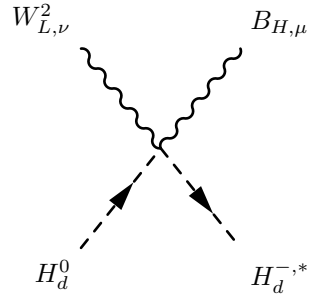

$$-\frac{1}{2}g_{A1}g_{A2}\sqrt{\frac{gA1^2}{gA1^2+gB1^2}}\frac{1}{\sqrt{gA2^2+gB2^2}}(g_{\mu\nu}) \quad (1235)$$


---

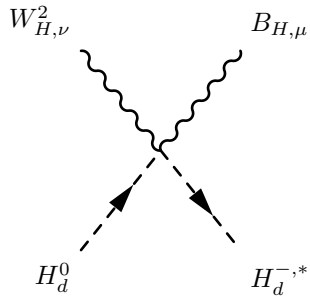

$$\frac{1}{2}g_{A1}g_{A2}\sqrt{\frac{gA1^2}{gA1^2+gB1^2}}\sqrt{\frac{gA2^2}{gA2^2+gB2^2}}(g_{\mu\nu}) \quad (1236)$$


---

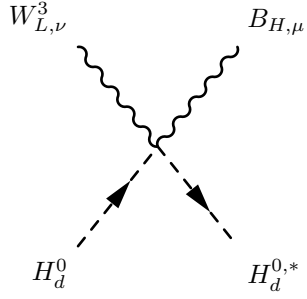

$$\frac{i}{2}g_{A1}g_{A2}\sqrt{\frac{g_{A1}^2}{g_{A1}^2+g_{B1}^2}g_{B2}}\frac{1}{\sqrt{g_{A2}^2+g_{B2}^2}}(g_{\mu\nu}) \quad (1237)$$


---

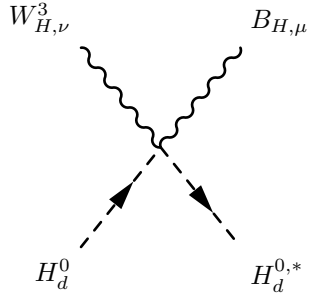

$$-\frac{i}{2}g_{A1}g_{A2}\sqrt{\frac{g_{A1}^2}{g_{A1}^2+g_{B1}^2}}\sqrt{\frac{g_{A2}^2}{g_{A2}^2+g_{B2}^2}}(g_{\mu\nu}) \quad (1238)$$


---

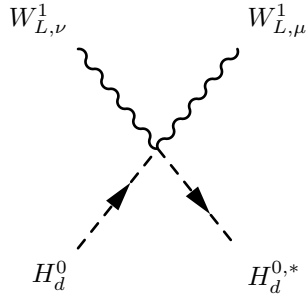

$$\frac{i}{2}g_{A2}^2g_{B2}^2(g_{A2}^2+g_{B2}^2)^{-1}(g_{\mu\nu}) \quad (1239)$$


---

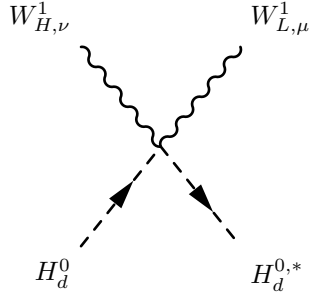

$$-\frac{i}{2}g_{B2}\left(\frac{g_{A2}^2}{g_{A2}^2+g_{B2}^2}\right)^{3/2}\sqrt{g_{A2}^2+g_{B2}^2}(g_{\mu\nu}) \quad (1240)$$


---

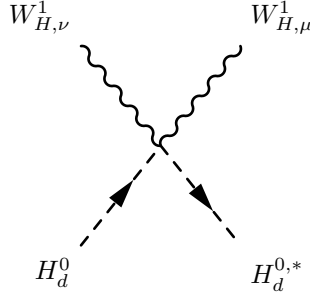

$$\frac{i}{2}g_{A2}^4(g_{A2}^2+g_{B2}^2)^{-1}(g_{\mu\nu}) \quad (1241)$$


---

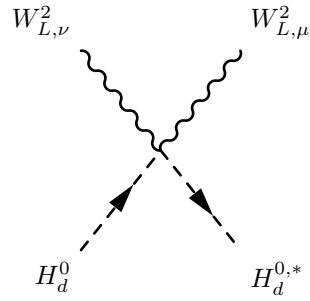

$$\frac{i}{2}g_{A2}^2g_{B2}^2(g_{A2}^2+g_{B2}^2)^{-1}(g_{\mu\nu}) \quad (1242)$$


---



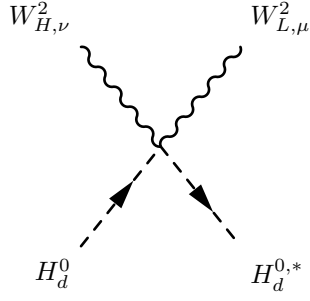

$$-\frac{i}{2}g_{B2}\left(\frac{g_{A2}^2}{g_{A2}^2+g_{B2}^2}\right)^{3/2}\sqrt{g_{A2}^2+g_{B2}^2}(g_{\mu\nu}) \quad (1243)$$


---

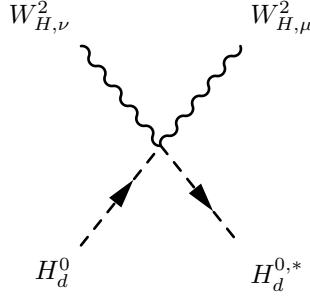

$$\frac{i}{2}g_{A2}^4(g_{A2}^2+g_{B2}^2)^{-1}(g_{\mu\nu}) \quad (1244)$$


---

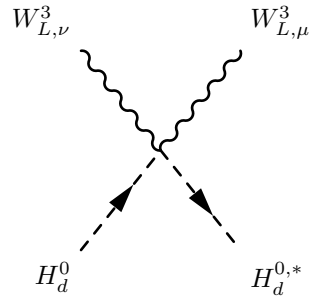

$$\frac{i}{2}g_{A2}^2g_{B2}^2(g_{A2}^2+g_{B2}^2)^{-1}(g_{\mu\nu}) \quad (1245)$$


---

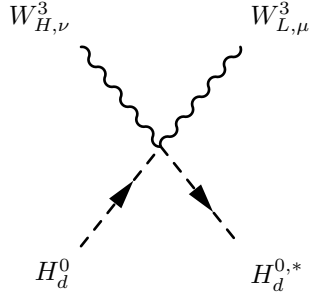

$$-\frac{i}{2}g_{B2}\left(\frac{gA2^2}{gA2^2+gB2^2}\right)^{3/2}\sqrt{gA2^2+gB2^2}\left(g_{\mu\nu}\right) \quad (1246)$$


---

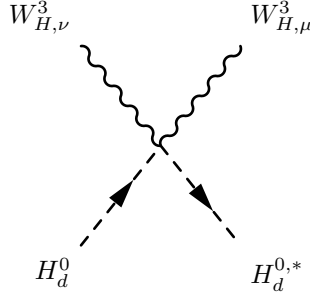

$$\frac{i}{2}g_{A2}^4\left(g_{A2}^2+g_{B2}^2\right)^{-1}\left(g_{\mu\nu}\right) \quad (1247)$$


---

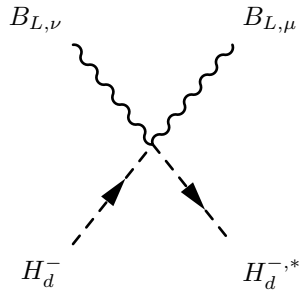

$$\frac{i}{2}g_{A1}^2g_{B1}^2\left(g_{A1}^2+g_{B1}^2\right)^{-1}\left(g_{\mu\nu}\right) \quad (1248)$$


---

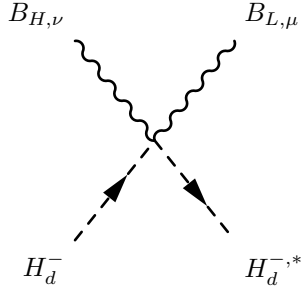

$$-\frac{i}{2}g_{B1}\left(\frac{gA1^2}{gA1^2+gB1^2}\right)^{3/2}\sqrt{gA1^2+gB1^2}(g_{\mu\nu}) \quad (1249)$$


---

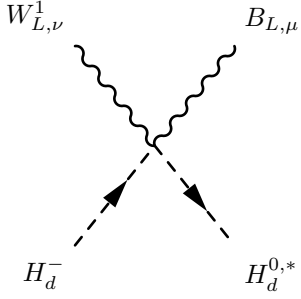

$$-\frac{i}{2}g_{A1}g_{A2}g_{B1}\frac{1}{\sqrt{gA1^2+gB1^2}}g_{B2}\frac{1}{\sqrt{gA2^2+gB2^2}}(g_{\mu\nu}) \quad (1250)$$


---

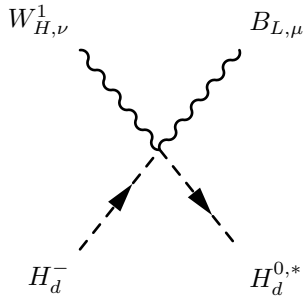

$$\frac{i}{2}g_{A1}g_{A2}g_{B1}\frac{1}{\sqrt{gA1^2+gB1^2}}\sqrt{\frac{gA2^2}{gA2^2+gB2^2}}(g_{\mu\nu}) \quad (1251)$$


---

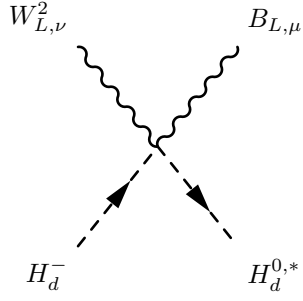

$$-\frac{1}{2}g_{A1}g_{A2}g_{B1}\frac{1}{\sqrt{g_{A1}^2+g_{B1}^2}}g_{B2}\frac{1}{\sqrt{g_{A2}^2+g_{B2}^2}}(g_{\mu\nu}) \quad (1252)$$


---

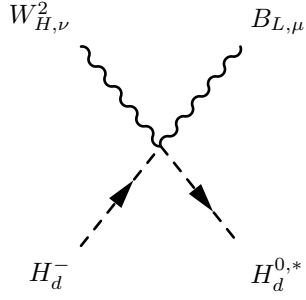

$$\frac{1}{2}g_{A1}g_{A2}g_{B1}\frac{1}{\sqrt{g_{A1}^2+g_{B1}^2}}\sqrt{\frac{g_{A2}^2}{g_{A2}^2+g_{B2}^2}}(g_{\mu\nu}) \quad (1253)$$


---

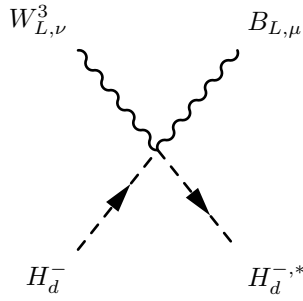

$$\frac{i}{2}g_{A1}g_{A2}g_{B1}\frac{1}{\sqrt{g_{A1}^2+g_{B1}^2}}g_{B2}\frac{1}{\sqrt{g_{A2}^2+g_{B2}^2}}(g_{\mu\nu}) \quad (1254)$$


---

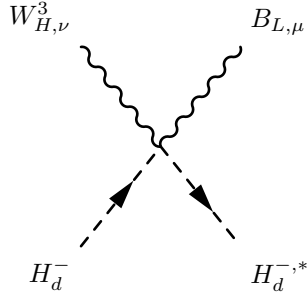

$$-\frac{i}{2}g_{A1}g_{A2}g_{B1}\frac{1}{\sqrt{g_{A1}^2+g_{B1}^2}}\sqrt{\frac{g_{A2}^2}{g_{A2}^2+g_{B2}^2}}(g_{\mu\nu}) \quad (1255)$$


---

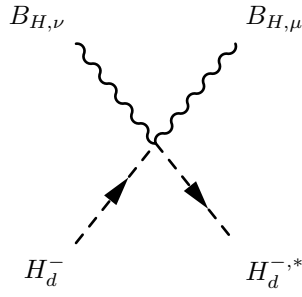

$$\frac{i}{2}g_{A1}^4(g_{A1}^2+g_{B1}^2)^{-1}(g_{\mu\nu}) \quad (1256)$$


---

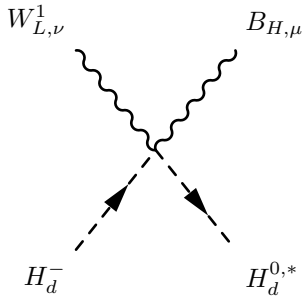

$$\frac{i}{2}g_{A1}g_{A2}\sqrt{\frac{g_{A1}^2}{g_{A1}^2+g_{B1}^2}}g_{B2}\frac{1}{\sqrt{g_{A2}^2+g_{B2}^2}}(g_{\mu\nu}) \quad (1257)$$


---

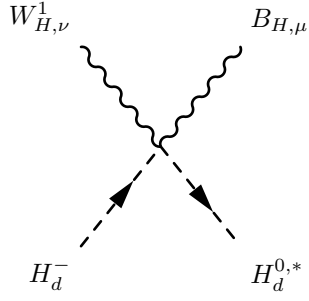

$$-\frac{i}{2}g_{A1}g_{A2}\sqrt{\frac{gA1^2}{gA1^2+gB1^2}}\sqrt{\frac{gA2^2}{gA2^2+gB2^2}}(g_{\mu\nu}) \quad (1258)$$


---

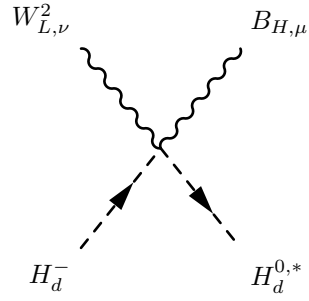

$$\frac{1}{2}g_{A1}g_{A2}\sqrt{\frac{gA1^2}{gA1^2+gB1^2}}\frac{1}{\sqrt{gA2^2+gB2^2}}(g_{\mu\nu}) \quad (1259)$$


---

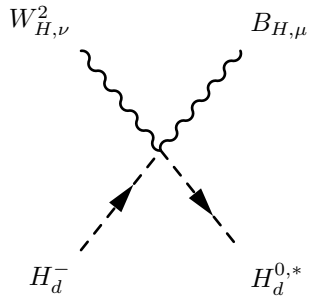

$$-\frac{1}{2}g_{A1}g_{A2}\sqrt{\frac{gA1^2}{gA1^2+gB1^2}}\sqrt{\frac{gA2^2}{gA2^2+gB2^2}}(g_{\mu\nu}) \quad (1260)$$


---

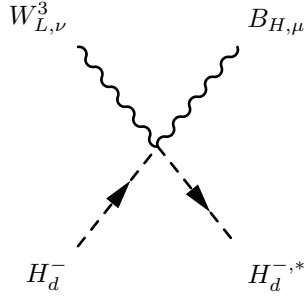

$$-\frac{i}{2}g_{A1}g_{A2}\sqrt{\frac{g_{A1}^2}{g_{A1}^2+g_{B1}^2}}g_{B2}\frac{1}{\sqrt{g_{A2}^2+g_{B2}^2}}(g_{\mu\nu}) \quad (1261)$$


---

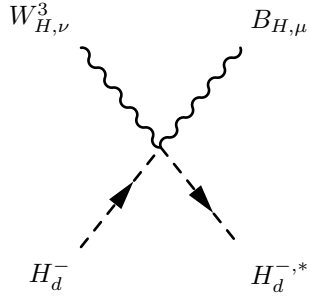

$$\frac{i}{2}g_{A1}g_{A2}\sqrt{\frac{g_{A1}^2}{g_{A1}^2+g_{B1}^2}}\sqrt{\frac{g_{A2}^2}{g_{A2}^2+g_{B2}^2}}(g_{\mu\nu}) \quad (1262)$$


---

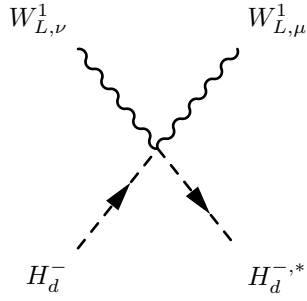

$$\frac{i}{2}g_{A2}^2g_{B2}^2(g_{A2}^2+g_{B2}^2)^{-1}(g_{\mu\nu}) \quad (1263)$$


---

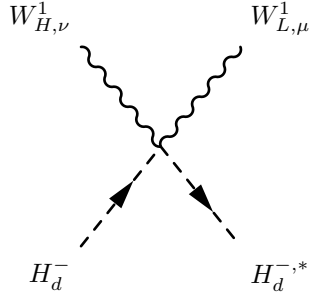

$$-\frac{i}{2}g_{B2}\left(\frac{gA2^2}{gA2^2+gB2^2}\right)^{3/2}\sqrt{gA2^2+gB2^2}(g_{\mu\nu}) \quad (1264)$$


---

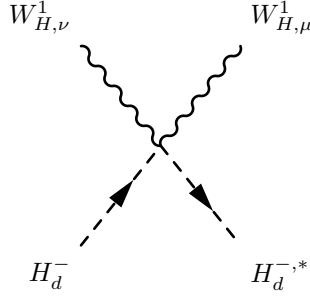

$$\frac{i}{2}g_{A2}^4(g_{A2}^2+g_{B2}^2)^{-1}(g_{\mu\nu}) \quad (1265)$$


---

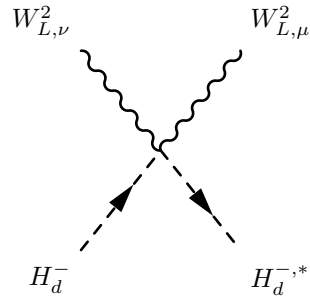

$$\frac{i}{2}g_{A2}^2g_{B2}^2(g_{A2}^2+g_{B2}^2)^{-1}(g_{\mu\nu}) \quad (1266)$$


---



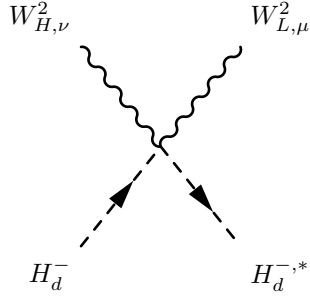

$$-\frac{i}{2}g_{B2}\left(\frac{gA2^2}{gA2^2+gB2^2}\right)^{3/2}\sqrt{gA2^2+gB2^2}(g_{\mu\nu}) \quad (1267)$$


---

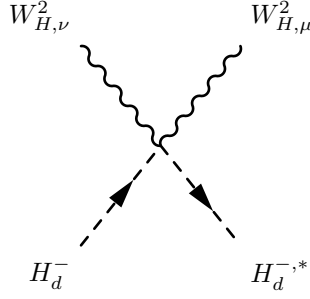

$$\frac{i}{2}g_{A2}^4(g_{A2}^2+g_{B2}^2)^{-1}(g_{\mu\nu}) \quad (1268)$$


---

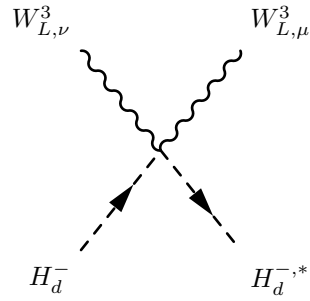

$$\frac{i}{2}g_{A2}^2g_{B2}^2(g_{A2}^2+g_{B2}^2)^{-1}(g_{\mu\nu}) \quad (1269)$$


---

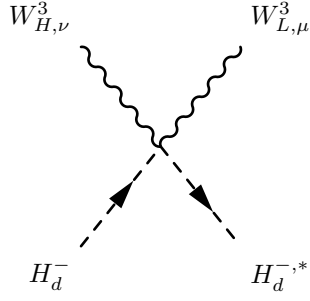

$$-\frac{i}{2}g_{B2}\left(\frac{g_{A2^2}}{g_{A2^2}+g_{B2^2}}\right)^{3/2}\sqrt{g_{A2^2}+g_{B2^2}}\left(g_{\mu\nu}\right) \quad (1270)$$


---

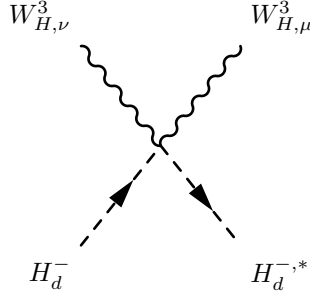

$$\frac{i}{2}g_{A2}^4\left(g_{A2}^2+g_{B2}^2\right)^{-1}\left(g_{\mu\nu}\right) \quad (1271)$$


---

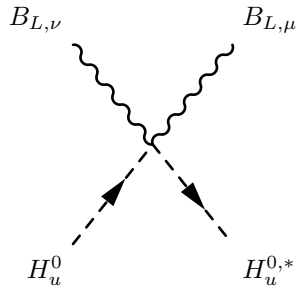

$$\frac{i}{2}g_{A1}^2g_{B1}^2\left(g_{A1}^2+g_{B1}^2\right)^{-1}\left(g_{\mu\nu}\right) \quad (1272)$$


---

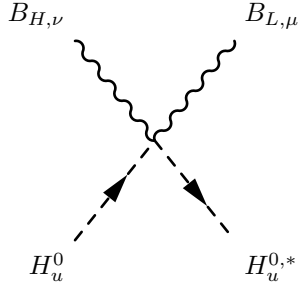

$$-\frac{i}{2}g_{B1}\left(\frac{gA1^2}{gA1^2+gB1^2}\right)^{3/2}\sqrt{gA1^2+gB1^2}(g_{\mu\nu}) \quad (1273)$$


---

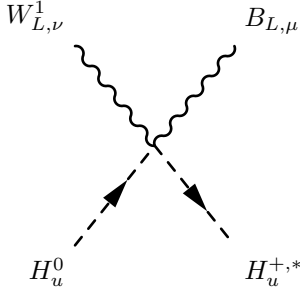

$$\frac{i}{2}g_{A1}g_{A2}g_{B1}\frac{1}{\sqrt{gA1^2+gB1^2}}g_{B2}\frac{1}{\sqrt{gA2^2+gB2^2}}(g_{\mu\nu}) \quad (1274)$$


---

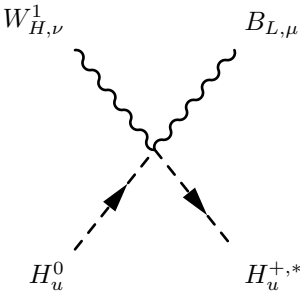

$$-\frac{i}{2}g_{A1}g_{A2}g_{B1}\frac{1}{\sqrt{gA1^2+gB1^2}}\sqrt{\frac{gA2^2}{gA2^2+gB2^2}}(g_{\mu\nu}) \quad (1275)$$


---

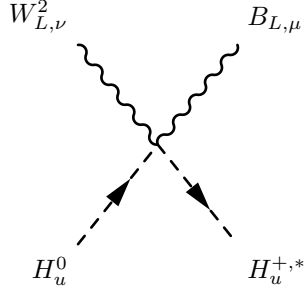

$$\frac{1}{2}g_{A1}g_{A2}g_{B1}\frac{1}{\sqrt{g_{A1}^2+g_{B1}^2}}g_{B2}\frac{1}{\sqrt{g_{A2}^2+g_{B2}^2}}(g_{\mu\nu}) \quad (1276)$$


---

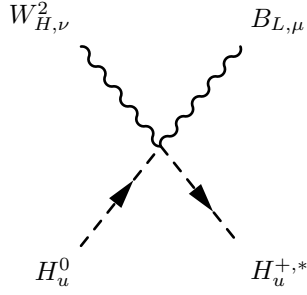

$$-\frac{1}{2}g_{A1}g_{A2}g_{B1}\frac{1}{\sqrt{g_{A1}^2+g_{B1}^2}}\sqrt{\frac{g_{A2}^2}{g_{A2}^2+g_{B2}^2}}(g_{\mu\nu}) \quad (1277)$$


---

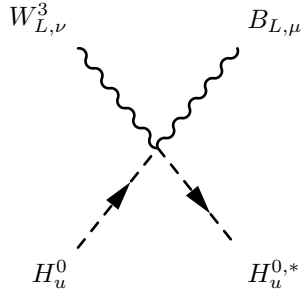

$$-\frac{i}{2}g_{A1}g_{A2}g_{B1}\frac{1}{\sqrt{g_{A1}^2+g_{B1}^2}}g_{B2}\frac{1}{\sqrt{g_{A2}^2+g_{B2}^2}}(g_{\mu\nu}) \quad (1278)$$


---

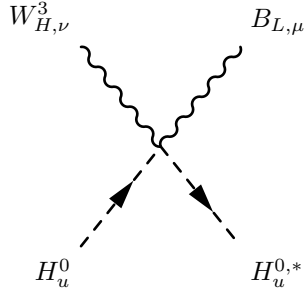

$$\frac{i}{2} g_{A1} g_{A2} g_{B1} \frac{1}{\sqrt{g_{A1}^2 + g_{B1}^2}} \sqrt{\frac{g_{A2}^2}{g_{A2}^2 + g_{B2}^2}} (g_{\mu\nu}) \quad (1279)$$


---

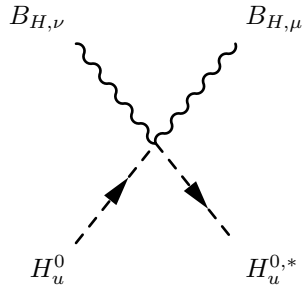

$$\frac{i}{2} g_{A1}^4 (g_{A1}^2 + g_{B1}^2)^{-1} (g_{\mu\nu}) \quad (1280)$$


---

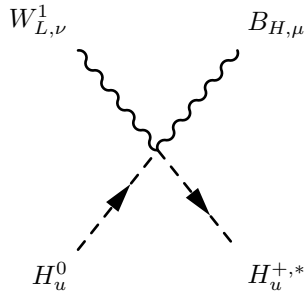

$$- \frac{i}{2} g_{A1} g_{A2} \sqrt{\frac{g_{A1}^2}{g_{A1}^2 + g_{B1}^2}} g_{B2} \frac{1}{\sqrt{g_{A2}^2 + g_{B2}^2}} (g_{\mu\nu}) \quad (1281)$$


---

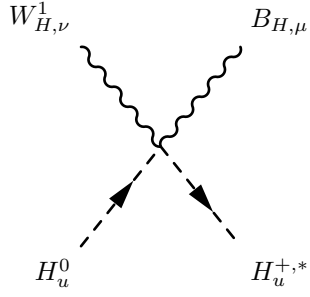

$$\frac{i}{2} g_{A1} g_{A2} \sqrt{\frac{gA1^2}{gA1^2 + gB1^2}} \sqrt{\frac{gA2^2}{gA2^2 + gB2^2}} (g_{\mu\nu}) \quad (1282)$$


---

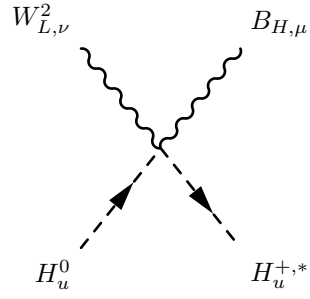

$$-\frac{1}{2} g_{A1} g_{A2} \sqrt{\frac{gA1^2}{gA1^2 + gB1^2}} g_{B2} \frac{1}{\sqrt{gA2^2 + gB2^2}} (g_{\mu\nu}) \quad (1283)$$


---

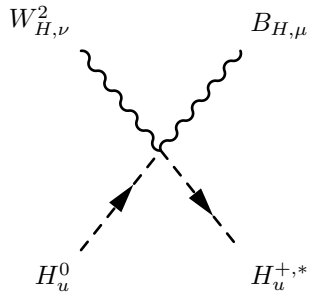

$$\frac{1}{2} g_{A1} g_{A2} \sqrt{\frac{gA1^2}{gA1^2 + gB1^2}} \sqrt{\frac{gA2^2}{gA2^2 + gB2^2}} (g_{\mu\nu}) \quad (1284)$$


---

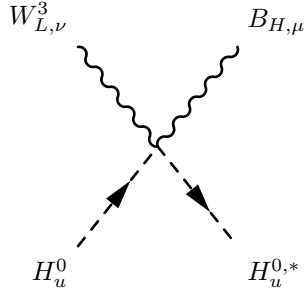

$$\frac{i}{2}g_{A1}g_{A2}\sqrt{\frac{g_{A1}^2}{g_{A1}^2+g_{B1}^2}g_{B2}}\frac{1}{\sqrt{g_{A2}^2+g_{B2}^2}}(g_{\mu\nu}) \quad (1285)$$


---

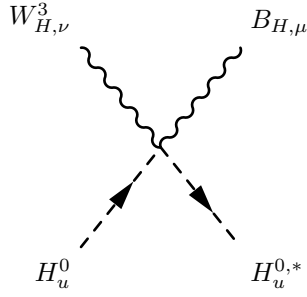

$$-\frac{i}{2}g_{A1}g_{A2}\sqrt{\frac{g_{A1}^2}{g_{A1}^2+g_{B1}^2}}\sqrt{\frac{g_{A2}^2}{g_{A2}^2+g_{B2}^2}}(g_{\mu\nu}) \quad (1286)$$


---

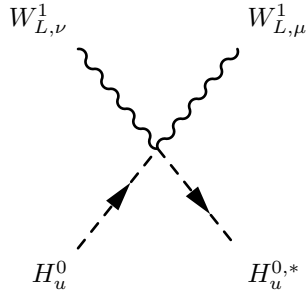

$$\frac{i}{2}g_{A2}^2g_{B2}^2(g_{A2}^2+g_{B2}^2)^{-1}(g_{\mu\nu}) \quad (1287)$$


---

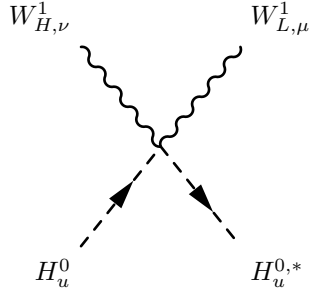

$$-\frac{i}{2}g_{B2}\left(\frac{gA2^2}{gA2^2+gB2^2}\right)^{3/2}\sqrt{gA2^2+gB2^2}\left(g_{\mu\nu}\right) \quad (1288)$$


---

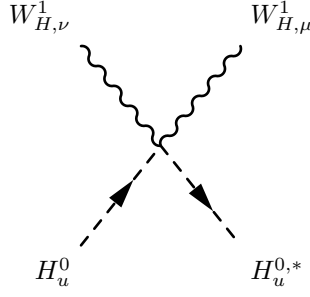

$$\frac{i}{2}g_{A2}^4\left(g_{A2}^2+g_{B2}^2\right)^{-1}\left(g_{\mu\nu}\right) \quad (1289)$$


---

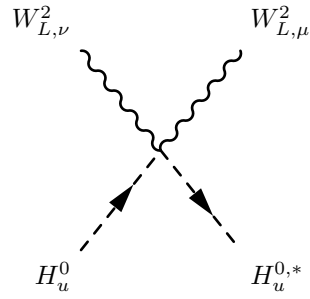

$$\frac{i}{2}g_{A2}^2g_{B2}^2\left(g_{A2}^2+g_{B2}^2\right)^{-1}\left(g_{\mu\nu}\right) \quad (1290)$$


---



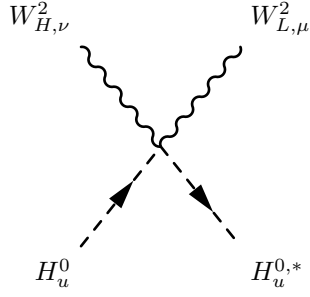

$$-\frac{i}{2}g_{B2}\left(\frac{g_{A2}^2}{g_{A2}^2+g_{B2}^2}\right)^{3/2}\sqrt{g_{A2}^2+g_{B2}^2}(g_{\mu\nu}) \quad (1291)$$


---

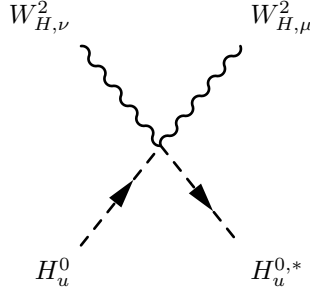

$$\frac{i}{2}g_{A2}^4\left(g_{A2}^2+g_{B2}^2\right)^{-1}(g_{\mu\nu}) \quad (1292)$$


---

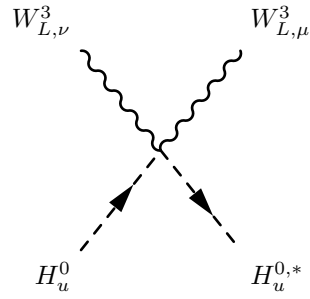

$$\frac{i}{2}g_{A2}^2g_{B2}^2\left(g_{A2}^2+g_{B2}^2\right)^{-1}(g_{\mu\nu}) \quad (1293)$$


---

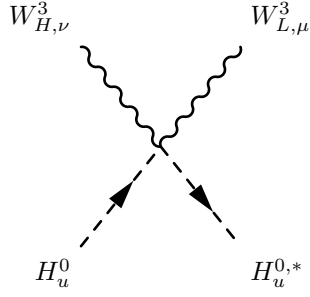

$$-\frac{i}{2}g_{B2}\left(\frac{gA2^2}{gA2^2+gB2^2}\right)^{3/2}\sqrt{gA2^2+gB2^2}\left(g_{\mu\nu}\right) \quad (1294)$$


---

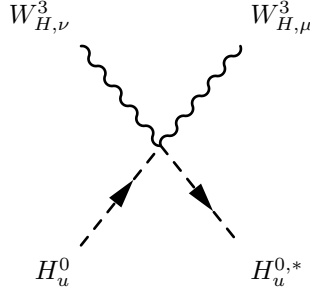

$$\frac{i}{2}g_{A2}^4\left(g_{A2}^2+g_{B2}^2\right)^{-1}\left(g_{\mu\nu}\right) \quad (1295)$$


---

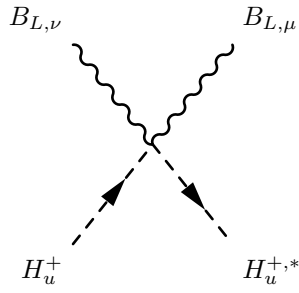

$$\frac{i}{2}g_{A1}^2g_{B1}^2\left(g_{A1}^2+g_{B1}^2\right)^{-1}\left(g_{\mu\nu}\right) \quad (1296)$$


---

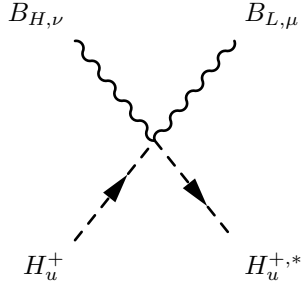

$$-\frac{i}{2}g_{B1}\left(\frac{gA1^2}{gA1^2+gB1^2}\right)^{3/2}\sqrt{gA1^2+gB1^2}(g_{\mu\nu}) \quad (1297)$$


---

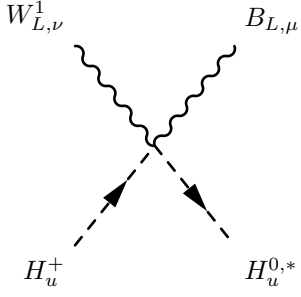

$$\frac{i}{2}g_{A1}g_{A2}g_{B1}\frac{1}{\sqrt{gA1^2+gB1^2}}g_{B2}\frac{1}{\sqrt{gA2^2+gB2^2}}(g_{\mu\nu}) \quad (1298)$$


---

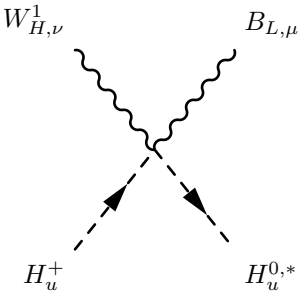

$$-\frac{i}{2}g_{A1}g_{A2}g_{B1}\frac{1}{\sqrt{gA1^2+gB1^2}}\sqrt{\frac{gA2^2}{gA2^2+gB2^2}}(g_{\mu\nu}) \quad (1299)$$


---

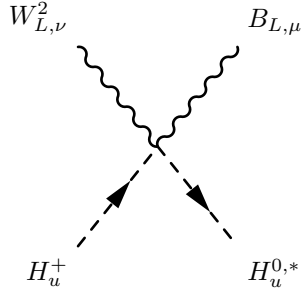

$$-\frac{1}{2}g_{A1}g_{A2}g_{B1}\frac{1}{\sqrt{g_{A1}^2+g_{B1}^2}}g_{B2}\frac{1}{\sqrt{g_{A2}^2+g_{B2}^2}}(g_{\mu\nu}) \quad (1300)$$


---

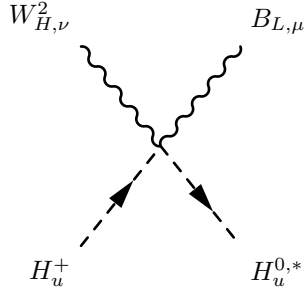

$$\frac{1}{2}g_{A1}g_{A2}g_{B1}\frac{1}{\sqrt{g_{A1}^2+g_{B1}^2}}\sqrt{\frac{g_{A2}^2}{g_{A2}^2+g_{B2}^2}}(g_{\mu\nu}) \quad (1301)$$


---

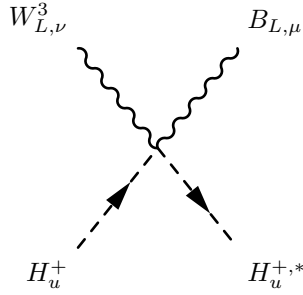

$$\frac{i}{2}g_{A1}g_{A2}g_{B1}\frac{1}{\sqrt{g_{A1}^2+g_{B1}^2}}g_{B2}\frac{1}{\sqrt{g_{A2}^2+g_{B2}^2}}(g_{\mu\nu}) \quad (1302)$$


---

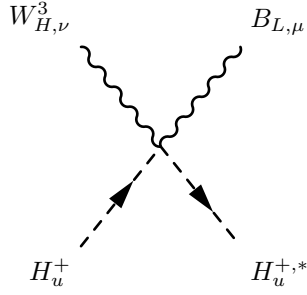

$$-\frac{i}{2}g_{A1}g_{A2}g_{B1}\frac{1}{\sqrt{g_{A1}^2+g_{B1}^2}}\sqrt{\frac{g_{A2}^2}{g_{A2}^2+g_{B2}^2}}(g_{\mu\nu}) \quad (1303)$$


---

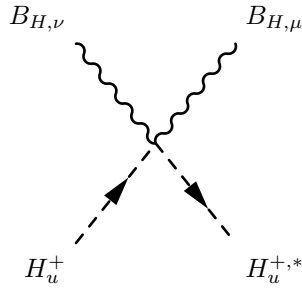

$$\frac{i}{2}g_{A1}^4(g_{A1}^2+g_{B1}^2)^{-1}(g_{\mu\nu}) \quad (1304)$$


---

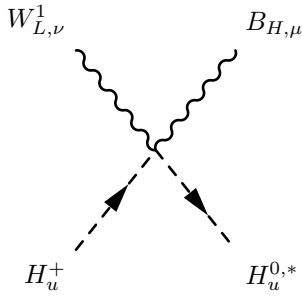

$$-\frac{i}{2}g_{A1}g_{A2}\sqrt{\frac{g_{A1}^2}{g_{A1}^2+g_{B1}^2}}g_{B2}\frac{1}{\sqrt{g_{A2}^2+g_{B2}^2}}(g_{\mu\nu}) \quad (1305)$$


---

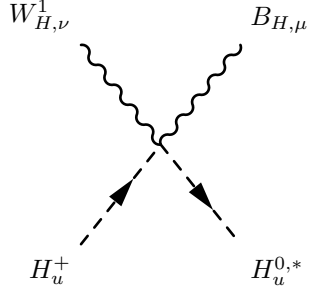

$$\frac{i}{2} g_{A1} g_{A2} \sqrt{\frac{g_{A1}^2}{g_{A1}^2 + g_{B1}^2}} \sqrt{\frac{g_{A2}^2}{g_{A2}^2 + g_{B2}^2}} (g_{\mu\nu}) \quad (1306)$$


---

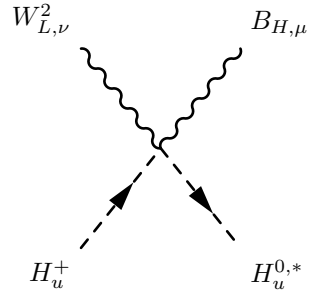

$$\frac{1}{2} g_{A1} g_{A2} \sqrt{\frac{g_{A1}^2}{g_{A1}^2 + g_{B1}^2}} \frac{1}{\sqrt{g_{A2}^2 + g_{B2}^2}} (g_{\mu\nu}) \quad (1307)$$


---

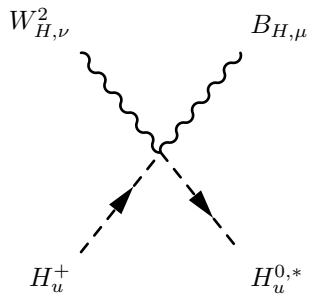

$$-\frac{1}{2} g_{A1} g_{A2} \sqrt{\frac{g_{A1}^2}{g_{A1}^2 + g_{B1}^2}} \sqrt{\frac{g_{A2}^2}{g_{A2}^2 + g_{B2}^2}} (g_{\mu\nu}) \quad (1308)$$


---

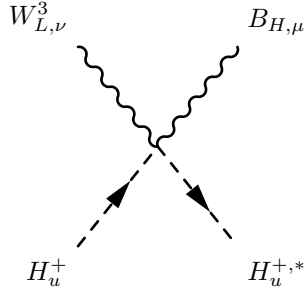

$$-\frac{i}{2}g_{A1}g_{A2}\sqrt{\frac{g_{A1}^2}{g_{A1}^2+g_{B1}^2}}g_{B2}\frac{1}{\sqrt{g_{A2}^2+g_{B2}^2}}(g_{\mu\nu}) \quad (1309)$$


---

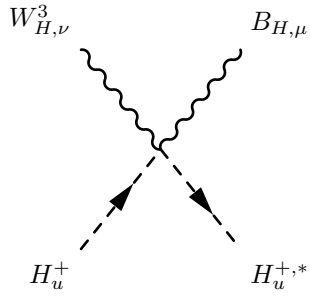

$$\frac{i}{2}g_{A1}g_{A2}\sqrt{\frac{g_{A1}^2}{g_{A1}^2+g_{B1}^2}}\sqrt{\frac{g_{A2}^2}{g_{A2}^2+g_{B2}^2}}(g_{\mu\nu}) \quad (1310)$$


---

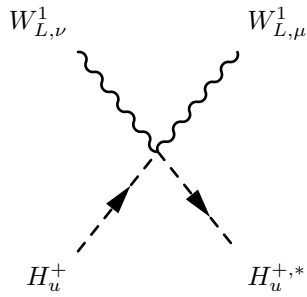

$$\frac{i}{2}g_{A2}^2g_{B2}^2\left(g_{A2}^2+g_{B2}^2\right)^{-1}(g_{\mu\nu}) \quad (1311)$$


---

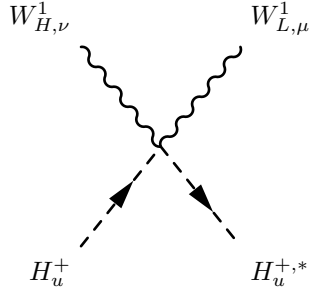

$$-\frac{i}{2}g_{B2}\left(\frac{gA2^2}{gA2^2+gB2^2}\right)^{3/2}\sqrt{gA2^2+gB2^2}(g_{\mu\nu}) \quad (1312)$$


---

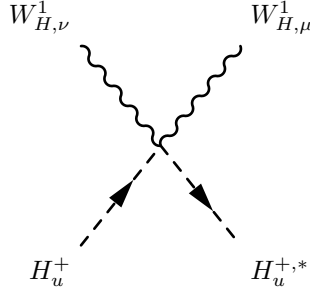

$$\frac{i}{2}g_{A2}^4(g_{A2}^2+g_{B2}^2)^{-1}(g_{\mu\nu}) \quad (1313)$$


---

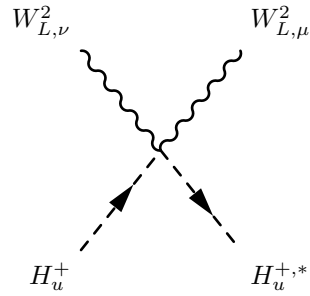

$$\frac{i}{2}g_{A2}^2g_{B2}^2(g_{A2}^2+g_{B2}^2)^{-1}(g_{\mu\nu}) \quad (1314)$$


---



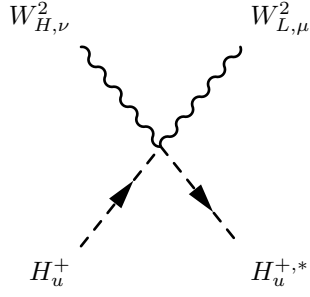

$$-\frac{i}{2}g_{B2}\left(\frac{gA2^2}{gA2^2+gB2^2}\right)^{3/2}\sqrt{gA2^2+gB2^2}(g_{\mu\nu}) \quad (1315)$$


---

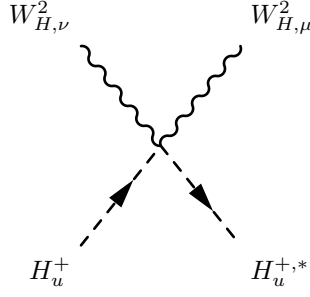

$$\frac{i}{2}g_{A2}^4(g_{A2}^2+g_{B2}^2)^{-1}(g_{\mu\nu}) \quad (1316)$$


---

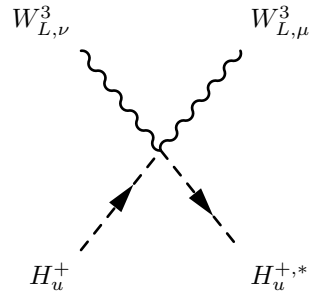

$$\frac{i}{2}g_{A2}^2g_{B2}^2(g_{A2}^2+g_{B2}^2)^{-1}(g_{\mu\nu}) \quad (1317)$$


---

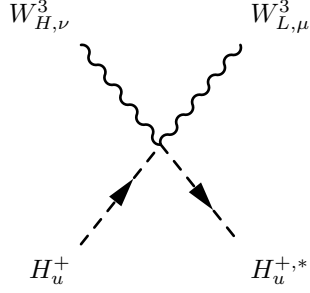

$$-\frac{i}{2}g_{B2}\left(\frac{gA2^2}{gA2^2+gB2^2}\right)^{3/2}\sqrt{gA2^2+gB2^2}(g_{\mu\nu}) \quad (1318)$$


---

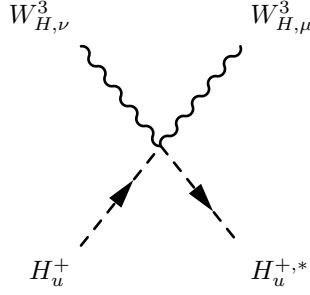

$$\frac{i}{2}g_{A2}^4(g_{A2}^2+g_{B2}^2)^{-1}(g_{\mu\nu}) \quad (1319)$$


---

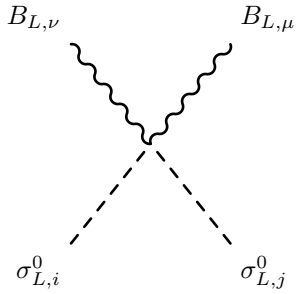

$$-2ig_{A1}g_{B1}^2\frac{1}{(gA1^2+gB1^2)^{3/2}}\left(g_{A1}^2\sqrt{\frac{gA1^2}{gA1^2+gB1^2}}-g_{A1}\sqrt{gA1^2+gB1^2}+g_{B1}^2\sqrt{\frac{gA1^2}{gA1^2+gB1^2}}\right)\left(Z_{Ls,i1}^{Di,*}Z_{Ls,j1}^{Di,*}+Z_{Ls,i2}^{Di,*}Z_{Ls,j2}^{Di,*}+Z_L^{Di,*}Z_{Ls,j1}^{Di,*}+Z_L^{Di,*}Z_{Ls,i2}^{Di,*}+Z_L^{Di,*}Z_{Ls,i1}^{Di,*}+Z_L^{Di,*}Z_{Ls,j2}^{Di,*}\right) \quad (1320)$$


---

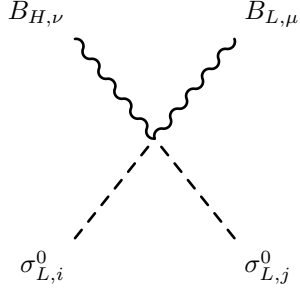

$$ig_{B1}(-g_{A1}^2 + g_{B1}^2) \frac{1}{(g_{A1}^2 + g_{B1}^2)^{3/2}} \left( g_{A1}^2 \sqrt{\frac{g_{A1}^2}{g_{A1}^2 + g_{B1}^2}} - g_{A1} \sqrt{g_{A1}^2 + g_{B1}^2} + g_{B1}^2 \sqrt{\frac{g_{A1}^2}{g_{A1}^2 + g_{B1}^2}} \right) \left( Z_{Ls,i1}^{Di,*} Z_{Ls,j1}^{Di,*} + Z_{Ls,i2}^{Di,*} Z_{Ls,j2}^{Di,*} \right) \quad (1321)$$


---

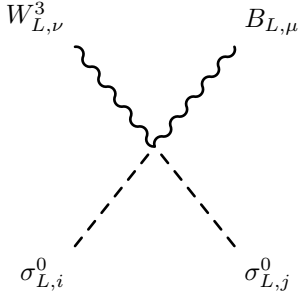

$$-ig_{B1} \frac{1}{\sqrt{g_{A1}^2 + g_{B1}^2}} \left( -g_{A1} + \sqrt{\frac{g_{A1}^2}{g_{A1}^2 + g_{B1}^2}} \sqrt{g_{A1}^2 + g_{B1}^2} \right) g_{B2} \frac{1}{\sqrt{g_{A2}^2 + g_{B2}^2}} \left( -g_{A2} + \sqrt{\frac{g_{A2}^2}{g_{A2}^2 + g_{B2}^2}} \sqrt{g_{A2}^2 + g_{B2}^2} \right) \left( Z_{Ls,i1}^{Di,*} Z_{Ls,j1}^{Di,*} + Z_{Ls,i2}^{Di,*} Z_{Ls,j2}^{Di,*} \right) \quad (1322)$$


---

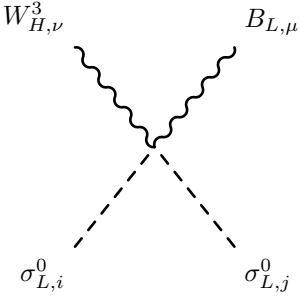

$$-ig_{B1} \frac{1}{\sqrt{g_{A1}^2 + g_{B1}^2}} \left( -g_{A1} + \sqrt{\frac{g_{A1}^2}{g_{A1}^2 + g_{B1}^2}} \sqrt{g_{A1}^2 + g_{B1}^2} \right) \frac{1}{\sqrt{g_{A2}^2 + g_{B2}^2}} \left( g_{A2} \sqrt{\frac{g_{A2}^2}{g_{A2}^2 + g_{B2}^2}} \sqrt{g_{A2}^2 + g_{B2}^2} + g_{B2}^2 \right) \left( Z_{Ls,i1}^{Di,*} Z_{Ls,j1}^{Di,*} + Z_{Ls,i2}^{Di,*} Z_{Ls,j2}^{Di,*} \right) \quad (1323)$$


---

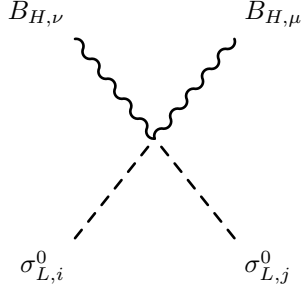

$$\begin{aligned}
& i \frac{1}{\left(gA1^2 + gB1^2\right)^{3/2}} \left( 2g_{A1}^3 g_{B1}^2 \sqrt{\frac{gA1^2}{gA1^2 + gB1^2}} + 2g_{A1} g_{B1}^4 \sqrt{\frac{gA1^2}{gA1^2 + gB1^2}} + g_{A1}^4 \sqrt{gA1^2 + gB1^2} \right. \\
& \left. + g_{B1}^4 \sqrt{gA1^2 + gB1^2} \right) \left( Z_{Ls,i1}^{Di,*} Z_{Ls,j1}^{Di,*} + Z_{Ls,i2}^{Di,*} Z_{Ls,j2}^{Di,*} + Z_{Ls,i3}^{Di,*} Z_{Ls,j3}^{Di,*} + Z_{Ls,i4}^{Di,*} Z_{Ls,j4}^{Di,*} \right) (g_{\mu\nu})
\end{aligned} \tag{1324}$$


---

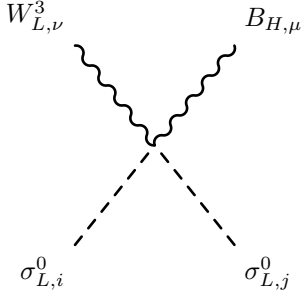

$$\begin{aligned}
& -i \frac{1}{\sqrt{gA1^2 + gB1^2}} \left( g_{A1} \sqrt{\frac{gA1^2}{gA1^2 + gB1^2}} \sqrt{gA1^2 + gB1^2} + g_{B1}^2 \right) g_{B2} \frac{1}{\sqrt{gA2^2 + gB2^2}} \left( -g_{A2} + \sqrt{\frac{gA2^2}{gA2^2 + gB2^2}} \sqrt{gA2^2 + gB2^2} \right) \left( Z_{Ls,i}^{Di,*} \right. \\
& \left. Z_{Ls,j}^{Di,*} \right)
\end{aligned} \tag{1325}$$


---

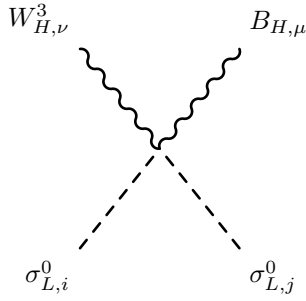

$$-i \frac{1}{\sqrt{gA1^2 + gB1^2}} \left( g_{A1} \sqrt{\frac{gA1^2}{gA1^2 + gB1^2}} \sqrt{gA1^2 + gB1^2} + g_{B1}^2 \right) \frac{1}{\sqrt{gA2^2 + gB2^2}} \left( g_{A2} \sqrt{\frac{gA2^2}{gA2^2 + gB2^2}} \sqrt{gA2^2 + gB2^2} + g_{B2}^2 \right) \left( Z_{Ls,i1}^{Di,*} Z_{Ls,j2}^{Di,*} \right. \\ \left. (1326) \right)$$


---

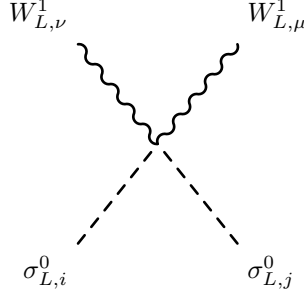

$$2ig_{B2}^2 \sqrt{\frac{gA2^2}{gA2^2 + gB2^2}} \frac{1}{\sqrt{gA2^2 + gB2^2}} \left( \sqrt{\frac{gA2^2}{gA2^2 + gB2^2}} \sqrt{gA2^2 + gB2^2} Z_{Ls,i2}^{Di,*} Z_{Ls,j2}^{Di,*} - g_{A2} Z_{Ls,i4}^{Di,*} Z_{Ls,j2}^{Di,*} \right. \\ + Z_{Ls,i1}^{Di,*} \left( -g_{A2} Z_{Ls,j3}^{Di,*} + \sqrt{\frac{gA2^2}{gA2^2 + gB2^2}} \sqrt{gA2^2 + gB2^2} Z_{Ls,j1}^{Di,*} \right) \\ + Z_{Ls,i3}^{Di,*} \left( -g_{A2} Z_{Ls,j1}^{Di,*} + \sqrt{\frac{gA2^2}{gA2^2 + gB2^2}} \sqrt{gA2^2 + gB2^2} Z_{Ls,j3}^{Di,*} \right) - g_{A2} Z_{Ls,i2}^{Di,*} Z_{Ls,j4}^{Di,*} \\ \left. + \sqrt{\frac{gA2^2}{gA2^2 + gB2^2}} \sqrt{gA2^2 + gB2^2} Z_{Ls,i4}^{Di,*} Z_{Ls,j4}^{Di,*} \right) (g_{\mu\nu}) \quad (1327)$$


---

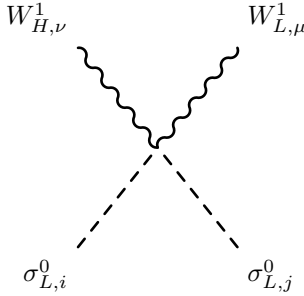

$$ig_{A2} g_{B2} \left( -g_{B2}^2 + g_{A2}^2 \right) \frac{1}{\sqrt{\frac{gA2^2}{gA2^2 + gB2^2}}} \frac{1}{(gA2^2 + gB2^2)^{3/2}} \left( -g_{A2} Z_{Ls,i2}^{Di,*} Z_{Ls,j2}^{Di,*} + \sqrt{\frac{gA2^2}{gA2^2 + gB2^2}} \sqrt{gA2^2 + gB2^2} Z_{Ls,i4}^{Di,*} Z_{Ls,j2}^{Di,*} \right. \\ \left. + Z_{Ls,i3}^{Di,*} \left( -g_{A2} Z_{Ls,j3}^{Di,*} + \sqrt{\frac{gA2^2}{gA2^2 + gB2^2}} \sqrt{gA2^2 + gB2^2} Z_{Ls,j1}^{Di,*} \right) \right)$$

$$\begin{aligned}
& + Z_{Ls,i1}^{Di,*} \left( -g_{A2} Z_{Ls,j1}^{Di,*} + \sqrt{\frac{g_{A2}^2}{g_{A2}^2 + g_{B2}^2}} \sqrt{g_{A2}^2 + g_{B2}^2} Z_{Ls,j3}^{Di,*} \right) \\
& + \sqrt{\frac{g_{A2}^2}{g_{A2}^2 + g_{B2}^2}} \sqrt{g_{A2}^2 + g_{B2}^2} Z_{Ls,i2}^{Di,*} Z_{Ls,j4}^{Di,*} - g_{A2} Z_{Ls,i4}^{Di,*} Z_{Ls,j4}^{Di,*} \Big) (g_{\mu\nu})
\end{aligned} \tag{1328}$$


---

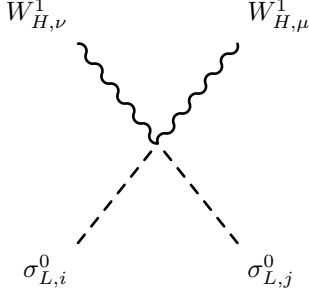

$$\begin{aligned}
& i \frac{1}{\sqrt{\frac{g_{A2}^2}{g_{A2}^2 + g_{B2}^2}}} \frac{1}{(g_{A2}^2 + g_{B2}^2)^{3/2}} \left( g_{A2}^4 \sqrt{\frac{g_{A2}^2}{g_{A2}^2 + g_{B2}^2}} \sqrt{g_{A2}^2 + g_{B2}^2} Z_{Ls,i2}^{Di,*} Z_{Ls,j2}^{Di,*} \right. \\
& + g_{B2}^4 \sqrt{\frac{g_{A2}^2}{g_{A2}^2 + g_{B2}^2}} \sqrt{g_{A2}^2 + g_{B2}^2} Z_{Ls,i2}^{Di,*} Z_{Ls,j2}^{Di,*} + 2g_{A2}^3 g_{B2}^2 Z_{Ls,i4}^{Di,*} Z_{Ls,j2}^{Di,*} \\
& + Z_{Ls,i1}^{Di,*} \left( 2g_{A2}^3 g_{B2}^2 Z_{Ls,j3}^{Di,*} + \sqrt{\frac{g_{A2}^2}{g_{A2}^2 + g_{B2}^2}} \sqrt{g_{A2}^2 + g_{B2}^2} (g_{A2}^4 + g_{B2}^4) Z_{Ls,j1}^{Di,*} \right) \\
& + Z_{Ls,i3}^{Di,*} \left( 2g_{A2}^3 g_{B2}^2 Z_{Ls,j1}^{Di,*} + \sqrt{\frac{g_{A2}^2}{g_{A2}^2 + g_{B2}^2}} \sqrt{g_{A2}^2 + g_{B2}^2} (g_{A2}^4 + g_{B2}^4) Z_{Ls,j3}^{Di,*} \right) \\
& + 2g_{A2}^3 g_{B2}^2 Z_{Ls,i2}^{Di,*} Z_{Ls,j4}^{Di,*} + g_{A2}^4 \sqrt{\frac{g_{A2}^2}{g_{A2}^2 + g_{B2}^2}} \sqrt{g_{A2}^2 + g_{B2}^2} Z_{Ls,i4}^{Di,*} Z_{Ls,j4}^{Di,*} \\
& \left. + g_{B2}^4 \sqrt{\frac{g_{A2}^2}{g_{A2}^2 + g_{B2}^2}} \sqrt{g_{A2}^2 + g_{B2}^2} Z_{Ls,i4}^{Di,*} Z_{Ls,j4}^{Di,*} \right) (g_{\mu\nu})
\end{aligned} \tag{1329}$$


---

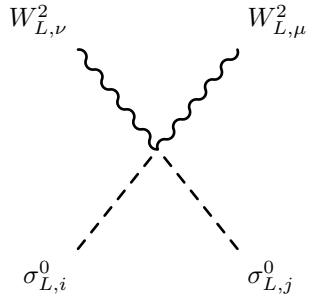

$$\begin{aligned}
& 2ig_{B2}^2 \sqrt{\frac{gA2^2}{gA2^2 + gB2^2}} \frac{1}{\sqrt{gA2^2 + gB2^2}} \left( \sqrt{\frac{gA2^2}{gA2^2 + gB2^2}} \sqrt{gA2^2 + gB2^2} Z_{Ls,i2}^{Di,*} Z_{Ls,j2}^{Di,*} - g_{A2} Z_{Ls,i4}^{Di,*} Z_{Ls,j2}^{Di,*} \right. \\
& + Z_{Ls,i1}^{Di,*} \left( -g_{A2} Z_{Ls,j3}^{Di,*} + \sqrt{\frac{gA2^2}{gA2^2 + gB2^2}} \sqrt{gA2^2 + gB2^2} Z_{Ls,j1}^{Di,*} \right) \\
& + Z_{Ls,i3}^{Di,*} \left( -g_{A2} Z_{Ls,j1}^{Di,*} + \sqrt{\frac{gA2^2}{gA2^2 + gB2^2}} \sqrt{gA2^2 + gB2^2} Z_{Ls,j3}^{Di,*} \right) - g_{A2} Z_{Ls,i2}^{Di,*} Z_{Ls,j4}^{Di,*} \\
& \left. + \sqrt{\frac{gA2^2}{gA2^2 + gB2^2}} \sqrt{gA2^2 + gB2^2} Z_{Ls,i4}^{Di,*} Z_{Ls,j4}^{Di,*} \right) (g_{\mu\nu}) \tag{1330}
\end{aligned}$$


---

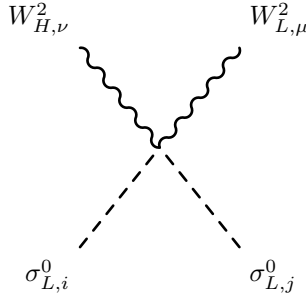

$$\begin{aligned}
& ig_{A2} g_{B2} \left( -g_{B2}^2 + g_{A2}^2 \right) \frac{1}{\sqrt{\frac{gA2^2}{gA2^2 + gB2^2}}} \frac{1}{(gA2^2 + gB2^2)^{3/2}} \left( -g_{A2} Z_{Ls,i2}^{Di,*} Z_{Ls,j2}^{Di,*} + \sqrt{\frac{gA2^2}{gA2^2 + gB2^2}} \sqrt{gA2^2 + gB2^2} Z_{Ls,i4}^{Di,*} Z_{Ls,j2}^{Di,*} \right. \\
& + Z_{Ls,i3}^{Di,*} \left( -g_{A2} Z_{Ls,j3}^{Di,*} + \sqrt{\frac{gA2^2}{gA2^2 + gB2^2}} \sqrt{gA2^2 + gB2^2} Z_{Ls,j1}^{Di,*} \right) \\
& + Z_{Ls,i1}^{Di,*} \left( -g_{A2} Z_{Ls,j1}^{Di,*} + \sqrt{\frac{gA2^2}{gA2^2 + gB2^2}} \sqrt{gA2^2 + gB2^2} Z_{Ls,j3}^{Di,*} \right) \\
& \left. + \sqrt{\frac{gA2^2}{gA2^2 + gB2^2}} \sqrt{gA2^2 + gB2^2} Z_{Ls,i2}^{Di,*} Z_{Ls,j4}^{Di,*} - g_{A2} Z_{Ls,i4}^{Di,*} Z_{Ls,j4}^{Di,*} \right) (g_{\mu\nu}) \tag{1331}
\end{aligned}$$


---

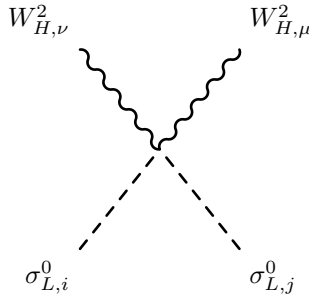

$$\begin{aligned}
& i \frac{1}{\sqrt{\frac{gA^2}{gA^2+gB^2}}} \frac{1}{(gA^2+gB^2)^{3/2}} \left( g_{A2}^4 \sqrt{\frac{gA^2}{gA^2+gB^2}} \sqrt{gA^2+gB^2} Z_{Ls,i2}^{Di,*} Z_{Ls,j2}^{Di,*} \right. \\
& + g_{B2}^4 \sqrt{\frac{gA^2}{gA^2+gB^2}} \sqrt{gA^2+gB^2} Z_{Ls,i2}^{Di,*} Z_{Ls,j2}^{Di,*} + 2g_{A2}^3 g_{B2}^2 Z_{Ls,i4}^{Di,*} Z_{Ls,j2}^{Di,*} \\
& + Z_{Ls,i1}^{Di,*} \left( 2g_{A2}^3 g_{B2}^2 Z_{Ls,j3}^{Di,*} + \sqrt{\frac{gA^2}{gA^2+gB^2}} \sqrt{gA^2+gB^2} (g_{A2}^4 + g_{B2}^4) Z_{Ls,j1}^{Di,*} \right) \\
& + Z_{Ls,i3}^{Di,*} \left( 2g_{A2}^3 g_{B2}^2 Z_{Ls,j1}^{Di,*} + \sqrt{\frac{gA^2}{gA^2+gB^2}} \sqrt{gA^2+gB^2} (g_{A2}^4 + g_{B2}^4) Z_{Ls,j3}^{Di,*} \right) \\
& + 2g_{A2}^3 g_{B2}^2 Z_{Ls,i2}^{Di,*} Z_{Ls,j4}^{Di,*} + g_{A2}^4 \sqrt{\frac{gA^2}{gA^2+gB^2}} \sqrt{gA^2+gB^2} Z_{Ls,i4}^{Di,*} Z_{Ls,j4}^{Di,*} \\
& \left. + g_{B2}^4 \sqrt{\frac{gA^2}{gA^2+gB^2}} \sqrt{gA^2+gB^2} Z_{Ls,i4}^{Di,*} Z_{Ls,j4}^{Di,*} \right) (g_{\mu\nu})
\end{aligned} \tag{1332}$$


---

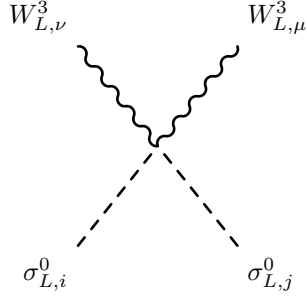

$$-2ig_{A2}g_{B2}^2 \frac{1}{(gA^2+gB^2)^{3/2}} \left( g_{A2}^2 \sqrt{\frac{gA^2}{gA^2+gB^2}} - g_{A2} \sqrt{gA^2+gB^2} + g_{B2}^2 \sqrt{\frac{gA^2}{gA^2+gB^2}} \right) \left( Z_{Ls,i1}^{Di,*} Z_{Ls,j1}^{Di,*} + Z_{Ls,i2}^{Di,*} Z_{Ls,j2}^{Di,*} + Z_{Ls,i3}^{Di,*} Z_{Ls,j3}^{Di,*} + Z_{Ls,i4}^{Di,*} Z_{Ls,j4}^{Di,*} \right)$$

(1333)

---

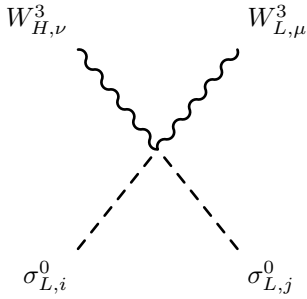



$$ig_{B2} \left( -g_{A2}^2 + g_{B2}^2 \right) \frac{1}{\left( gA2^2 + gB2^2 \right)^{3/2}} \left( g_{A2}^2 \sqrt{\frac{gA2^2}{gA2^2 + gB2^2}} - g_{A2} \sqrt{gA2^2 + gB2^2} + g_{B2}^2 \sqrt{\frac{gA2^2}{gA2^2 + gB2^2}} \right) \left( Z_{Ls,i1}^{Di,*} Z_{Ls,j1}^{Di,*} + Z_{Ls,i2}^{Di,*} Z_{Ls,j2}^{Di,*} \right) \quad (1334)$$


---

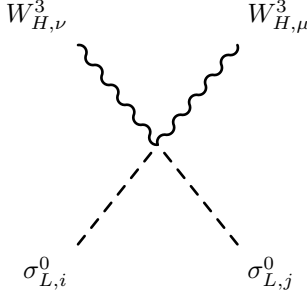

$$i \frac{1}{\left( gA2^2 + gB2^2 \right)^{3/2}} \left( 2g_{A2}^3 g_{B2}^2 \sqrt{\frac{gA2^2}{gA2^2 + gB2^2}} + 2g_{A2} g_{B2}^4 \sqrt{\frac{gA2^2}{gA2^2 + gB2^2}} + g_{A2}^4 \sqrt{gA2^2 + gB2^2} + g_{B2}^4 \sqrt{gA2^2 + gB2^2} \right) \left( Z_{Ls,i1}^{Di,*} Z_{Ls,j1}^{Di,*} + Z_{Ls,i2}^{Di,*} Z_{Ls,j2}^{Di,*} + Z_{Ls,i3}^{Di,*} Z_{Ls,j3}^{Di,*} + Z_{Ls,i4}^{Di,*} Z_{Ls,j4}^{Di,*} \right) (g_{\mu\nu}) \quad (1335)$$


---

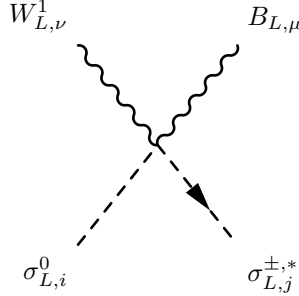

$$\begin{aligned} & \frac{1}{2} g_{B1} \frac{1}{\sqrt{gA1^2 + gB1^2}} \left( -g_{A1} + \sqrt{\frac{gA1^2}{gA1^2 + gB1^2}} \sqrt{gA1^2 + gB1^2} \right) g_{B2} \frac{1}{\sqrt{gA2^2 + gB2^2}} \left( -g_{A2} Z_{Ls,i2}^{Di,*} Z_{Ls,j2}^{od} + \sqrt{\frac{gA2^2}{gA2^2 + gB2^2}} \sqrt{gA2^2 + gB2^2} \right. \\ & - \sqrt{\frac{gA2^2}{gA2^2 + gB2^2}} \sqrt{gA2^2 + gB2^2} Z_{Ls,i2}^{Di,*} Z_{Ls,j3}^{od} + g_{A2} Z_{Ls,i4}^{Di,*} Z_{Ls,j3}^{od} \\ & + Z_{Ls,i1}^{Di,*} \left( g_{A2} Z_{Ls,j4}^{od} + \sqrt{\frac{gA2^2}{gA2^2 + gB2^2}} \sqrt{gA2^2 + gB2^2} Z_{Ls,j1}^{od} \right) \\ & \left. - Z_{Ls,i3}^{Di,*} \left( g_{A2} Z_{Ls,j1}^{od} + \sqrt{\frac{gA2^2}{gA2^2 + gB2^2}} \sqrt{gA2^2 + gB2^2} Z_{Ls,j4}^{od} \right) \right) (g_{\mu\nu}) \quad (1336) \end{aligned}$$


---

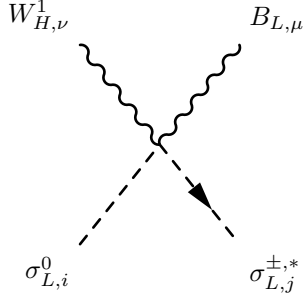

$$\begin{aligned}
& \frac{1}{2} g_{B1} \frac{1}{\sqrt{gA1^2 + gB1^2}} \left( -g_{A1} + \sqrt{\frac{gA1^2}{gA1^2 + gB1^2}} \sqrt{gA1^2 + gB1^2} \right) \frac{1}{\sqrt{gA2^2 + gB2^2}} \left( g_{A2} \sqrt{\frac{gA2^2}{gA2^2 + gB2^2}} \sqrt{gA2^2 + gB2^2} Z_{Ls,i2}^{Di,*} Z_{Ls,j2}^{od} + g_{B2} \sqrt{\frac{gA2^2}{gA2^2 + gB2^2}} \sqrt{gA2^2 + gB2^2} Z_{Ls,i2}^{Di,*} Z_{Ls,j2}^{od} \right. \\
& - g_{A2} \sqrt{\frac{gA2^2}{gA2^2 + gB2^2}} \sqrt{gA2^2 + gB2^2} Z_{Ls,i4}^{Di,*} Z_{Ls,j3}^{od} \\
& + Z_{Ls,i3}^{Di,*} \left( g_{A2} \sqrt{\frac{gA2^2}{gA2^2 + gB2^2}} \sqrt{gA2^2 + gB2^2} Z_{Ls,j1}^{od} - g_{B2}^2 Z_{Ls,j4}^{od} \right) \\
& \left. + Z_{Ls,i1}^{Di,*} \left( -g_{A2} \sqrt{\frac{gA2^2}{gA2^2 + gB2^2}} \sqrt{gA2^2 + gB2^2} Z_{Ls,j4}^{od} + g_{B2}^2 Z_{Ls,j1}^{od} \right) \right) (g_{\mu\nu}) \tag{1337}
\end{aligned}$$

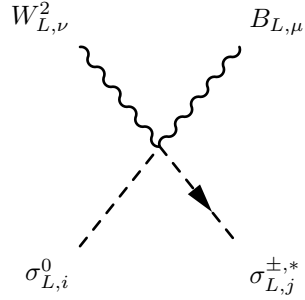

$$\begin{aligned}
& \frac{i}{2} g_{B1} \frac{1}{\sqrt{gA1^2 + gB1^2}} \left( -g_{A1} + \sqrt{\frac{gA1^2}{gA1^2 + gB1^2}} \sqrt{gA1^2 + gB1^2} \right) g_{B2} \frac{1}{\sqrt{gA2^2 + gB2^2}} \left( g_{A2} Z_{Ls,i2}^{Di,*} Z_{Ls,j2}^{od} - \sqrt{\frac{gA2^2}{gA2^2 + gB2^2}} \sqrt{gA2^2 + gB2^2} Z_{Ls,i2}^{Di,*} Z_{Ls,j2}^{od} \right. \\
& + \sqrt{\frac{gA2^2}{gA2^2 + gB2^2}} \sqrt{gA2^2 + gB2^2} Z_{Ls,i2}^{Di,*} Z_{Ls,j3}^{od} - g_{A2} Z_{Ls,i4}^{Di,*} Z_{Ls,j3}^{od} \\
& - Z_{Ls,i1}^{Di,*} \left( g_{A2} Z_{Ls,j4}^{od} + \sqrt{\frac{gA2^2}{gA2^2 + gB2^2}} \sqrt{gA2^2 + gB2^2} Z_{Ls,j1}^{od} \right) \\
& \left. + Z_{Ls,i3}^{Di,*} \left( g_{A2} Z_{Ls,j1}^{od} + \sqrt{\frac{gA2^2}{gA2^2 + gB2^2}} \sqrt{gA2^2 + gB2^2} Z_{Ls,j4}^{od} \right) \right) (g_{\mu\nu}) \tag{1338}
\end{aligned}$$

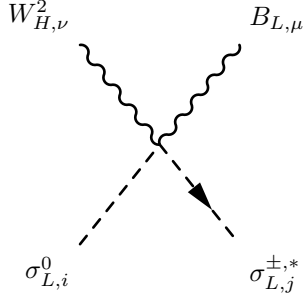

$$\begin{aligned}
& -\frac{i}{2}g_{B1}\frac{1}{\sqrt{gA1^2+gB1^2}}\left(-g_{A1}+\sqrt{\frac{gA1^2}{gA1^2+gB1^2}}\sqrt{gA1^2+gB1^2}\right)\frac{1}{\sqrt{gA2^2+gB2^2}}\left(g_{A2}\sqrt{\frac{gA2^2}{gA2^2+gB2^2}}\sqrt{gA2^2+gB2^2}Z_{Ls,i2}^{Di,*}Z_{Ls,j2}^{od}-\right. \\
& -g_{A2}\sqrt{\frac{gA2^2}{gA2^2+gB2^2}}\sqrt{gA2^2+gB2^2}Z_{Ls,i4}^{Di,*}Z_{Ls,j3}^{od} \\
& +Z_{Ls,i3}^{Di,*}\left(g_{A2}\sqrt{\frac{gA2^2}{gA2^2+gB2^2}}\sqrt{gA2^2+gB2^2}Z_{Ls,j1}^{od}-g_{B2}^2Z_{Ls,j4}^{od}\right) \\
& \left.+Z_{Ls,i1}^{Di,*}\left(-g_{A2}\sqrt{\frac{gA2^2}{gA2^2+gB2^2}}\sqrt{gA2^2+gB2^2}Z_{Ls,j4}^{od}+g_{B2}^2Z_{Ls,j1}^{od}\right)\right)\left(g_{\mu\nu}\right)
\end{aligned} \tag{1339}$$

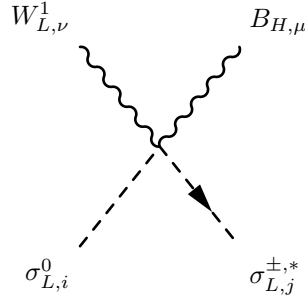

$$\begin{aligned}
& \frac{1}{2}\frac{1}{\sqrt{gA1^2+gB1^2}}\left(g_{A1}\sqrt{\frac{gA1^2}{gA1^2+gB1^2}}\sqrt{gA1^2+gB1^2}+g_{B1}^2\right)g_{B2}\frac{1}{\sqrt{gA2^2+gB2^2}}\left(-g_{A2}Z_{Ls,i2}^{Di,*}Z_{Ls,j2}^{od}+\sqrt{\frac{gA2^2}{gA2^2+gB2^2}}\sqrt{gA2^2+gB2^2}Z_{Ls,i2}^{Di,*}Z_{Ls,j2}^{od}-\right. \\
& -\sqrt{\frac{gA2^2}{gA2^2+gB2^2}}\sqrt{gA2^2+gB2^2}Z_{Ls,i2}^{Di,*}Z_{Ls,j3}^{od}+g_{A2}Z_{Ls,i4}^{Di,*}Z_{Ls,j3}^{od} \\
& +Z_{Ls,i1}^{Di,*}\left(g_{A2}Z_{Ls,j4}^{od}+\sqrt{\frac{gA2^2}{gA2^2+gB2^2}}\sqrt{gA2^2+gB2^2}Z_{Ls,j1}^{od}\right) \\
& \left.-Z_{Ls,i3}^{Di,*}\left(g_{A2}Z_{Ls,j1}^{od}+\sqrt{\frac{gA2^2}{gA2^2+gB2^2}}\sqrt{gA2^2+gB2^2}Z_{Ls,j4}^{od}\right)\right)\left(g_{\mu\nu}\right)
\end{aligned} \tag{1340}$$

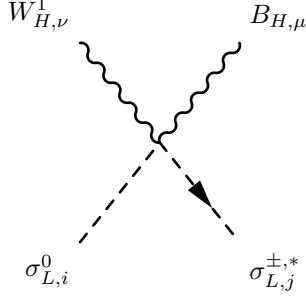

$$\begin{aligned}
& \frac{1}{2} \frac{1}{\sqrt{gA1^2 + gB1^2}} \left( gA1 \sqrt{\frac{gA1^2}{gA1^2 + gB1^2}} \sqrt{gA1^2 + gB1^2} + g_{B1}^2 \right) \frac{1}{\sqrt{gA2^2 + gB2^2}} \left( gA2 \sqrt{\frac{gA2^2}{gA2^2 + gB2^2}} \sqrt{gA2^2 + gB2^2} Z_{Ls,i2}^{Di,*} Z_{Ls,j2}^{od} + g_{B2}^2 \right) \\
& - gA2 \sqrt{\frac{gA2^2}{gA2^2 + gB2^2}} \sqrt{gA2^2 + gB2^2} Z_{Ls,i4}^{Di,*} Z_{Ls,j3}^{od} \\
& + Z_{Ls,i3}^{Di,*} \left( gA2 \sqrt{\frac{gA2^2}{gA2^2 + gB2^2}} \sqrt{gA2^2 + gB2^2} Z_{Ls,j1}^{od} - g_{B2}^2 Z_{Ls,j4}^{od} \right) \\
& + Z_{Ls,i1}^{Di,*} \left( -gA2 \sqrt{\frac{gA2^2}{gA2^2 + gB2^2}} \sqrt{gA2^2 + gB2^2} Z_{Ls,j4}^{od} + g_{B2}^2 Z_{Ls,j1}^{od} \right) \left( g_{\mu\nu} \right)
\end{aligned} \tag{1341}$$

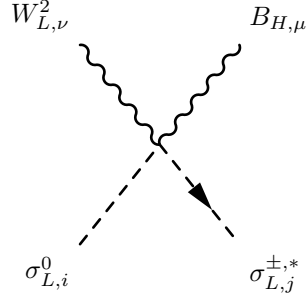

$$\begin{aligned}
& \frac{i}{2} \frac{1}{\sqrt{gA1^2 + gB1^2}} \left( gA1 \sqrt{\frac{gA1^2}{gA1^2 + gB1^2}} \sqrt{gA1^2 + gB1^2} + g_{B1}^2 \right) gB2 \frac{1}{\sqrt{gA2^2 + gB2^2}} \left( gA2 Z_{Ls,i2}^{Di,*} Z_{Ls,j2}^{od} - \sqrt{\frac{gA2^2}{gA2^2 + gB2^2}} \sqrt{gA2^2 + gB2^2} \right) \\
& + \sqrt{\frac{gA2^2}{gA2^2 + gB2^2}} \sqrt{gA2^2 + gB2^2} Z_{Ls,i2}^{Di,*} Z_{Ls,j3}^{od} - gA2 Z_{Ls,i4}^{Di,*} Z_{Ls,j3}^{od} \\
& - Z_{Ls,i1}^{Di,*} \left( gA2 Z_{Ls,j4}^{od} + \sqrt{\frac{gA2^2}{gA2^2 + gB2^2}} \sqrt{gA2^2 + gB2^2} Z_{Ls,j1}^{od} \right) \\
& + Z_{Ls,i3}^{Di,*} \left( gA2 Z_{Ls,j1}^{od} + \sqrt{\frac{gA2^2}{gA2^2 + gB2^2}} \sqrt{gA2^2 + gB2^2} Z_{Ls,j4}^{od} \right) \left( g_{\mu\nu} \right)
\end{aligned} \tag{1342}$$

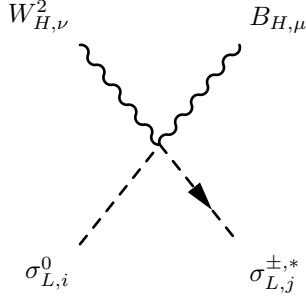

$$\begin{aligned}
& -\frac{i}{2} \frac{1}{\sqrt{gA1^2 + gB1^2}} \left( g_{A1} \sqrt{\frac{gA1^2}{gA1^2 + gB1^2}} \sqrt{gA1^2 + gB1^2} + g_{B1}^2 \right) \frac{1}{\sqrt{gA2^2 + gB2^2}} \left( g_{A2} \sqrt{\frac{gA2^2}{gA2^2 + gB2^2}} \sqrt{gA2^2 + gB2^2} Z_{Ls,i2}^{Di,*} Z_{Ls,j2}^{od} + g_{B2}^2 Z_{Ls,i2}^{od} Z_{Ls,j2}^{Di,*} \right) \\
& - g_{A2} \sqrt{\frac{gA2^2}{gA2^2 + gB2^2}} \sqrt{gA2^2 + gB2^2} Z_{Ls,i4}^{Di,*} Z_{Ls,j3}^{od} \\
& + Z_{Ls,i3}^{Di,*} \left( g_{A2} \sqrt{\frac{gA2^2}{gA2^2 + gB2^2}} \sqrt{gA2^2 + gB2^2} Z_{Ls,j1}^{od} - g_{B2}^2 Z_{Ls,j4}^{od} \right) \\
& + Z_{Ls,i1}^{Di,*} \left( -g_{A2} \sqrt{\frac{gA2^2}{gA2^2 + gB2^2}} \sqrt{gA2^2 + gB2^2} Z_{Ls,j4}^{od} + g_{B2}^2 Z_{Ls,j1}^{od} \right) \Big) (g_{\mu\nu})
\end{aligned} \tag{1343}$$


---

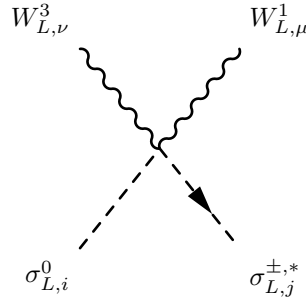

$$\begin{aligned}
& \frac{1}{2} g_{A2} g_{B2}^2 \sqrt{\frac{gA2^2}{gA2^2 + gB2^2}} \frac{1}{\sqrt{gA2^2 + gB2^2}} \left( Z_{Ls,i1}^{Di,*} \left( -Z_{Ls,j4}^{od} + Z_{Ls,j1}^{od} \right) + Z_{Ls,i3}^{Di,*} \left( -Z_{Ls,j1}^{od} + Z_{Ls,j4}^{od} \right) + \left( -Z_{Ls,i4}^{Di,*} + Z_{Ls,i2}^{Di,*} \right) \left( -Z_{Ls,j3}^{od} + Z_{Ls,j2}^{od} \right) \right)
\end{aligned} \tag{1344}$$


---

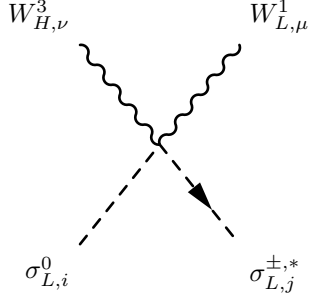

$$\frac{1}{2}g_{A2}g_{B2}\left(g_{A2}^2+g_{B2}^2\right)^{-1}\left(g_{B2}^2Z_{Ls,i2}^{Di,*}Z_{Ls,j2}^{od}+g_{A2}^2Z_{Ls,i4}^{Di,*}Z_{Ls,j2}^{od}+g_{A2}^2Z_{Ls,i2}^{Di,*}Z_{Ls,j3}^{od}+g_{B2}^2Z_{Ls,i4}^{Di,*}Z_{Ls,j3}^{od}-Z_{Ls,i3}^{Di,*}\left(g_{A2}^2Z_{Ls,j4}^{od}+g_{B2}^2Z_{Ls,j1}^{od}\right)-Z_{Ls,i1}^{Di,*}\left(g_{A2}^2Z_{Ls,j1}^{od}+g_{B2}^2Z_{Ls,j4}^{od}\right)\right)\left(g_{\mu\nu}\right) \quad (1345)$$


---

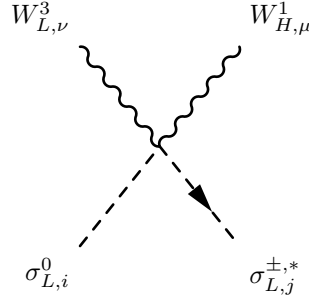

$$\frac{1}{2}g_{A2}g_{B2}\left(g_{A2}^2+g_{B2}^2\right)^{-1}\left(-g_{A2}^2Z_{Ls,i2}^{Di,*}Z_{Ls,j2}^{od}-g_{B2}^2Z_{Ls,i4}^{Di,*}Z_{Ls,j2}^{od}-g_{B2}^2Z_{Ls,i2}^{Di,*}Z_{Ls,j3}^{od}-g_{A2}^2Z_{Ls,i4}^{Di,*}Z_{Ls,j3}^{od}+Z_{Ls,i1}^{Di,*}\left(g_{A2}^2Z_{Ls,j4}^{od}+g_{B2}^2Z_{Ls,j1}^{od}\right)+Z_{Ls,i3}^{Di,*}\left(g_{A2}^2Z_{Ls,j1}^{od}+g_{B2}^2Z_{Ls,j4}^{od}\right)\right)\left(g_{\mu\nu}\right) \quad (1346)$$


---

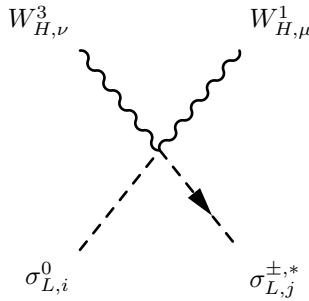

$$-\frac{1}{2}g_{A2}g_{B2}^2\sqrt{\frac{g_{A2}^2}{g_{A2}^2+g_{B2}^2}}\frac{1}{\sqrt{g_{A2}^2+g_{B2}^2}}\left(Z_{Ls,i1}^{Di,*}\left(-Z_{Ls,j4}^{od}+Z_{Ls,j1}^{od}\right)+Z_{Ls,i3}^{Di,*}\left(-Z_{Ls,j1}^{od}+Z_{Ls,j4}^{od}\right)+\left(-Z_{Ls,i4}^{Di,*}+Z_{Ls,i2}^{Di,*}\right)\left(-Z_{Ls,j1}^{od}+Z_{Ls,j4}^{od}\right)\right) \quad (1347)$$


---

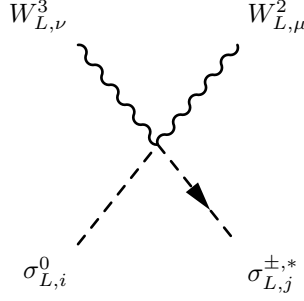

$$-\frac{i}{2}g_{A2}g_{B2}^2\sqrt{\frac{g_{A2}^2}{g_{A2}^2+g_{B2}^2}}\frac{1}{\sqrt{g_{A2}^2+g_{B2}^2}}\left(Z_{Ls,i1}^{Di,*}\left(-Z_{Ls,j4}^{od}+Z_{Ls,j1}^{od}\right)+Z_{Ls,i3}^{Di,*}\left(-Z_{Ls,j1}^{od}+Z_{Ls,j4}^{od}\right)+\left(-Z_{Ls,i4}^{Di,*}+Z_{Ls,i2}^{Di,*}\right)\left(-Z_{Ls,i1}^{od}+Z_{Ls,i3}^{od}\right)\right) \quad (1348)$$


---

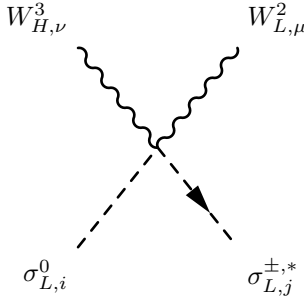

$$\frac{i}{2}g_{A2}g_{B2}\left(g_{A2}^2+g_{B2}^2\right)^{-1}\left(-g_{B2}^2Z_{Ls,i2}^{Di,*}Z_{Ls,j2}^{od}-g_{A2}^2Z_{Ls,i4}^{Di,*}Z_{Ls,j2}^{od}-g_{A2}^2Z_{Ls,i2}^{Di,*}Z_{Ls,j3}^{od}-g_{B2}^2Z_{Ls,i4}^{Di,*}Z_{Ls,j3}^{od}+Z_{Ls,i3}^{Di,*}\left(g_{A2}^2Z_{Ls,j4}^{od}+g_{B2}^2Z_{Ls,j1}^{od}\right)+Z_{Ls,i1}^{Di,*}\left(g_{A2}^2Z_{Ls,j1}^{od}+g_{B2}^2Z_{Ls,j4}^{od}\right)\right)\left(g_{\mu\nu}\right) \quad (1349)$$


---

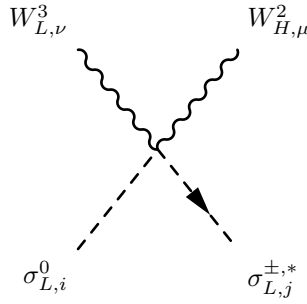

$$\frac{i}{2}g_{A2}g_{B2}\left(g_{A2}^2+g_{B2}^2\right)^{-1}\left(g_{A2}^2Z_{Ls,i2}^{Di,*}Z_{Ls,j2}^{od}+g_{B2}^2Z_{Ls,i4}^{Di,*}Z_{Ls,j2}^{od}+g_{B2}^2Z_{Ls,i2}^{Di,*}Z_{Ls,j3}^{od}+g_{A2}^2Z_{Ls,i4}^{Di,*}Z_{Ls,j3}^{od}-Z_{Ls,i1}^{Di,*}\left(g_{A2}^2Z_{Ls,j4}^{od}+g_{B2}^2Z_{Ls,j1}^{od}\right)-Z_{Ls,i3}^{Di,*}\left(g_{A2}^2Z_{Ls,j1}^{od}+g_{B2}^2Z_{Ls,j4}^{od}\right)\right)\left(g_{\mu\nu}\right) \quad (1350)$$


---

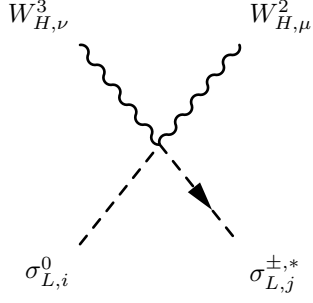

$$\frac{i}{2}g_{A2}g_{B2}^2\sqrt{\frac{g_{A2}^2}{g_{A2}^2+g_{B2}^2}}\frac{1}{\sqrt{g_{A2}^2+g_{B2}^2}}\left(Z_{Ls,i1}^{Di,*}\left(-Z_{Ls,j4}^{od}+Z_{Ls,j1}^{od}\right)+Z_{Ls,i3}^{Di,*}\left(-Z_{Ls,j1}^{od}+Z_{Ls,j4}^{od}\right)+\left(-Z_{Ls,i4}^{Di,*}+Z_{Ls,i2}^{Di,*}\right)\left(-Z_{Ls,j3}^{od}\right.\right. \\ \left.\left.\right)\right) \quad (1351)$$


---

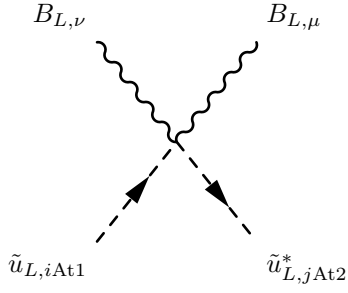

$$\frac{i}{18}g_{A1}^2g_{B1}^2\left(g_{A1}^2+g_{B1}^2\right)^{-1}\delta_{At1At2}\delta_{ij}\left(g_{\mu\nu}\right) \quad (1352)$$


---

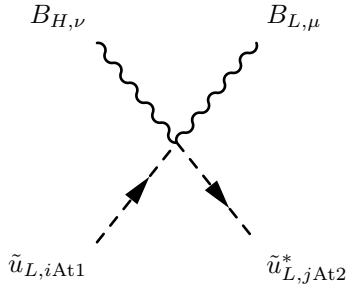

$$-\frac{i}{18}g_{B1}\left(\frac{g_{A1}^2}{g_{A1}^2+g_{B1}^2}\right)^{3/2}\sqrt{g_{A1}^2+g_{B1}^2}\delta_{At1At2}\delta_{ij}\left(g_{\mu\nu}\right) \quad (1353)$$


---



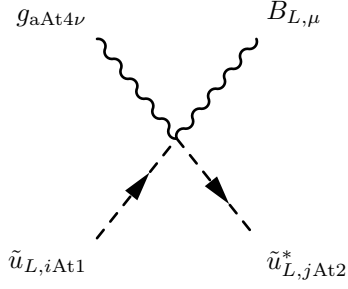

$$\frac{i}{6} g_3 g_{A1} g_{B1} \frac{1}{\sqrt{g_{A1}^2 + g_{B1}^2}} \delta_{ij} \lambda_{At2,At1}^{aAt4} (g_{\mu\nu}) \quad (1354)$$


---

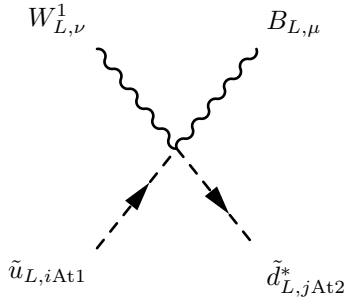

$$\frac{i}{6} g_{A1} g_{A2} g_{B1} \frac{1}{\sqrt{g_{A1}^2 + g_{B1}^2}} g_{B2} \frac{1}{\sqrt{g_{A2}^2 + g_{B2}^2}} \delta_{At1At2} \delta_{ij} (g_{\mu\nu}) \quad (1355)$$


---

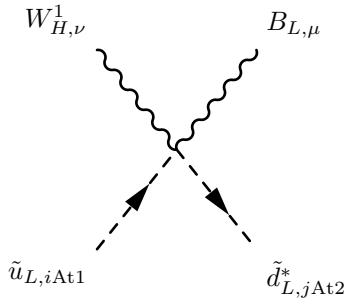

$$-\frac{i}{6} g_{A1} g_{A2} g_{B1} \frac{1}{\sqrt{g_{A1}^2 + g_{B1}^2}} \sqrt{\frac{g_{A2}^2}{g_{A2}^2 + g_{B2}^2}} \delta_{At1At2} \delta_{ij} (g_{\mu\nu}) \quad (1356)$$


---

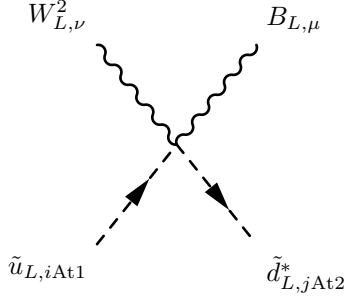

$$-\frac{1}{6}g_{A1}g_{A2}g_{B1}\frac{1}{\sqrt{g_{A1}^2+g_{B1}^2}}g_{B2}\frac{1}{\sqrt{g_{A2}^2+g_{B2}^2}}\delta_{\text{At}1\text{At}2}\delta_{ij}\left(g_{\mu\nu}\right) \quad (1357)$$


---

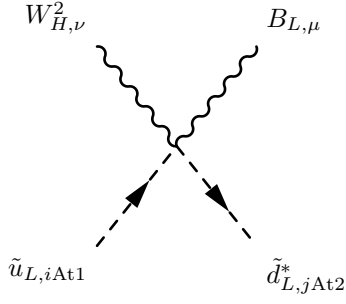

$$\frac{1}{6}g_{A1}g_{A2}g_{B1}\frac{1}{\sqrt{g_{A1}^2+g_{B1}^2}}\sqrt{\frac{g_{A2}^2}{g_{A2}^2+g_{B2}^2}}\delta_{\text{At}1\text{At}2}\delta_{ij}\left(g_{\mu\nu}\right) \quad (1358)$$


---

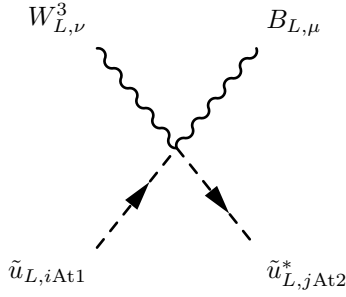

$$\frac{i}{6}g_{A1}g_{A2}g_{B1}\frac{1}{\sqrt{g_{A1}^2+g_{B1}^2}}g_{B2}\frac{1}{\sqrt{g_{A2}^2+g_{B2}^2}}\delta_{\text{At}1\text{At}2}\delta_{ij}\left(g_{\mu\nu}\right) \quad (1359)$$


---

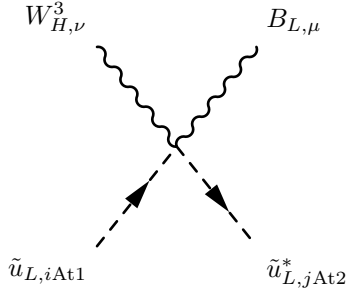

$$-\frac{i}{6}g_{A1}g_{A2}g_{B1}\frac{1}{\sqrt{g_{A1}^2+g_{B1}^2}}\sqrt{\frac{g_{A2}^2}{g_{A2}^2+g_{B2}^2}}\delta_{\text{At}1\text{At}2}\delta_{ij}\left(g_{\mu\nu}\right) \quad (1360)$$


---

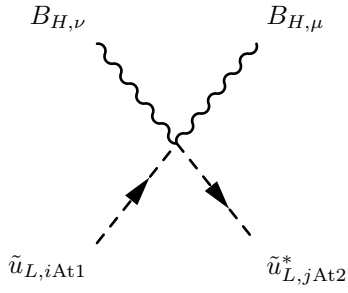

$$\frac{i}{18}g_{A1}^4\left(g_{A1}^2+g_{B1}^2\right)^{-1}\delta_{\text{At}1\text{At}2}\delta_{ij}\left(g_{\mu\nu}\right) \quad (1361)$$


---

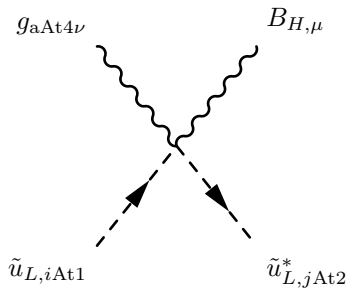

$$-\frac{i}{6}g_3g_{A1}\sqrt{\frac{g_{A1}^2}{g_{A1}^2+g_{B1}^2}}\delta_{ij}\lambda_{\text{At}2,\text{At}1}^{\text{aAt}4}\left(g_{\mu\nu}\right) \quad (1362)$$


---

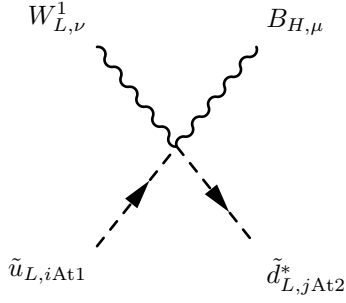

$$-\frac{i}{6}g_{A1}g_{A2}\sqrt{\frac{g_{A1}^2}{g_{A1}^2+g_{B1}^2}g_{B2}}\frac{1}{\sqrt{g_{A2}^2+g_{B2}^2}}\delta_{\text{At}1\text{At}2}\delta_{ij}\left(g_{\mu\nu}\right) \quad (1363)$$


---

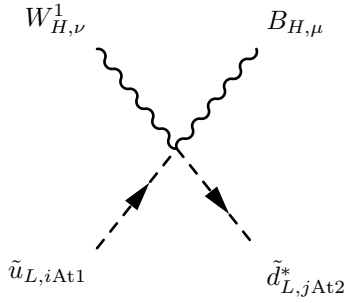

$$\frac{i}{6}g_{A1}g_{A2}\sqrt{\frac{g_{A1}^2}{g_{A1}^2+g_{B1}^2}}\sqrt{\frac{g_{A2}^2}{g_{A2}^2+g_{B2}^2}}\delta_{\text{At}1\text{At}2}\delta_{ij}\left(g_{\mu\nu}\right) \quad (1364)$$


---

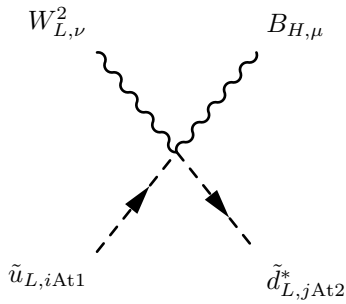

$$\frac{1}{6}g_{A1}g_{A2}\sqrt{\frac{g_{A1}^2}{g_{A1}^2+g_{B1}^2}g_{B2}}\frac{1}{\sqrt{g_{A2}^2+g_{B2}^2}}\delta_{\text{At}1\text{At}2}\delta_{ij}\left(g_{\mu\nu}\right) \quad (1365)$$


---

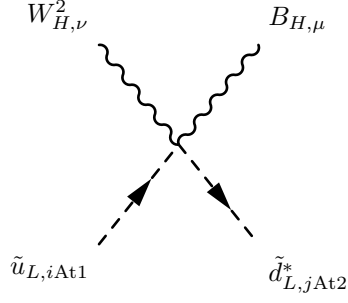

$$-\frac{1}{6}g_{A1}g_{A2}\sqrt{\frac{g_{A1}^2}{g_{A1}^2+g_{B1}^2}}\sqrt{\frac{g_{A2}^2}{g_{A2}^2+g_{B2}^2}}\delta_{\text{At}1\text{At}2}\delta_{ij}\left(g_{\mu\nu}\right) \quad (1366)$$


---

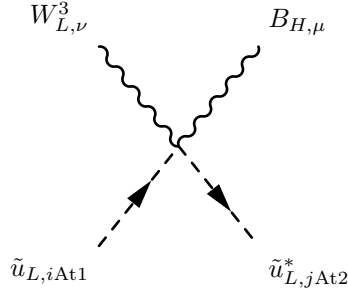

$$-\frac{i}{6}g_{A1}g_{A2}\sqrt{\frac{g_{A1}^2}{g_{A1}^2+g_{B1}^2}}g_{B2}\frac{1}{\sqrt{g_{A2}^2+g_{B2}^2}}\delta_{\text{At}1\text{At}2}\delta_{ij}\left(g_{\mu\nu}\right) \quad (1367)$$


---

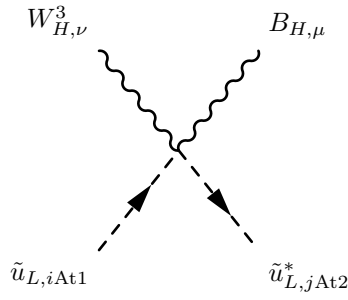

$$\frac{i}{6}g_{A1}g_{A2}\sqrt{\frac{g_{A1}^2}{g_{A1}^2+g_{B1}^2}}\sqrt{\frac{g_{A2}^2}{g_{A2}^2+g_{B2}^2}}\delta_{\text{At}1\text{At}2}\delta_{ij}\left(g_{\mu\nu}\right) \quad (1368)$$


---

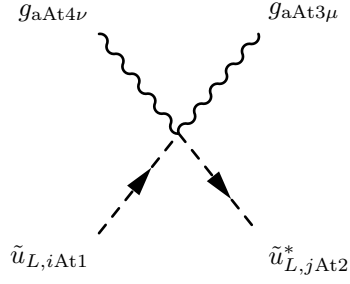

$$\frac{i}{4}g_3^2\delta_{ij}\left(\sum_{a=1}^3\lambda_{a,At1}^{aAt3}\lambda_{At2,a}^{aAt4}+\sum_{a=1}^3\lambda_{At2,a}^{aAt3}\lambda_{a,At1}^{aAt4}\right)\left(g_{\mu\nu}\right) \quad (1369)$$


---

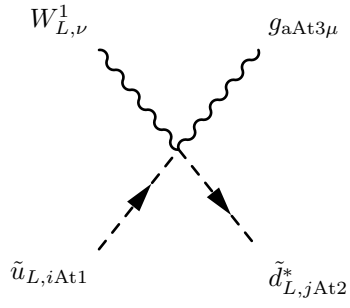

$$\frac{i}{2}g_3g_{A2}g_{B2}\frac{1}{\sqrt{gA2^2+gB2^2}}\delta_{ij}\lambda_{At2,At1}^{aAt3}\left(g_{\mu\nu}\right) \quad (1370)$$


---

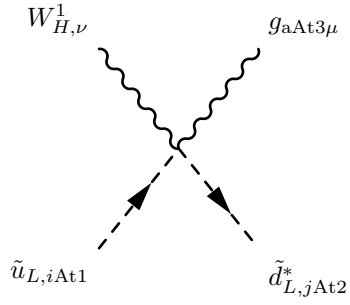

$$-\frac{i}{2}g_3g_{A2}\sqrt{\frac{gA2^2}{gA2^2+gB2^2}}\delta_{ij}\lambda_{At2,At1}^{aAt3}\left(g_{\mu\nu}\right) \quad (1371)$$


---

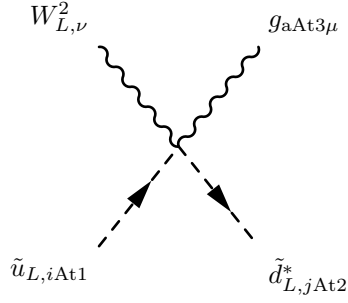

$$-\frac{1}{2}g_3g_{A2}g_{B2}\frac{1}{\sqrt{g_{A2}^2+g_{B2}^2}}\delta_{ij}\lambda_{At2,At1}^{aAt3}\left(g_{\mu\nu}\right) \quad (1372)$$


---

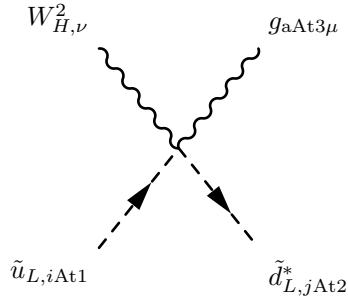

$$\frac{1}{2}g_3g_{A2}\sqrt{\frac{g_{A2}^2}{g_{A2}^2+g_{B2}^2}}\delta_{ij}\lambda_{At2,At1}^{aAt3}\left(g_{\mu\nu}\right) \quad (1373)$$


---

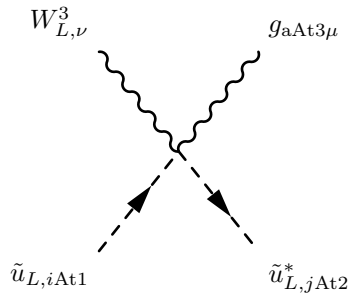

$$\frac{i}{2}g_3g_{A2}g_{B2}\frac{1}{\sqrt{g_{A2}^2+g_{B2}^2}}\delta_{ij}\lambda_{At2,At1}^{aAt3}\left(g_{\mu\nu}\right) \quad (1374)$$


---

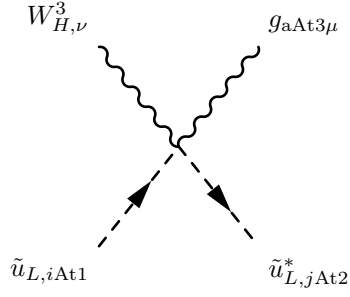

$$-\frac{i}{2}g_3g_{A2}\sqrt{\frac{g_{A2}^2}{g_{A2}^2+g_{B2}^2}}\delta_{ij}\lambda_{At2,At1}^{aAt3}(g_{\mu\nu}) \quad (1375)$$


---

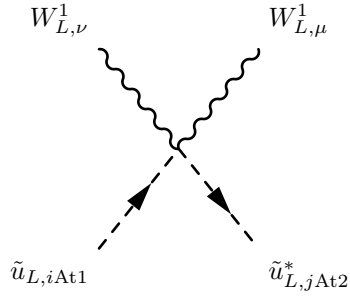

$$\frac{i}{2}g_{A2}^2g_{B2}^2(g_{A2}^2+g_{B2}^2)^{-1}\delta_{At1At2}\delta_{ij}(g_{\mu\nu}) \quad (1376)$$


---

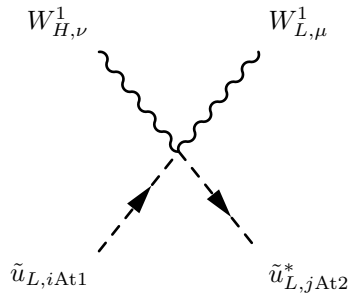

$$-\frac{i}{2}g_{B2}\left(\frac{g_{A2}^2}{g_{A2}^2+g_{B2}^2}\right)^{3/2}\sqrt{g_{A2}^2+g_{B2}^2}\delta_{At1At2}\delta_{ij}(g_{\mu\nu}) \quad (1377)$$


---



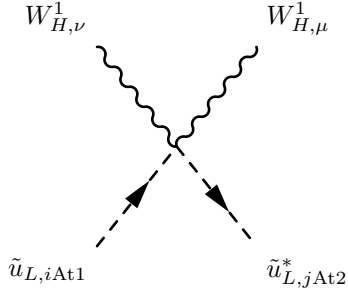

$$\frac{i}{2}g_{A2}^4\left(g_{A2}^2+g_{B2}^2\right)^{-1}\delta_{At1At2}\delta_{ij}\left(g_{\mu\nu}\right) \quad (1378)$$


---

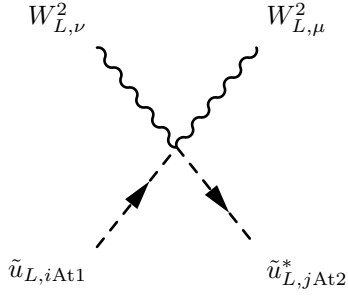

$$\frac{i}{2}g_{A2}^2g_{B2}^2\left(g_{A2}^2+g_{B2}^2\right)^{-1}\delta_{At1At2}\delta_{ij}\left(g_{\mu\nu}\right) \quad (1379)$$


---

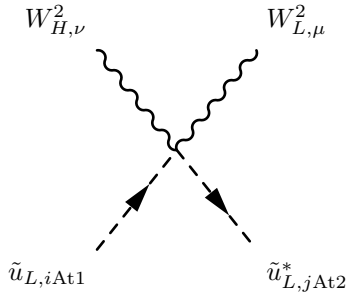

$$-\frac{i}{2}g_{B2}\left(\frac{g_{A2}^2}{g_{A2}^2+g_{B2}^2}\right)^{3/2}\sqrt{g_{A2}^2+g_{B2}^2}\delta_{At1At2}\delta_{ij}\left(g_{\mu\nu}\right) \quad (1380)$$


---

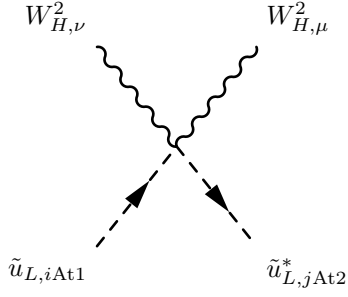

$$\frac{i}{2}g_{A2}^4\left(g_{A2}^2+g_{B2}^2\right)^{-1}\delta_{At1At2}\delta_{ij}\left(g_{\mu\nu}\right) \quad (1381)$$


---

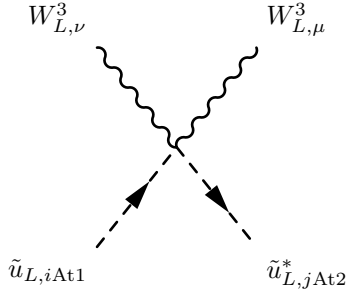

$$\frac{i}{2}g_{A2}^2g_{B2}^2\left(g_{A2}^2+g_{B2}^2\right)^{-1}\delta_{At1At2}\delta_{ij}\left(g_{\mu\nu}\right) \quad (1382)$$


---

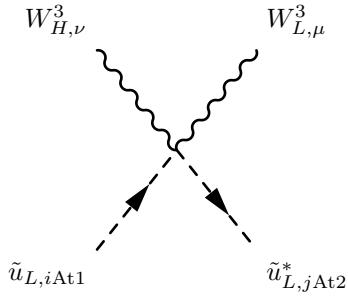

$$-\frac{i}{2}g_{B2}\left(\frac{g_{A2}^2}{g_{A2}^2+g_{B2}^2}\right)^{3/2}\sqrt{g_{A2}^2+g_{B2}^2}\delta_{At1At2}\delta_{ij}\left(g_{\mu\nu}\right) \quad (1383)$$


---

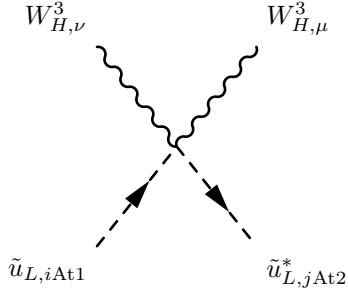

$$\frac{i}{2} g_{A2}^4 \left( g_{A2}^2 + g_{B2}^2 \right)^{-1} \delta_{At1At2} \delta_{ij} \left( g_{\mu\nu} \right) \quad (1384)$$


---

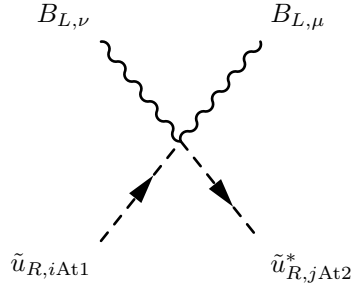

$$\frac{8i}{9} g_{A1}^2 g_{B1}^2 \left( g_{A1}^2 + g_{B1}^2 \right)^{-1} \delta_{At1At2} \delta_{ij} \left( g_{\mu\nu} \right) \quad (1385)$$


---

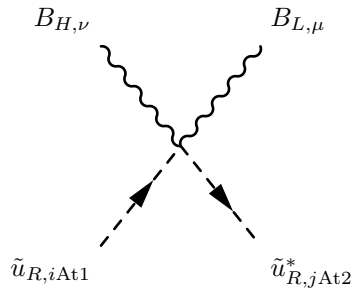

$$- \frac{8i}{9} g_{B1} \left( \frac{g_{A1}^2}{g_{A1}^2 + g_{B1}^2} \right)^{3/2} \sqrt{g_{A1}^2 + g_{B1}^2} \delta_{At1At2} \delta_{ij} \left( g_{\mu\nu} \right) \quad (1386)$$


---

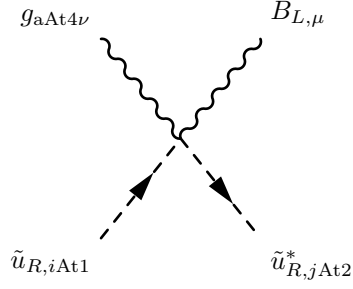

$$\frac{2i}{3} g_3 g_{A1} g_{B1} \frac{1}{\sqrt{g_{A1}^2 + g_{B1}^2}} \delta_{ij} \lambda_{At2,At1}^{aAt4} (g_{\mu\nu}) \quad (1387)$$


---

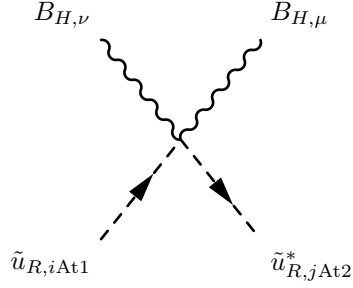

$$\frac{8i}{9} g_{A1}^4 (g_{A1}^2 + g_{B1}^2)^{-1} \delta_{At1At2} \delta_{ij} (g_{\mu\nu}) \quad (1388)$$


---

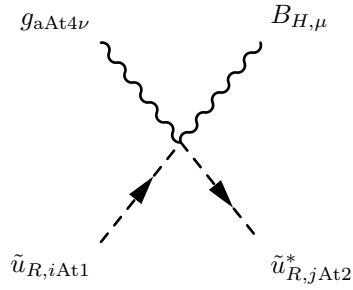

$$-\frac{2i}{3} g_3 g_{A1} \sqrt{\frac{g_{A1}^2}{g_{A1}^2 + g_{B1}^2}} \delta_{ij} \lambda_{At2,At1}^{aAt4} (g_{\mu\nu}) \quad (1389)$$


---

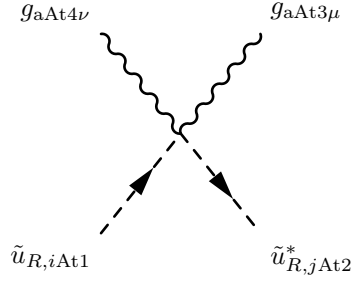

$$\frac{i}{4}g_3^2\delta_{ij}\left(\sum_{a=1}^3\lambda_{a,At1}^{aAt3}\lambda_{At2,a}^{aAt4}+\sum_{a=1}^3\lambda_{At2,a}^{aAt3}\lambda_{a,At1}^{aAt4}\right)\left(g_{\mu\nu}\right) \quad (1390)$$


---

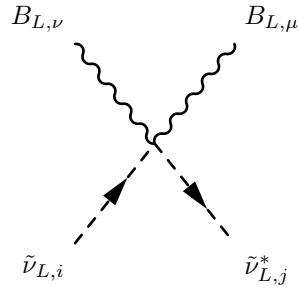

$$\frac{i}{2}g_{A1}^2g_{B1}^2\left(g_{A1}^2+g_{B1}^2\right)^{-1}\delta_{ij}\left(g_{\mu\nu}\right) \quad (1391)$$


---

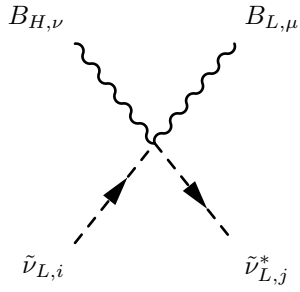

$$-\frac{i}{2}g_{B1}\left(\frac{gA1^2}{gA1^2+gB1^2}\right)^{3/2}\sqrt{gA1^2+gB1^2}\delta_{ij}\left(g_{\mu\nu}\right) \quad (1392)$$


---

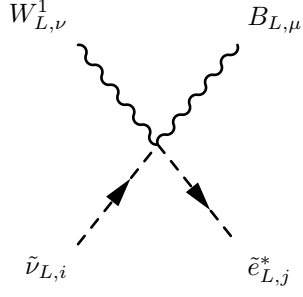

$$-\frac{i}{2}g_{A1}g_{A2}g_{B1}\frac{1}{\sqrt{g_{A1}^2+g_{B1}^2}}g_{B2}\frac{1}{\sqrt{g_{A2}^2+g_{B2}^2}}\delta_{ij}\left(g_{\mu\nu}\right) \quad (1393)$$


---

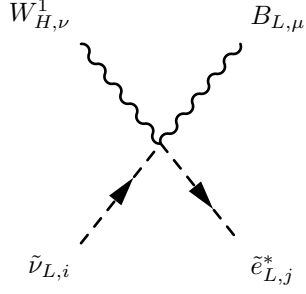

$$\frac{i}{2}g_{A1}g_{A2}g_{B1}\frac{1}{\sqrt{g_{A1}^2+g_{B1}^2}}\sqrt{\frac{g_{A2}^2}{g_{A2}^2+g_{B2}^2}}\delta_{ij}\left(g_{\mu\nu}\right) \quad (1394)$$


---

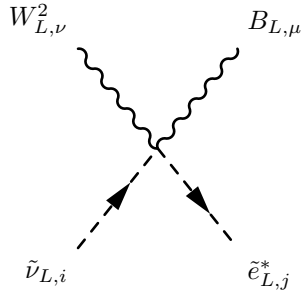

$$\frac{1}{2}g_{A1}g_{A2}g_{B1}\frac{1}{\sqrt{g_{A1}^2+g_{B1}^2}}g_{B2}\frac{1}{\sqrt{g_{A2}^2+g_{B2}^2}}\delta_{ij}\left(g_{\mu\nu}\right) \quad (1395)$$


---

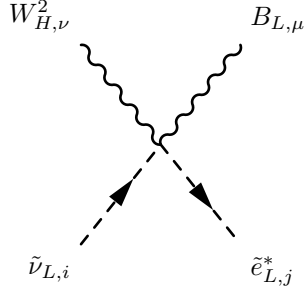

$$-\frac{1}{2}g_{A1}g_{A2}g_{B1}\frac{1}{\sqrt{g_{A1}^2+g_{B1}^2}}\sqrt{\frac{g_{A2}^2}{g_{A2}^2+g_{B2}^2}}\delta_{ij}\left(g_{\mu\nu}\right) \quad (1396)$$


---

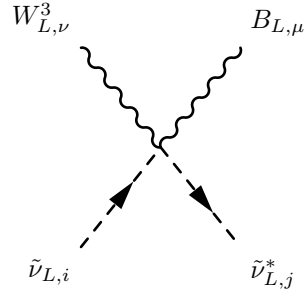

$$-\frac{i}{2}g_{A1}g_{A2}g_{B1}\frac{1}{\sqrt{g_{A1}^2+g_{B1}^2}}g_{B2}\frac{1}{\sqrt{g_{A2}^2+g_{B2}^2}}\delta_{ij}\left(g_{\mu\nu}\right) \quad (1397)$$


---

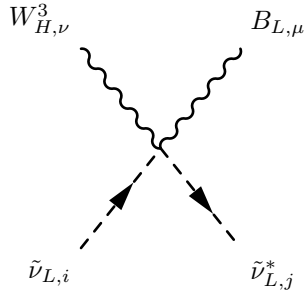

$$\frac{i}{2}g_{A1}g_{A2}g_{B1}\frac{1}{\sqrt{g_{A1}^2+g_{B1}^2}}\sqrt{\frac{g_{A2}^2}{g_{A2}^2+g_{B2}^2}}\delta_{ij}\left(g_{\mu\nu}\right) \quad (1398)$$


---

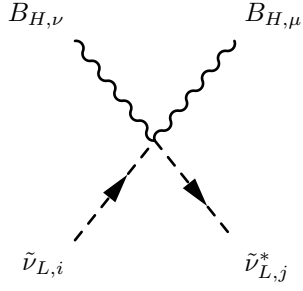

$$\frac{i}{2}g_{A1}^4\left(g_{A1}^2+g_{B1}^2\right)^{-1}\delta_{ij}\left(g_{\mu\nu}\right) \quad (1399)$$


---

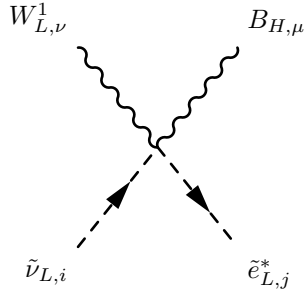

$$\frac{i}{2}g_{A1}g_{A2}\sqrt{\frac{g_{A1}^2}{g_{A1}^2+g_{B1}^2}}g_{B2}\frac{1}{\sqrt{g_{A2}^2+g_{B2}^2}}\delta_{ij}\left(g_{\mu\nu}\right) \quad (1400)$$


---

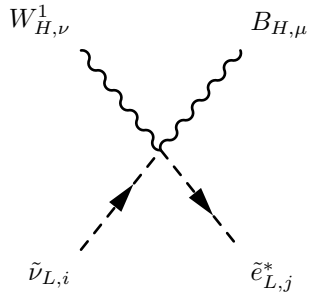

$$-\frac{i}{2}g_{A1}g_{A2}\sqrt{\frac{g_{A1}^2}{g_{A1}^2+g_{B1}^2}}\sqrt{\frac{g_{A2}^2}{g_{A2}^2+g_{B2}^2}}\delta_{ij}\left(g_{\mu\nu}\right) \quad (1401)$$


---



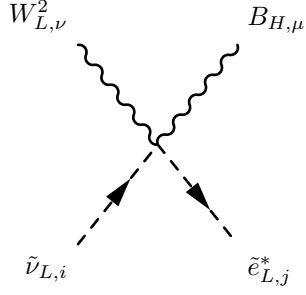

$$-\frac{1}{2}g_{A1}g_{A2}\sqrt{\frac{g_{A1}^2}{g_{A1}^2+g_{B1}^2}}g_{B2}\frac{1}{\sqrt{g_{A2}^2+g_{B2}^2}}\delta_{ij}\left(g_{\mu\nu}\right) \quad (1402)$$


---

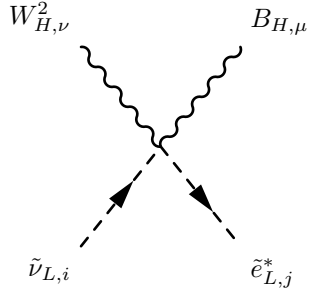

$$\frac{1}{2}g_{A1}g_{A2}\sqrt{\frac{g_{A1}^2}{g_{A1}^2+g_{B1}^2}}\sqrt{\frac{g_{A2}^2}{g_{A2}^2+g_{B2}^2}}\delta_{ij}\left(g_{\mu\nu}\right) \quad (1403)$$


---

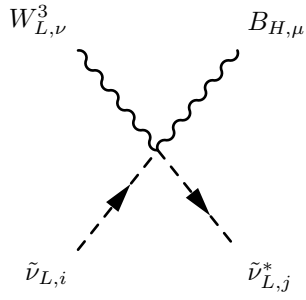

$$\frac{i}{2}g_{A1}g_{A2}\sqrt{\frac{g_{A1}^2}{g_{A1}^2+g_{B1}^2}}g_{B2}\frac{1}{\sqrt{g_{A2}^2+g_{B2}^2}}\delta_{ij}\left(g_{\mu\nu}\right) \quad (1404)$$


---

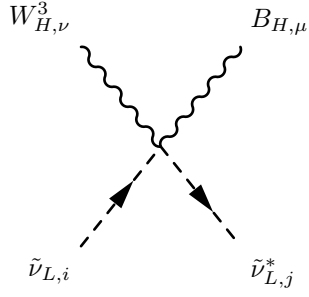

$$-\frac{i}{2}g_{A1}g_{A2}\sqrt{\frac{g_{A1}^2}{g_{A1}^2+g_{B1}^2}}\sqrt{\frac{g_{A2}^2}{g_{A2}^2+g_{B2}^2}}\delta_{ij}\left(g_{\mu\nu}\right) \quad (1405)$$


---

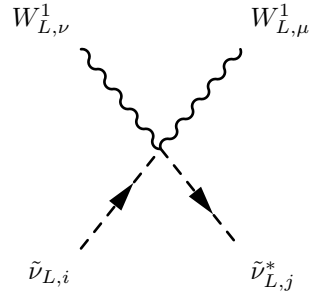

$$\frac{i}{2}g_{A2}^2g_{B2}^2\left(g_{A2}^2+g_{B2}^2\right)^{-1}\delta_{ij}\left(g_{\mu\nu}\right) \quad (1406)$$


---

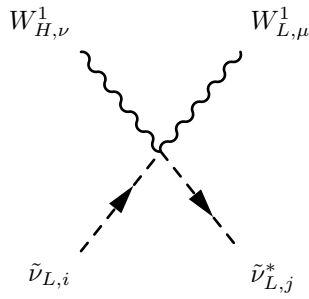

$$-\frac{i}{2}g_{B2}\left(\frac{g_{A2}^2}{g_{A2}^2+g_{B2}^2}\right)^{3/2}\sqrt{g_{A2}^2+g_{B2}^2}\delta_{ij}\left(g_{\mu\nu}\right) \quad (1407)$$


---

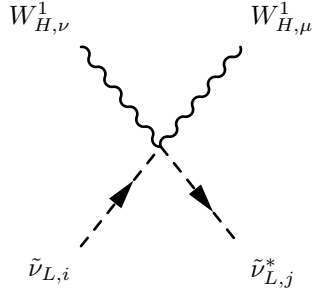

$$\frac{i}{2}g_{A2}^4\left(g_{A2}^2+g_{B2}^2\right)^{-1}\delta_{ij}\left(g_{\mu\nu}\right) \quad (1408)$$


---

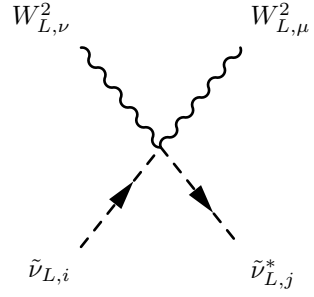

$$\frac{i}{2}g_{A2}^2g_{B2}^2\left(g_{A2}^2+g_{B2}^2\right)^{-1}\delta_{ij}\left(g_{\mu\nu}\right) \quad (1409)$$


---

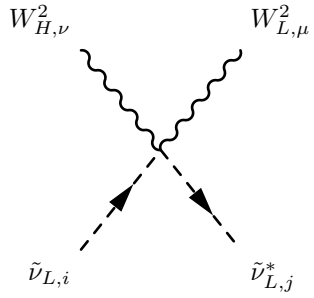

$$-\frac{i}{2}g_{B2}\left(\frac{g_{A2}^2}{g_{A2}^2+g_{B2}^2}\right)^{3/2}\sqrt{g_{A2}^2+g_{B2}^2}\delta_{ij}\left(g_{\mu\nu}\right) \quad (1410)$$


---

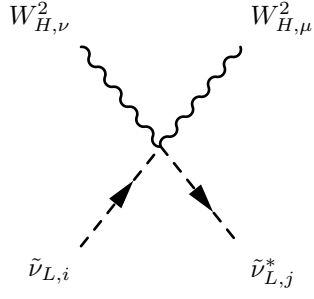

$$\frac{i}{2}g_{A2}^4\left(g_{A2}^2+g_{B2}^2\right)^{-1}\delta_{ij}\left(g_{\mu\nu}\right) \quad (1411)$$


---

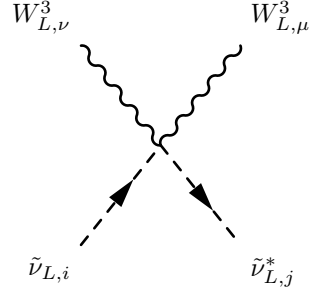

$$\frac{i}{2}g_{A2}^2g_{B2}^2\left(g_{A2}^2+g_{B2}^2\right)^{-1}\delta_{ij}\left(g_{\mu\nu}\right) \quad (1412)$$


---

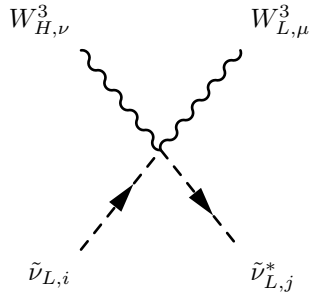

$$-\frac{i}{2}g_{B2}\left(\frac{g_{A2}^2}{g_{A2}^2+g_{B2}^2}\right)^{3/2}\sqrt{g_{A2}^2+g_{B2}^2}\delta_{ij}\left(g_{\mu\nu}\right) \quad (1413)$$


---

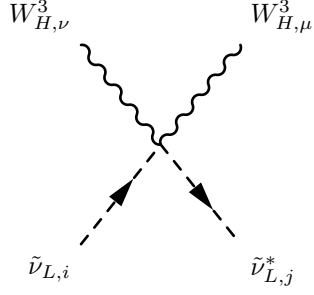

$$\frac{i}{2}g_{A2}^4\left(g_{A2}^2+g_{B2}^2\right)^{-1}\delta_{ij}\left(g_{\mu\nu}\right) \quad (1414)$$


---

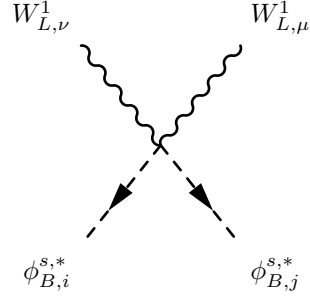

$$-ig_{A2}^2g_{B2}^2\left(g_{A2}^2+g_{B2}^2\right)^{-1}\left(B_{A,i1}^sB_{A,j2}^s+B_{A,i2}^sB_{A,j1}^s\right)\left(g_{\mu\nu}\right) \quad (1415)$$


---

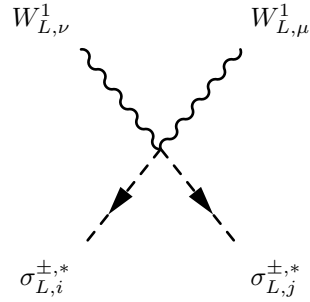

$$-ig_{A2}g_{B2}^2\sqrt{\frac{\text{gA}2^2}{\text{gA}2^2+\text{gB}2^2}}\frac{1}{\sqrt{\text{gA}2^2+\text{gB}2^2}}\left(Z_{Ls,i1}^{od}Z_{Ls,j4}^{od}+Z_{Ls,i2}^{od}Z_{Ls,j3}^{od}+Z_{Ls,i3}^{od}Z_{Ls,j2}^{od}+Z_{Ls,i4}^{od}Z_{Ls,j1}^{od}\right)\left(g_{\mu\nu}\right) \quad (1416)$$


---

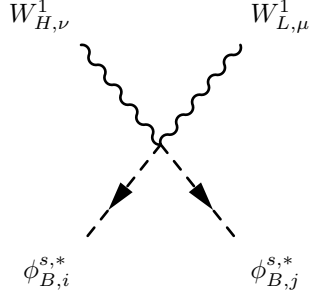

$$-ig_{B2}^3 \sqrt{\frac{gA2^2}{gA2^2 + gB2^2}} \frac{1}{\sqrt{gA2^2 + gB2^2}} \left( B_{A,i1}^s B_{A,j2}^s + B_{A,i2}^s B_{A,j1}^s \right) (g_{\mu\nu}) \quad (1417)$$


---

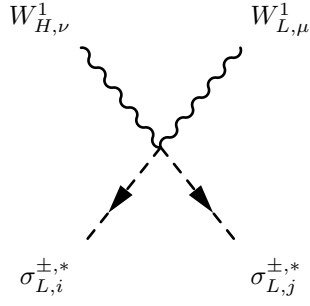

$$\frac{i}{2} g_{A2} g_{B2} \left( -g_{B2}^2 + g_{A2}^2 \right) \left( g_{A2}^2 + g_{B2}^2 \right)^{-1} \left( Z_{Ls,i1}^{od} Z_{Ls,j4}^{od} + Z_{Ls,i2}^{od} Z_{Ls,j3}^{od} + Z_{Ls,i3}^{od} Z_{Ls,j2}^{od} + Z_{Ls,i4}^{od} Z_{Ls,j1}^{od} \right) (g_{\mu\nu}) \quad (1418)$$


---

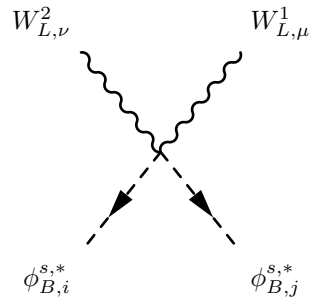

$$-g_{A2}^2 g_{B2}^2 \left( g_{A2}^2 + g_{B2}^2 \right)^{-1} \left( B_{A,i1}^s B_{A,j2}^s + B_{A,i2}^s B_{A,j1}^s \right) (g_{\mu\nu}) \quad (1419)$$


---

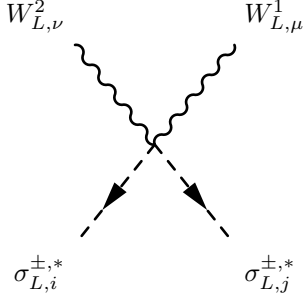

$$-g_{A2}g_{B2}^2\sqrt{\frac{gA2^2}{gA2^2+gB2^2}}\frac{1}{\sqrt{gA2^2+gB2^2}}\left(Z_{Ls,i1}^{od}Z_{Ls,j4}^{od}+Z_{Ls,i2}^{od}Z_{Ls,j3}^{od}+Z_{Ls,i3}^{od}Z_{Ls,j2}^{od}+Z_{Ls,i4}^{od}Z_{Ls,j1}^{od}\right)\left(g_{\mu\nu}\right) \quad (1420)$$


---

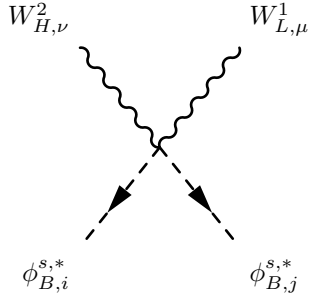

$$-g_{B2}^3\sqrt{\frac{gA2^2}{gA2^2+gB2^2}}\frac{1}{\sqrt{gA2^2+gB2^2}}\left(B_{A,i1}^sB_{A,j2}^s+B_{A,i2}^sB_{A,j1}^s\right)\left(g_{\mu\nu}\right) \quad (1421)$$


---

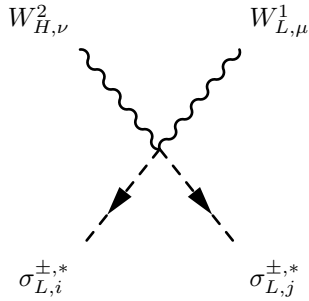

$$\frac{1}{2}g_{A2}g_{B2}\left(-g_{B2}^2+g_{A2}^2\right)\left(g_{A2}^2+g_{B2}^2\right)^{-1}\left(Z_{Ls,i1}^{od}Z_{Ls,j4}^{od}+Z_{Ls,i2}^{od}Z_{Ls,j3}^{od}+Z_{Ls,i3}^{od}Z_{Ls,j2}^{od}+Z_{Ls,i4}^{od}Z_{Ls,j1}^{od}\right)\left(g_{\mu\nu}\right) \quad (1422)$$


---

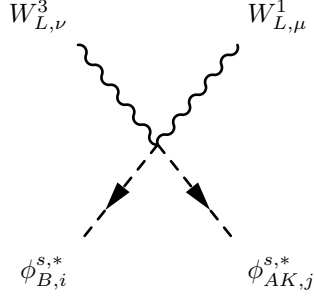

$$-i \frac{1}{\sqrt{2}} g_{A2}^2 g_{B2}^2 (g_{A2}^2 + g_{B2}^2)^{-1} Z_{AK,j2}^s B_{A,i2}^s (g_{\mu\nu}) \quad (1423)$$


---

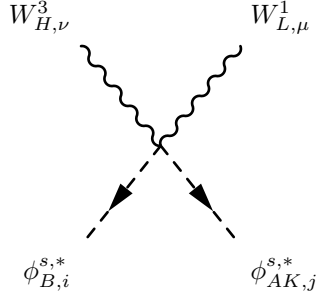

$$-i \frac{1}{\sqrt{2}} g_{B2}^3 \sqrt{\frac{g_{A2}^2}{g_{A2}^2 + g_{B2}^2}} \frac{1}{\sqrt{g_{A2}^2 + g_{B2}^2}} Z_{AK,j2}^s B_{A,i2}^s (g_{\mu\nu}) \quad (1424)$$


---

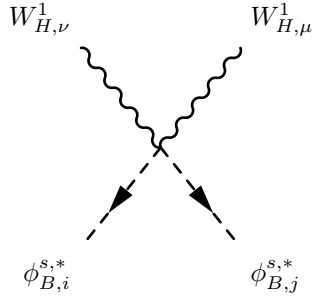

$$-i g_{B2}^4 (g_{A2}^2 + g_{B2}^2)^{-1} (B_{A,i1}^s B_{A,j2}^s + B_{A,i2}^s B_{A,j1}^s) (g_{\mu\nu}) \quad (1425)$$


---



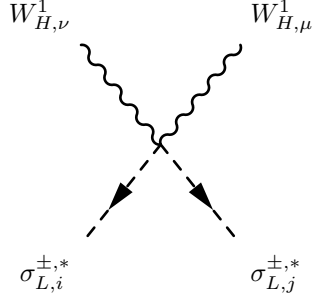

$$ig_{A2}g_{B2}^2\sqrt{\frac{g_{A2}^2}{g_{A2}^2+g_{B2}^2}}\frac{1}{\sqrt{g_{A2}^2+g_{B2}^2}}\left(Z_{Ls,i1}^{od}Z_{Ls,j4}^{od}+Z_{Ls,i2}^{od}Z_{Ls,j3}^{od}+Z_{Ls,i3}^{od}Z_{Ls,j2}^{od}+Z_{Ls,i4}^{od}Z_{Ls,j1}^{od}\right)\left(g_{\mu\nu}\right) \quad (1426)$$


---

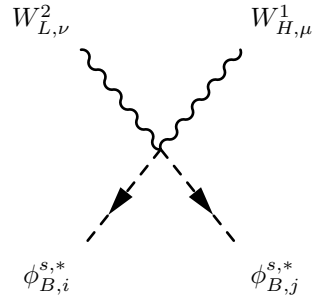

$$-g_{B2}^3\sqrt{\frac{g_{A2}^2}{g_{A2}^2+g_{B2}^2}}\frac{1}{\sqrt{g_{A2}^2+g_{B2}^2}}\left(B_{A,i1}^sB_{A,j2}^s+B_{A,i2}^sB_{A,j1}^s\right)\left(g_{\mu\nu}\right) \quad (1427)$$


---

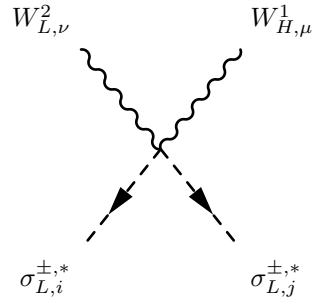

$$\frac{1}{2}g_{A2}g_{B2}\left(-g_{B2}^2+g_{A2}^2\right)\left(g_{A2}^2+g_{B2}^2\right)^{-1}\left(Z_{Ls,i1}^{od}Z_{Ls,j4}^{od}+Z_{Ls,i2}^{od}Z_{Ls,j3}^{od}+Z_{Ls,i3}^{od}Z_{Ls,j2}^{od}+Z_{Ls,i4}^{od}Z_{Ls,j1}^{od}\right)\left(g_{\mu\nu}\right) \quad (1428)$$


---

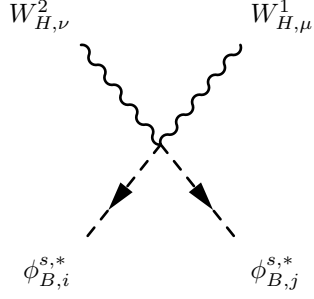

$$-g_{B2}^4 \left( g_{A2}^2 + g_{B2}^2 \right)^{-1} \left( B_{A,i1}^s B_{A,j2}^s + B_{A,i2}^s B_{A,j1}^s \right) \left( g_{\mu\nu} \right) \quad (1429)$$


---

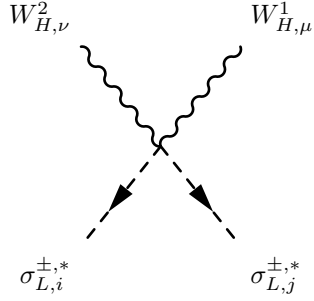

$$g_{A2} g_{B2}^2 \sqrt{\frac{g_{A2}^2}{g_{A2}^2 + g_{B2}^2}} \frac{1}{\sqrt{g_{A2}^2 + g_{B2}^2}} \left( Z_{Ls,i1}^{od} Z_{Ls,j4}^{od} + Z_{Ls,i2}^{od} Z_{Ls,j3}^{od} + Z_{Ls,i3}^{od} Z_{Ls,j2}^{od} + Z_{Ls,i4}^{od} Z_{Ls,j1}^{od} \right) \left( g_{\mu\nu} \right) \quad (1430)$$


---

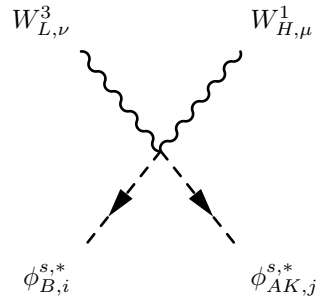

$$-i \frac{1}{\sqrt{2}} g_{B2}^3 \sqrt{\frac{g_{A2}^2}{g_{A2}^2 + g_{B2}^2}} \frac{1}{\sqrt{g_{A2}^2 + g_{B2}^2}} Z_{AK,j2}^s B_{A,i2}^s \left( g_{\mu\nu} \right) \quad (1431)$$


---

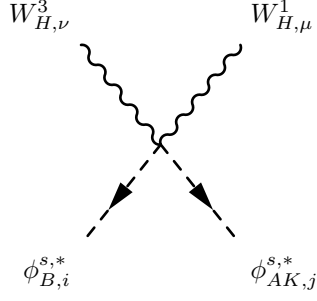

$$-i \frac{1}{\sqrt{2}} g_{B2}^4 \left( g_{A2}^2 + g_{B2}^2 \right)^{-1} Z_{AK,j2}^s B_{A,i2}^s \left( g_{\mu\nu} \right) \quad (1432)$$


---

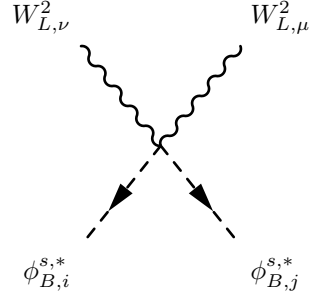

$$i g_{A2}^2 g_{B2}^2 \left( g_{A2}^2 + g_{B2}^2 \right)^{-1} \left( B_{A,i1}^s B_{A,j2}^s + B_{A,i2}^s B_{A,j1}^s \right) \left( g_{\mu\nu} \right) \quad (1433)$$


---

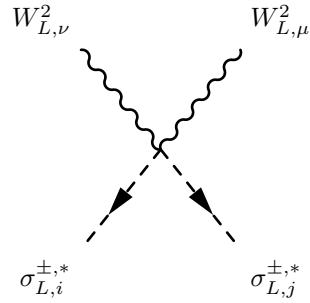

$$i g_{A2} g_{B2}^2 \sqrt{\frac{g_{A2}^2}{g_{A2}^2 + g_{B2}^2}} \frac{1}{\sqrt{g_{A2}^2 + g_{B2}^2}} \left( Z_{Ls,i1}^{od} Z_{Ls,j4}^{od} + Z_{Ls,i2}^{od} Z_{Ls,j3}^{od} + Z_{Ls,i3}^{od} Z_{Ls,j2}^{od} + Z_{Ls,i4}^{od} Z_{Ls,j1}^{od} \right) \left( g_{\mu\nu} \right) \quad (1434)$$


---

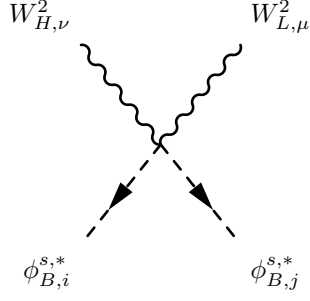

$$ig_{B2}^3 \sqrt{\frac{gA2^2}{gA2^2 + gB2^2}} \frac{1}{\sqrt{gA2^2 + gB2^2}} \left( B_{A,i1}^s B_{A,j2}^s + B_{A,i2}^s B_{A,j1}^s \right) (g_{\mu\nu}) \quad (1435)$$


---

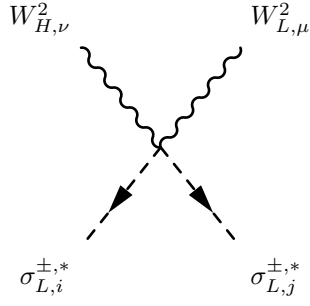

$$-\frac{i}{2} g_{A2} g_{B2} \left( -g_{B2}^2 + g_{A2}^2 \right) \left( g_{A2}^2 + g_{B2}^2 \right)^{-1} \left( Z_{Ls,i1}^{od} Z_{Ls,j4}^{od} + Z_{Ls,i2}^{od} Z_{Ls,j3}^{od} + Z_{Ls,i3}^{od} Z_{Ls,j2}^{od} + Z_{Ls,i4}^{od} Z_{Ls,j1}^{od} \right) (g_{\mu\nu}) \quad (1436)$$


---

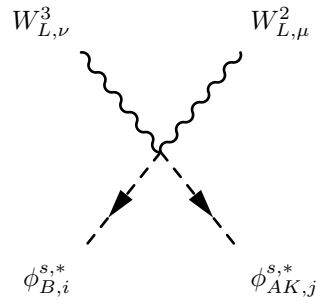

$$-\frac{1}{\sqrt{2}} g_{A2}^2 g_{B2}^2 \left( g_{A2}^2 + g_{B2}^2 \right)^{-1} Z_{AK,j2}^s B_{A,i2}^s (g_{\mu\nu}) \quad (1437)$$


---

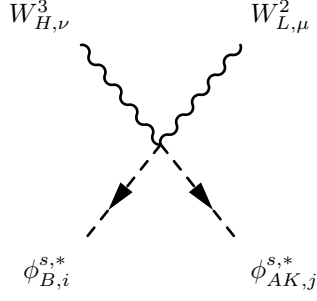

$$-\frac{1}{\sqrt{2}}g_{B2}^3\sqrt{\frac{gA2^2}{gA2^2+gB2^2}}\frac{1}{\sqrt{gA2^2+gB2^2}}Z_{AK,j2}^sB_{A,i2}^s\left(g_{\mu\nu}\right) \quad (1438)$$


---

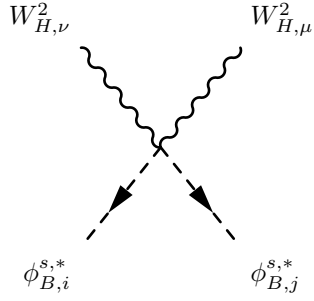

$$ig_{B2}^4\left(g_{A2}^2+g_{B2}^2\right)^{-1}\left(B_{A,i1}^sB_{A,j2}^s+B_{A,i2}^sB_{A,j1}^s\right)\left(g_{\mu\nu}\right) \quad (1439)$$


---

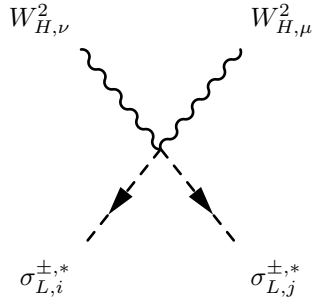

$$-ig_{A2}g_{B2}^2\sqrt{\frac{gA2^2}{gA2^2+gB2^2}}\frac{1}{\sqrt{gA2^2+gB2^2}}\left(Z_{Ls,i1}^{od}Z_{Ls,j4}^{od}+Z_{Ls,i2}^{od}Z_{Ls,j3}^{od}+Z_{Ls,i3}^{od}Z_{Ls,j2}^{od}+Z_{Ls,i4}^{od}Z_{Ls,j1}^{od}\right)\left(g_{\mu\nu}\right) \quad (1440)$$


---

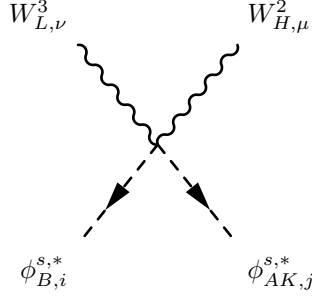

$$-\frac{1}{\sqrt{2}}g_{B2}^3\sqrt{\frac{g_{A2}^2}{g_{A2}^2+g_{B2}^2}}\frac{1}{\sqrt{g_{A2}^2+g_{B2}^2}}Z_{AK,j2}^sB_{A,i2}^s(g_{\mu\nu}) \quad (1441)$$


---

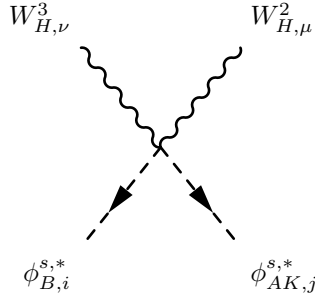

$$-\frac{1}{\sqrt{2}}g_{B2}^4(g_{A2}^2+g_{B2}^2)^{-1}Z_{AK,j2}^sB_{A,i2}^s(g_{\mu\nu}) \quad (1442)$$


---

## 9.9 Four Vector Boson-Interaction

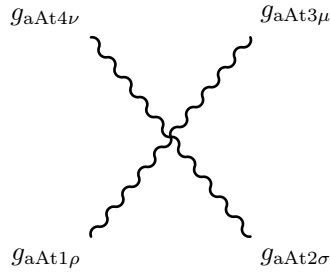

$$-ig_3^2\left(\sum_{a=1}^8f_{aAt1,aAt4,a}f_{aAt2,aAt3,a}+\sum_{a=1}^8f_{aAt1,aAt3,a}f_{aAt2,aAt4,a}\right)(g_{\rho\sigma}g_{\mu\nu}) \quad (1443)$$

$$+ ig_3^2 \left( - \sum_{a=1}^8 f_{aAt1,aAt2,a} f_{aAt3,aAt4,a} + \sum_{a=1}^8 f_{aAt1,aAt4,a} f_{aAt2,aAt3,a} \right) (g_{\rho\mu} g_{\sigma\nu}) \quad (1444)$$

$$+ ig_3^2 \left( \sum_{a=1}^8 f_{aAt1,aAt3,a} f_{aAt2,aAt4,a} + \sum_{a=1}^8 f_{aAt1,aAt2,a} f_{aAt3,aAt4,a} \right) (g_{\rho\nu} g_{\sigma\mu}) \quad (1445)$$

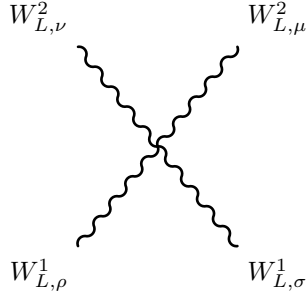

$$- 2ig_{A2}^2 g_{B2}^2 (g_{A2}^2 + g_{B2}^2)^{-1} (g_{\rho\sigma} g_{\mu\nu}) \quad (1446)$$

$$+ ig_{A2}^2 g_{B2}^2 (g_{A2}^2 + g_{B2}^2)^{-1} (g_{\rho\mu} g_{\sigma\nu}) \quad (1447)$$

$$+ ig_{A2}^2 g_{B2}^2 (g_{A2}^2 + g_{B2}^2)^{-1} (g_{\rho\nu} g_{\sigma\mu}) \quad (1448)$$

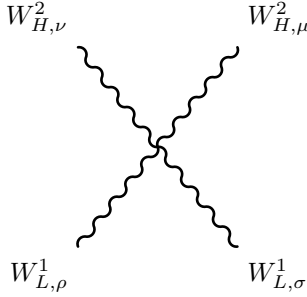

$$- 2ig_{A2}^2 g_{B2}^2 (g_{A2}^2 + g_{B2}^2)^{-1} (g_{\rho\sigma} g_{\mu\nu}) \quad (1449)$$

$$+ ig_{A2}^2 g_{B2}^2 (g_{A2}^2 + g_{B2}^2)^{-1} (g_{\rho\mu} g_{\sigma\nu}) \quad (1450)$$

$$+ ig_{A2}^2 g_{B2}^2 (g_{A2}^2 + g_{B2}^2)^{-1} (g_{\rho\nu} g_{\sigma\mu}) \quad (1451)$$

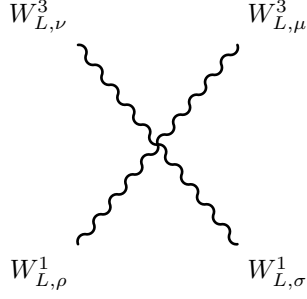

$$- 2i g_{A2}^2 g_{B2}^2 \left( g_{A2}^2 + g_{B2}^2 \right)^{-1} \left( g_{\rho\sigma} g_{\mu\nu} \right) \quad (1452)$$

$$+ i g_{A2}^2 g_{B2}^2 \left( g_{A2}^2 + g_{B2}^2 \right)^{-1} \left( g_{\rho\mu} g_{\sigma\nu} \right) \quad (1453)$$

$$+ i g_{A2}^2 g_{B2}^2 \left( g_{A2}^2 + g_{B2}^2 \right)^{-1} \left( g_{\rho\nu} g_{\sigma\mu} \right) \quad (1454)$$


---

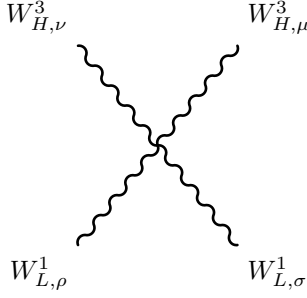

$$- 2i g_{A2}^2 g_{B2}^2 \left( g_{A2}^2 + g_{B2}^2 \right)^{-1} \left( g_{\rho\sigma} g_{\mu\nu} \right) \quad (1455)$$

$$+ i g_{A2}^2 g_{B2}^2 \left( g_{A2}^2 + g_{B2}^2 \right)^{-1} \left( g_{\rho\mu} g_{\sigma\nu} \right) \quad (1456)$$

$$+ i g_{A2}^2 g_{B2}^2 \left( g_{A2}^2 + g_{B2}^2 \right)^{-1} \left( g_{\rho\nu} g_{\sigma\mu} \right) \quad (1457)$$


---

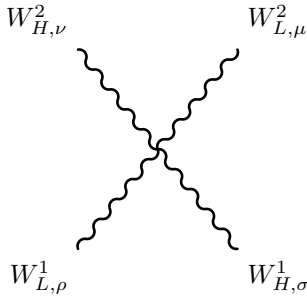



$$- 2ig_{A2}^2 g_{B2}^2 (g_{A2}^2 + g_{B2}^2)^{-1} (g_{\rho\sigma} g_{\mu\nu}) \quad (1458)$$

$$+ ig_{A2}^2 g_{B2}^2 (g_{A2}^2 + g_{B2}^2)^{-1} (g_{\rho\mu} g_{\sigma\nu}) \quad (1459)$$

$$+ ig_{A2}^2 g_{B2}^2 (g_{A2}^2 + g_{B2}^2)^{-1} (g_{\rho\nu} g_{\sigma\mu}) \quad (1460)$$

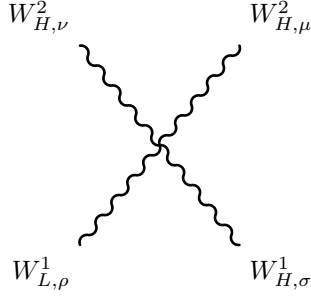

$$2ig_{B2} (-g_{B2}^2 + g_{A2}^2) \sqrt{\frac{gA2^2}{gA2^2 + gB2^2}} \frac{1}{\sqrt{gA2^2 + gB2^2}} (g_{\rho\sigma} g_{\mu\nu}) \quad (1461)$$

$$+ -ig_{B2} (-g_{B2}^2 + g_{A2}^2) \sqrt{\frac{gA2^2}{gA2^2 + gB2^2}} \frac{1}{\sqrt{gA2^2 + gB2^2}} (g_{\rho\mu} g_{\sigma\nu}) \quad (1462)$$

$$+ -ig_{B2} (-g_{B2}^2 + g_{A2}^2) \sqrt{\frac{gA2^2}{gA2^2 + gB2^2}} \frac{1}{\sqrt{gA2^2 + gB2^2}} (g_{\rho\nu} g_{\sigma\mu}) \quad (1463)$$

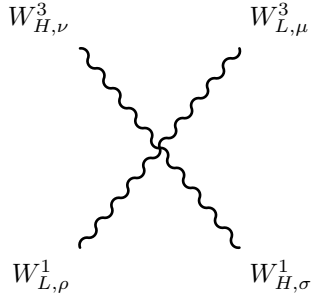

$$- 2ig_{A2}^2 g_{B2}^2 (g_{A2}^2 + g_{B2}^2)^{-1} (g_{\rho\sigma} g_{\mu\nu}) \quad (1464)$$

$$+ ig_{A2}^2 g_{B2}^2 (g_{A2}^2 + g_{B2}^2)^{-1} (g_{\rho\mu} g_{\sigma\nu}) \quad (1465)$$

$$+ ig_{A2}^2 g_{B2}^2 (g_{A2}^2 + g_{B2}^2)^{-1} (g_{\rho\nu} g_{\sigma\mu}) \quad (1466)$$

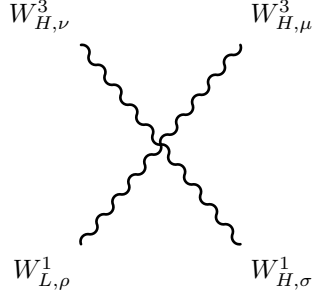

$$2ig_{B2}\left(-g_{B2}^2 + g_{A2}^2\right)\sqrt{\frac{gA2^2}{gA2^2 + gB2^2}}\frac{1}{\sqrt{gA2^2 + gB2^2}}\left(g_{\rho\sigma}g_{\mu\nu}\right) \quad (1467)$$

$$+ -ig_{B2}\left(-g_{B2}^2 + g_{A2}^2\right)\sqrt{\frac{gA2^2}{gA2^2 + gB2^2}}\frac{1}{\sqrt{gA2^2 + gB2^2}}\left(g_{\rho\mu}g_{\sigma\nu}\right) \quad (1468)$$

$$+ -ig_{B2}\left(-g_{B2}^2 + g_{A2}^2\right)\sqrt{\frac{gA2^2}{gA2^2 + gB2^2}}\frac{1}{\sqrt{gA2^2 + gB2^2}}\left(g_{\rho\nu}g_{\sigma\mu}\right) \quad (1469)$$


---

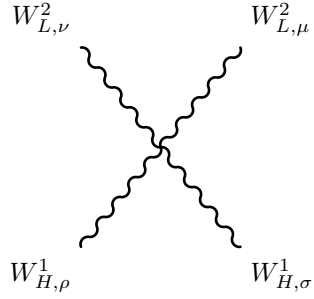

$$- 2ig_{A2}^2g_{B2}^2\left(g_{A2}^2 + g_{B2}^2\right)^{-1}\left(g_{\rho\sigma}g_{\mu\nu}\right) \quad (1470)$$

$$+ ig_{A2}^2g_{B2}^2\left(g_{A2}^2 + g_{B2}^2\right)^{-1}\left(g_{\rho\mu}g_{\sigma\nu}\right) \quad (1471)$$

$$+ ig_{A2}^2g_{B2}^2\left(g_{A2}^2 + g_{B2}^2\right)^{-1}\left(g_{\rho\nu}g_{\sigma\mu}\right) \quad (1472)$$


---

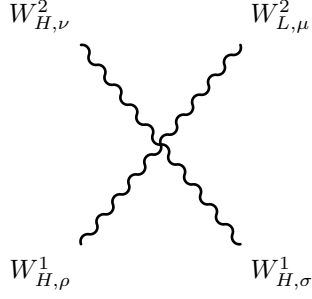

$$2ig_{B2}\left(-g_{B2}^2+g_{A2}^2\right)\sqrt{\frac{gA2^2}{gA2^2+gB2^2}}\frac{1}{\sqrt{gA2^2+gB2^2}}\left(g_{\rho\sigma}g_{\mu\nu}\right) \quad (1473)$$

$$+ -ig_{B2}\left(-g_{B2}^2+g_{A2}^2\right)\sqrt{\frac{gA2^2}{gA2^2+gB2^2}}\frac{1}{\sqrt{gA2^2+gB2^2}}\left(g_{\rho\mu}g_{\sigma\nu}\right) \quad (1474)$$

$$+ -ig_{B2}\left(-g_{B2}^2+g_{A2}^2\right)\sqrt{\frac{gA2^2}{gA2^2+gB2^2}}\frac{1}{\sqrt{gA2^2+gB2^2}}\left(g_{\rho\nu}g_{\sigma\mu}\right) \quad (1475)$$


---

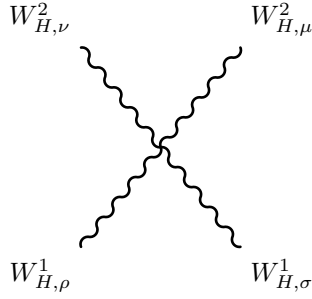

$$-2i\left(g_{A2}^2+g_{B2}^2\right)^{-1}\left(-g_{A2}^2g_{B2}^2+g_{A2}^4+g_{B2}^4\right)\left(g_{\rho\sigma}g_{\mu\nu}\right) \quad (1476)$$

$$+i\left(g_{A2}^2+g_{B2}^2\right)^{-1}\left(-g_{A2}^2g_{B2}^2+g_{A2}^4+g_{B2}^4\right)\left(g_{\rho\mu}g_{\sigma\nu}\right) \quad (1477)$$

$$+i\left(g_{A2}^2+g_{B2}^2\right)^{-1}\left(-g_{A2}^2g_{B2}^2+g_{A2}^4+g_{B2}^4\right)\left(g_{\rho\nu}g_{\sigma\mu}\right) \quad (1478)$$


---

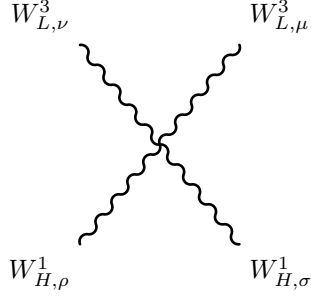

$$-2ig_{A2}^2g_{B2}^2\left(g_{A2}^2+g_{B2}^2\right)^{-1}\left(g_{\rho\sigma}g_{\mu\nu}\right) \quad (1479)$$

$$+ig_{A2}^2g_{B2}^2\left(g_{A2}^2+g_{B2}^2\right)^{-1}\left(g_{\rho\mu}g_{\sigma\nu}\right) \quad (1480)$$

$$+ig_{A2}^2g_{B2}^2\left(g_{A2}^2+g_{B2}^2\right)^{-1}\left(g_{\rho\nu}g_{\sigma\mu}\right) \quad (1481)$$

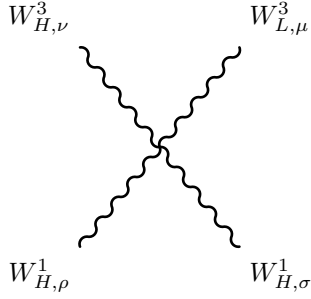

$$2ig_{B2}\left(-g_{B2}^2+g_{A2}^2\right)\sqrt{\frac{gA2^2}{gA2^2+gB2^2}}\frac{1}{\sqrt{gA2^2+gB2^2}}\left(g_{\rho\sigma}g_{\mu\nu}\right) \quad (1482)$$

$$+ -ig_{B2}\left(-g_{B2}^2+g_{A2}^2\right)\sqrt{\frac{gA2^2}{gA2^2+gB2^2}}\frac{1}{\sqrt{gA2^2+gB2^2}}\left(g_{\rho\mu}g_{\sigma\nu}\right) \quad (1483)$$

$$+ -ig_{B2}\left(-g_{B2}^2+g_{A2}^2\right)\sqrt{\frac{gA2^2}{gA2^2+gB2^2}}\frac{1}{\sqrt{gA2^2+gB2^2}}\left(g_{\rho\nu}g_{\sigma\mu}\right) \quad (1484)$$

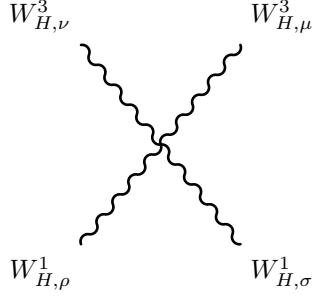

$$- 2i \left( g_{A2}^2 + g_{B2}^2 \right)^{-1} \left( - g_{A2}^2 g_{B2}^2 + g_{A2}^4 + g_{B2}^4 \right) \left( g_{\rho\sigma} g_{\mu\nu} \right) \quad (1485)$$

$$+ i \left( g_{A2}^2 + g_{B2}^2 \right)^{-1} \left( - g_{A2}^2 g_{B2}^2 + g_{A2}^4 + g_{B2}^4 \right) \left( g_{\rho\mu} g_{\sigma\nu} \right) \quad (1486)$$

$$+ i \left( g_{A2}^2 + g_{B2}^2 \right)^{-1} \left( - g_{A2}^2 g_{B2}^2 + g_{A2}^4 + g_{B2}^4 \right) \left( g_{\rho\nu} g_{\sigma\mu} \right) \quad (1487)$$


---

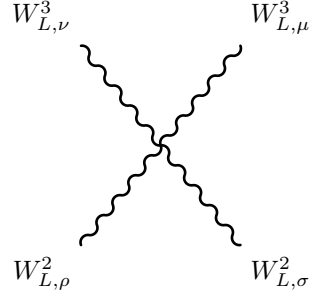

$$- 2i g_{A2}^2 g_{B2}^2 \left( g_{A2}^2 + g_{B2}^2 \right)^{-1} \left( g_{\rho\sigma} g_{\mu\nu} \right) \quad (1488)$$

$$+ i g_{A2}^2 g_{B2}^2 \left( g_{A2}^2 + g_{B2}^2 \right)^{-1} \left( g_{\rho\mu} g_{\sigma\nu} \right) \quad (1489)$$

$$+ i g_{A2}^2 g_{B2}^2 \left( g_{A2}^2 + g_{B2}^2 \right)^{-1} \left( g_{\rho\nu} g_{\sigma\mu} \right) \quad (1490)$$


---

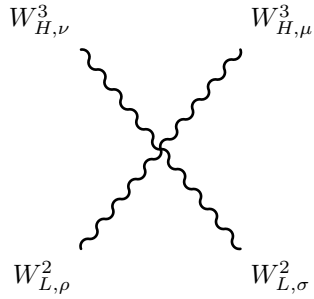

$$- 2ig_{A2}^2 g_{B2}^2 (g_{A2}^2 + g_{B2}^2)^{-1} (g_{\rho\sigma} g_{\mu\nu}) \quad (1491)$$

$$+ ig_{A2}^2 g_{B2}^2 (g_{A2}^2 + g_{B2}^2)^{-1} (g_{\rho\mu} g_{\sigma\nu}) \quad (1492)$$

$$+ ig_{A2}^2 g_{B2}^2 (g_{A2}^2 + g_{B2}^2)^{-1} (g_{\rho\nu} g_{\sigma\mu}) \quad (1493)$$

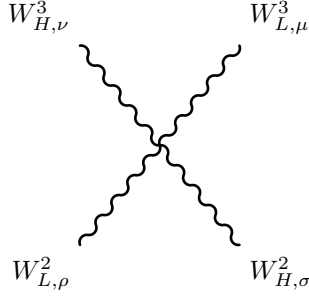

$$- 2ig_{A2}^2 g_{B2}^2 (g_{A2}^2 + g_{B2}^2)^{-1} (g_{\rho\sigma} g_{\mu\nu}) \quad (1494)$$

$$+ ig_{A2}^2 g_{B2}^2 (g_{A2}^2 + g_{B2}^2)^{-1} (g_{\rho\mu} g_{\sigma\nu}) \quad (1495)$$

$$+ ig_{A2}^2 g_{B2}^2 (g_{A2}^2 + g_{B2}^2)^{-1} (g_{\rho\nu} g_{\sigma\mu}) \quad (1496)$$

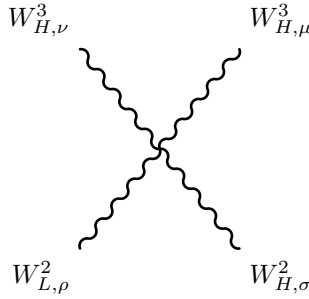

$$2ig_{B2} (-g_{B2}^2 + g_{A2}^2) \sqrt{\frac{gA2^2}{gA2^2 + gB2^2}} \frac{1}{\sqrt{gA2^2 + gB2^2}} (g_{\rho\sigma} g_{\mu\nu}) \quad (1497)$$

$$+ -ig_{B2} (-g_{B2}^2 + g_{A2}^2) \sqrt{\frac{gA2^2}{gA2^2 + gB2^2}} \frac{1}{\sqrt{gA2^2 + gB2^2}} (g_{\rho\mu} g_{\sigma\nu}) \quad (1498)$$

$$+ -ig_{B2} (-g_{B2}^2 + g_{A2}^2) \sqrt{\frac{gA2^2}{gA2^2 + gB2^2}} \frac{1}{\sqrt{gA2^2 + gB2^2}} (g_{\rho\nu} g_{\sigma\mu}) \quad (1499)$$

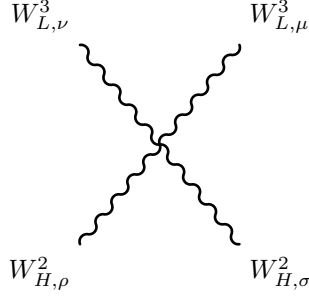

$$-2ig_{A2}^2g_{B2}^2\left(g_{A2}^2+g_{B2}^2\right)^{-1}\left(g_{\rho\sigma}g_{\mu\nu}\right) \quad (1500)$$

$$+ig_{A2}^2g_{B2}^2\left(g_{A2}^2+g_{B2}^2\right)^{-1}\left(g_{\rho\mu}g_{\sigma\nu}\right) \quad (1501)$$

$$+ig_{A2}^2g_{B2}^2\left(g_{A2}^2+g_{B2}^2\right)^{-1}\left(g_{\rho\nu}g_{\sigma\mu}\right) \quad (1502)$$

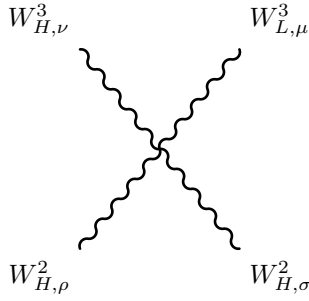

$$2ig_{B2}\left(-g_{B2}^2+g_{A2}^2\right)\sqrt{\frac{gA2^2}{gA2^2+gB2^2}}\frac{1}{\sqrt{gA2^2+gB2^2}}\left(g_{\rho\sigma}g_{\mu\nu}\right) \quad (1503)$$

$$+ -ig_{B2}\left(-g_{B2}^2+g_{A2}^2\right)\sqrt{\frac{gA2^2}{gA2^2+gB2^2}}\frac{1}{\sqrt{gA2^2+gB2^2}}\left(g_{\rho\mu}g_{\sigma\nu}\right) \quad (1504)$$

$$+ -ig_{B2}\left(-g_{B2}^2+g_{A2}^2\right)\sqrt{\frac{gA2^2}{gA2^2+gB2^2}}\frac{1}{\sqrt{gA2^2+gB2^2}}\left(g_{\rho\nu}g_{\sigma\mu}\right) \quad (1505)$$

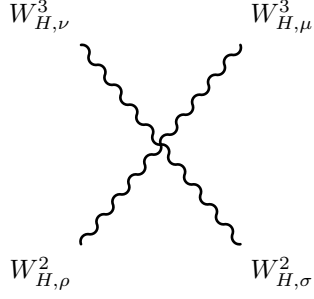

$$- 2i \left( g_{A2}^2 + g_{B2}^2 \right)^{-1} \left( - g_{A2}^2 g_{B2}^2 + g_{A2}^4 + g_{B2}^4 \right) \left( g_{\rho\sigma} g_{\mu\nu} \right) \quad (1506)$$

$$+ i \left( g_{A2}^2 + g_{B2}^2 \right)^{-1} \left( - g_{A2}^2 g_{B2}^2 + g_{A2}^4 + g_{B2}^4 \right) \left( g_{\rho\mu} g_{\sigma\nu} \right) \quad (1507)$$

$$+ i \left( g_{A2}^2 + g_{B2}^2 \right)^{-1} \left( - g_{A2}^2 g_{B2}^2 + g_{A2}^4 + g_{B2}^4 \right) \left( g_{\rho\nu} g_{\sigma\mu} \right) \quad (1508)$$

## 9.10 Two Ghosts-One Vector Boson-Interaction

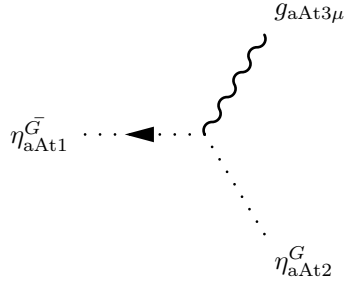

$$g_3 f_{aAt1,aAt2,aAt3} \left( p_\mu^{\eta_{aAt2}^G} \right) \quad (1509)$$

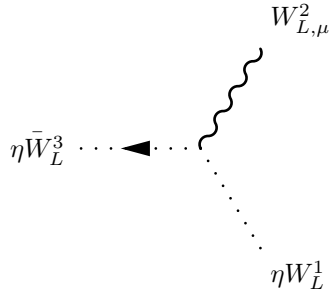



$$g_{A2}g_{B2}\frac{1}{\left(g_{A2}^2+g_{B2}^2\right)^{3/2}}\left(g_{A2}\sqrt{\frac{g_{A2}^2}{g_{A2}^2+g_{B2}^2}}\sqrt{g_{A2}^2+g_{B2}^2}+g_{B2}^2\right)\left(p_\mu^{\eta W_L^1}\right) \quad (1510)$$


---

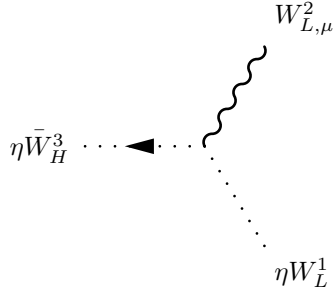

$$-g_{A2}g_{B2}^2\frac{1}{\left(g_{A2}^2+g_{B2}^2\right)^{3/2}}\left(-g_{A2}+\sqrt{\frac{g_{A2}^2}{g_{A2}^2+g_{B2}^2}}\sqrt{g_{A2}^2+g_{B2}^2}\right)\left(p_\mu^{\eta W_L^1}\right) \quad (1511)$$


---

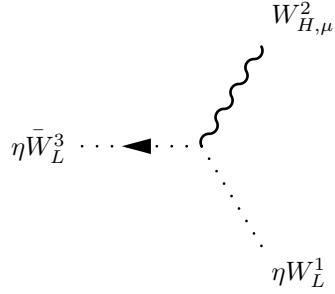

$$-g_{A2}g_{B2}^2\frac{1}{\left(g_{A2}^2+g_{B2}^2\right)^{3/2}}\left(-g_{A2}+\sqrt{\frac{g_{A2}^2}{g_{A2}^2+g_{B2}^2}}\sqrt{g_{A2}^2+g_{B2}^2}\right)\left(p_\mu^{\eta W_L^1}\right) \quad (1512)$$


---

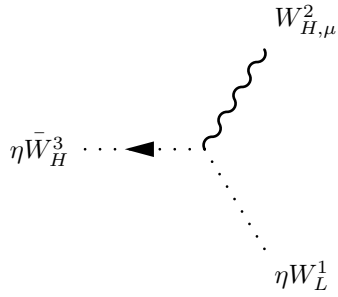

$$\left(g_{A2}^{-2}g_{B2}^3\left(\frac{gA2^2}{gA2^2+gB2^2}\right)^{3/2}+g_{A2}^3g_{B2}\frac{1}{\left(gA2^2+gB2^2\right)^{3/2}}\right)\left(p_\mu^{\eta W_L^1}\right) \quad (1513)$$


---

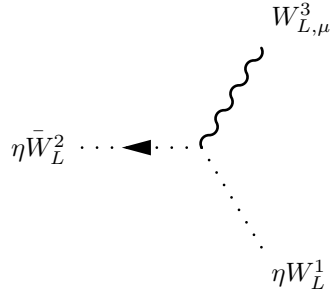

$$-g_{A2}g_{B2}\frac{1}{\left(gA2^2+gB2^2\right)^{3/2}}\left(g_{A2}\sqrt{\frac{gA2^2}{gA2^2+gB2^2}}\sqrt{gA2^2+gB2^2}+g_{B2}^2\right)\left(p_\mu^{\eta W_L^1}\right) \quad (1514)$$


---

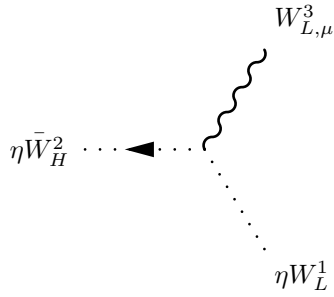

$$g_{A2}g_{B2}^2\frac{1}{\left(gA2^2+gB2^2\right)^{3/2}}\left(-g_{A2}+\sqrt{\frac{gA2^2}{gA2^2+gB2^2}}\sqrt{gA2^2+gB2^2}\right)\left(p_\mu^{\eta W_L^1}\right) \quad (1515)$$


---

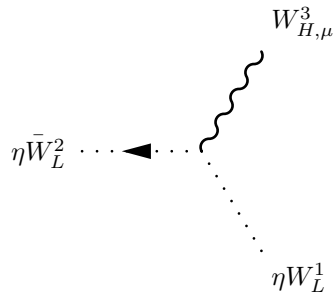

$$g_{A2}g_{B2}^2\frac{1}{\left(g_{A2}^2+g_{B2}^2\right)^{3/2}}\left(-g_{A2}+\sqrt{\frac{g_{A2}^2}{g_{A2}^2+g_{B2}^2}}\sqrt{g_{A2}^2+g_{B2}^2}\right)\left(p_{\mu}^{\eta W_L^1}\right) \quad (1516)$$


---

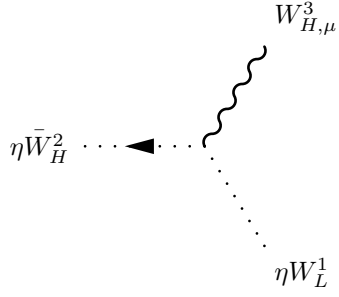

$$-g_{B2}\frac{1}{\left(g_{A2}^2+g_{B2}^2\right)^{3/2}}\left(g_{B2}^2\sqrt{\frac{g_{A2}^2}{g_{A2}^2+g_{B2}^2}}\sqrt{g_{A2}^2+g_{B2}^2}+g_{A2}^3\right)\left(p_{\mu}^{\eta W_L^1}\right) \quad (1517)$$


---

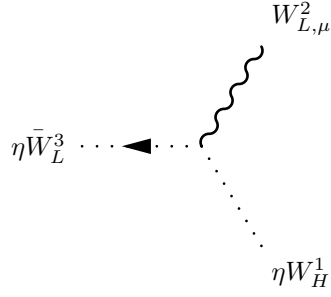

$$-g_{A2}g_{B2}^2\frac{1}{\left(g_{A2}^2+g_{B2}^2\right)^{3/2}}\left(-g_{A2}+\sqrt{\frac{g_{A2}^2}{g_{A2}^2+g_{B2}^2}}\sqrt{g_{A2}^2+g_{B2}^2}\right)\left(p_{\mu}^{\eta W_H^1}\right) \quad (1518)$$


---

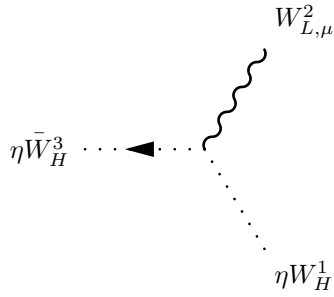

$$\left(g_{A2}^{-2}g_{B2}^3\left(\frac{gA2^2}{gA2^2+gB2^2}\right)^{3/2}+g_{A2}^3g_{B2}\frac{1}{\left(gA2^2+gB2^2\right)^{3/2}}\right)\left(p_\mu^{\eta W_H^1}\right) \quad (1519)$$


---

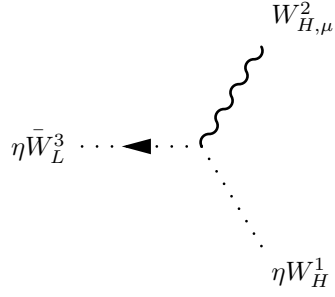

$$\left(g_{A2}^{-2}g_{B2}^3\left(\frac{gA2^2}{gA2^2+gB2^2}\right)^{3/2}+g_{A2}^3g_{B2}\frac{1}{\left(gA2^2+gB2^2\right)^{3/2}}\right)\left(p_\mu^{\eta W_H^1}\right) \quad (1520)$$


---

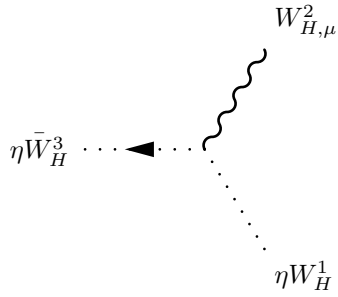

$$\frac{1}{\left(gA2^2+gB2^2\right)^{3/2}}\left(-g_{A2}\left(\frac{gA2^2}{gA2^2+gB2^2}\right)^{3/2}\left(gA2^2+gB2^2\right)^{3/2}+g_{B2}^4\right)\left(p_\mu^{\eta W_H^1}\right) \quad (1521)$$


---

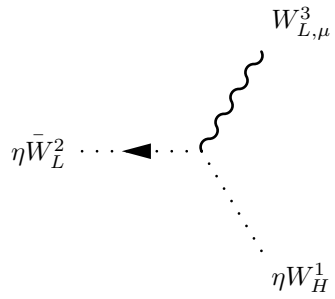

$$g_{A2}g_{B2}^2 \frac{1}{\left(g_{A2}^2 + g_{B2}^2\right)^{3/2}} \left( -g_{A2} + \sqrt{\frac{g_{A2}^2}{g_{A2}^2 + g_{B2}^2}} \sqrt{g_{A2}^2 + g_{B2}^2} \right) \left( p_\mu^{\eta W_H^1} \right) \quad (1522)$$


---

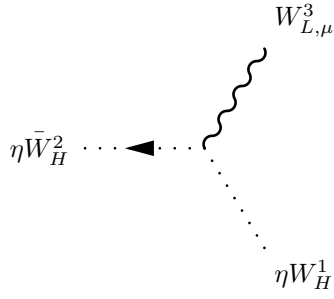

$$-g_{B2} \frac{1}{\left(g_{A2}^2 + g_{B2}^2\right)^{3/2}} \left( g_{B2}^2 \sqrt{\frac{g_{A2}^2}{g_{A2}^2 + g_{B2}^2}} \sqrt{g_{A2}^2 + g_{B2}^2} + g_{A2}^3 \right) \left( p_\mu^{\eta W_H^1} \right) \quad (1523)$$


---

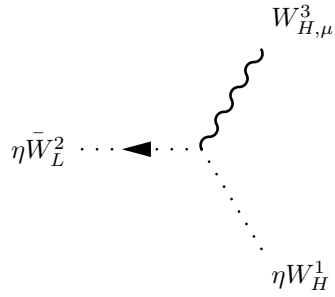

$$-g_{B2} \frac{1}{\left(g_{A2}^2 + g_{B2}^2\right)^{3/2}} \left( g_{B2}^2 \sqrt{\frac{g_{A2}^2}{g_{A2}^2 + g_{B2}^2}} \sqrt{g_{A2}^2 + g_{B2}^2} + g_{A2}^3 \right) \left( p_\mu^{\eta W_H^1} \right) \quad (1524)$$


---

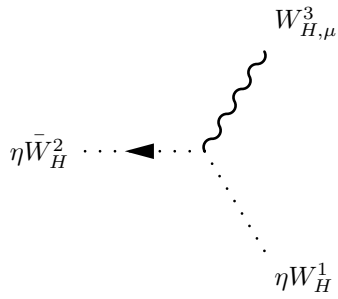

$$\left(g_{A2} \left(\frac{gA2^2}{gA2^2 + gB2^2}\right)^{3/2} - g_{B2}^4 \frac{1}{\left(gA2^2 + gB2^2\right)^{3/2}}\right) \left(p_\mu^{\eta W_H^1}\right) \quad (1525)$$


---

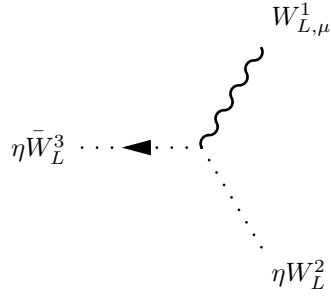

$$- g_{A2} g_{B2} \frac{1}{\left(gA2^2 + gB2^2\right)^{3/2}} \left(g_{A2} \sqrt{\frac{gA2^2}{gA2^2 + gB2^2}} \sqrt{gA2^2 + gB2^2} + g_{B2}^2\right) \left(p_\mu^{\eta W_L^2}\right) \quad (1526)$$


---

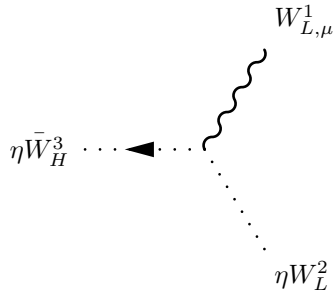

$$g_{A2} g_{B2}^2 \frac{1}{\left(gA2^2 + gB2^2\right)^{3/2}} \left(-g_{A2} + \sqrt{\frac{gA2^2}{gA2^2 + gB2^2}} \sqrt{gA2^2 + gB2^2}\right) \left(p_\mu^{\eta W_L^2}\right) \quad (1527)$$


---

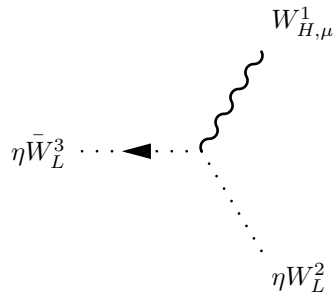

$$g_{A2}g_{B2}^2 \frac{1}{\left(g_{A2}^2 + g_{B2}^2\right)^{3/2}} \left( -g_{A2} + \sqrt{\frac{g_{A2}^2}{g_{A2}^2 + g_{B2}^2}} \sqrt{g_{A2}^2 + g_{B2}^2} \right) \left( p_\mu^{\eta W_L^2} \right) \quad (1528)$$


---

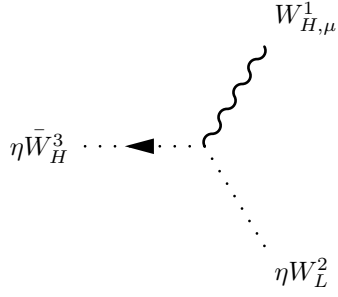

$$-g_{B2} \frac{1}{\left(g_{A2}^2 + g_{B2}^2\right)^{3/2}} \left( g_{B2}^2 \sqrt{\frac{g_{A2}^2}{g_{A2}^2 + g_{B2}^2}} \sqrt{g_{A2}^2 + g_{B2}^2} + g_{A2}^3 \right) \left( p_\mu^{\eta W_L^2} \right) \quad (1529)$$


---

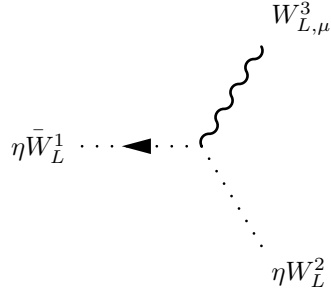

$$g_{A2}g_{B2} \frac{1}{\left(g_{A2}^2 + g_{B2}^2\right)^{3/2}} \left( g_{A2} \sqrt{\frac{g_{A2}^2}{g_{A2}^2 + g_{B2}^2}} \sqrt{g_{A2}^2 + g_{B2}^2} + g_{B2}^2 \right) \left( p_\mu^{\eta W_L^2} \right) \quad (1530)$$


---

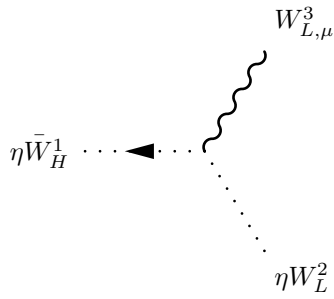

$$-g_{A2}g_{B2}^2\frac{1}{\left(gA2^2+gB2^2\right)^{3/2}}\left(-g_{A2}+\sqrt{\frac{gA2^2}{gA2^2+gB2^2}}\sqrt{gA2^2+gB2^2}\right)\left(p_\mu^{\eta W_L^2}\right) \quad (1531)$$


---

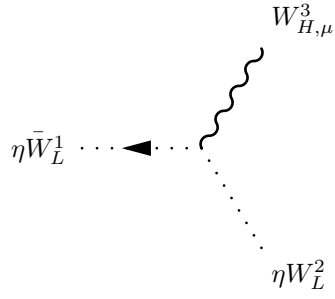

$$-g_{A2}g_{B2}^2\frac{1}{\left(gA2^2+gB2^2\right)^{3/2}}\left(-g_{A2}+\sqrt{\frac{gA2^2}{gA2^2+gB2^2}}\sqrt{gA2^2+gB2^2}\right)\left(p_\mu^{\eta W_L^2}\right) \quad (1532)$$


---

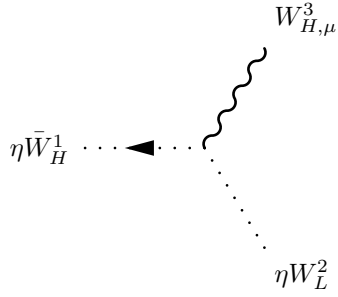

$$\left(g_{A2}^{-2}g_{B2}^3\left(\frac{gA2^2}{gA2^2+gB2^2}\right)^{3/2}+g_{A2}^3g_{B2}\frac{1}{\left(gA2^2+gB2^2\right)^{3/2}}\right)\left(p_\mu^{\eta W_L^2}\right) \quad (1533)$$


---

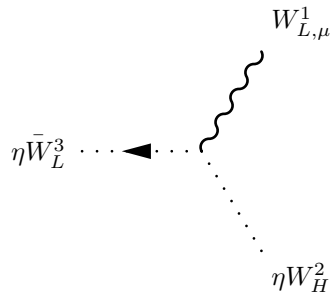



$$g_{A2}g_{B2}^2 \frac{1}{\left(g_{A2}^2 + g_{B2}^2\right)^{3/2}} \left( -g_{A2} + \sqrt{\frac{g_{A2}^2}{g_{A2}^2 + g_{B2}^2}} \sqrt{g_{A2}^2 + g_{B2}^2} \right) \left( p_\mu^{\eta W_H^2} \right) \quad (1534)$$


---

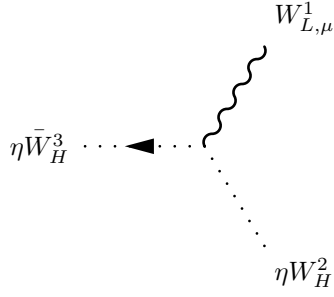

$$-g_{B2} \frac{1}{\left(g_{A2}^2 + g_{B2}^2\right)^{3/2}} \left( g_{B2}^2 \sqrt{\frac{g_{A2}^2}{g_{A2}^2 + g_{B2}^2}} \sqrt{g_{A2}^2 + g_{B2}^2} + g_{A2}^3 \right) \left( p_\mu^{\eta W_H^2} \right) \quad (1535)$$


---

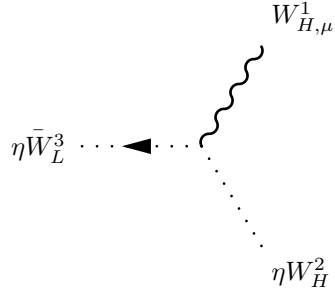

$$-g_{B2} \frac{1}{\left(g_{A2}^2 + g_{B2}^2\right)^{3/2}} \left( g_{B2}^2 \sqrt{\frac{g_{A2}^2}{g_{A2}^2 + g_{B2}^2}} \sqrt{g_{A2}^2 + g_{B2}^2} + g_{A2}^3 \right) \left( p_\mu^{\eta W_H^2} \right) \quad (1536)$$


---

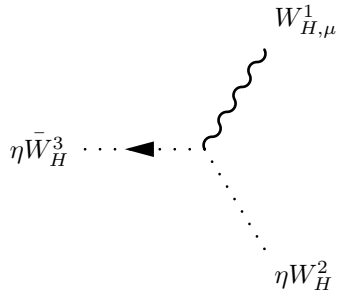

$$\left(g_{A2} \left(\frac{gA2^2}{gA2^2 + gB2^2}\right)^{3/2} - g_{B2}^4 \frac{1}{\left(gA2^2 + gB2^2\right)^{3/2}}\right) \left(p_\mu^{\eta W_H^2}\right) \quad (1537)$$


---

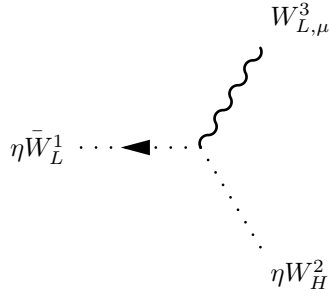

$$-g_{A2} g_{B2}^2 \frac{1}{\left(gA2^2 + gB2^2\right)^{3/2}} \left(-g_{A2} + \sqrt{\frac{gA2^2}{gA2^2 + gB2^2}} \sqrt{gA2^2 + gB2^2}\right) \left(p_\mu^{\eta W_H^2}\right) \quad (1538)$$


---

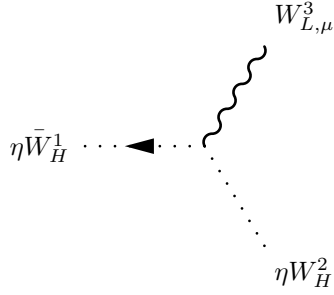

$$\left(g_{A2}^{-2} g_{B2}^3 \left(\frac{gA2^2}{gA2^2 + gB2^2}\right)^{3/2} + g_{A2}^3 g_{B2} \frac{1}{\left(gA2^2 + gB2^2\right)^{3/2}}\right) \left(p_\mu^{\eta W_H^2}\right) \quad (1539)$$


---

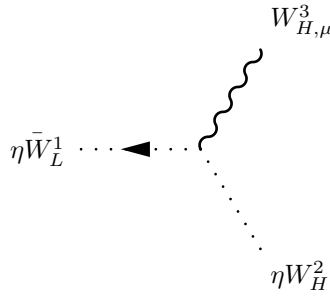

$$\left(g_{A2}^{-2}g_{B2}^3\left(\frac{gA2^2}{gA2^2+gB2^2}\right)^{3/2}+g_{A2}^3g_{B2}\frac{1}{\left(gA2^2+gB2^2\right)^{3/2}}\right)\left(p_\mu^{\eta W_H^2}\right) \quad (1540)$$


---

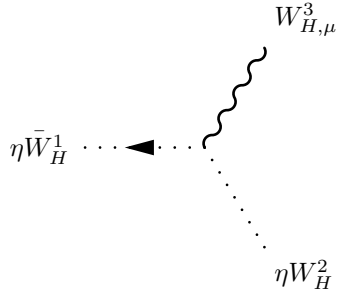

$$\frac{1}{\left(gA2^2+gB2^2\right)^{3/2}}\left(-g_{A2}\left(\frac{gA2^2}{gA2^2+gB2^2}\right)^{3/2}\left(gA2^2+gB2^2\right)^{3/2}+g_{B2}^4\right)\left(p_\mu^{\eta W_H^2}\right) \quad (1541)$$


---

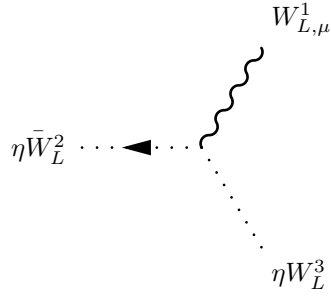

$$g_{A2}g_{B2}\frac{1}{\left(gA2^2+gB2^2\right)^{3/2}}\left(g_{A2}\sqrt{\frac{gA2^2}{gA2^2+gB2^2}}\sqrt{gA2^2+gB2^2}+g_{B2}^2\right)\left(p_\mu^{\eta W_L^3}\right) \quad (1542)$$


---

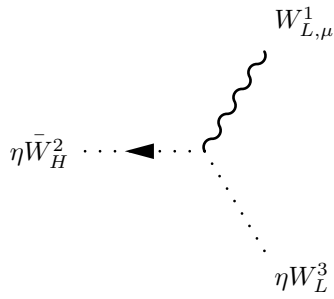

$$-g_{A2}g_{B2}^2\frac{1}{\left(gA2^2+gB2^2\right)^{3/2}}\left(-g_{A2}+\sqrt{\frac{gA2^2}{gA2^2+gB2^2}}\sqrt{gA2^2+gB2^2}\right)\left(p_\mu^{\eta W_L^3}\right) \quad (1543)$$


---

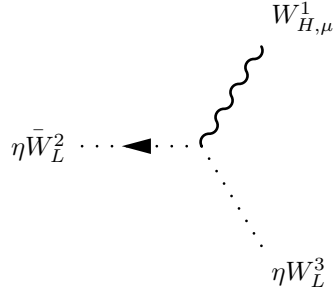

$$-g_{A2}g_{B2}^2\frac{1}{\left(gA2^2+gB2^2\right)^{3/2}}\left(-g_{A2}+\sqrt{\frac{gA2^2}{gA2^2+gB2^2}}\sqrt{gA2^2+gB2^2}\right)\left(p_\mu^{\eta W_L^3}\right) \quad (1544)$$


---

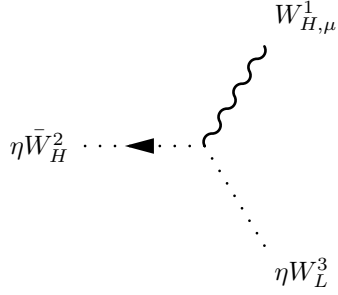

$$\left(g_{A2}^{-2}g_{B2}^3\left(\frac{gA2^2}{gA2^2+gB2^2}\right)^{3/2}+g_{A2}^3g_{B2}\frac{1}{\left(gA2^2+gB2^2\right)^{3/2}}\right)\left(p_\mu^{\eta W_L^3}\right) \quad (1545)$$


---

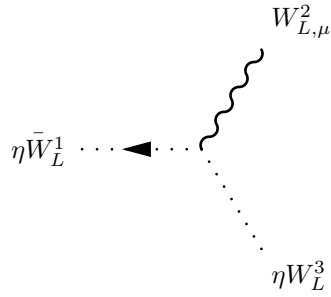

$$-g_{A2}g_{B2}\frac{1}{\left(g_{A2}^2+g_{B2}^2\right)^{3/2}}\left(g_{A2}\sqrt{\frac{g_{A2}^2}{g_{A2}^2+g_{B2}^2}}\sqrt{g_{A2}^2+g_{B2}^2}+g_{B2}^2\right)\left(p_\mu^{\eta W_L^3}\right) \quad (1546)$$


---

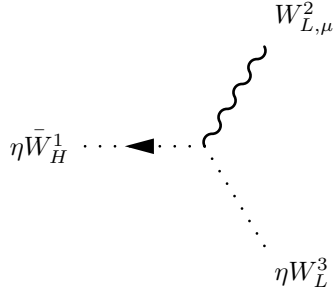

$$g_{A2}g_{B2}^2\frac{1}{\left(g_{A2}^2+g_{B2}^2\right)^{3/2}}\left(-g_{A2}+\sqrt{\frac{g_{A2}^2}{g_{A2}^2+g_{B2}^2}}\sqrt{g_{A2}^2+g_{B2}^2}\right)\left(p_\mu^{\eta W_L^3}\right) \quad (1547)$$


---

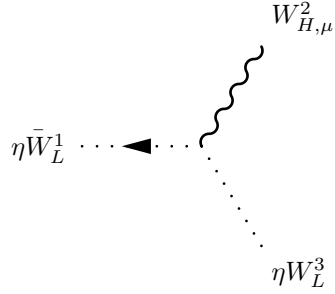

$$g_{A2}g_{B2}^2\frac{1}{\left(g_{A2}^2+g_{B2}^2\right)^{3/2}}\left(-g_{A2}+\sqrt{\frac{g_{A2}^2}{g_{A2}^2+g_{B2}^2}}\sqrt{g_{A2}^2+g_{B2}^2}\right)\left(p_\mu^{\eta W_L^3}\right) \quad (1548)$$


---

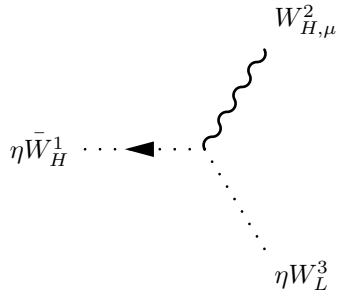

$$-g_{B2} \frac{1}{\left(g_{A2}^2 + g_{B2}^2\right)^{3/2}} \left(g_{B2}^2 \sqrt{\frac{g_{A2}^2}{g_{A2}^2 + g_{B2}^2}} \sqrt{g_{A2}^2 + g_{B2}^2} + g_{A2}^3\right) \left(p_\mu^{\eta W_L^3}\right) \quad (1549)$$


---

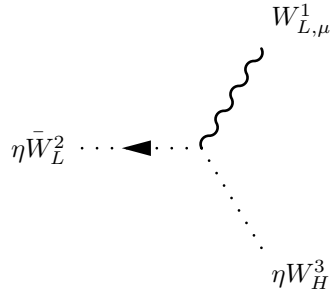

$$-g_{A2} g_{B2}^2 \frac{1}{\left(g_{A2}^2 + g_{B2}^2\right)^{3/2}} \left(-g_{A2} + \sqrt{\frac{g_{A2}^2}{g_{A2}^2 + g_{B2}^2}} \sqrt{g_{A2}^2 + g_{B2}^2}\right) \left(p_\mu^{\eta W_H^3}\right) \quad (1550)$$


---

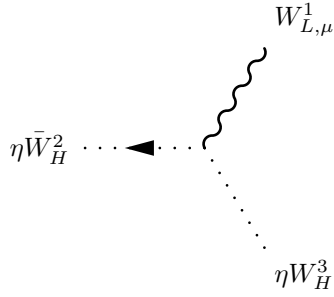

$$\left(g_{A2}^{-2} g_{B2}^3 \left(\frac{g_{A2}^2}{g_{A2}^2 + g_{B2}^2}\right)^{3/2} + g_{A2}^3 g_{B2} \frac{1}{\left(g_{A2}^2 + g_{B2}^2\right)^{3/2}}\right) \left(p_\mu^{\eta W_H^3}\right) \quad (1551)$$


---

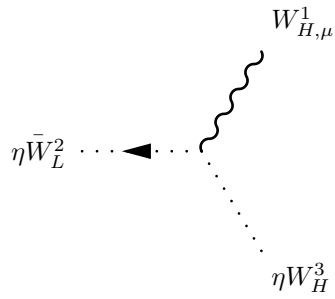

$$\left(g_{A2}^{-2}g_{B2}^3\left(\frac{gA2^2}{gA2^2+gB2^2}\right)^{3/2}+g_{A2}^3g_{B2}\frac{1}{\left(gA2^2+gB2^2\right)^{3/2}}\right)\left(p_\mu^{\eta W_H^3}\right) \quad (1552)$$


---

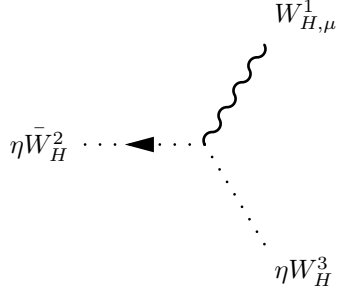

$$\frac{1}{\left(gA2^2+gB2^2\right)^{3/2}}\left(-g_{A2}\left(\frac{gA2^2}{gA2^2+gB2^2}\right)^{3/2}\left(gA2^2+gB2^2\right)^{3/2}+g_{B2}^4\right)\left(p_\mu^{\eta W_H^3}\right) \quad (1553)$$


---

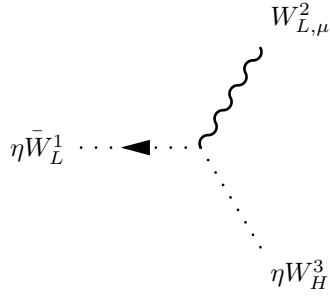

$$g_{A2}g_{B2}^2\frac{1}{\left(gA2^2+gB2^2\right)^{3/2}}\left(-g_{A2}+\sqrt{\frac{gA2^2}{gA2^2+gB2^2}}\sqrt{gA2^2+gB2^2}\right)\left(p_\mu^{\eta W_H^3}\right) \quad (1554)$$


---

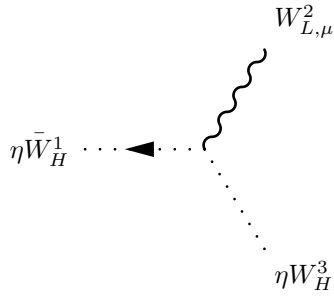

$$-g_{B2} \frac{1}{\left(g_{A2}^2 + g_{B2}^2\right)^{3/2}} \left(g_{B2}^2 \sqrt{\frac{g_{A2}^2}{g_{A2}^2 + g_{B2}^2}} \sqrt{g_{A2}^2 + g_{B2}^2} + g_{A2}^3\right) \left(p_\mu^{\eta W_H^3}\right) \quad (1555)$$


---

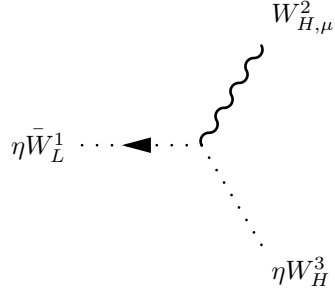

$$-g_{B2} \frac{1}{\left(g_{A2}^2 + g_{B2}^2\right)^{3/2}} \left(g_{B2}^2 \sqrt{\frac{g_{A2}^2}{g_{A2}^2 + g_{B2}^2}} \sqrt{g_{A2}^2 + g_{B2}^2} + g_{A2}^3\right) \left(p_\mu^{\eta W_H^3}\right) \quad (1556)$$


---

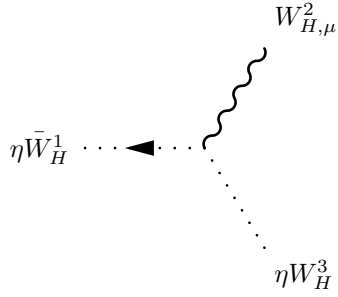

$$\left(g_{A2} \left(\frac{g_{A2}^2}{g_{A2}^2 + g_{B2}^2}\right)^{3/2} - g_{B2}^4 \frac{1}{\left(g_{A2}^2 + g_{B2}^2\right)^{3/2}}\right) \left(p_\mu^{\eta W_H^3}\right) \quad (1557)$$


---

## 9.11 Two Ghosts-One Scalar-Interaction

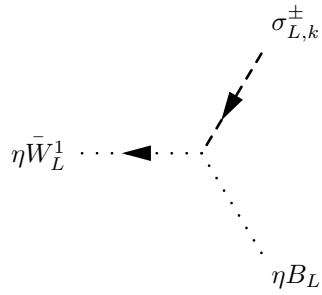



$$\frac{i}{4}g_{B1}\frac{1}{\sqrt{gA1^2+gB1^2}}\Big(-g_{A1}+\sqrt{\frac{gA1^2}{gA1^2+gB1^2}}\sqrt{gA1^2+gB1^2}\Big)g_{B2}\frac{1}{\sqrt{gA2^2+gB2^2}}\Big(-g_{A2}+\sqrt{\frac{gA2^2}{gA2^2+gB2^2}}\sqrt{gA2^2+gB2^2}\Big)v_{Lv}\Big(2$$

(1558)

---

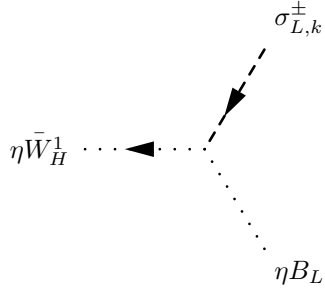

$$\frac{i}{4}g_{B1}\frac{1}{\sqrt{gA1^2+gB1^2}}\Big(-g_{A1}+\sqrt{\frac{gA1^2}{gA1^2+gB1^2}}\sqrt{gA1^2+gB1^2}\Big)\frac{1}{\sqrt{gA2^2+gB2^2}}\Big(g_{A2}\sqrt{\frac{gA2^2}{gA2^2+gB2^2}}\sqrt{gA2^2+gB2^2}+g_{B2}^2\Big)v_{Lv}\Big(Z_{Ls}^{od}$$

(1559)

---

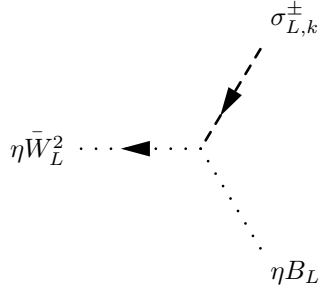

$$-\frac{1}{4}g_{B1}\frac{1}{\sqrt{gA1^2+gB1^2}}\Big(-g_{A1}+\sqrt{\frac{gA1^2}{gA1^2+gB1^2}}\sqrt{gA1^2+gB1^2}\Big)g_{B2}\frac{1}{\sqrt{gA2^2+gB2^2}}\Big(-g_{A2}+\sqrt{\frac{gA2^2}{gA2^2+gB2^2}}\sqrt{gA2^2+gB2^2}\Big)v_{Lv}$$

(1560)

---

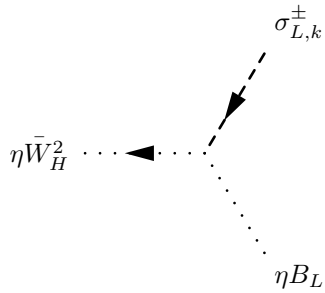

$$-\frac{1}{4}g_{B1}\frac{1}{\sqrt{g_{A1}^2+g_{B1}^2}}\left(-g_{A1}+\sqrt{\frac{g_{A1}^2}{g_{A1}^2+g_{B1}^2}}\sqrt{g_{A1}^2+g_{B1}^2}\right)\frac{1}{\sqrt{g_{A2}^2+g_{B2}^2}}\left(g_{A2}\sqrt{\frac{g_{A2}^2}{g_{A2}^2+g_{B2}^2}}\sqrt{g_{A2}^2+g_{B2}^2}+g_{B2}^2\right)v_{Lv}\left(2\right. \\ \left.(1561)\right.$$


---

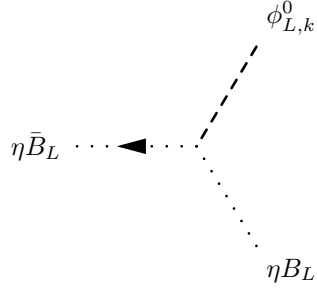

$$2ig_{A1}g_{B1}^2\frac{1}{\left(g_{A1}^2+g_{B1}^2\right)^{3/2}}\left(g_{A1}^2\sqrt{\frac{g_{A1}^2}{g_{A1}^2+g_{B1}^2}}-g_{A1}\sqrt{g_{A1}^2+g_{B1}^2}+g_{B1}^2\sqrt{\frac{g_{A1}^2}{g_{A1}^2+g_{B1}^2}}\right)v_{Lv}\left(Z_{Ls,k1}^{DR,*}+Z_{Ls,k2}^{DR,*}+Z_{Ls,k3}^{DR,*}+Z_{Ls,k4}^{DR,*}\right) \\ \left.(1562)\right.$$


---

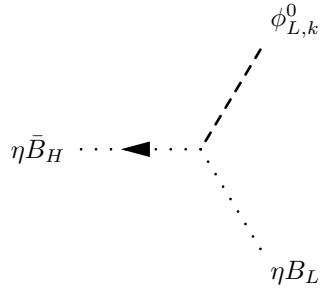

$$-ig_{B1}\left(-g_{A1}^2+g_{B1}^2\right)\frac{1}{\left(g_{A1}^2+g_{B1}^2\right)^{3/2}}\left(g_{A1}^2\sqrt{\frac{g_{A1}^2}{g_{A1}^2+g_{B1}^2}}-g_{A1}\sqrt{g_{A1}^2+g_{B1}^2}+g_{B1}^2\sqrt{\frac{g_{A1}^2}{g_{A1}^2+g_{B1}^2}}\right)v_{Lv}\left(Z_{Ls,k1}^{DR,*}+Z_{Ls,k2}^{DR,*}+Z_{Ls,k3}^{DR,*}+Z_{Ls,k4}^{DR,*}\right) \\ \left.(1563)\right.$$


---

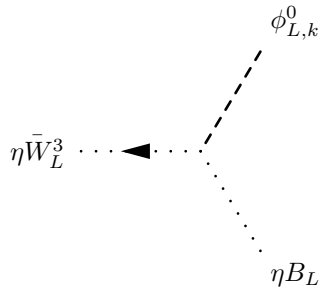

$$ig_{B1}\frac{1}{\sqrt{gA1^2+gB1^2}}\Big(-g_{A1}+\sqrt{\frac{gA1^2}{gA1^2+gB1^2}}\sqrt{gA1^2+gB1^2}\Big)g_{B2}\frac{1}{\sqrt{gA2^2+gB2^2}}\Big(-g_{A2}+\sqrt{\frac{gA2^2}{gA2^2+gB2^2}}\sqrt{gA2^2+gB2^2}\Big)v_{Lv}\Big(-Z$$

(1564)

---

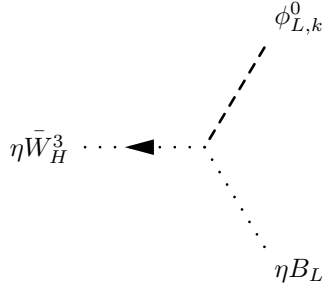

$$ig_{B1}\frac{1}{\sqrt{gA1^2+gB1^2}}\Big(-g_{A1}+\sqrt{\frac{gA1^2}{gA1^2+gB1^2}}\sqrt{gA1^2+gB1^2}\Big)\frac{1}{\sqrt{gA2^2+gB2^2}}\Big(g_{A2}\sqrt{\frac{gA2^2}{gA2^2+gB2^2}}\sqrt{gA2^2+gB2^2}+g_{B2}^2\Big)v_{Lv}\Big(-Z$$

(1565)

---

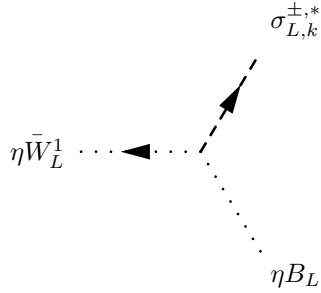

$$\frac{i}{4}g_{B1}\frac{1}{\sqrt{gA1^2+gB1^2}}\Big(-g_{A1}+\sqrt{\frac{gA1^2}{gA1^2+gB1^2}}\sqrt{gA1^2+gB1^2}\Big)g_{B2}\frac{1}{\sqrt{gA2^2+gB2^2}}\Big(-g_{A2}+\sqrt{\frac{gA2^2}{gA2^2+gB2^2}}\sqrt{gA2^2+gB2^2}\Big)v_{Lv}\xi_W$$

(1566)

---

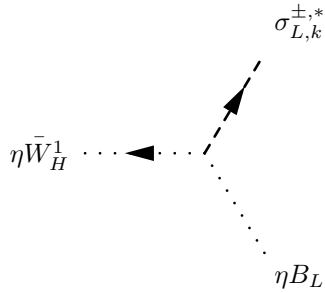

$$\frac{i}{4}g_{B1}\frac{1}{\sqrt{gA1^2+gB1^2}}\left(-g_{A1}+\sqrt{\frac{gA1^2}{gA1^2+gB1^2}}\sqrt{gA1^2+gB1^2}\right)\frac{1}{\sqrt{gA2^2+gB2^2}}\left(g_{A2}\sqrt{\frac{gA2^2}{gA2^2+gB2^2}}\sqrt{gA2^2+gB2^2}+g_{B2}^2\right)v_Lv\xi_{W_H^1} \quad (1567)$$


---

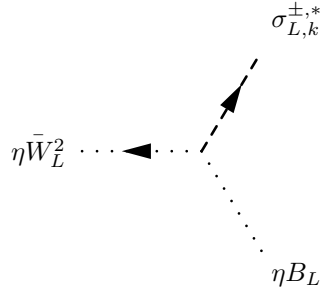

$$\frac{1}{4}g_{B1}\frac{1}{\sqrt{gA1^2+gB1^2}}\left(-g_{A1}+\sqrt{\frac{gA1^2}{gA1^2+gB1^2}}\sqrt{gA1^2+gB1^2}\right)g_{B2}\frac{1}{\sqrt{gA2^2+gB2^2}}\left(-g_{A2}+\sqrt{\frac{gA2^2}{gA2^2+gB2^2}}\sqrt{gA2^2+gB2^2}\right)v_Lv\xi_{W_H^1} \quad (1568)$$


---

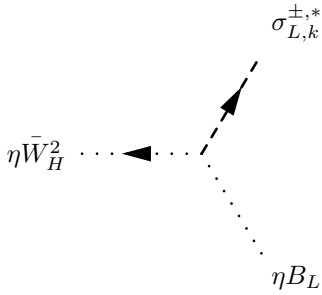

$$\frac{1}{4}g_{B1}\frac{1}{\sqrt{gA1^2+gB1^2}}\left(-g_{A1}+\sqrt{\frac{gA1^2}{gA1^2+gB1^2}}\sqrt{gA1^2+gB1^2}\right)\frac{1}{\sqrt{gA2^2+gB2^2}}\left(g_{A2}\sqrt{\frac{gA2^2}{gA2^2+gB2^2}}\sqrt{gA2^2+gB2^2}+g_{B2}^2\right)v_Lv\xi_{W_H^2} \quad (1569)$$


---

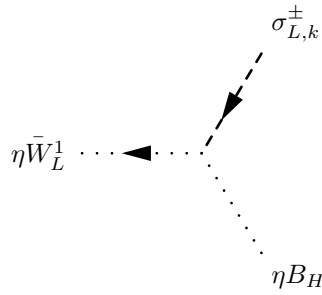

$$\frac{i}{4} \frac{1}{\sqrt{gA1^2 + gB1^2}} \left( g_{A1} \sqrt{\frac{gA1^2}{gA1^2 + gB1^2}} \sqrt{gA1^2 + gB1^2} + g_{B1}^2 \right) g_{B2} \frac{1}{\sqrt{gA2^2 + gB2^2}} \left( -g_{A2} + \sqrt{\frac{gA2^2}{gA2^2 + gB2^2}} \sqrt{gA2^2 + gB2^2} \right) v_{Lv} \left( Z_{Lv}^{od} \right) \quad (1570)$$


---

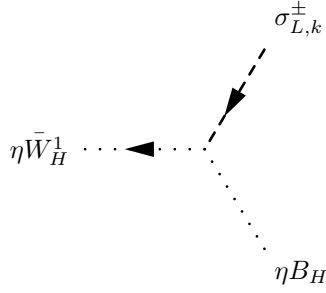

$$\frac{i}{4} \frac{1}{\sqrt{gA1^2 + gB1^2}} \left( g_{A1} \sqrt{\frac{gA1^2}{gA1^2 + gB1^2}} \sqrt{gA1^2 + gB1^2} + g_{B1}^2 \right) \frac{1}{\sqrt{gA2^2 + gB2^2}} \left( g_{A2} \sqrt{\frac{gA2^2}{gA2^2 + gB2^2}} \sqrt{gA2^2 + gB2^2} + g_{B2}^2 \right) v_{Lv} \left( Z_{Lv}^{od,*} \right) \quad (1571)$$


---

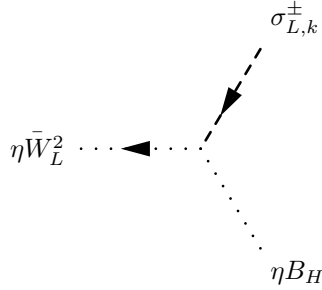

$$-\frac{1}{4} \frac{1}{\sqrt{gA1^2 + gB1^2}} \left( g_{A1} \sqrt{\frac{gA1^2}{gA1^2 + gB1^2}} \sqrt{gA1^2 + gB1^2} + g_{B1}^2 \right) g_{B2} \frac{1}{\sqrt{gA2^2 + gB2^2}} \left( -g_{A2} + \sqrt{\frac{gA2^2}{gA2^2 + gB2^2}} \sqrt{gA2^2 + gB2^2} \right) v_{Lv} \left( Z_{Lv}^{od,*} \right) \quad (1572)$$


---

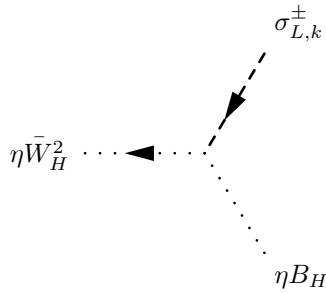

$$-\frac{1}{4}\frac{1}{\sqrt{gA1^2+gB1^2}}\left(g_{A1}\sqrt{\frac{gA1^2}{gA1^2+gB1^2}}\sqrt{gA1^2+gB1^2}+g_{B1}^2\right)\frac{1}{\sqrt{gA2^2+gB2^2}}\left(g_{A2}\sqrt{\frac{gA2^2}{gA2^2+gB2^2}}\sqrt{gA2^2+gB2^2}+g_{B2}^2\right)v_{Lv}\left(Z_{Ls}^{od}\right. \\ (1573)$$


---

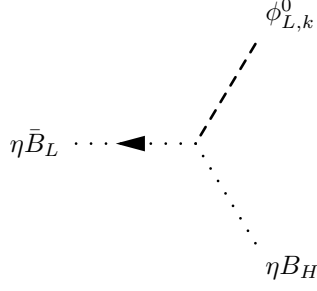

$$-ig_{B1}\left(-g_{A1}^2+g_{B1}^2\right)\frac{1}{\left(gA1^2+gB1^2\right)^{3/2}}\left(g_{A1}^2\sqrt{\frac{gA1^2}{gA1^2+gB1^2}}-g_{A1}\sqrt{gA1^2+gB1^2}+g_{B1}^2\sqrt{\frac{gA1^2}{gA1^2+gB1^2}}\right)v_{Lv}\left(Z_{Ls,k1}^{DR,*}+Z_{Ls,k2}^{DR,*}+\right. \\ (1574)$$


---

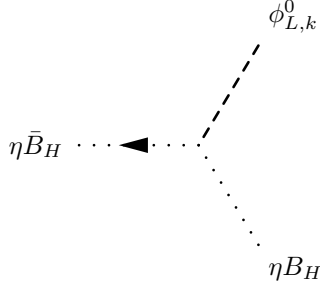

$$-i\frac{1}{\left(gA1^2+gB1^2\right)^{3/2}}\left(2g_{A1}^3g_{B1}^2\sqrt{\frac{gA1^2}{gA1^2+gB1^2}}+2g_{A1}g_{B1}^4\sqrt{\frac{gA1^2}{gA1^2+gB1^2}}+g_{A1}^4\sqrt{gA1^2+gB1^2}\right. \\ \left.+g_{B1}^4\sqrt{gA1^2+gB1^2}\right)v_{Lv}\left(Z_{Ls,k1}^{DR,*}+Z_{Ls,k2}^{DR,*}+Z_{Ls,k3}^{DR,*}+Z_{Ls,k4}^{DR,*}\right)\xi_{B_H} \\ (1575)$$


---

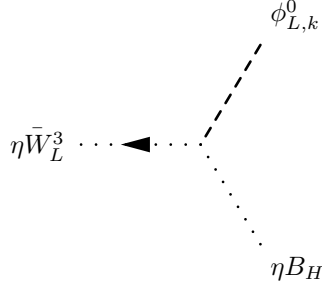

$$i \frac{1}{\sqrt{gA1^2 + gB1^2}} \left( g_{A1} \sqrt{\frac{gA1^2}{gA1^2 + gB1^2}} \sqrt{gA1^2 + gB1^2 + g_{B1}^2} \right) g_{B2} \frac{1}{\sqrt{gA2^2 + gB2^2}} \left( -g_{A2} + \sqrt{\frac{gA2^2}{gA2^2 + gB2^2}} \sqrt{gA2^2 + gB2^2} \right) v_{Lv} \left( -Z_{Ls,} \right) \quad (1576)$$


---

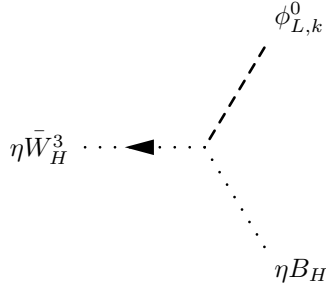

$$i \frac{1}{\sqrt{gA1^2 + gB1^2}} \left( g_{A1} \sqrt{\frac{gA1^2}{gA1^2 + gB1^2}} \sqrt{gA1^2 + gB1^2 + g_{B1}^2} \right) \frac{1}{\sqrt{gA2^2 + gB2^2}} \left( g_{A2} \sqrt{\frac{gA2^2}{gA2^2 + gB2^2}} \sqrt{gA2^2 + gB2^2 + g_{B2}^2} \right) v_{Lv} \left( -Z_{Ls,}^{DR} \right) \quad (1577)$$


---

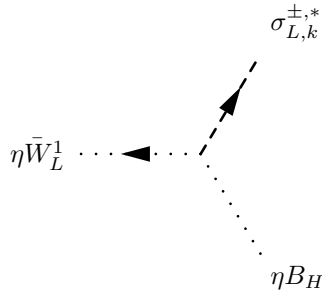

$$\frac{i}{4} \frac{1}{\sqrt{gA1^2 + gB1^2}} \left( g_{A1} \sqrt{\frac{gA1^2}{gA1^2 + gB1^2}} \sqrt{gA1^2 + gB1^2 + g_{B1}^2} \right) g_{B2} \frac{1}{\sqrt{gA2^2 + gB2^2}} \left( -g_{A2} + \sqrt{\frac{gA2^2}{gA2^2 + gB2^2}} \sqrt{gA2^2 + gB2^2} \right) v_{Lv} \xi_{W_L^1} \left( \right) \quad (1578)$$


---

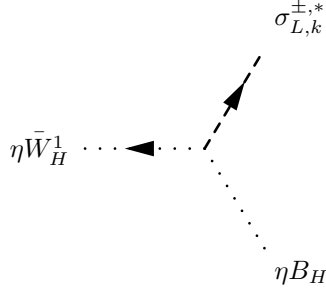

$$\frac{i}{4} \frac{1}{\sqrt{gA_1^2 + gB_1^2}} \left( g_{A1} \sqrt{\frac{gA_1^2}{gA_1^2 + gB_1^2}} \sqrt{gA_1^2 + gB_1^2 + g_{B1}^2} \right) \frac{1}{\sqrt{gA_2^2 + gB_2^2}} \left( g_{A2} \sqrt{\frac{gA_2^2}{gA_2^2 + gB_2^2}} \sqrt{gA_2^2 + gB_2^2 + g_{B2}^2} \right) v_{Lv} \xi_{W_H^1} \left( Z_L \right) \quad (1579)$$


---

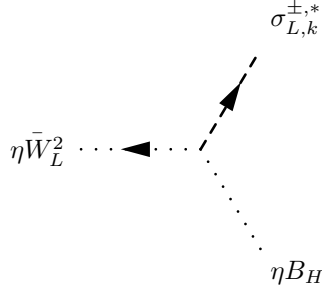

$$\frac{1}{4} \frac{1}{\sqrt{gA_1^2 + gB_1^2}} \left( g_{A1} \sqrt{\frac{gA_1^2}{gA_1^2 + gB_1^2}} \sqrt{gA_1^2 + gB_1^2 + g_{B1}^2} \right) g_{B2} \frac{1}{\sqrt{gA_2^2 + gB_2^2}} \left( -g_{A2} + \sqrt{\frac{gA_2^2}{gA_2^2 + gB_2^2}} \sqrt{gA_2^2 + gB_2^2} \right) v_{Lv} \xi_{W_L^2} \left( Z_L \right) \quad (1580)$$


---

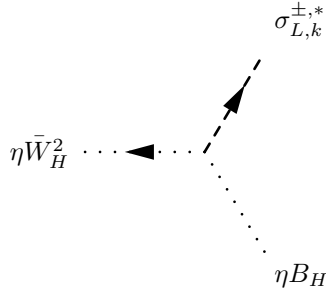

$$\frac{1}{4} \frac{1}{\sqrt{gA_1^2 + gB_1^2}} \left( g_{A1} \sqrt{\frac{gA_1^2}{gA_1^2 + gB_1^2}} \sqrt{gA_1^2 + gB_1^2 + g_{B1}^2} \right) \frac{1}{\sqrt{gA_2^2 + gB_2^2}} \left( g_{A2} \sqrt{\frac{gA_2^2}{gA_2^2 + gB_2^2}} \sqrt{gA_2^2 + gB_2^2 + g_{B2}^2} \right) v_{Lv} \xi_{W_H^2} \left( Z_L \right) \quad (1581)$$


---



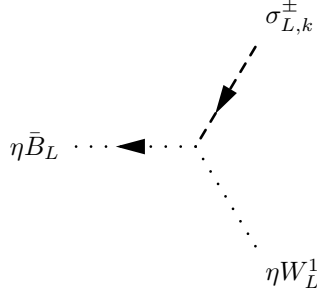

$$\frac{i}{2} g_{B1} \frac{1}{\sqrt{g_{A1}^2 + g_{B1}^2}} \left( -g_{A1} + \sqrt{\frac{g_{A1}^2}{g_{A1}^2 + g_{B1}^2}} \sqrt{g_{A1}^2 + g_{B1}^2} \right) g_{B2} \frac{1}{\sqrt{g_{A2}^2 + g_{B2}^2}} \left( -g_{A2} + \sqrt{\frac{g_{A2}^2}{g_{A2}^2 + g_{B2}^2}} \sqrt{g_{A2}^2 + g_{B2}^2} \right) v_{Lv} \left( Z_{Lv}^{od,*} \right) \quad (1582)$$


---

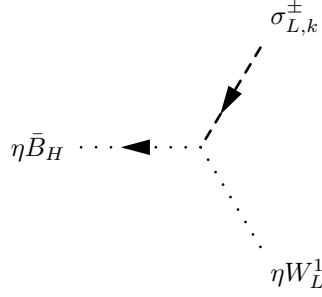

$$\frac{i}{2} \frac{1}{\sqrt{g_{A1}^2 + g_{B1}^2}} \left( g_{A1} \sqrt{\frac{g_{A1}^2}{g_{A1}^2 + g_{B1}^2}} \sqrt{g_{A1}^2 + g_{B1}^2} + g_{B1}^2 \right) g_{B2} \frac{1}{\sqrt{g_{A2}^2 + g_{B2}^2}} \left( -g_{A2} + \sqrt{\frac{g_{A2}^2}{g_{A2}^2 + g_{B2}^2}} \sqrt{g_{A2}^2 + g_{B2}^2} \right) v_{Lv} \left( Z_{Lv}^{od,*} \right) \quad (1583)$$


---

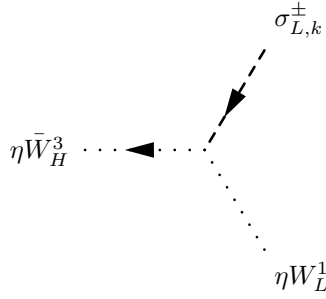

$$-\frac{i}{2} g_{B2} \frac{1}{\sqrt{g_{A2}^2 + g_{B2}^2}} \left( g_{A2}^2 \sqrt{\frac{g_{A2}^2}{g_{A2}^2 + g_{B2}^2}} + g_{A2} \sqrt{g_{A2}^2 + g_{B2}^2} + g_{B2}^2 \sqrt{\frac{g_{A2}^2}{g_{A2}^2 + g_{B2}^2}} \right) v_{Lv} \left( -Z_{Lv,k2}^{od,*} - Z_{Lv,k4}^{od,*} + Z_{Lv,k1}^{od,*} + Z_{Lv,k3}^{od,*} \right) \quad (1584)$$


---

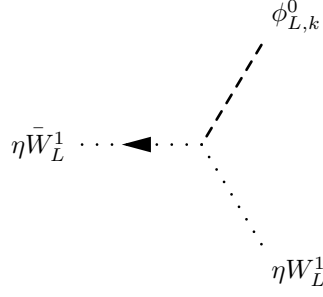

$$ig_{A2}g_{B2}^2 \frac{1}{\left(g_{A2}^2 + g_{B2}^2\right)^{3/2}} \left( g_{A2}^2 \sqrt{\frac{g_{A2}^2}{g_{A2}^2 + g_{B2}^2}} - g_{A2} \sqrt{g_{A2}^2 + g_{B2}^2} + g_{B2}^2 \sqrt{\frac{g_{A2}^2}{g_{A2}^2 + g_{B2}^2}} \right) v_{Lv} \left( Z_{Ls,k1}^{DR,*} + Z_{Ls,k2}^{DR,*} + Z_{Ls,k3}^{DR,*} + Z_{Ls,k4}^{DR,*} \right) \quad (1585)$$


---

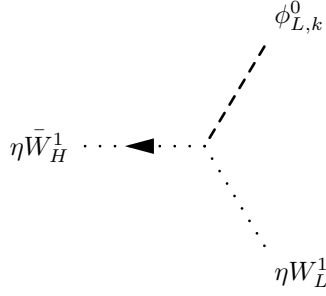

$$-\frac{i}{2}g_{B2} \left( -g_{A2}^2 + g_{B2}^2 \right) \frac{1}{\left(g_{A2}^2 + g_{B2}^2\right)^{3/2}} \left( g_{A2}^2 \sqrt{\frac{g_{A2}^2}{g_{A2}^2 + g_{B2}^2}} - g_{A2} \sqrt{g_{A2}^2 + g_{B2}^2} + g_{B2}^2 \sqrt{\frac{g_{A2}^2}{g_{A2}^2 + g_{B2}^2}} \right) v_{Lv} \left( Z_{Ls,k1}^{DR,*} + Z_{Ls,k2}^{DR,*} + Z_{Ls,k3}^{DR,*} + Z_{Ls,k4}^{DR,*} \right) \quad (1586)$$


---

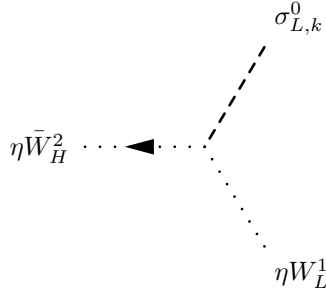

$$\frac{i}{2}g_{B2}\frac{1}{\sqrt{gA2^2+gB2^2}}\left(g_{A2}^2\sqrt{\frac{gA2^2}{gA2^2+gB2^2}}+g_{A2}\sqrt{gA2^2+gB2^2}+g_{B2}^2\sqrt{\frac{gA2^2}{gA2^2+gB2^2}}\right)v_{Lv}\left(-Z_{Ls,k2}^{Di,*}-Z_{Ls,k3}^{Di,*}+Z_{Ls,k1}^{Di,*}+Z_{Ls,k4}^{Di,*}\right)\xi_W$$

(1587)

---

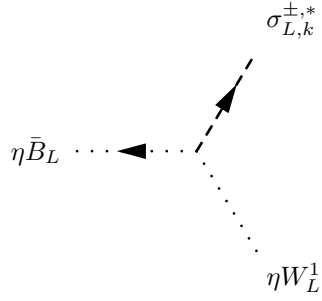

$$\frac{i}{2}g_{B1}\frac{1}{\sqrt{gA1^2+gB1^2}}\left(-g_{A1}+\sqrt{\frac{gA1^2}{gA1^2+gB1^2}}\sqrt{gA1^2+gB1^2}\right)g_{B2}\frac{1}{\sqrt{gA2^2+gB2^2}}\left(-g_{A2}+\sqrt{\frac{gA2^2}{gA2^2+gB2^2}}\sqrt{gA2^2+gB2^2}\right)v_{Lv}\xi_B$$

(1588)

---

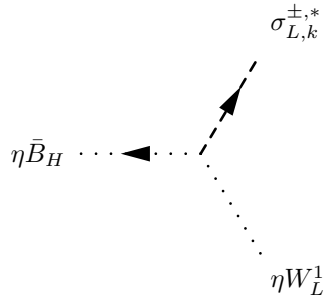

$$\frac{i}{2}\frac{1}{\sqrt{gA1^2+gB1^2}}\left(g_{A1}\sqrt{\frac{gA1^2}{gA1^2+gB1^2}}\sqrt{gA1^2+gB1^2}+g_{B1}^2\right)g_{B2}\frac{1}{\sqrt{gA2^2+gB2^2}}\left(-g_{A2}+\sqrt{\frac{gA2^2}{gA2^2+gB2^2}}\sqrt{gA2^2+gB2^2}\right)v_{Lv}\xi_{B_H}\left(\right)$$

(1589)

---

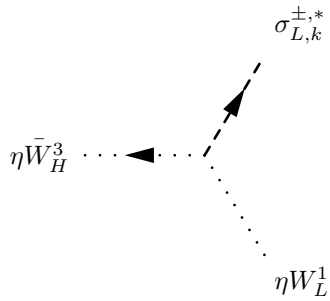

$$-\frac{i}{2}g_{B2}\frac{1}{\sqrt{g_{A2}^2+g_{B2}^2}}\left(g_{A2}^2\sqrt{\frac{g_{A2}^2}{g_{A2}^2+g_{B2}^2}}+g_{A2}\sqrt{g_{A2}^2+g_{B2}^2}+g_{B2}^2\sqrt{\frac{g_{A2}^2}{g_{A2}^2+g_{B2}^2}}\right)v_{Lv}\xi_{W_H^3}\left(-Z_{Ls,k2}^{od}-Z_{Ls,k4}^{od}+Z_{Ls,k1}^{od}+Z_{Ls,k3}^{od}\right) \quad (1590)$$


---

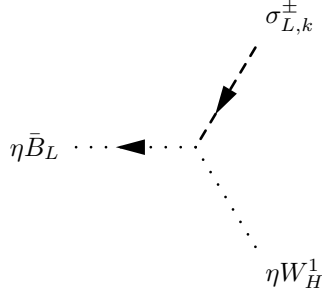

$$\frac{i}{2}g_{B1}\frac{1}{\sqrt{g_{A1}^2+g_{B1}^2}}\left(-g_{A1}+\sqrt{\frac{g_{A1}^2}{g_{A1}^2+g_{B1}^2}}\sqrt{g_{A1}^2+g_{B1}^2}\right)\frac{1}{\sqrt{g_{A2}^2+g_{B2}^2}}\left(g_{A2}\sqrt{\frac{g_{A2}^2}{g_{A2}^2+g_{B2}^2}}\sqrt{g_{A2}^2+g_{B2}^2}+g_{B2}^2\right)v_{Lv}\left(Z_{Ls,k1}^{od}+Z_{Ls,k2}^{od}+Z_{Ls,k3}^{od}+Z_{Ls,k4}^{od}\right) \quad (1591)$$


---

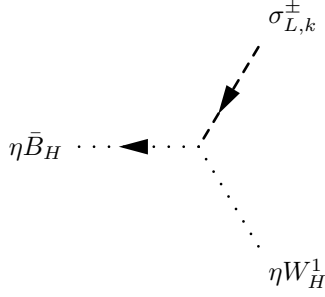

$$\frac{i}{2}\frac{1}{\sqrt{g_{A1}^2+g_{B1}^2}}\left(g_{A1}\sqrt{\frac{g_{A1}^2}{g_{A1}^2+g_{B1}^2}}\sqrt{g_{A1}^2+g_{B1}^2}+g_{B1}^2\right)\frac{1}{\sqrt{g_{A2}^2+g_{B2}^2}}\left(g_{A2}\sqrt{\frac{g_{A2}^2}{g_{A2}^2+g_{B2}^2}}\sqrt{g_{A2}^2+g_{B2}^2}+g_{B2}^2\right)v_{Lv}\left(Z_{Ls,k1}^{od,*}+Z_{Ls,k2}^{od,*}+Z_{Ls,k3}^{od,*}+Z_{Ls,k4}^{od,*}\right) \quad (1592)$$


---

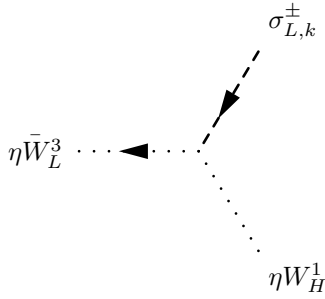

$$-\frac{i}{2}g_{B2}\frac{1}{\sqrt{g_{A2}^2+g_{B2}^2}}\left(g_{A2}^2\sqrt{\frac{g_{A2}^2}{g_{A2}^2+g_{B2}^2}}-g_{A2}\sqrt{g_{A2}^2+g_{B2}^2}+g_{B2}^2\sqrt{\frac{g_{A2}^2}{g_{A2}^2+g_{B2}^2}}\right)v_{Lv}\left(-Z_{Ls,k2}^{od,*}-Z_{Ls,k4}^{od,*}+Z_{Ls,k1}^{od,*}+Z_{Ls,k3}^{od,*}\right) \quad (1593)$$


---

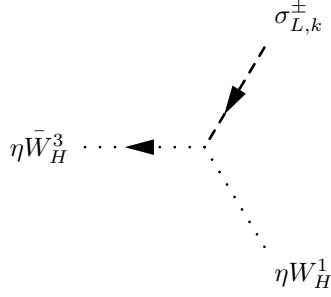

$$\frac{i}{2}\left(-g_{B2}^2+g_{A2}^2\right)v_{Lv}\left(-Z_{Ls,k2}^{od,*}-Z_{Ls,k4}^{od,*}+Z_{Ls,k1}^{od,*}+Z_{Ls,k3}^{od,*}\right)\xi_{W_H^3} \quad (1594)$$


---

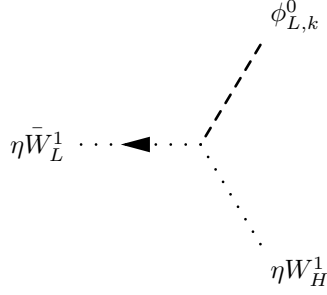

$$-\frac{i}{2}g_{B2}\left(-g_{A2}^2+g_{B2}^2\right)\frac{1}{\left(g_{A2}^2+g_{B2}^2\right)^{3/2}}\left(g_{A2}^2\sqrt{\frac{g_{A2}^2}{g_{A2}^2+g_{B2}^2}}-g_{A2}\sqrt{g_{A2}^2+g_{B2}^2}+g_{B2}^2\sqrt{\frac{g_{A2}^2}{g_{A2}^2+g_{B2}^2}}\right)v_{Lv}\left(Z_{Ls,k1}^{DR,*}+Z_{Ls,k2}^{DR,*}+\right) \quad (1595)$$


---

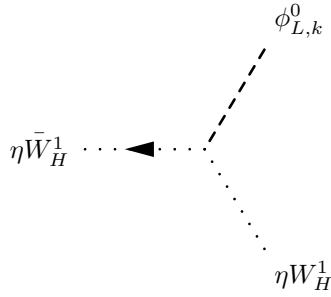

$$\begin{aligned}
& -\frac{i}{2} \frac{1}{\left(gA2^2 + gB2^2\right)^{3/2}} \left( 2g_{A2}^3 g_{B2}^2 \sqrt{\frac{gA2^2}{gA2^2 + gB2^2}} + 2g_{A2} g_{B2}^4 \sqrt{\frac{gA2^2}{gA2^2 + gB2^2}} + g_{A2}^4 \sqrt{gA2^2 + gB2^2} \right. \\
& \left. + g_{B2}^4 \sqrt{gA2^2 + gB2^2} \right) v_{Lv} \left( Z_{Ls,k1}^{DR,*} + Z_{Ls,k2}^{DR,*} + Z_{Ls,k3}^{DR,*} + Z_{Ls,k4}^{DR,*} \right) \xi_{W_H^1}
\end{aligned} \tag{1596}$$


---

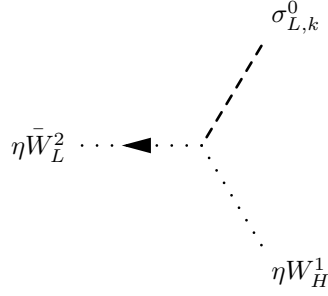

$$\begin{aligned}
& \frac{i}{2} g_{B2} \frac{1}{\sqrt{gA2^2 + gB2^2}} \left( g_{A2}^2 \sqrt{\frac{gA2^2}{gA2^2 + gB2^2}} - g_{A2} \sqrt{gA2^2 + gB2^2} + g_{B2}^2 \sqrt{\frac{gA2^2}{gA2^2 + gB2^2}} \right) v_{Lv} \left( -Z_{Ls,k2}^{Di,*} - Z_{Ls,k3}^{Di,*} + Z_{Ls,k1}^{Di,*} + Z_{Ls,k4}^{Di,*} \right) \xi_{W_H^2}
\end{aligned} \tag{1597}$$


---

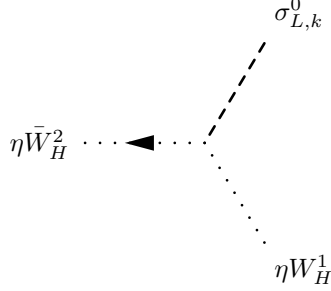

$$-\frac{i}{2} \left( -g_{B2}^2 + g_{A2}^2 \right) v_{Lv} \left( -Z_{Ls,k2}^{Di,*} - Z_{Ls,k3}^{Di,*} + Z_{Ls,k1}^{Di,*} + Z_{Ls,k4}^{Di,*} \right) \xi_{W_H^2} \tag{1598}$$


---

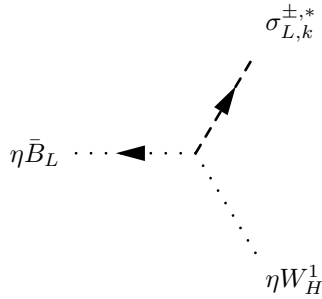

$$\frac{i}{2}g_{B1}\frac{1}{\sqrt{gA1^2+gB1^2}}\left(-g_{A1}+\sqrt{\frac{gA1^2}{gA1^2+gB1^2}}\sqrt{gA1^2+gB1^2}\right)\frac{1}{\sqrt{gA2^2+gB2^2}}\left(g_{A2}\sqrt{\frac{gA2^2}{gA2^2+gB2^2}}\sqrt{gA2^2+gB2^2}+g_{B2}^2\right)v_{Lv}\xi_{B_L}\left(\right. \\ \left.\right) \quad (1599)$$


---

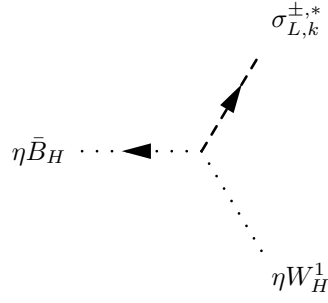

$$\frac{i}{2}\frac{1}{\sqrt{gA1^2+gB1^2}}\left(g_{A1}\sqrt{\frac{gA1^2}{gA1^2+gB1^2}}\sqrt{gA1^2+gB1^2}+g_{B1}^2\right)\frac{1}{\sqrt{gA2^2+gB2^2}}\left(g_{A2}\sqrt{\frac{gA2^2}{gA2^2+gB2^2}}\sqrt{gA2^2+gB2^2}+g_{B2}^2\right)v_{Lv}\xi_{B_H}\left(Z_{L^o}^o\right. \\ \left.\right) \quad (1600)$$


---

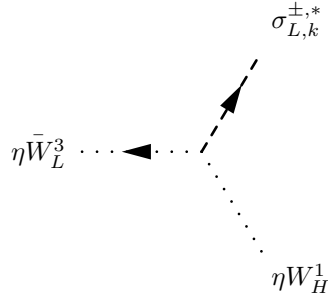

$$-\frac{i}{2}g_{B2}\frac{1}{\sqrt{gA2^2+gB2^2}}\left(g_{A2}^2\sqrt{\frac{gA2^2}{gA2^2+gB2^2}}-g_{A2}\sqrt{gA2^2+gB2^2}+g_{B2}^2\sqrt{\frac{gA2^2}{gA2^2+gB2^2}}\right)v_{Lv}\xi_{W_L^3}\left(-Z_{Ls,k2}^{od}-Z_{Ls,k4}^{od}+Z_{Ls,k1}^{od}+Z_{L^o}^{od}\right) \\ \left.\right) \quad (1601)$$


---

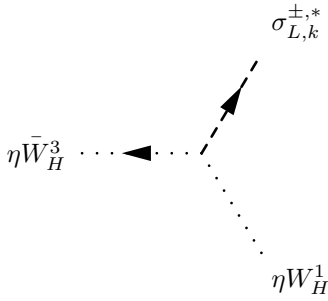

$$\frac{i}{2} \left( -g_{B2}^2 + g_{A2}^2 \right) v_L v \xi_{W_H^3} \left( -Z_{Ls,k2}^{od} - Z_{Ls,k4}^{od} + Z_{Ls,k1}^{od} + Z_{Ls,k3}^{od} \right) \quad (1602)$$


---

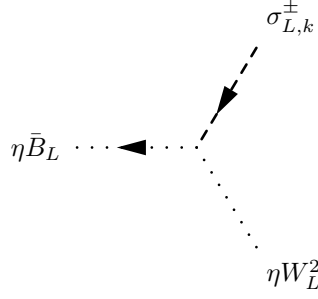

$$-\frac{1}{2} g_{B1} \frac{1}{\sqrt{g_{A1}^2 + g_{B1}^2}} \left( -g_{A1} + \sqrt{\frac{g_{A1}^2}{g_{A1}^2 + g_{B1}^2}} \sqrt{g_{A1}^2 + g_{B1}^2} \right) g_{B2} \frac{1}{\sqrt{g_{A2}^2 + g_{B2}^2}} \left( -g_{A2} + \sqrt{\frac{g_{A2}^2}{g_{A2}^2 + g_{B2}^2}} \sqrt{g_{A2}^2 + g_{B2}^2} \right) v_L v \quad (1603)$$


---

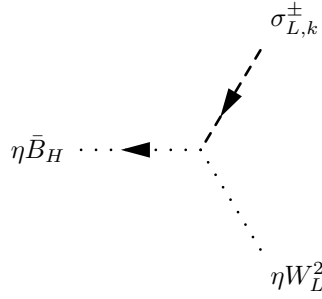

$$-\frac{1}{2} \frac{1}{\sqrt{g_{A1}^2 + g_{B1}^2}} \left( g_{A1} \sqrt{\frac{g_{A1}^2}{g_{A1}^2 + g_{B1}^2}} \sqrt{g_{A1}^2 + g_{B1}^2} + g_{B1}^2 \right) g_{B2} \frac{1}{\sqrt{g_{A2}^2 + g_{B2}^2}} \left( -g_{A2} + \sqrt{\frac{g_{A2}^2}{g_{A2}^2 + g_{B2}^2}} \sqrt{g_{A2}^2 + g_{B2}^2} \right) v_L v \quad (1604)$$


---

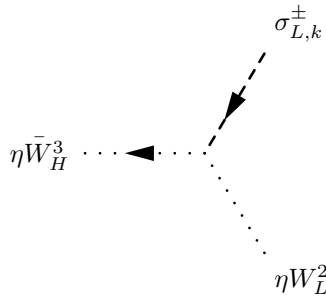



$$\frac{1}{2}g_{B2}\frac{1}{\sqrt{g_{A2^2}+g_{B2^2}}}\left(g_{A2}^2\sqrt{\frac{g_{A2^2}}{g_{A2^2}+g_{B2^2}}}+g_{A2}\sqrt{g_{A2^2}+g_{B2^2}}+g_{B2}^2\sqrt{\frac{g_{A2^2}}{g_{A2^2}+g_{B2^2}}}\right)v_{Lv}\left(-Z_{Ls,k2}^{od,*}-Z_{Ls,k4}^{od,*}+Z_{Ls,k1}^{od,*}+Z_{Ls,k3}^{od,*}\right)\xi_W$$


---

(1605)

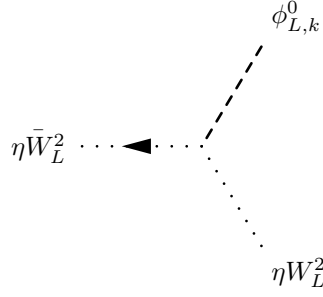

$$ig_{A2}g_{B2}^2\frac{1}{\left(g_{A2^2}+g_{B2^2}\right)^{3/2}}\left(g_{A2}^2\sqrt{\frac{g_{A2^2}}{g_{A2^2}+g_{B2^2}}}-g_{A2}\sqrt{g_{A2^2}+g_{B2^2}}+g_{B2}^2\sqrt{\frac{g_{A2^2}}{g_{A2^2}+g_{B2^2}}}\right)v_{Lv}\left(Z_{Ls,k1}^{DR,*}+Z_{Ls,k2}^{DR,*}+Z_{Ls,k3}^{DR,*}+Z_{Ls,k4}^{DR,*}\right)\xi_W$$


---

(1606)

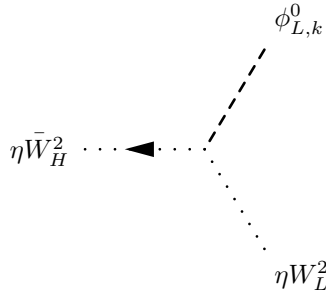

$$-\frac{i}{2}g_{B2}\left(-g_{A2}^2+g_{B2}^2\right)\frac{1}{\left(g_{A2^2}+g_{B2^2}\right)^{3/2}}\left(g_{A2}^2\sqrt{\frac{g_{A2^2}}{g_{A2^2}+g_{B2^2}}}-g_{A2}\sqrt{g_{A2^2}+g_{B2^2}}+g_{B2}^2\sqrt{\frac{g_{A2^2}}{g_{A2^2}+g_{B2^2}}}\right)v_{Lv}\left(Z_{Ls,k1}^{DR,*}+Z_{Ls,k2}^{DR,*}+Z_{Ls,k3}^{DR,*}+Z_{Ls,k4}^{DR,*}\right)\xi_W$$


---

(1607)

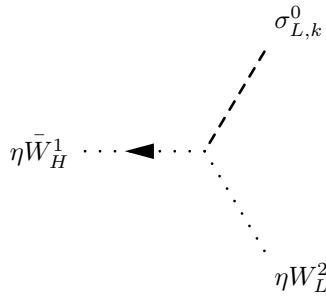

$$-\frac{i}{2}g_{B2}\frac{1}{\sqrt{gA2^2+gB2^2}}\left(g_{A2}^2\sqrt{\frac{gA2^2}{gA2^2+gB2^2}}+g_{A2}\sqrt{gA2^2+gB2^2}+g_{B2}^2\sqrt{\frac{gA2^2}{gA2^2+gB2^2}}\right)v_{Lv}\left(-Z_{Ls,k2}^{Di,*}-Z_{Ls,k3}^{Di,*}+Z_{Ls,k1}^{Di,*}+Z_{Ls,k4}^{Di,*}\right) \quad (1608)$$


---

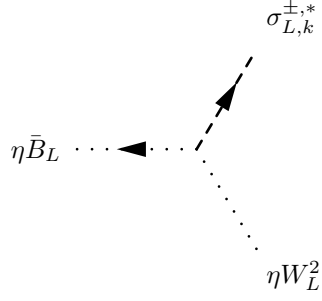

$$\frac{1}{2}g_{B1}\frac{1}{\sqrt{gA1^2+gB1^2}}\left(-g_{A1}+\sqrt{\frac{gA1^2}{gA1^2+gB1^2}}\sqrt{gA1^2+gB1^2}\right)g_{B2}\frac{1}{\sqrt{gA2^2+gB2^2}}\left(-g_{A2}+\sqrt{\frac{gA2^2}{gA2^2+gB2^2}}\sqrt{gA2^2+gB2^2}\right)v_{Lv}\xi_{Bv} \quad (1609)$$


---

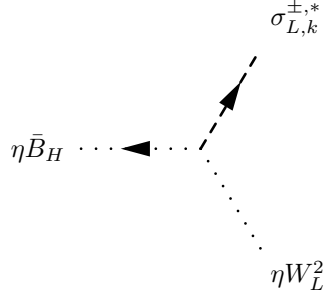

$$\frac{1}{2}\frac{1}{\sqrt{gA1^2+gB1^2}}\left(g_{A1}\sqrt{\frac{gA1^2}{gA1^2+gB1^2}}\sqrt{gA1^2+gB1^2}+g_{B1}^2\right)g_{B2}\frac{1}{\sqrt{gA2^2+gB2^2}}\left(-g_{A2}+\sqrt{\frac{gA2^2}{gA2^2+gB2^2}}\sqrt{gA2^2+gB2^2}\right)v_{Lv}\xi_{Bv} \quad (1610)$$


---

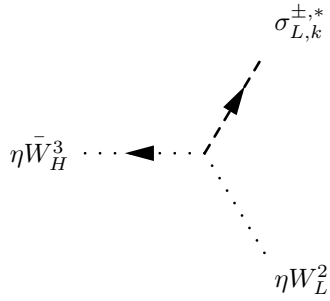

$$-\frac{1}{2}g_{B2}\frac{1}{\sqrt{g_{A2}^2+g_{B2}^2}}\left(g_{A2}^2\sqrt{\frac{g_{A2}^2}{g_{A2}^2+g_{B2}^2}}+g_{A2}\sqrt{g_{A2}^2+g_{B2}^2}+g_{B2}^2\sqrt{\frac{g_{A2}^2}{g_{A2}^2+g_{B2}^2}}\right)v_{Lv}\xi_{W_H^3}\left(-Z_{Ls,k2}^{od}-Z_{Ls,k4}^{od}+Z_{Ls,k1}^{od}+Z_L^{od}\right) \quad (1611)$$


---

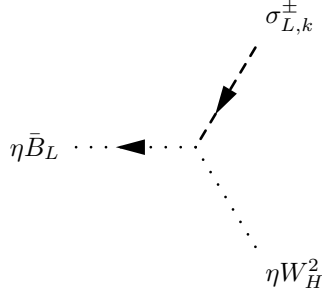

$$-\frac{1}{2}g_{B1}\frac{1}{\sqrt{g_{A1}^2+g_{B1}^2}}\left(-g_{A1}+\sqrt{\frac{g_{A1}^2}{g_{A1}^2+g_{B1}^2}}\sqrt{g_{A1}^2+g_{B1}^2}\right)\frac{1}{\sqrt{g_{A2}^2+g_{B2}^2}}\left(g_{A2}\sqrt{\frac{g_{A2}^2}{g_{A2}^2+g_{B2}^2}}\sqrt{g_{A2}^2+g_{B2}^2}+g_{B2}^2\right)v_{Lv}\left(Z_{Ls,k2}^{od}+Z_{Ls,k4}^{od}-Z_{Ls,k1}^{od}-Z_L^{od}\right) \quad (1612)$$


---

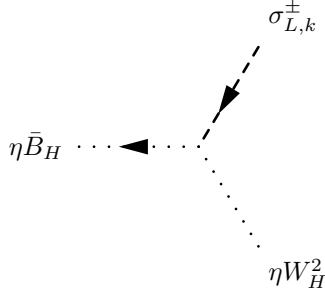

$$-\frac{1}{2}\frac{1}{\sqrt{g_{A1}^2+g_{B1}^2}}\left(g_{A1}\sqrt{\frac{g_{A1}^2}{g_{A1}^2+g_{B1}^2}}\sqrt{g_{A1}^2+g_{B1}^2}+g_{B1}^2\right)\frac{1}{\sqrt{g_{A2}^2+g_{B2}^2}}\left(g_{A2}\sqrt{\frac{g_{A2}^2}{g_{A2}^2+g_{B2}^2}}\sqrt{g_{A2}^2+g_{B2}^2}+g_{B2}^2\right)v_{Lv}\left(Z_{Ls,k2}^{od}+Z_{Ls,k4}^{od}-Z_{Ls,k1}^{od}-Z_L^{od}\right) \quad (1613)$$


---

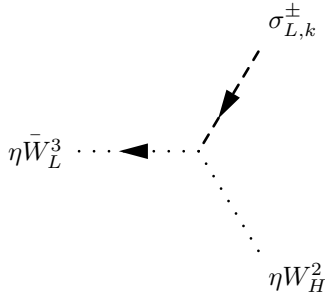

$$\frac{1}{2}g_{B2}\frac{1}{\sqrt{g_{A2}^2+g_{B2}^2}}\left(g_{A2}^2\sqrt{\frac{g_{A2}^2}{g_{A2}^2+g_{B2}^2}}-g_{A2}\sqrt{g_{A2}^2+g_{B2}^2}+g_{B2}^2\sqrt{\frac{g_{A2}^2}{g_{A2}^2+g_{B2}^2}}\right)v_{Lv}\left(-Z_{Ls,k2}^{od,*}-Z_{Ls,k4}^{od,*}+Z_{Ls,k1}^{od,*}+Z_{Ls,k3}^{od,*}\right)\xi_W$$


---

(1614)

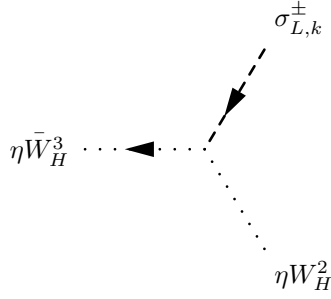

$$-\frac{1}{2}\left(-g_{B2}^2+g_{A2}^2\right)v_{Lv}\left(-Z_{Ls,k2}^{od,*}-Z_{Ls,k4}^{od,*}+Z_{Ls,k1}^{od,*}+Z_{Ls,k3}^{od,*}\right)\xi_{W_H^3}$$


---

(1615)

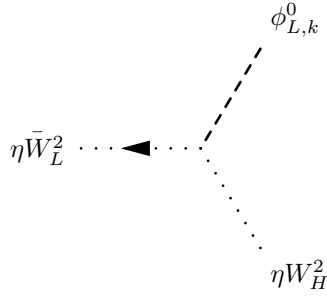

$$-\frac{i}{2}g_{B2}\left(-g_{A2}^2+g_{B2}^2\right)\frac{1}{\left(g_{A2}^2+g_{B2}^2\right)^{3/2}}\left(g_{A2}^2\sqrt{\frac{g_{A2}^2}{g_{A2}^2+g_{B2}^2}}-g_{A2}\sqrt{g_{A2}^2+g_{B2}^2}+g_{B2}^2\sqrt{\frac{g_{A2}^2}{g_{A2}^2+g_{B2}^2}}\right)v_{Lv}\left(Z_{Ls,k1}^{DR,*}+Z_{Ls,k2}^{DR,*}+\right.$$


---

(1616)

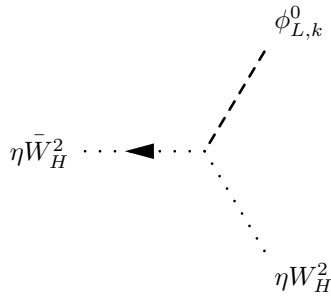

$$\begin{aligned}
& -\frac{i}{2} \frac{1}{\left(gA2^2 + gB2^2\right)^{3/2}} \left( 2g_{A2}^3 g_{B2}^2 \sqrt{\frac{gA2^2}{gA2^2 + gB2^2}} + 2g_{A2} g_{B2}^4 \sqrt{\frac{gA2^2}{gA2^2 + gB2^2}} + g_{A2}^4 \sqrt{gA2^2 + gB2^2} \right. \\
& \left. + g_{B2}^4 \sqrt{gA2^2 + gB2^2} \right) v_{Lv} \left( Z_{Ls,k1}^{DR,*} + Z_{Ls,k2}^{DR,*} + Z_{Ls,k3}^{DR,*} + Z_{Ls,k4}^{DR,*} \right) \xi_{W_H^2}
\end{aligned} \tag{1617}$$


---

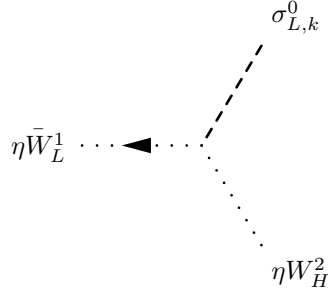

$$\begin{aligned}
& -\frac{i}{2} g_{B2} \frac{1}{\sqrt{gA2^2 + gB2^2}} \left( g_{A2}^2 \sqrt{\frac{gA2^2}{gA2^2 + gB2^2}} - g_{A2} \sqrt{gA2^2 + gB2^2} + g_{B2}^2 \sqrt{\frac{gA2^2}{gA2^2 + gB2^2}} \right) v_{Lv} \left( -Z_{Ls,k2}^{Di,*} - Z_{Ls,k3}^{Di,*} + Z_{Ls,k1}^{Di,*} + Z_{Ls,k4}^{Di,*} \right) \xi_{W_H^1}
\end{aligned} \tag{1618}$$


---

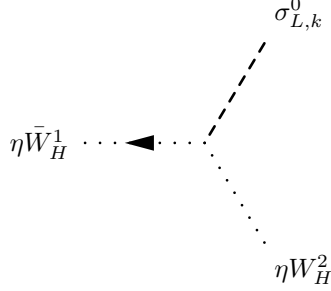

$$\frac{i}{2} \left( -g_{B2}^2 + g_{A2}^2 \right) v_{Lv} \left( -Z_{Ls,k2}^{Di,*} - Z_{Ls,k3}^{Di,*} + Z_{Ls,k1}^{Di,*} + Z_{Ls,k4}^{Di,*} \right) \xi_{W_H^1} \tag{1619}$$


---

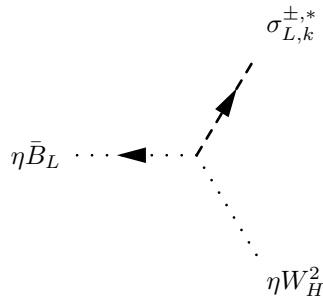

$$\frac{1}{2}g_{B1}\frac{1}{\sqrt{gA1^2+gB1^2}}\left(-g_{A1}+\sqrt{\frac{gA1^2}{gA1^2+gB1^2}}\sqrt{gA1^2+gB1^2}\right)\frac{1}{\sqrt{gA2^2+gB2^2}}\left(g_{A2}\sqrt{\frac{gA2^2}{gA2^2+gB2^2}}\sqrt{gA2^2+gB2^2}+g_{B2}^2\right)v_{Lv}\xi_{B_L}\left(\right. \\ \left.\right) \quad (1620)$$


---

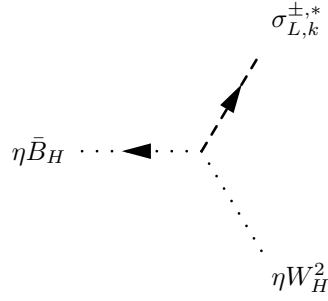

$$\frac{1}{2}\frac{1}{\sqrt{gA1^2+gB1^2}}\left(g_{A1}\sqrt{\frac{gA1^2}{gA1^2+gB1^2}}\sqrt{gA1^2+gB1^2}+g_{B1}^2\right)\frac{1}{\sqrt{gA2^2+gB2^2}}\left(g_{A2}\sqrt{\frac{gA2^2}{gA2^2+gB2^2}}\sqrt{gA2^2+gB2^2}+g_{B2}^2\right)v_{Lv}\xi_{B_H}\left(Z_{L}^o\right. \\ \left.\right) \quad (1621)$$


---

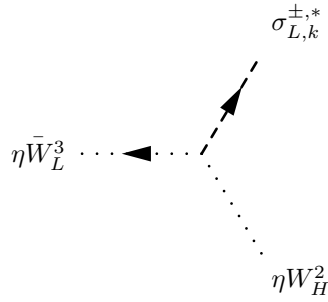

$$-\frac{1}{2}g_{B2}\frac{1}{\sqrt{gA2^2+gB2^2}}\left(g_{A2}^2\sqrt{\frac{gA2^2}{gA2^2+gB2^2}}-g_{A2}\sqrt{gA2^2+gB2^2}+g_{B2}^2\sqrt{\frac{gA2^2}{gA2^2+gB2^2}}\right)v_{Lv}\xi_{W_L^3}\left(-Z_{Ls,k2}^{od}-Z_{Ls,k4}^{od}+Z_{Ls,k1}^{od}+Z_{L}^o\right. \\ \left.\right) \quad (1622)$$


---

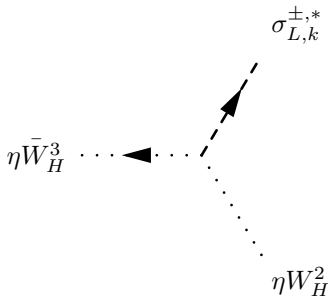

$$\frac{1}{2} \left( -g_{B2}^2 + g_{A2}^2 \right) v_L v \xi_{W_H^3} \left( -Z_{Ls,k2}^{od} - Z_{Ls,k4}^{od} + Z_{Ls,k1}^{od} + Z_{Ls,k3}^{od} \right) \quad (1623)$$


---

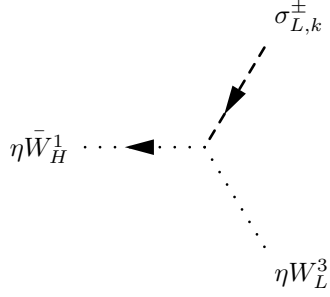

$$\frac{i}{4} g_{B2} \frac{1}{\sqrt{g_{A2}^2 + g_{B2}^2}} \left( g_{A2}^2 \sqrt{\frac{g_{A2}^2}{g_{A2}^2 + g_{B2}^2}} + g_{A2} \sqrt{g_{A2}^2 + g_{B2}^2} + g_{B2}^2 \sqrt{\frac{g_{A2}^2}{g_{A2}^2 + g_{B2}^2}} \right) v_L v \left( -Z_{Ls,k2}^{od,*} - Z_{Ls,k4}^{od,*} + Z_{Ls,k1}^{od,*} + Z_{Ls,k3}^{od,*} \right) \xi_{W_L^3} \quad (1624)$$


---

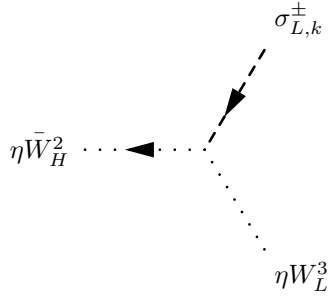

$$-\frac{1}{4} g_{B2} \frac{1}{\sqrt{g_{A2}^2 + g_{B2}^2}} \left( g_{A2}^2 \sqrt{\frac{g_{A2}^2}{g_{A2}^2 + g_{B2}^2}} + g_{A2} \sqrt{g_{A2}^2 + g_{B2}^2} + g_{B2}^2 \sqrt{\frac{g_{A2}^2}{g_{A2}^2 + g_{B2}^2}} \right) v_L v \left( -Z_{Ls,k2}^{od,*} - Z_{Ls,k4}^{od,*} + Z_{Ls,k1}^{od,*} + Z_{Ls,k3}^{od,*} \right) \quad (1625)$$


---

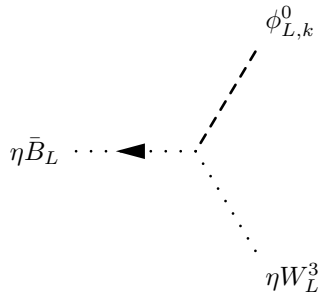

$$ig_{B1}\frac{1}{\sqrt{gA1^2+gB1^2}}\left(-g_{A1}+\sqrt{\frac{gA1^2}{gA1^2+gB1^2}}\sqrt{gA1^2+gB1^2}\right)g_{B2}\frac{1}{\sqrt{gA2^2+gB2^2}}\left(-g_{A2}+\sqrt{\frac{gA2^2}{gA2^2+gB2^2}}\sqrt{gA2^2+gB2^2}\right)v_{Lv}\left(-\right. \\ \left.\right) \quad (1626)$$


---

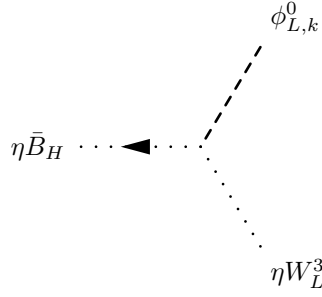

$$i\frac{1}{\sqrt{gA1^2+gB1^2}}\left(g_{A1}\sqrt{\frac{gA1^2}{gA1^2+gB1^2}}\sqrt{gA1^2+gB1^2}+g_{B1}^2\right)g_{B2}\frac{1}{\sqrt{gA2^2+gB2^2}}\left(-g_{A2}+\sqrt{\frac{gA2^2}{gA2^2+gB2^2}}\sqrt{gA2^2+gB2^2}\right)v_{Lv}\left(-Z\right. \\ \left.\right) \quad (1627)$$


---

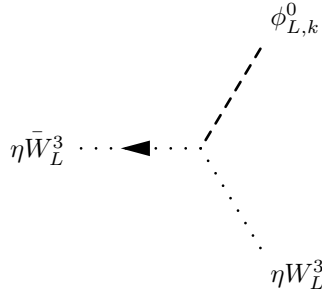

$$2ig_{A2}g_{B2}^2\frac{1}{\left(gA2^2+gB2^2\right)^{3/2}}\left(g_{A2}^2\sqrt{\frac{gA2^2}{gA2^2+gB2^2}}-g_{A2}\sqrt{gA2^2+gB2^2}+g_{B2}^2\sqrt{\frac{gA2^2}{gA2^2+gB2^2}}\right)v_{Lv}\left(Z_{Ls,k1}^{DR,*}+Z_{Ls,k2}^{DR,*}+Z_{Ls,k3}^{DR,*}+Z_{Ls,k4}^{DR,*}\right) \\ \left.\right) \quad (1628)$$


---

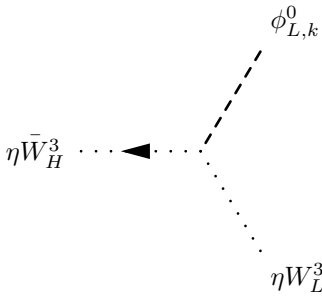



$$-ig_{B2}\left(-g_{A2}^2+g_{B2}^2\right)\frac{1}{\left(gA2^2+gB2^2\right)^{3/2}}\left(g_{A2}^2\sqrt{\frac{gA2^2}{gA2^2+gB2^2}}-g_{A2}\sqrt{gA2^2+gB2^2}+g_{B2}^2\sqrt{\frac{gA2^2}{gA2^2+gB2^2}}\right)v_{Lv}\left(Z_{Ls,k1}^{DR,*}+Z_{Ls,k2}^{DR,*}+\right.$$


---

(1629)

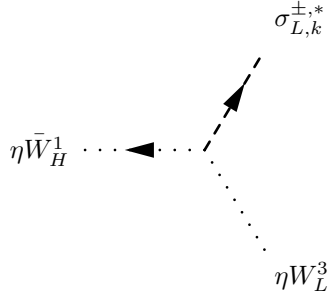

$$\frac{i}{4}g_{B2}\frac{1}{\sqrt{gA2^2+gB2^2}}\left(g_{A2}^2\sqrt{\frac{gA2^2}{gA2^2+gB2^2}}+g_{A2}\sqrt{gA2^2+gB2^2}+g_{B2}^2\sqrt{\frac{gA2^2}{gA2^2+gB2^2}}\right)v_{Lv}\xi_{W_H^1}\left(-Z_{Ls,k2}^{od}-Z_{Ls,k4}^{od}+Z_{Ls,k1}^{od}+Z_{Ls,k3}^{od}+\right.$$


---

(1630)

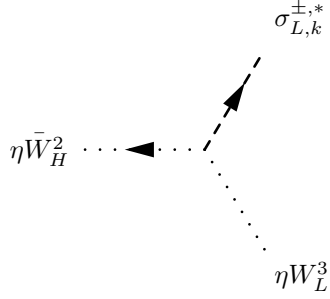

$$\frac{1}{4}g_{B2}\frac{1}{\sqrt{gA2^2+gB2^2}}\left(g_{A2}^2\sqrt{\frac{gA2^2}{gA2^2+gB2^2}}+g_{A2}\sqrt{gA2^2+gB2^2}+g_{B2}^2\sqrt{\frac{gA2^2}{gA2^2+gB2^2}}\right)v_{Lv}\xi_{W_H^2}\left(-Z_{Ls,k2}^{od}-Z_{Ls,k4}^{od}+Z_{Ls,k1}^{od}+Z_{Ls,k3}^{od}+\right.$$


---

(1631)

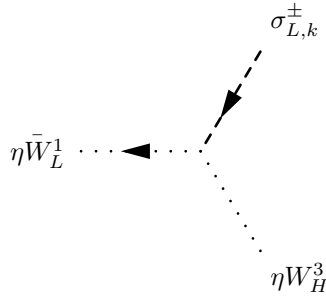

$$\frac{i}{4}g_{B2}\frac{1}{\sqrt{g_{A2^2}+g_{B2^2}}}\left(g_{A2}^2\sqrt{\frac{g_{A2^2}}{g_{A2^2}+g_{B2^2}}}-g_{A2}\sqrt{g_{A2^2}+g_{B2^2}}+g_{B2}^2\sqrt{\frac{g_{A2^2}}{g_{A2^2}+g_{B2^2}}}\right)v_{Lv}\left(-Z_{Ls,k2}^{od,*}-Z_{Ls,k4}^{od,*}+Z_{Ls,k1}^{od,*}+Z_{Ls,k3}^{od,*}\right)\xi_W$$

(1632)

---

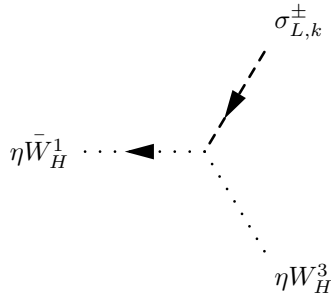

$$-\frac{i}{4}\left(-g_{B2}^2+g_{A2}^2\right)v_{Lv}\left(-Z_{Ls,k2}^{od,*}-Z_{Ls,k4}^{od,*}+Z_{Ls,k1}^{od,*}+Z_{Ls,k3}^{od,*}\right)\xi_{W_H^1}$$

(1633)

---

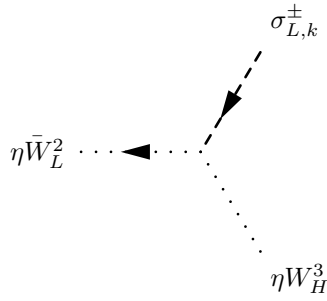

$$-\frac{1}{4}g_{B2}\frac{1}{\sqrt{g_{A2^2}+g_{B2^2}}}\left(g_{A2}^2\sqrt{\frac{g_{A2^2}}{g_{A2^2}+g_{B2^2}}}-g_{A2}\sqrt{g_{A2^2}+g_{B2^2}}+g_{B2}^2\sqrt{\frac{g_{A2^2}}{g_{A2^2}+g_{B2^2}}}\right)v_{Lv}\left(-Z_{Ls,k2}^{od,*}-Z_{Ls,k4}^{od,*}+Z_{Ls,k1}^{od,*}+Z_{Ls,k3}^{od,*}\right)\xi_W$$

(1634)

---

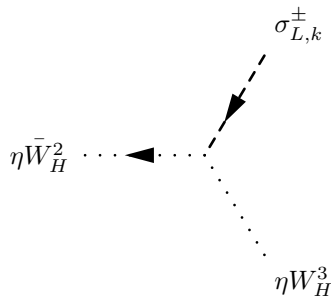

$$\frac{1}{4} \left( -g_{B2}^2 + g_{A2}^2 \right) v_{Lv} \left( -Z_{Ls,k2}^{od,*} - Z_{Ls,k4}^{od,*} + Z_{Ls,k1}^{od,*} + Z_{Ls,k3}^{od,*} \right) \xi_{W_H^2} \quad (1635)$$


---

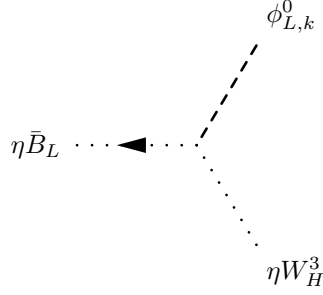

$$ig_{B1} \frac{1}{\sqrt{g_{A1}^2 + g_{B1}^2}} \left( -g_{A1} + \sqrt{\frac{g_{A1}^2}{g_{A1}^2 + g_{B1}^2}} \sqrt{g_{A1}^2 + g_{B1}^2} \right) \frac{1}{\sqrt{g_{A2}^2 + g_{B2}^2}} \left( g_{A2} \sqrt{\frac{g_{A2}^2}{g_{A2}^2 + g_{B2}^2}} \sqrt{g_{A2}^2 + g_{B2}^2} + g_{B2}^2 \right) v_{Lv} \left( -Z_{Ls,k2}^{od,*} - Z_{Ls,k4}^{od,*} + Z_{Ls,k1}^{od,*} + Z_{Ls,k3}^{od,*} \right) \xi_{W_H^2} \quad (1636)$$


---

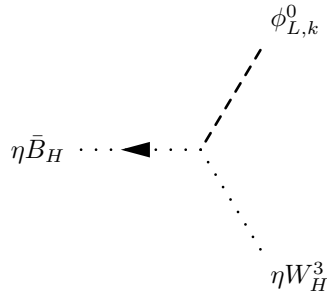

$$i \frac{1}{\sqrt{g_{A1}^2 + g_{B1}^2}} \left( g_{A1} \sqrt{\frac{g_{A1}^2}{g_{A1}^2 + g_{B1}^2}} \sqrt{g_{A1}^2 + g_{B1}^2} + g_{B1}^2 \right) \frac{1}{\sqrt{g_{A2}^2 + g_{B2}^2}} \left( g_{A2} \sqrt{\frac{g_{A2}^2}{g_{A2}^2 + g_{B2}^2}} \sqrt{g_{A2}^2 + g_{B2}^2} + g_{B2}^2 \right) v_{Lv} \left( -Z_{Ls,k2}^{DR,*} - Z_{Ls,k4}^{DR,*} + Z_{Ls,k1}^{DR,*} + Z_{Ls,k3}^{DR,*} \right) \xi_{W_H^2} \quad (1637)$$


---

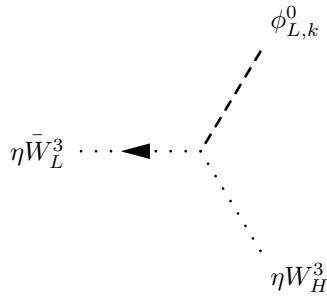

$$-ig_{B2}\left(-g_{A2}^2+g_{B2}^2\right)\frac{1}{\left(gA2^2+gB2^2\right)^{3/2}}\left(g_{A2}^2\sqrt{\frac{gA2^2}{gA2^2+gB2^2}}-g_{A2}\sqrt{gA2^2+gB2^2}+g_{B2}^2\sqrt{\frac{gA2^2}{gA2^2+gB2^2}}\right)v_{Lv}\left(Z_{Ls,k1}^{DR,*}+Z_{Ls,k2}^{DR,*}+\right. \\ \left.+\right) \quad (1638)$$


---

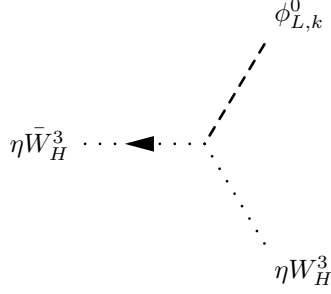

$$-i\frac{1}{\left(gA2^2+gB2^2\right)^{3/2}}\left(2g_{A2}^3g_{B2}^2\sqrt{\frac{gA2^2}{gA2^2+gB2^2}}+2g_{A2}g_{B2}^4\sqrt{\frac{gA2^2}{gA2^2+gB2^2}}+g_{A2}^4\sqrt{gA2^2+gB2^2}\right. \\ \left.+g_{B2}^4\sqrt{gA2^2+gB2^2}\right)v_{Lv}\left(Z_{Ls,k1}^{DR,*}+Z_{Ls,k2}^{DR,*}+Z_{Ls,k3}^{DR,*}+Z_{Ls,k4}^{DR,*}\right)\xi_{W_H^3} \quad (1639)$$


---

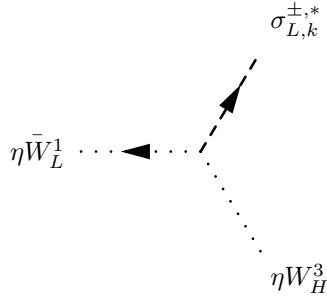

$$\frac{i}{4}g_{B2}\frac{1}{\sqrt{gA2^2+gB2^2}}\left(g_{A2}^2\sqrt{\frac{gA2^2}{gA2^2+gB2^2}}-g_{A2}\sqrt{gA2^2+gB2^2}+g_{B2}^2\sqrt{\frac{gA2^2}{gA2^2+gB2^2}}\right)v_{Lv}\xi_{W_L^1}\left(-Z_{Ls,k2}^{od}-Z_{Ls,k4}^{od}+Z_{Ls,k1}^{od}+Z_{Ls,k3}^{od}\right) \quad (1640)$$


---

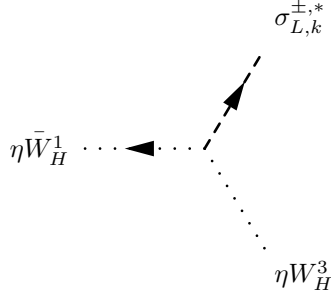

$$-\frac{i}{4}\left(-g_{B2}^2+g_{A2}^2\right)v_Lv\xi_{W_H^1}\left(-Z_{Ls,k2}^{od}-Z_{Ls,k4}^{od}+Z_{Ls,k1}^{od}+Z_{Ls,k3}^{od}\right) \quad (1641)$$


---

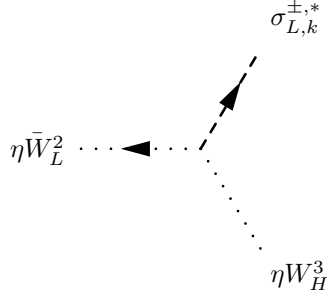

$$\frac{1}{4}g_{B2}\frac{1}{\sqrt{g_{A2}^2+g_{B2}^2}}\left(g_{A2}^2\sqrt{\frac{g_{A2}^2}{g_{A2}^2+g_{B2}^2}}-g_{A2}\sqrt{g_{A2}^2+g_{B2}^2}+g_{B2}^2\sqrt{\frac{g_{A2}^2}{g_{A2}^2+g_{B2}^2}}\right)v_Lv\xi_{W_L^2}\left(-Z_{Ls,k2}^{od}-Z_{Ls,k4}^{od}+Z_{Ls,k1}^{od}+Z_{Ls,k3}^{od}\right) \quad (1642)$$


---

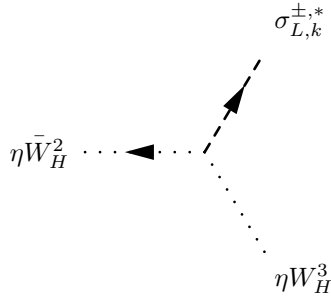

$$-\frac{1}{4}\left(-g_{B2}^2+g_{A2}^2\right)v_Lv\xi_{W_H^2}\left(-Z_{Ls,k2}^{od}-Z_{Ls,k4}^{od}+Z_{Ls,k1}^{od}+Z_{Ls,k3}^{od}\right) \quad (1643)$$


---
